# Supplementary material for: The COS CGM Compendium V: The Dichotomy of OVI Associated with Low- and High-Metallicity Cool Gas at z < 1
Source: arXiv:2403.02374 source file (2024-09-07)
Supplement: Supplementary file 1 [file NF_profiles.pdf]

J000559.23+160948.9,  $z=0.305789$ , RF=1

Normalized Flux

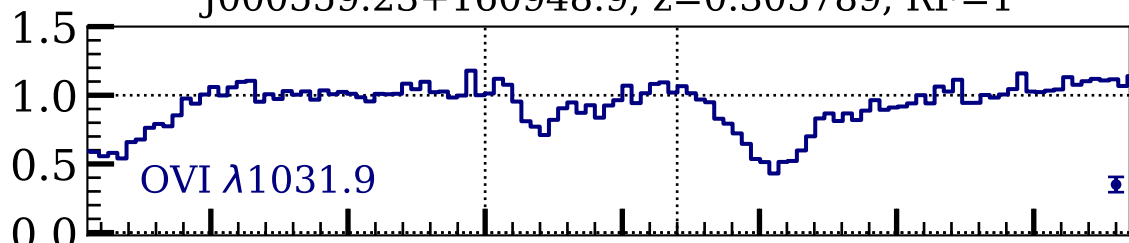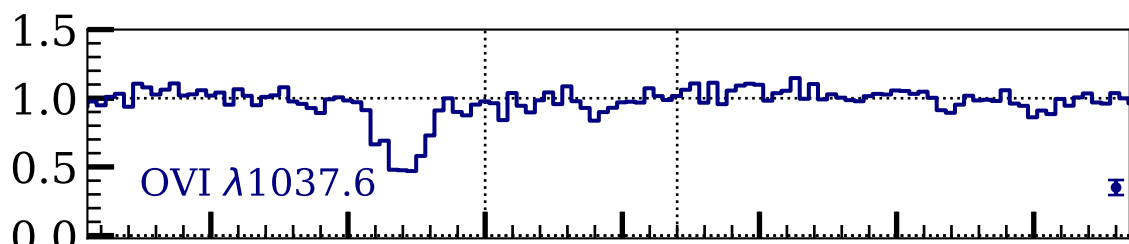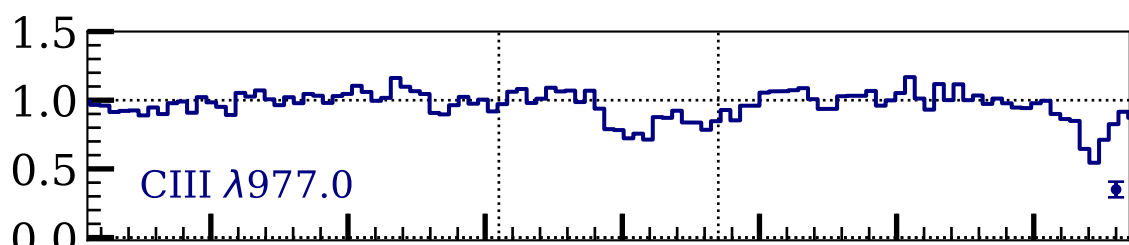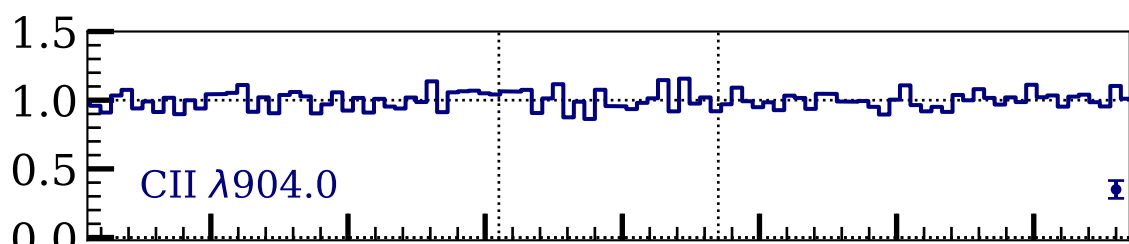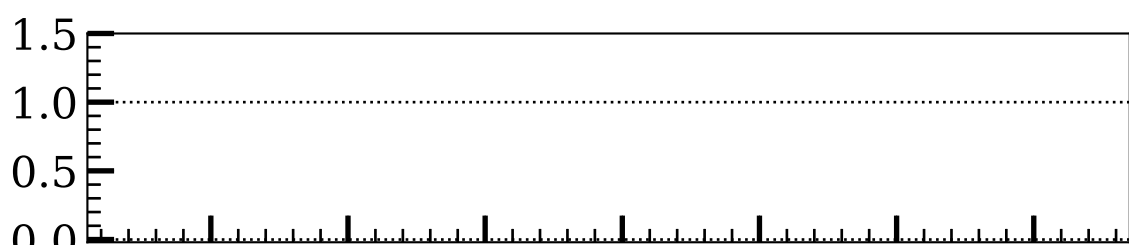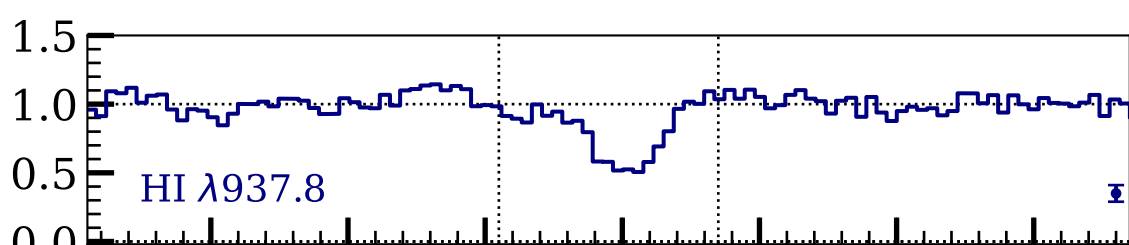

-300 -200 -100 0 100 200 300

Rest-Frame Velocity ( $\text{km s}^{-1}$ )

J000559.23+160948.9,  $z=0.347925$ , RF=1

Normalized Flux

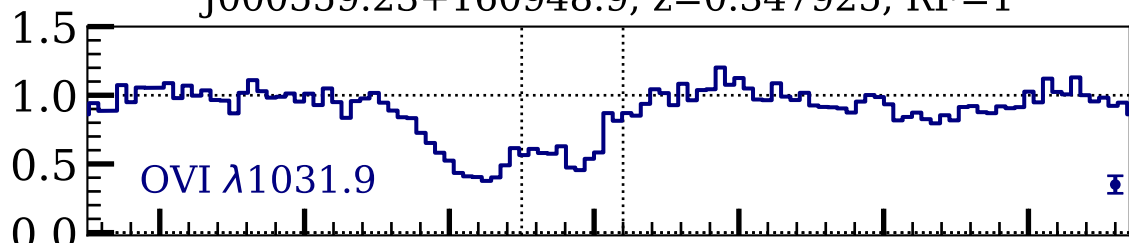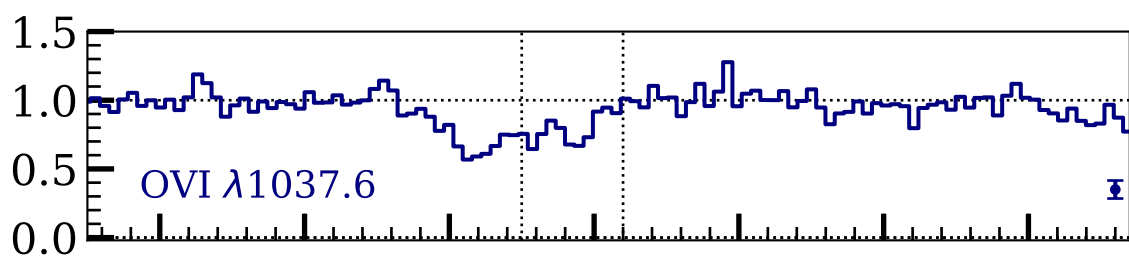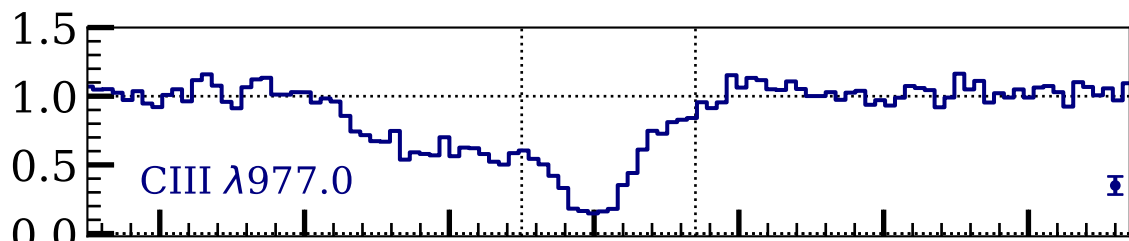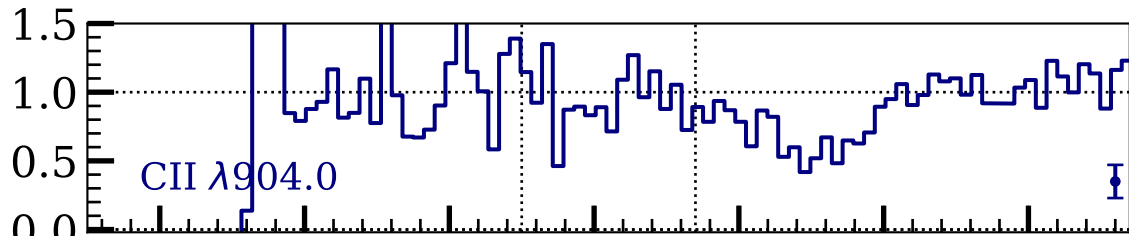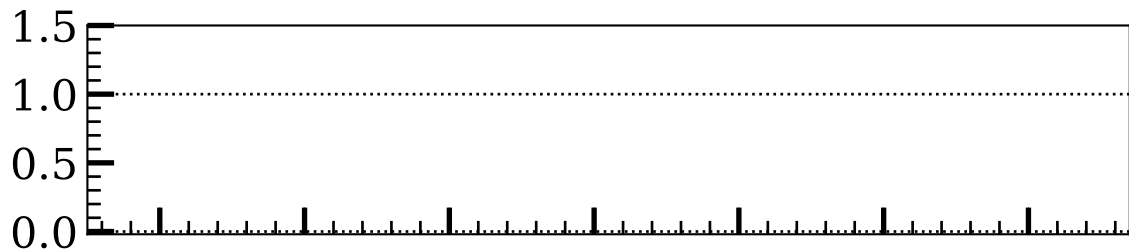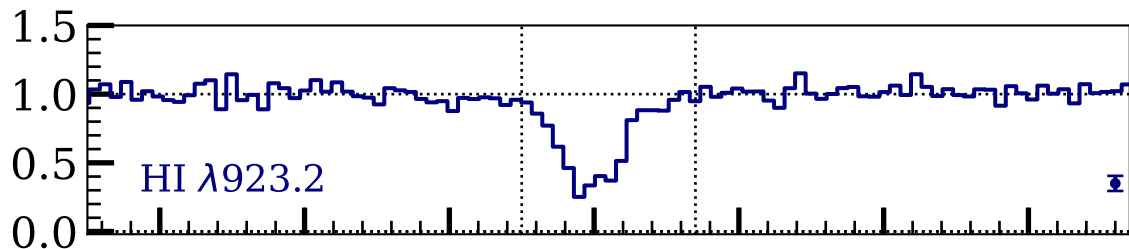

Rest-Frame Velocity ( $\text{km s}^{-1}$ )

J000559.23+160948.9,  $z=0.366204$ , RF=1

Normalized Flux

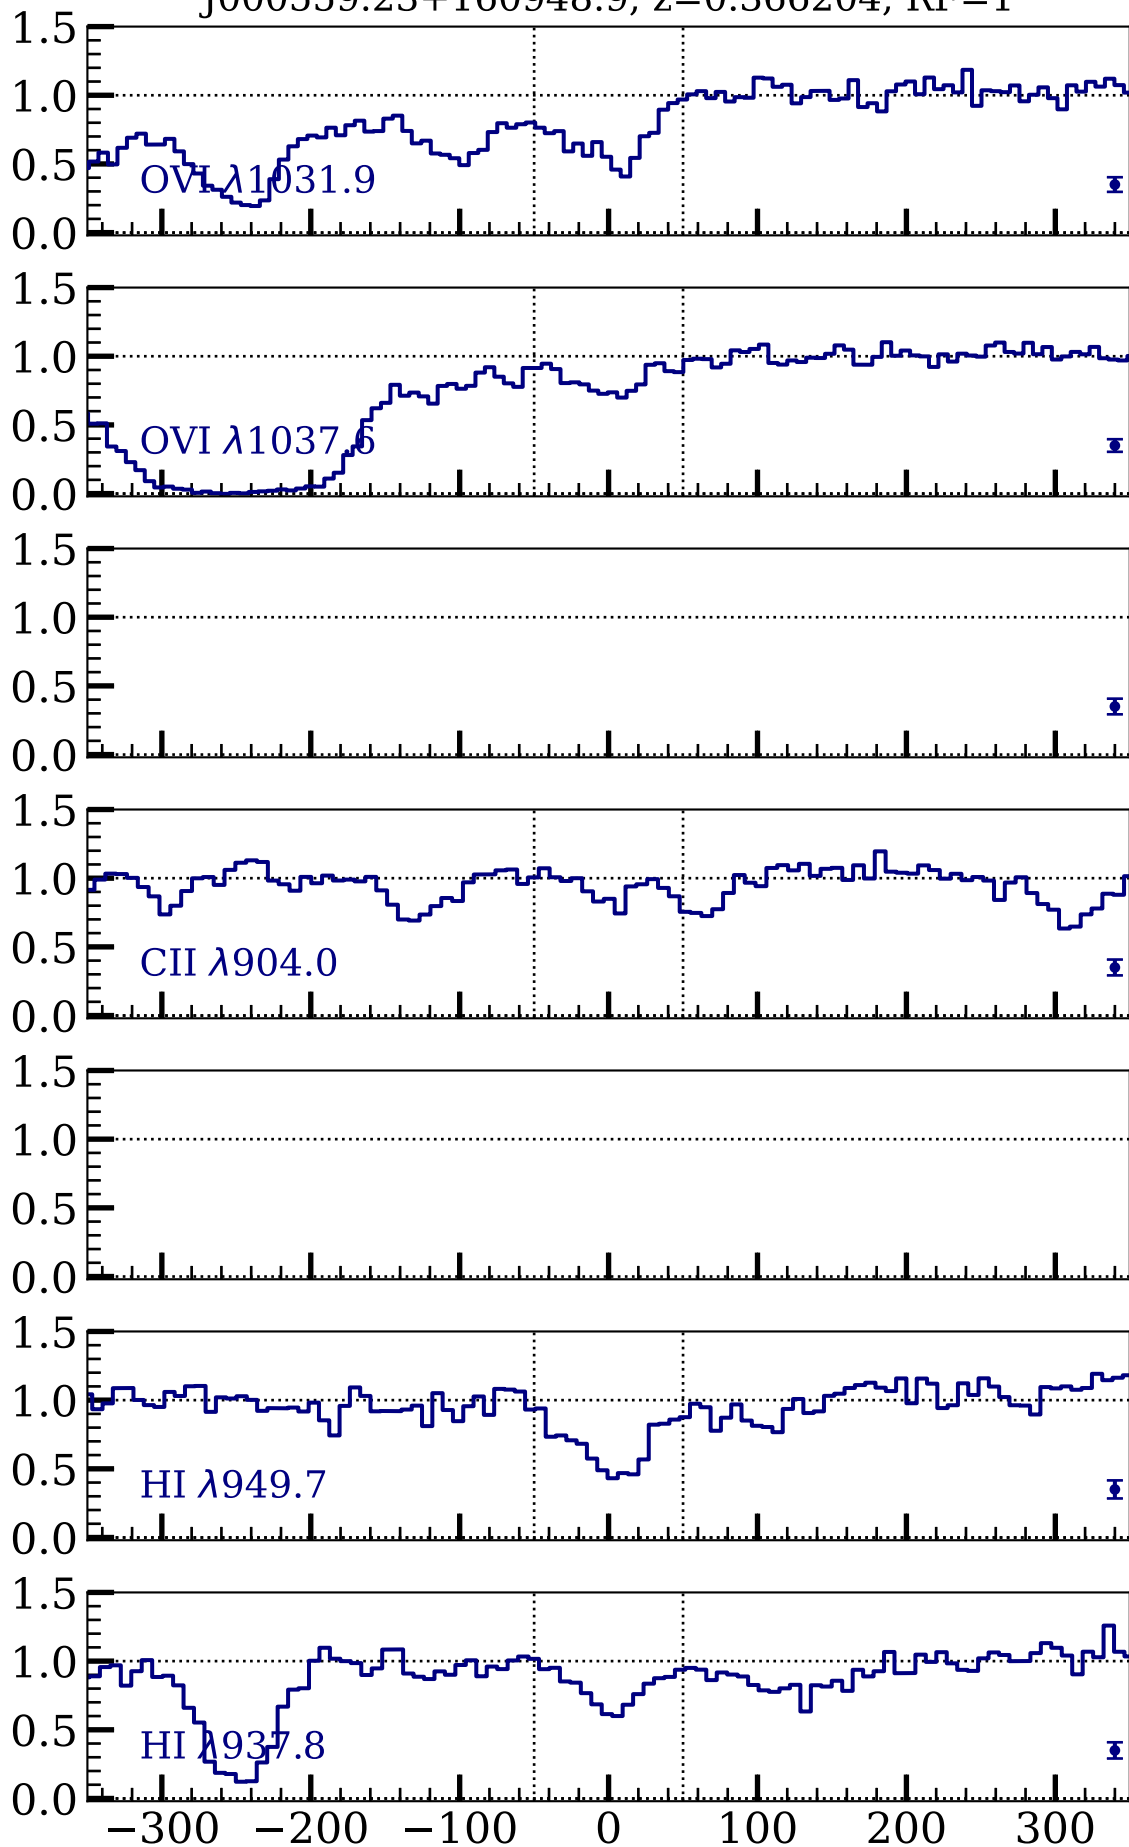

Rest-Frame Velocity (km s<sup>-1</sup>)

J004222.29-103743.8,  $z=0.316052$ , RF=1

Normalized Flux

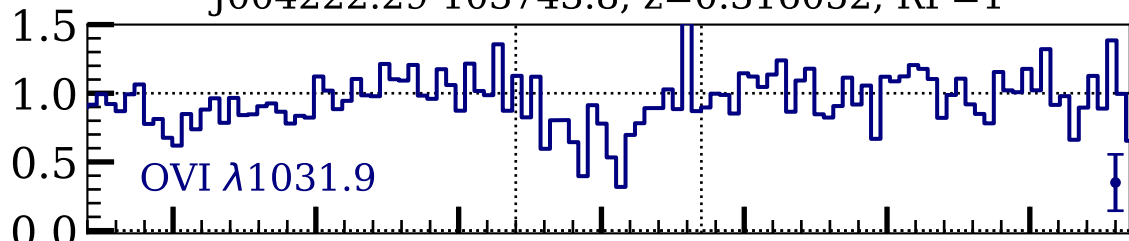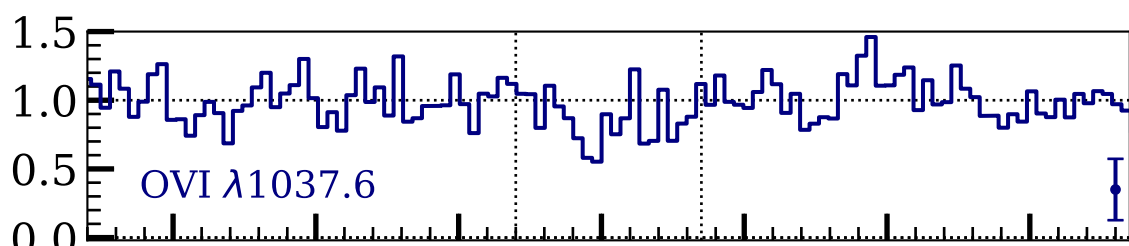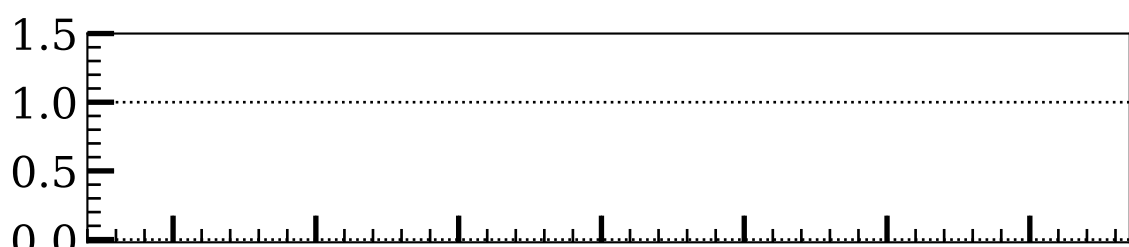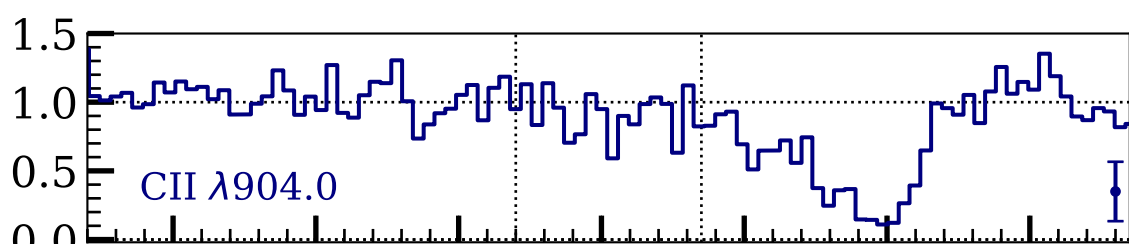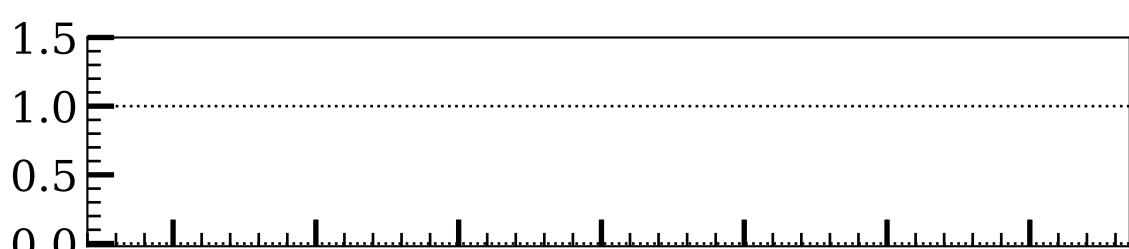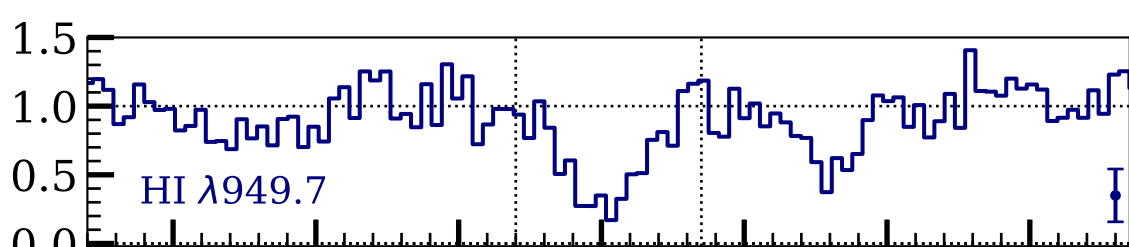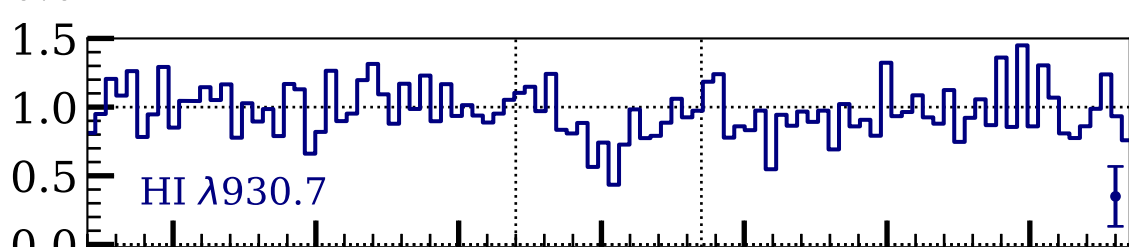

Rest-Frame Velocity ( $\text{km s}^{-1}$ )



J004705.89+031954.9,  $z=0.313870$ , RF=1

Normalized Flux

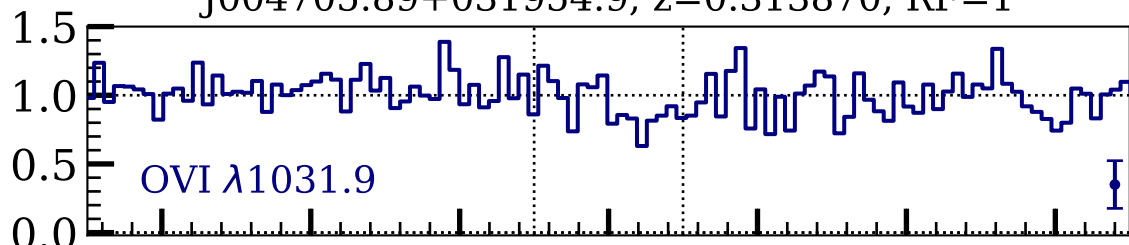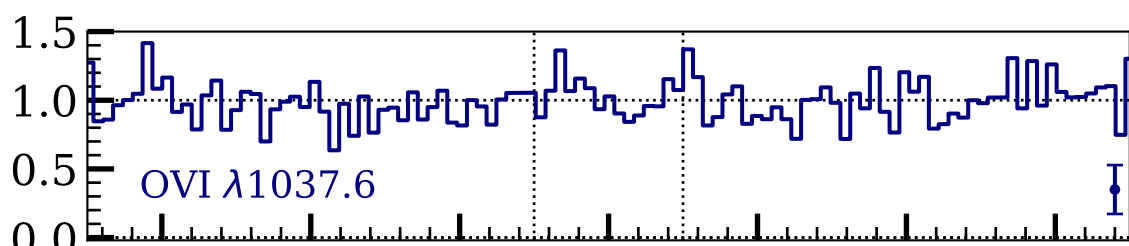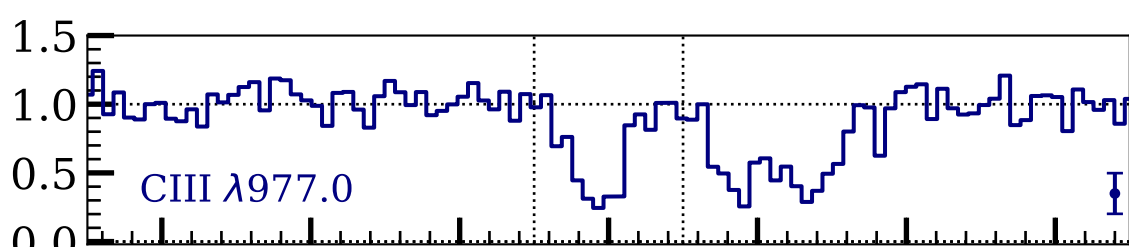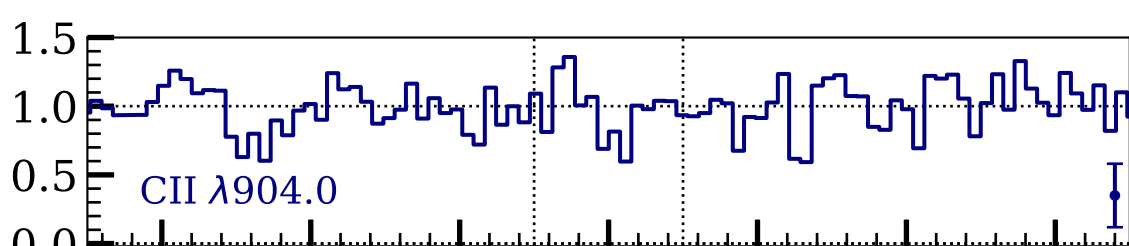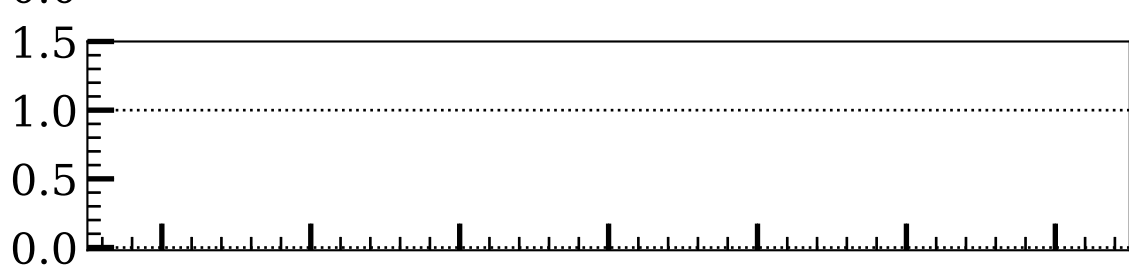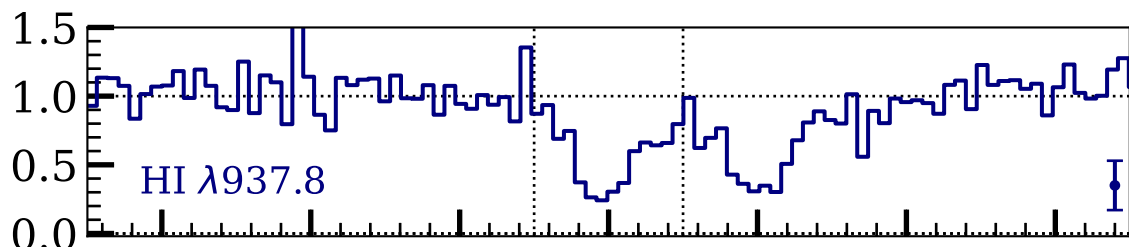

Rest-Frame Velocity ( $\text{km s}^{-1}$ )

J004705.89+031954.9,  $z=0.314257$ , RF=1

Normalized Flux

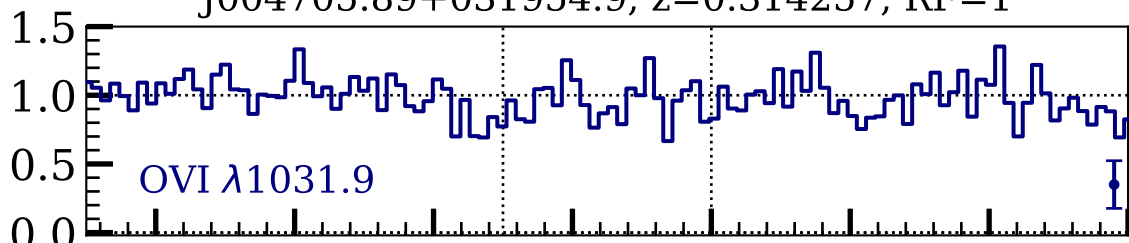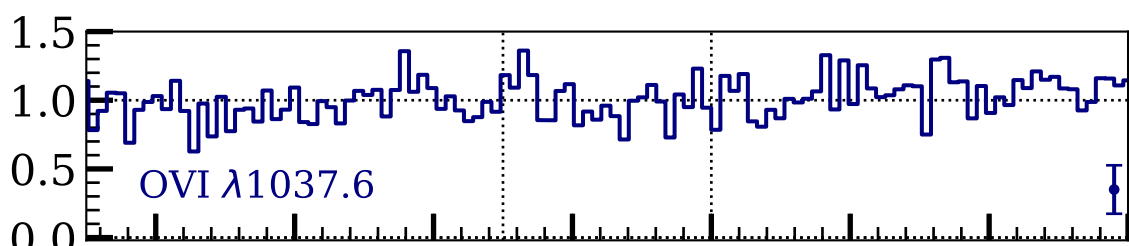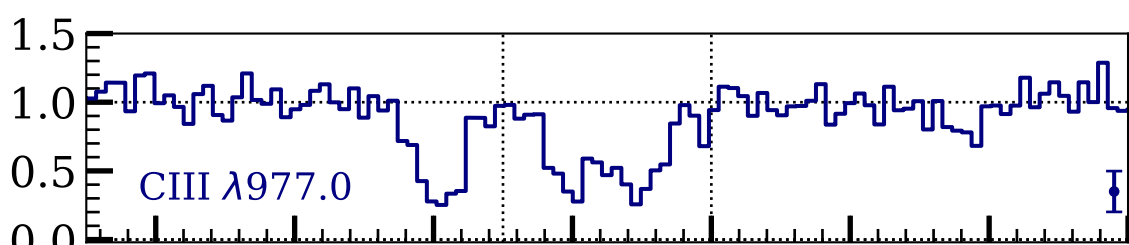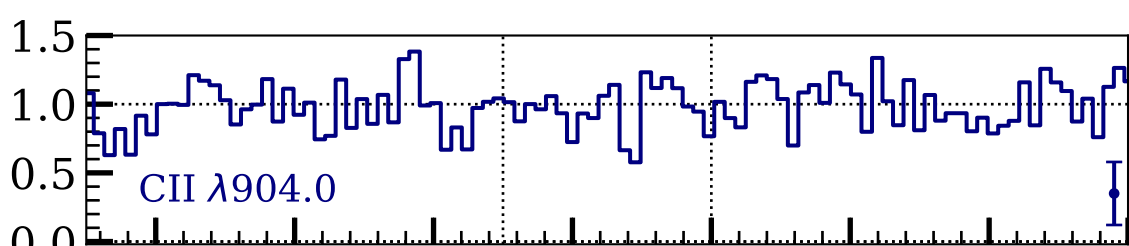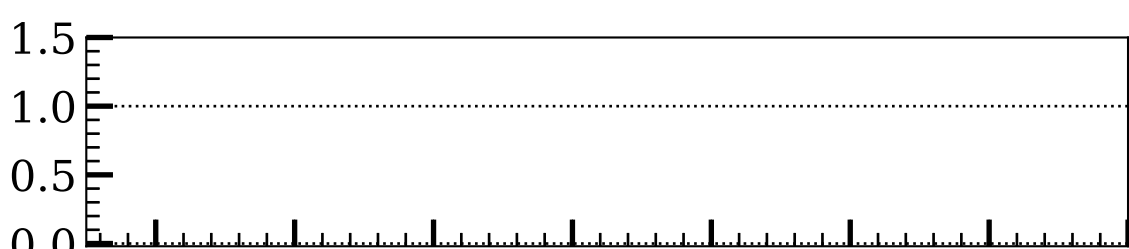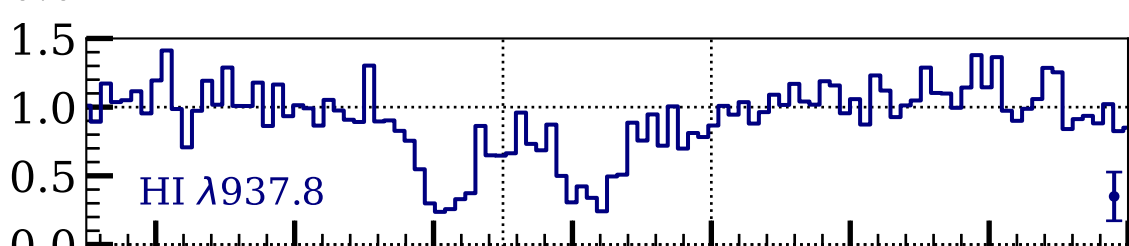

Rest-Frame Velocity ( $\text{km s}^{-1}$ )

J011013.14-021952.8,  $z=0.227191$ , RF=1

Normalized Flux

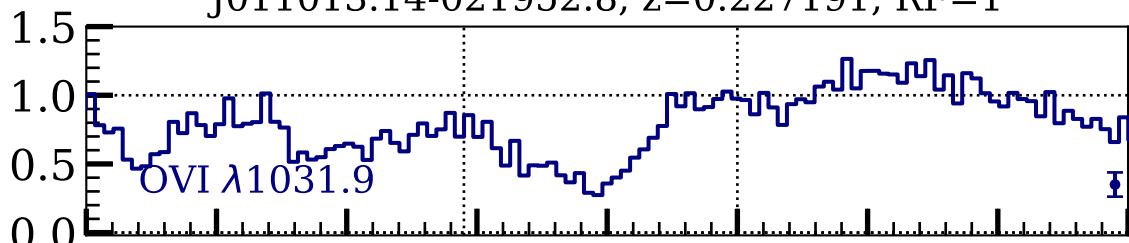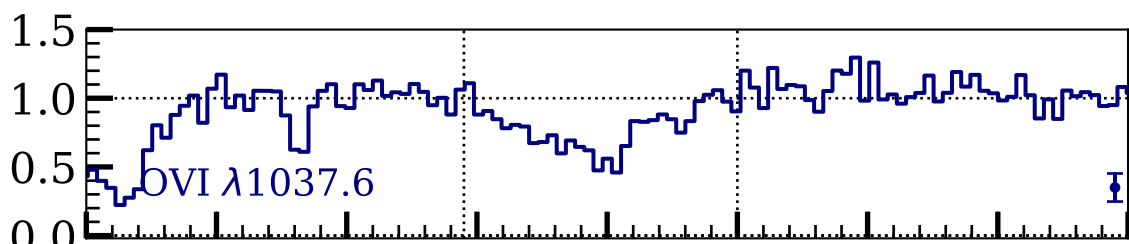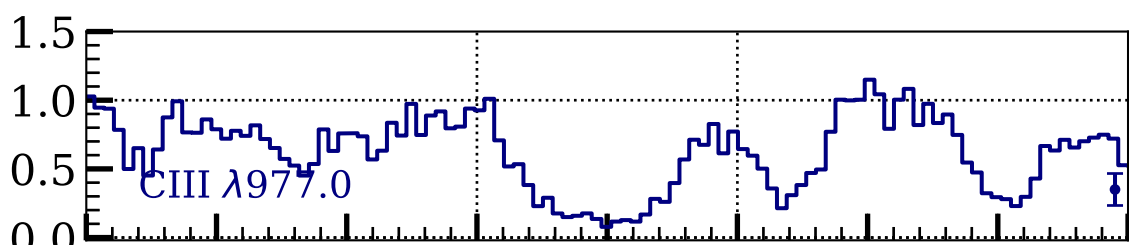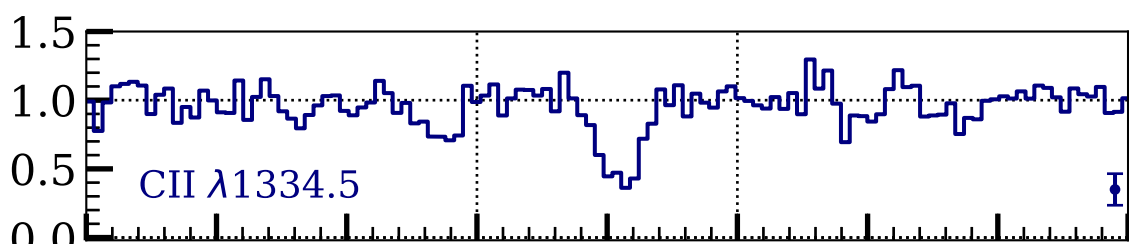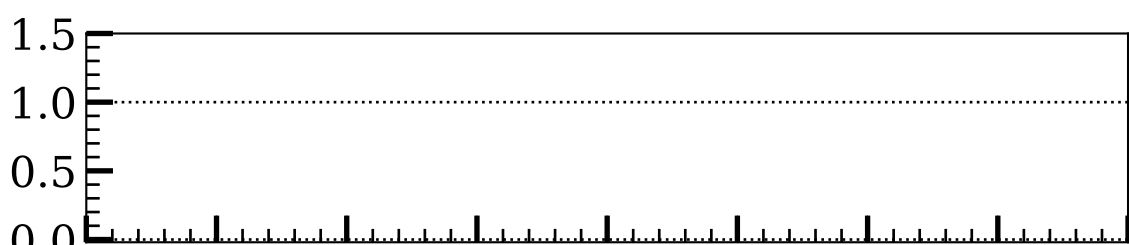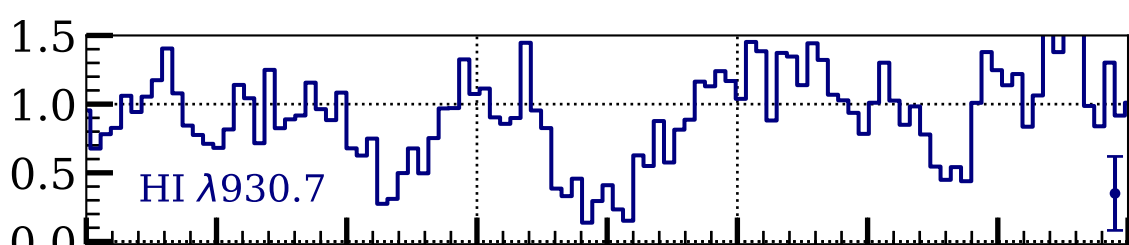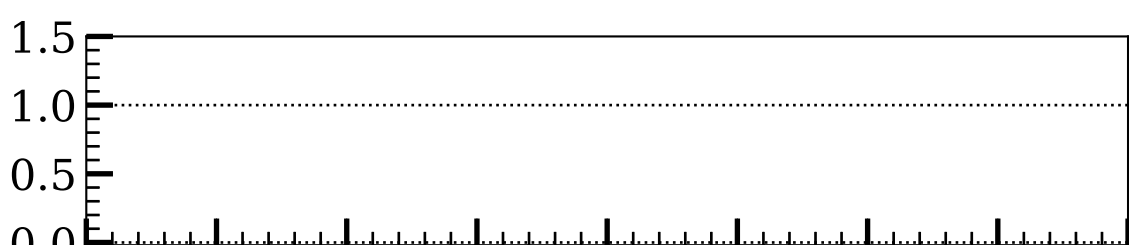

Rest-Frame Velocity (km s<sup>-1</sup>)

J011013.14-021952.8,  $z=0.536490$ , RF=1

Normalized Flux

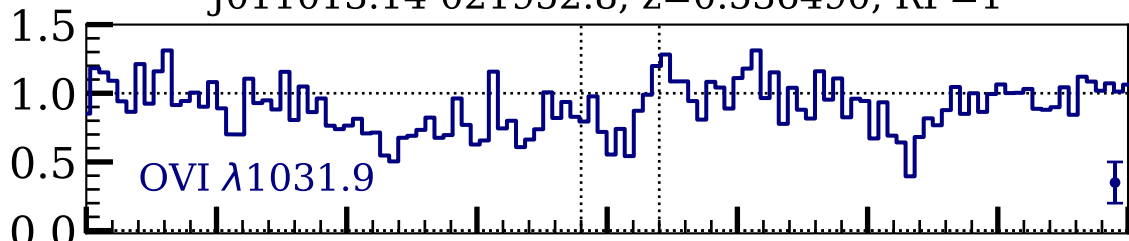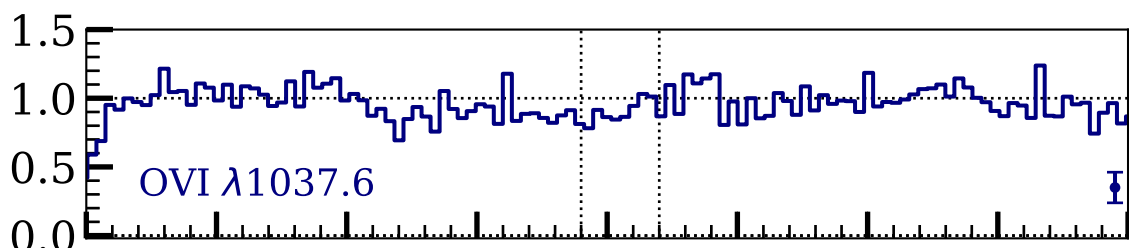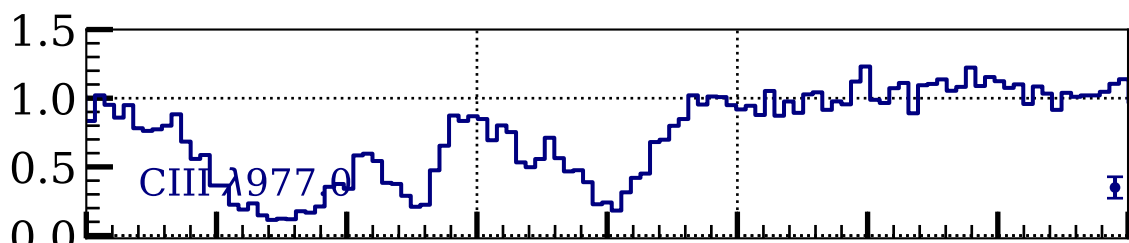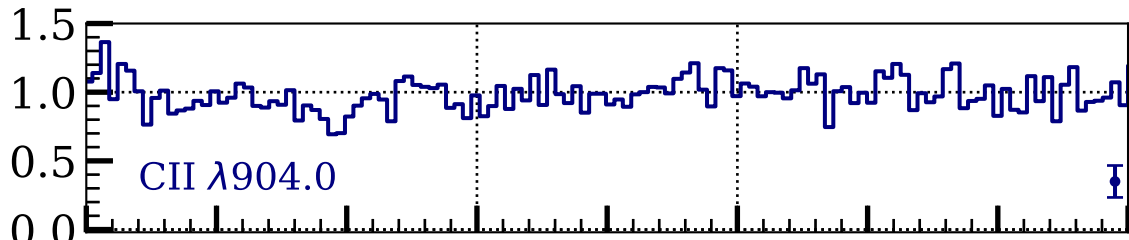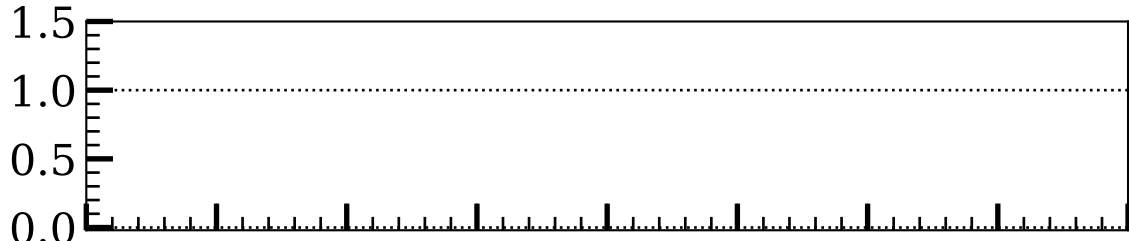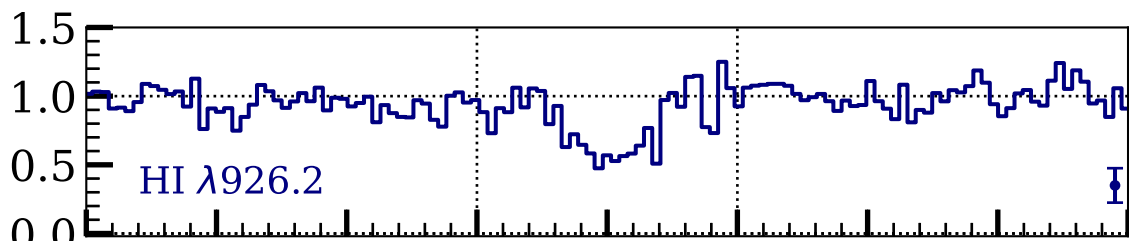

Rest-Frame Velocity ( $\text{km s}^{-1}$ )

Normalized Flux

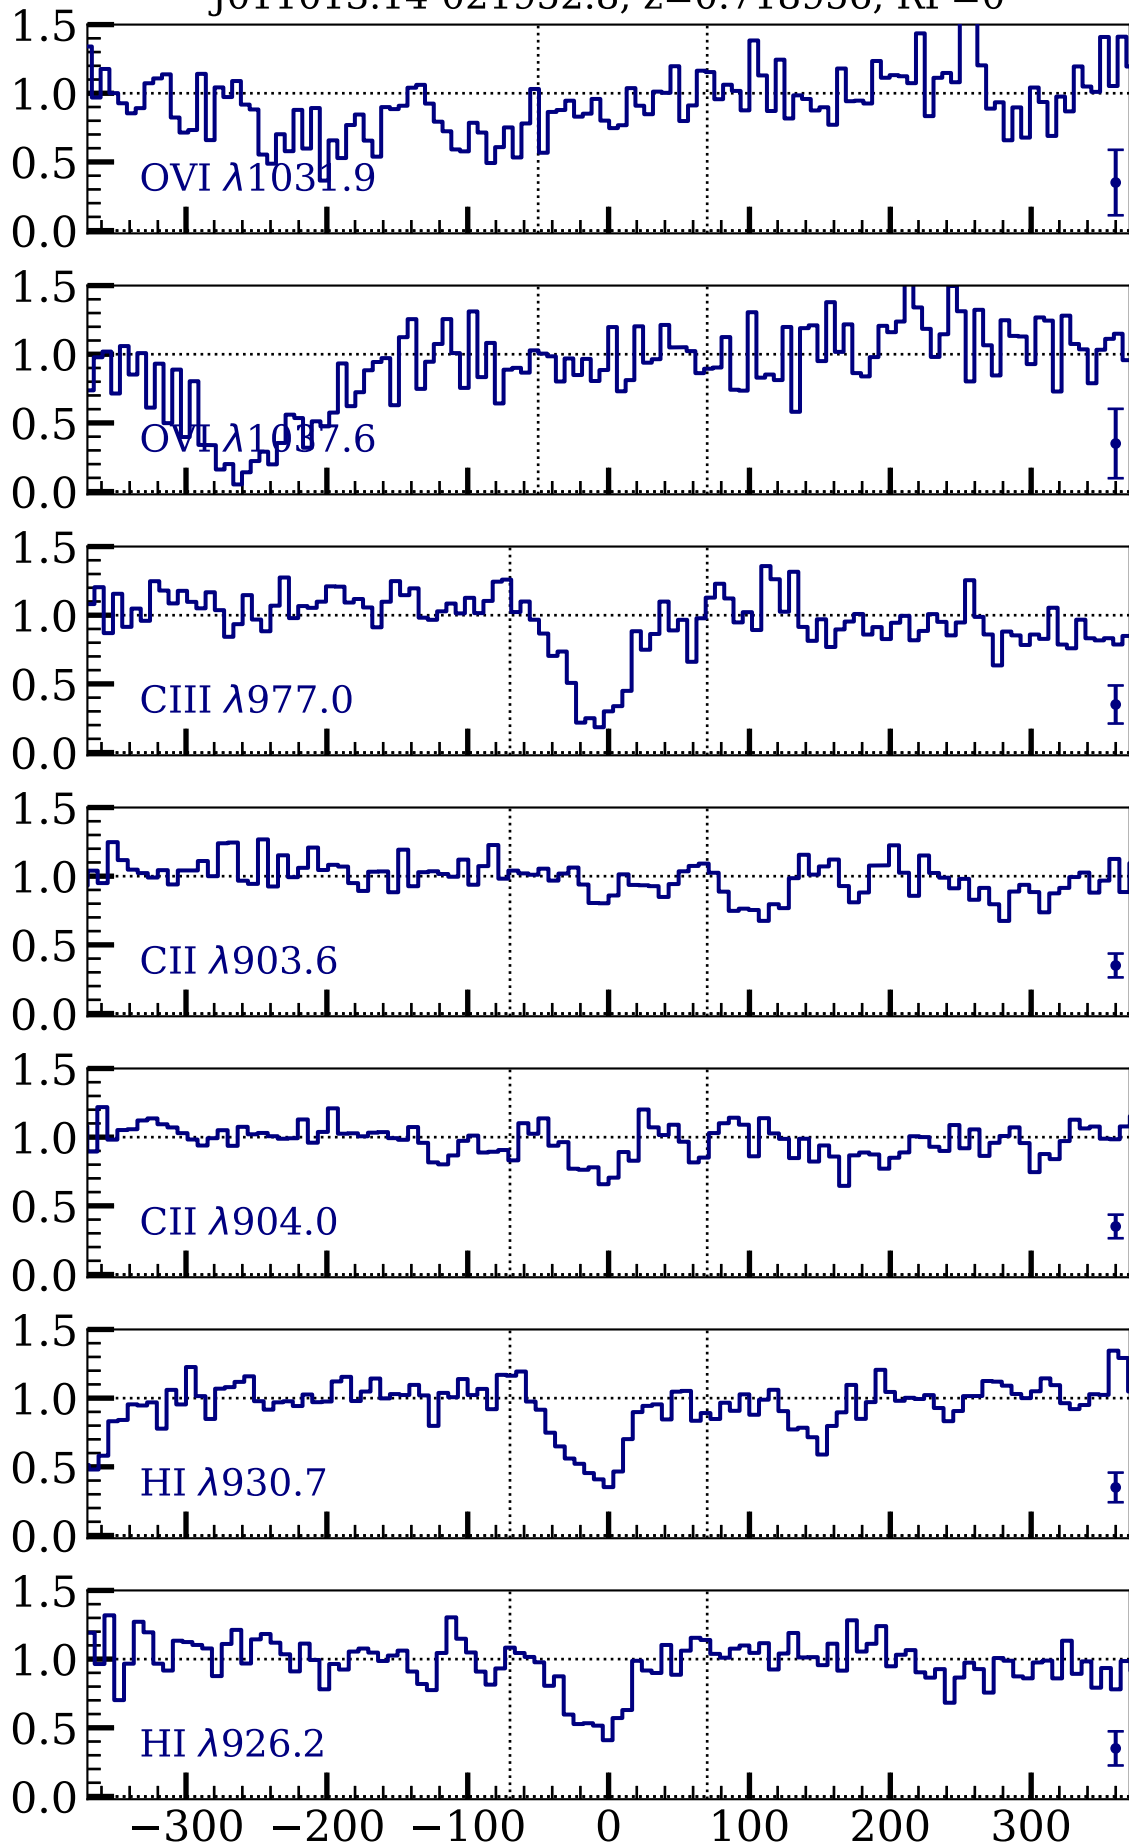Rest-Frame Velocity (km s<sup>-1</sup>)

J011016.25-021851.0,  $z=0.399146$ , RF=1

Normalized Flux

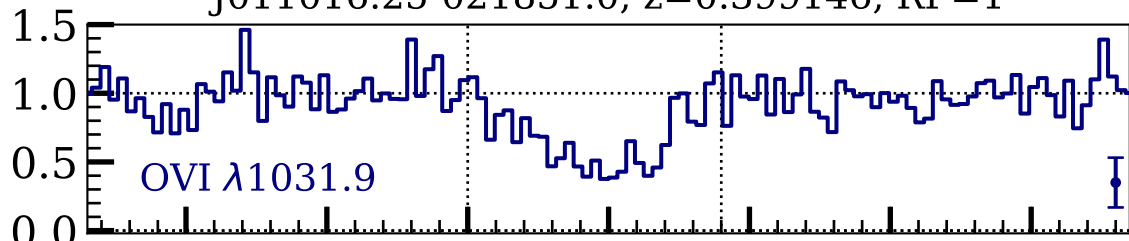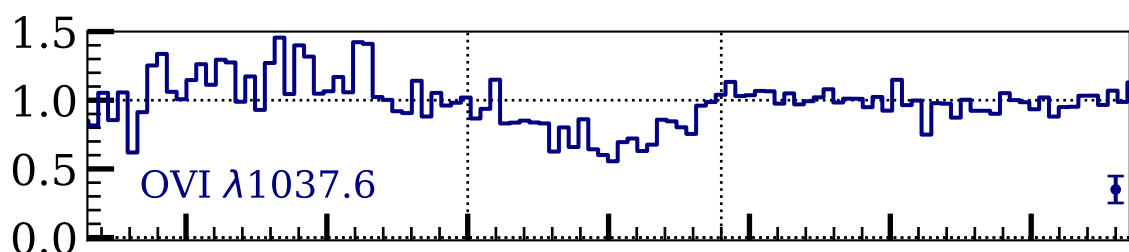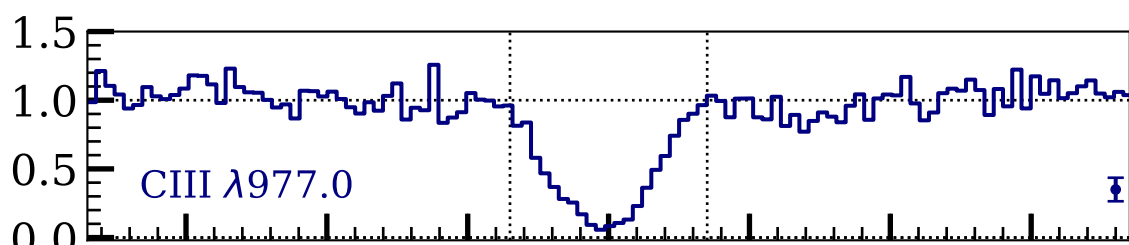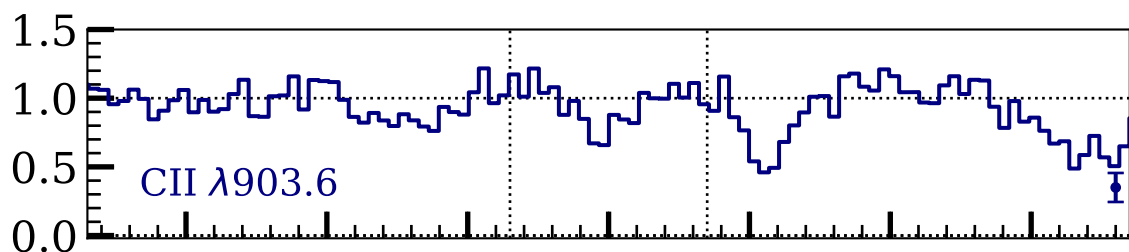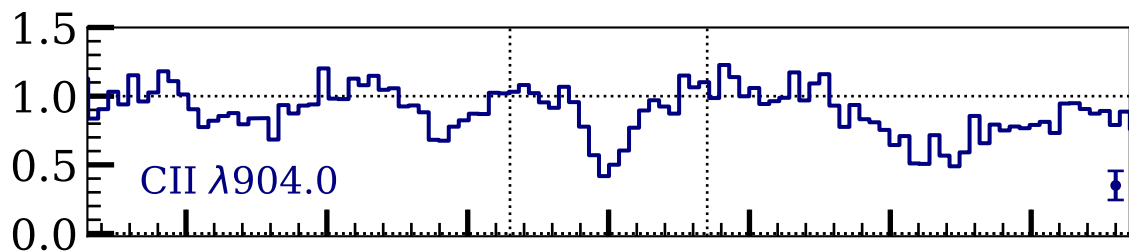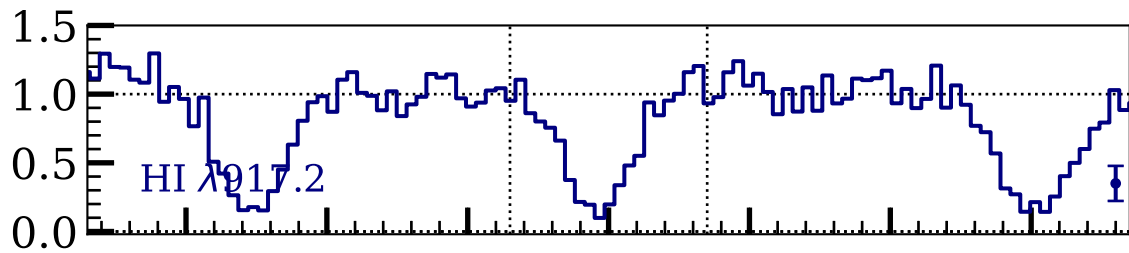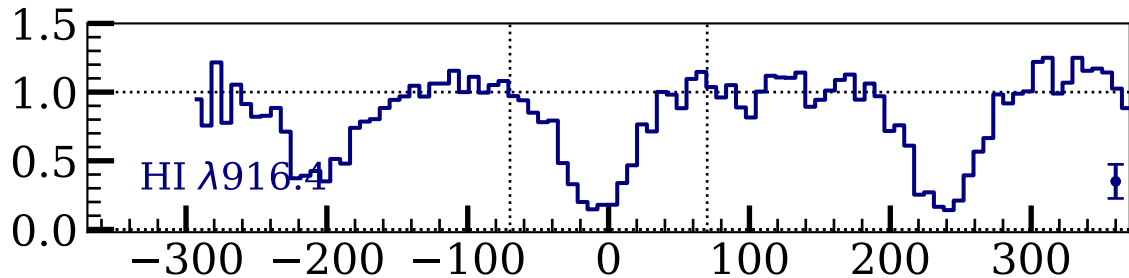

Rest-Frame Velocity ( $\text{km s}^{-1}$ )

J011016.25-021851.0,  $z=0.535375$ , RF=1

Normalized Flux

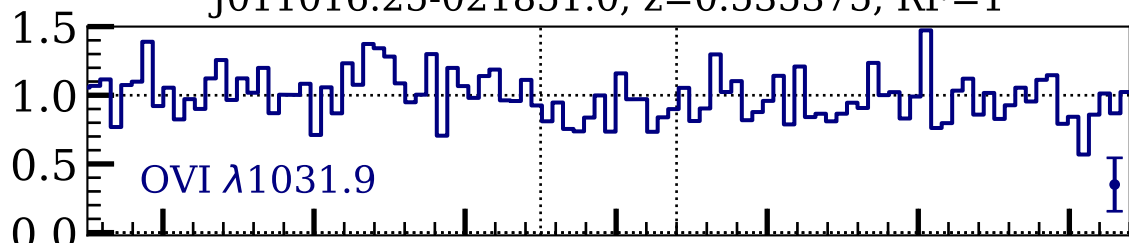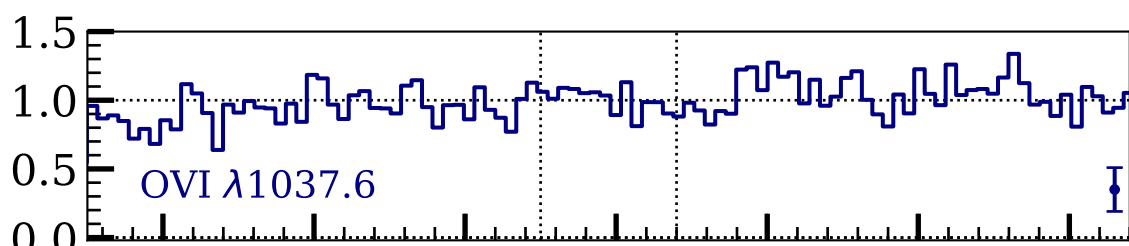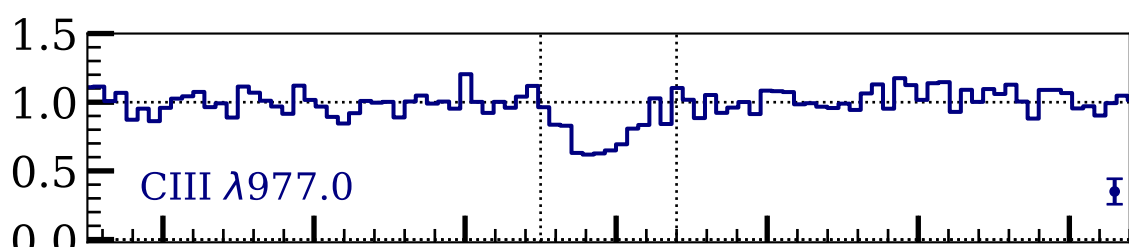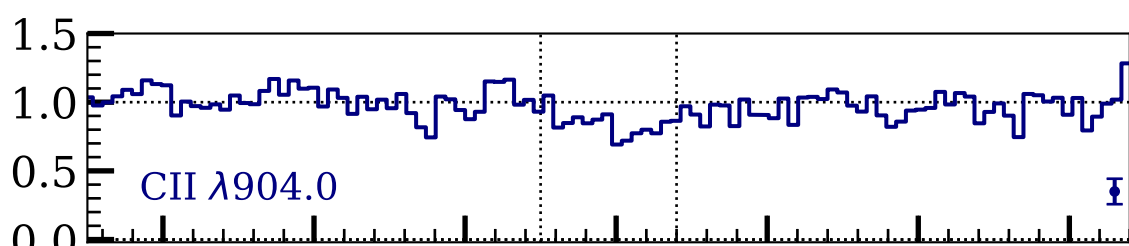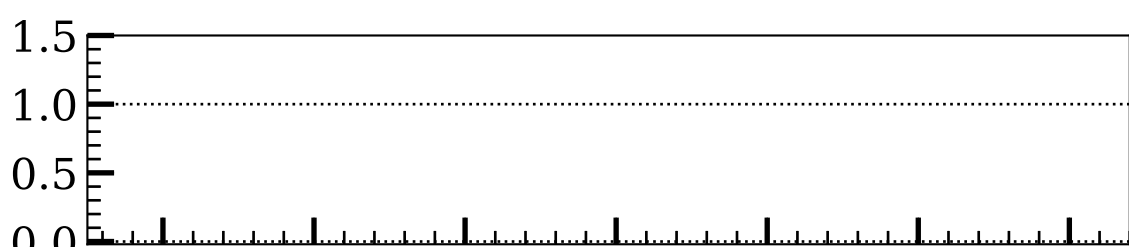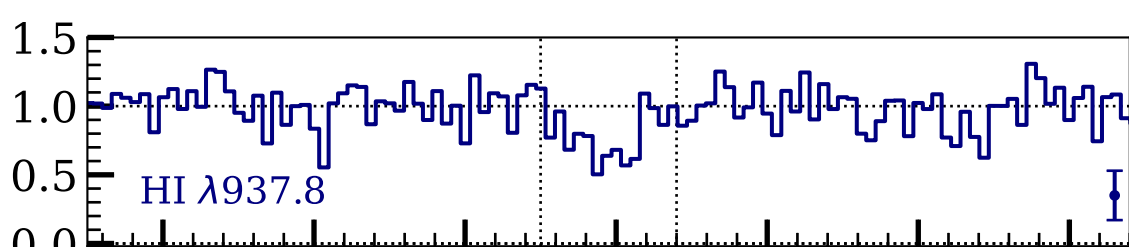

Rest-Frame Velocity ( $\text{km s}^{-1}$ )

J011016.25-021851.0,  $z=0.717956$ , RF=0

Normalized Flux

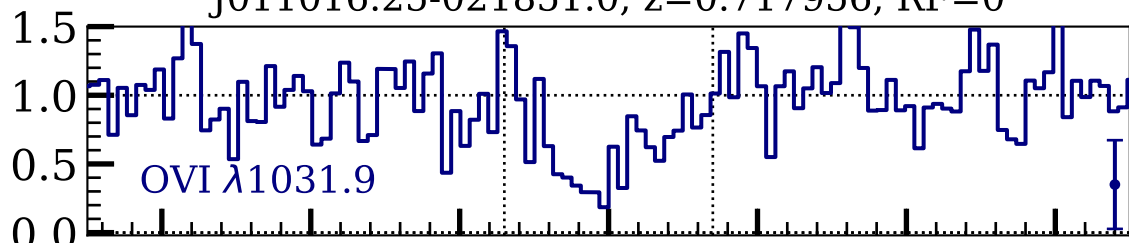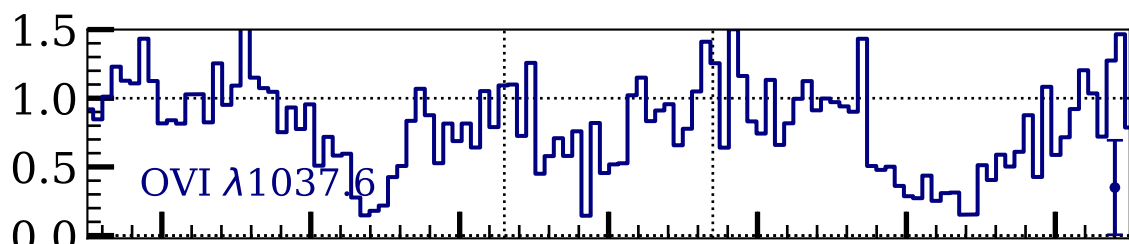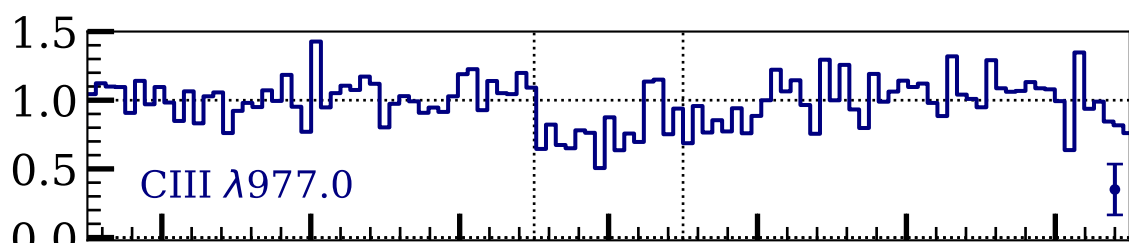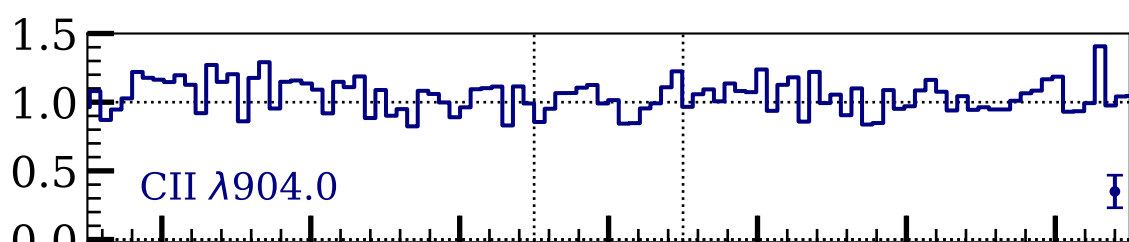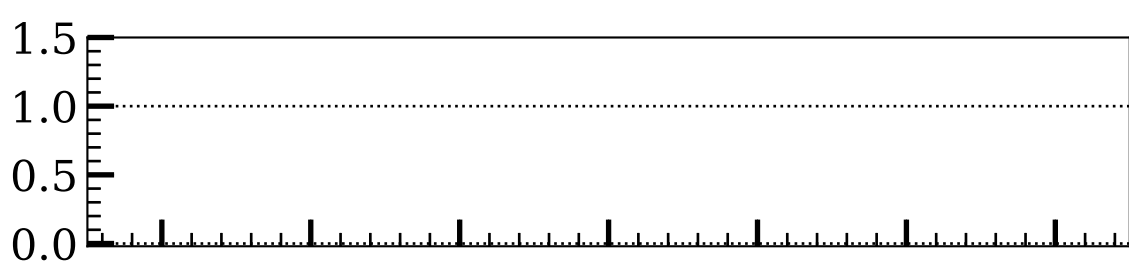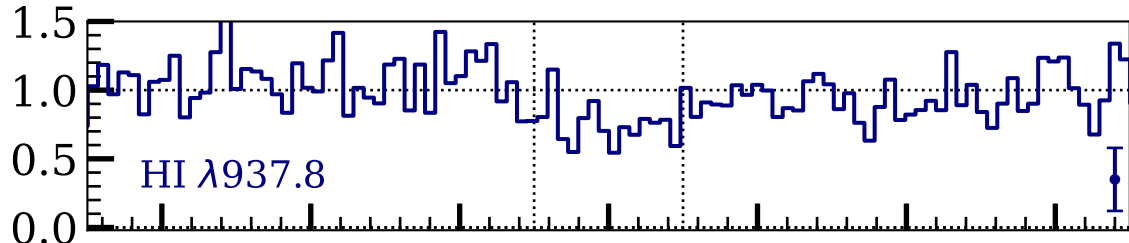

Rest-Frame Velocity ( $\text{km s}^{-1}$ )



J011623.04+142940.5,  $z=0.333777$ , RF=0

Normalized Flux

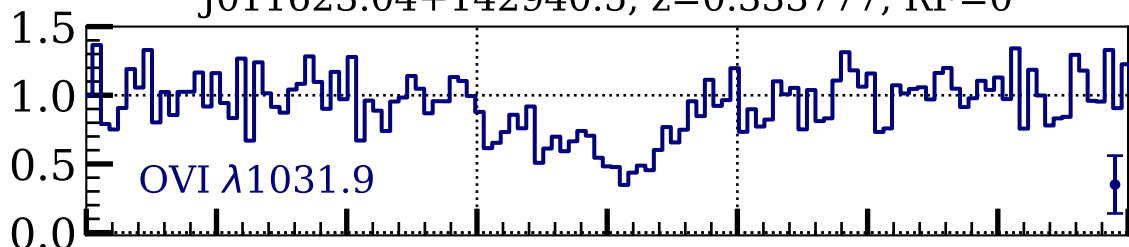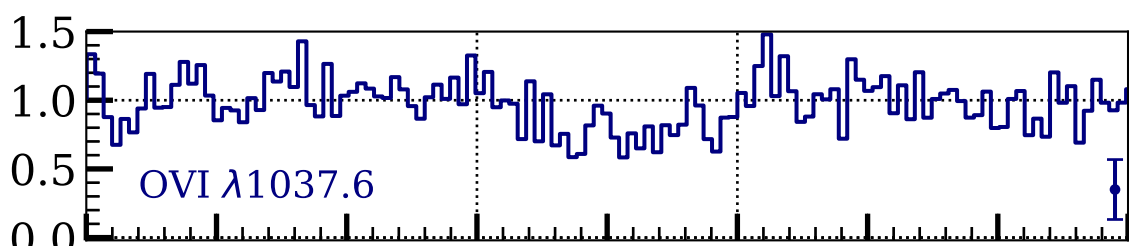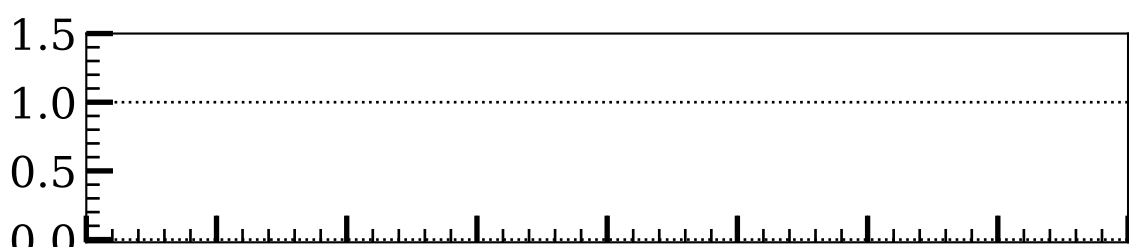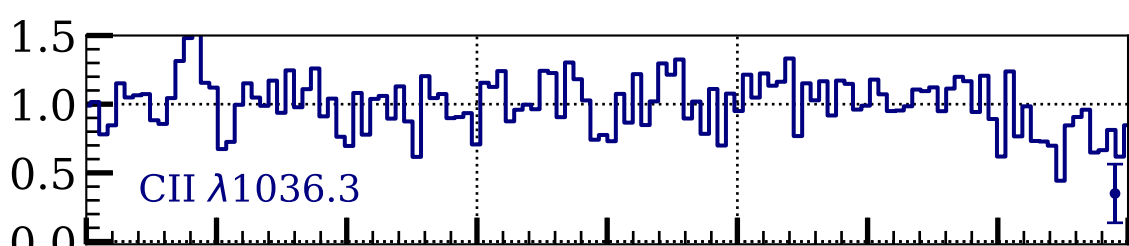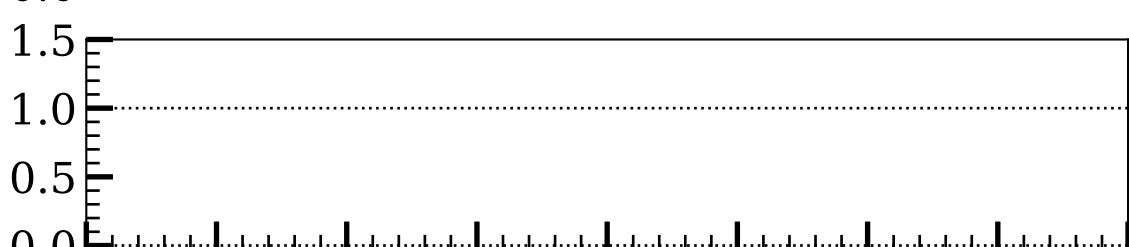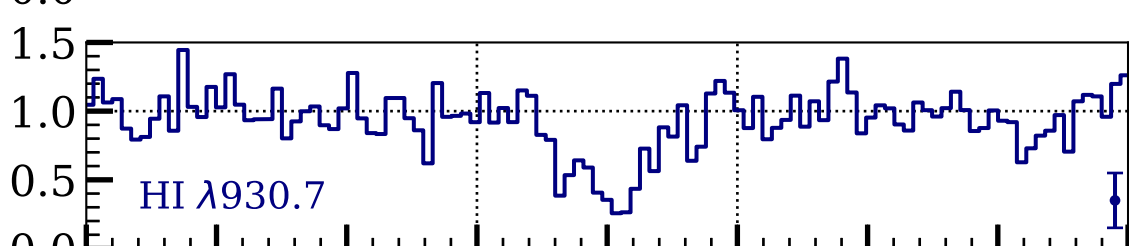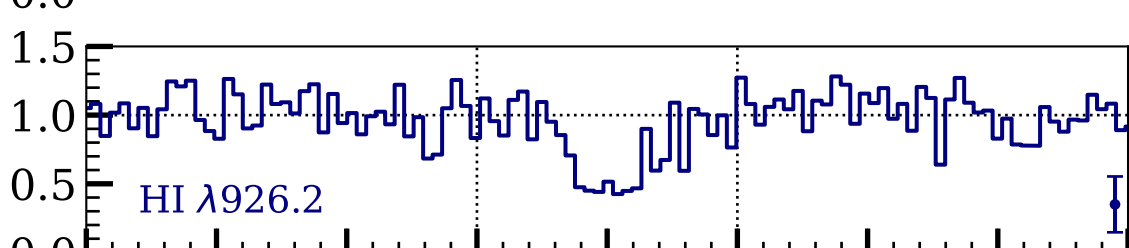

Rest-Frame Velocity ( $\text{km s}^{-1}$ )

J011935.69-282131.4,  $z=0.348326$ , RF=1

Normalized Flux

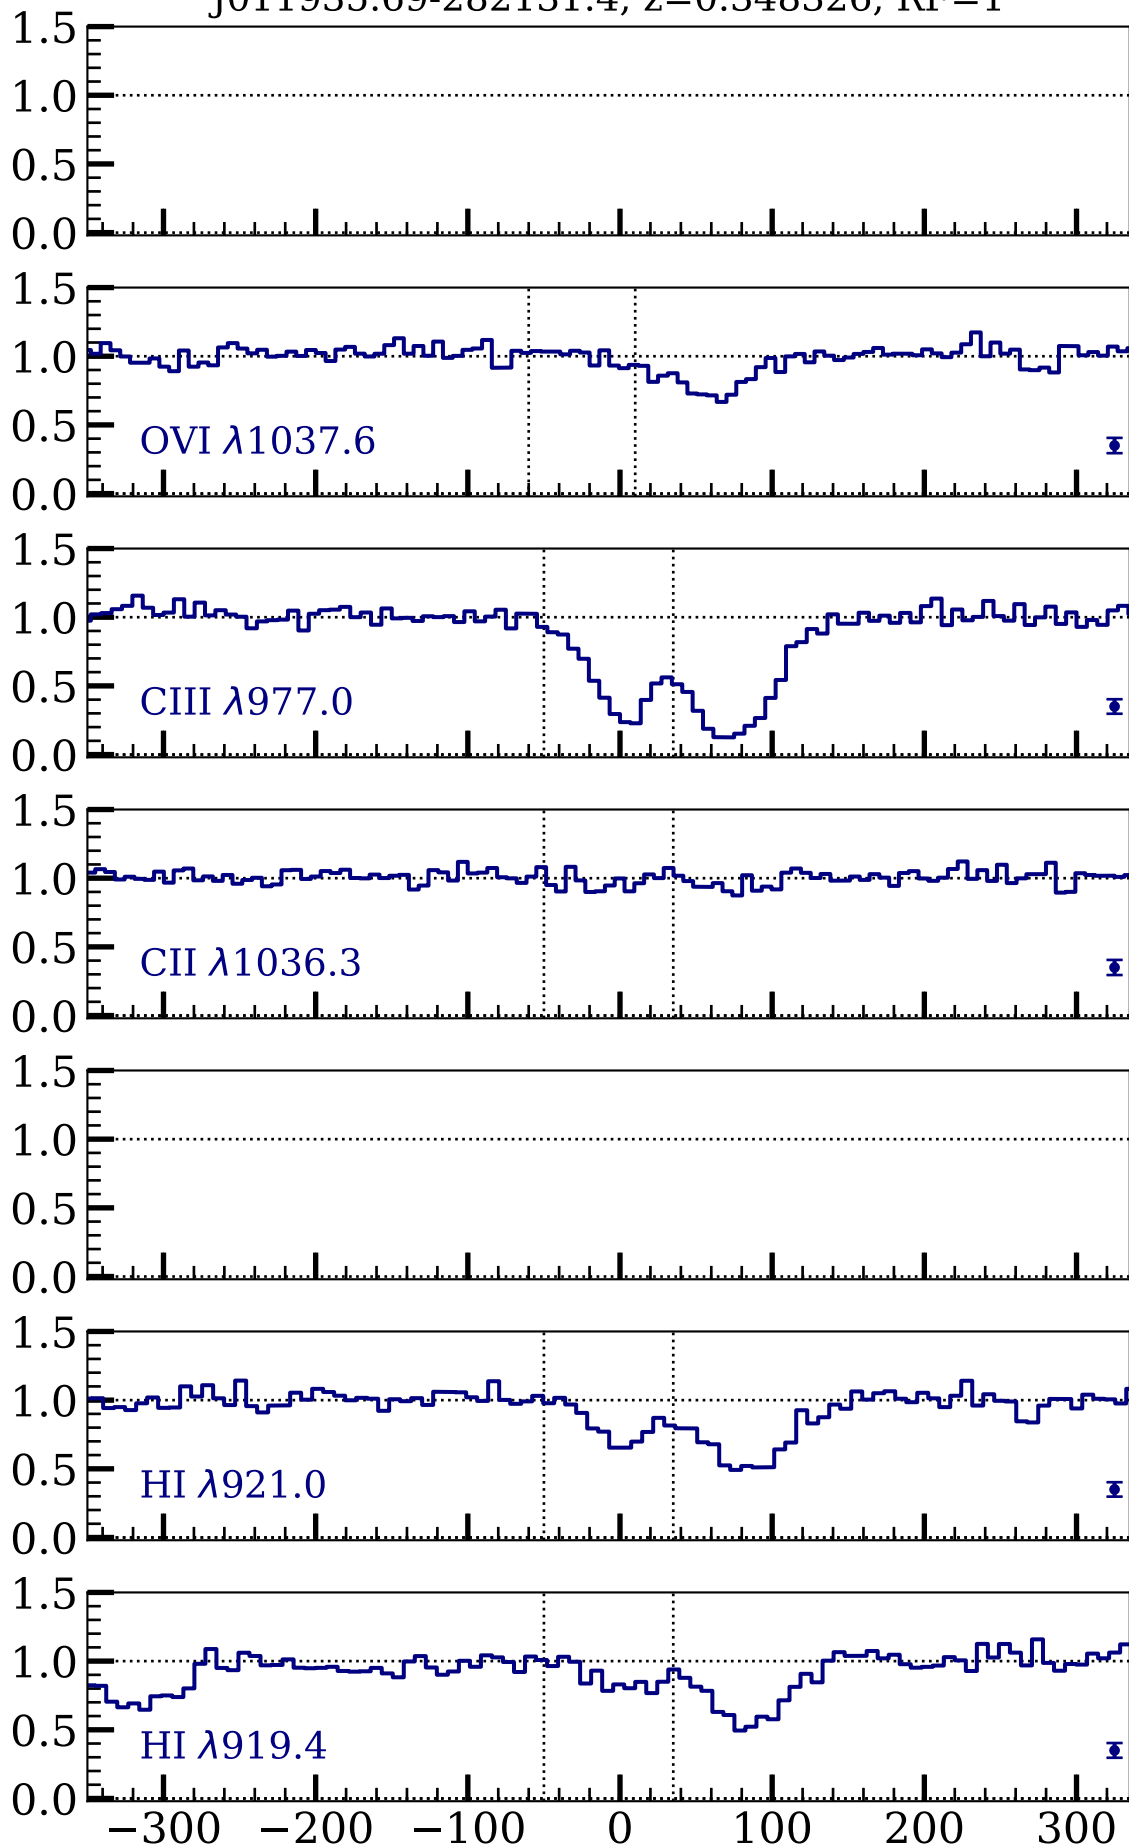

Rest-Frame Velocity (km s<sup>-1</sup>)

J011935.69-282131.4,  $z=0.348731$ , RF=1

Normalized Flux

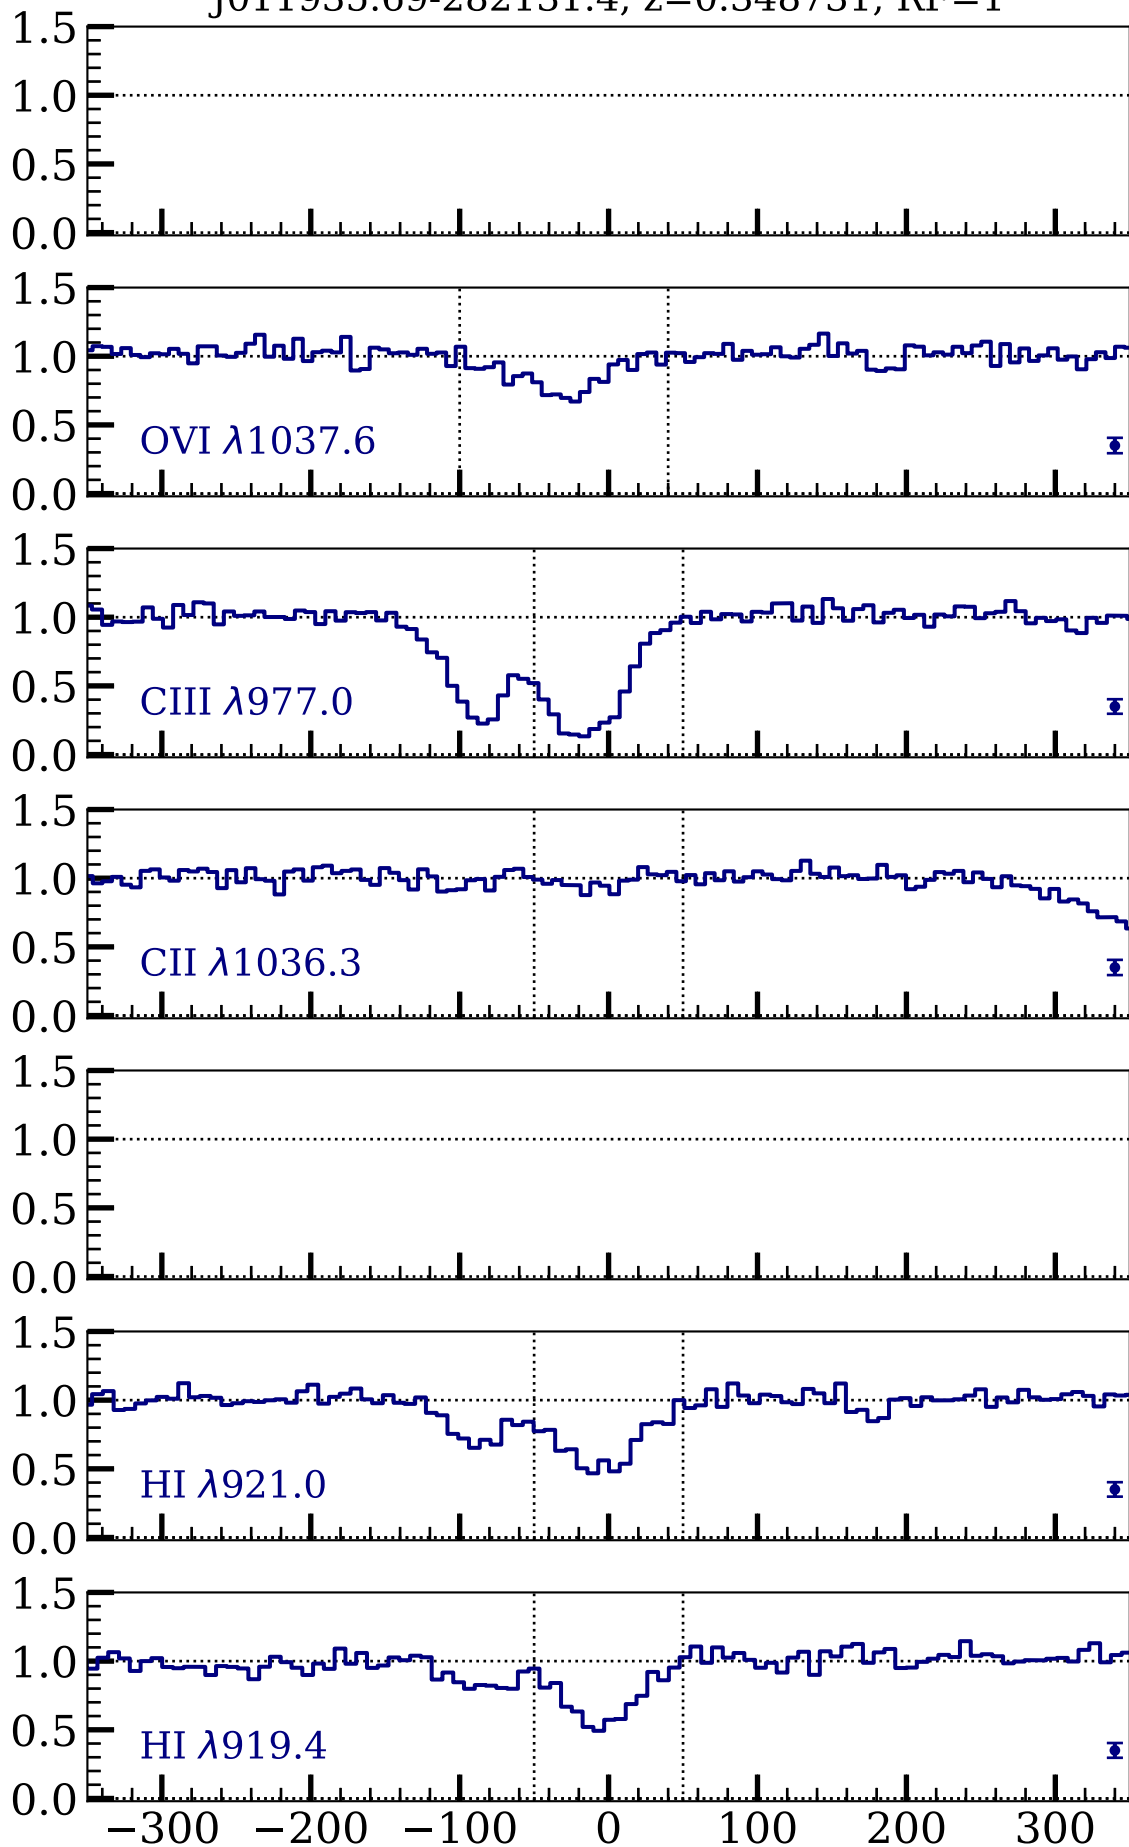

Rest-Frame Velocity ( $\text{km s}^{-1}$ )

J012236.76-284321.3,  $z=0.364959$ , RF=1

Normalized Flux

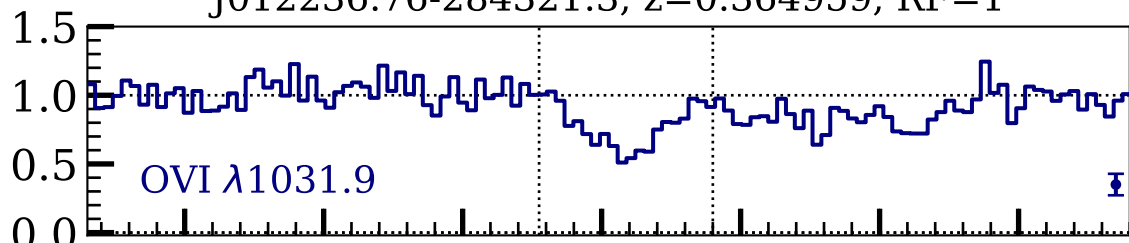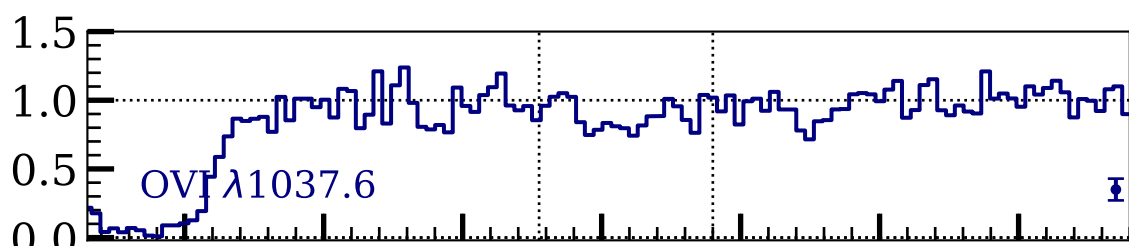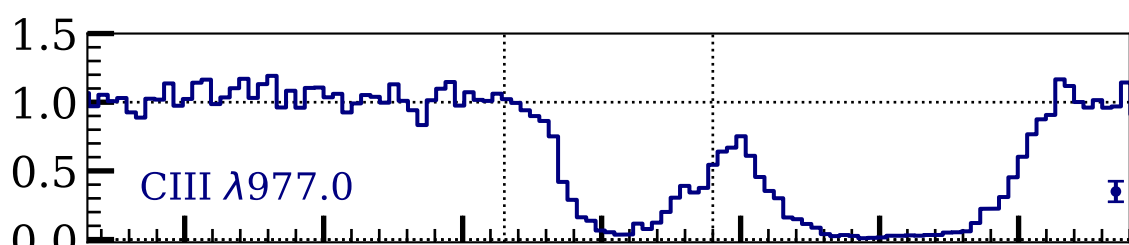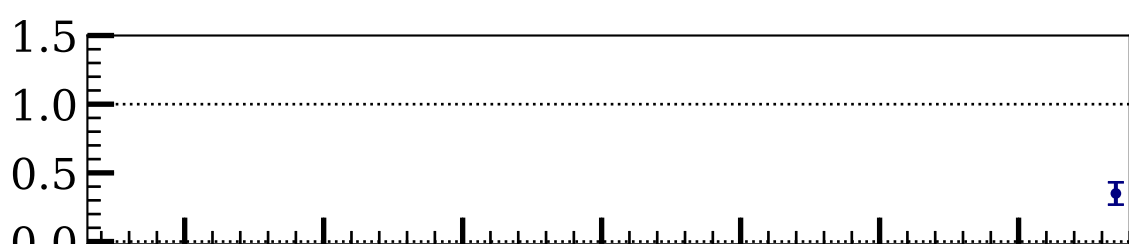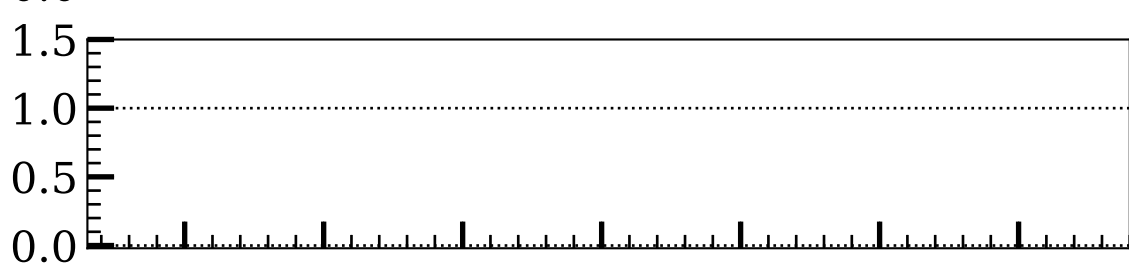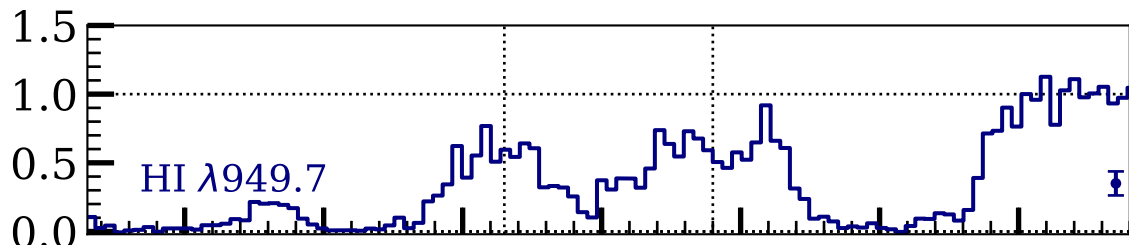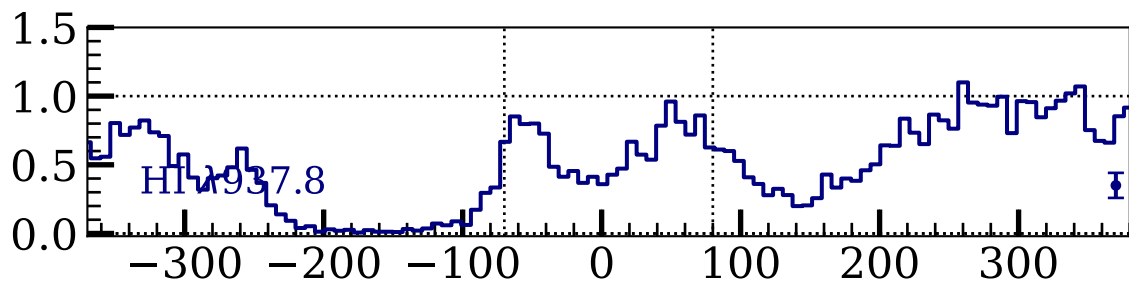

Rest-Frame Velocity ( $\text{km s}^{-1}$ )

J015513.20-450611.9,  $z=0.225958$ , RF=1

Normalized Flux

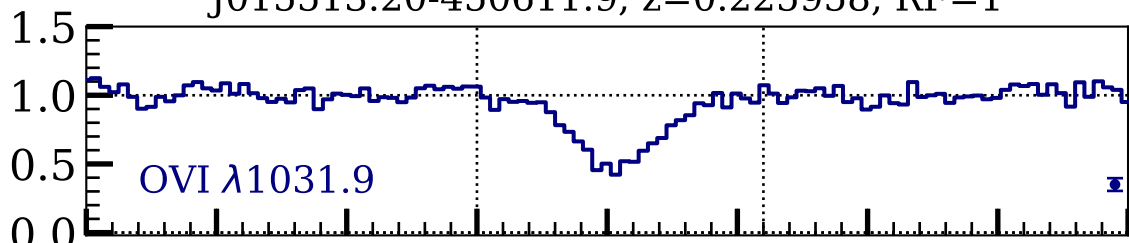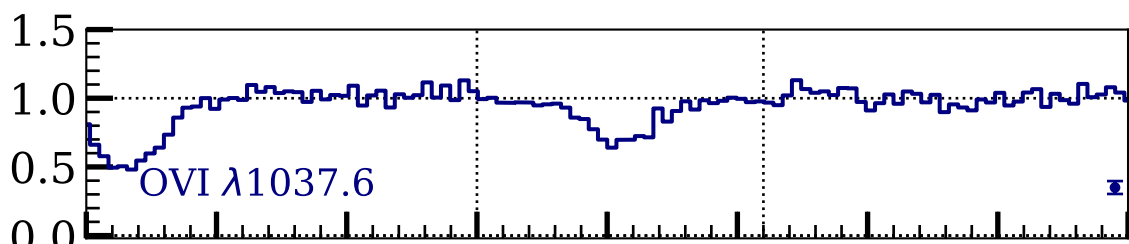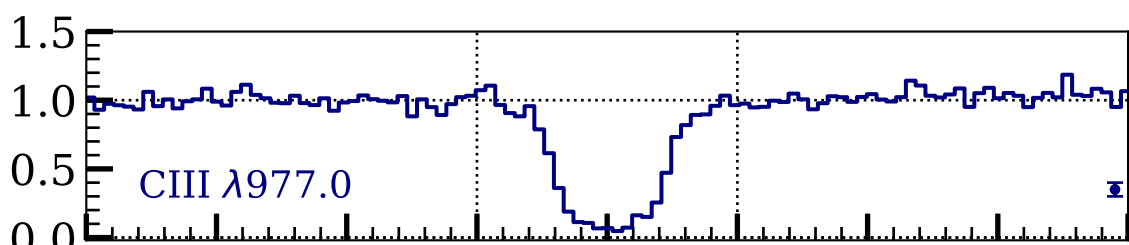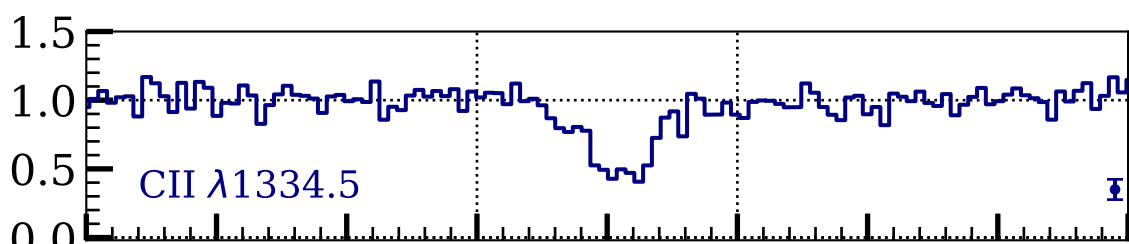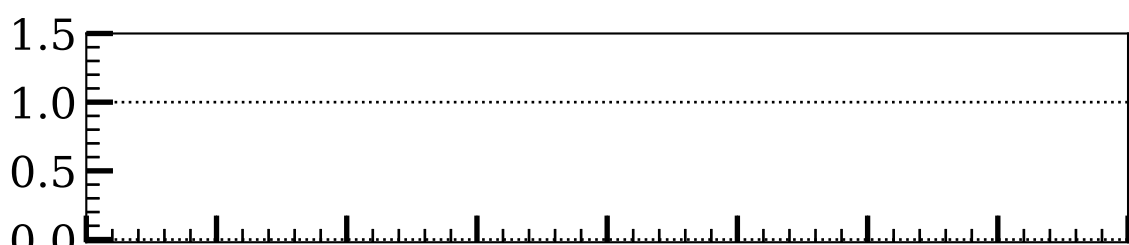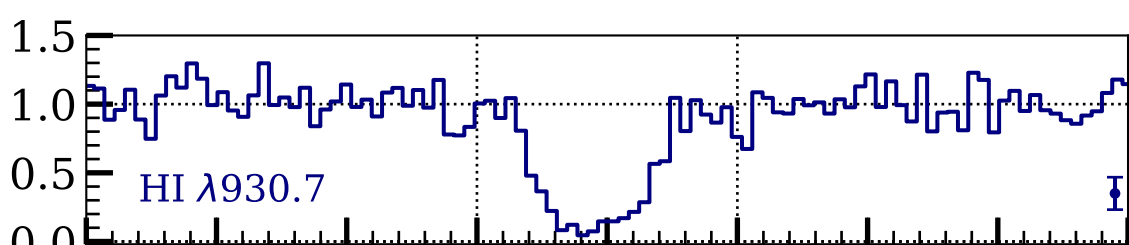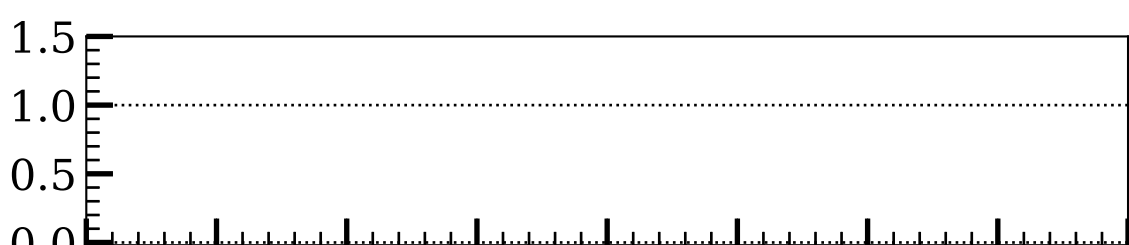

Rest-Frame Velocity ( $\text{km s}^{-1}$ )

J020157.16-113233.1,  $z=0.322565$ , RF=1

Normalized Flux

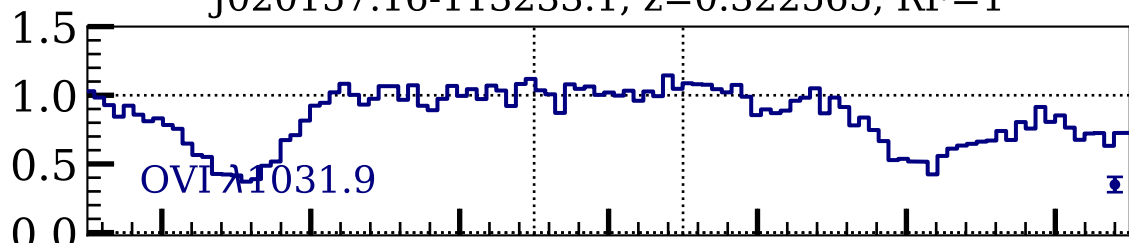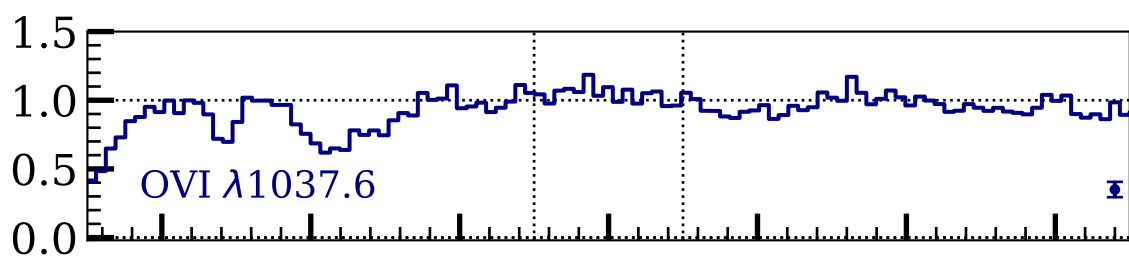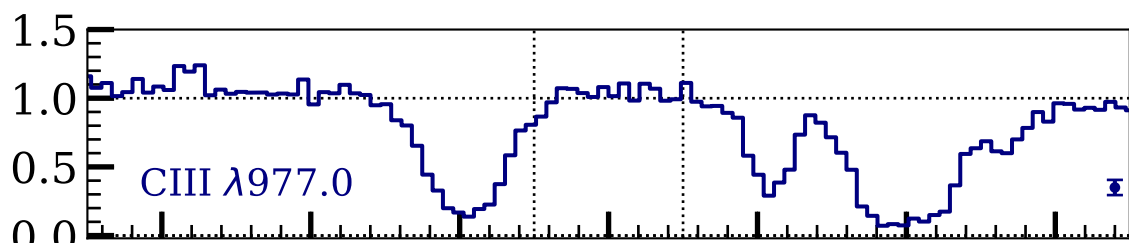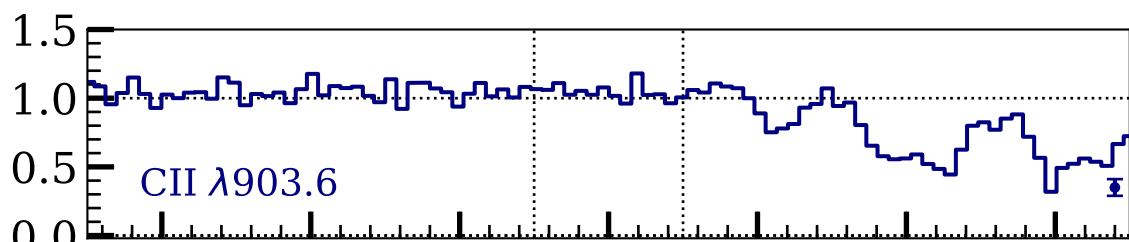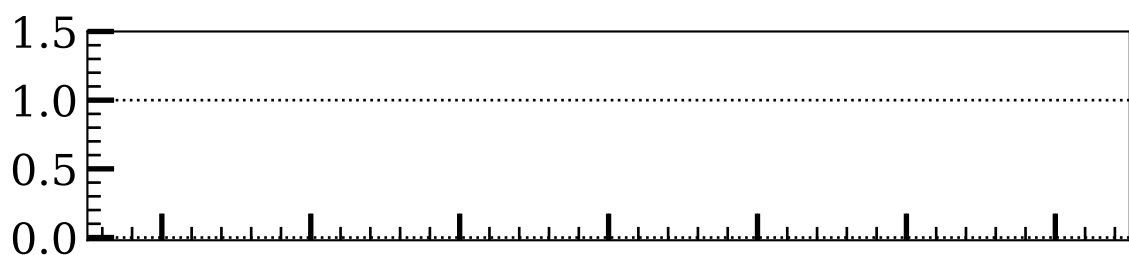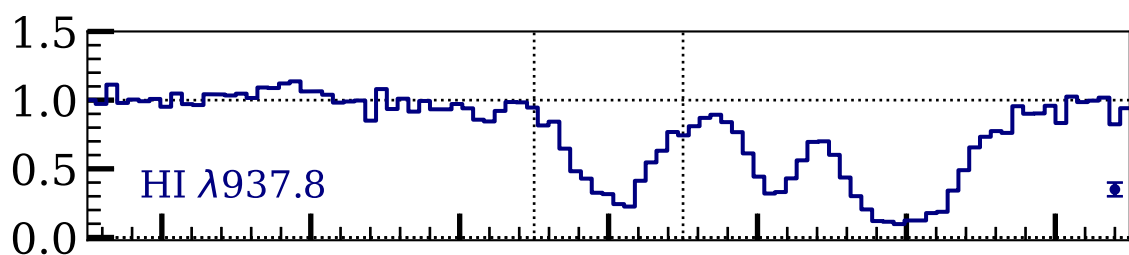

Rest-Frame Velocity ( $\text{km s}^{-1}$ )

J020157.16-113233.1,  $z=0.323073$ , RF=1

Normalized Flux

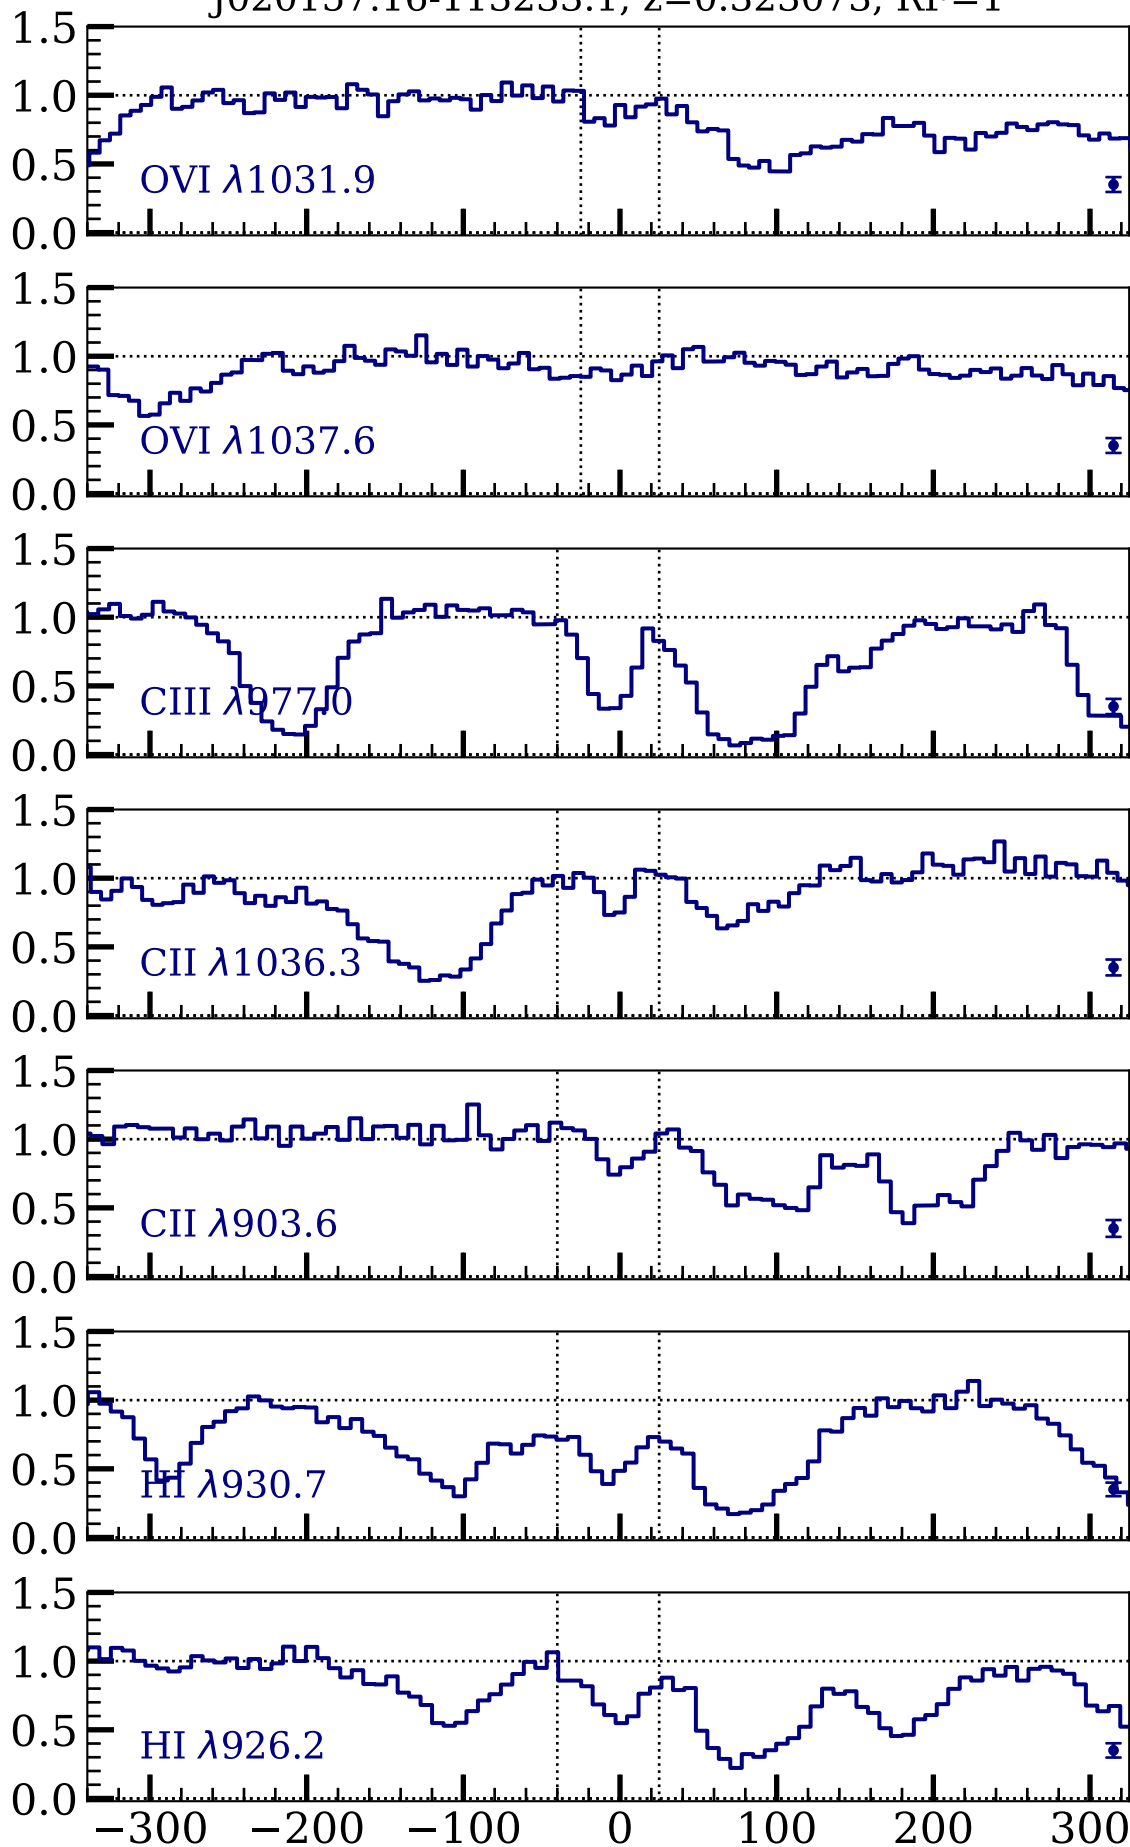

Normalized Flux

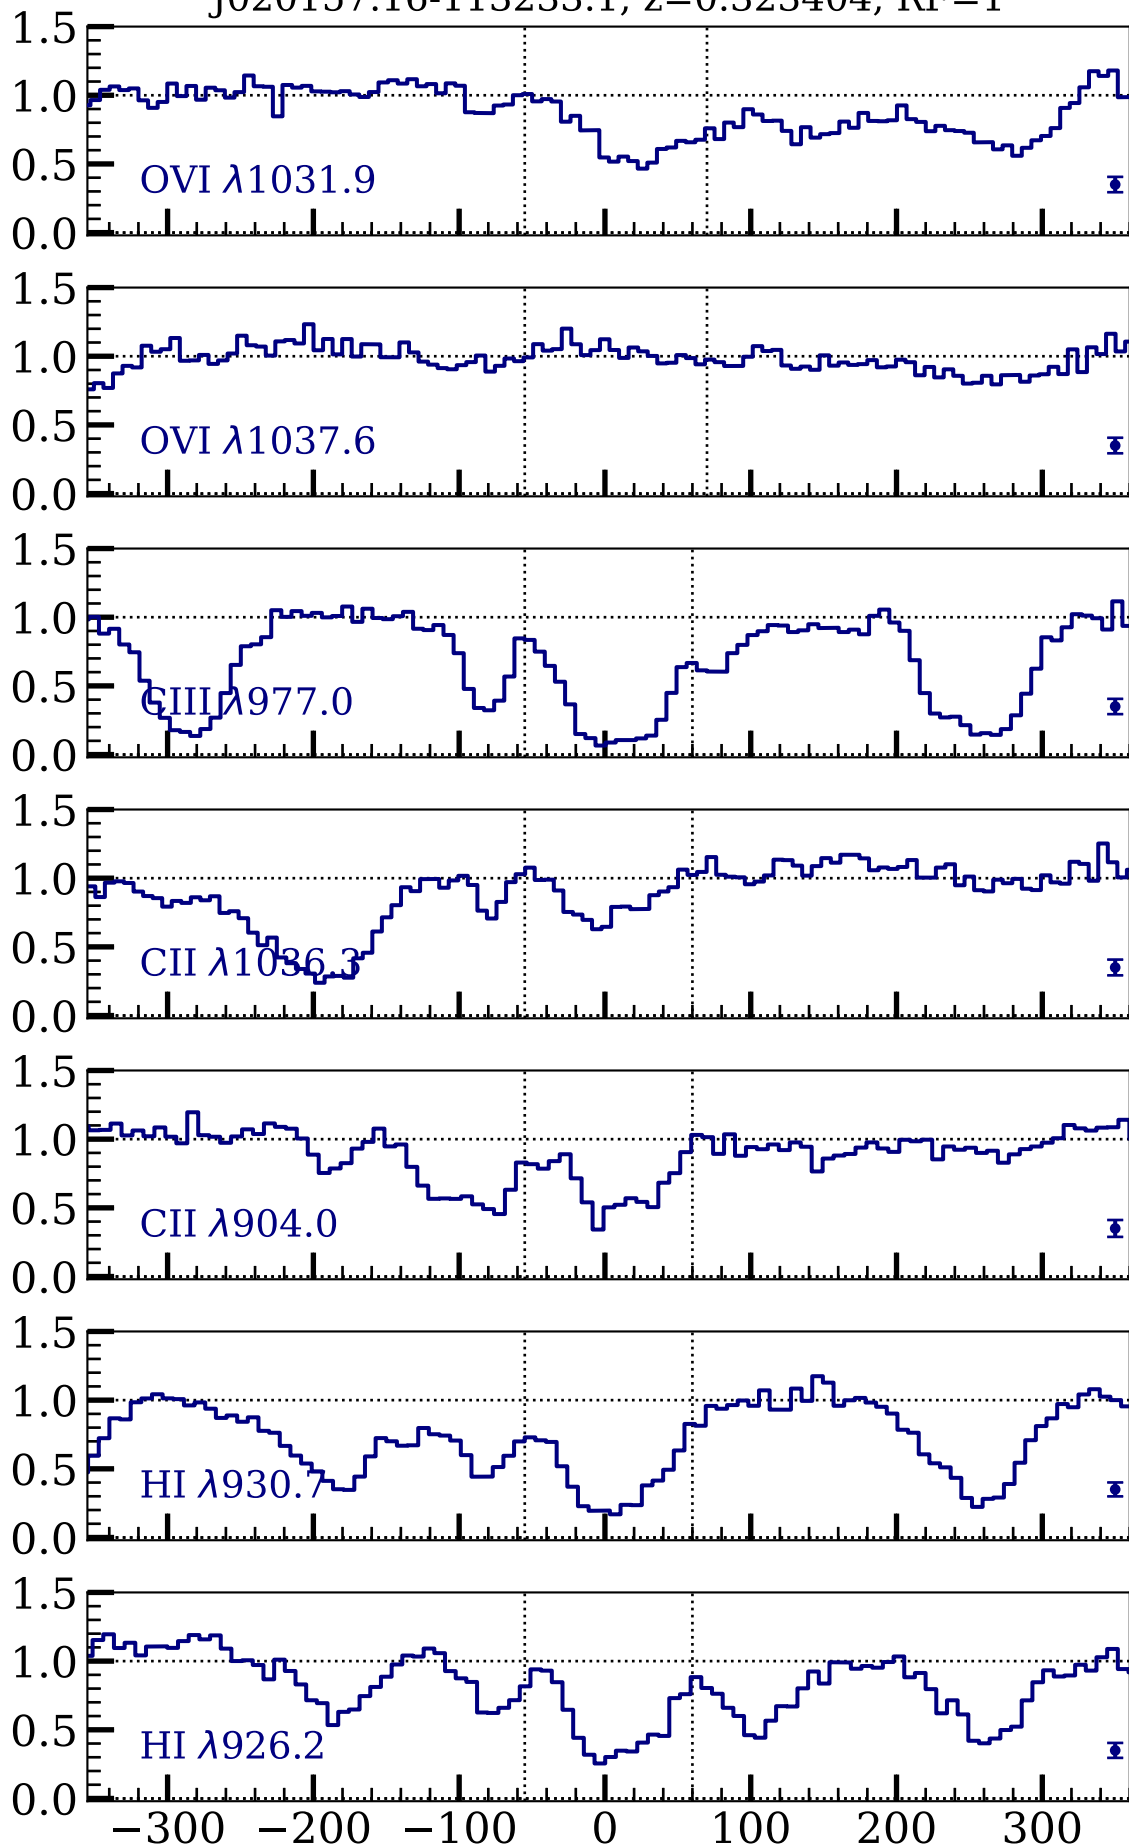Rest-Frame Velocity (km s<sup>-1</sup>)



Normalized Flux

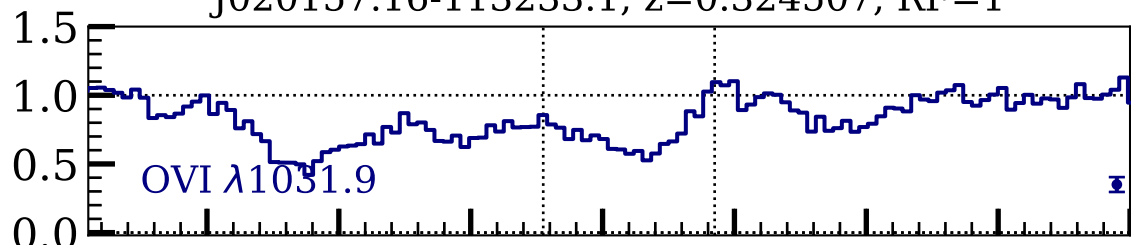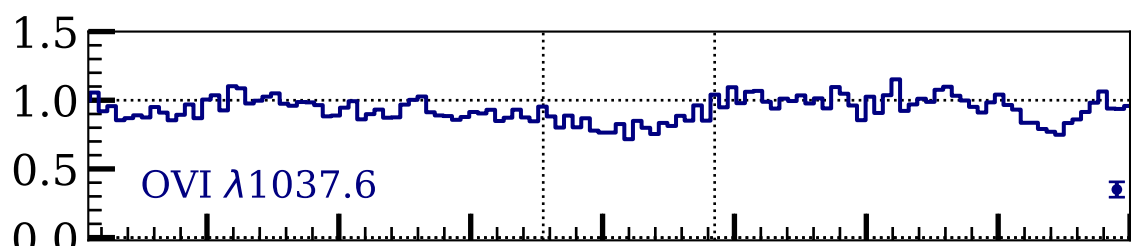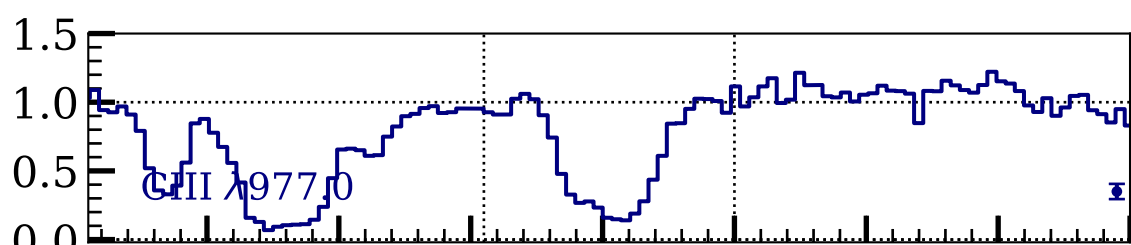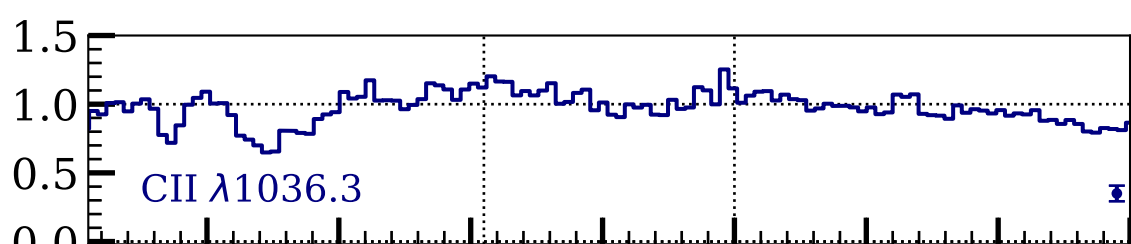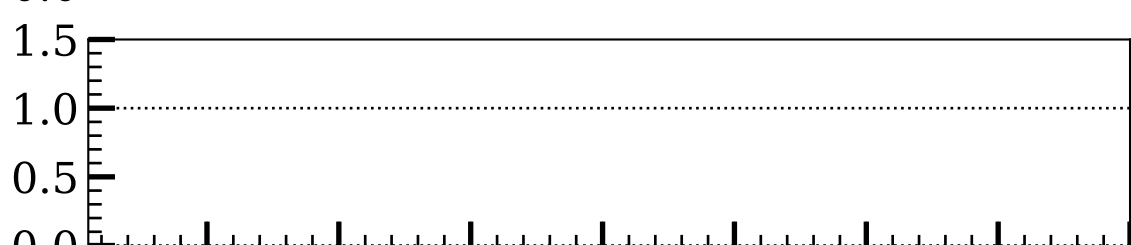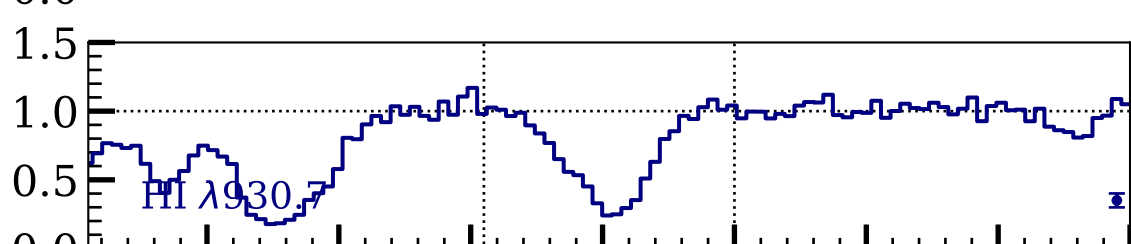Rest-Frame Velocity ( $\text{km s}^{-1}$ )

J023507.38-040205.6,  $z=0.322464$ , RF=1

Normalized Flux

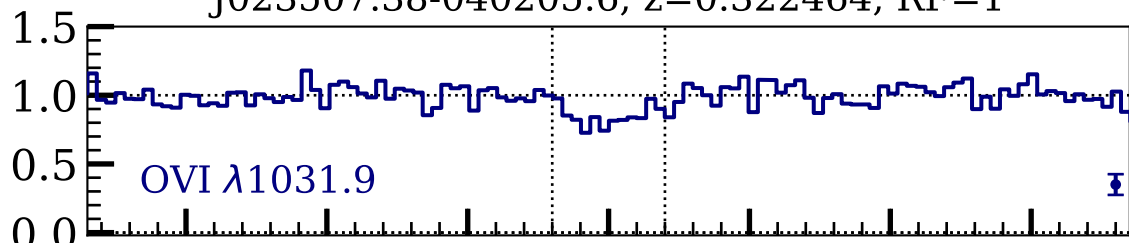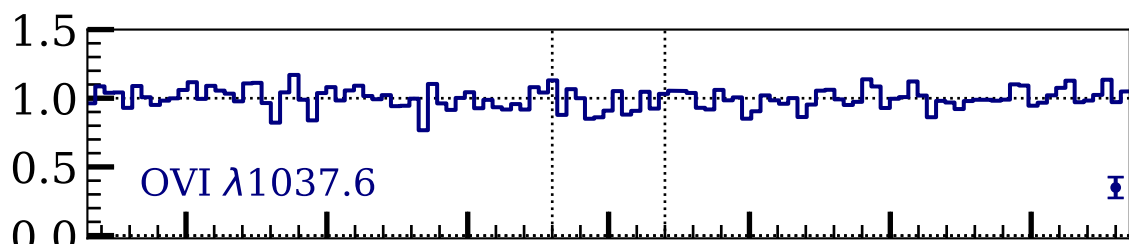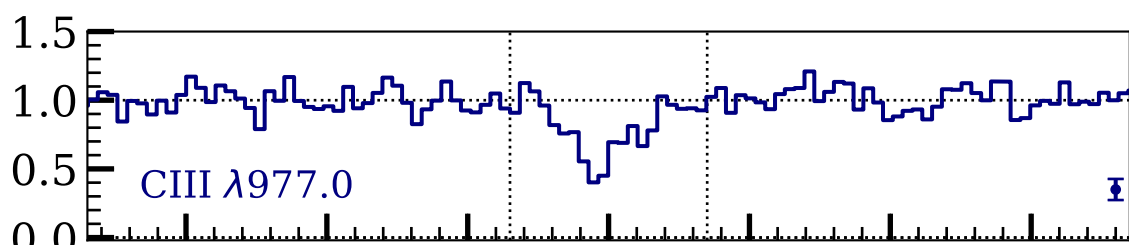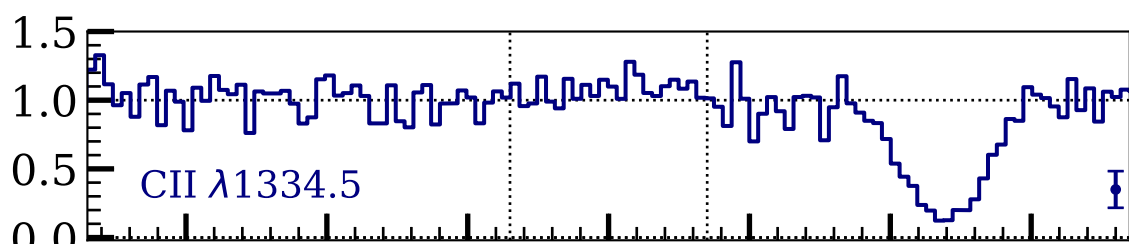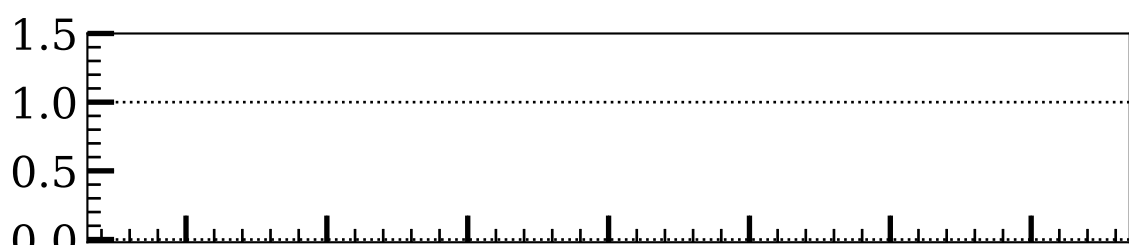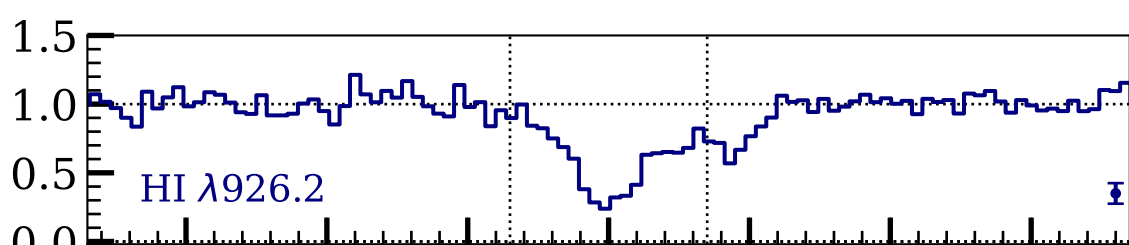

Rest-Frame Velocity ( $\text{km s}^{-1}$ )

J023507.38-040205.6,  $z=0.738890$ , RF=0

Normalized Flux

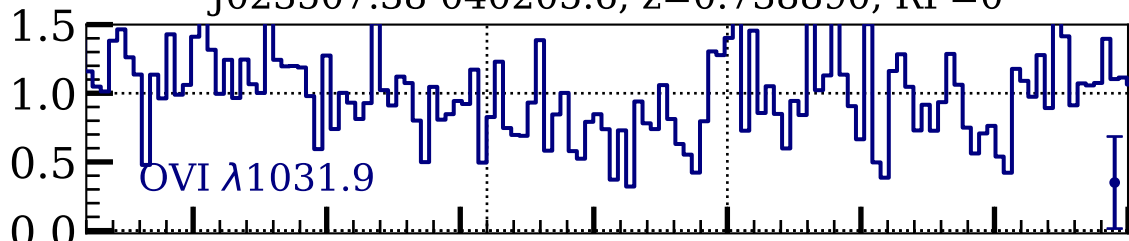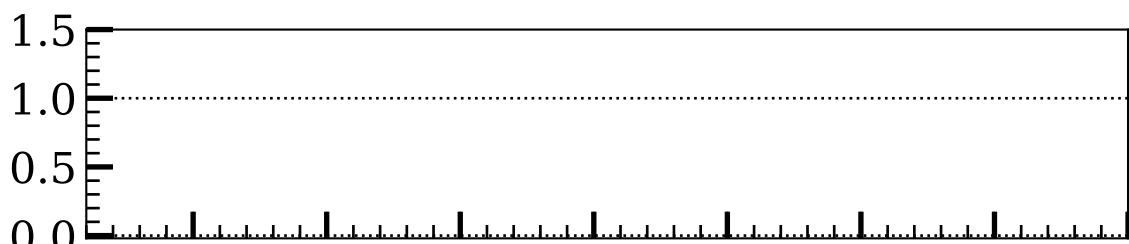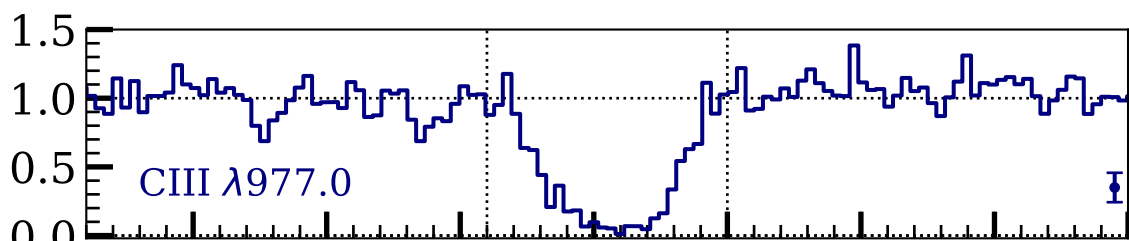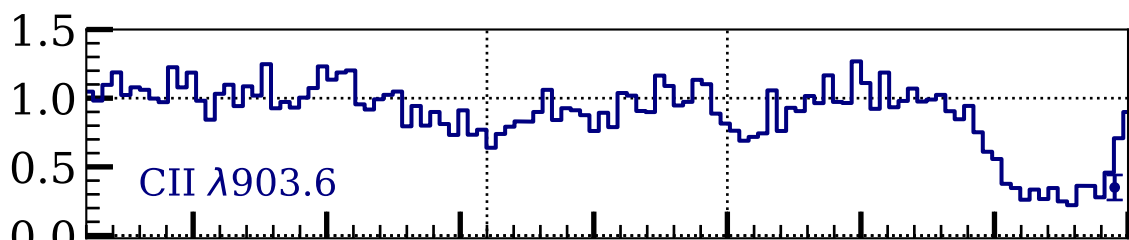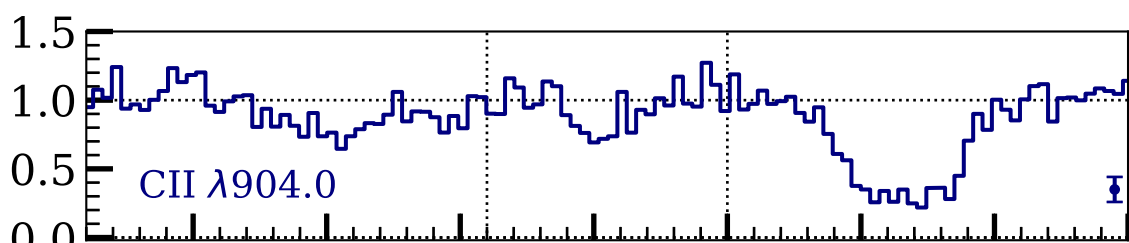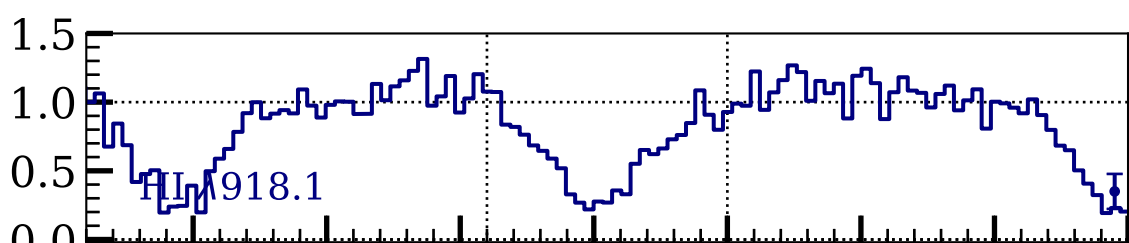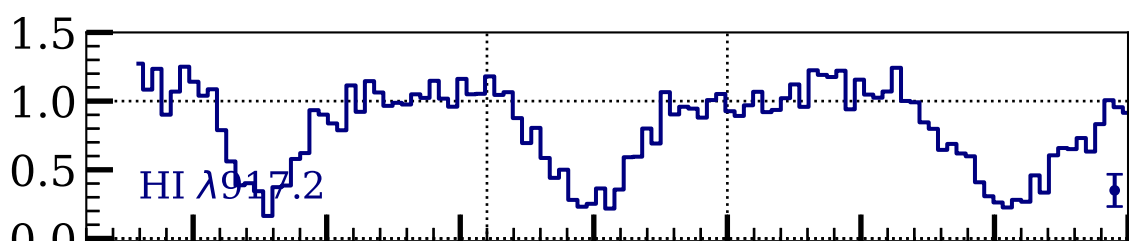

Rest-Frame Velocity ( $\text{km s}^{-1}$ )

J024337.66-303048.0,  $z=0.303706$ , RF=1

Normalized Flux

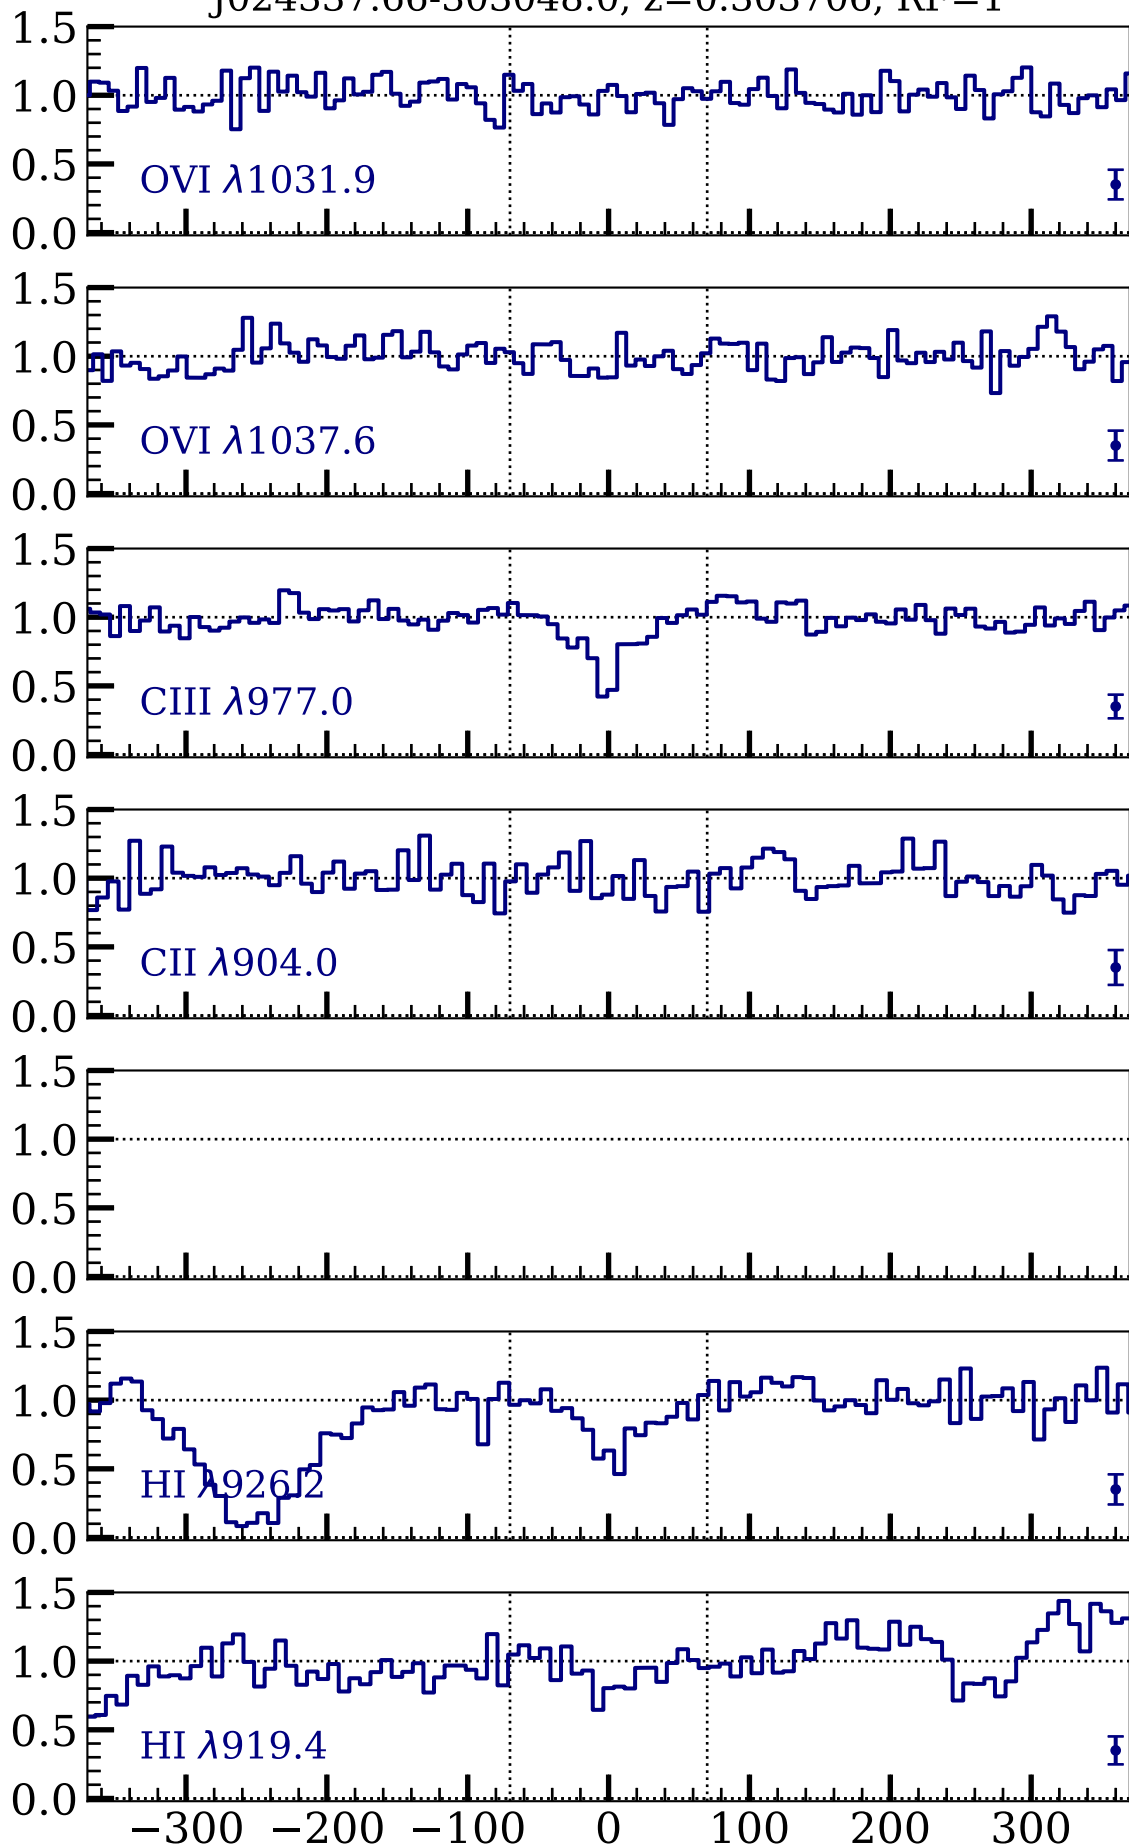

Rest-Frame Velocity (km s<sup>-1</sup>)

J024649.86-300741.3,  $z=0.312304$ , RF=1

Normalized Flux

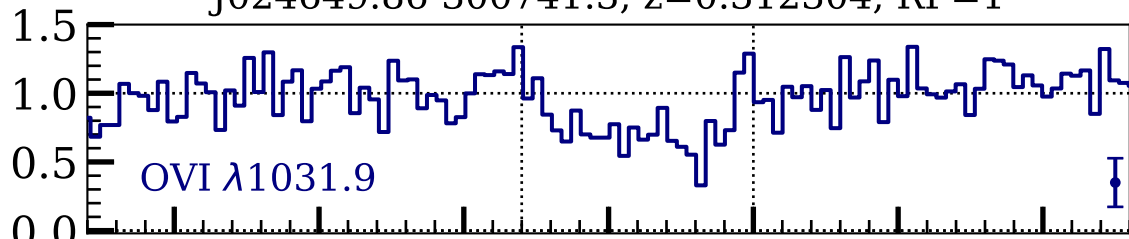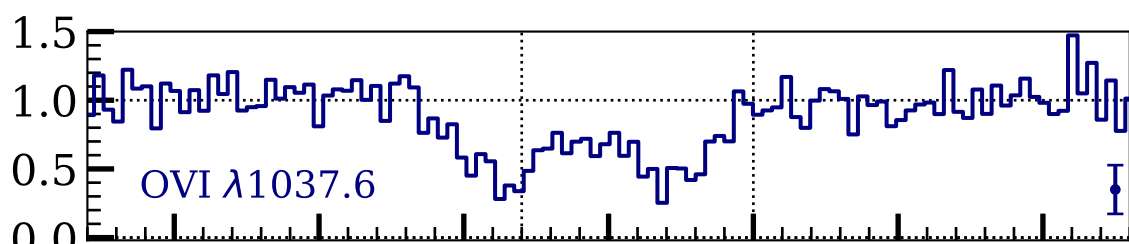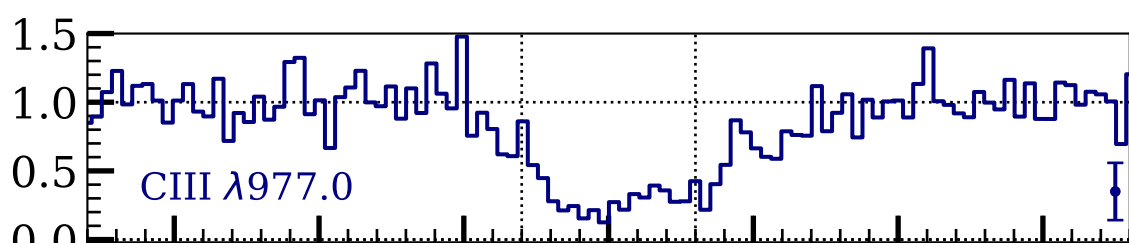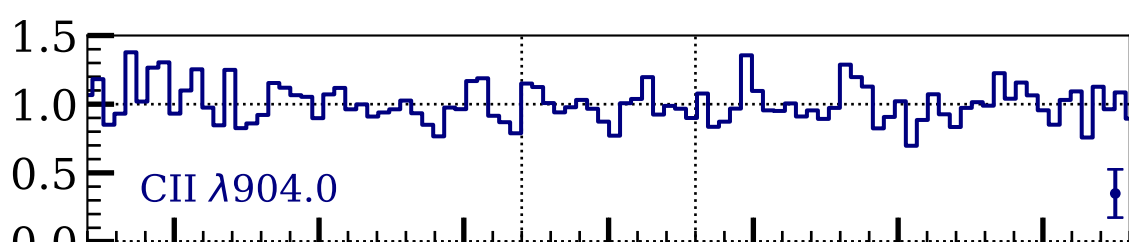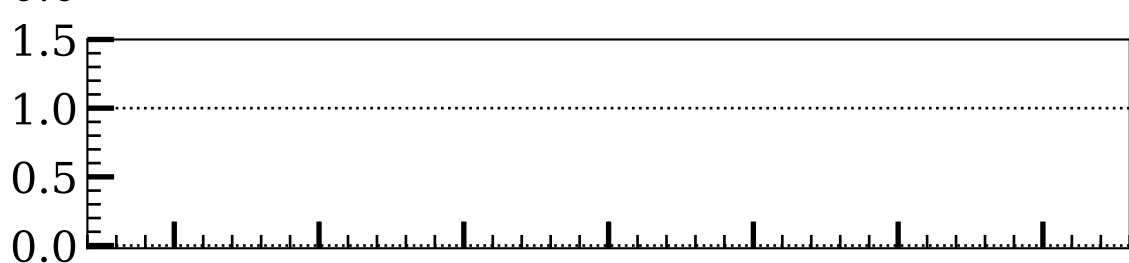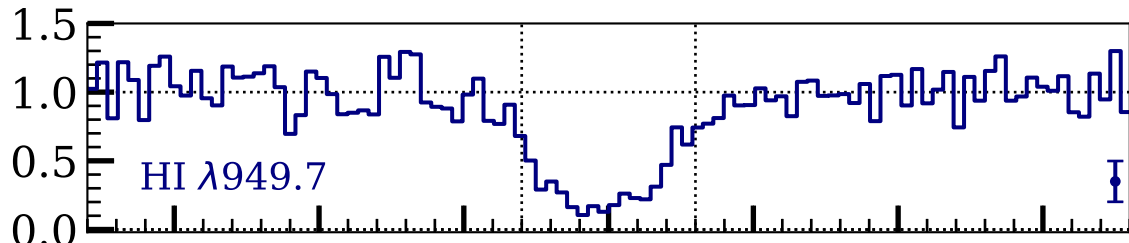

Rest-Frame Velocity ( $\text{km s}^{-1}$ )

J024649.86-300741.3,  $z=0.335895$ , RF=1

Normalized Flux

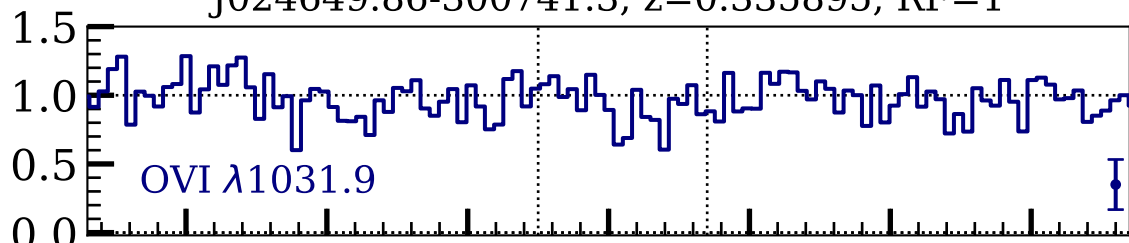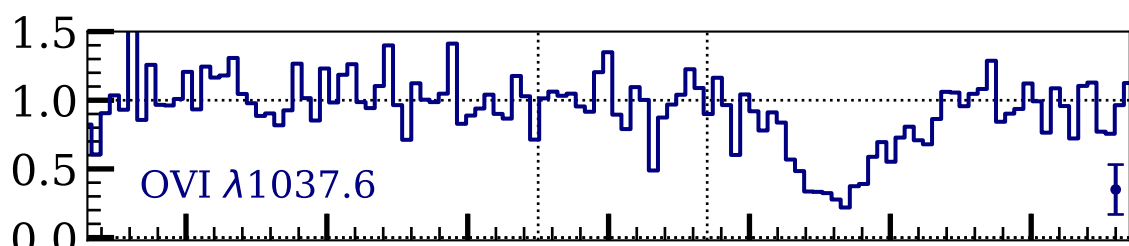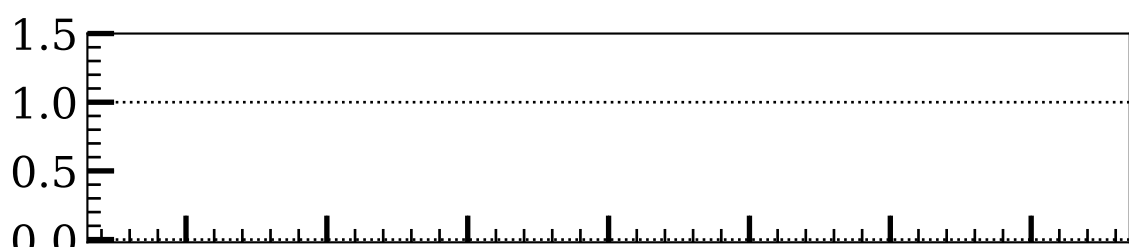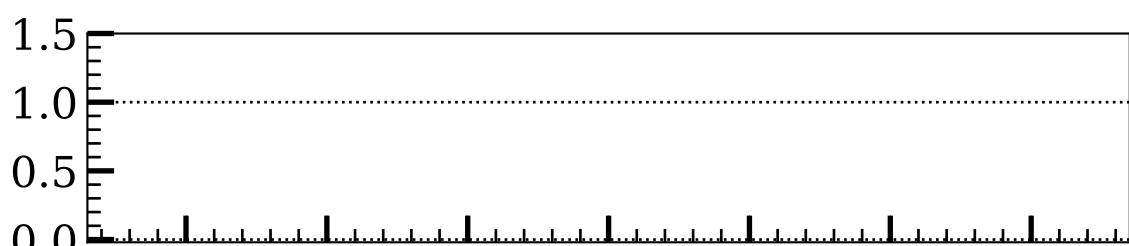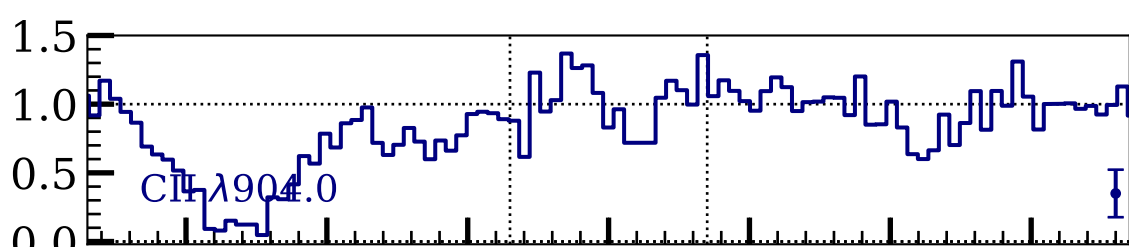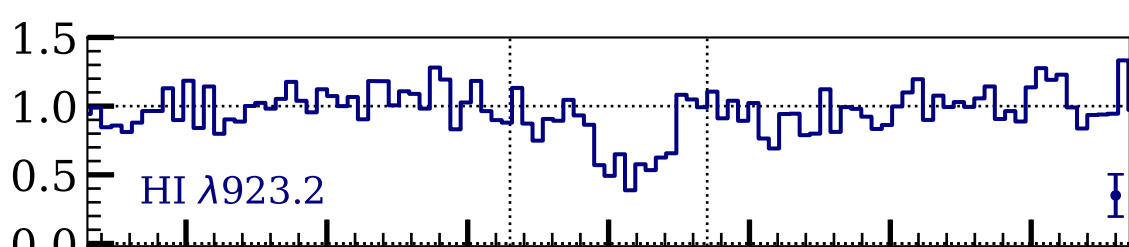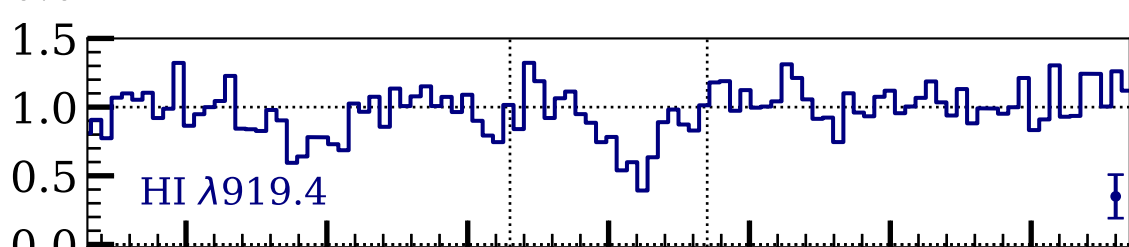

Rest-Frame Velocity ( $\text{km s}^{-1}$ )

J035128.56-142908.0,  $z=0.328476$ , RF=1

Normalized Flux

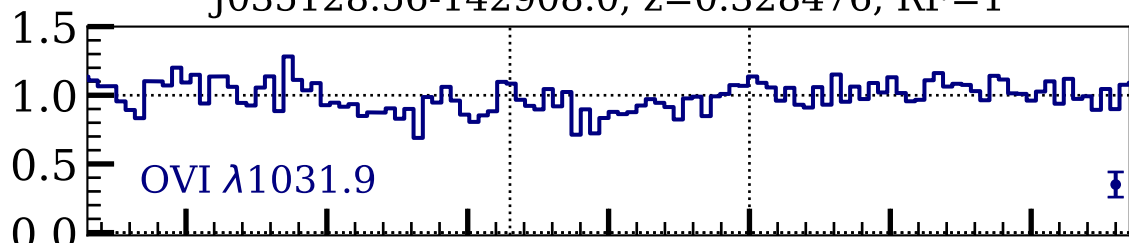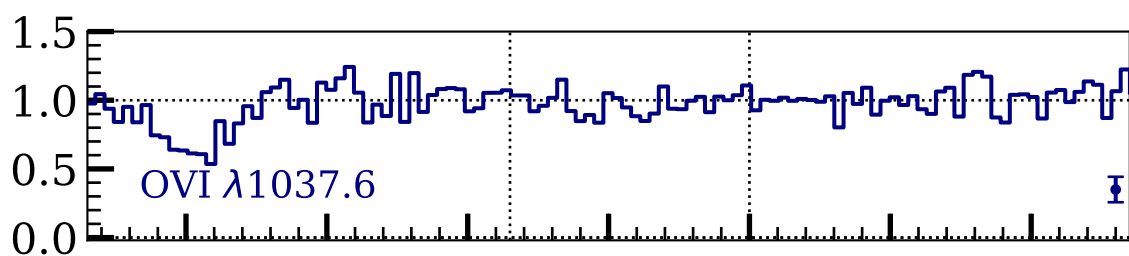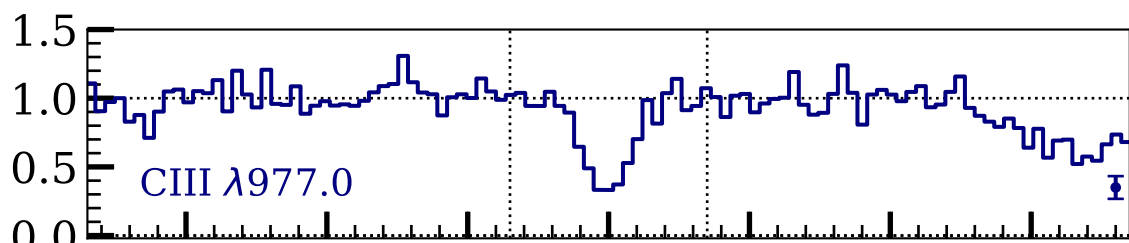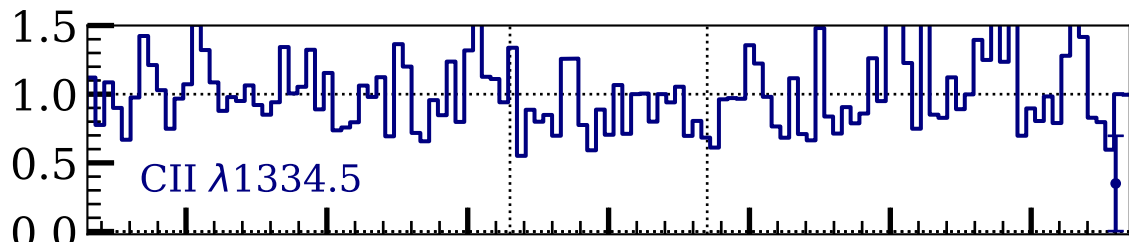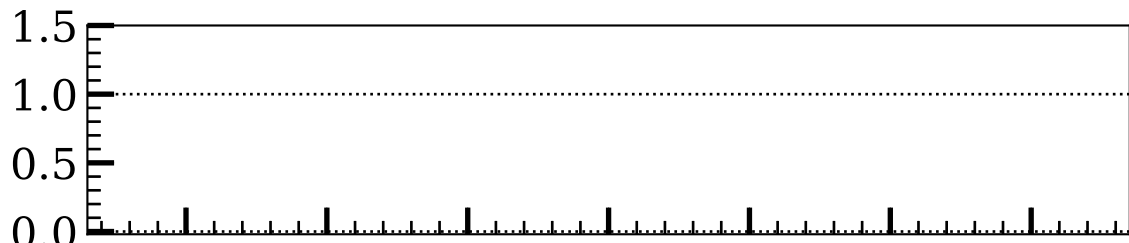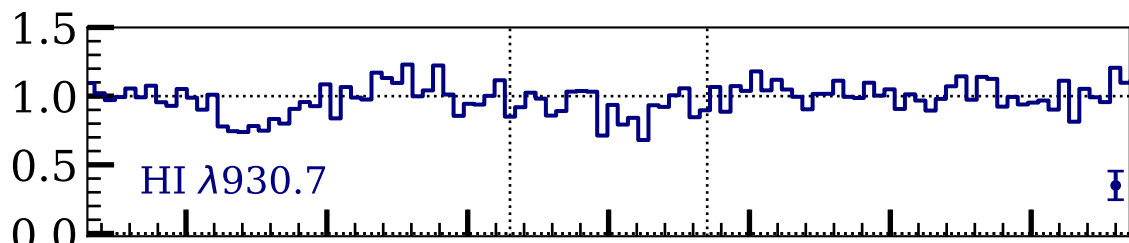

Rest-Frame Velocity ( $\text{km s}^{-1}$ )

J035128.56-142908.0,  $z=0.356924$ , RF=1

Normalized Flux

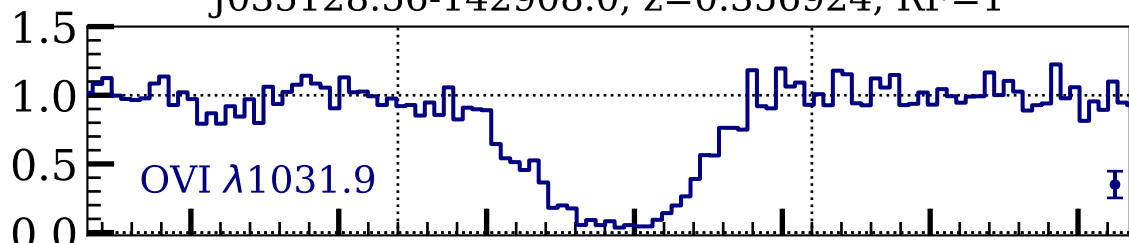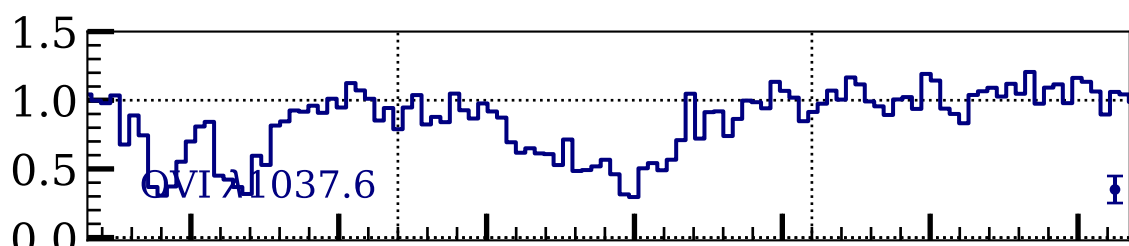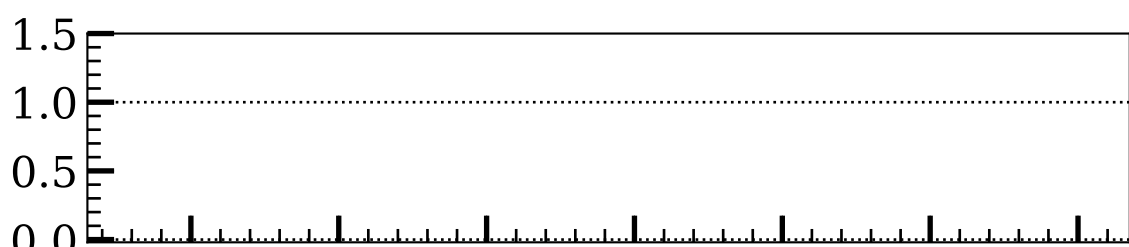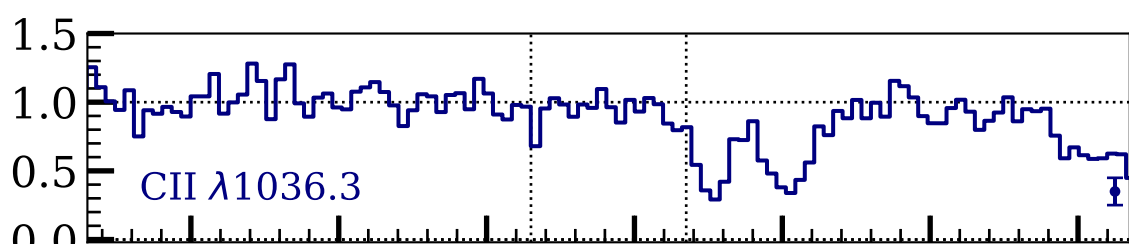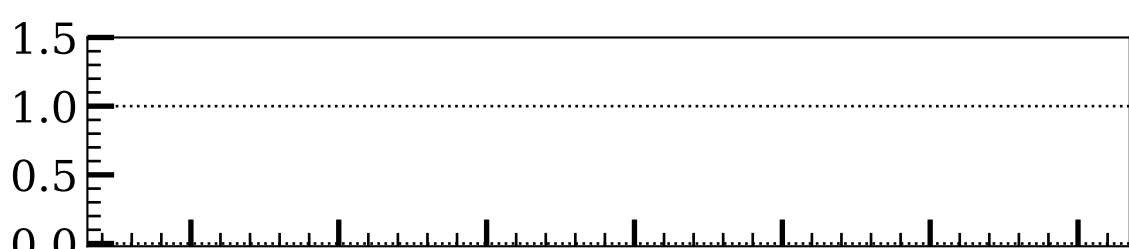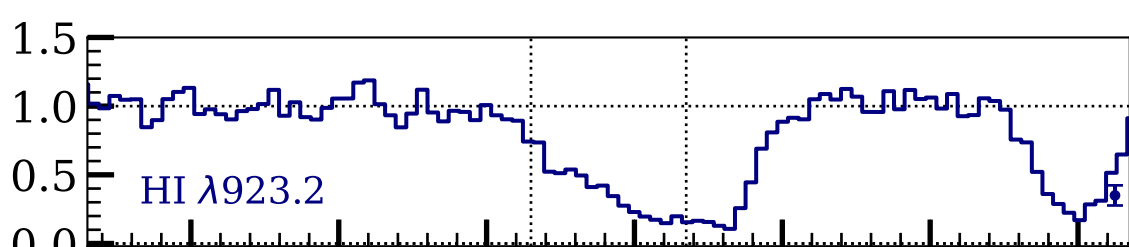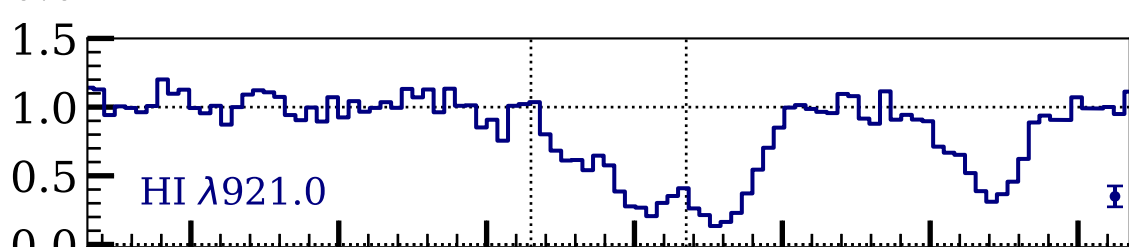

Rest-Frame Velocity ( $\text{km s}^{-1}$ )



Normalized Flux

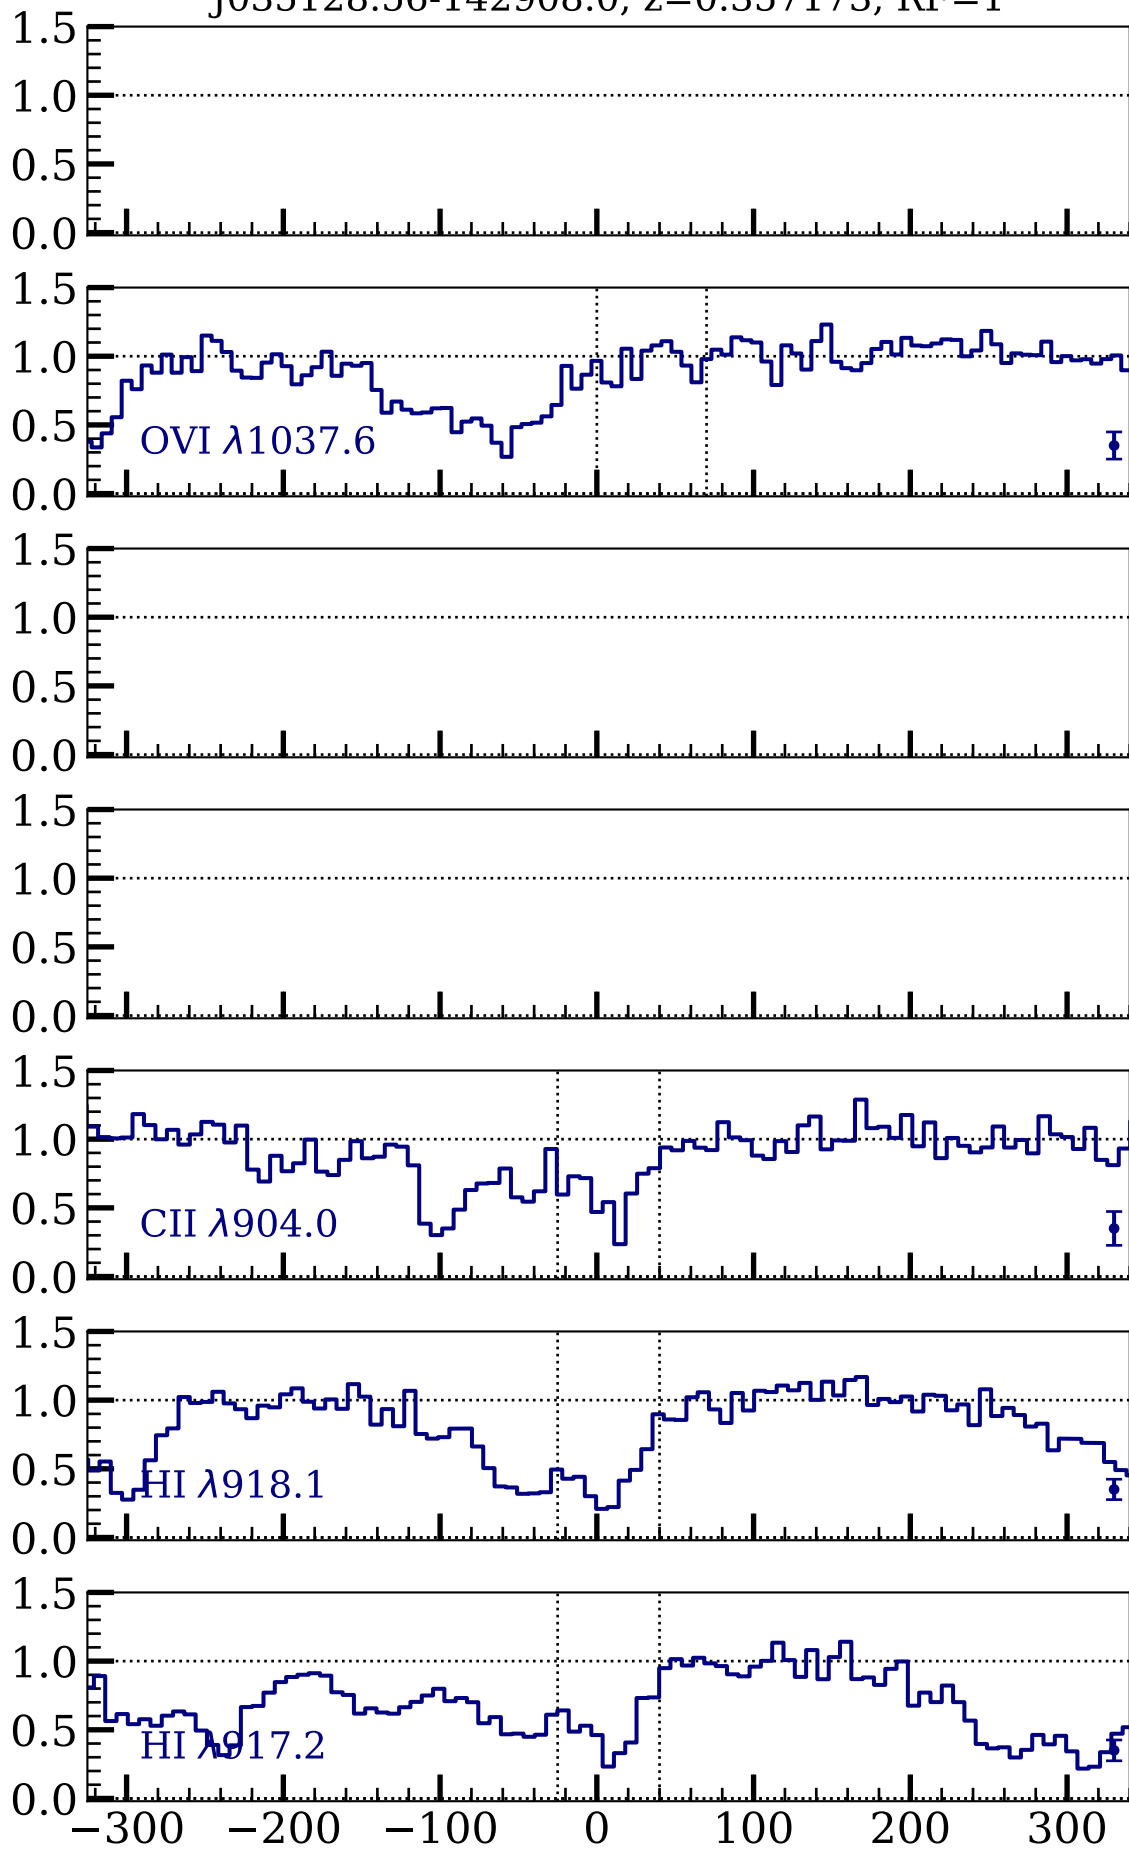Rest-Frame Velocity (km s<sup>-1</sup>)

J035128.56-142908.0,  $z=0.439804$ , RF=1

Normalized Flux

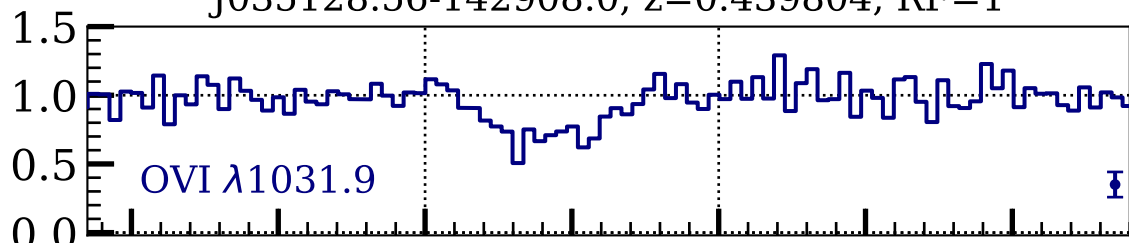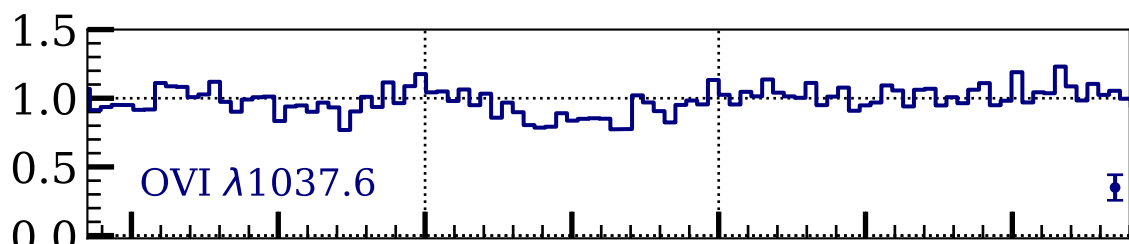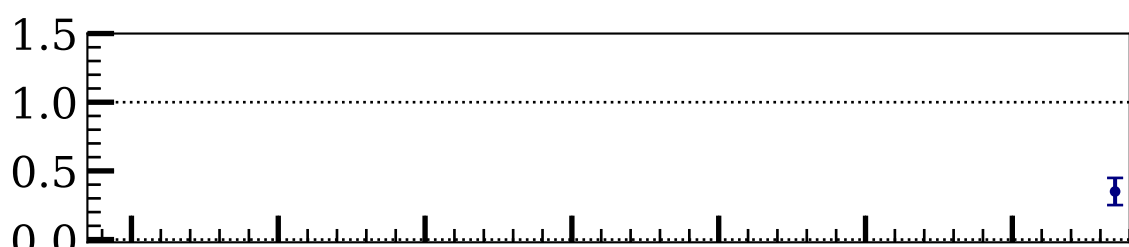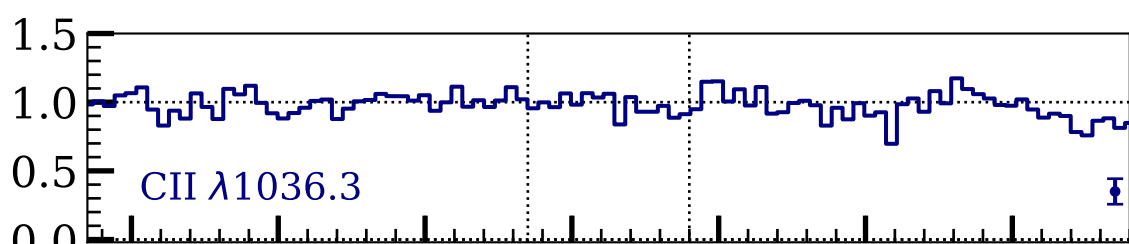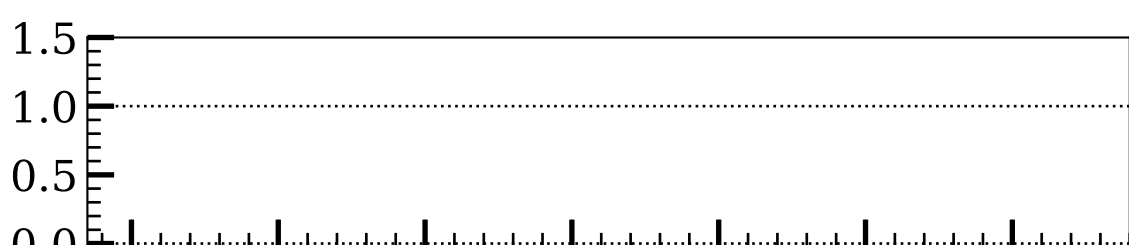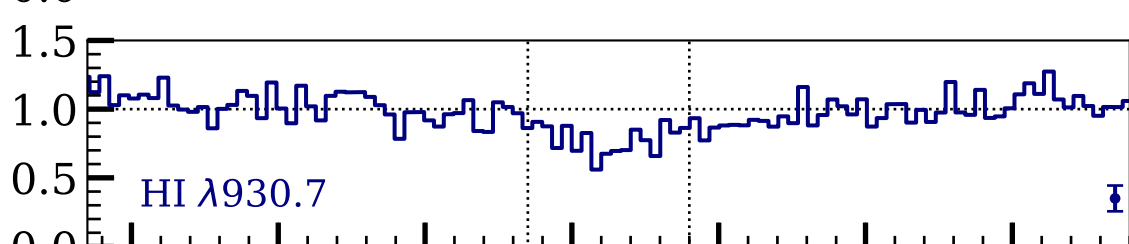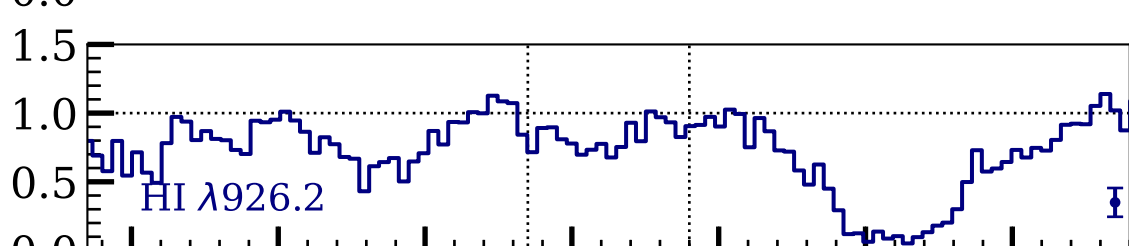

Rest-Frame Velocity ( $\text{km s}^{-1}$ )

J040148.98-054056.5,  $z=0.219453$ , RF=1

Normalized Flux

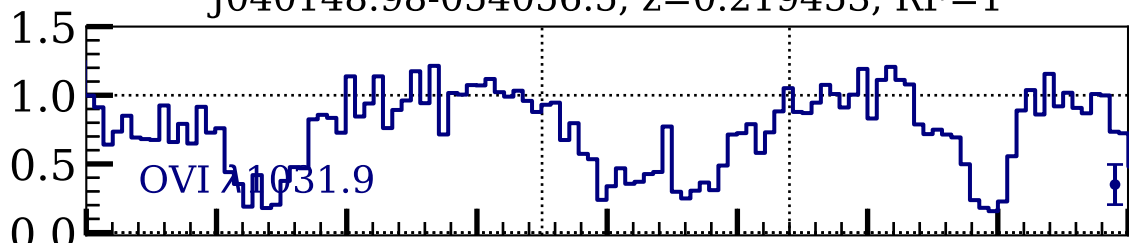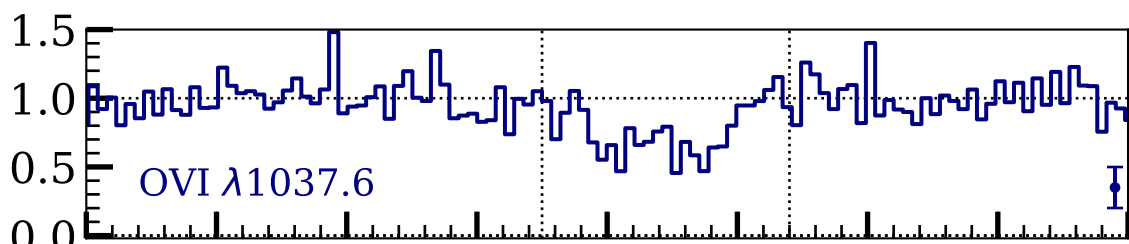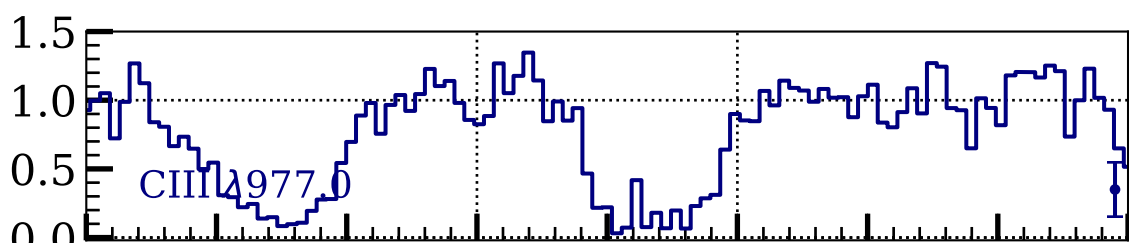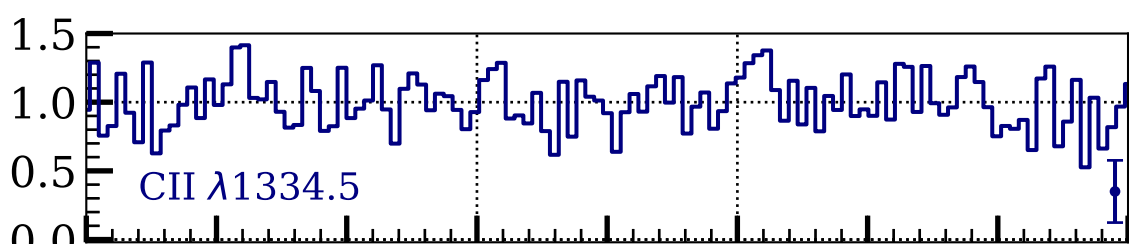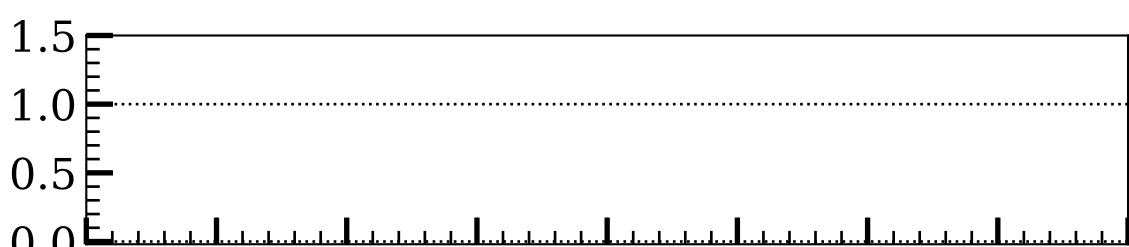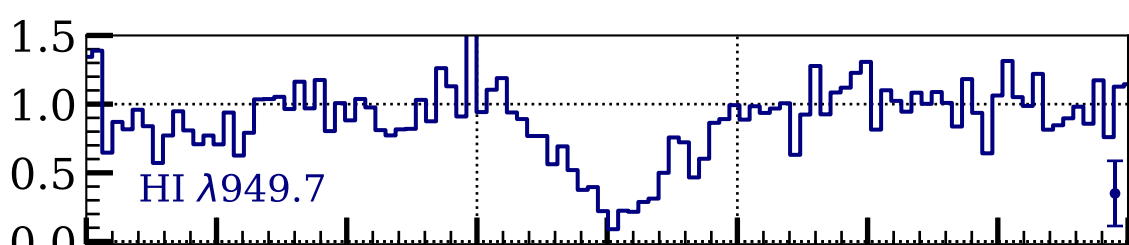

Rest-Frame Velocity ( $\text{km s}^{-1}$ )

J040148.98-054056.5,  $z=0.323769$ , RF=1

Normalized Flux

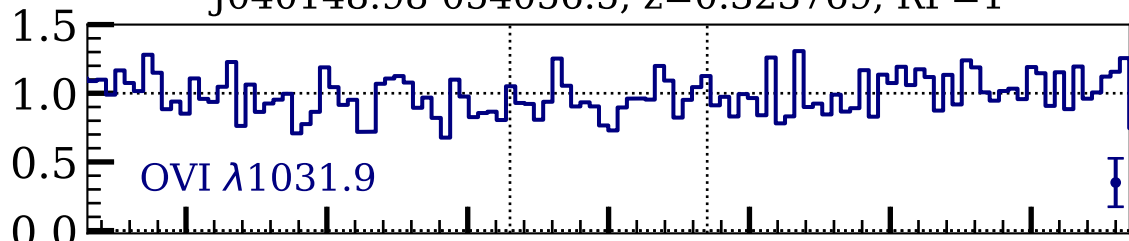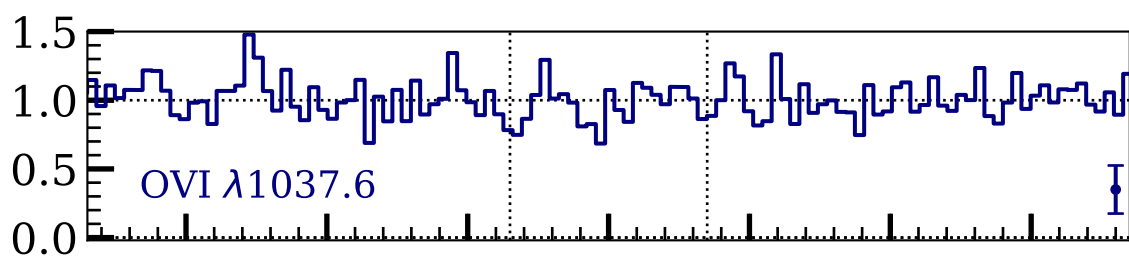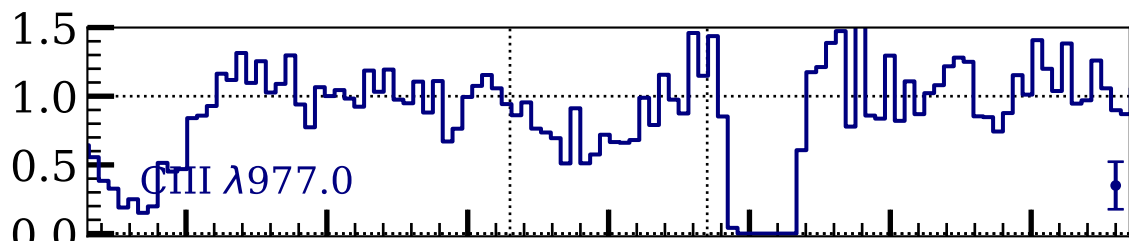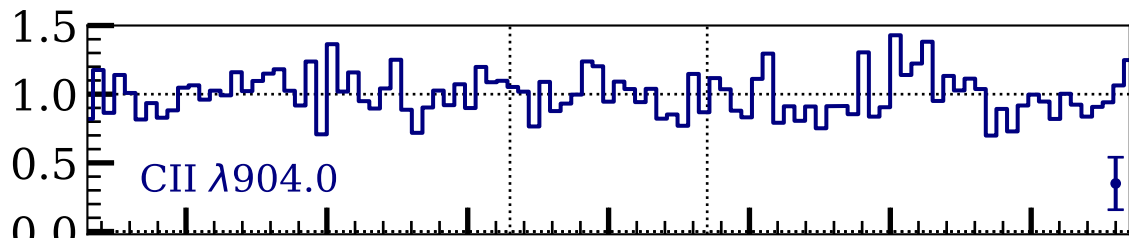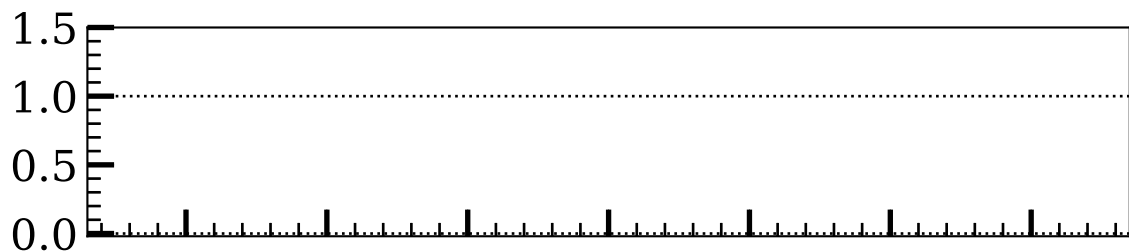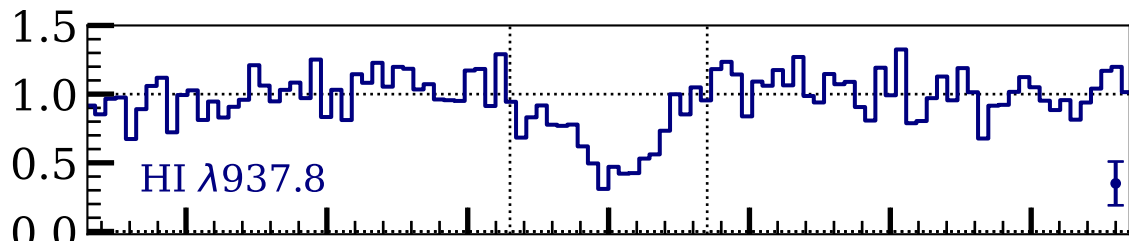

Rest-Frame Velocity ( $\text{km s}^{-1}$ )

J040748.42-121136.3,  $z=0.167160$ , RF=1

Normalized Flux

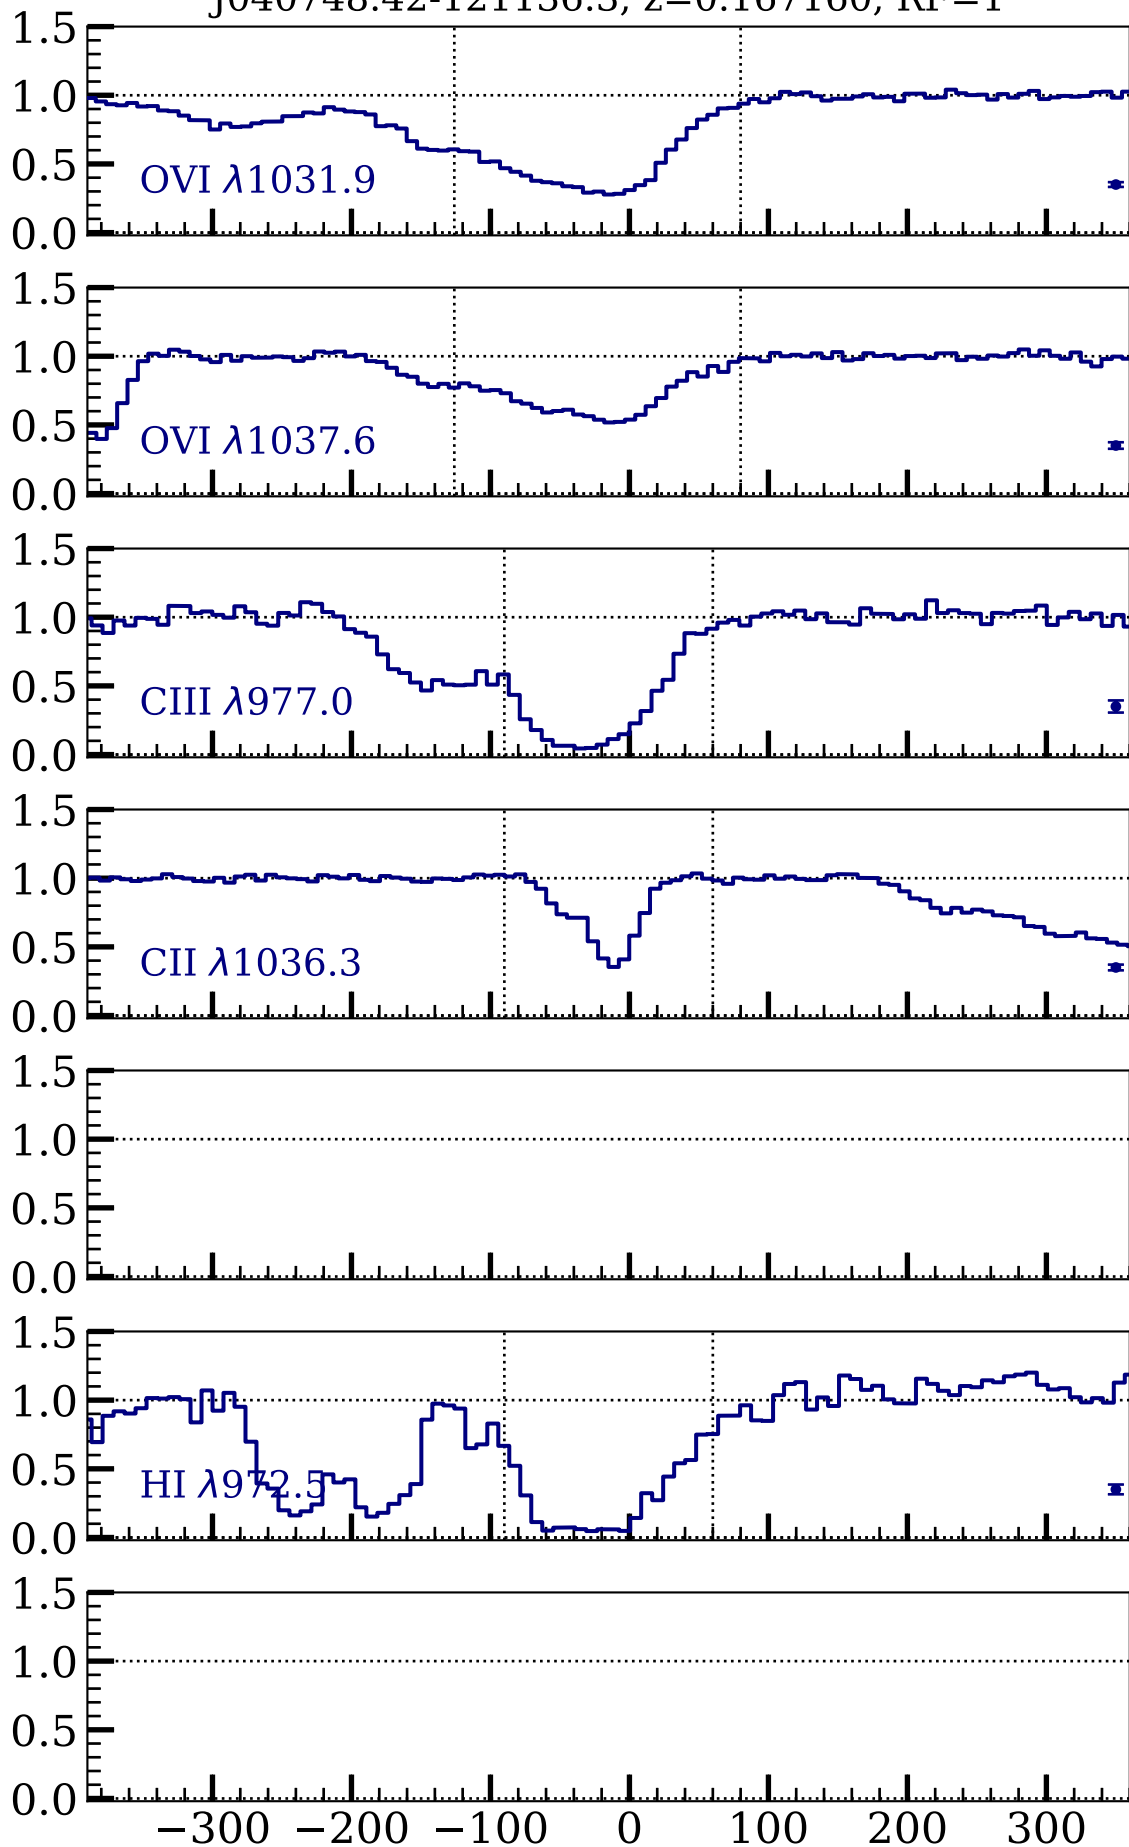

Rest-Frame Velocity (km s<sup>-1</sup>)

J040748.42-121136.3,  $z=0.360742$ , RF=1

Normalized Flux

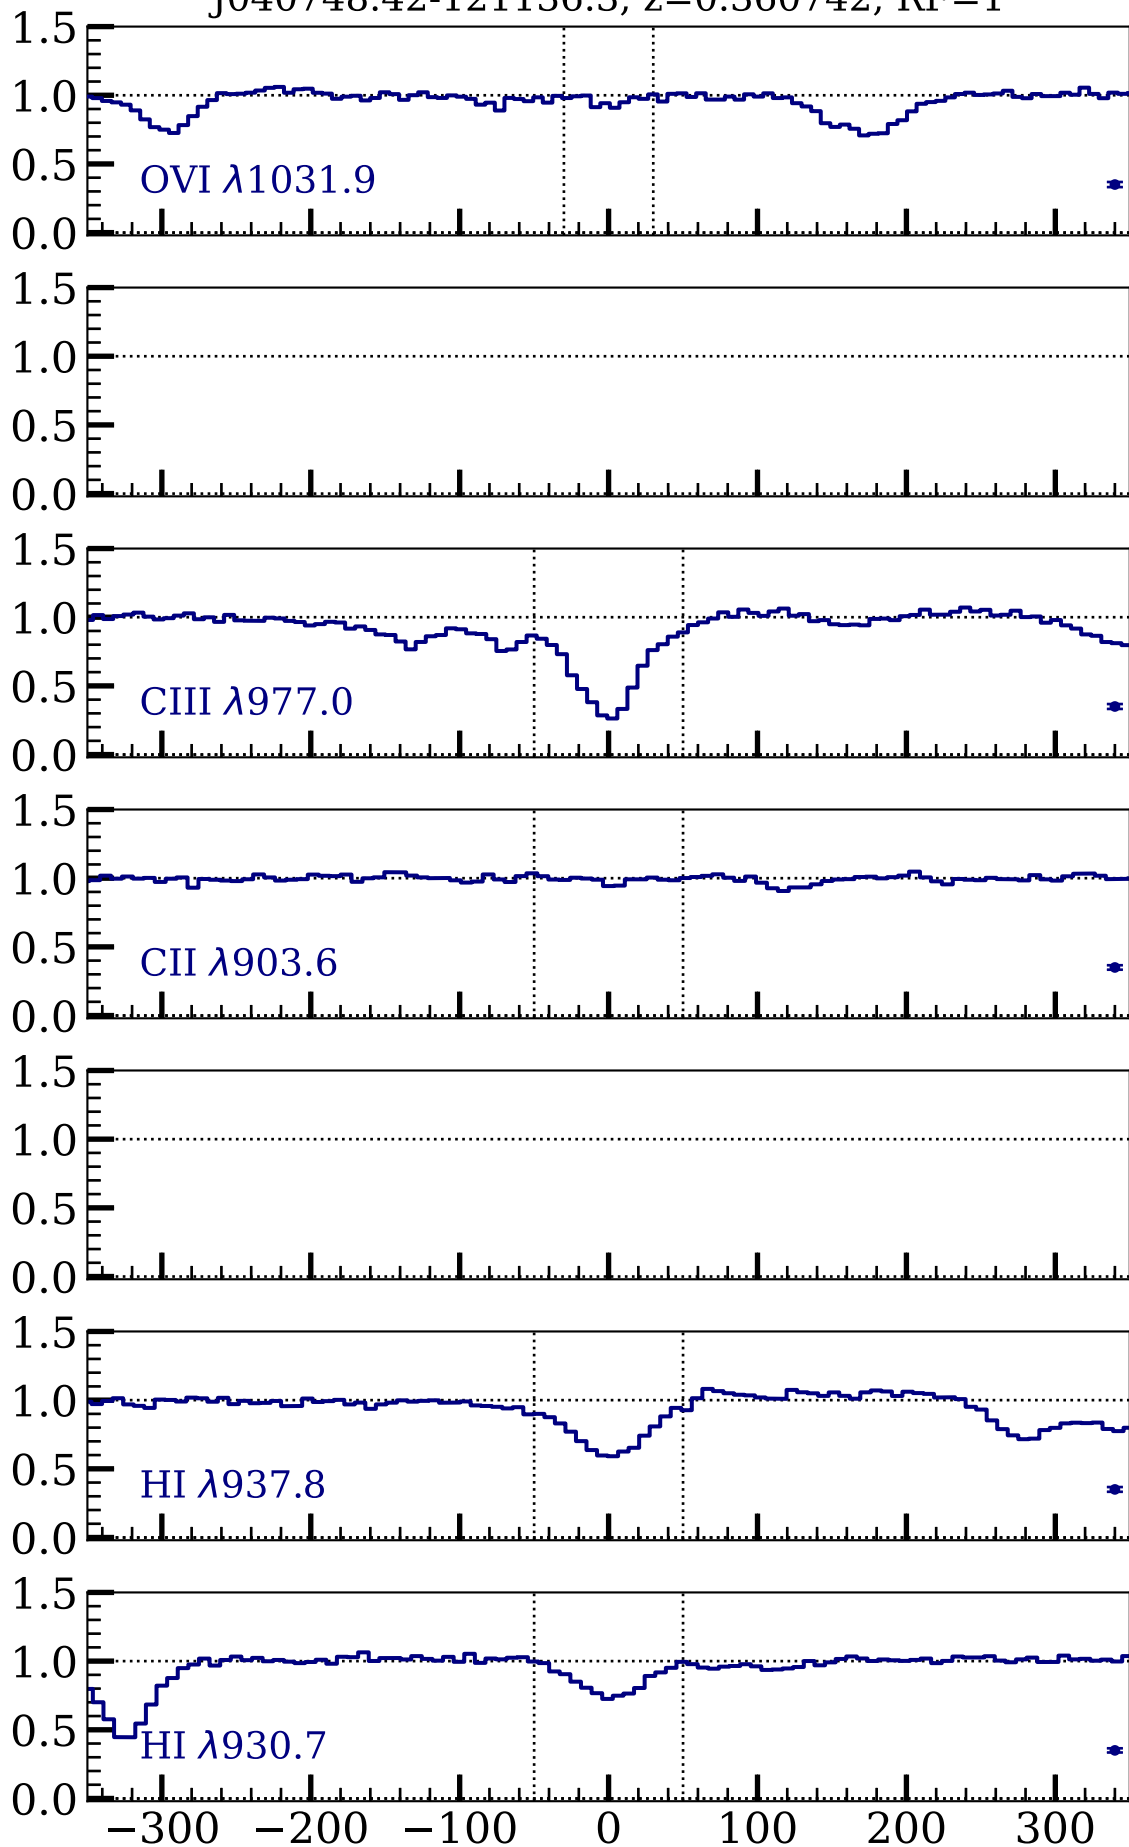

Rest-Frame Velocity (km s<sup>-1</sup>)

J044011.90-524818.0,  $z=0.327932$ , RF=1

Normalized Flux

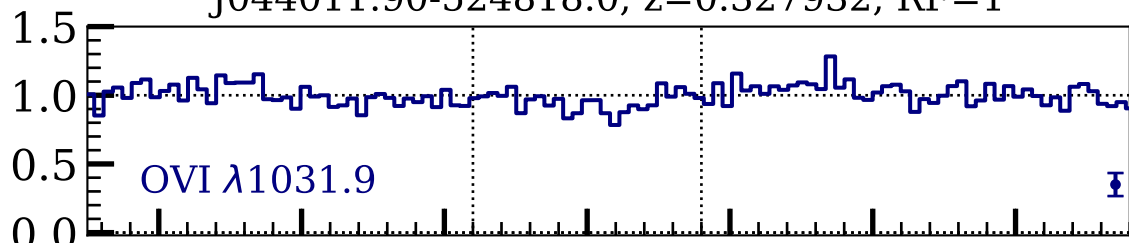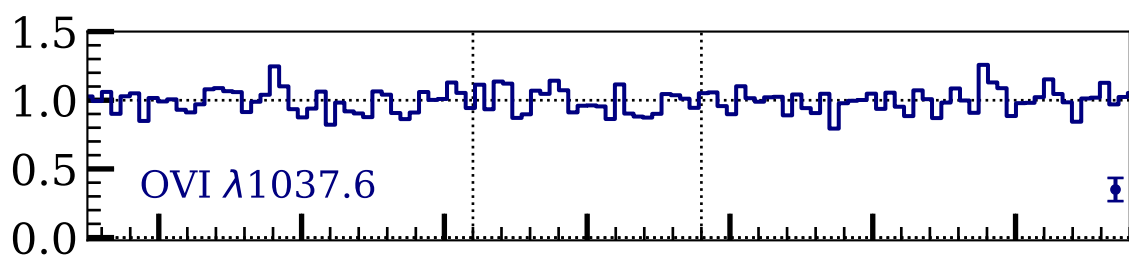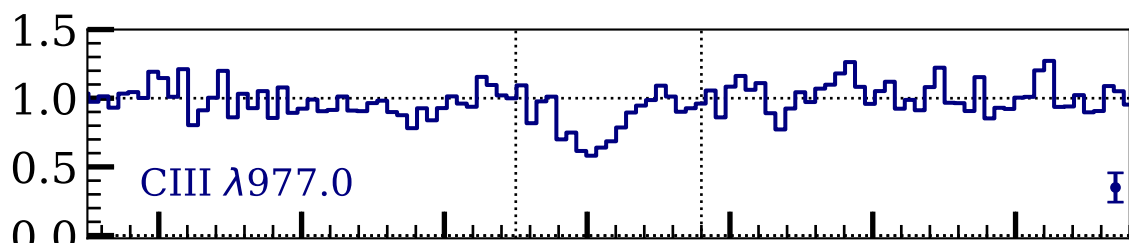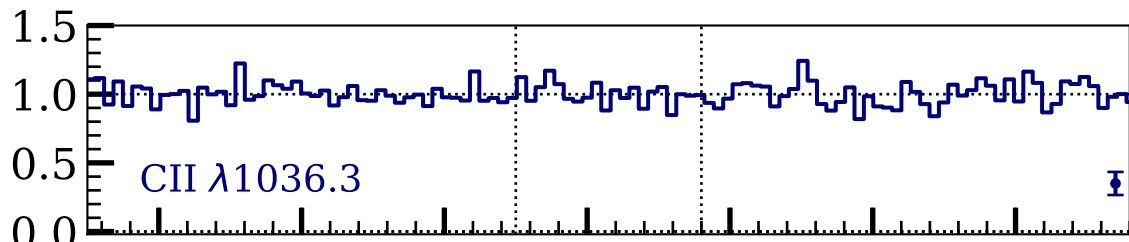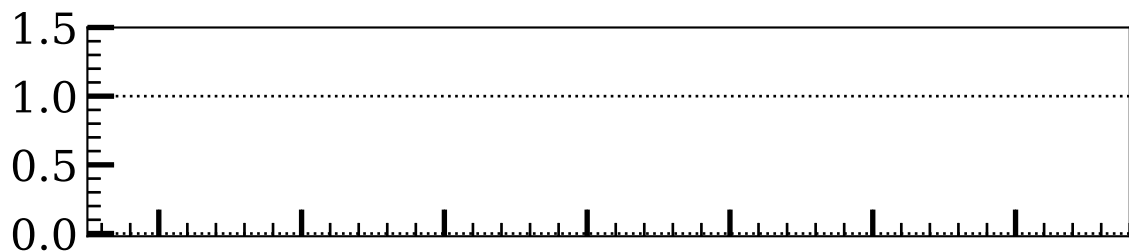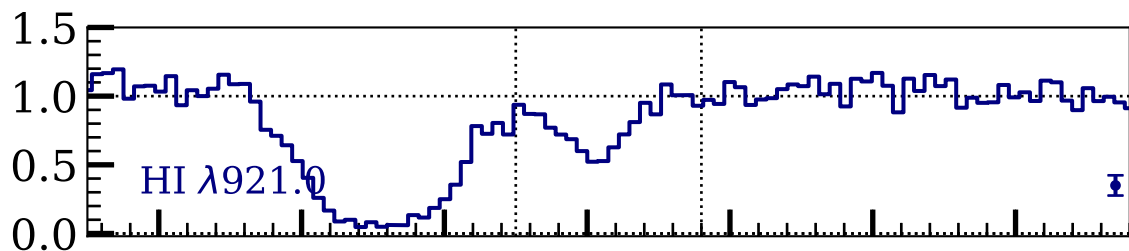

Rest-Frame Velocity ( $\text{km s}^{-1}$ )

J044011.90-524818.0,  $z=0.614962$ , RF=1

Normalized Flux

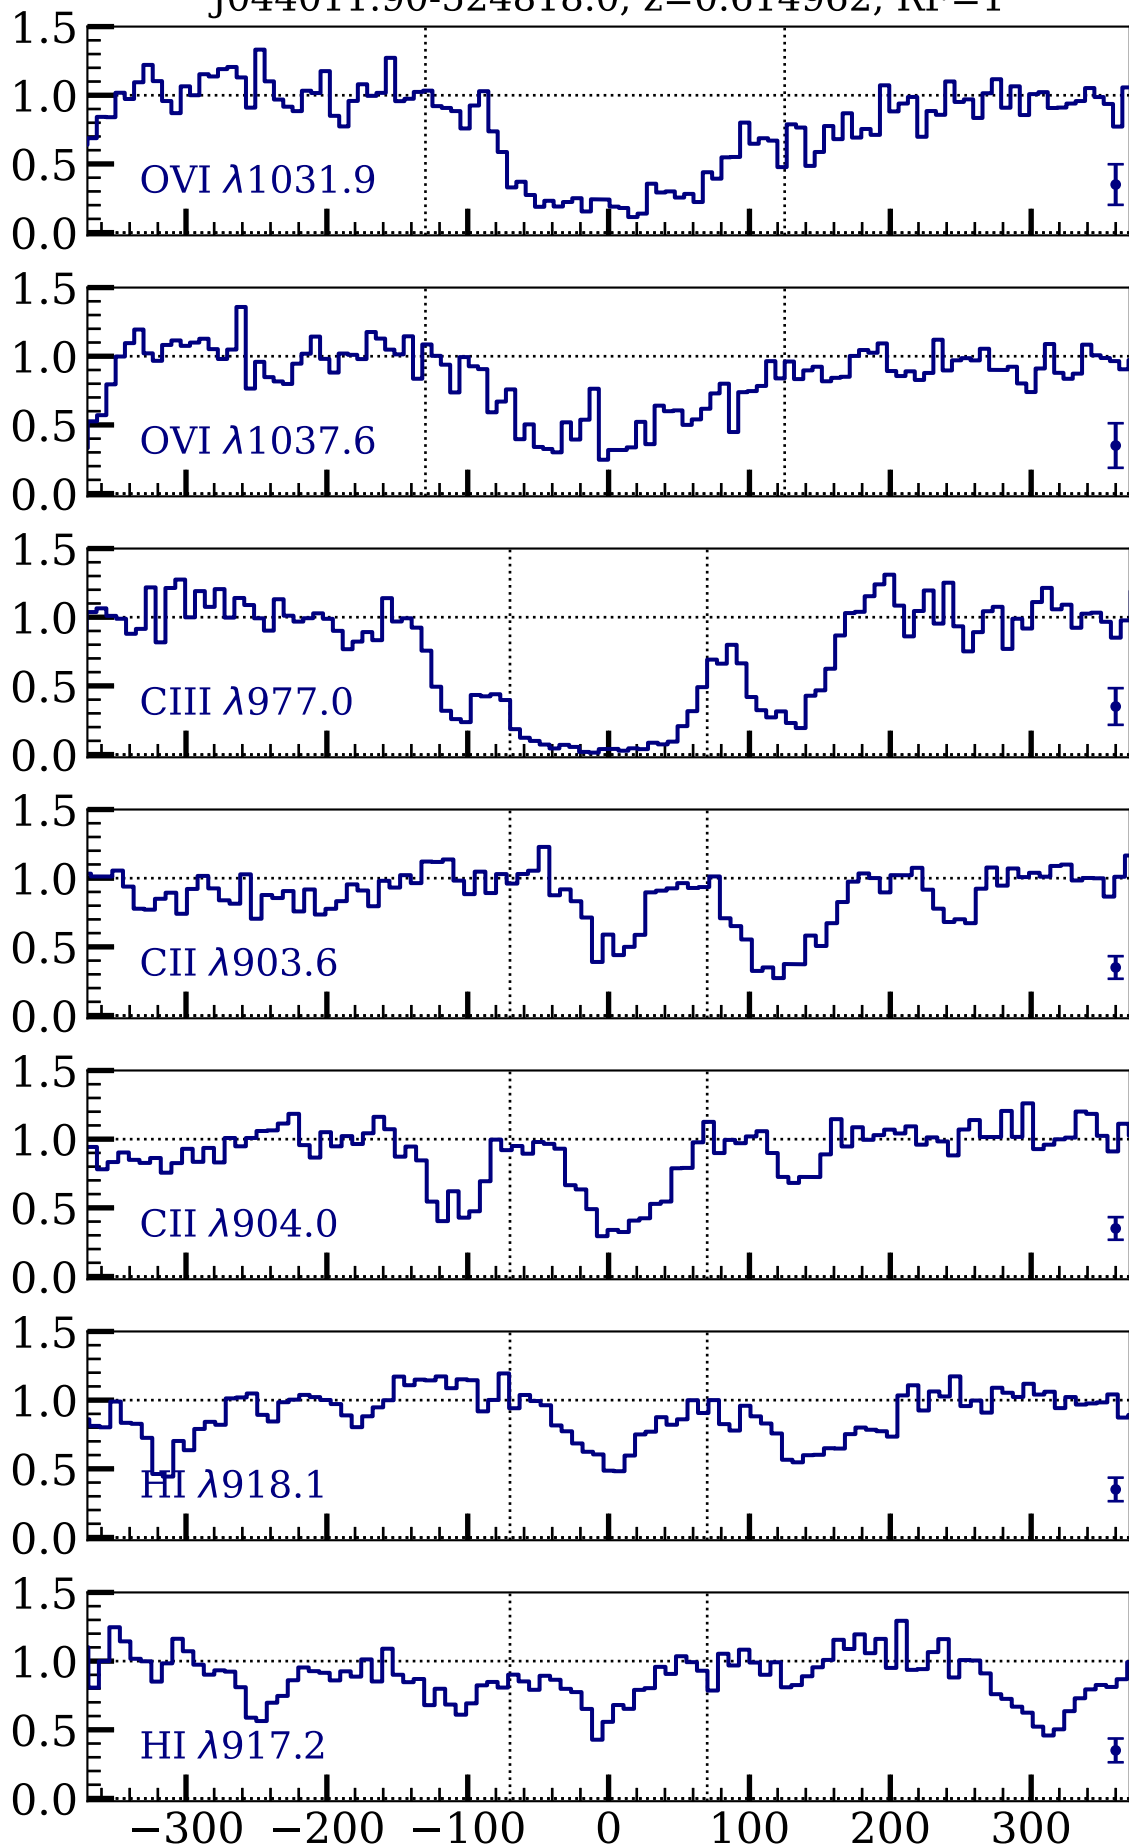

Rest-Frame Velocity (km s<sup>-1</sup>)



J044011.90-524818.0,  $z=0.615662$ , RF=1

Normalized Flux

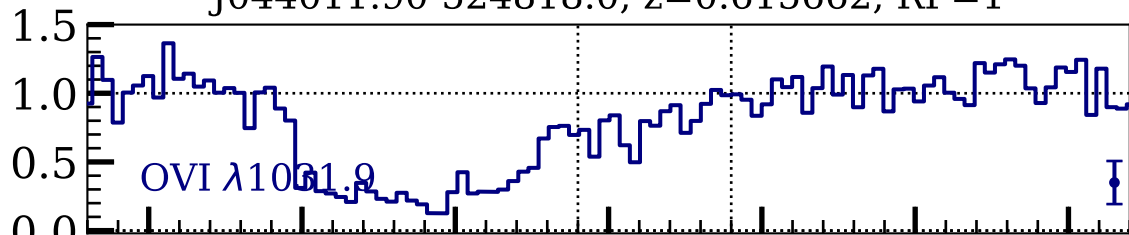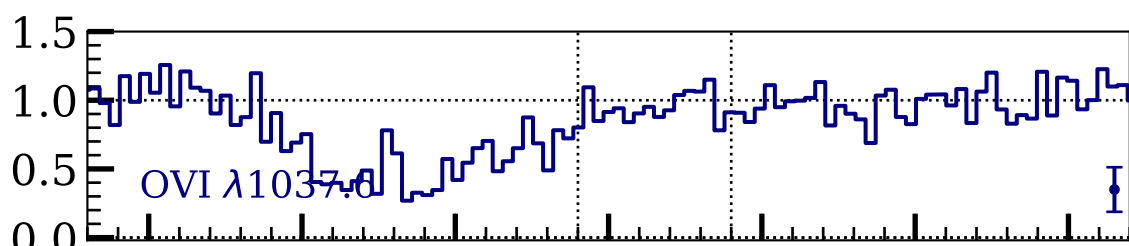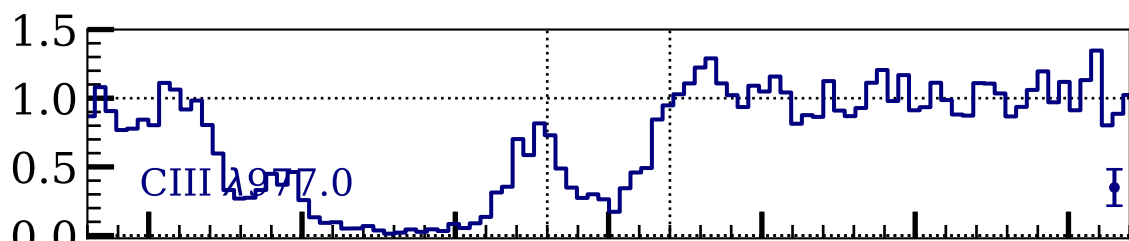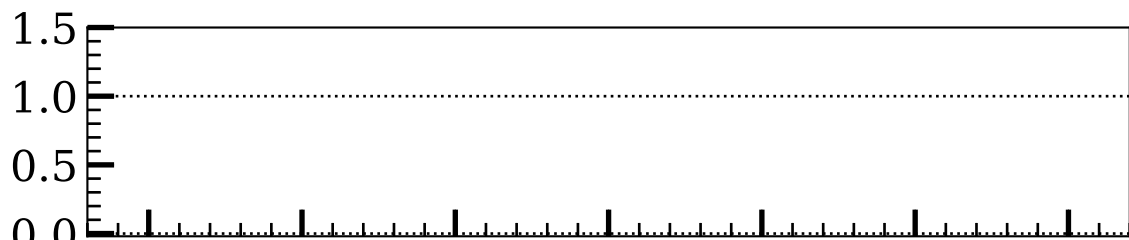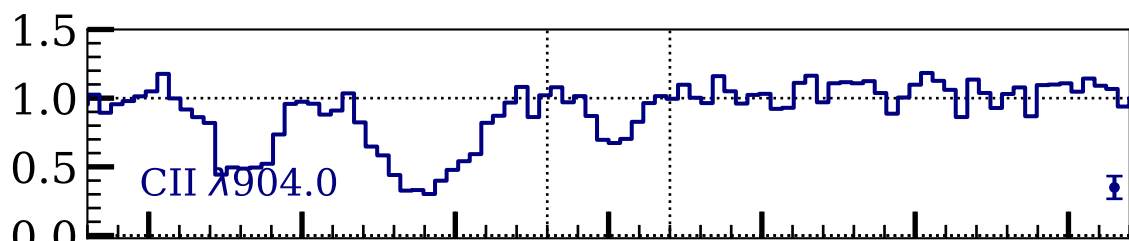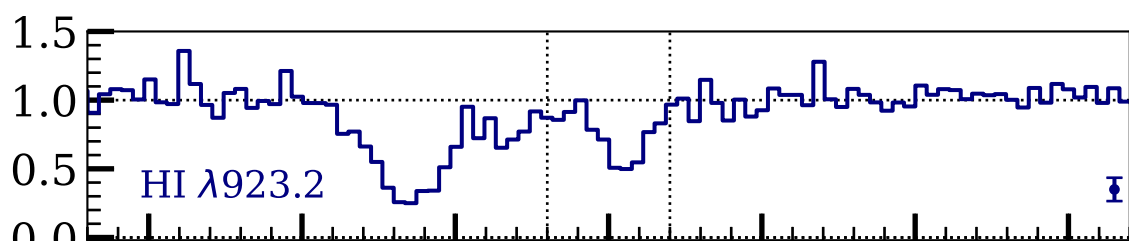

Rest-Frame Velocity ( $\text{km s}^{-1}$ )

J055224.49-640210.7,  $z=0.345149$ , RF=1

Normalized Flux

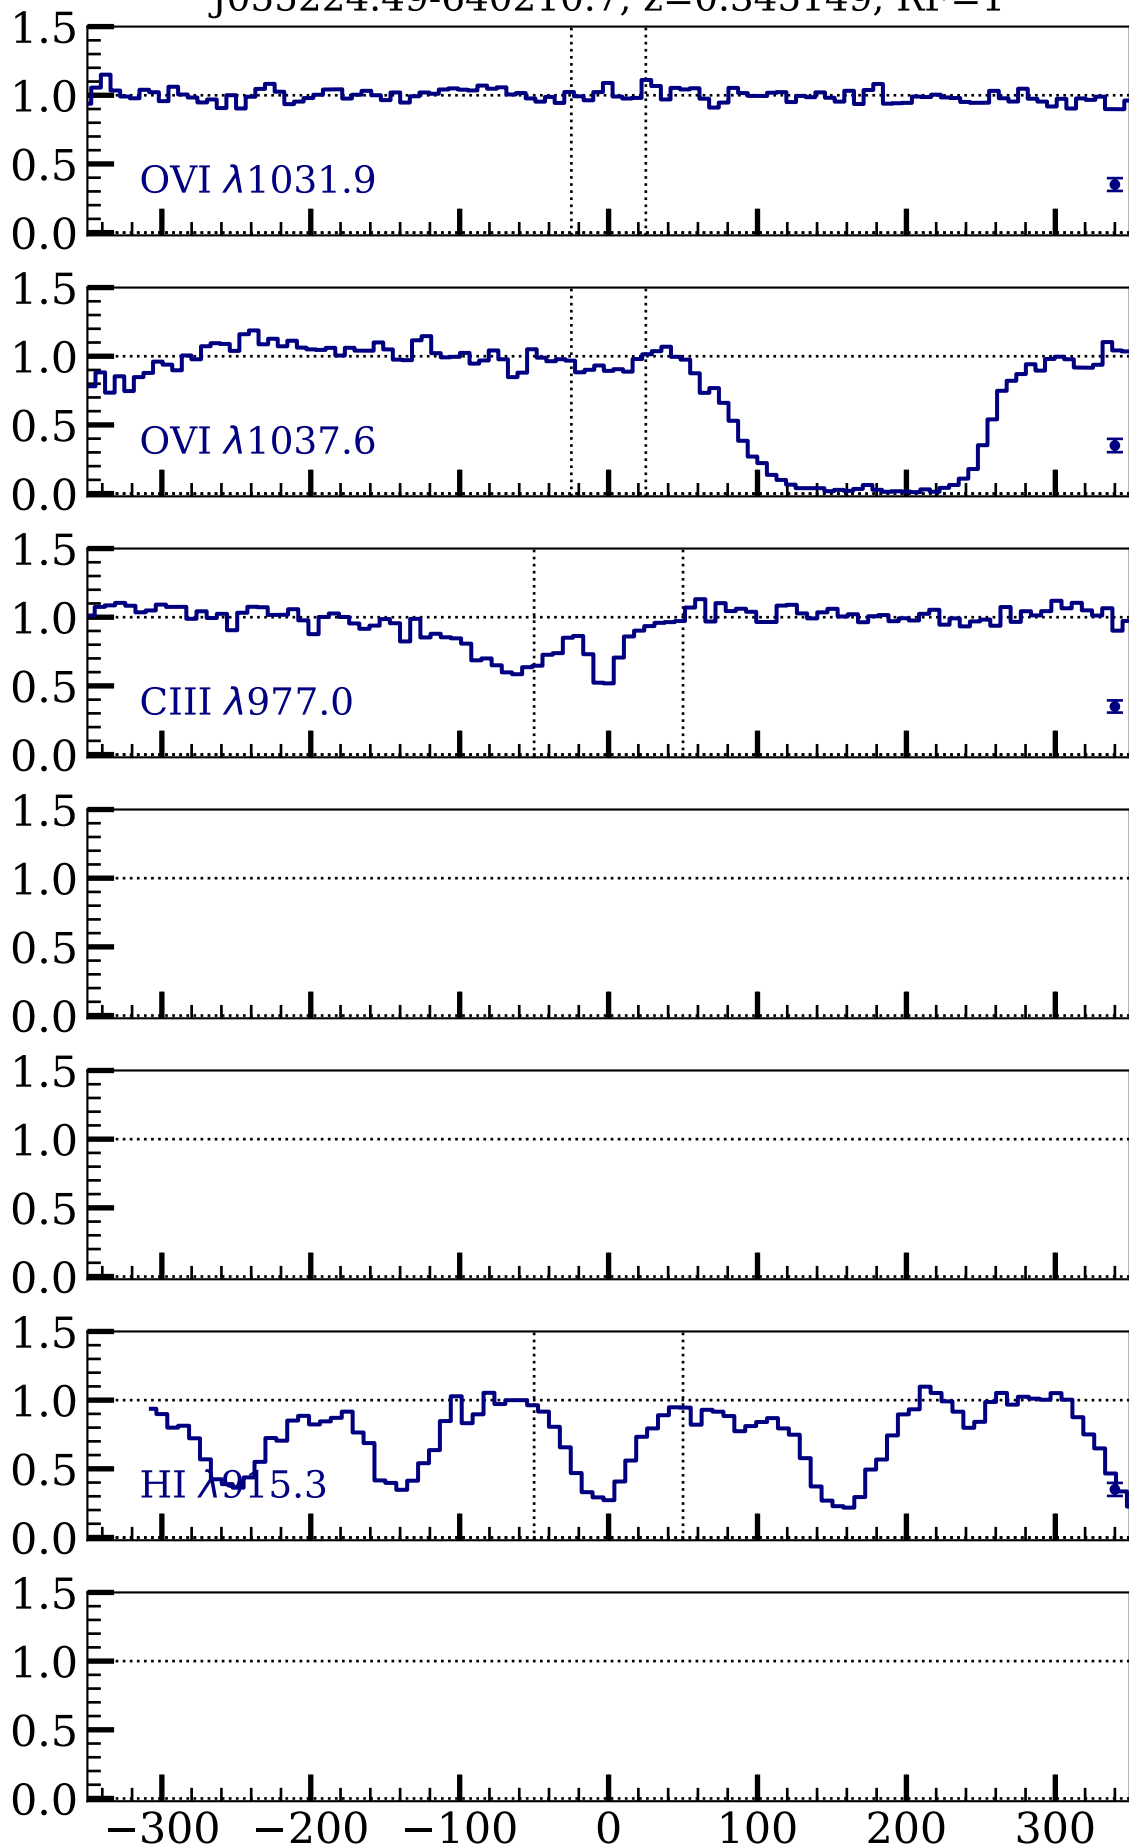

Rest-Frame Velocity (km s<sup>-1</sup>)

J055224.49-640210.7,  $z=0.446088$ , RF=1

Normalized Flux

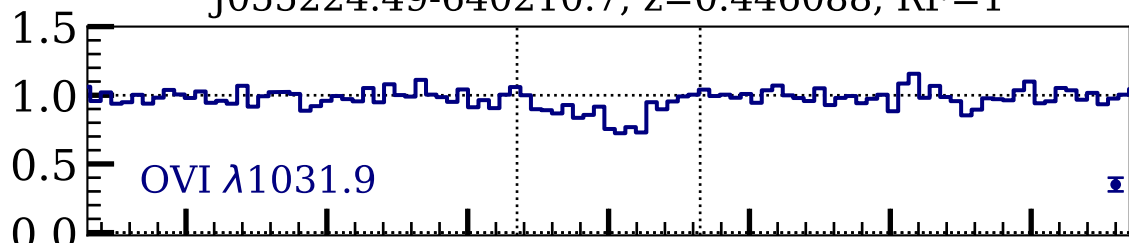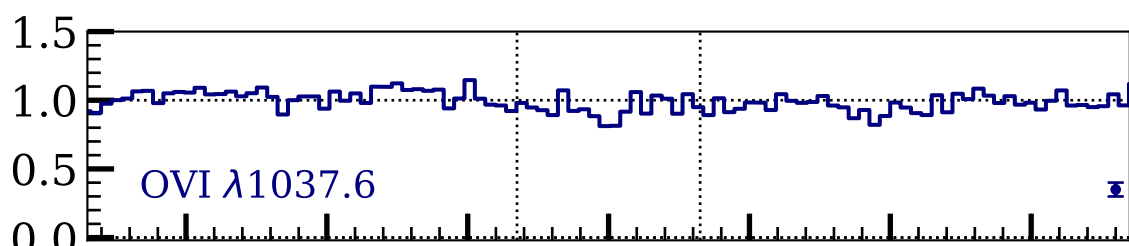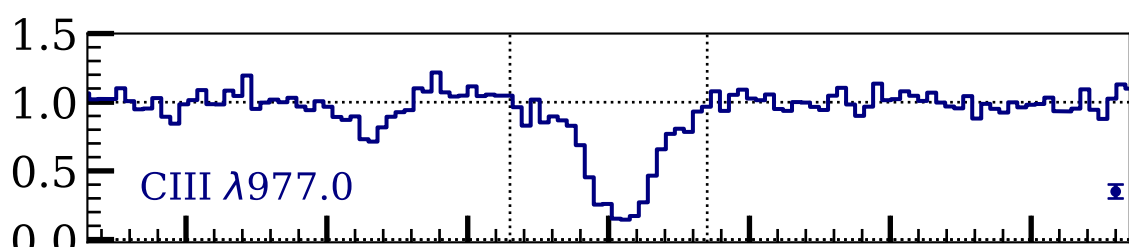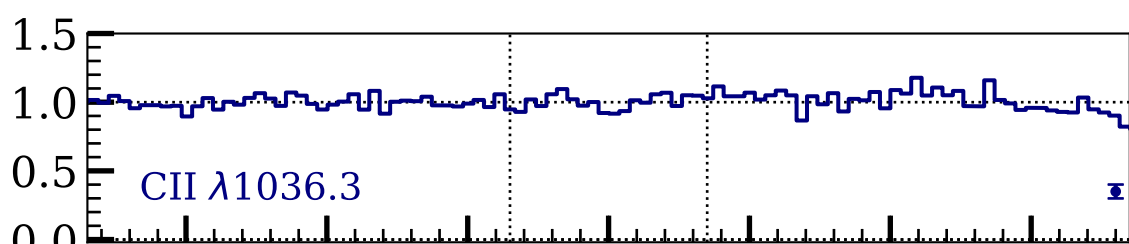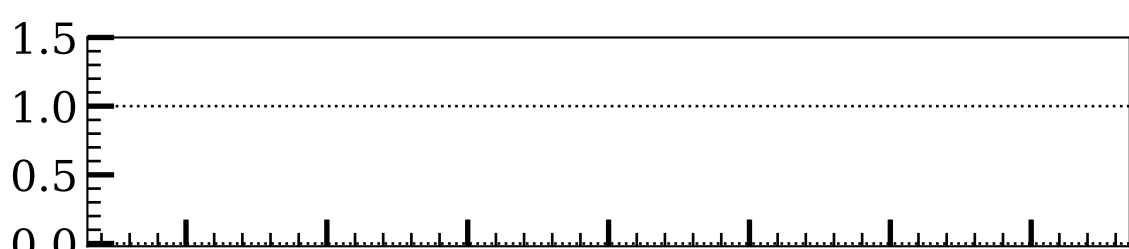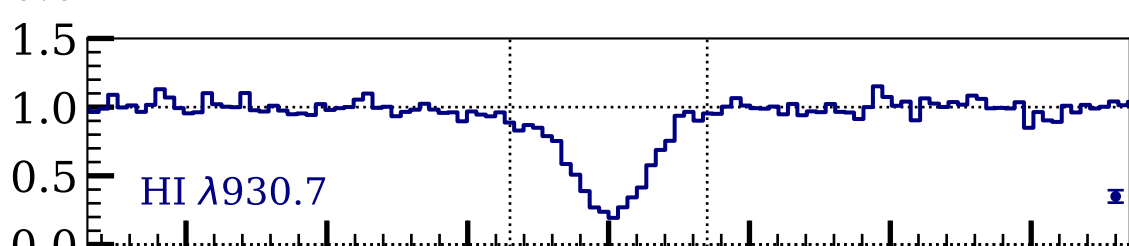

Rest-Frame Velocity ( $\text{km s}^{-1}$ )

J063546.49-751616.8,  $z=0.417468$ , RF=1

Normalized Flux

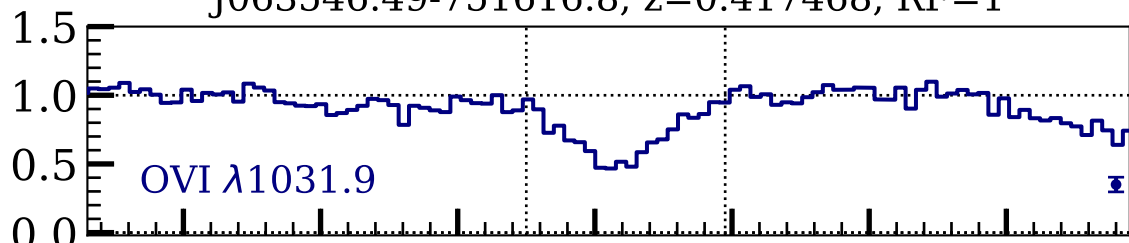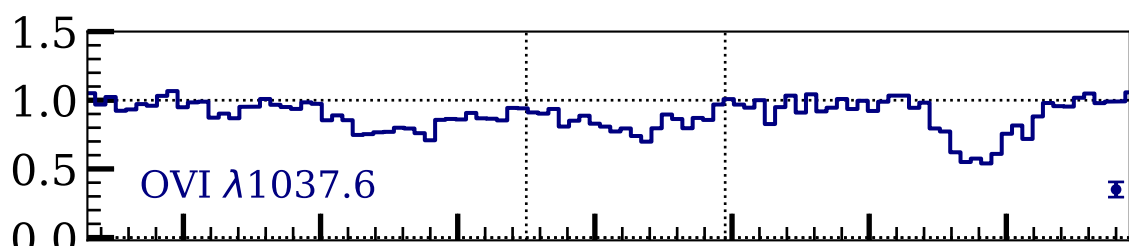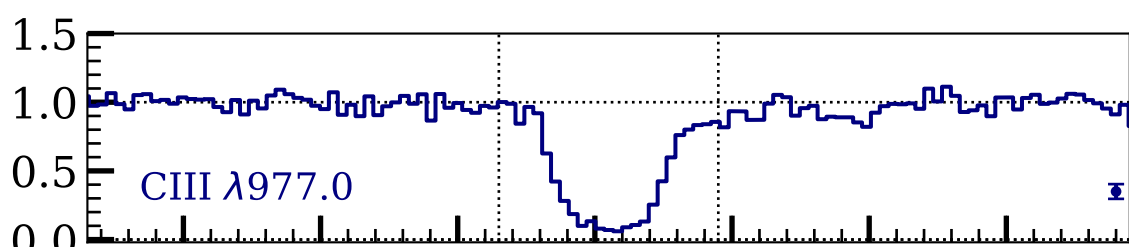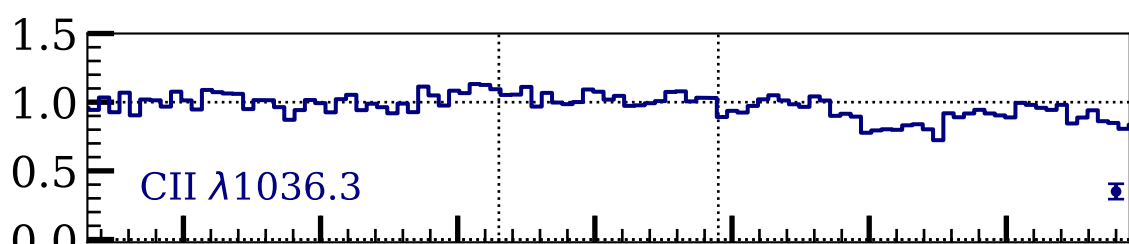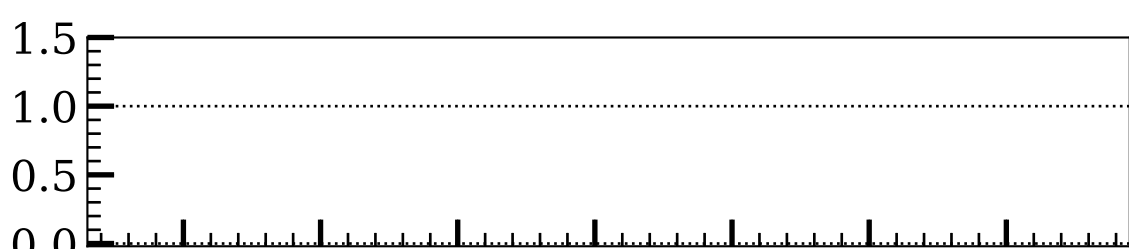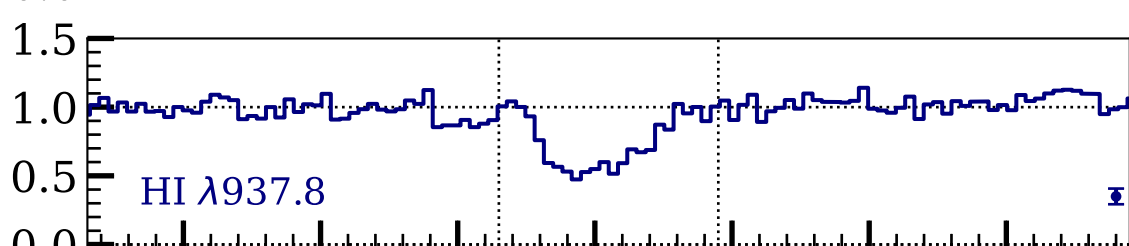

Rest-Frame Velocity ( $\text{km s}^{-1}$ )

J063546.49-751616.8,  $z=0.452768$ , RF=1

Normalized Flux

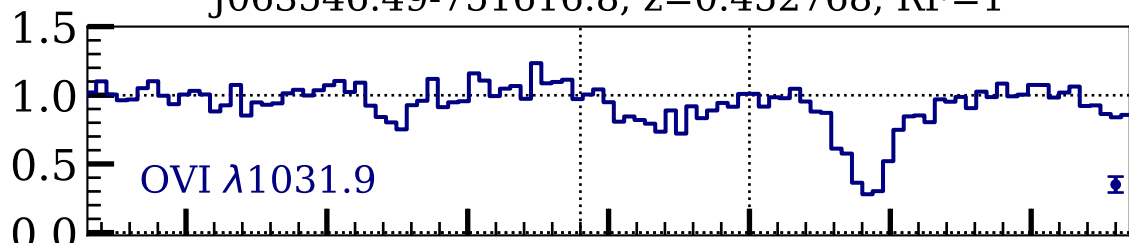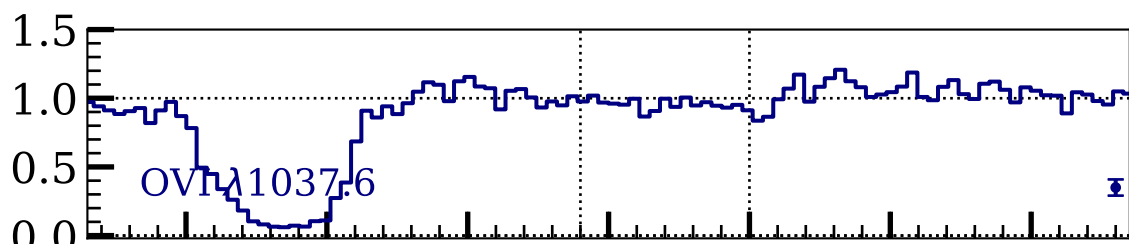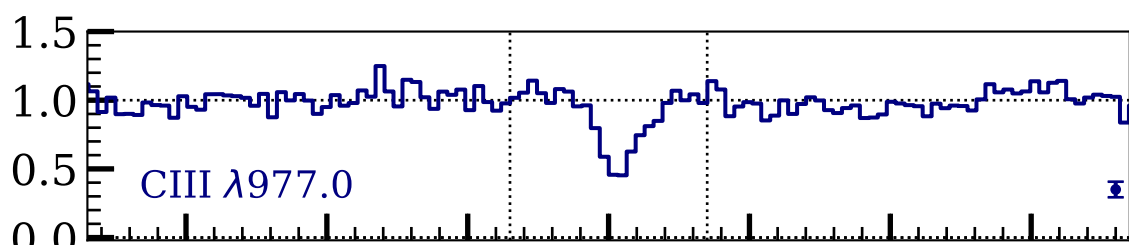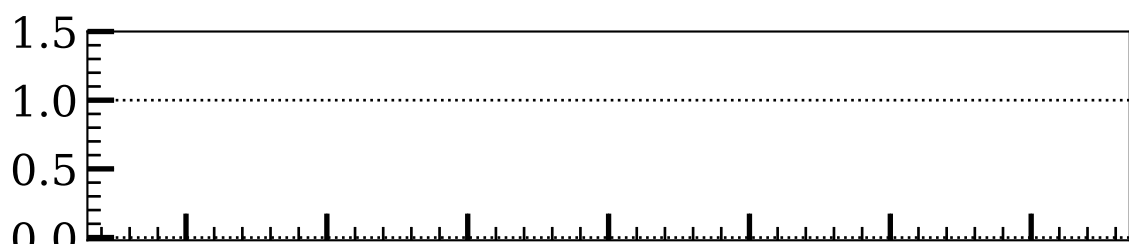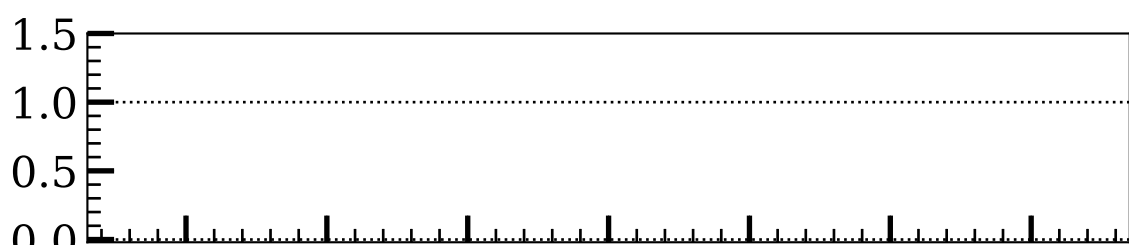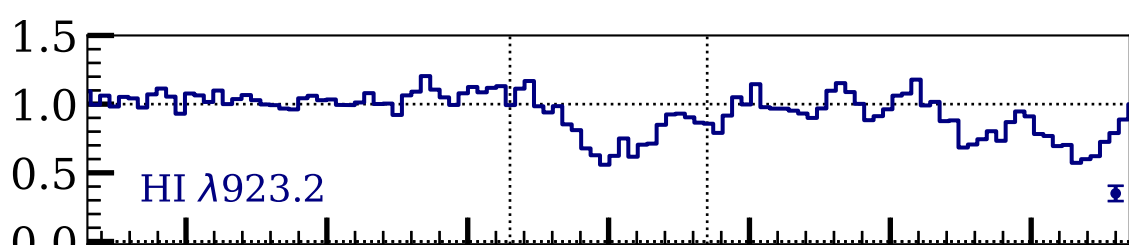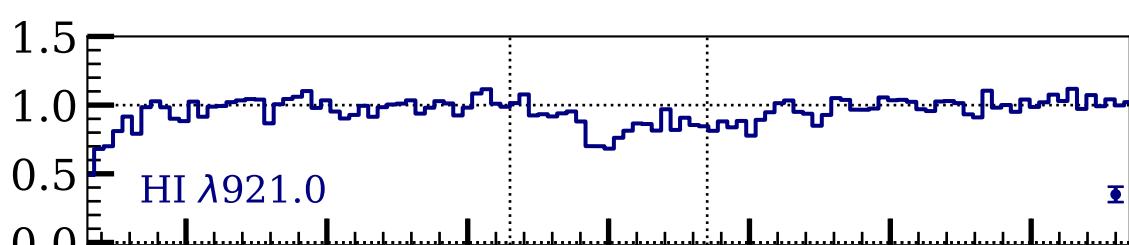

Rest-Frame Velocity ( $\text{km s}^{-1}$ )

J063546.49-751616.8,  $z=0.468486$ , RF=1

Normalized Flux

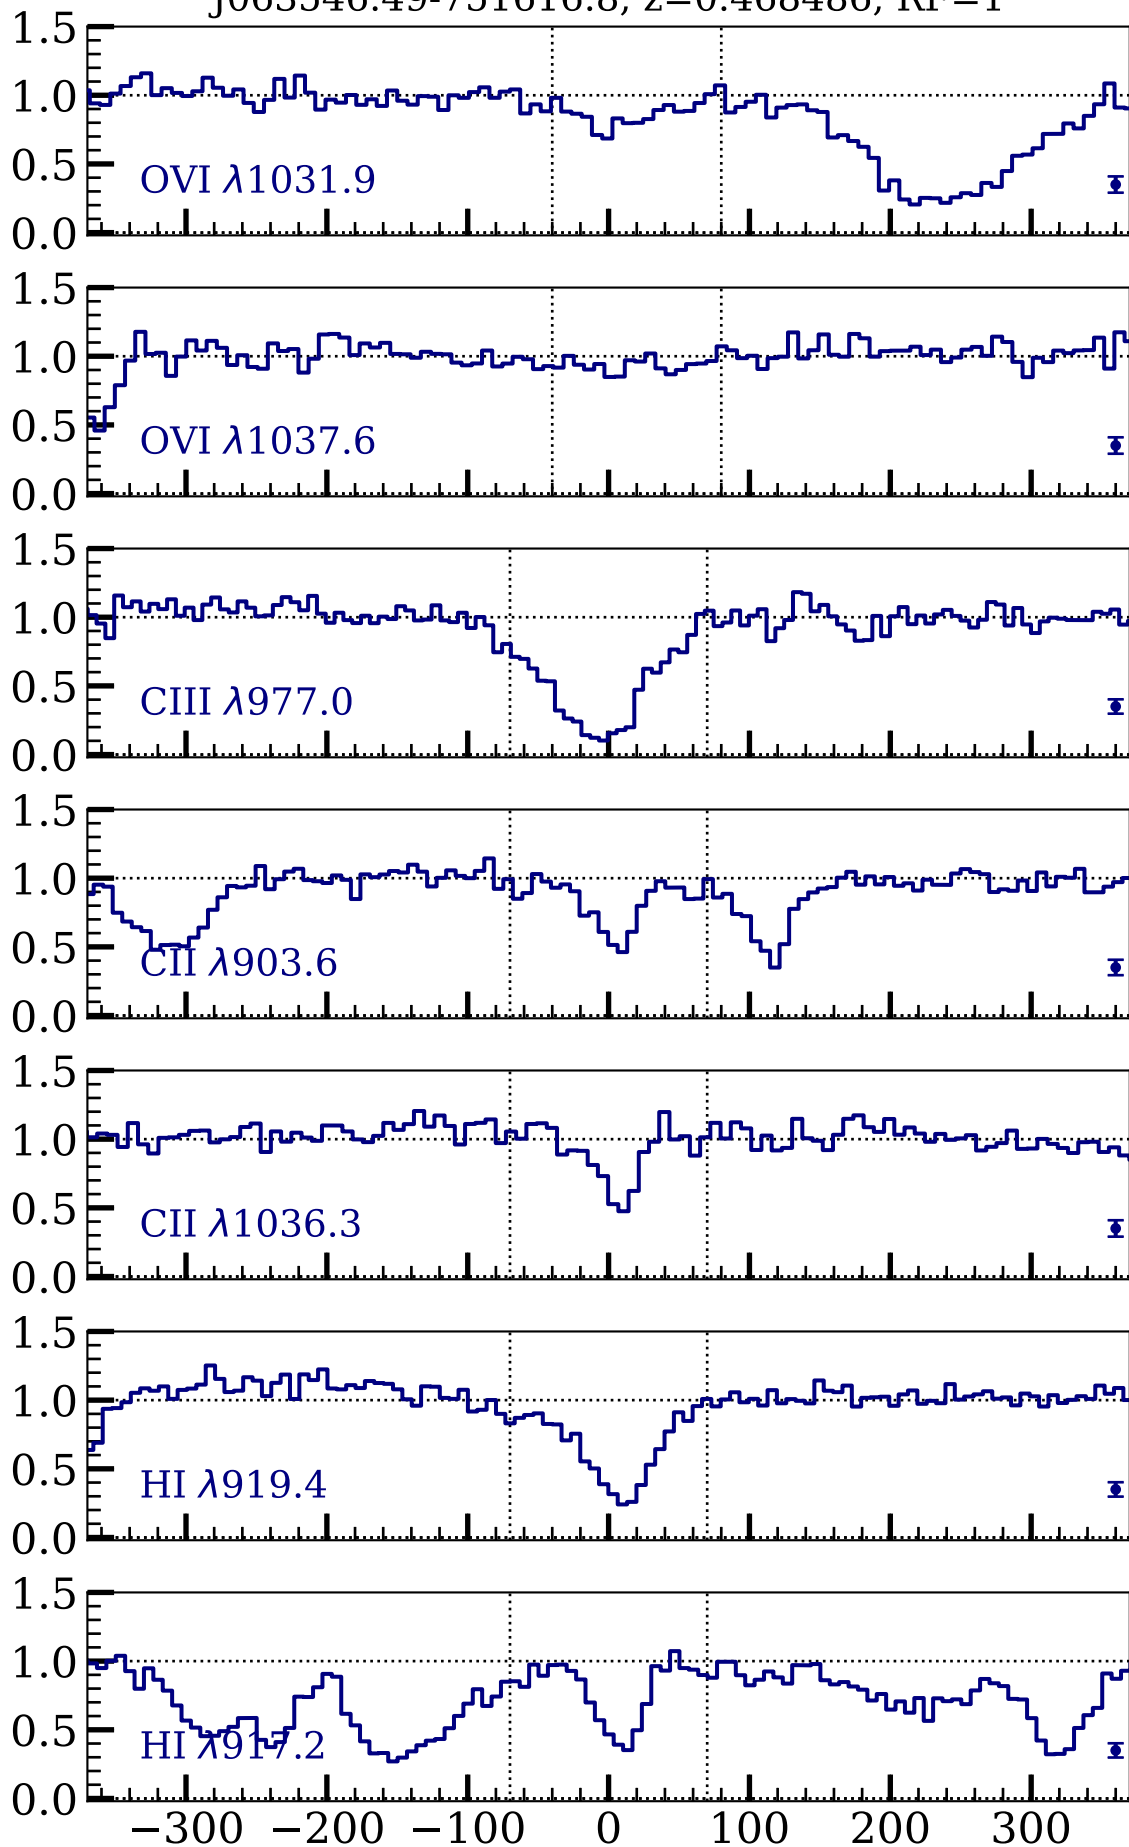

Rest-Frame Velocity (km s<sup>-1</sup>)

J071950.89+742757.0,  $z=0.377707$ , RF=1

Normalized Flux

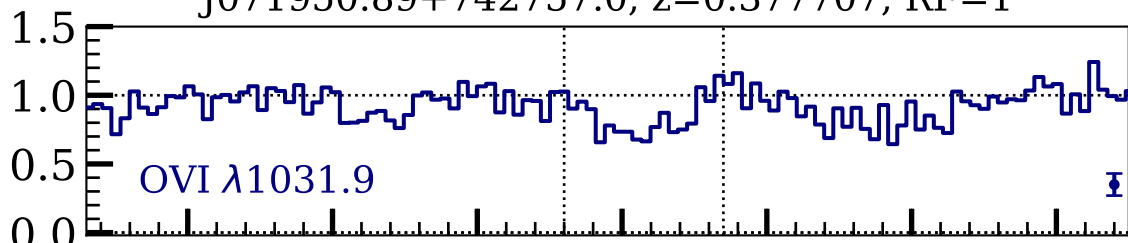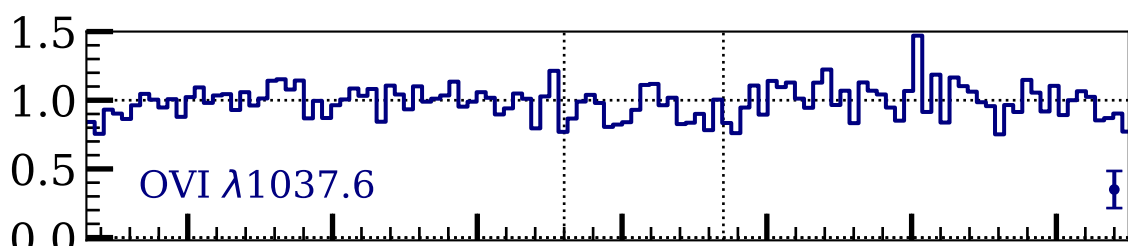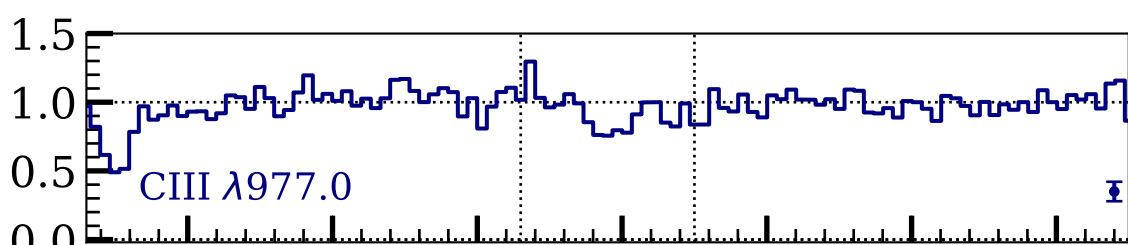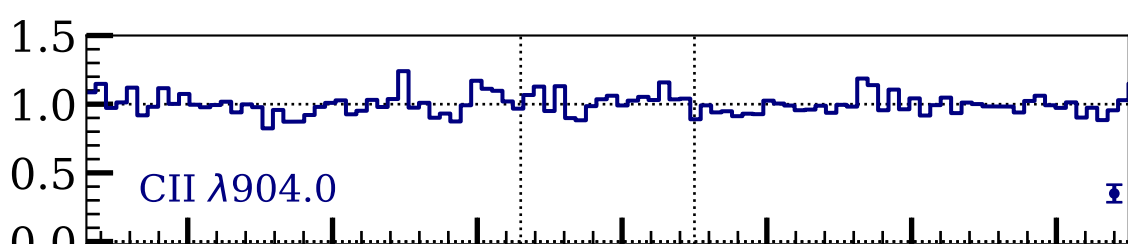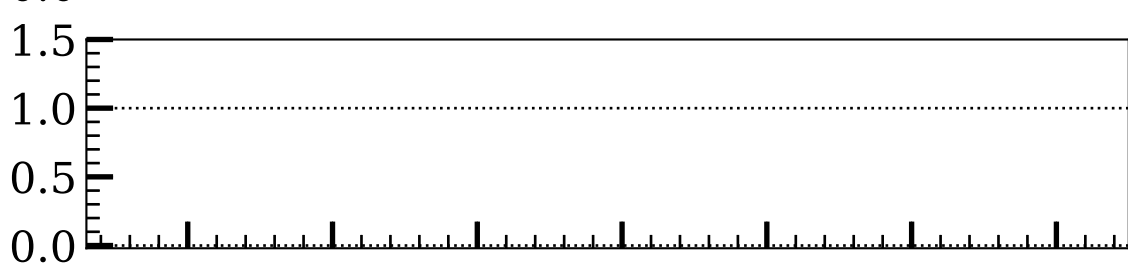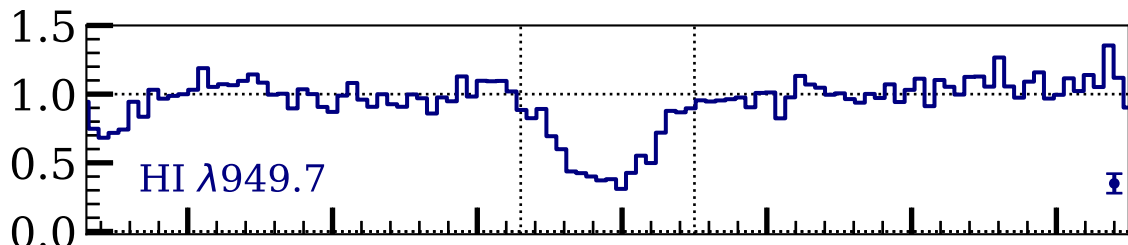

Rest-Frame Velocity ( $\text{km s}^{-1}$ )

J075112.30+291938.3,  $z=0.431765$ , RF=1

Normalized Flux

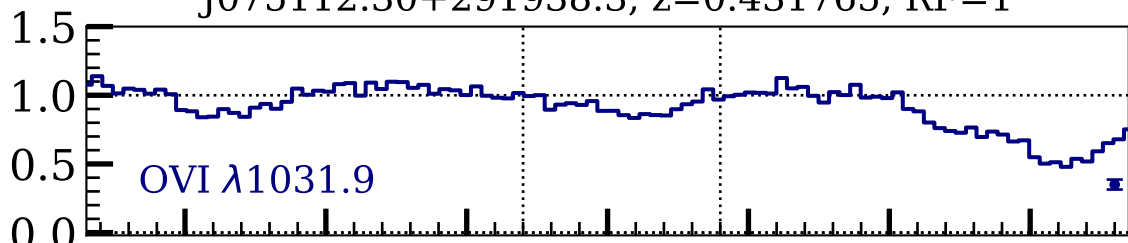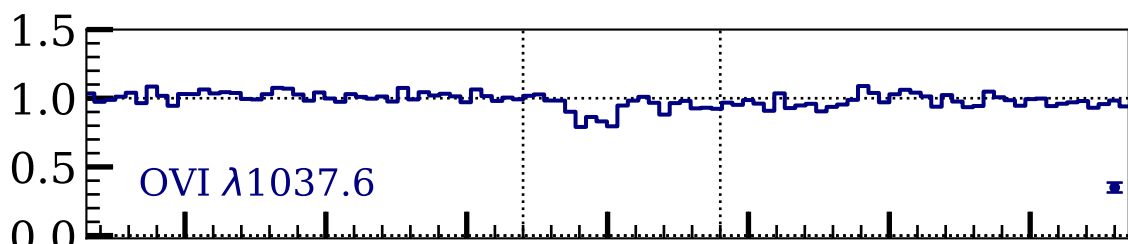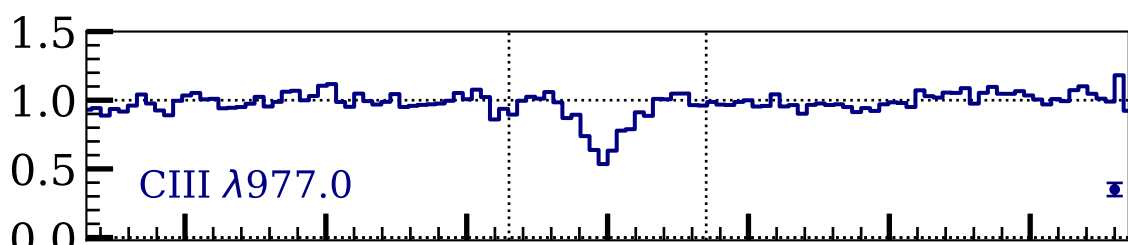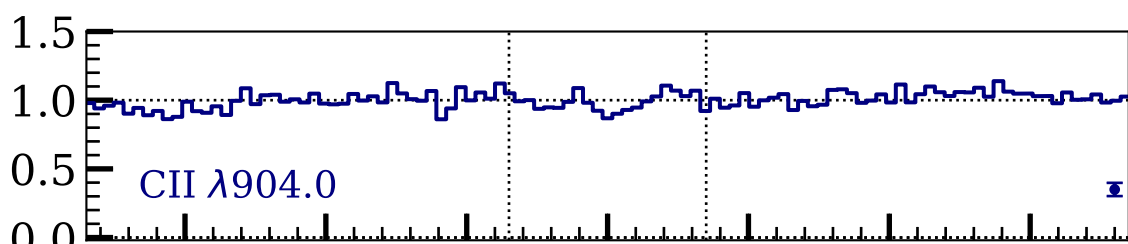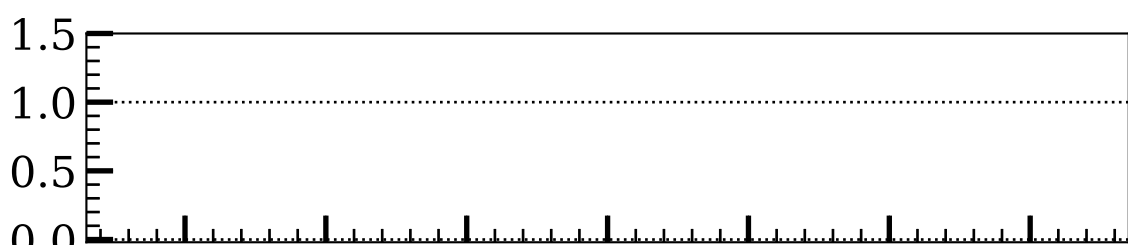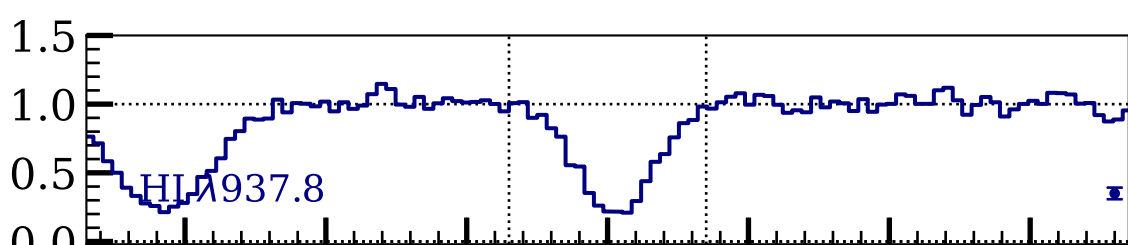

Rest-Frame Velocity ( $\text{km s}^{-1}$ )



J075112.30+291938.3,  $z=0.494502$ , RF=1

Normalized Flux

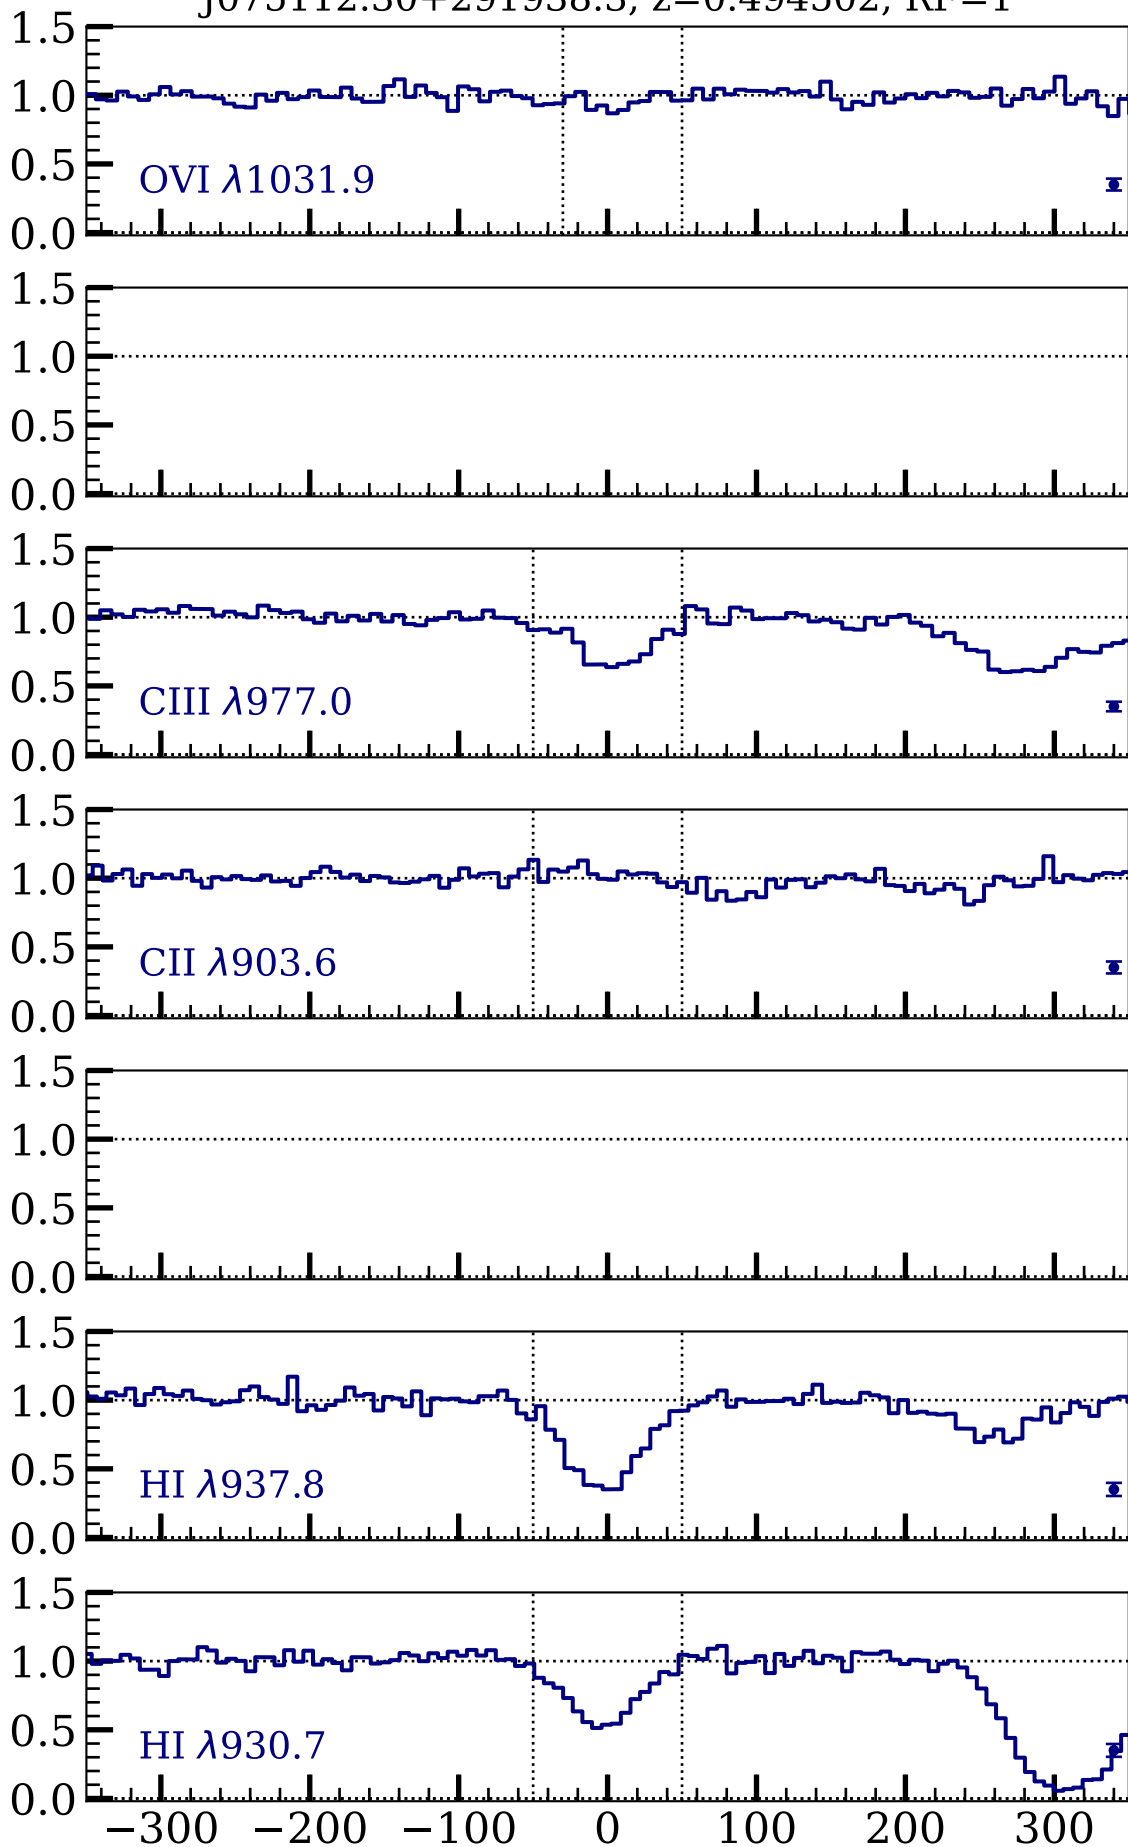

Rest-Frame Velocity (km s<sup>-1</sup>)

J080908.13+461925.6,  $z=0.619130$ , RF=1

Normalized Flux

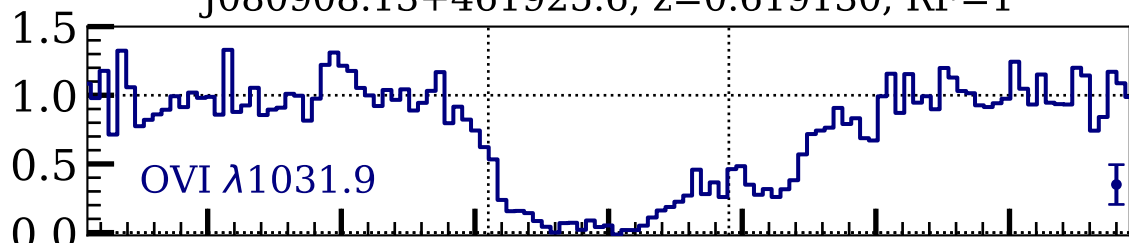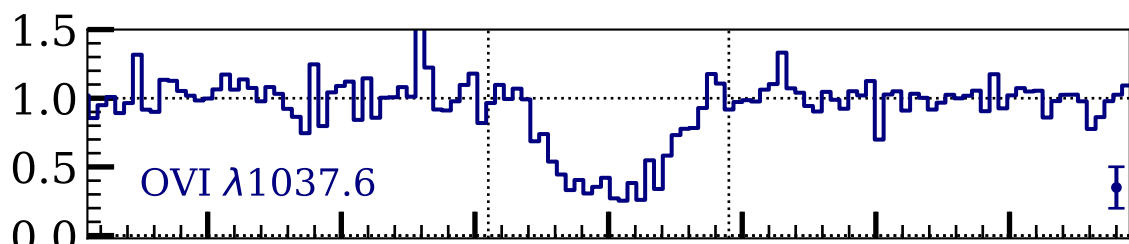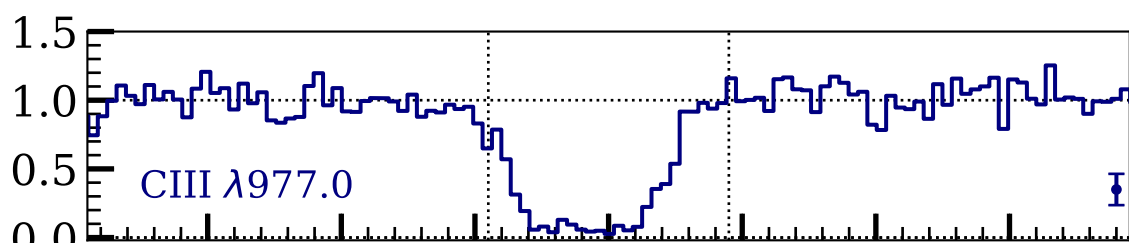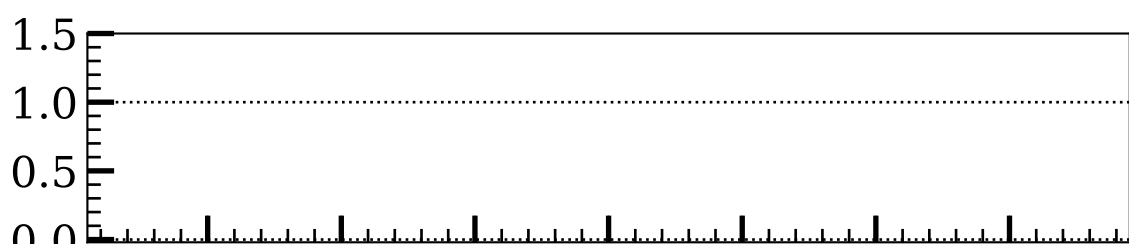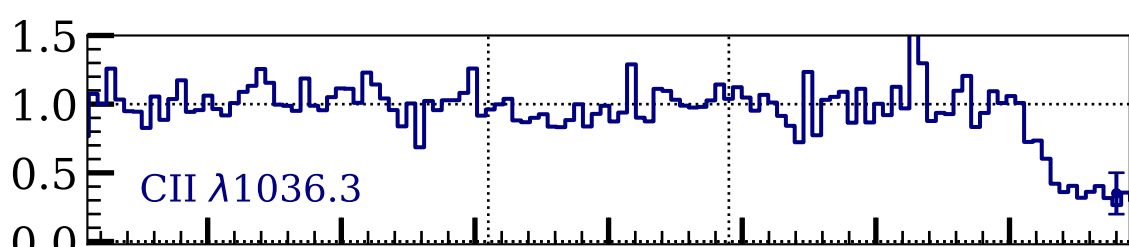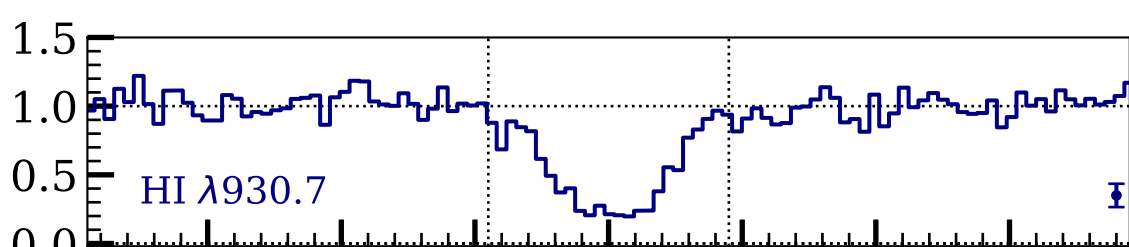

-300 -200 -100 0 100 200 300

Rest-Frame Velocity ( $\text{km s}^{-1}$ )

J084349.47+411741.6,  $z=0.533507$ , RF=0

Normalized Flux

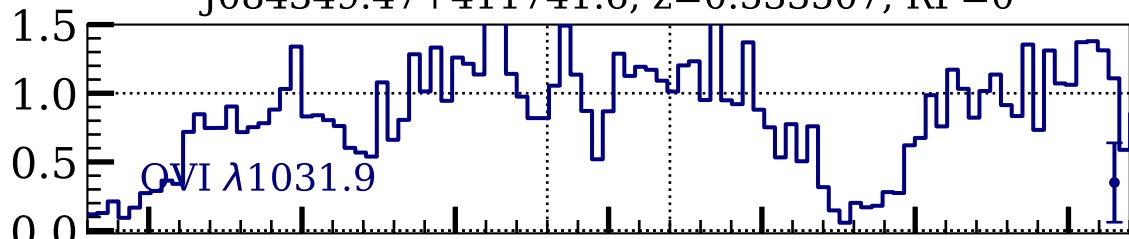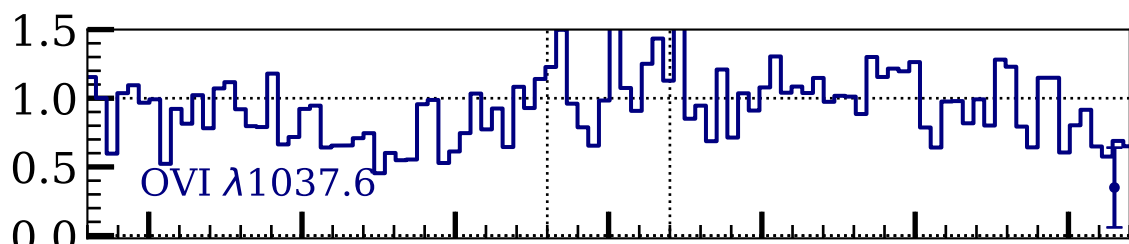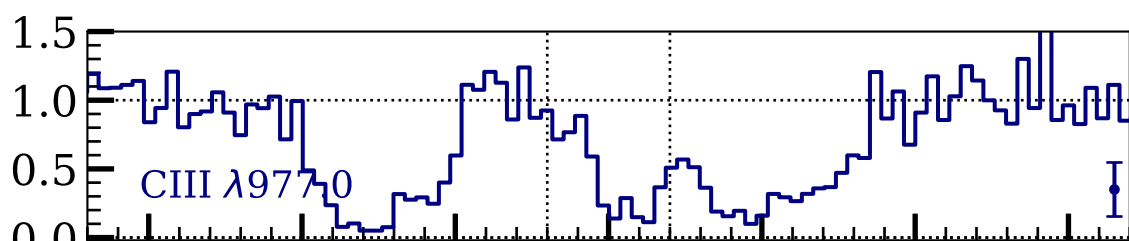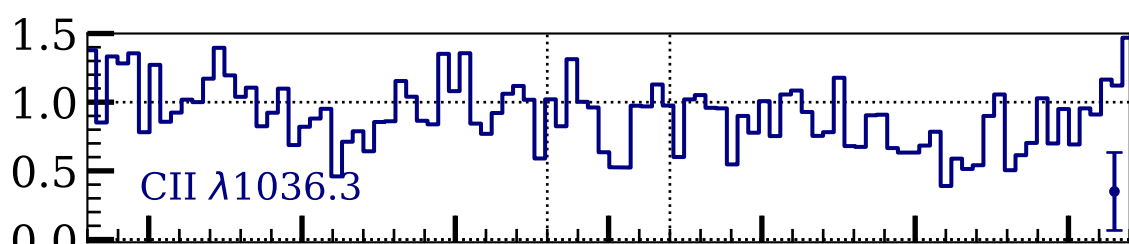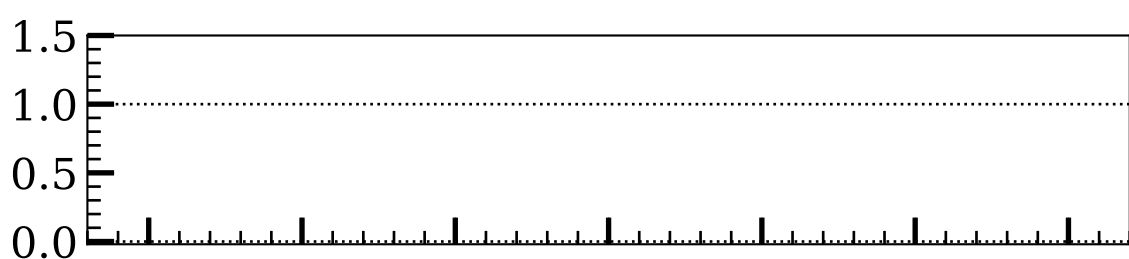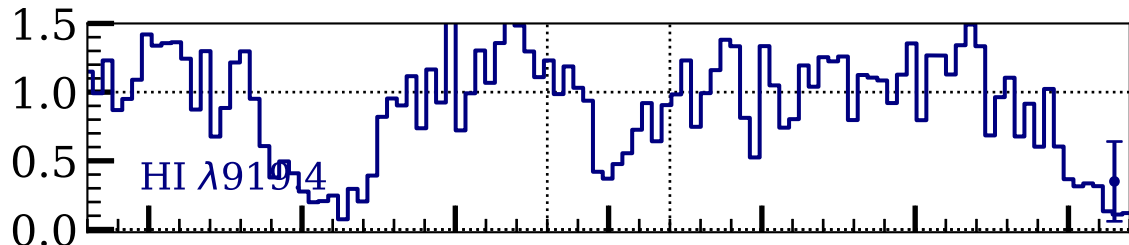

Rest-Frame Velocity ( $\text{km s}^{-1}$ )

J084349.47+411741.6,  $z=0.541051$ , RF=0

Normalized Flux

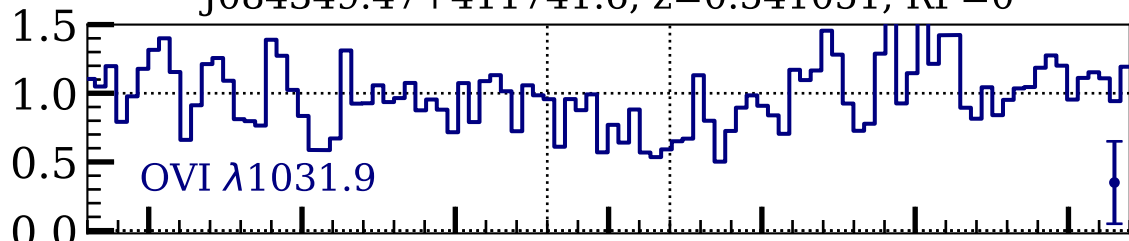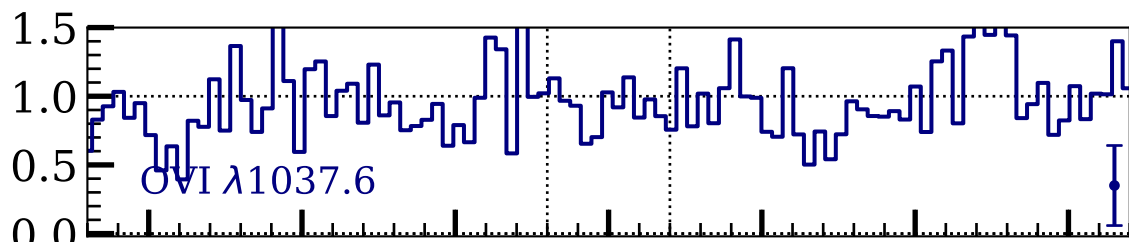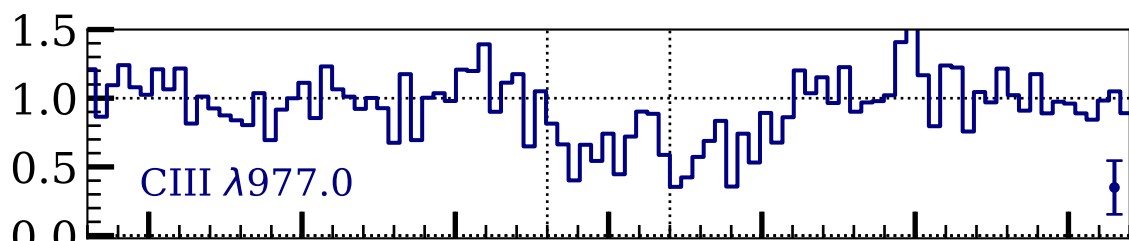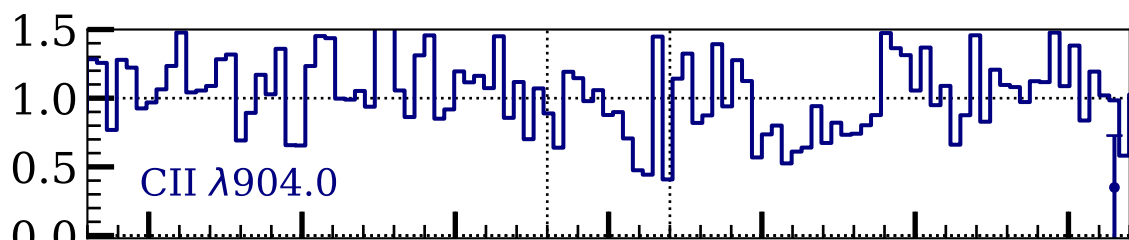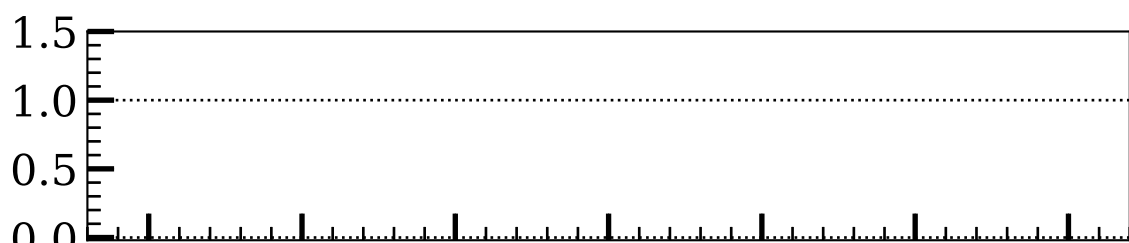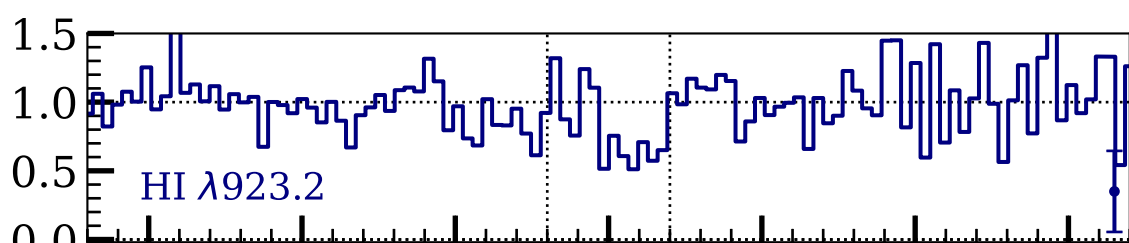

Rest-Frame Velocity ( $\text{km s}^{-1}$ )

J084349.47+411741.6,  $z=0.543679$ , RF=0

Normalized Flux

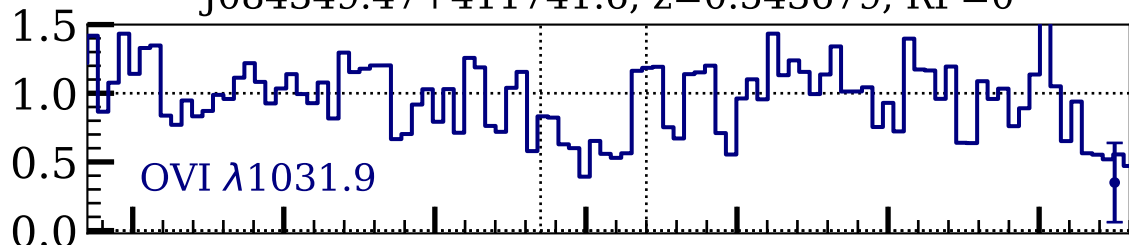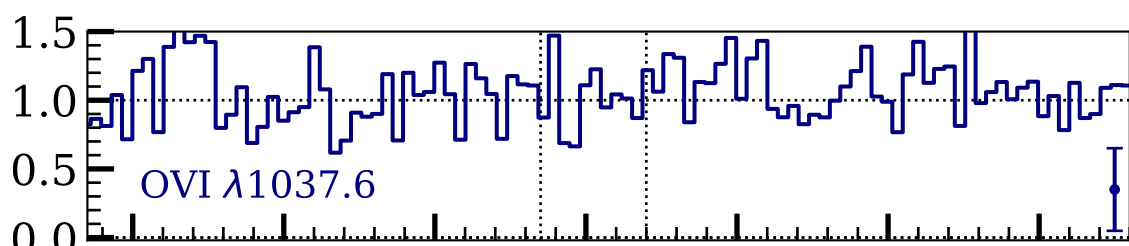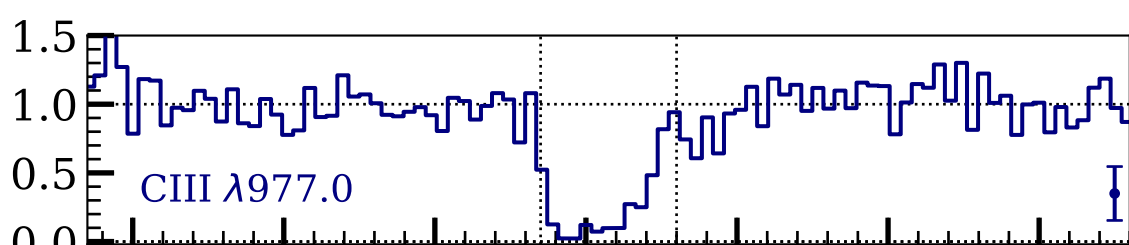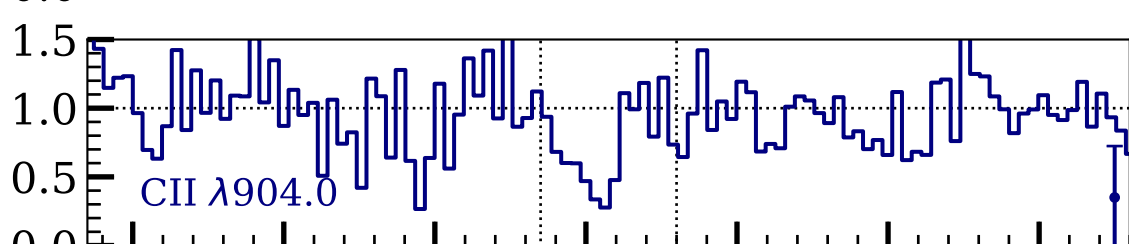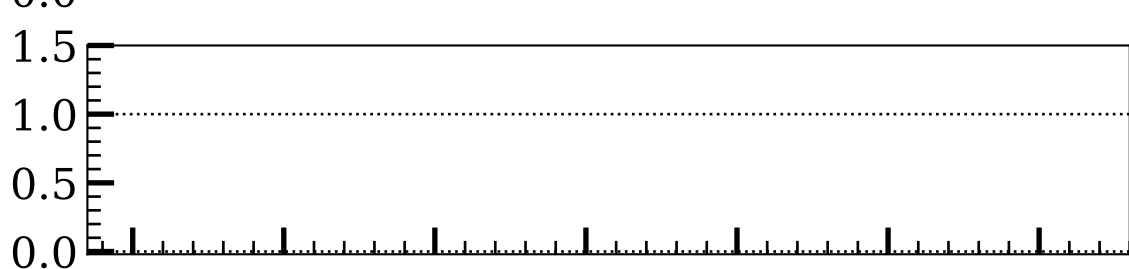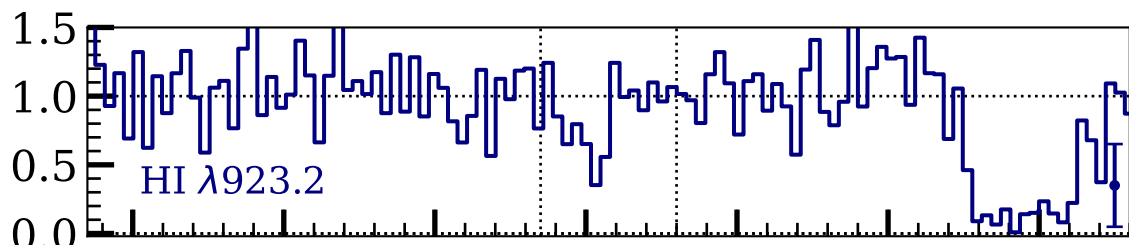

Rest-Frame Velocity ( $\text{km s}^{-1}$ )

J091440.38+282330.6,  $z=0.244249$ , RF=1

Normalized Flux

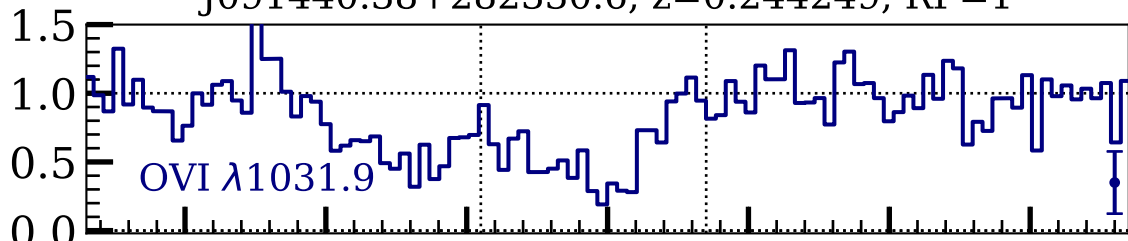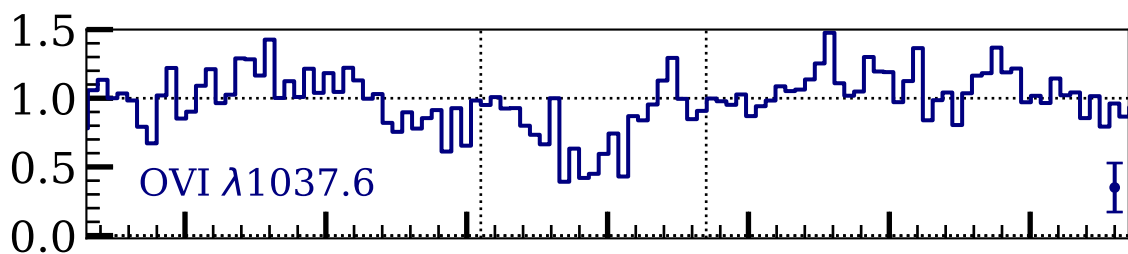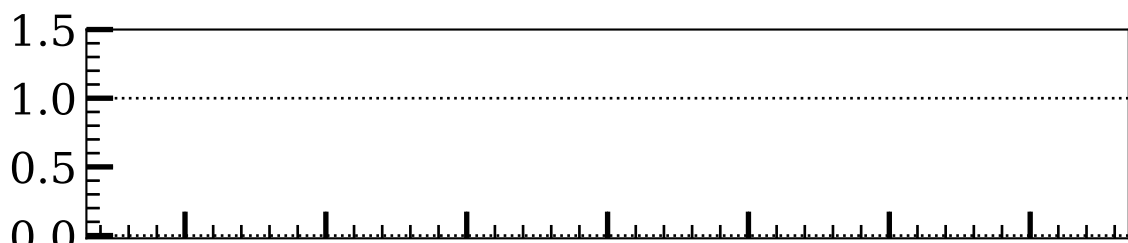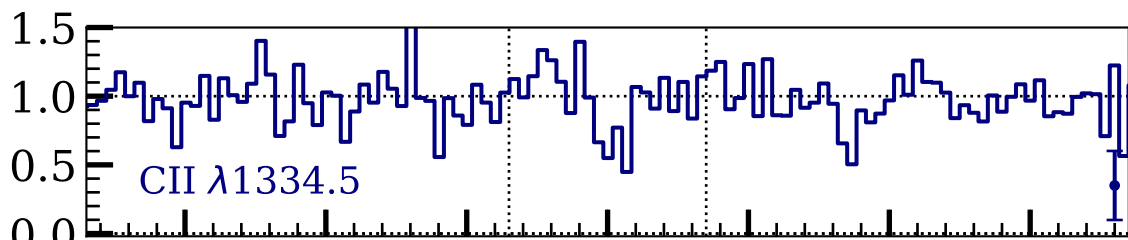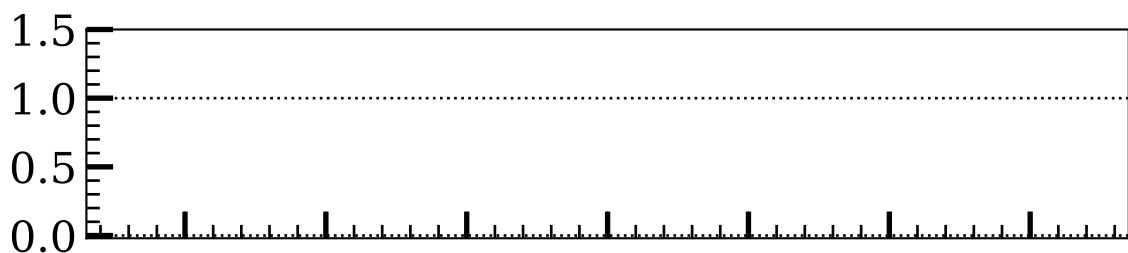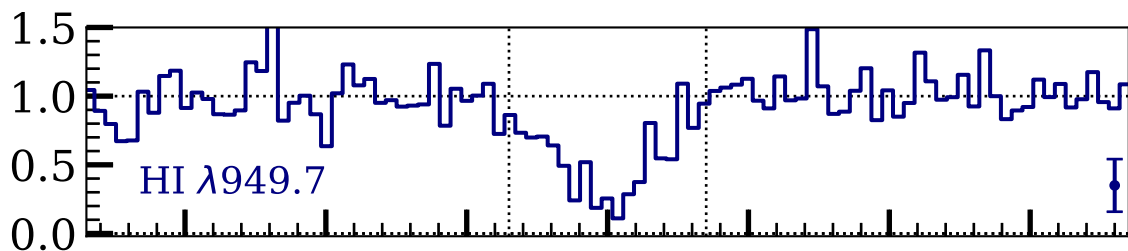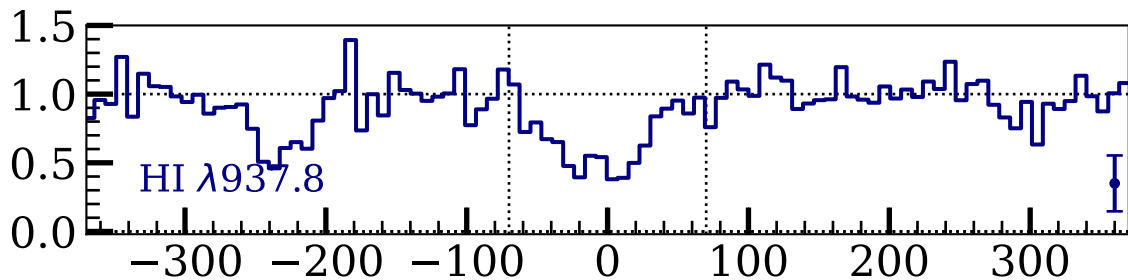

Rest-Frame Velocity ( $\text{km s}^{-1}$ )

J091440.38+282330.6,  $z=0.599535$ , RF=0

Normalized Flux

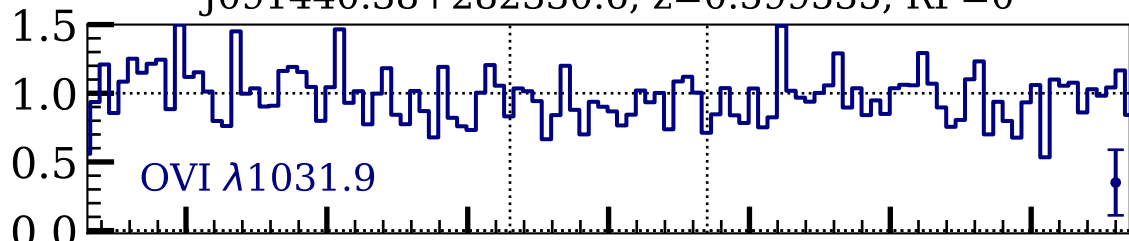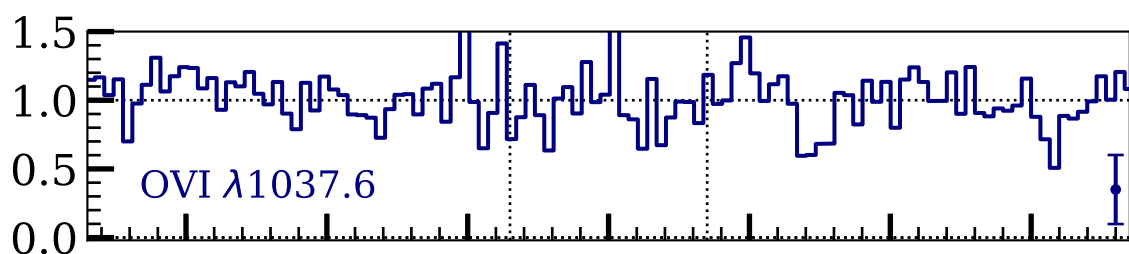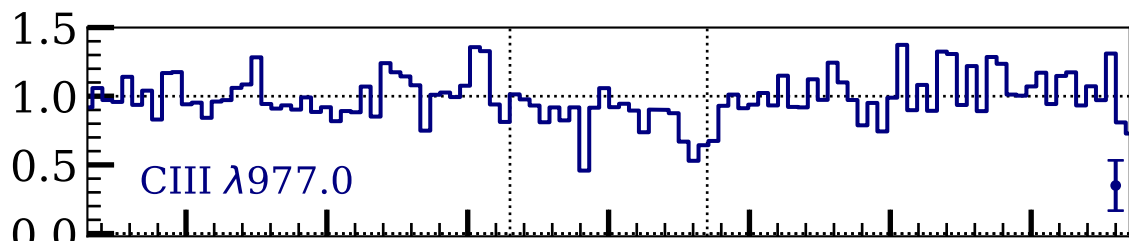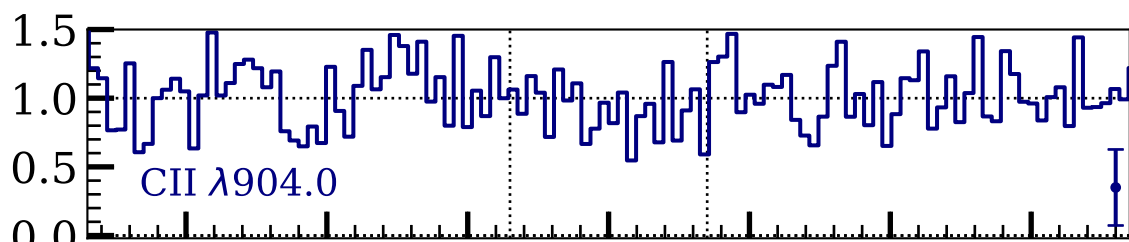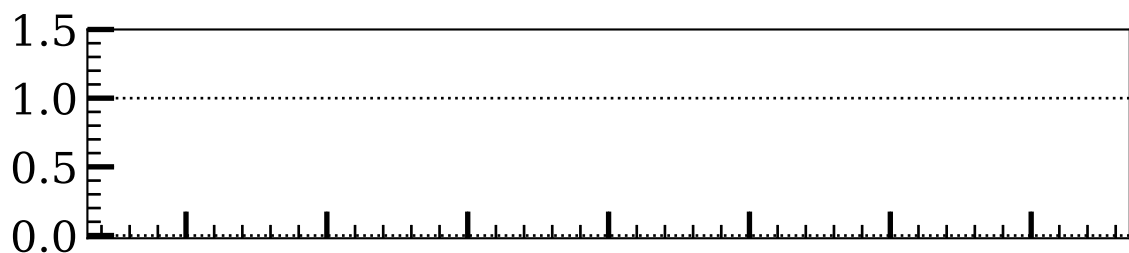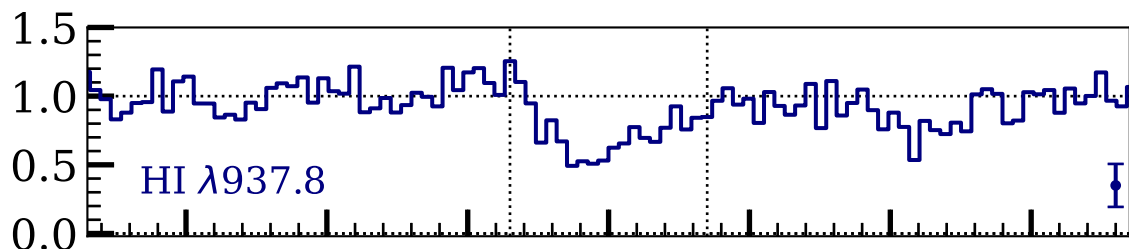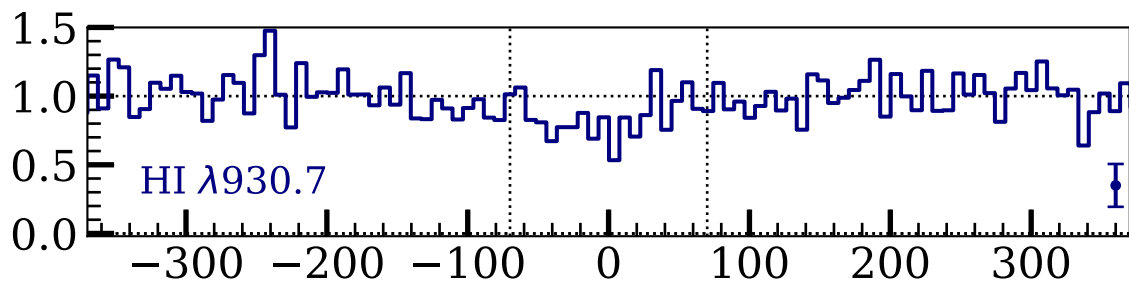

Rest-Frame Velocity ( $\text{km s}^{-1}$ )

Normalized Flux

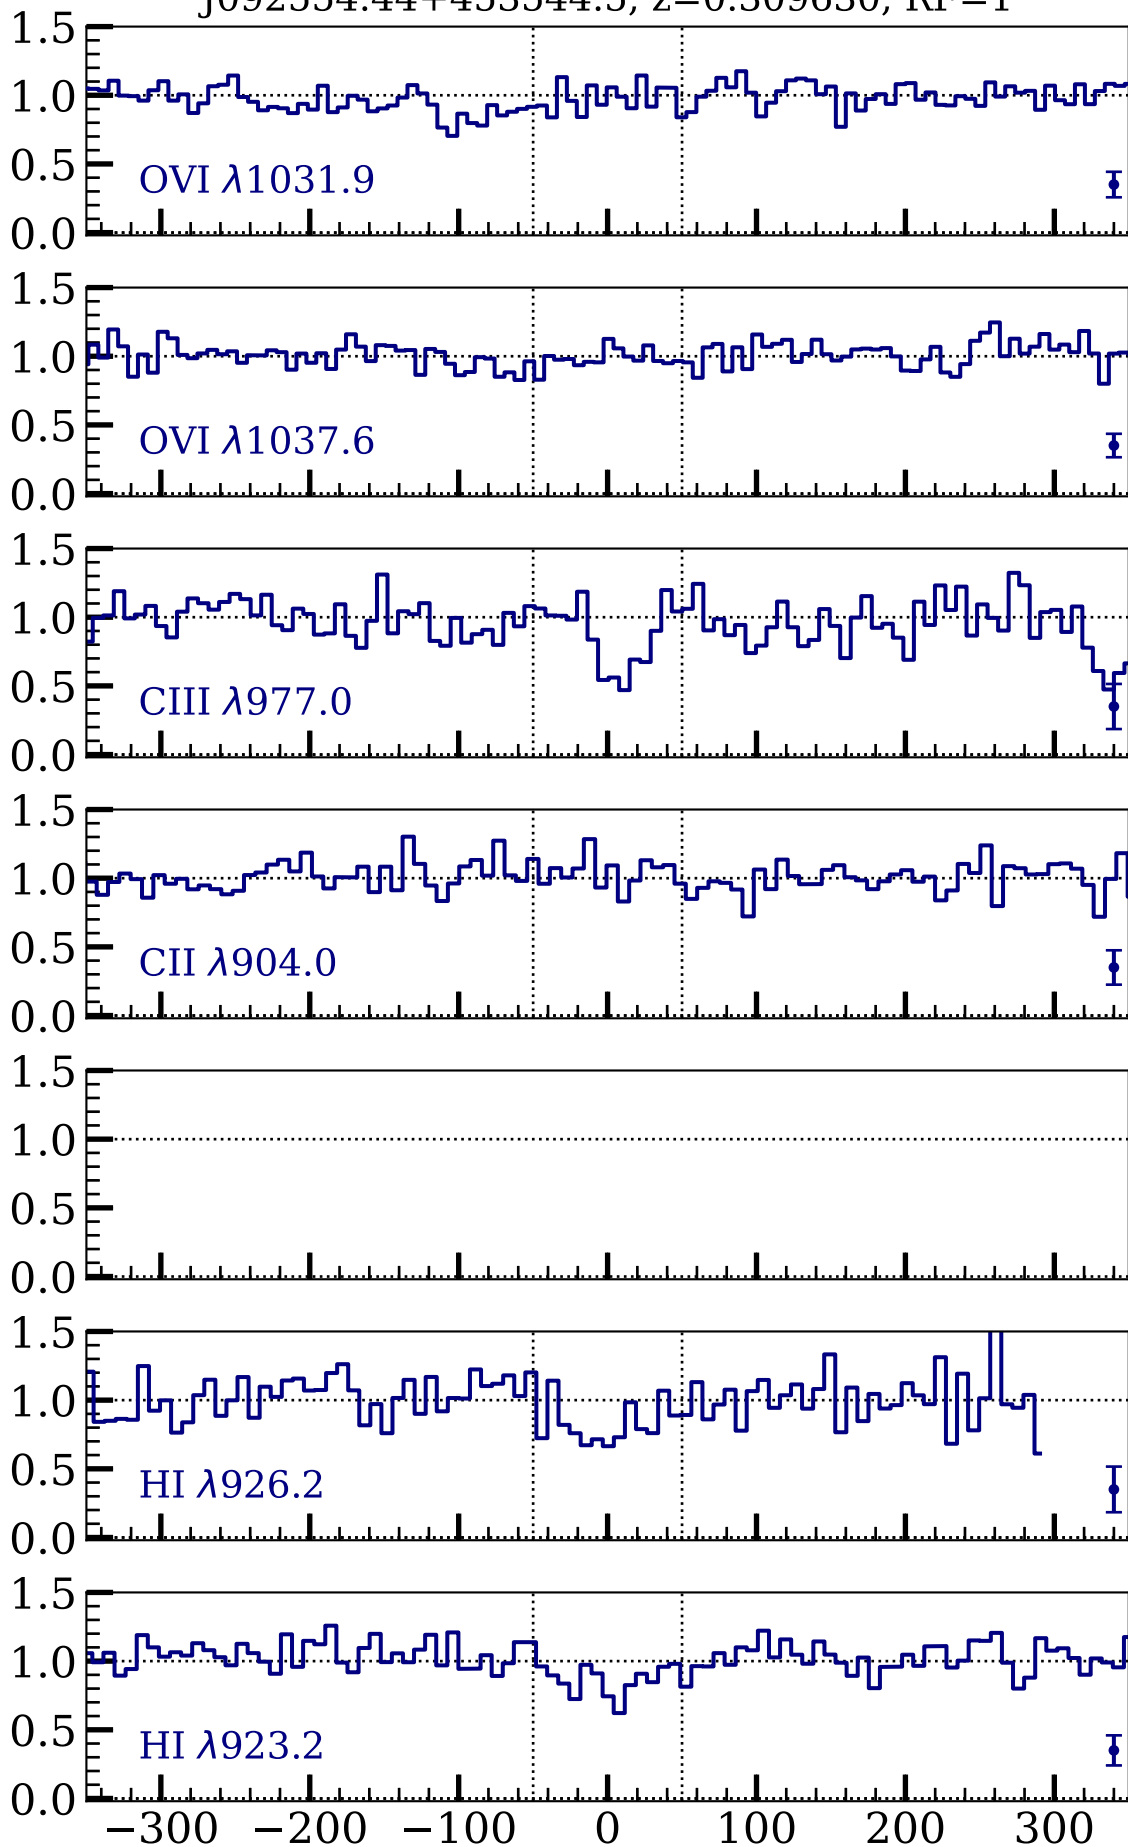Rest-Frame Velocity (km s<sup>-1</sup>)



J093518.19+020415.5,  $z=0.354712$ , RF=0

Normalized Flux

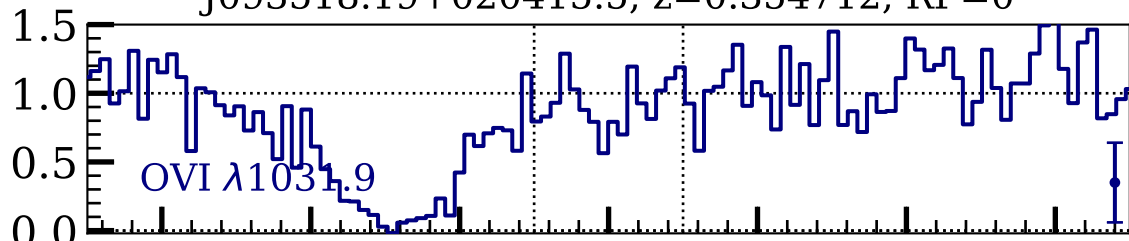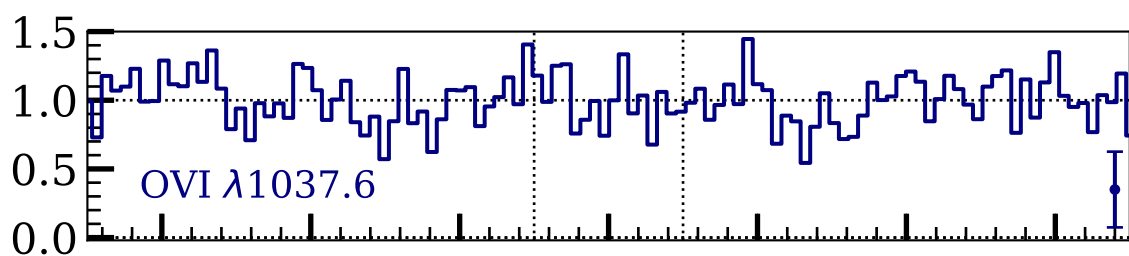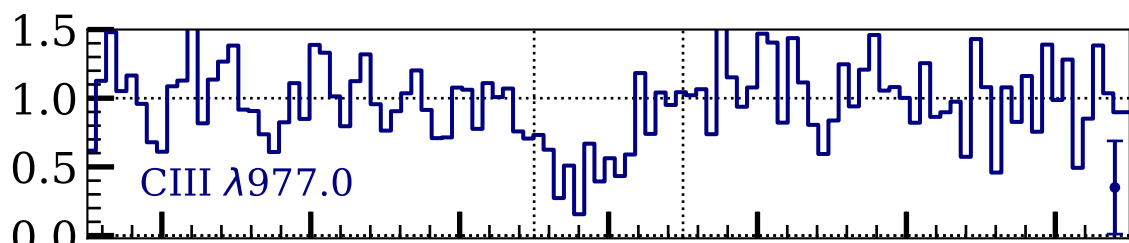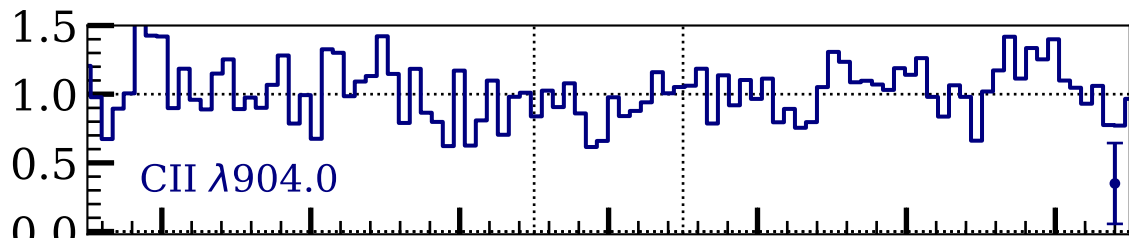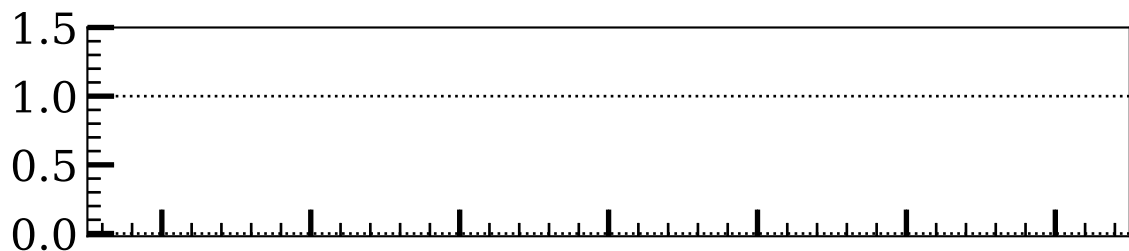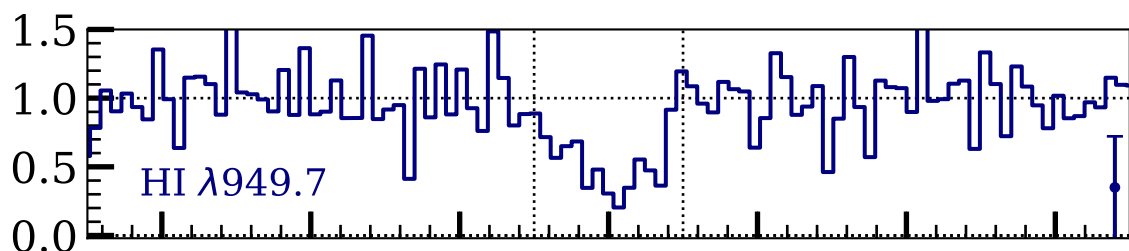

Rest-Frame Velocity ( $\text{km s}^{-1}$ )

J093603.88+320709.3,  $z=0.390435$ , RF=0

Normalized Flux

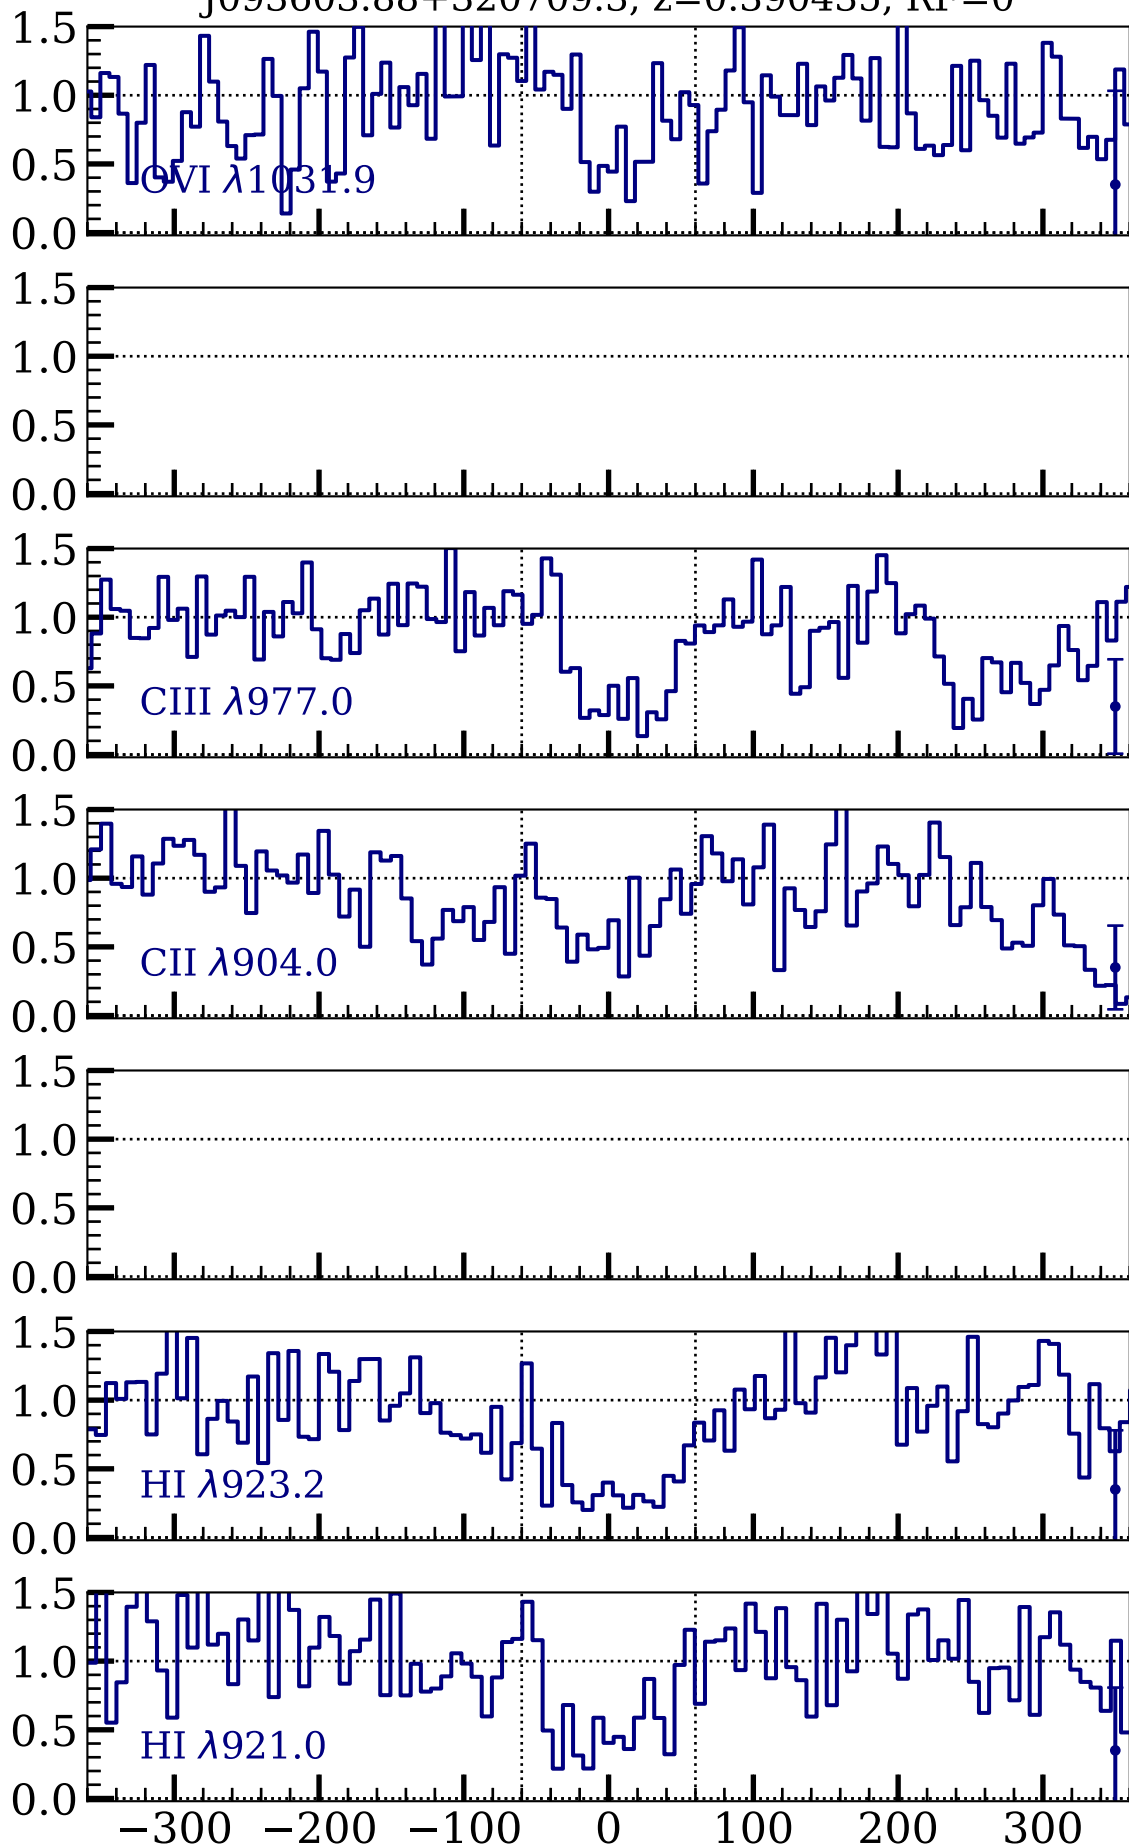

Rest-Frame Velocity (km s<sup>-1</sup>)

J094331.61+053131.4,  $z=0.229019$ , RF=1

Normalized Flux

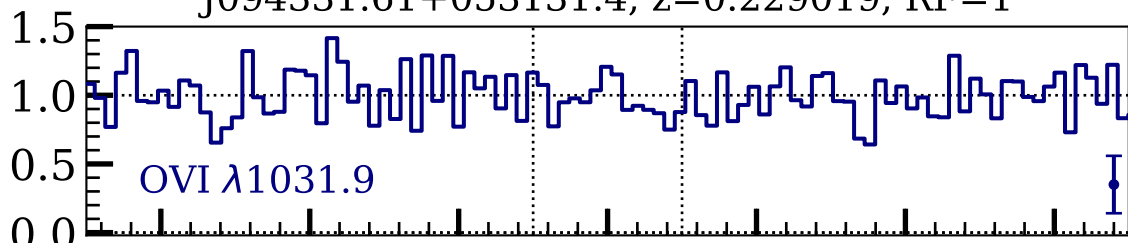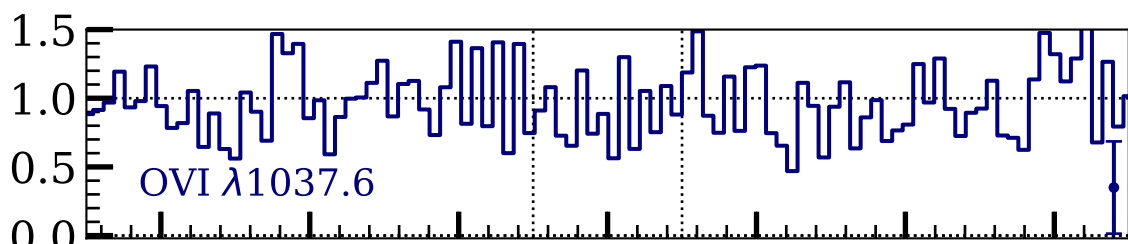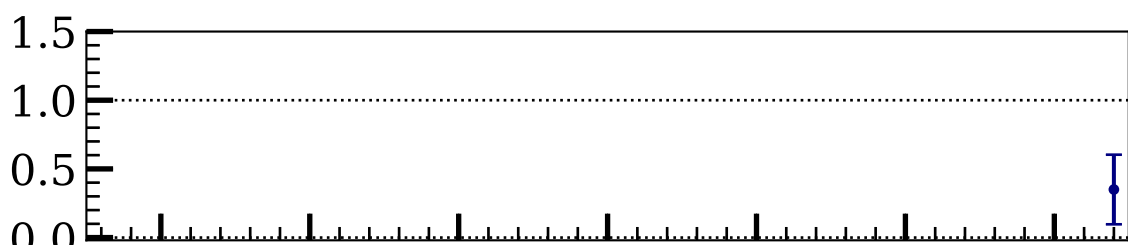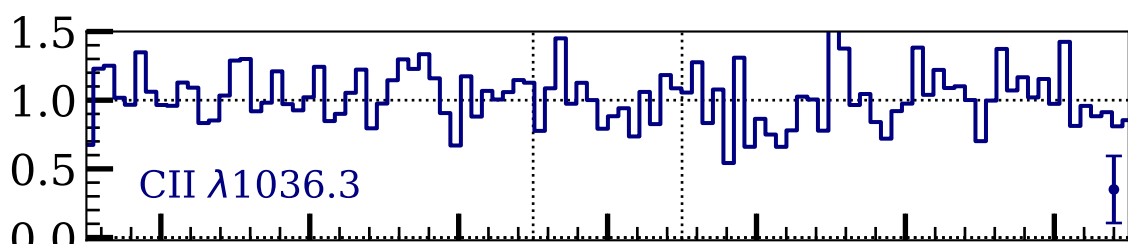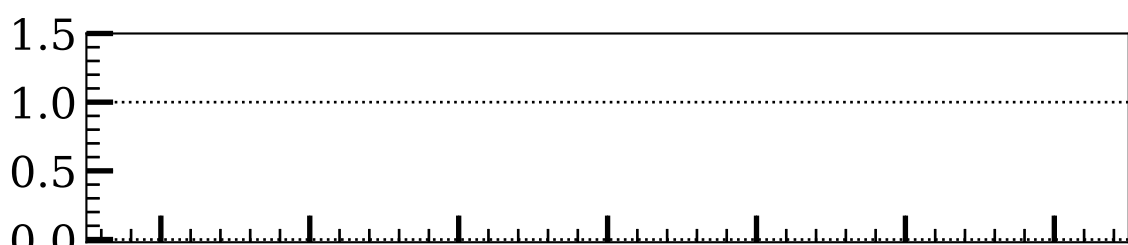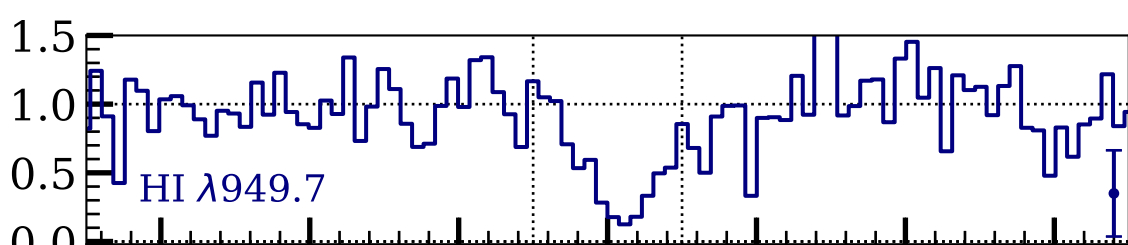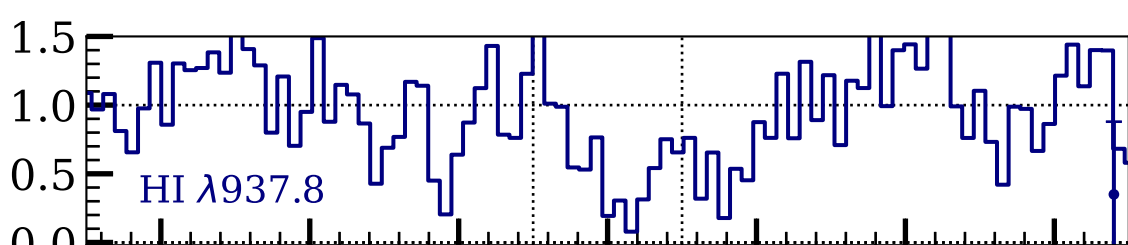

Rest-Frame Velocity ( $\text{km s}^{-1}$ )

J094331.61+053131.4,  $z=0.354599$ , RF=0

Normalized Flux

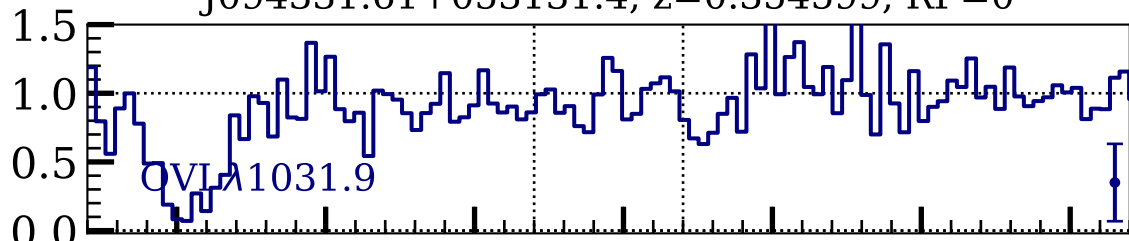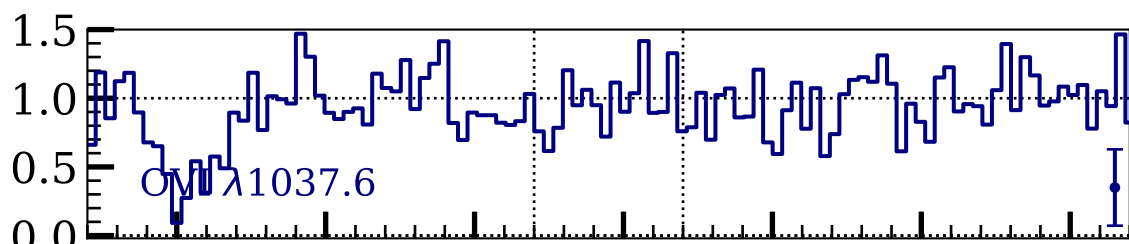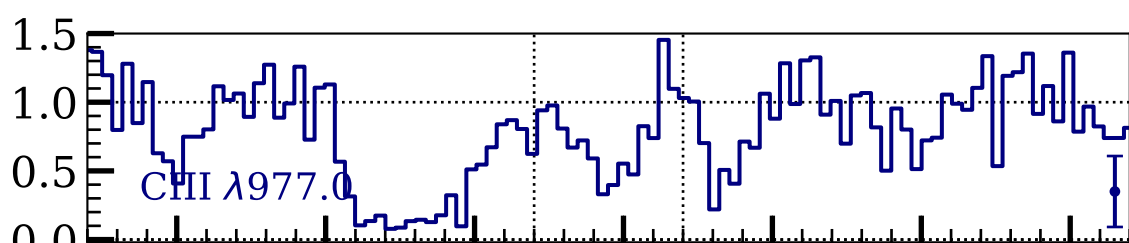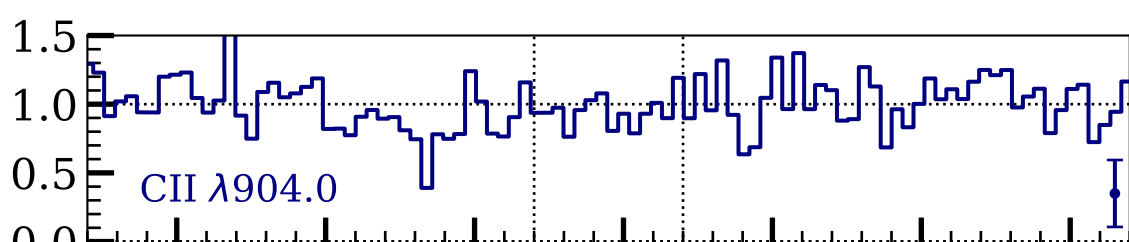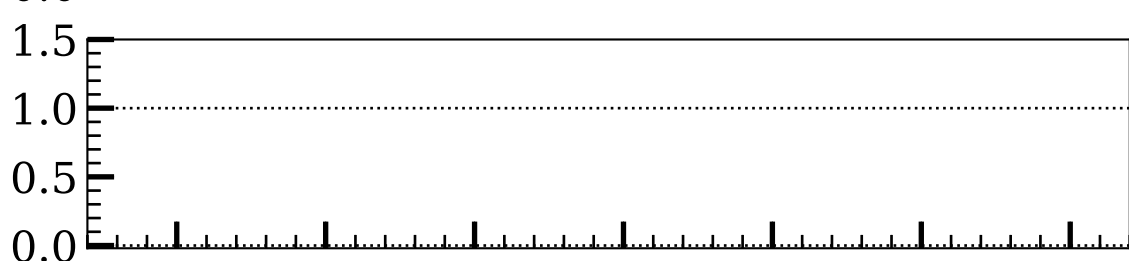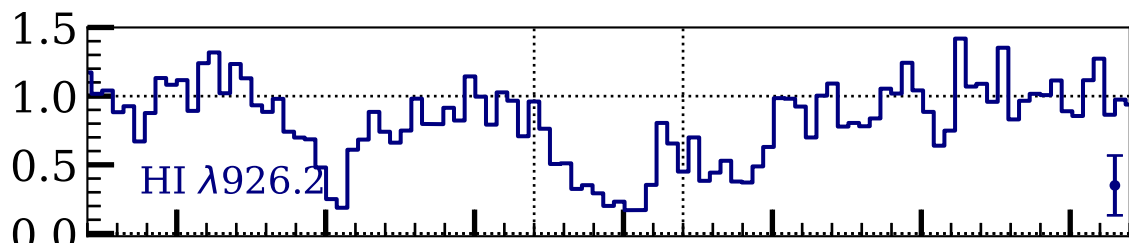

Rest-Frame Velocity ( $\text{km s}^{-1}$ )

J094331.61+053131.4,  $z=0.354927$ , RF=0

Normalized Flux

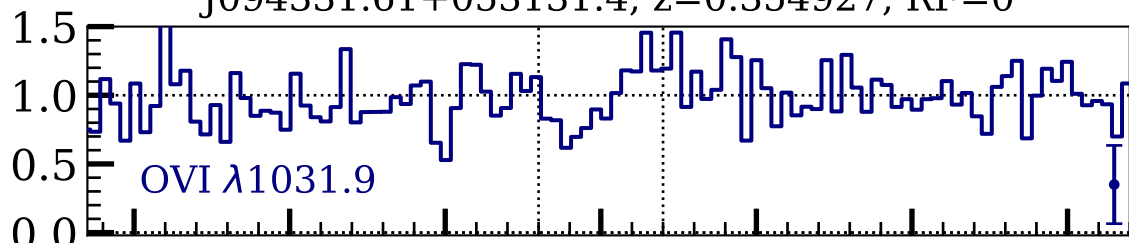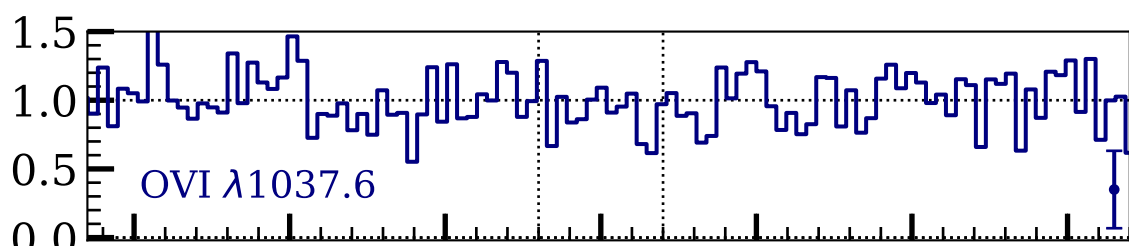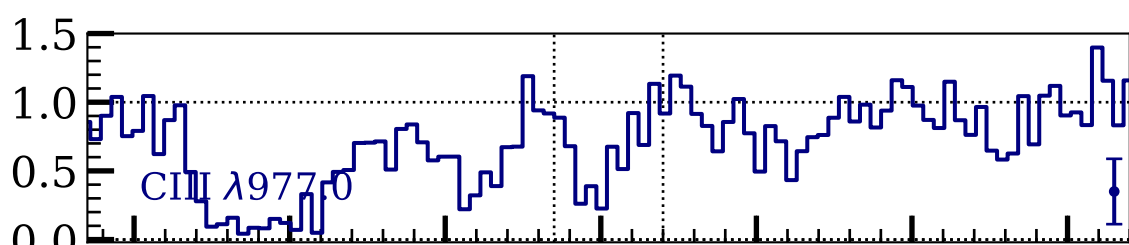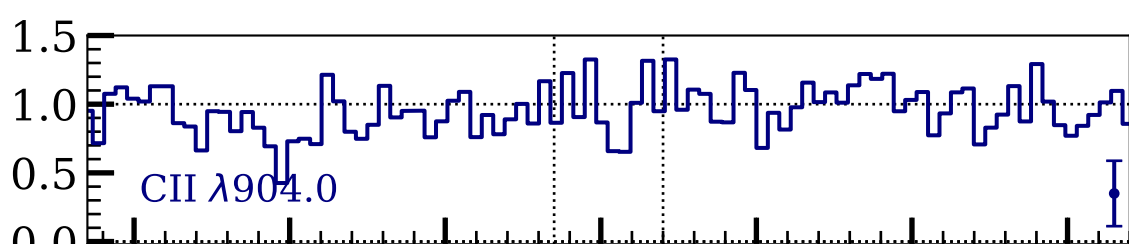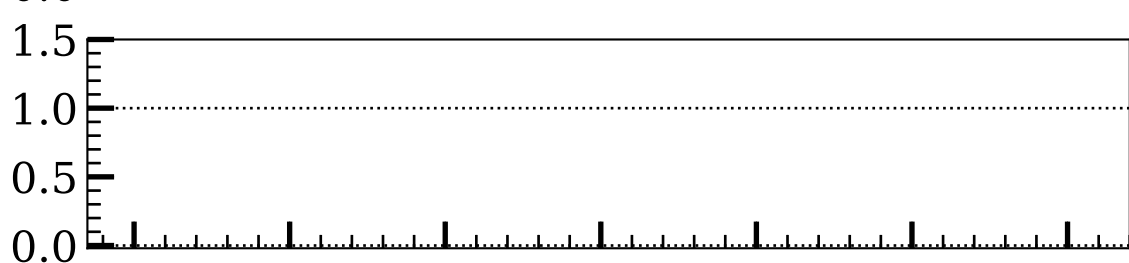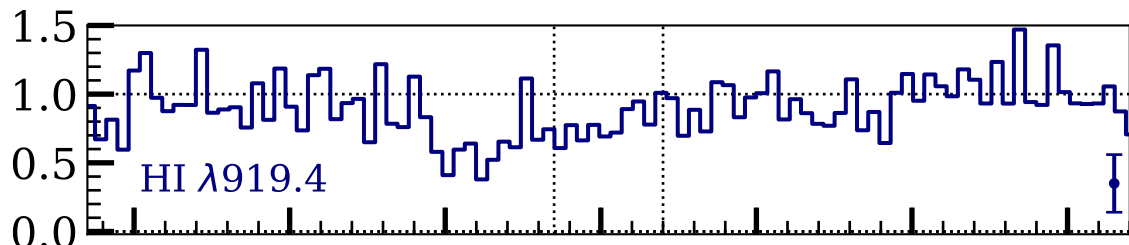

Rest-Frame Velocity ( $\text{km s}^{-1}$ )

J100102.64+594414.2,  $z=0.415649$ , RF=1

Normalized Flux

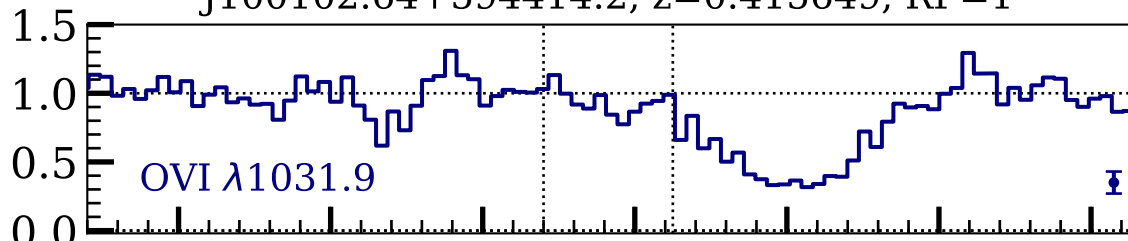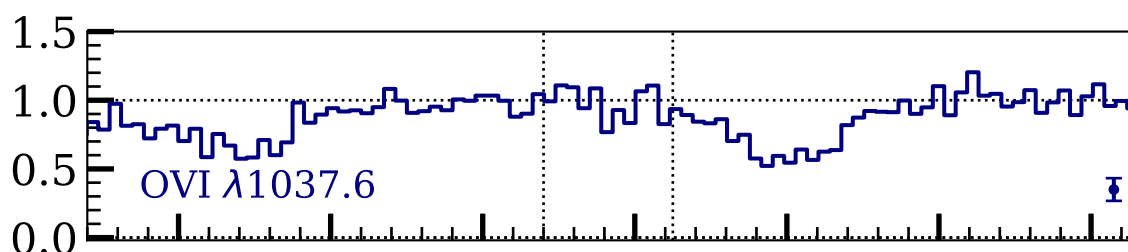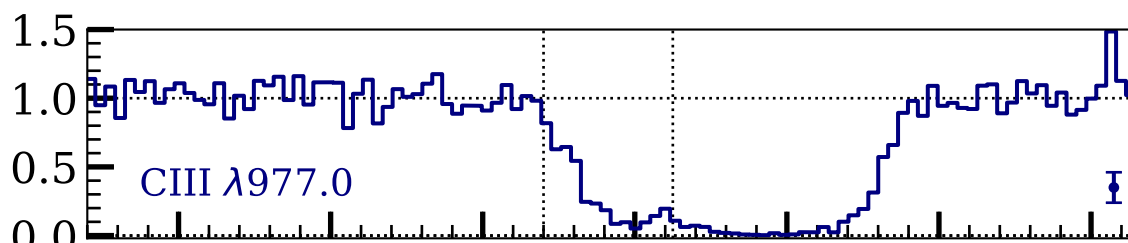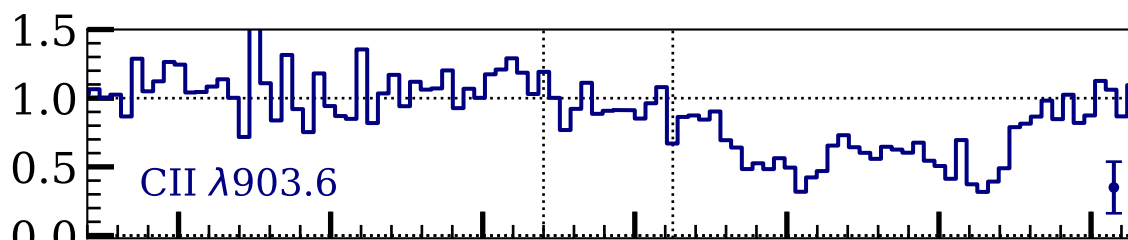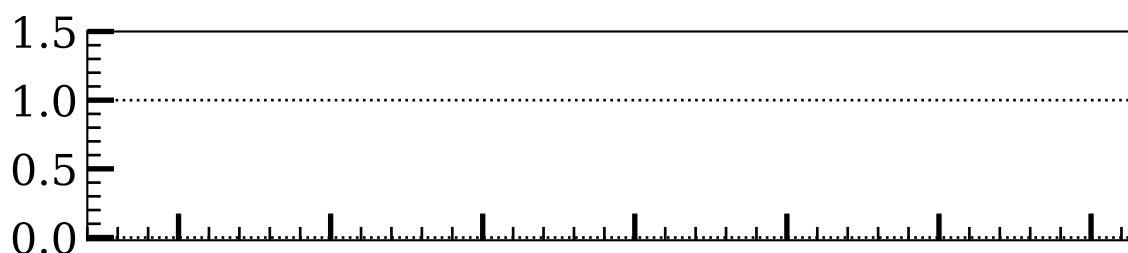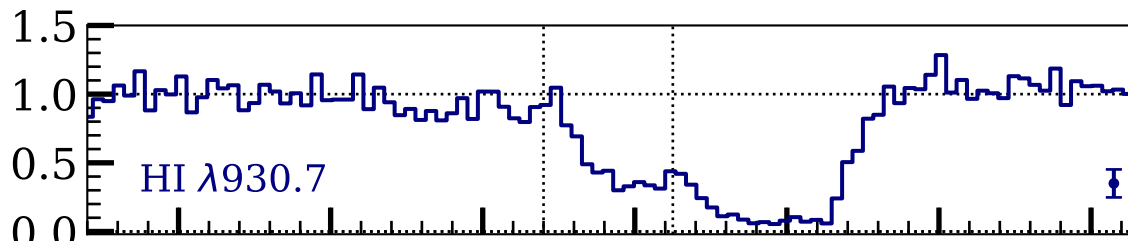

Rest-Frame Velocity ( $\text{km s}^{-1}$ )

J100102.64+594414.2,  $z=0.416042$ , RF=1

Normalized Flux

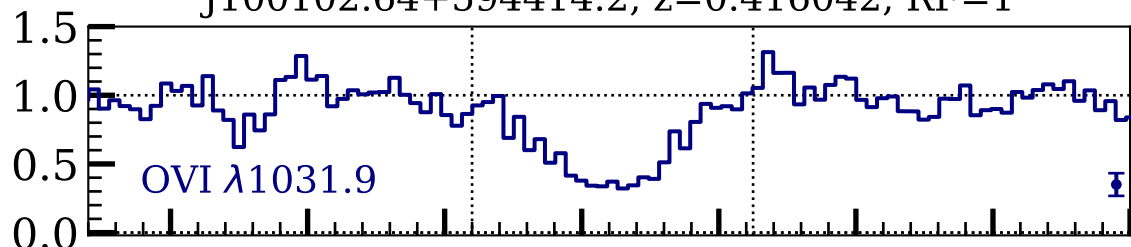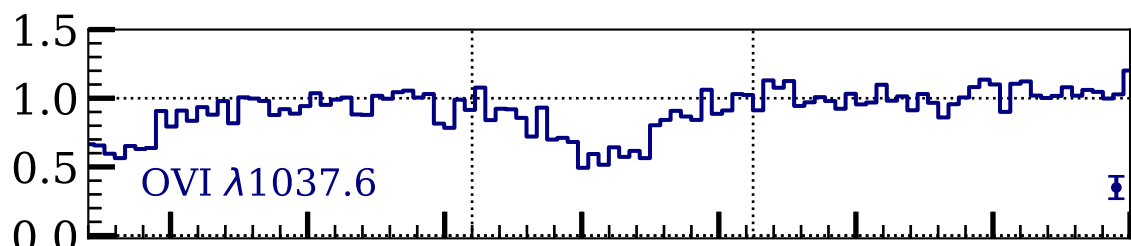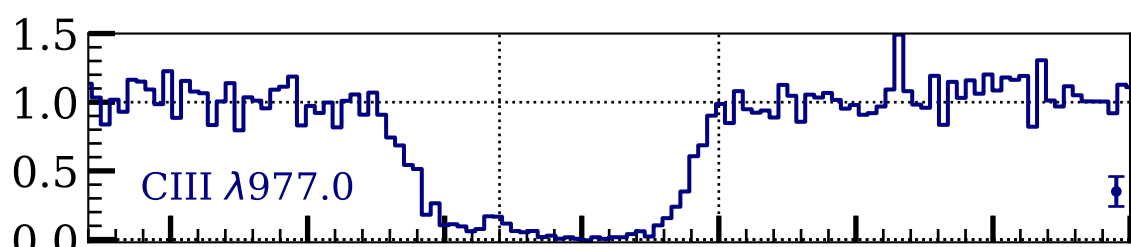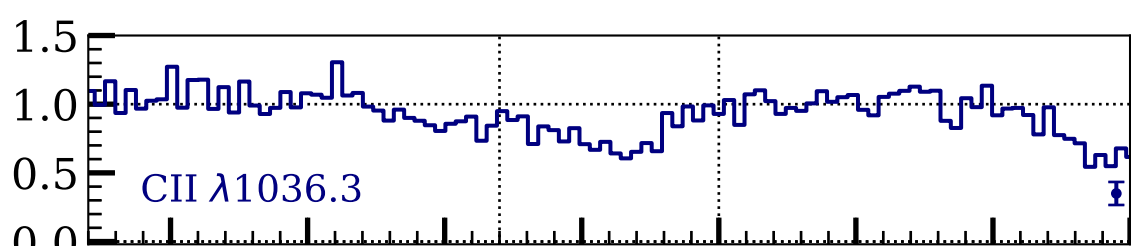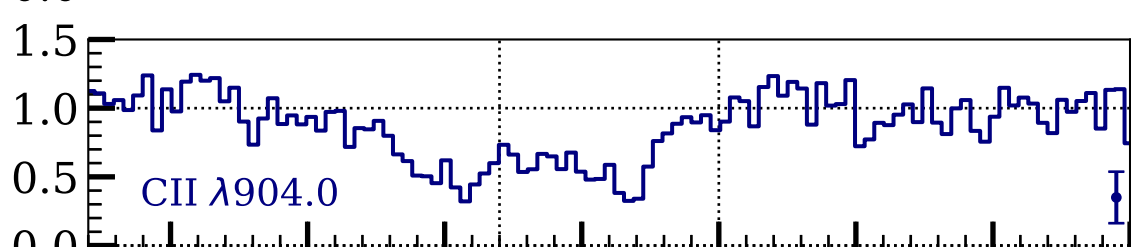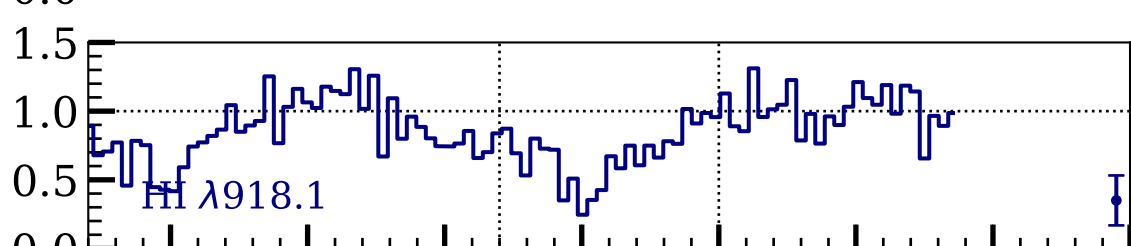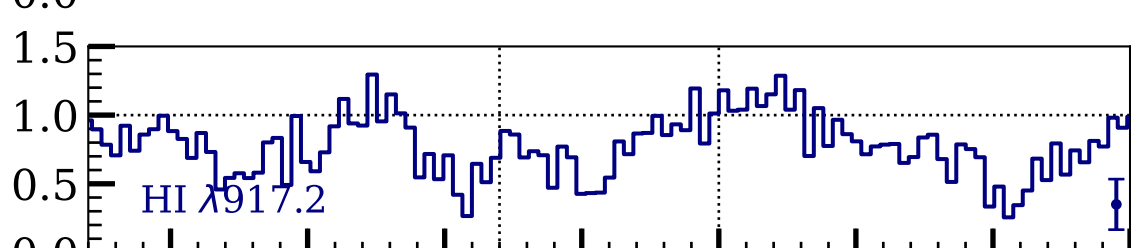

Rest-Frame Velocity ( $\text{km s}^{-1}$ )

J100110.20+291137.5,  $z=0.556468$ , RF=0

Normalized Flux

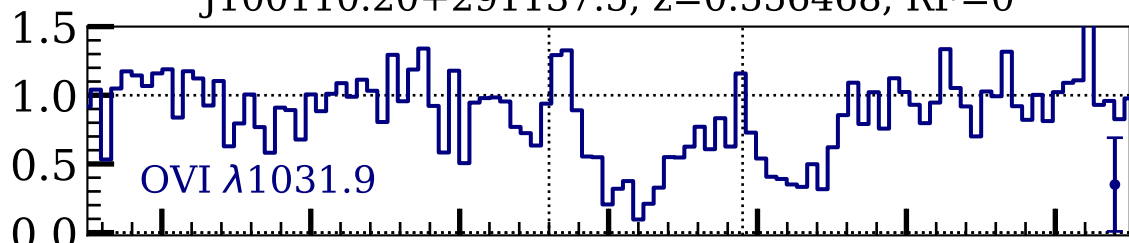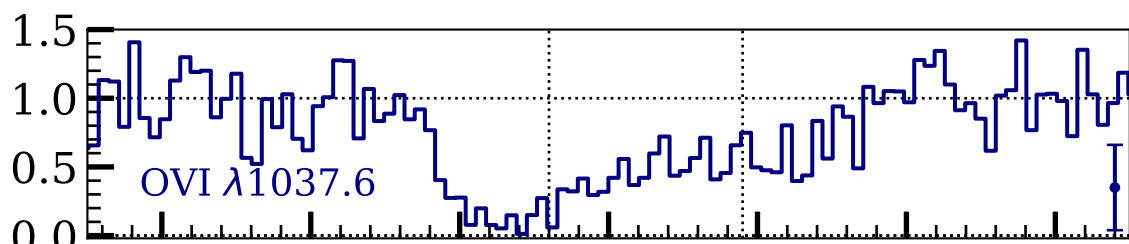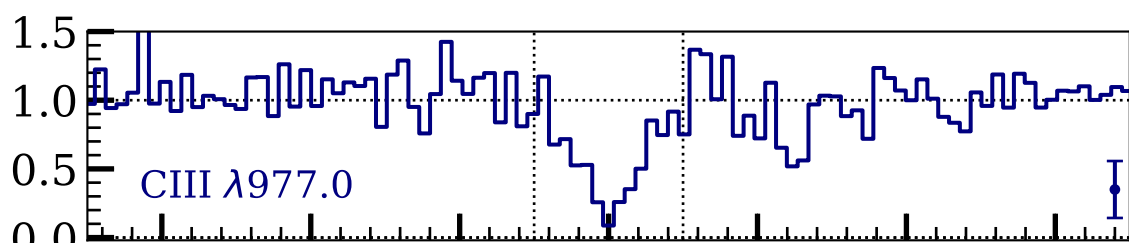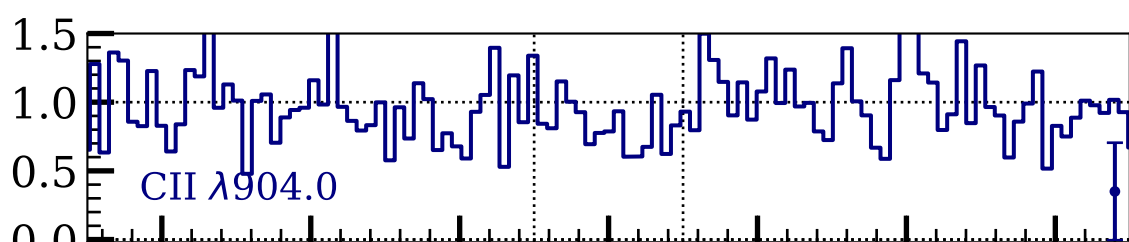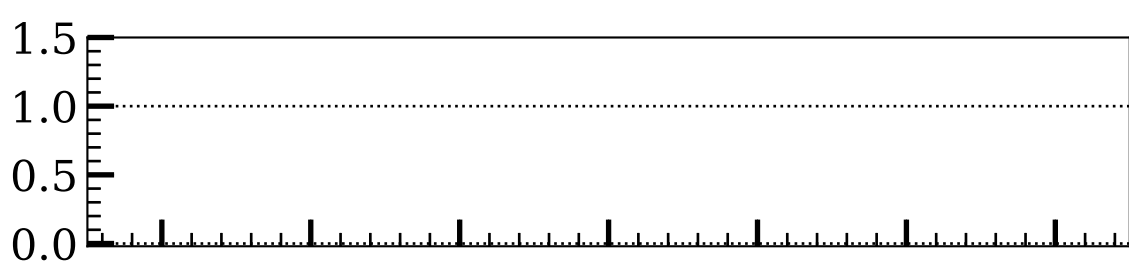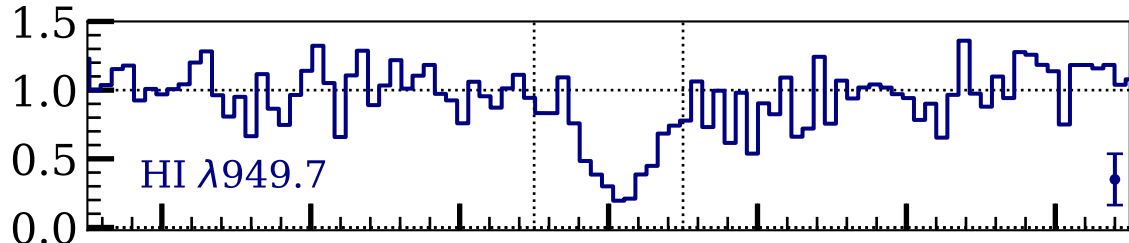

Rest-Frame Velocity ( $\text{km s}^{-1}$ )



J100535.25+013445.5,  $z=0.418522$ , RF=1

Normalized Flux

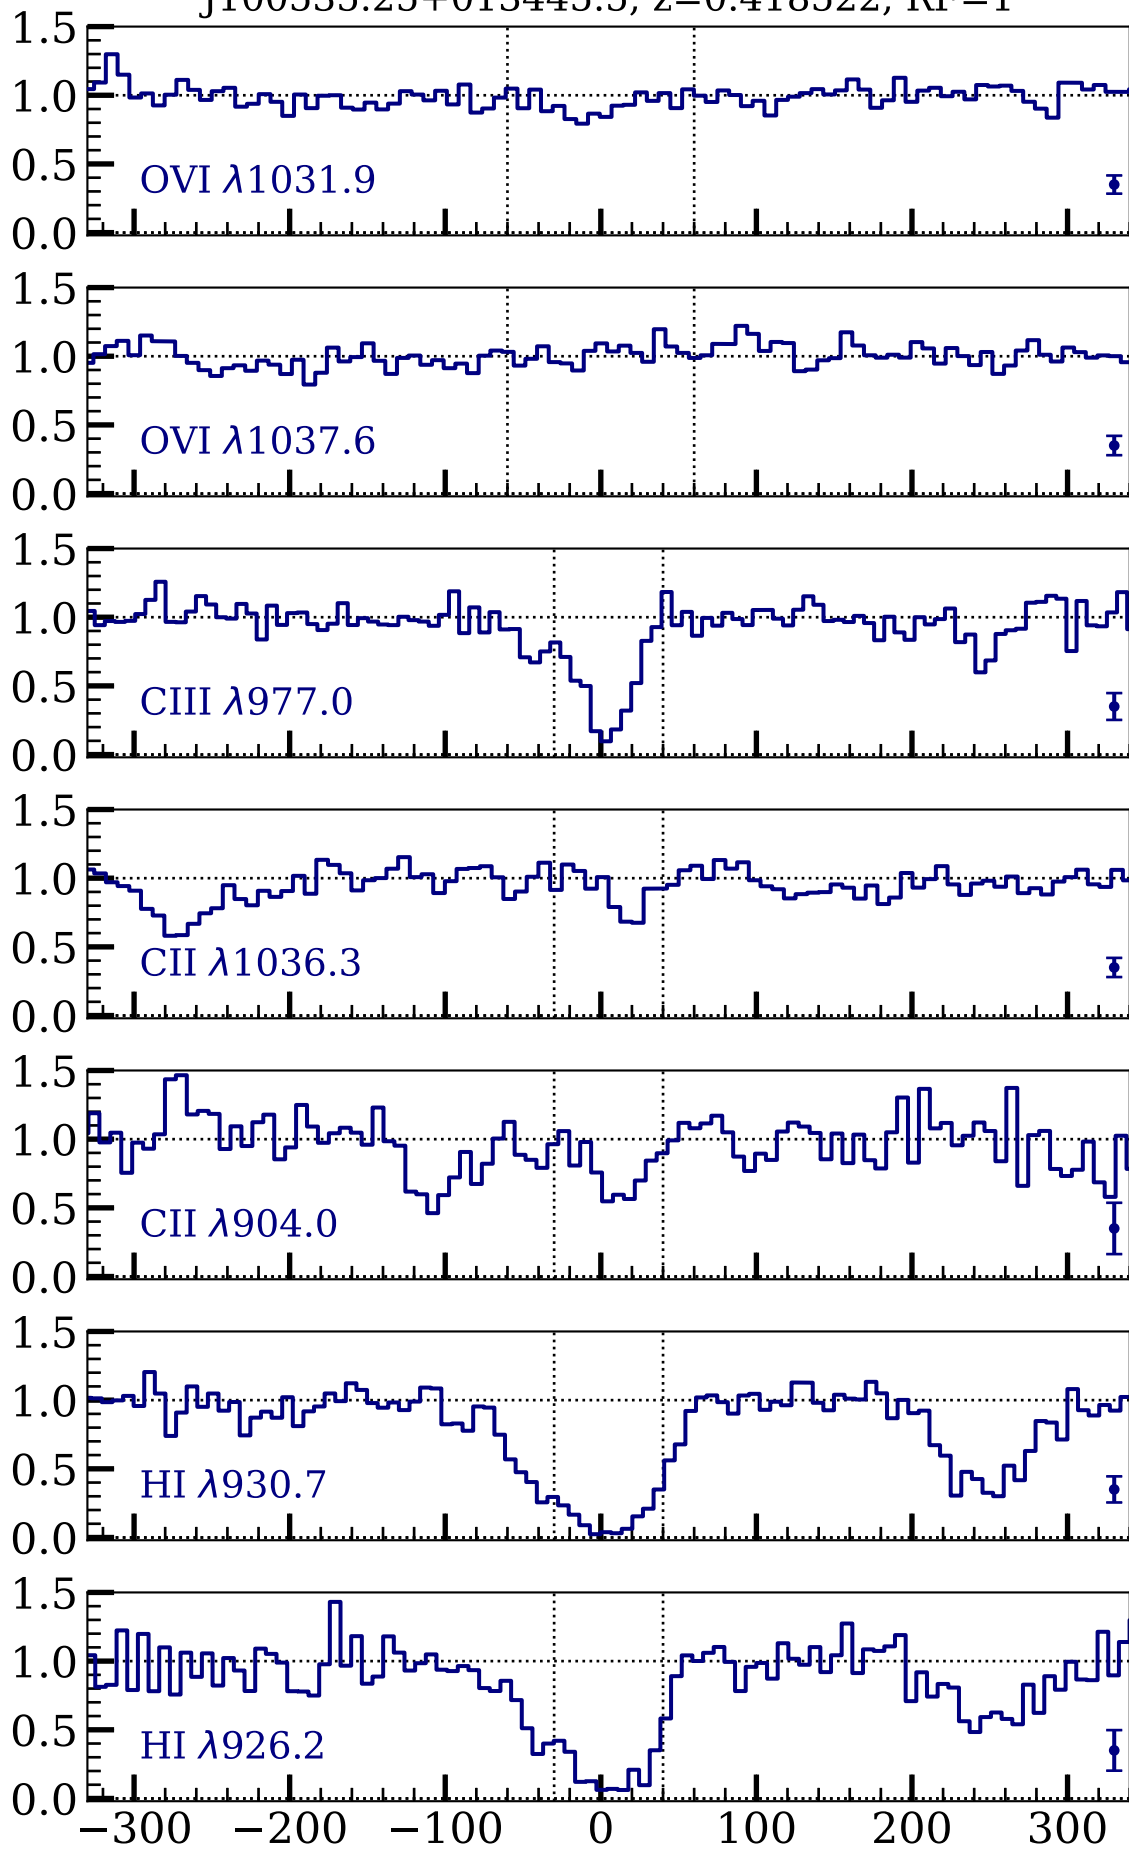

J100535.25+013445.5,  $z=0.419686$ , RF=1

Normalized Flux

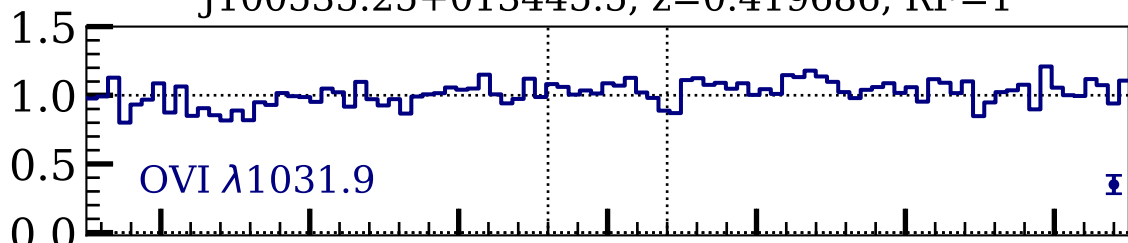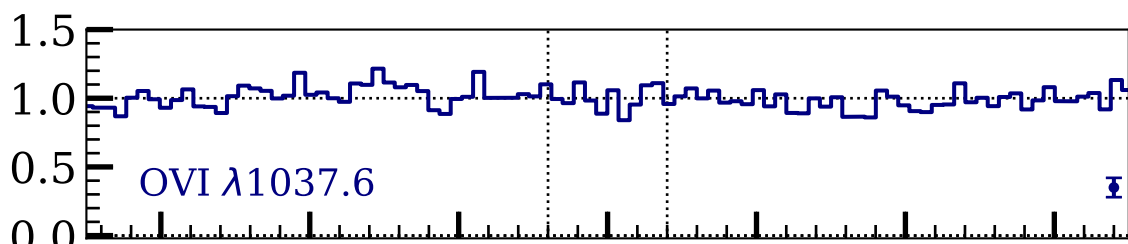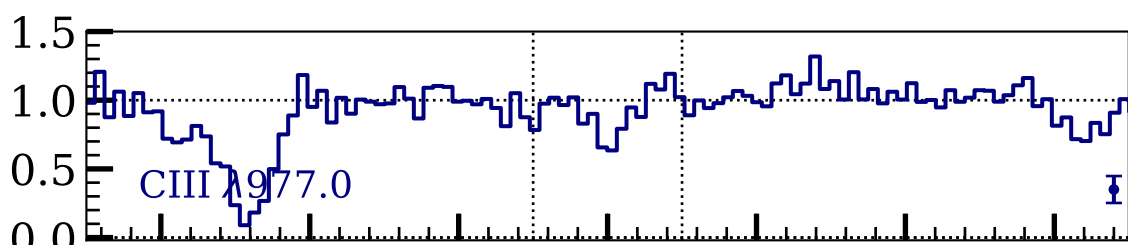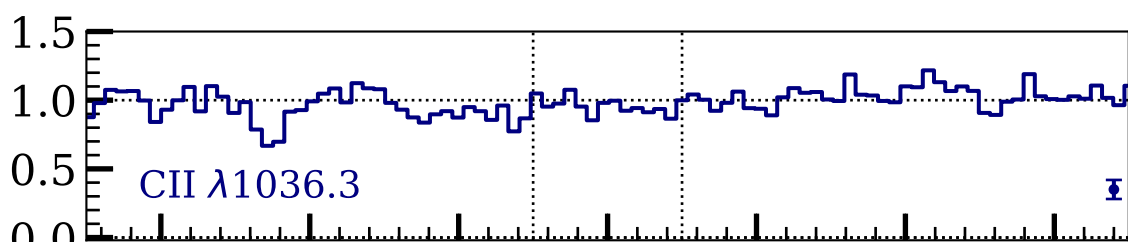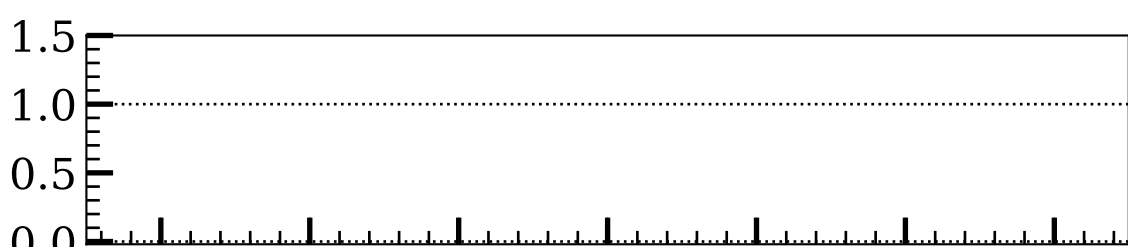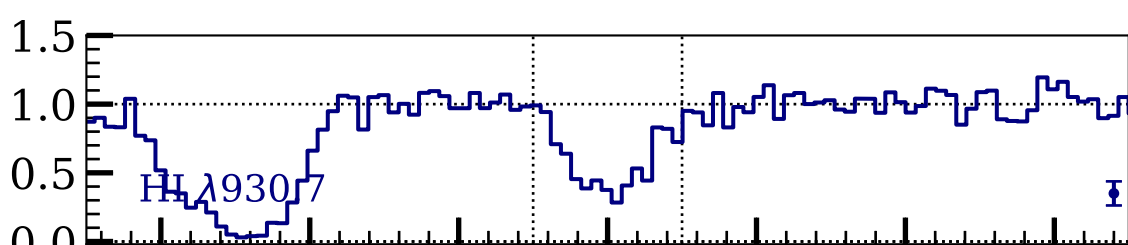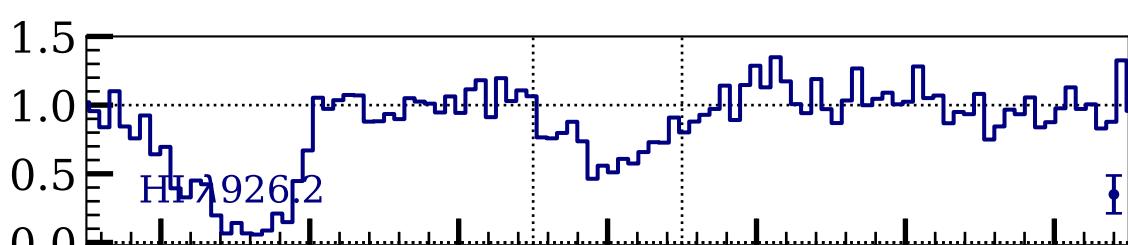

Rest-Frame Velocity ( $\text{km s}^{-1}$ )

J100902.06+071343.8,  $z=0.337193$ , RF=1

Normalized Flux

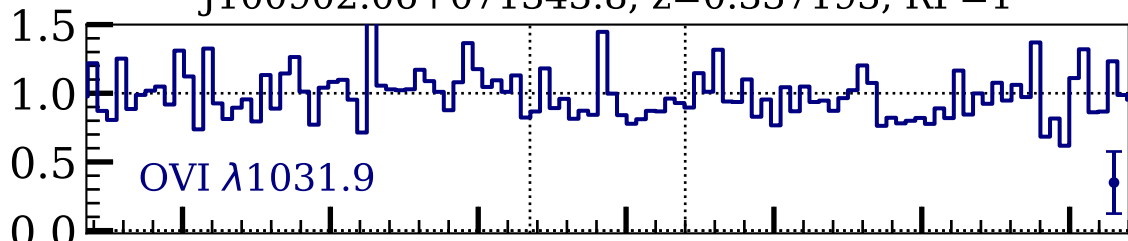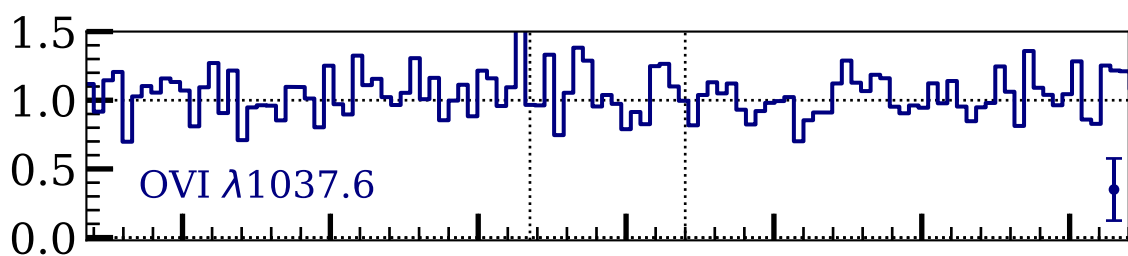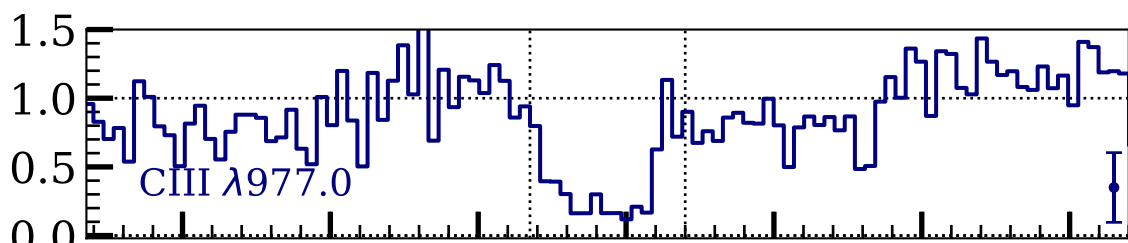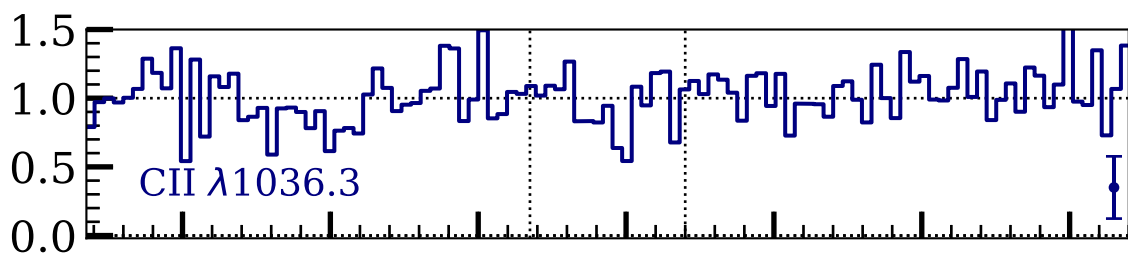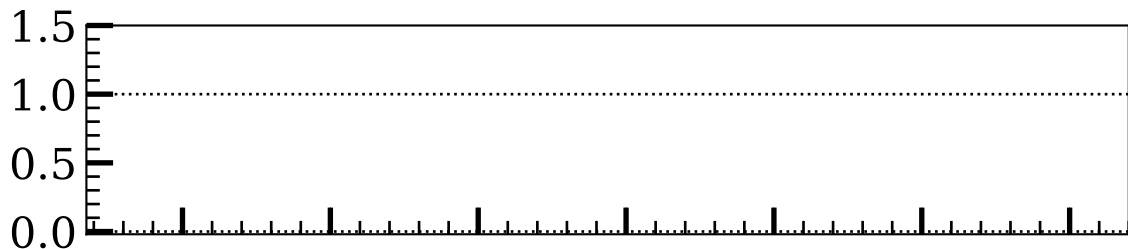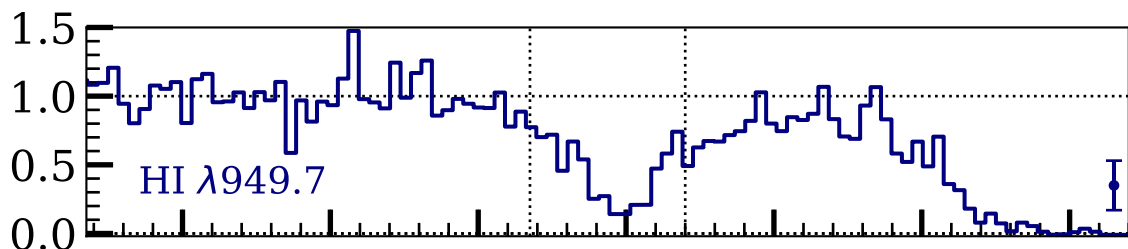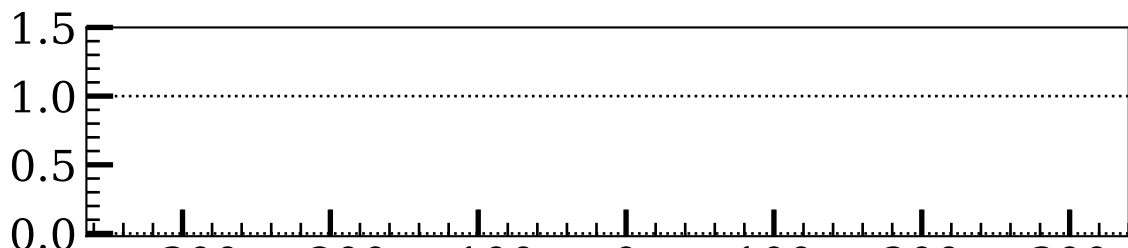

Rest-Frame Velocity (km s<sup>-1</sup>)

J100902.06+071343.8,  $z=0.355352$ , RF=0

Normalized Flux

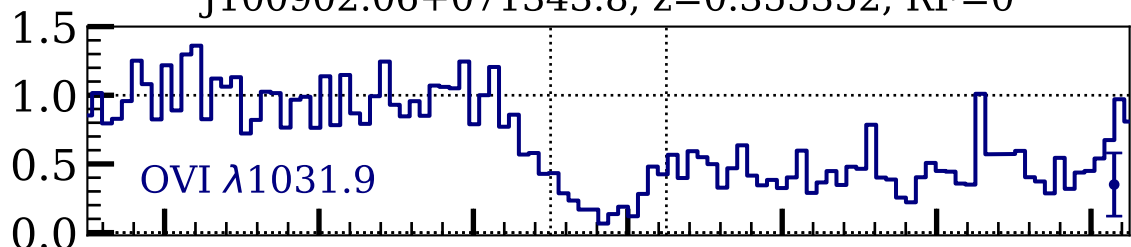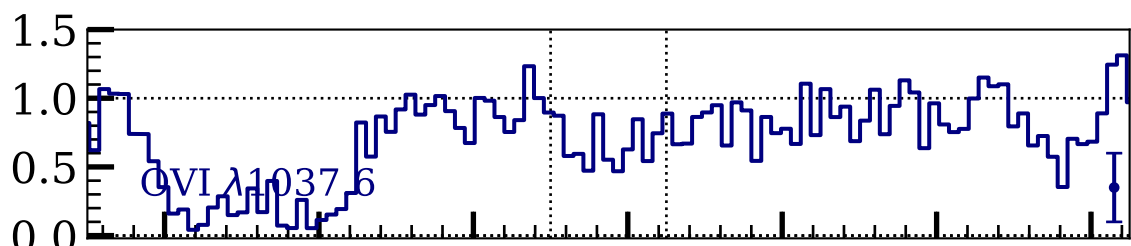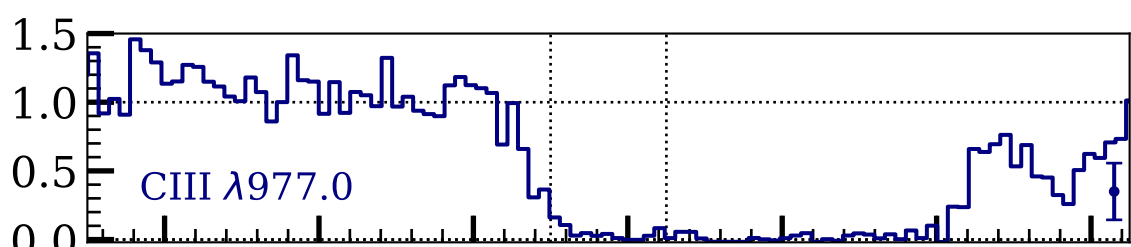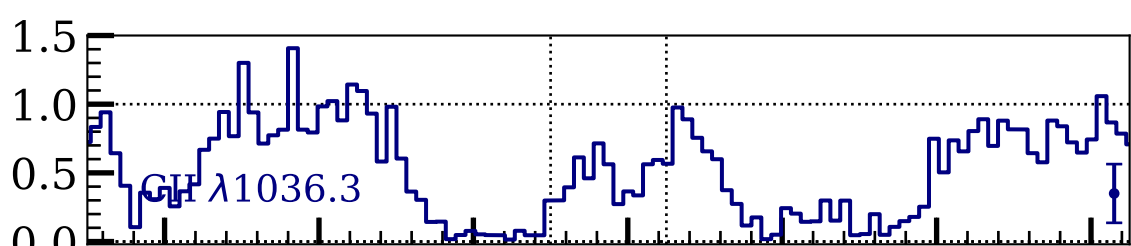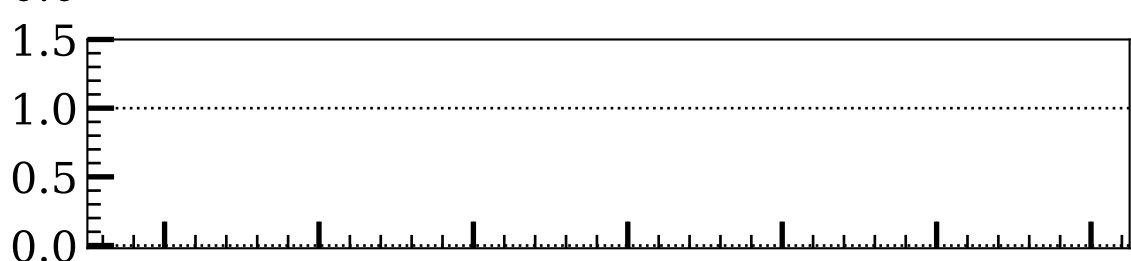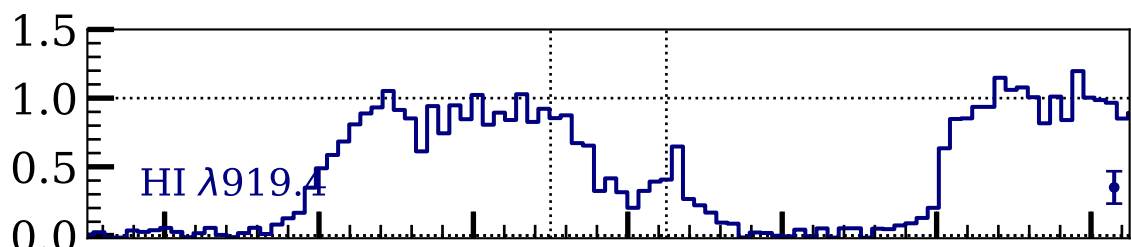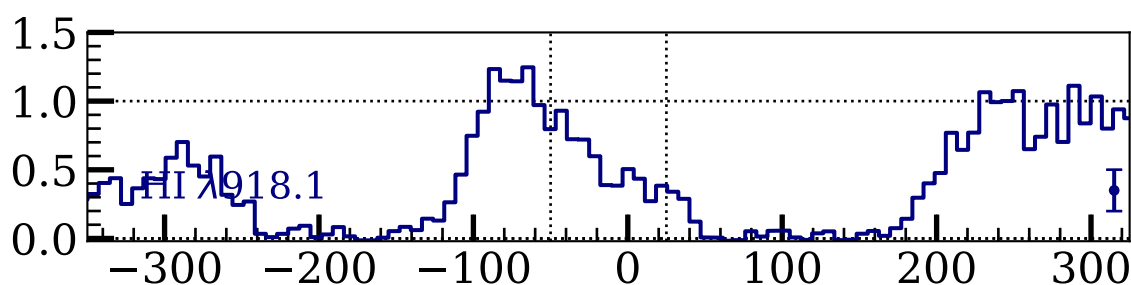

Rest-Frame Velocity ( $\text{km s}^{-1}$ )

J101622.60+470643.3,  $z=0.263820$ , RF=0

Normalized Flux

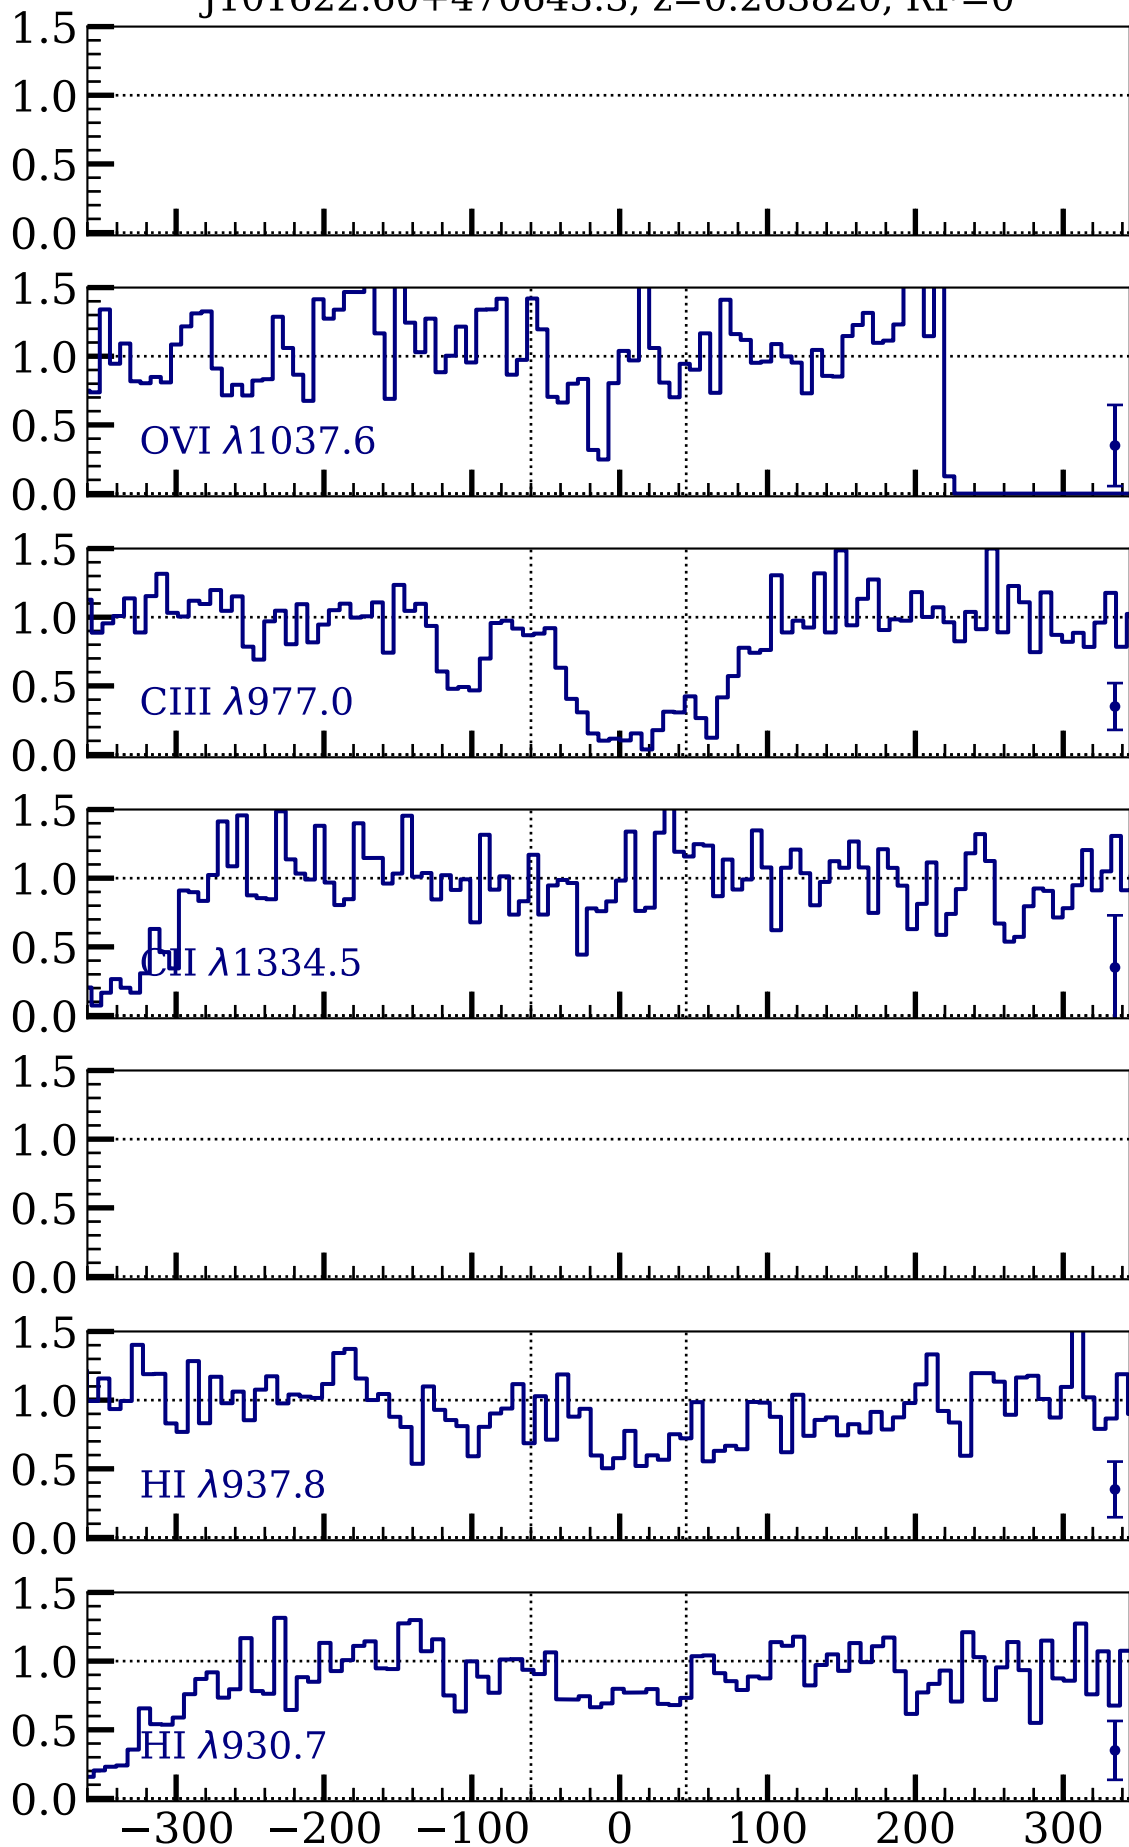

Rest-Frame Velocity (km s<sup>-1</sup>)

J101622.60+470643.3,  $z=0.432210$ , RF=1

Normalized Flux

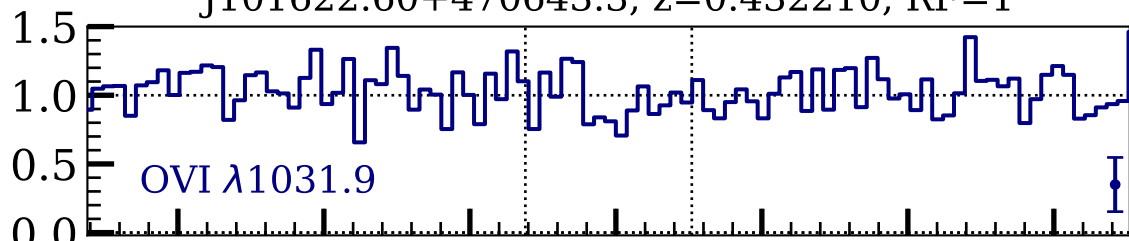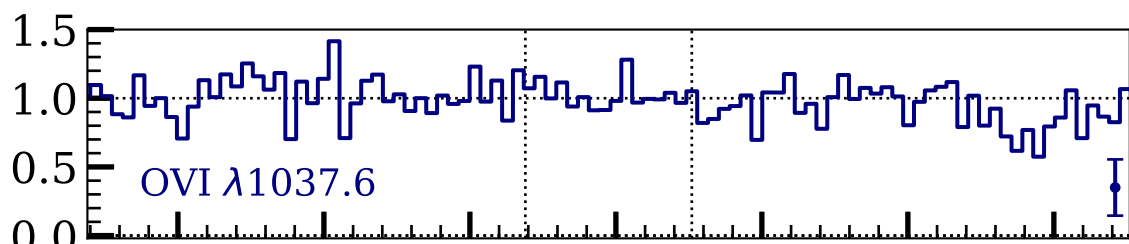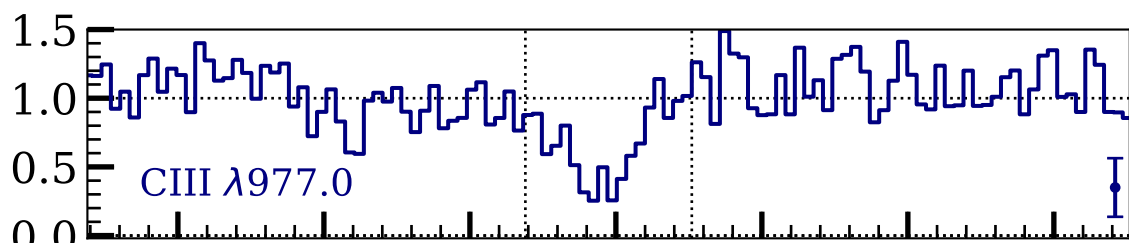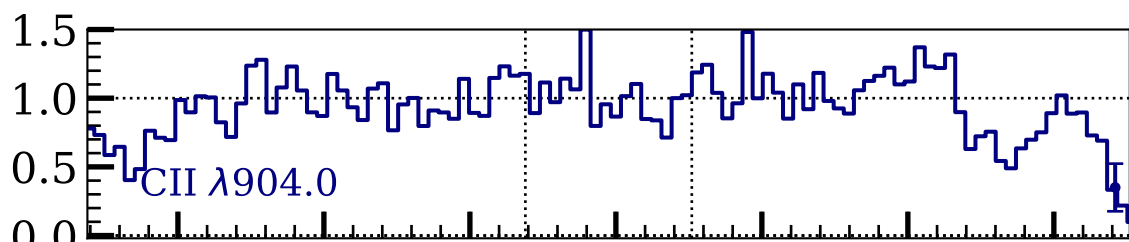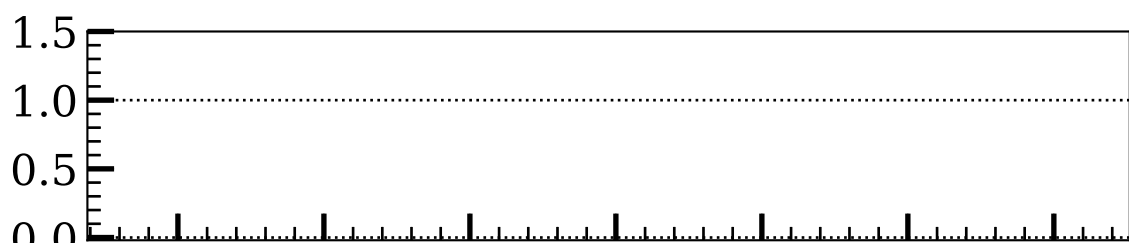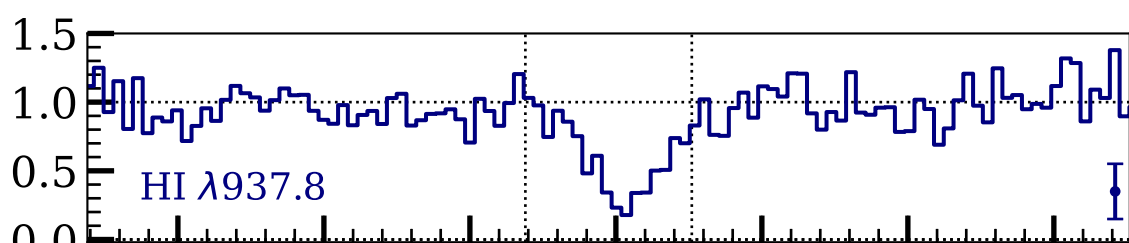

Rest-Frame Velocity ( $\text{km s}^{-1}$ )

J101622.60+470643.3,  $z=0.664722$ , RF=0

Normalized Flux

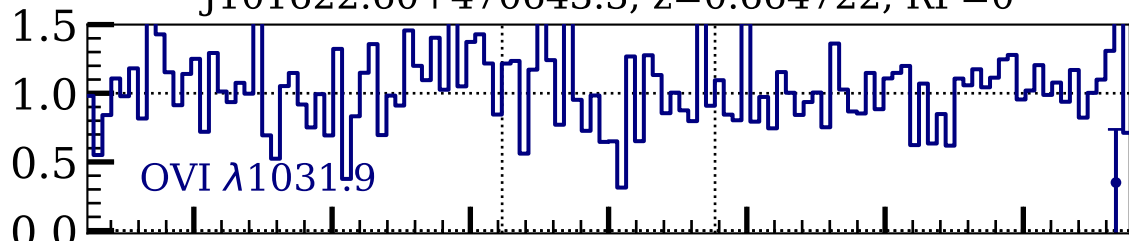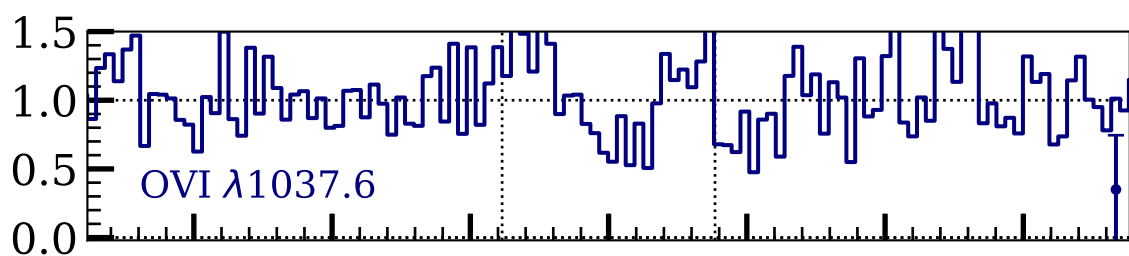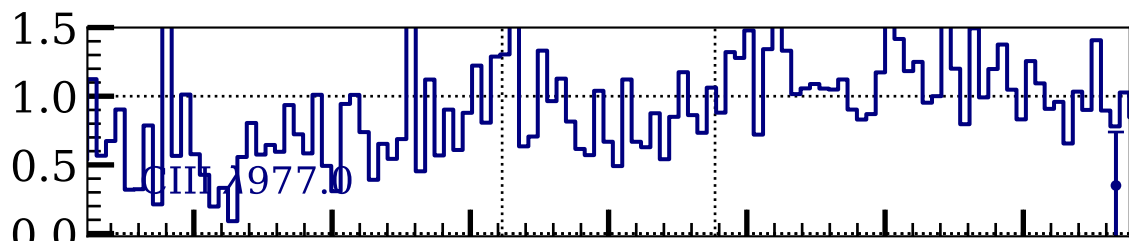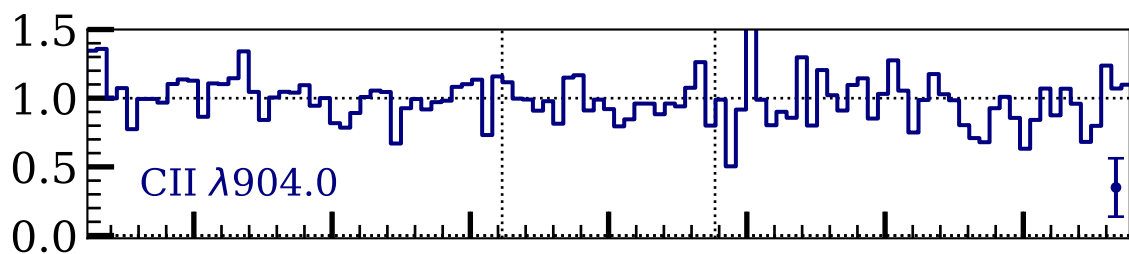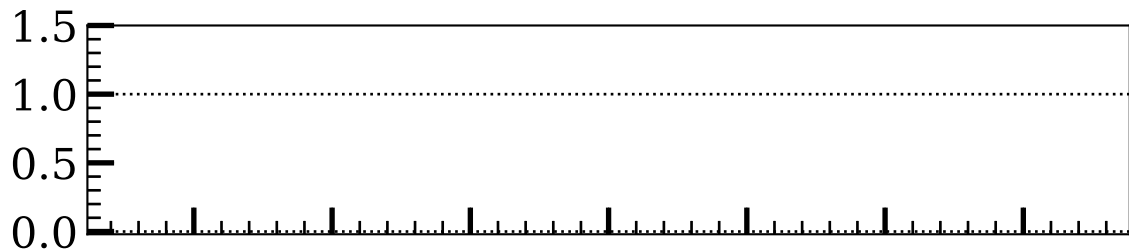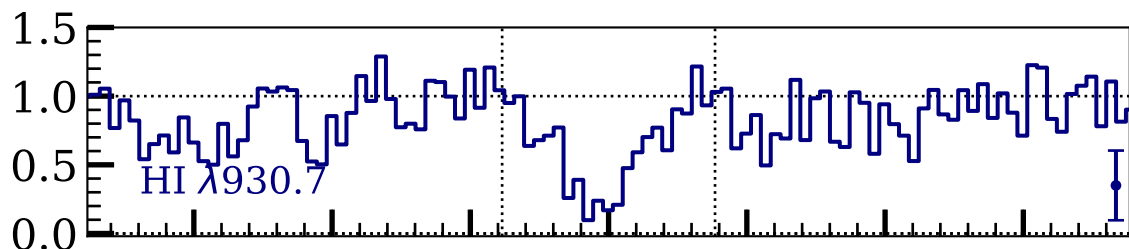

Rest-Frame Velocity ( $\text{km s}^{-1}$ )

J101622.60+470643.3,  $z=0.727771$ , RF=0

Normalized Flux

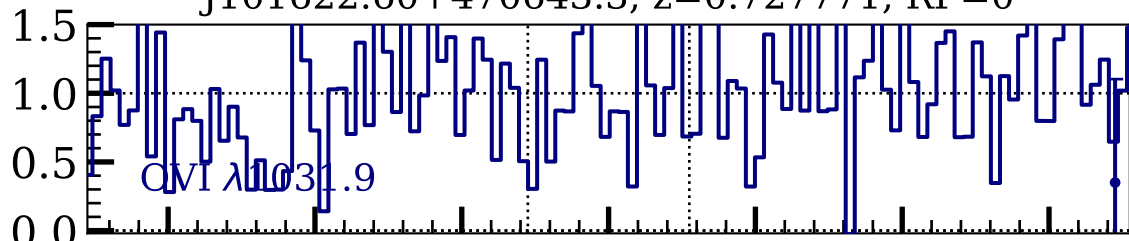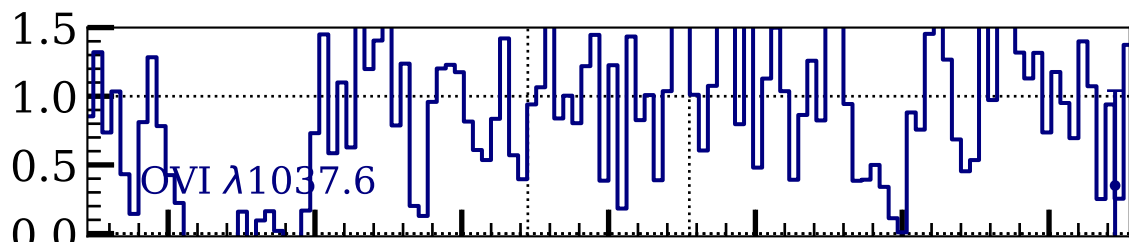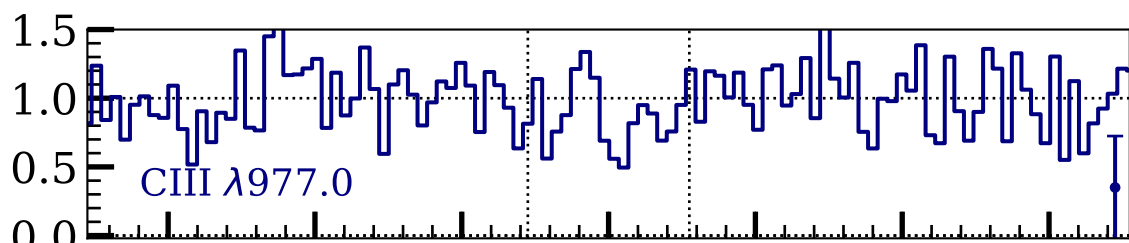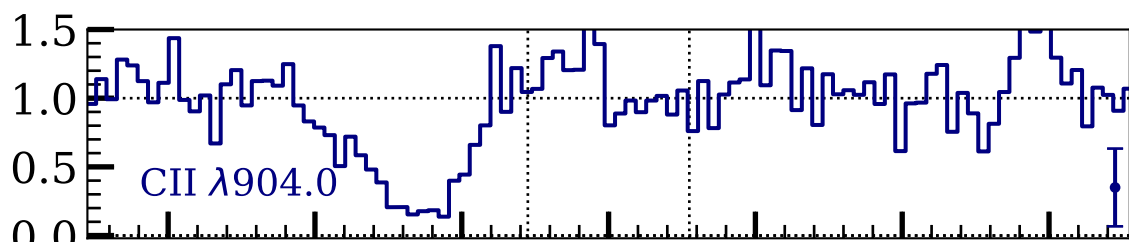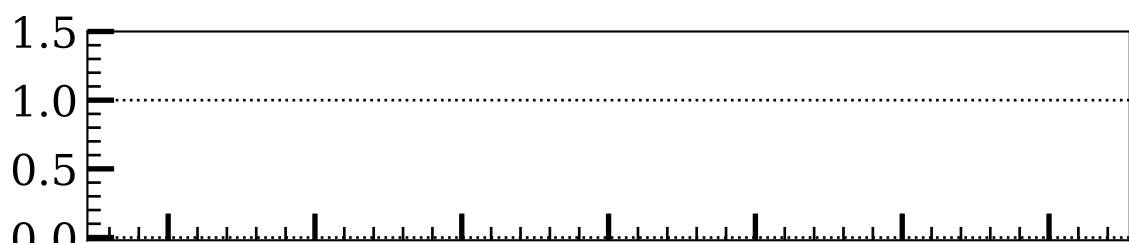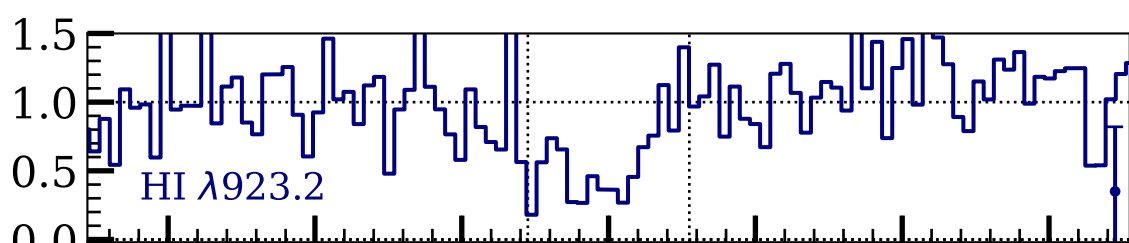

Rest-Frame Velocity ( $\text{km s}^{-1}$ )



J104117.16+061016.9,  $z=0.654403$ , RF=1

Normalized Flux

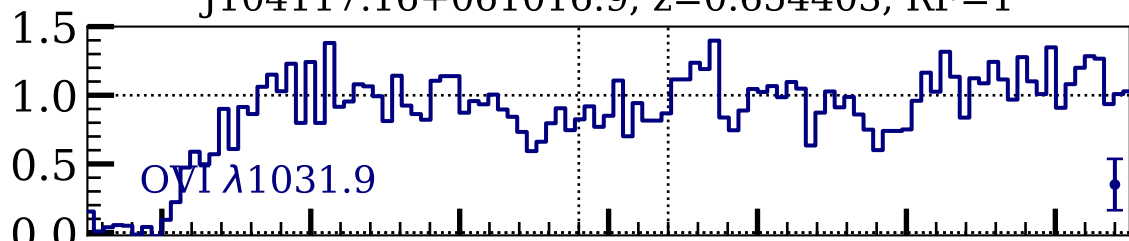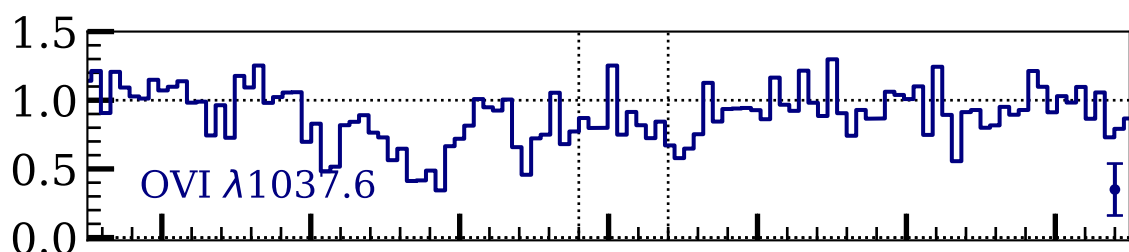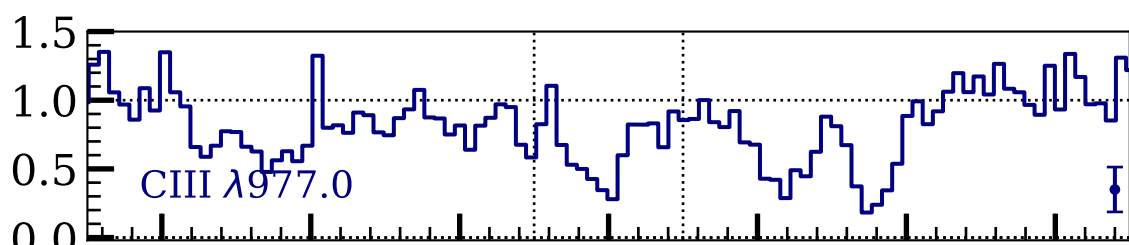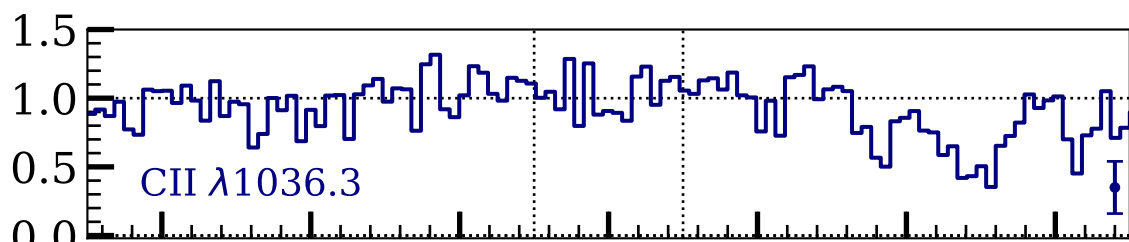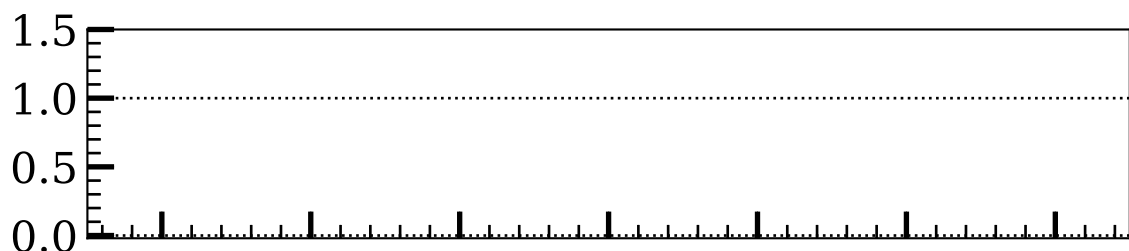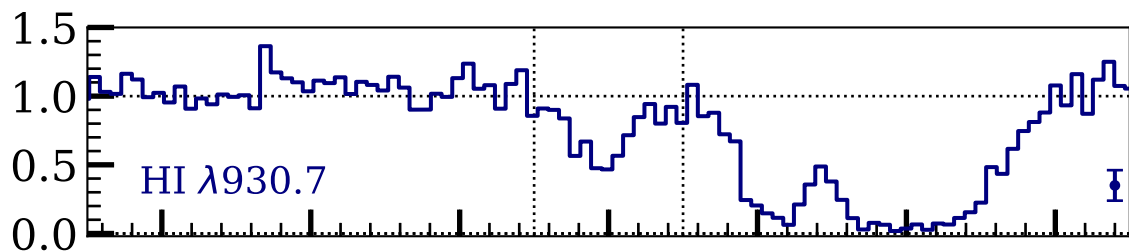

Rest-Frame Velocity ( $\text{km s}^{-1}$ )

J104117.16+061016.9,  $z=0.655059$ , RF=1

Normalized Flux

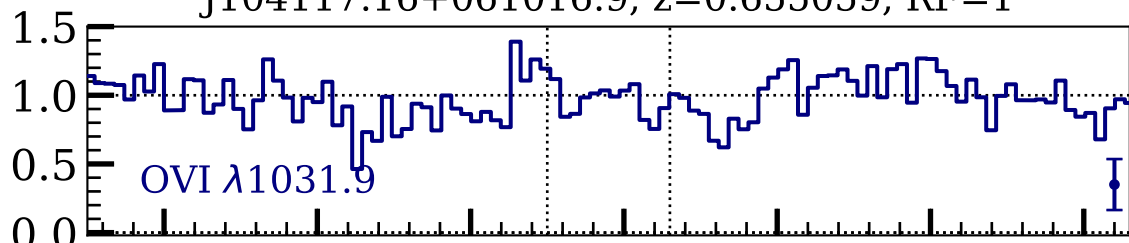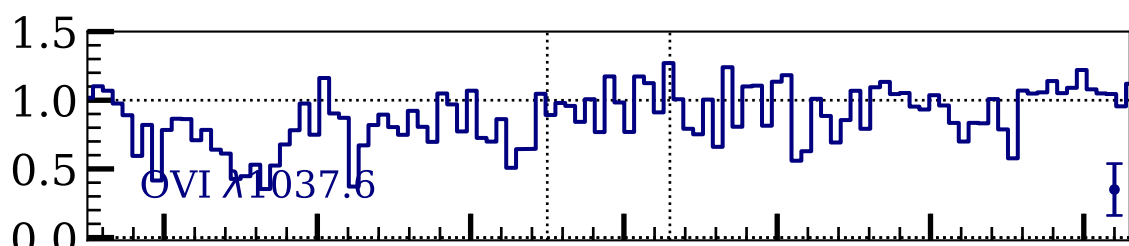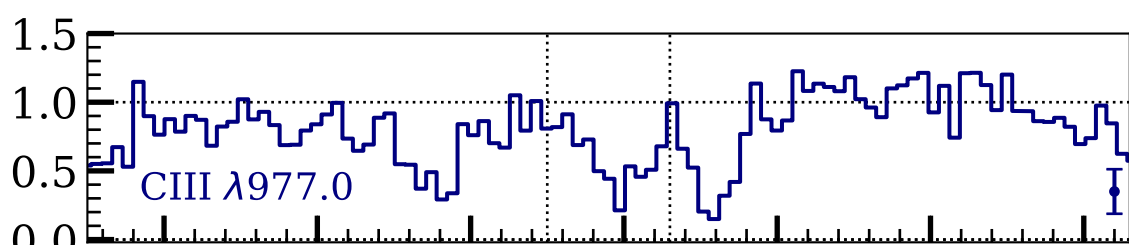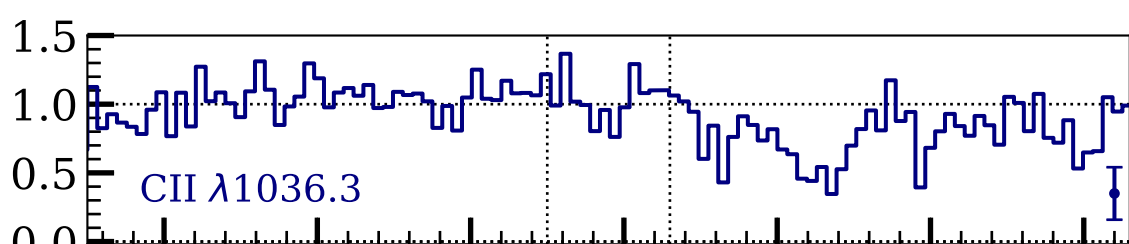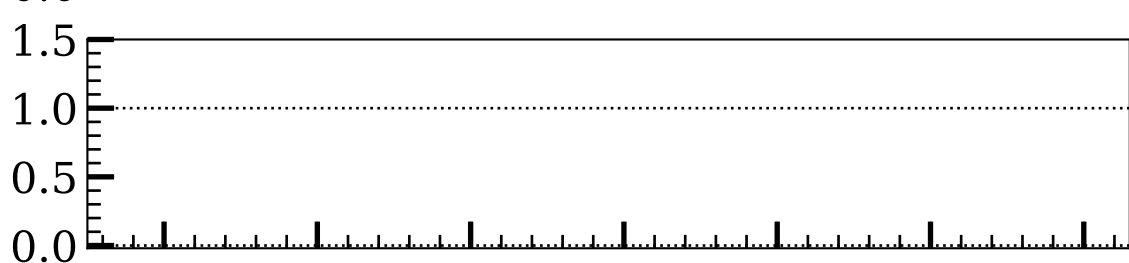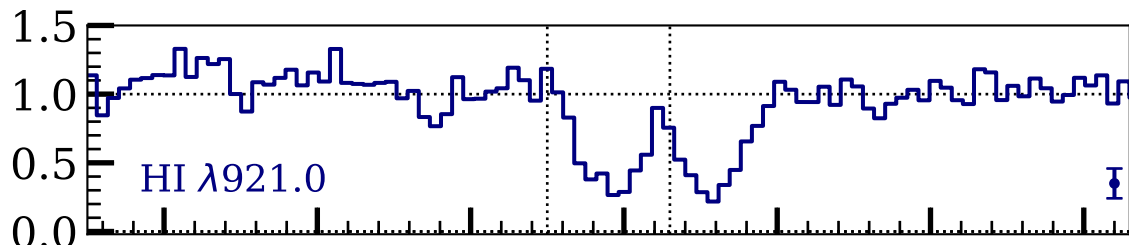

Rest-Frame Velocity ( $\text{km s}^{-1}$ )

J104117.16+061016.9,  $z=0.655390$ , RF=1

Normalized Flux

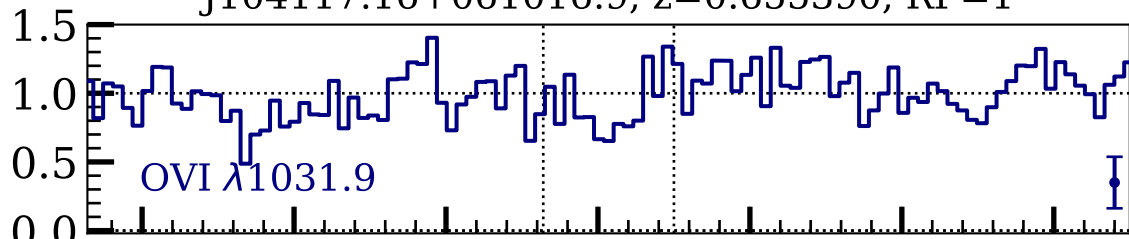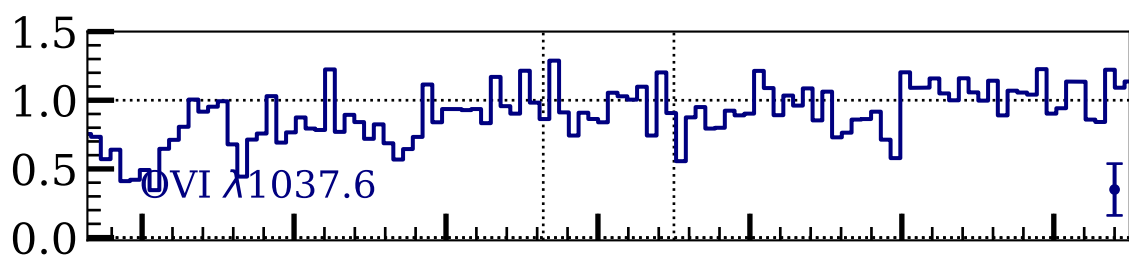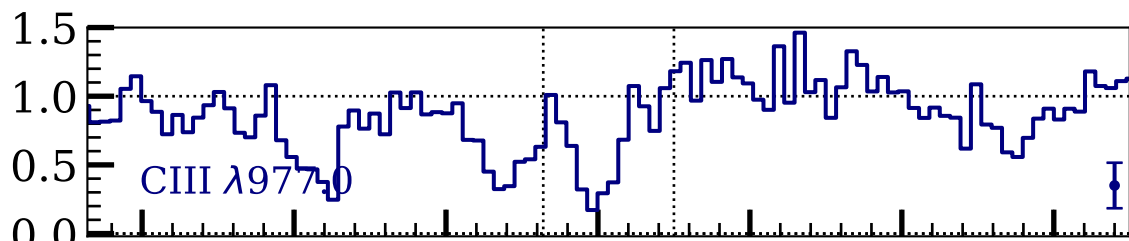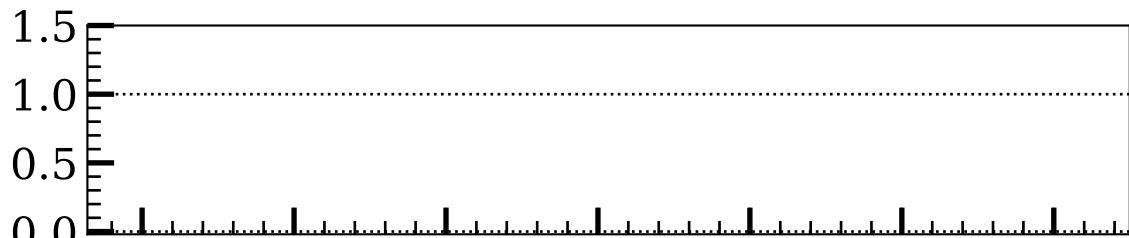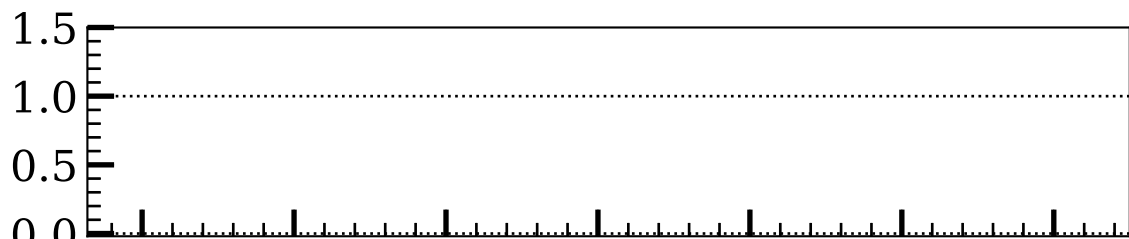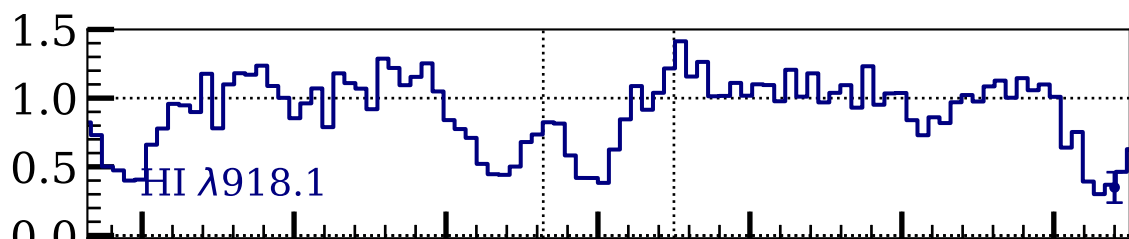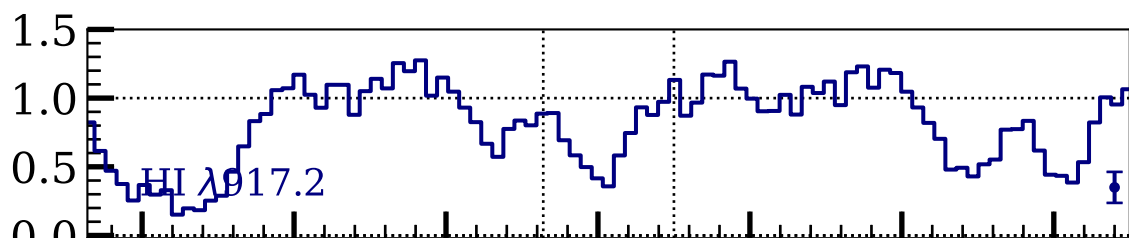

Rest-Frame Velocity (km s<sup>-1</sup>)

J105945.24+144143.0,  $z=0.465822$ , RF=1

Normalized Flux

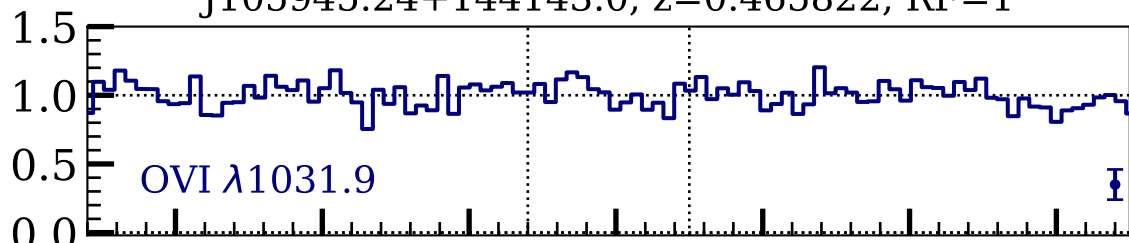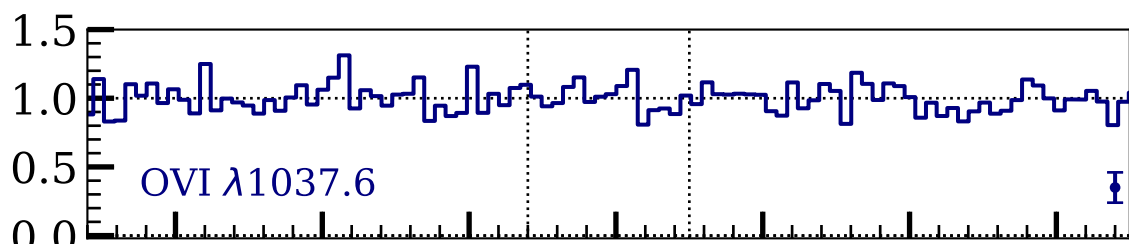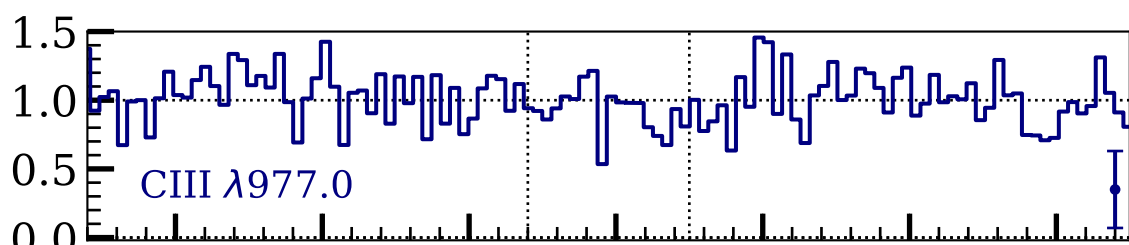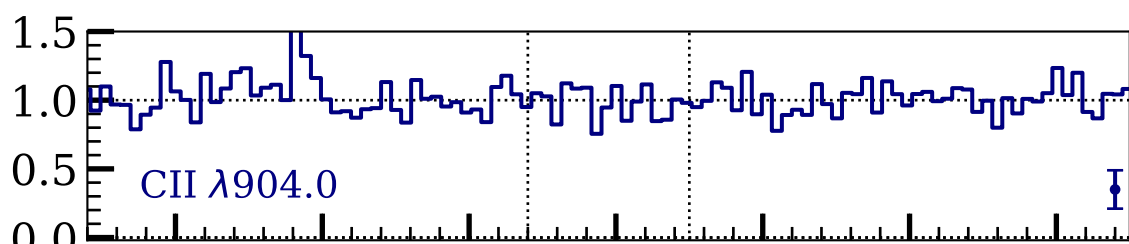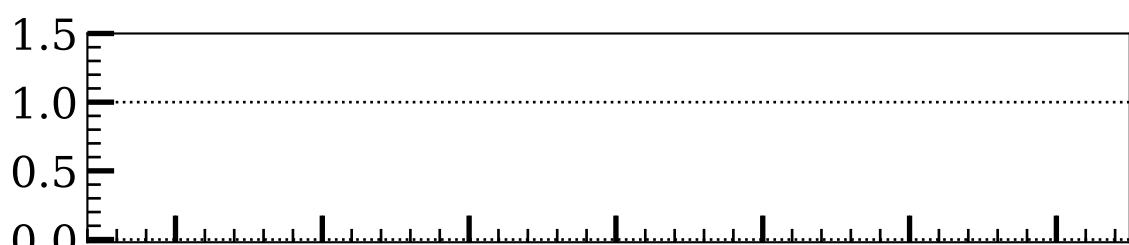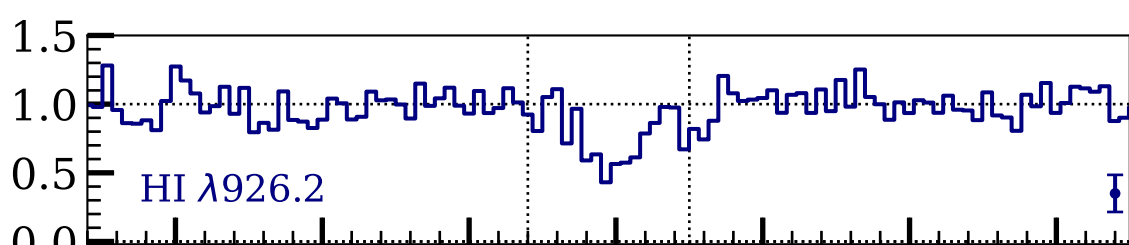

Rest-Frame Velocity ( $\text{km s}^{-1}$ )

J105945.24+144143.0,  $z=0.576490$ , RF=1

Normalized Flux

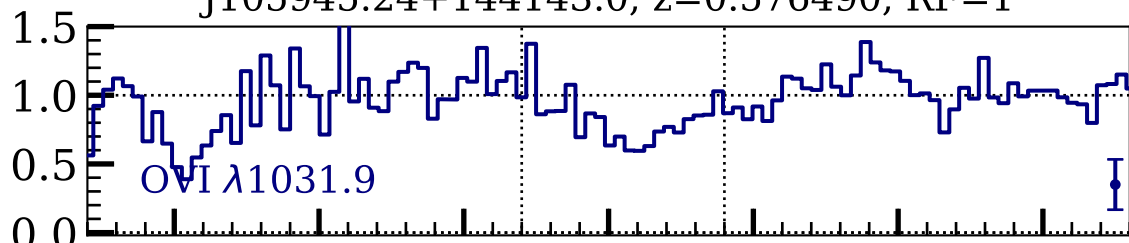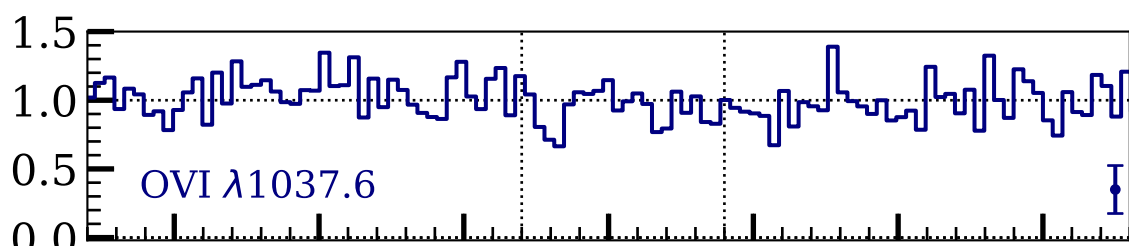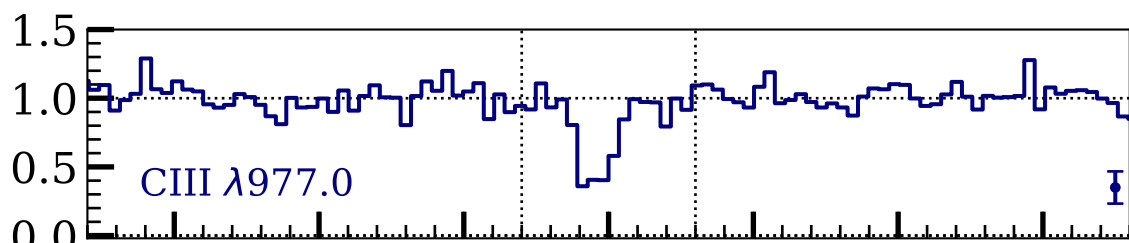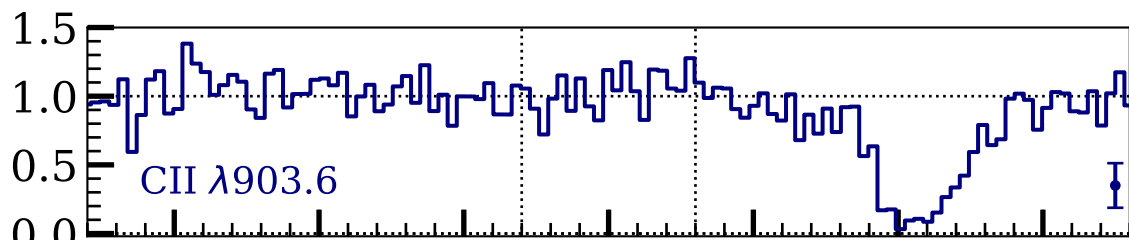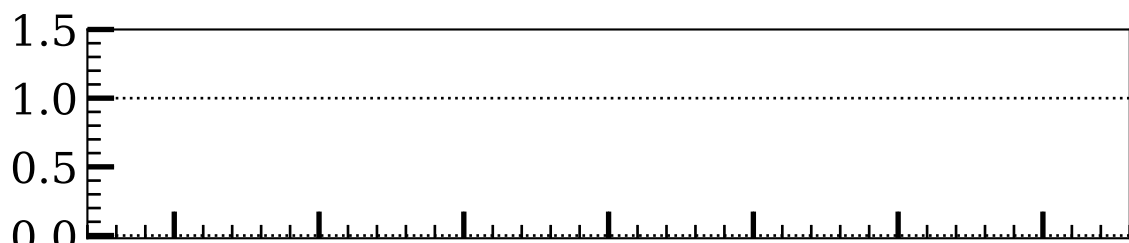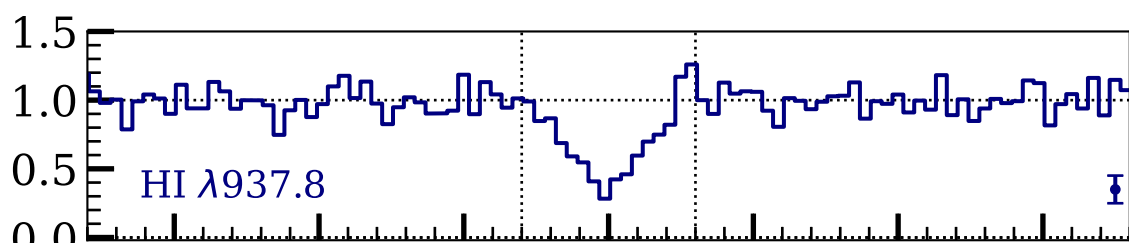

Rest-Frame Velocity ( $\text{km s}^{-1}$ )

J105956.14+121151.1,  $z=0.332377$ , RF=1

Normalized Flux

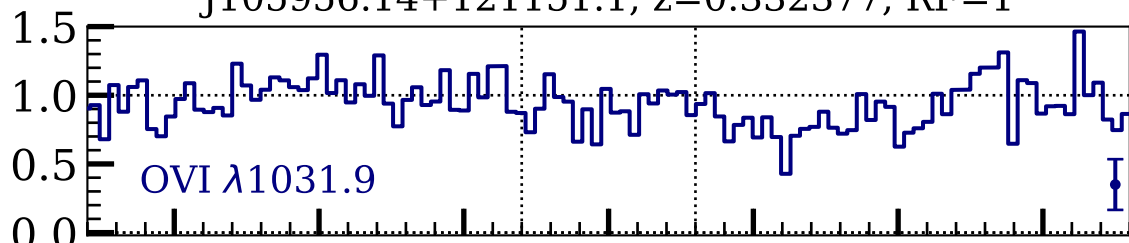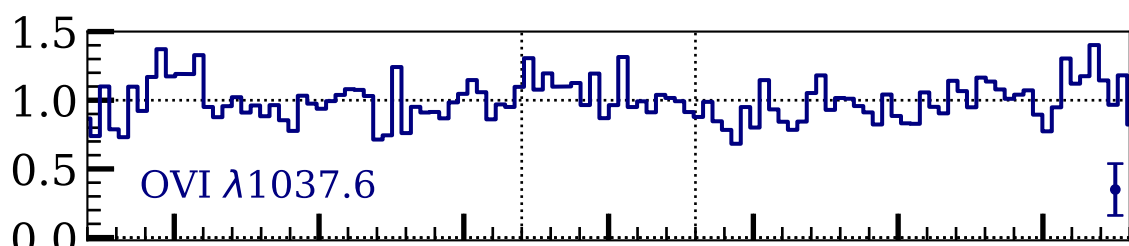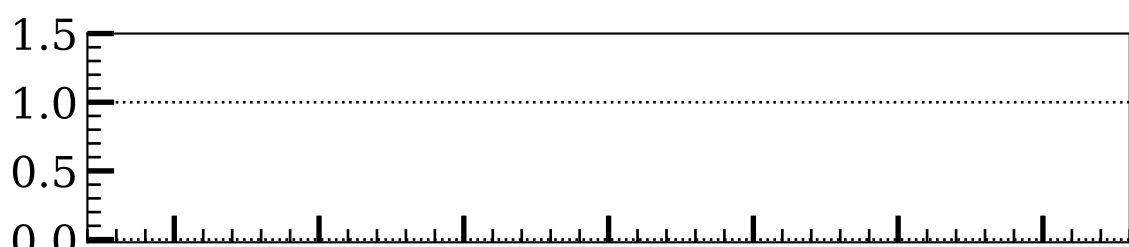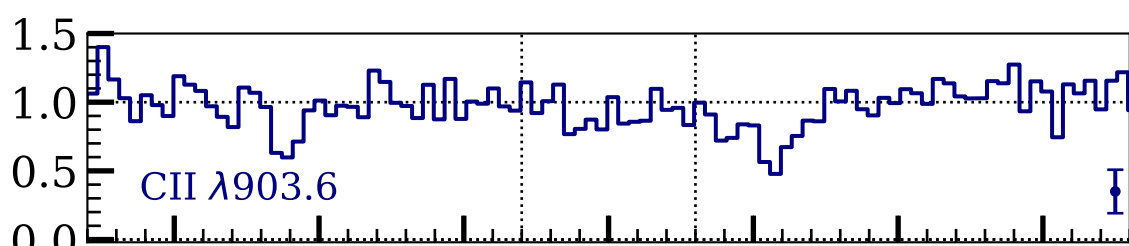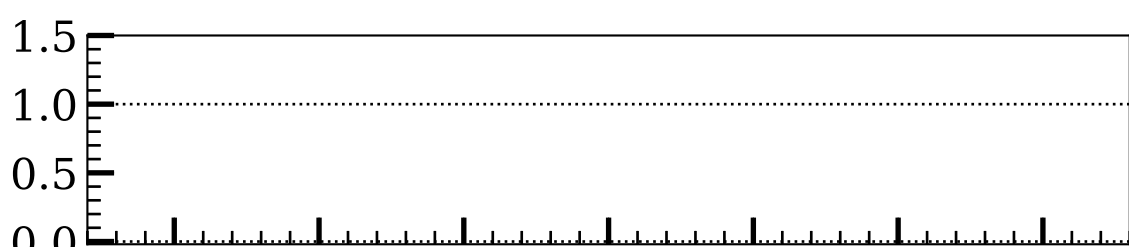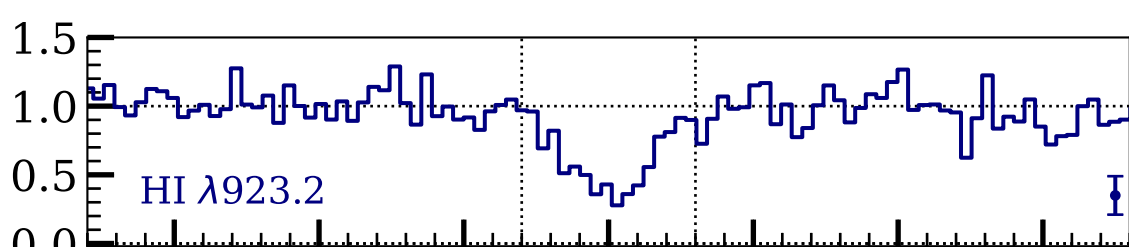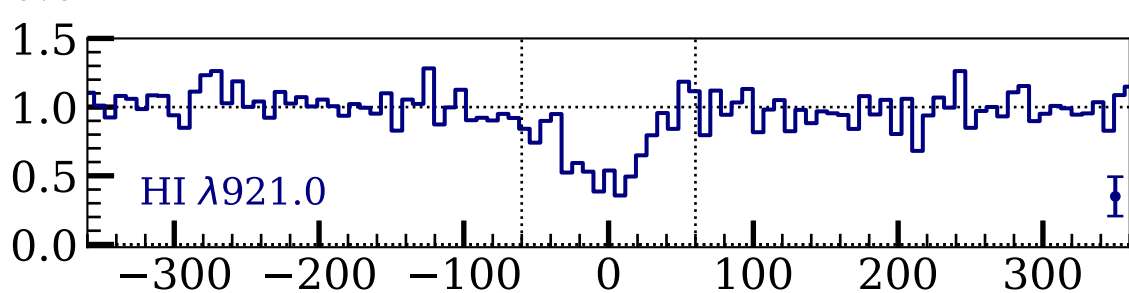

Rest-Frame Velocity ( $\text{km s}^{-1}$ )

J110047.85+104613.2,  $z=0.415099$ , RF=0

Normalized Flux

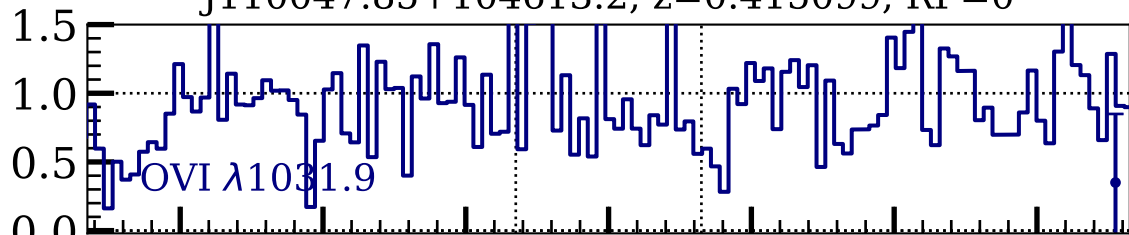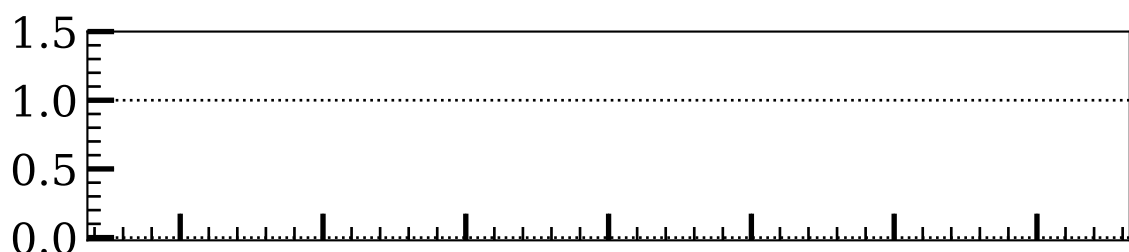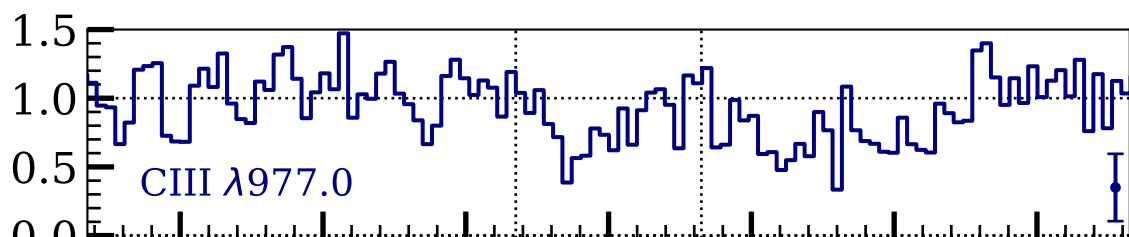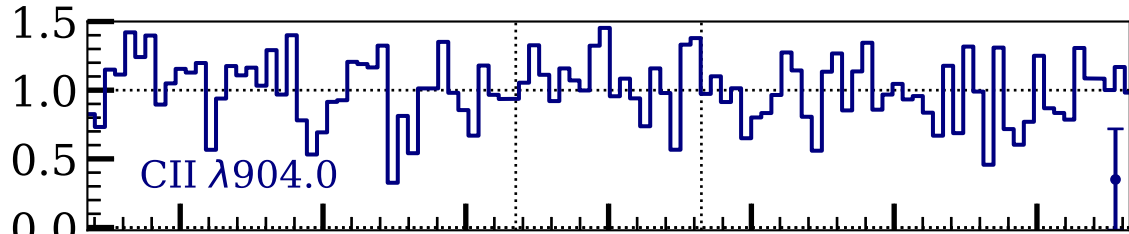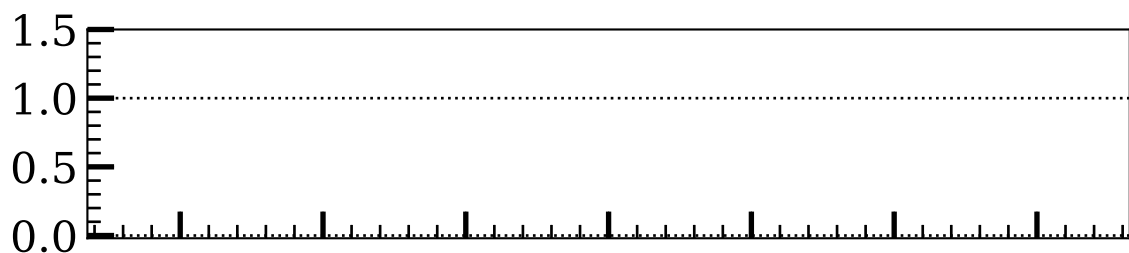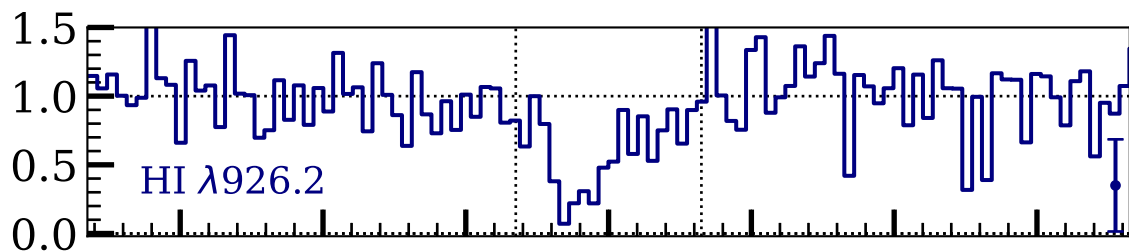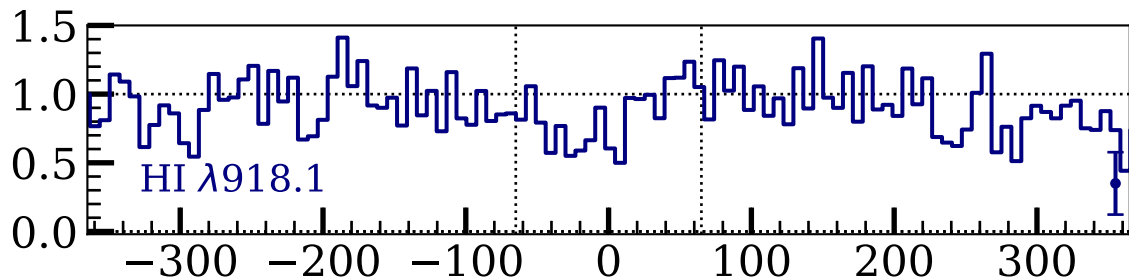

Rest-Frame Velocity ( $\text{km s}^{-1}$ )

J110539.79+342534.3,  $z=0.238808$ , RF=1

Normalized Flux

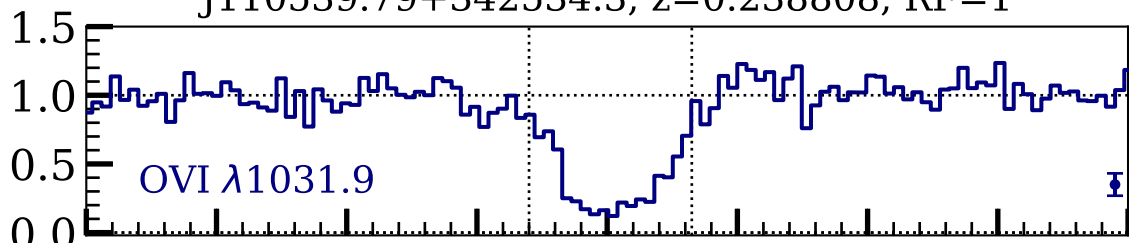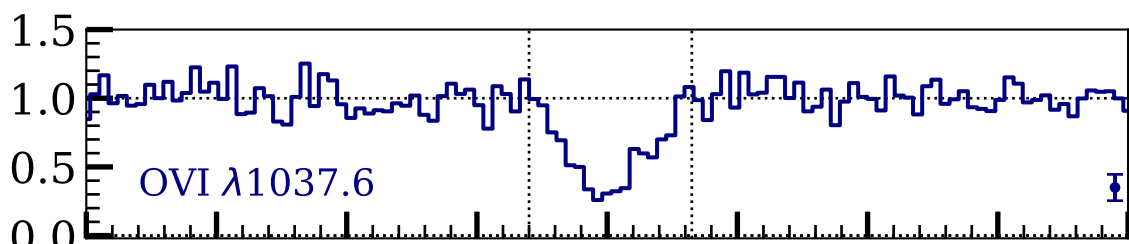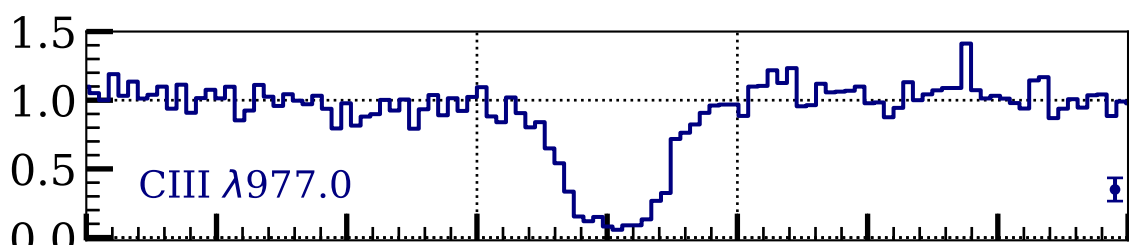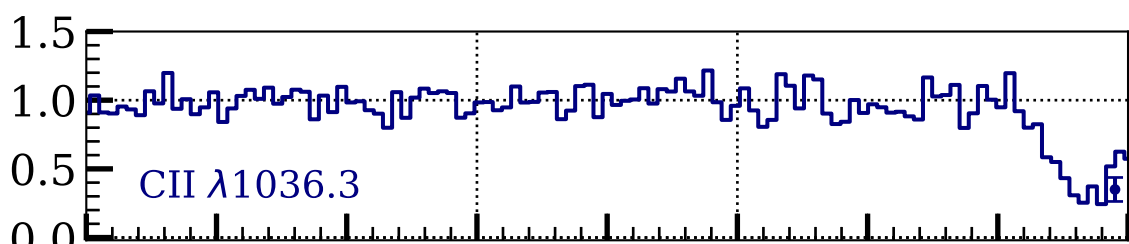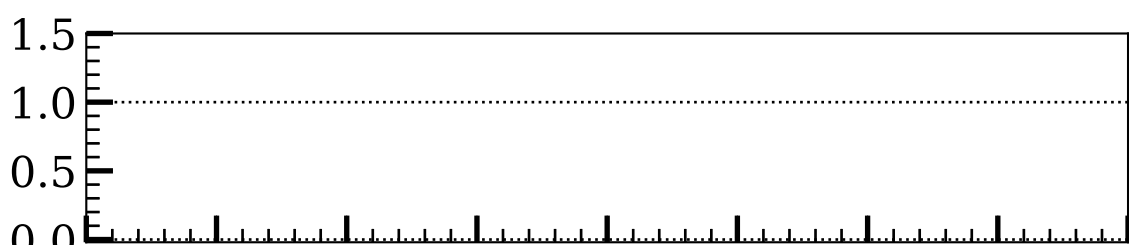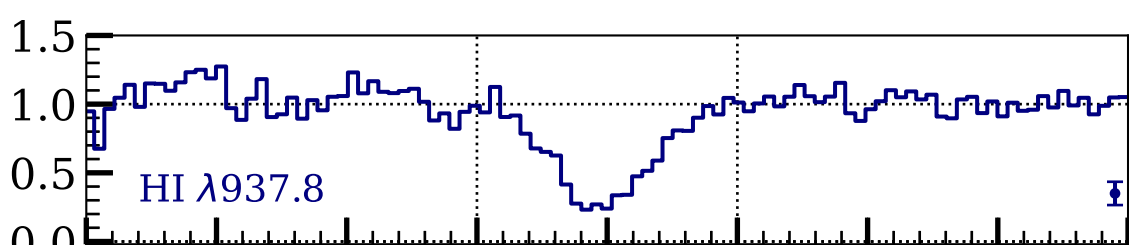

Rest-Frame Velocity ( $\text{km s}^{-1}$ )



J111132.20+554725.9,  $z=0.617506$ , RF=1

Normalized Flux

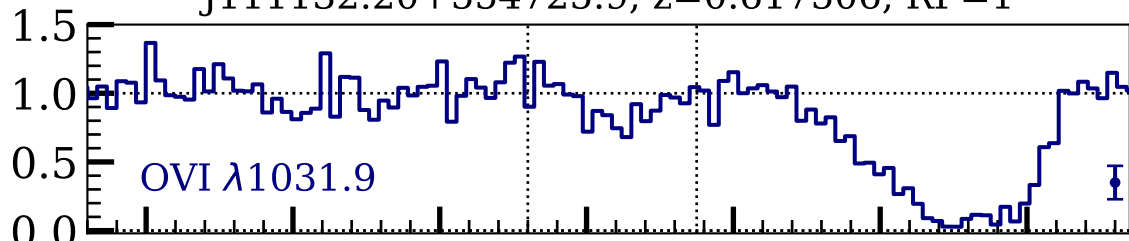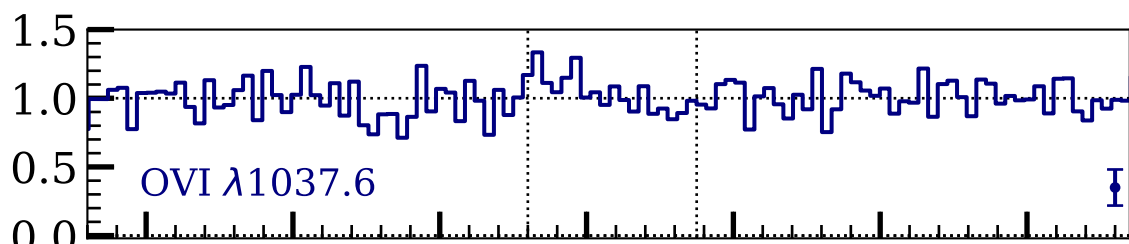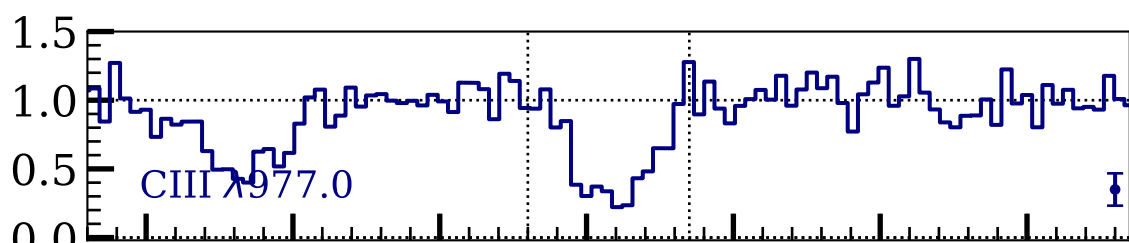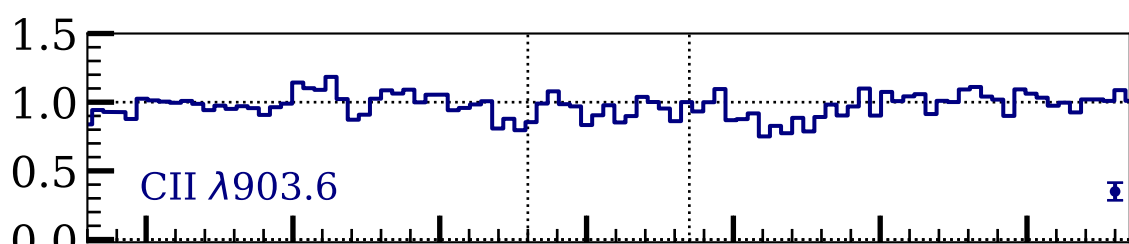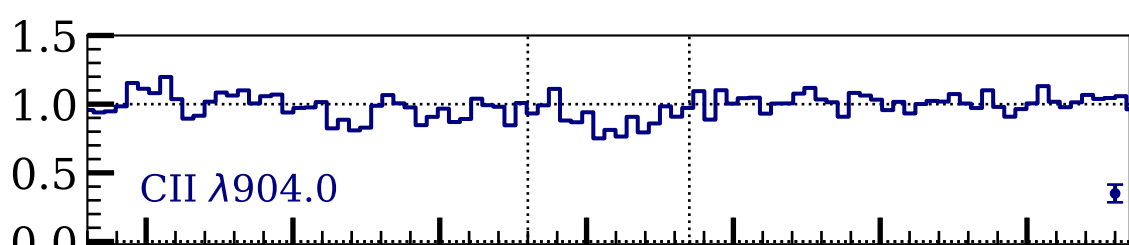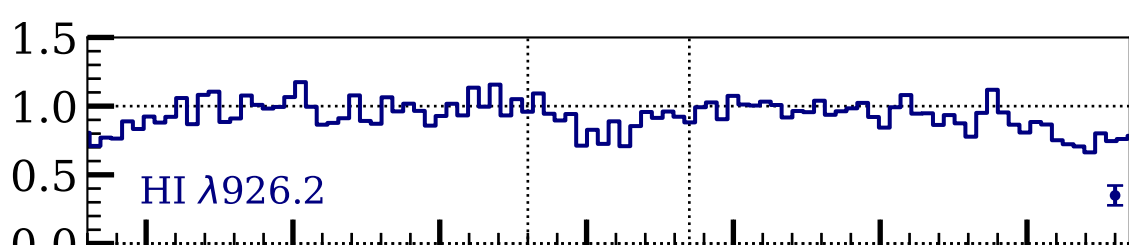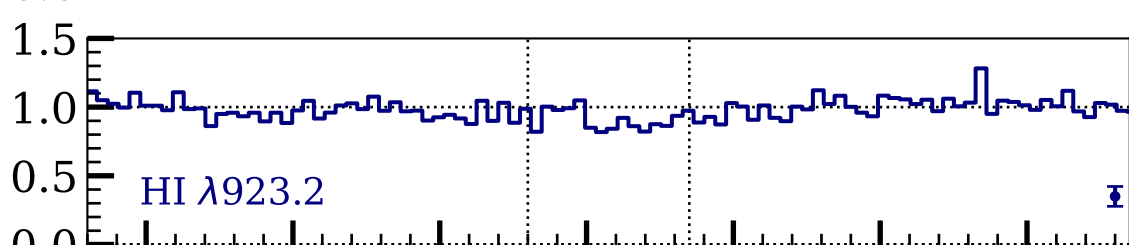

Rest-Frame Velocity ( $\text{km s}^{-1}$ )

J111132.20+554725.9,  $z=0.682730$ , RF=1

Normalized Flux

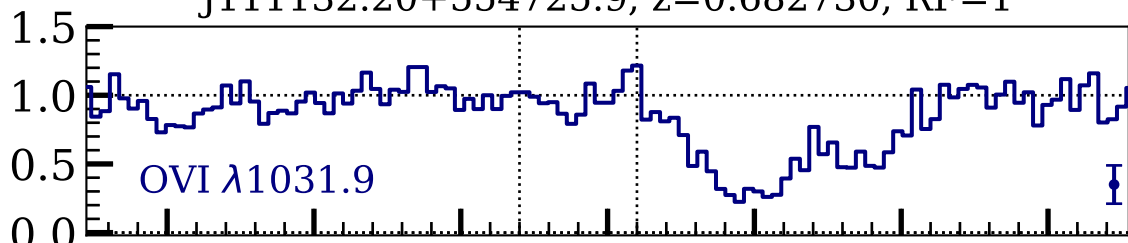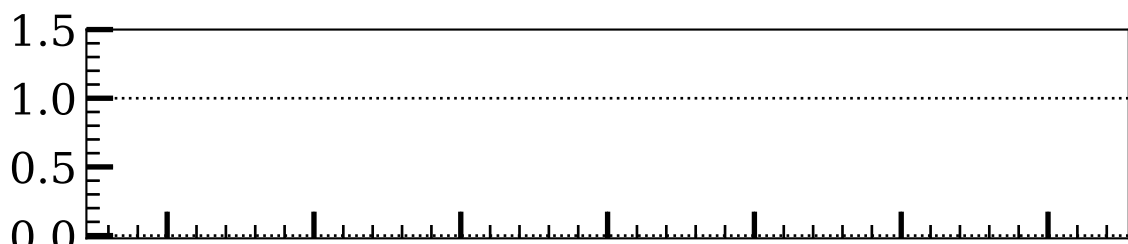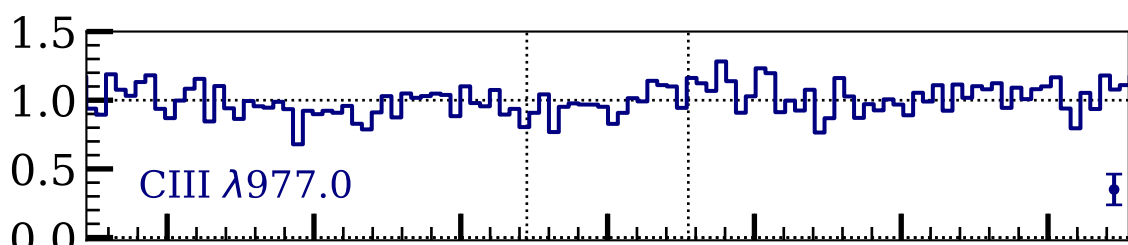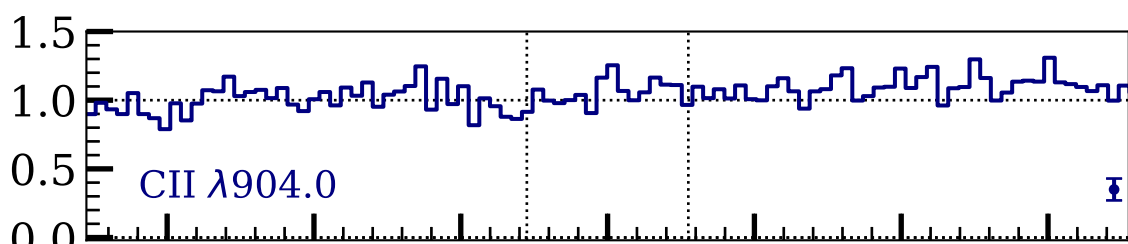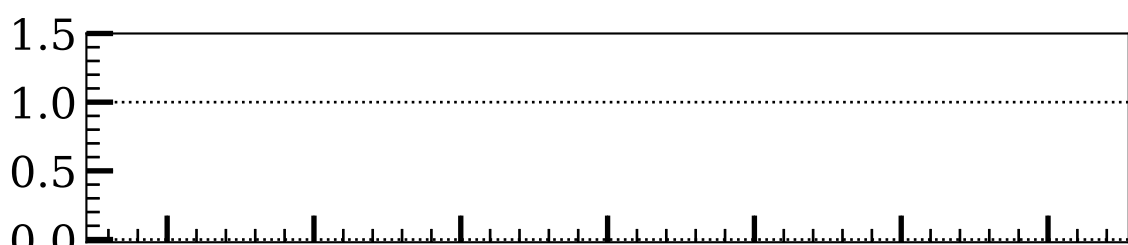

Rest-Frame Velocity ( $\text{km s}^{-1}$ )

J111239.11+353928.2,  $z=0.246496$ , RF=0

Normalized Flux

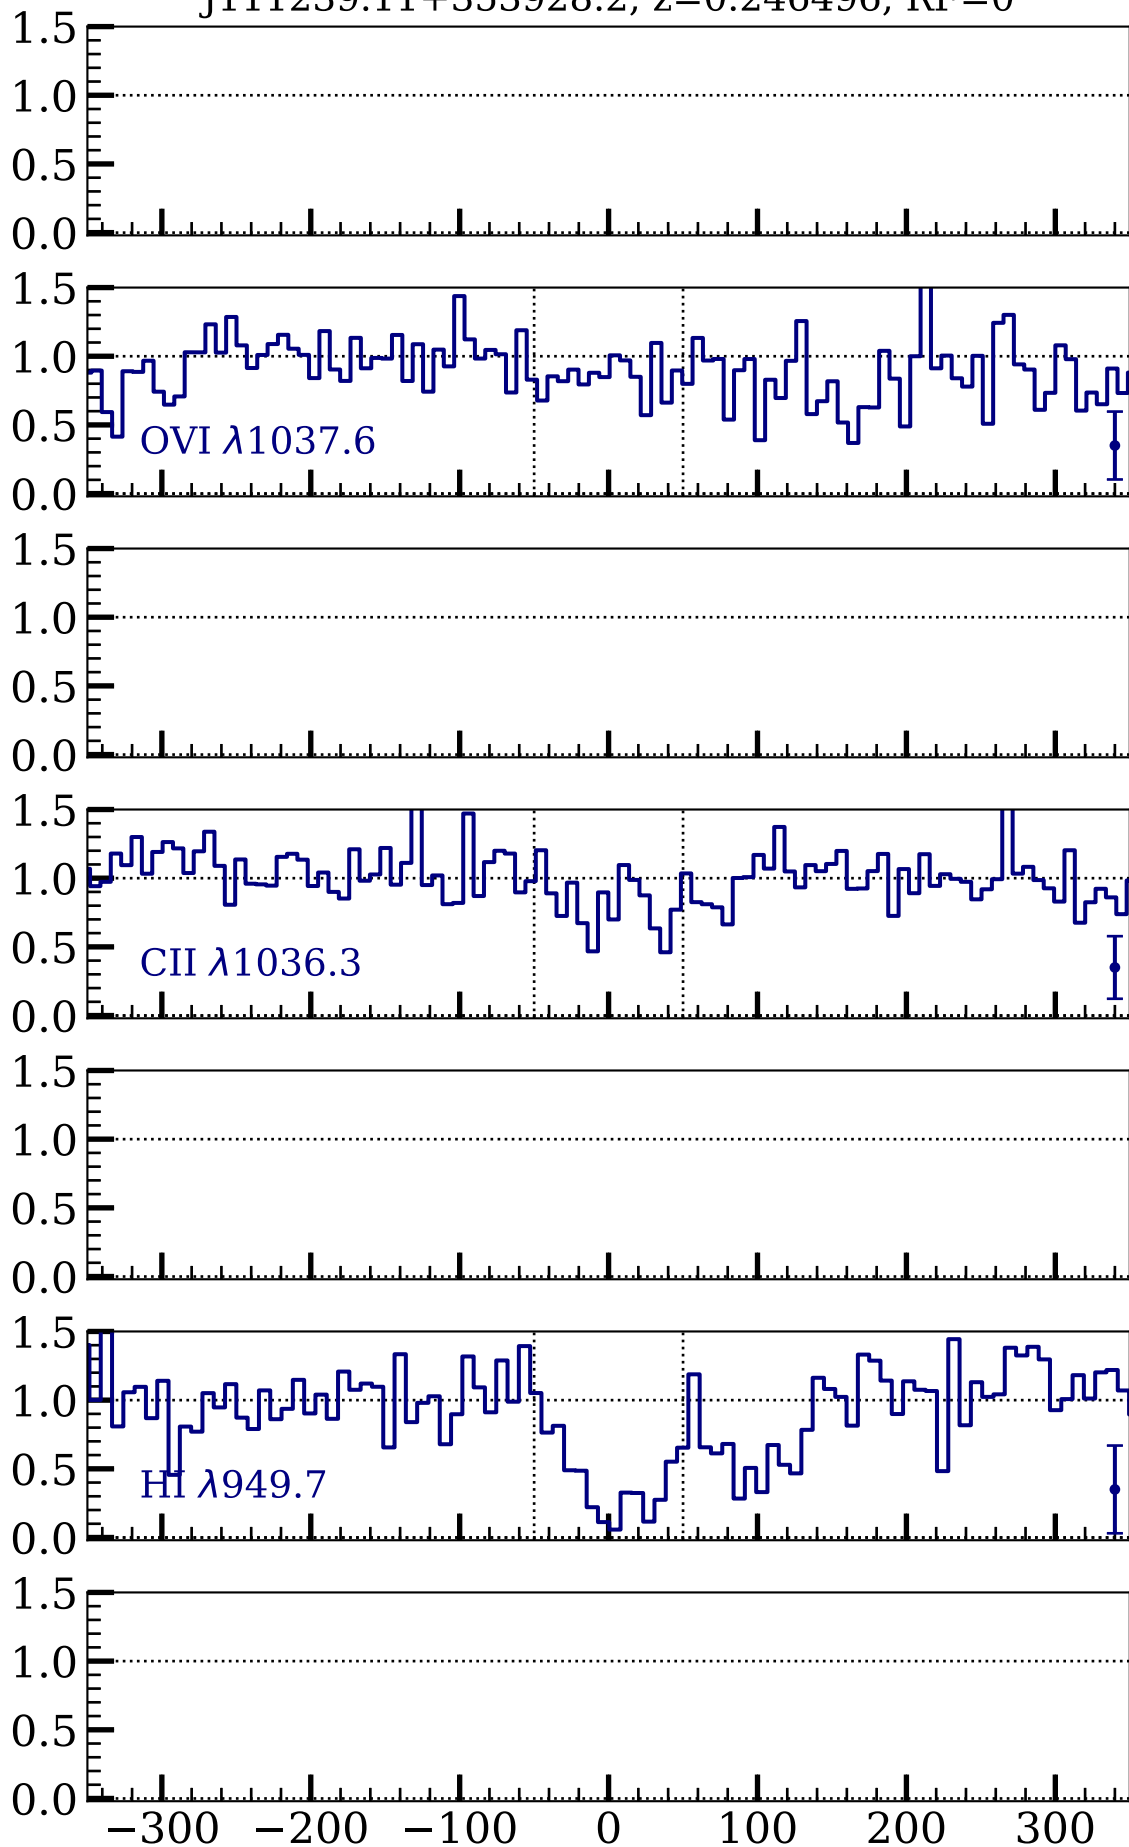

Rest-Frame Velocity ( $\text{km s}^{-1}$ )

J111507.65+023757.5,  $z=0.369213$ , RF=1

Normalized Flux

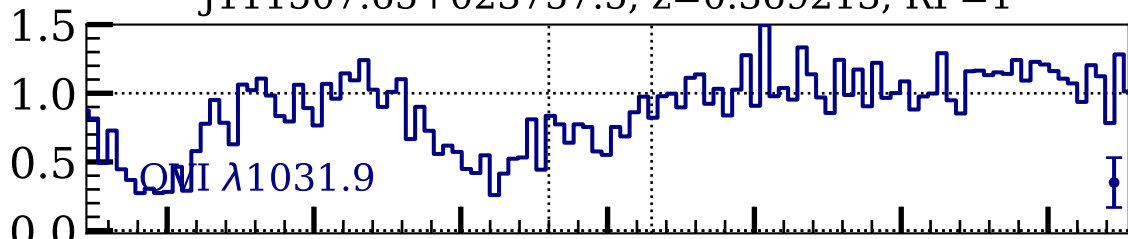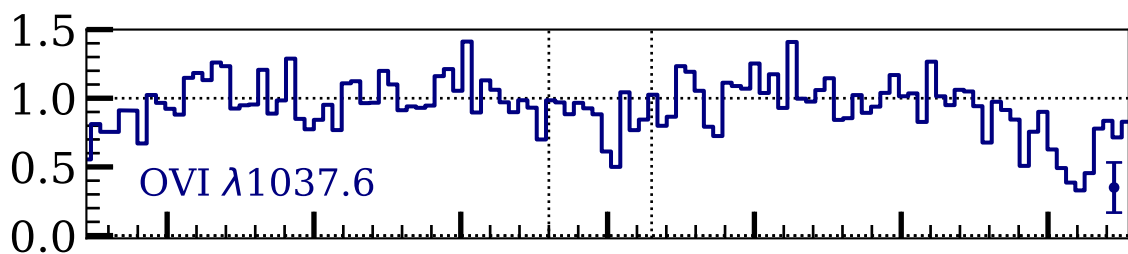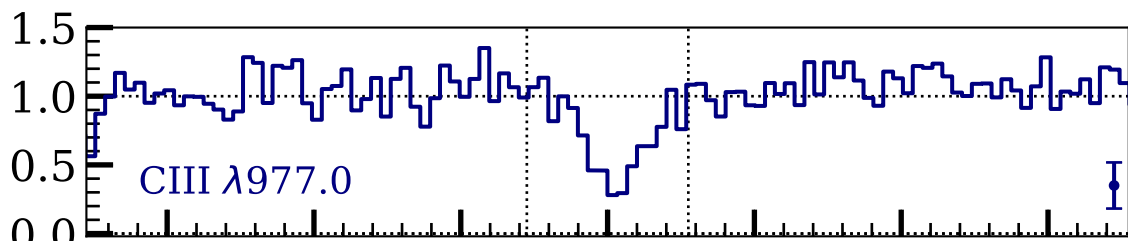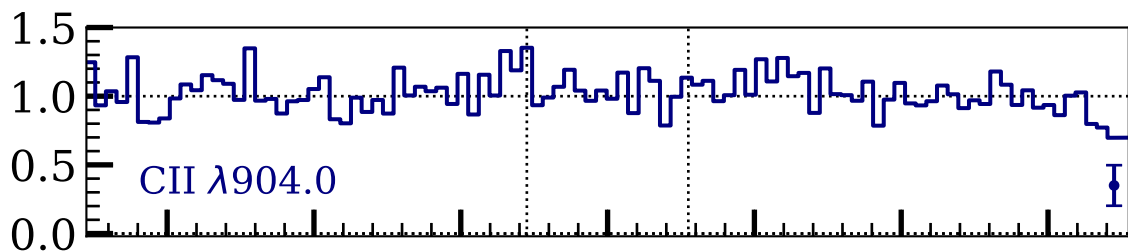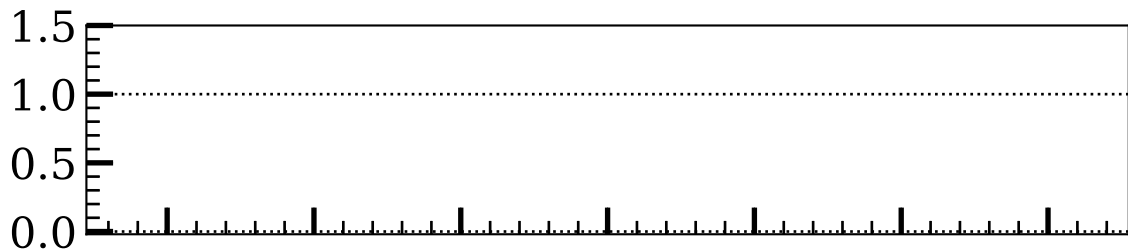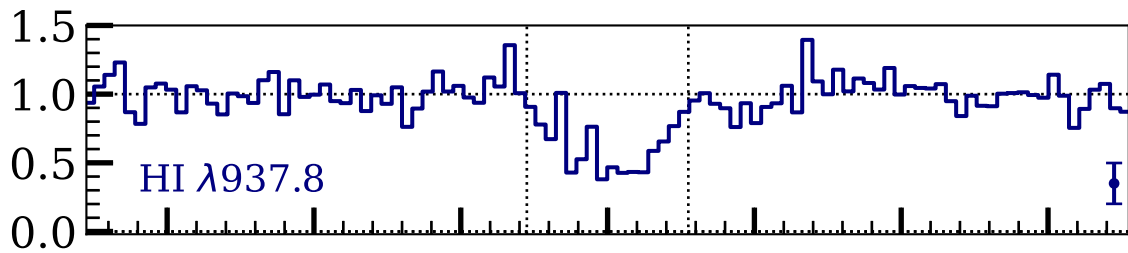

Rest-Frame Velocity ( $\text{km s}^{-1}$ )

J111754.23+263416.6,  $z=0.351969$ , RF=1

Normalized Flux

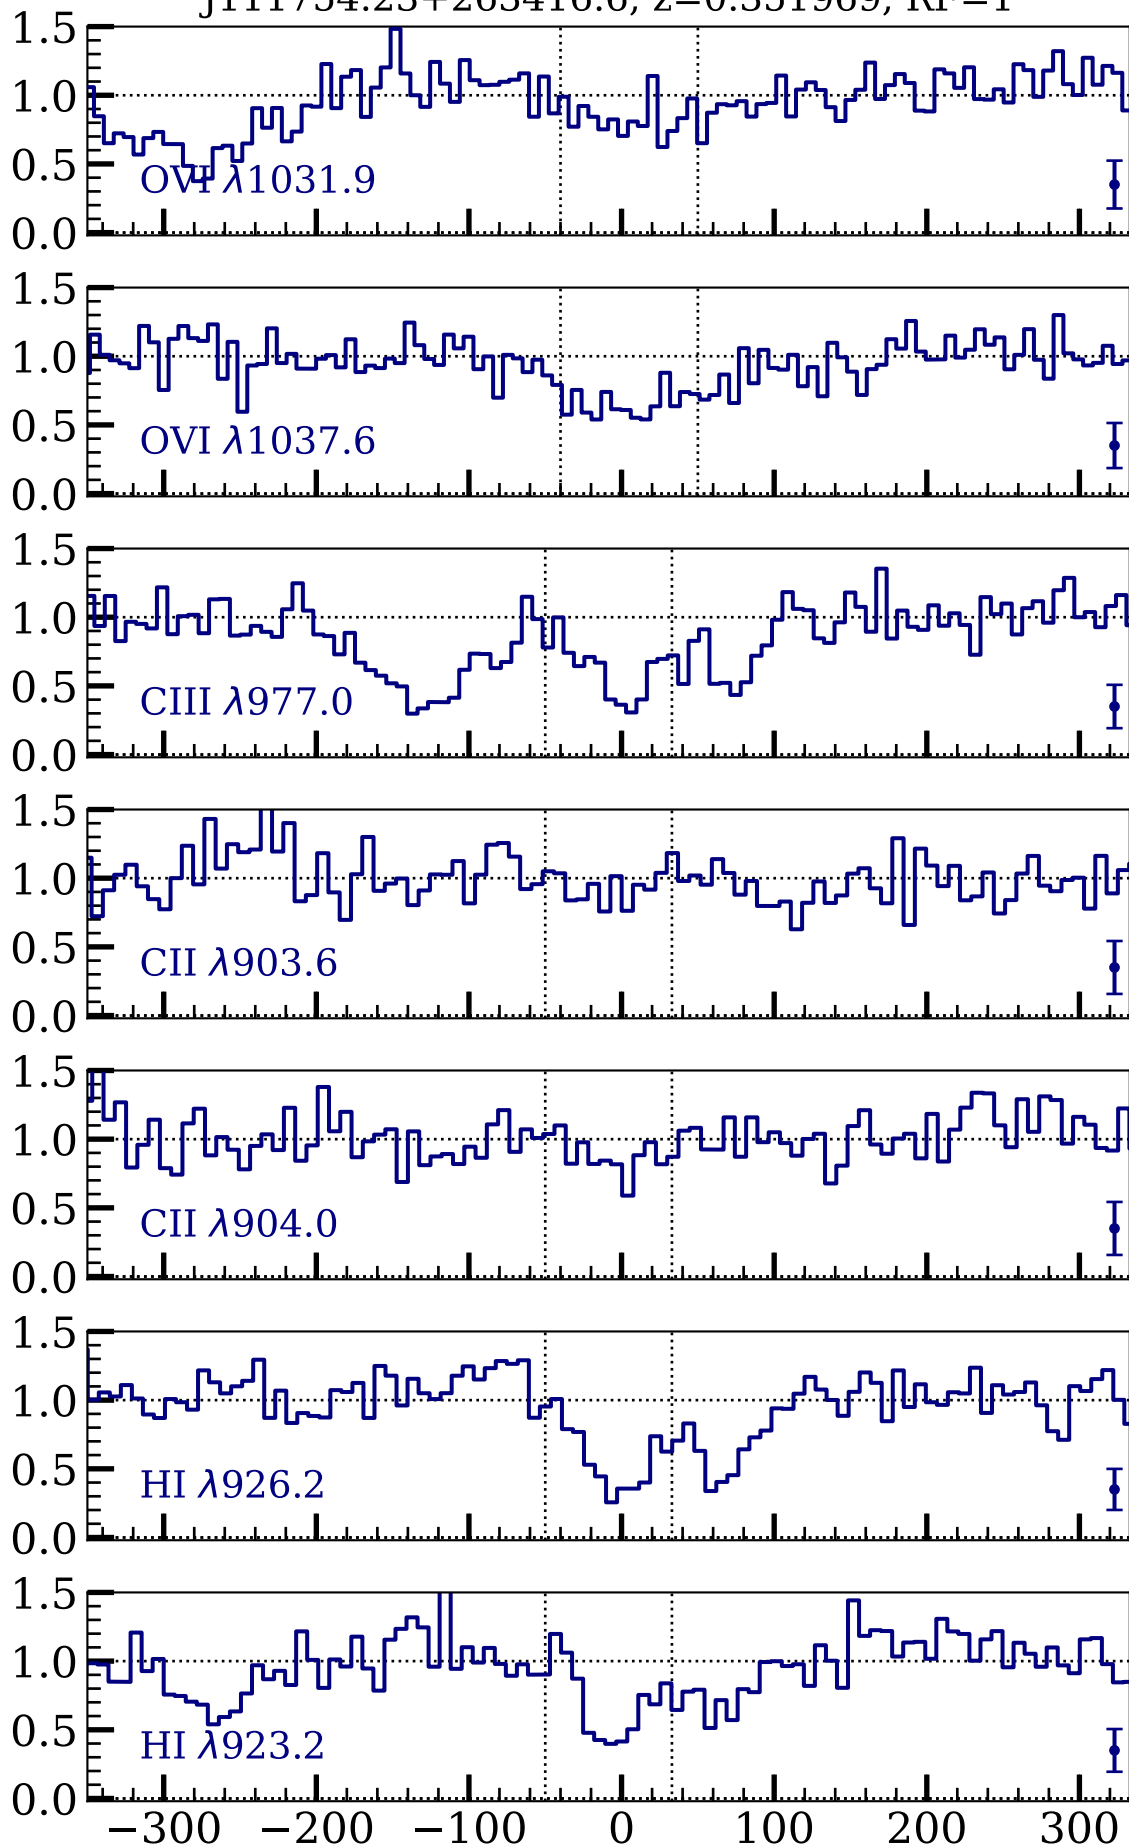

Rest-Frame Velocity (km s<sup>-1</sup>)

J111754.23+263416.6,  $z=0.352307$ , RF=1

Normalized Flux

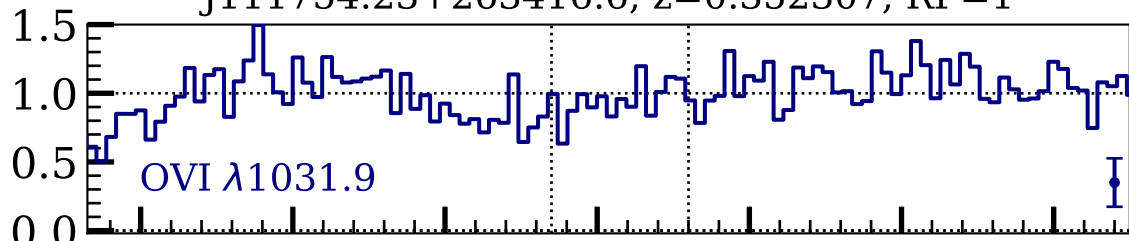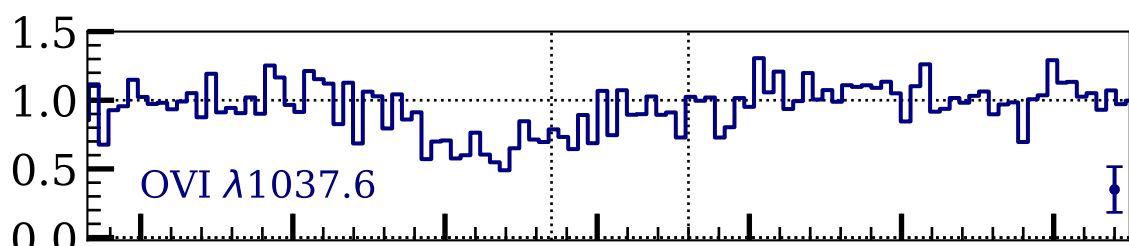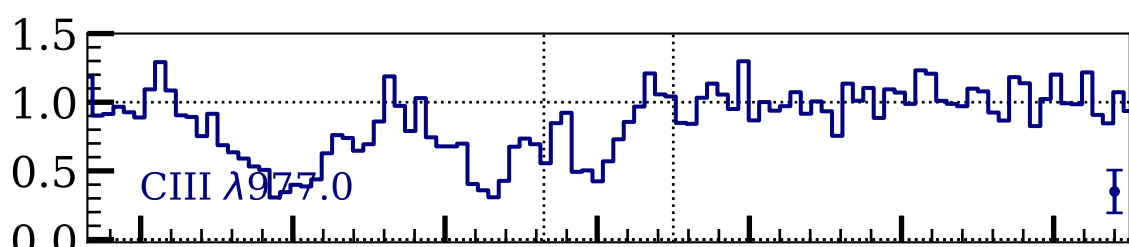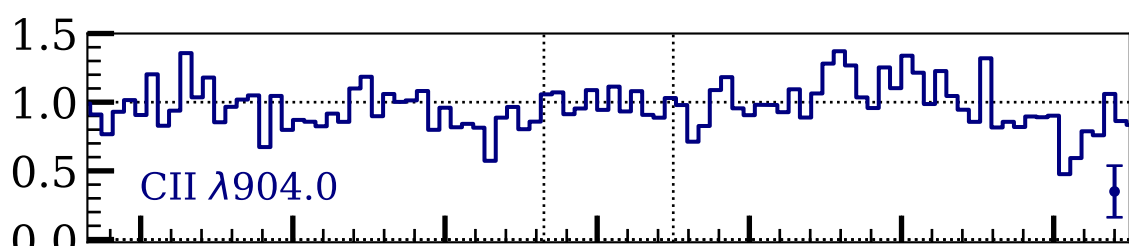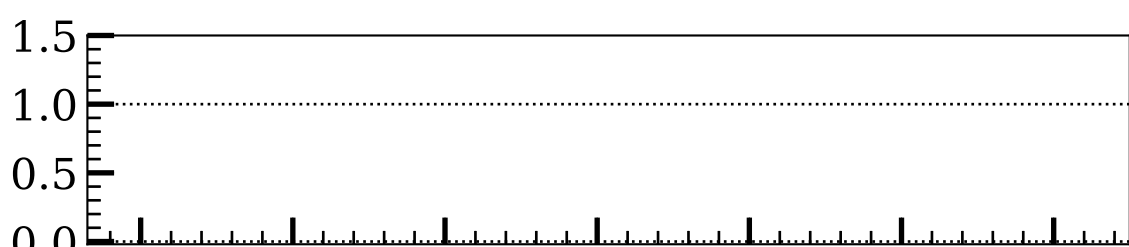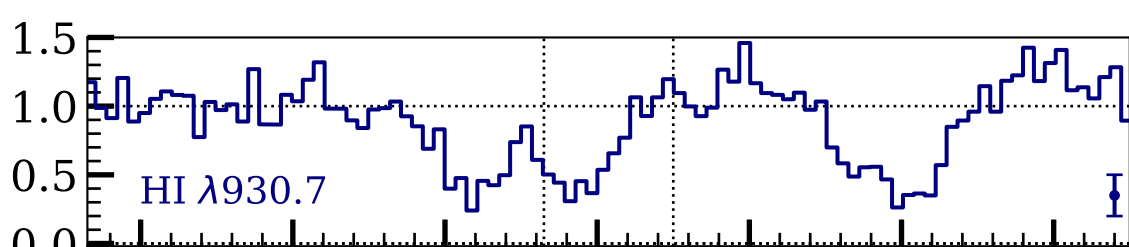

Rest-Frame Velocity ( $\text{km s}^{-1}$ )

J111908.59+211918.0,  $z=0.138500$ , RF=1

Normalized Flux

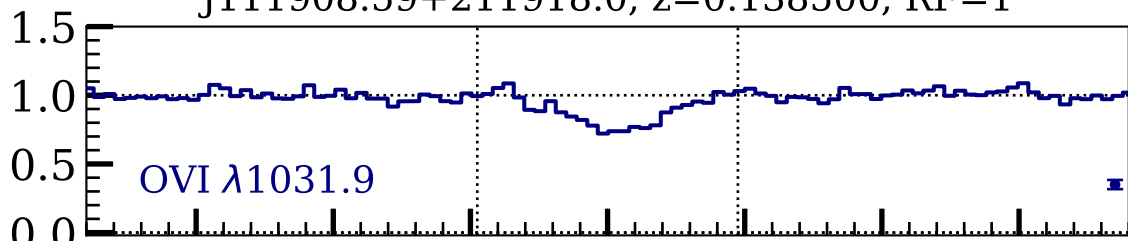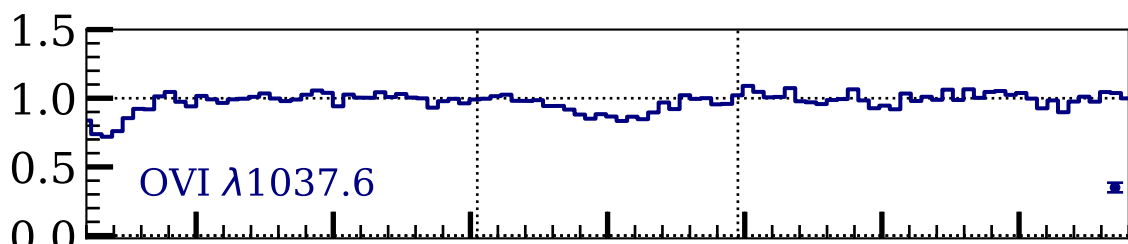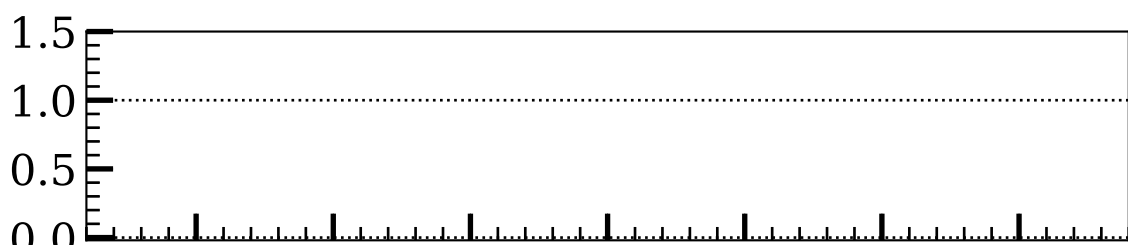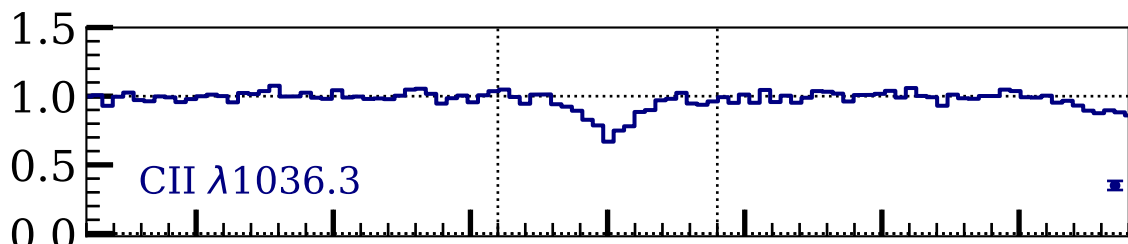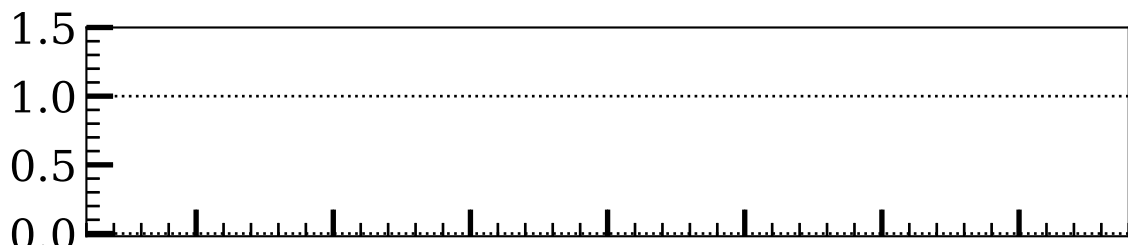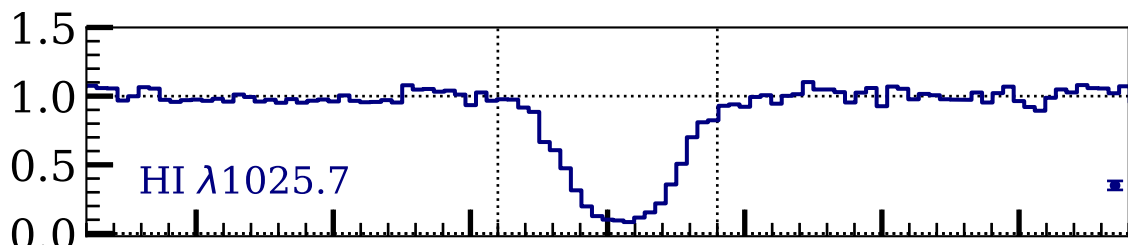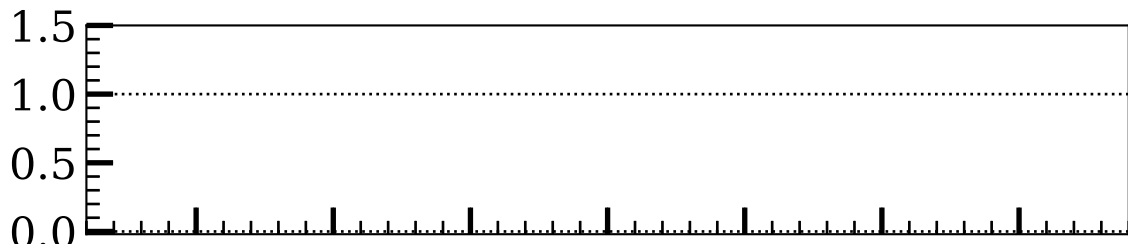

Rest-Frame Velocity ( $\text{km s}^{-1}$ )

J112553.78+591021.6,  $z=0.557529$ , RF=0

Normalized Flux

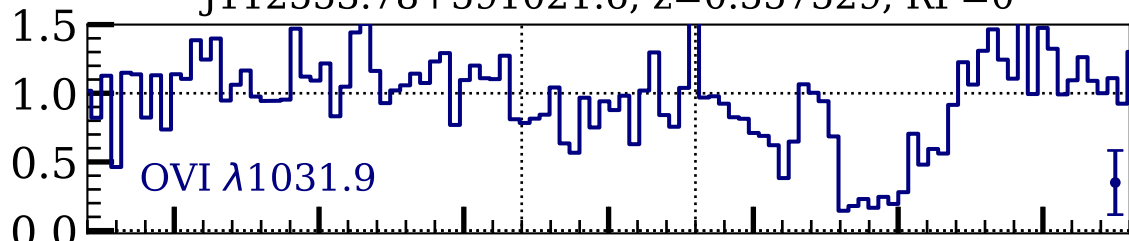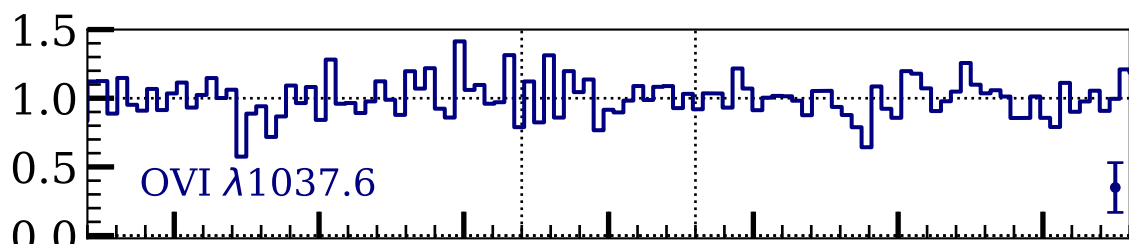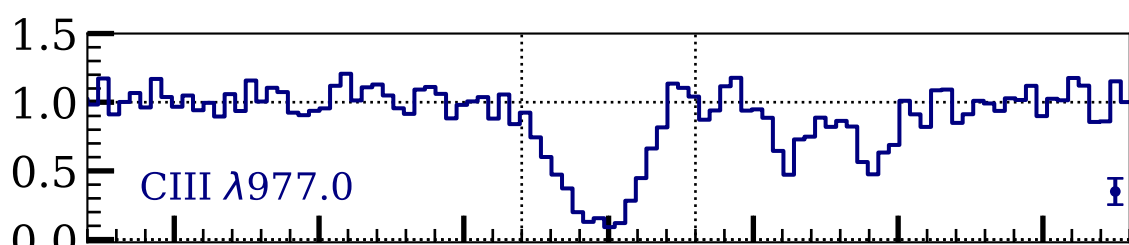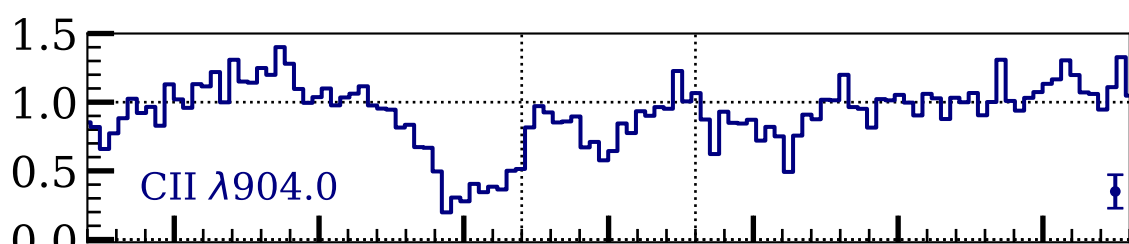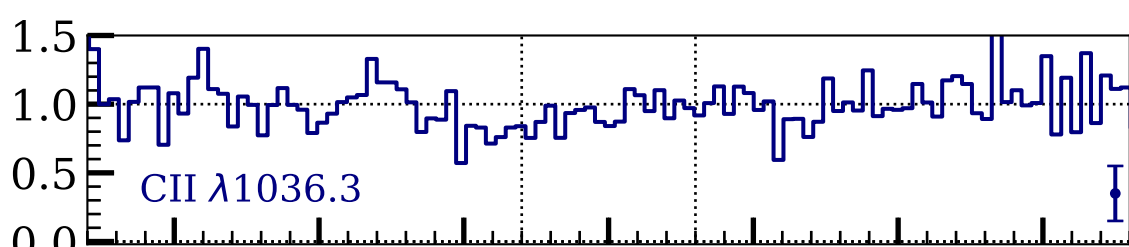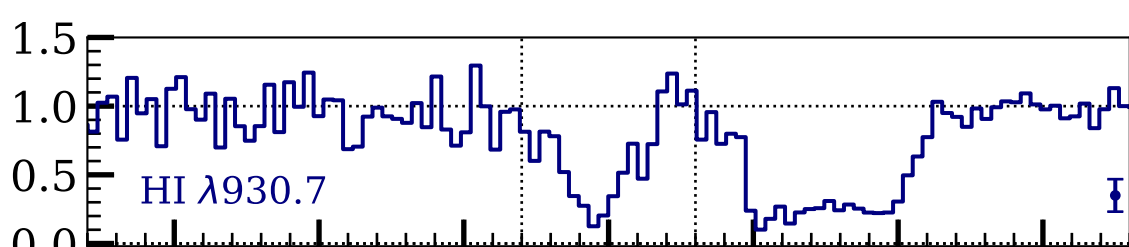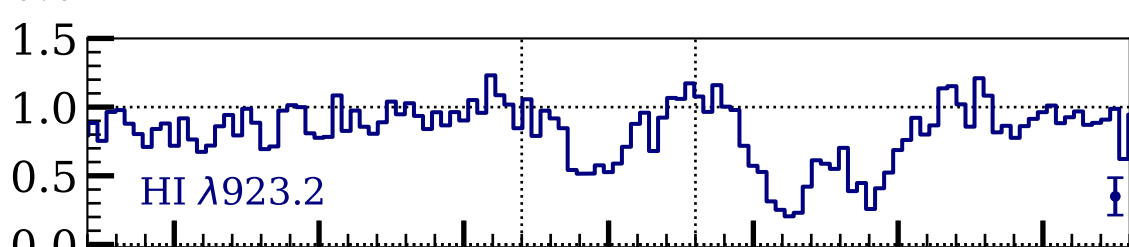

Rest-Frame Velocity ( $\text{km s}^{-1}$ )



J112553.78+591021.6,  $z=0.558200$ , RF=0

Normalized Flux

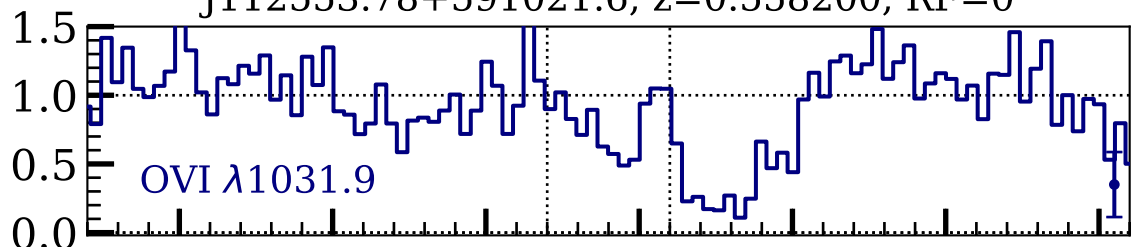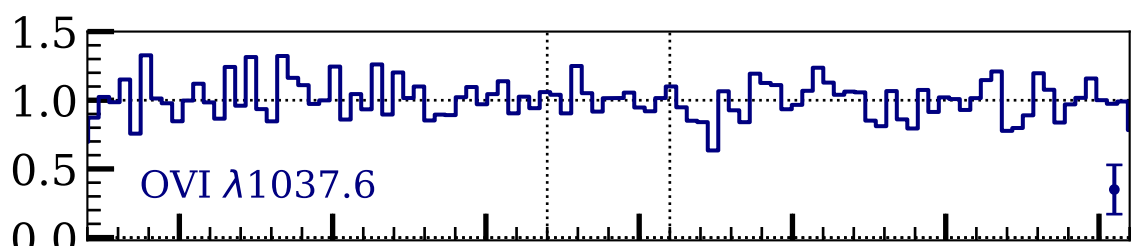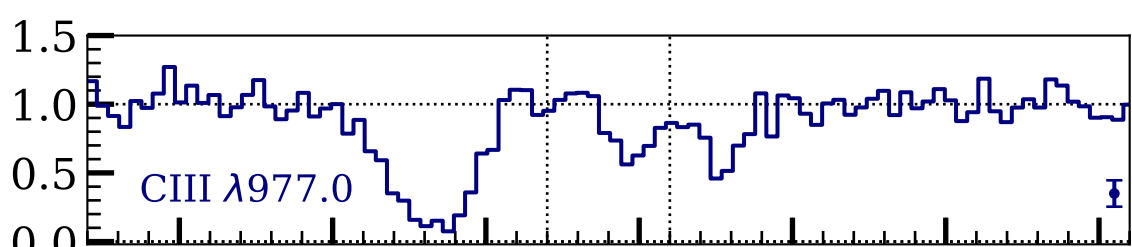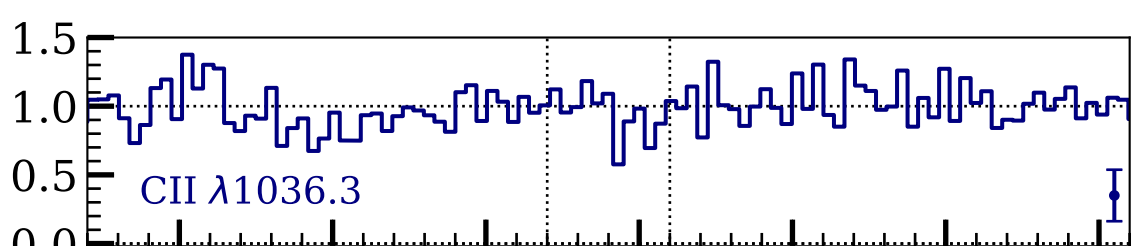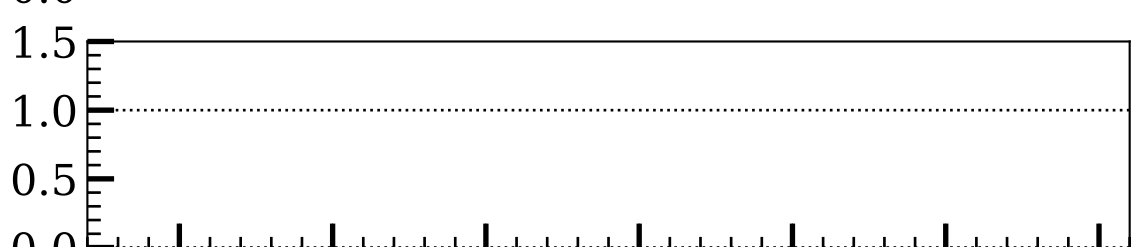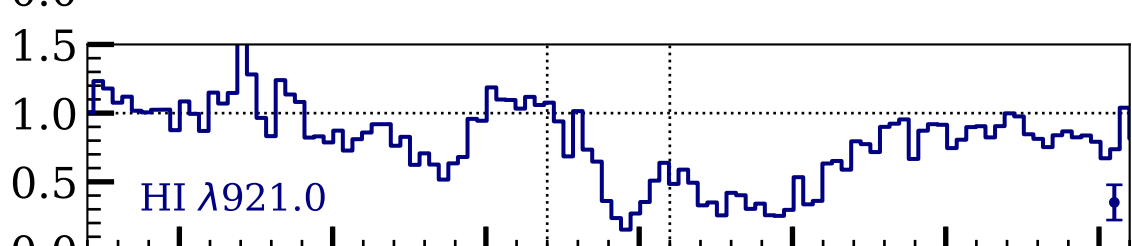

Rest-Frame Velocity ( $\text{km s}^{-1}$ )

J112553.78+591021.6,  $z=0.558450$ , RF=1

Normalized Flux

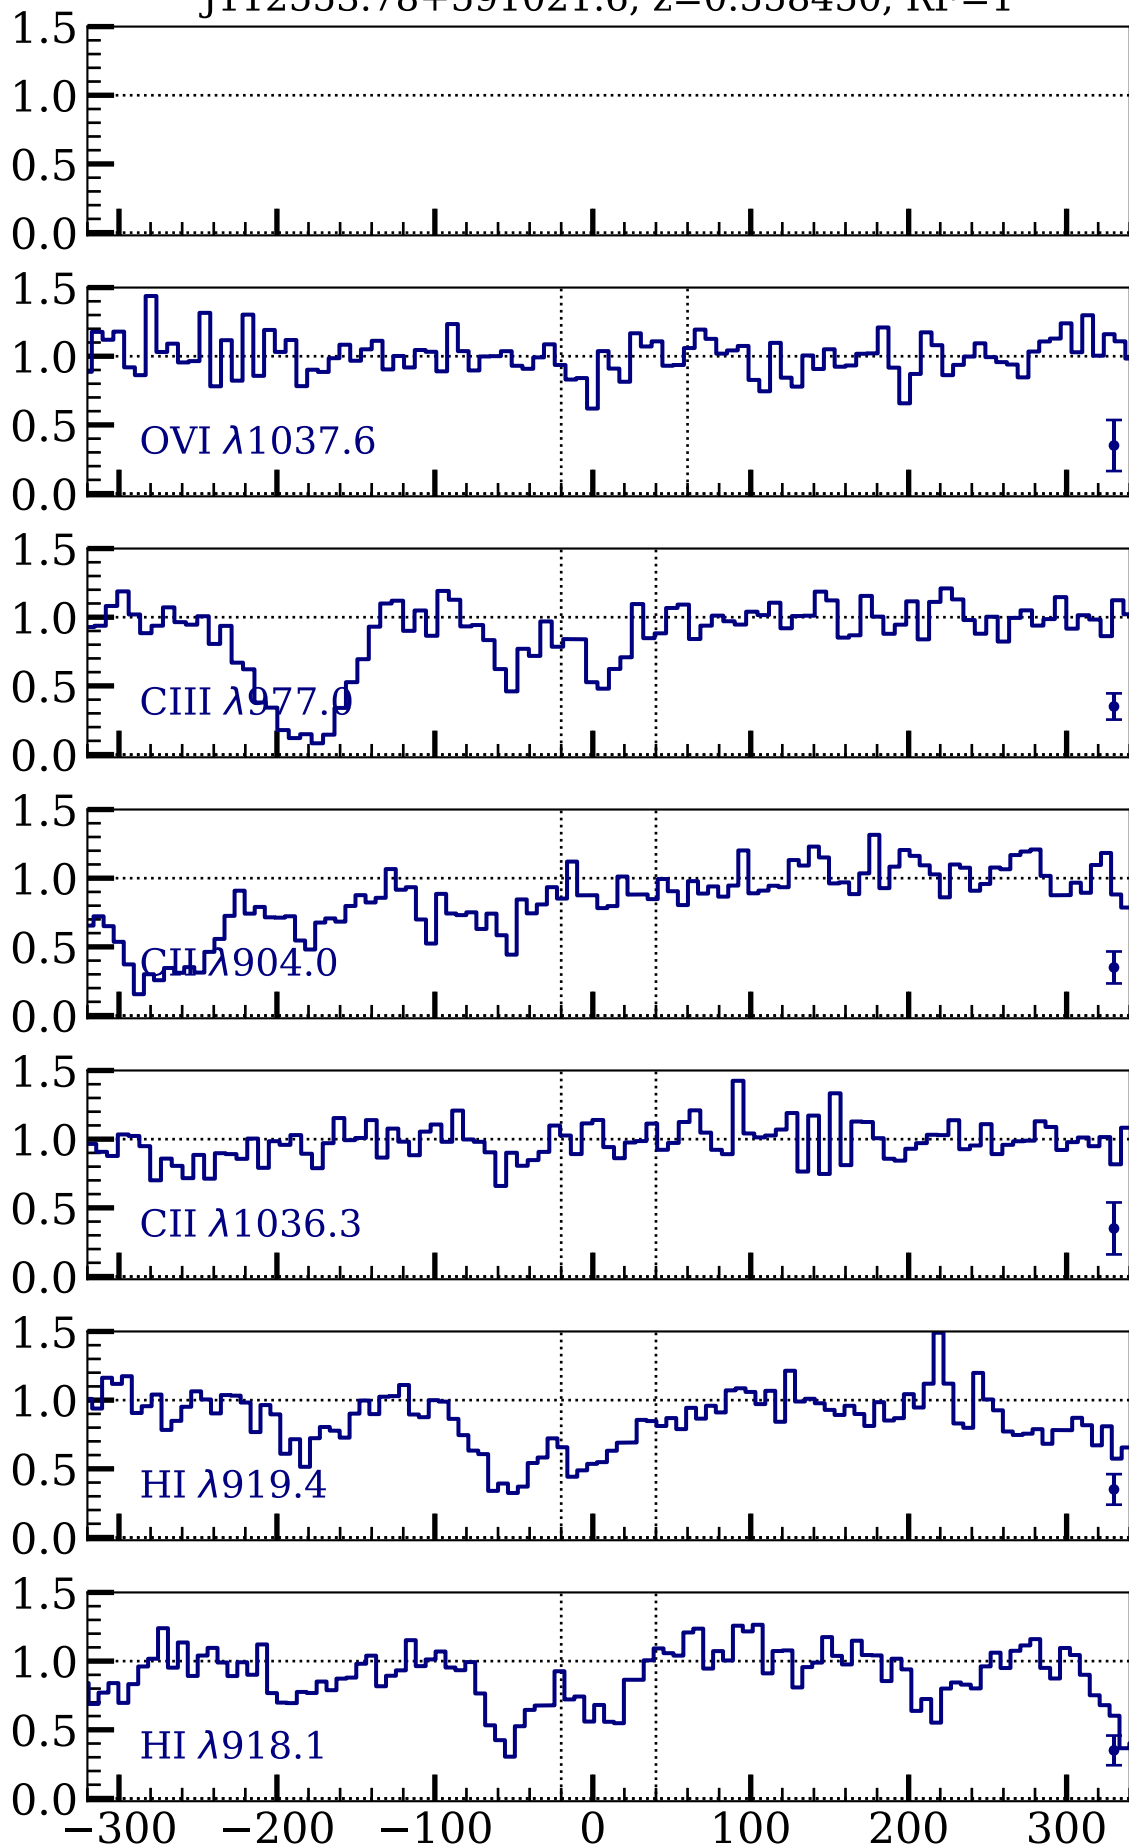

Rest-Frame Velocity (km s<sup>-1</sup>)

J112553.78+591021.6,  $z=0.678351$ , RF=1

Normalized Flux

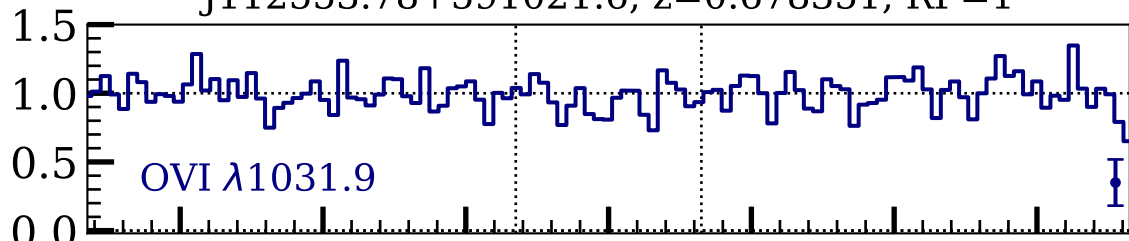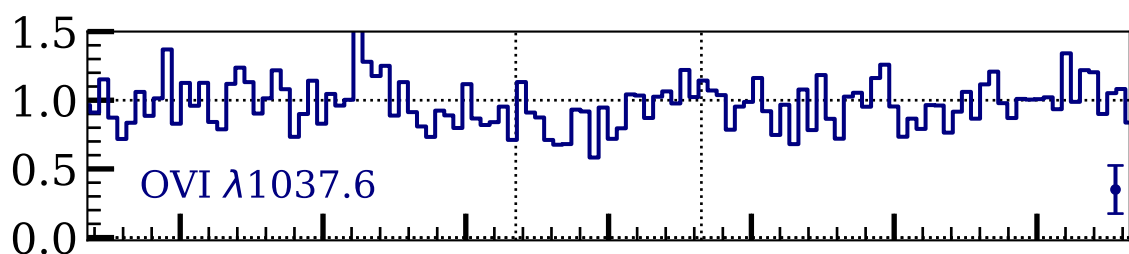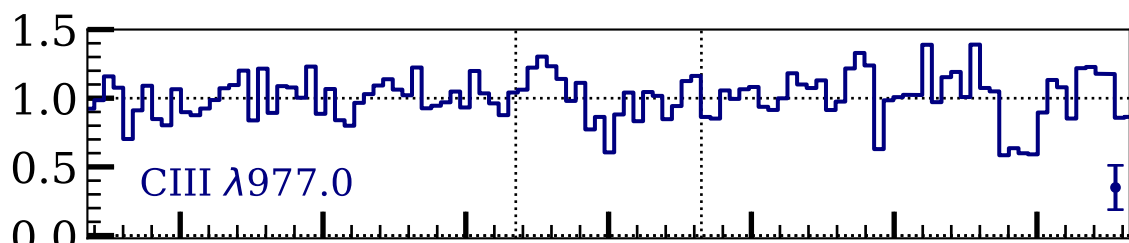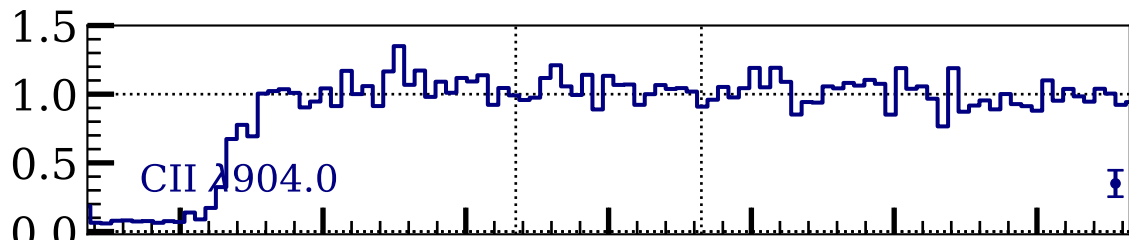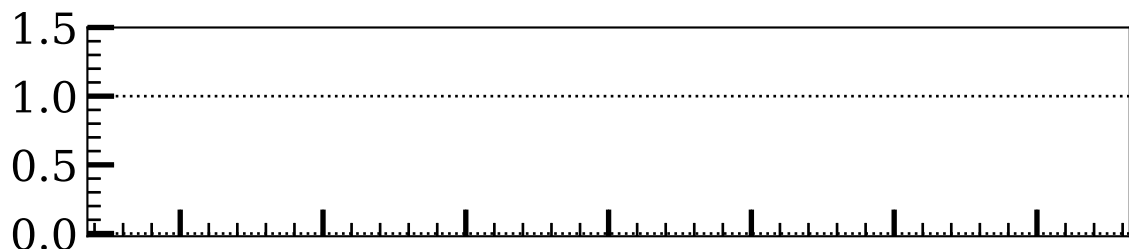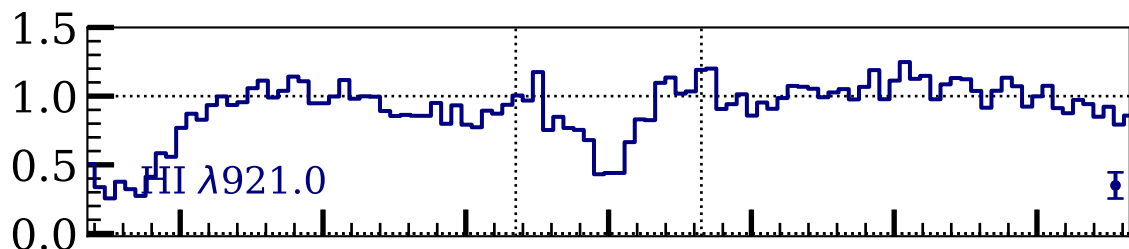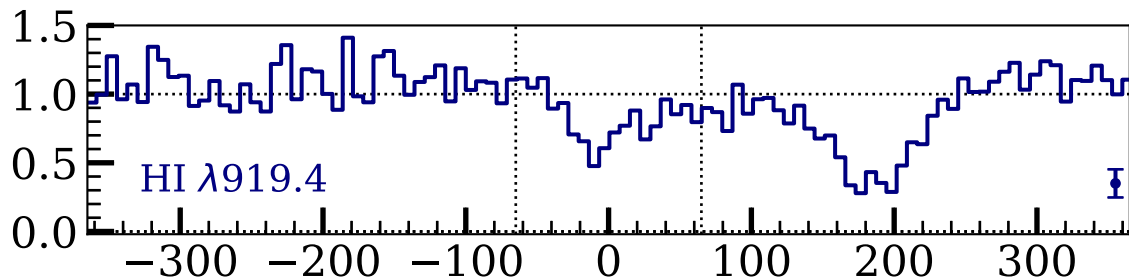

Rest-Frame Velocity ( $\text{km s}^{-1}$ )

J113457.71+255527.8,  $z=0.431964$ , RF=1

Normalized Flux

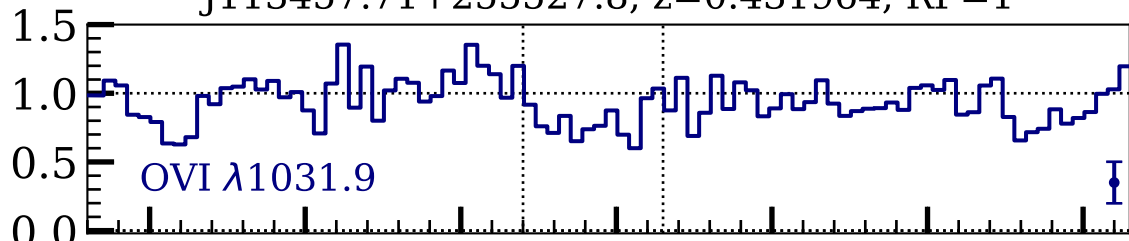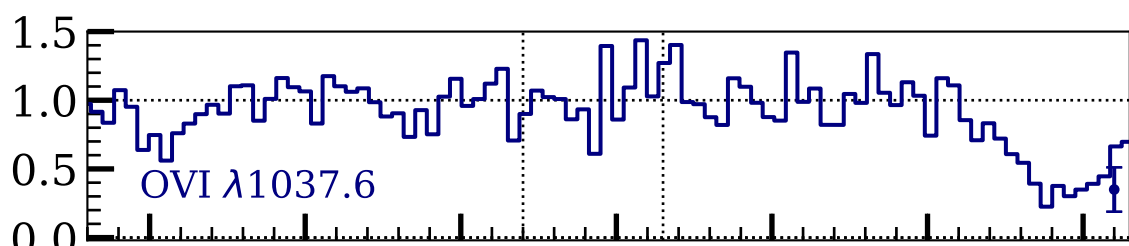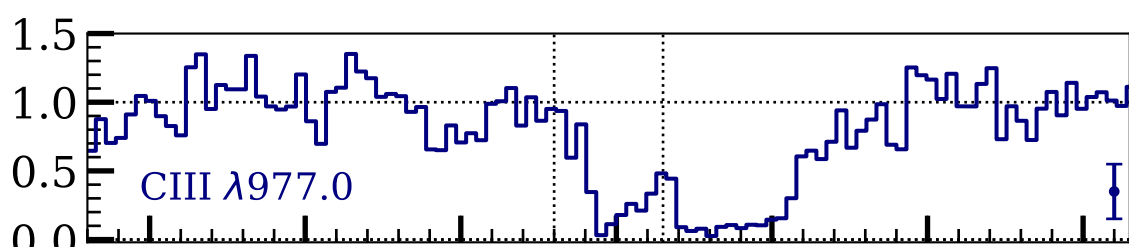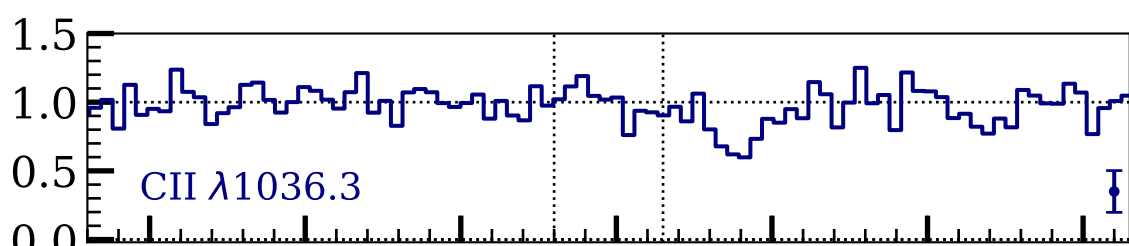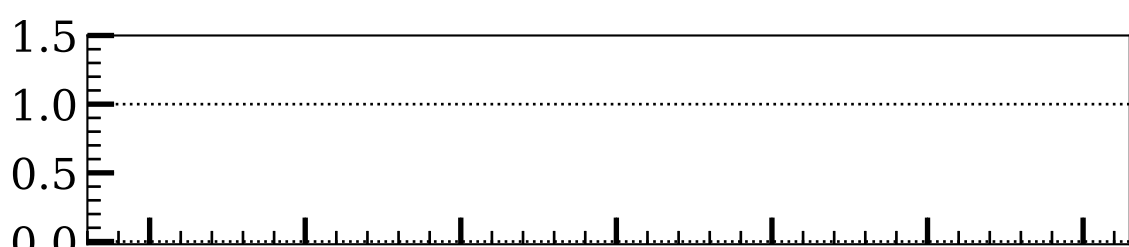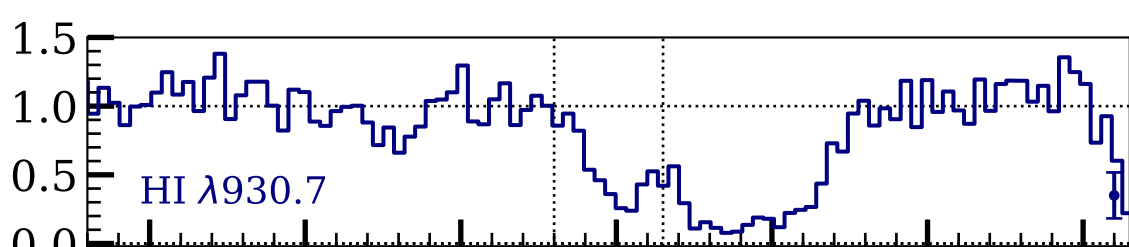

Rest-Frame Velocity ( $\text{km s}^{-1}$ )

J113457.71+255527.8,  $z=0.432313$ , RF=1

Normalized Flux

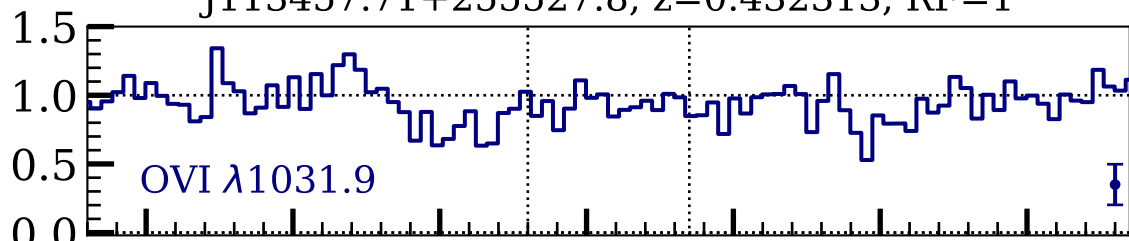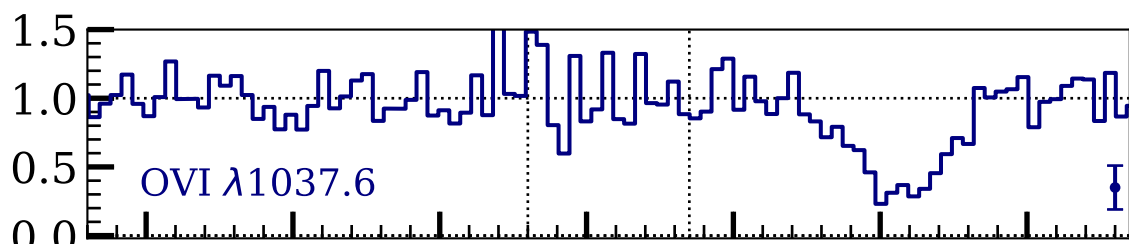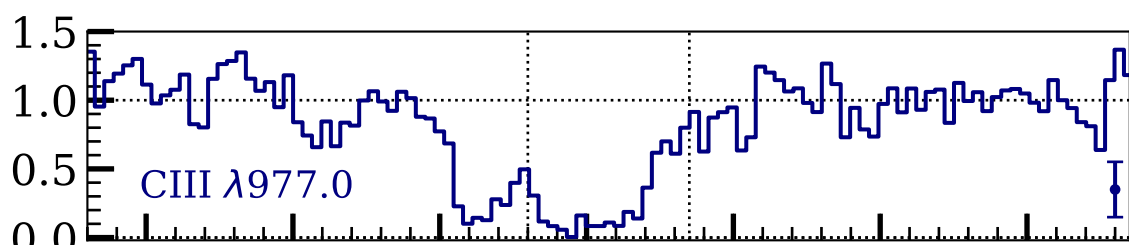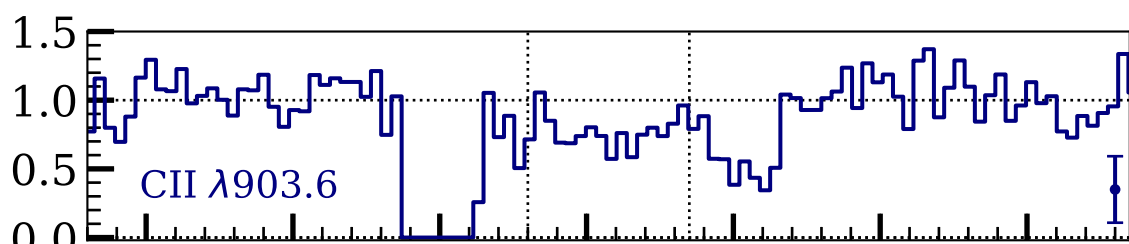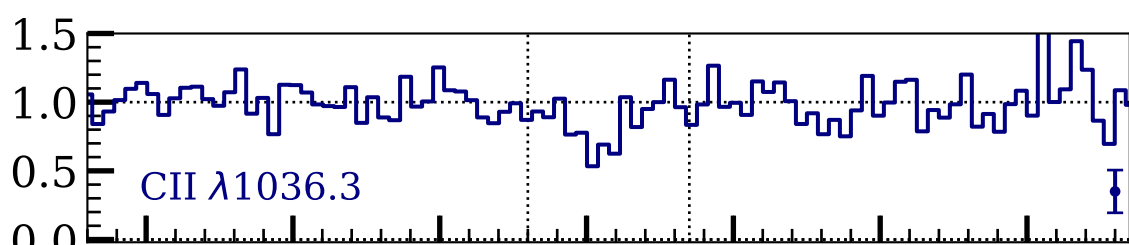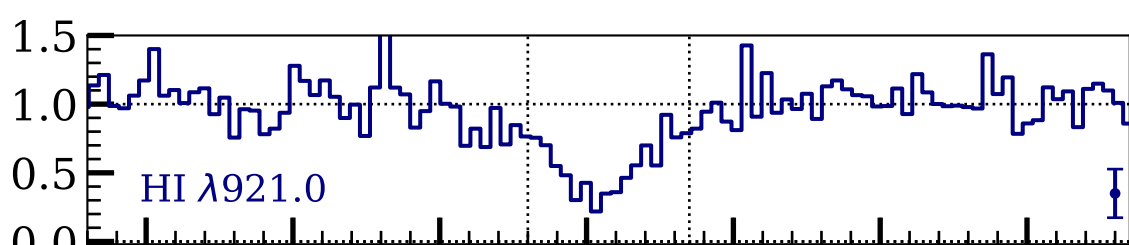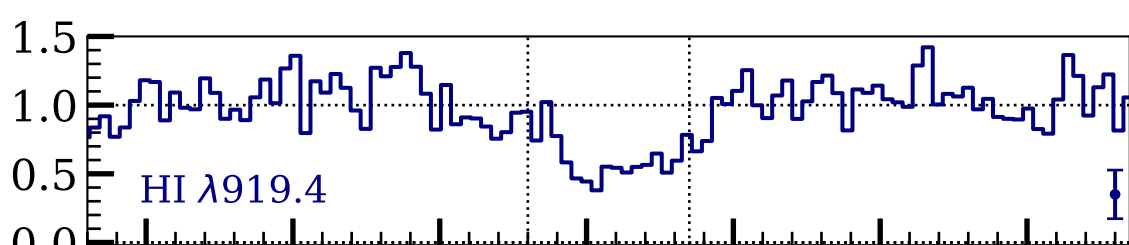

Rest-Frame Velocity ( $\text{km s}^{-1}$ )

J113910.70-135044.0,  $z=0.319498$ , RF=1

Normalized Flux

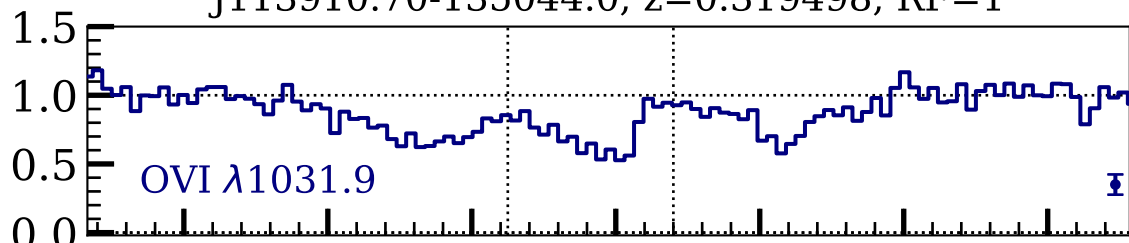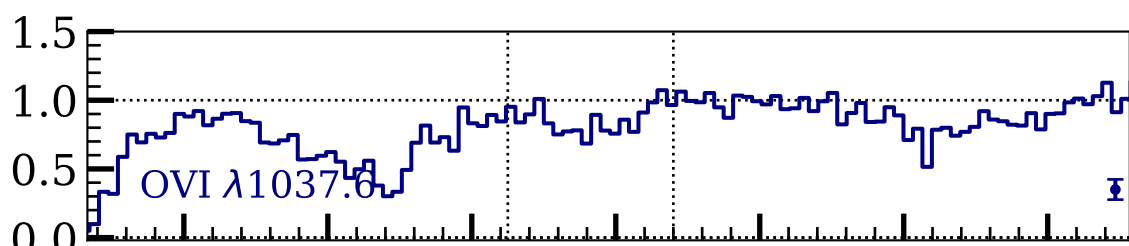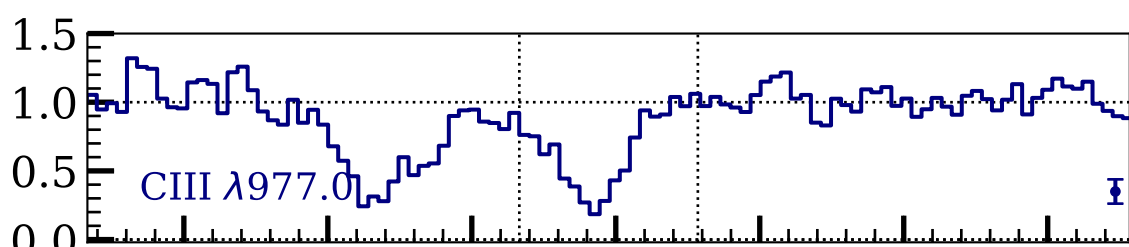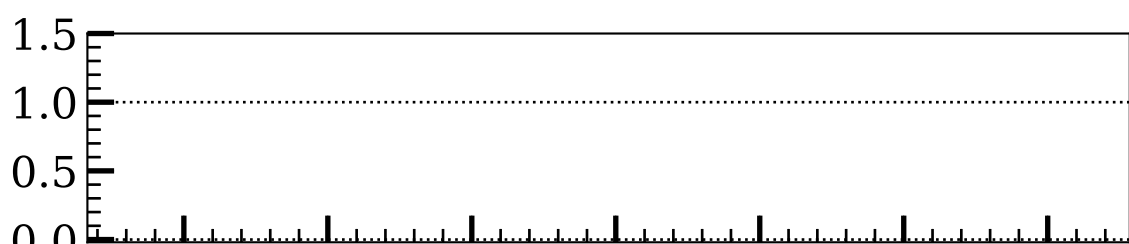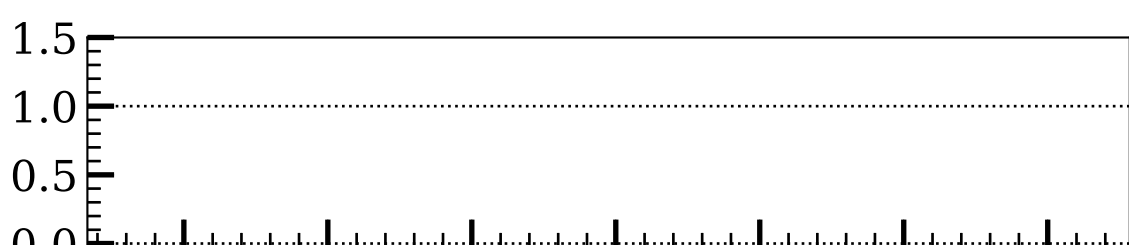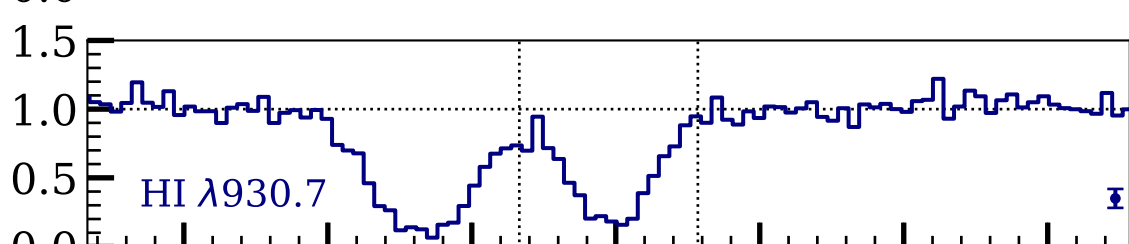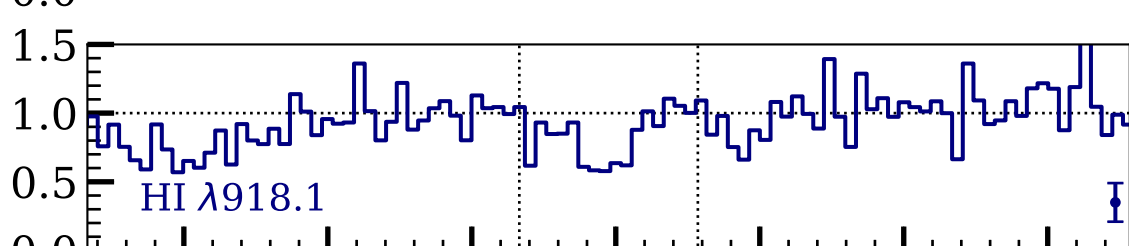

Rest-Frame Velocity ( $\text{km s}^{-1}$ )

J113956.98+654749.1,  $z=0.325653$ , RF=1

Normalized Flux

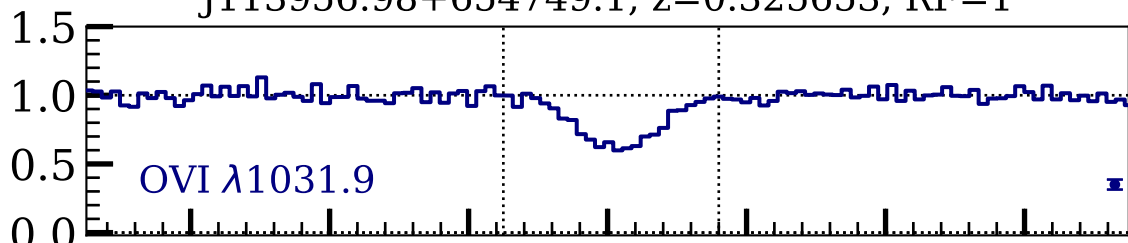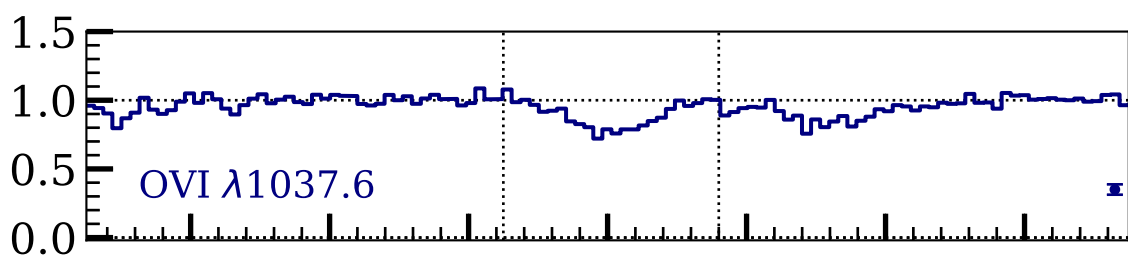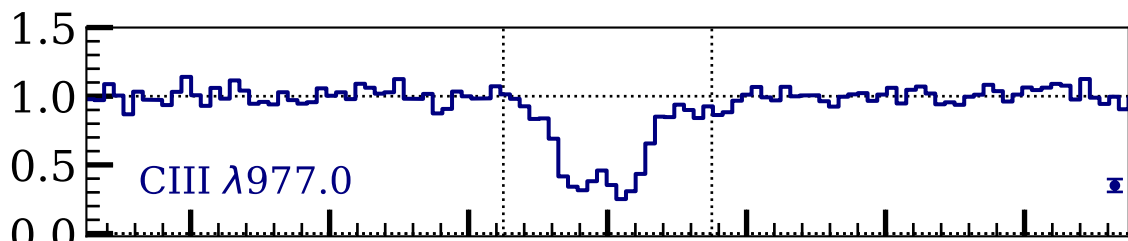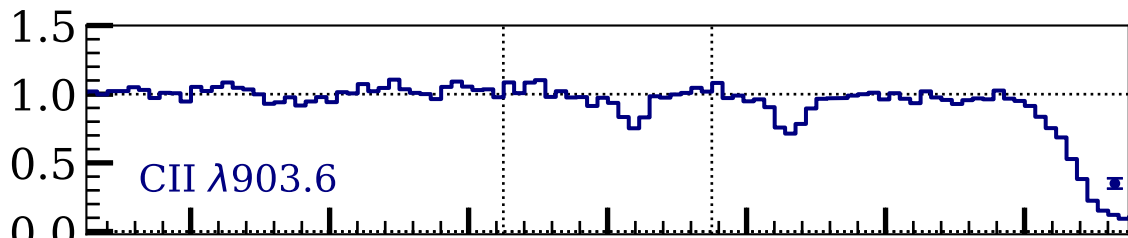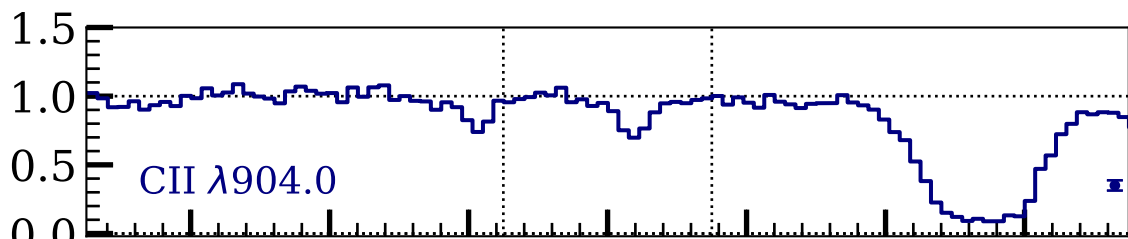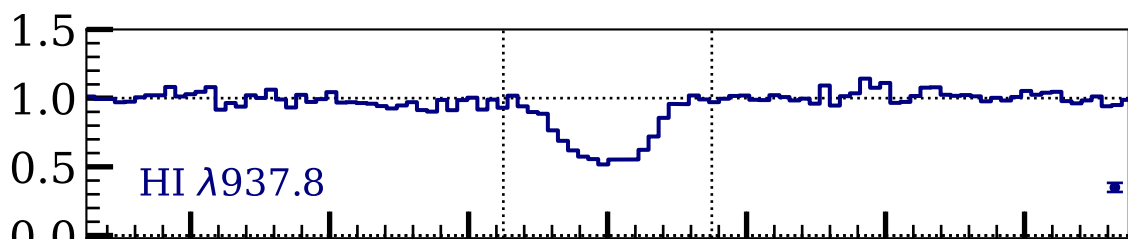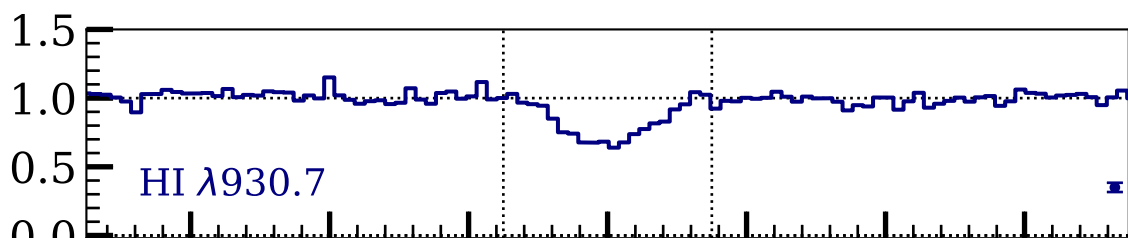

Rest-Frame Velocity ( $\text{km s}^{-1}$ )

J113956.98+654749.1,  $z=0.527941$ , RF=1

Normalized Flux

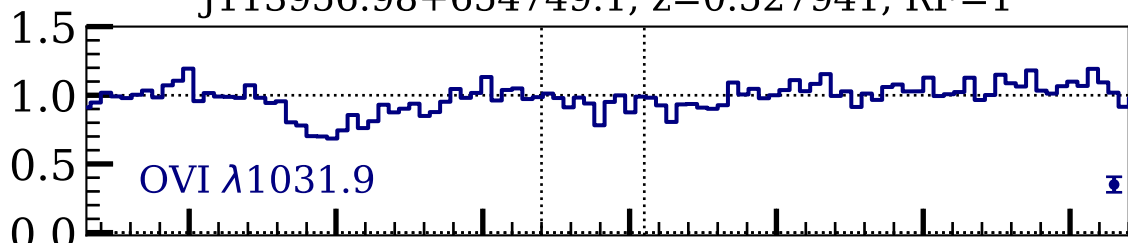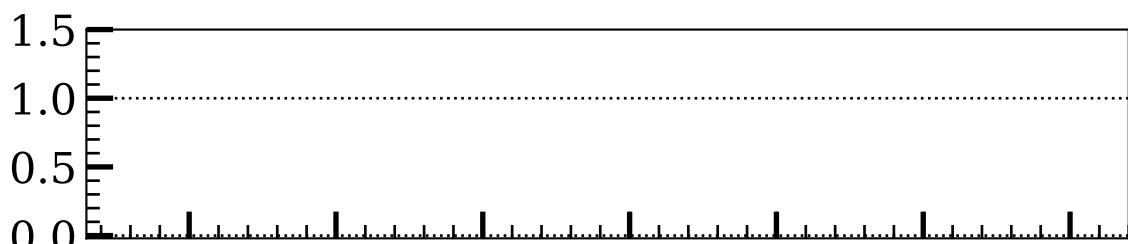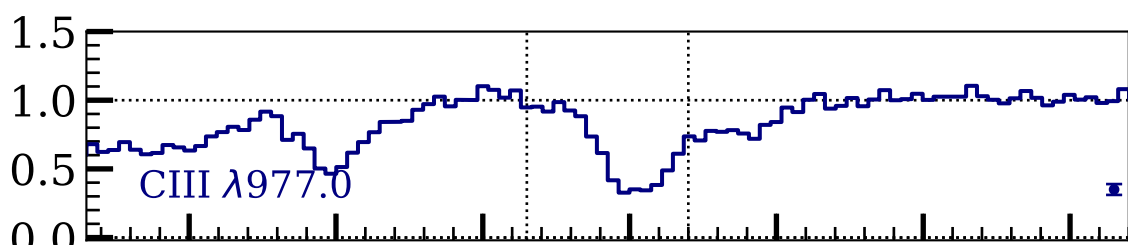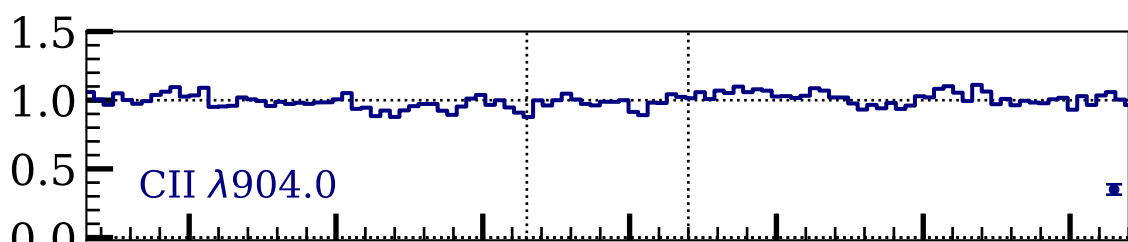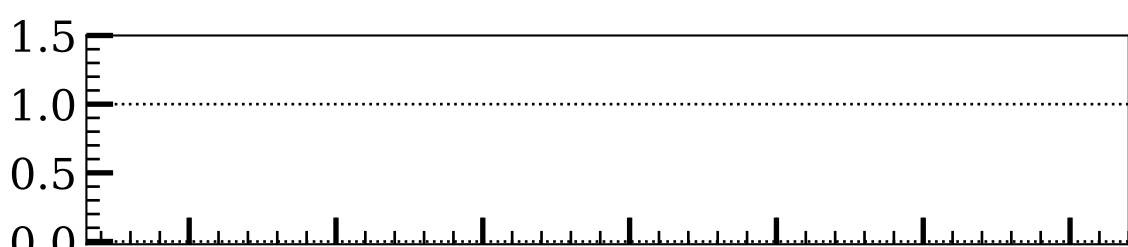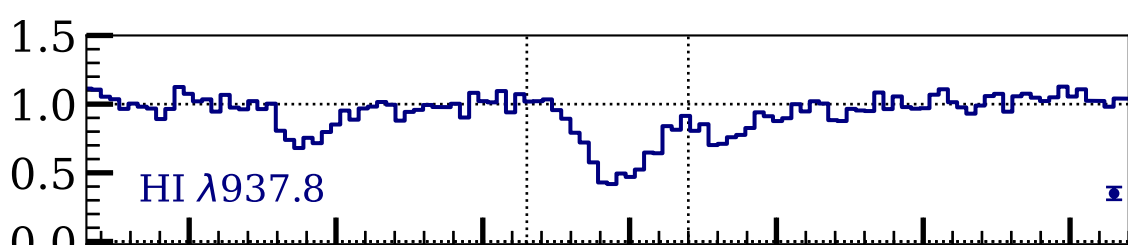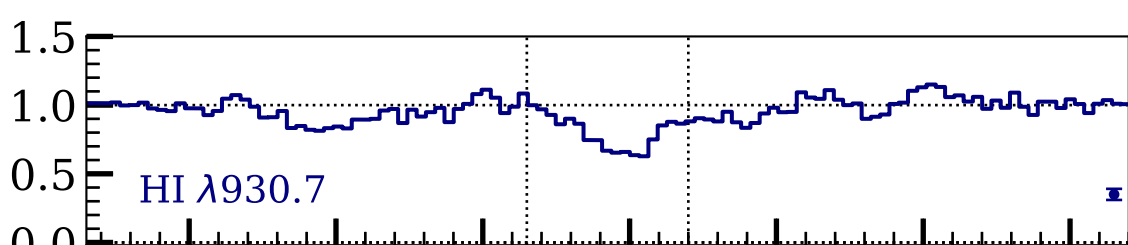

Rest-Frame Velocity ( $\text{km s}^{-1}$ )



J115120.46+543733.0,  $z=0.252465$ , RF=1

Normalized Flux

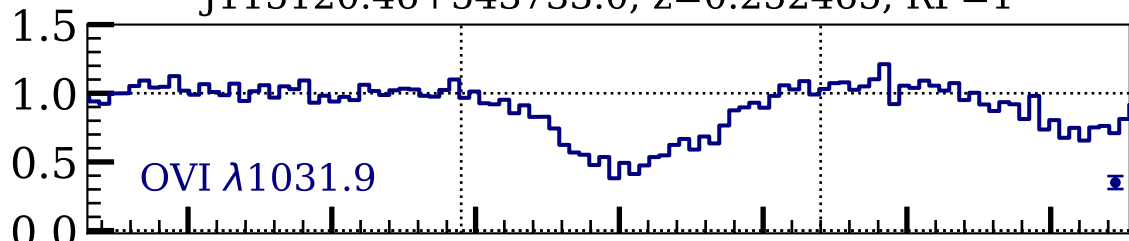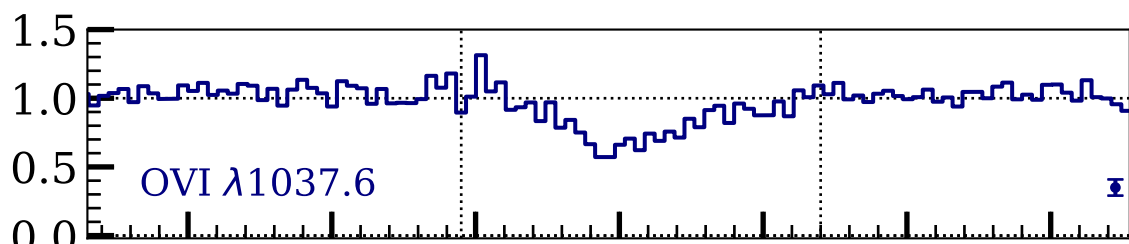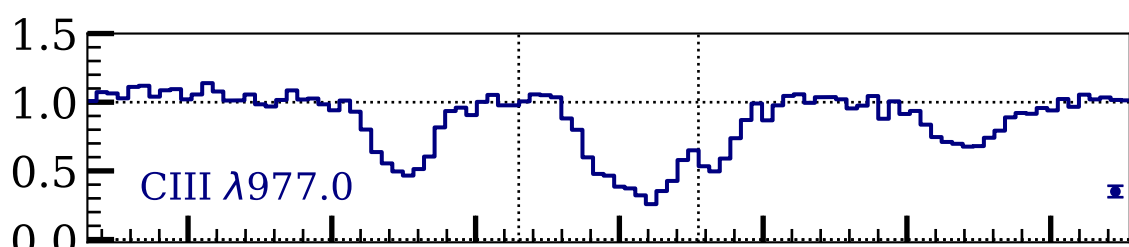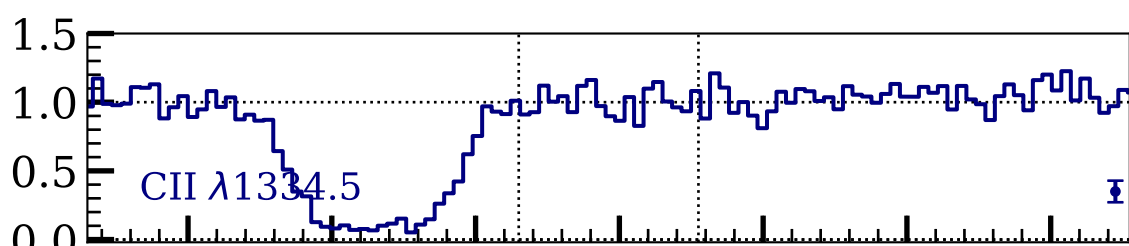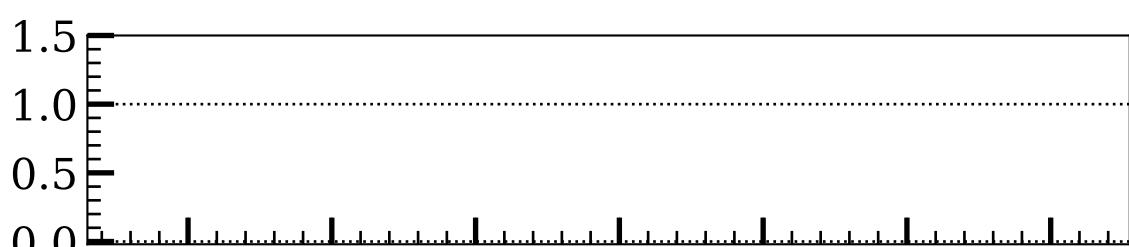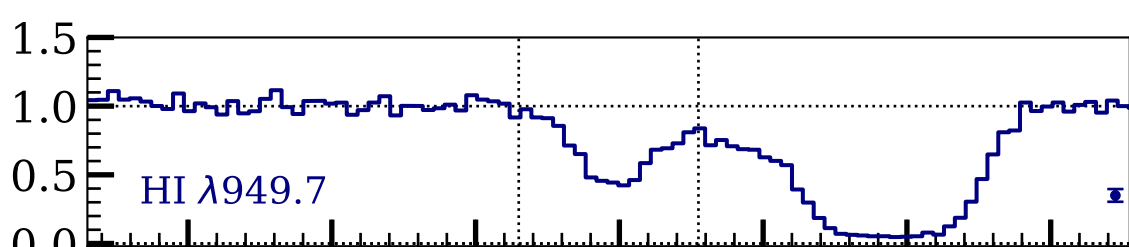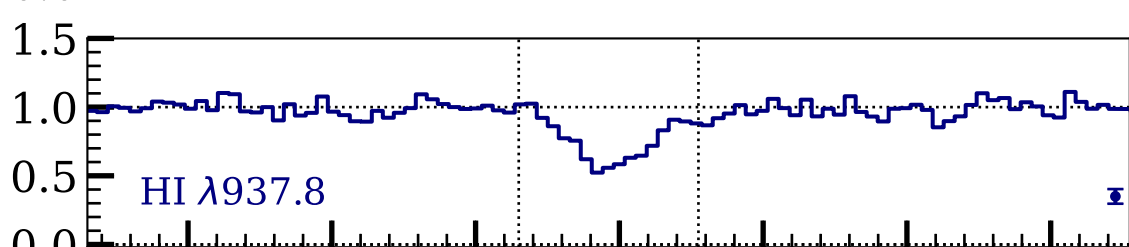

Rest-Frame Velocity ( $\text{km s}^{-1}$ )

J115120.46+543733.0,  $z=0.688567$ , RF=1

Normalized Flux

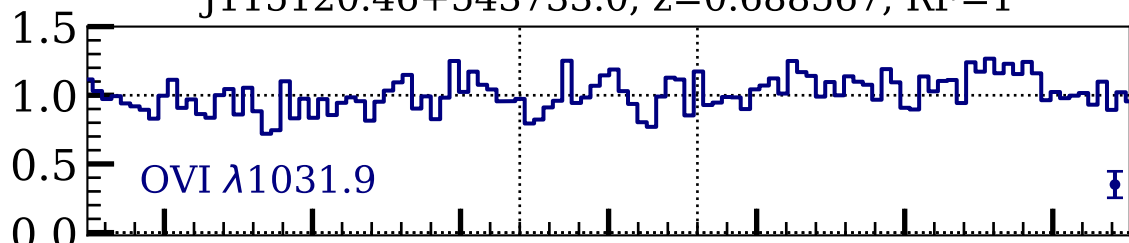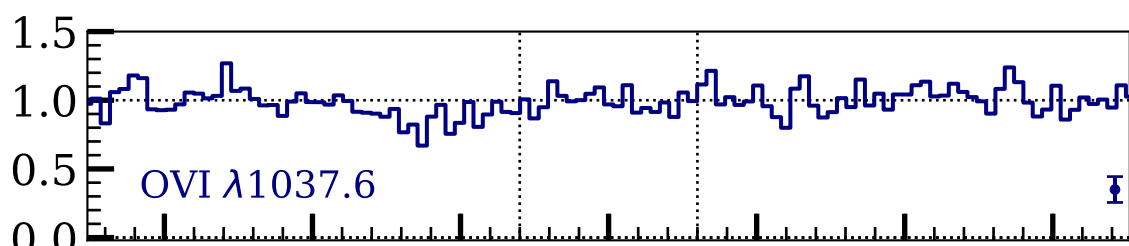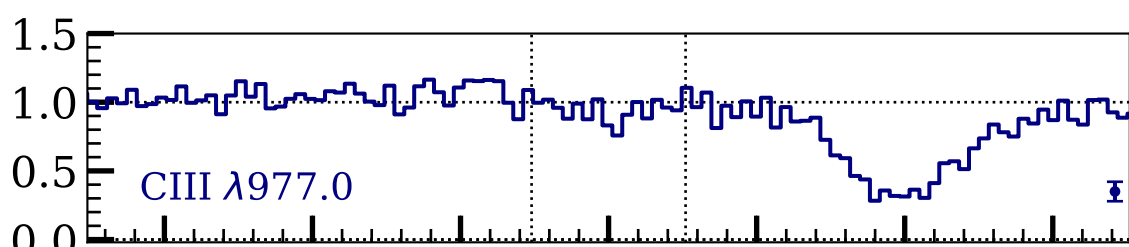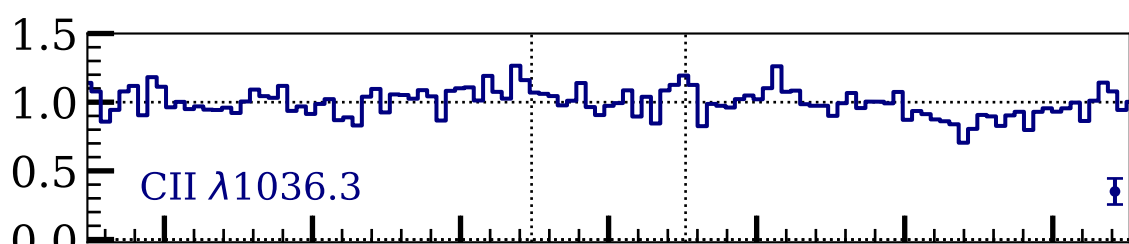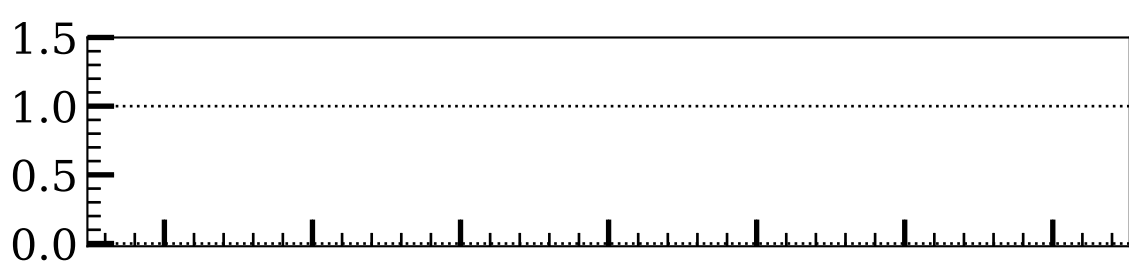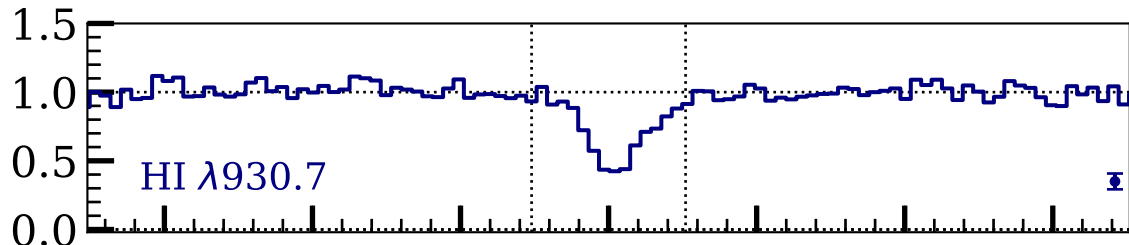

Rest-Frame Velocity ( $\text{km s}^{-1}$ )

J120158.75-135459.9,  $z=0.409358$ , RF=0

Normalized Flux

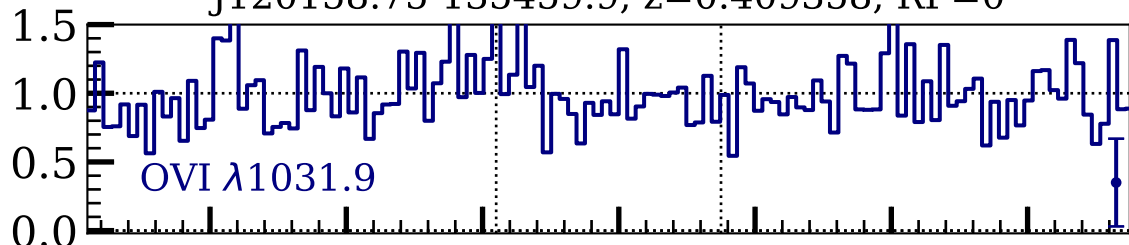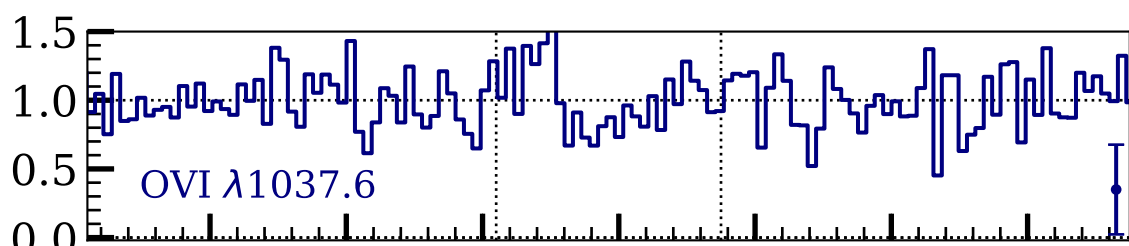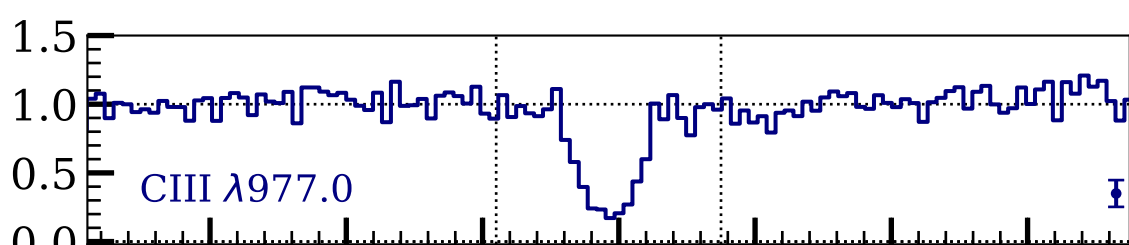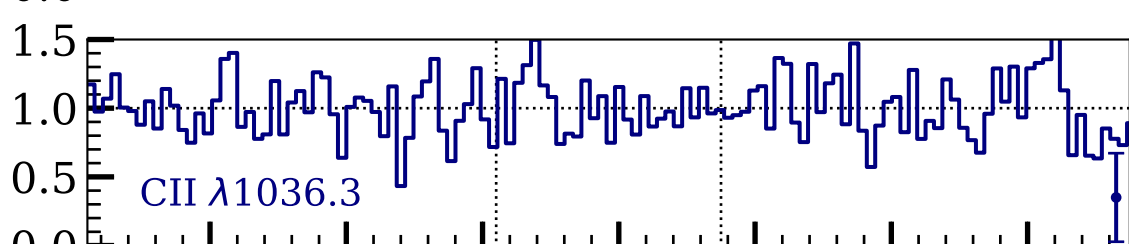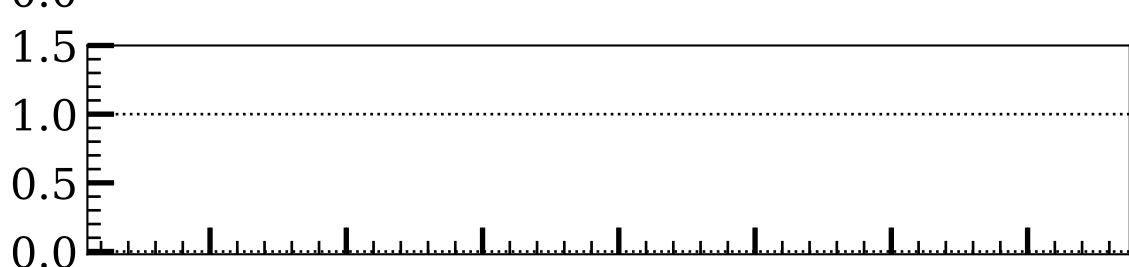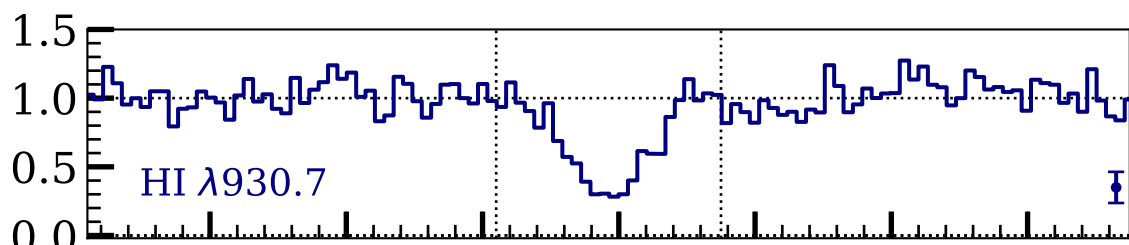

-300 -200 -100 0 100 200 300

Rest-Frame Velocity ( $\text{km s}^{-1}$ )

J121430.55+082508.1,  $z=0.324710$ , RF=1

Normalized Flux

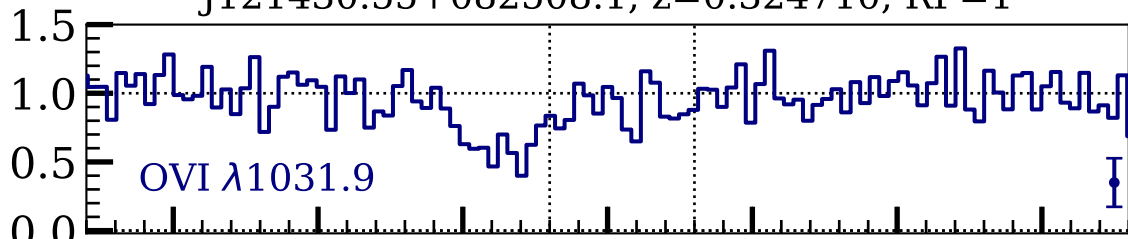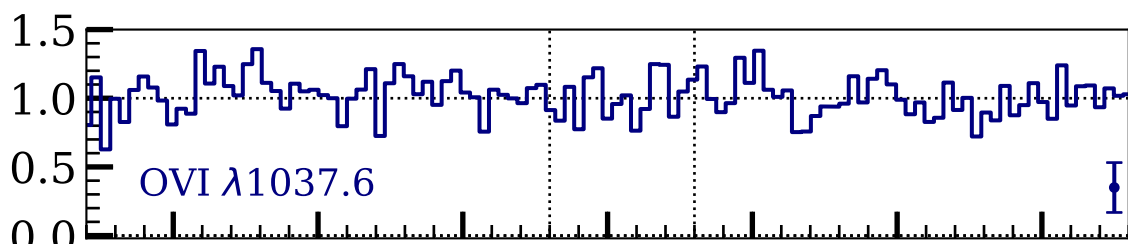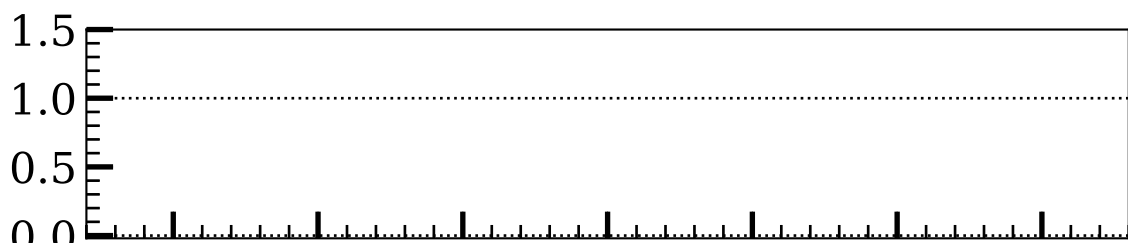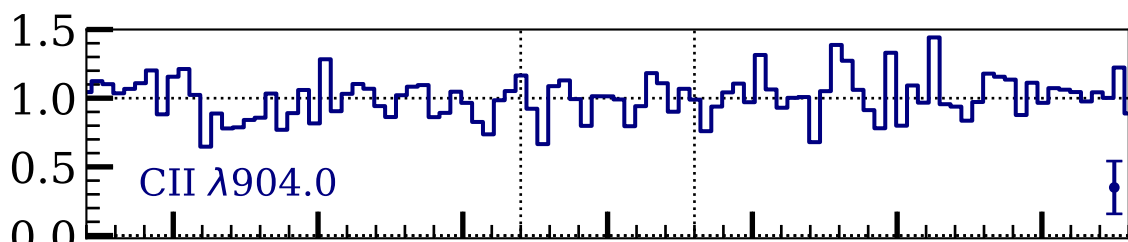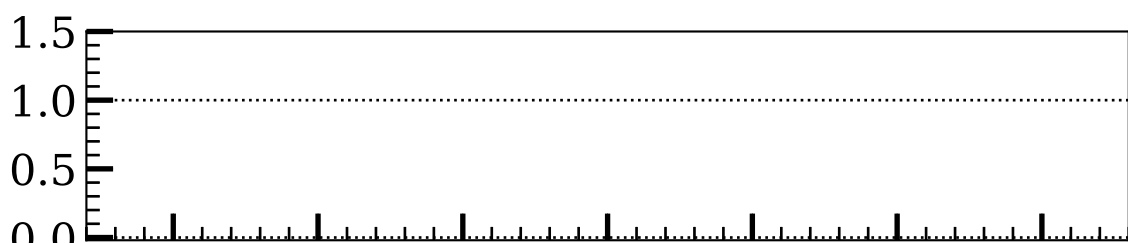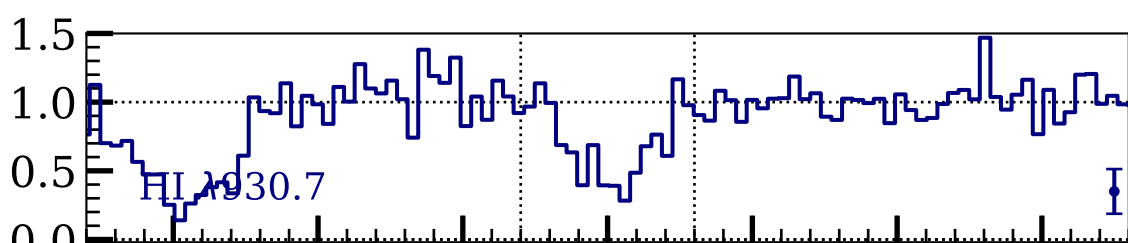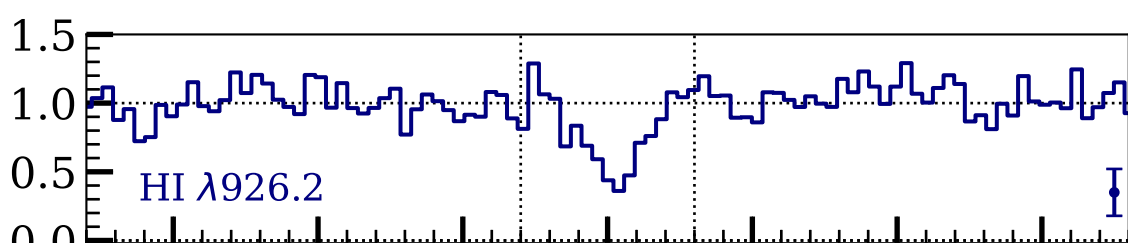

Rest-Frame Velocity ( $\text{km s}^{-1}$ )

J121430.55+082508.1,  $z=0.383836$ , RF=1

Normalized Flux

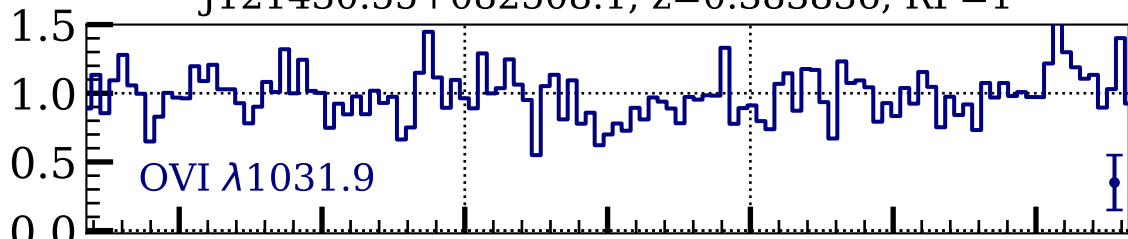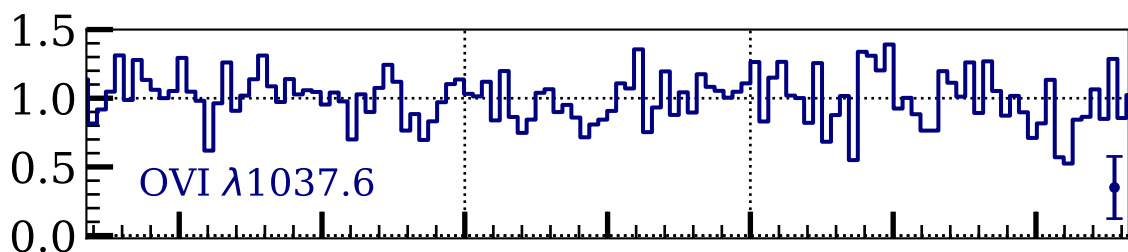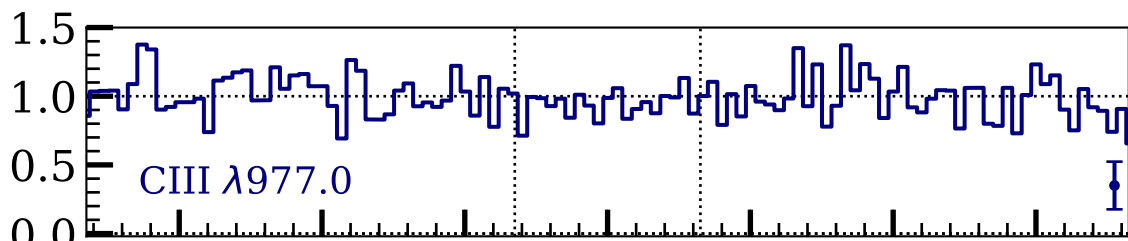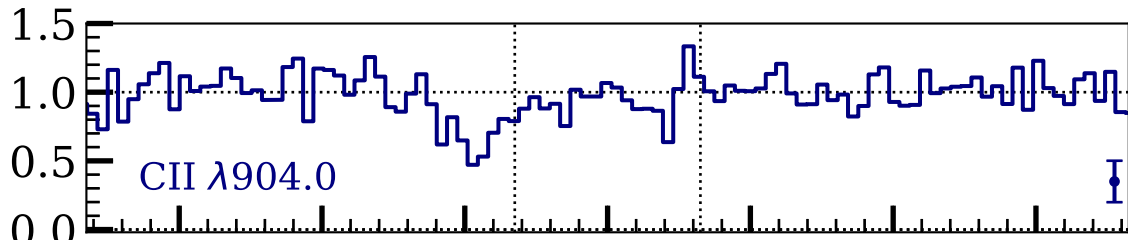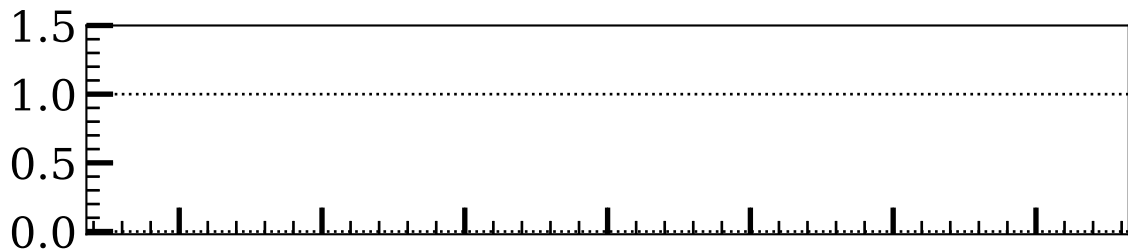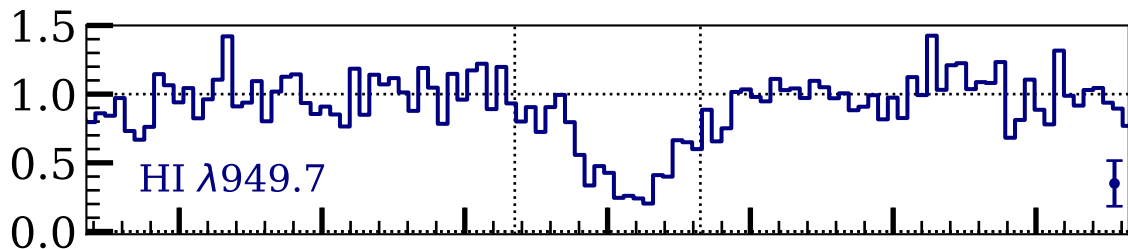

Rest-Frame Velocity ( $\text{km s}^{-1}$ )

J121640.56+071224.3,  $z=0.382433$ , RF=0

Normalized Flux

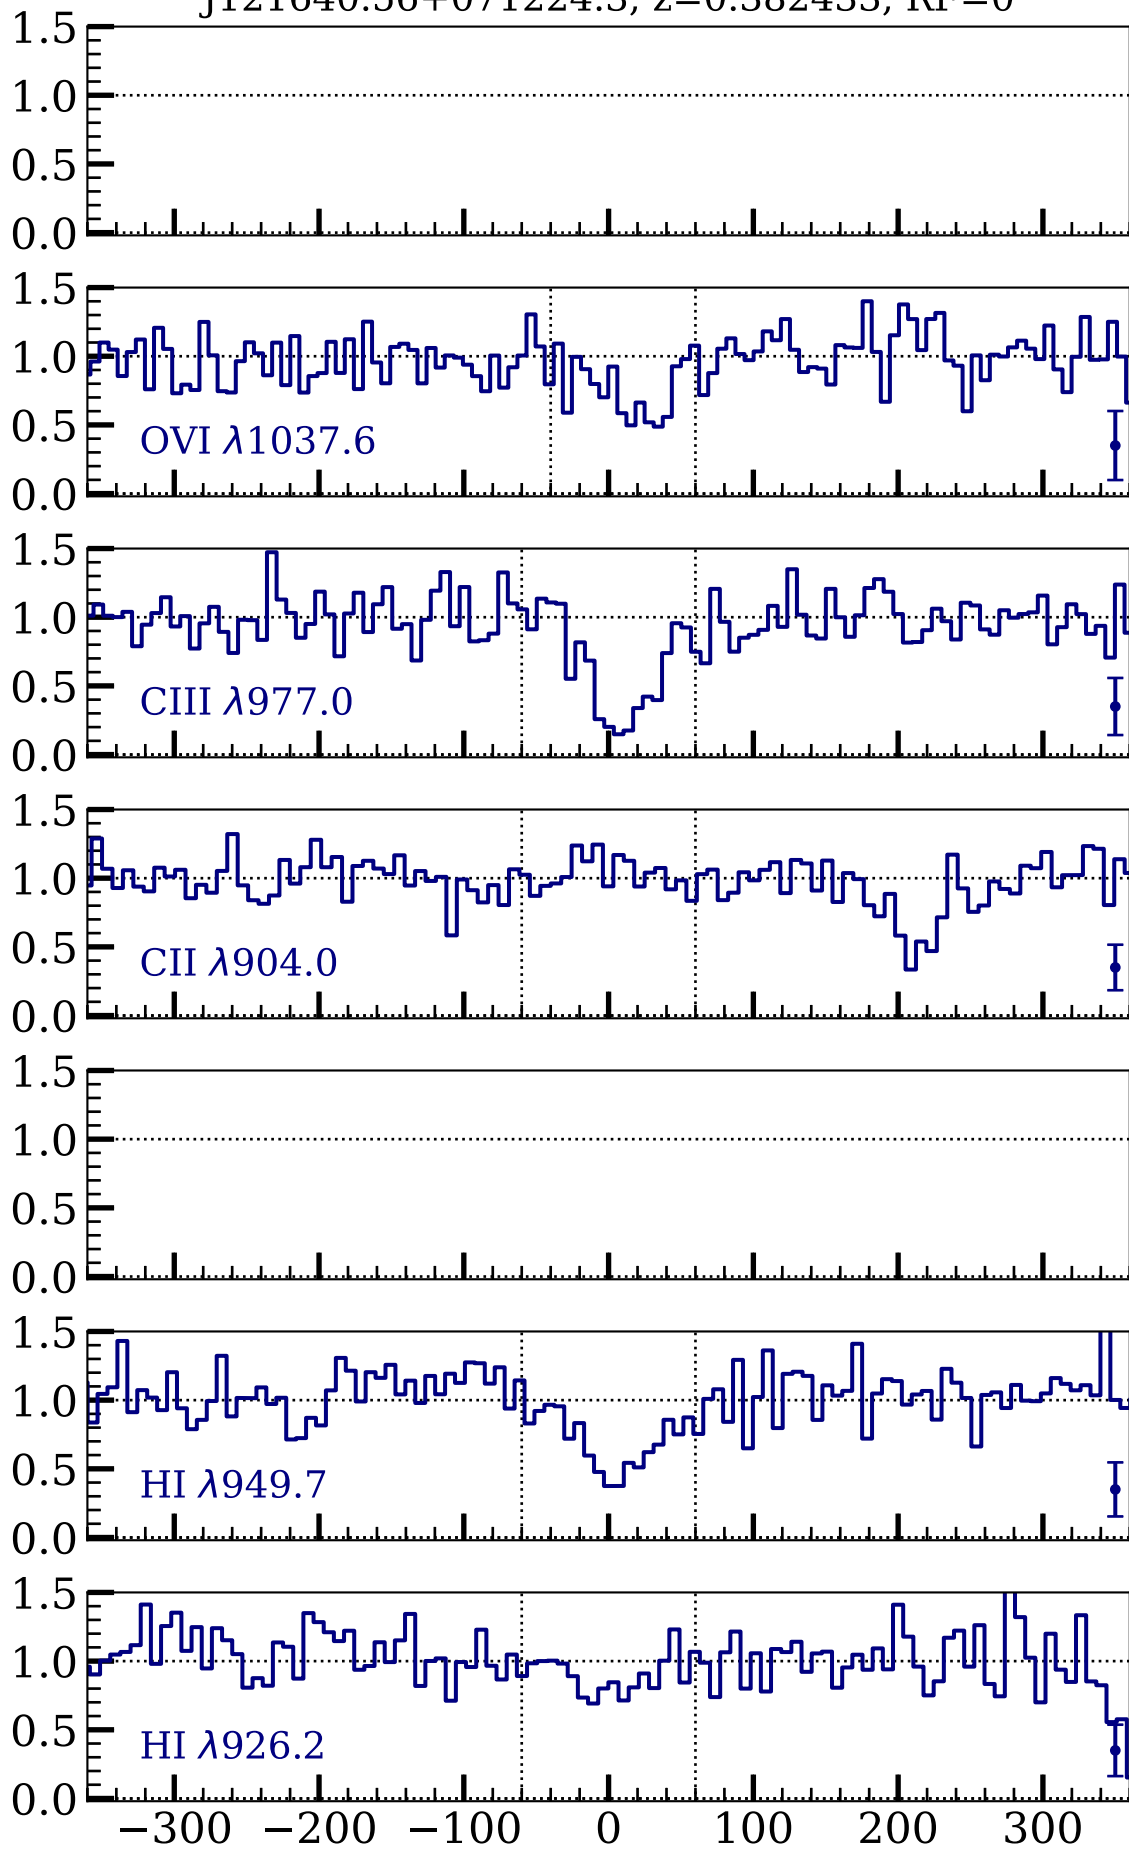

Rest-Frame Velocity (km s<sup>-1</sup>)

J121920.93+063838.5,  $z=0.282308$ , RF=1

Normalized Flux

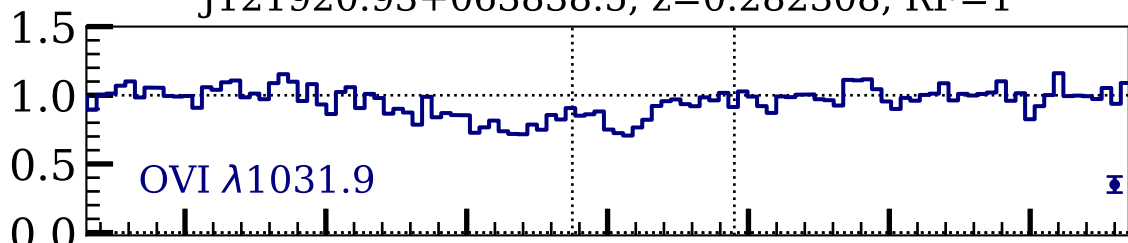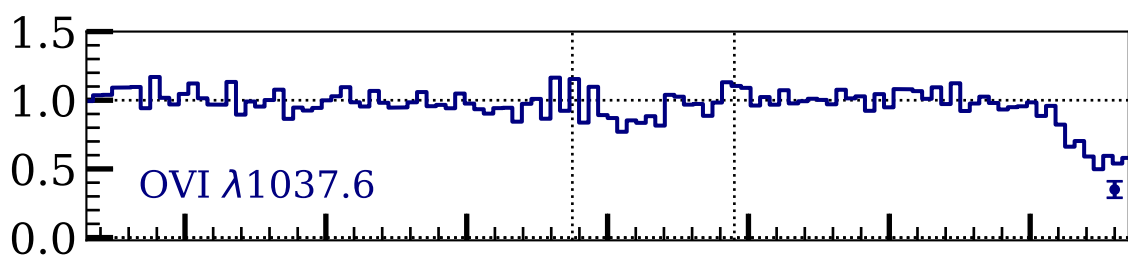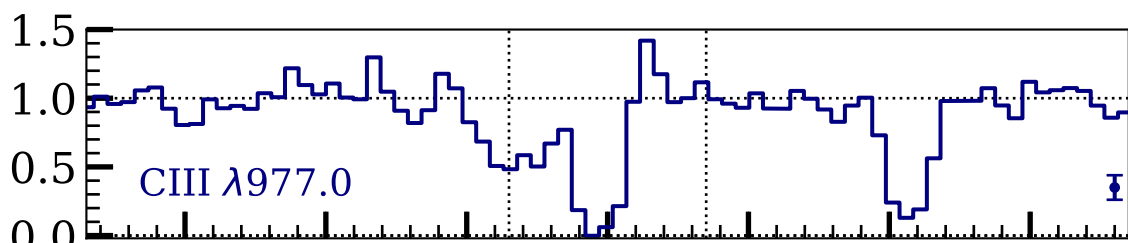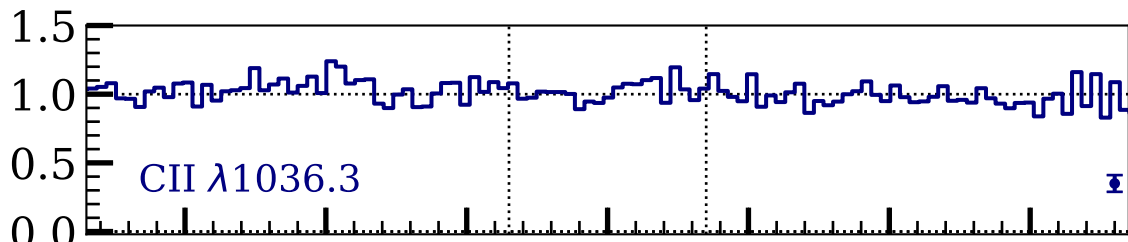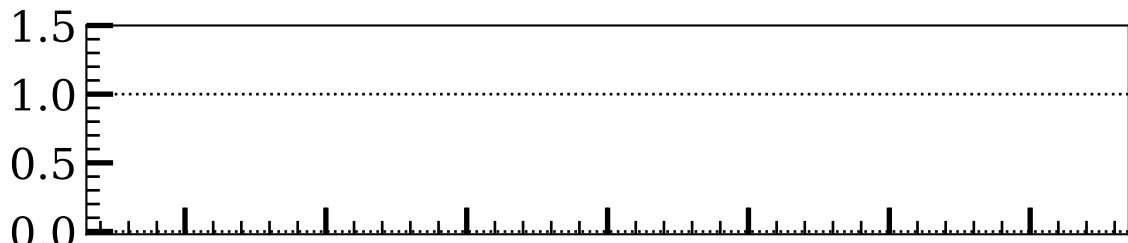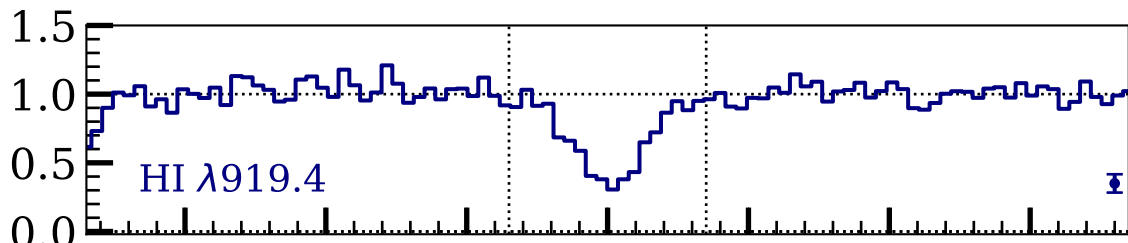

Rest-Frame Velocity ( $\text{km s}^{-1}$ )

J122317.79+092306.9,  $z=0.379535$ , RF=1

Normalized Flux

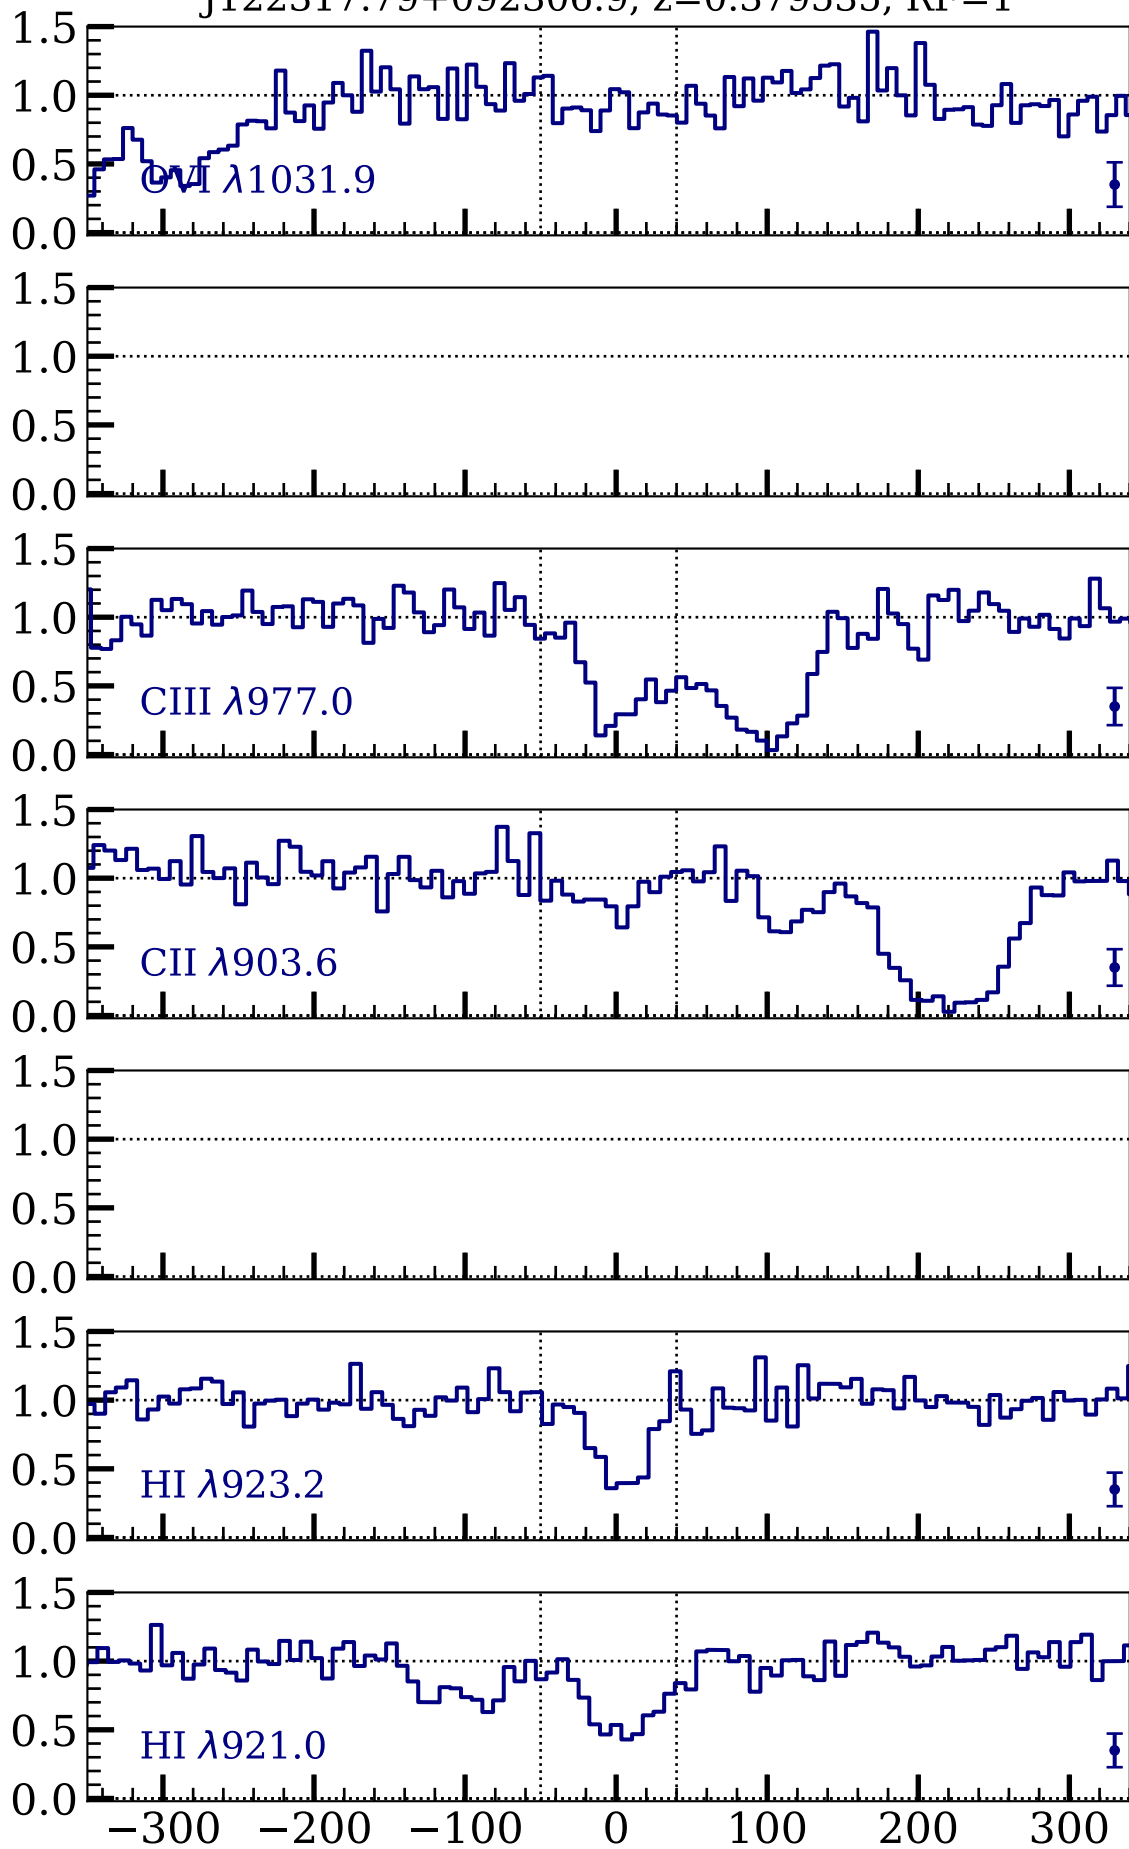

Rest-Frame Velocity (km s<sup>-1</sup>)



J122454.44+212246.3,  $z=0.378447$ , RF=1

Normalized Flux

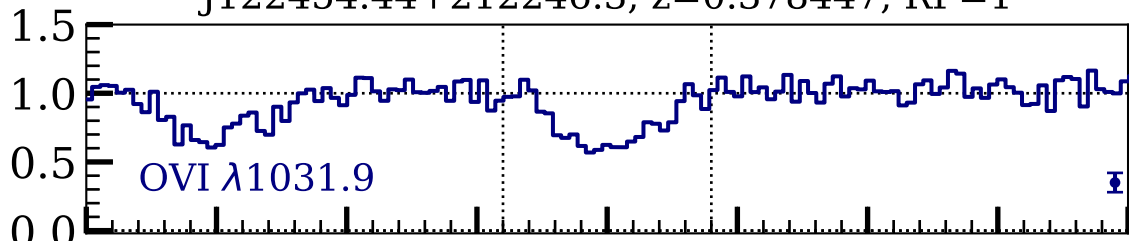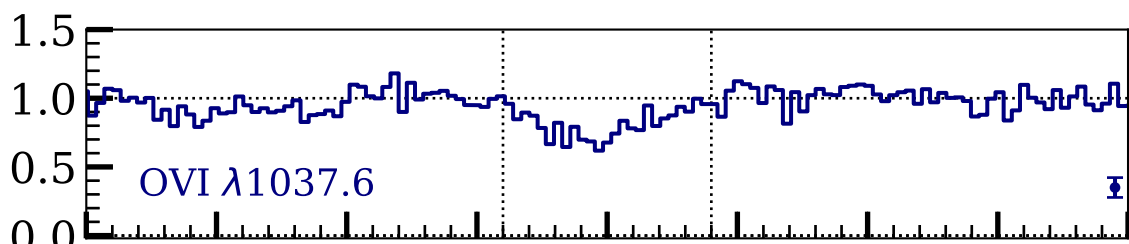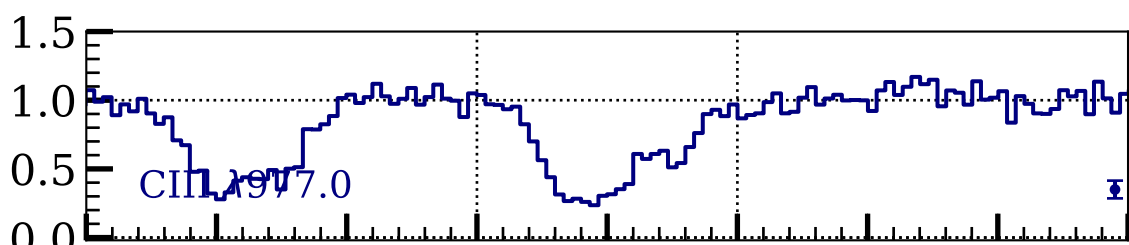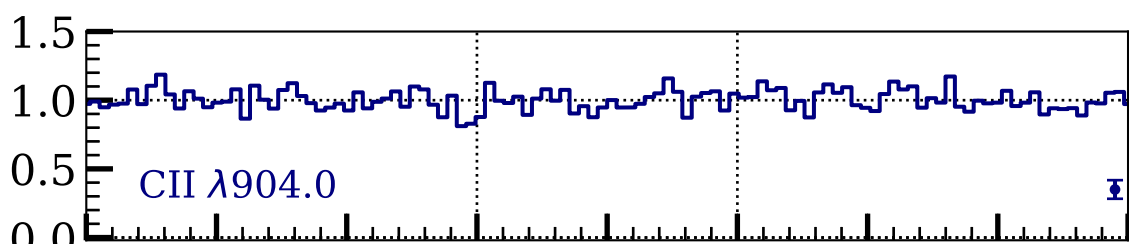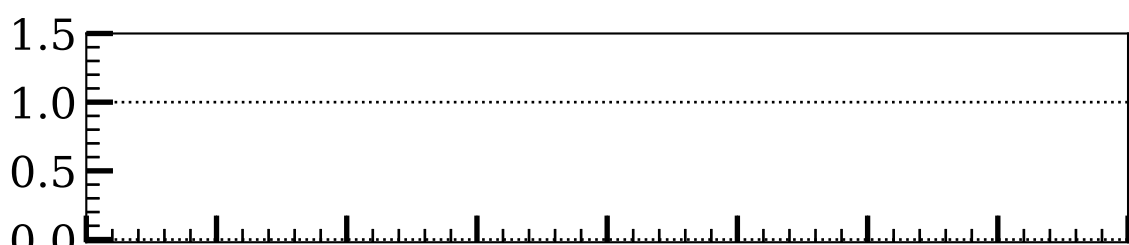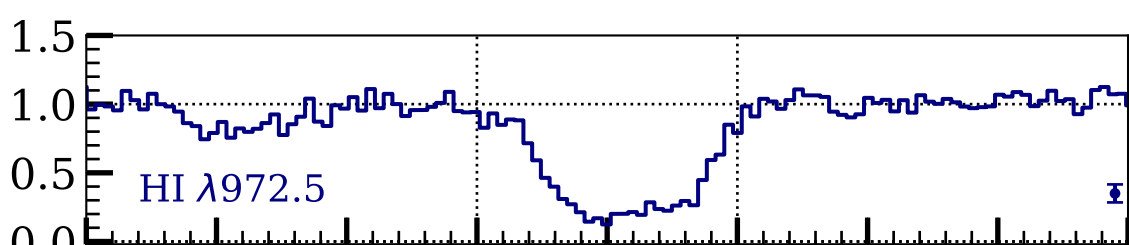

Rest-Frame Velocity ( $\text{km s}^{-1}$ )

J122454.44+212246.3,  $z=0.420788$ , RF=1

Normalized Flux

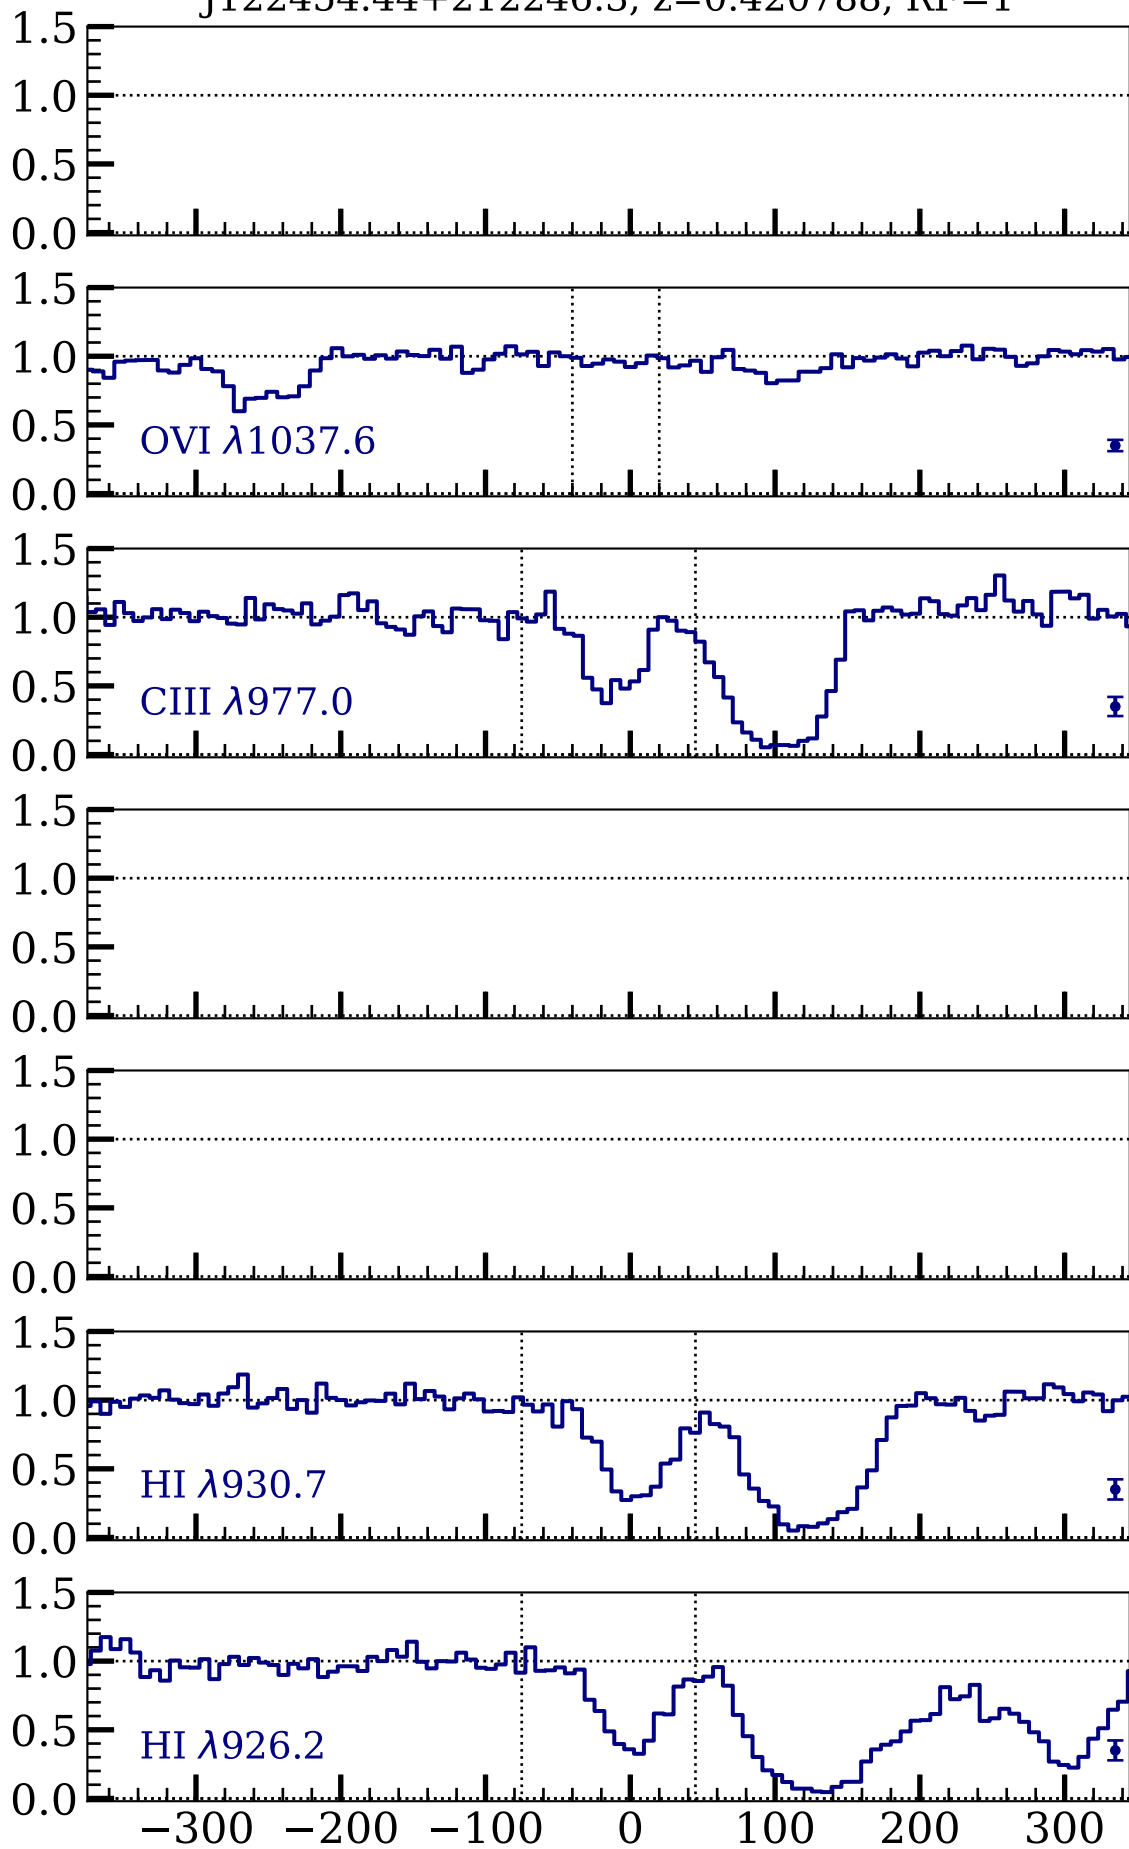

Rest-Frame Velocity (km s<sup>-1</sup>)

J122454.44+212246.3,  $z=0.421357$ , RF=1

Normalized Flux

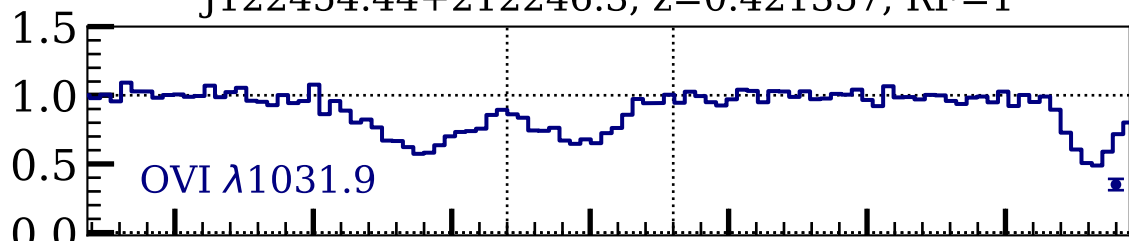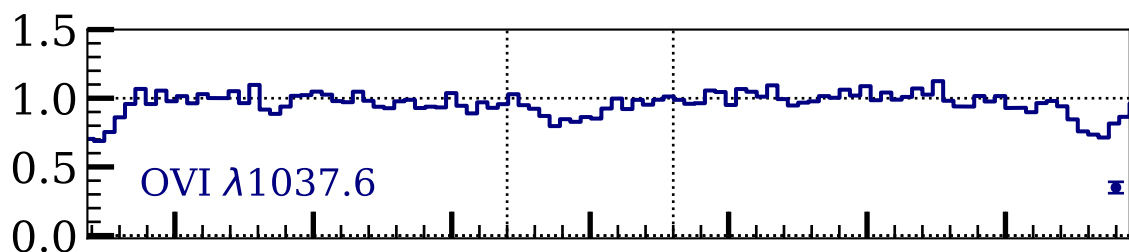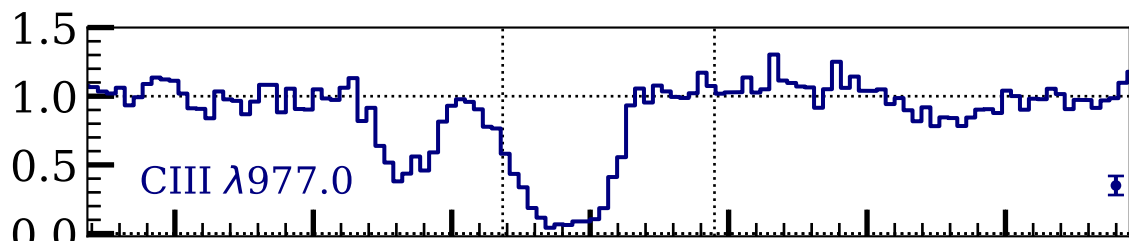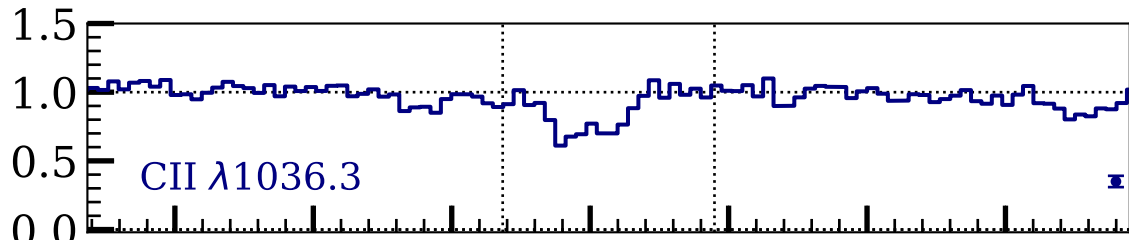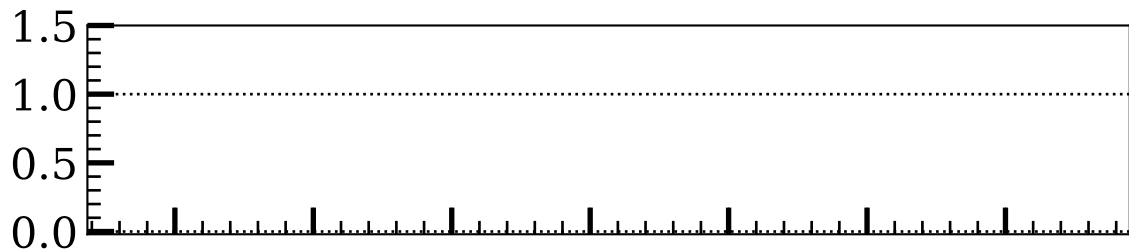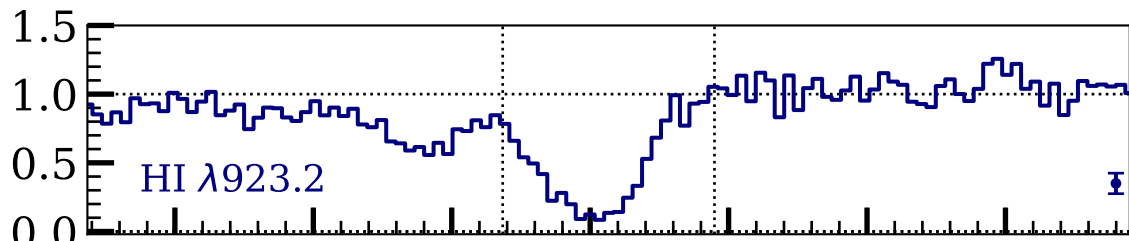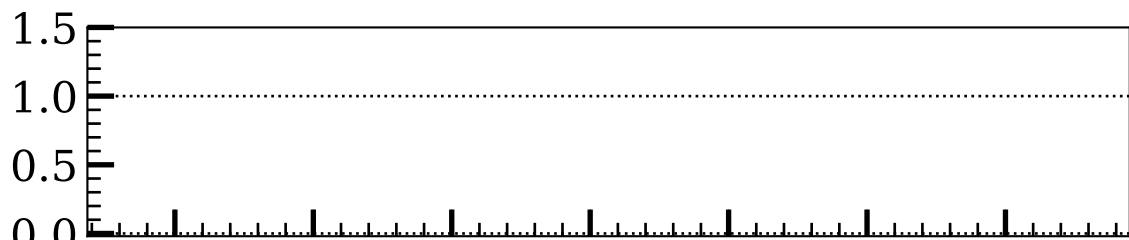

Rest-Frame Velocity ( $\text{km s}^{-1}$ )

J122512.93+121835.7,  $z=0.324970$ , RF=1

Normalized Flux

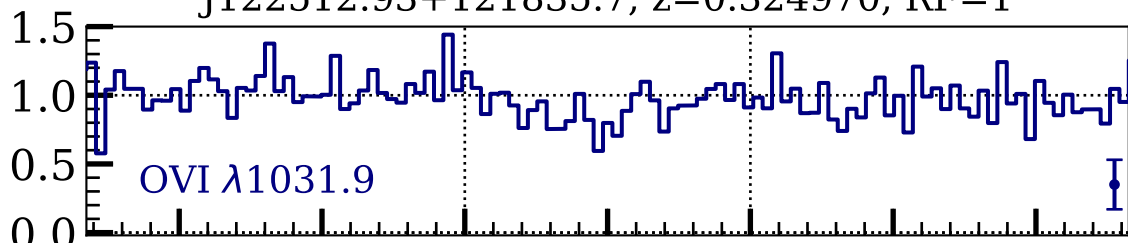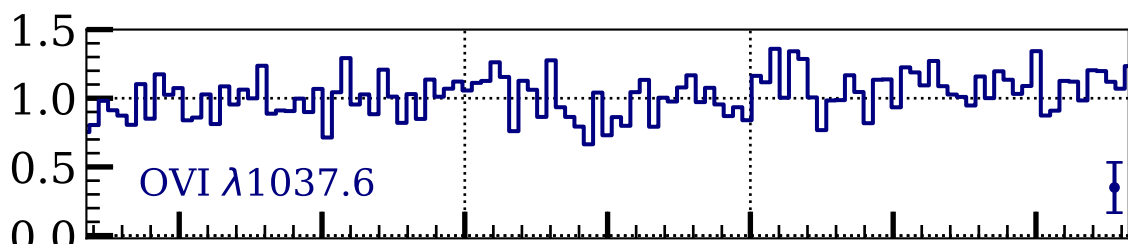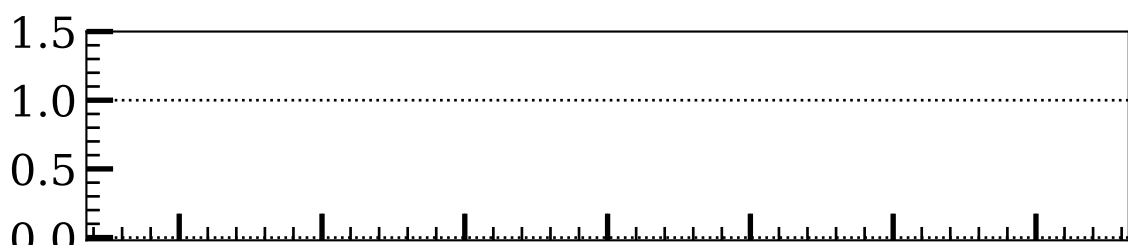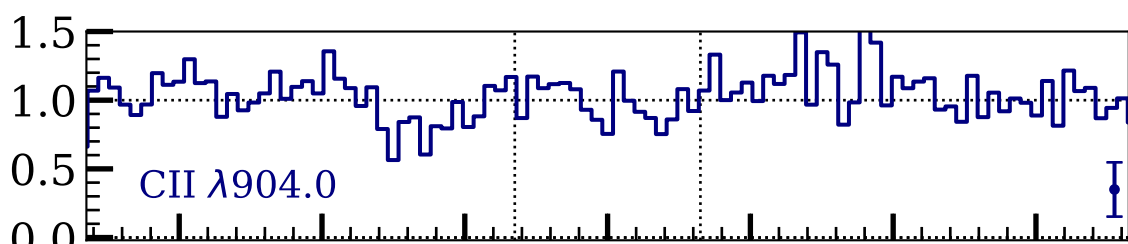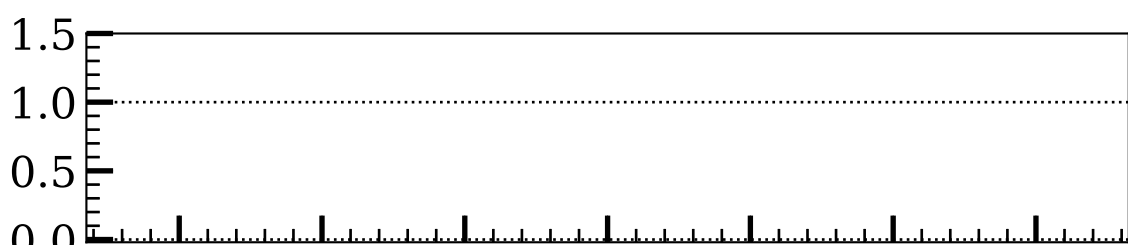

Rest-Frame Velocity (km s<sup>-1</sup>)

J123304.05-003134.1,  $z=0.318758$ , RF=1

Normalized Flux

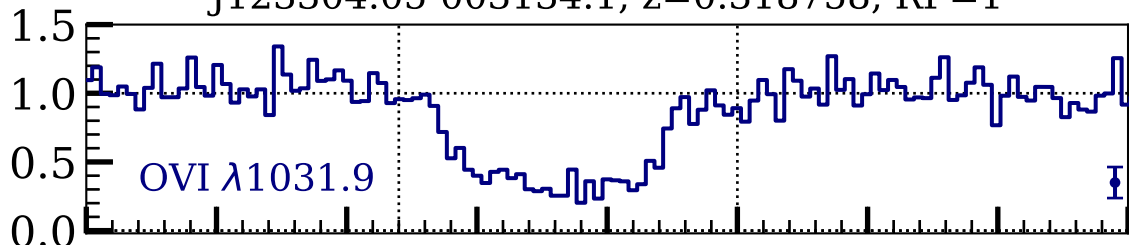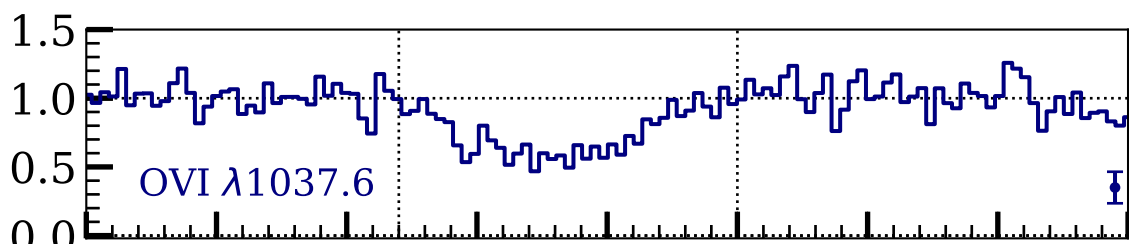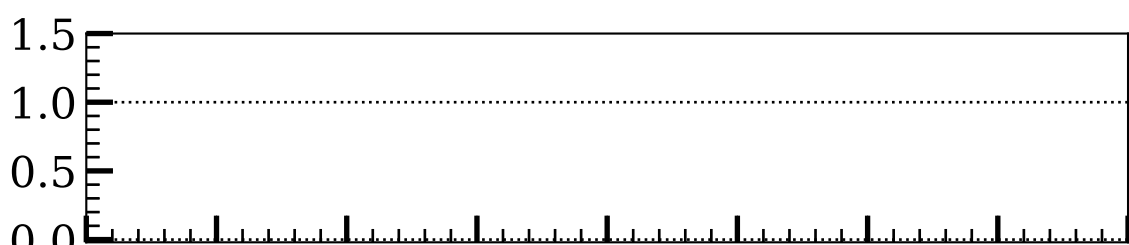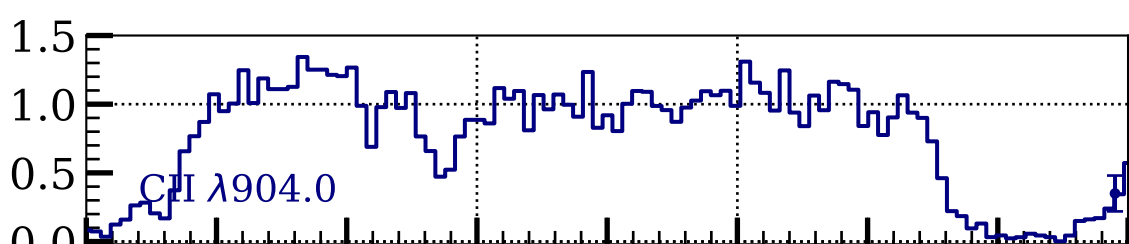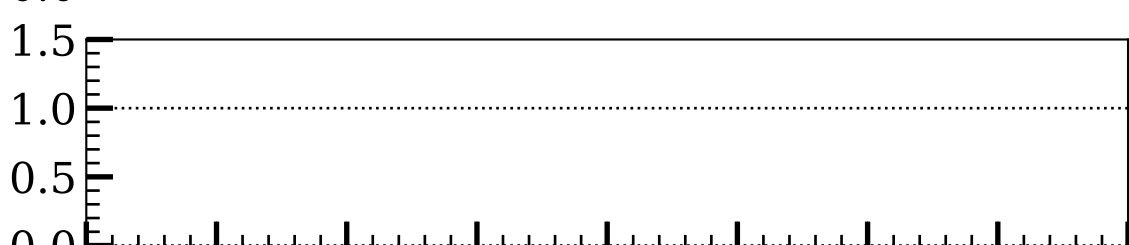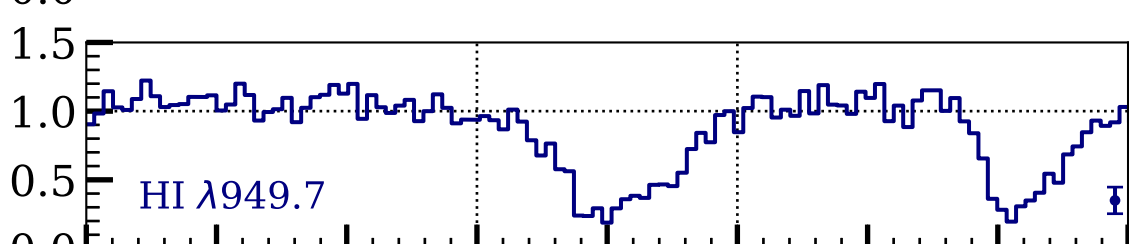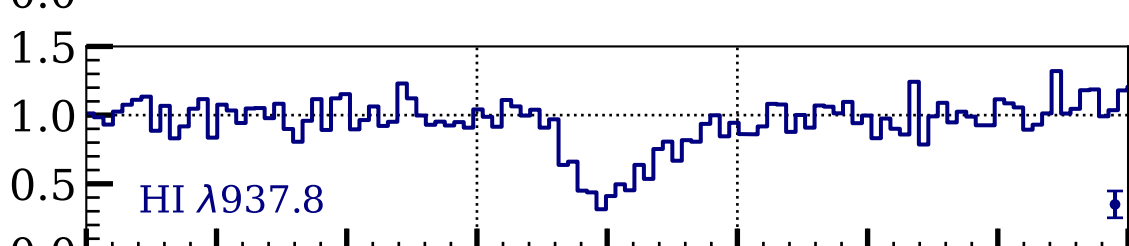

Rest-Frame Velocity ( $\text{km s}^{-1}$ )

J123335.07+475800.4,  $z=0.284947$ , RF=1

Normalized Flux

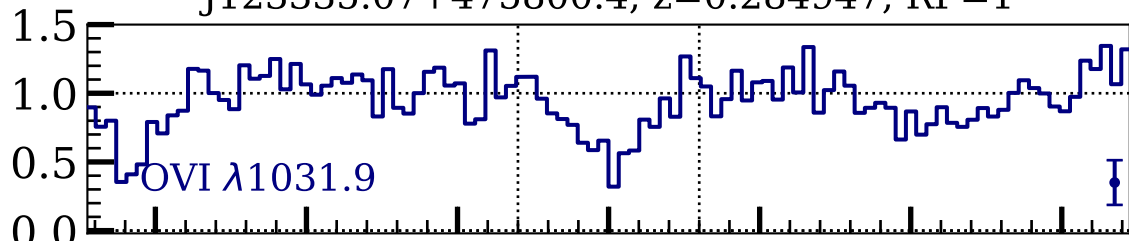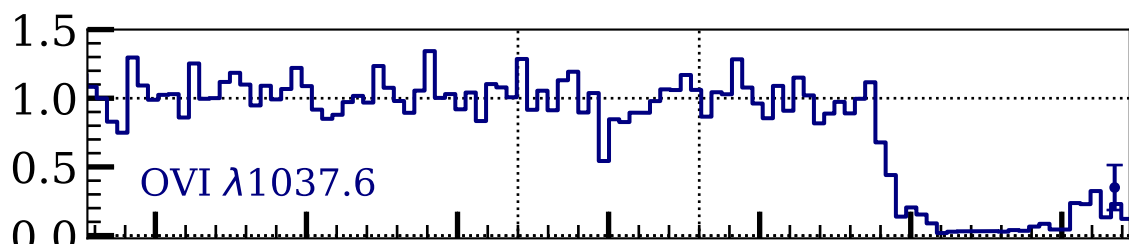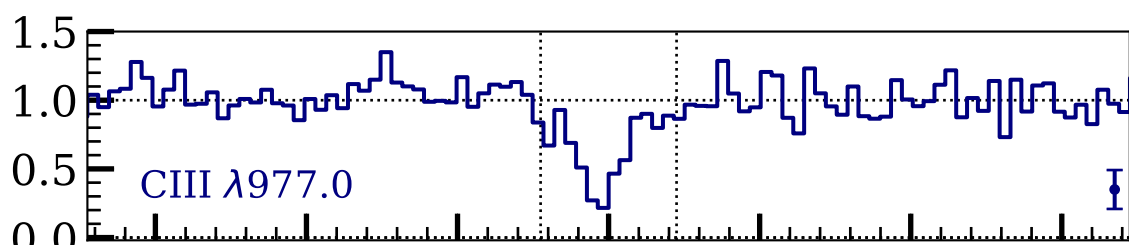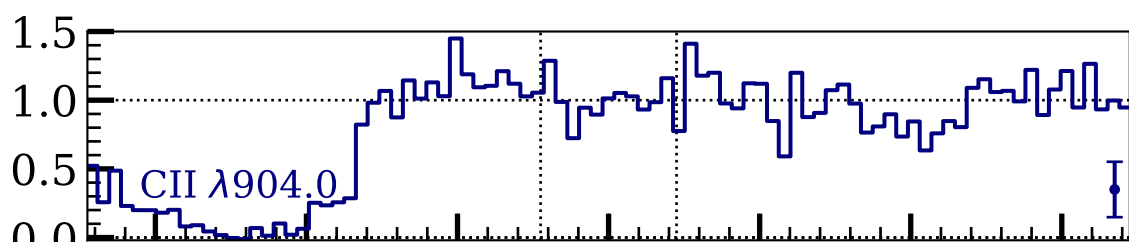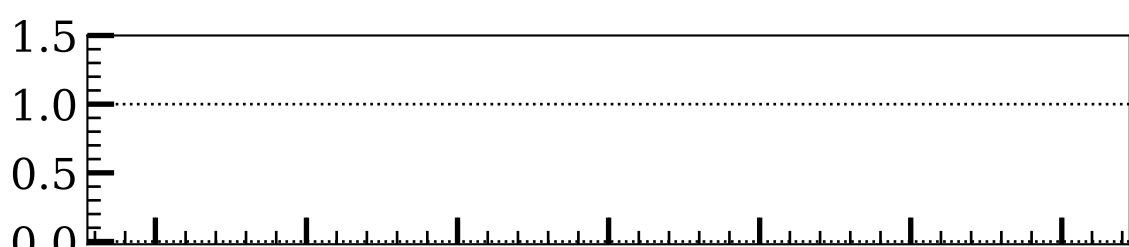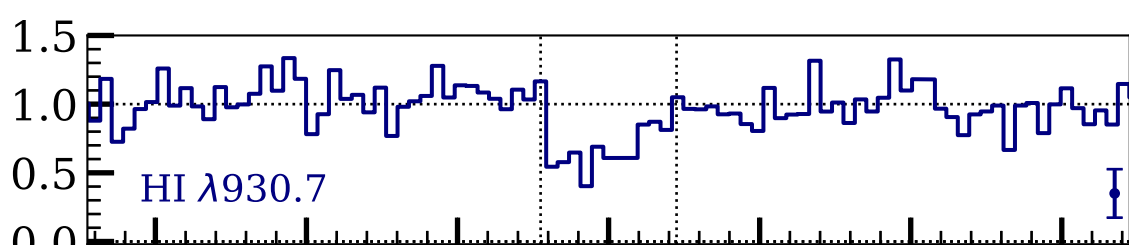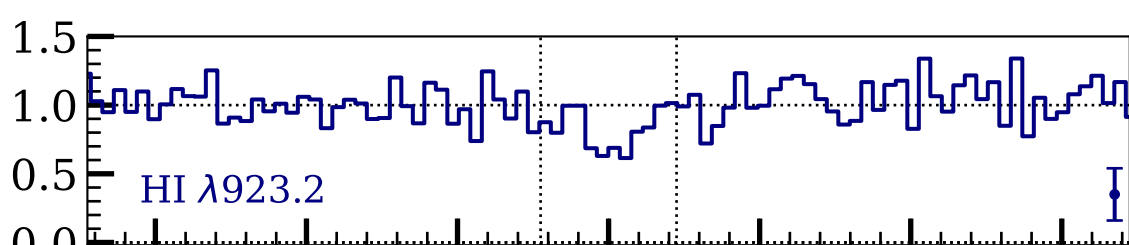

Rest-Frame Velocity ( $\text{km s}^{-1}$ )

J124154.02+572107.3,  $z=0.217947$ , RF=1

Normalized Flux

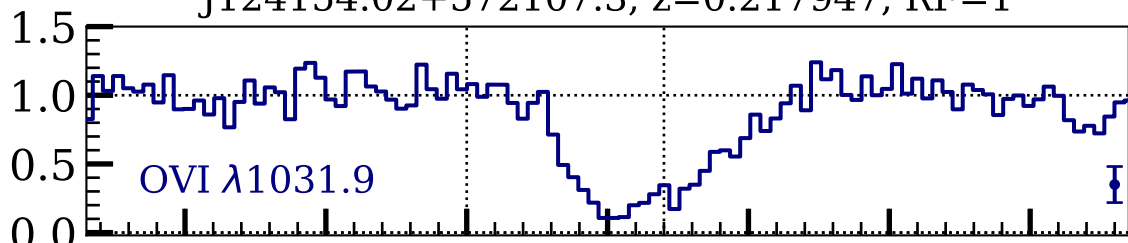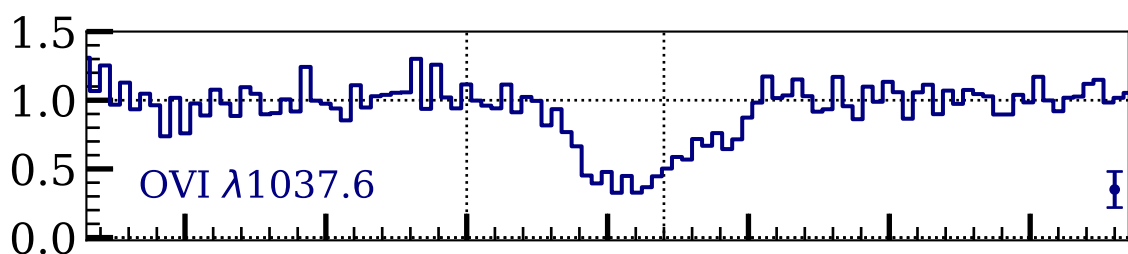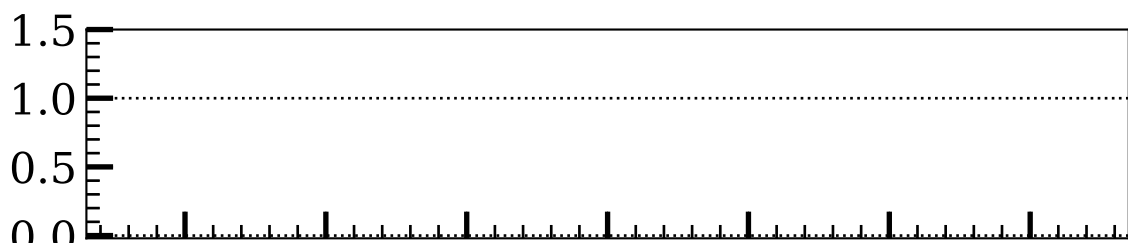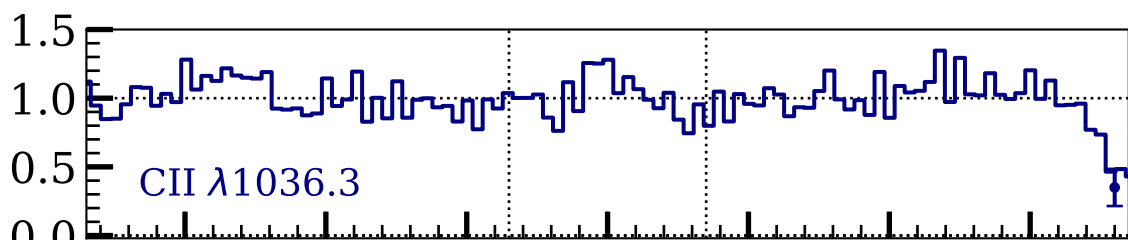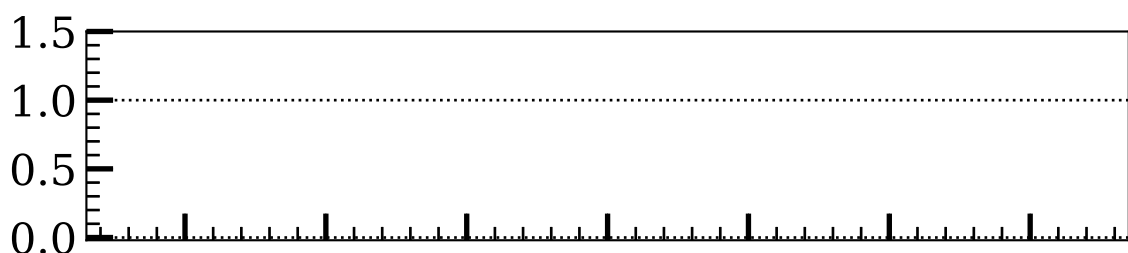

Rest-Frame Velocity ( $\text{km s}^{-1}$ )

J124511.26+335610.1,  $z=0.556684$ , RF=0

Normalized Flux

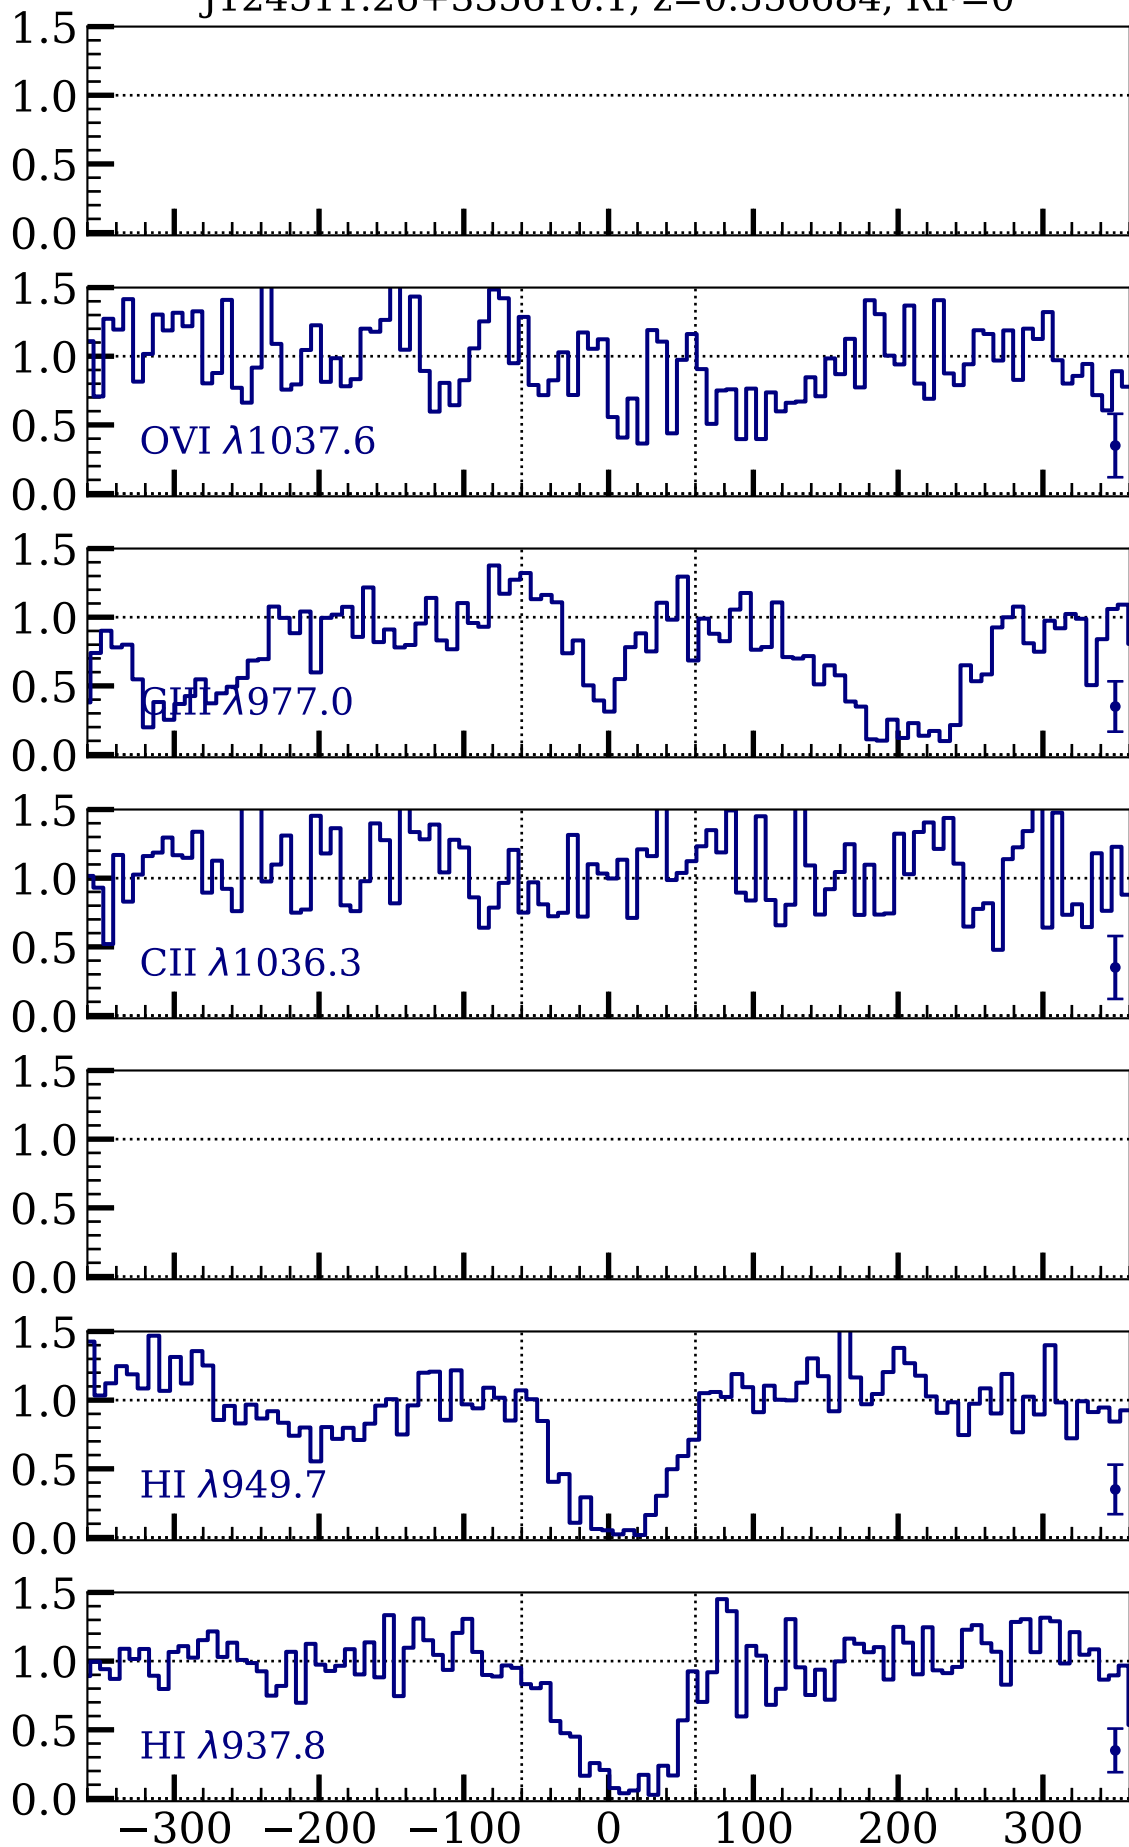

Rest-Frame Velocity (km s<sup>-1</sup>)



J124511.26+335610.1,  $z=0.587563$ , RF=1

Normalized Flux

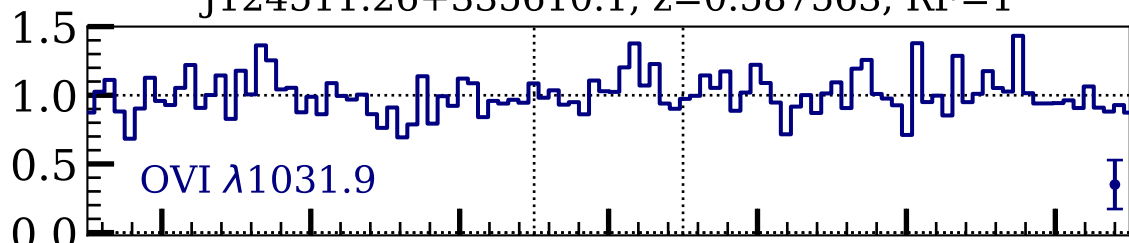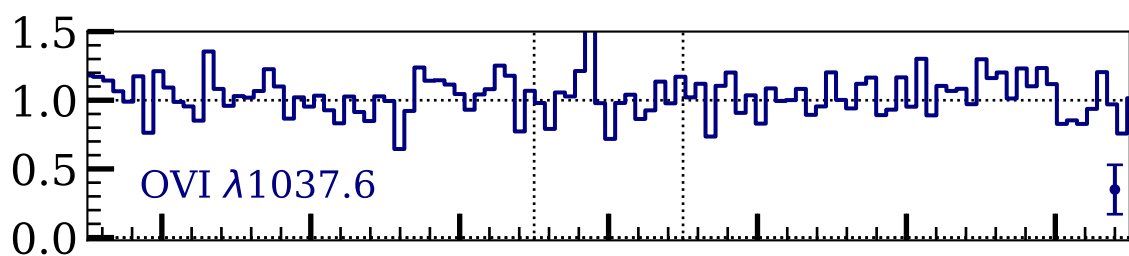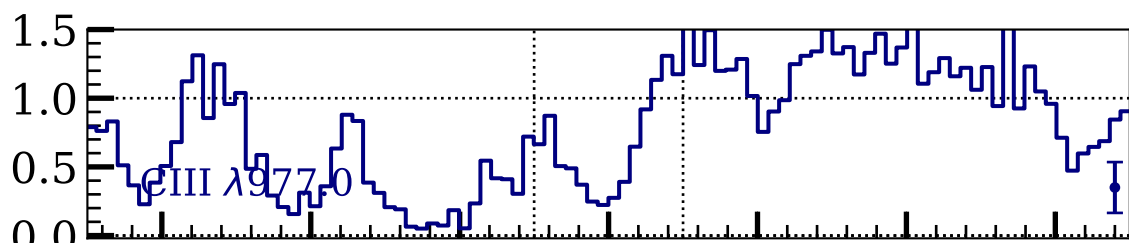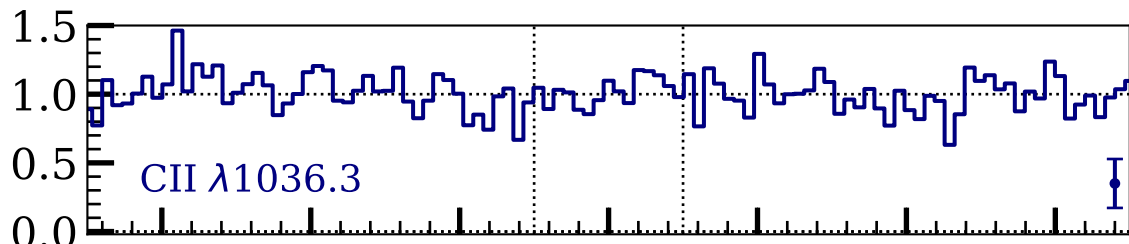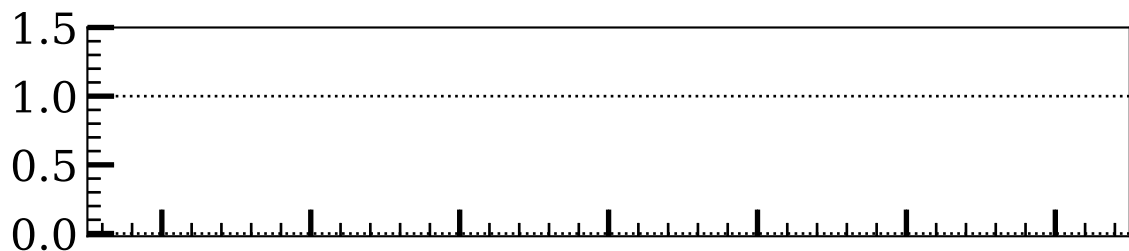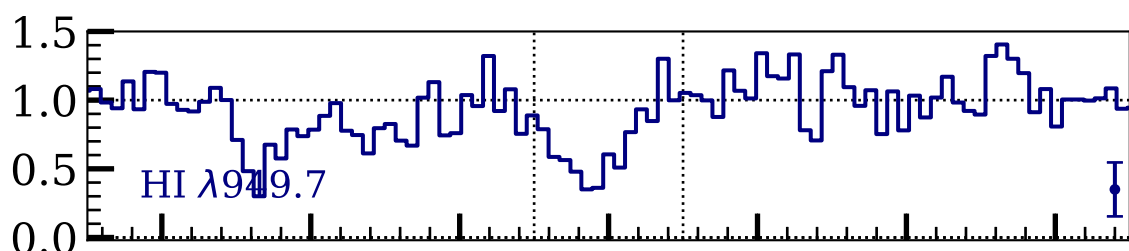

Rest-Frame Velocity ( $\text{km s}^{-1}$ )

J124511.26+335610.1,  $z=0.644918$ , RF=0

Normalized Flux

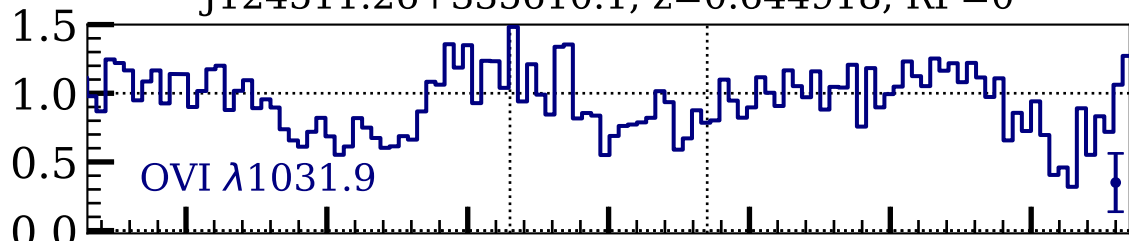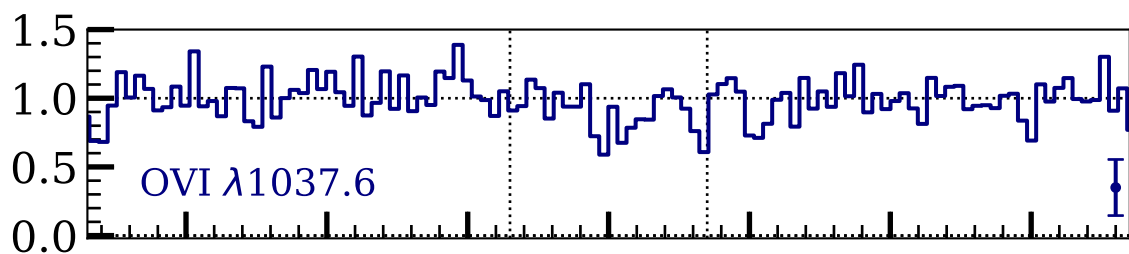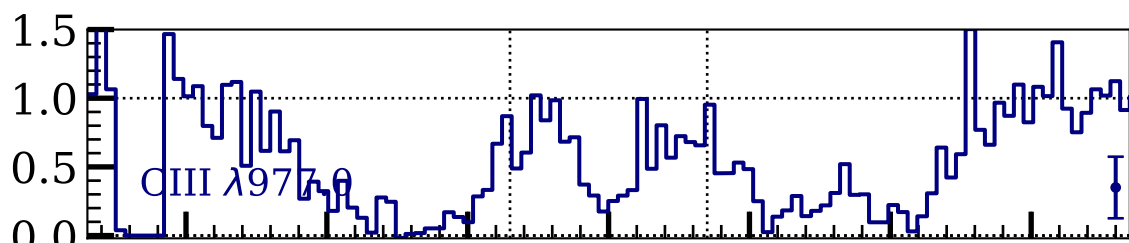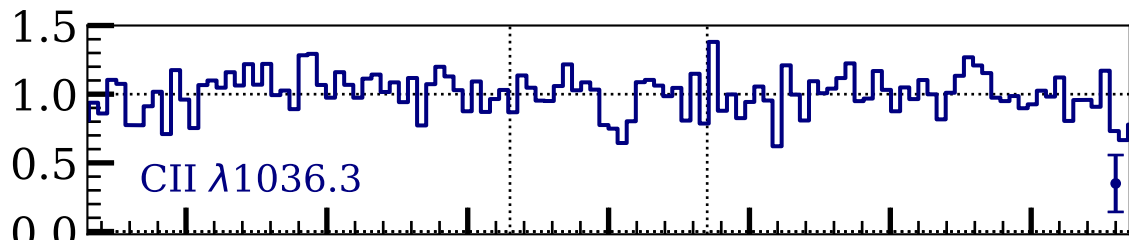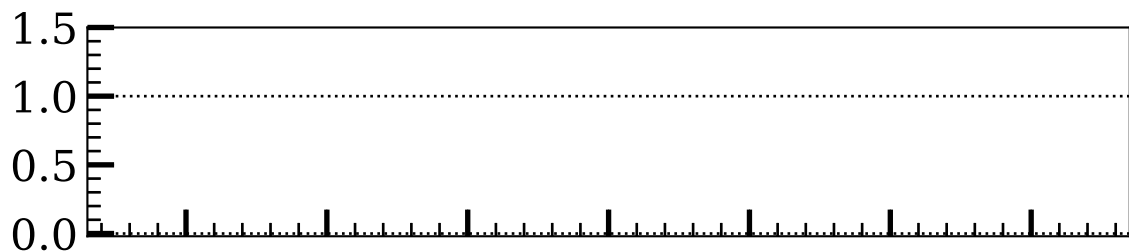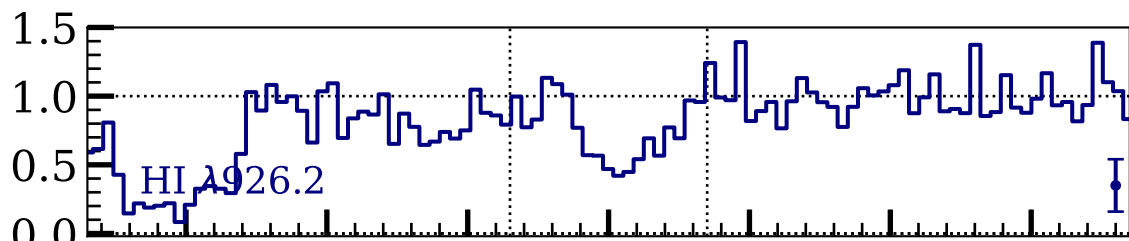

Rest-Frame Velocity ( $\text{km s}^{-1}$ )

J124511.26+335610.1,  $z=0.688948$ , RF=0

Normalized Flux

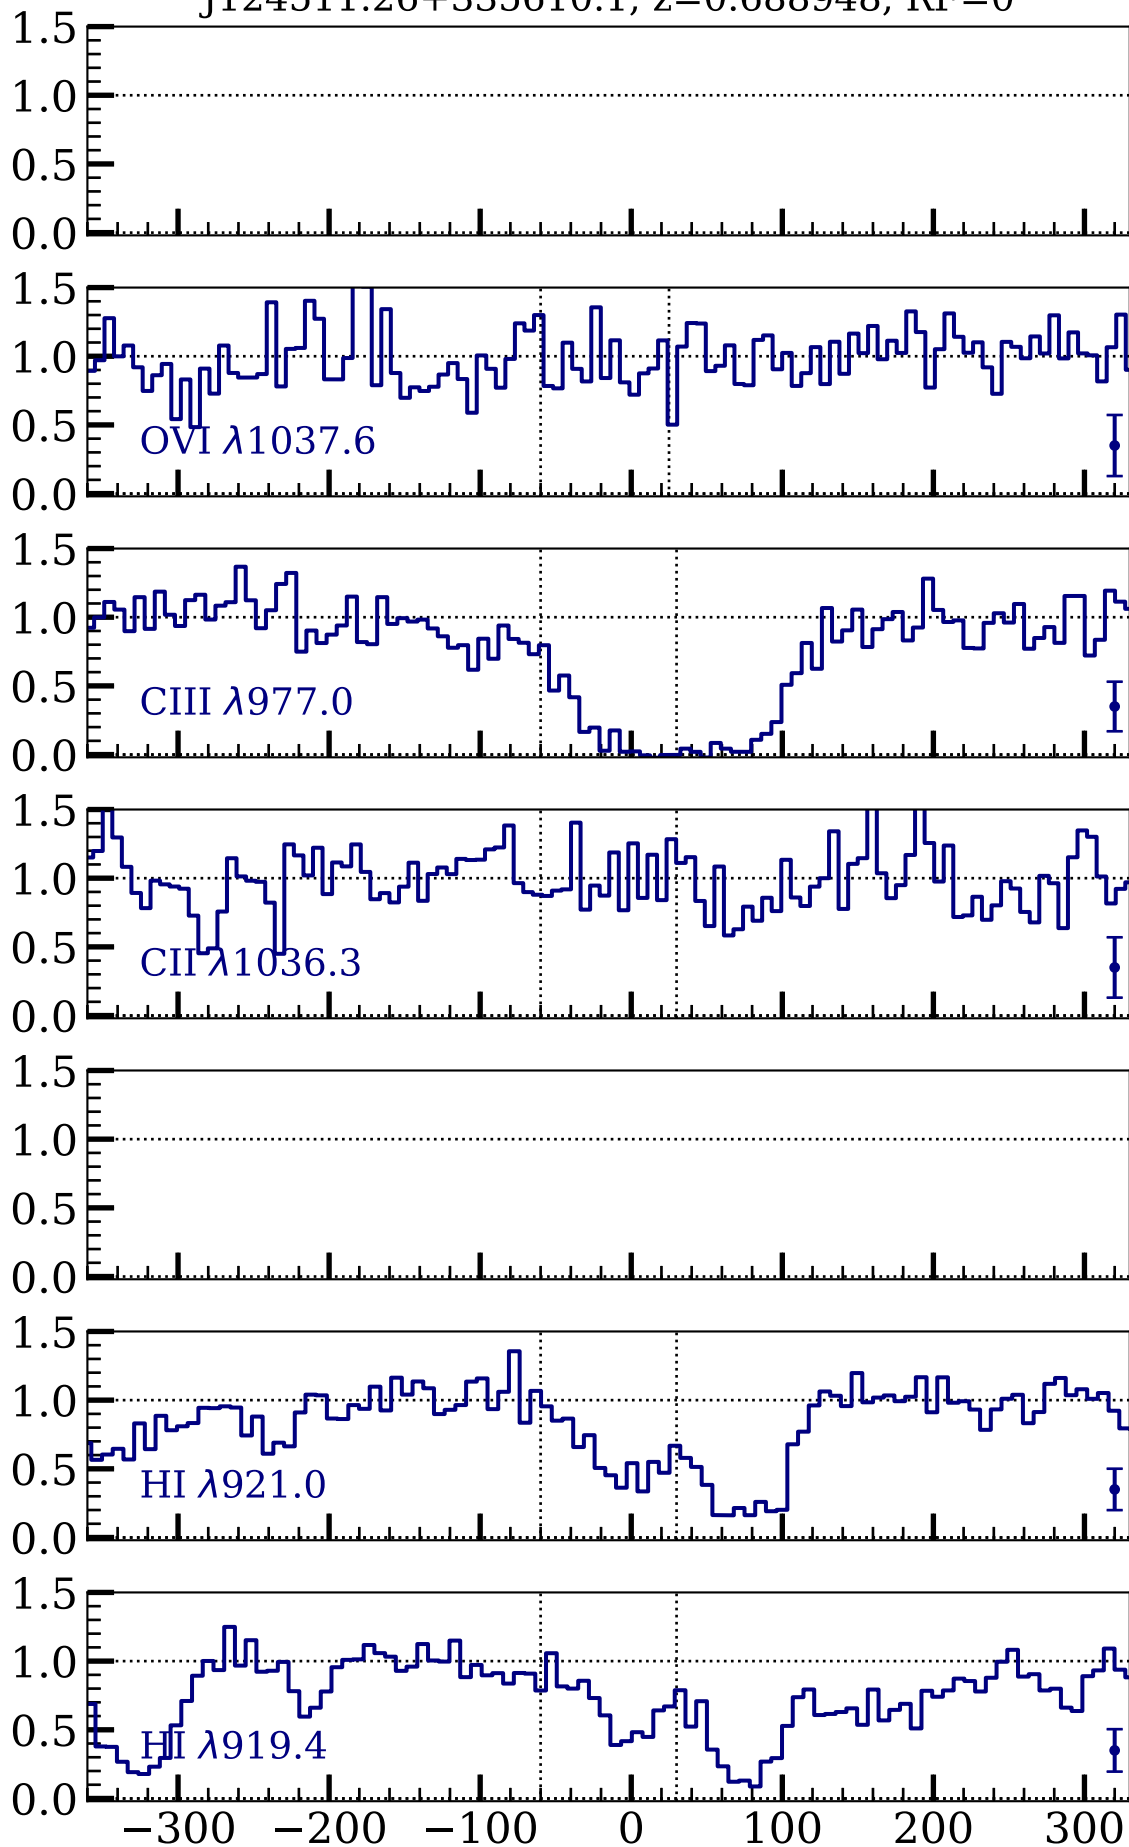

Rest-Frame Velocity (km s<sup>-1</sup>)

J124511.26+335610.1,  $z=0.689370$ , RF=0

Normalized Flux

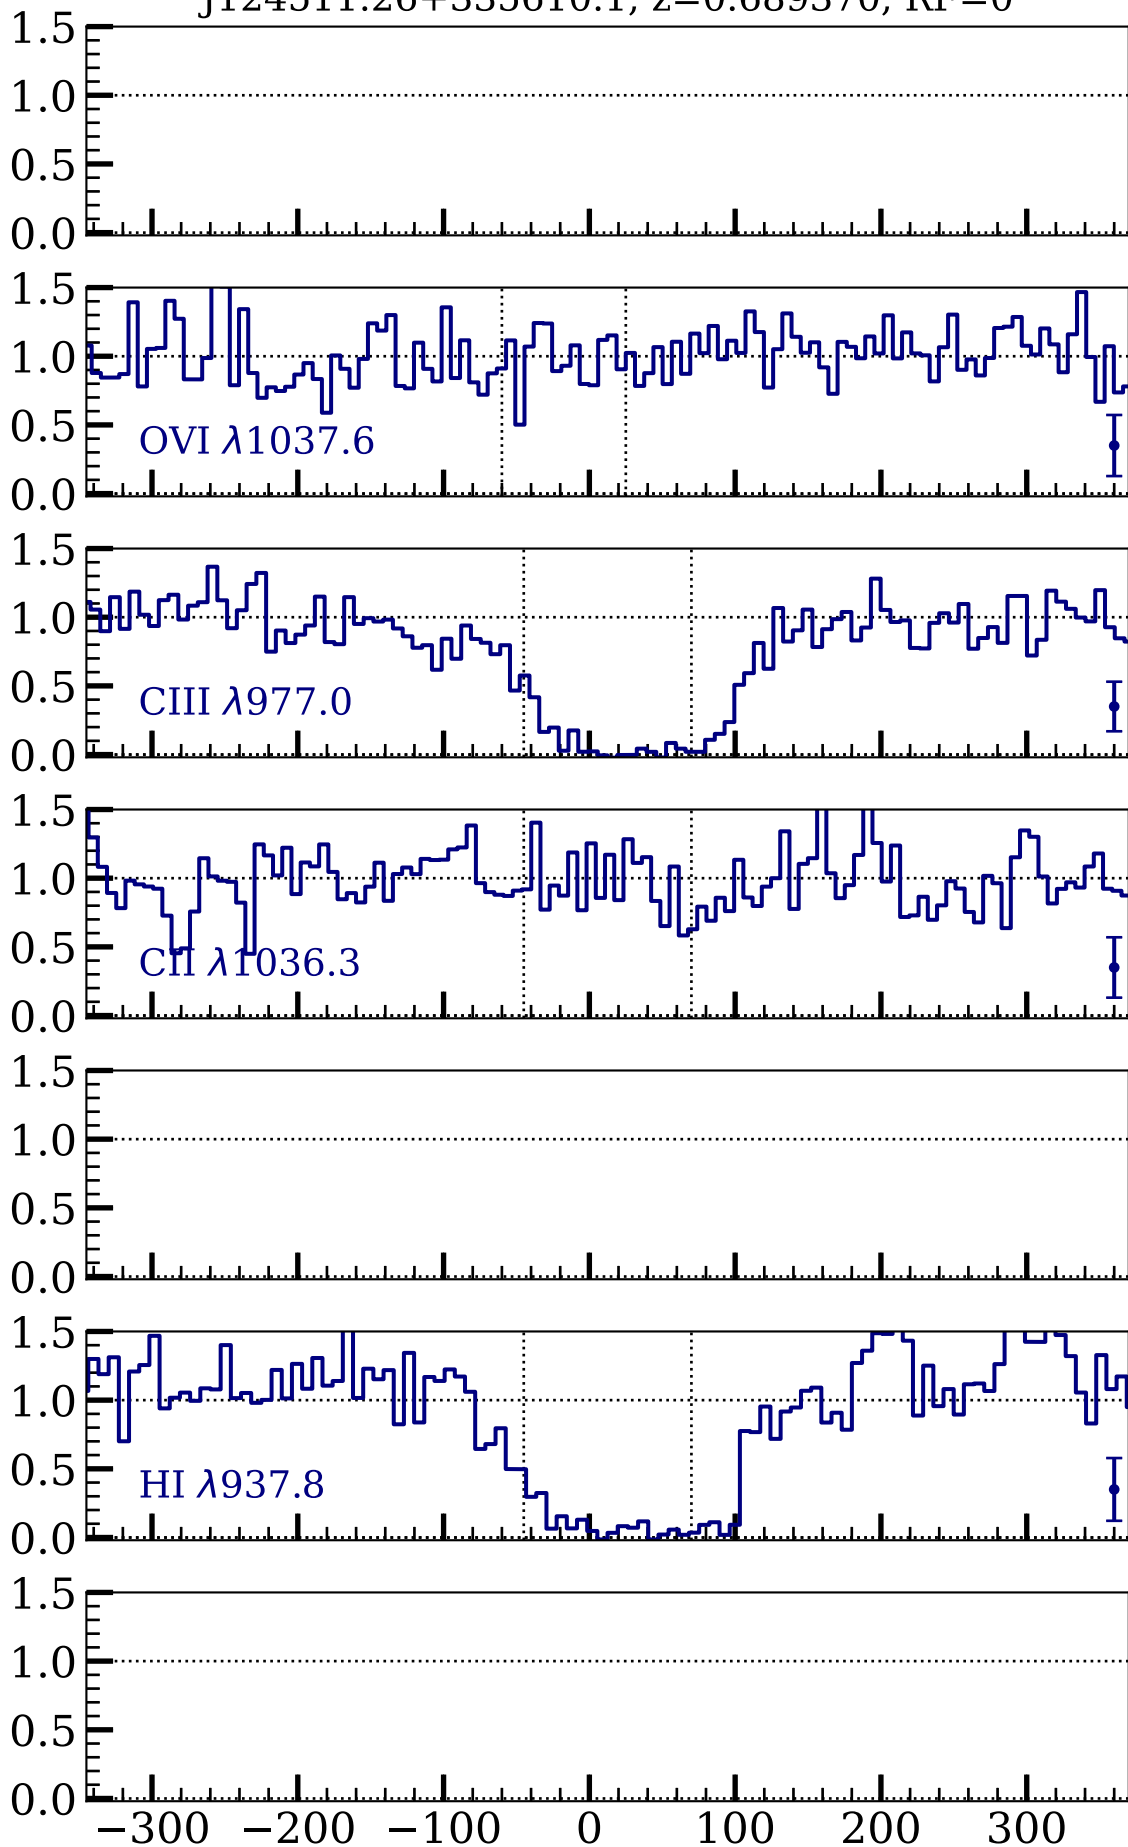

Rest-Frame Velocity (km s<sup>-1</sup>)

J124511.26+335610.1,  $z=0.712976$ , RF=0

Normalized Flux

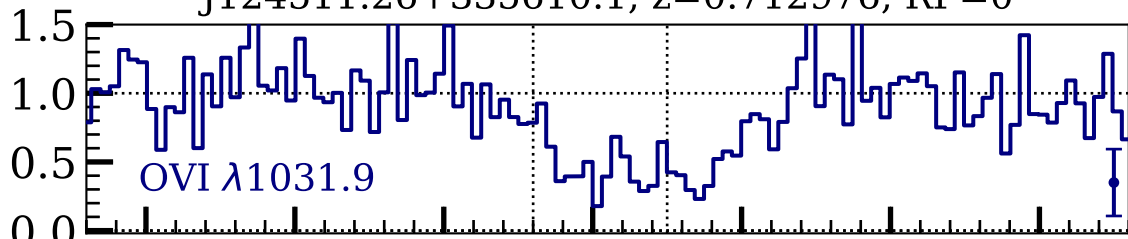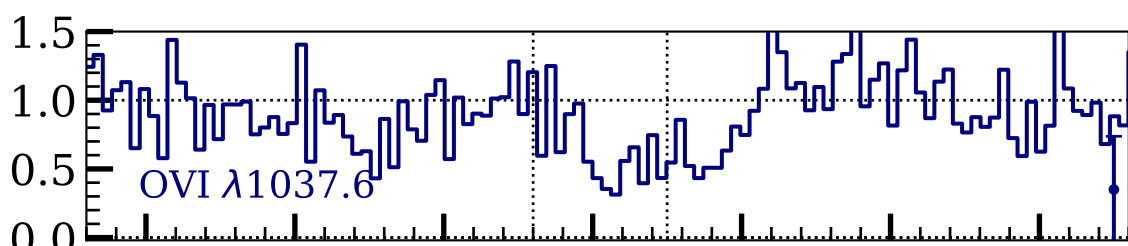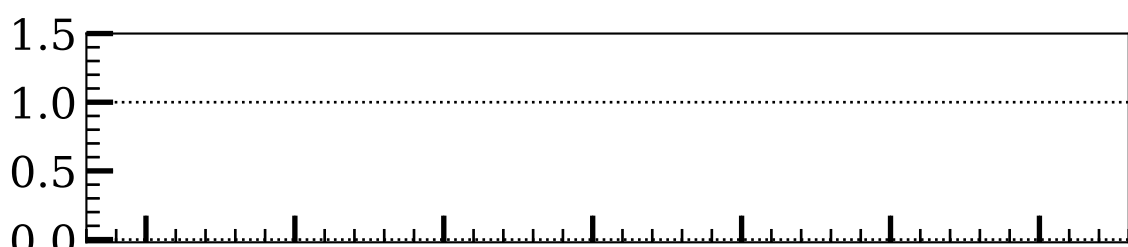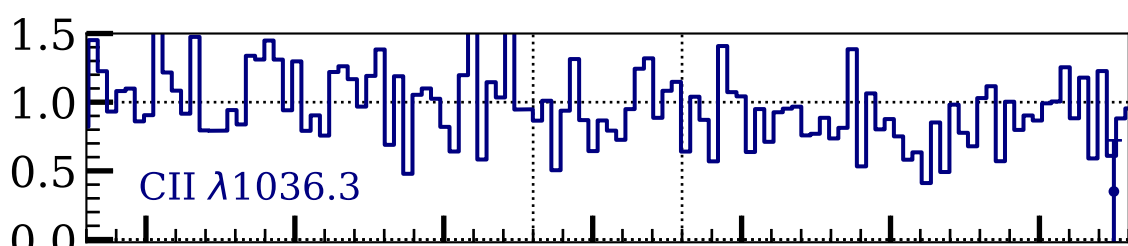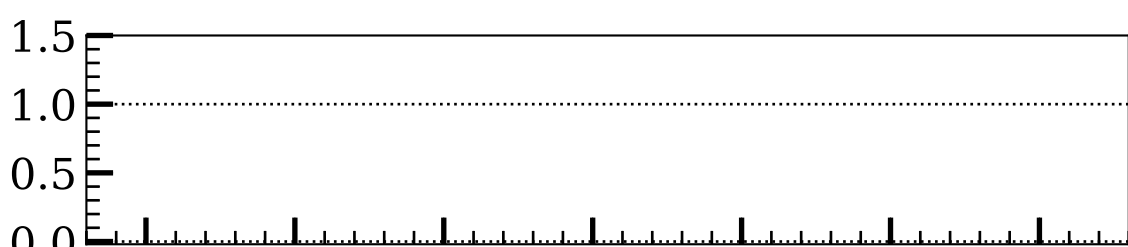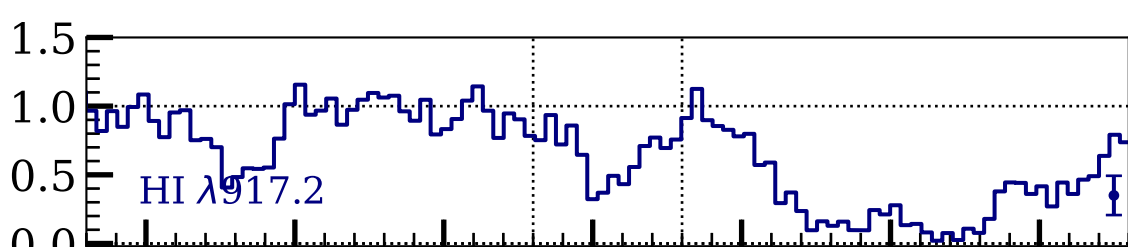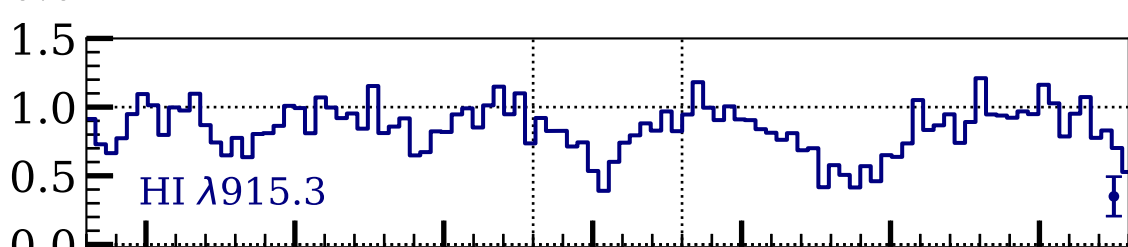

Rest-Frame Velocity ( $\text{km s}^{-1}$ )

J125846.65+242739.1,  $z=0.226199$ , RF=1

Normalized Flux

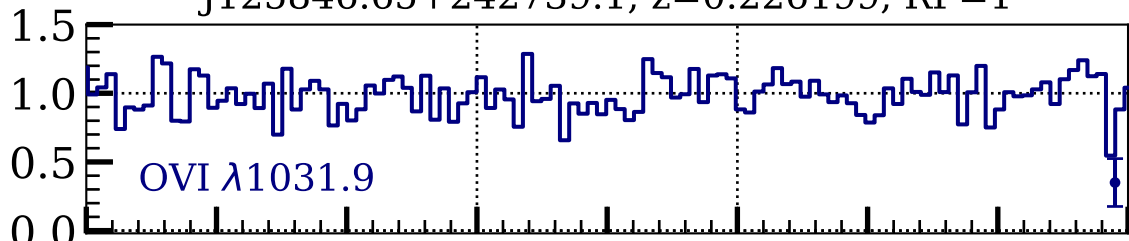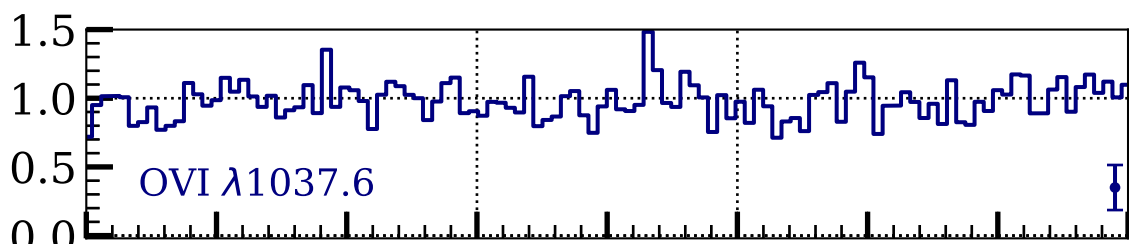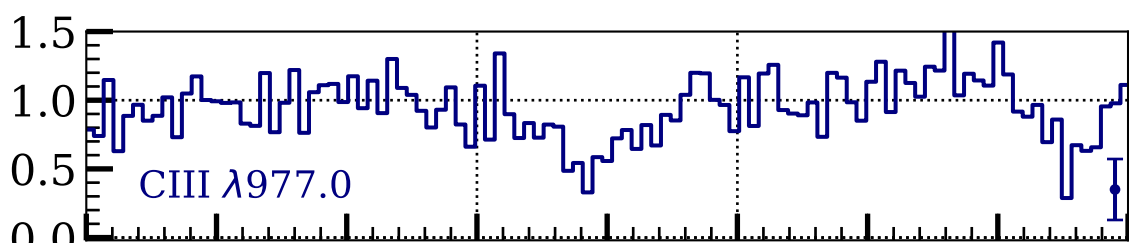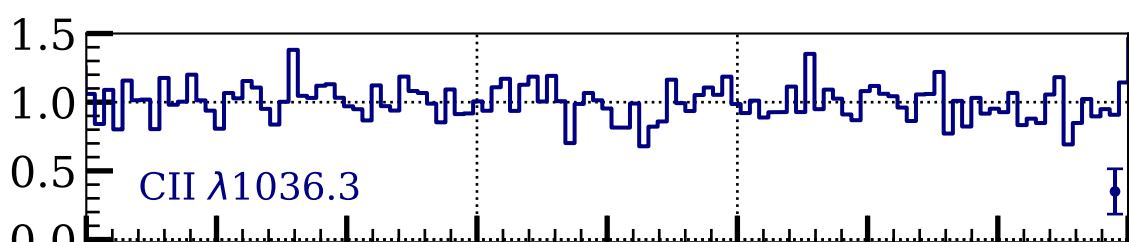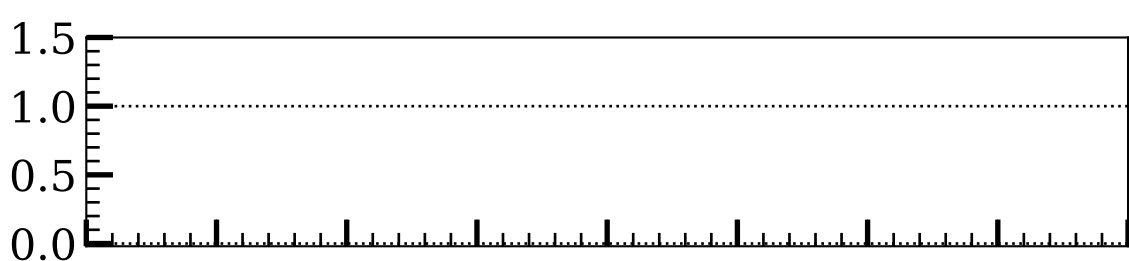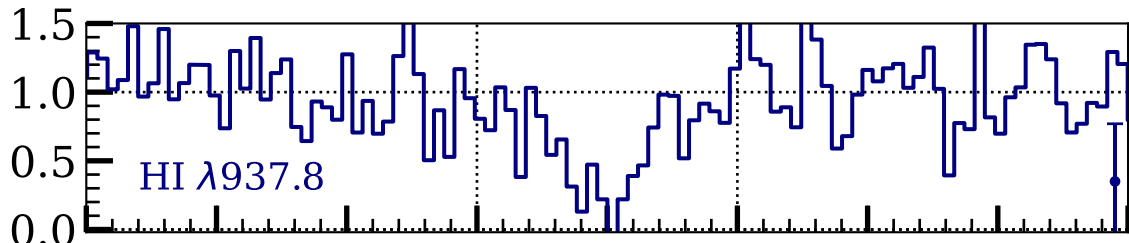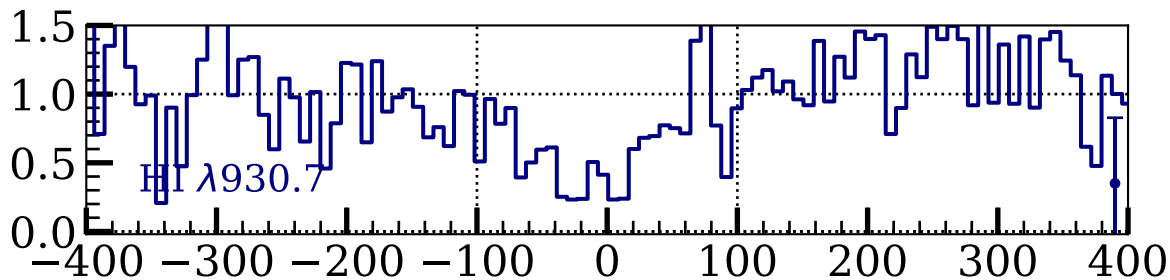

Rest-Frame Velocity ( $\text{km s}^{-1}$ )

J130429.02+311308.2,  $z=0.309948$ , RF=1

Normalized Flux

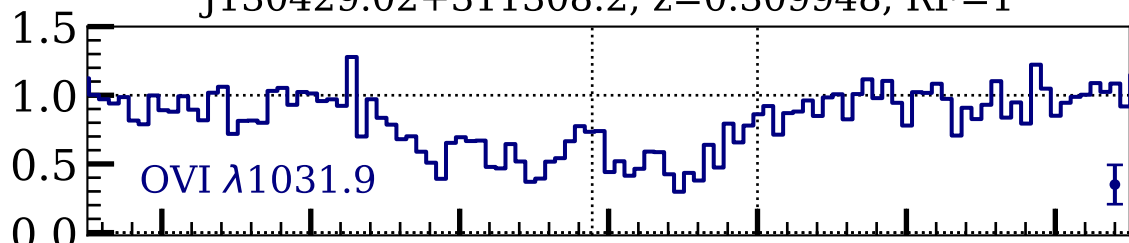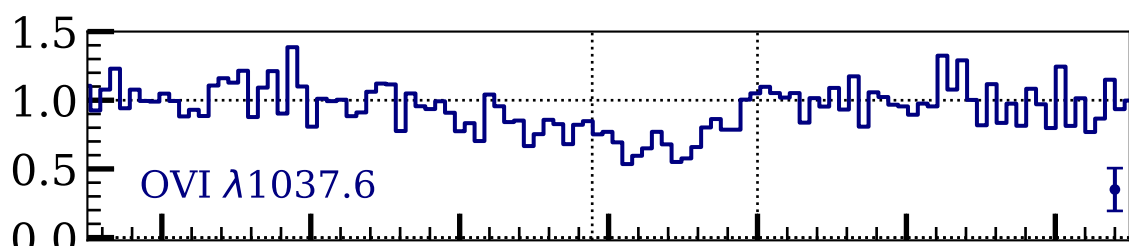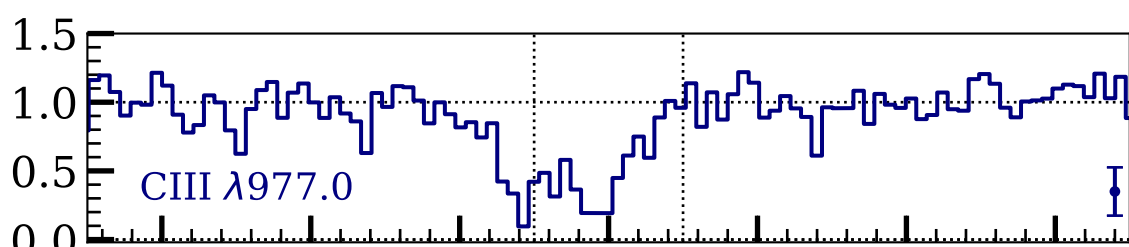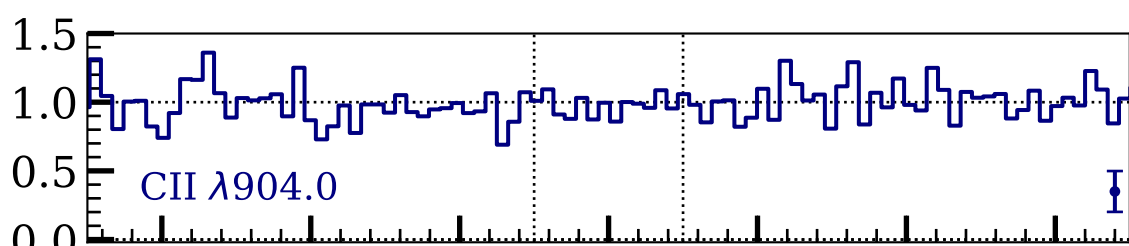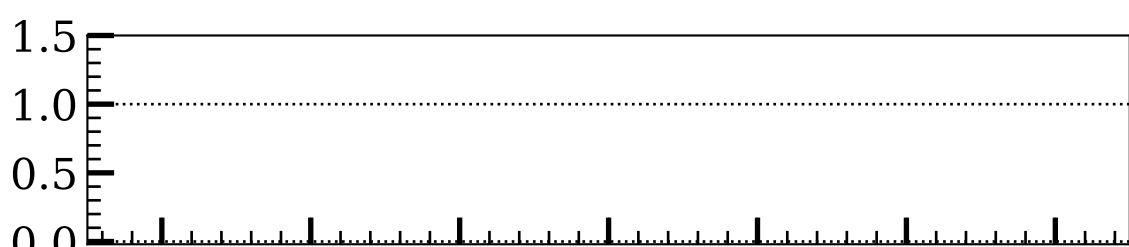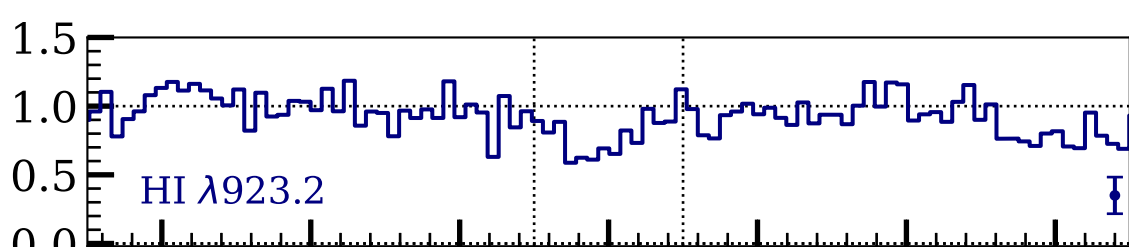

Rest-Frame Velocity ( $\text{km s}^{-1}$ )

J130451.40+245445.9,  $z=0.276315$ , RF=1

Normalized Flux

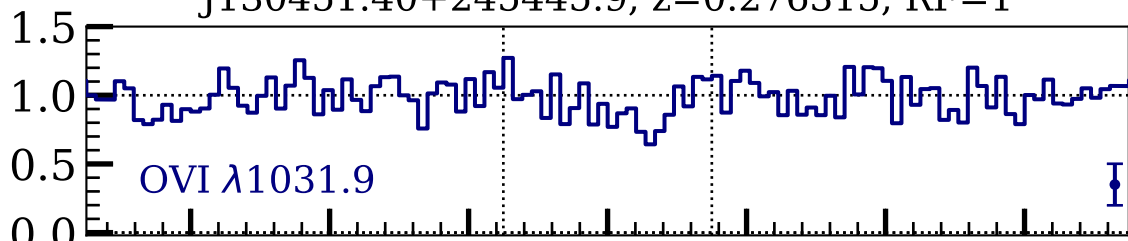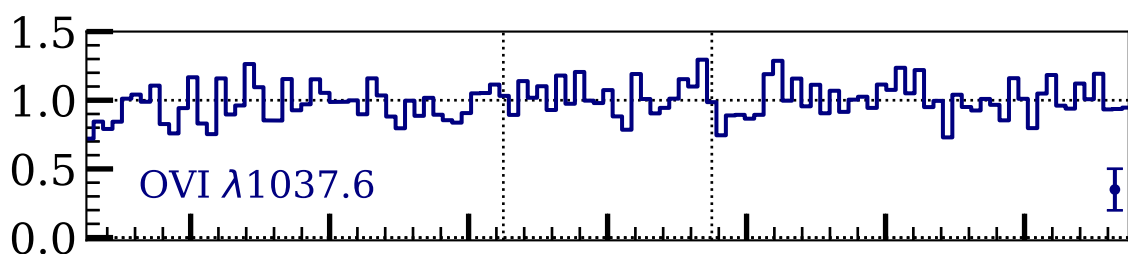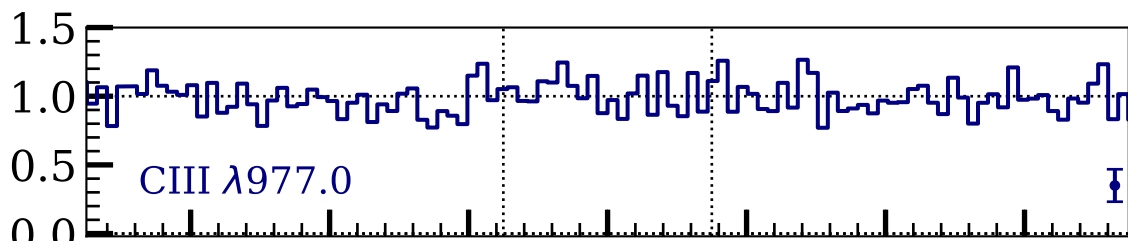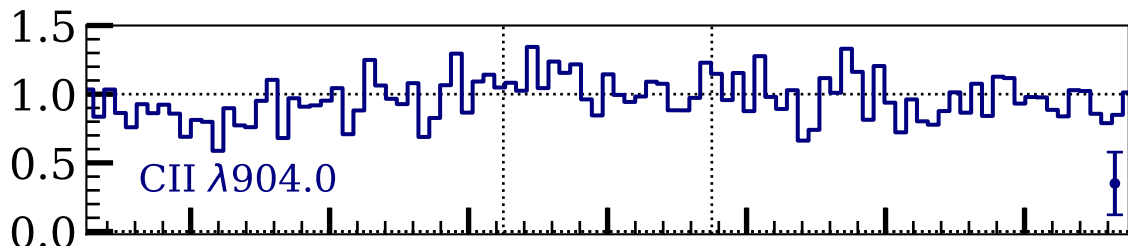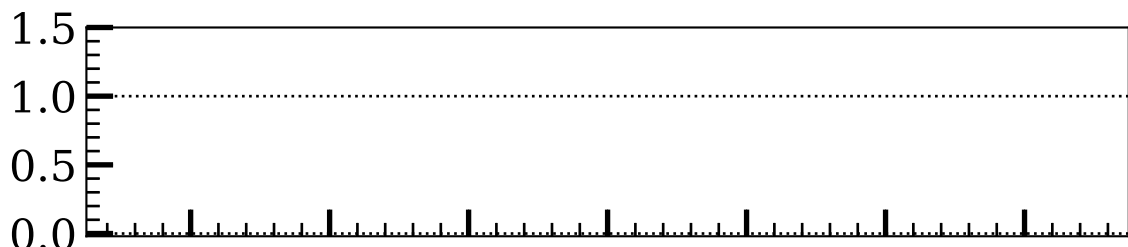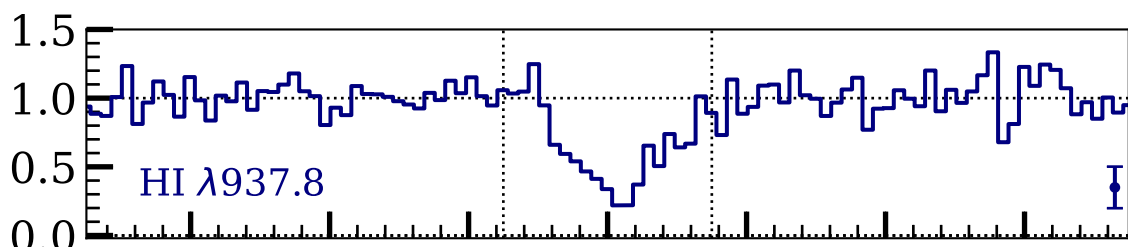

Rest-Frame Velocity ( $\text{km s}^{-1}$ )



J133045.15+281321.5,  $z=0.275547$ , RF=1

Normalized Flux

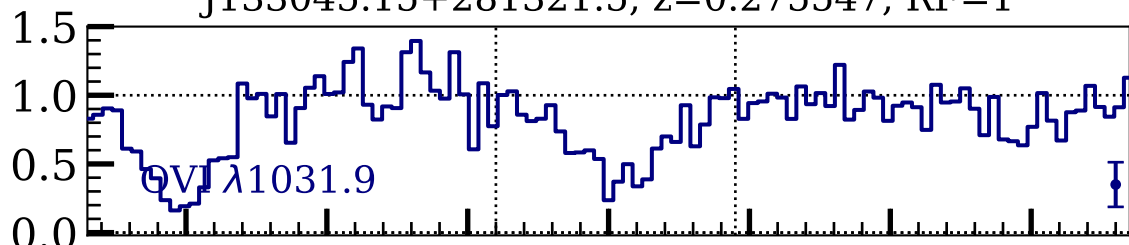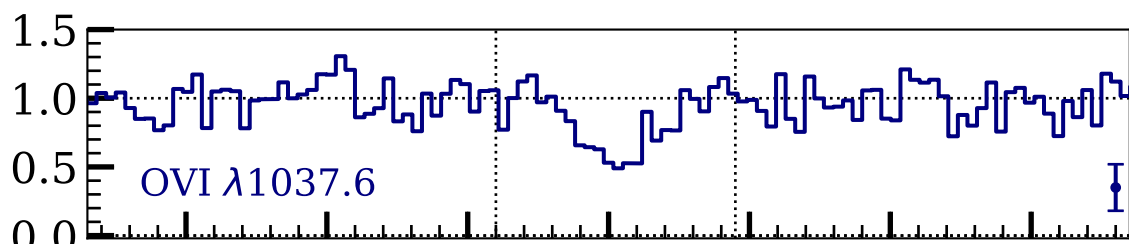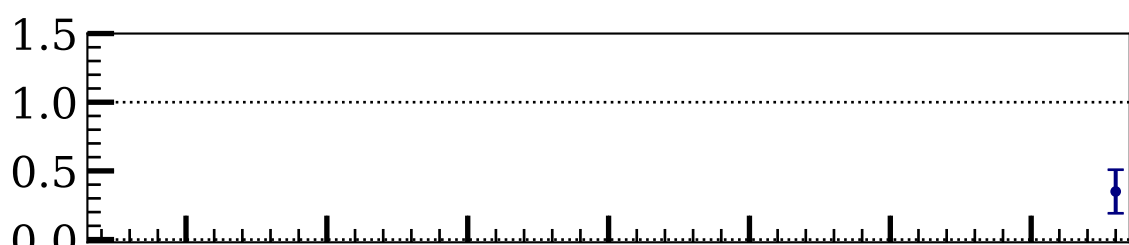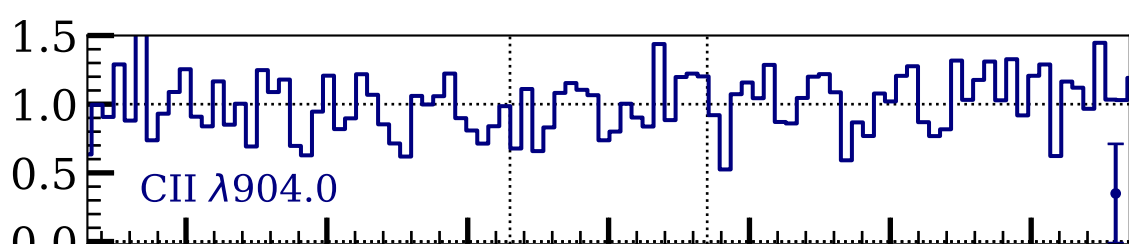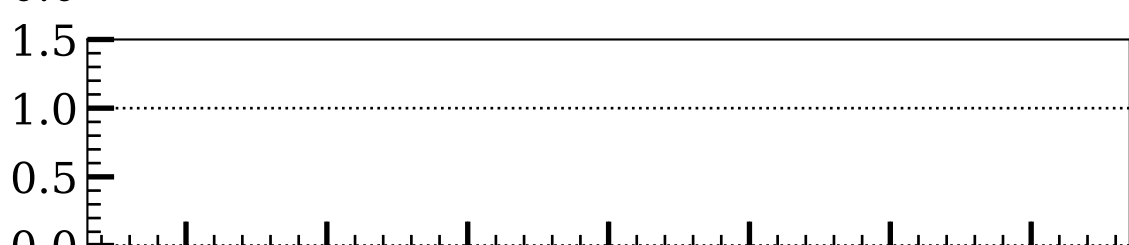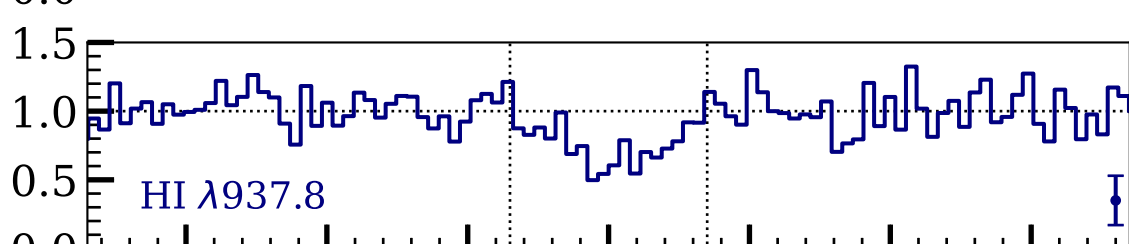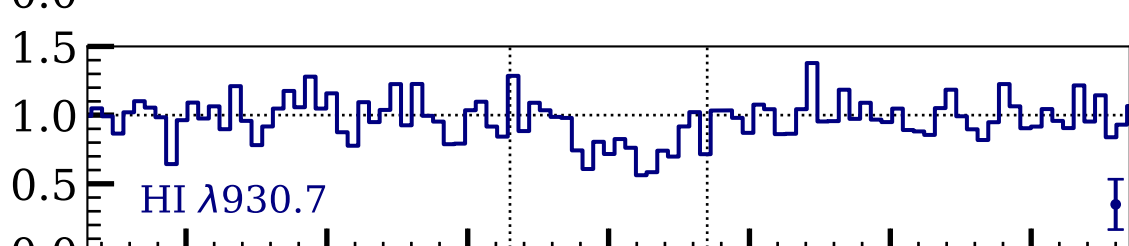

Rest-Frame Velocity ( $\text{km s}^{-1}$ )

J134100.78+412314.0,  $z=0.348827$ , RF=1

Normalized Flux

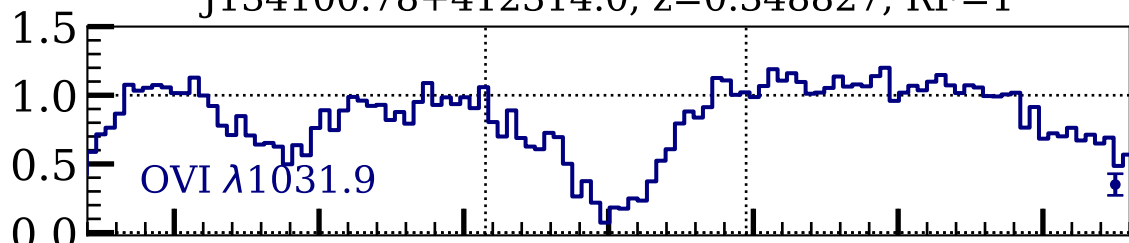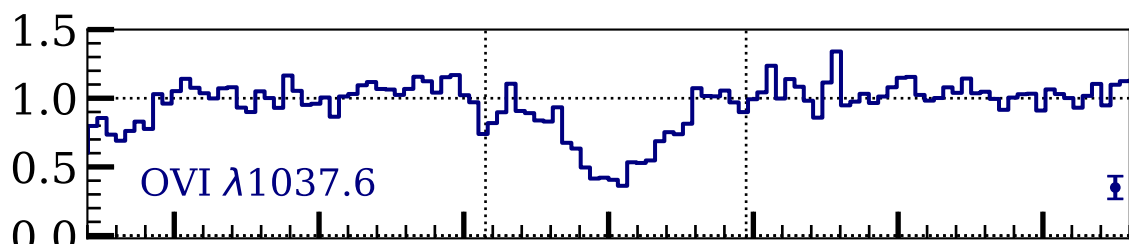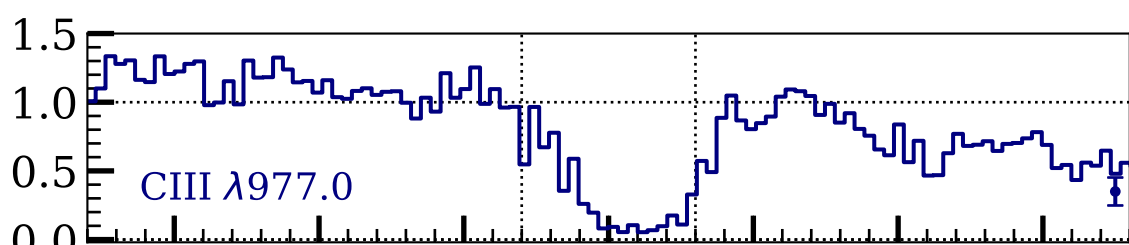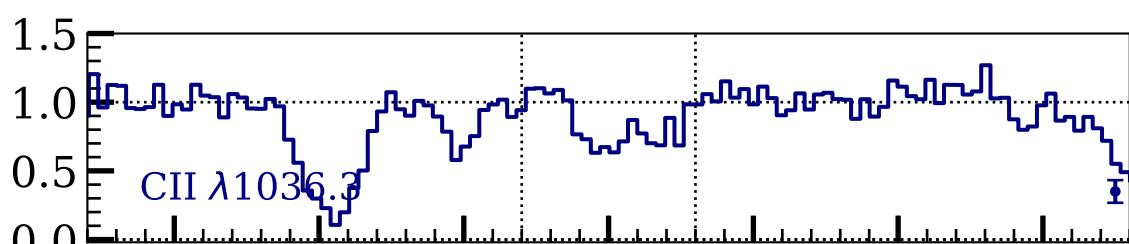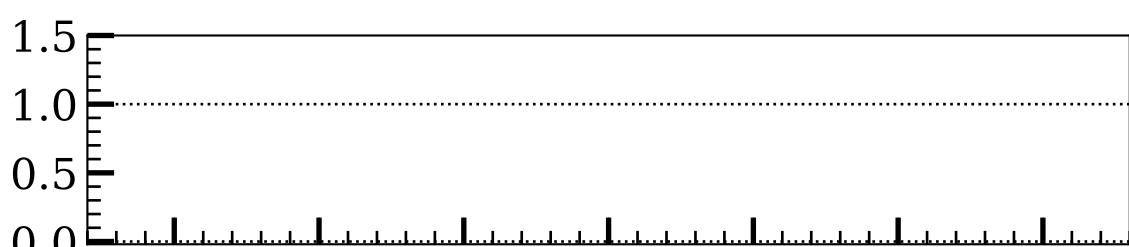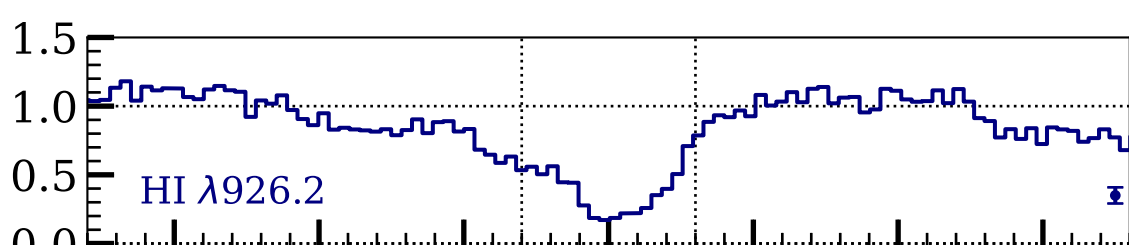

Rest-Frame Velocity ( $\text{km s}^{-1}$ )

J134100.78+412314.0,  $z=0.620752$ , RF=1

Normalized Flux

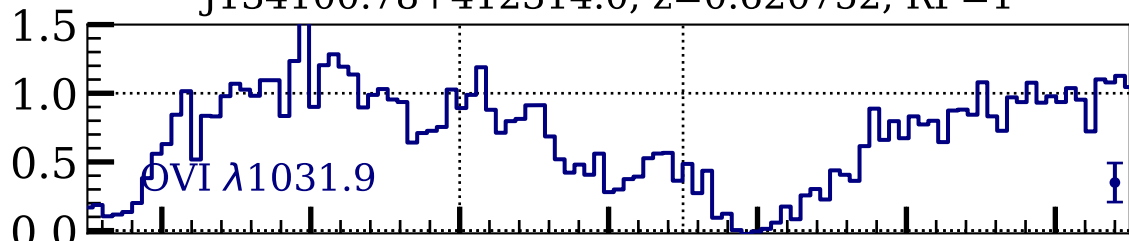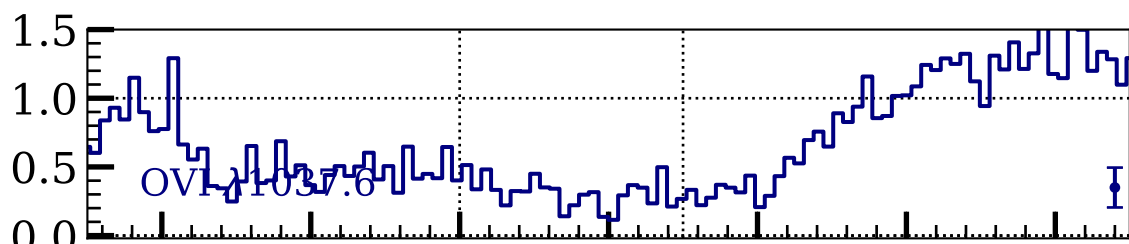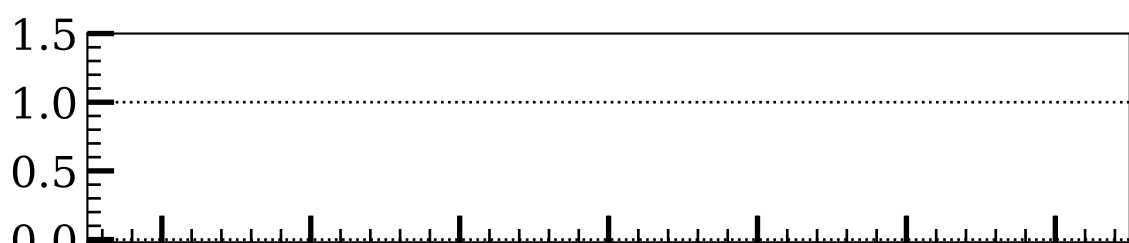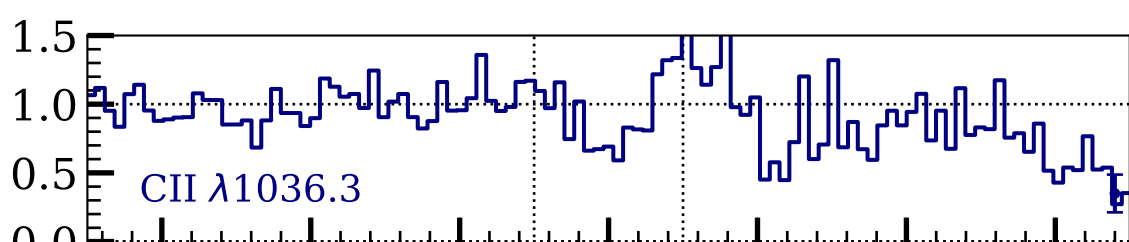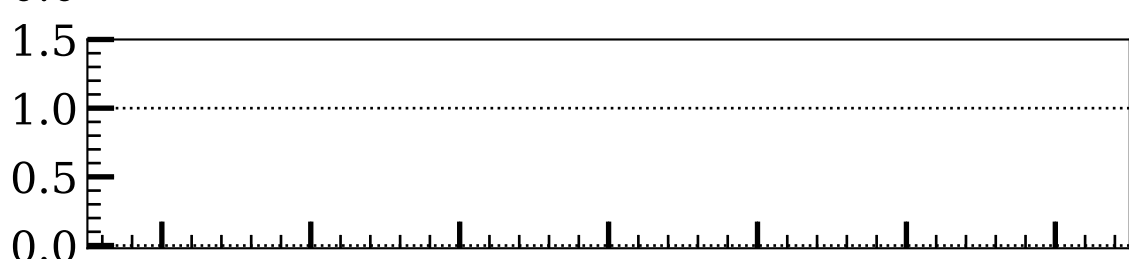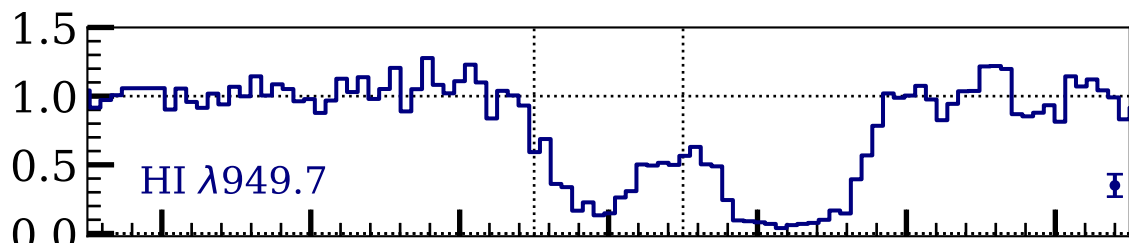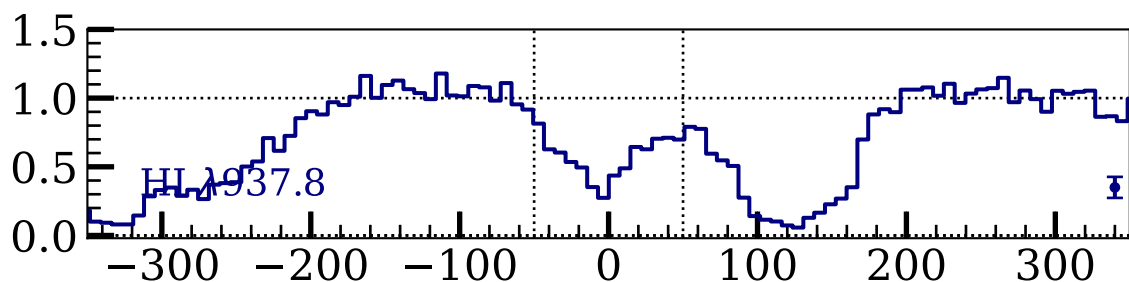

Rest-Frame Velocity ( $\text{km s}^{-1}$ )

J134100.78+412314.0,  $z=0.621428$ , RF=1

Normalized Flux

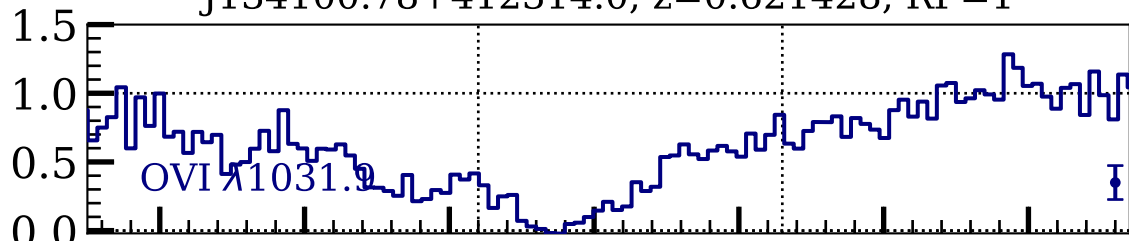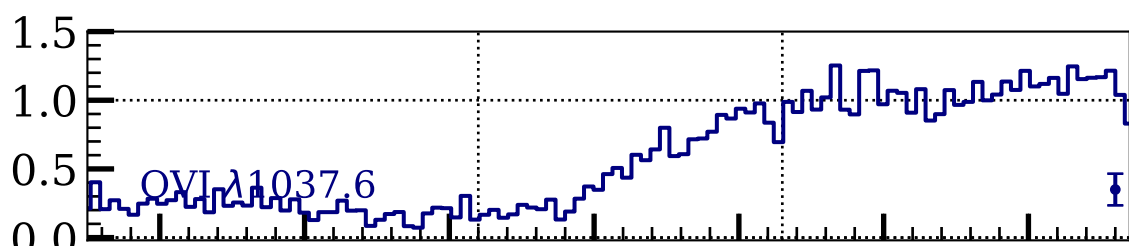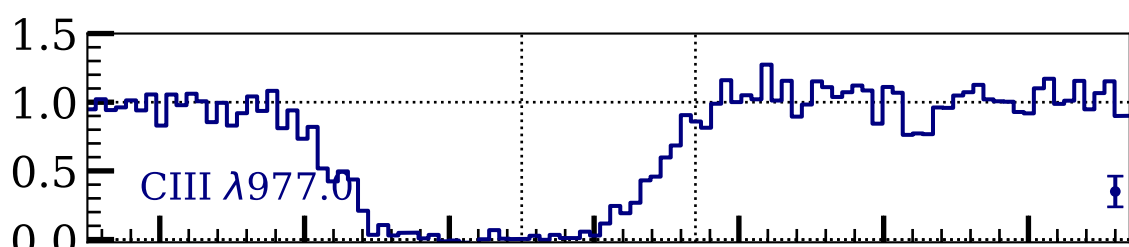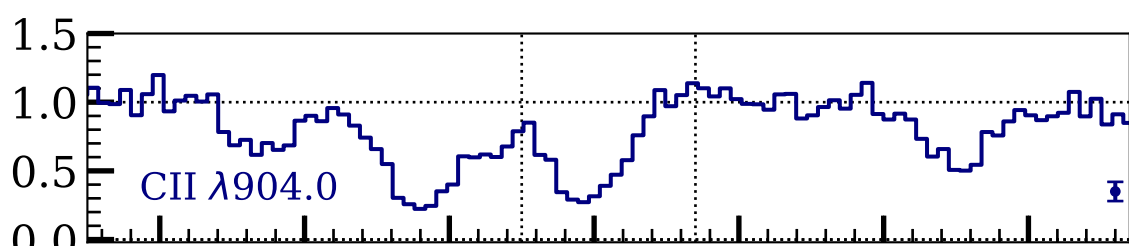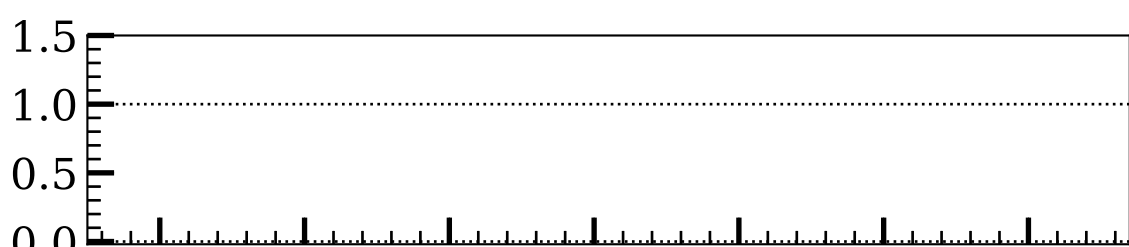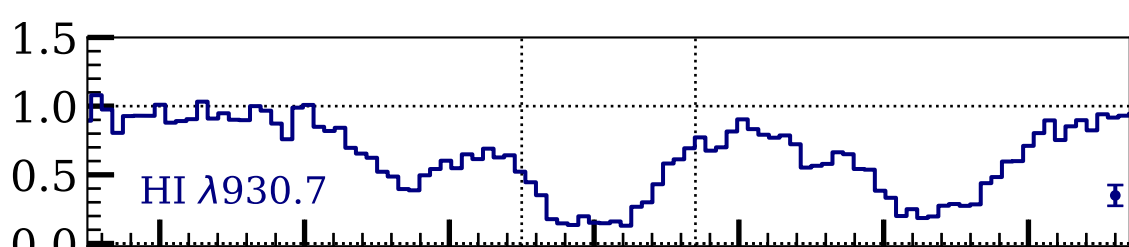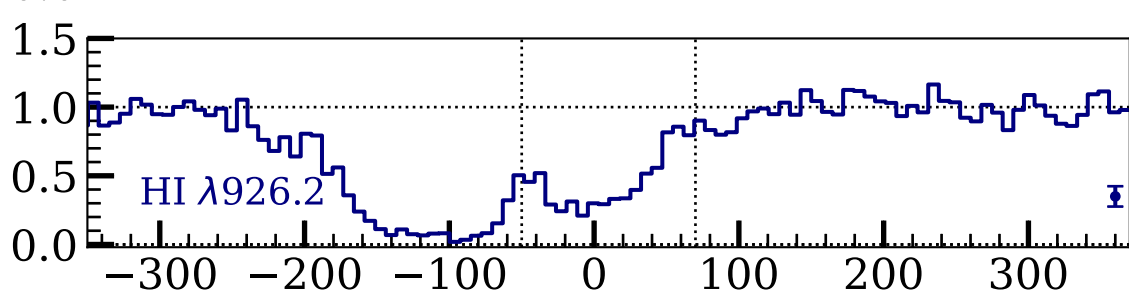

Rest-Frame Velocity ( $\text{km s}^{-1}$ )

J134100.78+412314.0,  $z=0.686086$ , RF=1

Normalized Flux

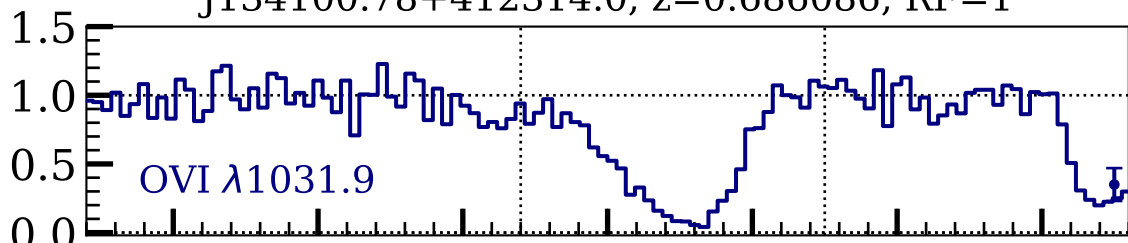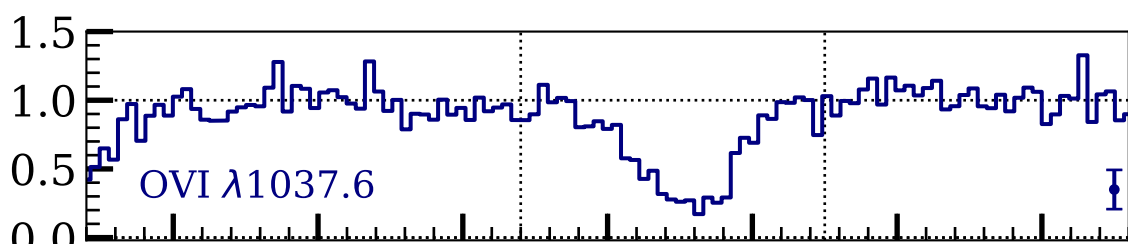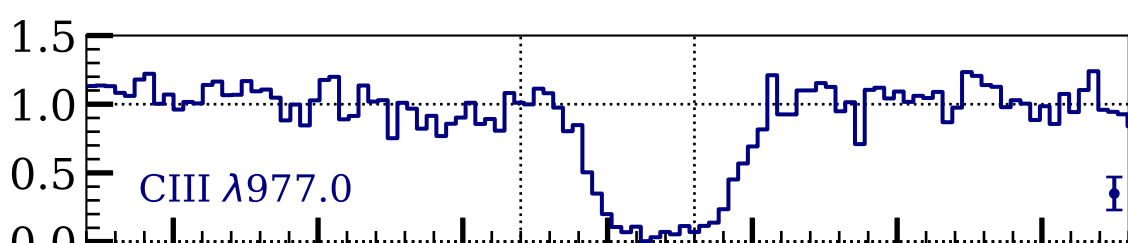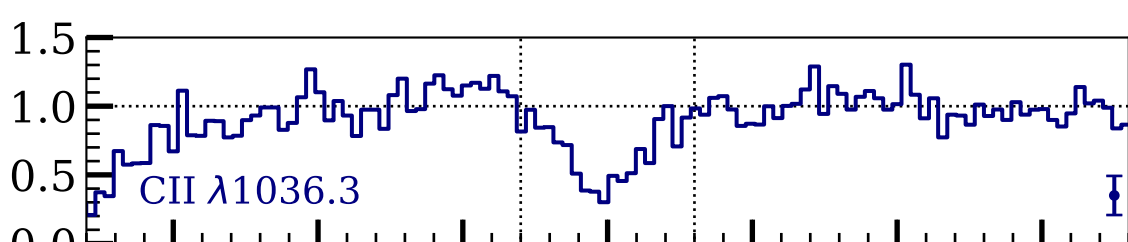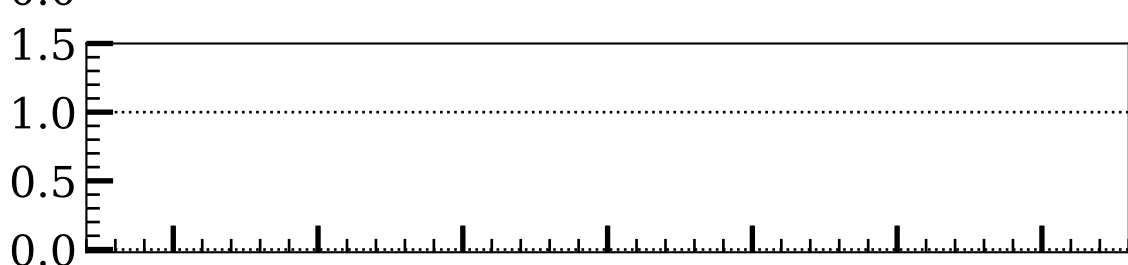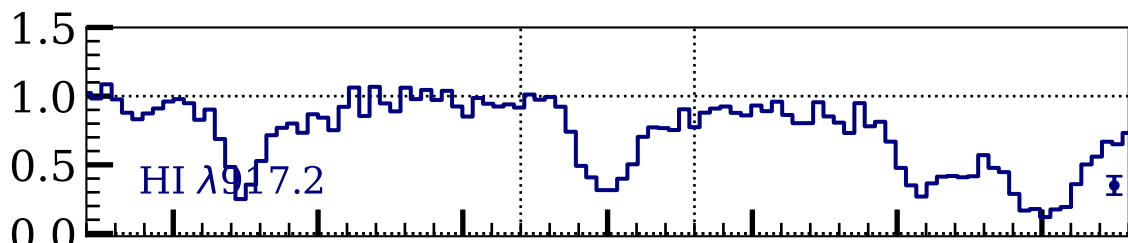

Rest-Frame Velocity ( $\text{km s}^{-1}$ )

J134447.55+554656.8,  $z=0.404153$ , RF=0

Normalized Flux

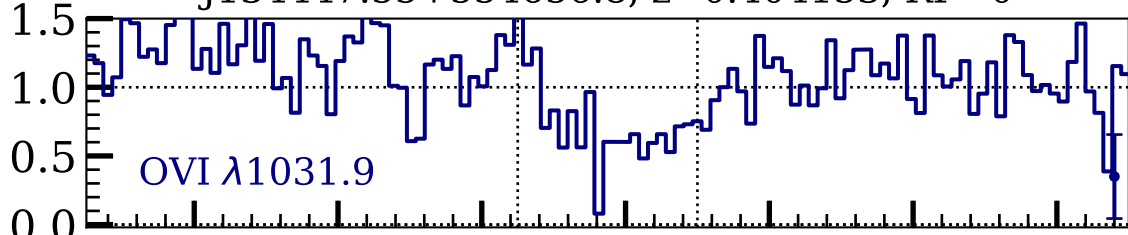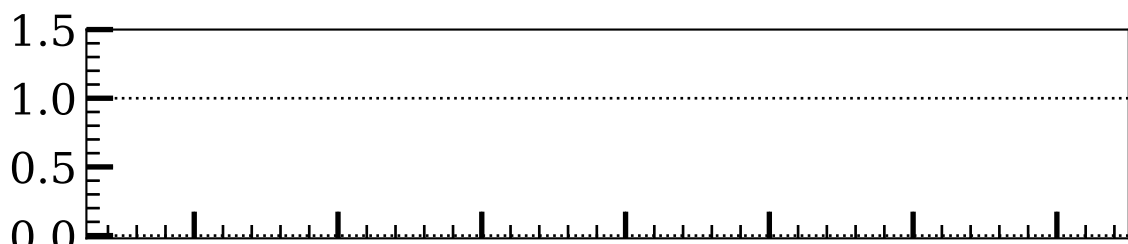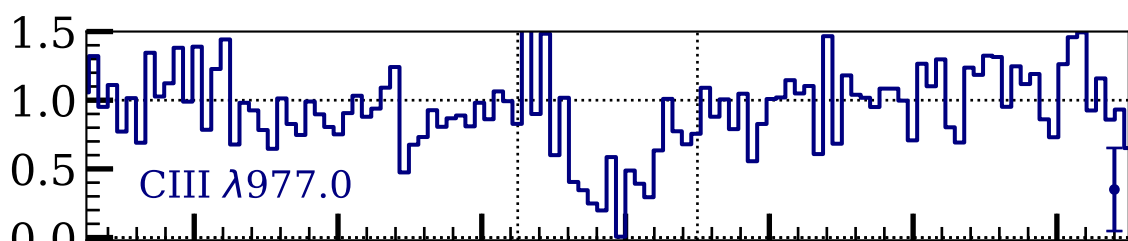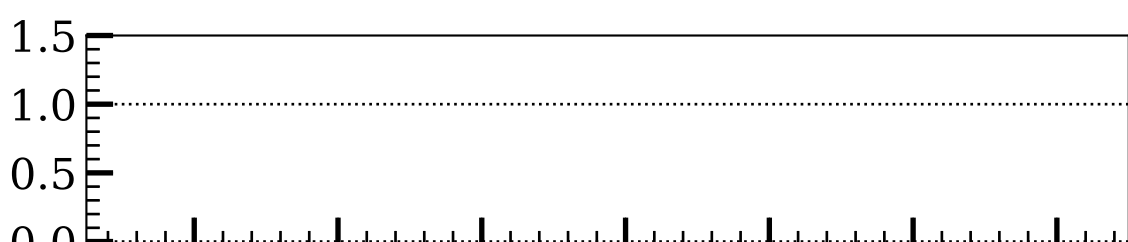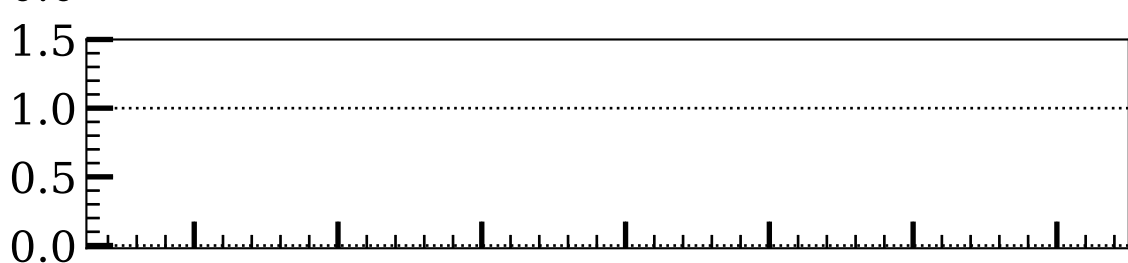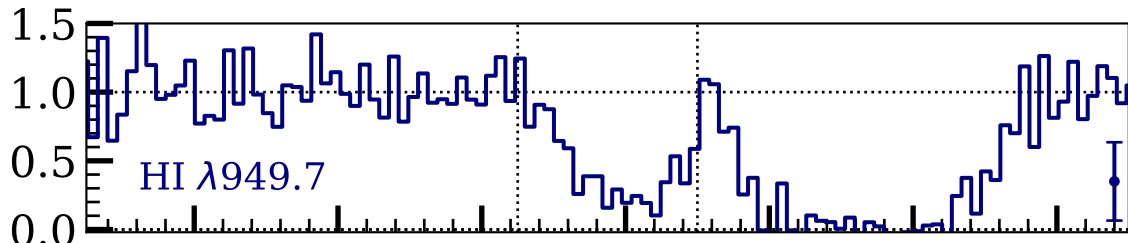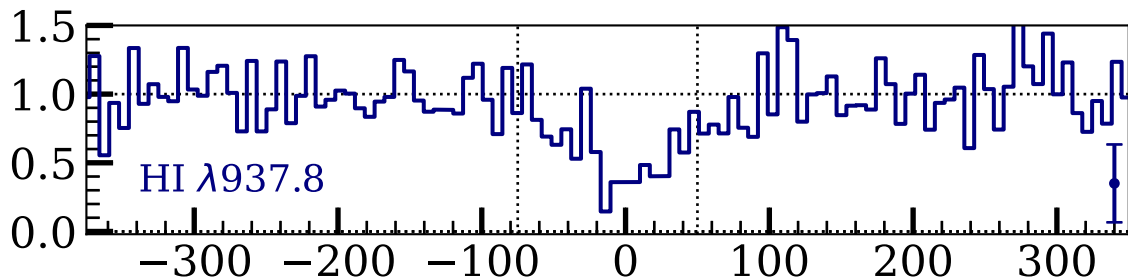

Rest-Frame Velocity ( $\text{km s}^{-1}$ )

J135726.26+043541.3,  $z=0.610248$ , RF=1

Normalized Flux

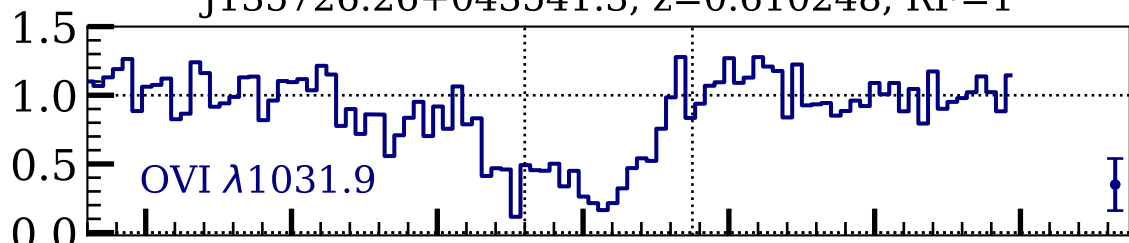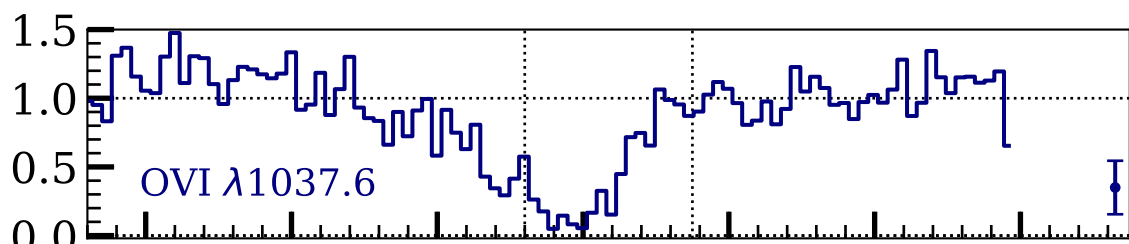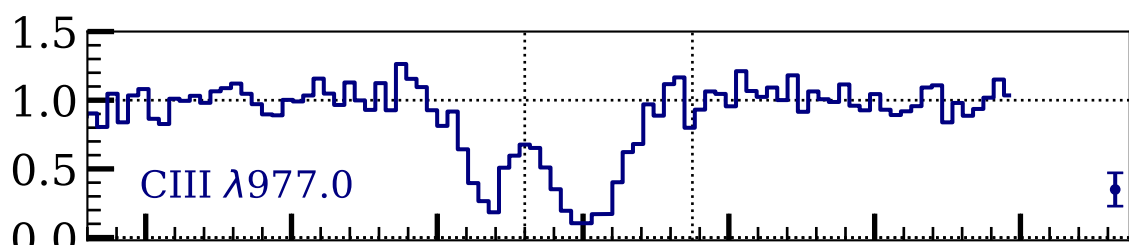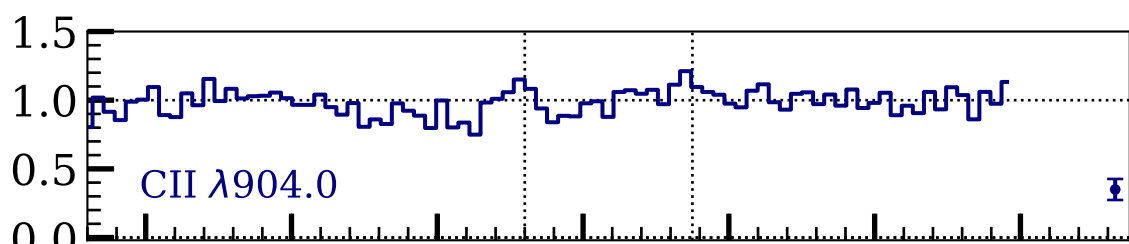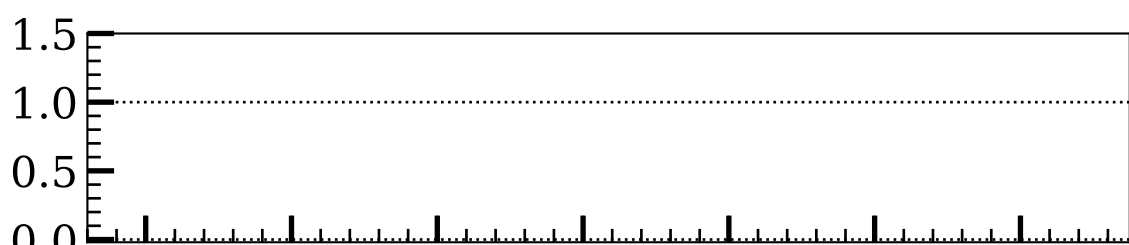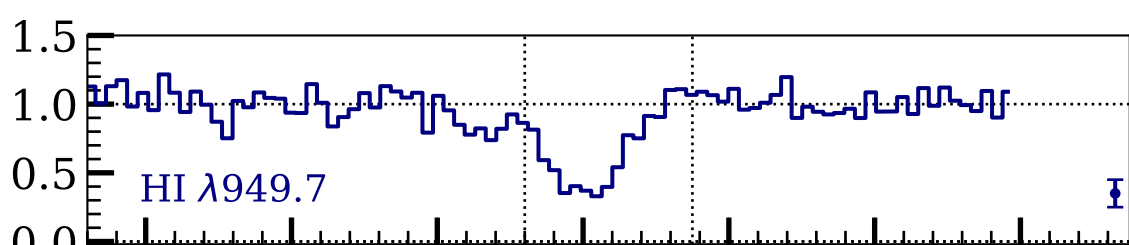

Rest-Frame Velocity ( $\text{km s}^{-1}$ )

J140732.25+550725.4,  $z=0.243328$ , RF=1

Normalized Flux

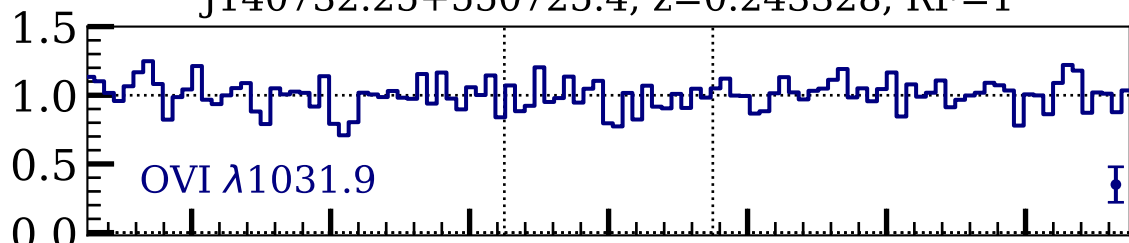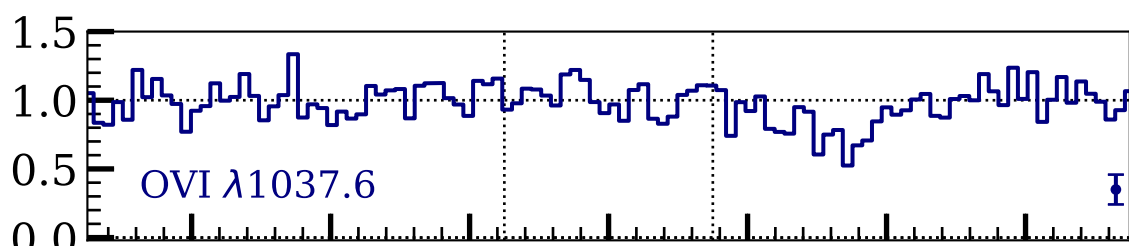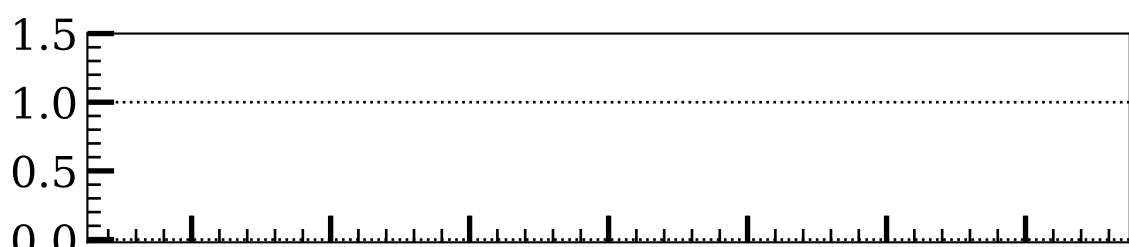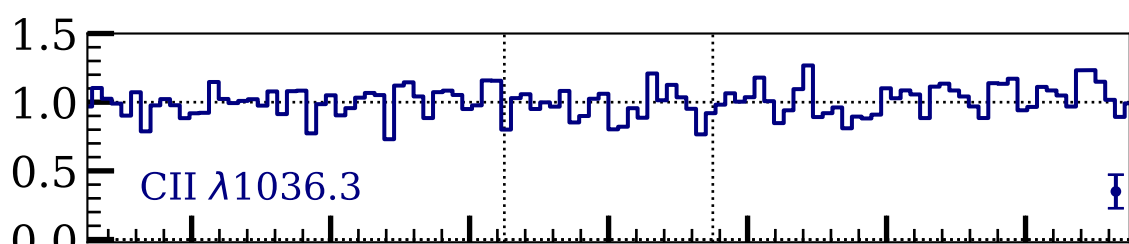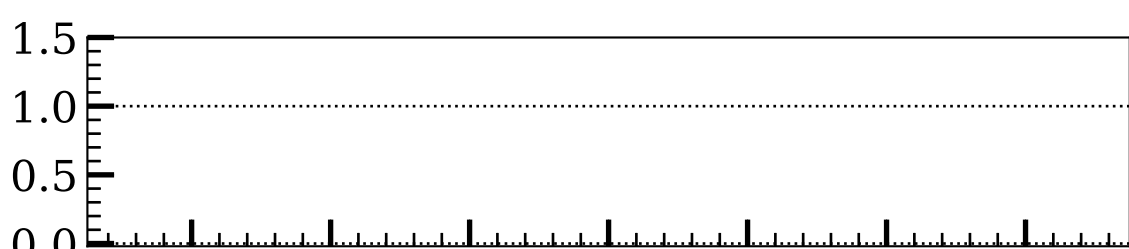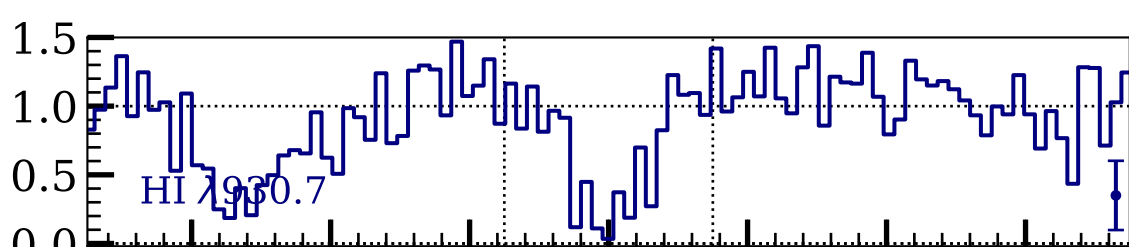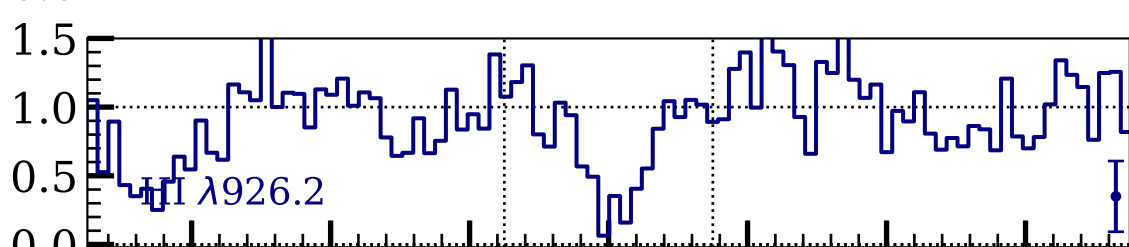

Rest-Frame Velocity (km s<sup>-1</sup>)



J140732.25+550725.4,  $z=0.246911$ , RF=1

Normalized Flux

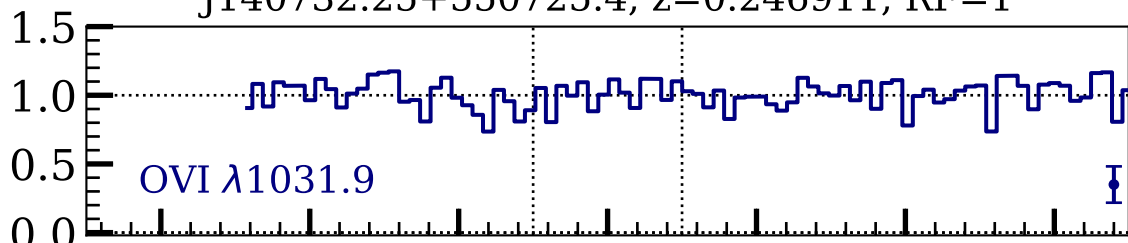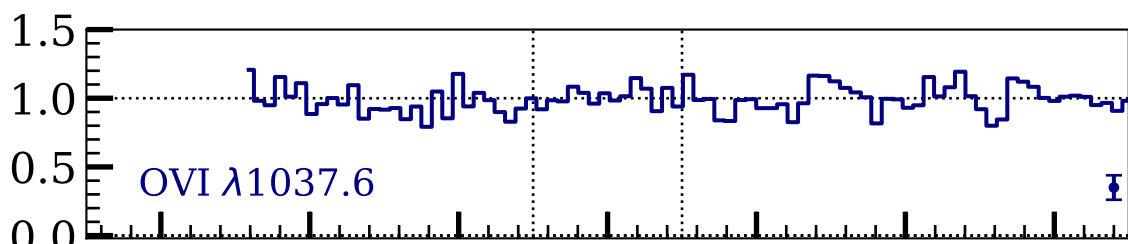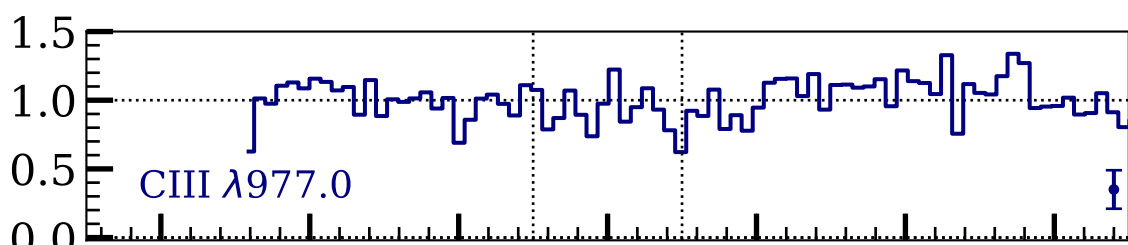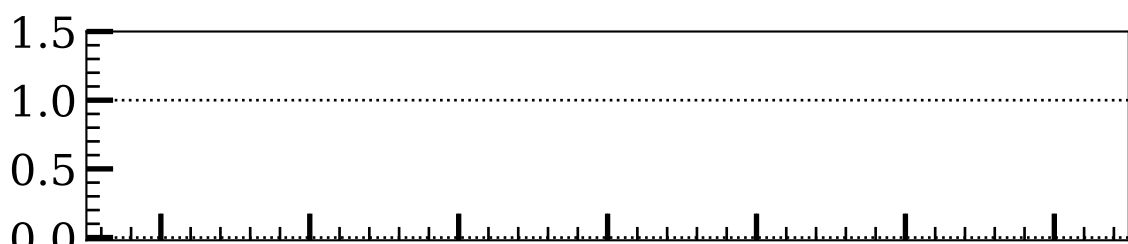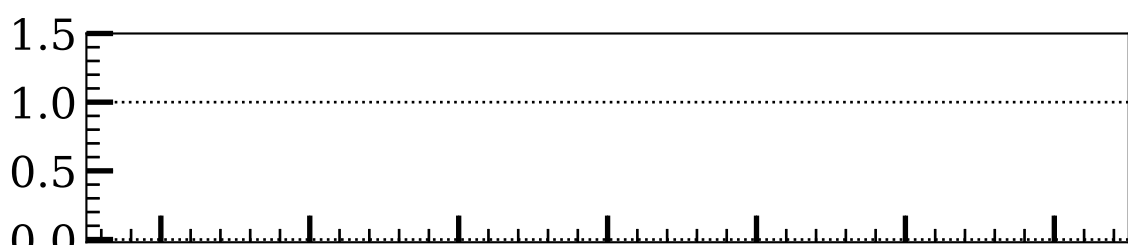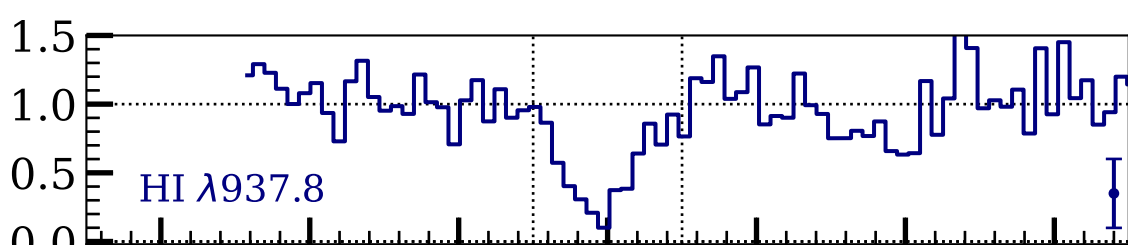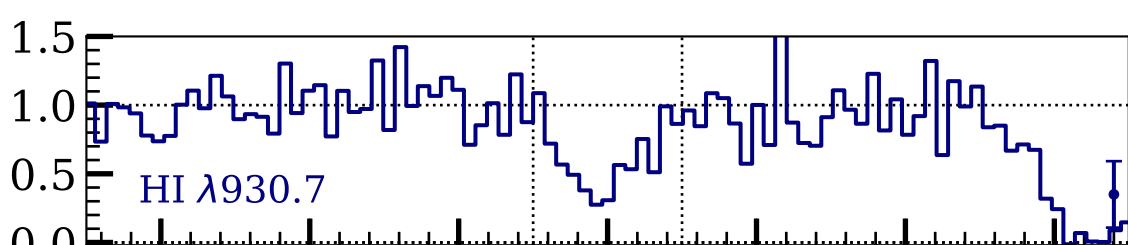

Rest-Frame Velocity ( $\text{km s}^{-1}$ )

J140923.90+261820.9,  $z=0.574868$ , RF=1

Normalized Flux

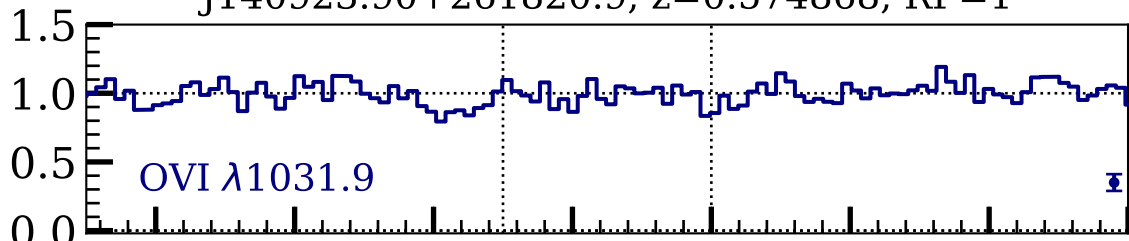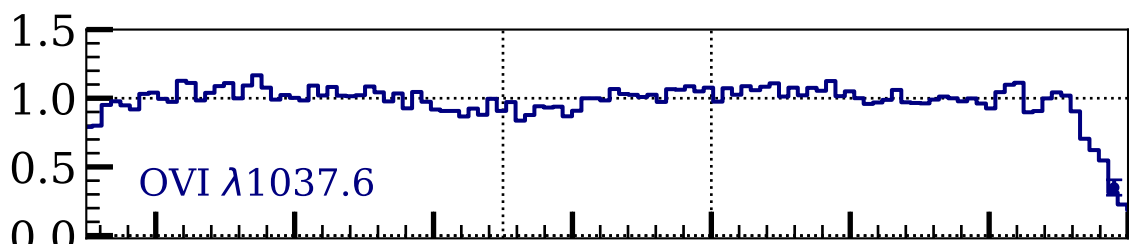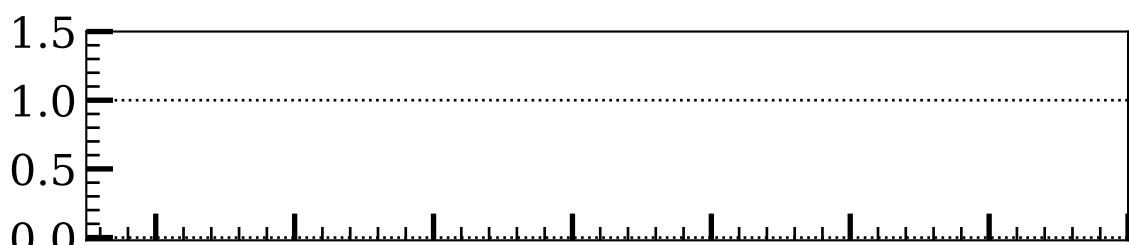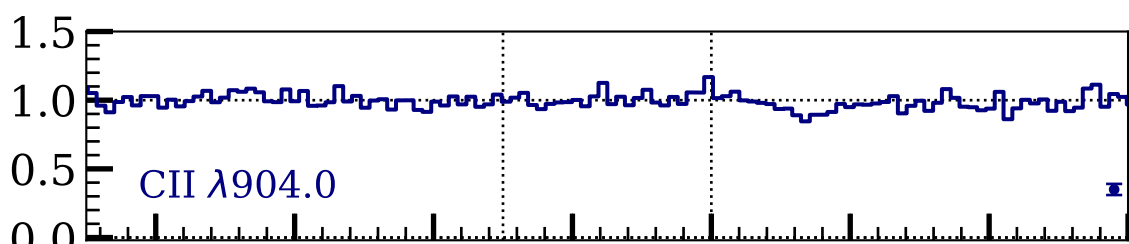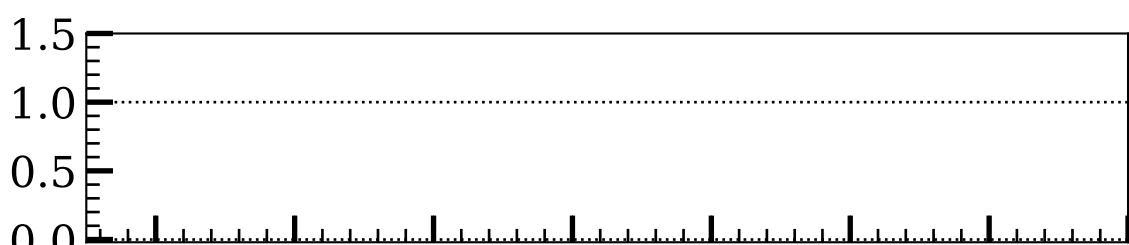

Rest-Frame Velocity ( $\text{km s}^{-1}$ )

J140923.90+261820.9,  $z=0.599561$ , RF=1

Normalized Flux

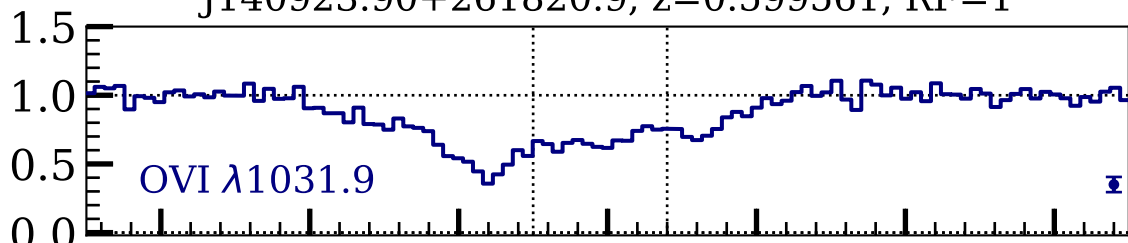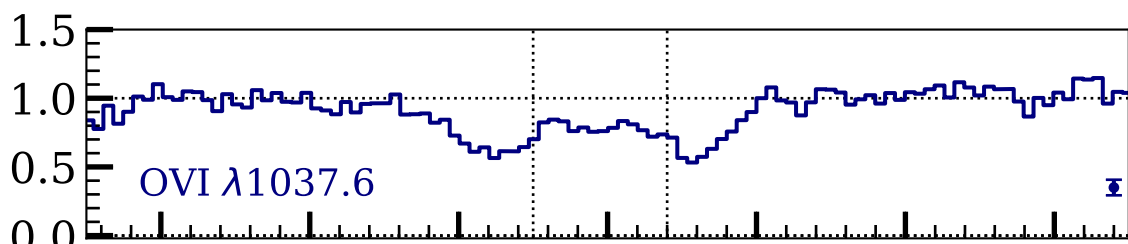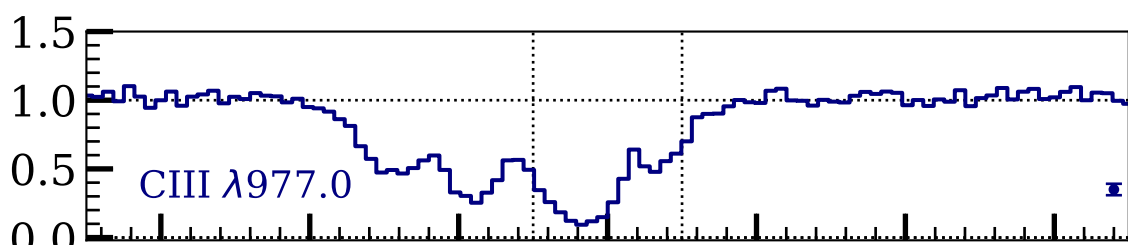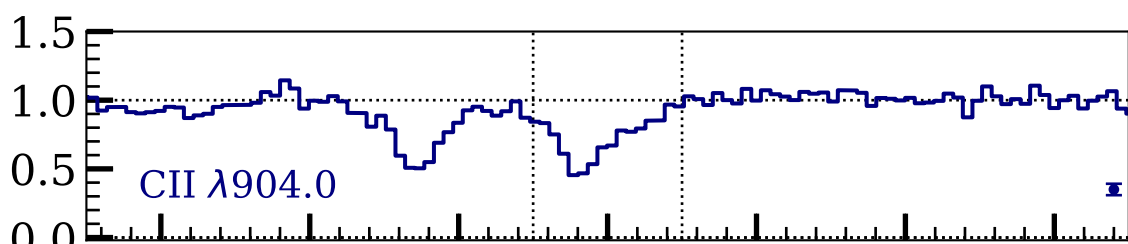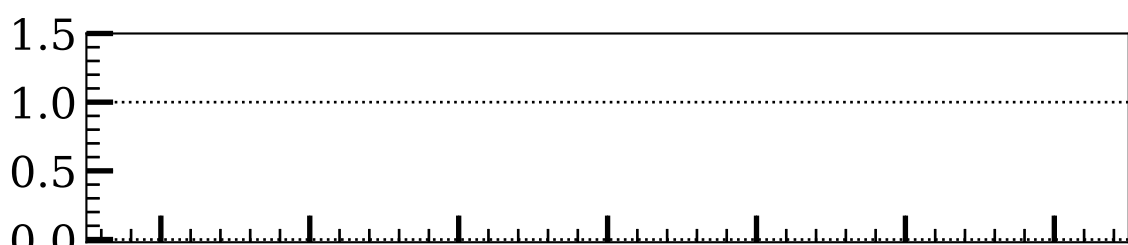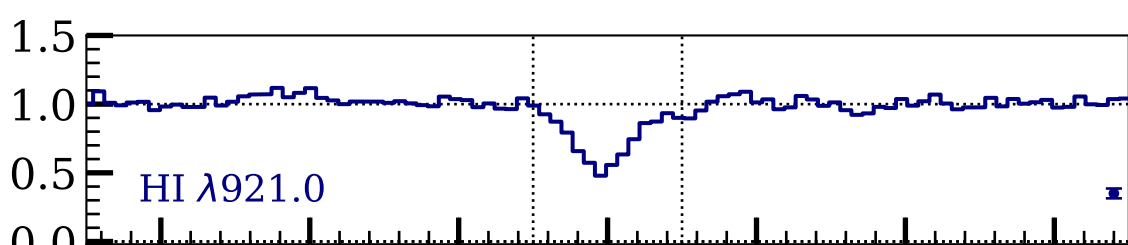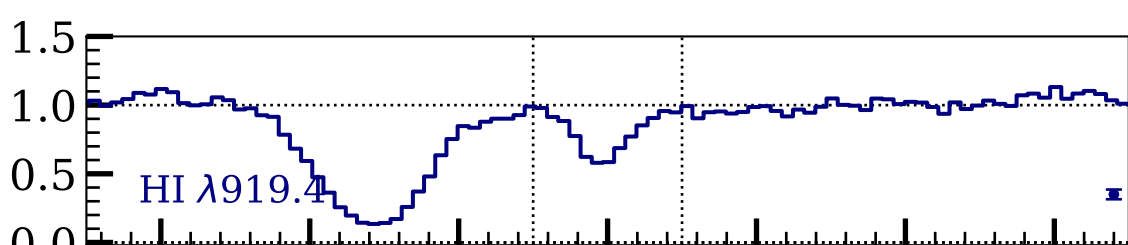

Rest-Frame Velocity ( $\text{km s}^{-1}$ )

J140923.90+261820.9,  $z=0.682684$ , RF=1

Normalized Flux

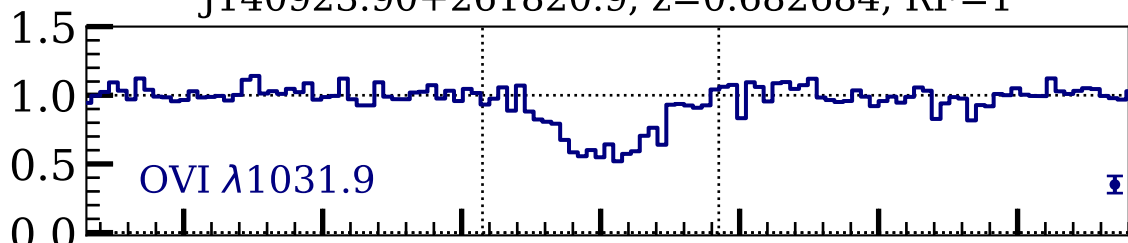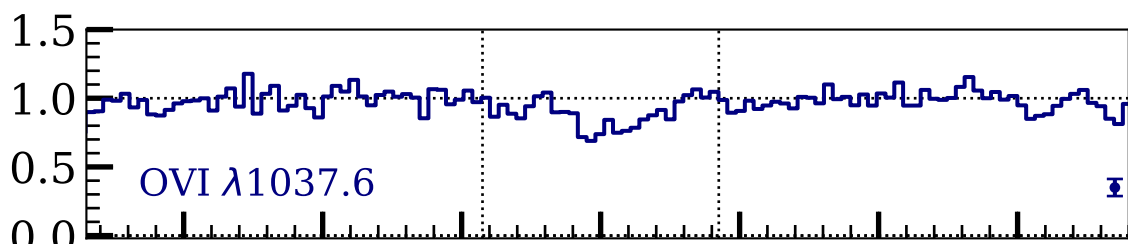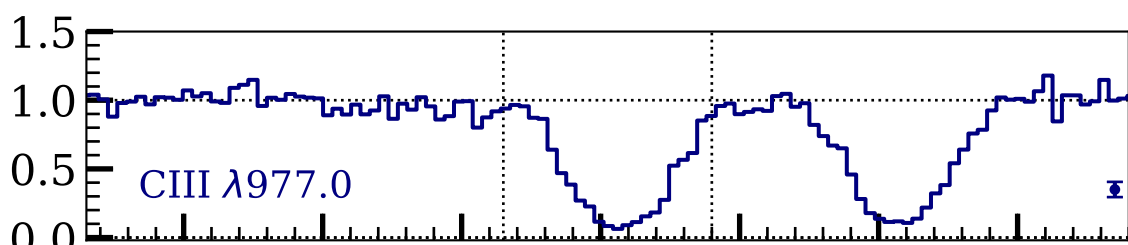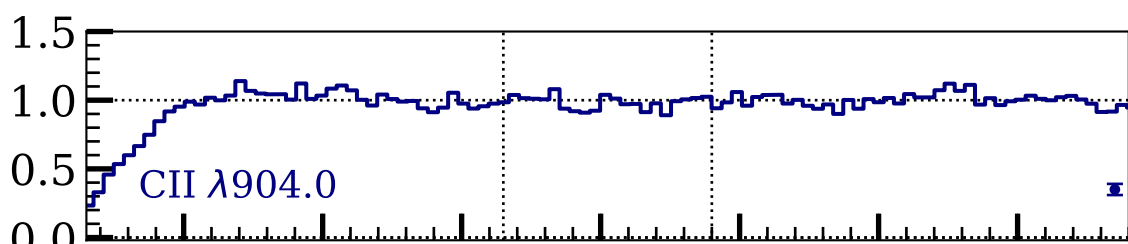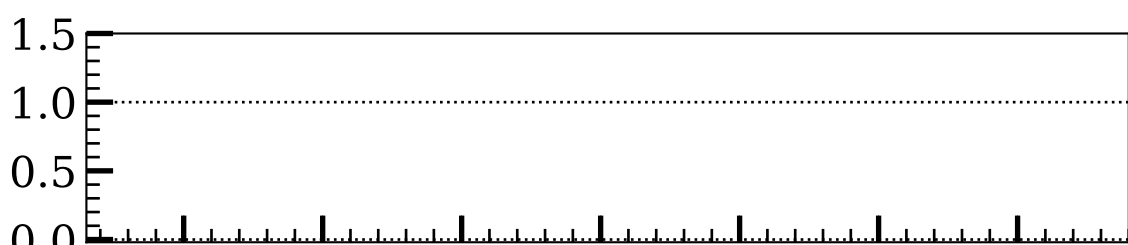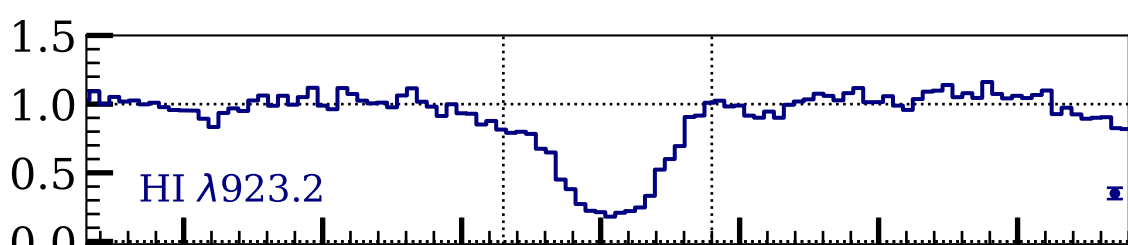

Rest-Frame Velocity ( $\text{km s}^{-1}$ )

J141038.39+230447.1,  $z=0.349849$ , RF=1

Normalized Flux

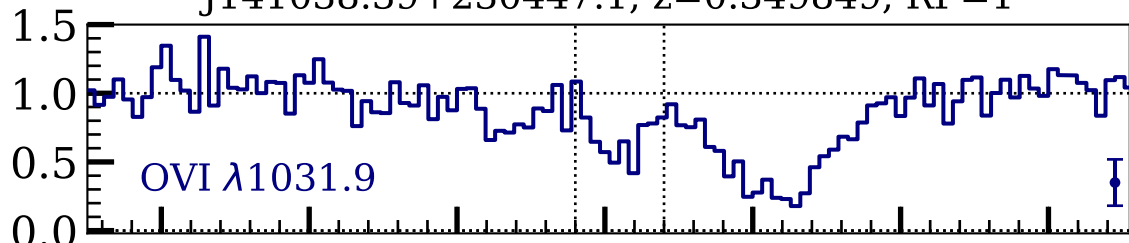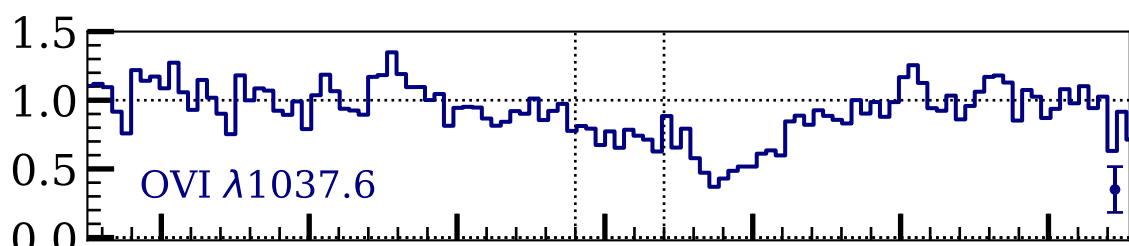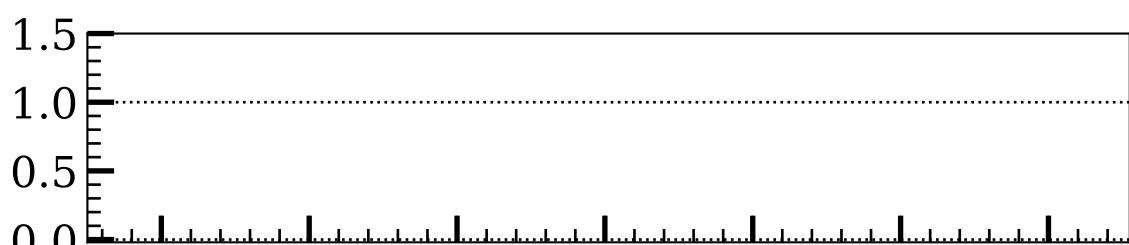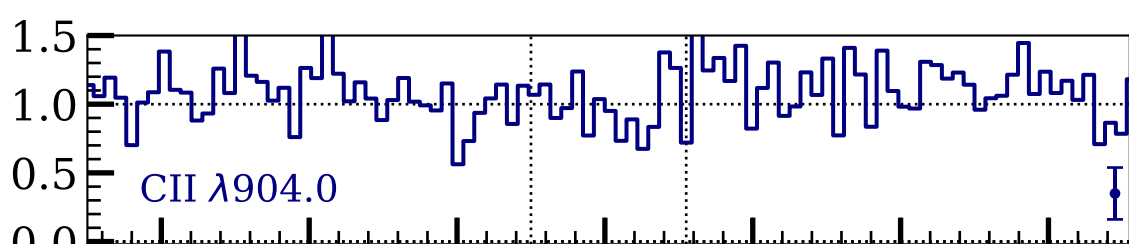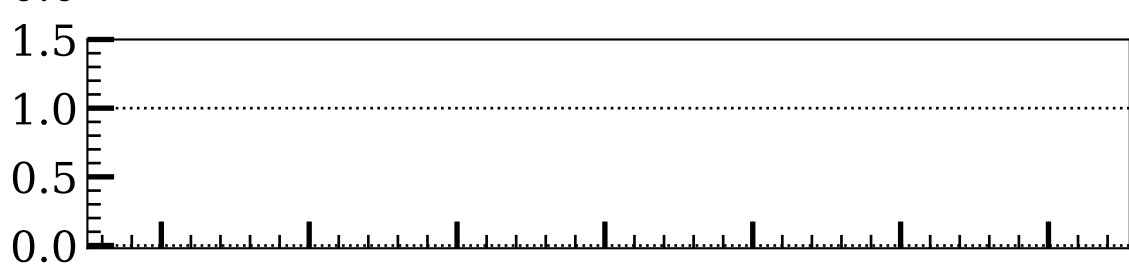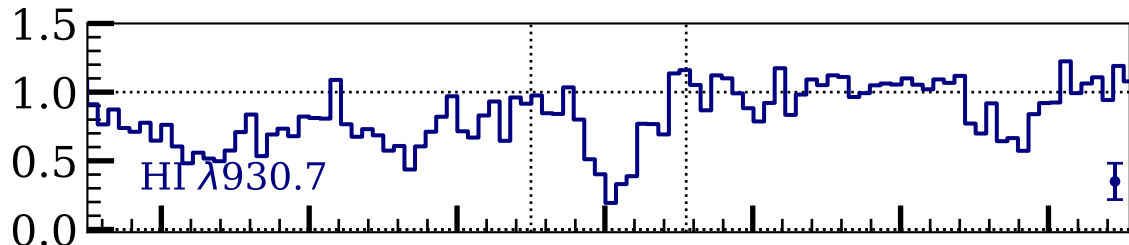

Rest-Frame Velocity ( $\text{km s}^{-1}$ )

J141038.39+230447.1,  $z=0.351043$ , RF=1

Normalized Flux

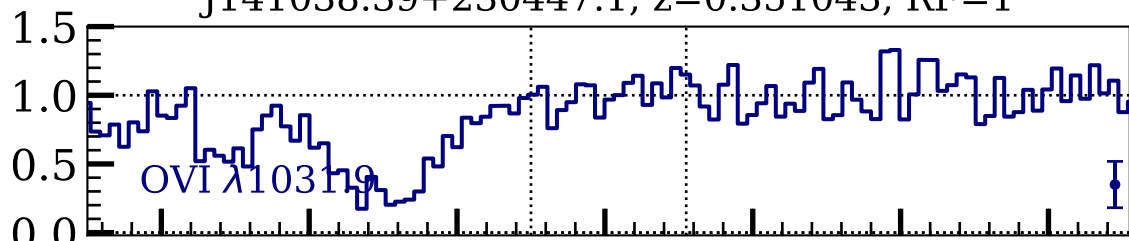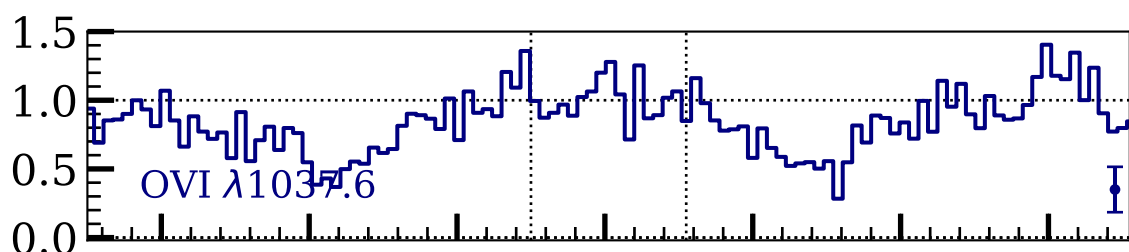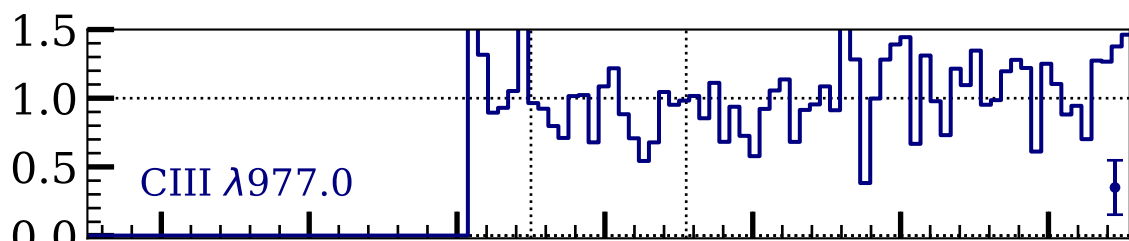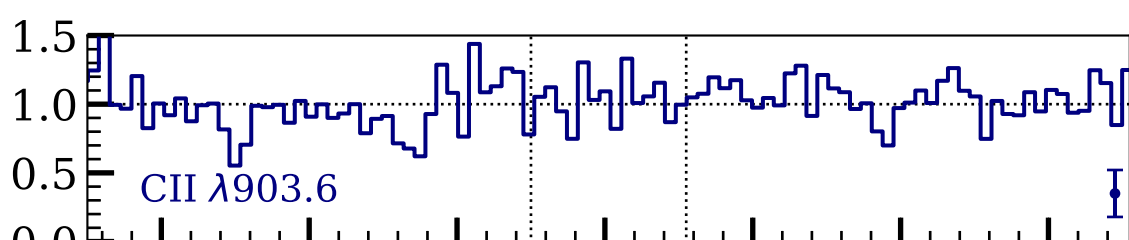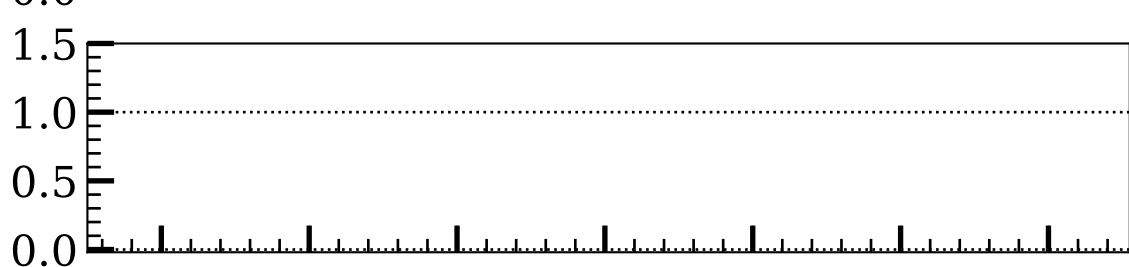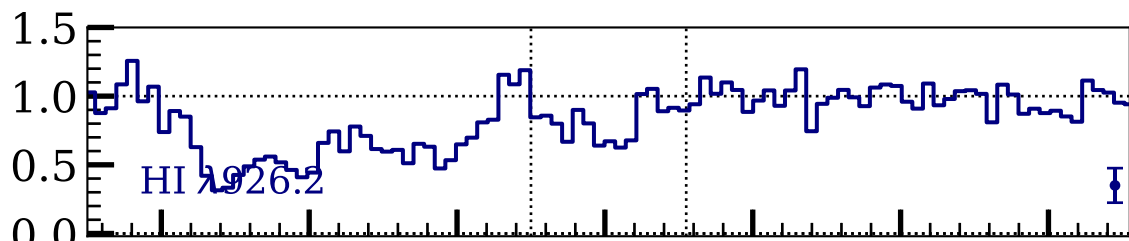

Rest-Frame Velocity ( $\text{km s}^{-1}$ )

J141038.39+230447.1,  $z=0.535079$ , RF=1

Normalized Flux

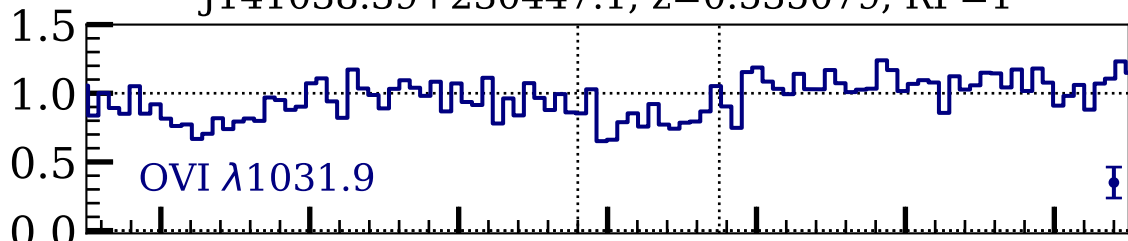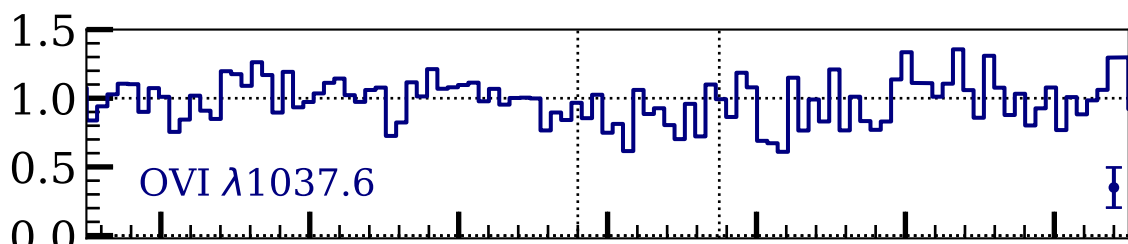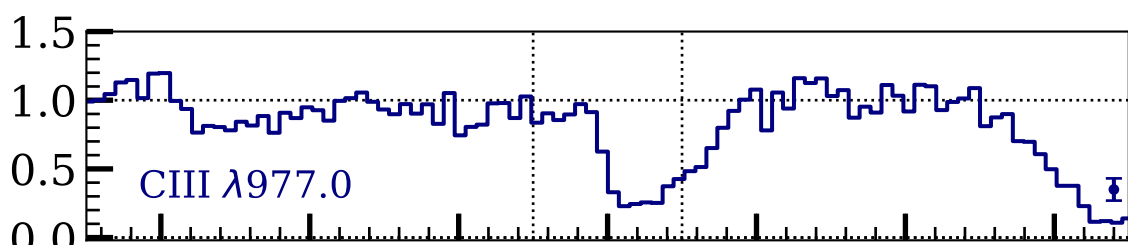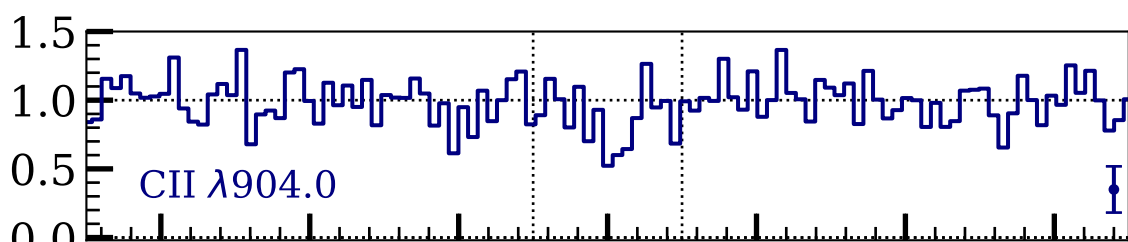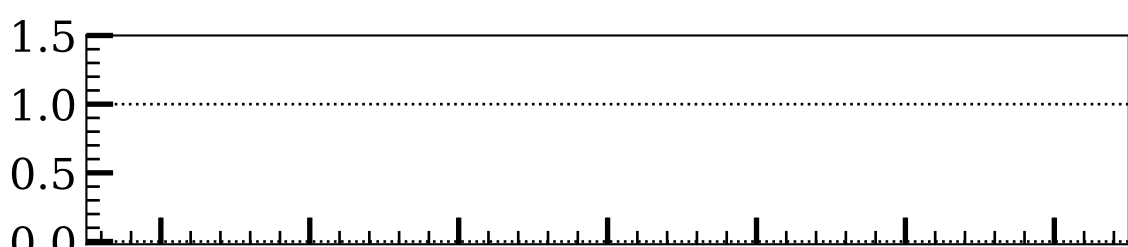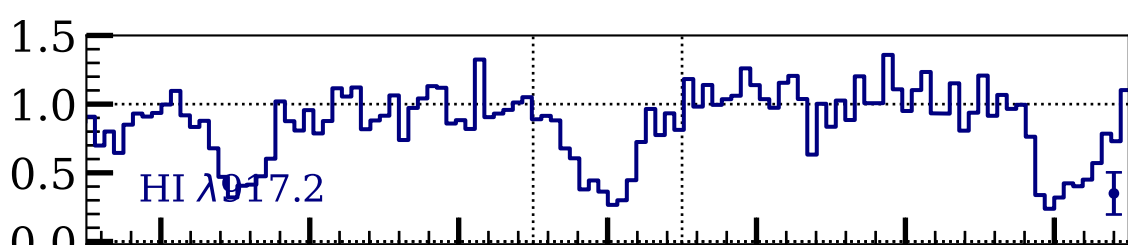

Rest-Frame Velocity ( $\text{km s}^{-1}$ )

J141910.20+420746.9,  $z=0.288976$ , RF=0

Normalized Flux

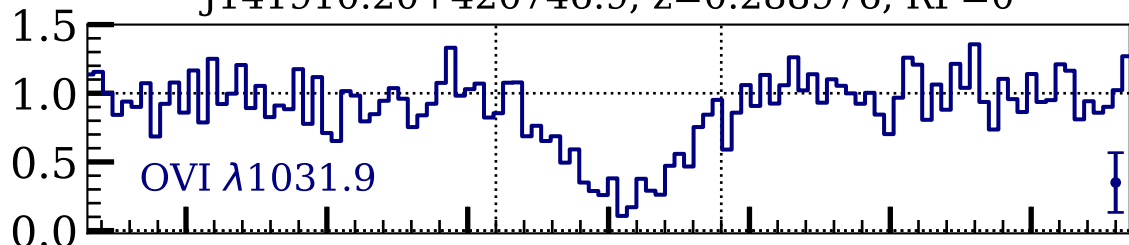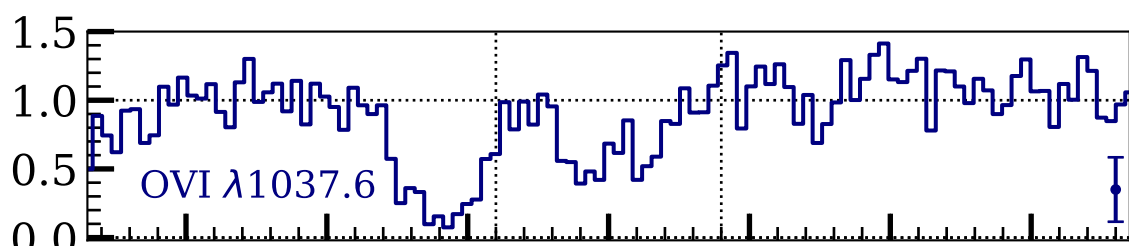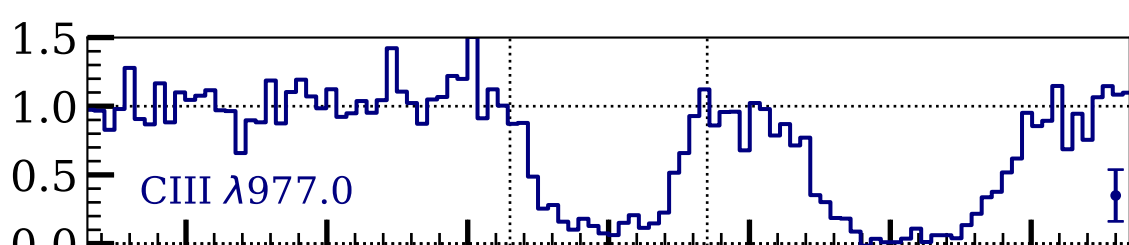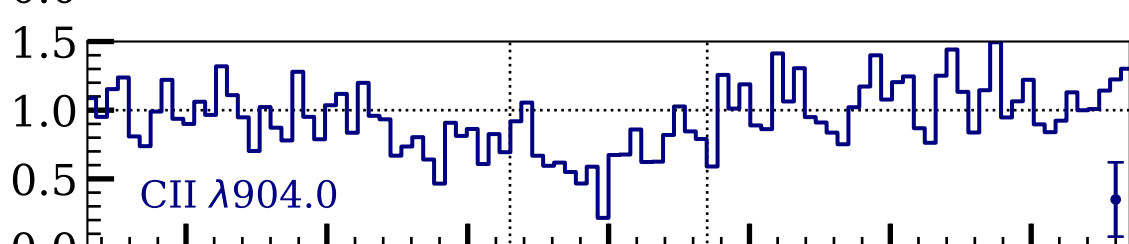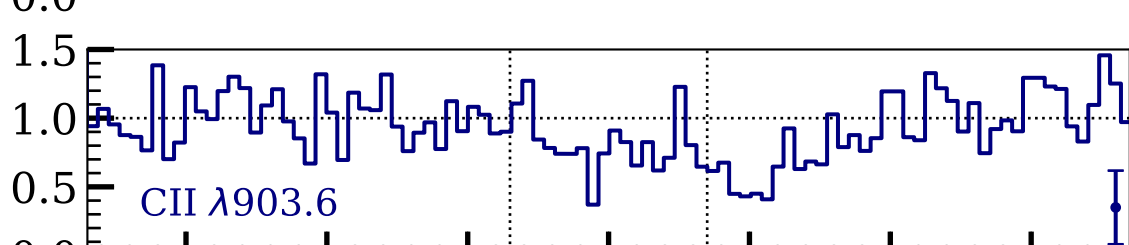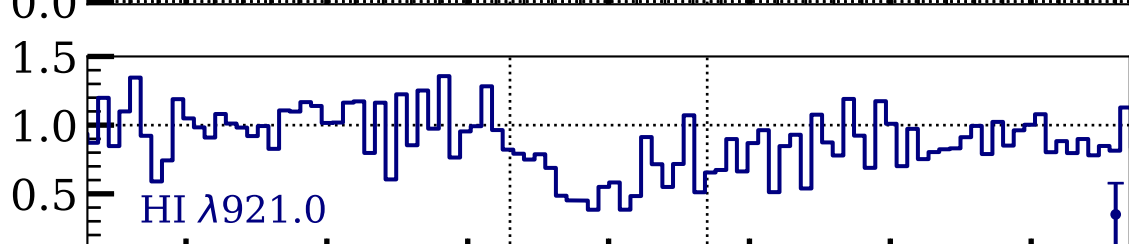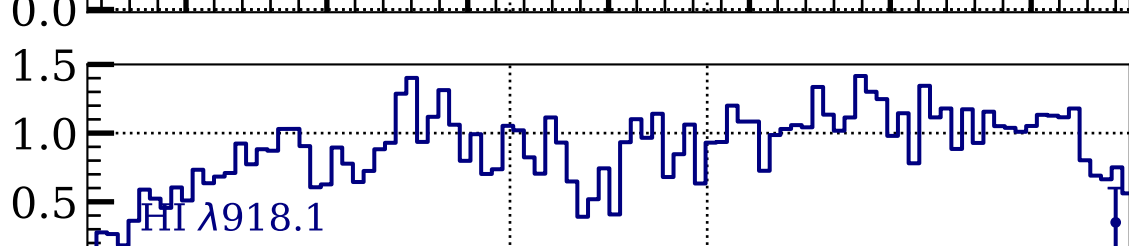

Rest-Frame Velocity ( $\text{km s}^{-1}$ )



J141910.20+420746.9,  $z=0.425592$ , RF=1

Normalized Flux

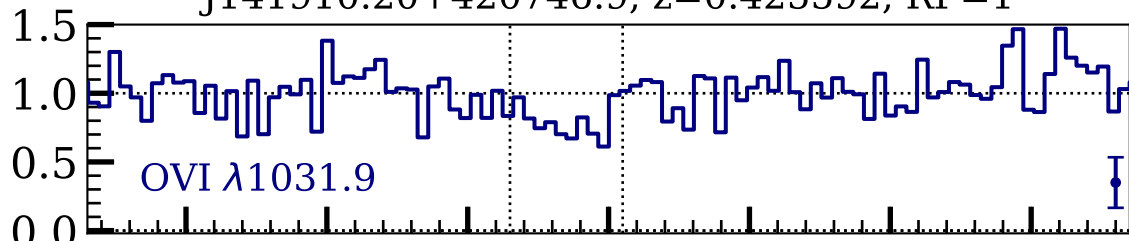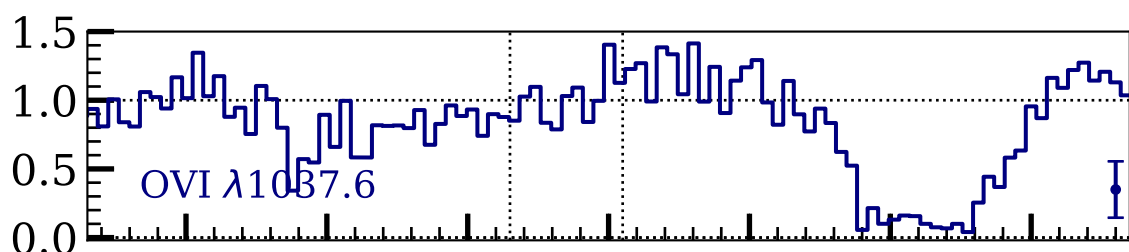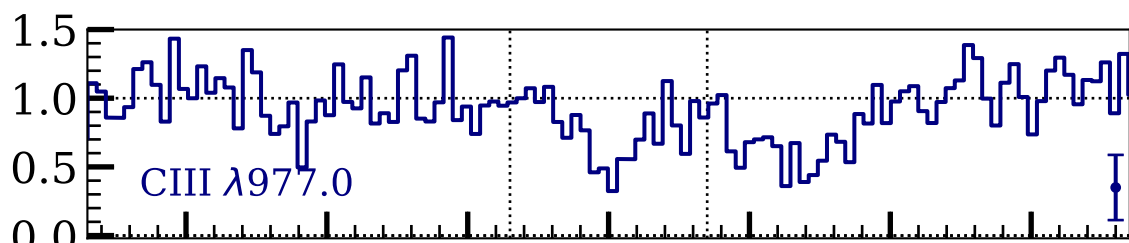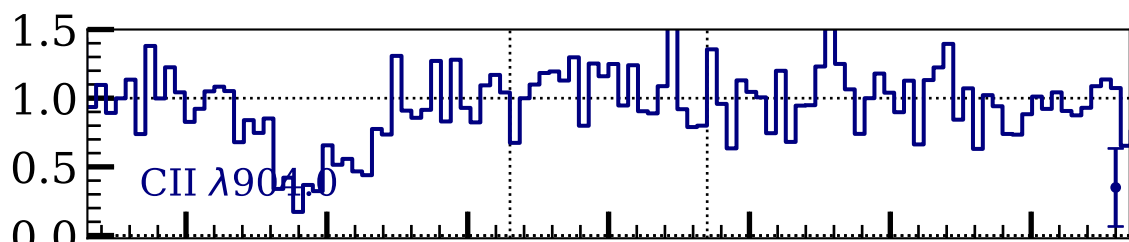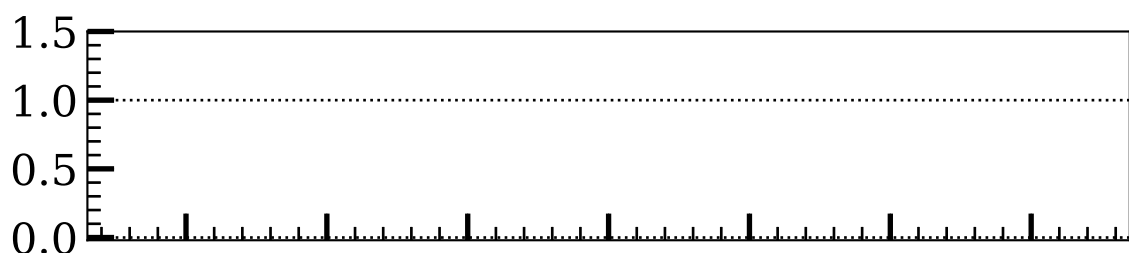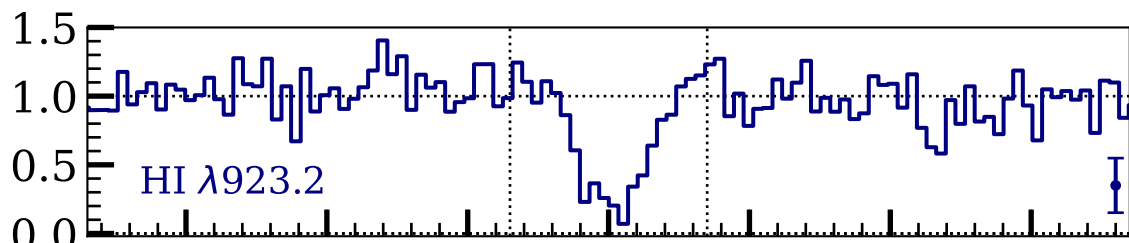

Rest-Frame Velocity (km s<sup>-1</sup>)

J141910.20+420746.9,  $z=0.522082$ , RF=0

Normalized Flux

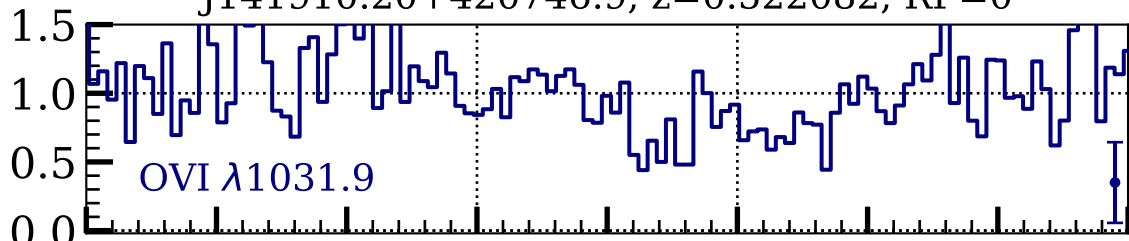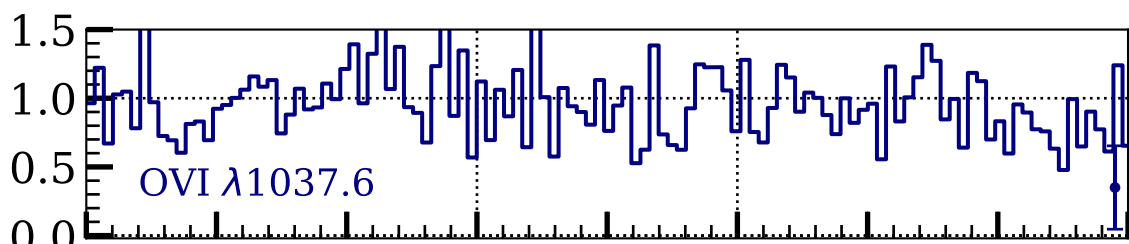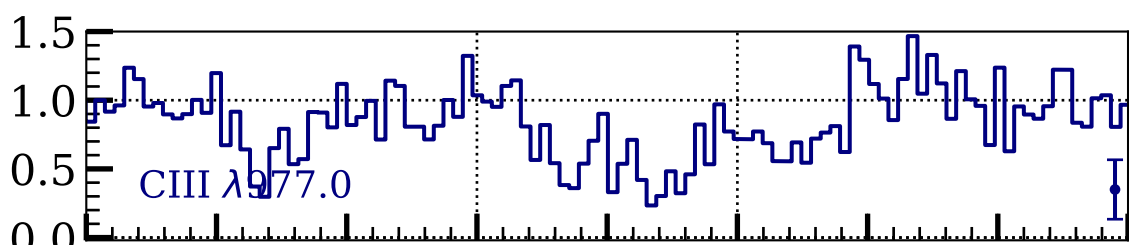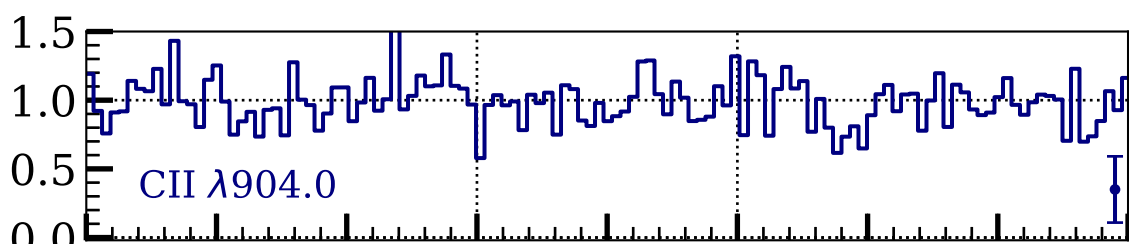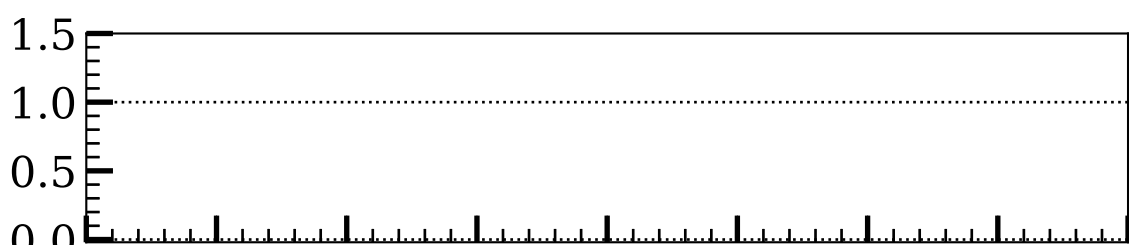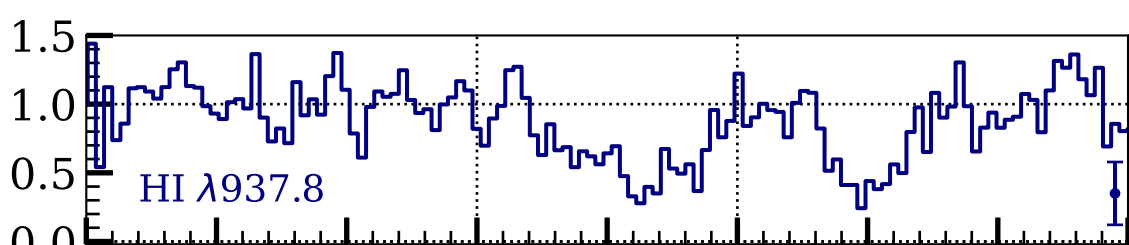

Rest-Frame Velocity ( $\text{km s}^{-1}$ )

J141910.20+420746.9,  $z=0.534585$ , RF=0

Normalized Flux

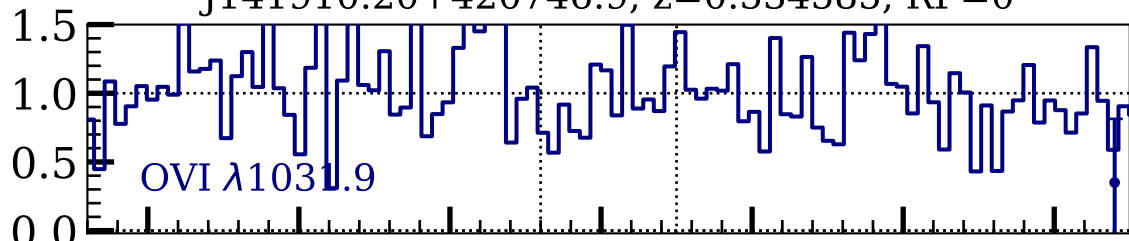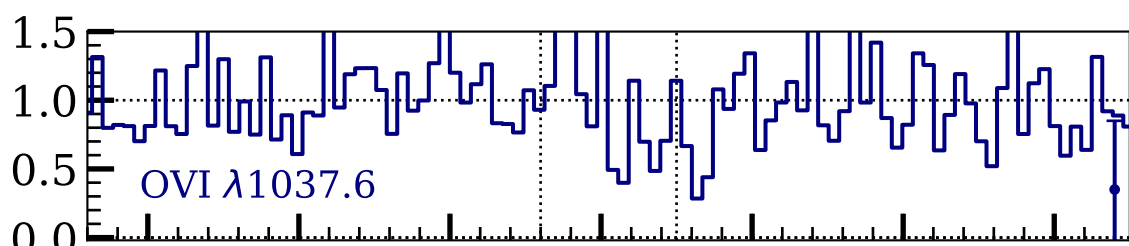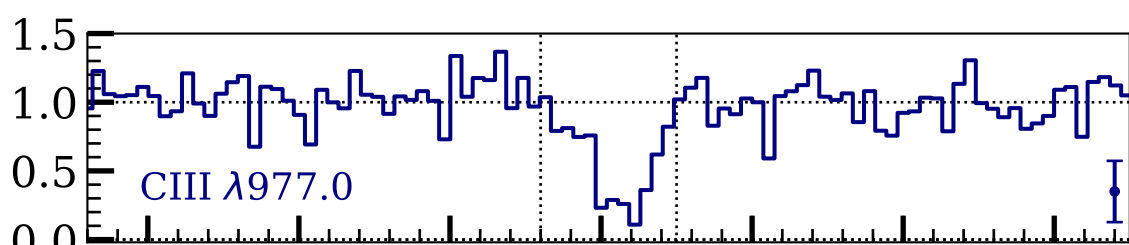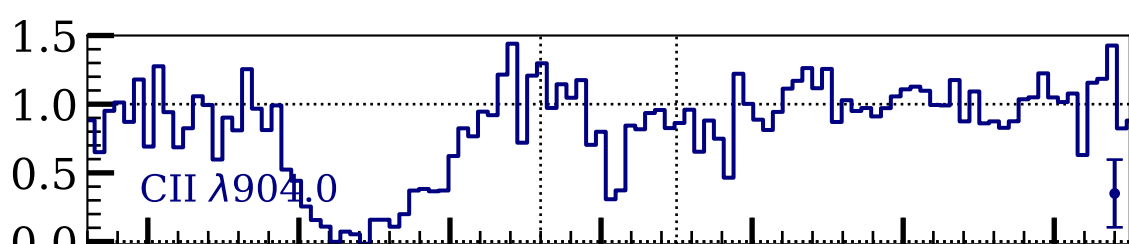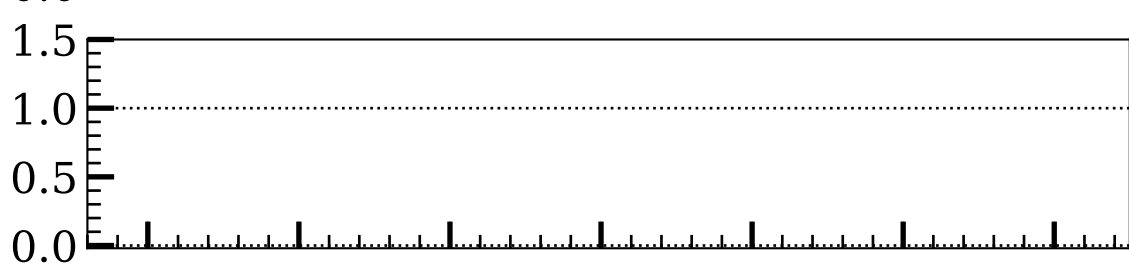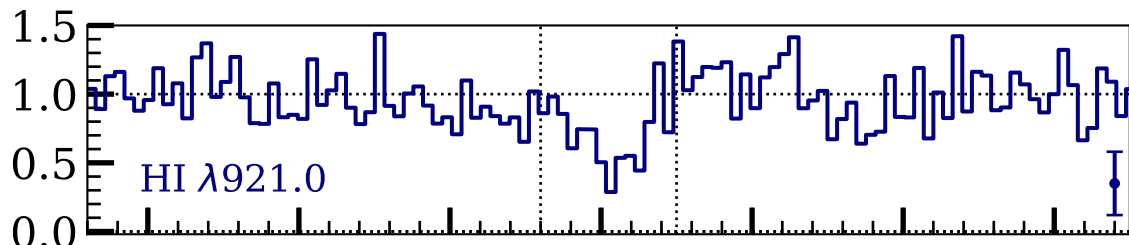

Rest-Frame Velocity ( $\text{km s}^{-1}$ )

J141910.20+420746.9,  $z=0.608265$ , RF=0

Normalized Flux

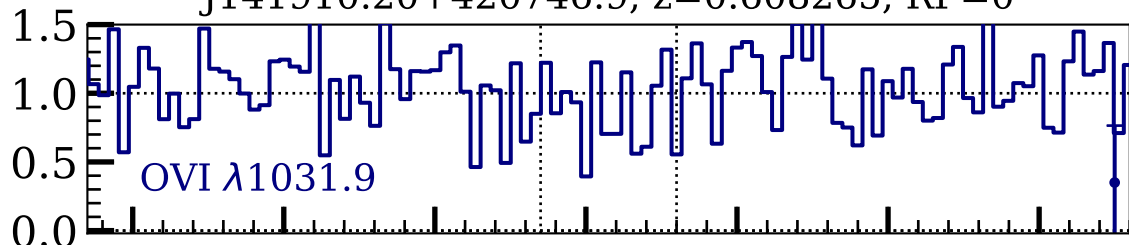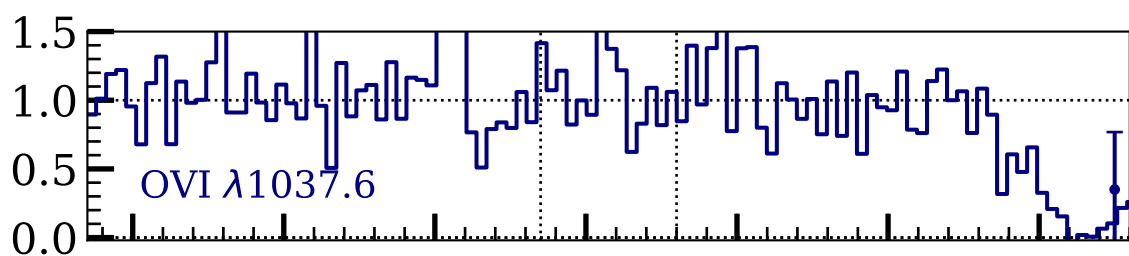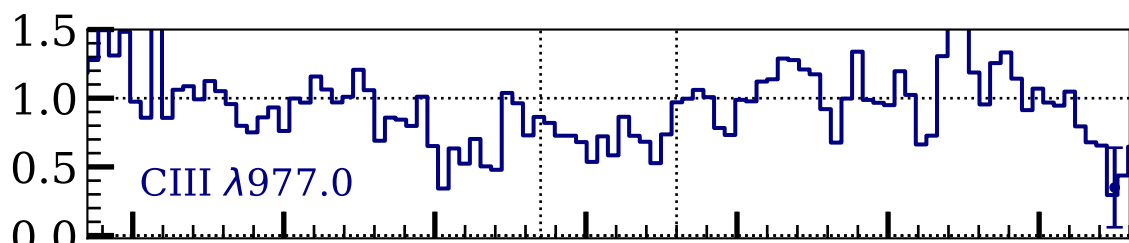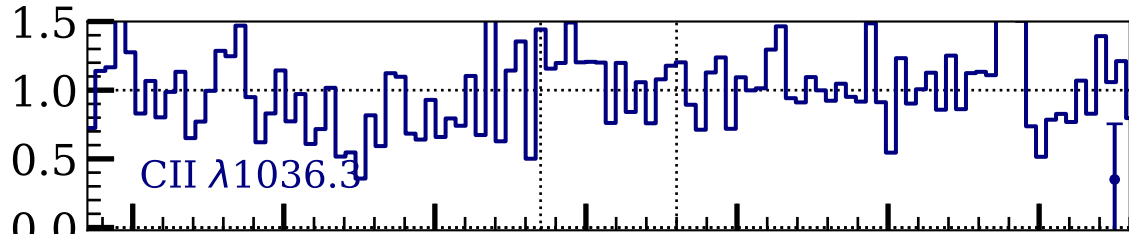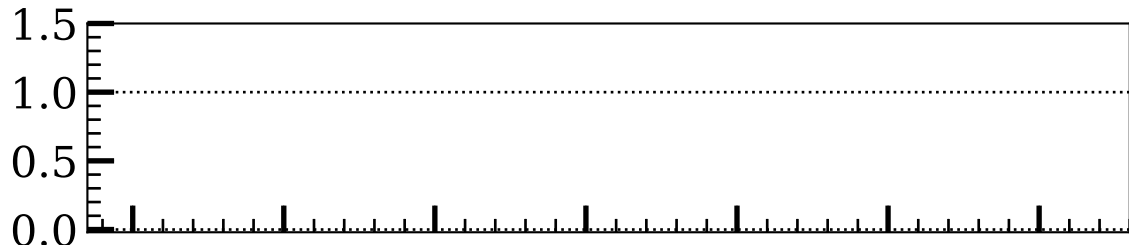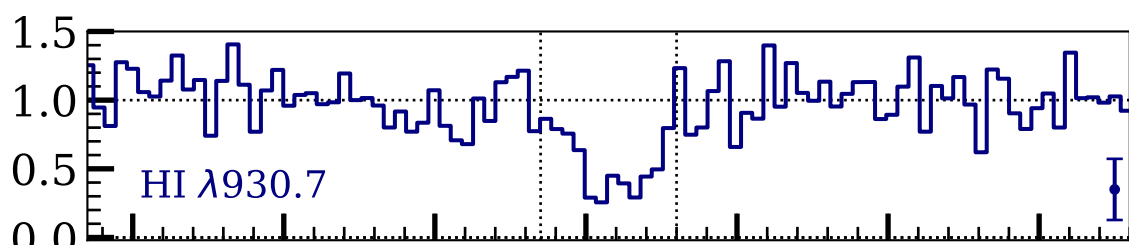

Rest-Frame Velocity ( $\text{km s}^{-1}$ )

J142735.59+263214.6,  $z=0.366054$ , RF=0

Normalized Flux

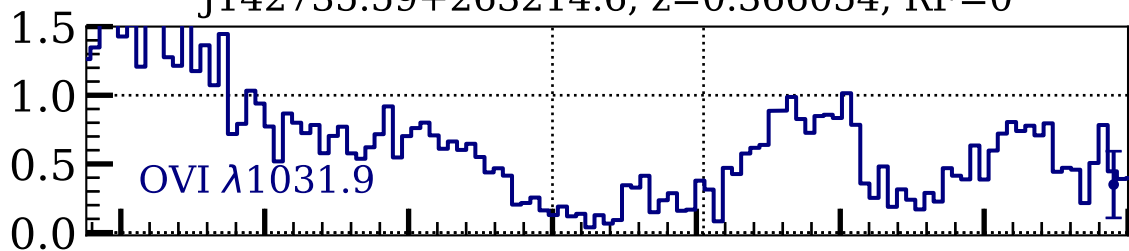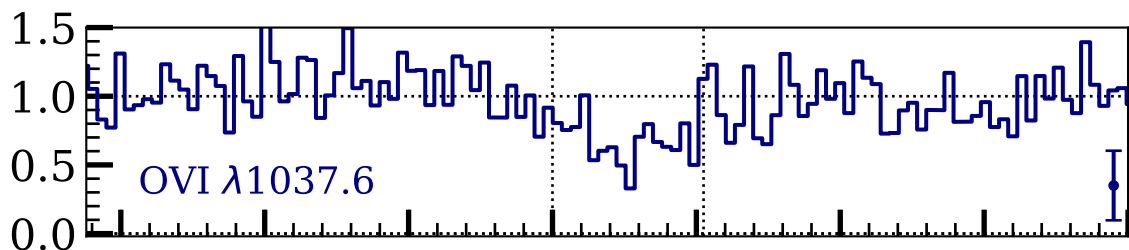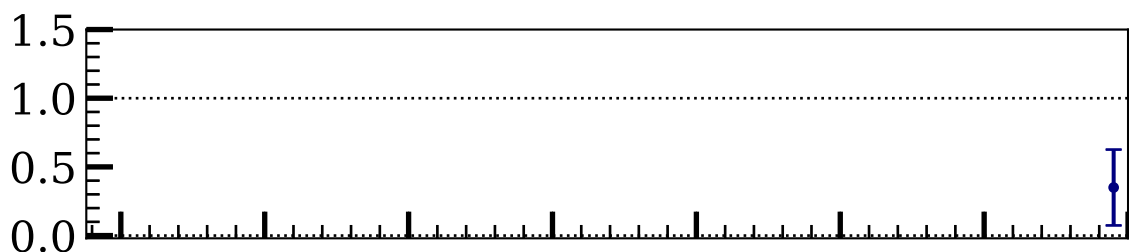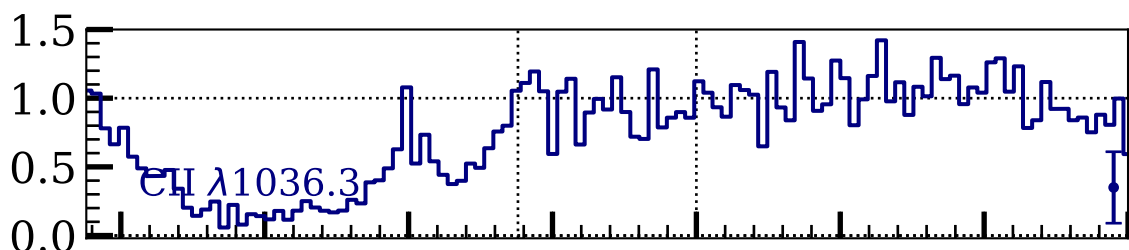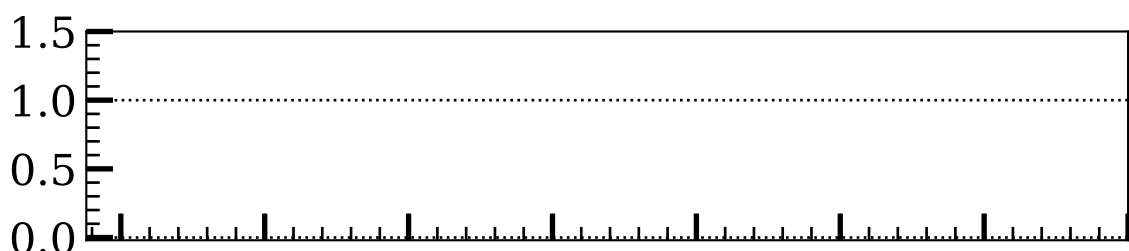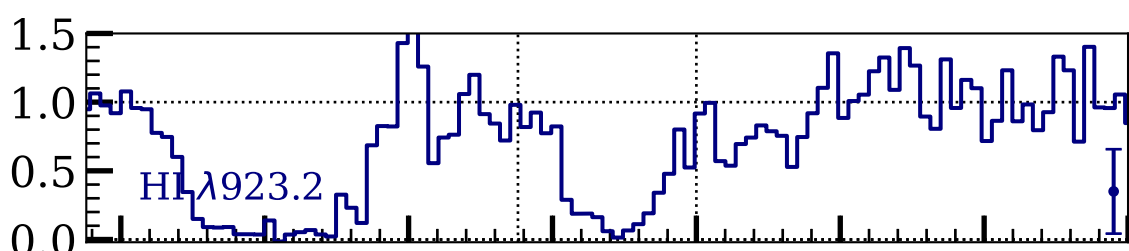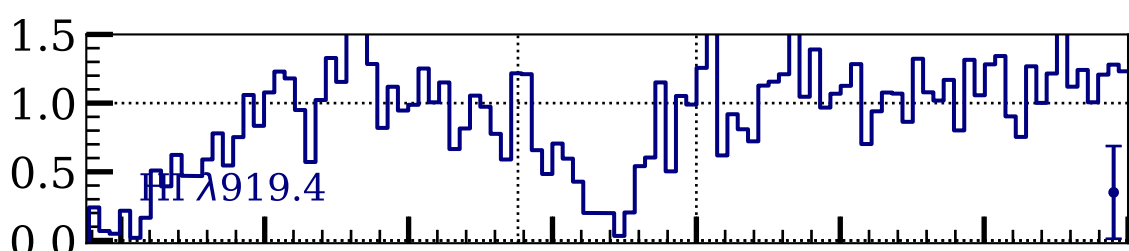

Rest-Frame Velocity ( $\text{km s}^{-1}$ )

J142859.03+322506.8,  $z=0.382333$ , RF=1

Normalized Flux

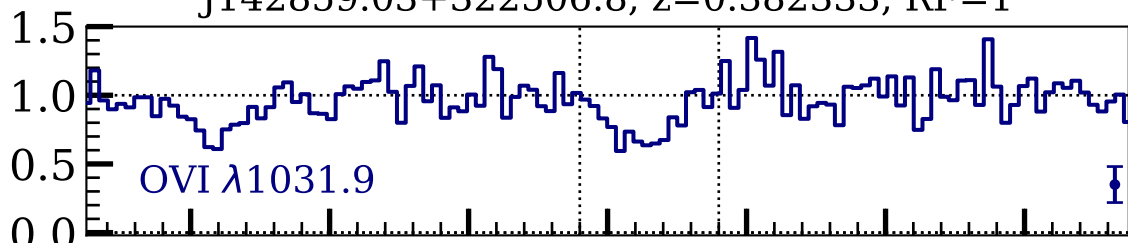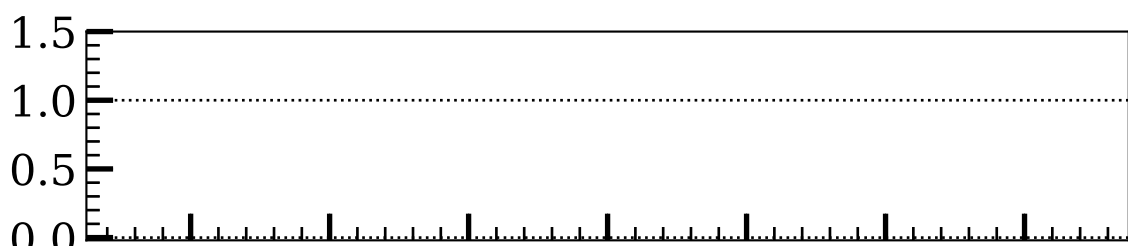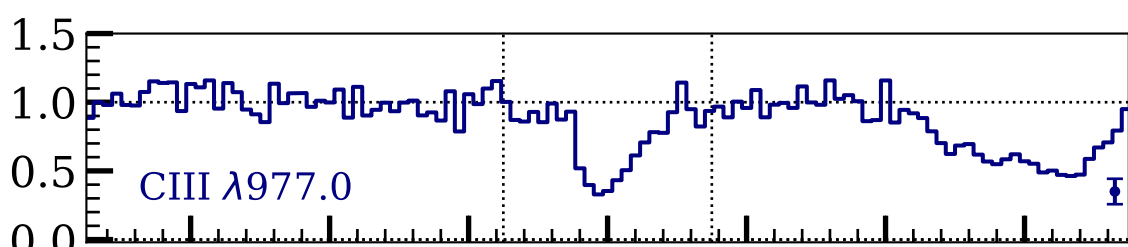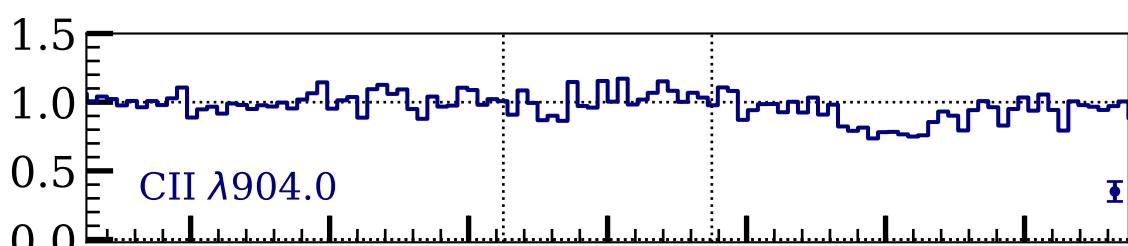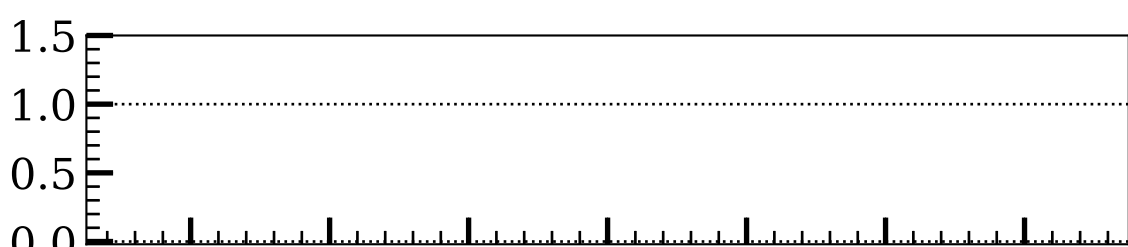

Rest-Frame Velocity ( $\text{km s}^{-1}$ )

J143511.53+360437.2,  $z=0.372981$ , RF=1

Normalized Flux

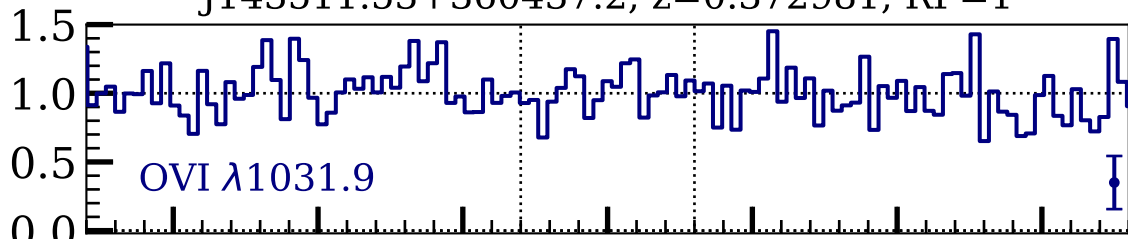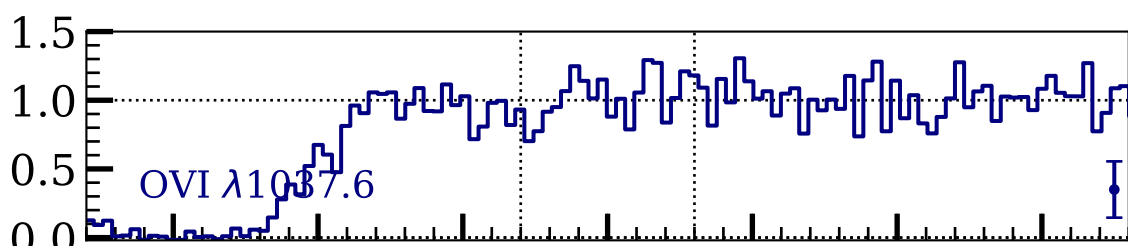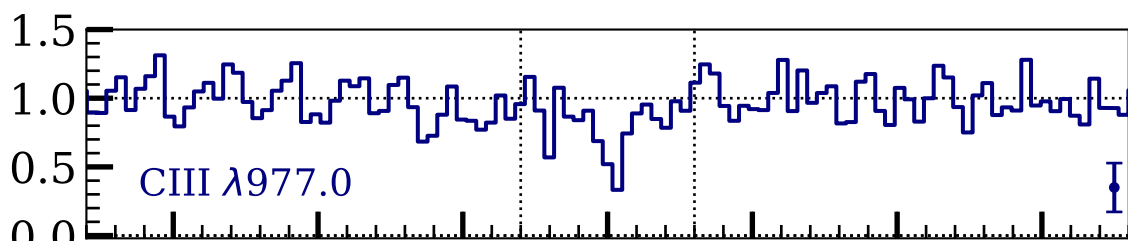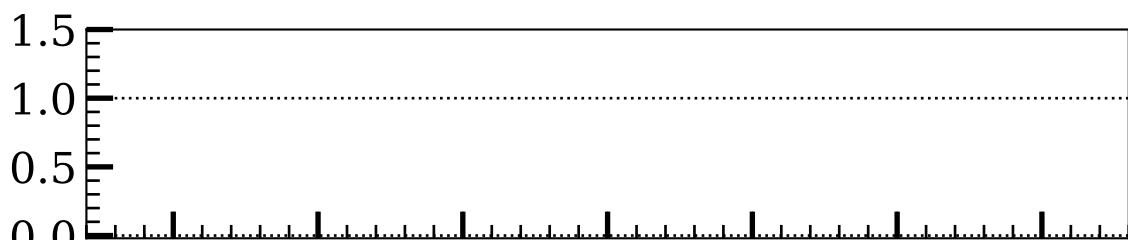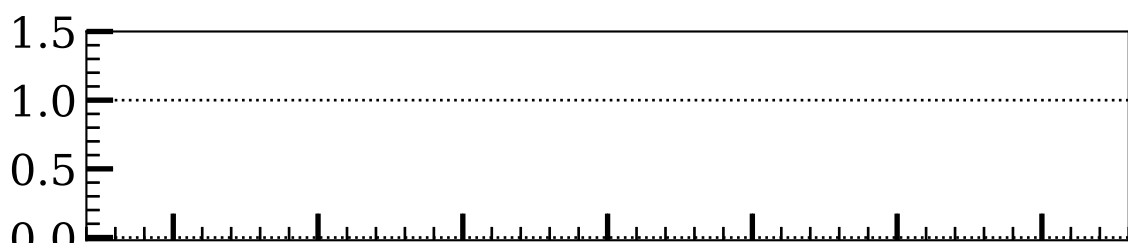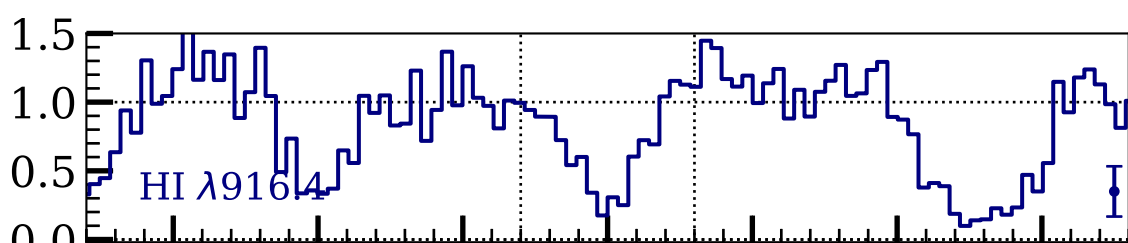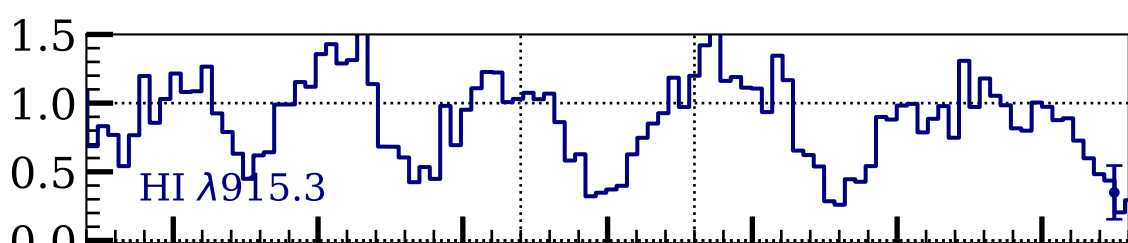

Rest-Frame Velocity ( $\text{km s}^{-1}$ )

J143511.53+360437.2,  $z=0.387594$ , RF=0

Normalized Flux

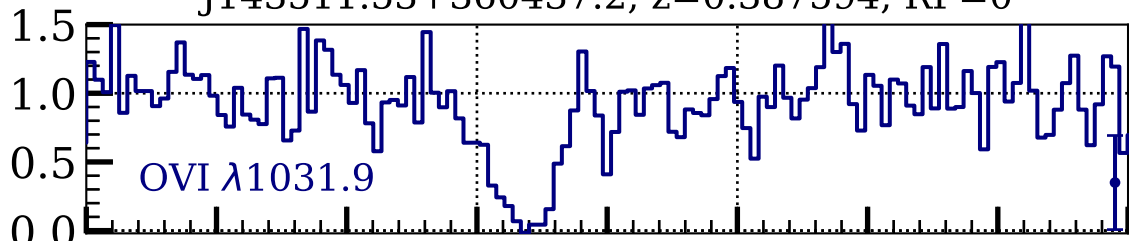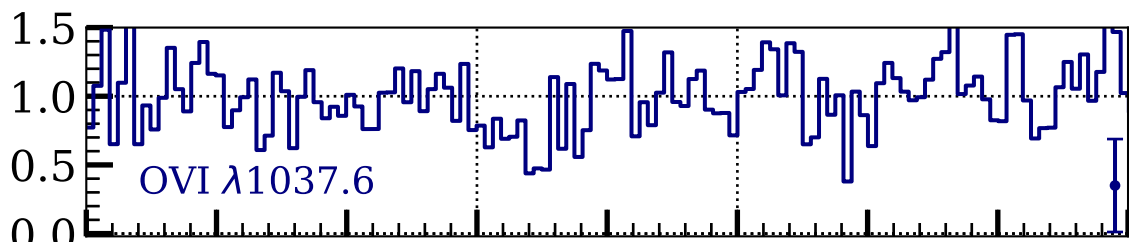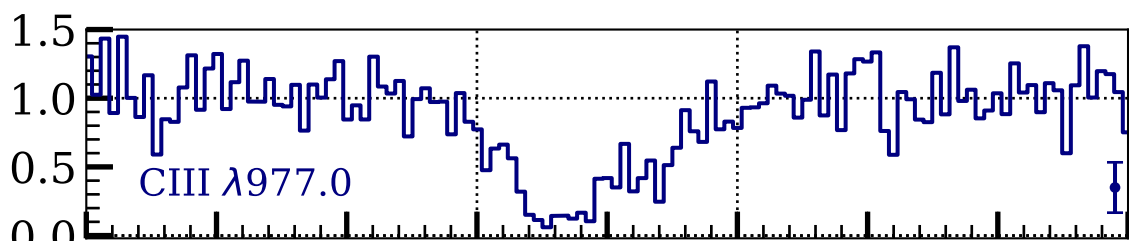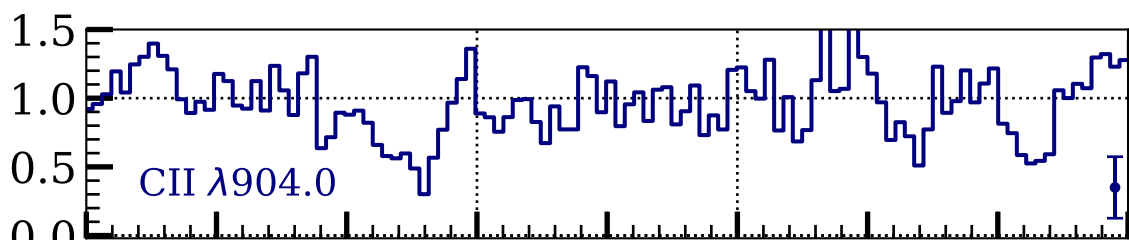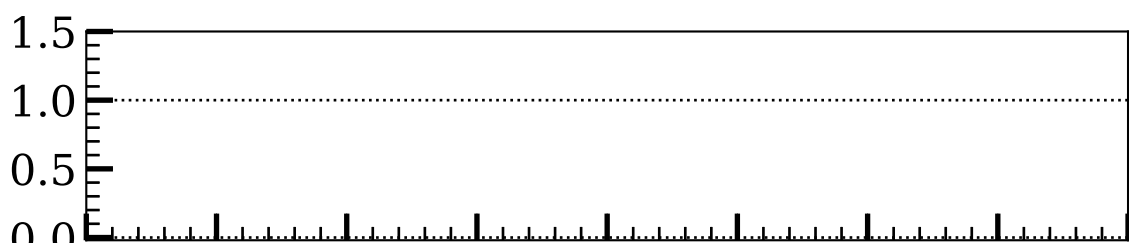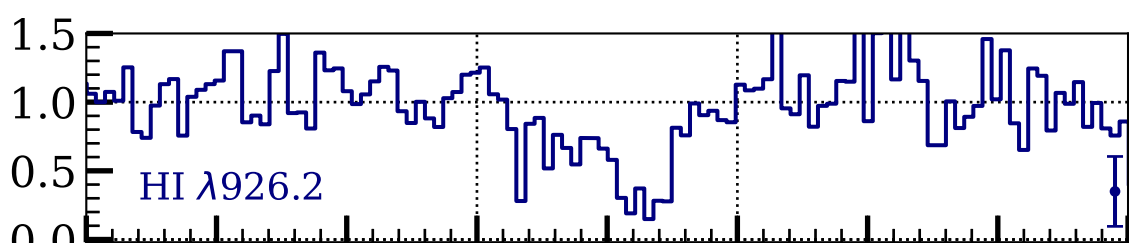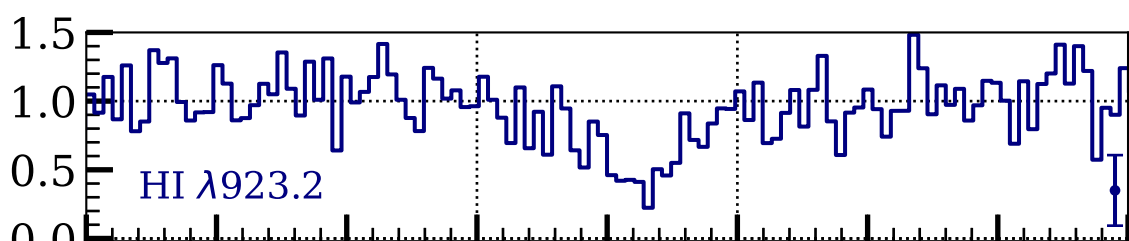

Rest-Frame Velocity ( $\text{km s}^{-1}$ )



J143748.28-014710.7,  $z=0.298949$ , RF=1

Normalized Flux

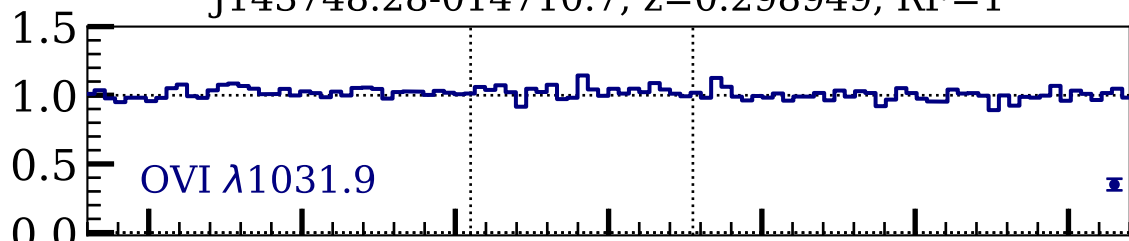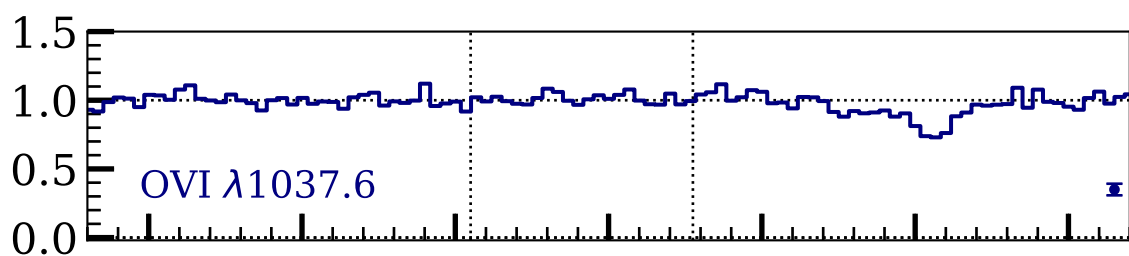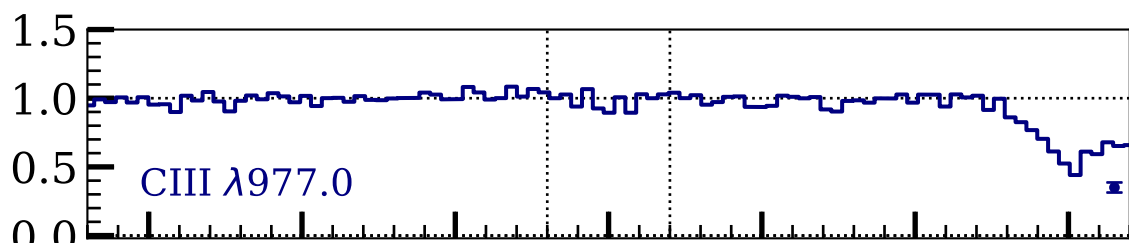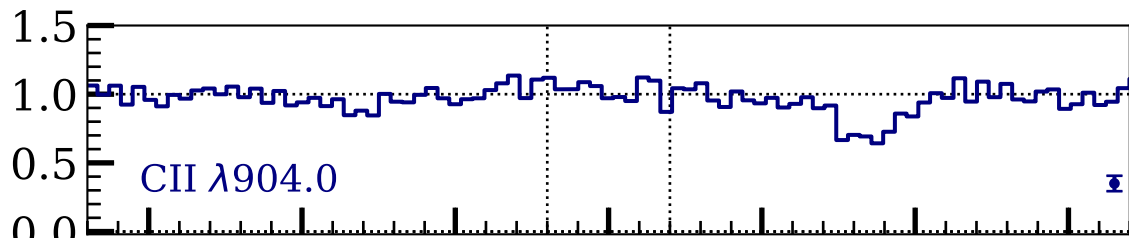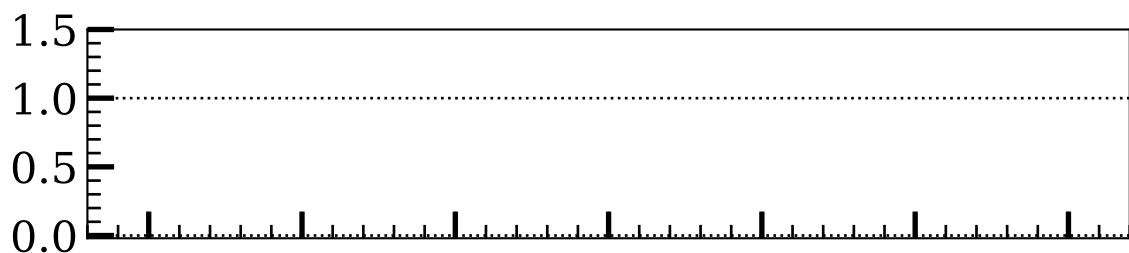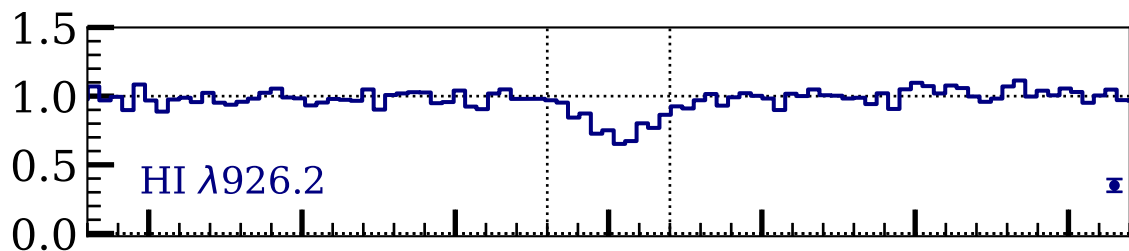

Rest-Frame Velocity ( $\text{km s}^{-1}$ )

J143748.28-014710.7,  $z=0.612744$ , RF=1

Normalized Flux

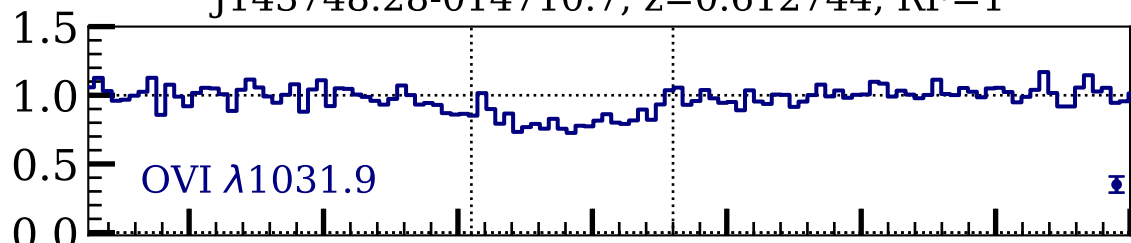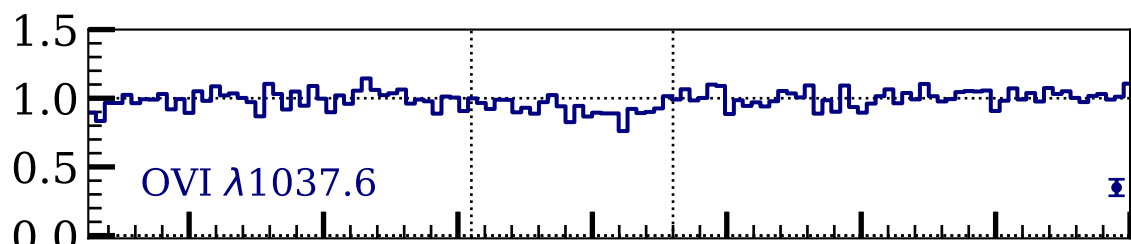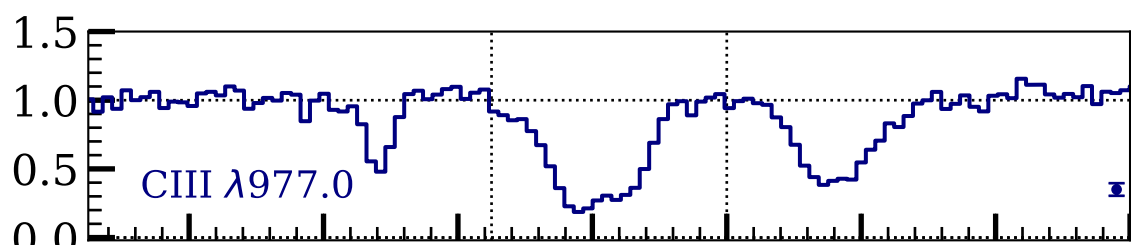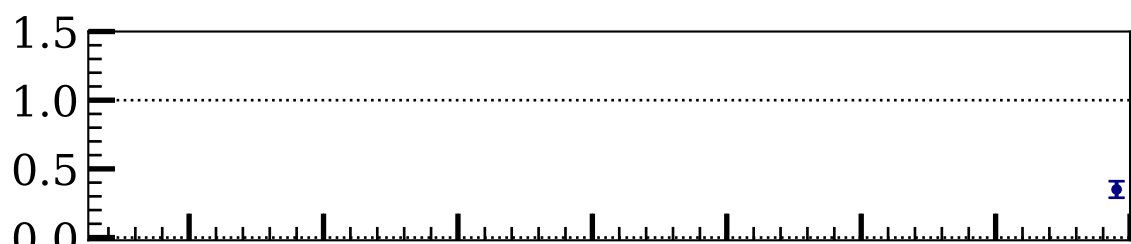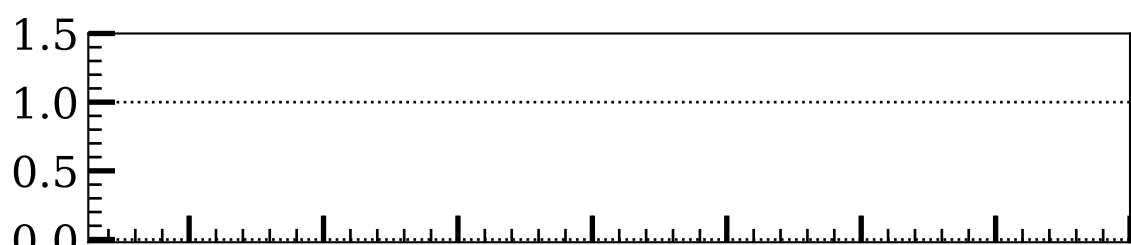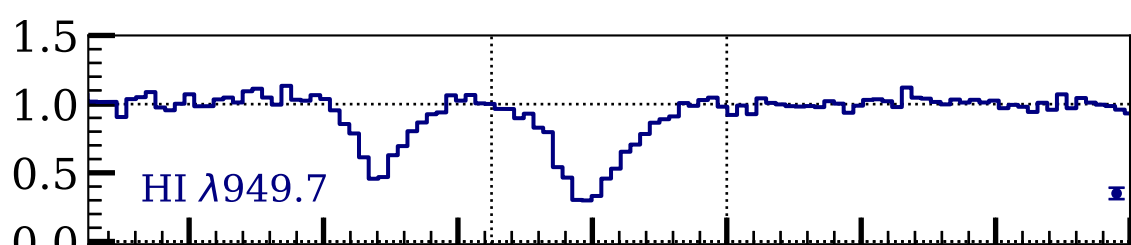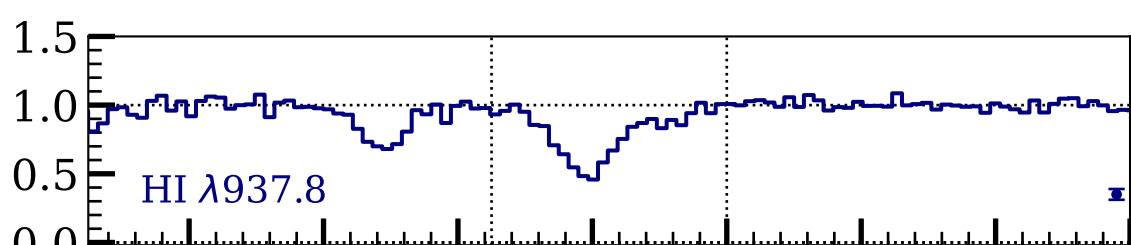

Rest-Frame Velocity ( $\text{km s}^{-1}$ )

J143748.28-014710.7,  $z=0.681207$ , RF=1

Normalized Flux

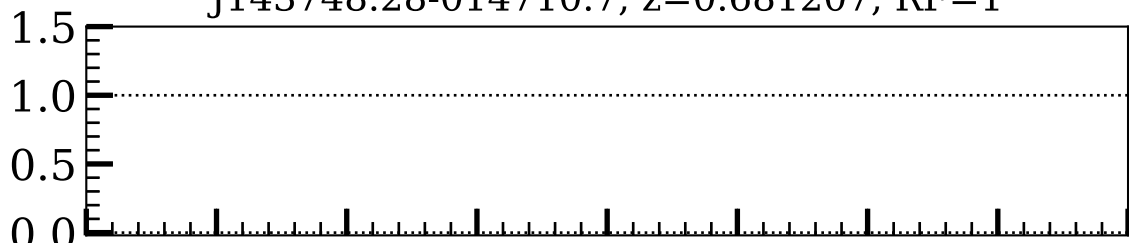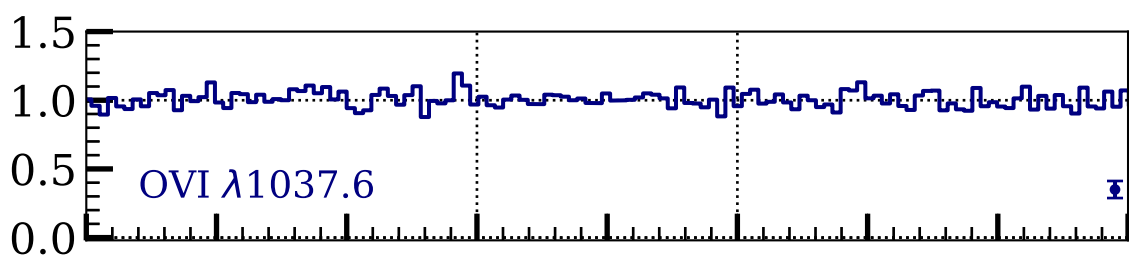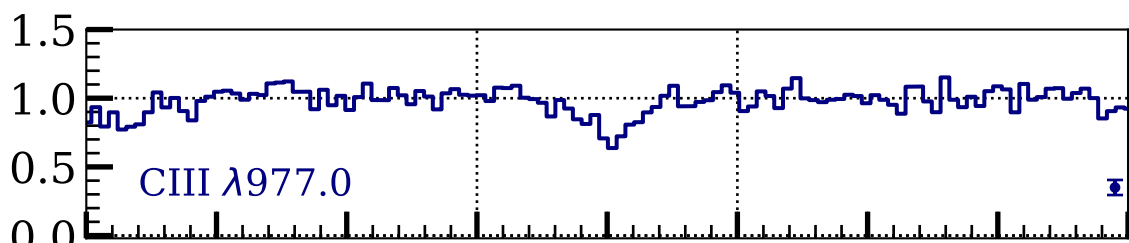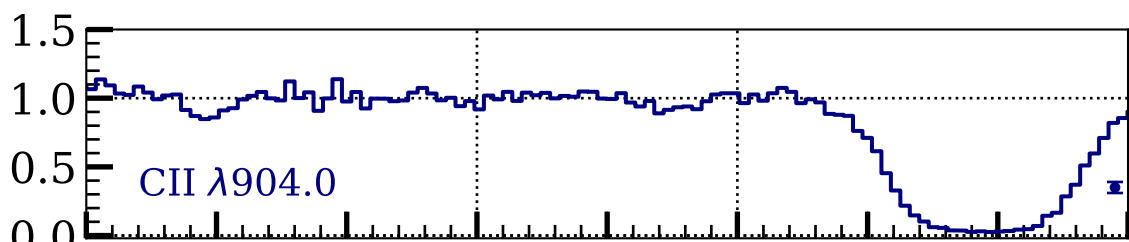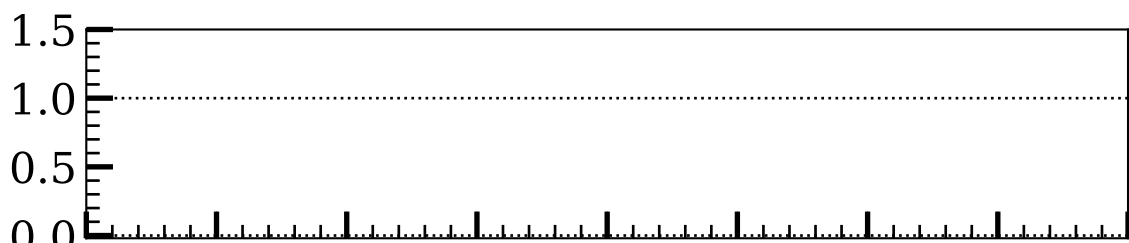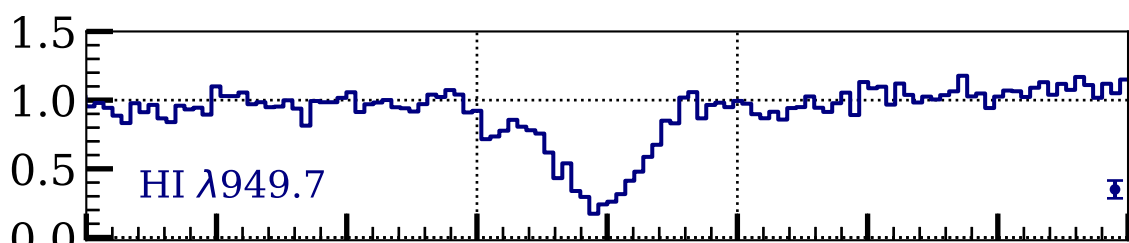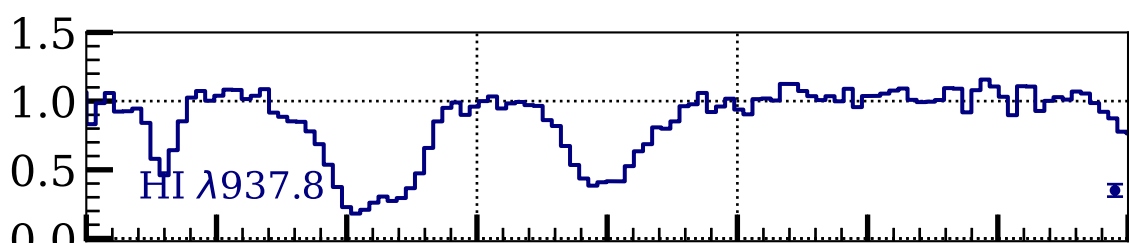

Rest-Frame Velocity (km s<sup>-1</sup>)

J150030.64+551708.8,  $z=0.347272$ , RF=1

Normalized Flux

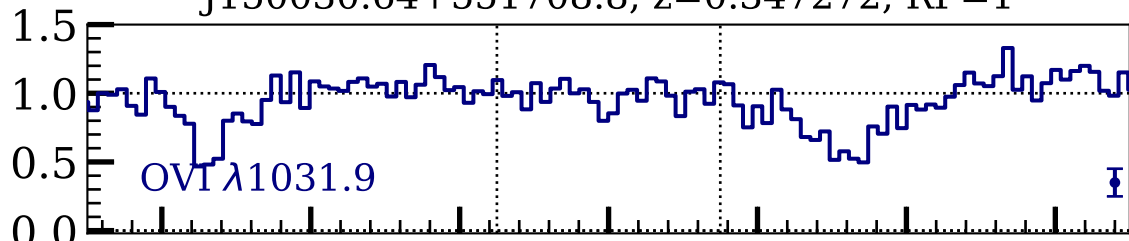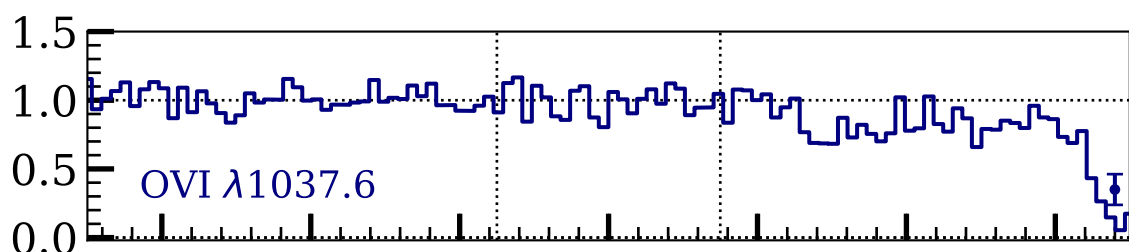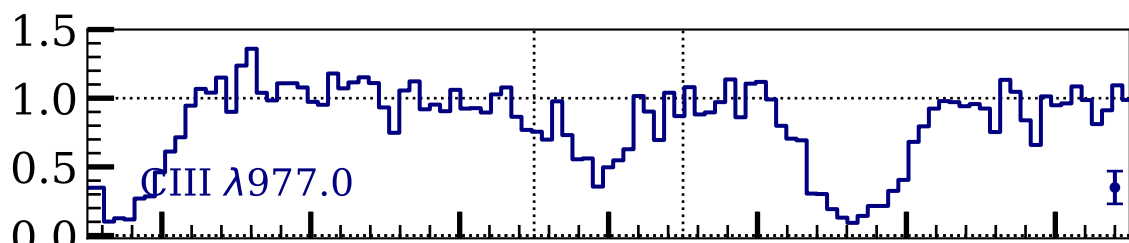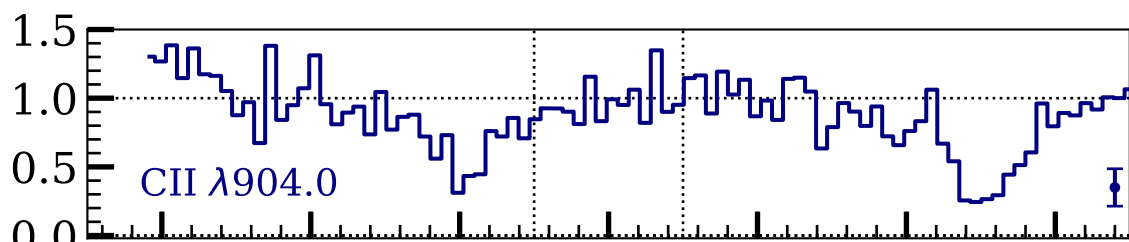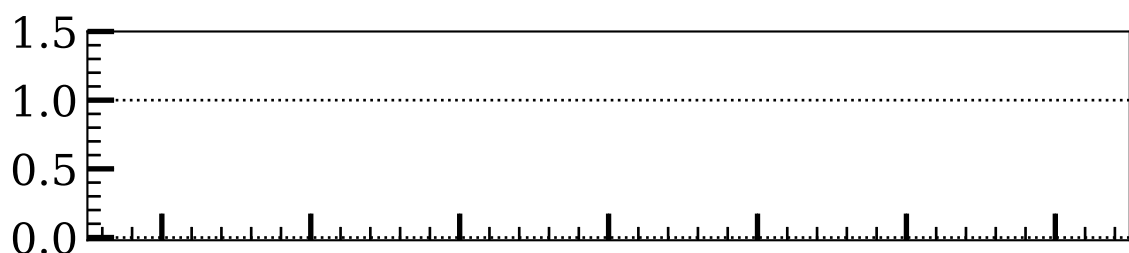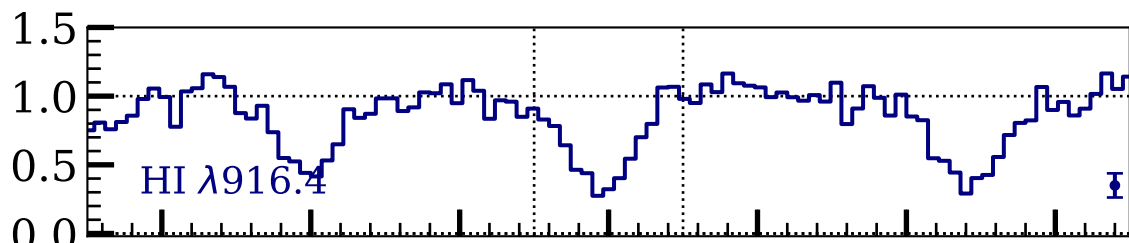

Rest-Frame Velocity ( $\text{km s}^{-1}$ )

J150030.64+551708.8,  $z=0.347999$ , RF=1

Normalized Flux

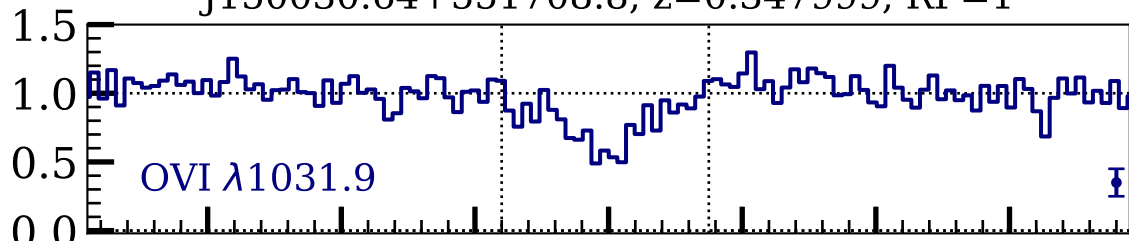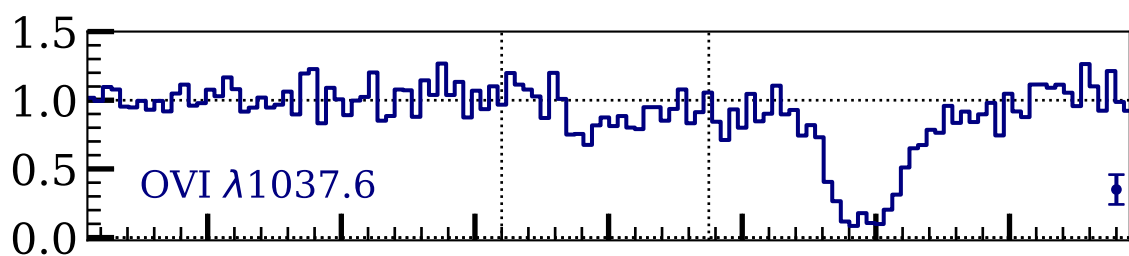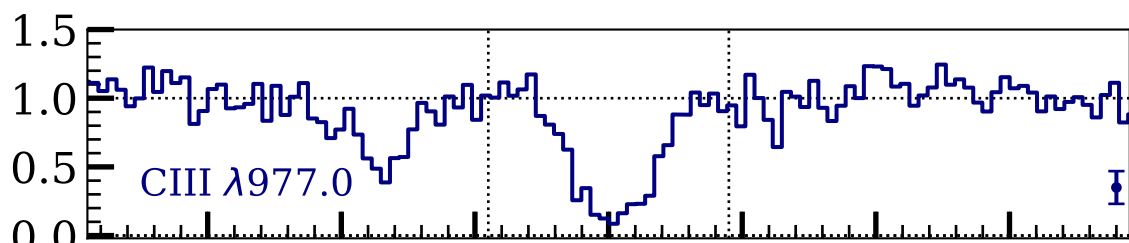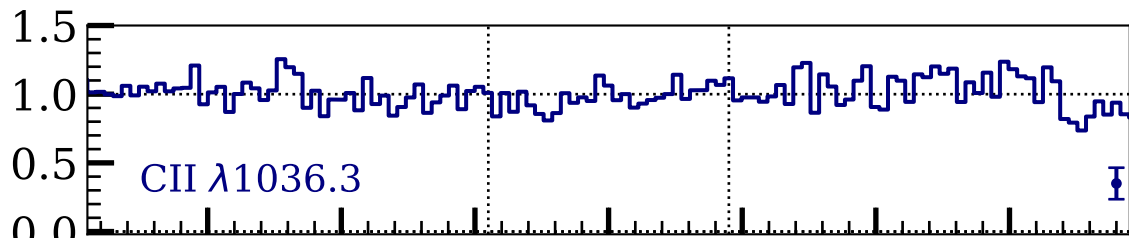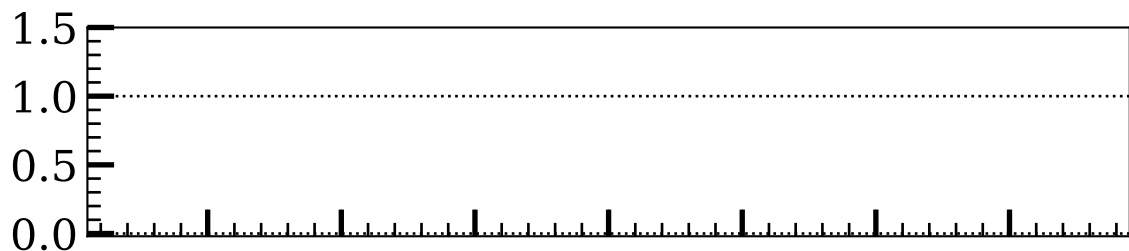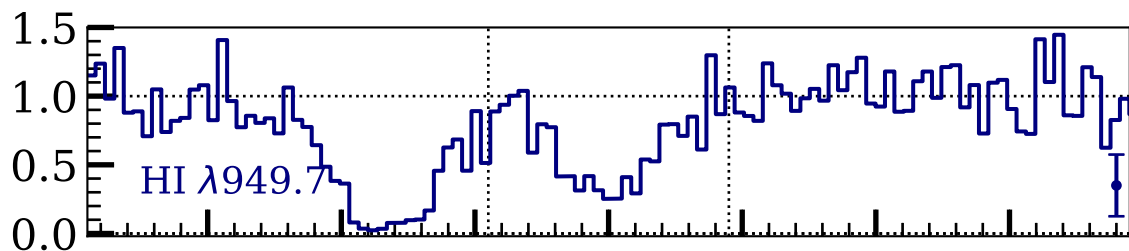

Rest-Frame Velocity ( $\text{km s}^{-1}$ )

J152424.58+095829.7,  $z=0.518500$ , RF=1

Normalized Flux

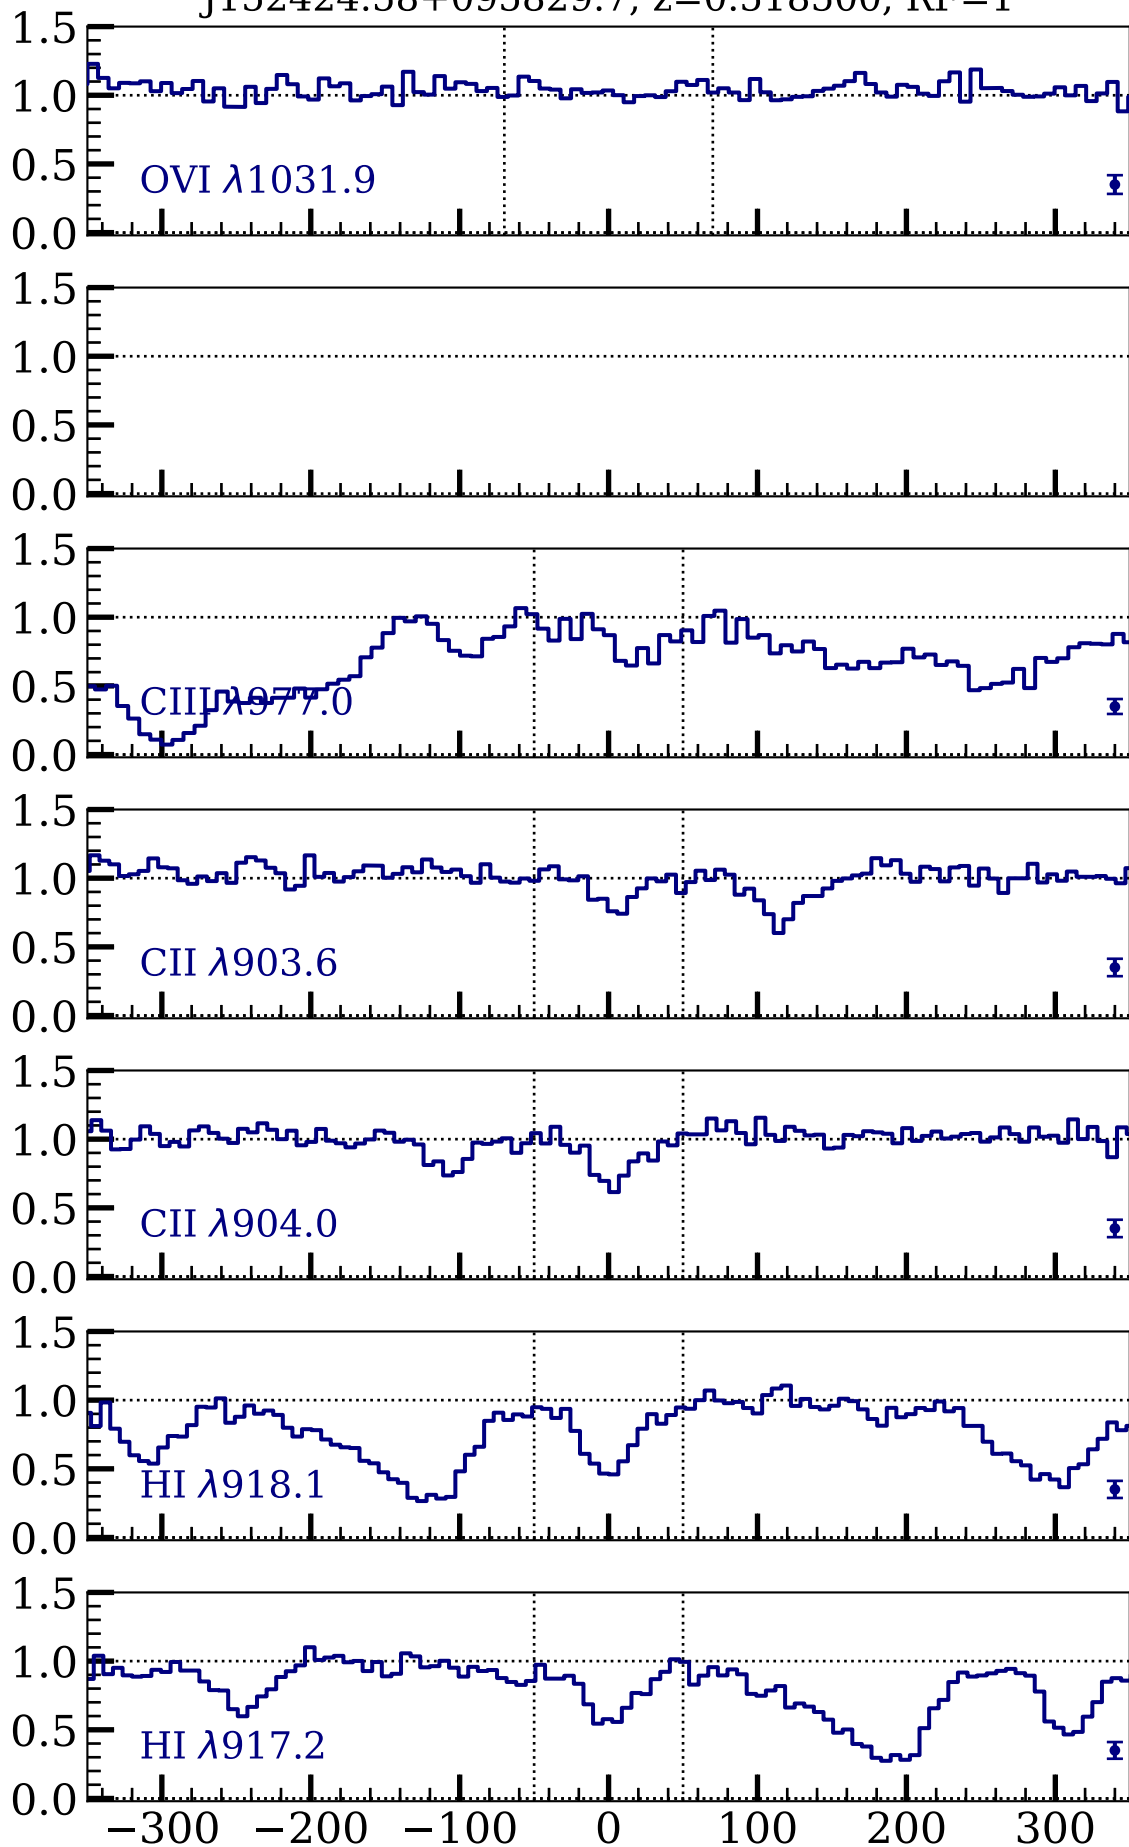

Rest-Frame Velocity (km s<sup>-1</sup>)

J152424.58+095829.7,  $z=0.571825$ , RF=1

Normalized Flux

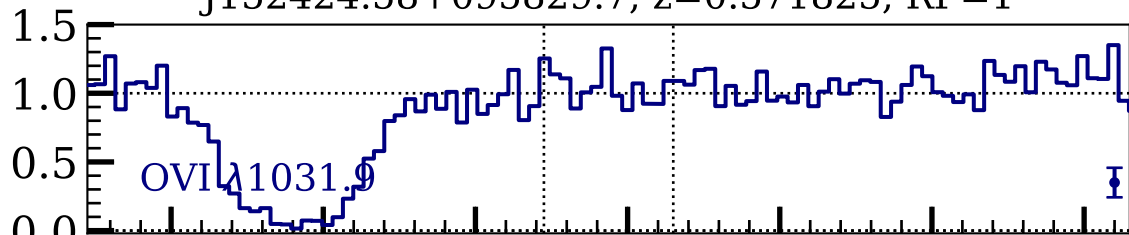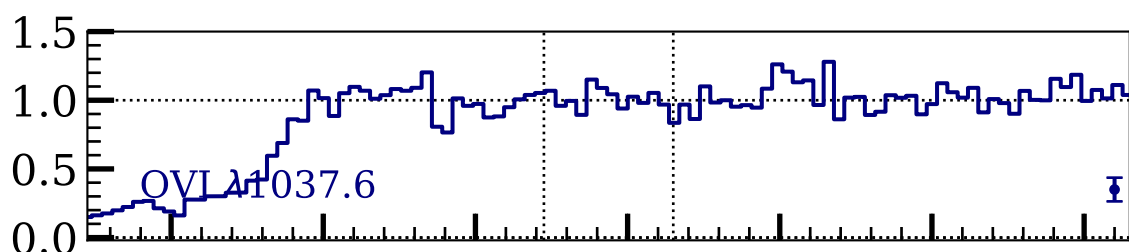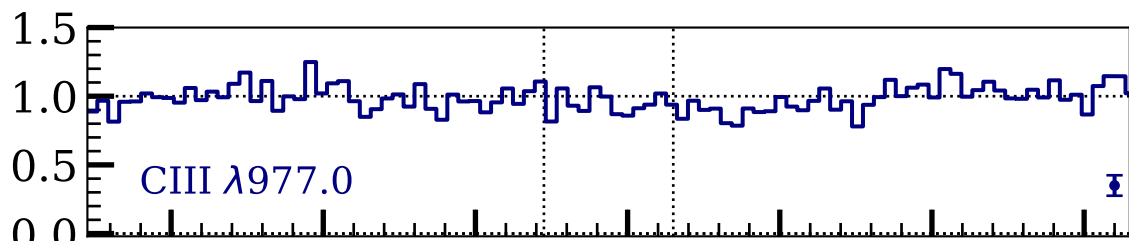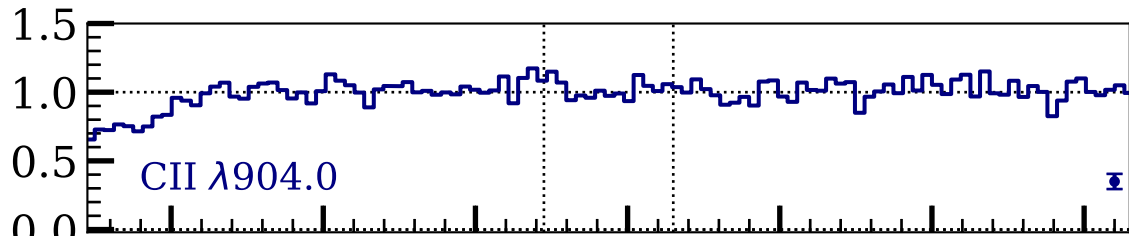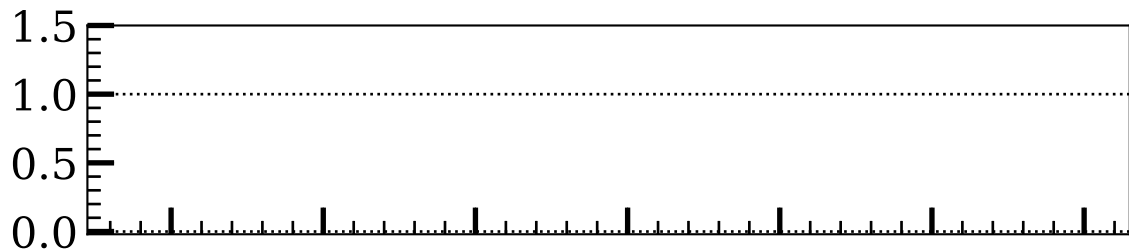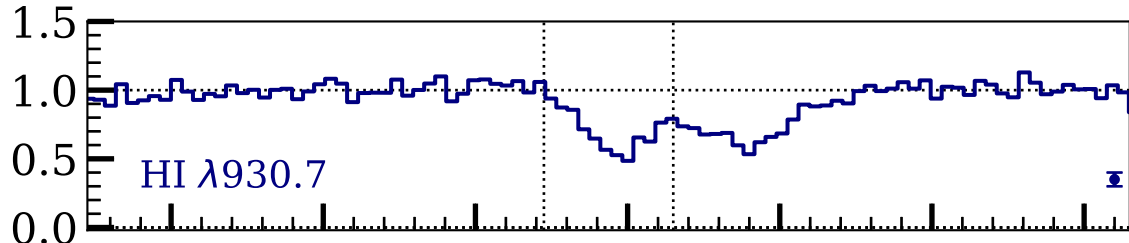

Rest-Frame Velocity ( $\text{km s}^{-1}$ )

J152424.58+095829.7,  $z=0.675378$ , RF=1

Normalized Flux

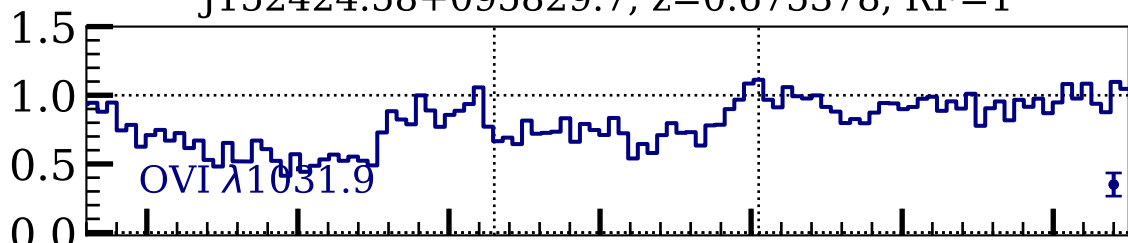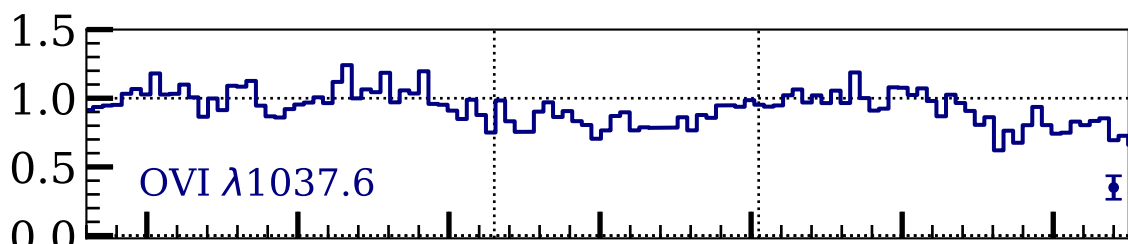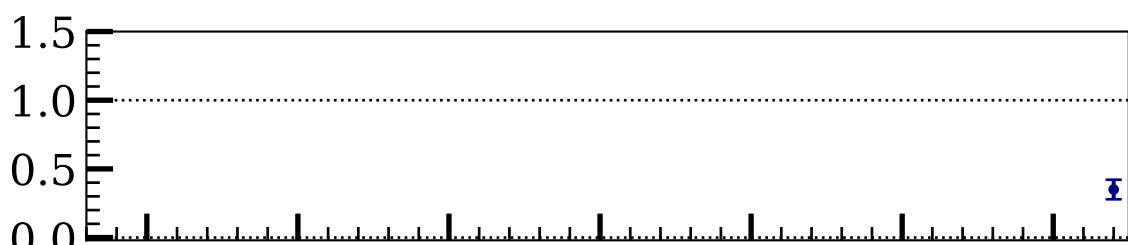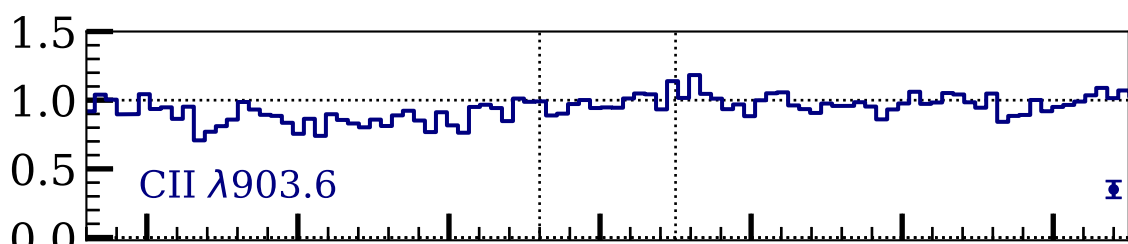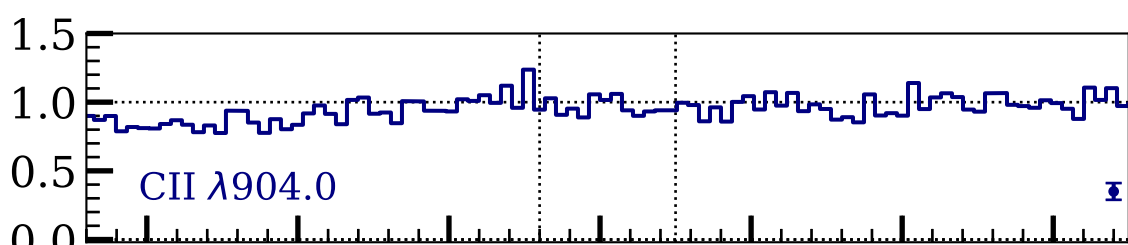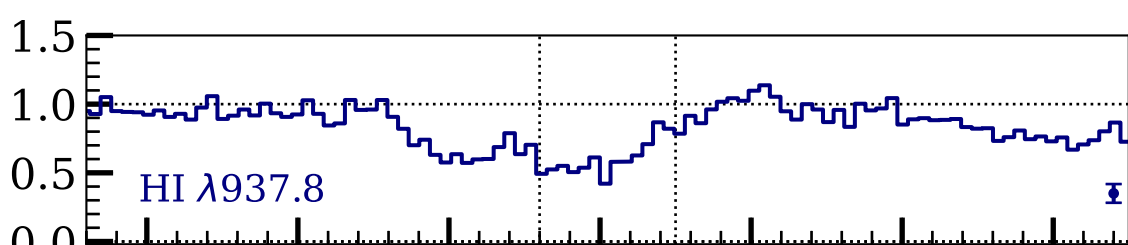

Rest-Frame Velocity (km s<sup>-1</sup>)



J152424.58+095829.7,  $z=0.728885$ , RF=1

Normalized Flux

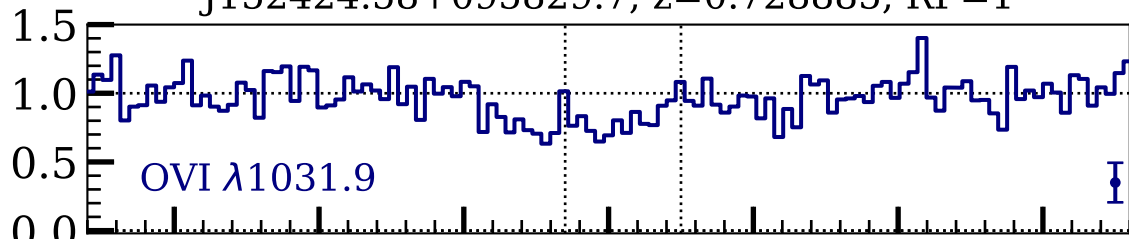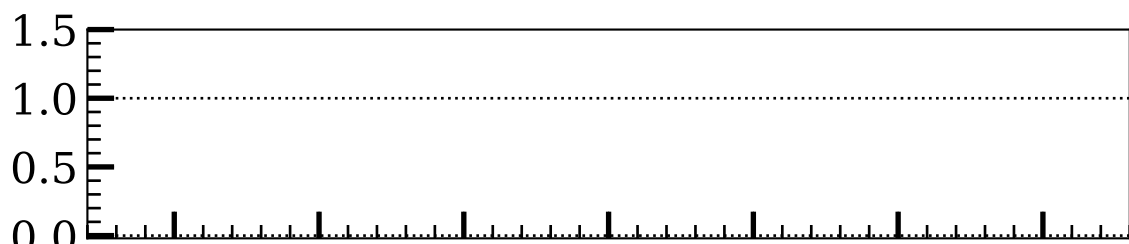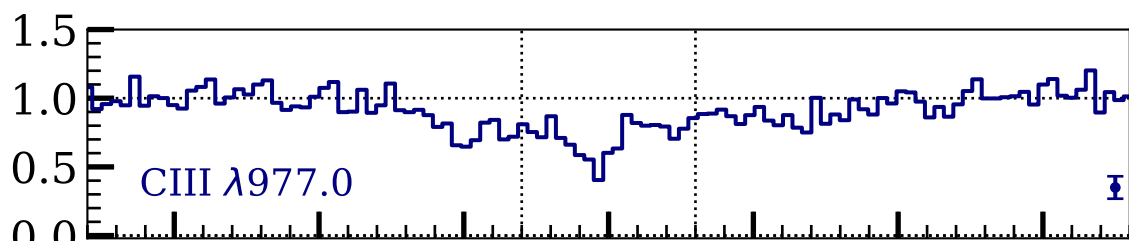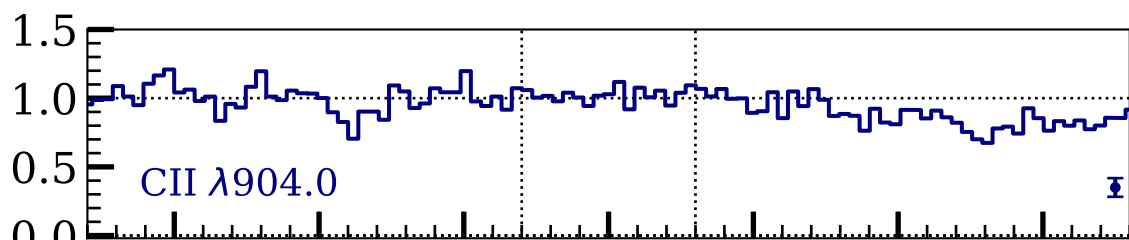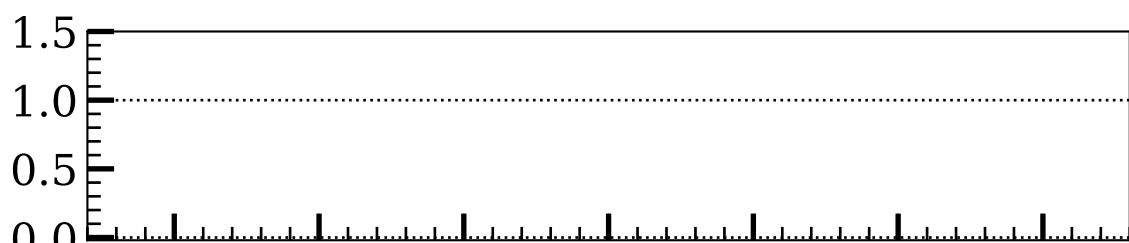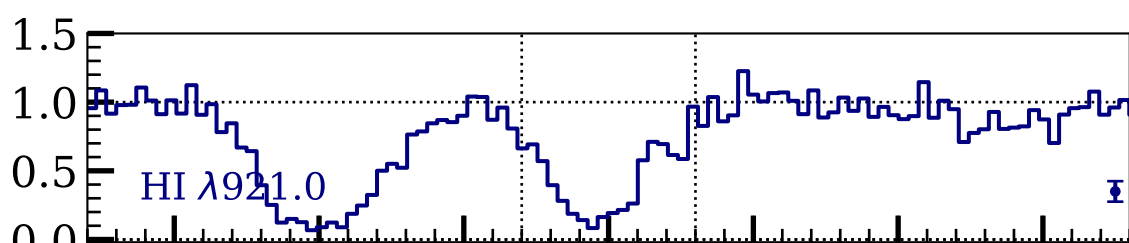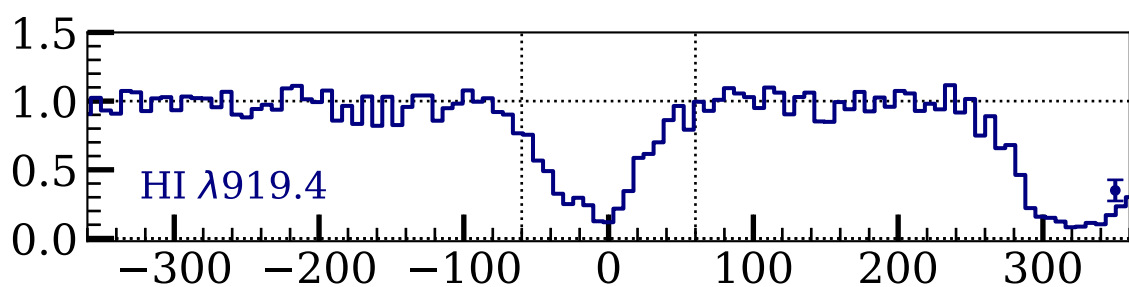

Rest-Frame Velocity (km s<sup>-1</sup>)

J154121.48+281706.2,  $z=0.282454$ , RF=0

Normalized Flux

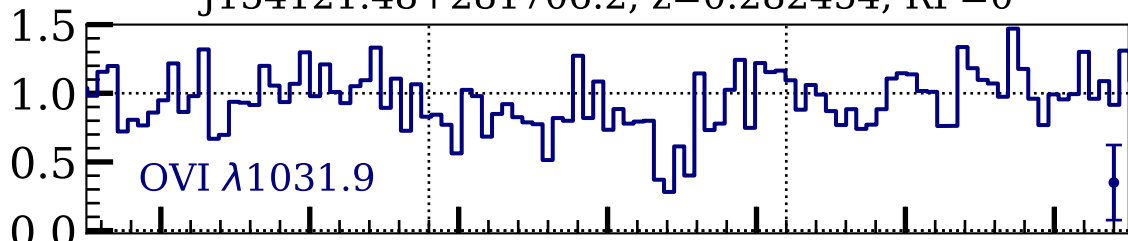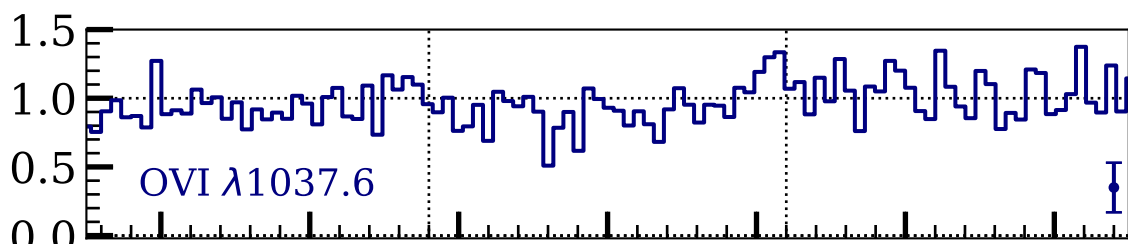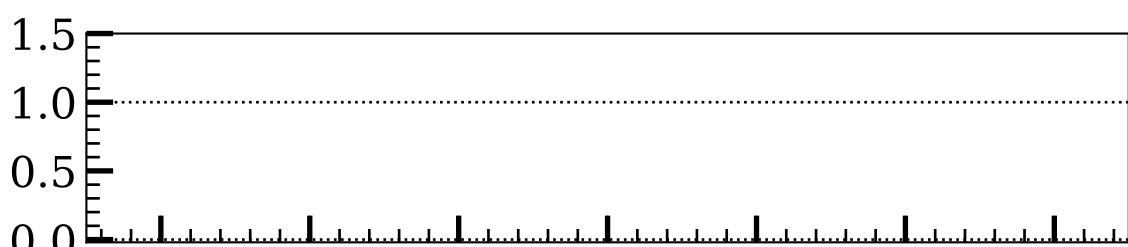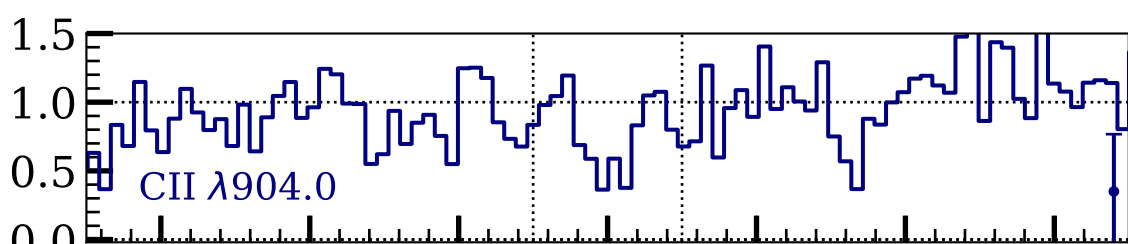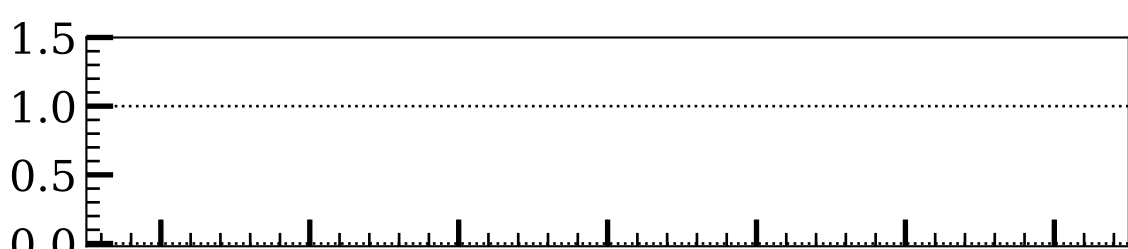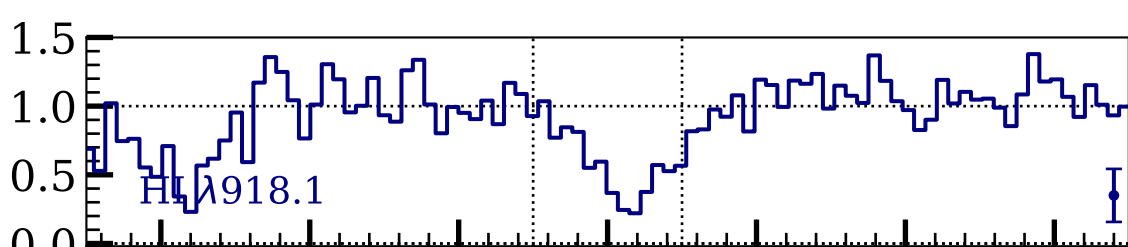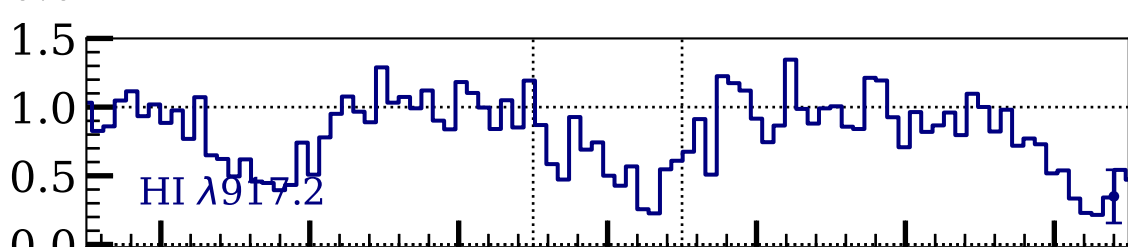

Rest-Frame Velocity ( $\text{km s}^{-1}$ )

J155048.29+400144.9,  $z=0.312618$ , RF=1

Normalized Flux

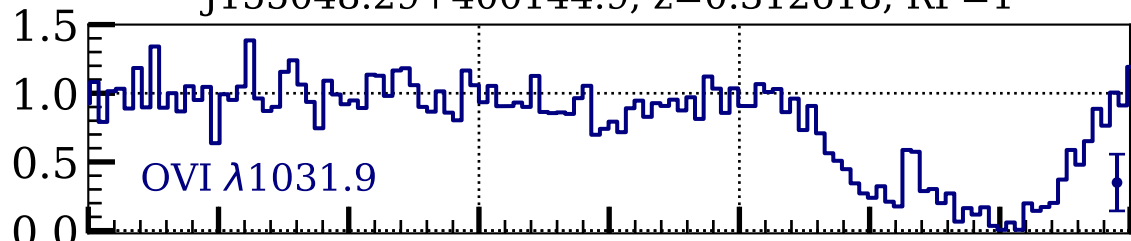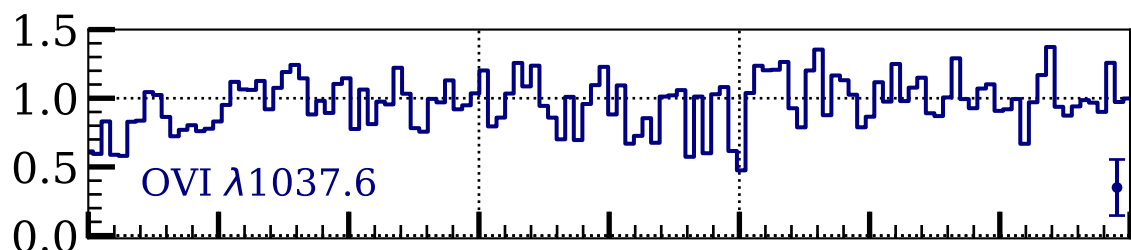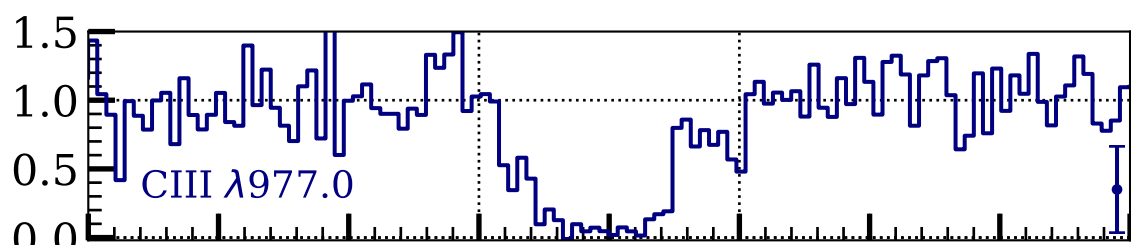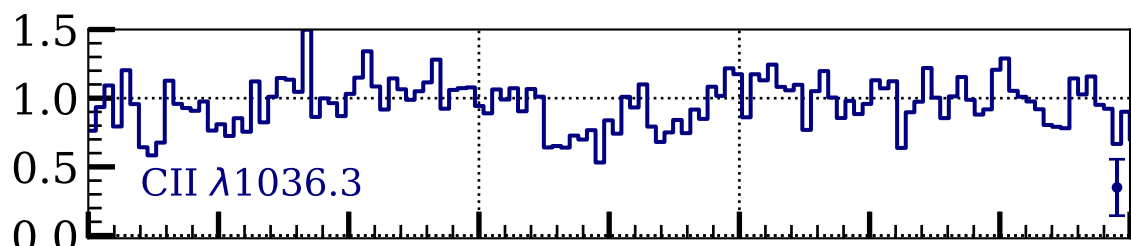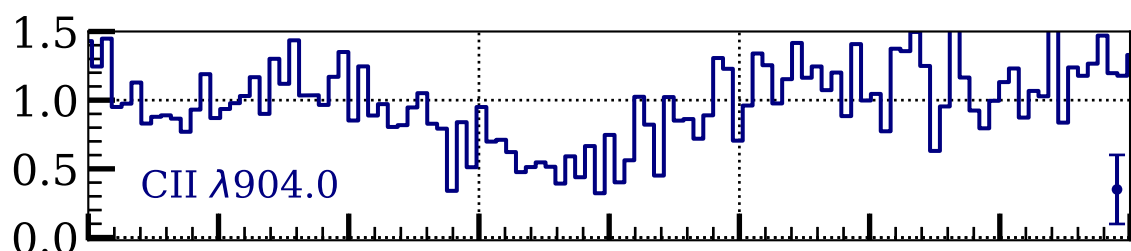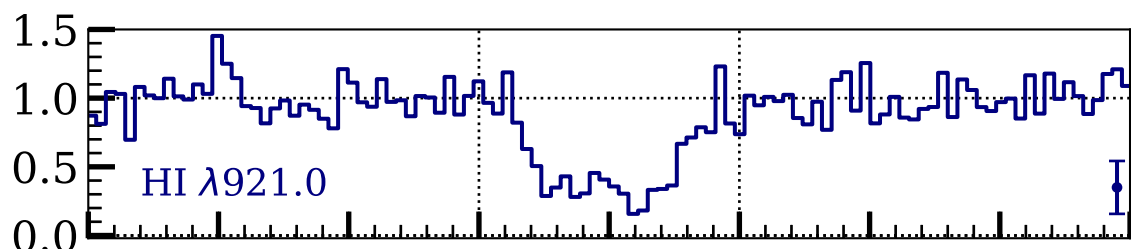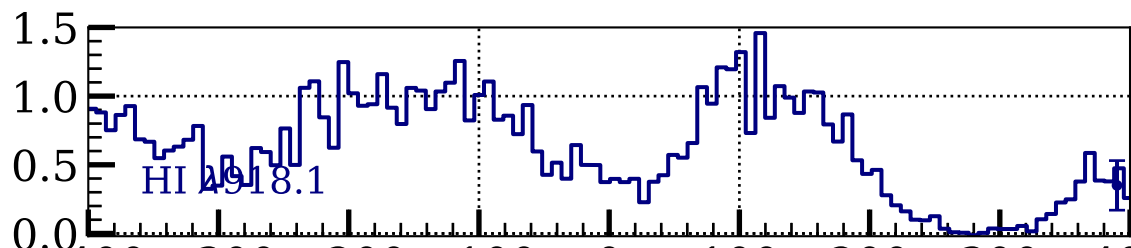

Rest-Frame Velocity ( $\text{km s}^{-1}$ )

J155048.29+400144.9,  $z=0.427306$ , RF=1

Normalized Flux

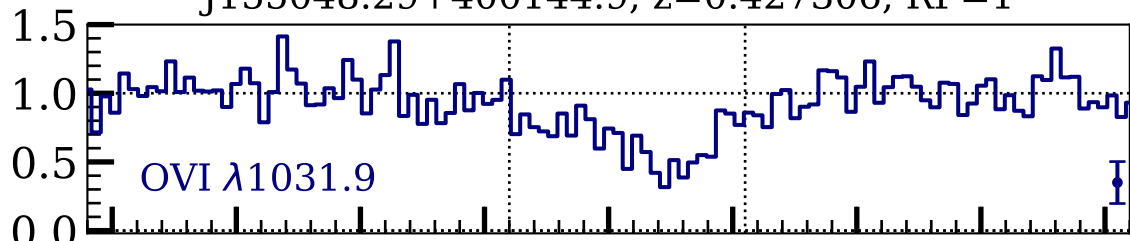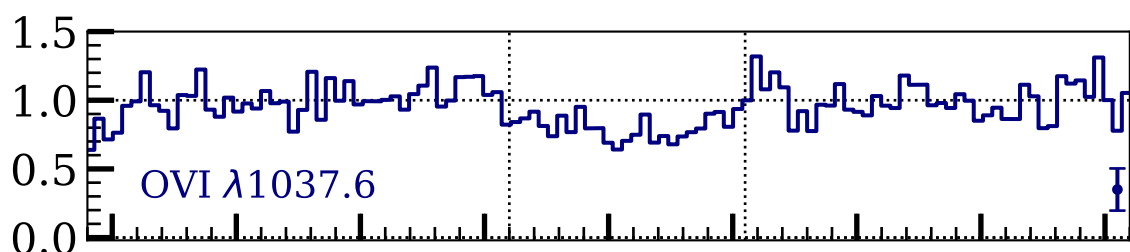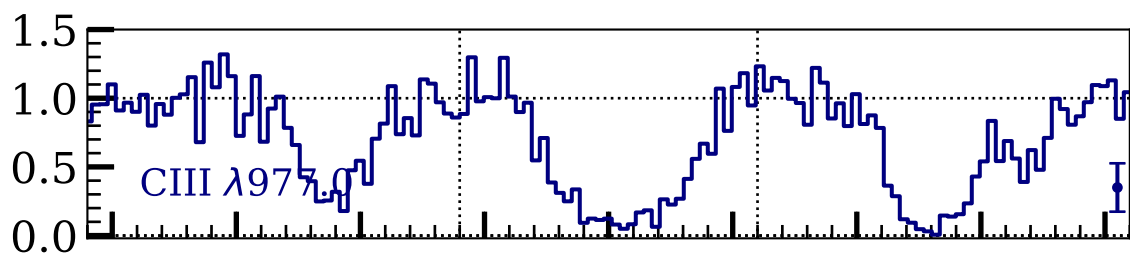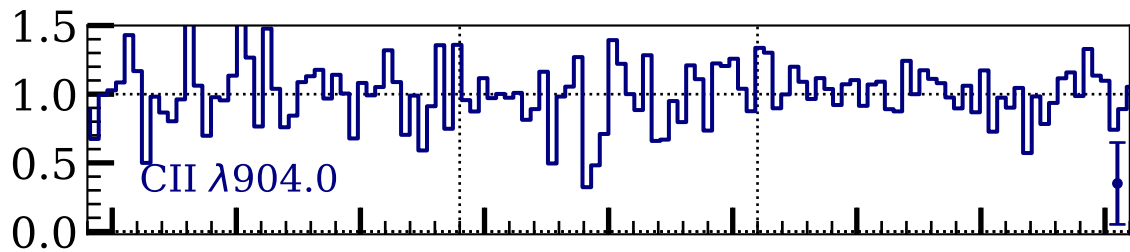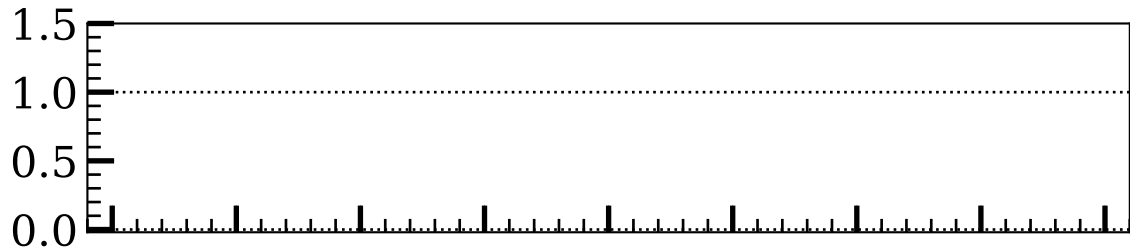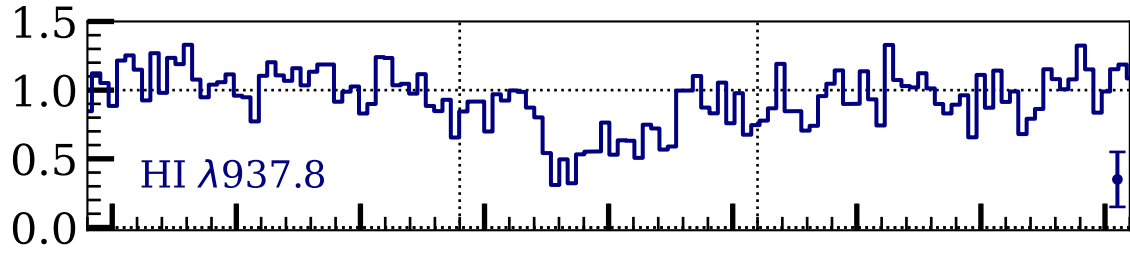

Rest-Frame Velocity ( $\text{km s}^{-1}$ )

J155048.29+400144.9,  $z=0.491977$ , RF=1

Normalized Flux

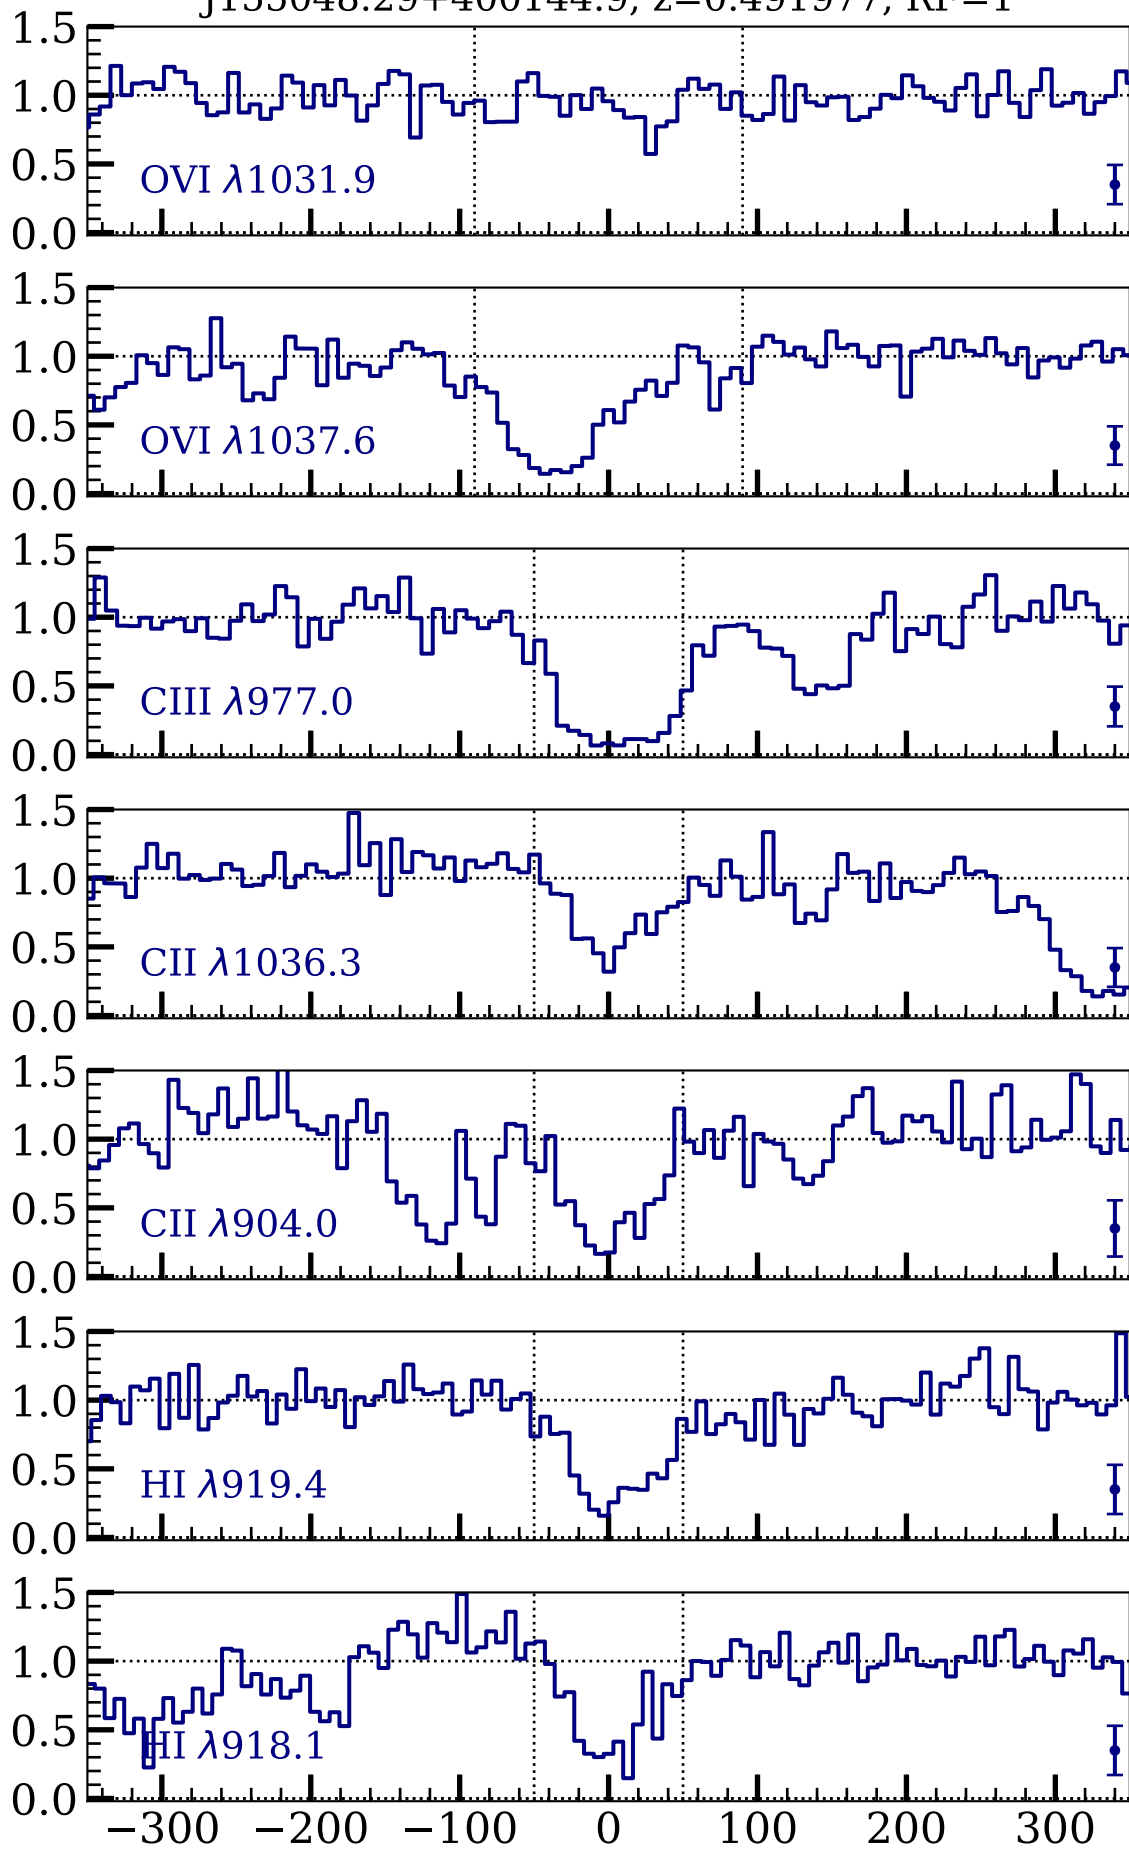

Rest-Frame Velocity (km s<sup>-1</sup>)

J155048.29+400144.9,  $z=0.492632$ , RF=1

Normalized Flux

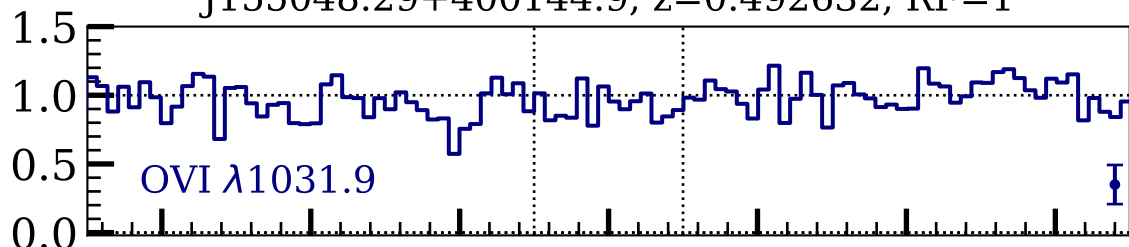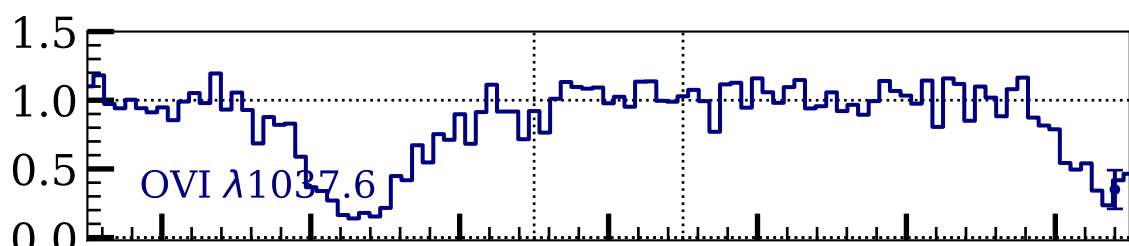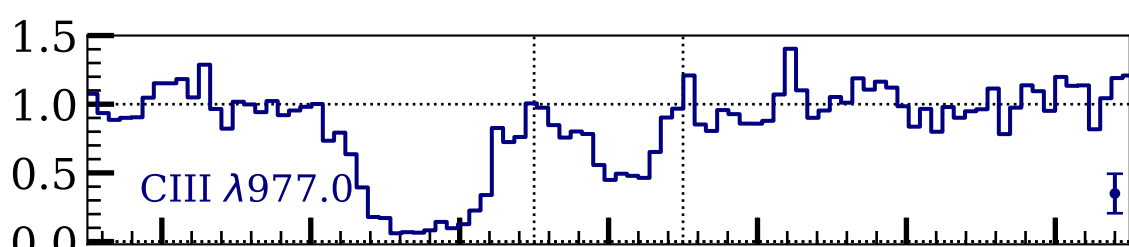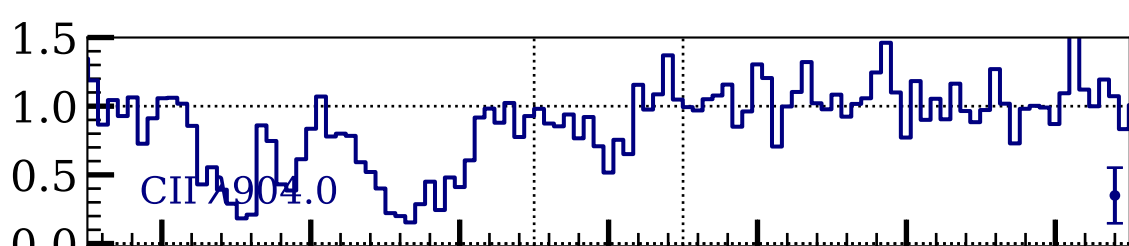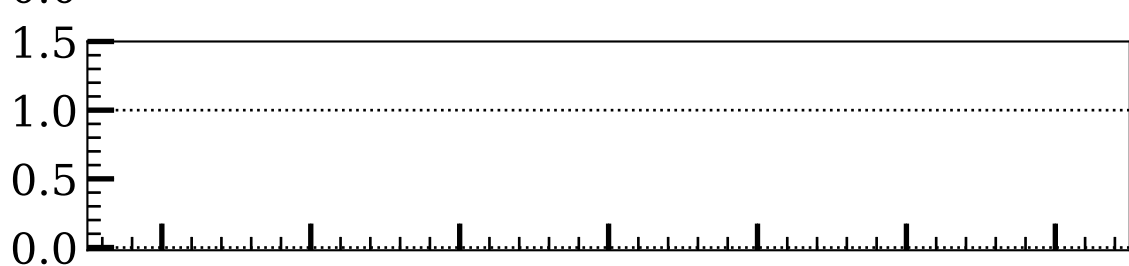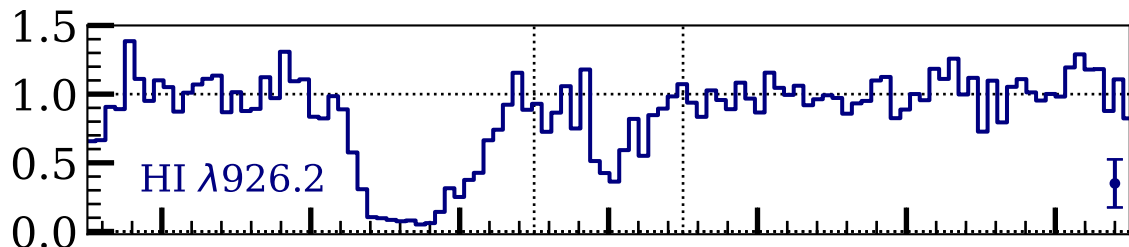

Rest-Frame Velocity ( $\text{km s}^{-1}$ )

J155232.54+570516.5,  $z=0.366020$ , RF=1

Normalized Flux

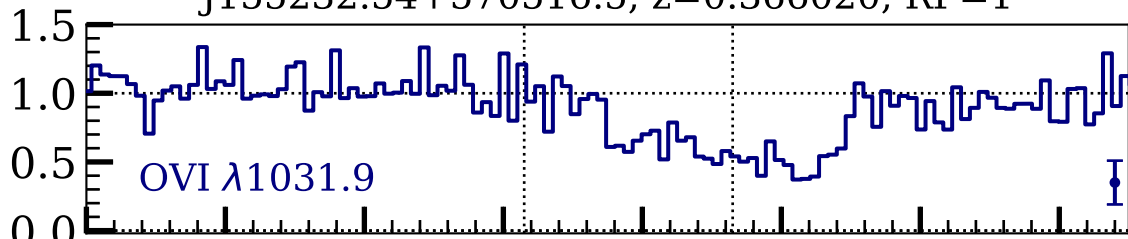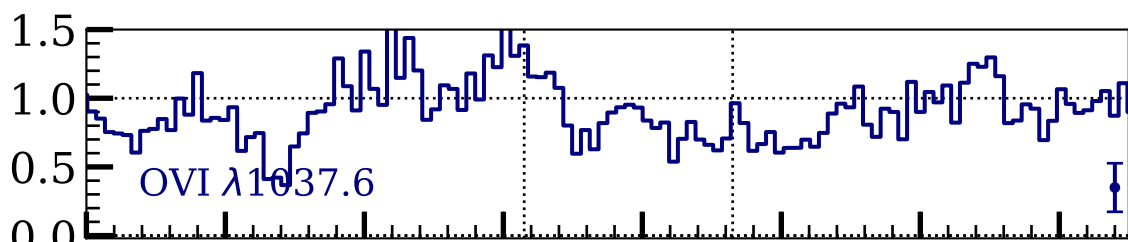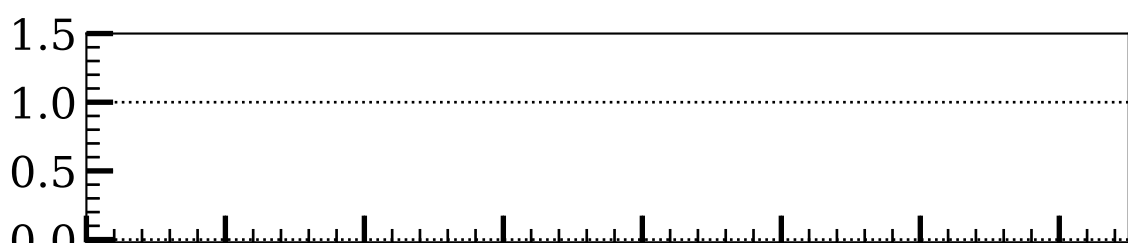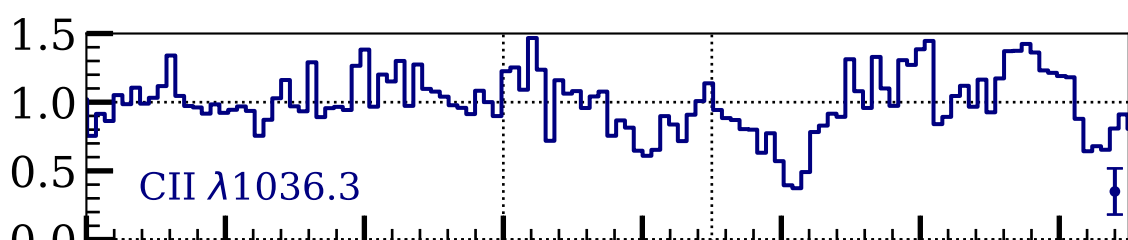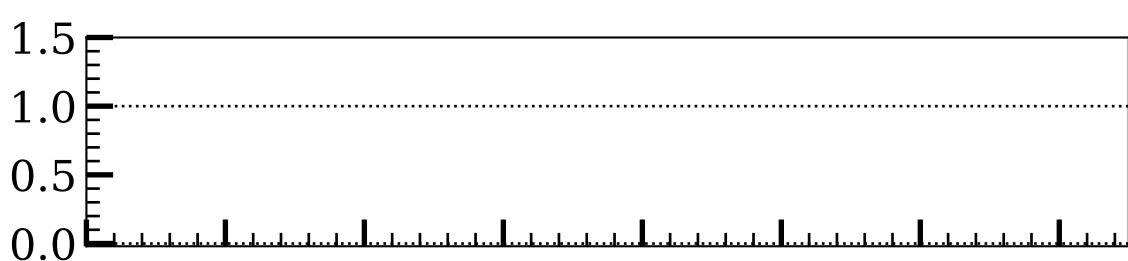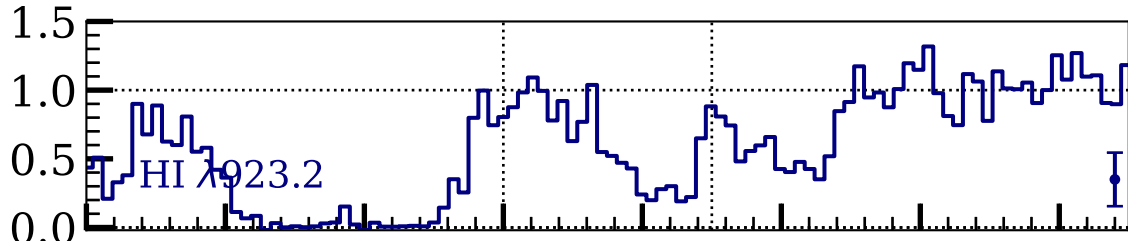

Rest-Frame Velocity ( $\text{km s}^{-1}$ )

J155232.54+570516.5,  $z=0.366521$ , RF=1

Normalized Flux

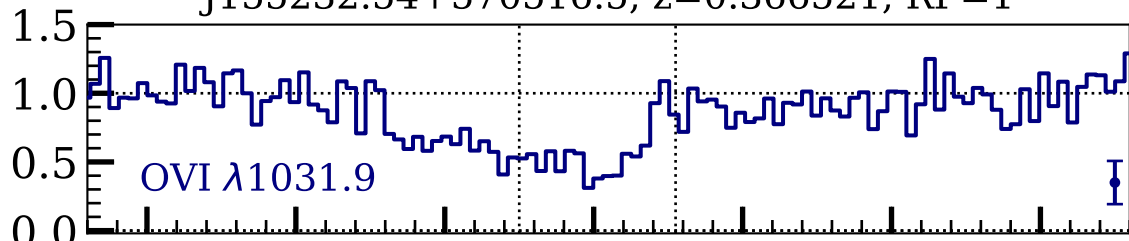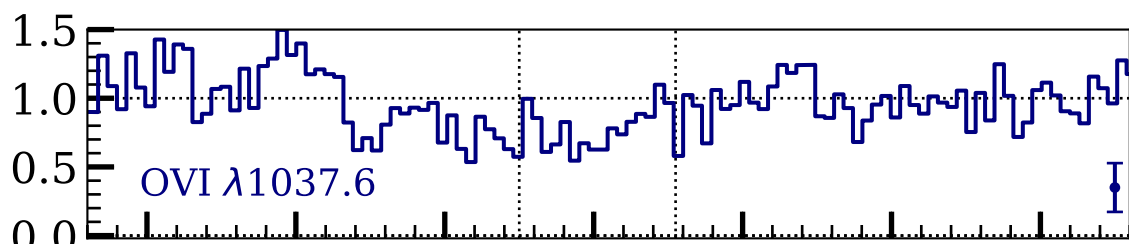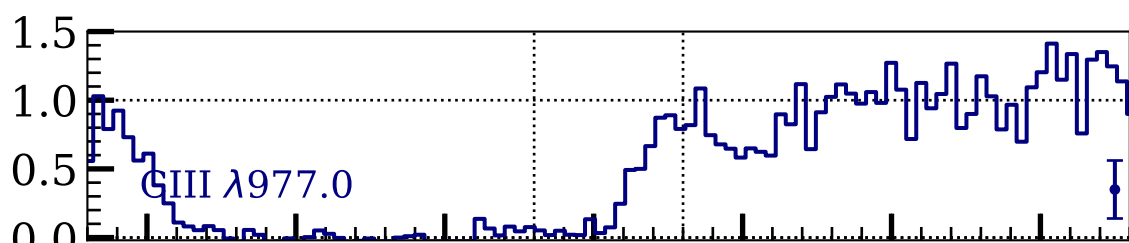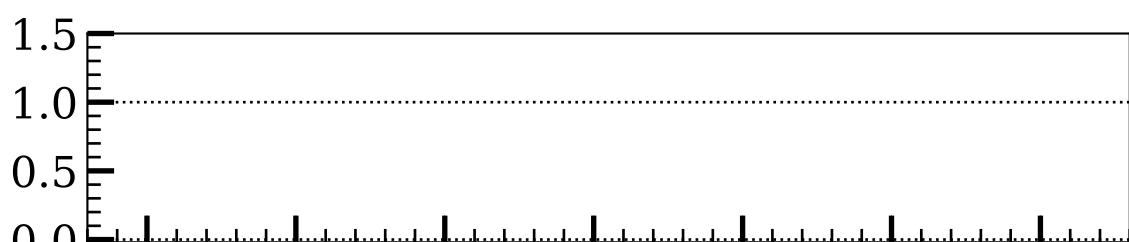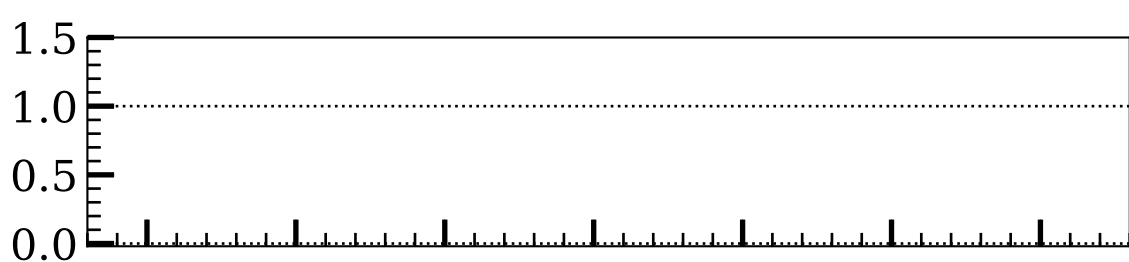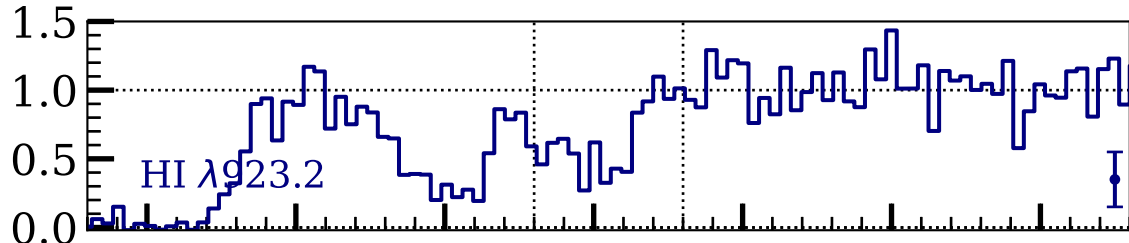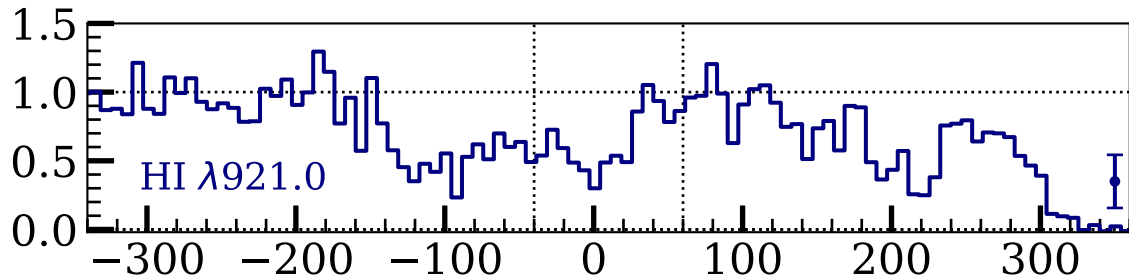

Rest-Frame Velocity ( $\text{km s}^{-1}$ )



J155304.92+354828.6,  $z=0.217943$ , RF=1

Normalized Flux

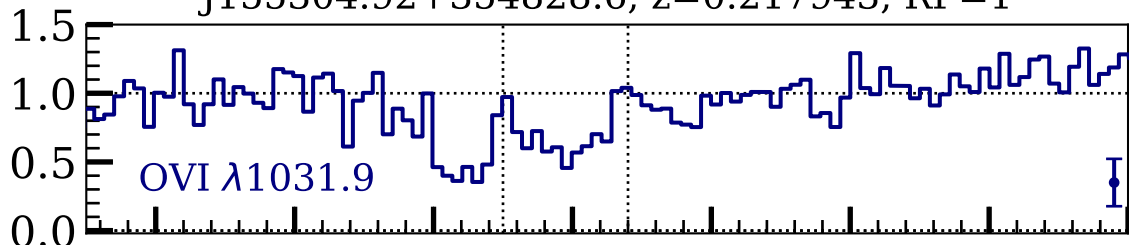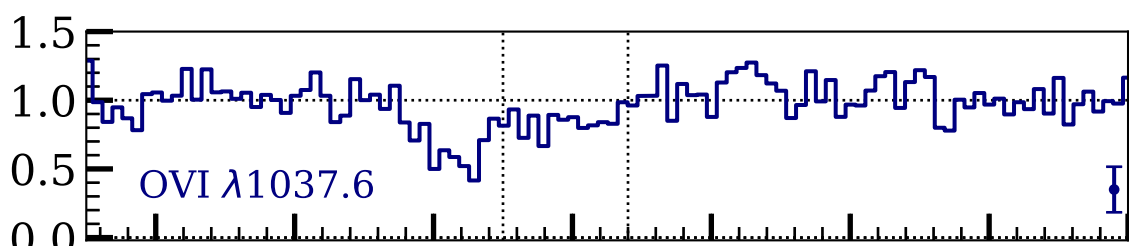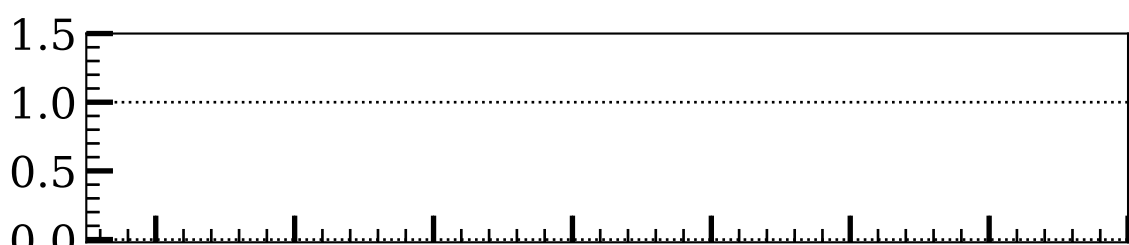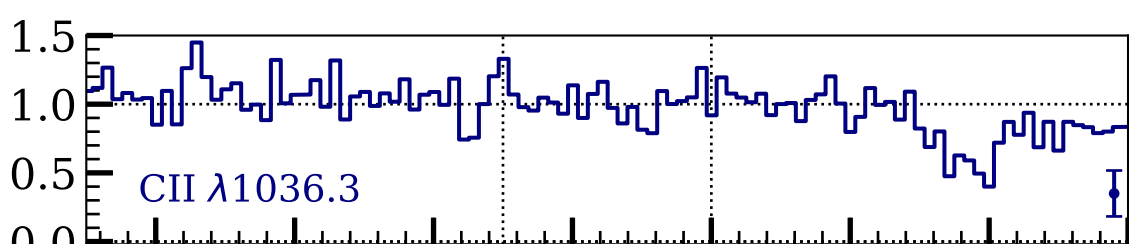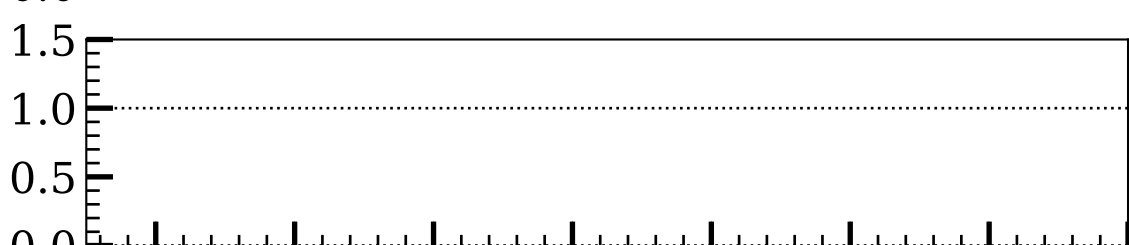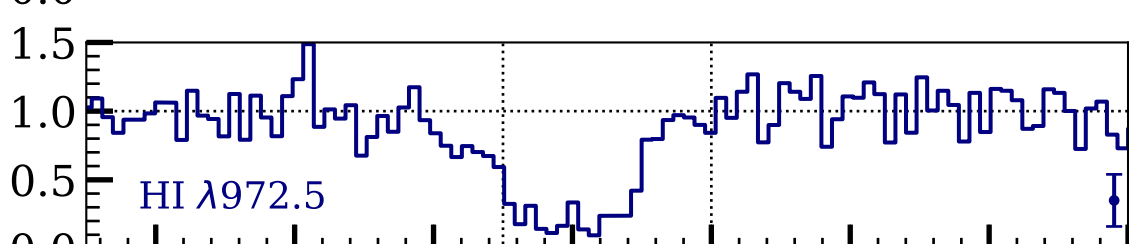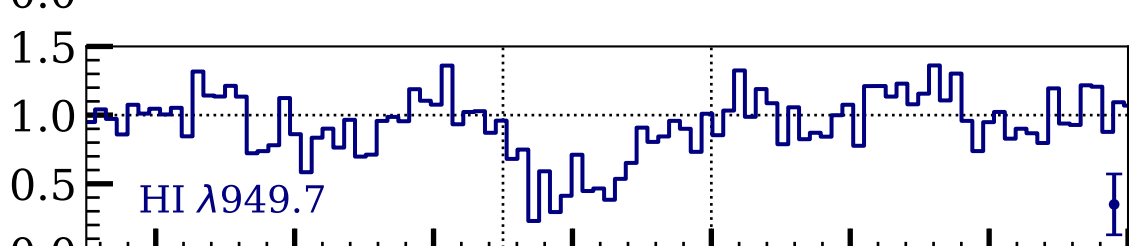

Rest-Frame Velocity (km s<sup>-1</sup>)

J155304.92+354828.6,  $z=0.475466$ , RF=1

Normalized Flux

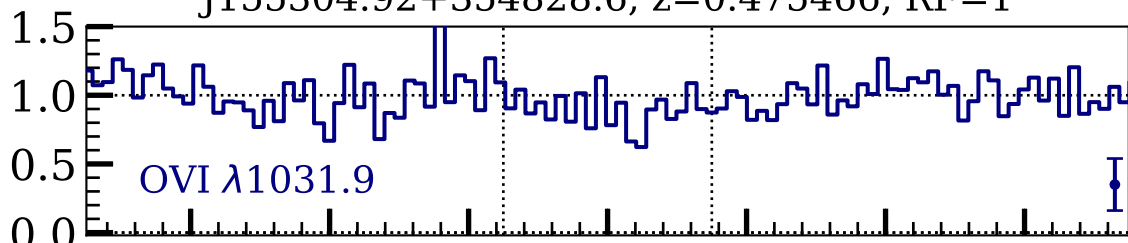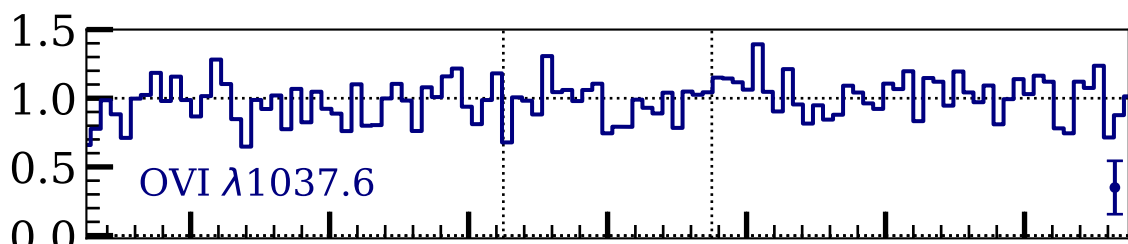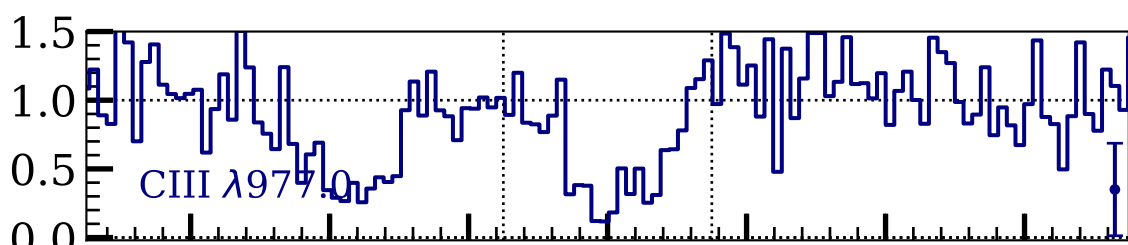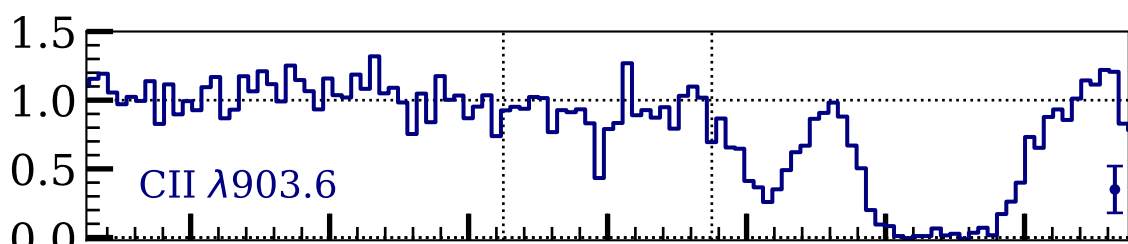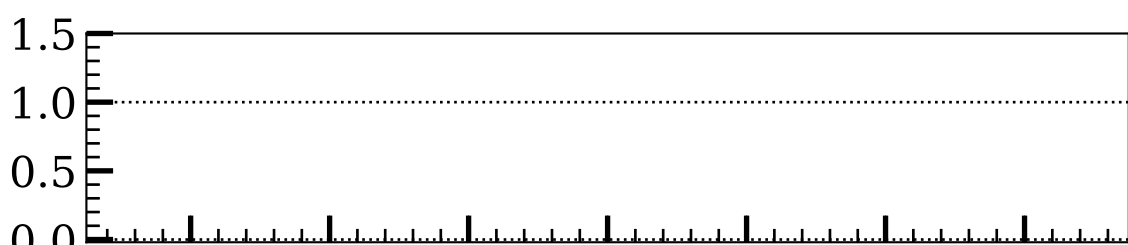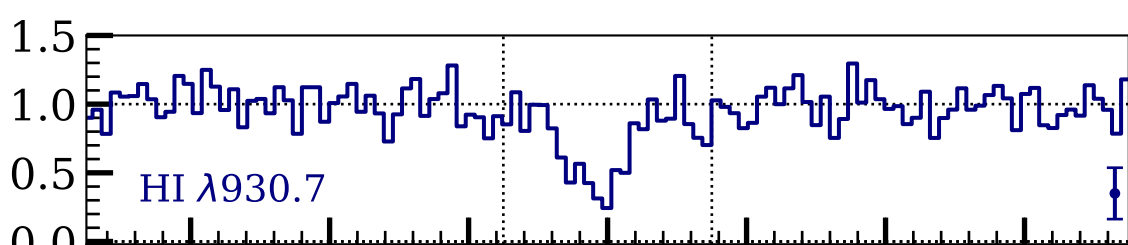

Rest-Frame Velocity ( $\text{km s}^{-1}$ )

J155504.39+362848.0,  $z=0.576033$ , RF=0

Normalized Flux

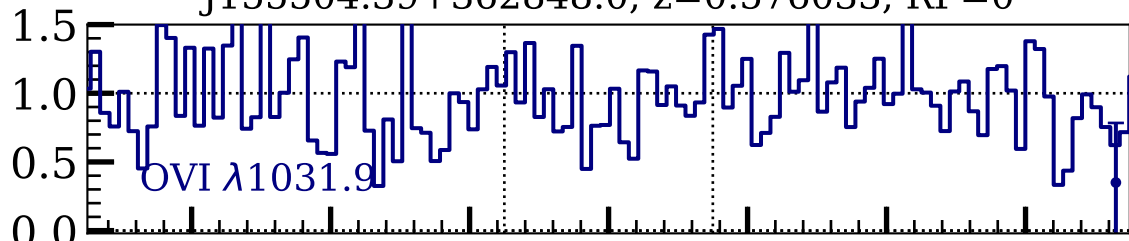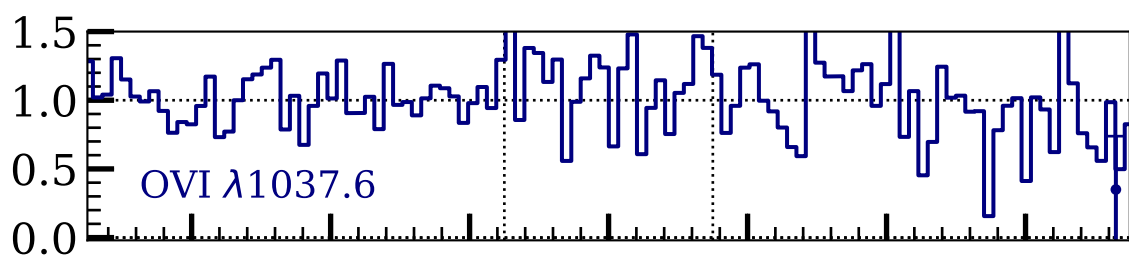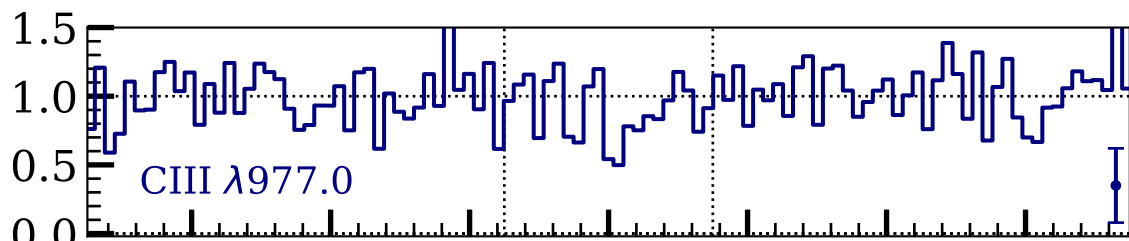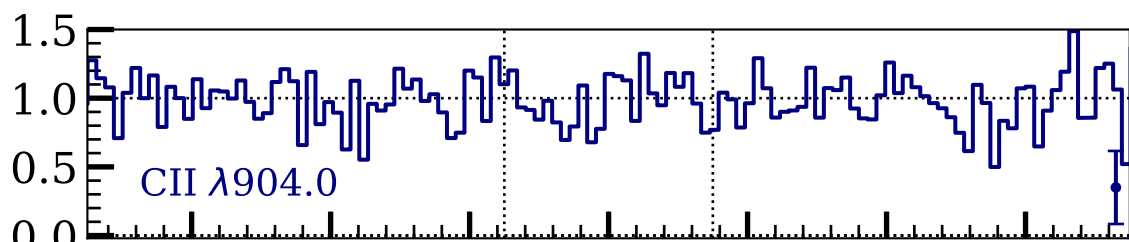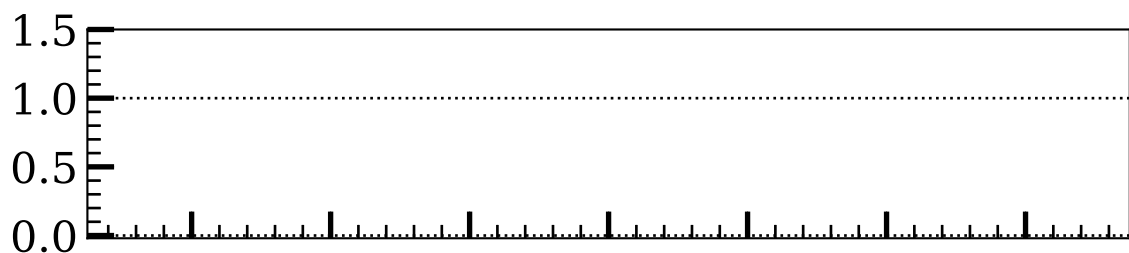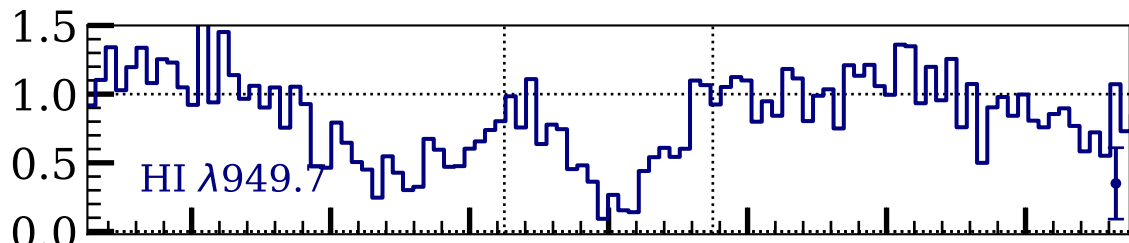

Rest-Frame Velocity ( $\text{km s}^{-1}$ )

J161916.54+334238.4,  $z=0.269400$ , RF=1

Normalized Flux

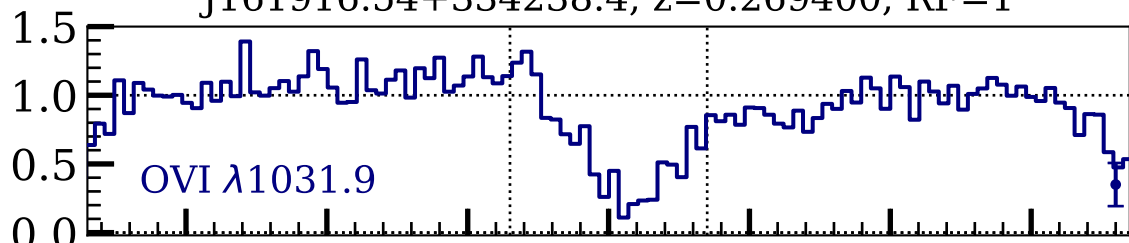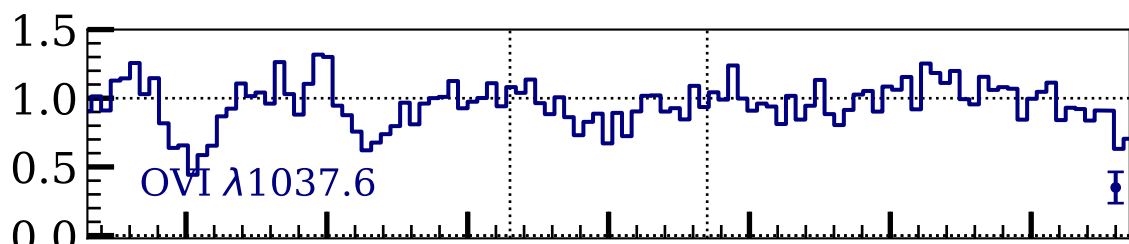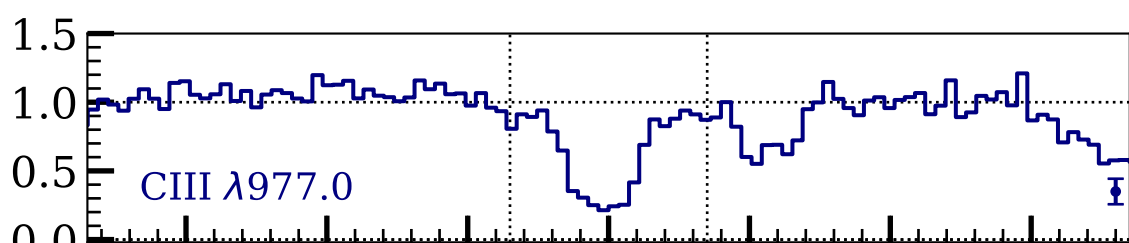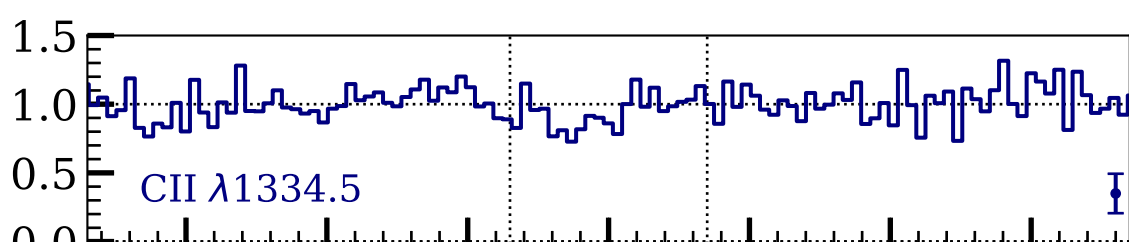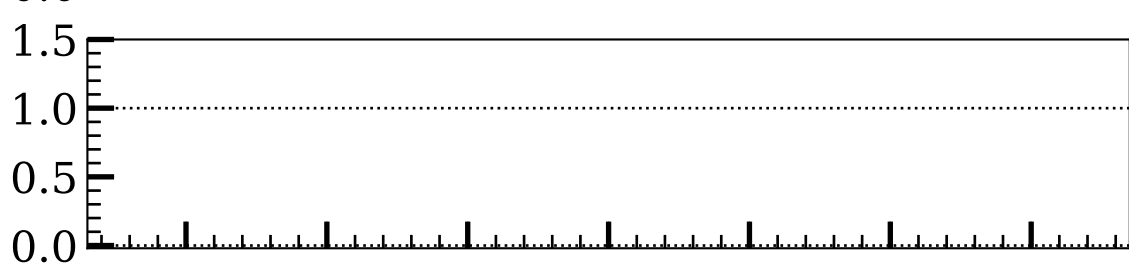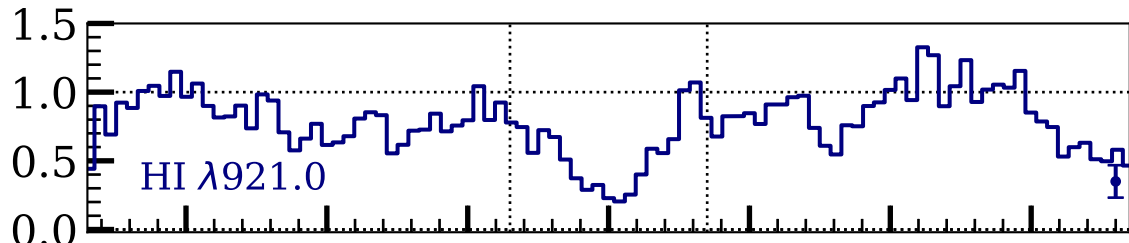

Rest-Frame Velocity ( $\text{km s}^{-1}$ )

J161916.54+334238.4,  $z=0.442306$ , RF=1

Normalized Flux

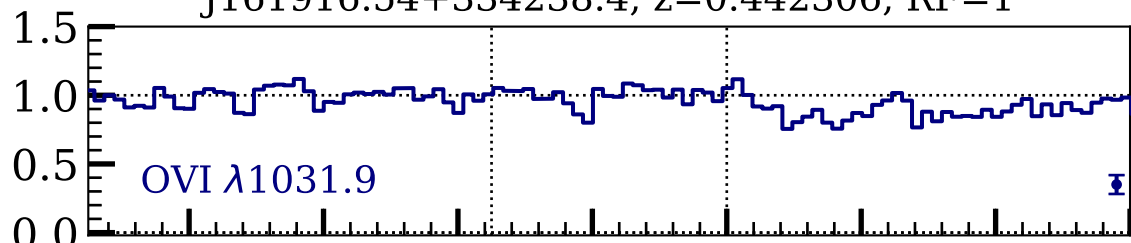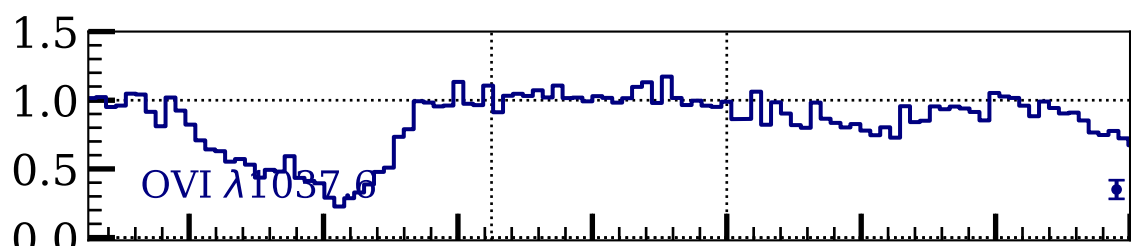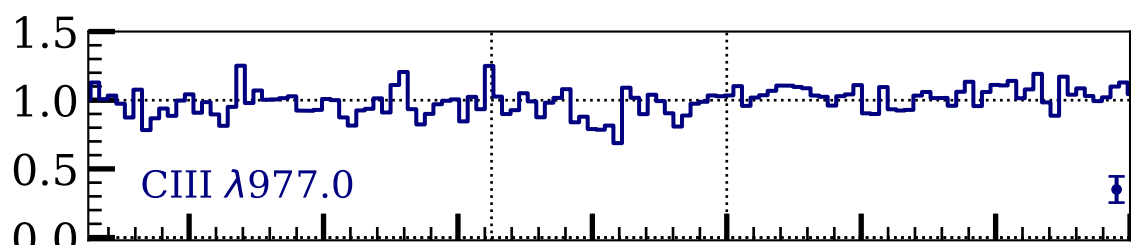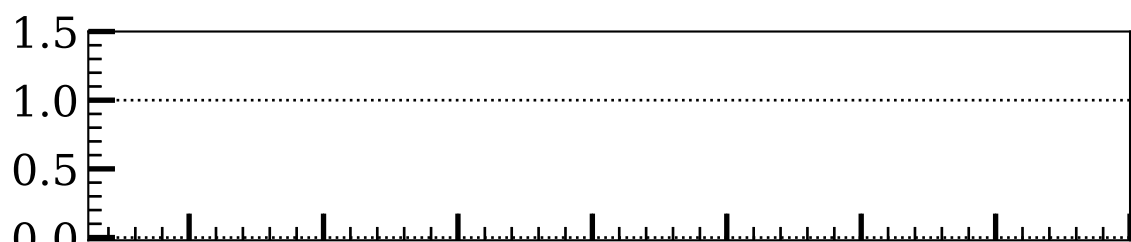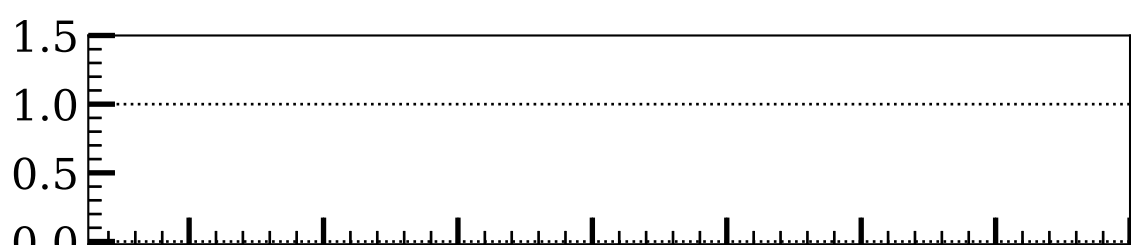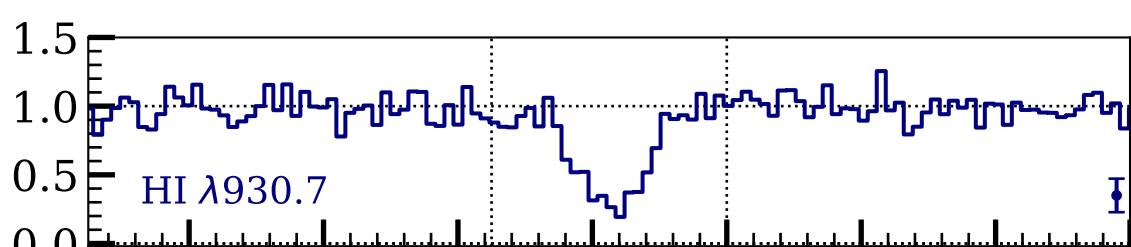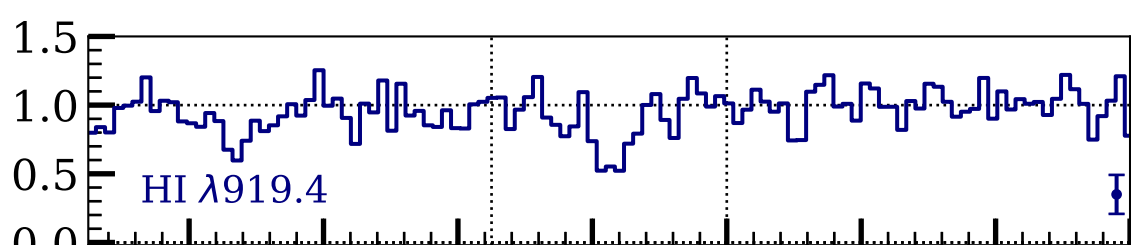

Rest-Frame Velocity ( $\text{km s}^{-1}$ )

J163201.12+373749.9,  $z=0.273950$ , RF=1

Normalized Flux

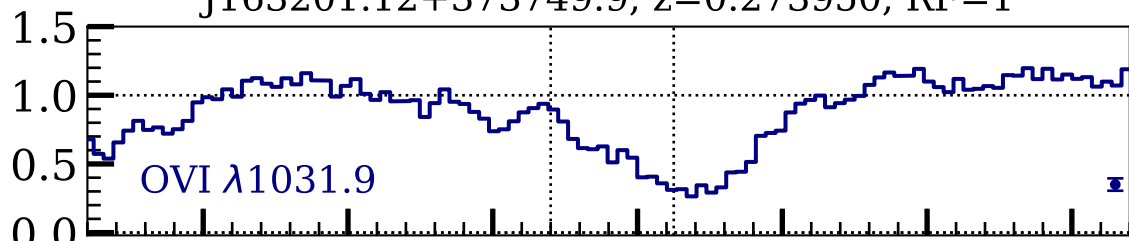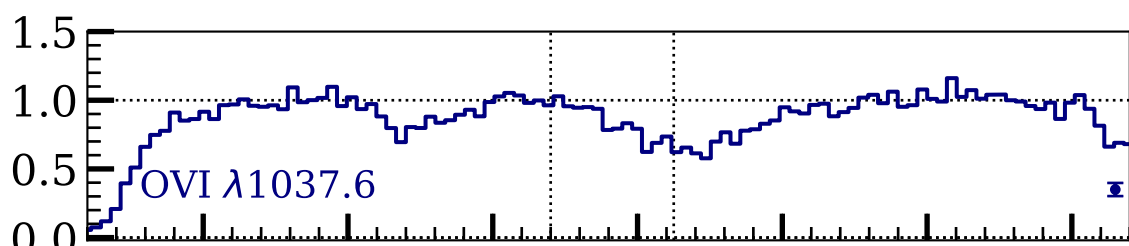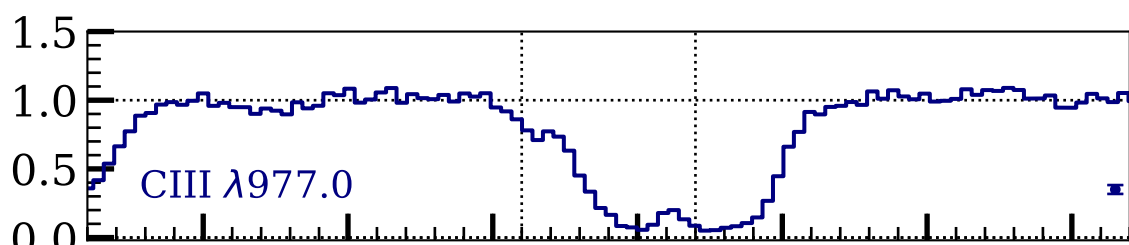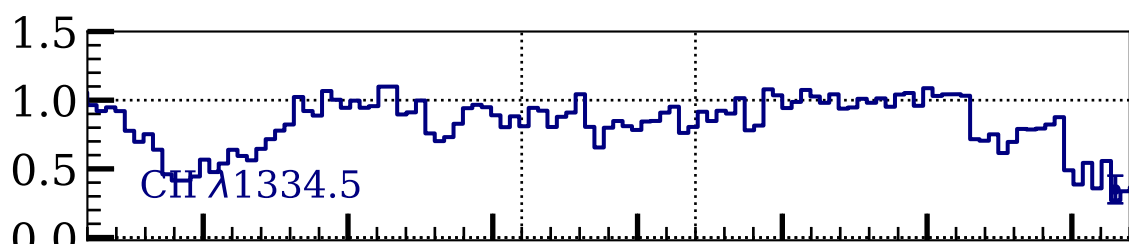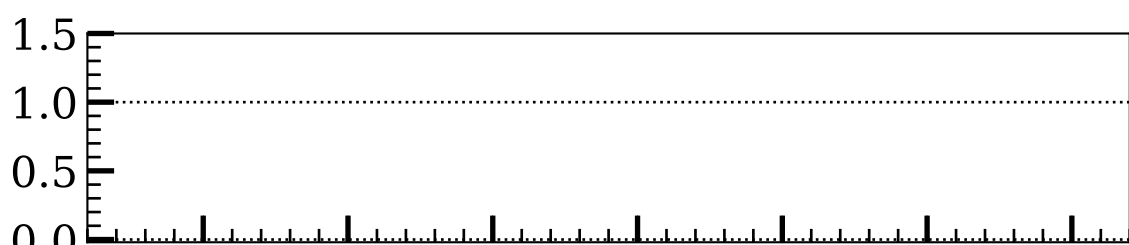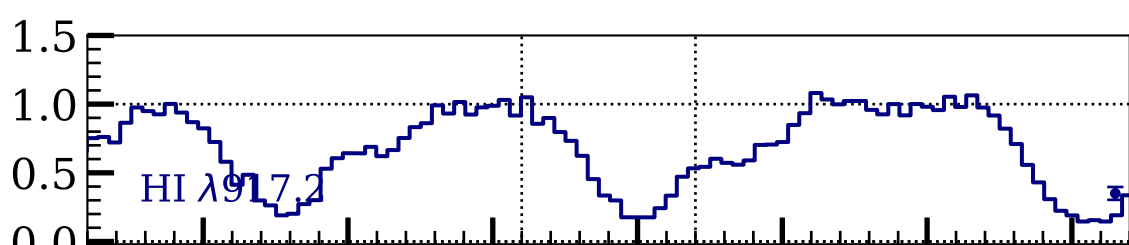

Rest-Frame Velocity ( $\text{km s}^{-1}$ )

J163201.12+373749.9,  $z=0.417740$ , RF=1

Normalized Flux

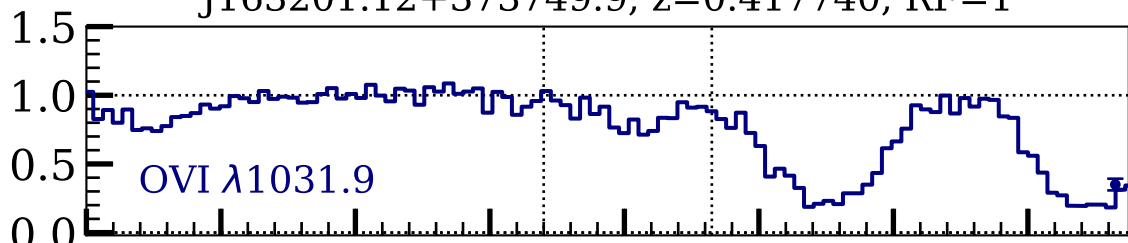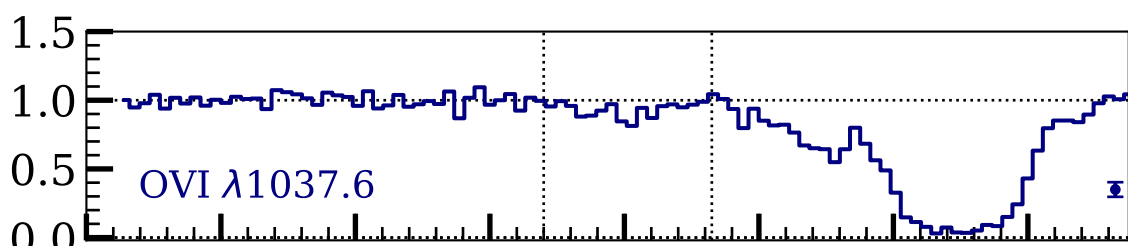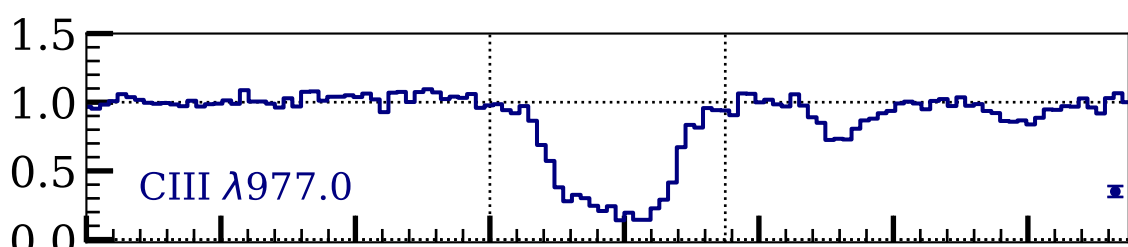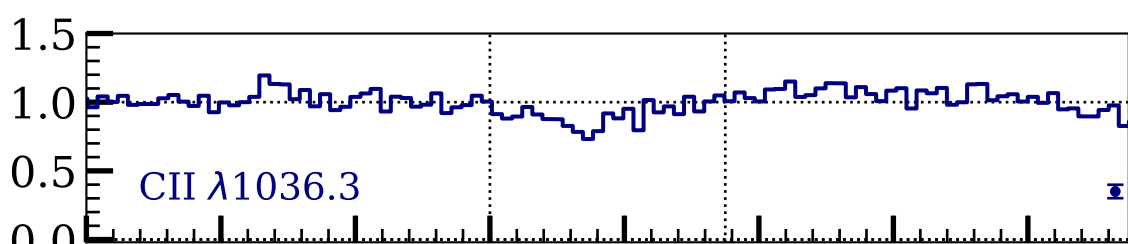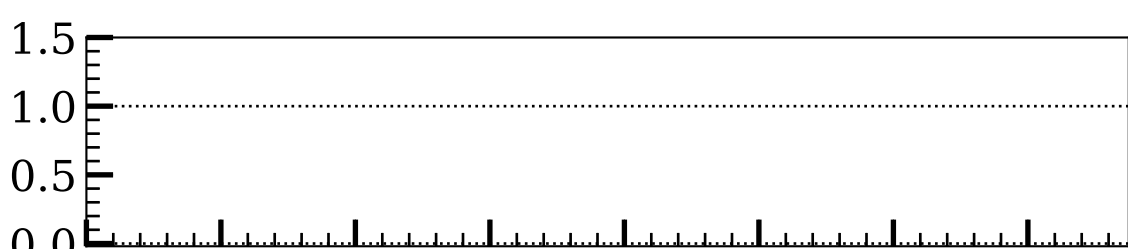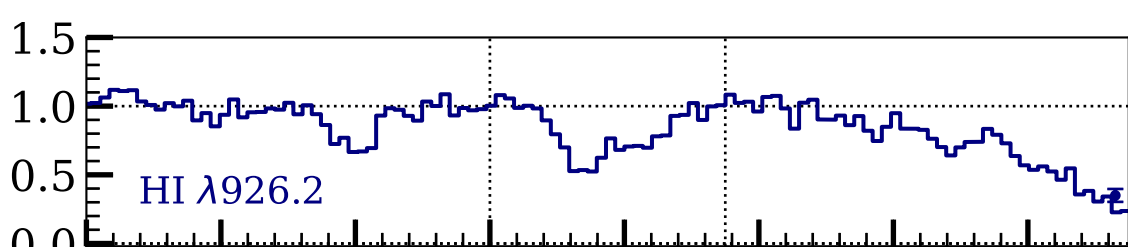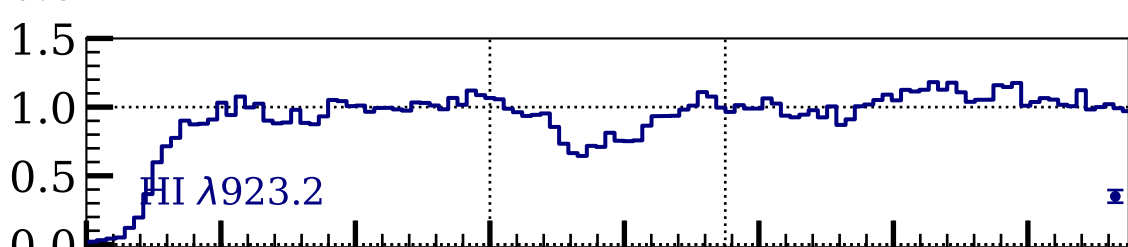

Rest-Frame Velocity ( $\text{km s}^{-1}$ )

J215647.46+224249.8,  $z=0.592763$ , RF=0

Normalized Flux

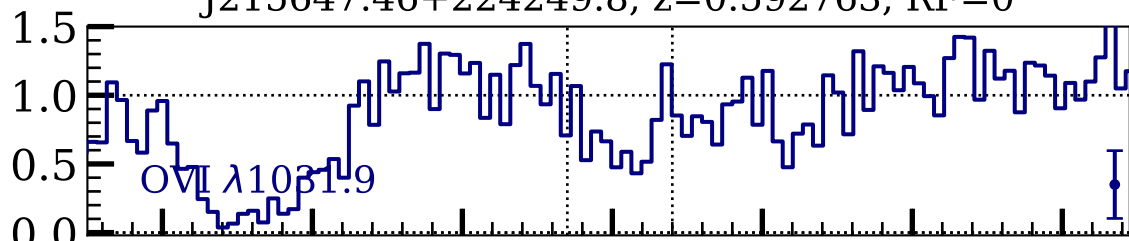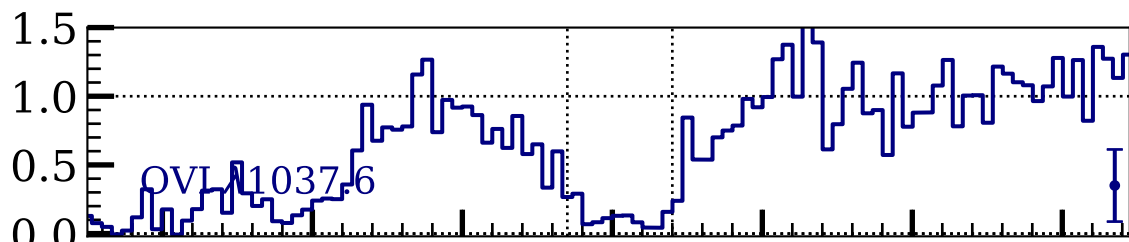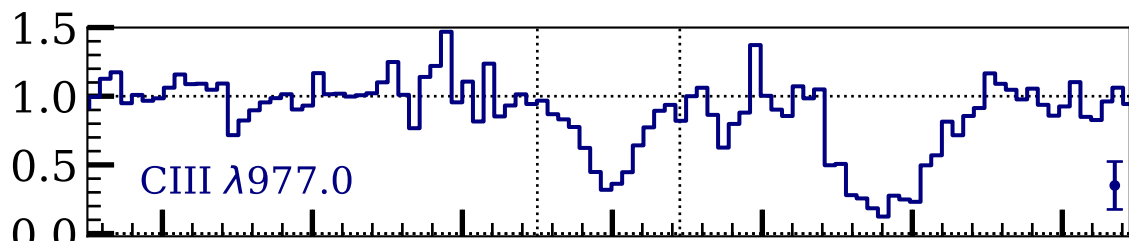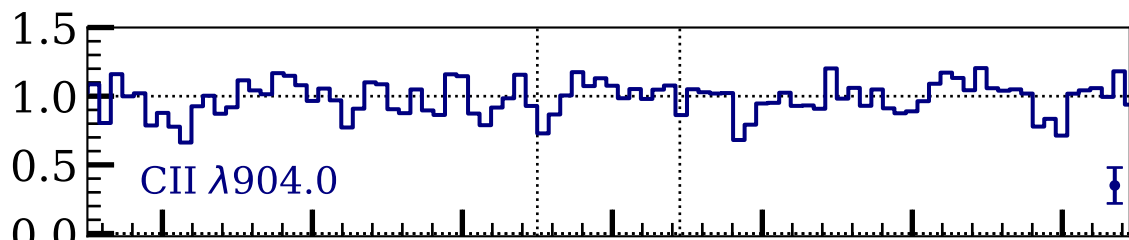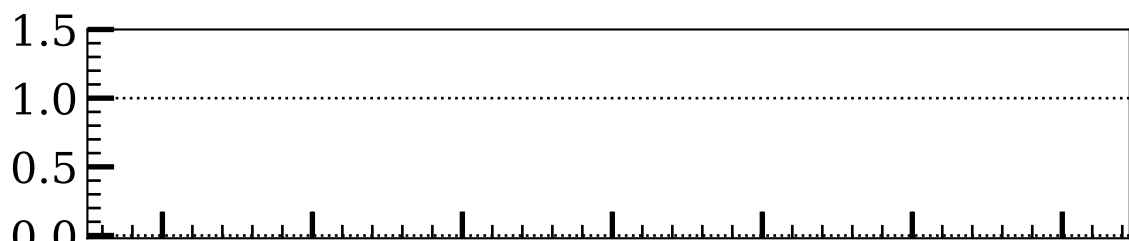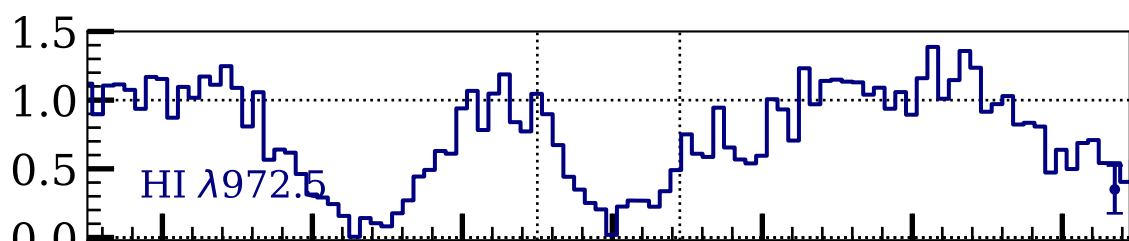

Rest-Frame Velocity ( $\text{km s}^{-1}$ )



J215647.46+224249.8,  $z=0.619964$ , RF=0

Normalized Flux

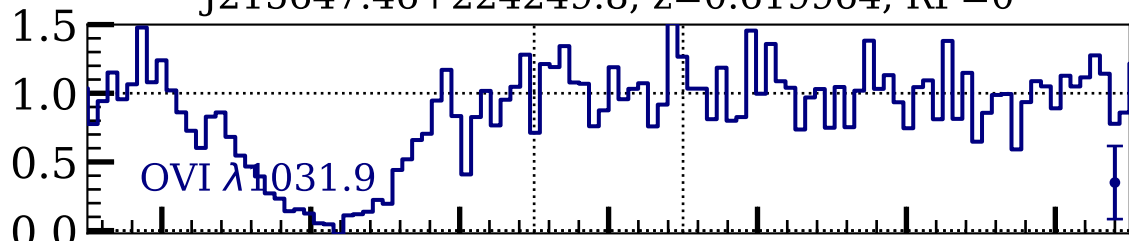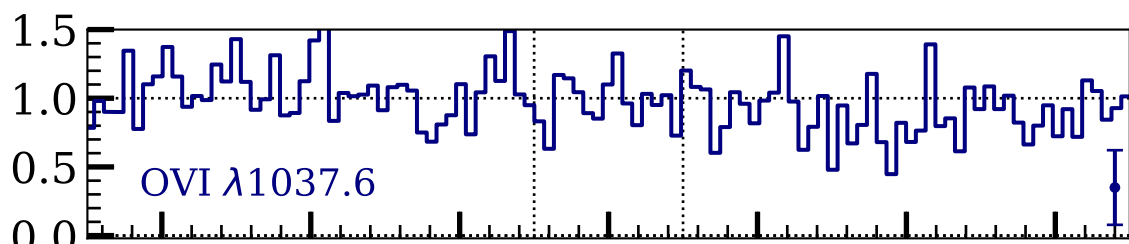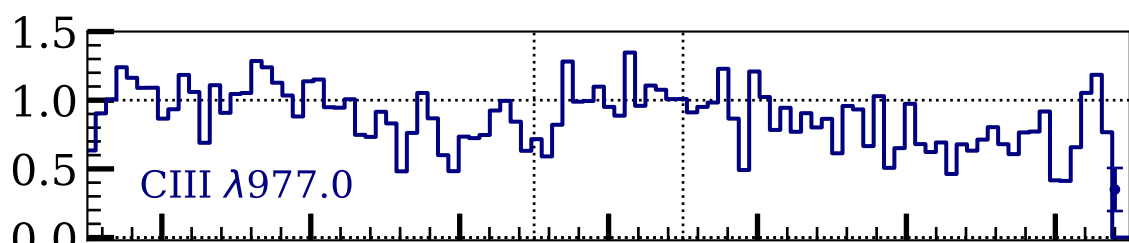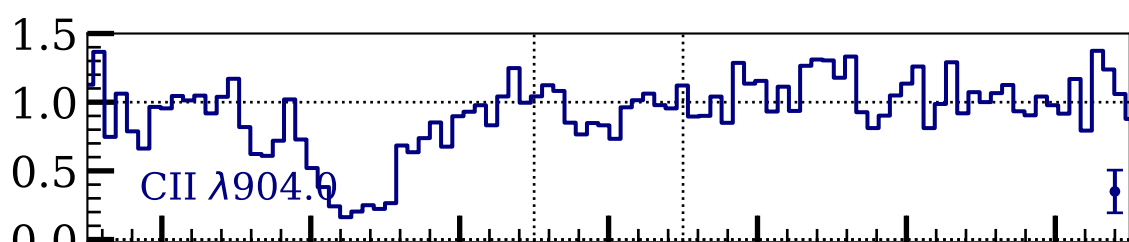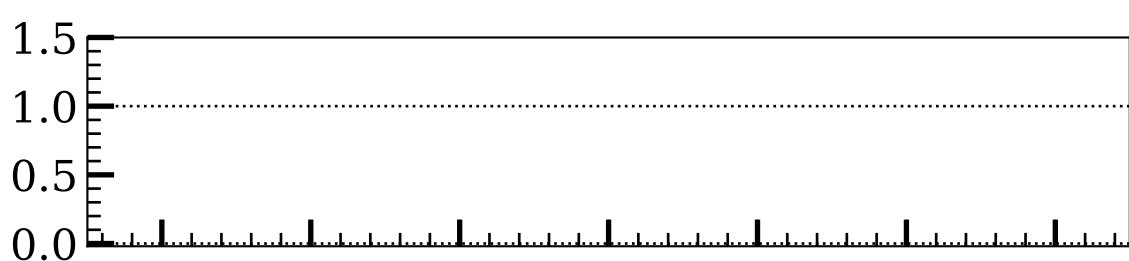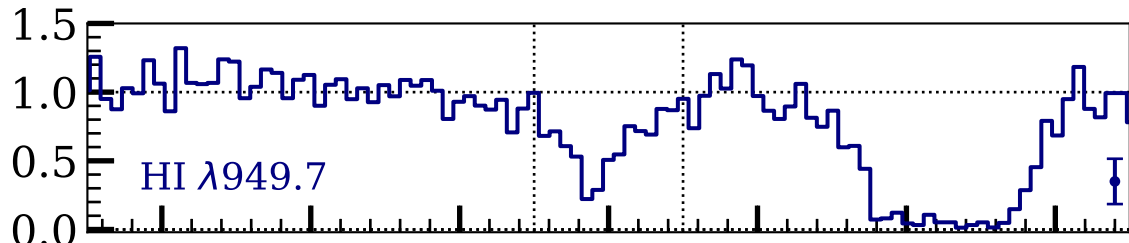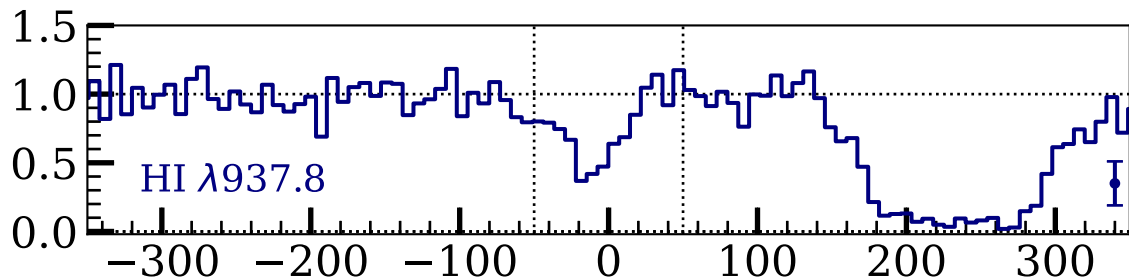

Rest-Frame Velocity ( $\text{km s}^{-1}$ )

J215647.46+224249.8,  $z=0.621016$ , RF=0

Normalized Flux

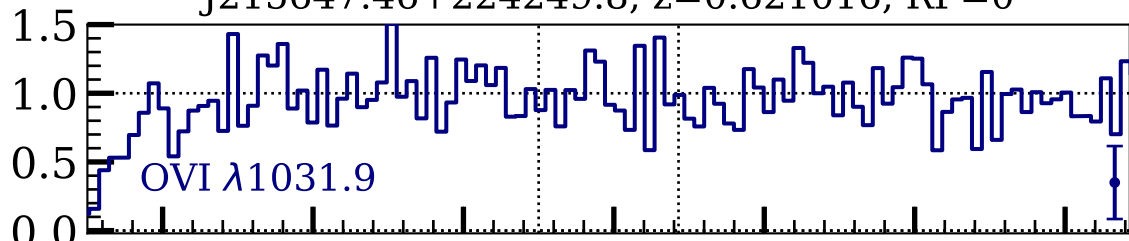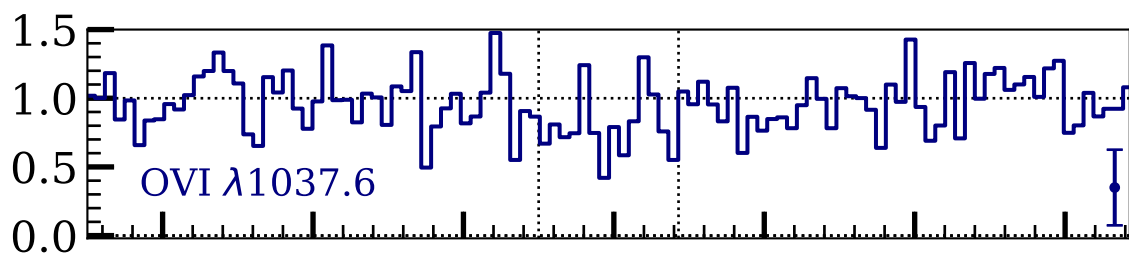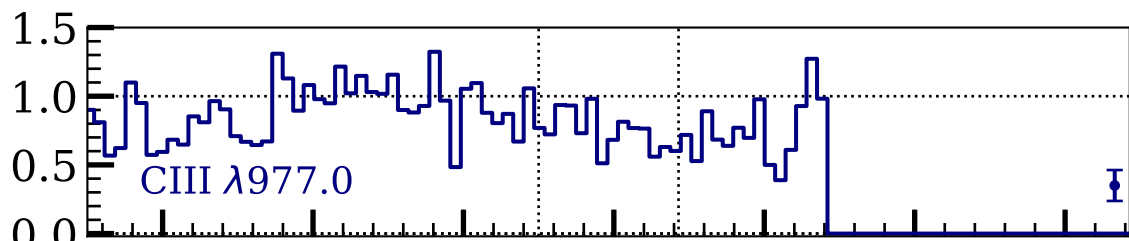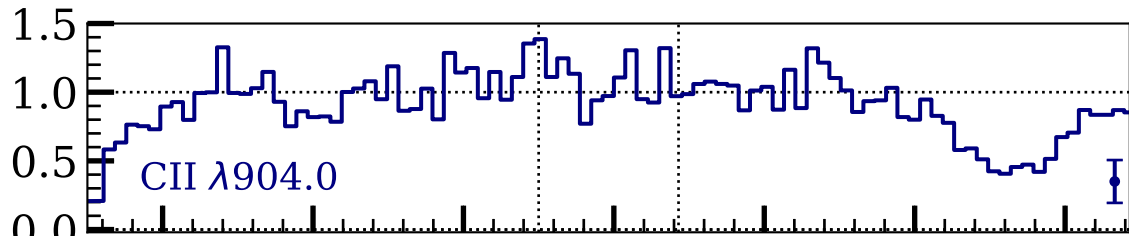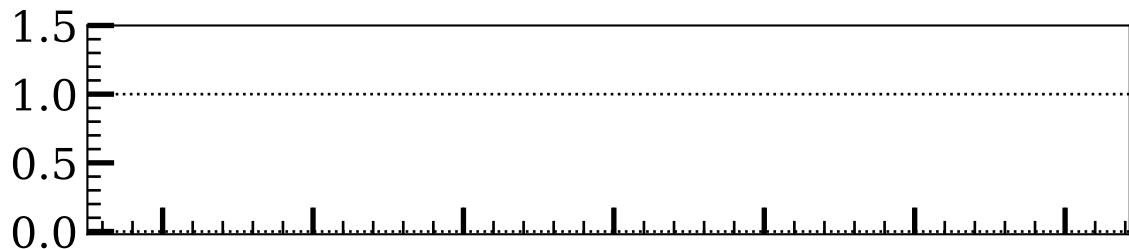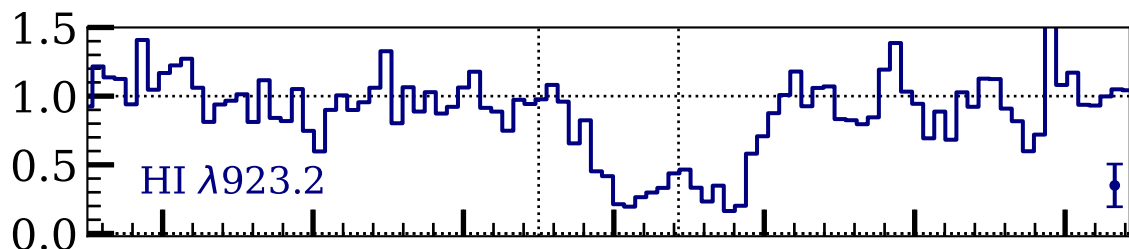

Rest-Frame Velocity ( $\text{km s}^{-1}$ )

J215647.46+224249.8,  $z=0.621378$ , RF=0

Normalized Flux

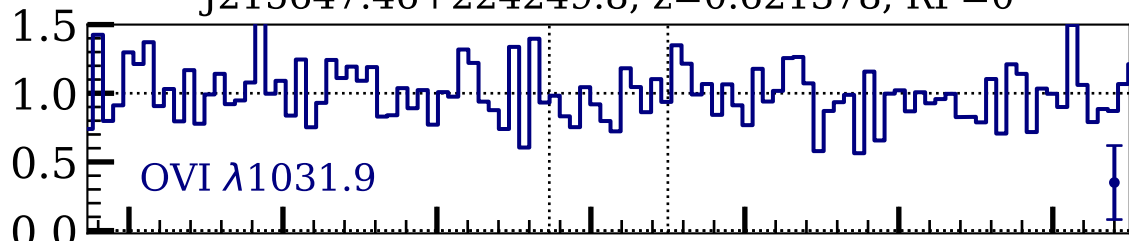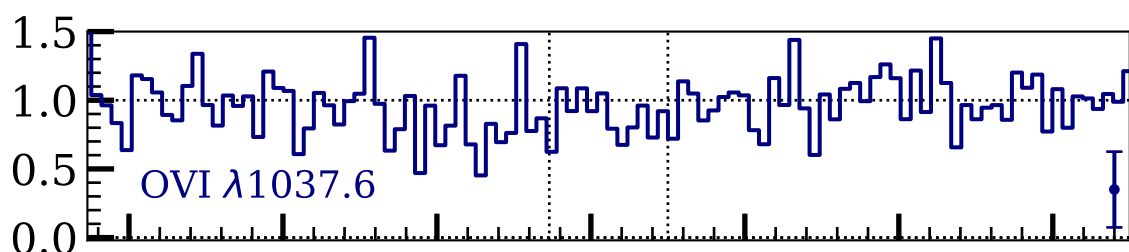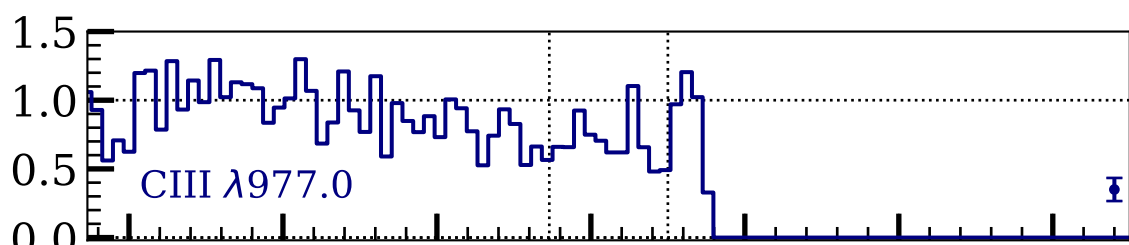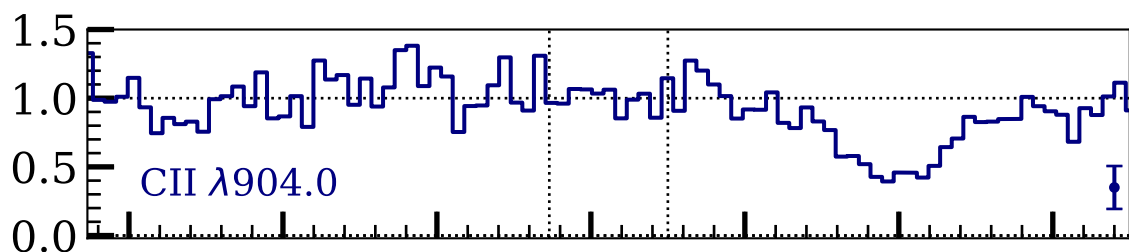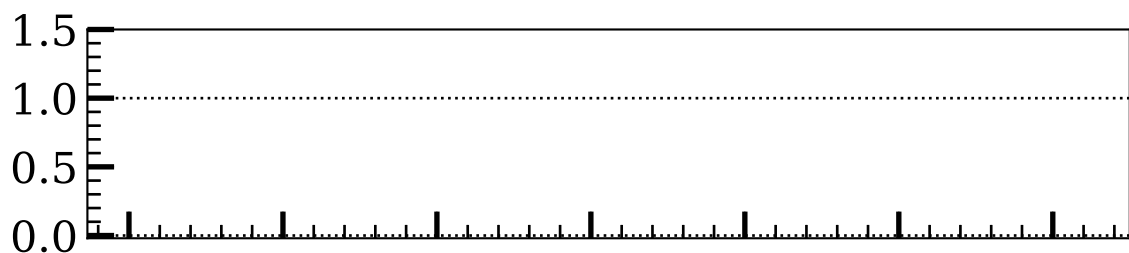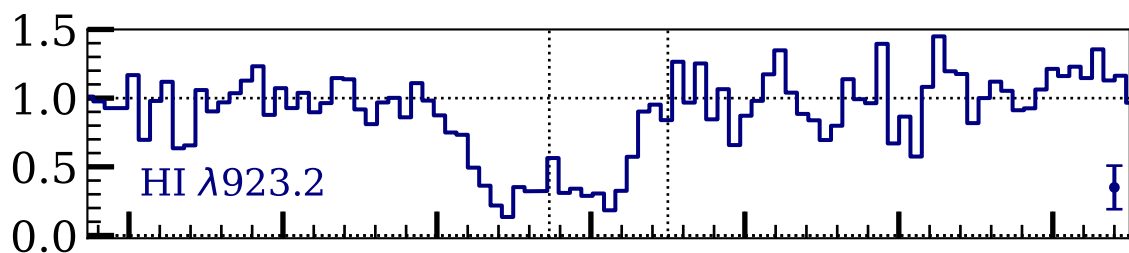

Rest-Frame Velocity ( $\text{km s}^{-1}$ )

J225357.75+160853.1,  $z=0.320621$ , RF=0

Normalized Flux

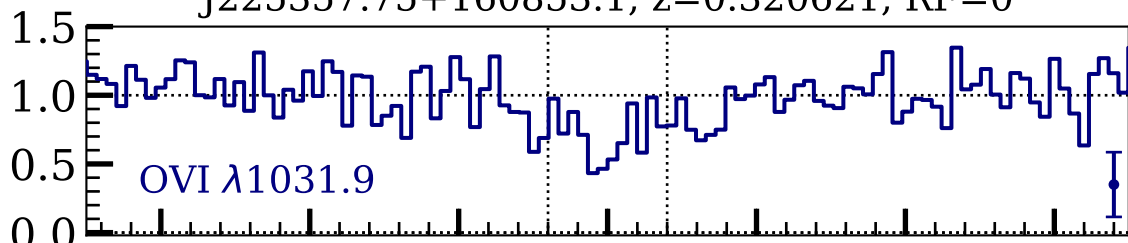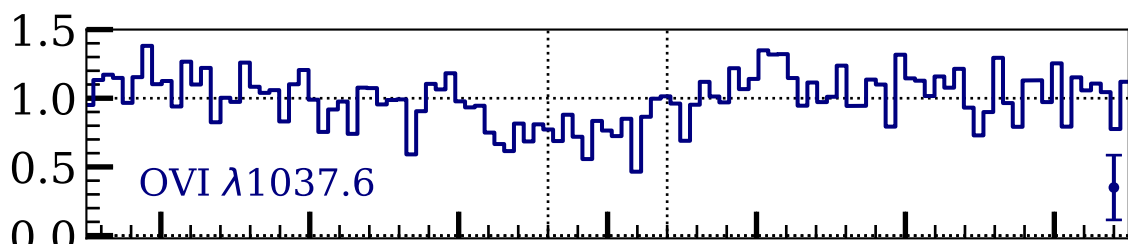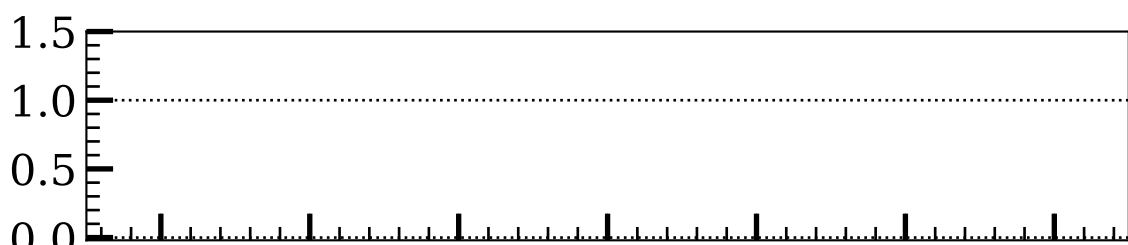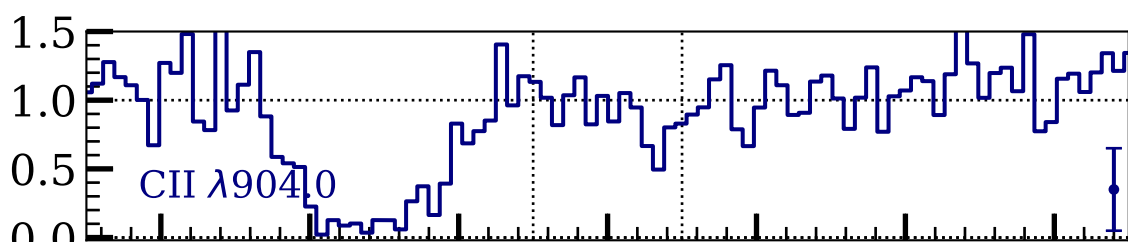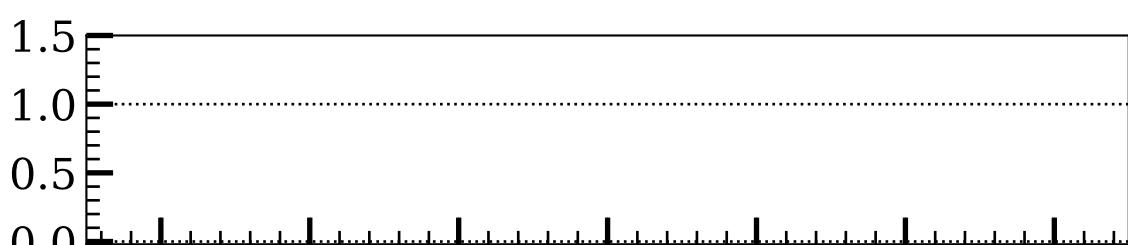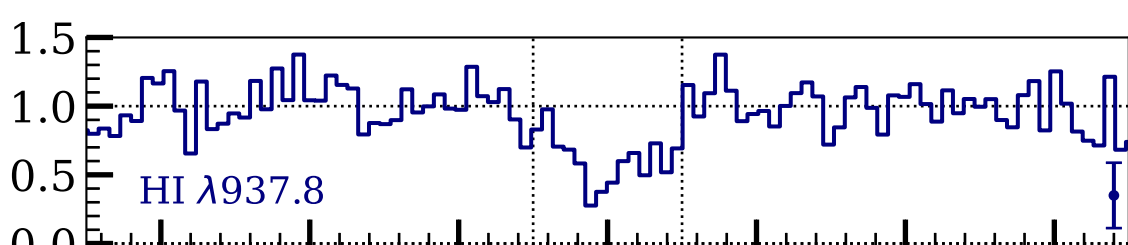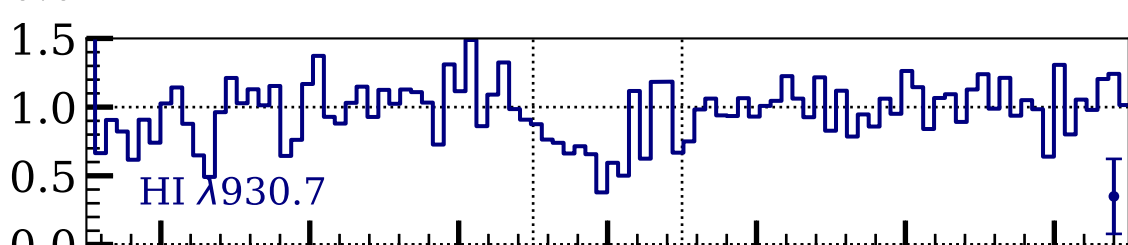

Rest-Frame Velocity ( $\text{km s}^{-1}$ )

J225738.20+134045.4,  $z=0.498882$ , RF=1

Normalized Flux

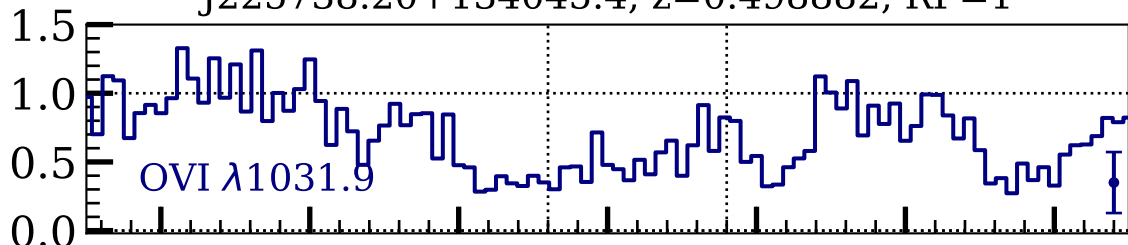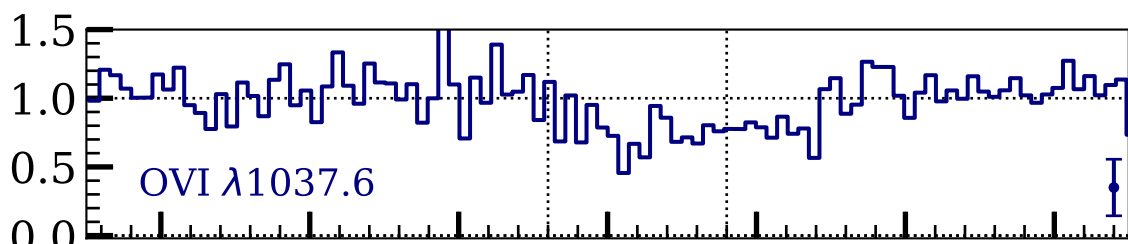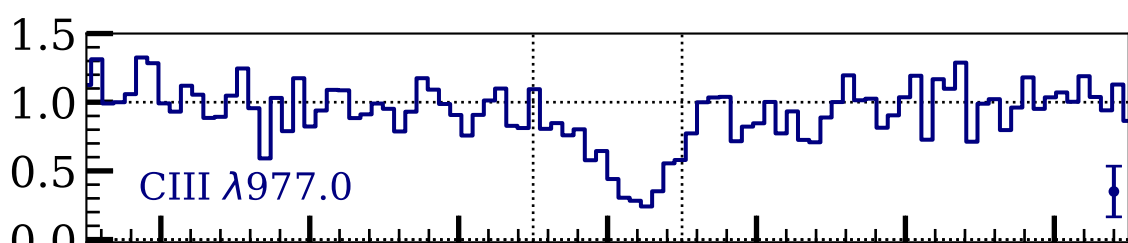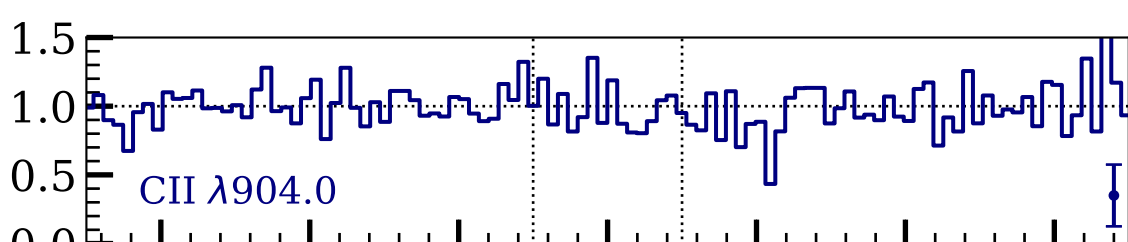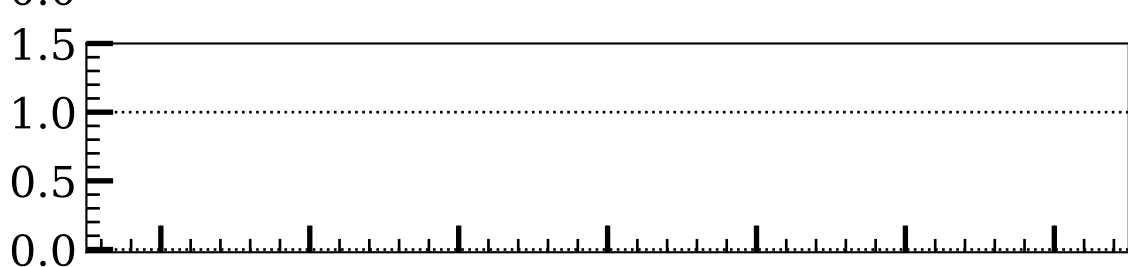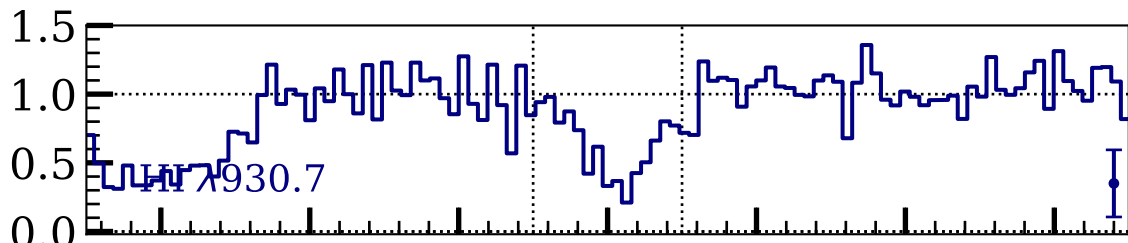

Rest-Frame Velocity ( $\text{km s}^{-1}$ )

J234500.43-005936.0,  $z=0.548121$ , RF=0

Normalized Flux

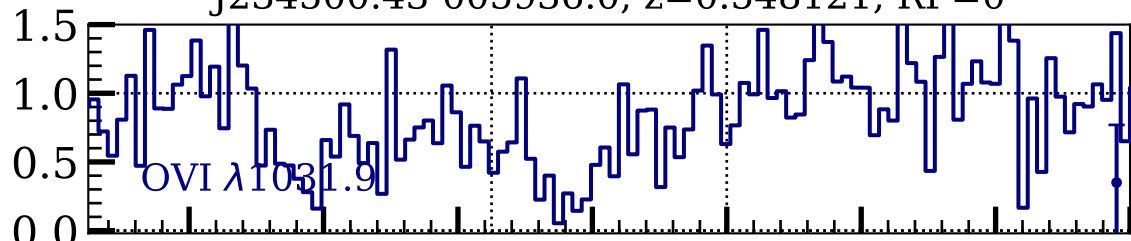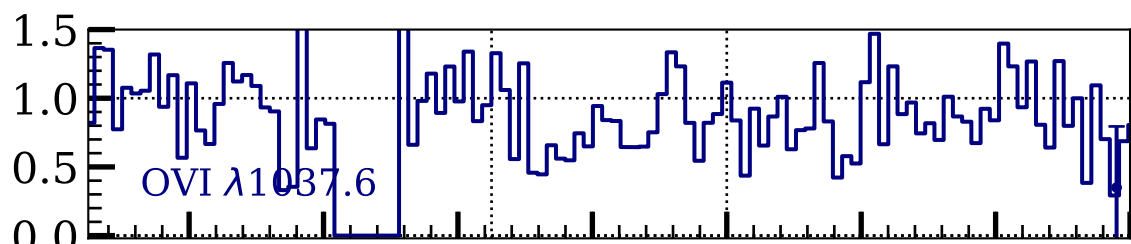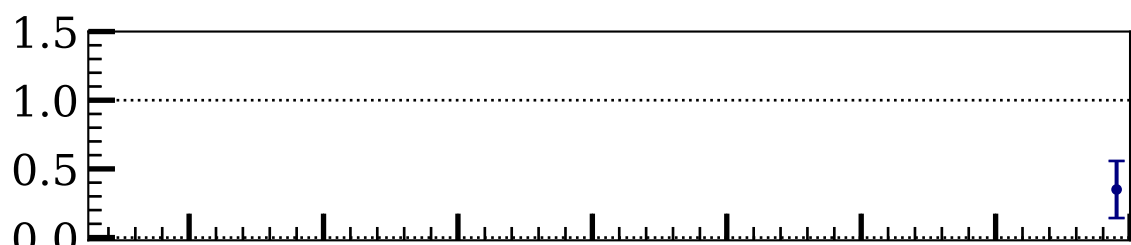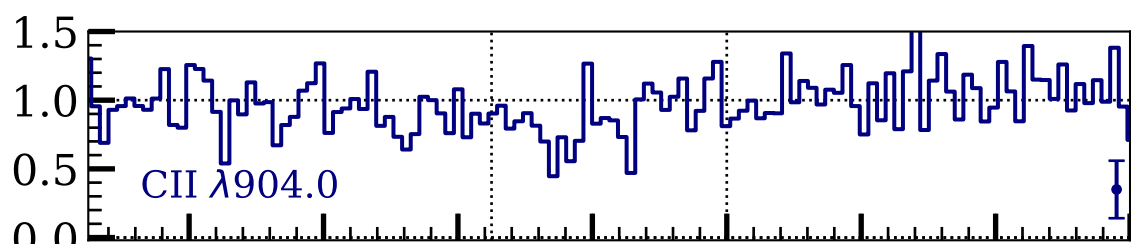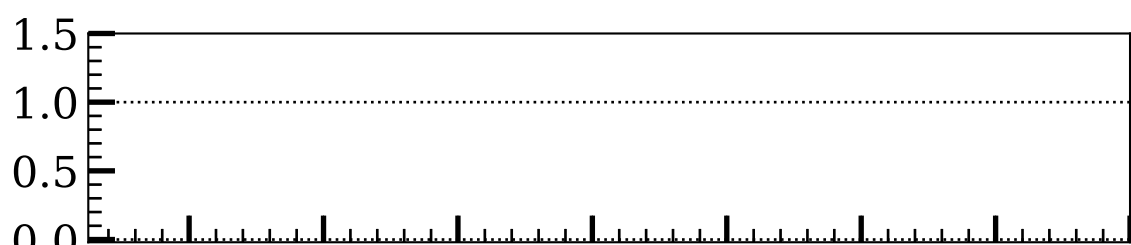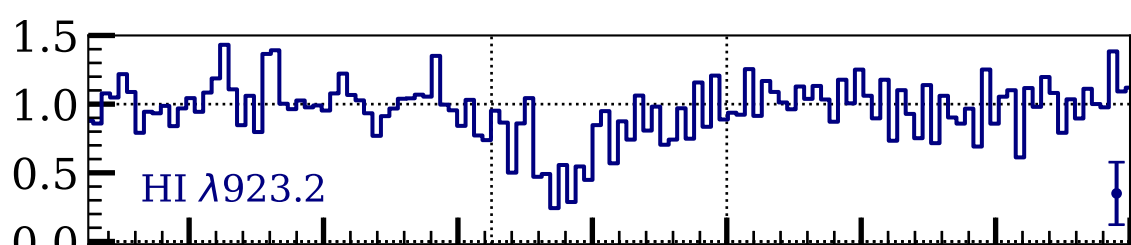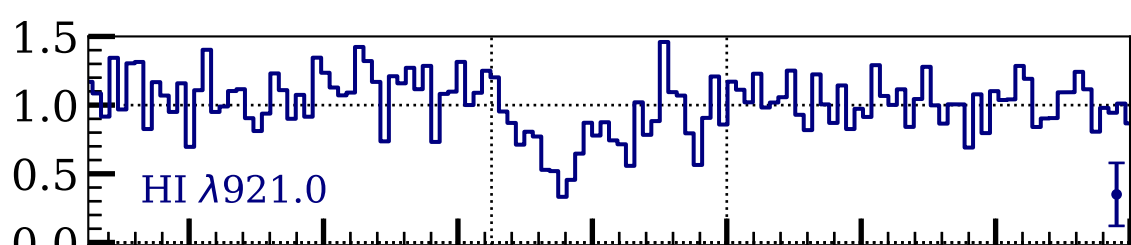

Rest-Frame Velocity (km s<sup>-1</sup>)
