# Supplementary material for: The COS CGM Compendium V: The Dichotomy of OVI Associated with Low- and High-Metallicity Cool Gas at z < 1
Source: arXiv:2403.02374 source file (2024-09-07)

J000559.23+160948.9,  $z=0.305789$ , RF=1

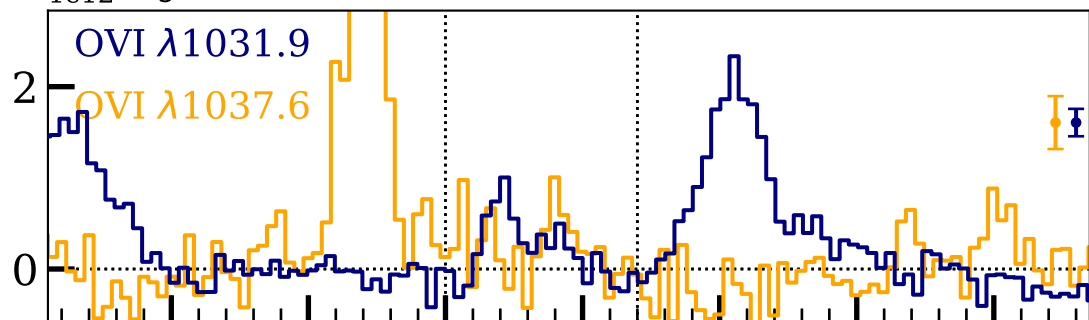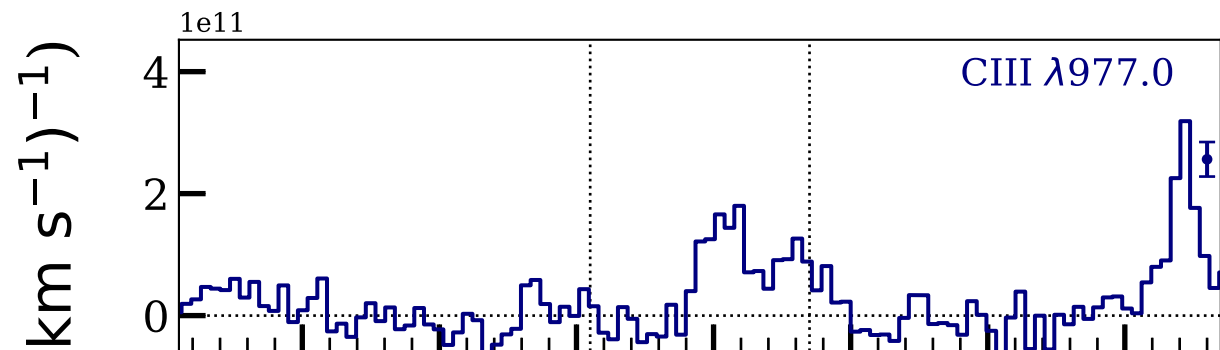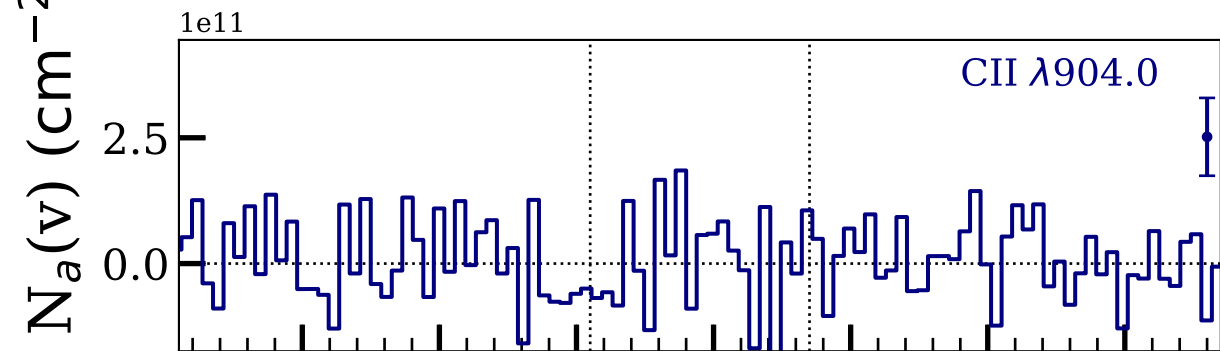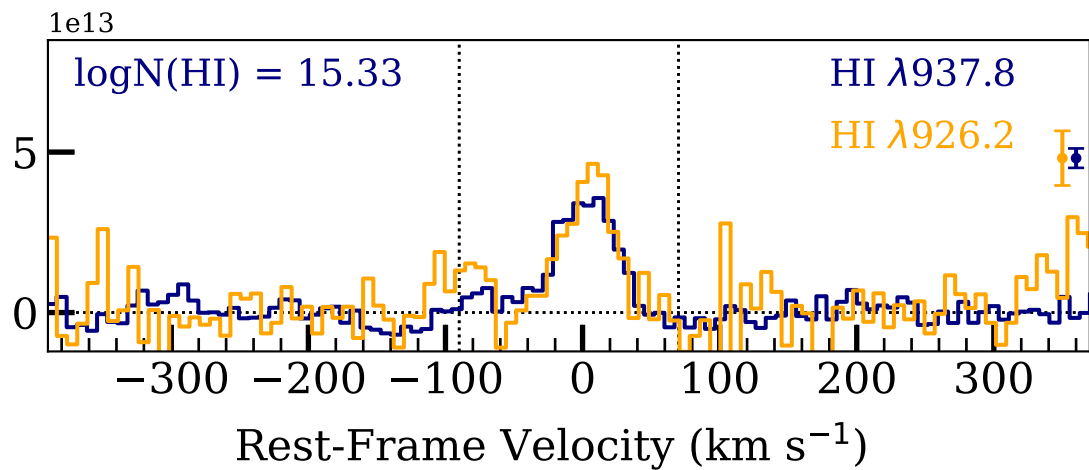

J000559.23+160948.9,  $z=0.347925$ , RF=1

$N_a(v) \text{ (cm}^{-2} \text{ (km s}^{-1})^{-1})$

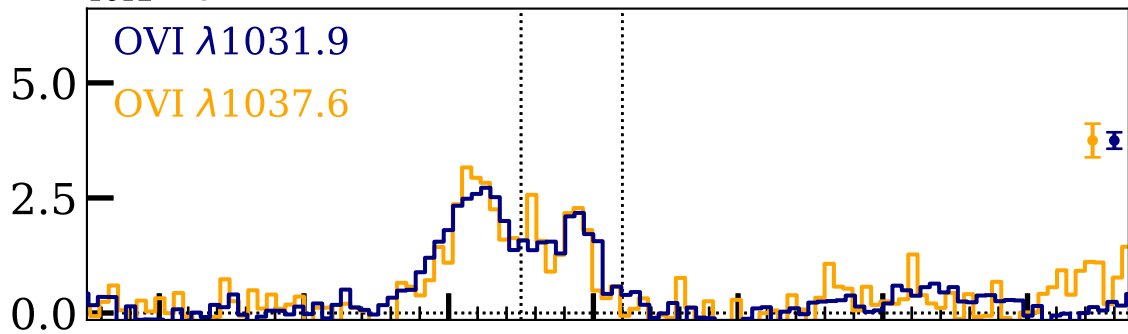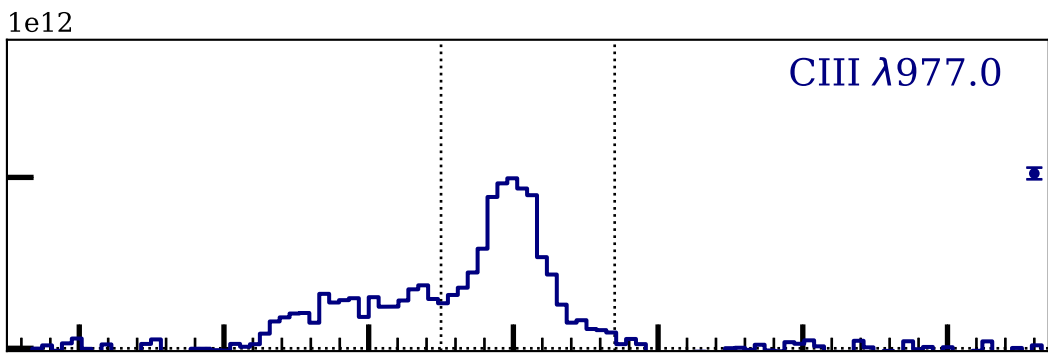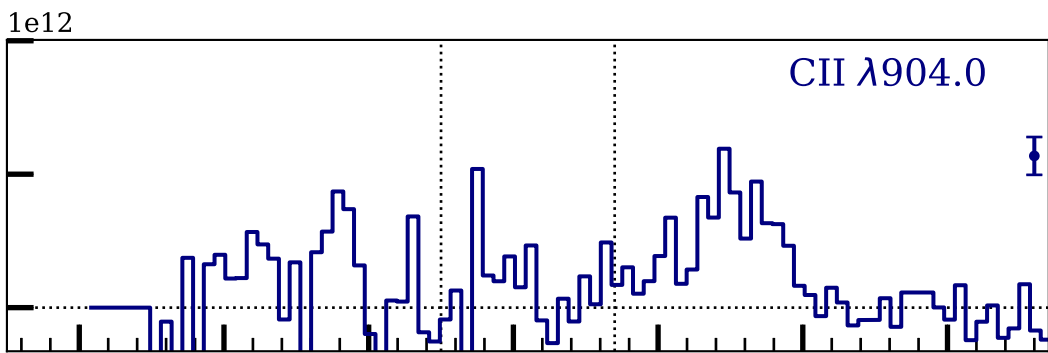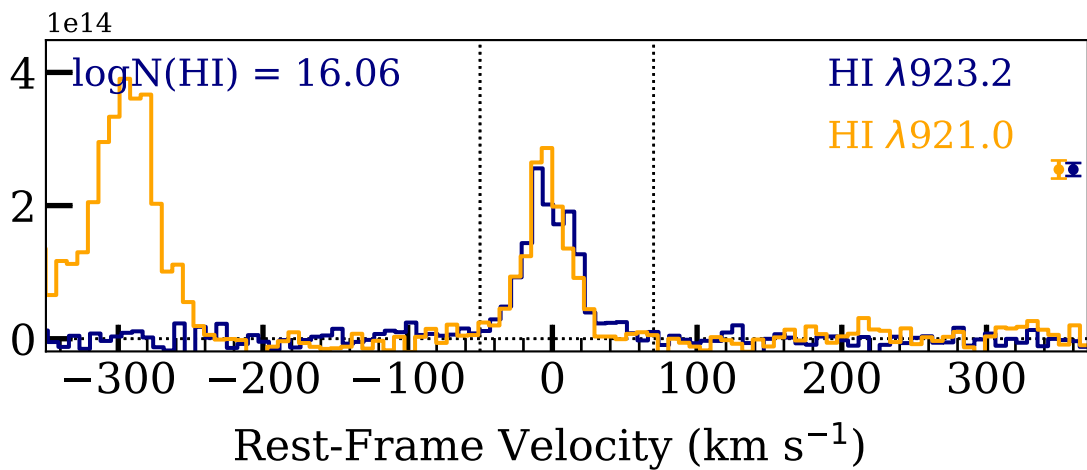

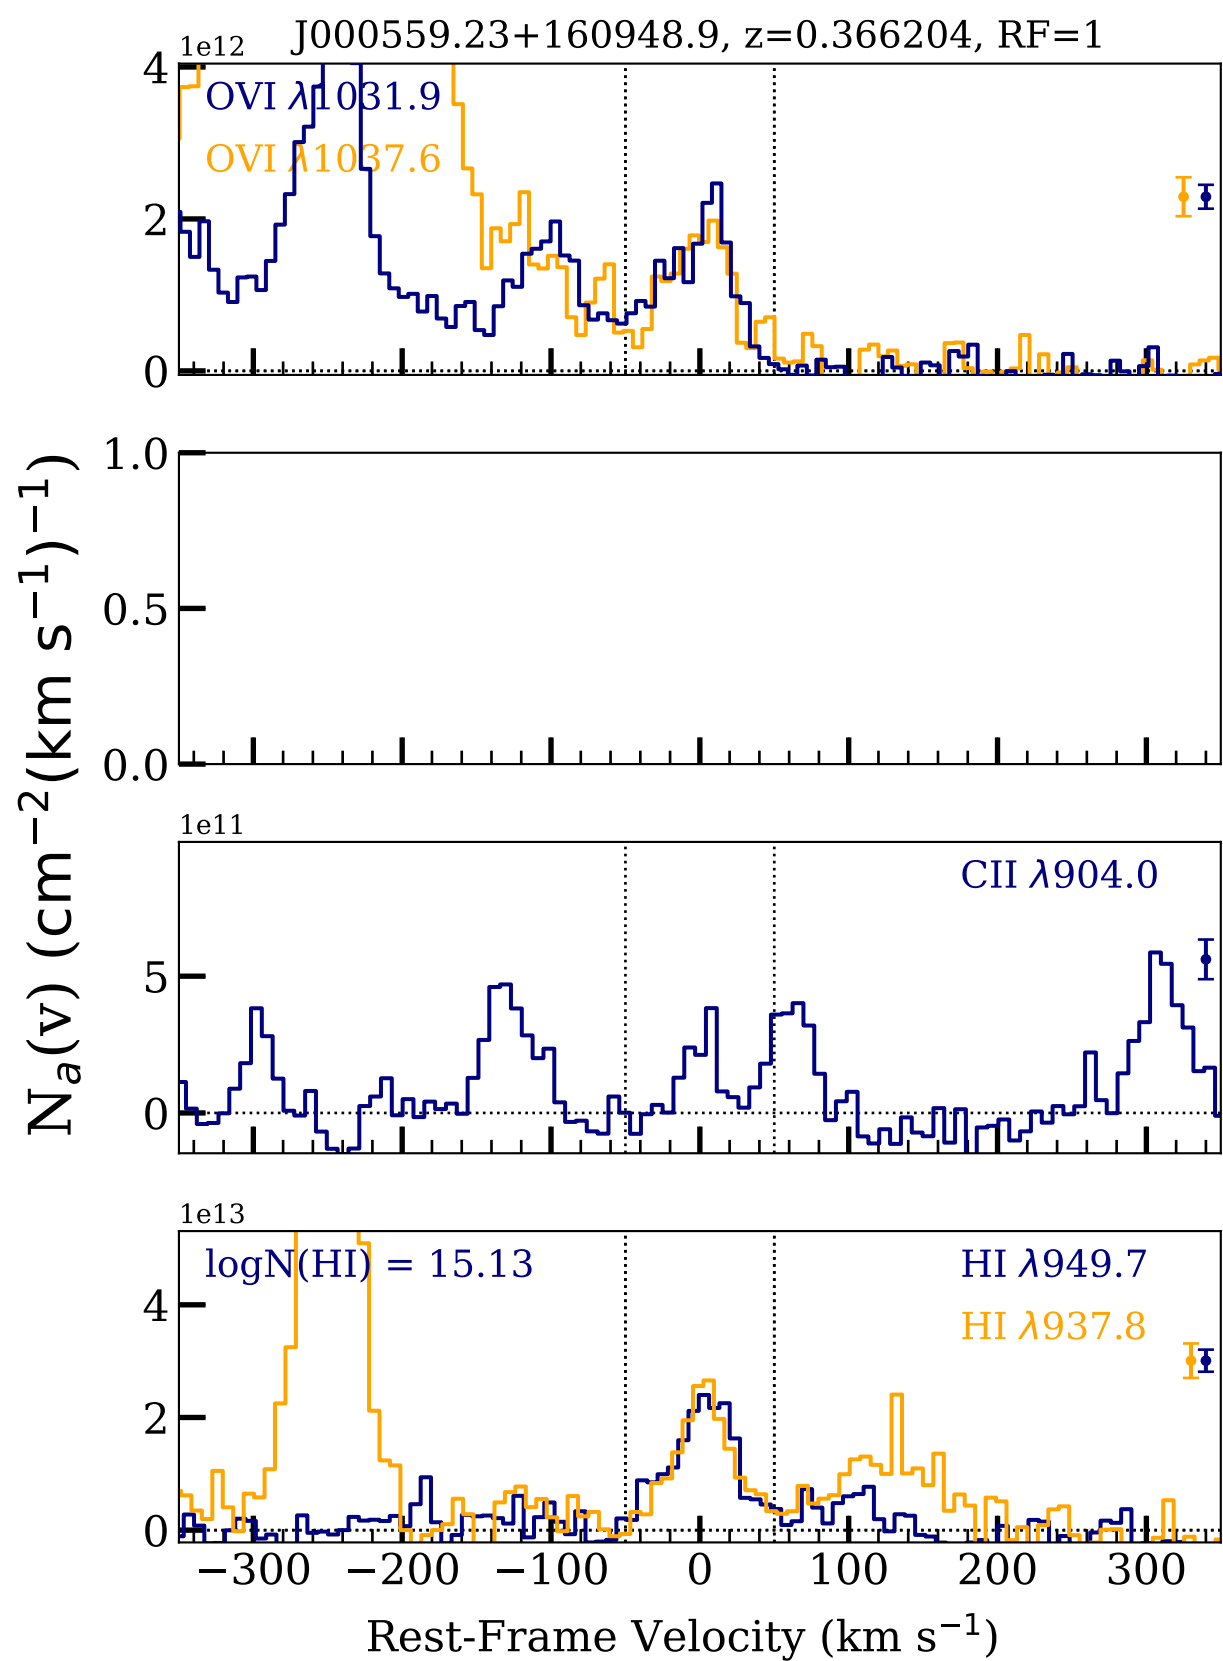

J004222.29-103743.8,  $z=0.316052$ , RF=1

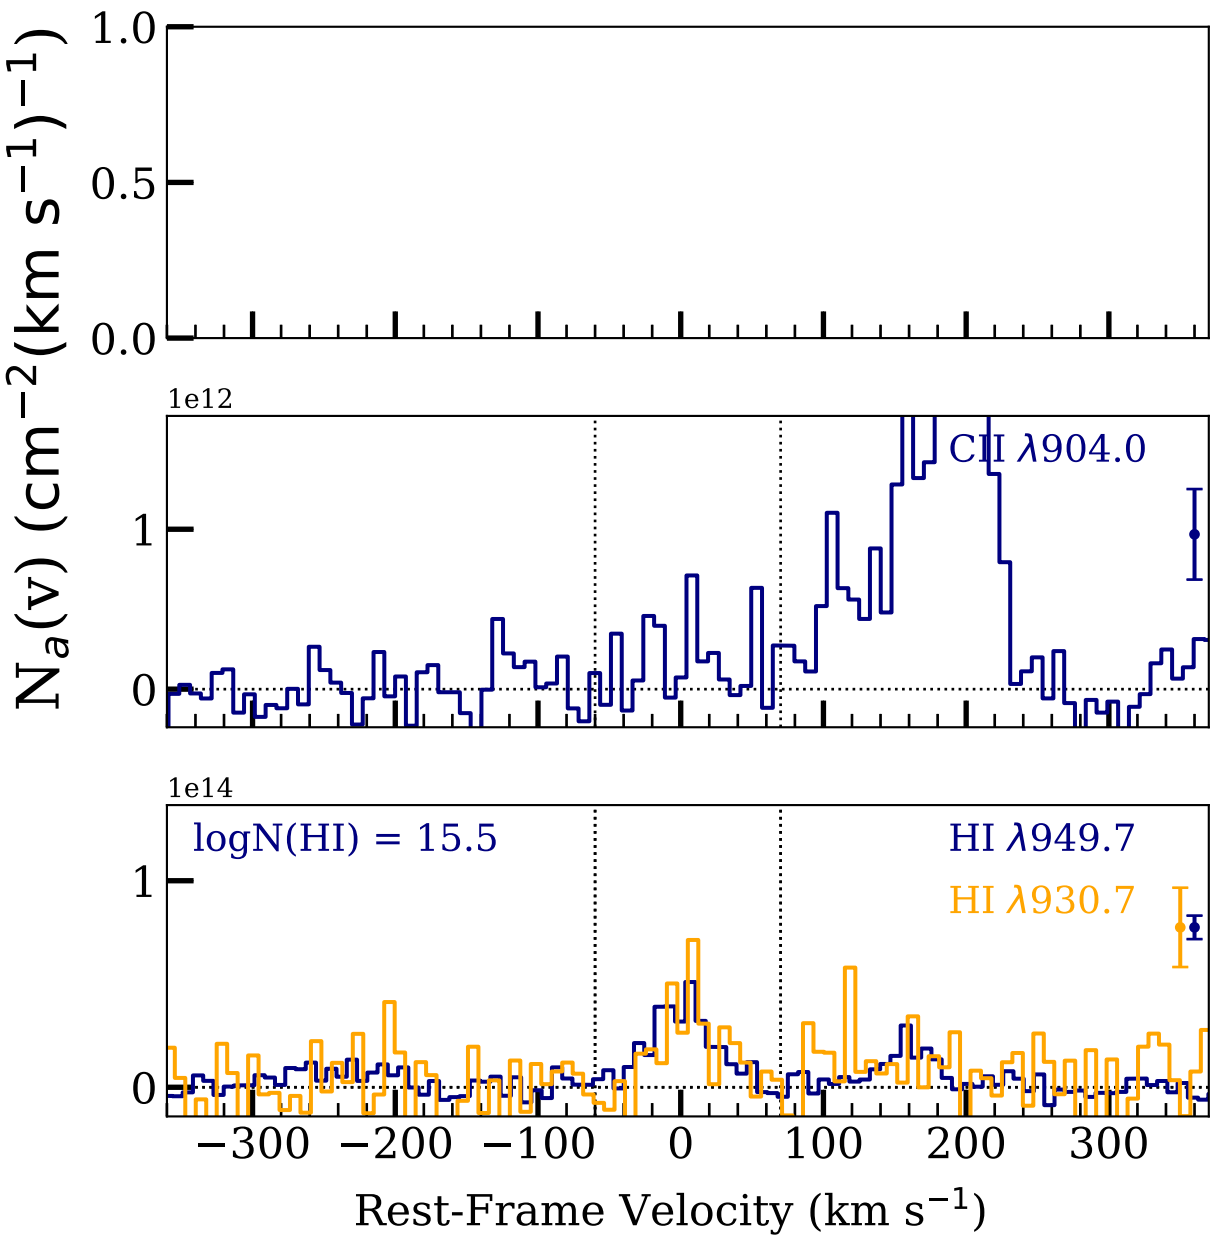

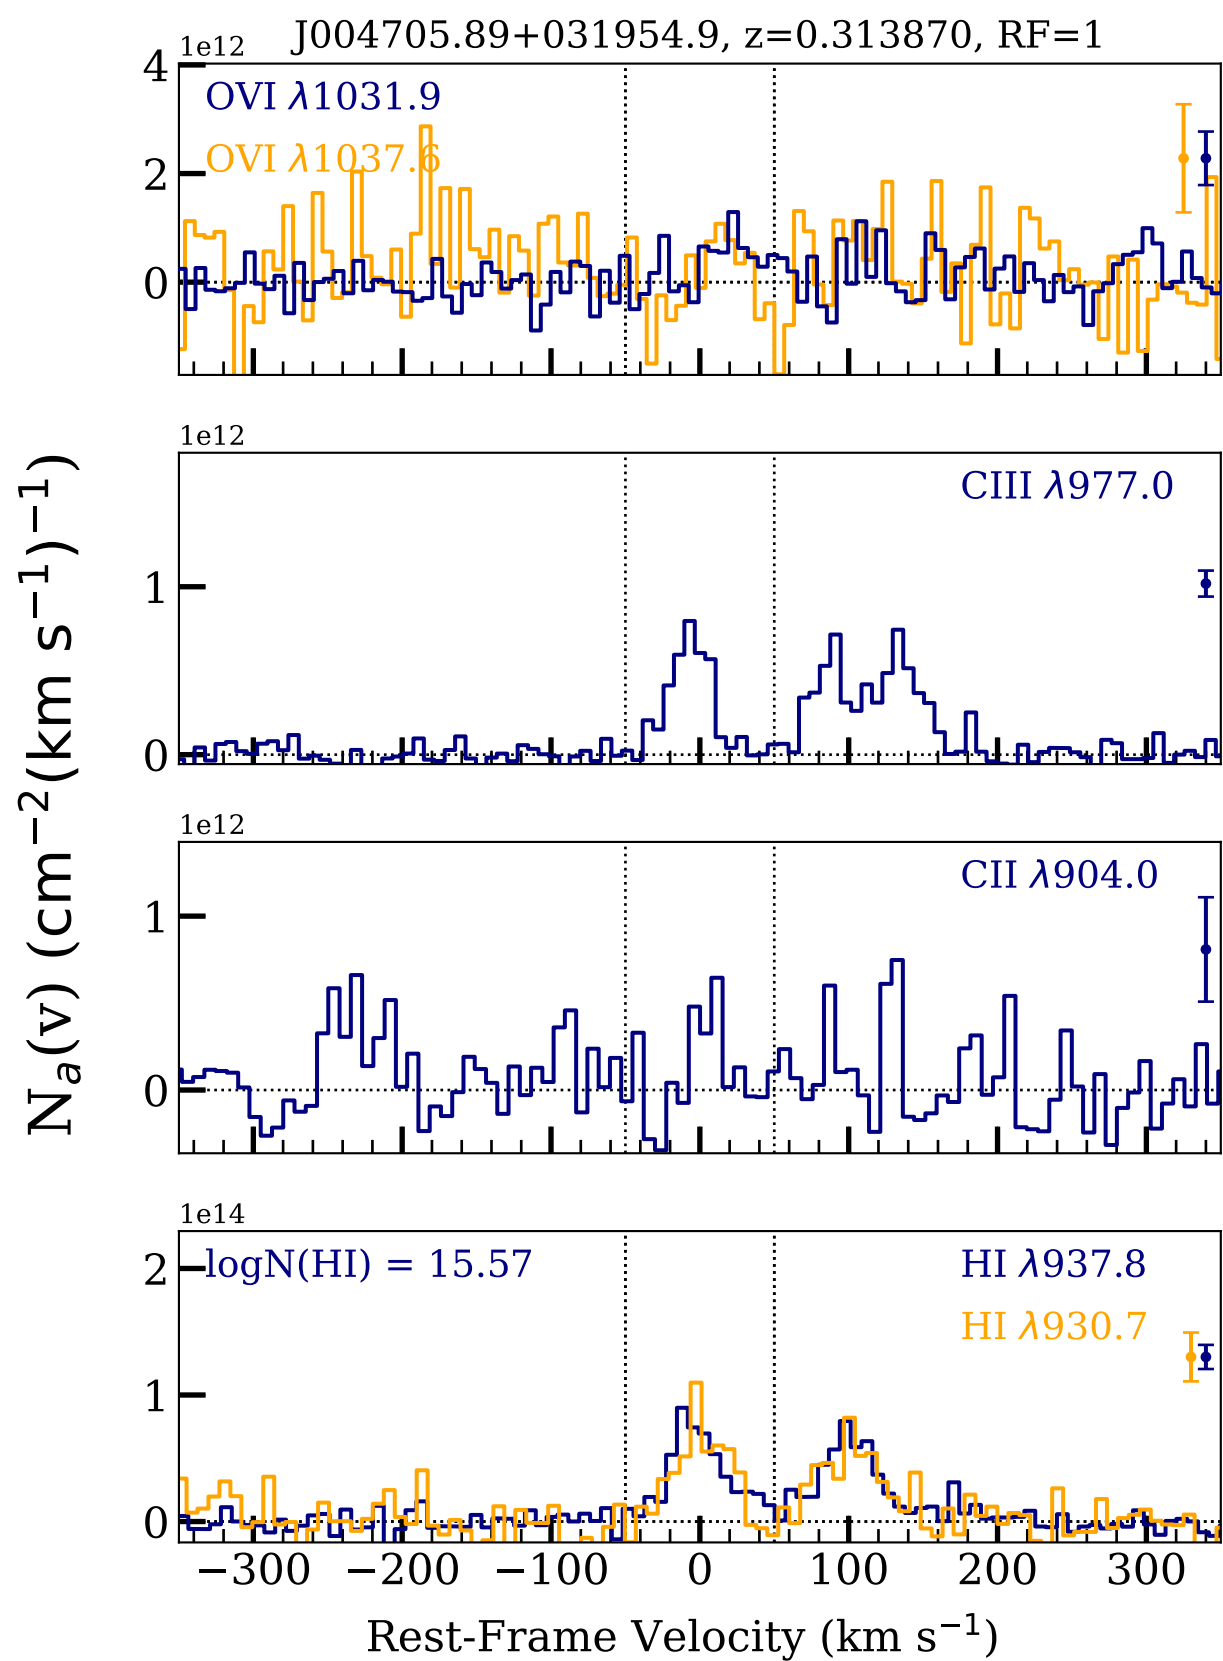

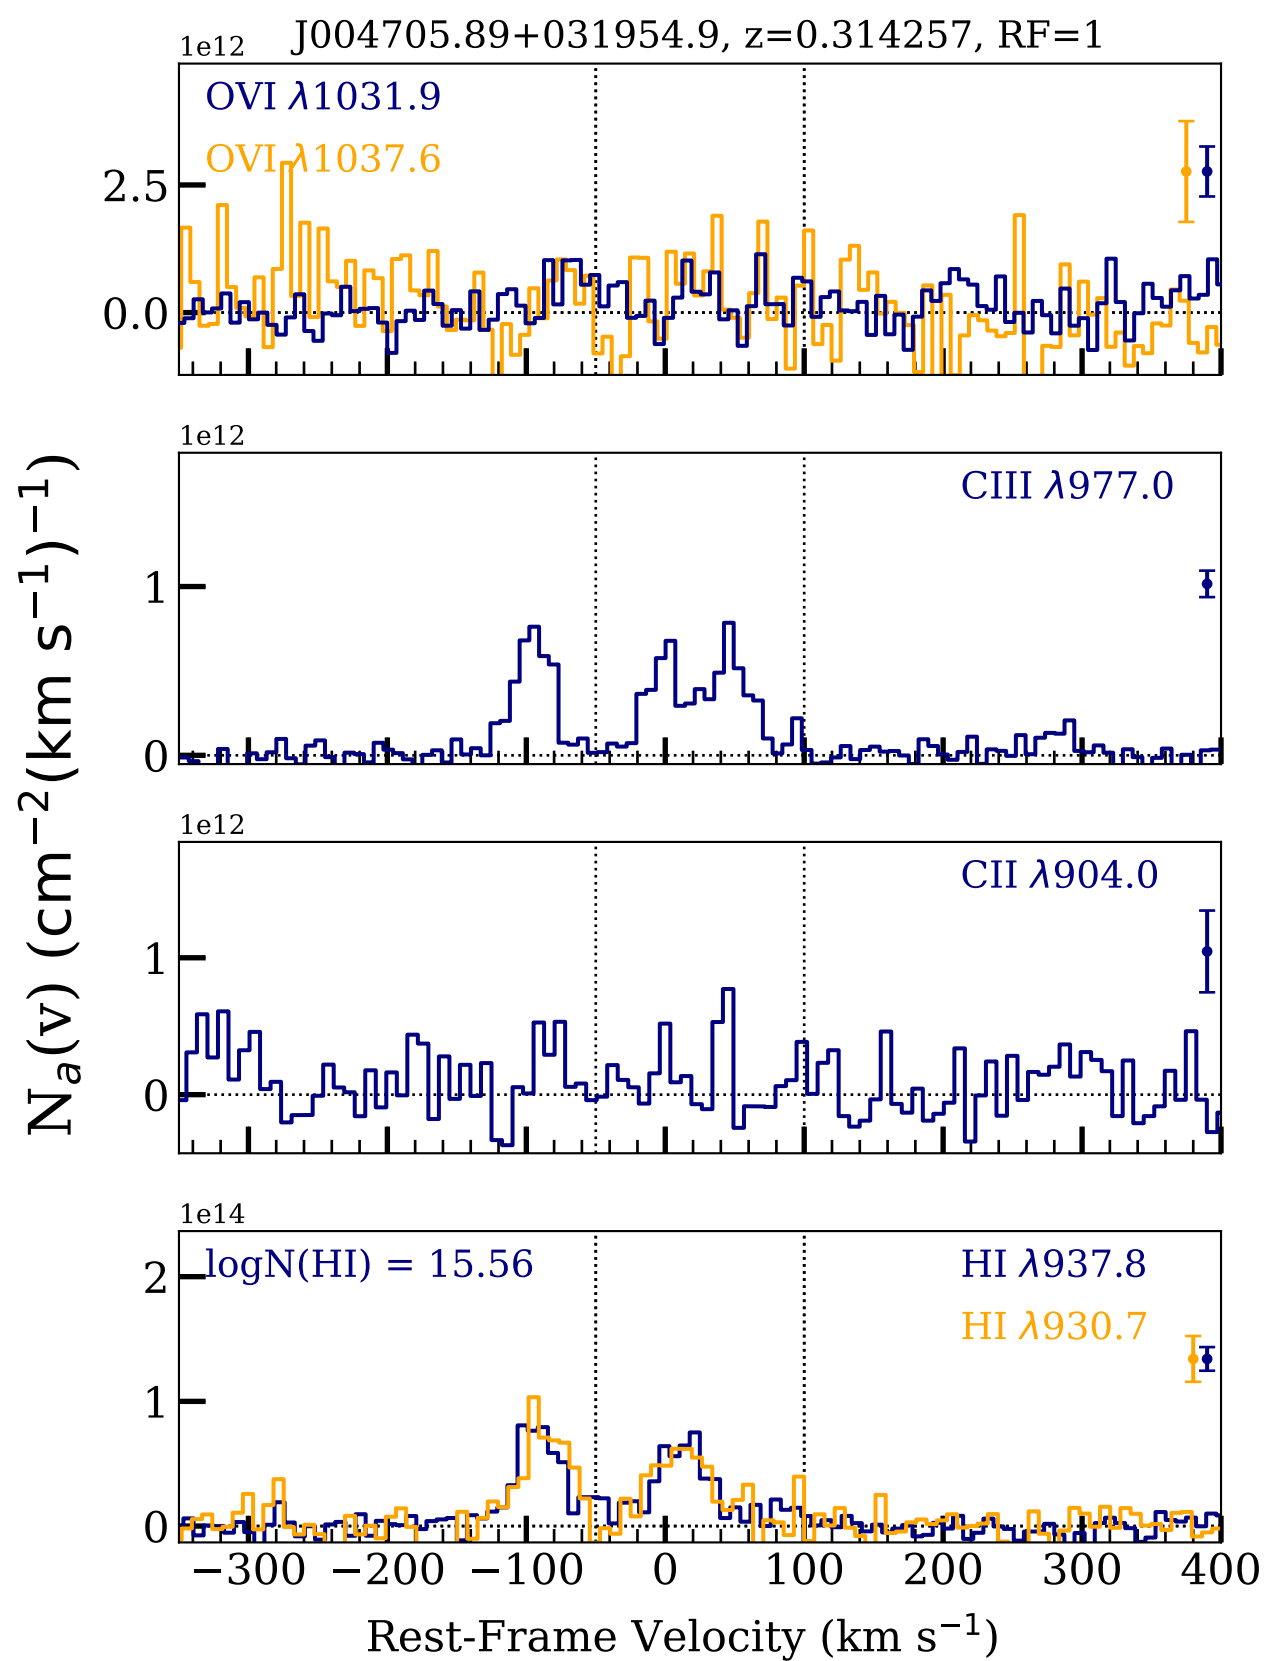

J011013.14-021952.8,  $z=0.227191$ , RF=1

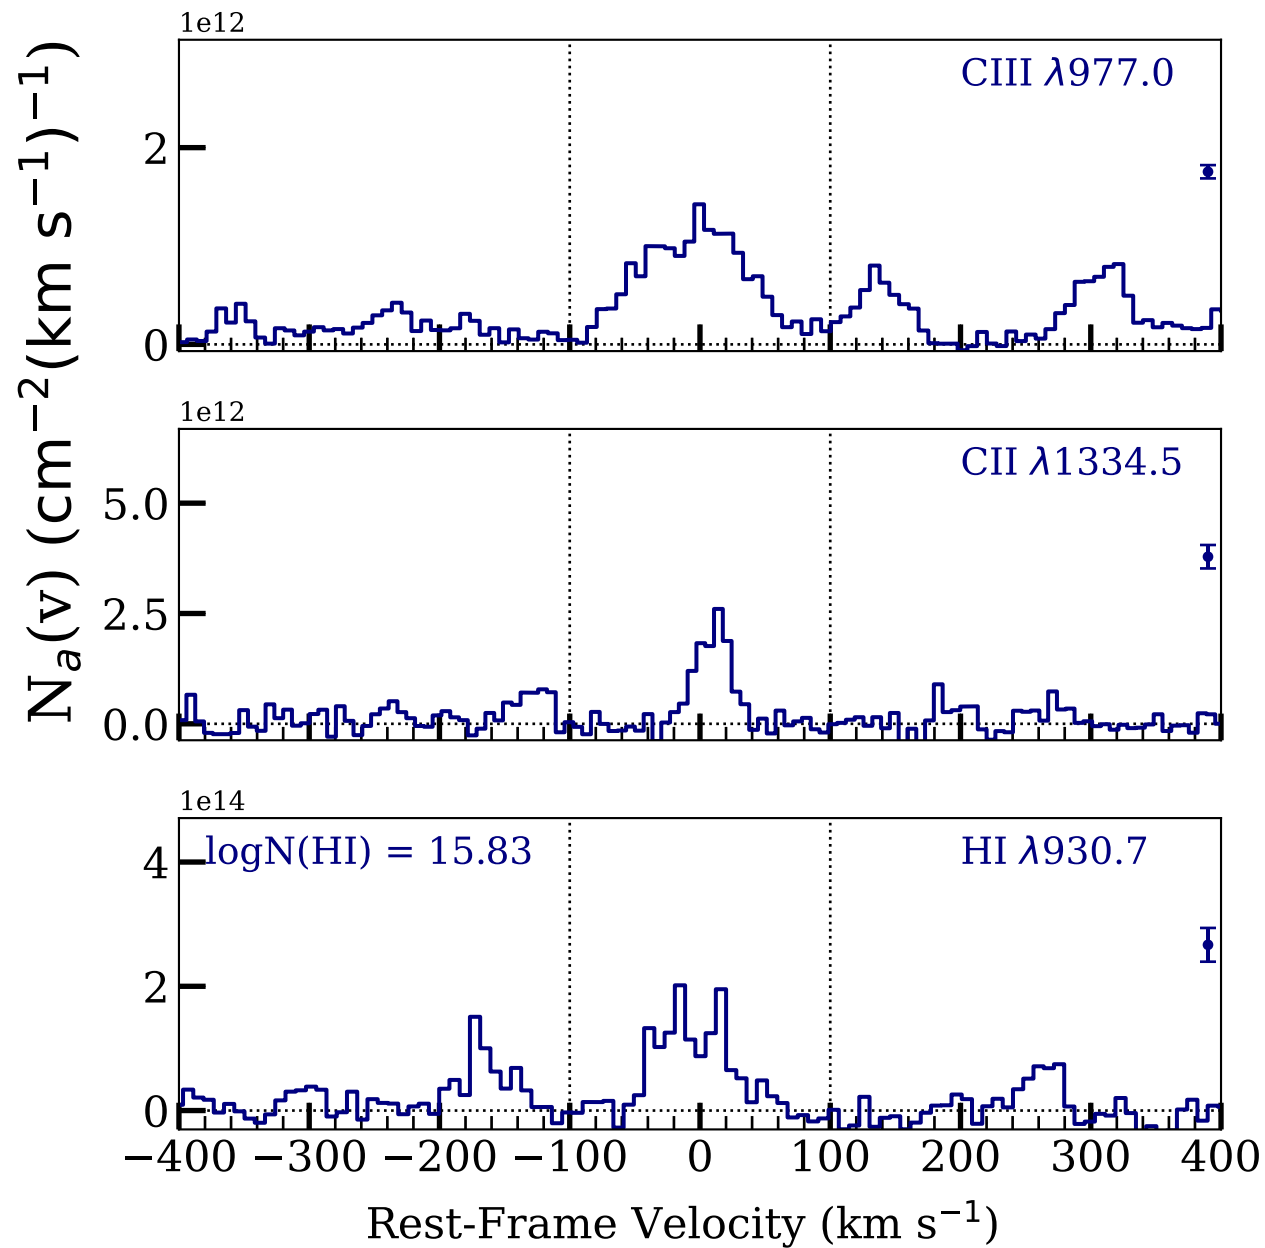

J011013.14-021952.8,  $z=0.536490$ , RF=1

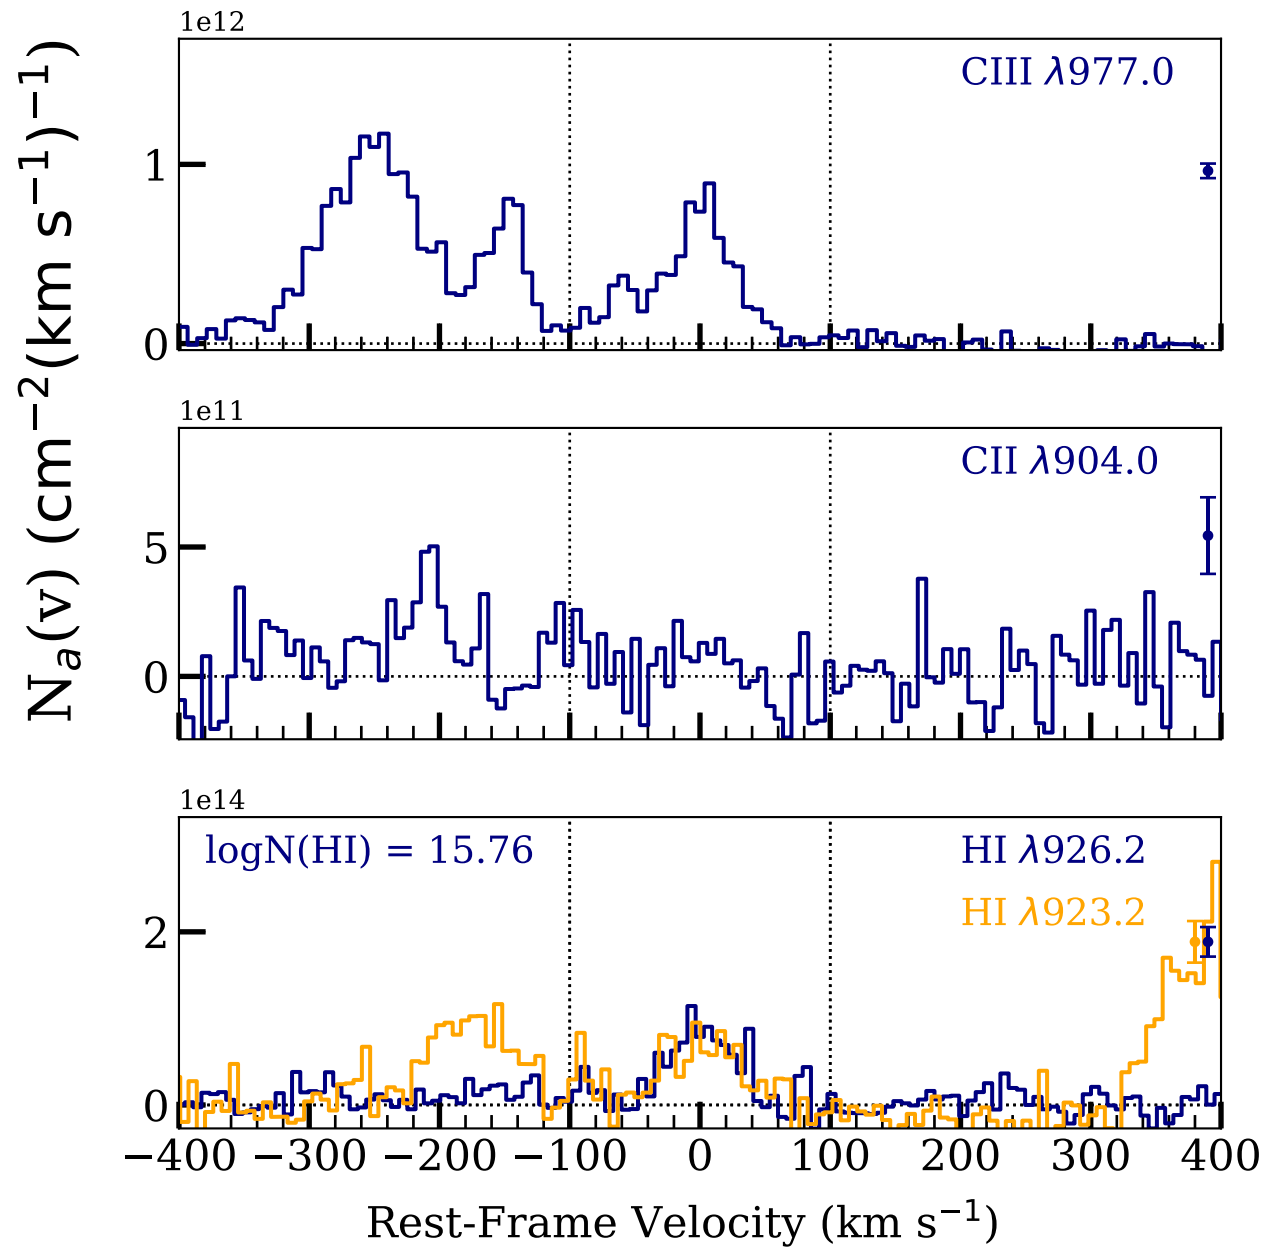



J011013.14-021952.8,  $z=0.718956$ , RF=0

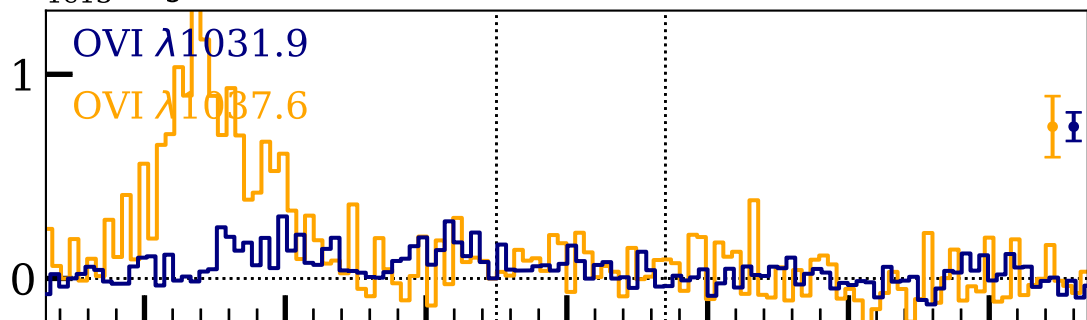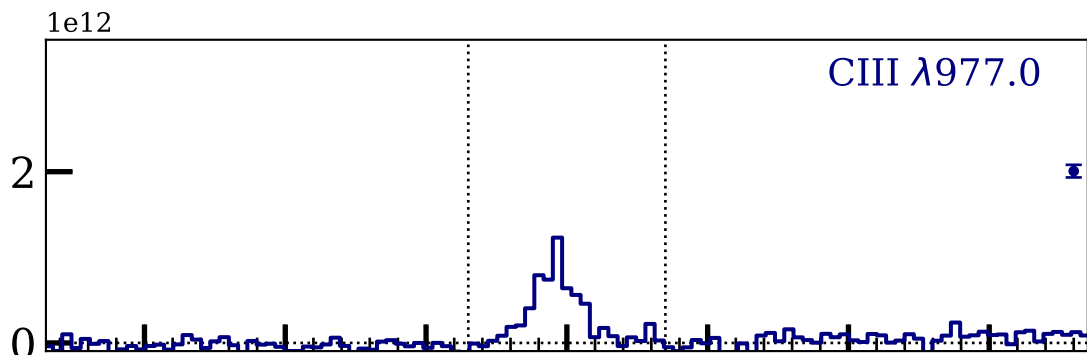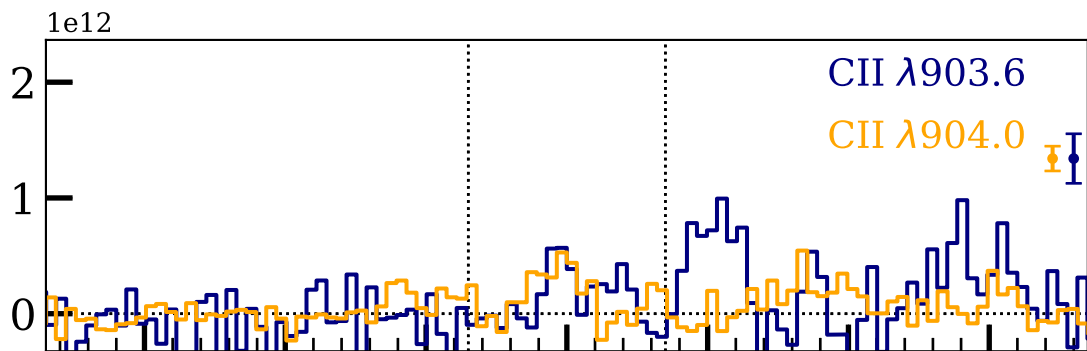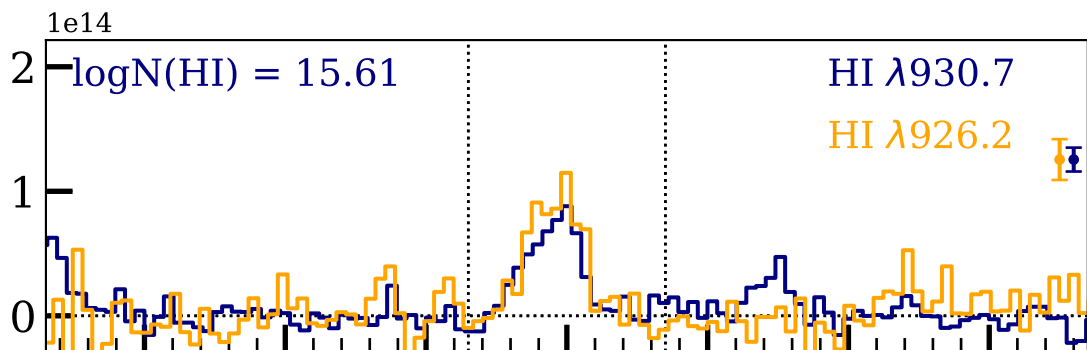

Rest-Frame Velocity ( $\text{km s}^{-1}$ )

J011016.25-021851.0, z=0.399146, RF=1

$N_a(v)$  ( $\text{cm}^{-2}(\text{km s}^{-1})^{-1}$ )

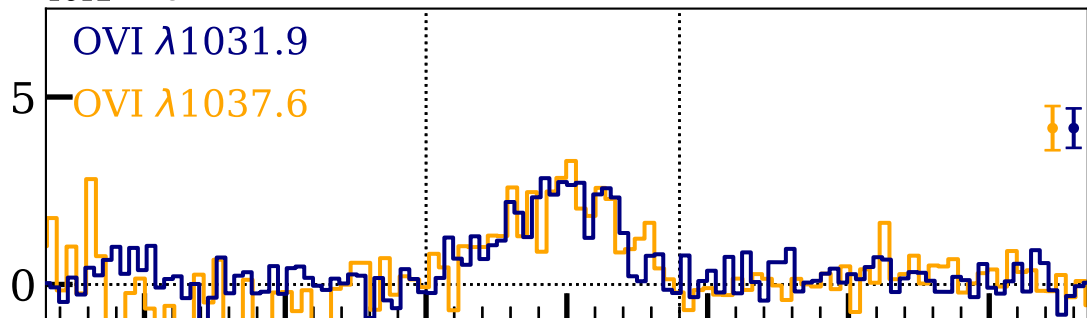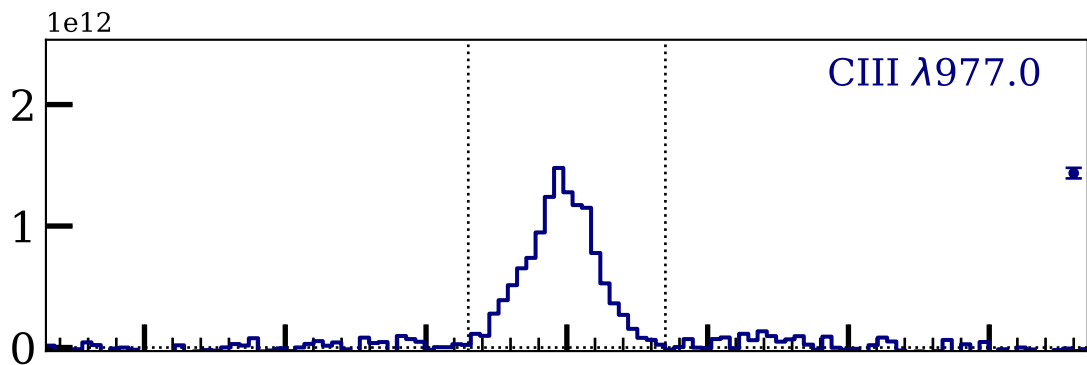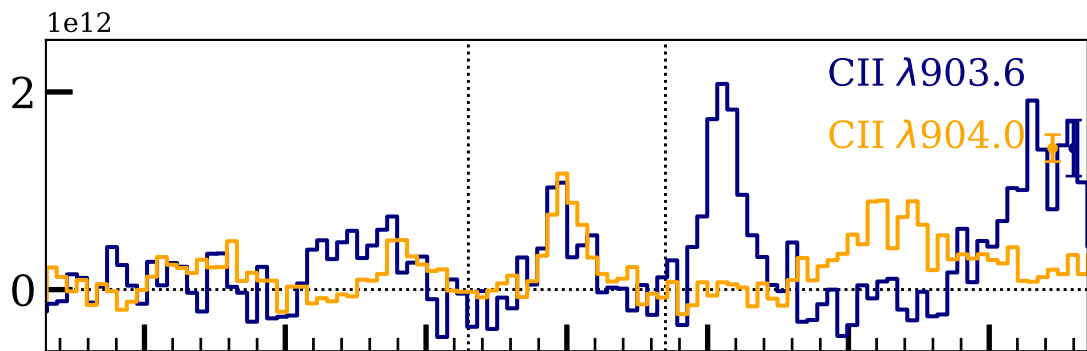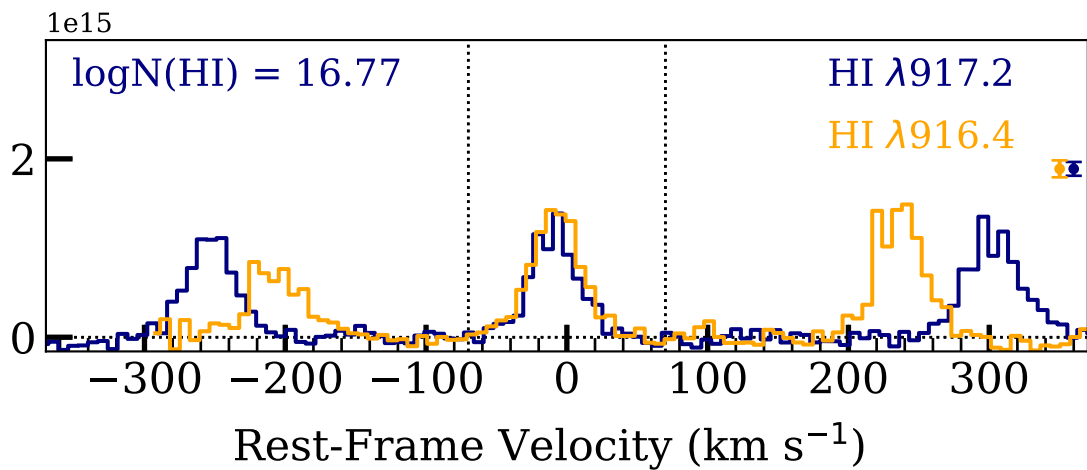

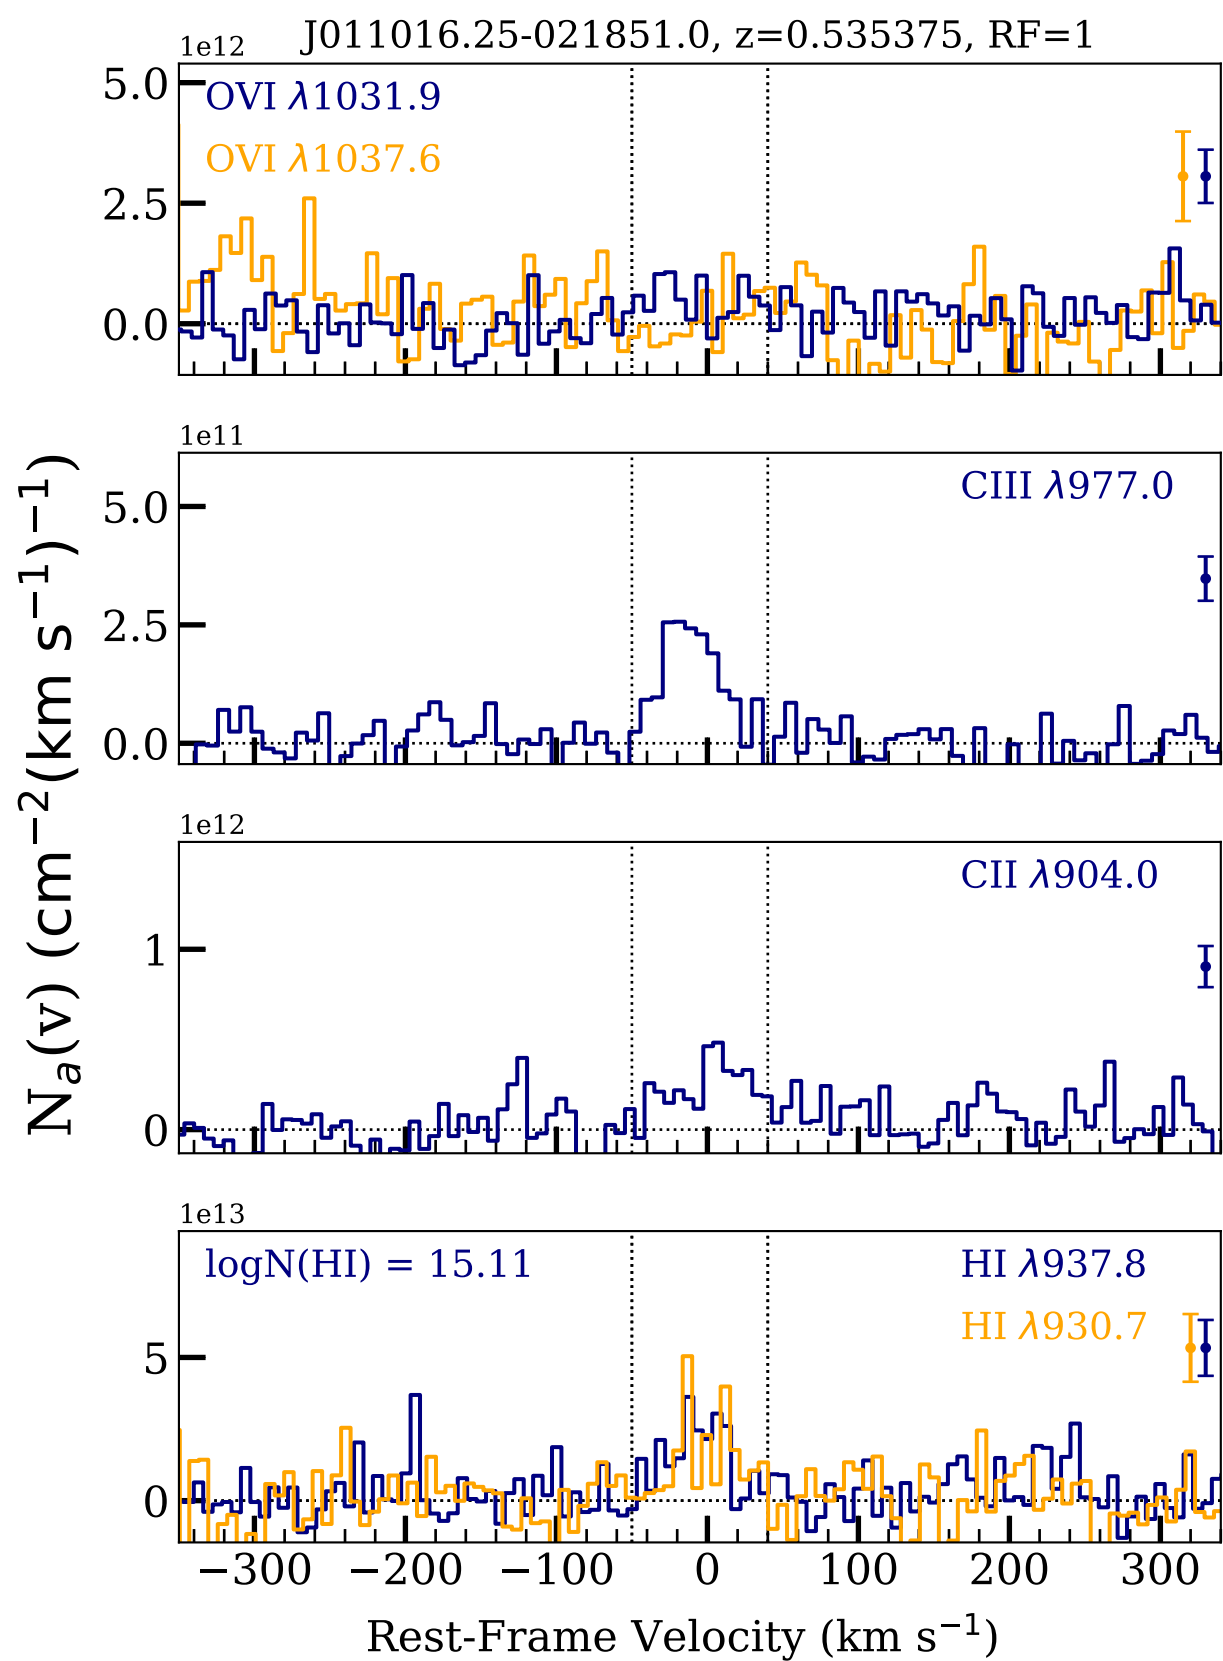

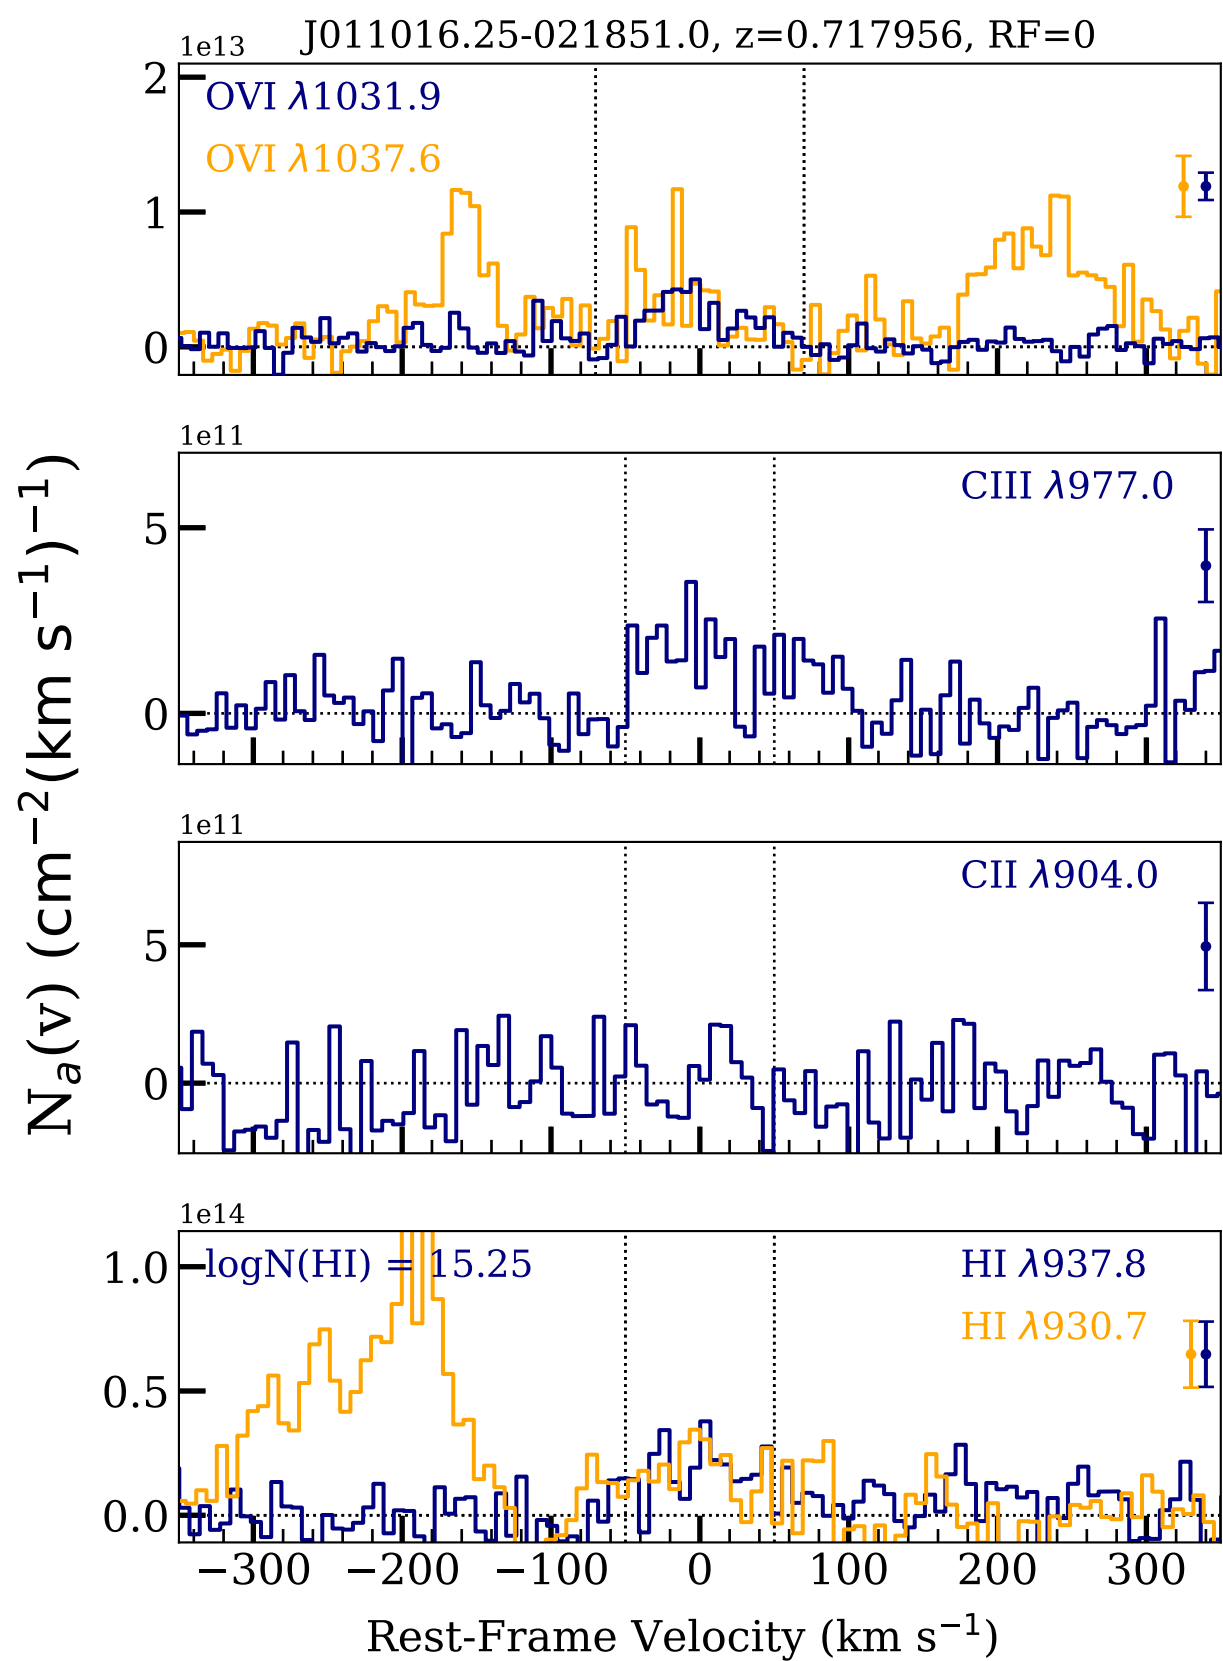

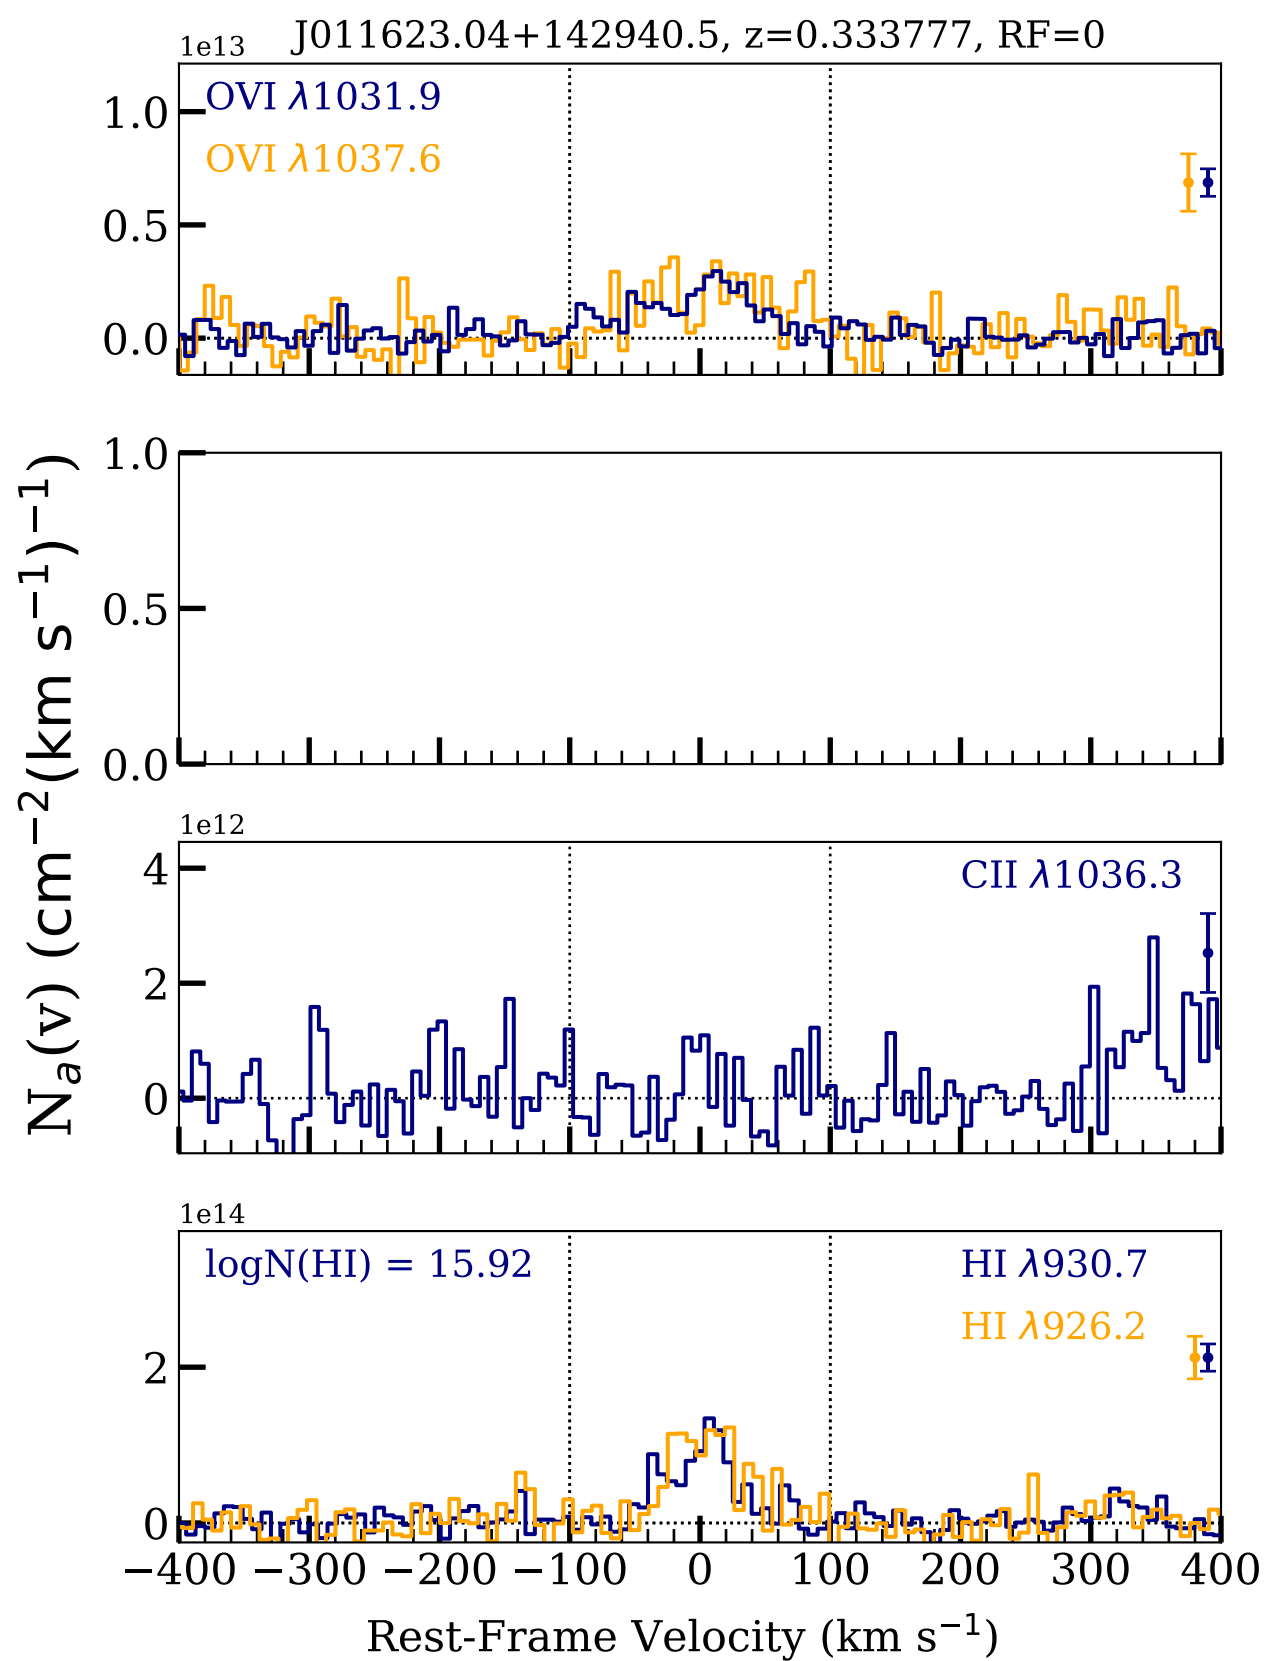

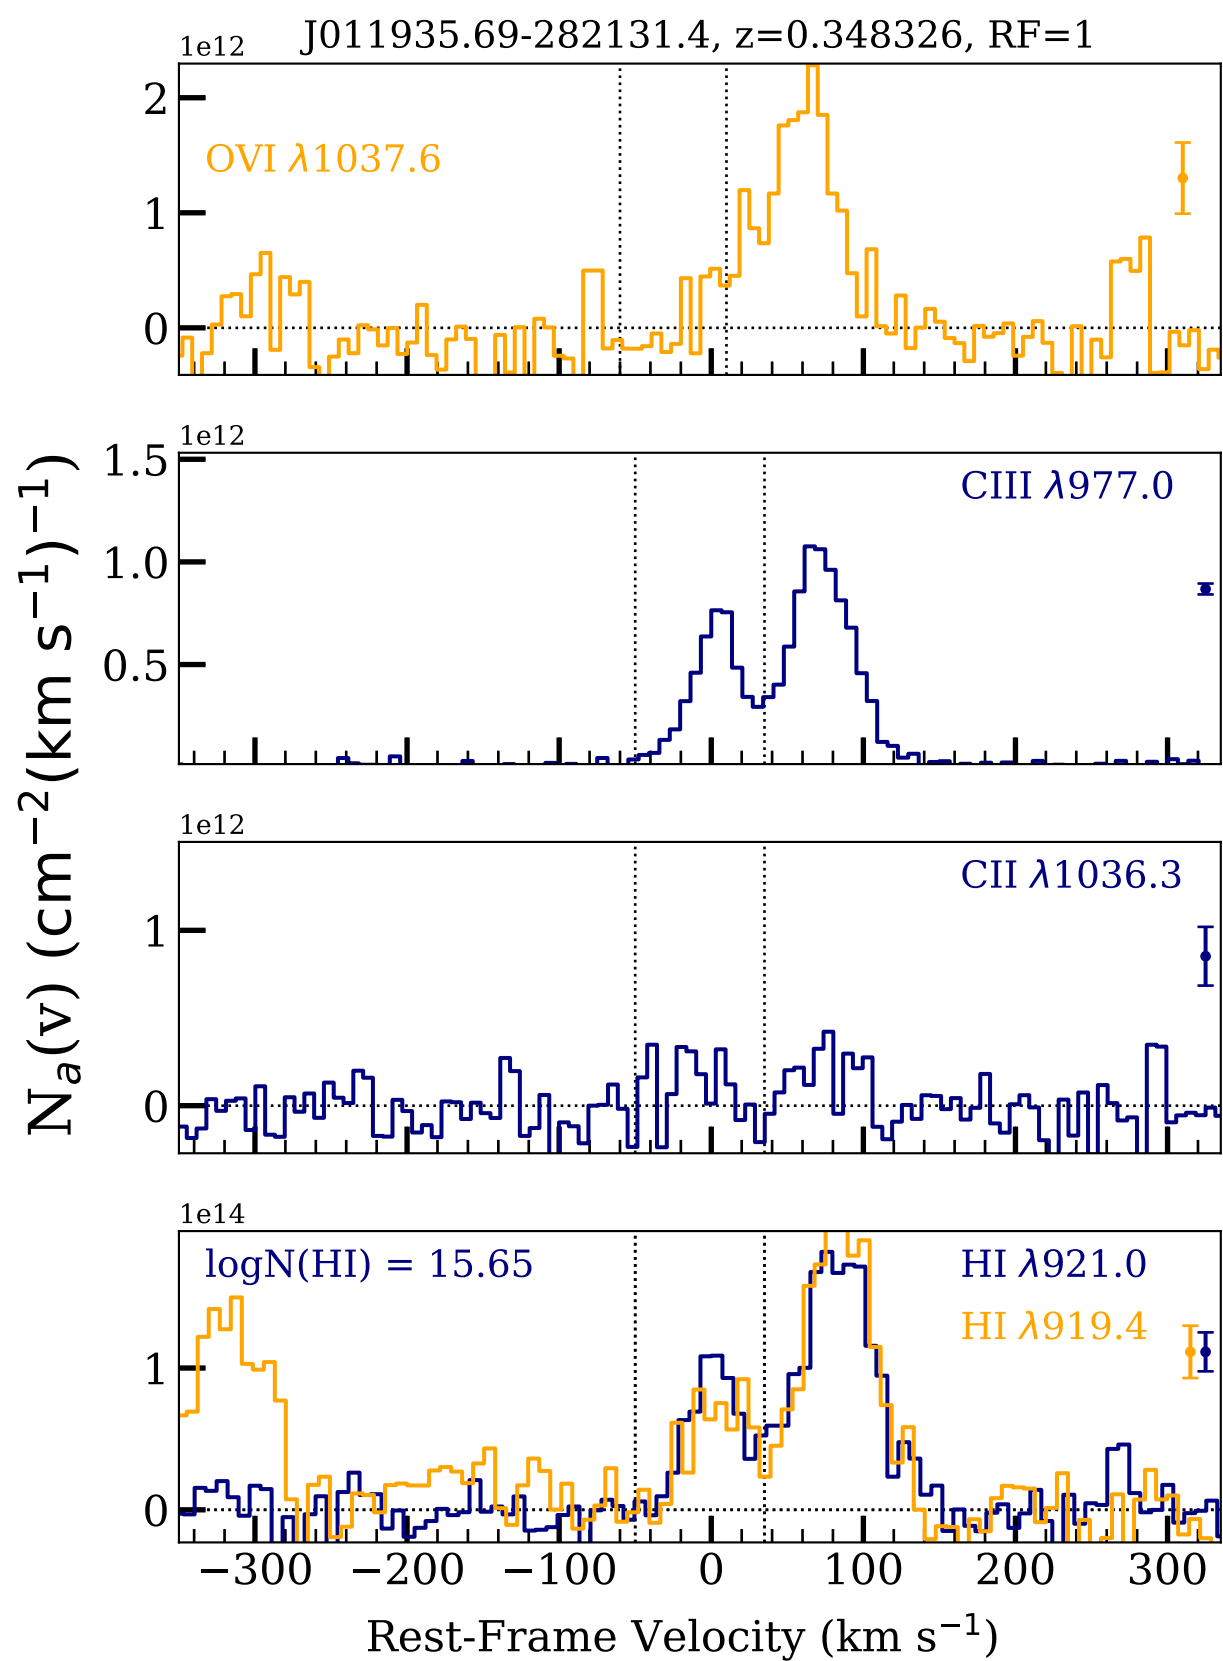

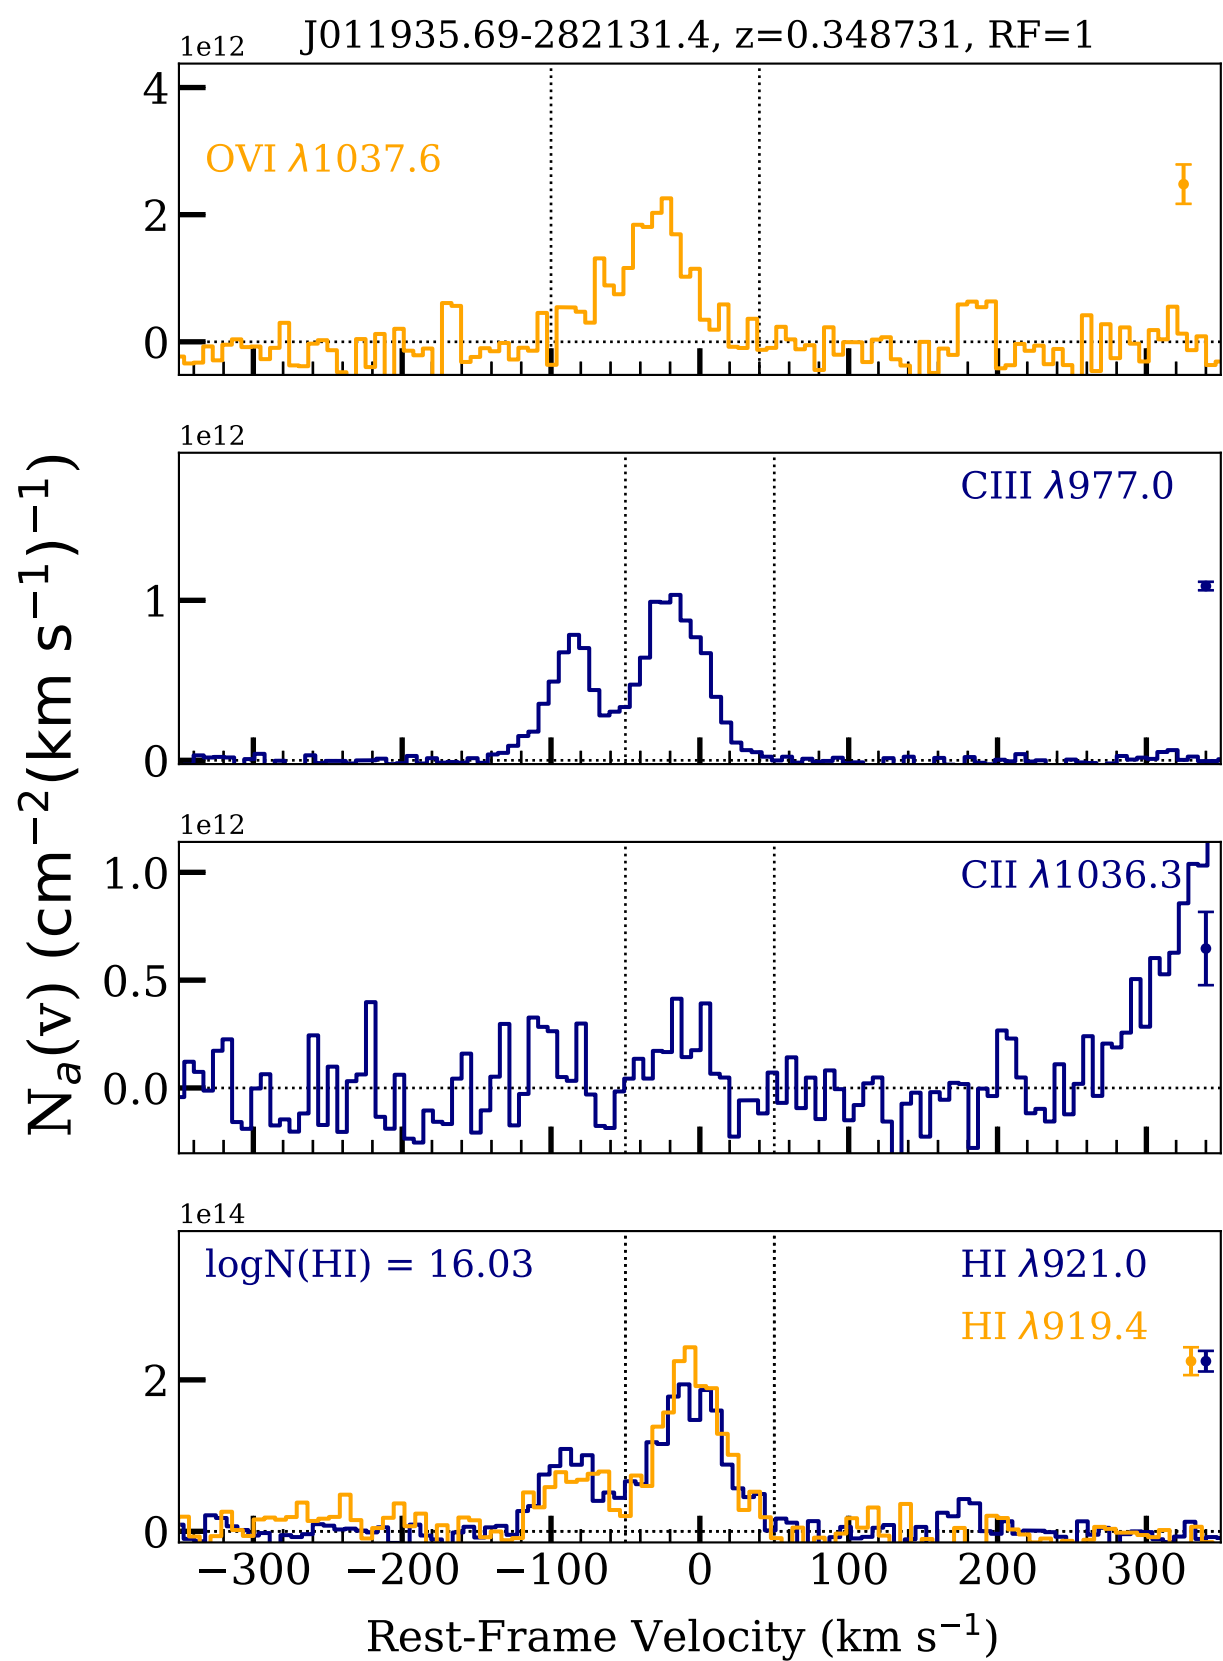

J012236.76-284321.3,  $z=0.364959$ , RF=1

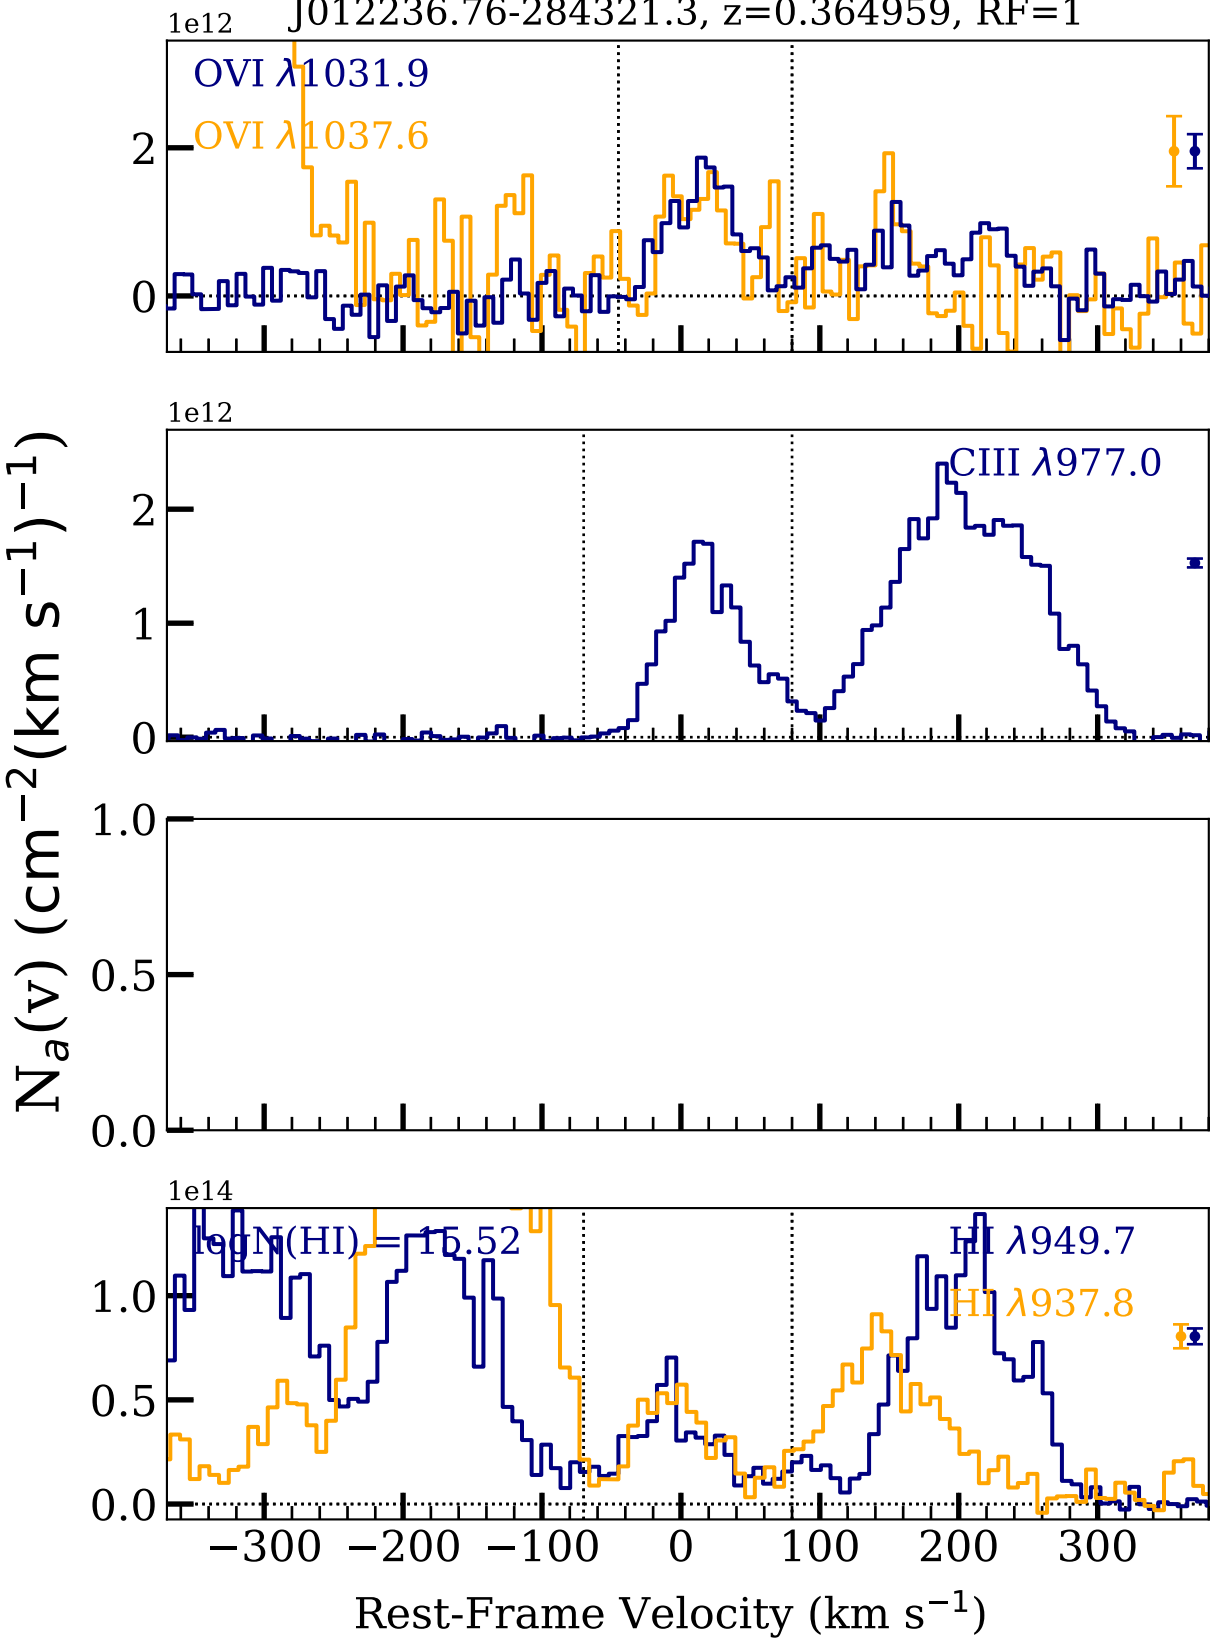



J015513.20-450611.9,  $z=0.225958$ , RF=1

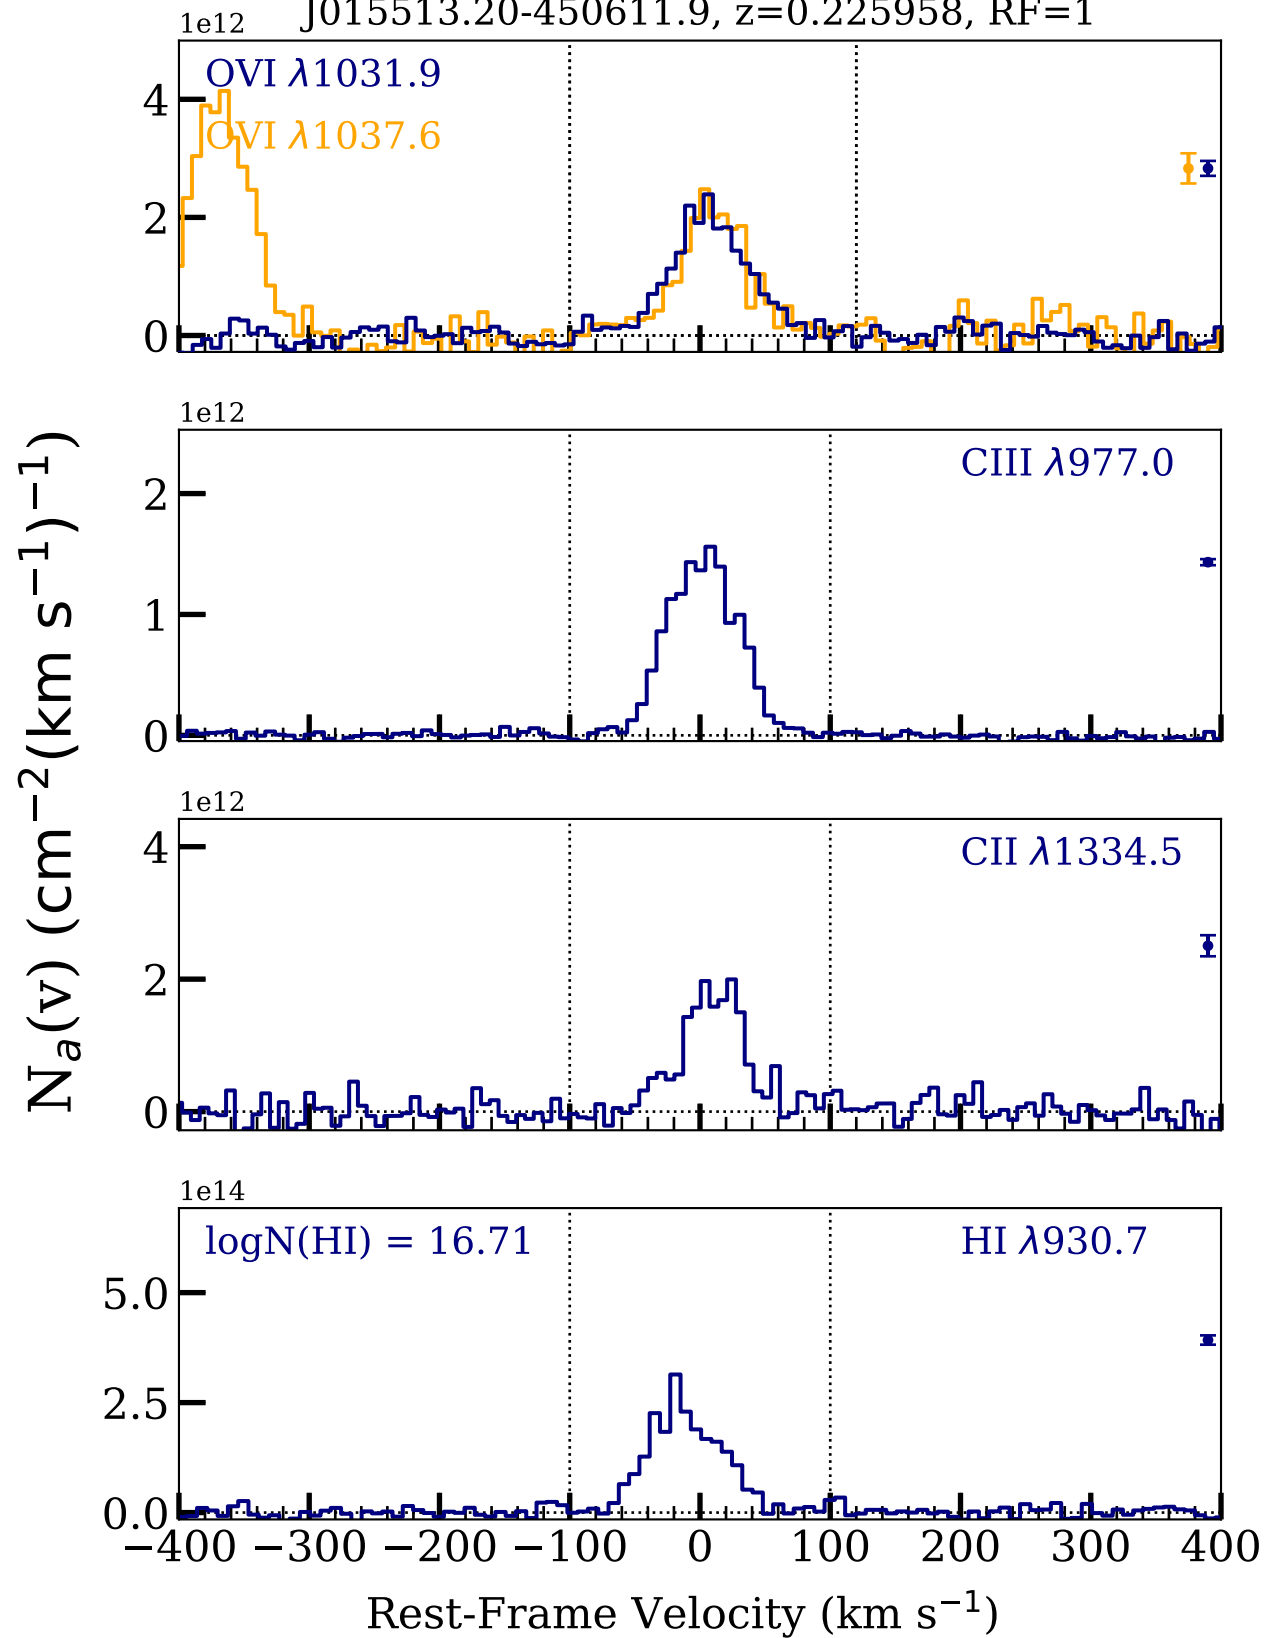

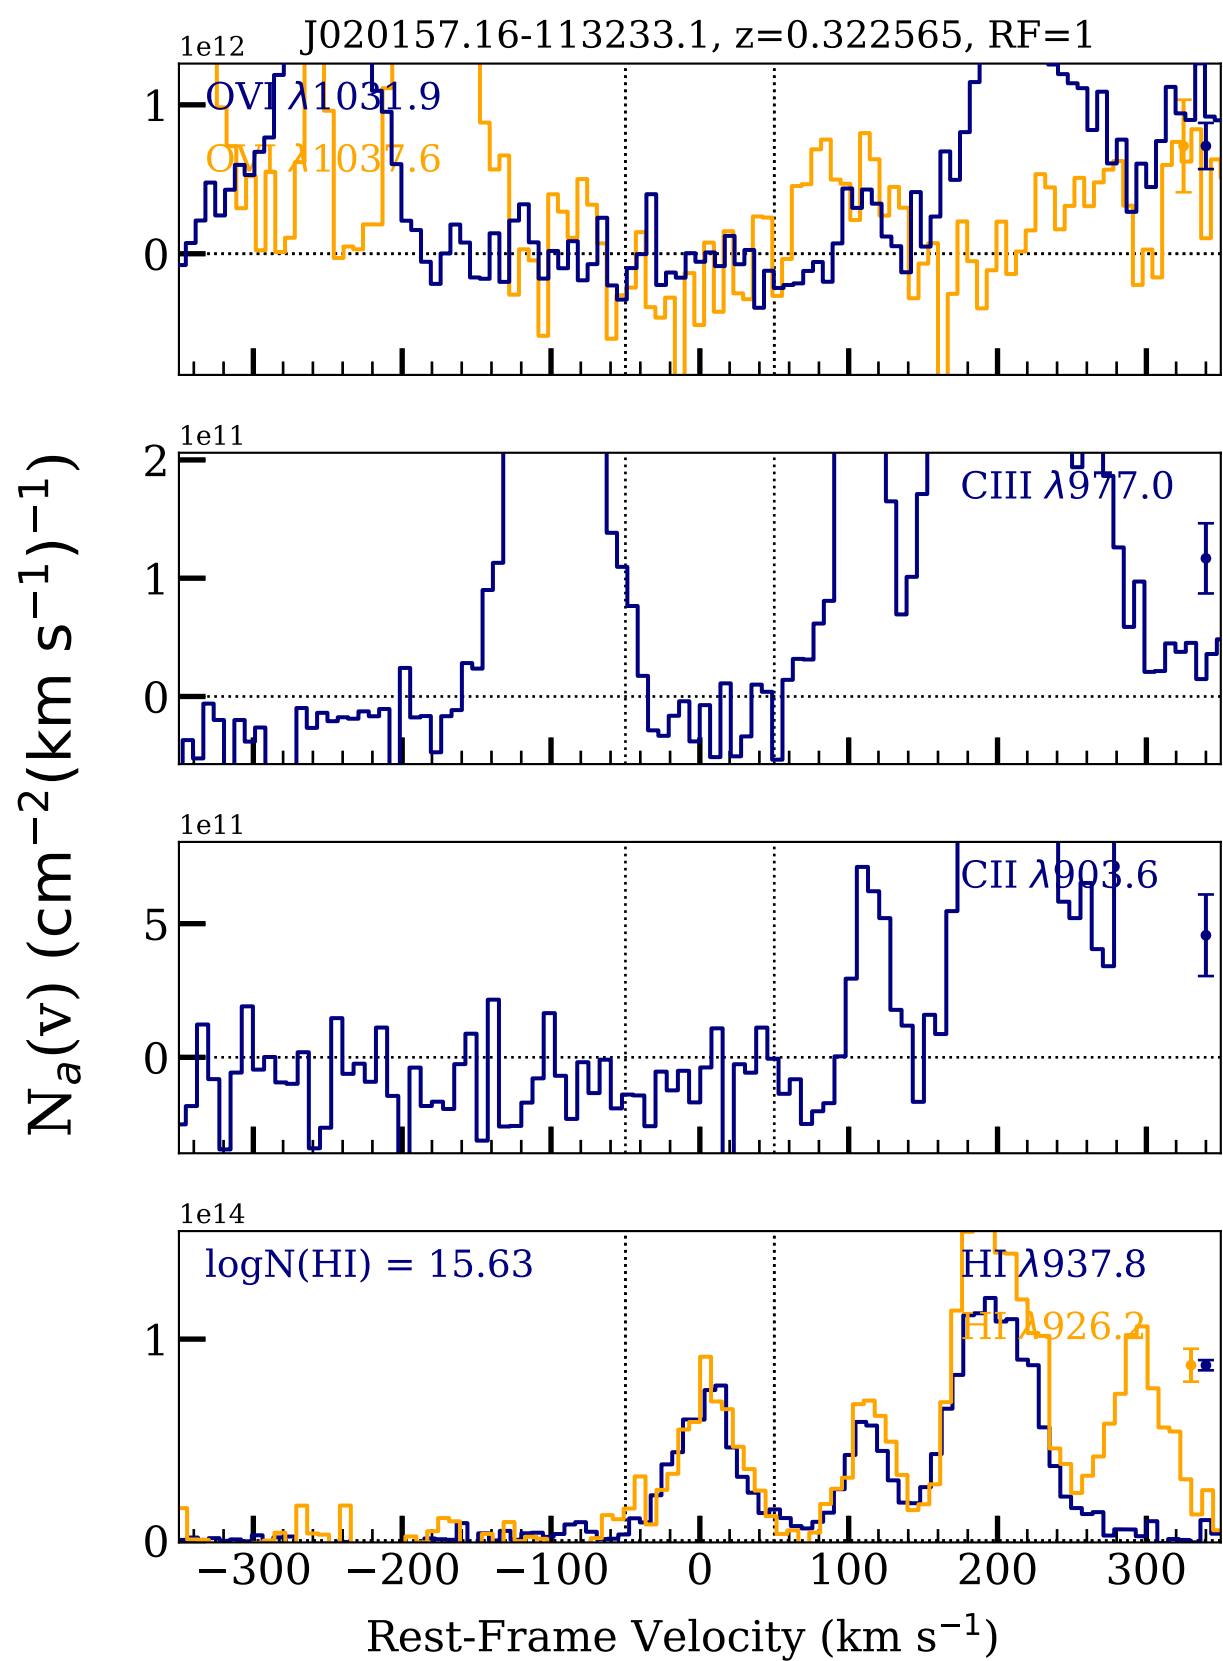

J020157.16-113233.1,  $z=0.323073$ , RF=1

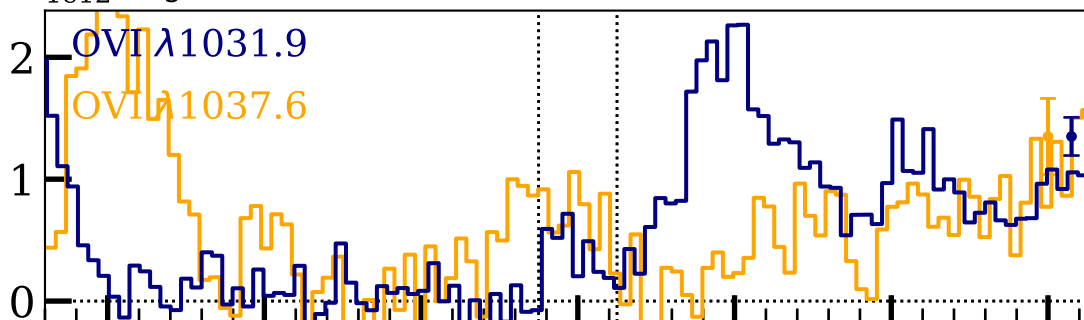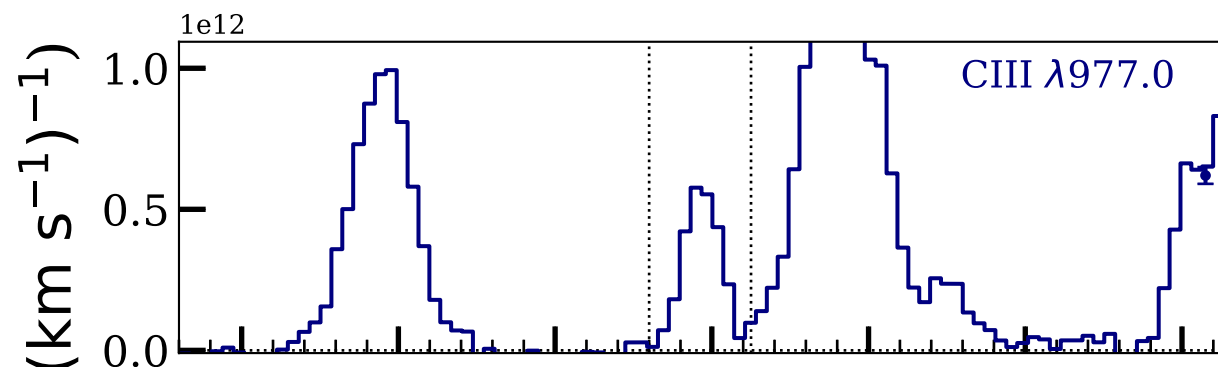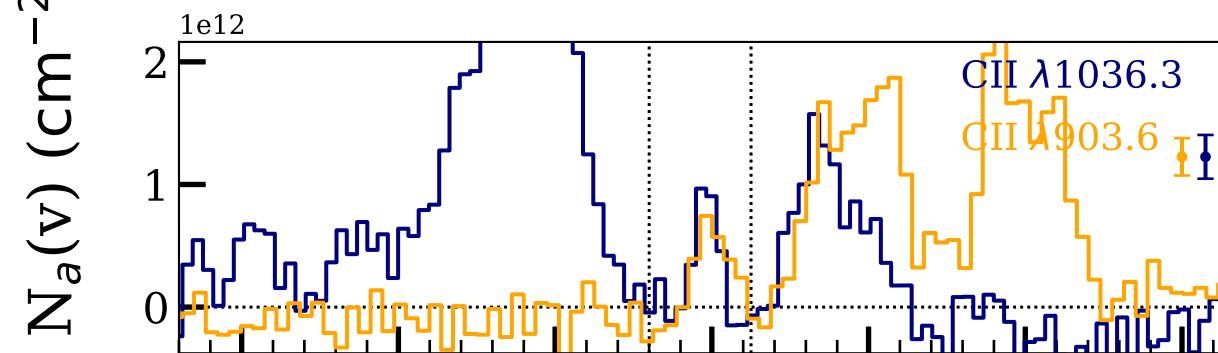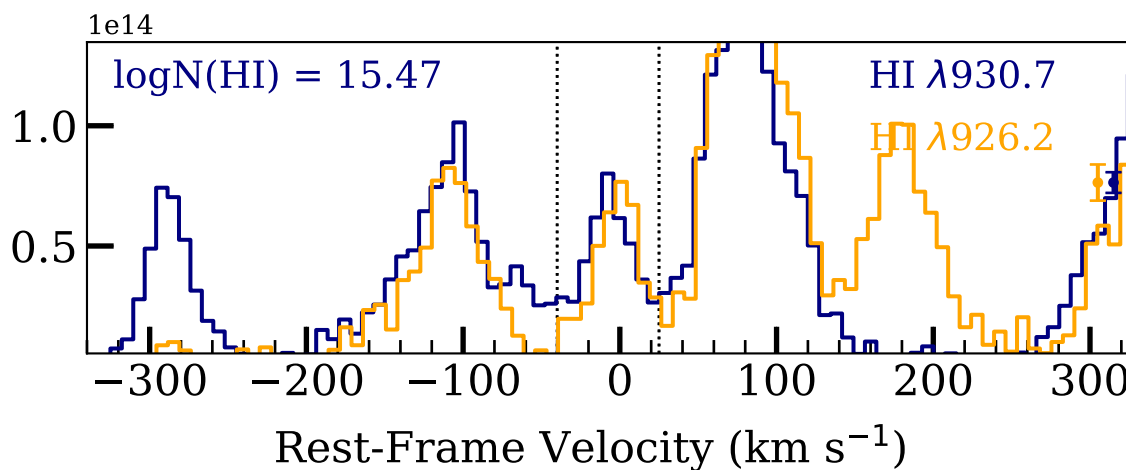

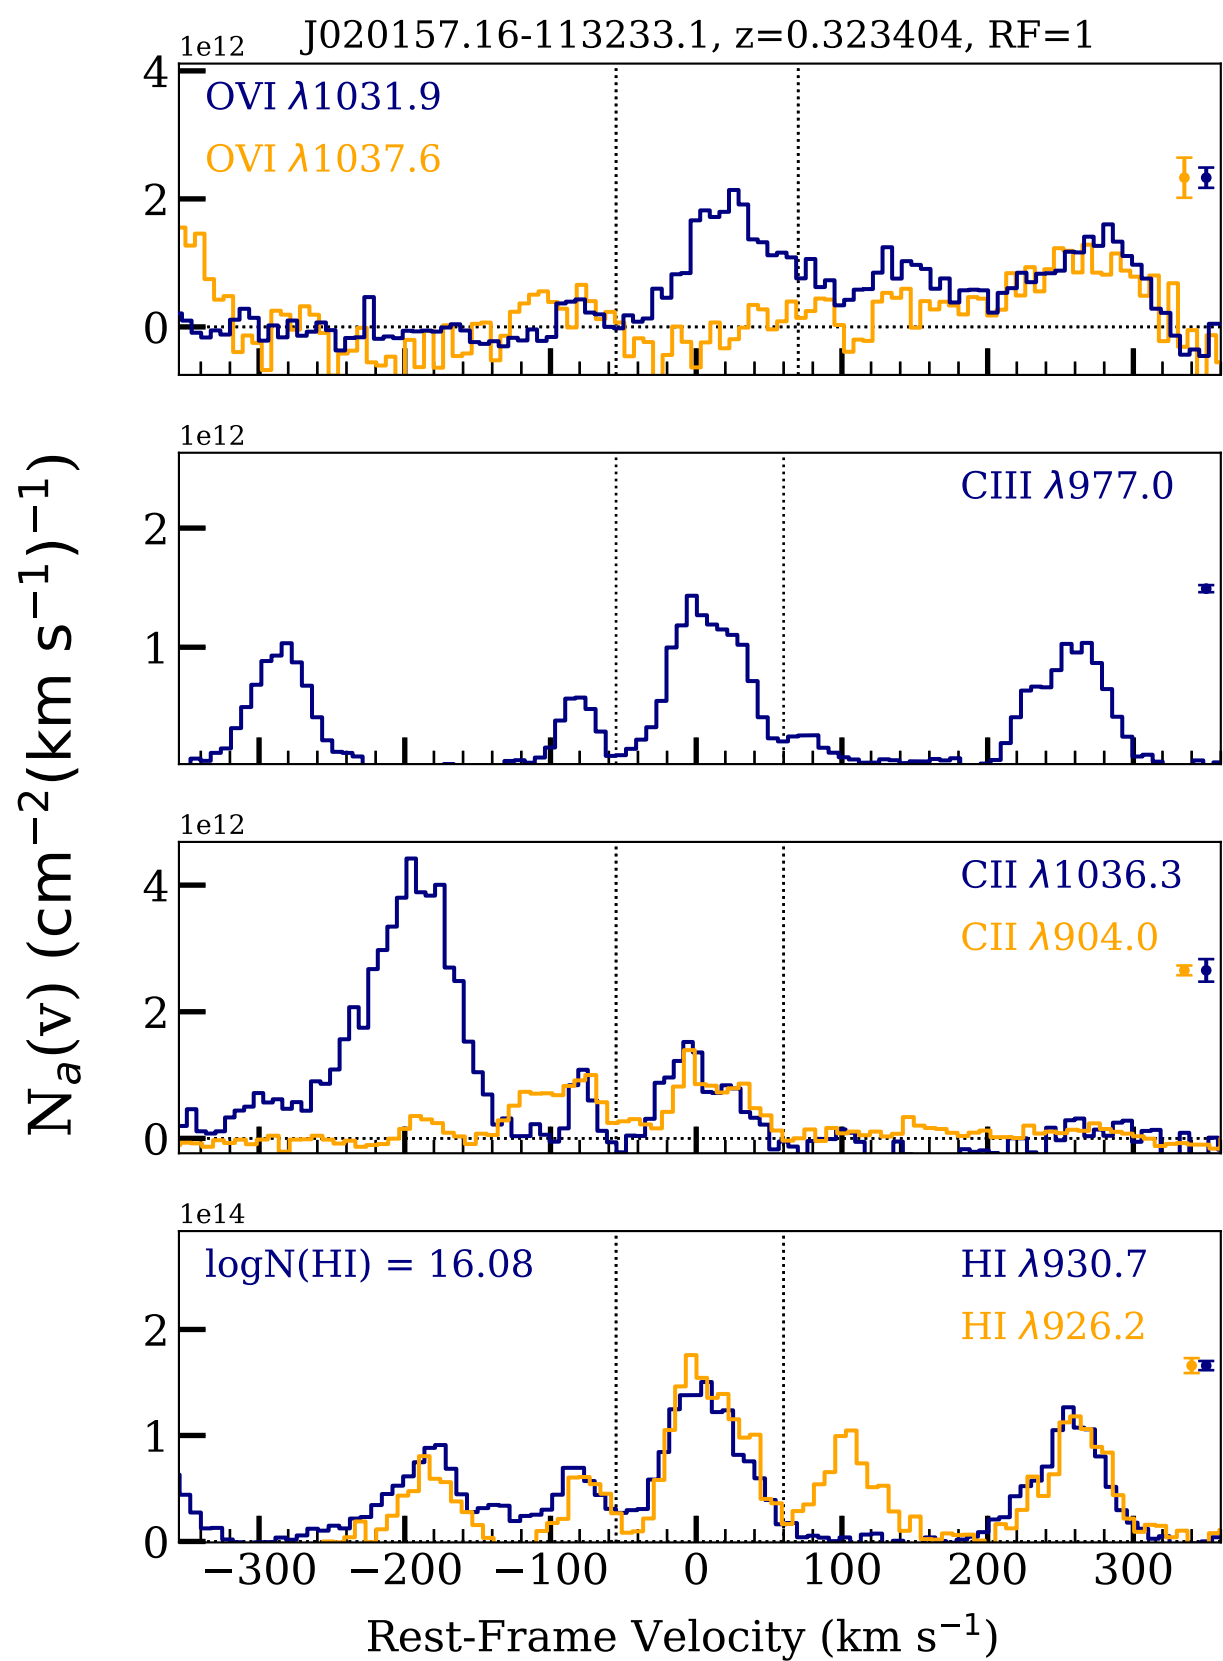

J020157.16-113233.1,  $z=0.324507$ , RF=1

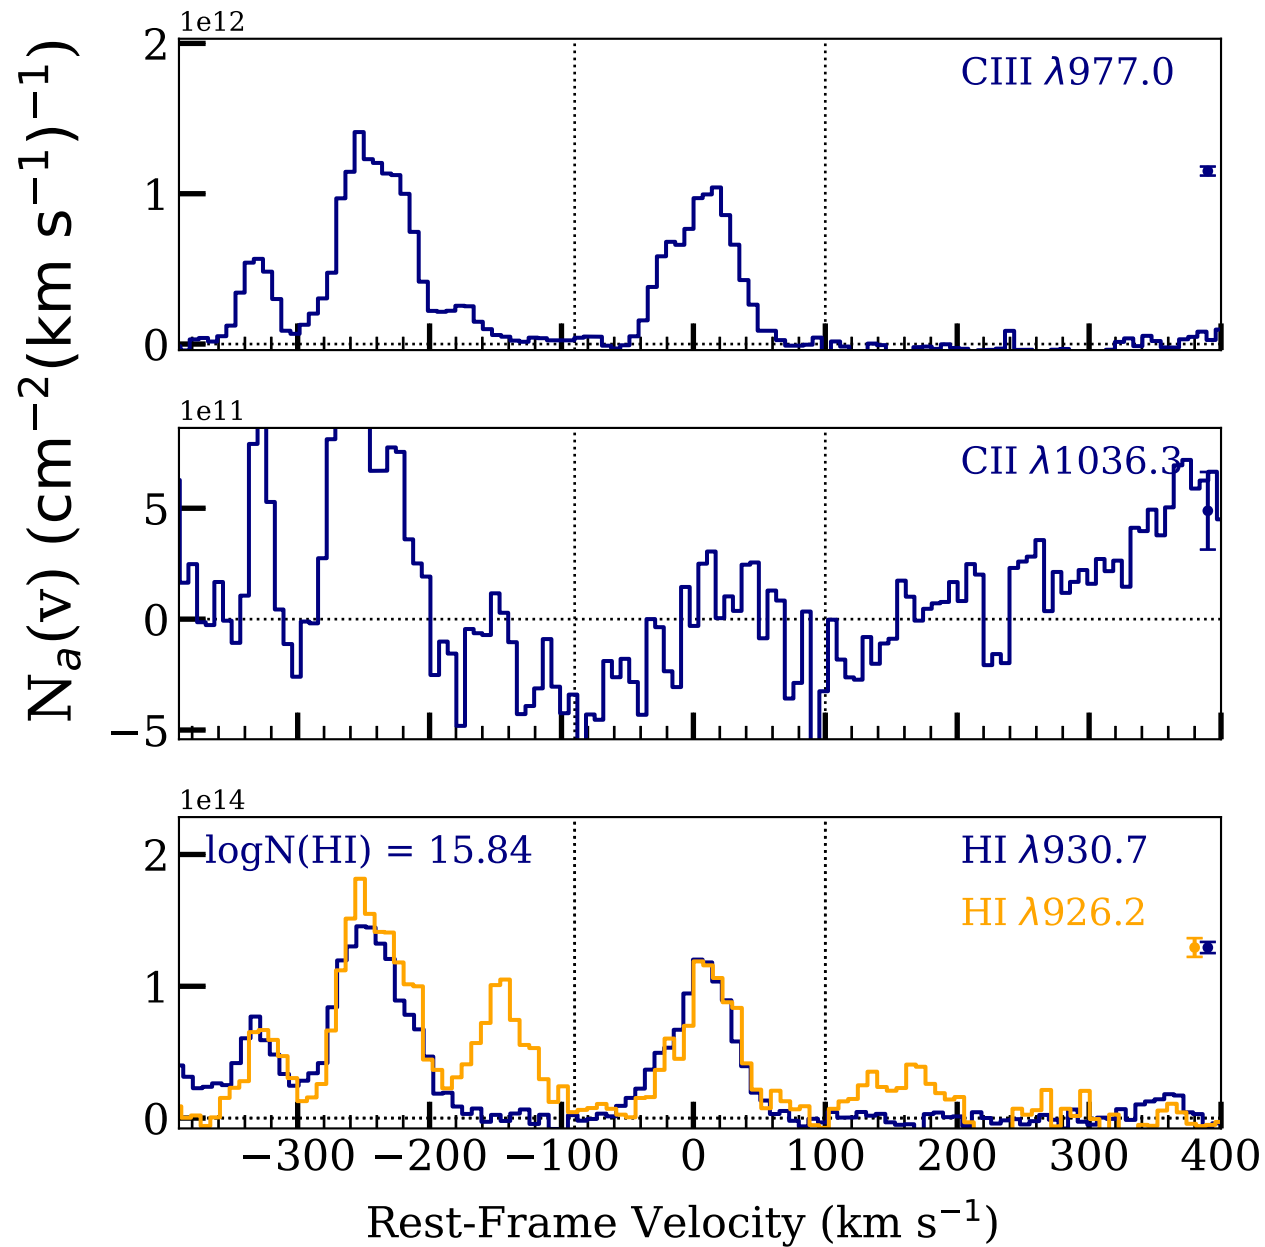

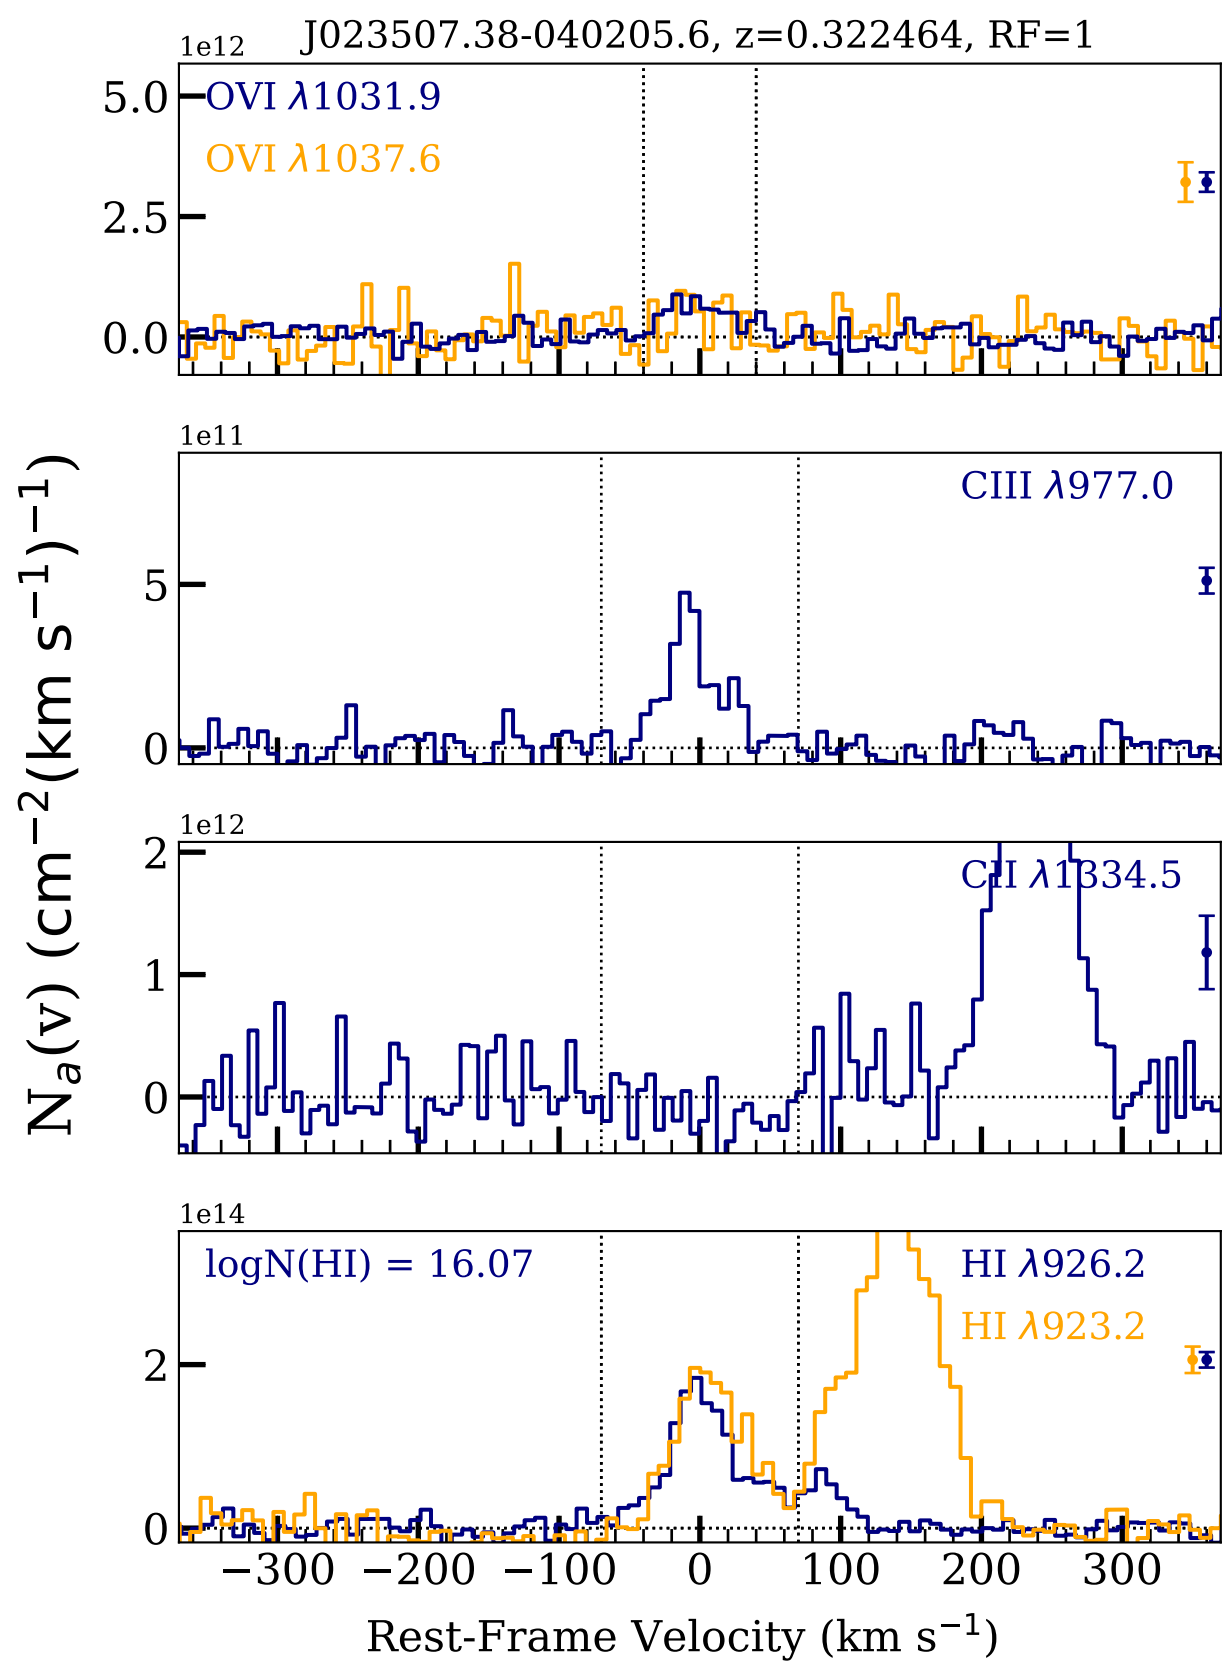

J023507.38-040205.6,  $z=0.738890$ , RF=0

$N_a(v)$  ( $\text{cm}^{-2}(\text{km s}^{-1})^{-1}$ )

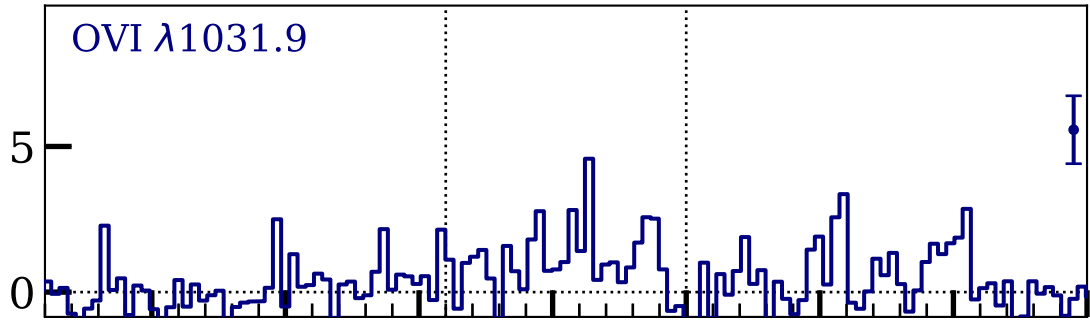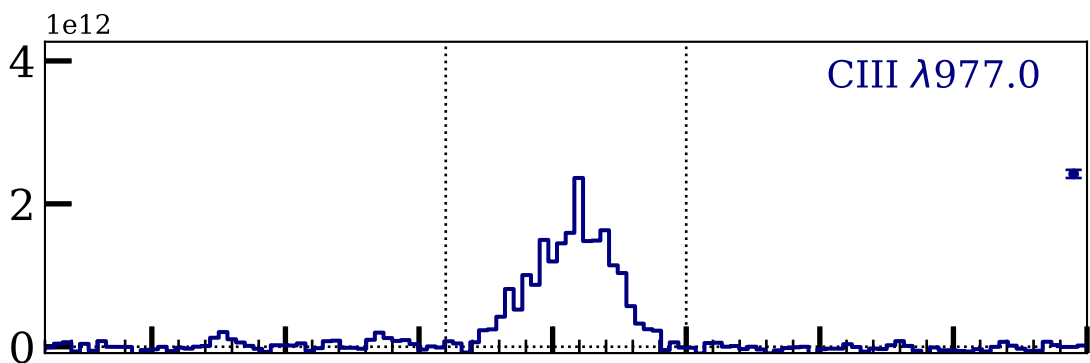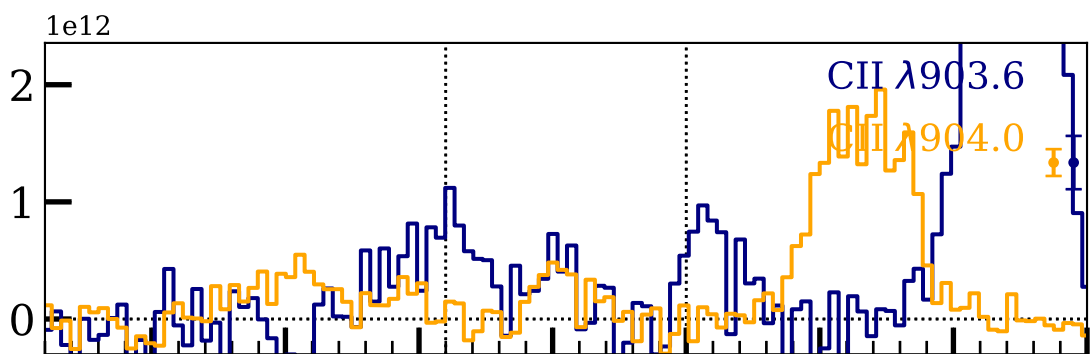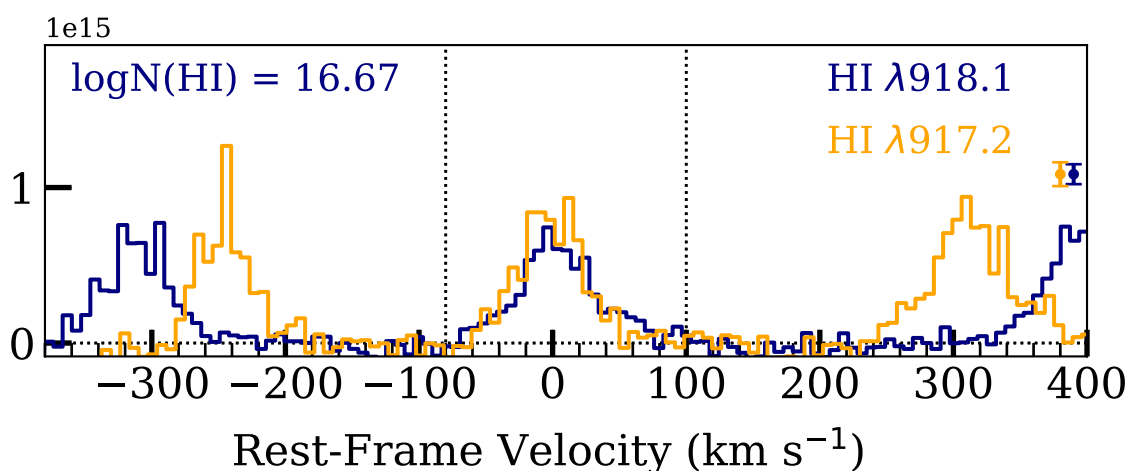

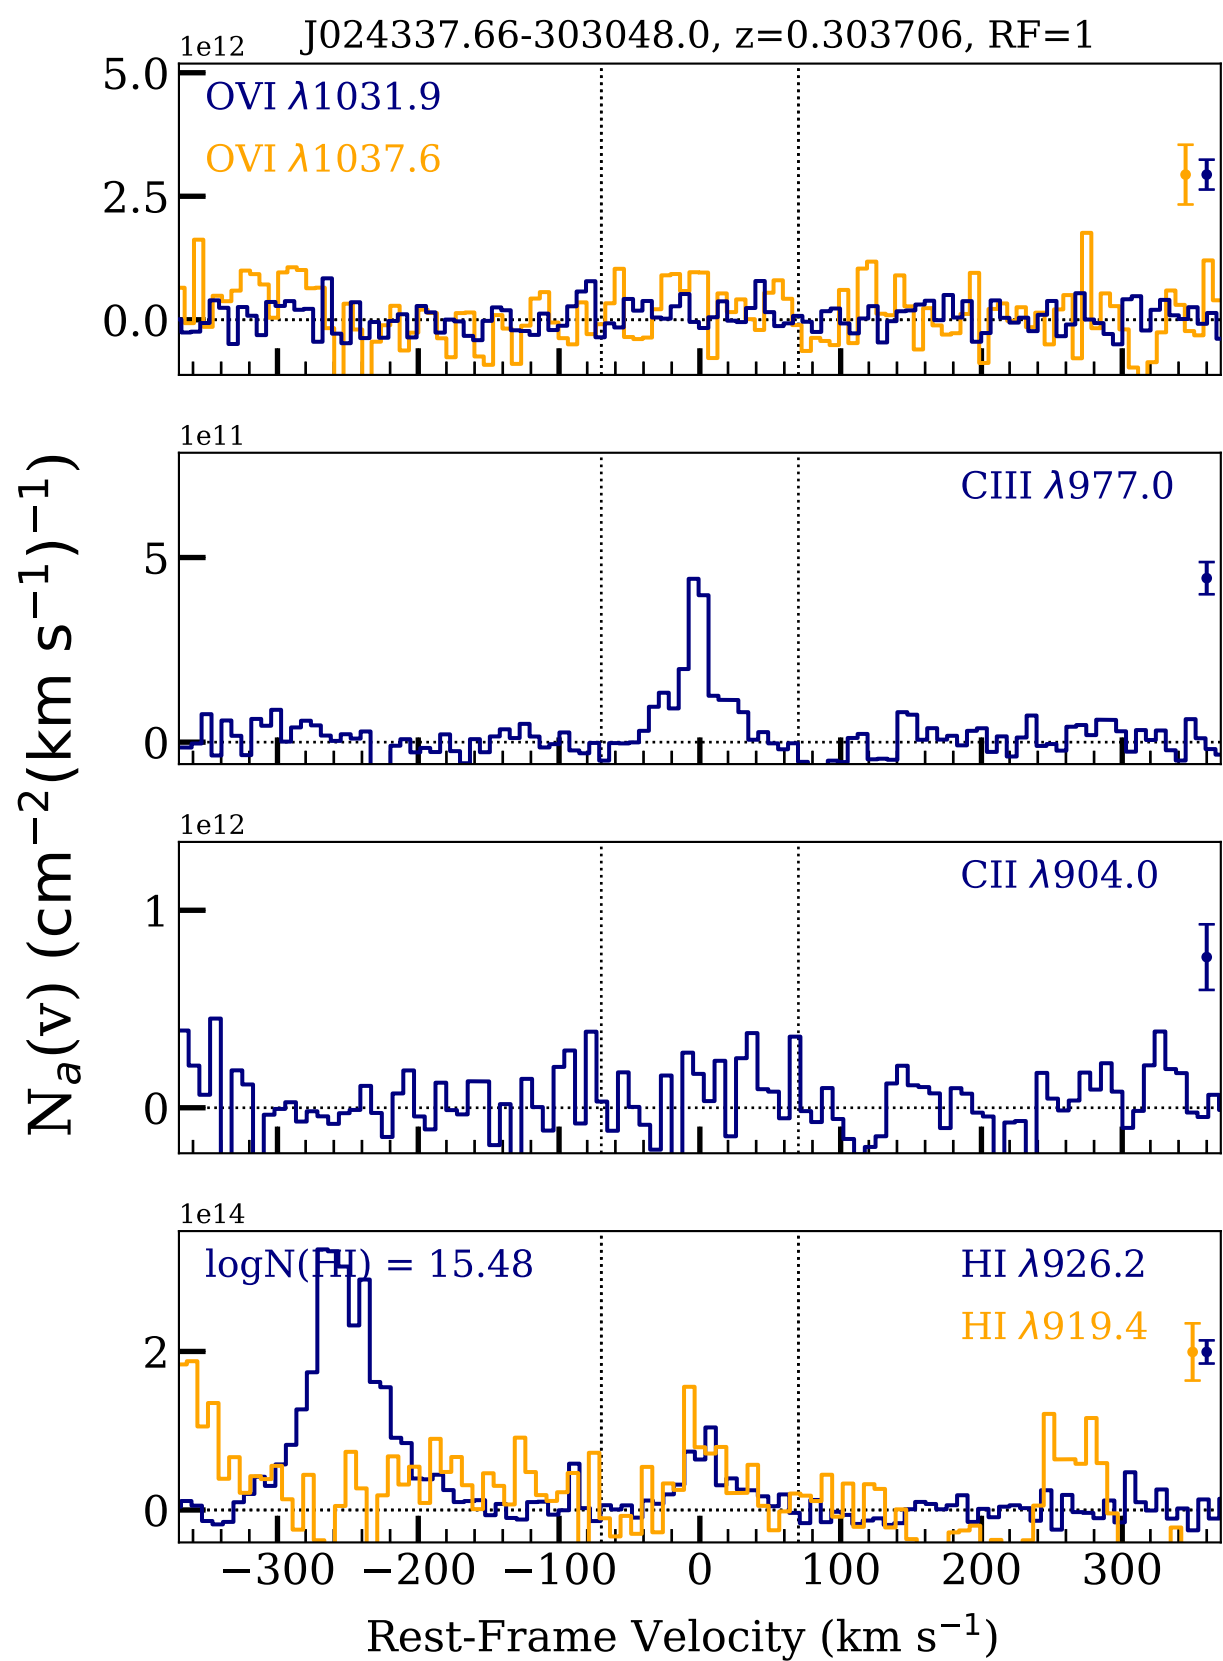



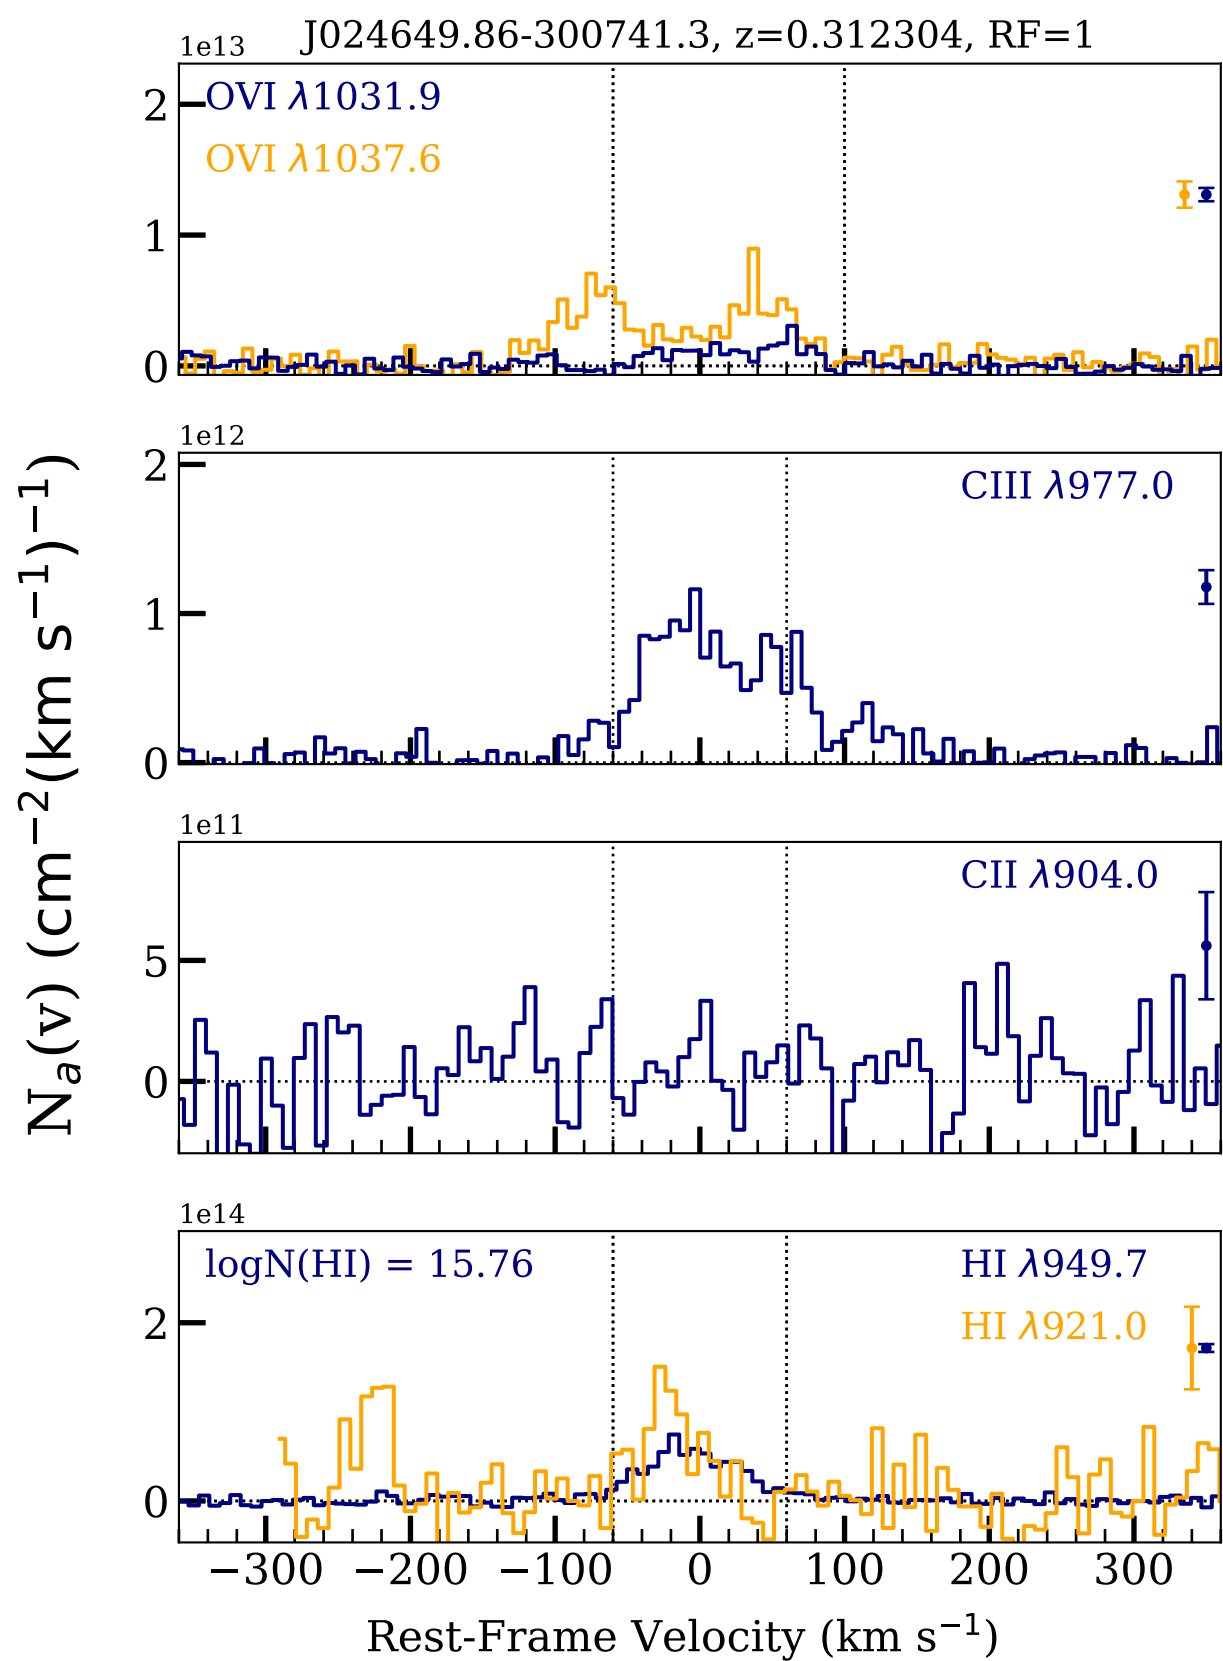

1e12 J024649.86-300741.3, z=0.335895, RF=1

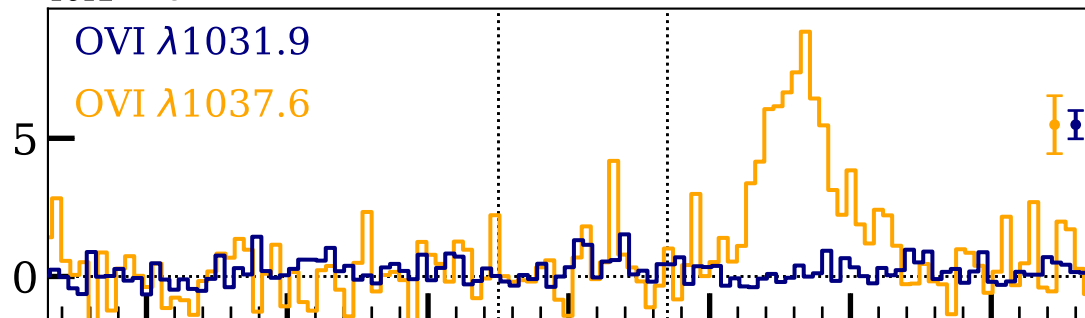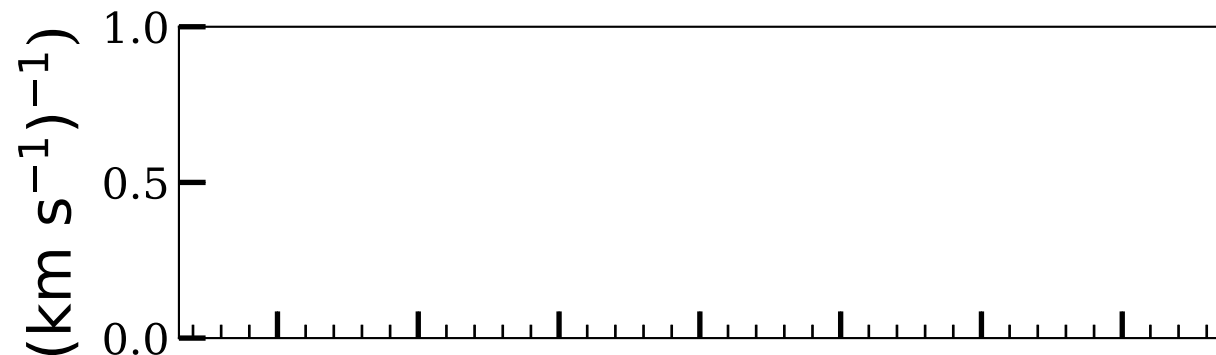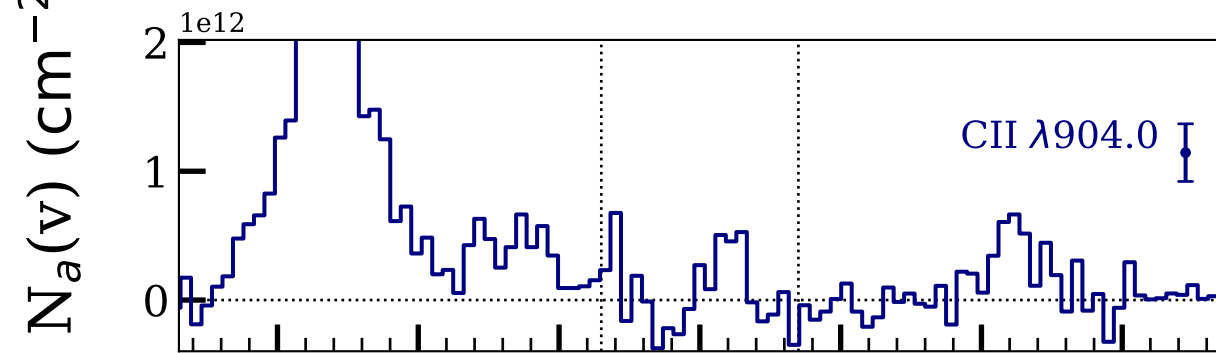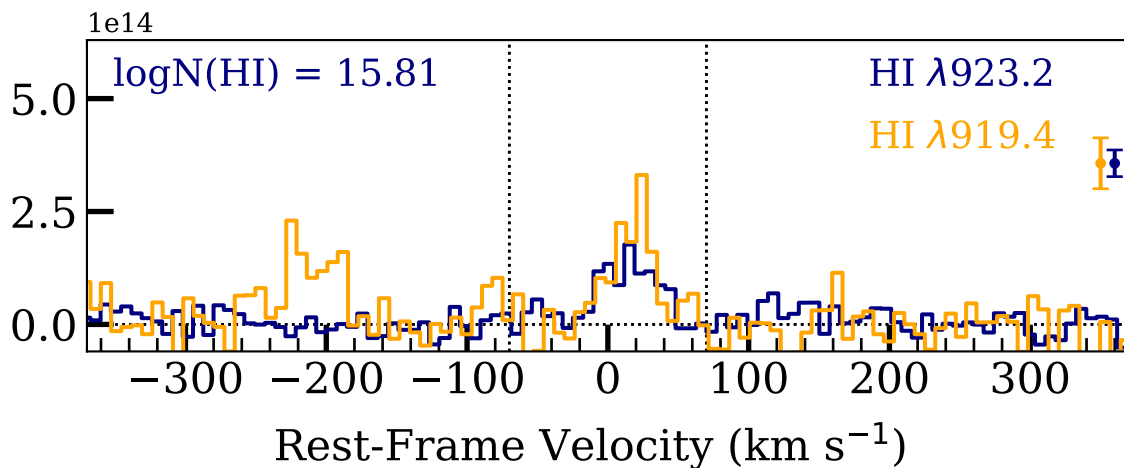

J035128.56-142908.0,  $z=0.328476$ , RF=1

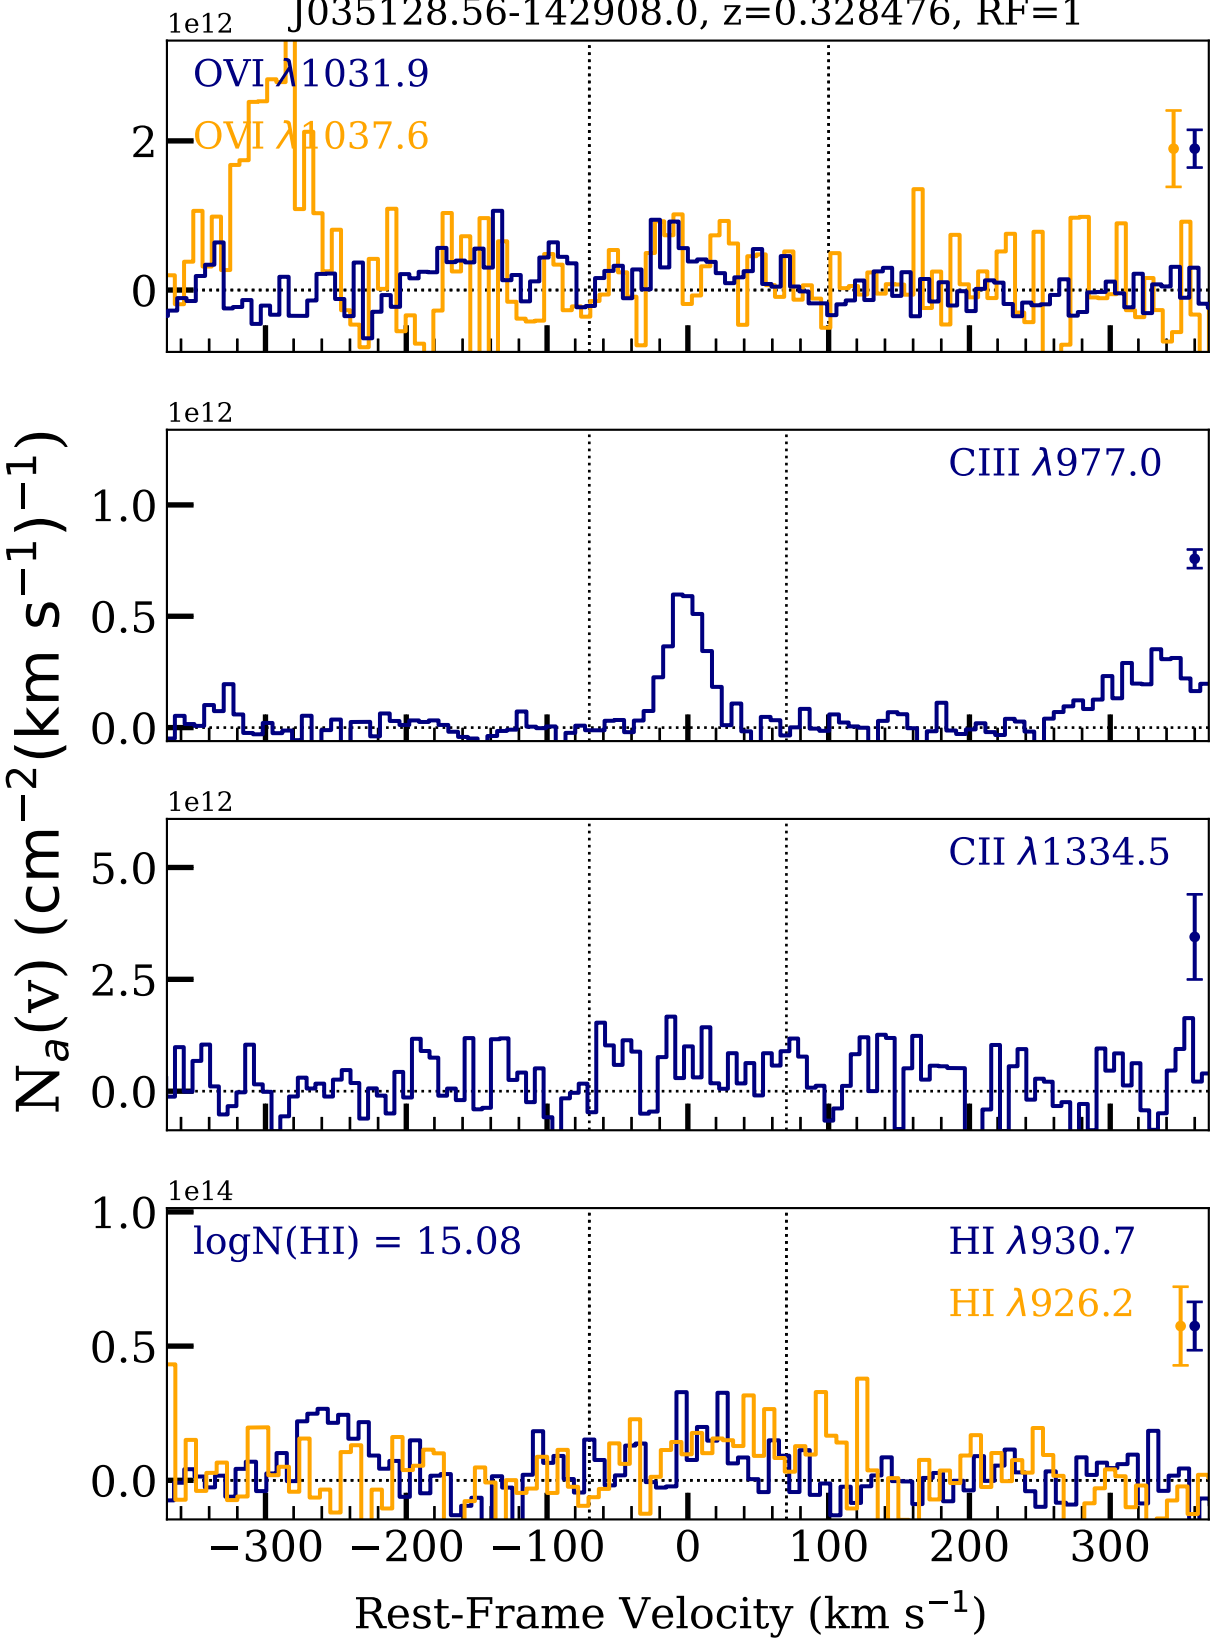

J035128.56-142908.0,  $z=0.356924$ , RF=1

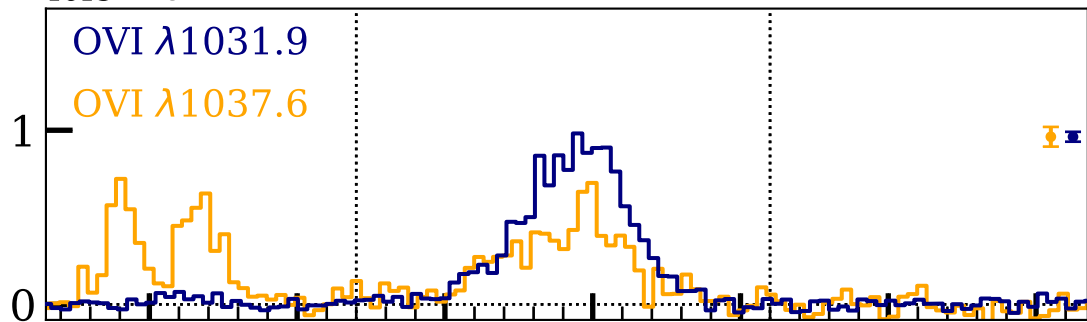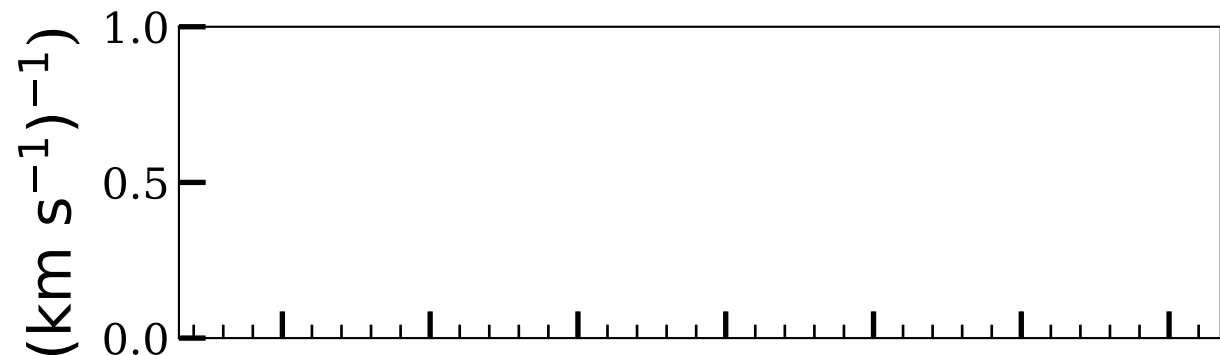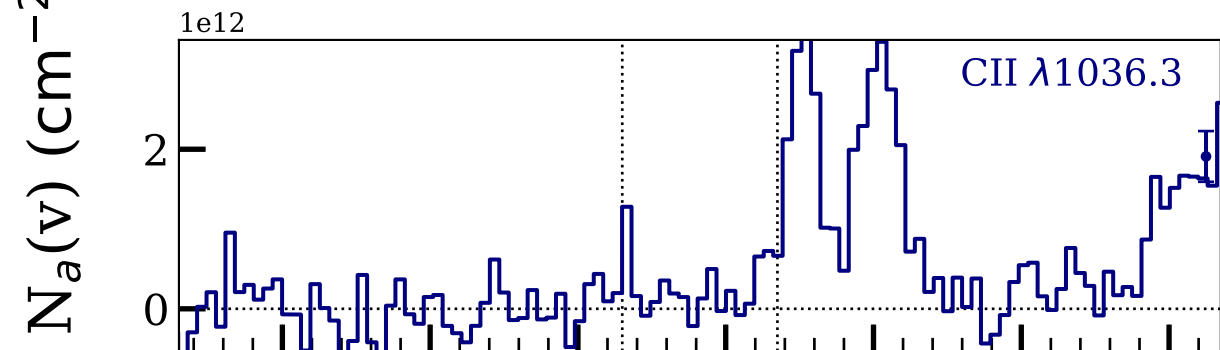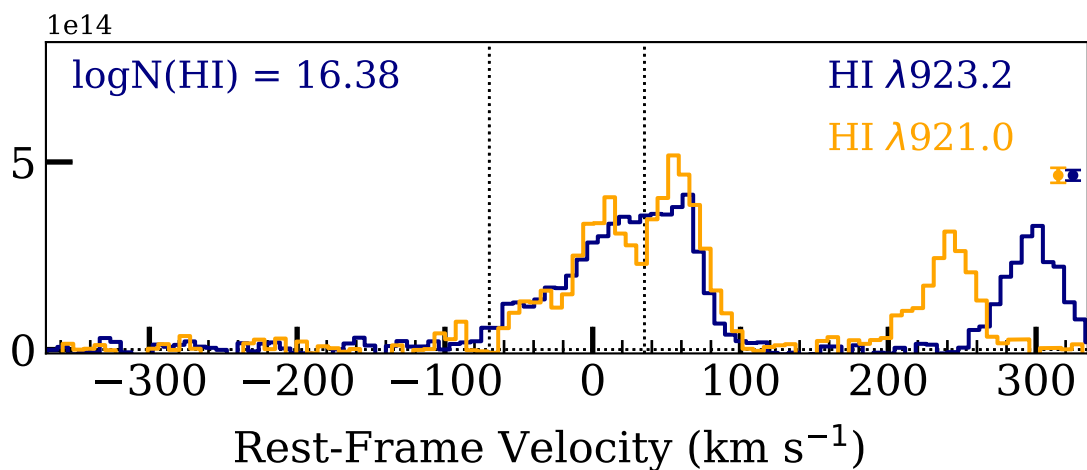

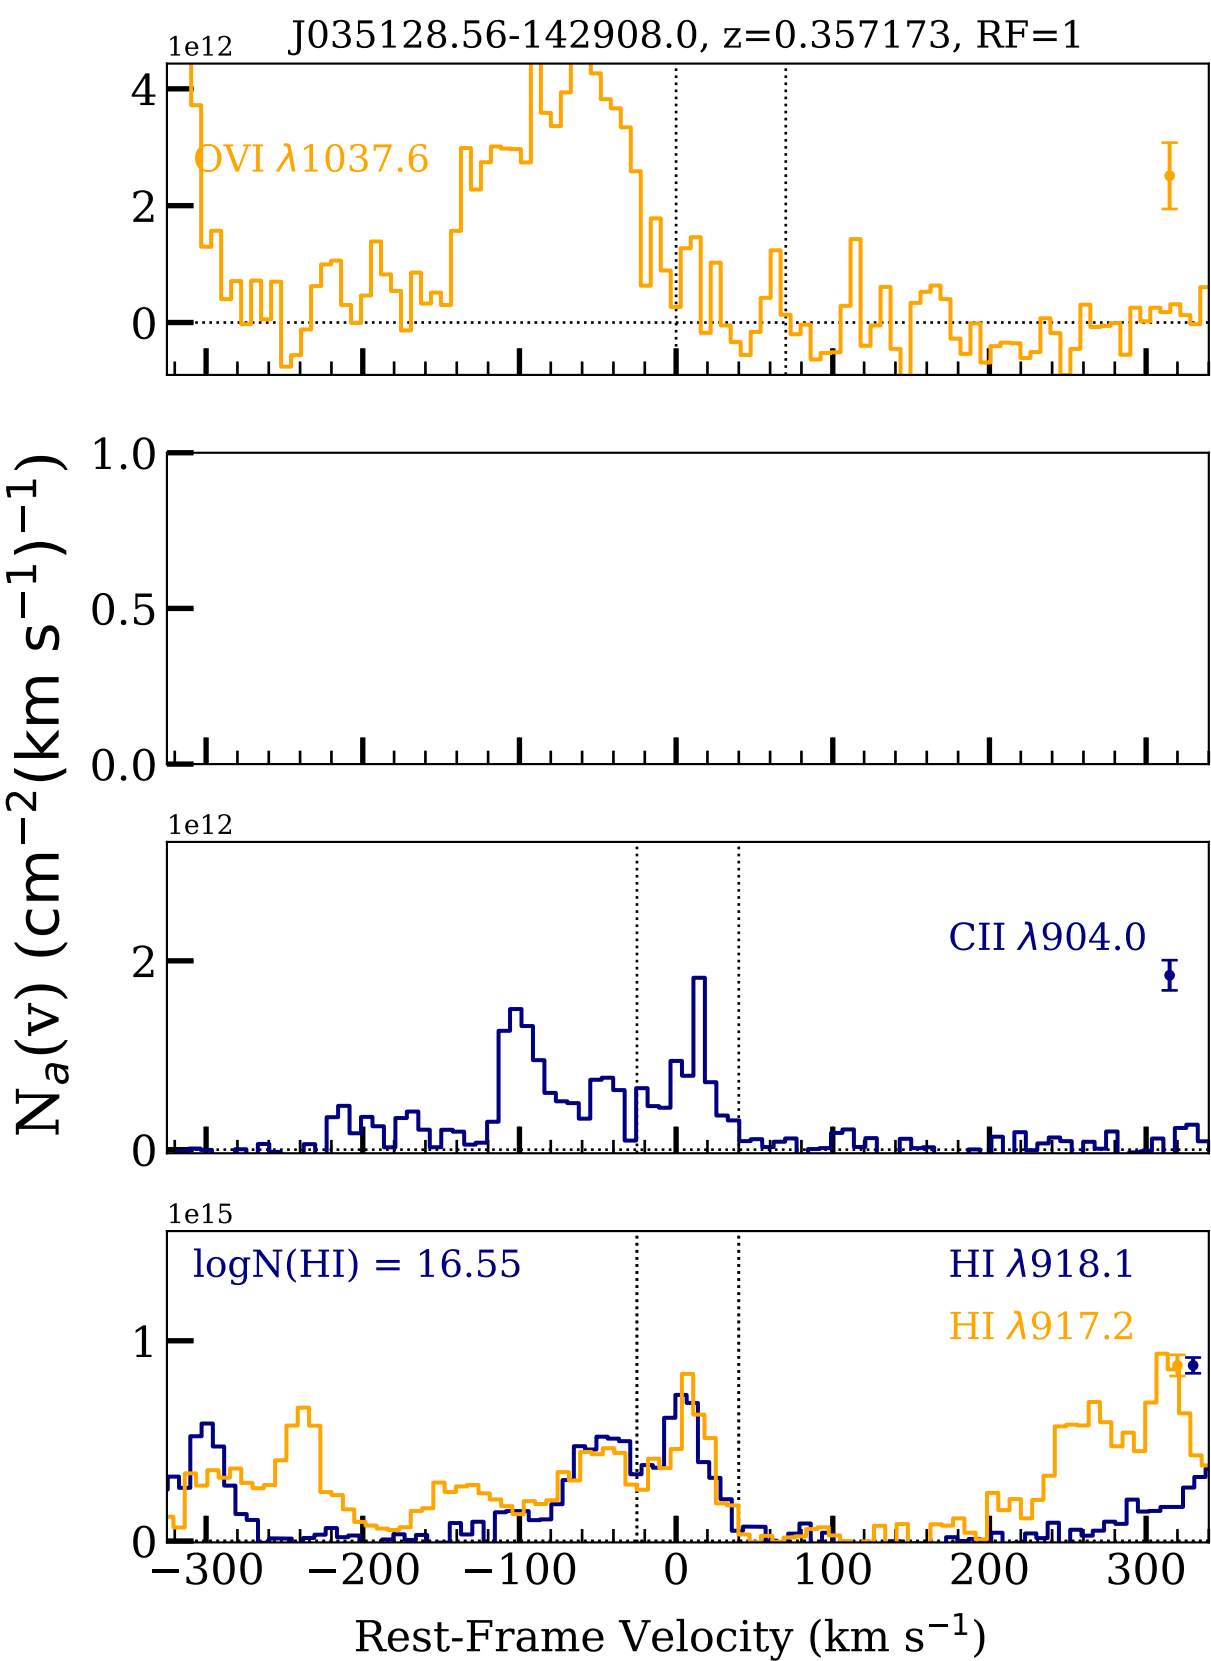

J035128.56-142908.0,  $z=0.439804$ , RF=1

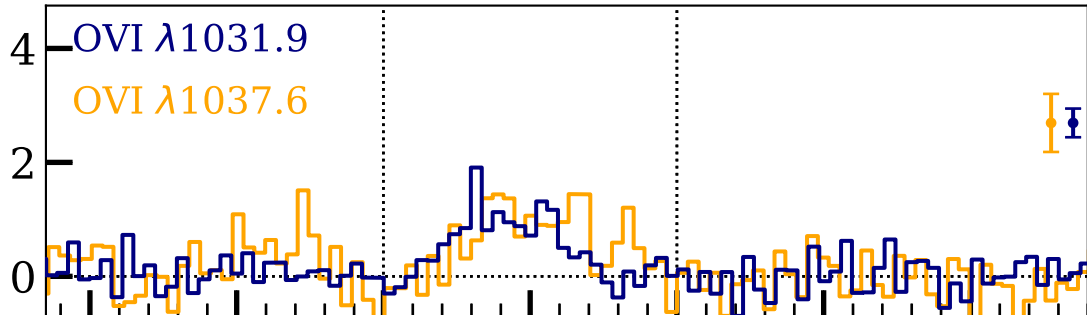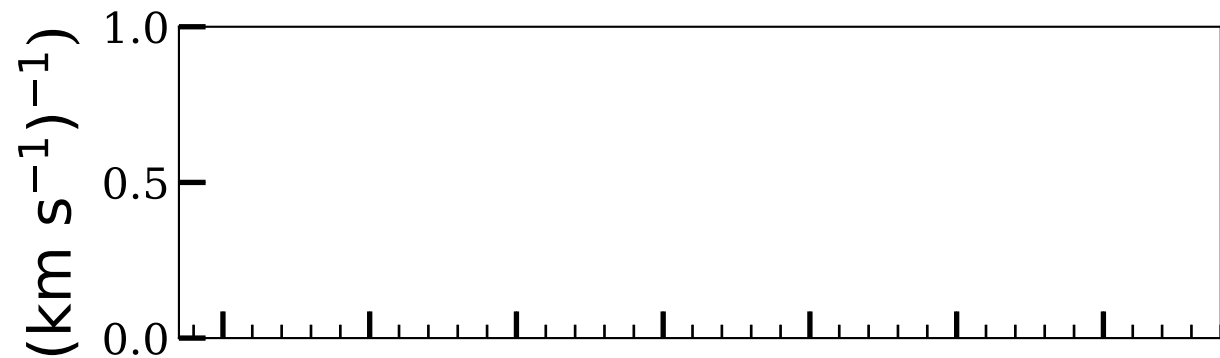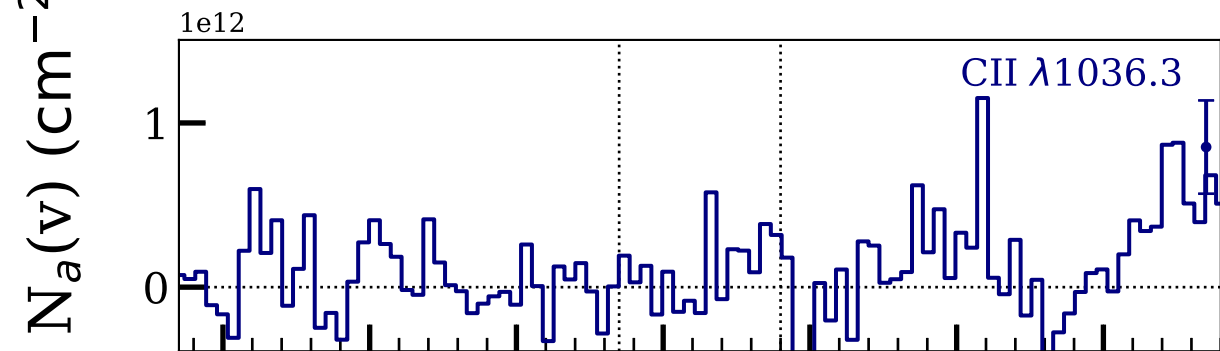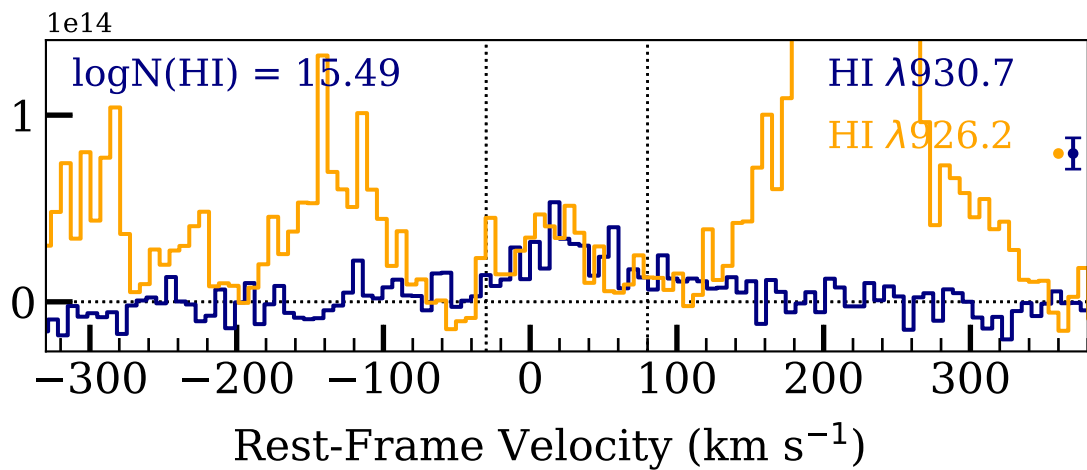

J040148.98-054056.5,  $z=0.219453$ , RF=1

$N_a(v) \text{ (cm}^{-2} \text{ (km s}^{-1})^{-1})$

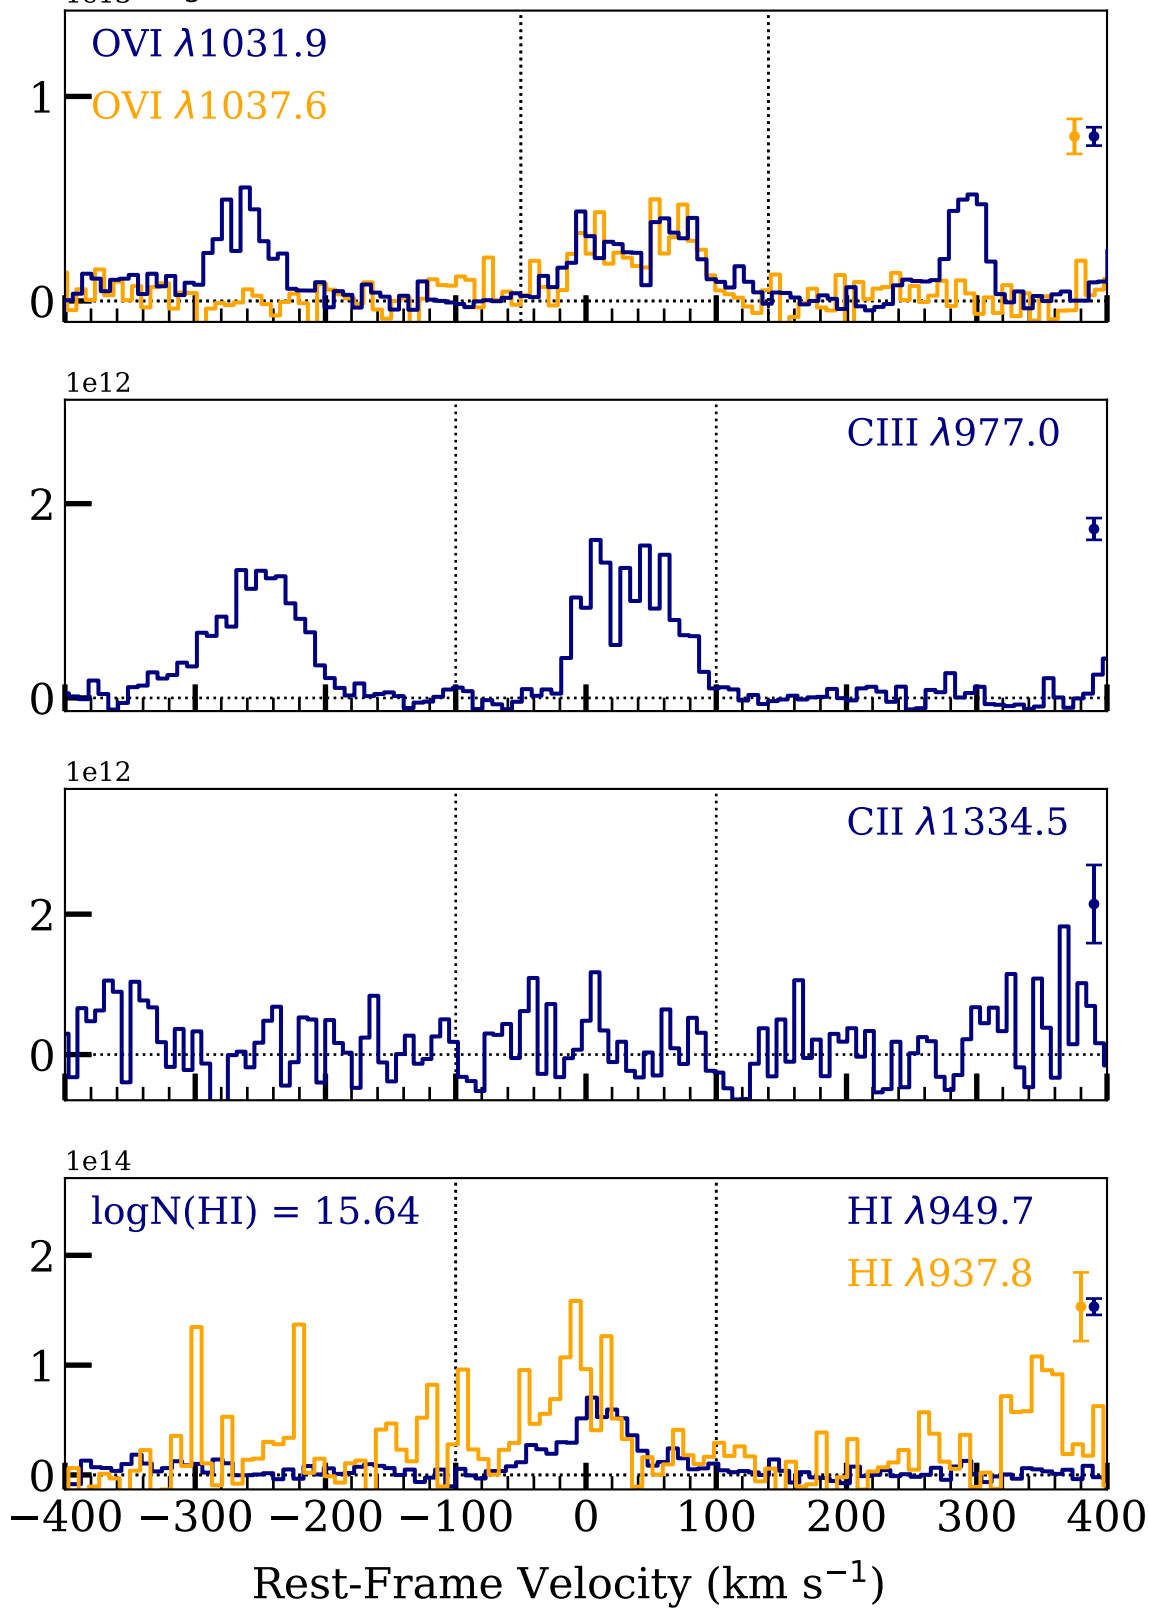

J040148.98-054056.5,  $z=0.323769$ , RF=1

$N_a(v)$  ( $\text{cm}^{-2}(\text{km s}^{-1})^{-1}$ )

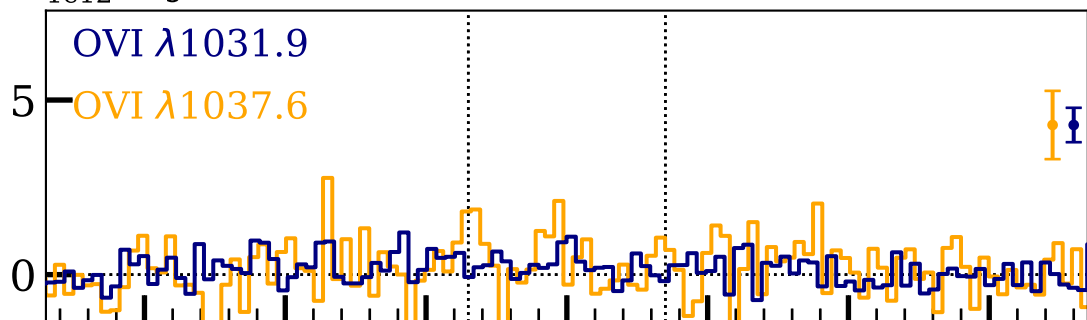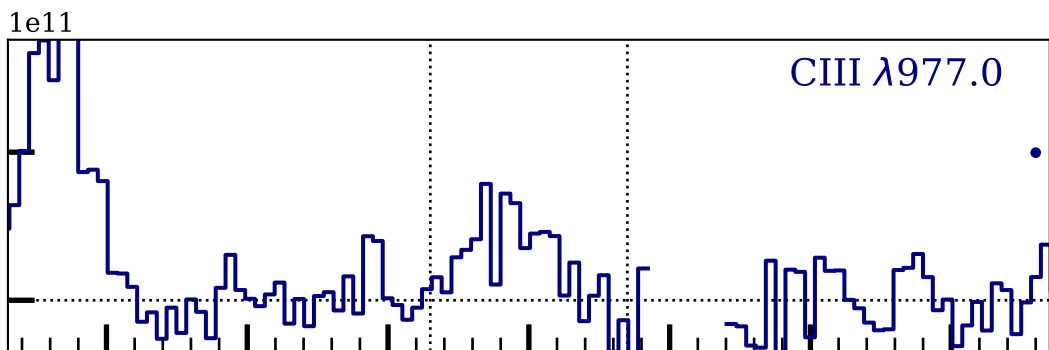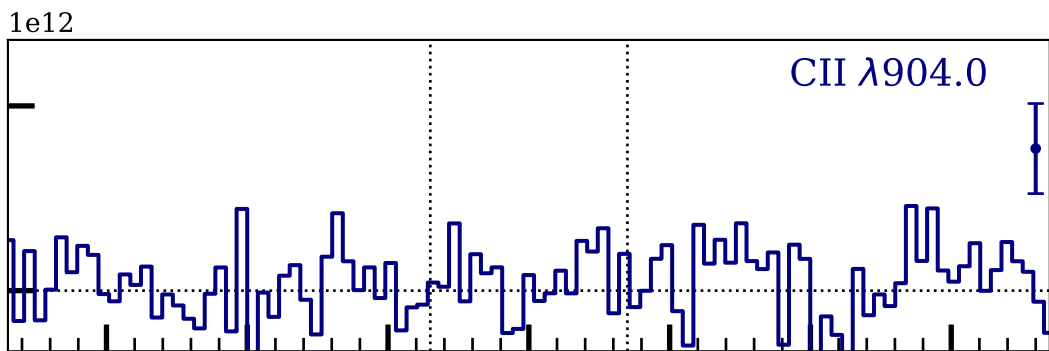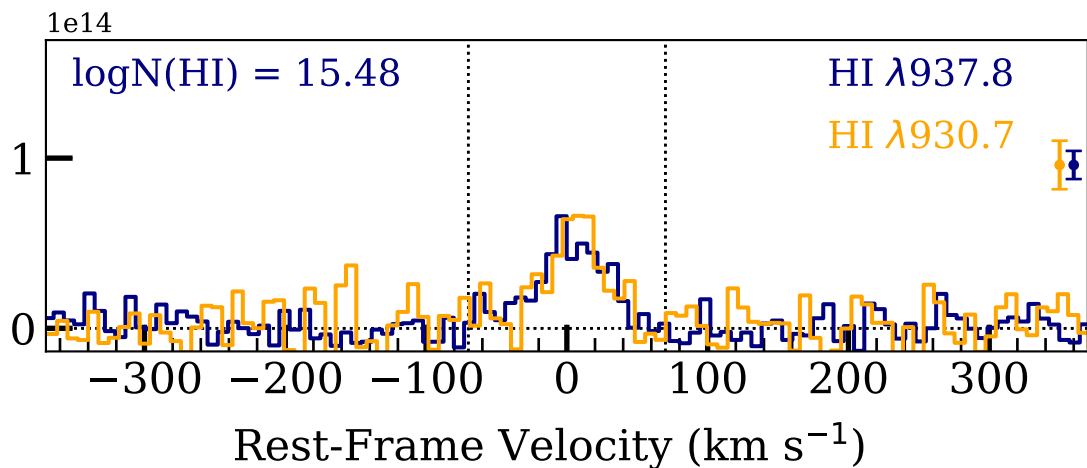



J040748.42-121136.3,  $z=0.167160$ , RF=1

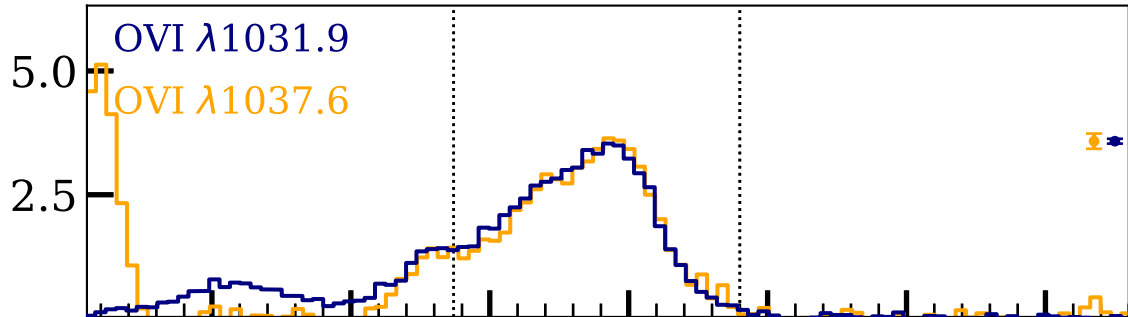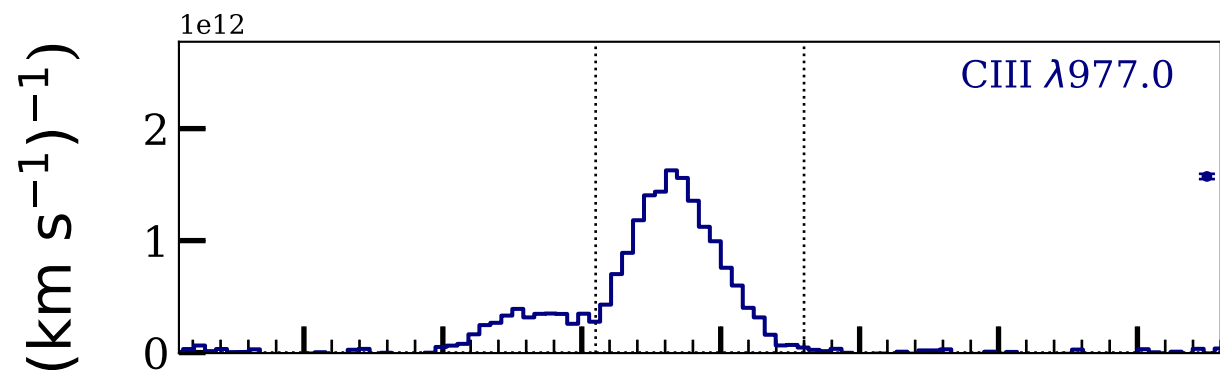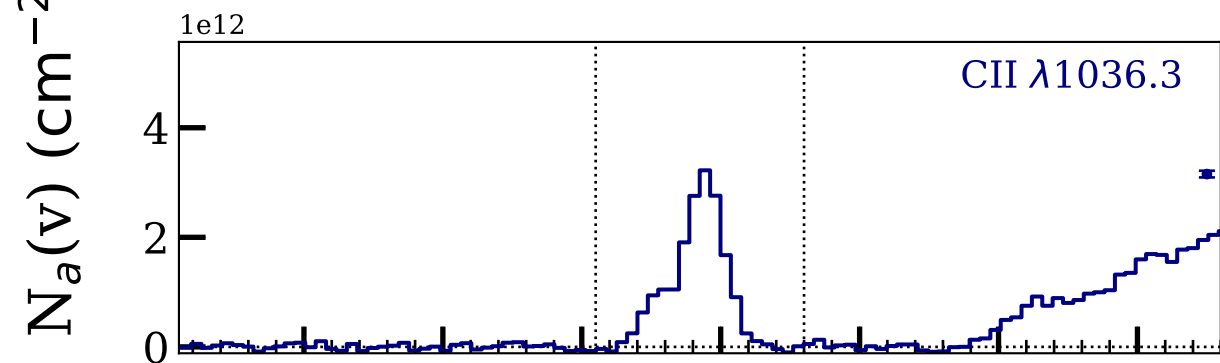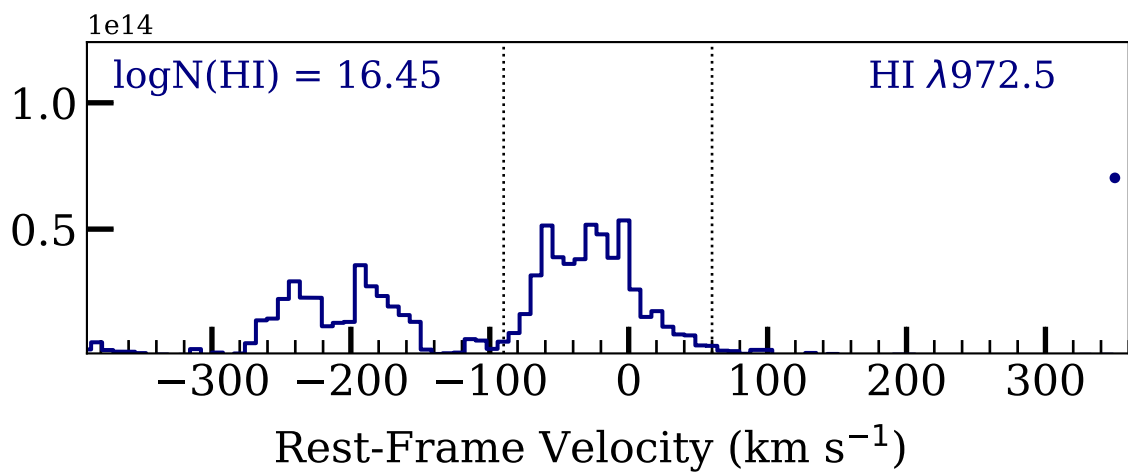

J040748.42-121136.3,  $z=0.360742$ , RF=1

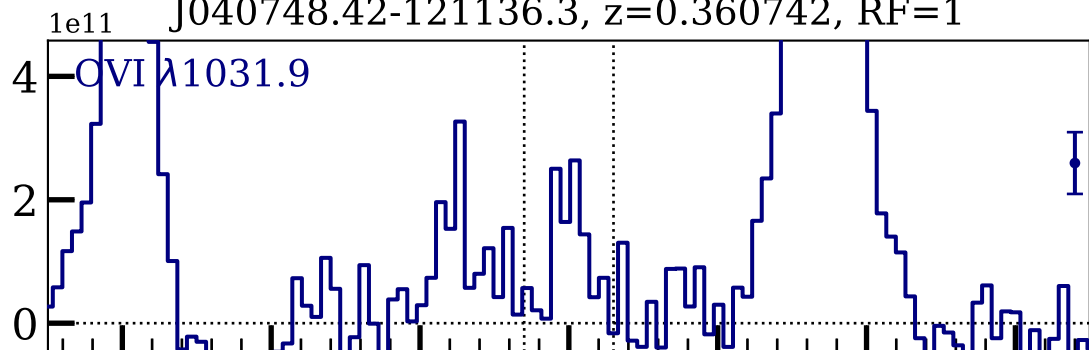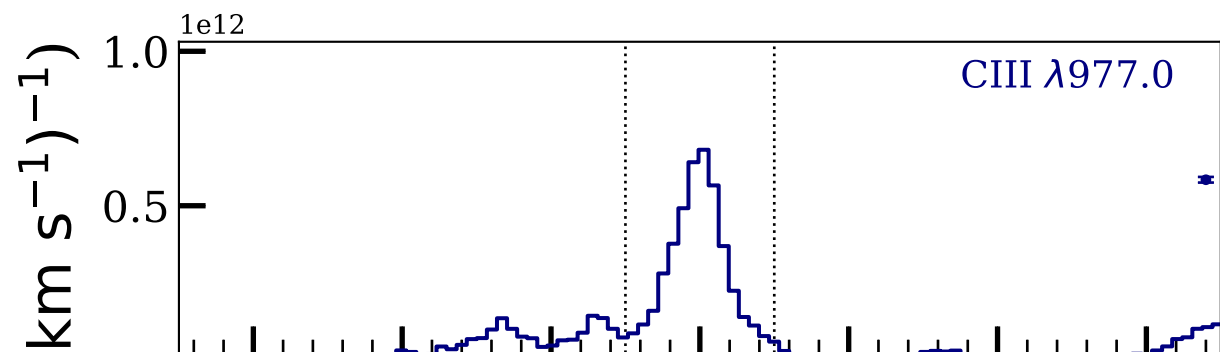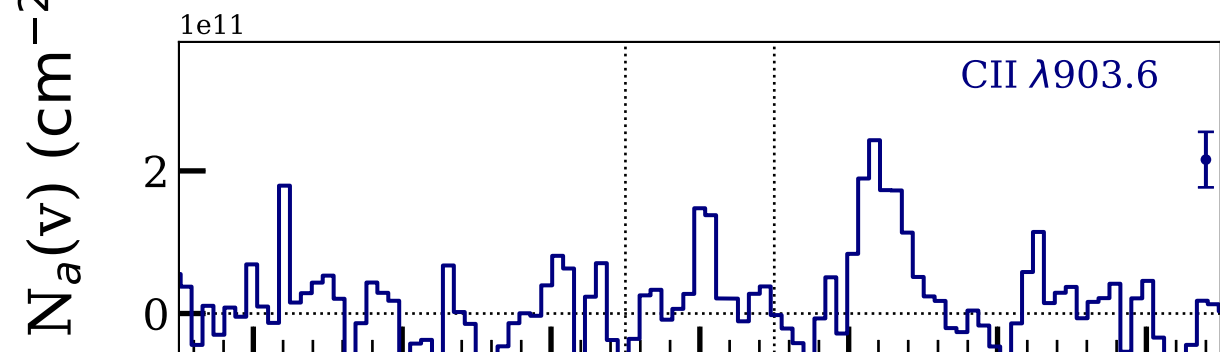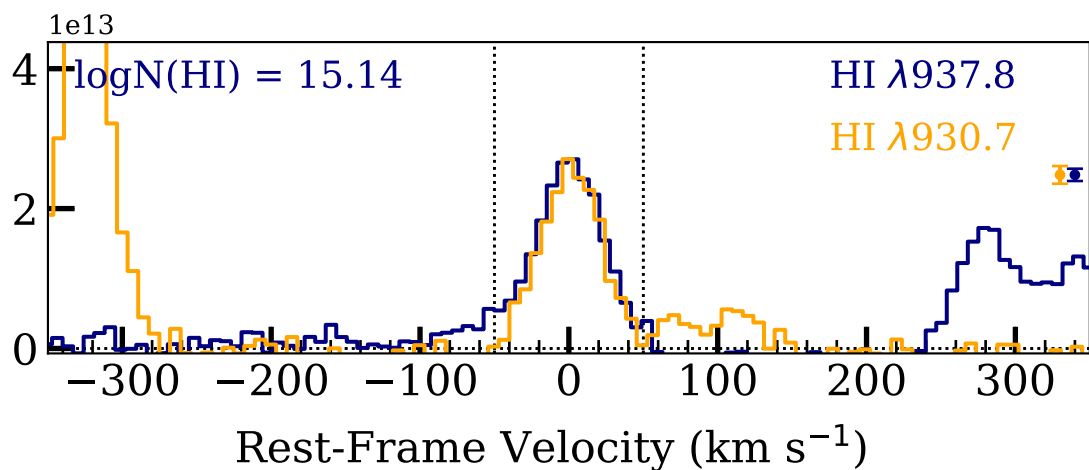

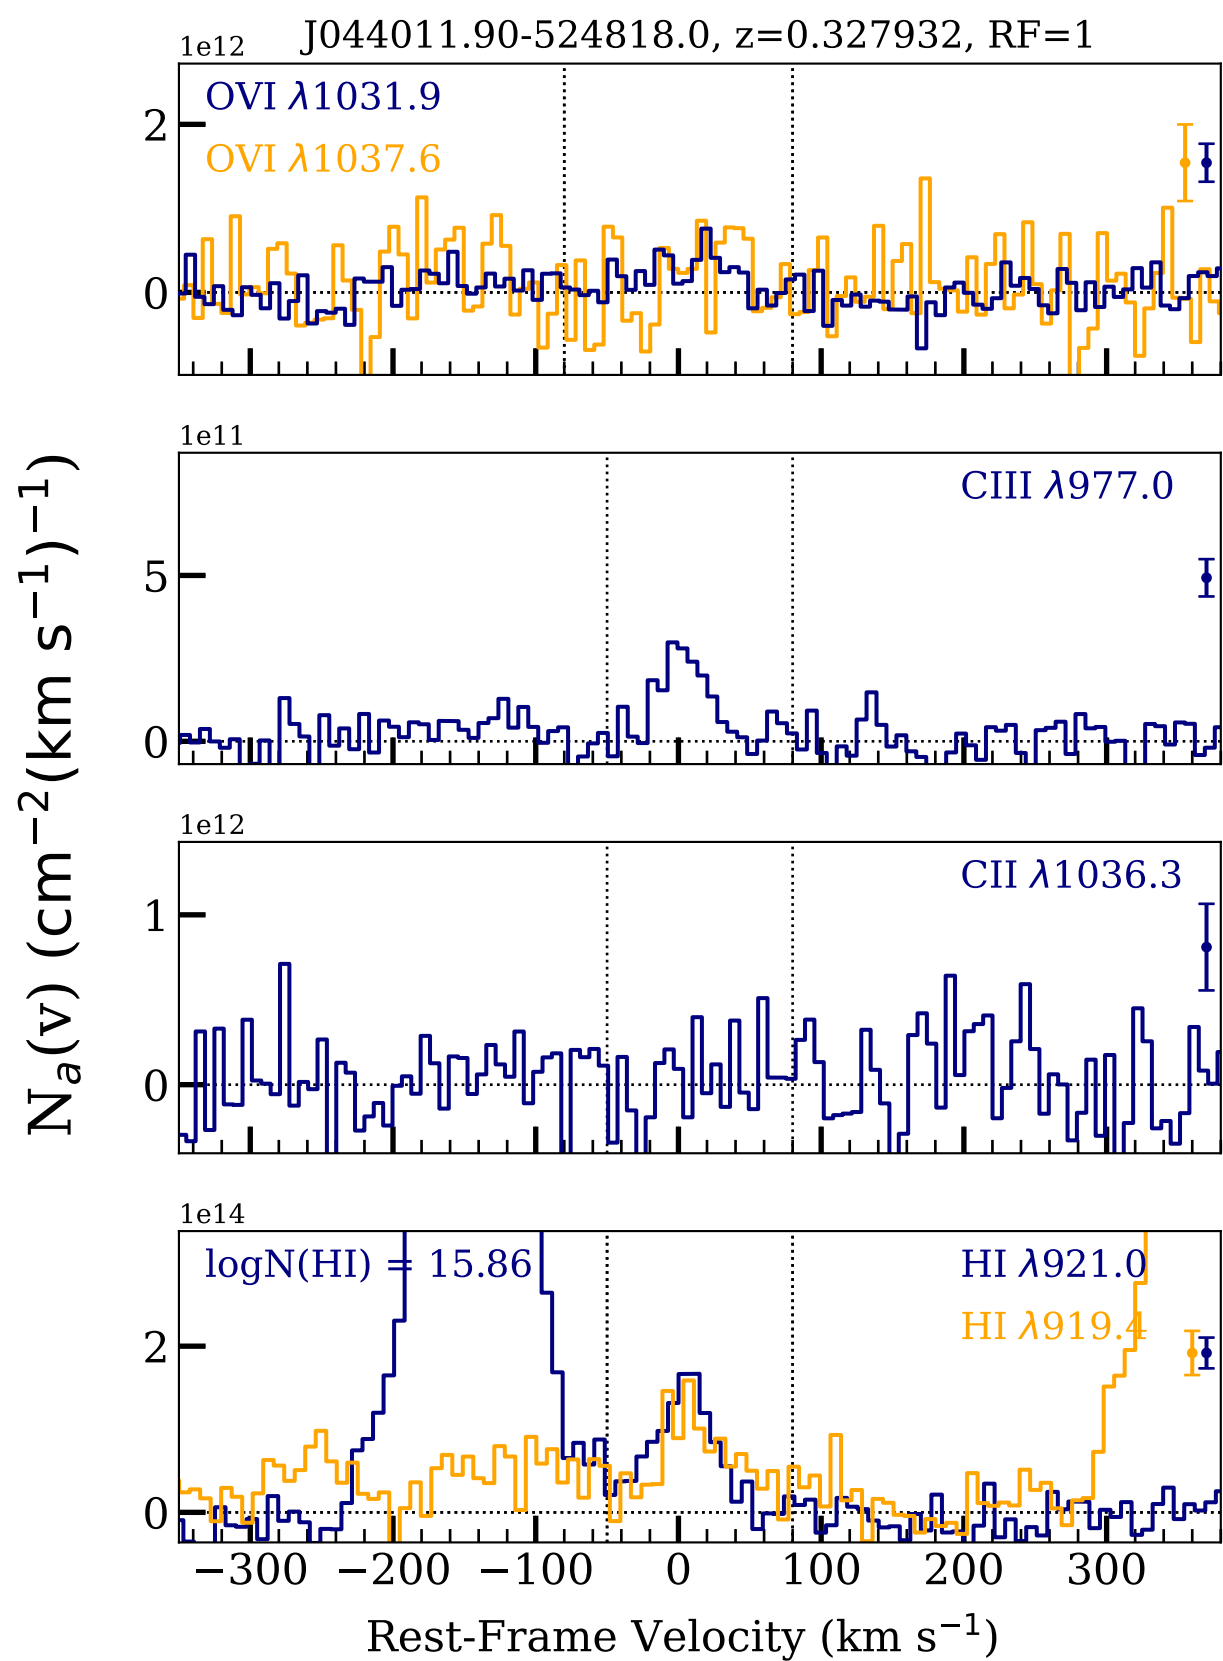

J044011.90-524818.0,  $z=0.614962$ , RF=1

$N_a(v) \text{ (cm}^{-2} \text{ (km s}^{-1} \text{)}^{-1} \text{)}$

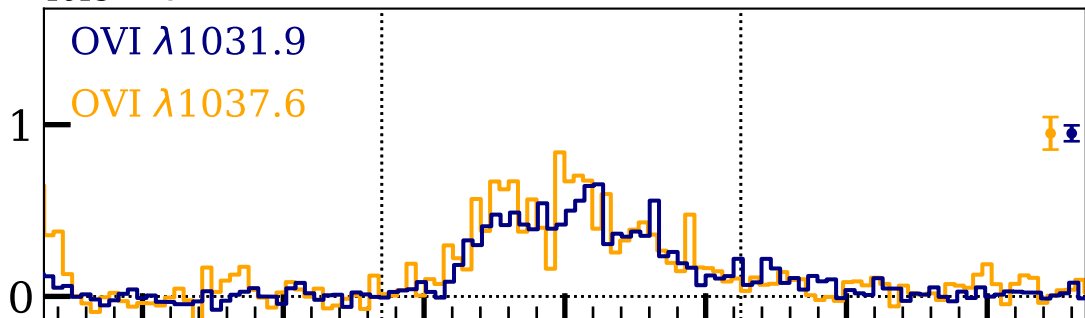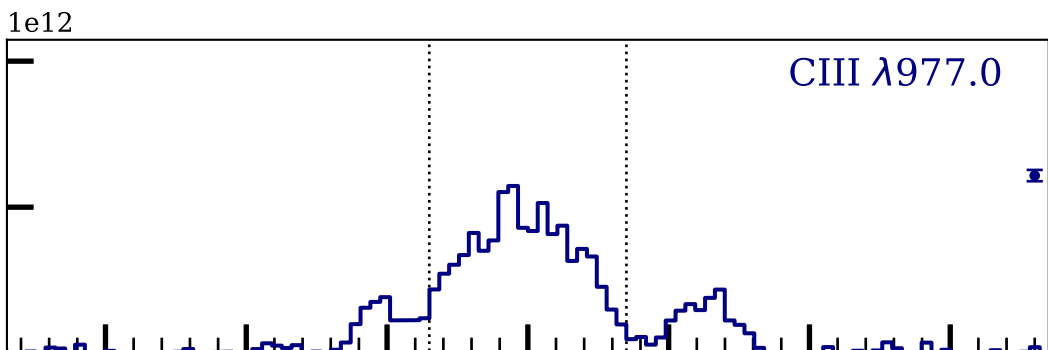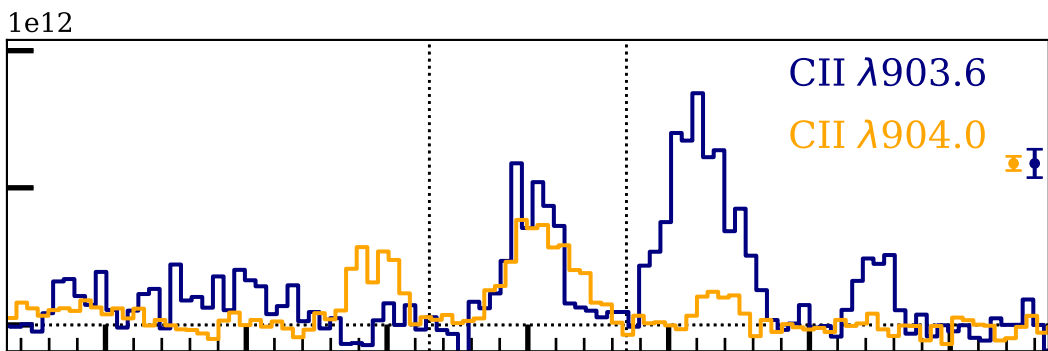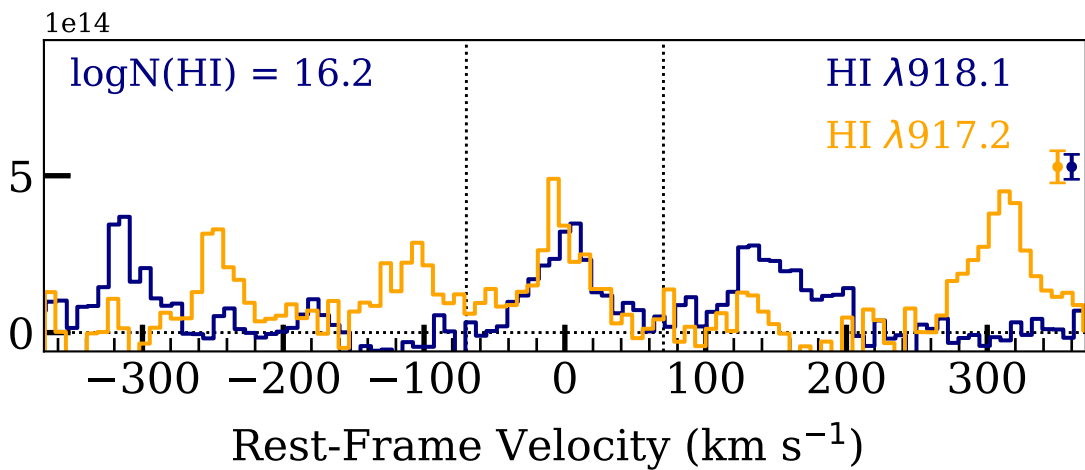

J044011.90-524818.0, z=0.615662, RF=1

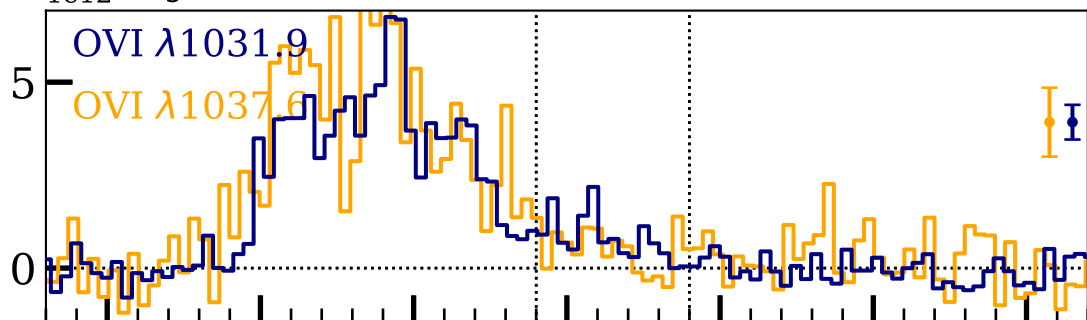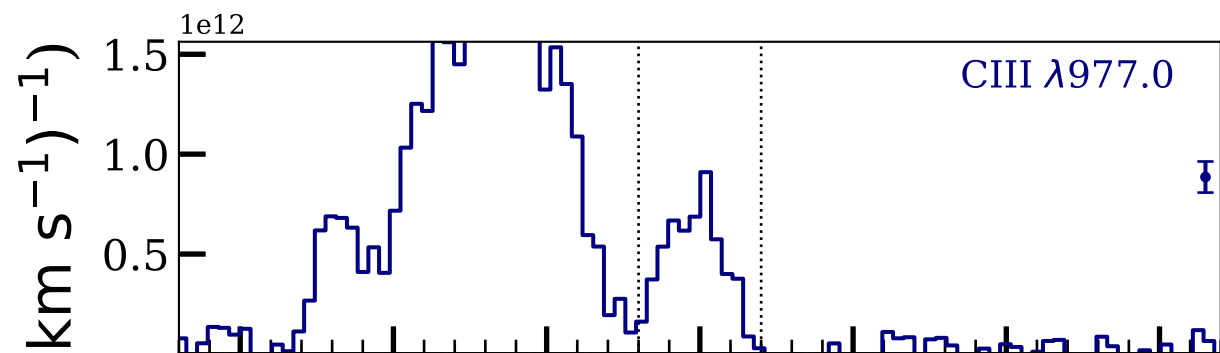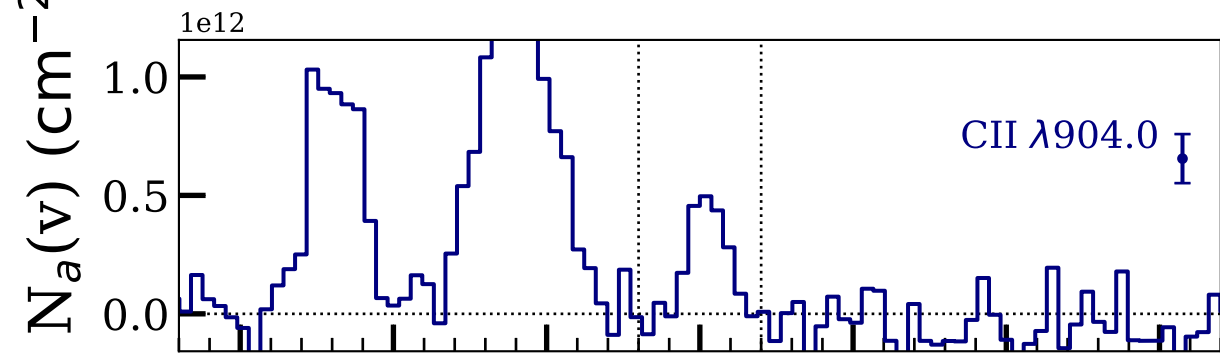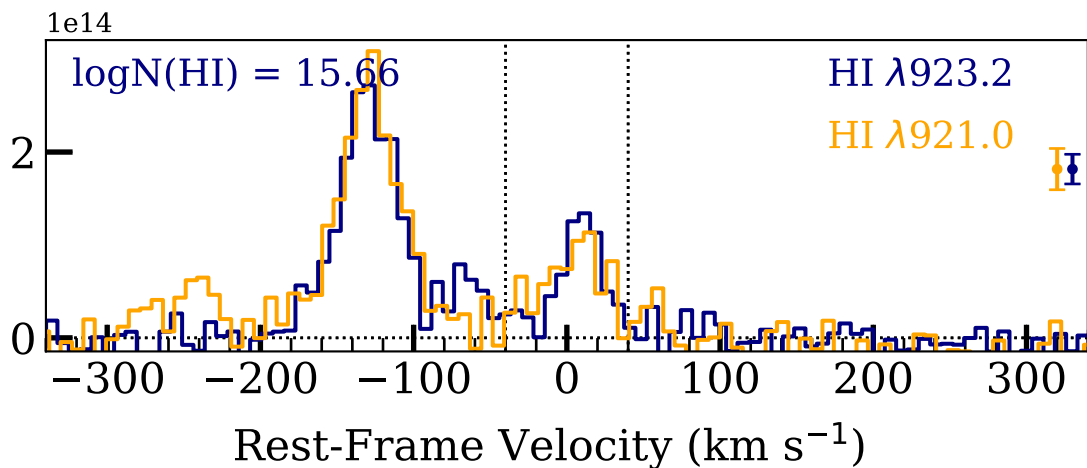

J055224.49-640210.7,  $z=0.345149$ , RF=1

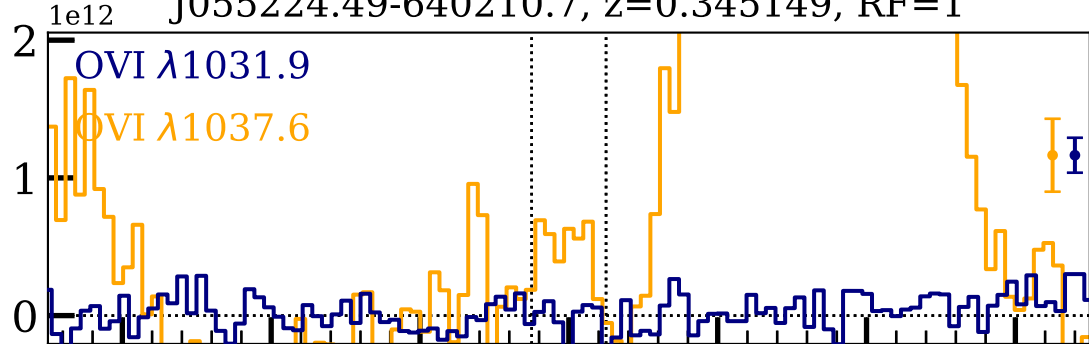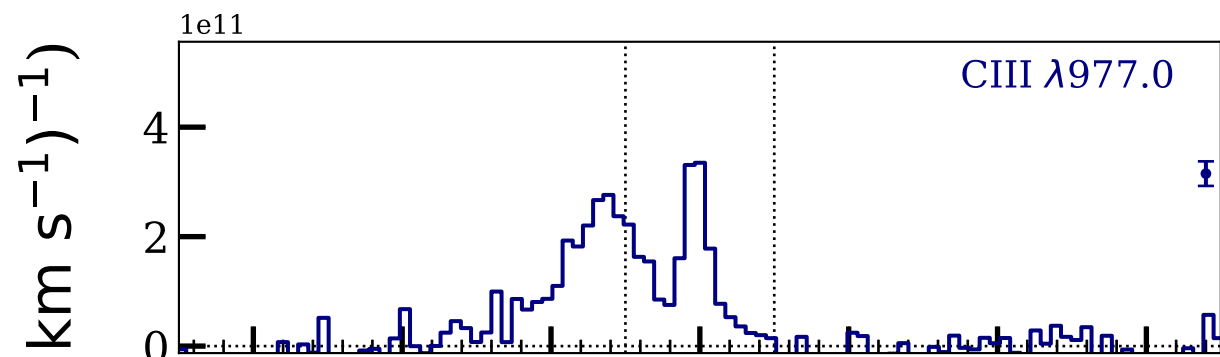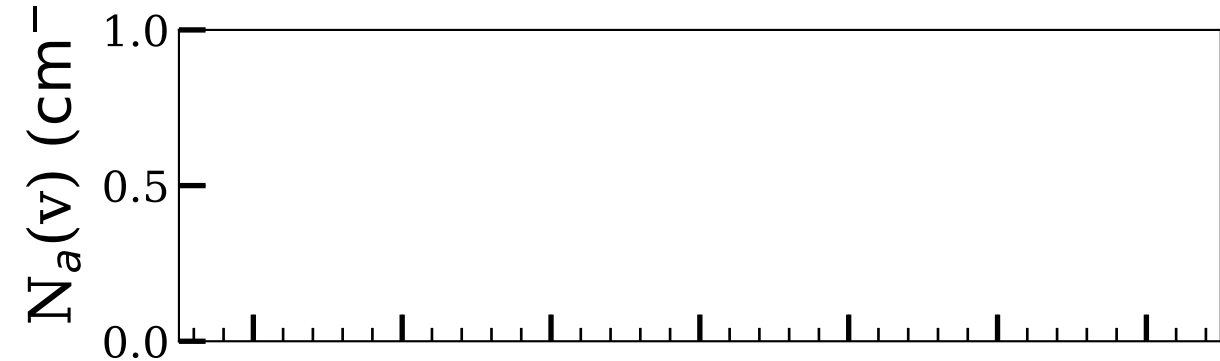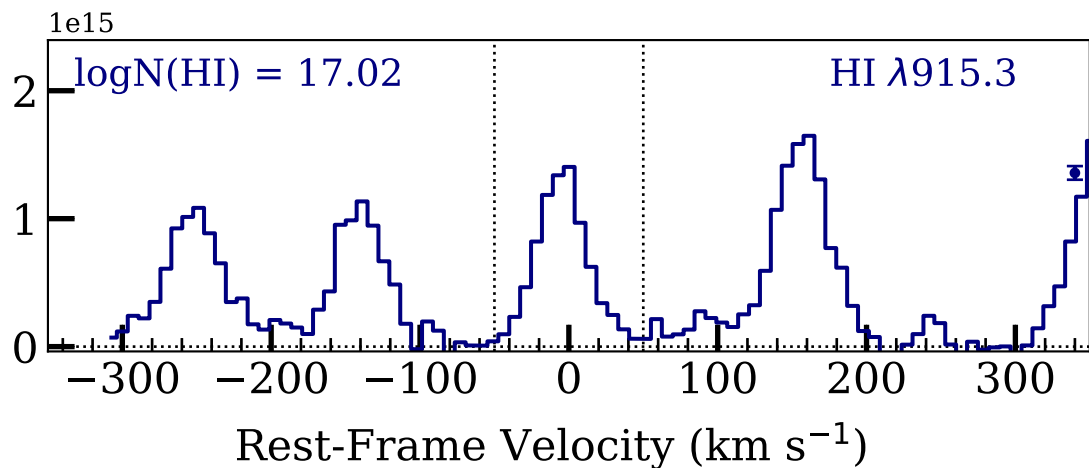

J055224.49-640210.7,  $z=0.446088$ , RF=1

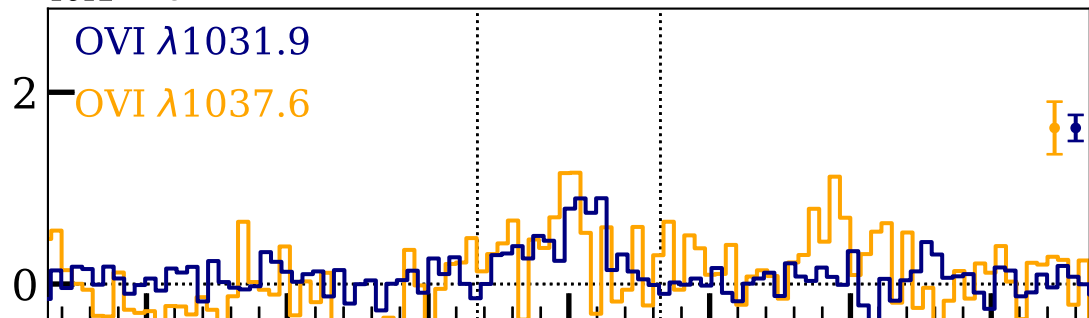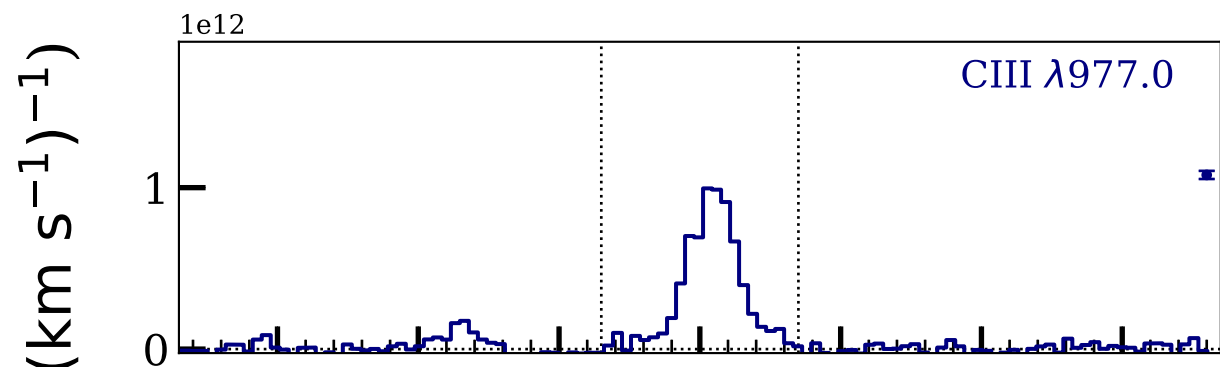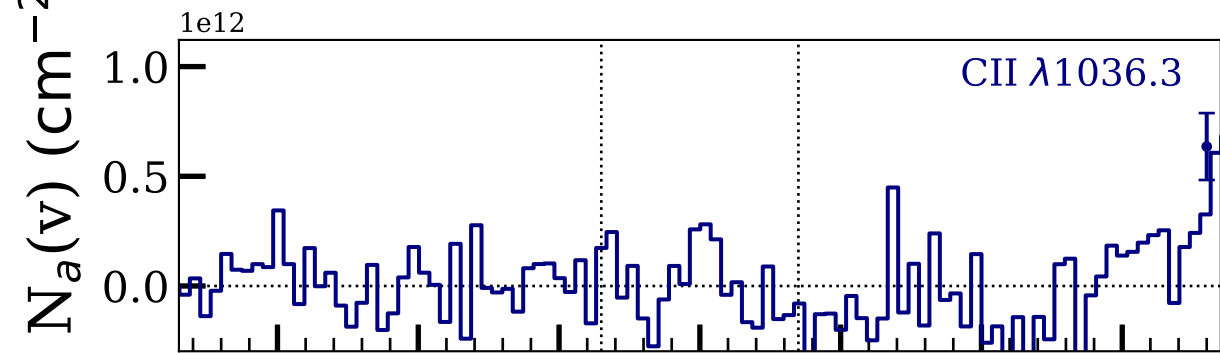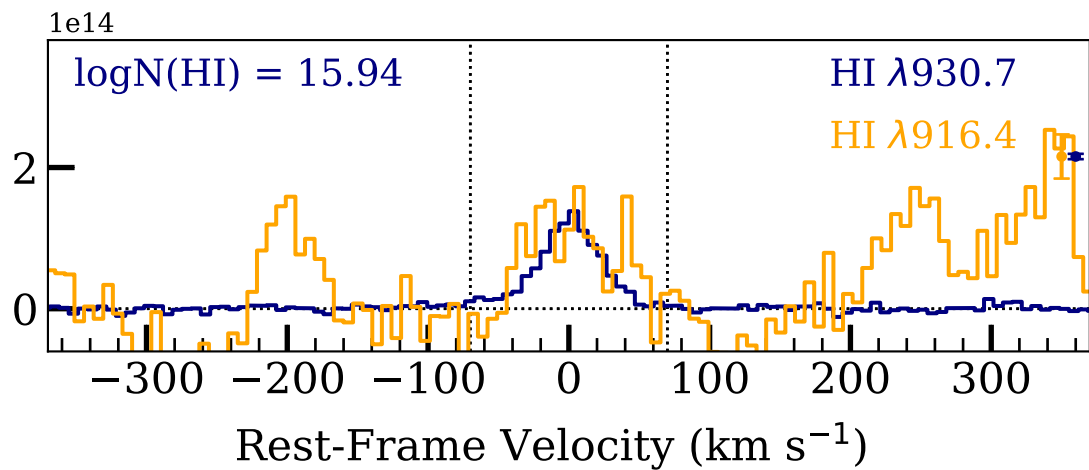

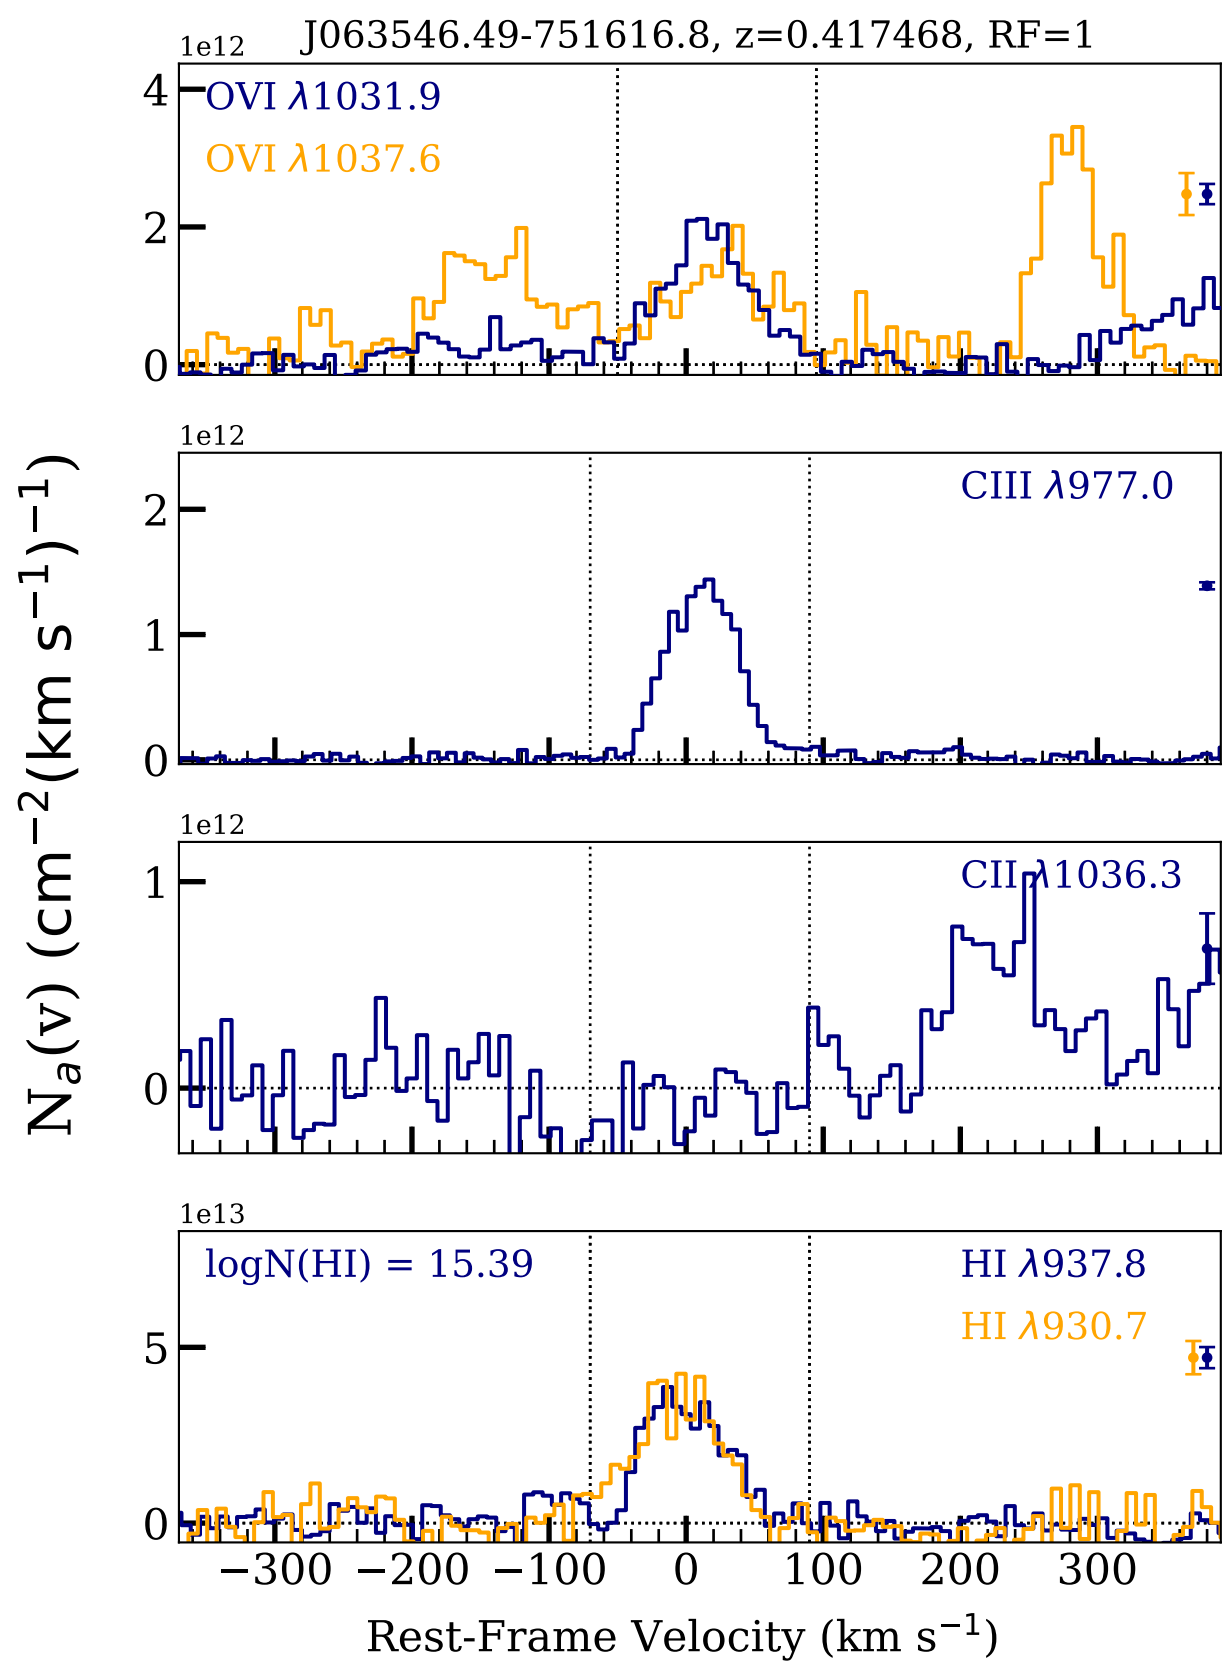



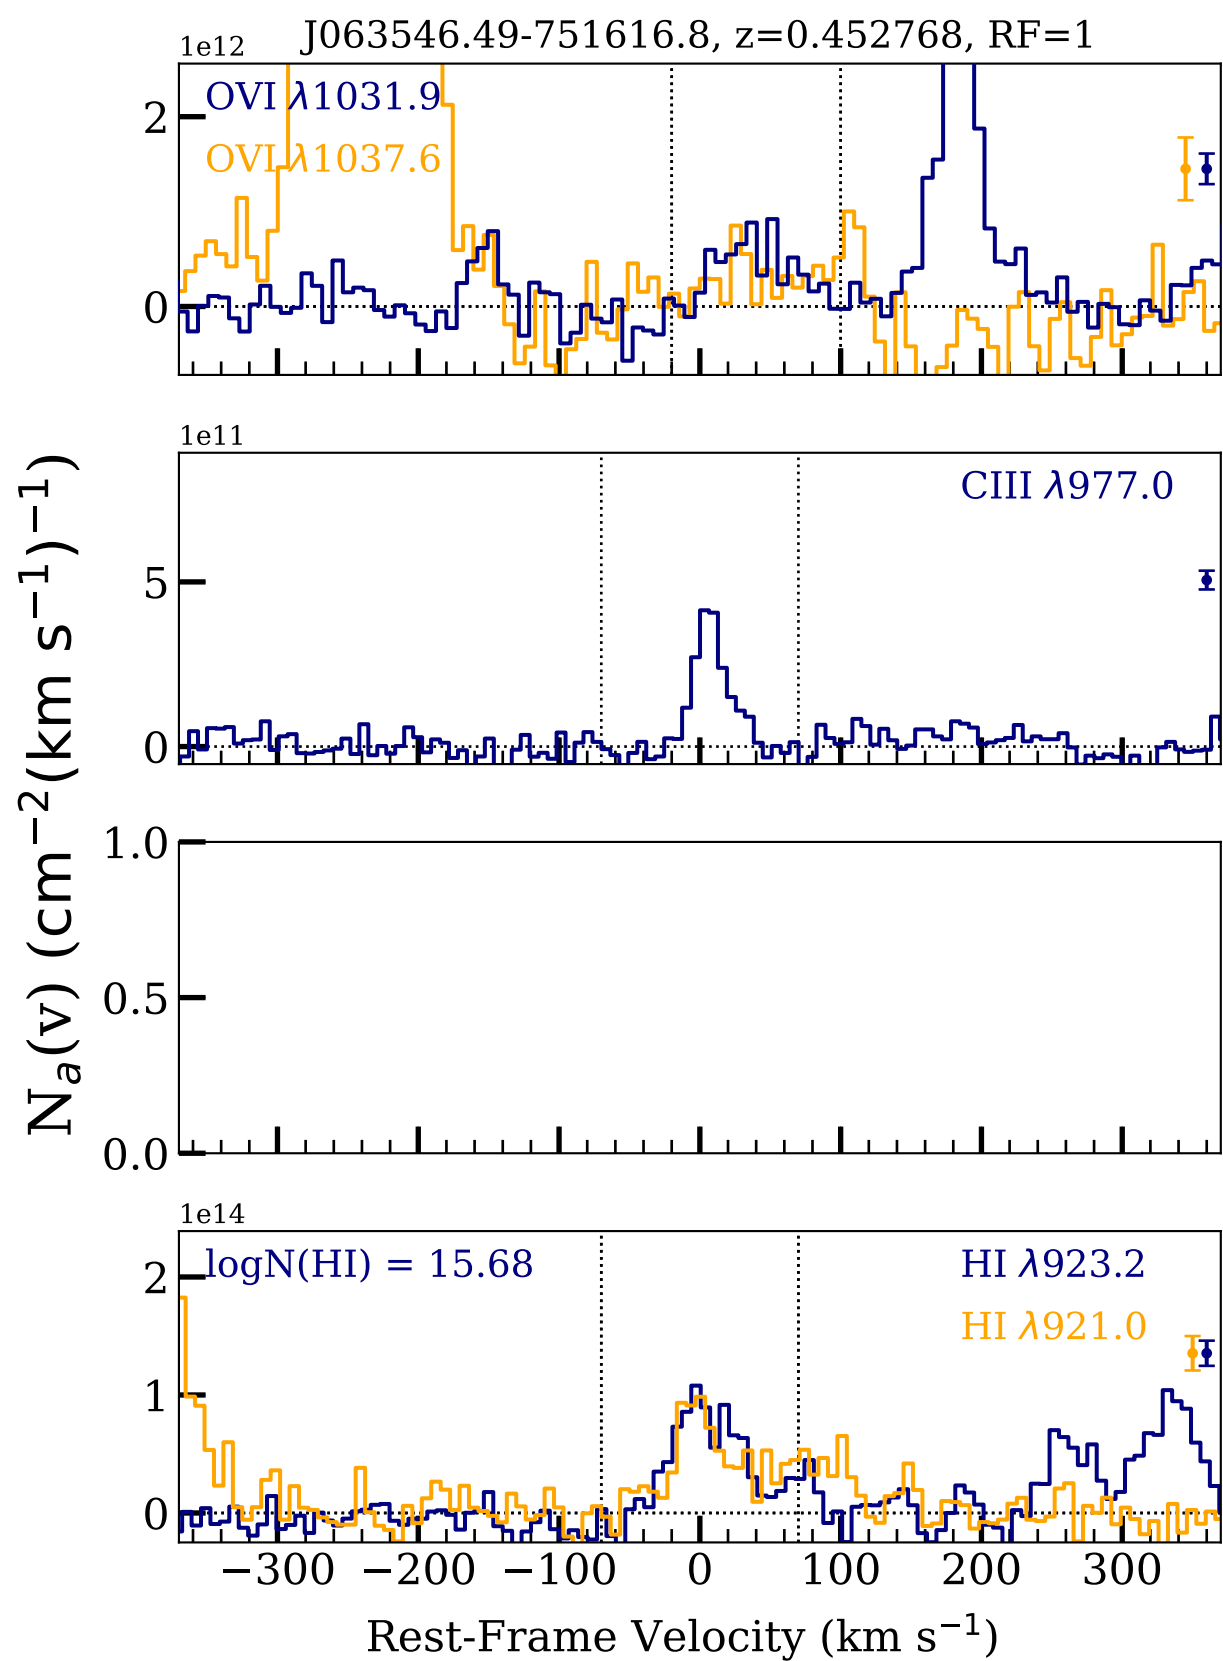

J063546.49-751616.8,  $z=0.468486$ , RF=1

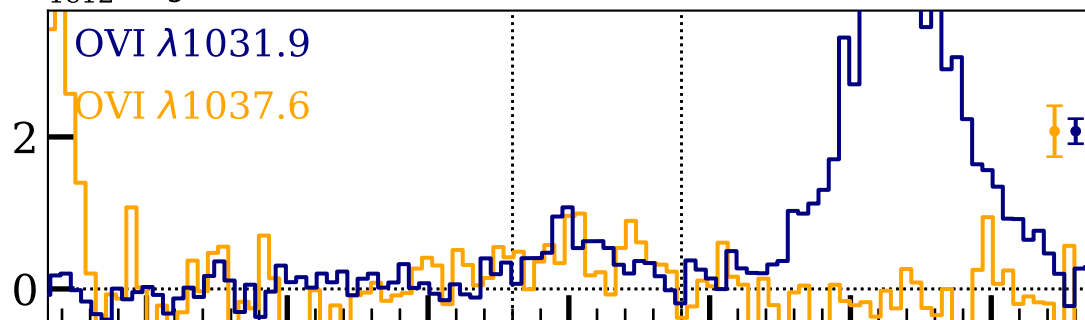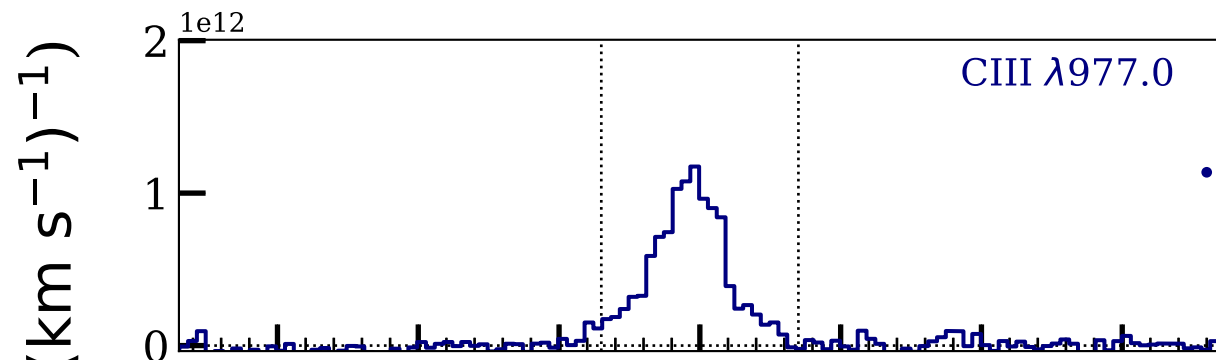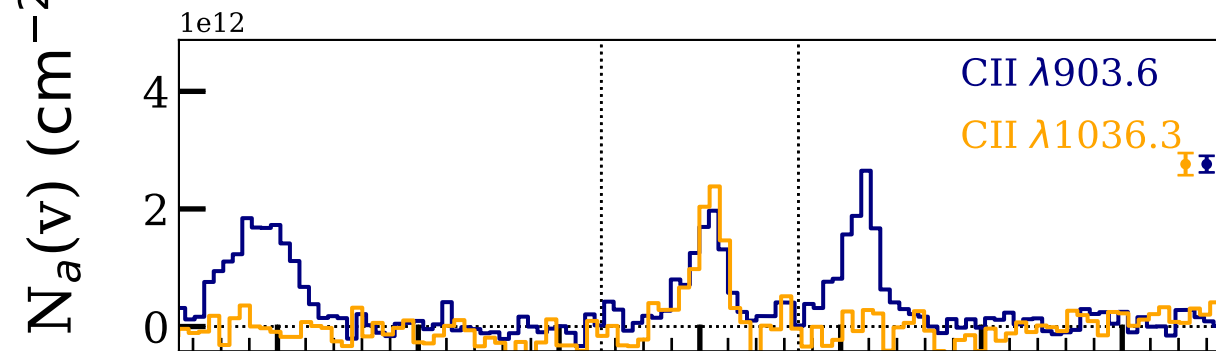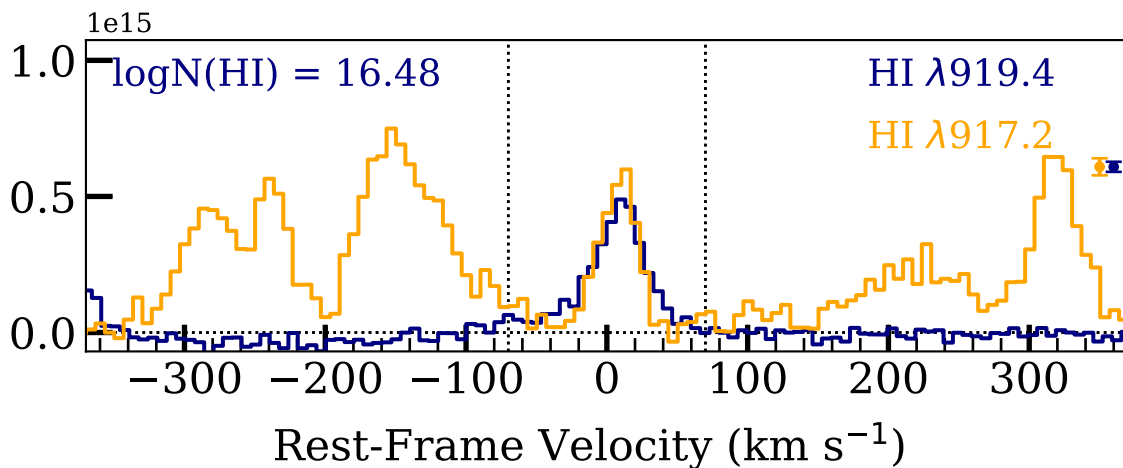

J071950.89+742757.0,  $z=0.377707$ , RF=1

$N_a(v)$  ( $\text{cm}^{-2}(\text{km s}^{-1})^{-1}$ )

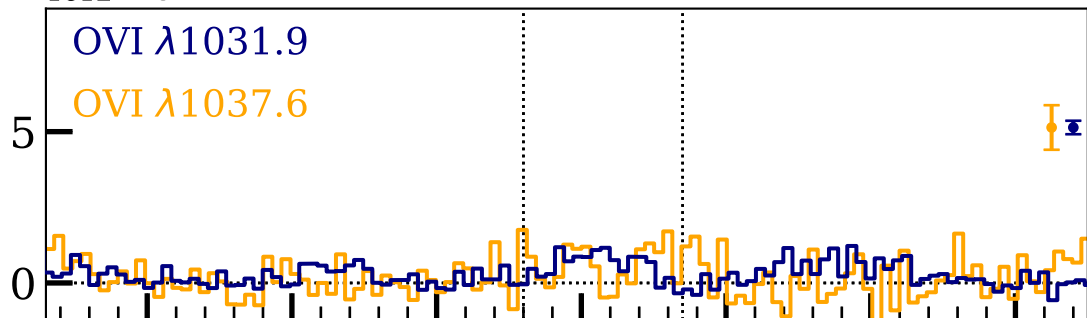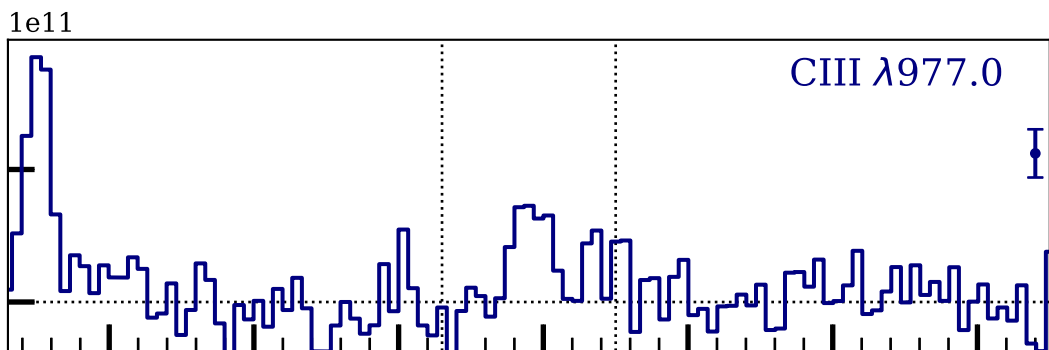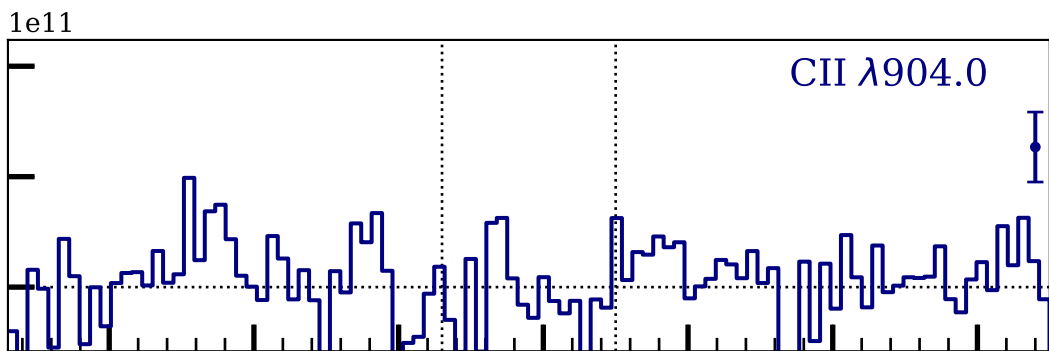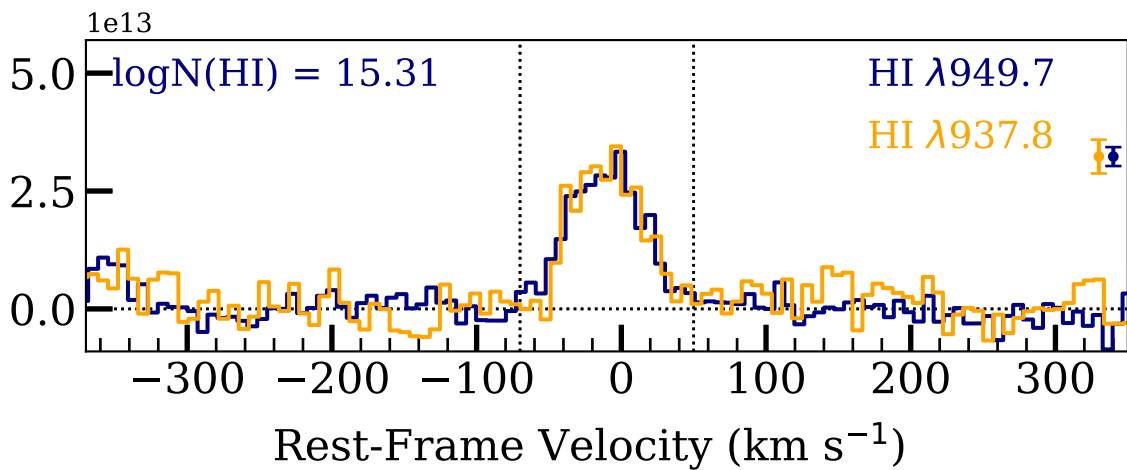

J075112.30+291938.3,  $z=0.431765$ , RF=1

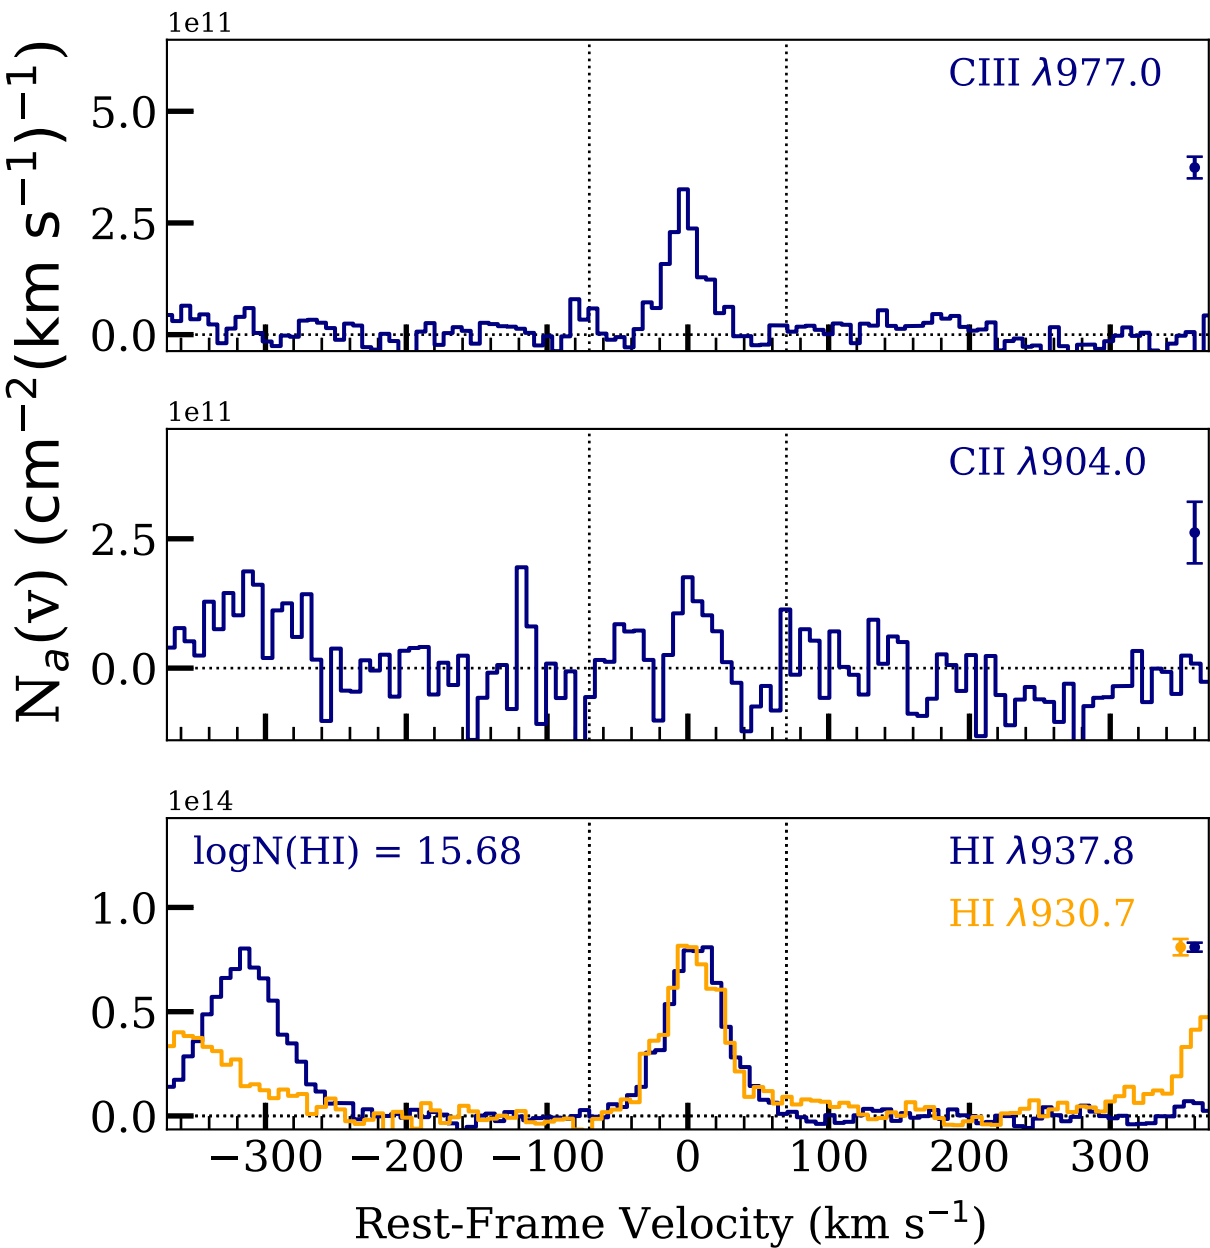

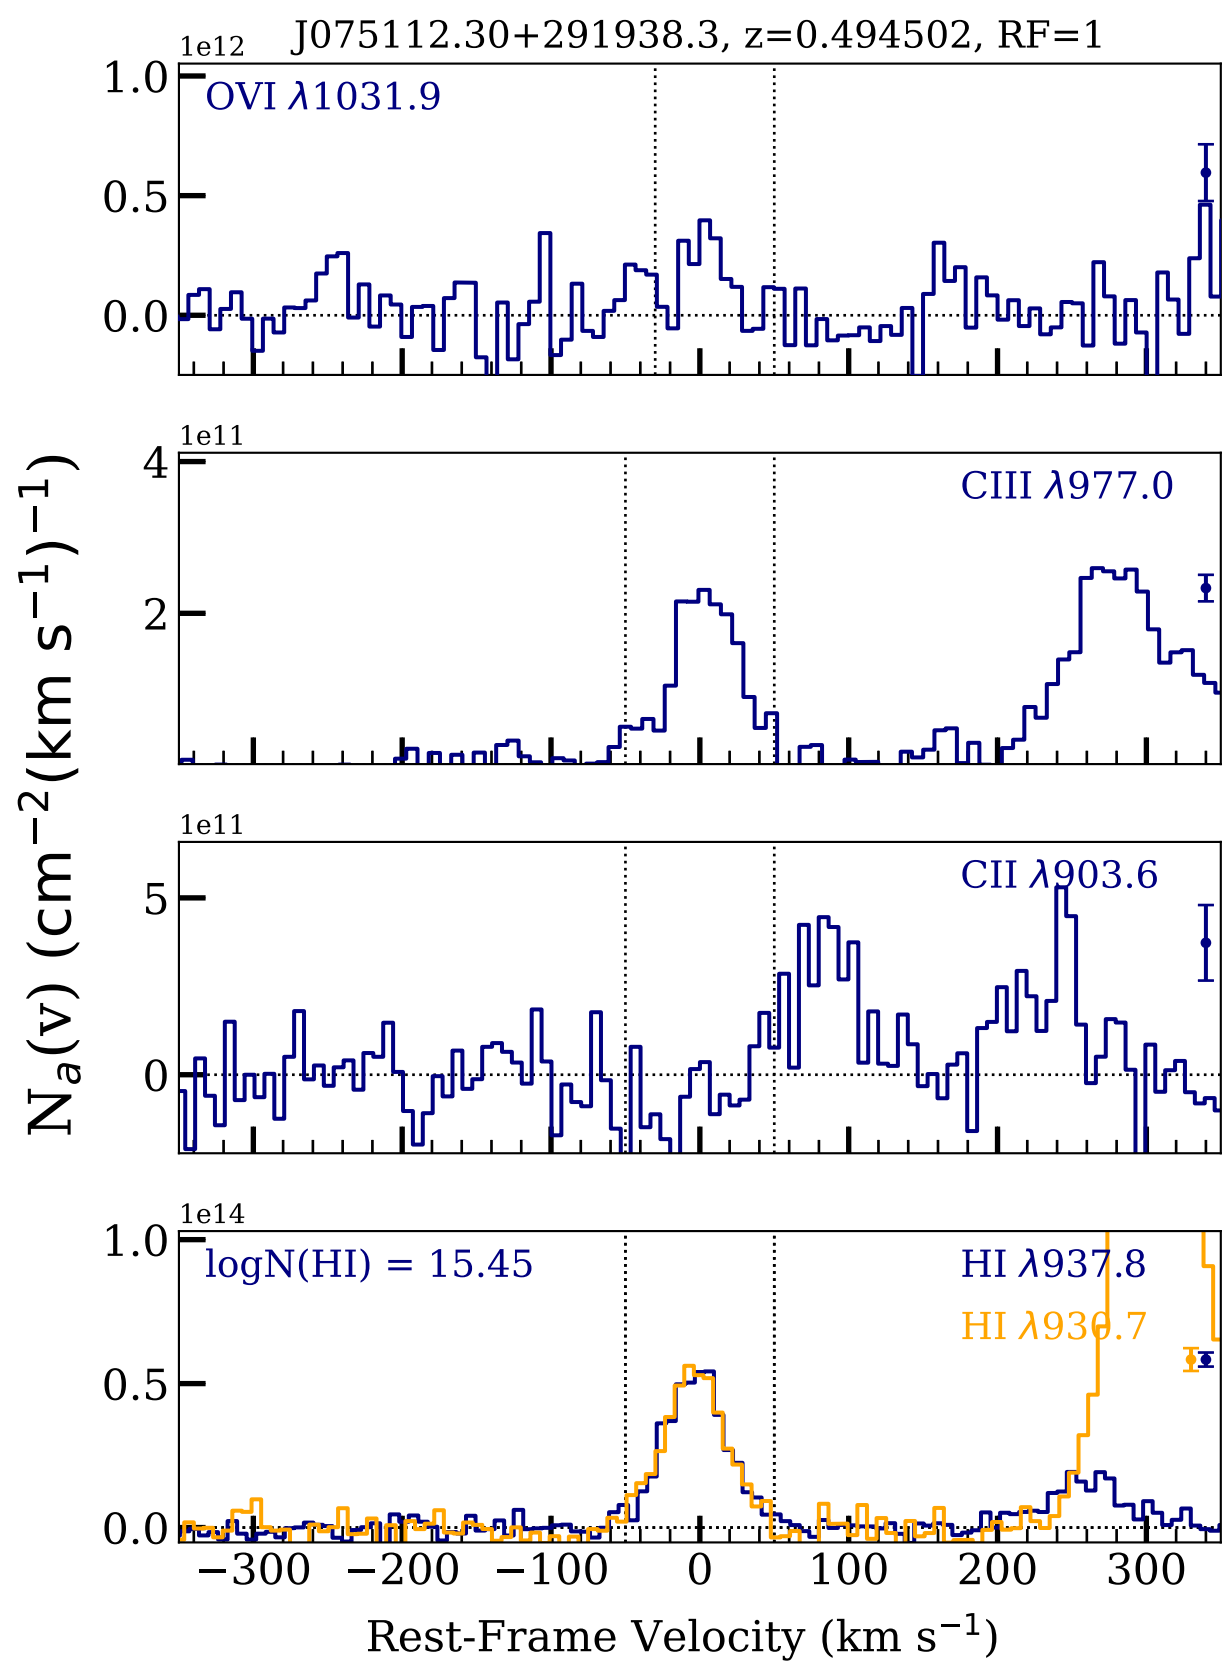

J080908.13+461925.6,  $z=0.619130$ , RF=1

$N_a(v) \text{ (cm}^{-2} \text{ (km s}^{-1} \text{)}^{-1} \text{)}$

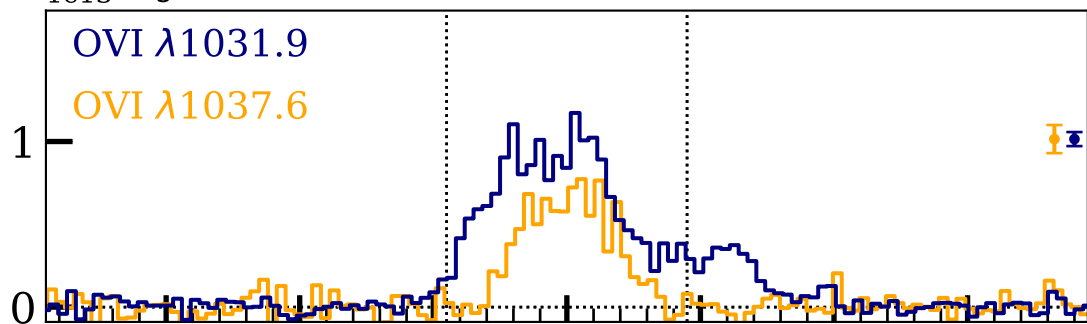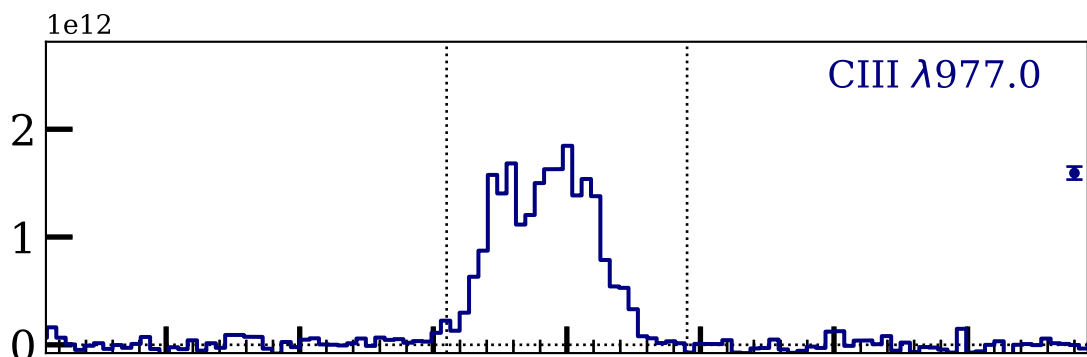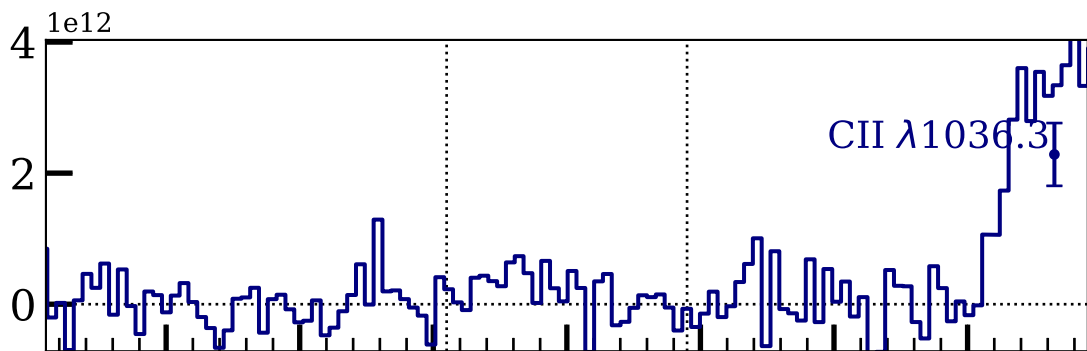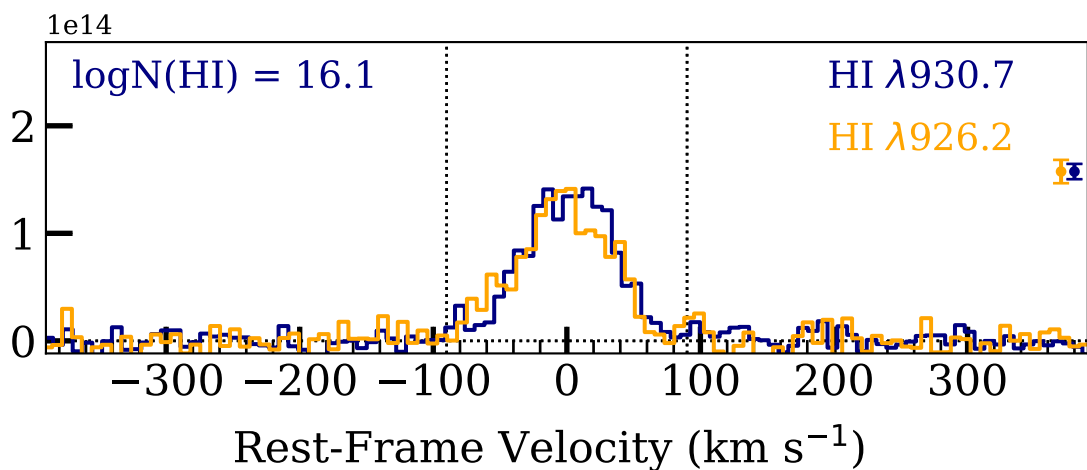

J084349.47+411741.6,  $z=0.533507$ , RF=0

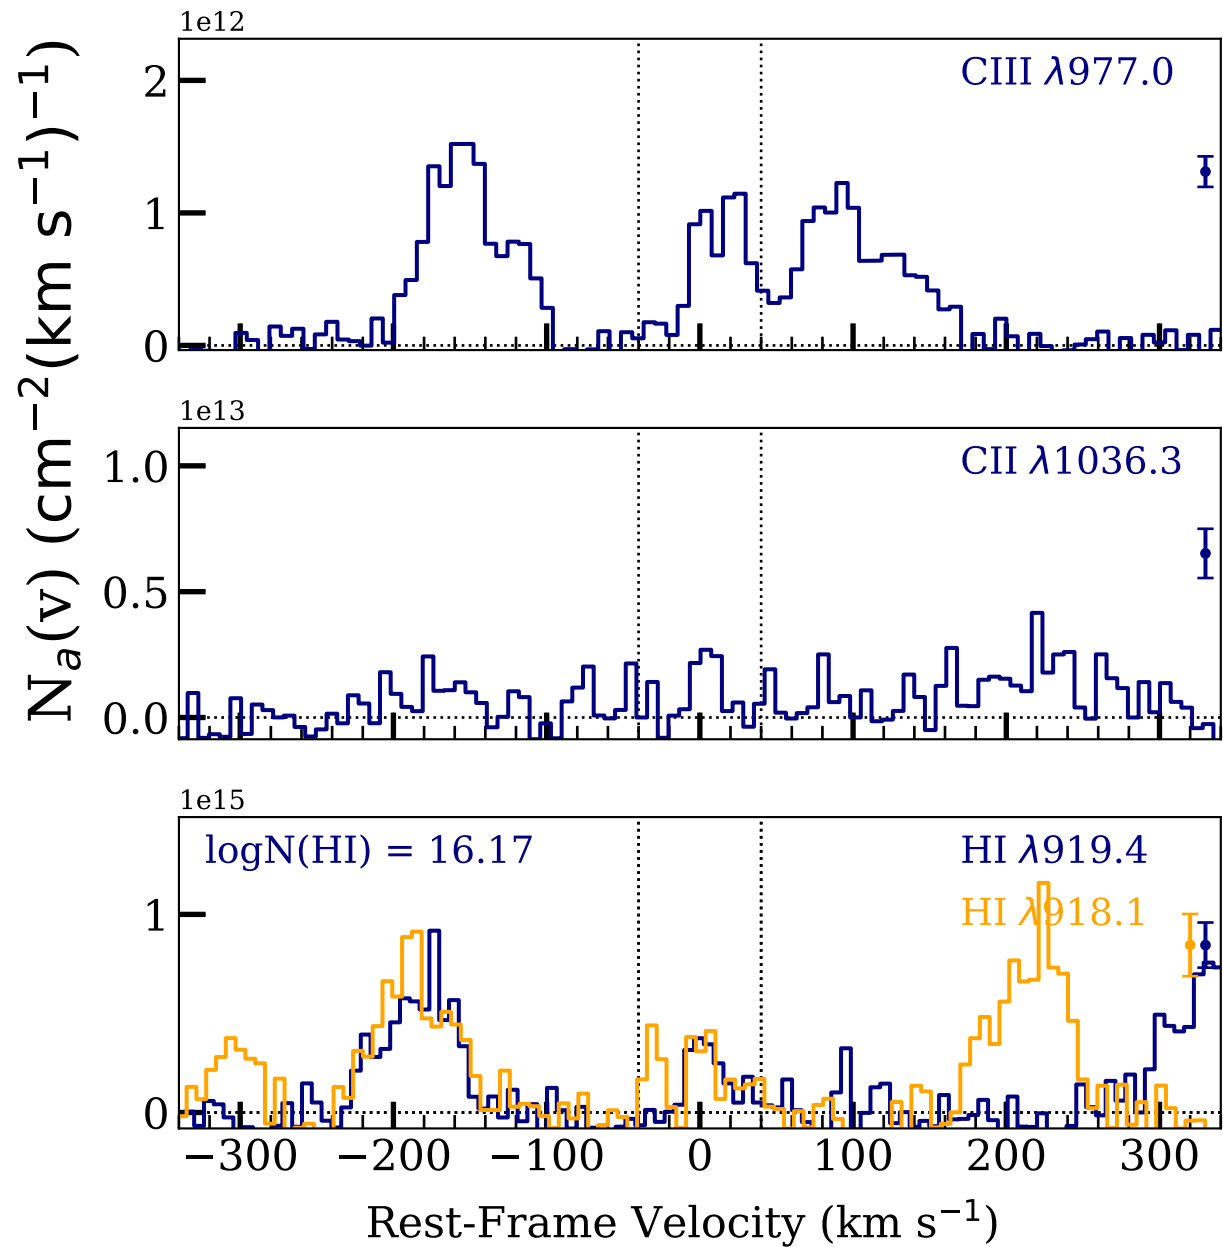

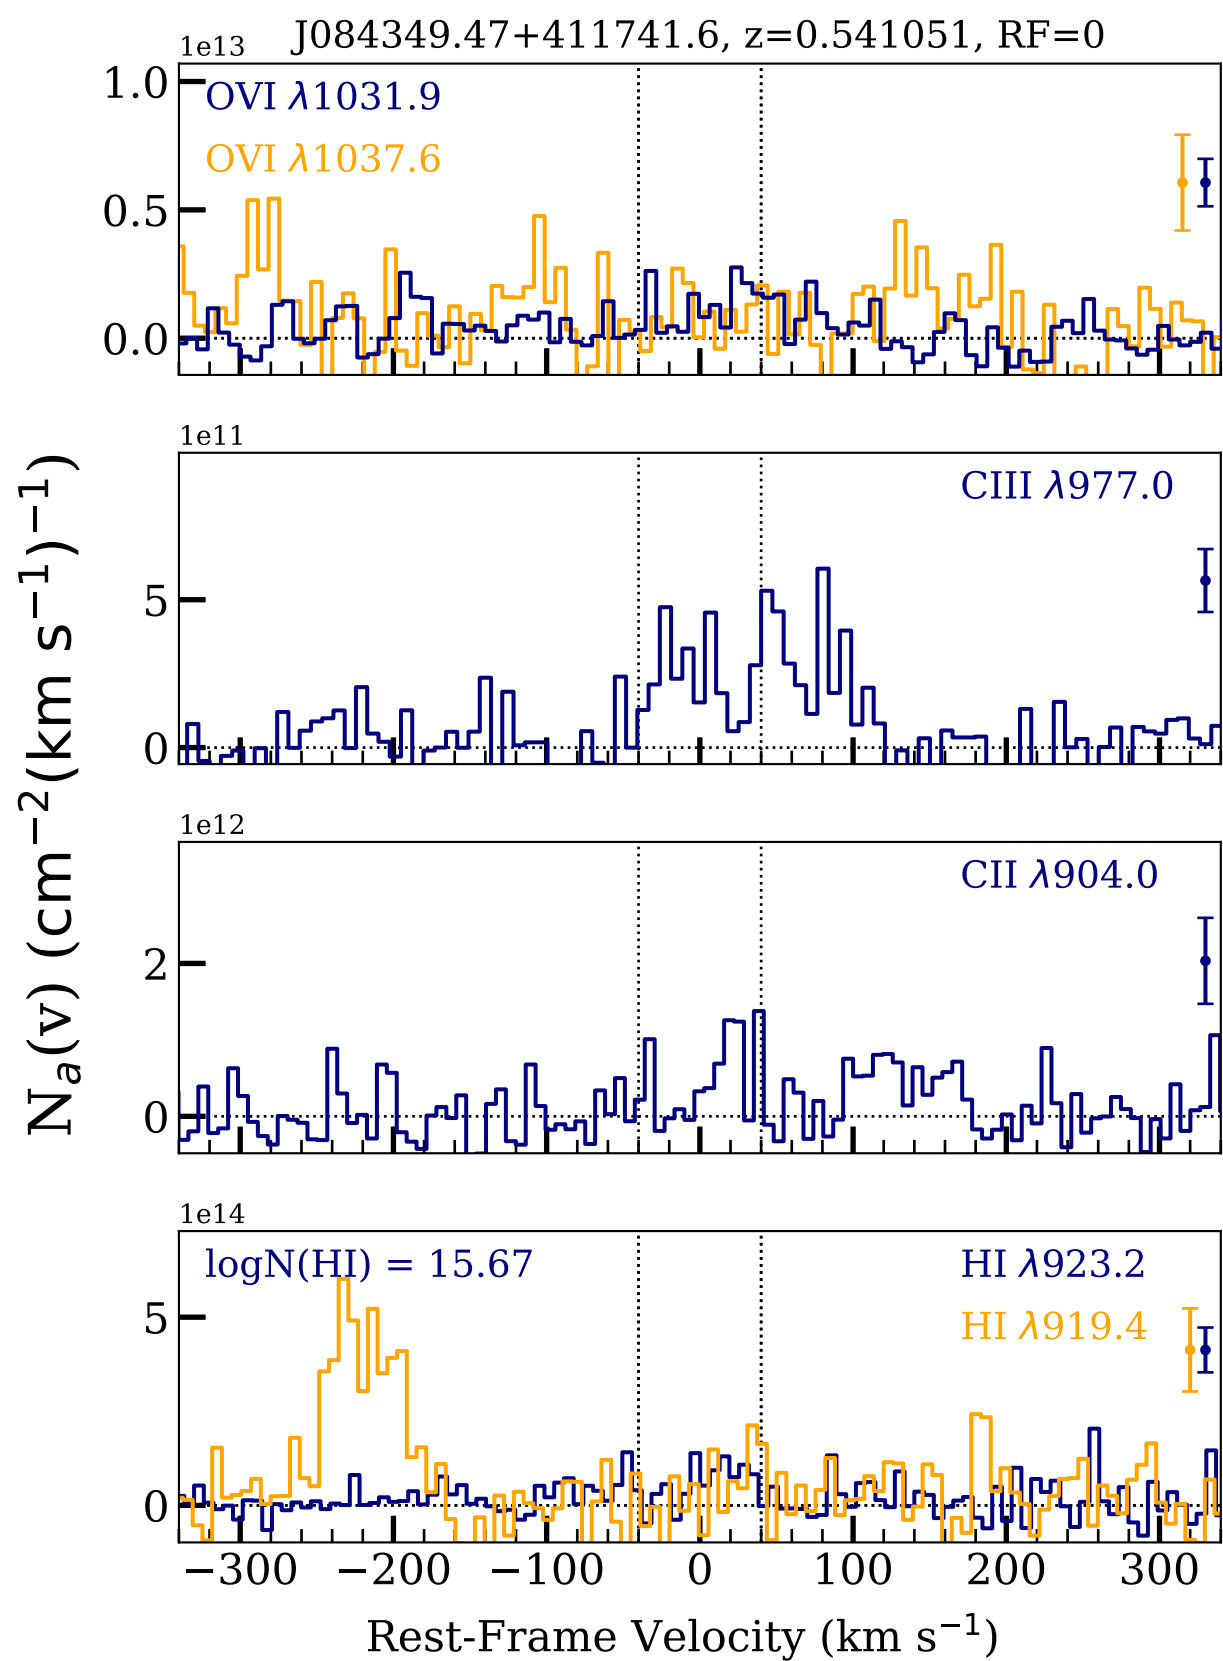



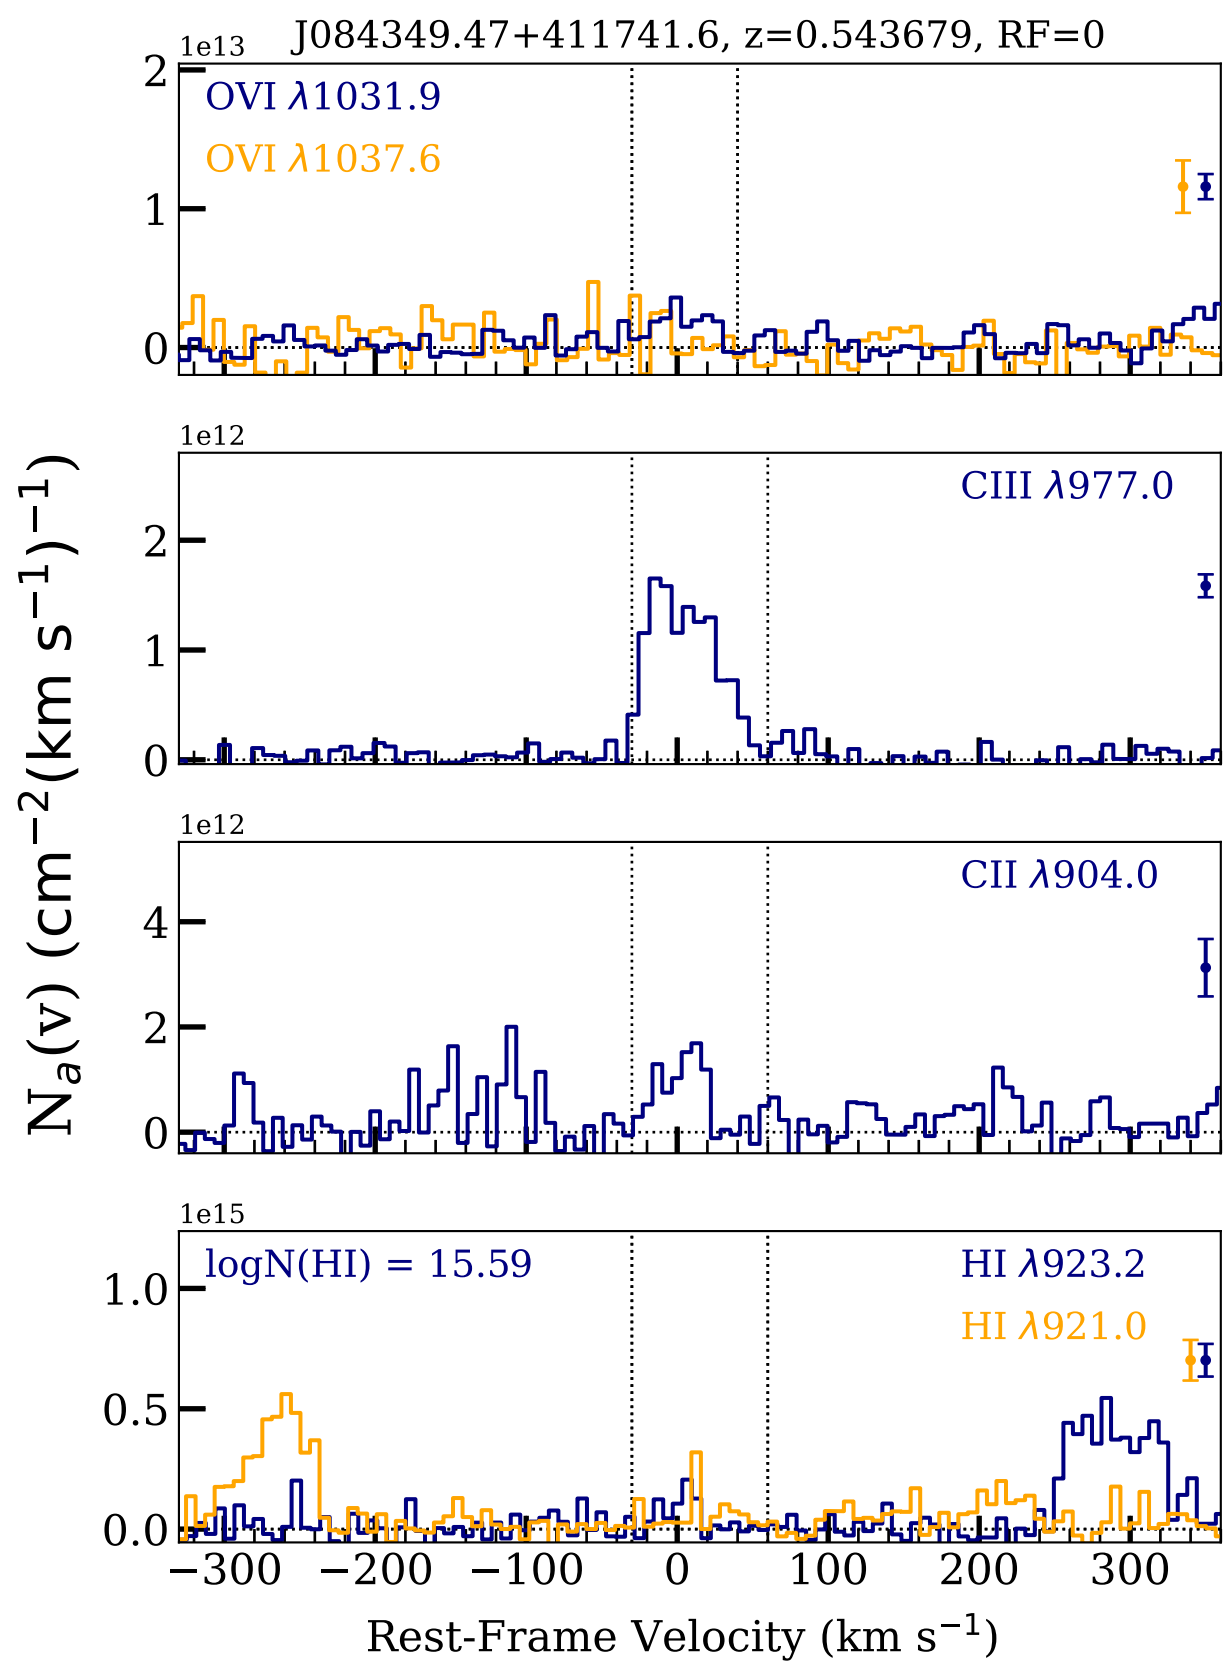

J091440.38+282330.6,  $z=0.244249$ , RF=1

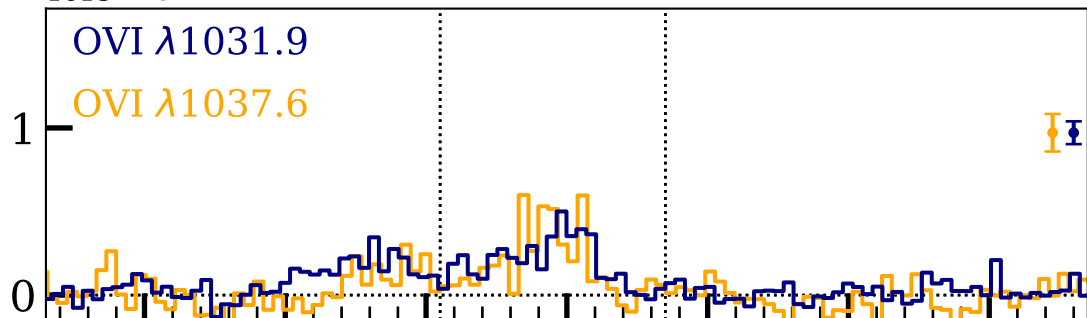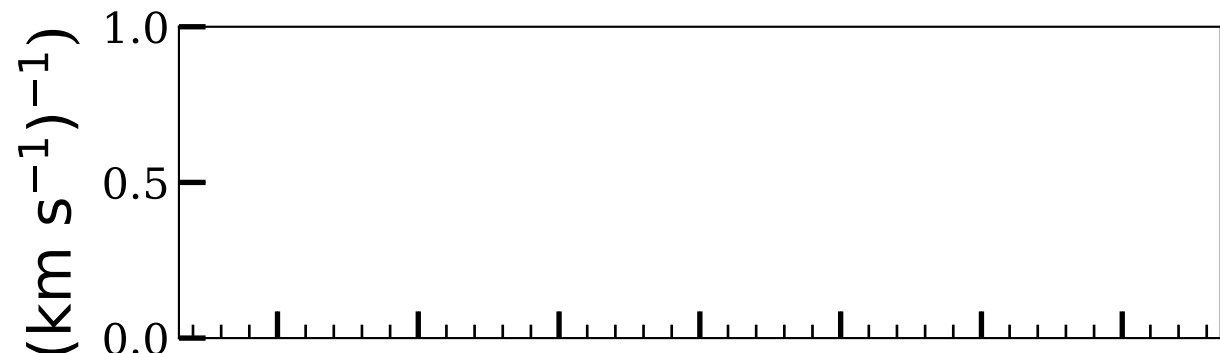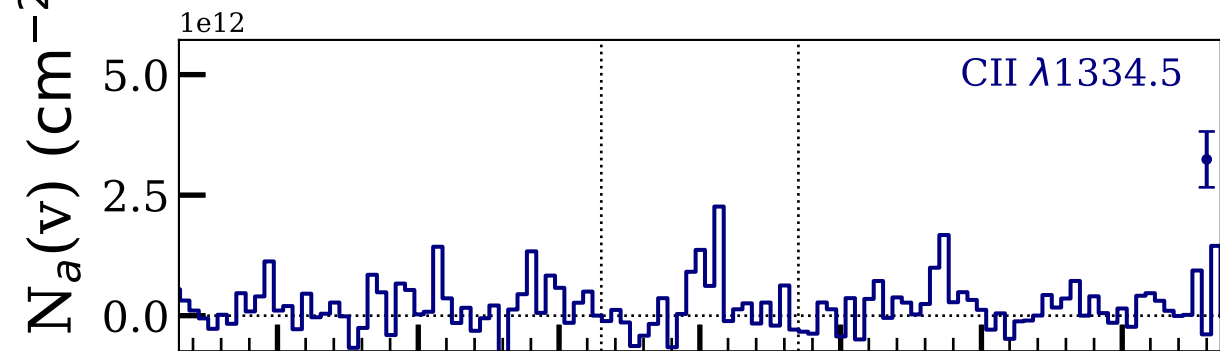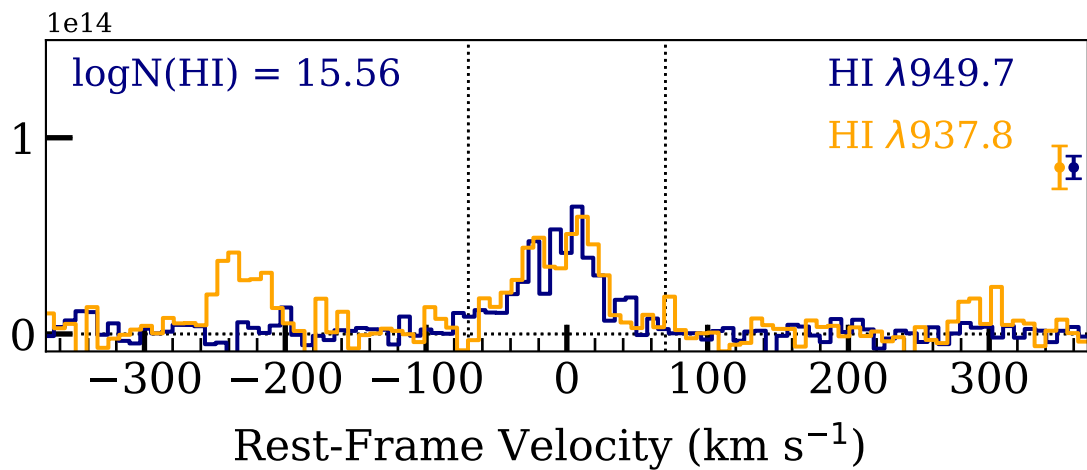

J091440.38+282330.6,  $z=0.599535$ , RF=0

$N_a(v)$  ( $\text{cm}^{-2}(\text{km s}^{-1})^{-1}$ )

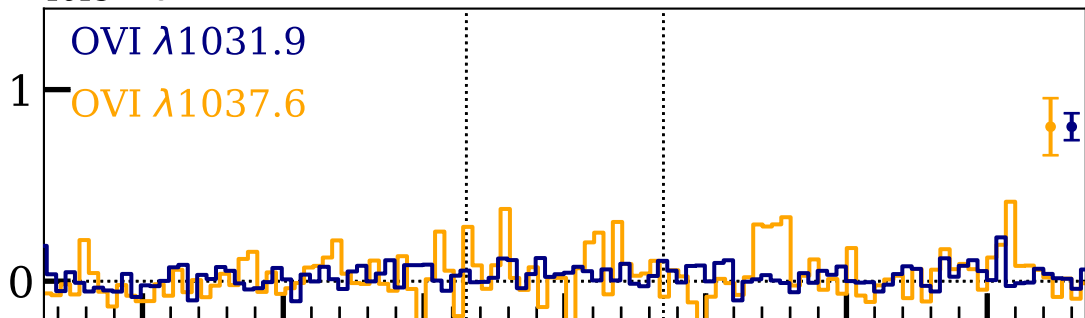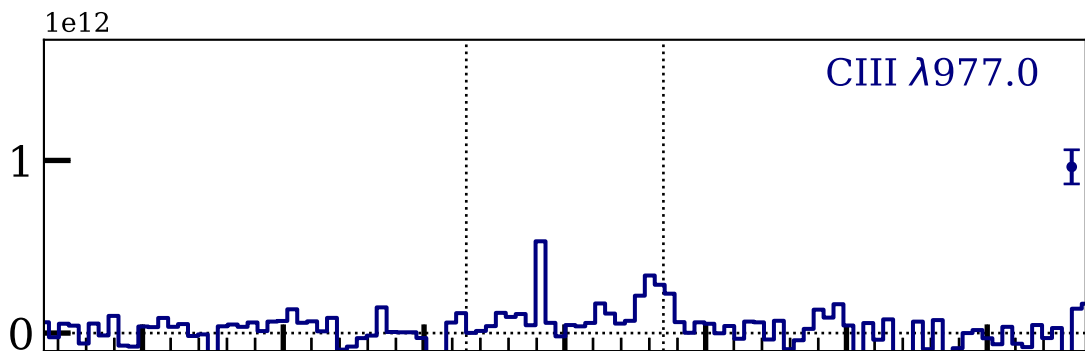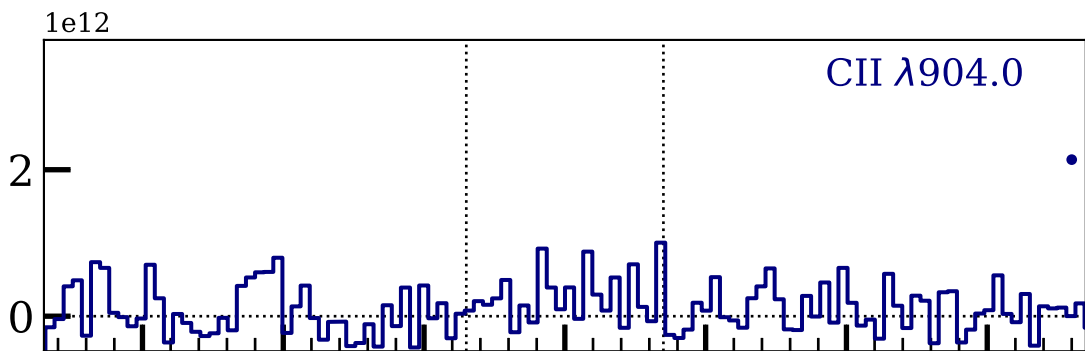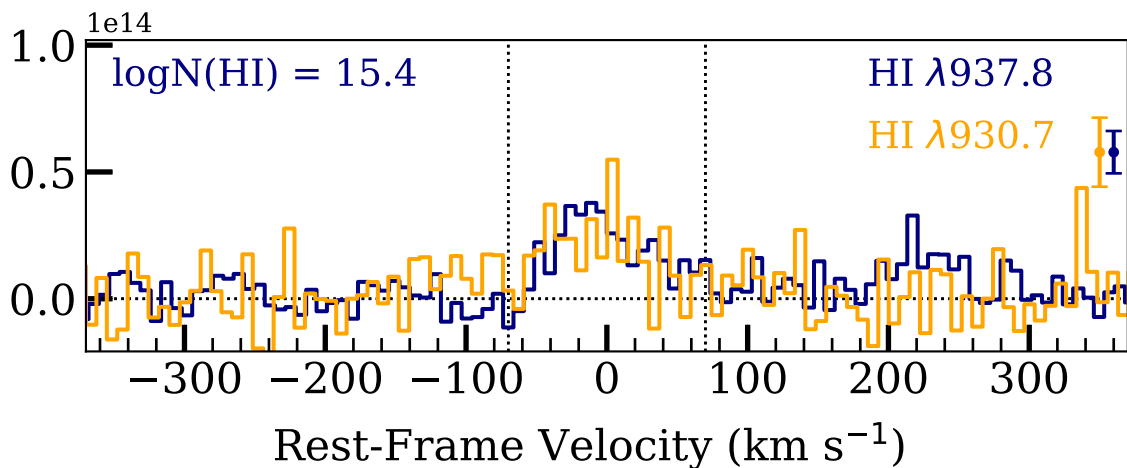

J092554.44+453544.5,  $z=0.309630$ , RF=1

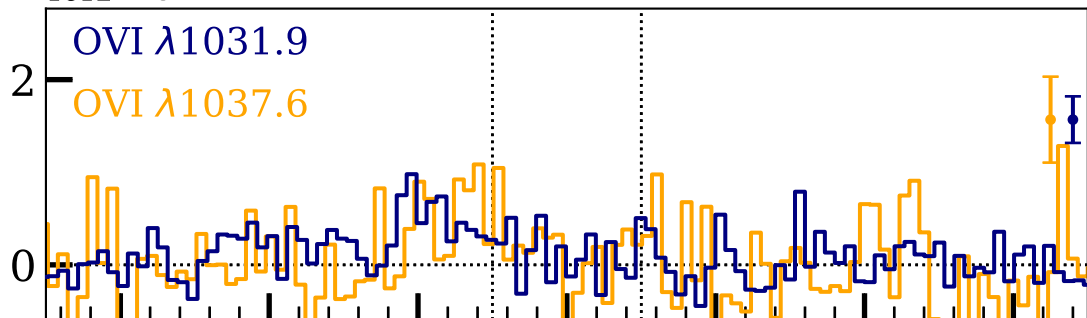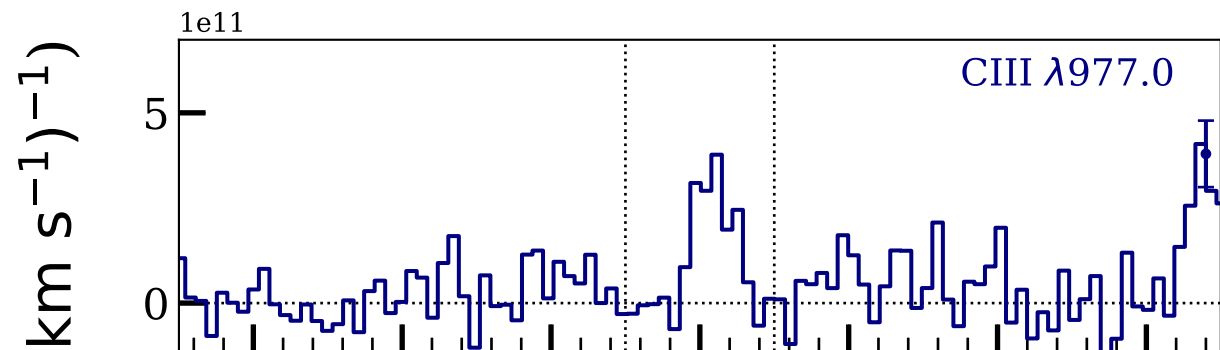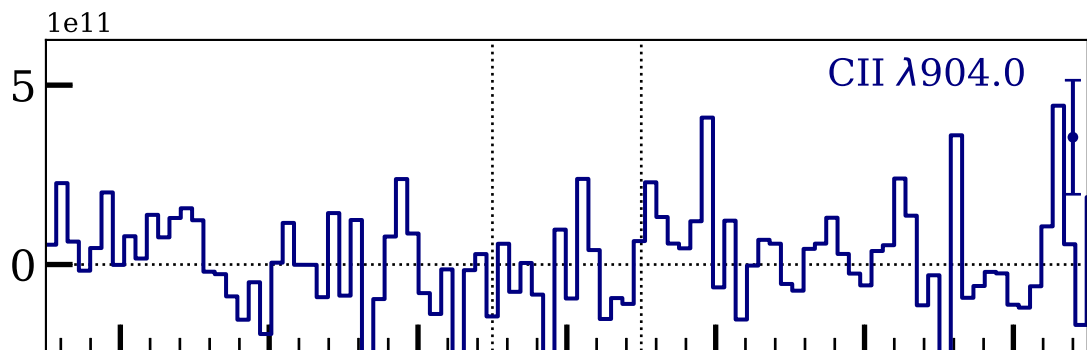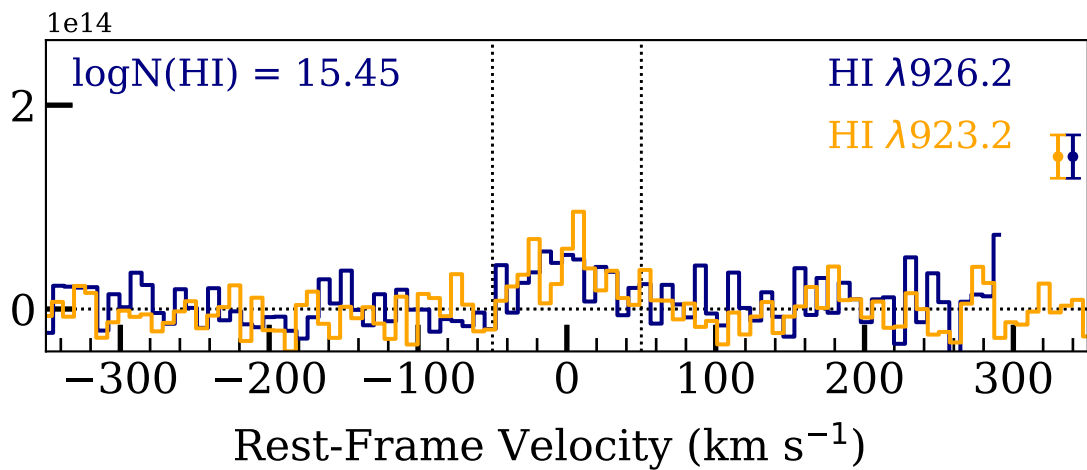

J093518.19+020415.5,  $z=0.354712$ , RF=0

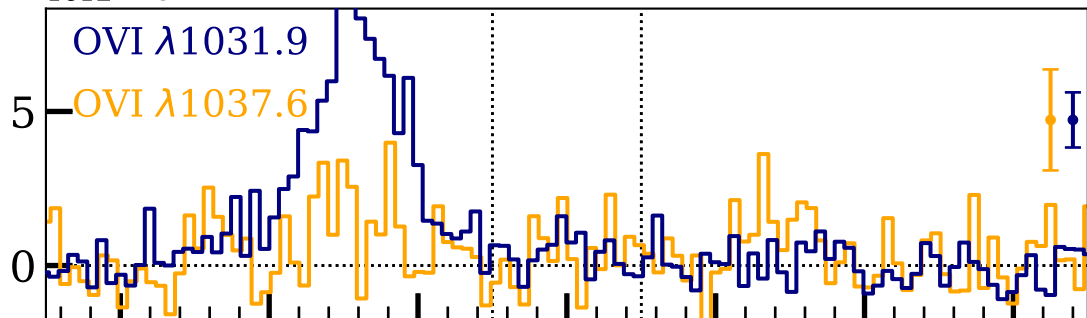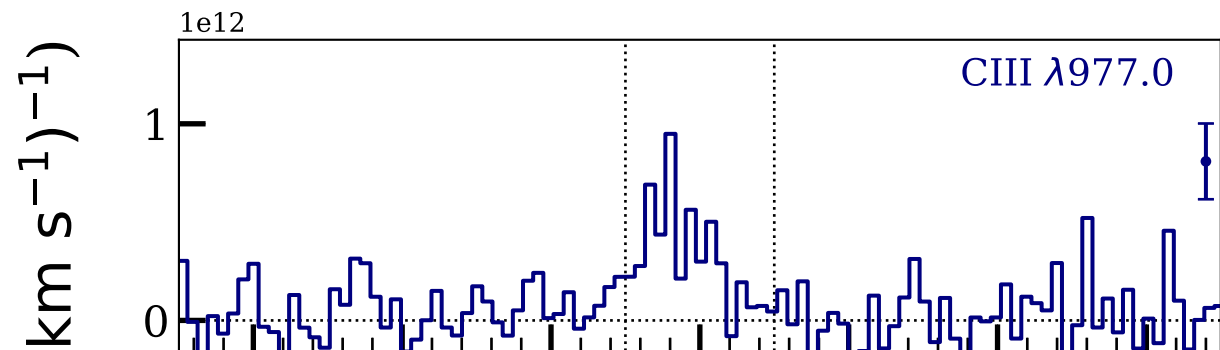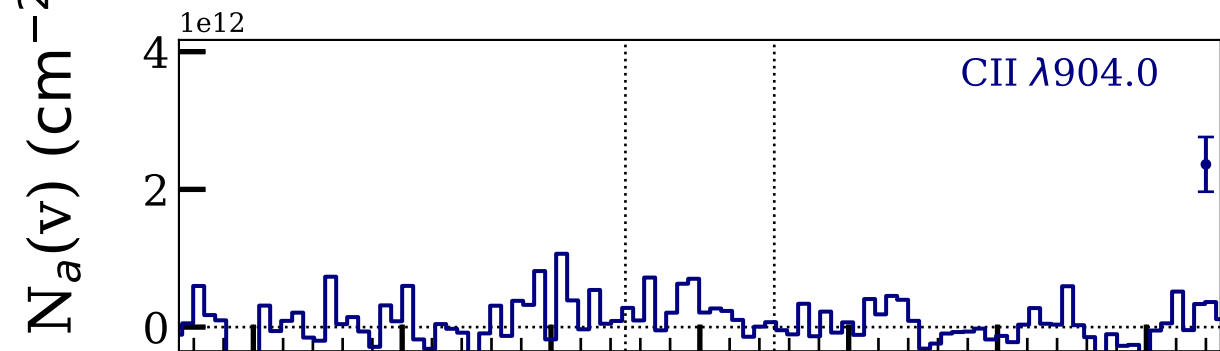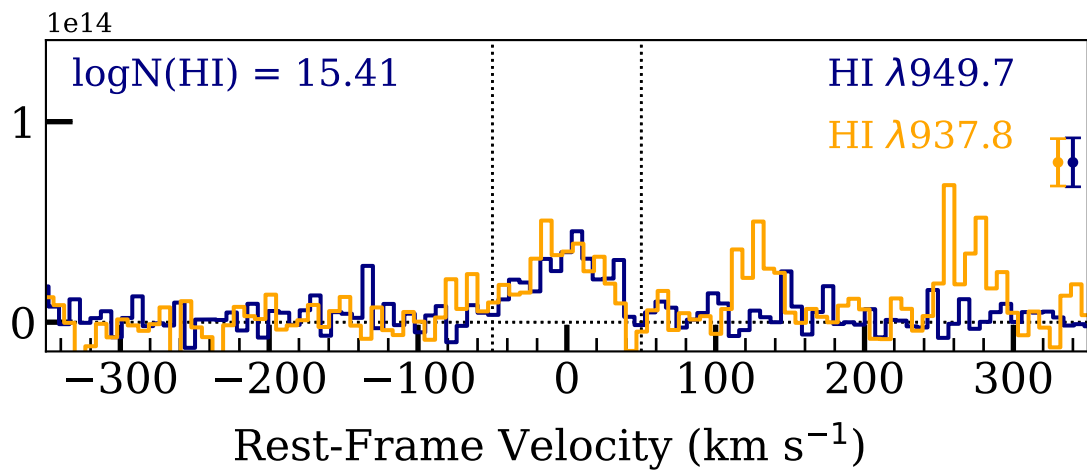

J093603.88+320709.3,  $z=0.390435$ , RF=0

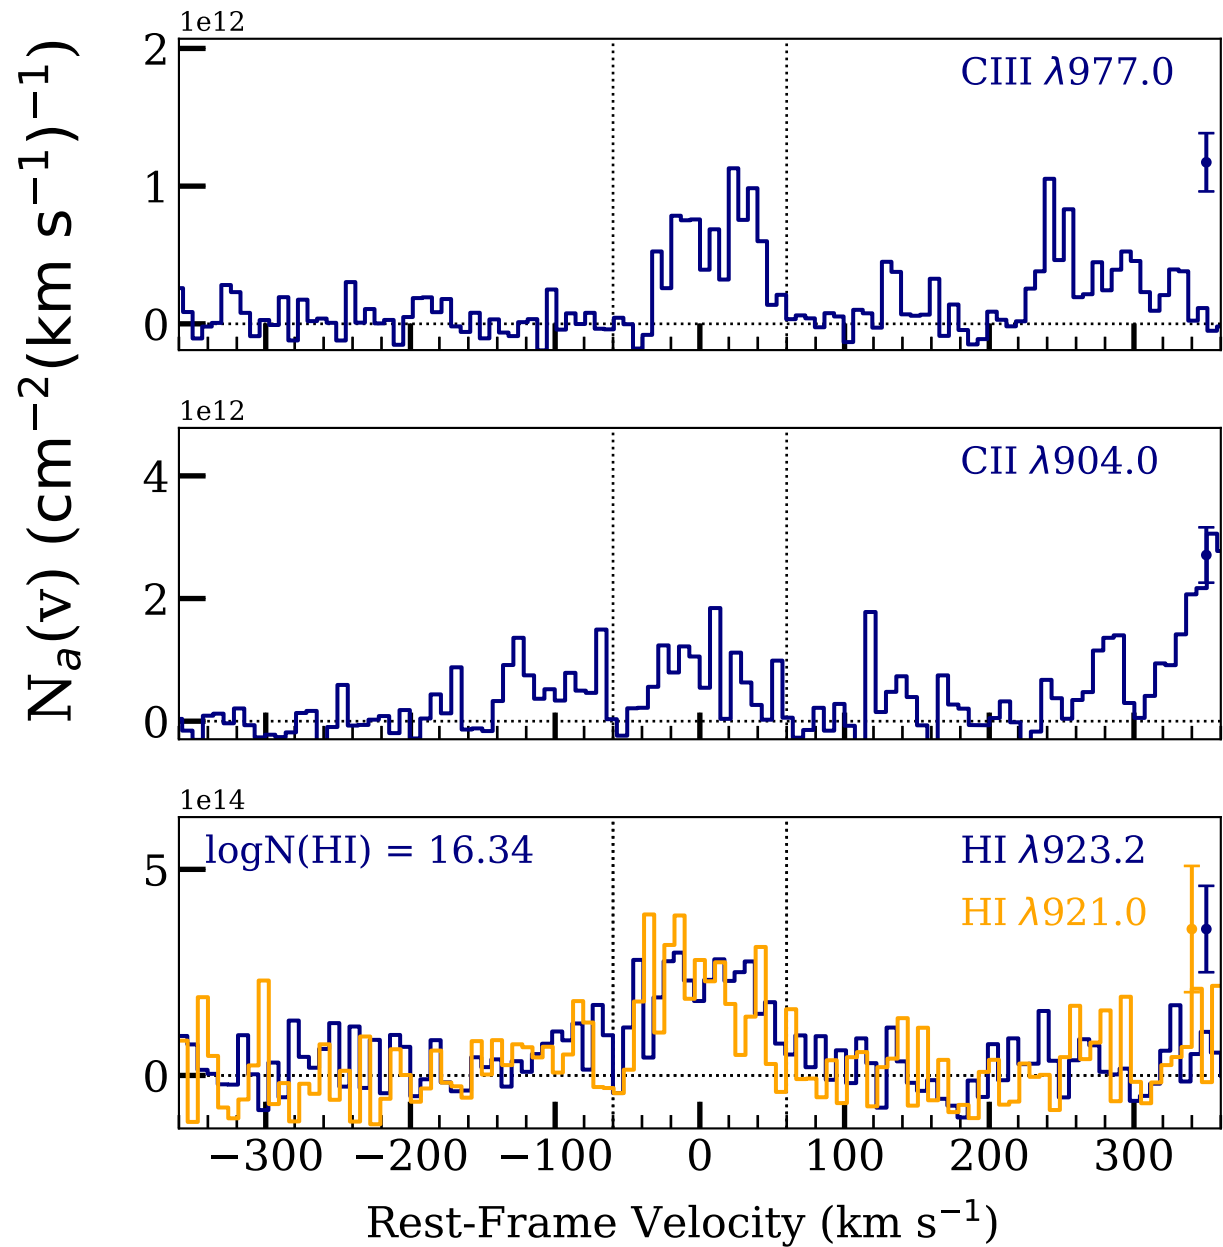

J094331.61+053131.4,  $z=0.229019$ , RF=1

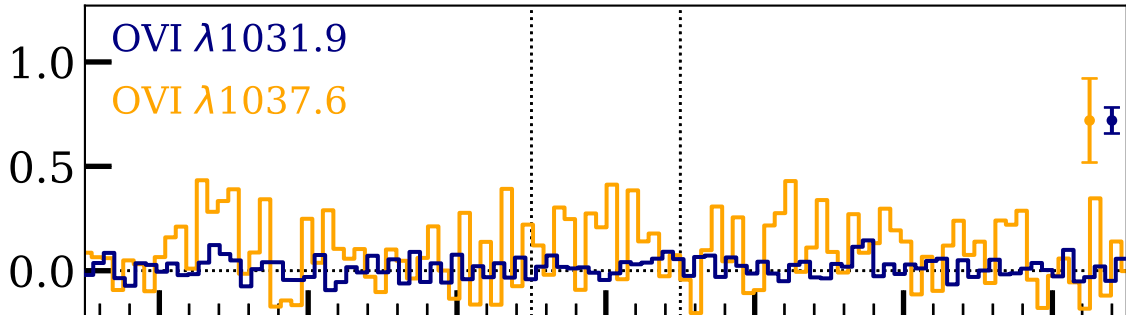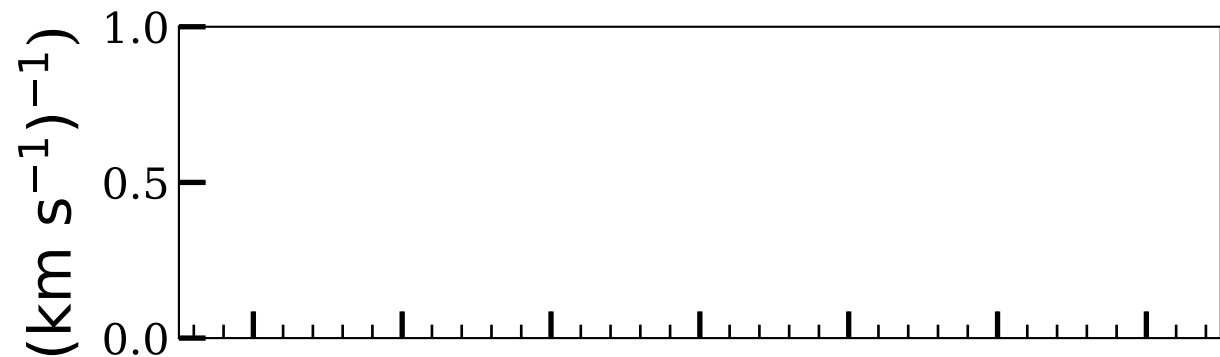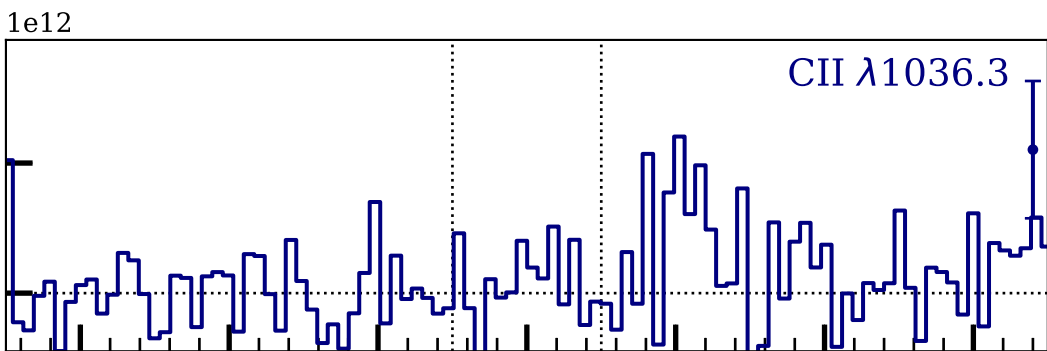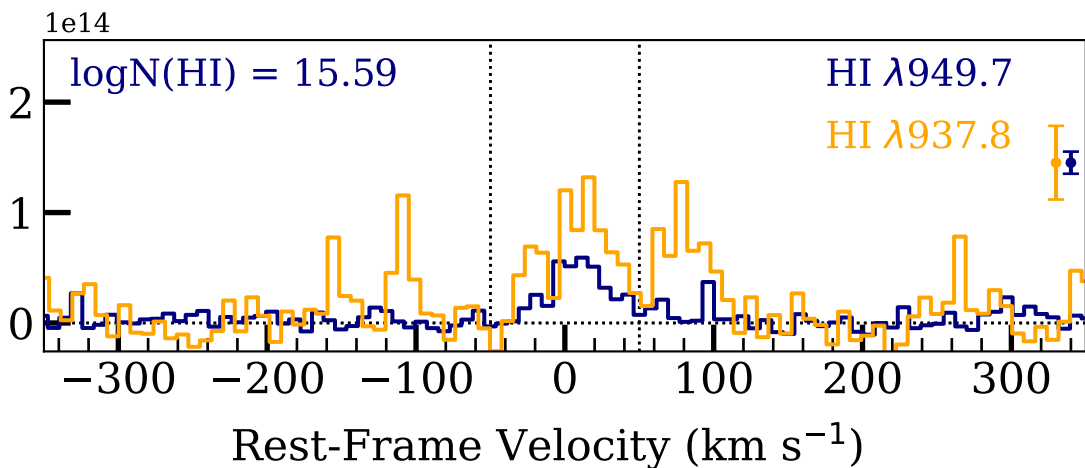

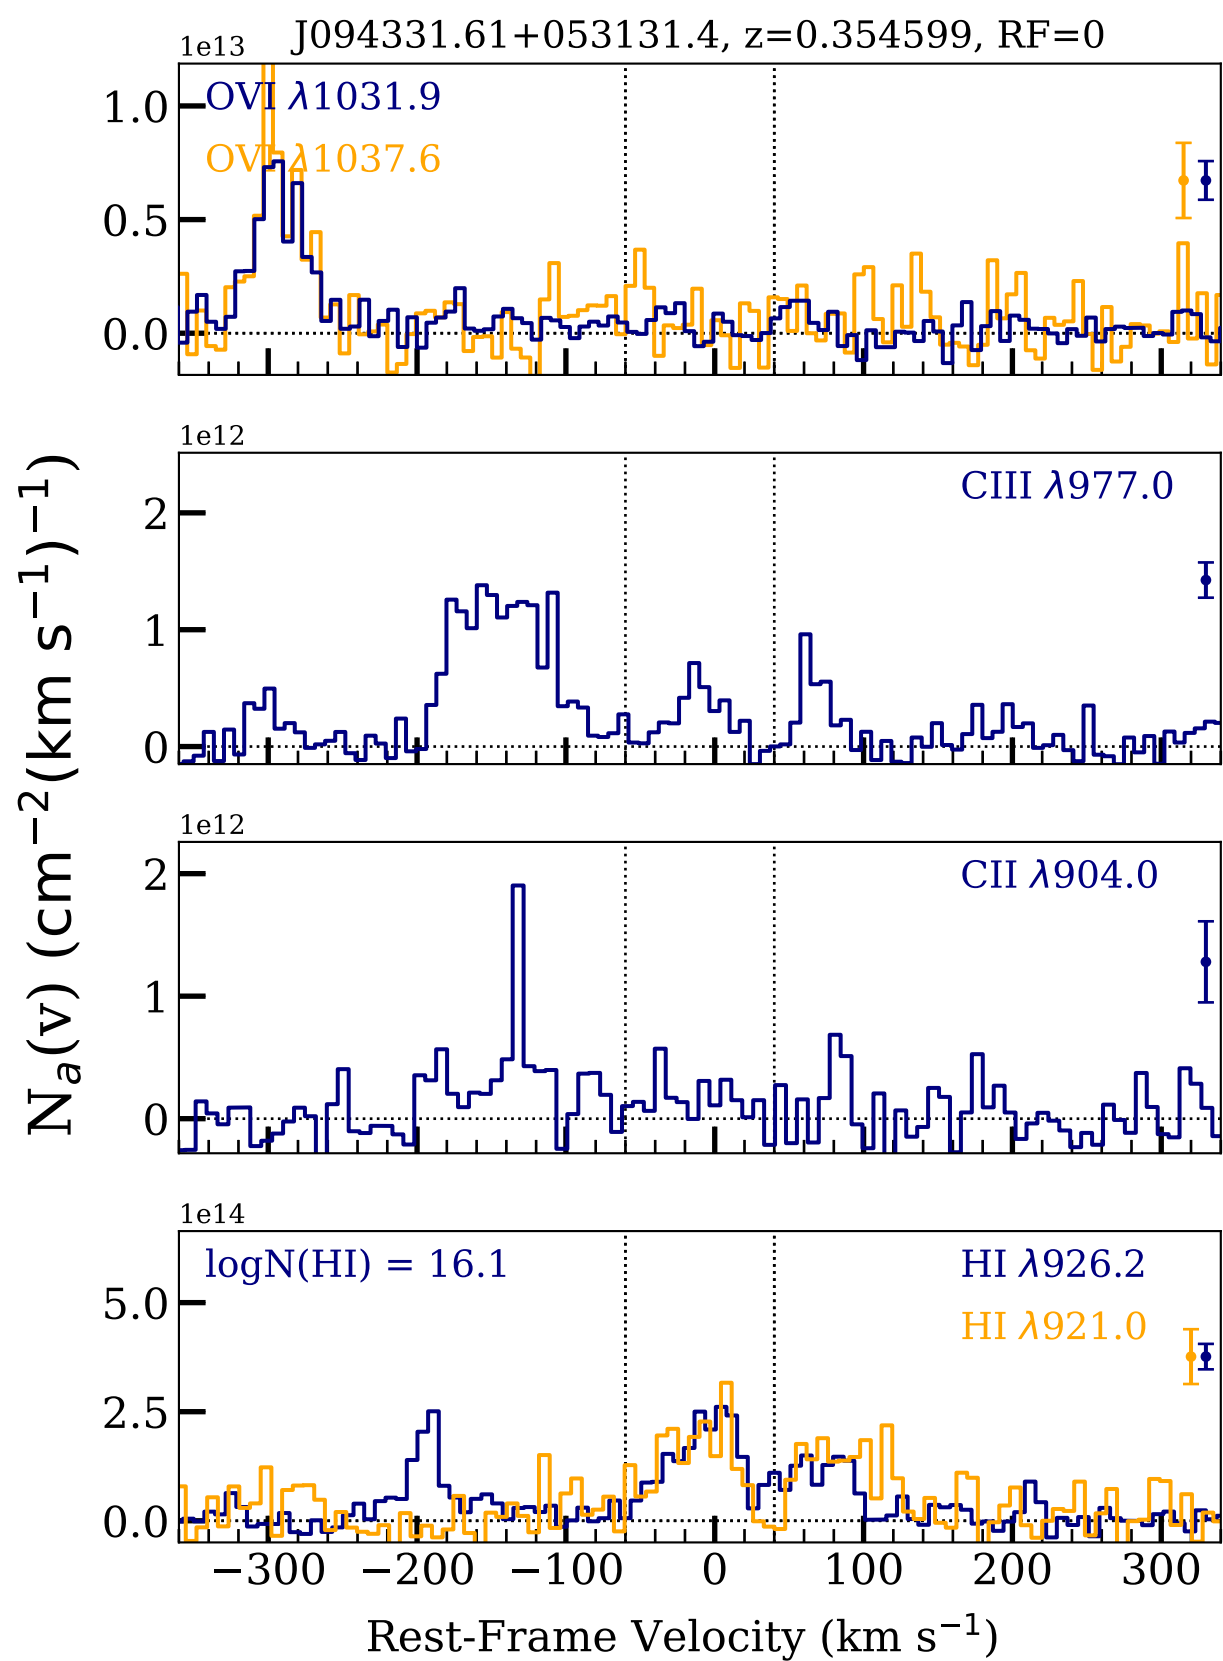



J094331.61+053131.4,  $z=0.354927$ , RF=0

$N_a(v) \text{ (cm}^{-2} \text{ (km s}^{-1} \text{)}^{-1} \text{)}$

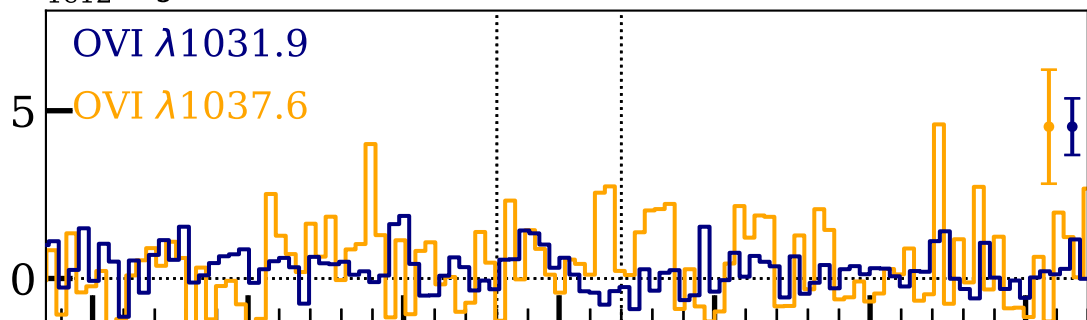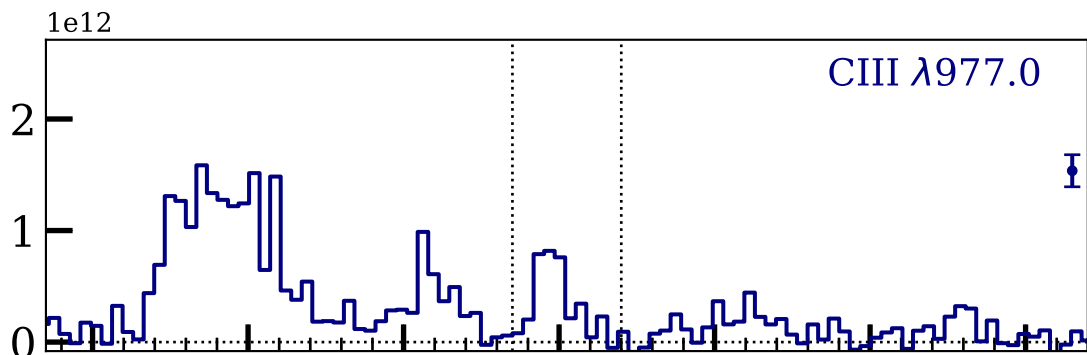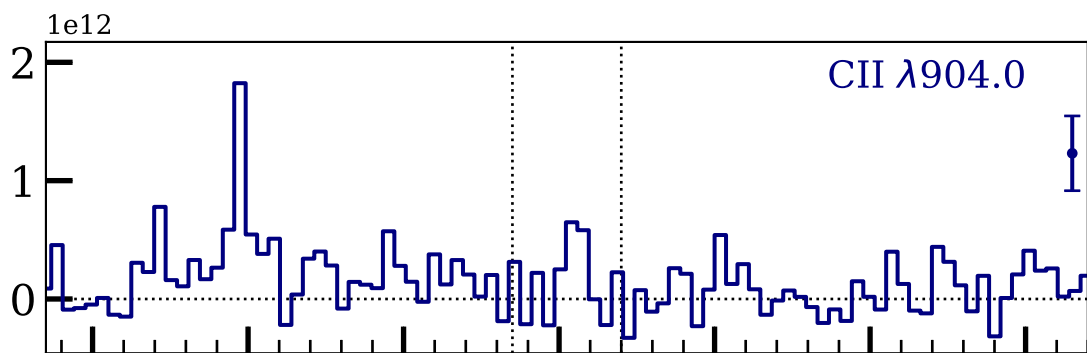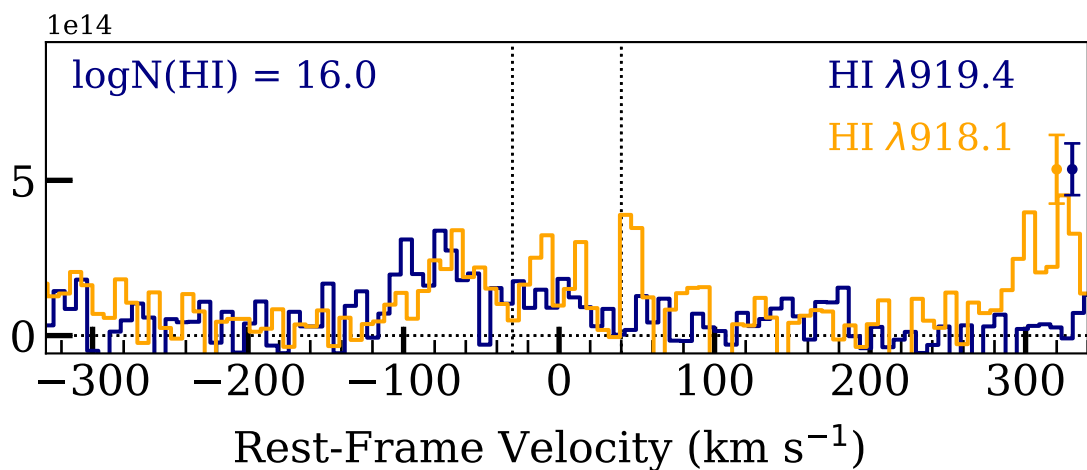

J100102.64+594414.2,  $z=0.415649$ , RF=1

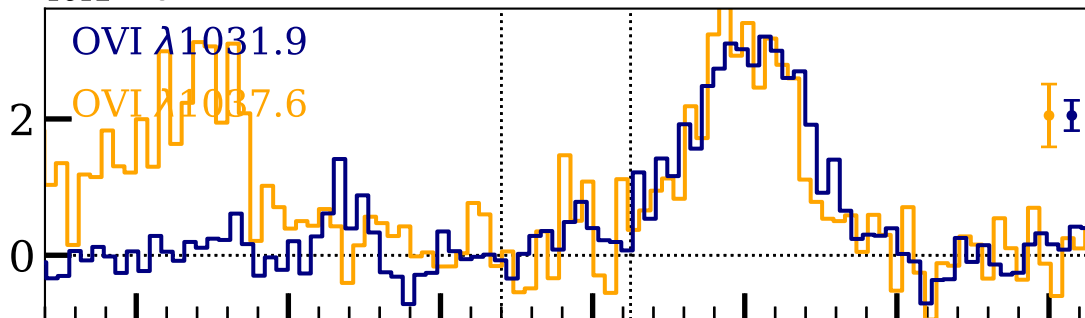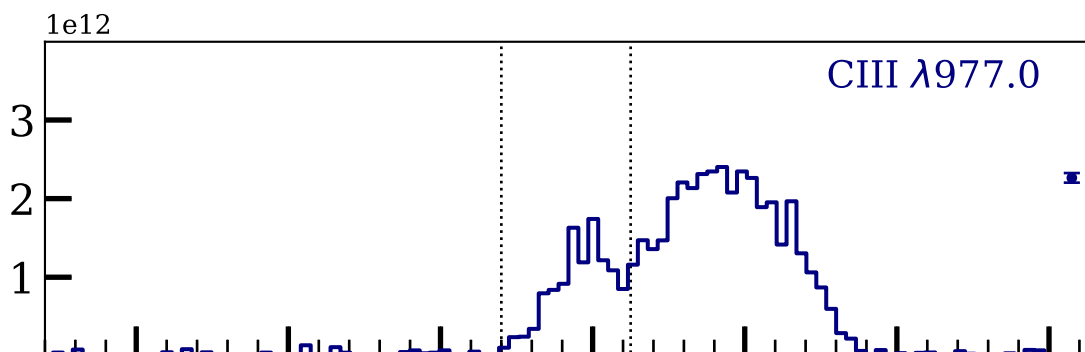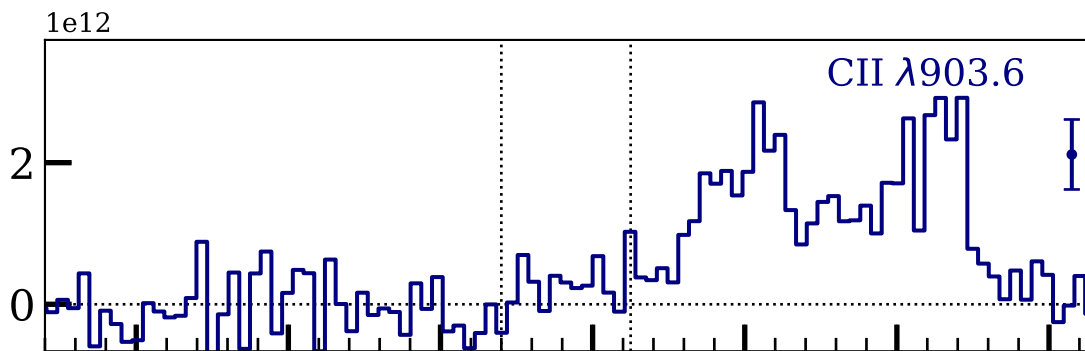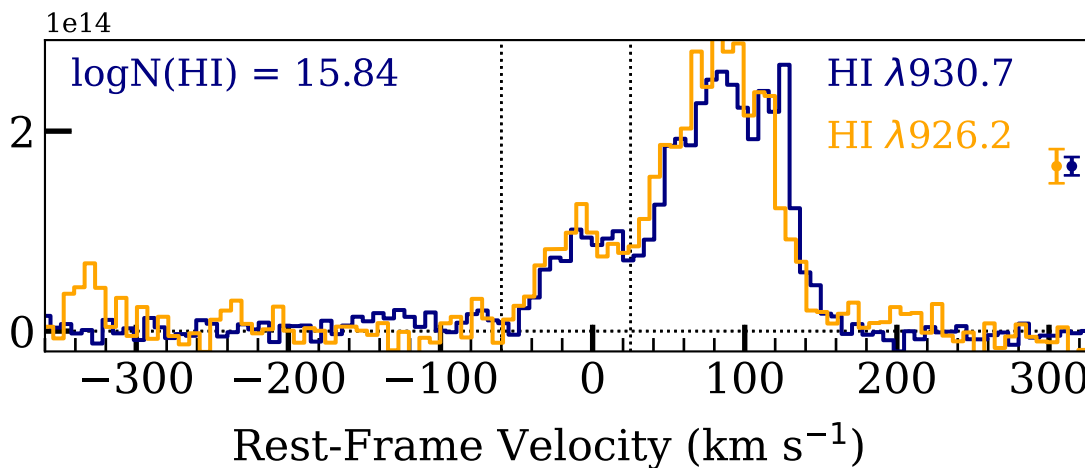

J100102.64+594414.2,  $z=0.416042$ , RF=1

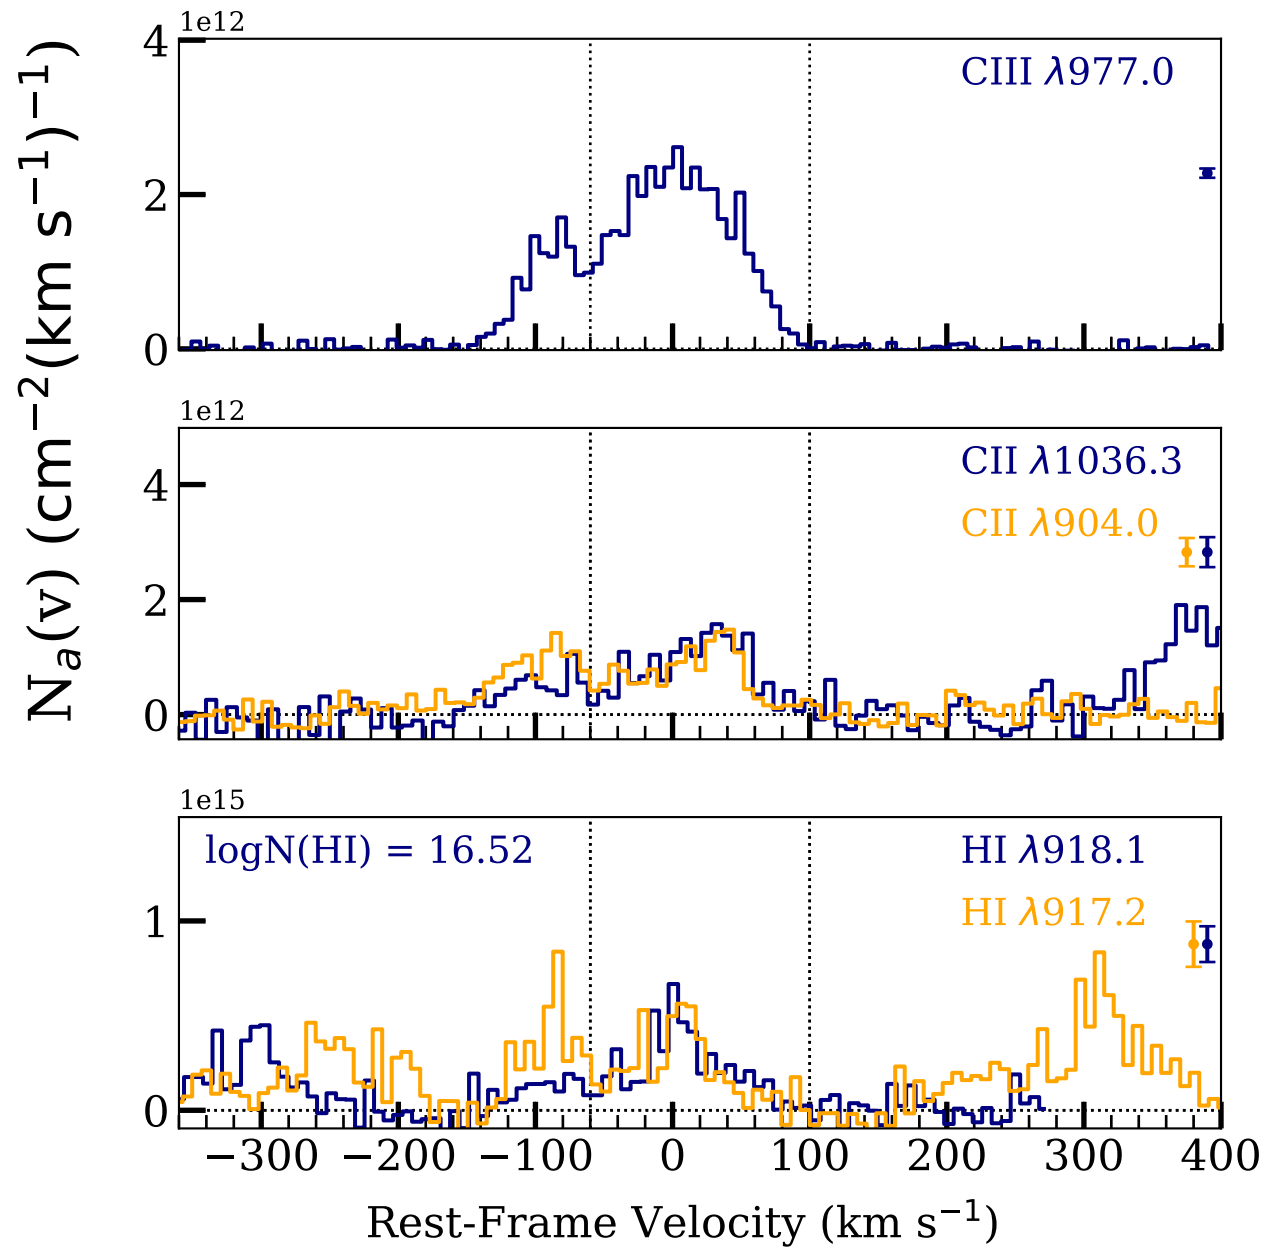

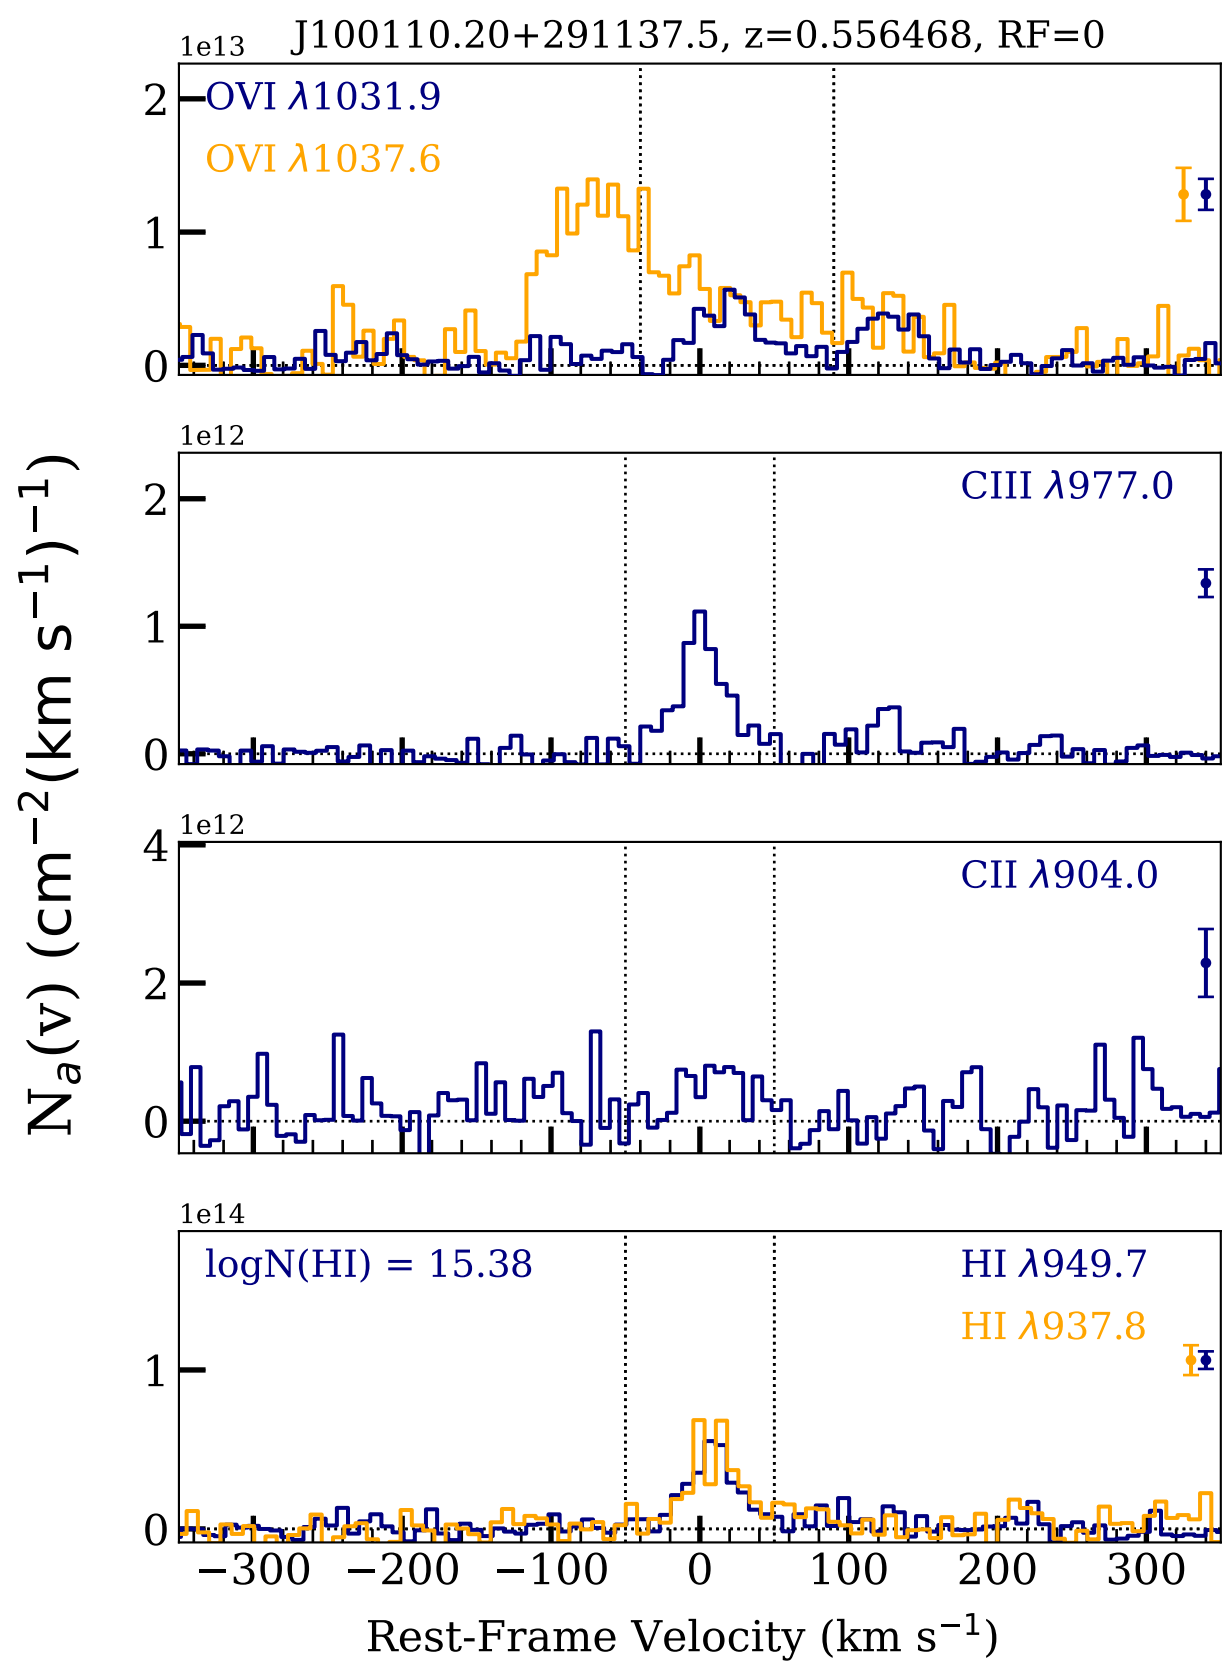

J100535.25+013445.5,  $z=0.418522$ , RF=1

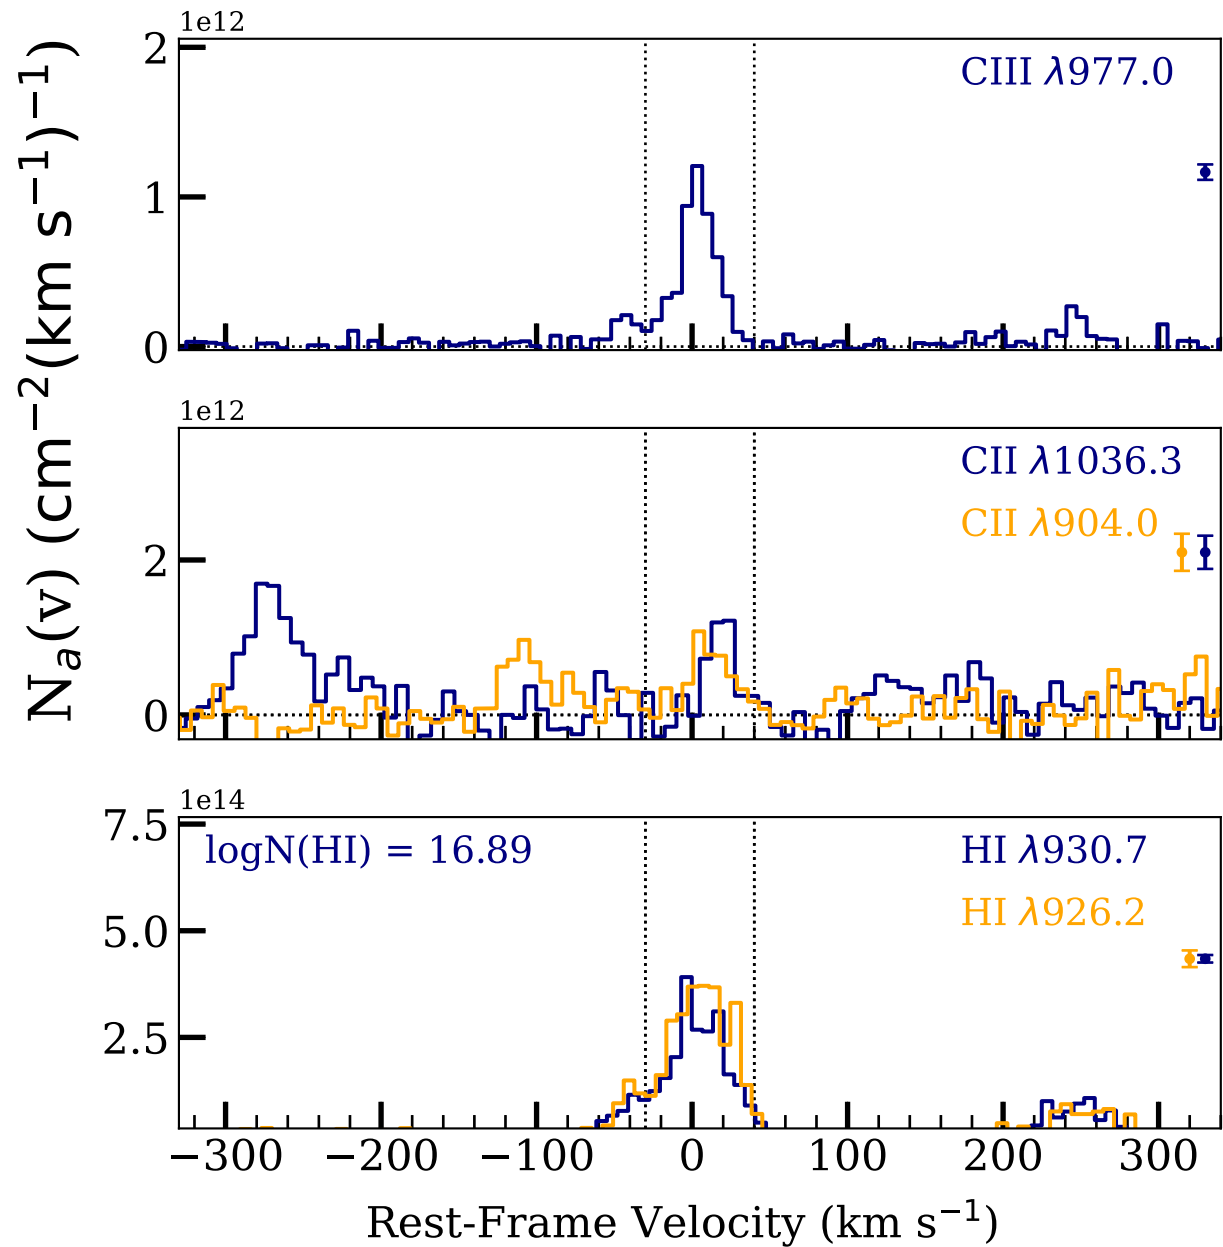

J100535.25+013445.5,  $z=0.419686$ , RF=1

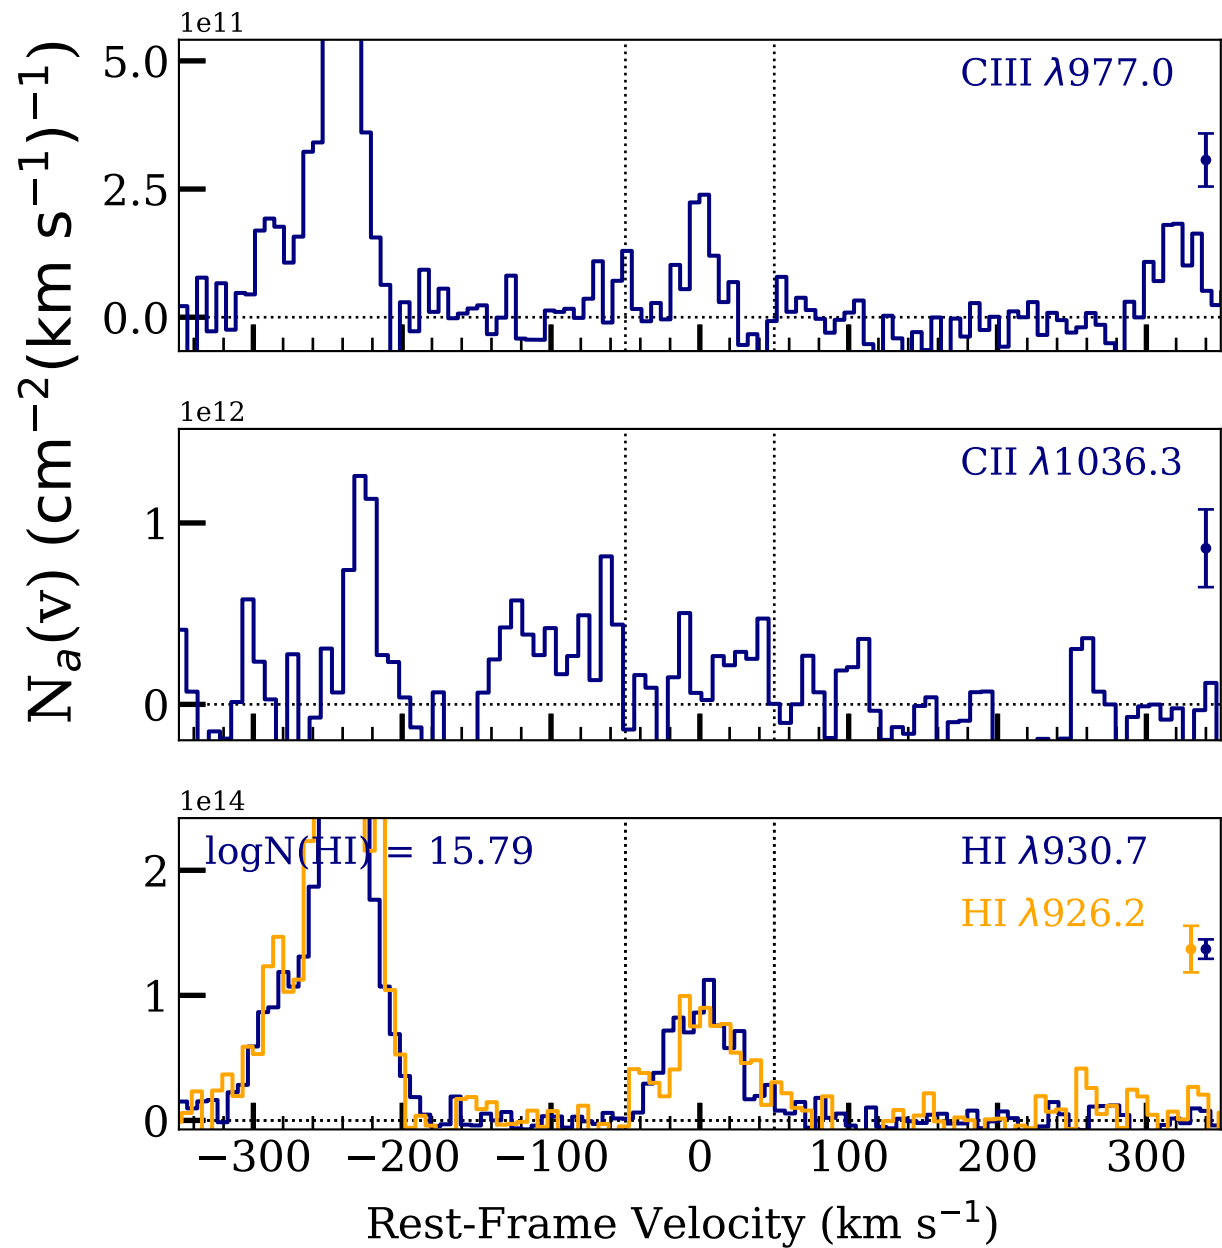

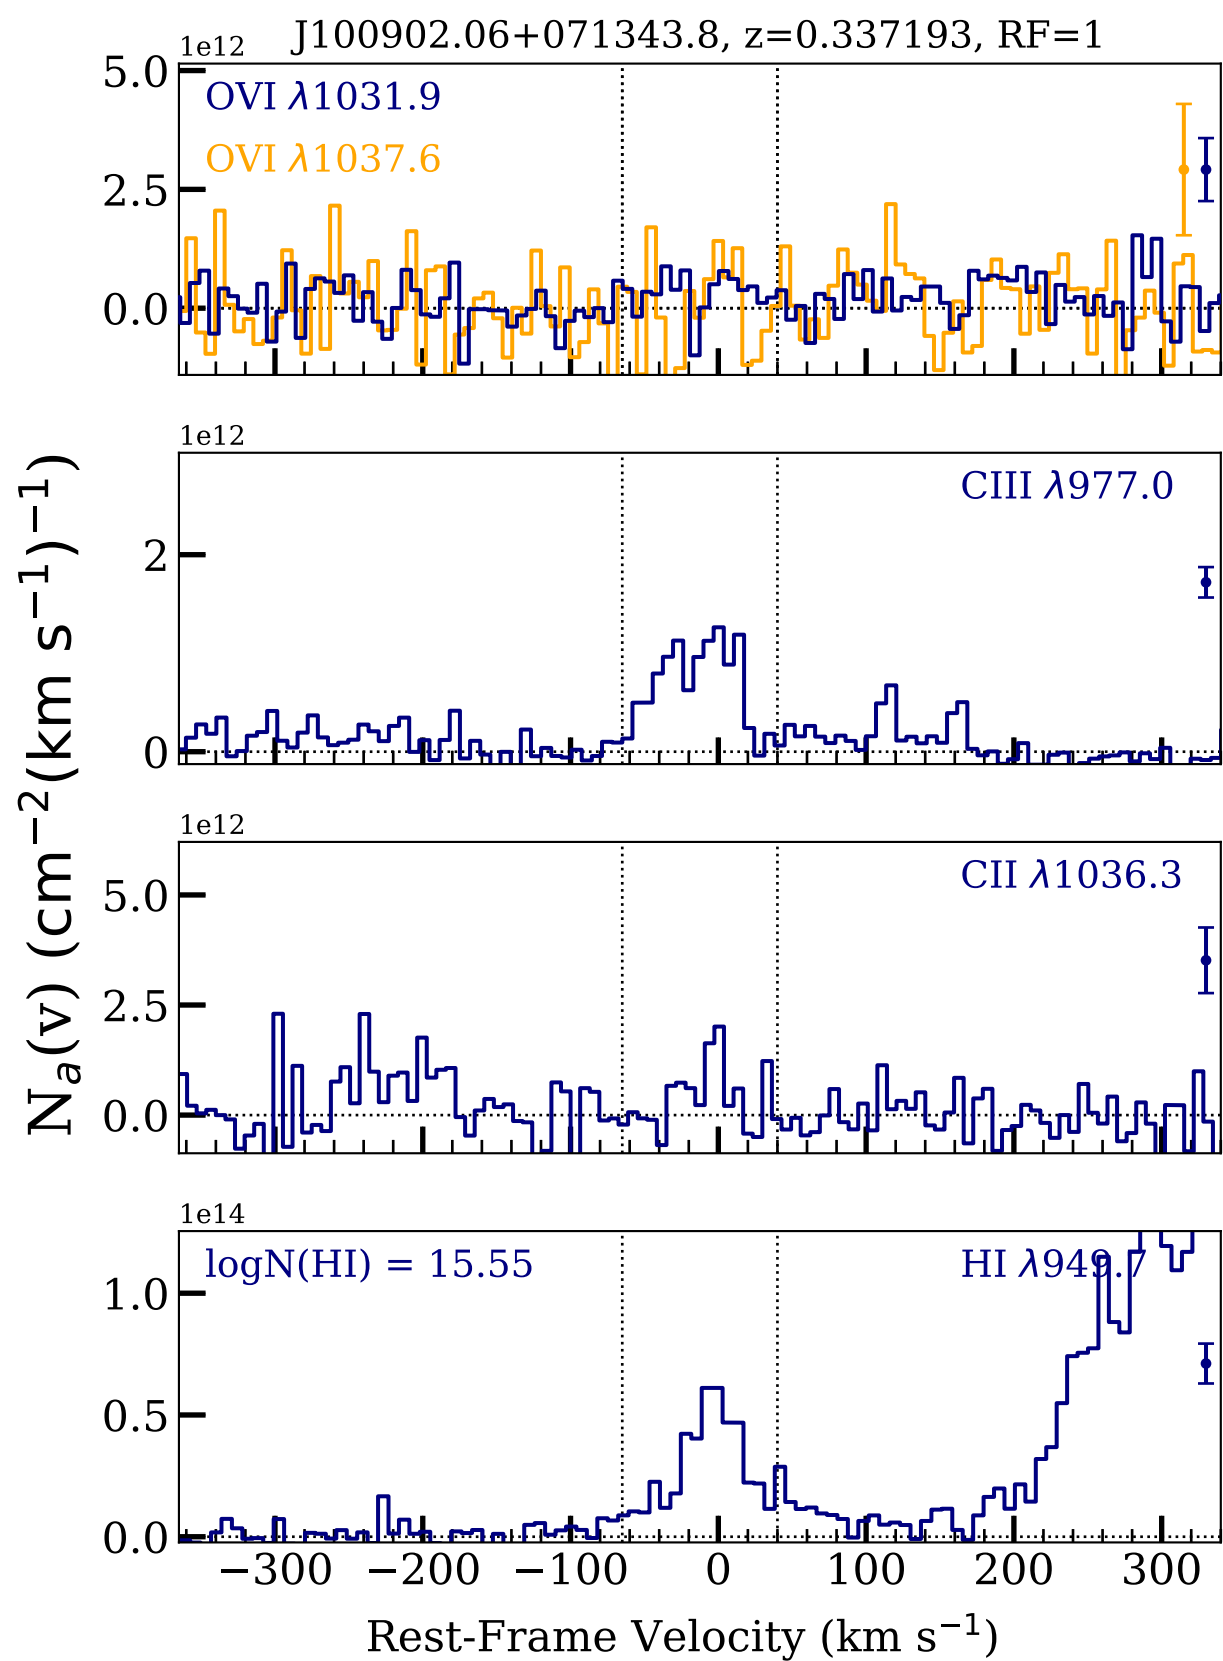

J100902.06+071343.8,  $z=0.355352$ , RF=0

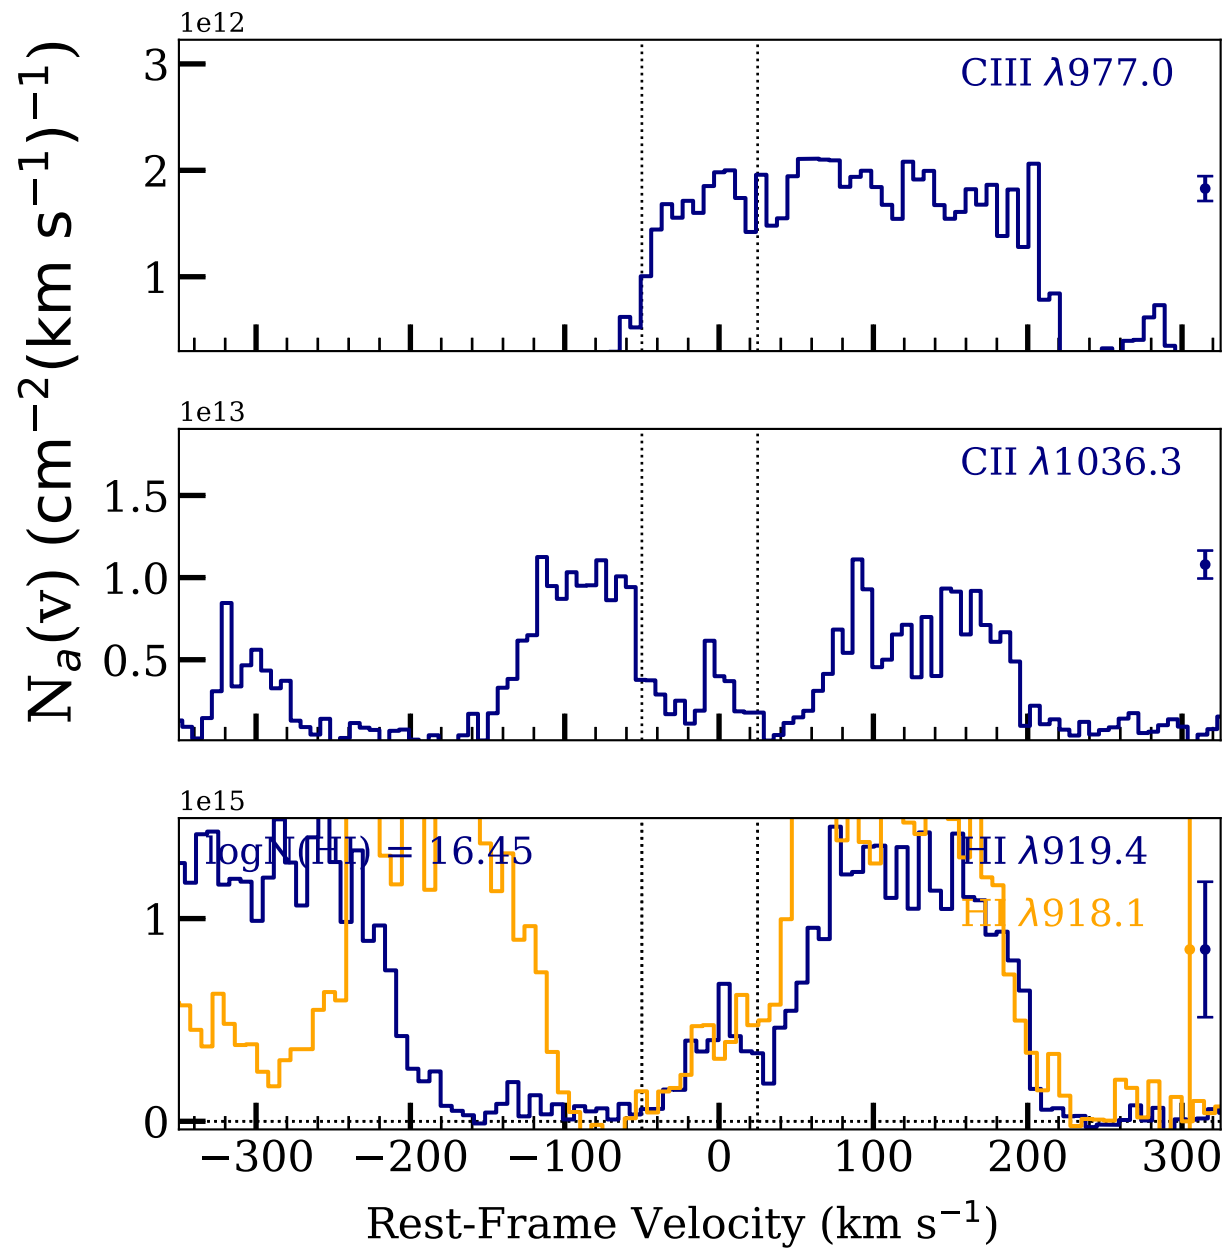



J101622.60+470643.3,  $z=0.263820$ , RF=0

$N_a(v)$  ( $\text{cm}^{-2}(\text{km s}^{-1})^{-1}$ )

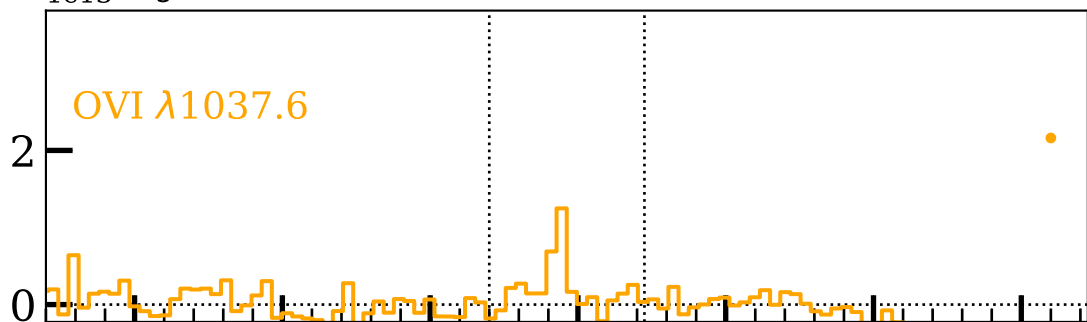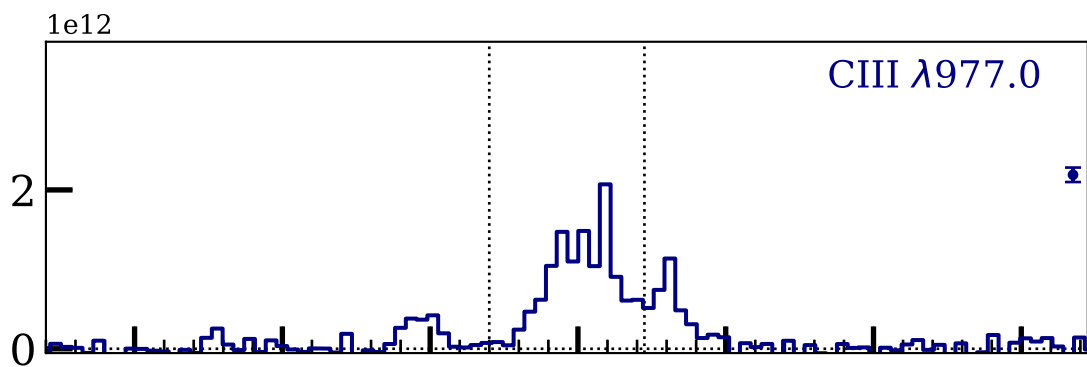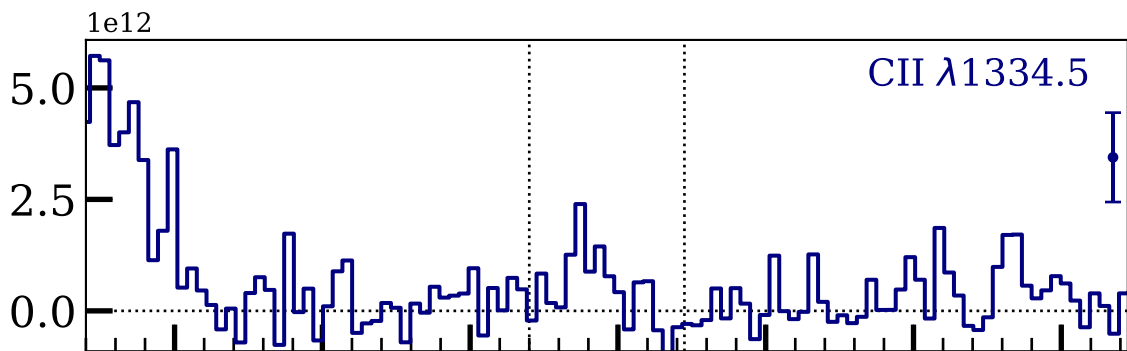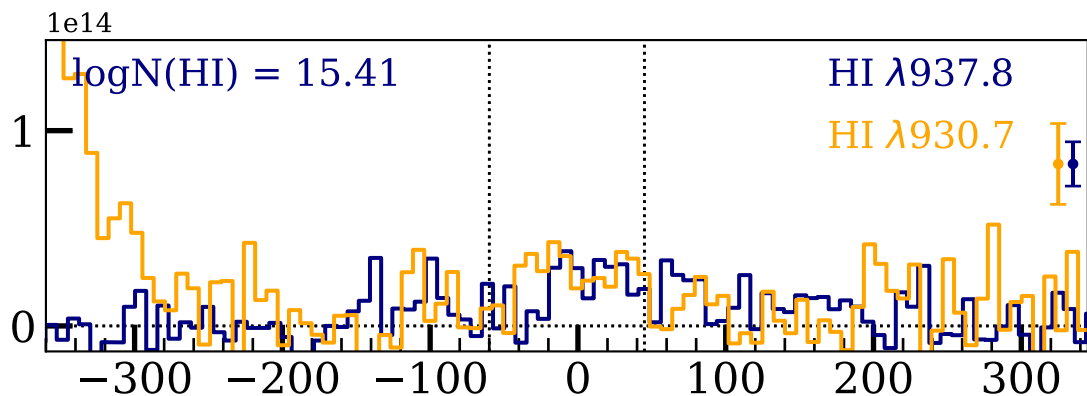

Rest-Frame Velocity ( $\text{km s}^{-1}$ )

J101622.60+470643.3,  $z=0.432210$ , RF=1

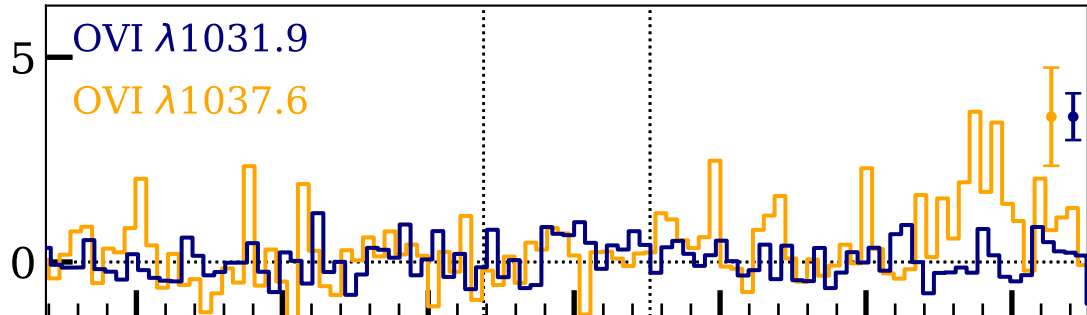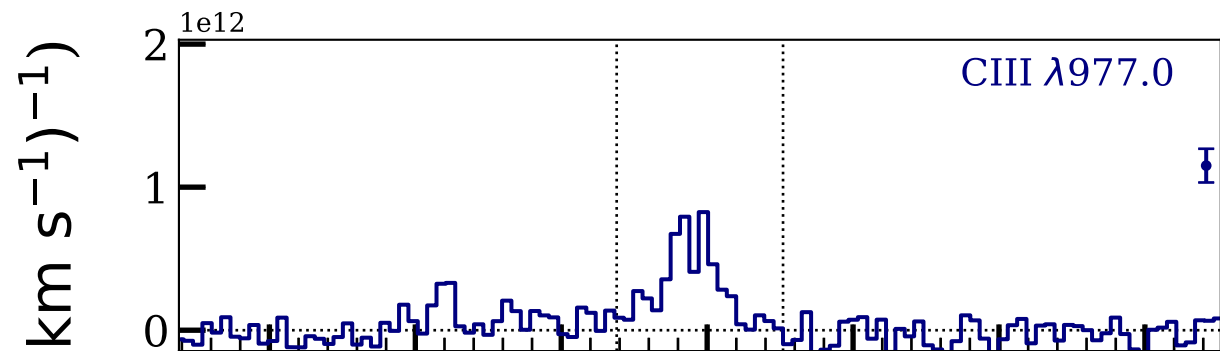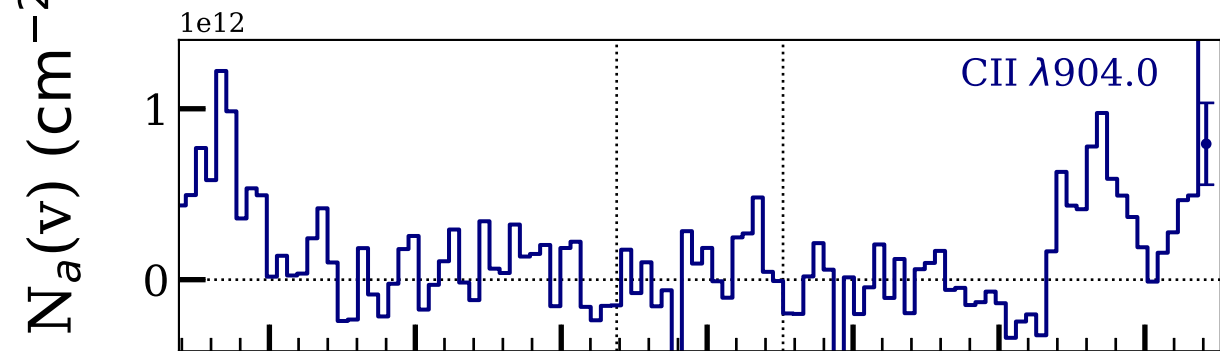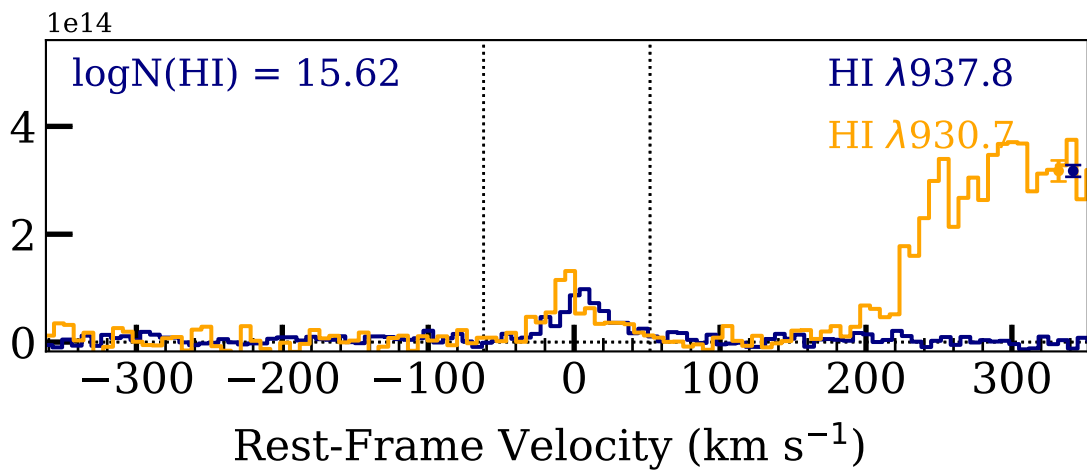

J101622.60+470643.3,  $z=0.664722$ , RF=0

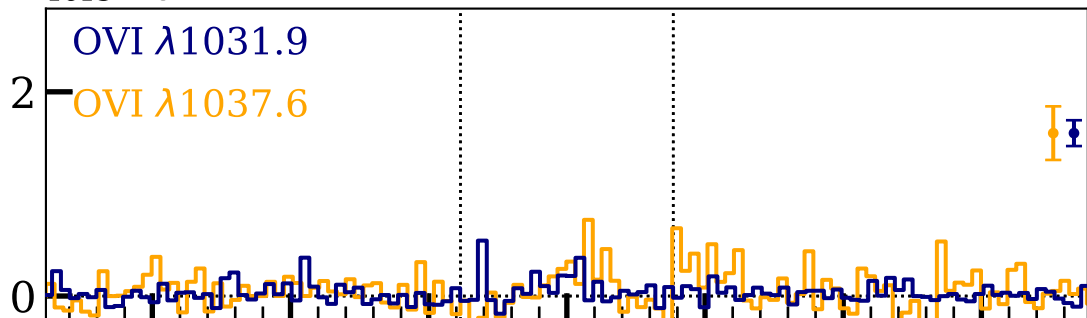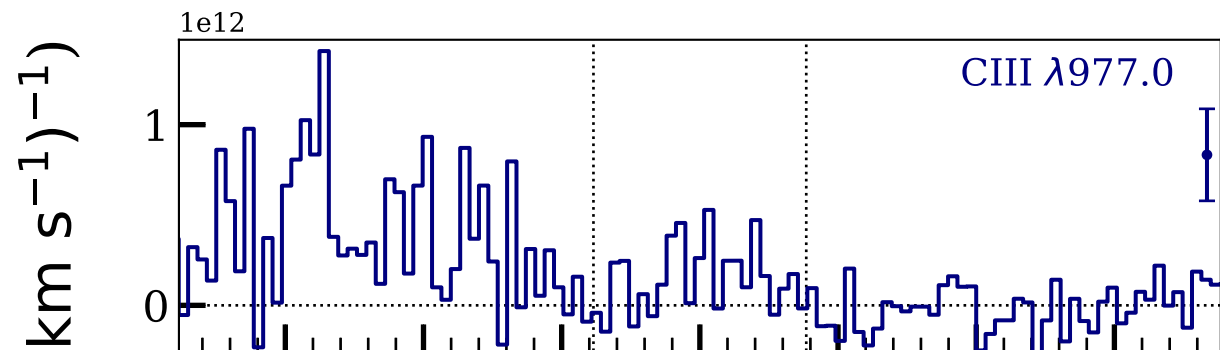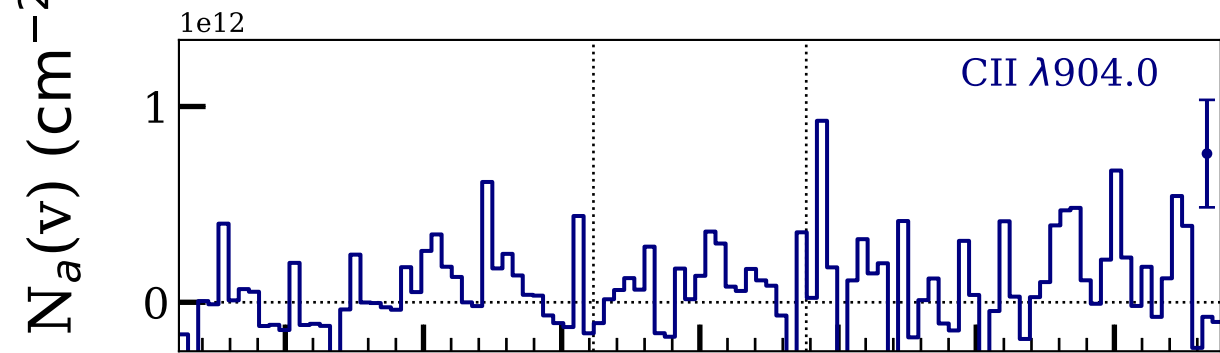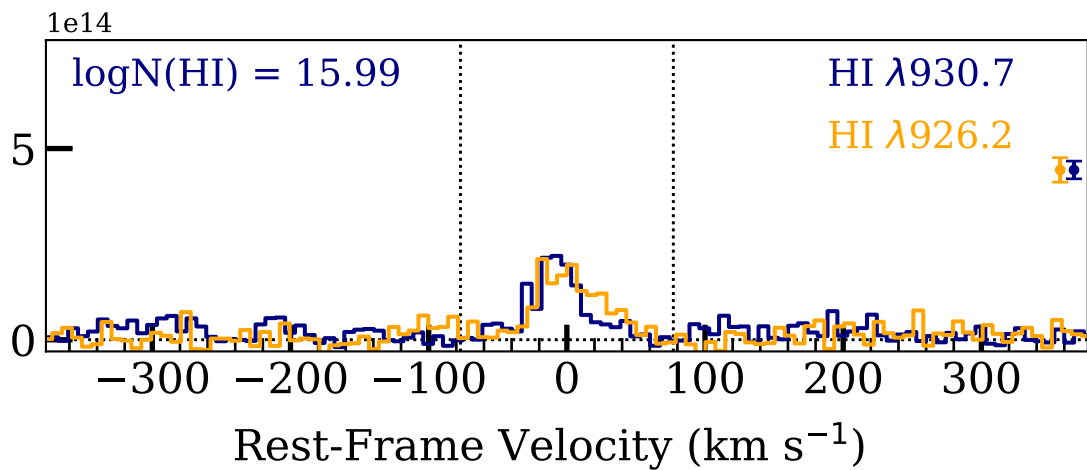

J101622.60+470643.3,  $z=0.727771$ , RF=0

$N_a(v)$  ( $\text{cm}^{-2}(\text{km s}^{-1})^{-1}$ )

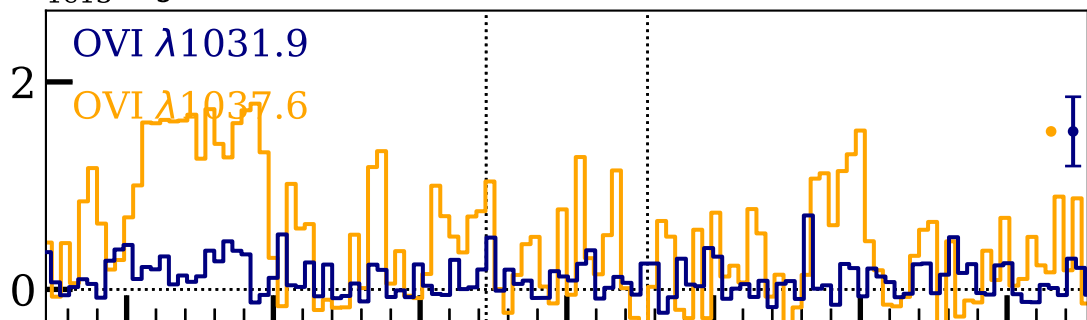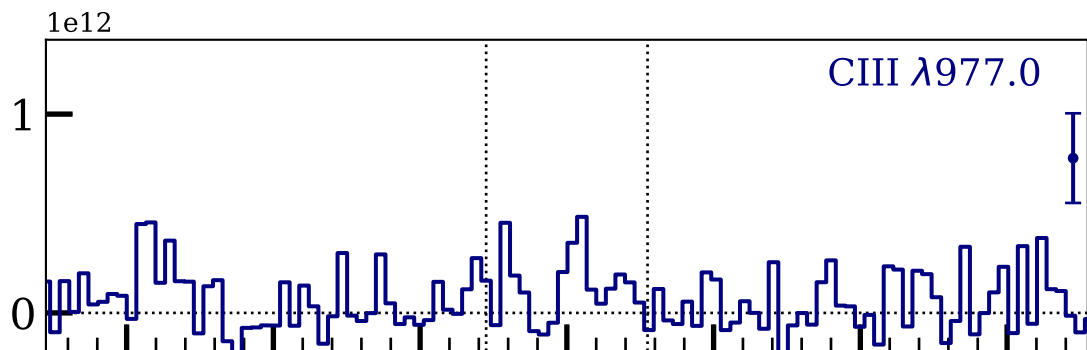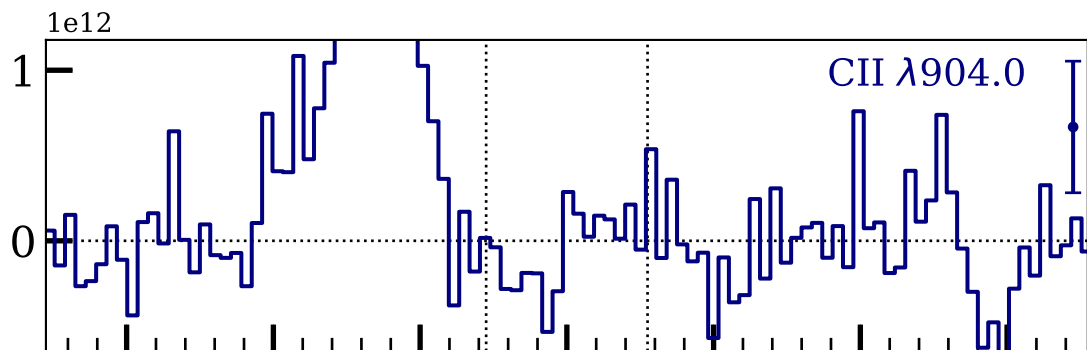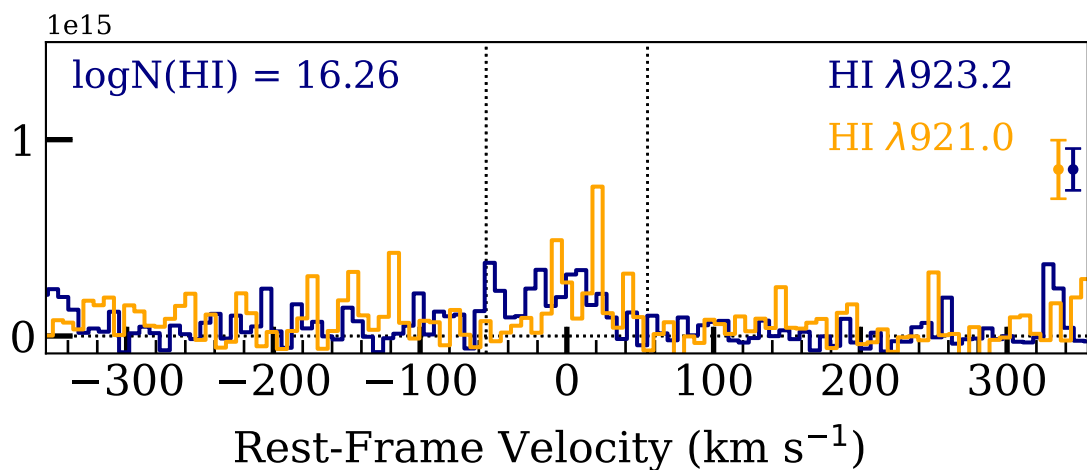

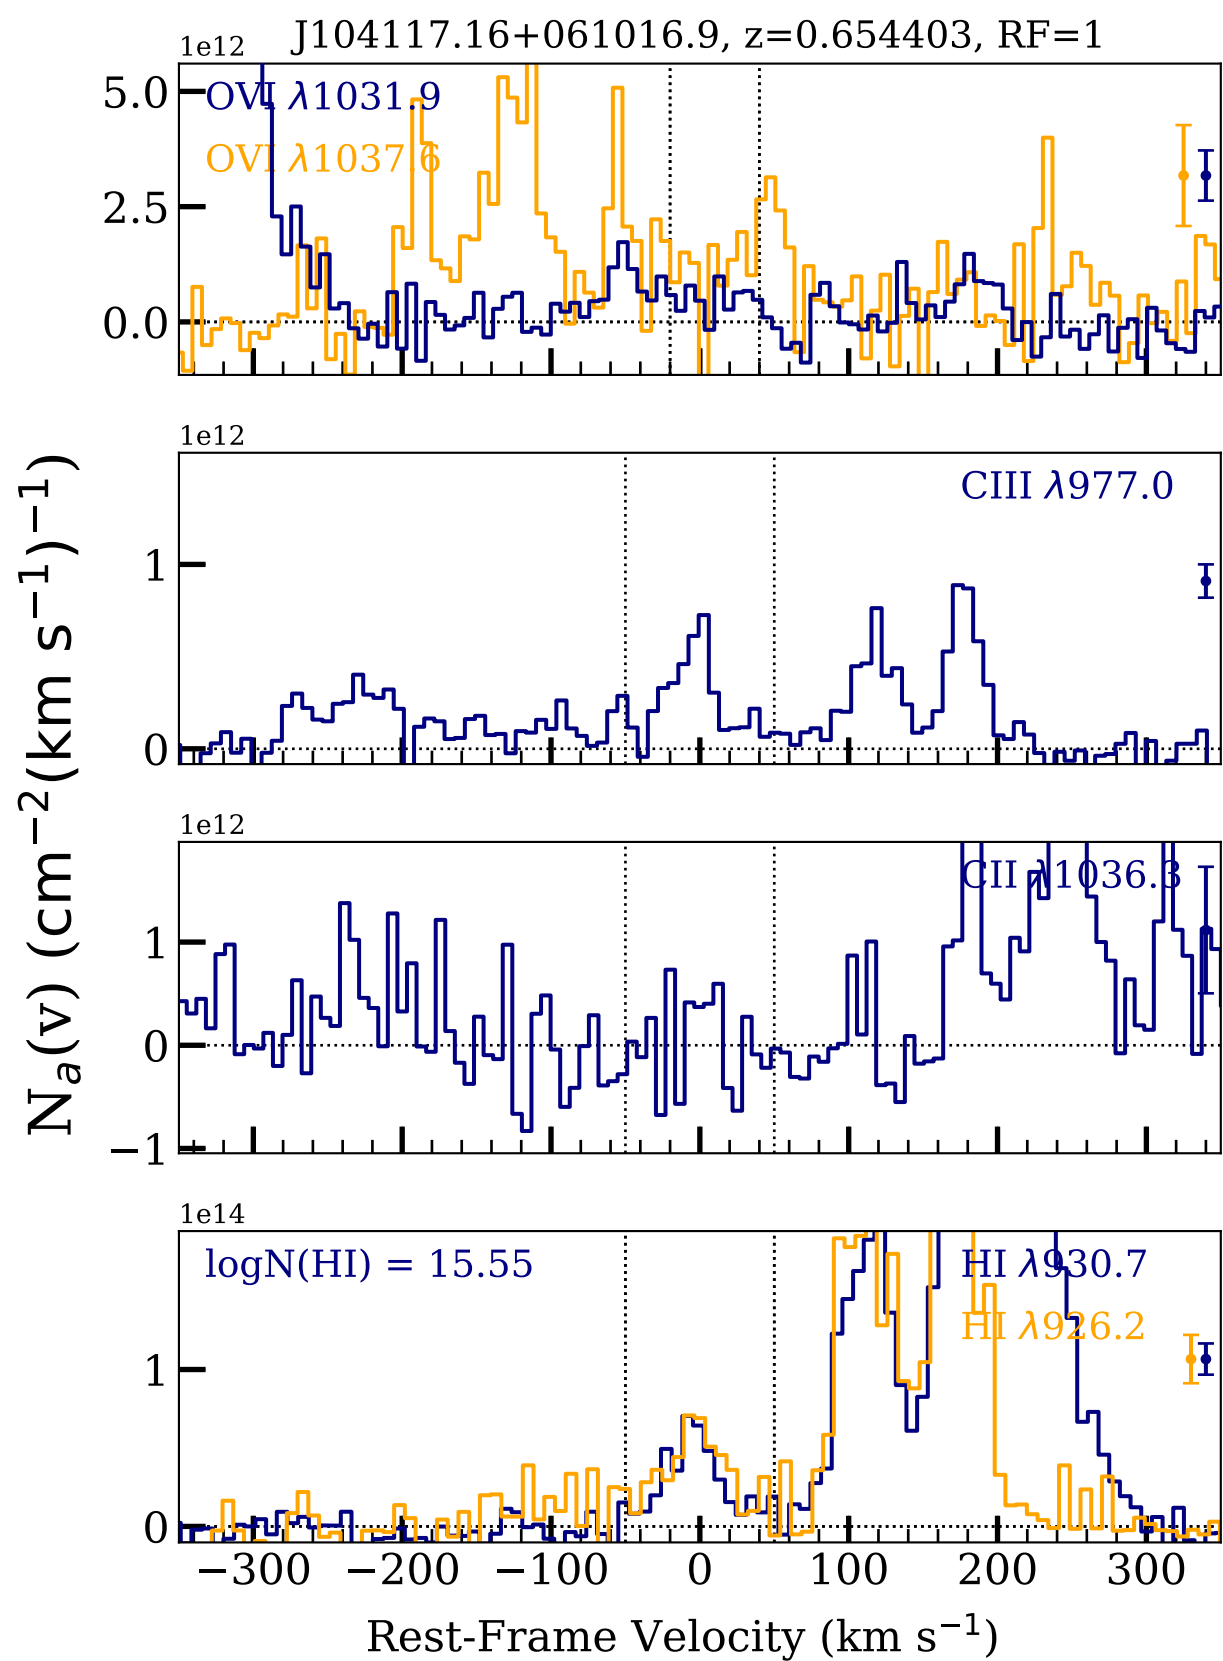

J104117.16+061016.9,  $z=0.655059$ , RF=1

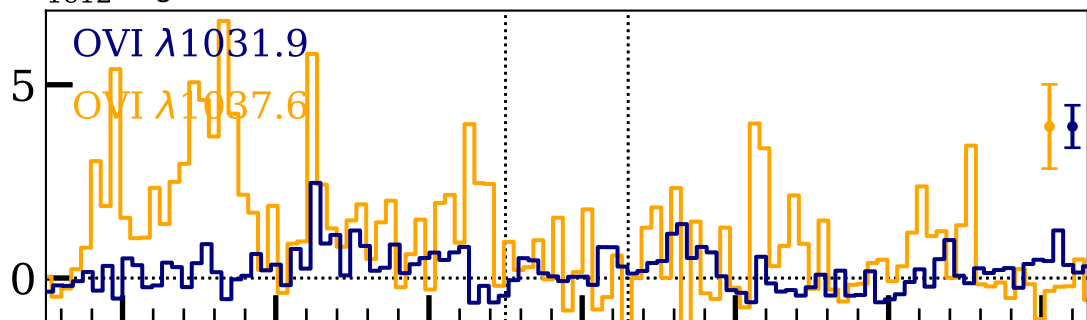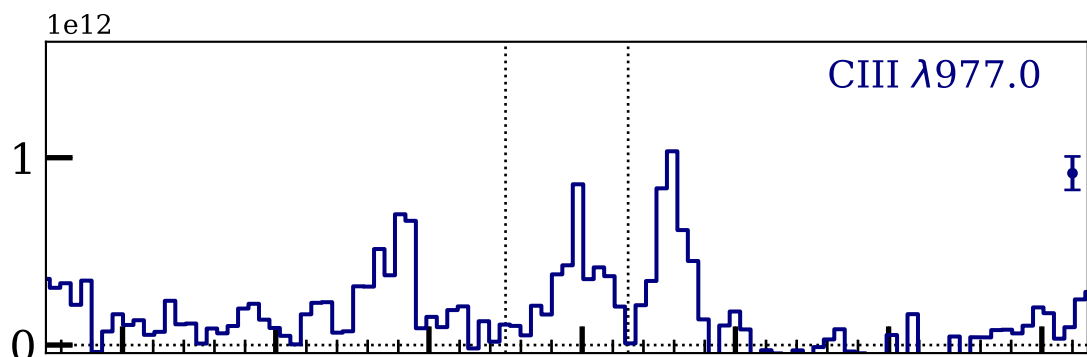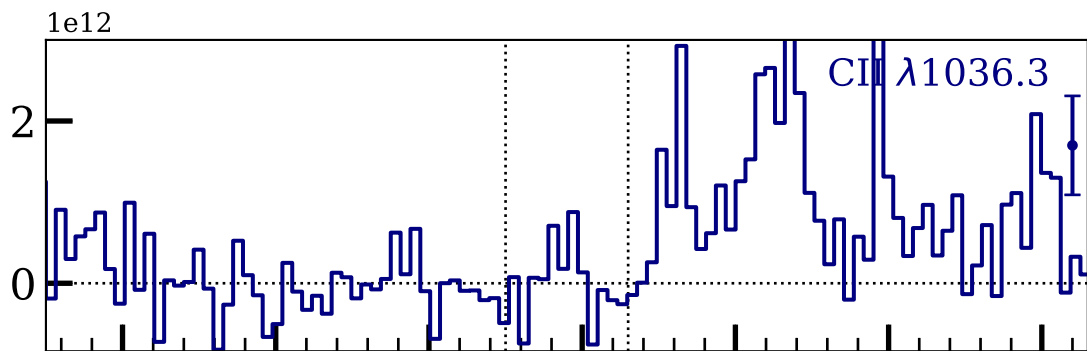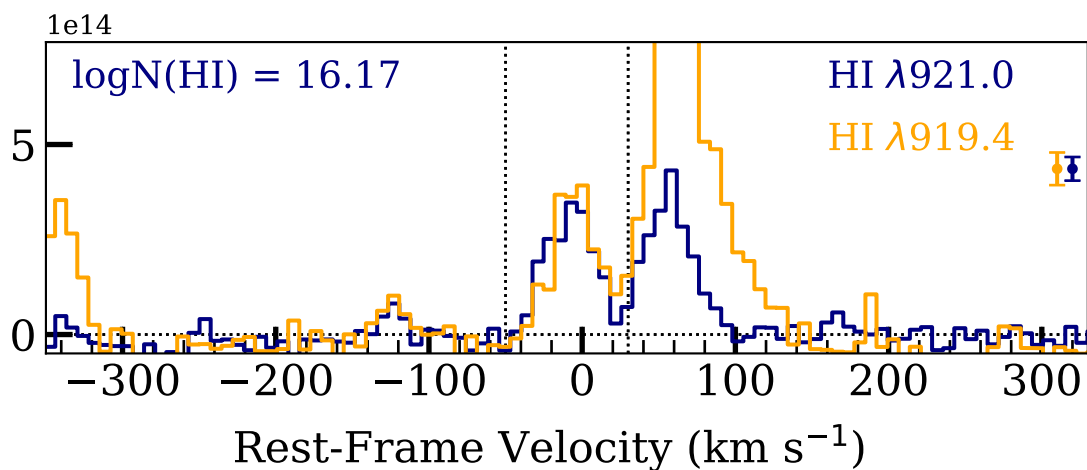

J104117.16+061016.9,  $z=0.655390$ , RF=1

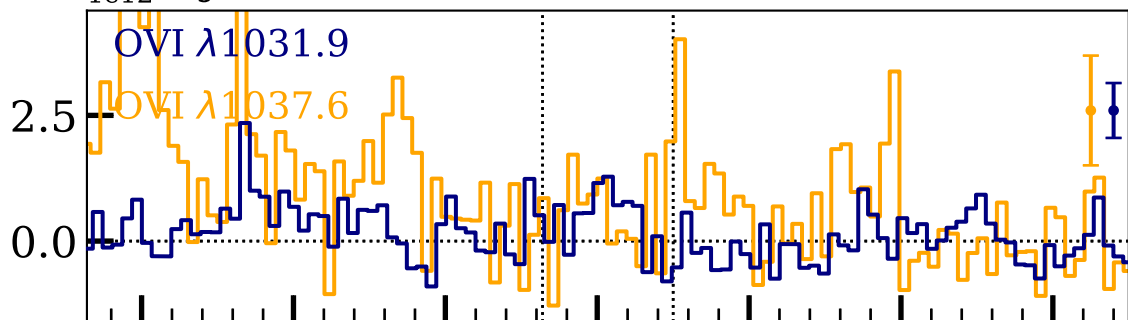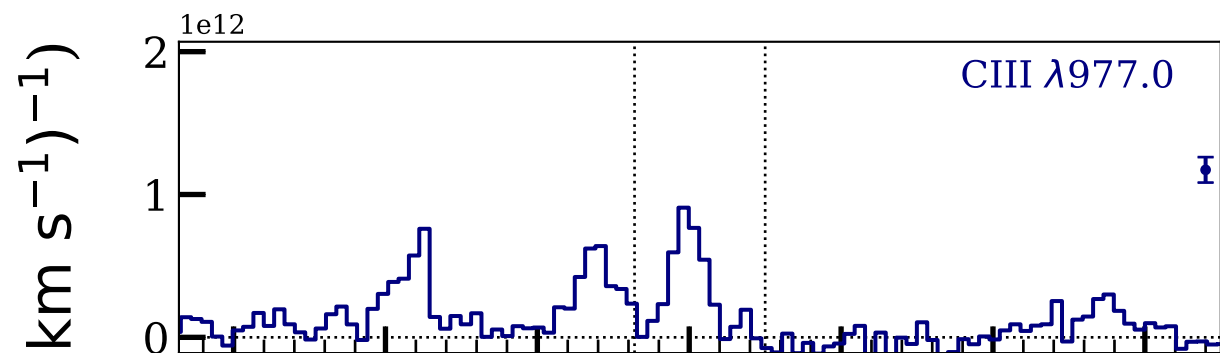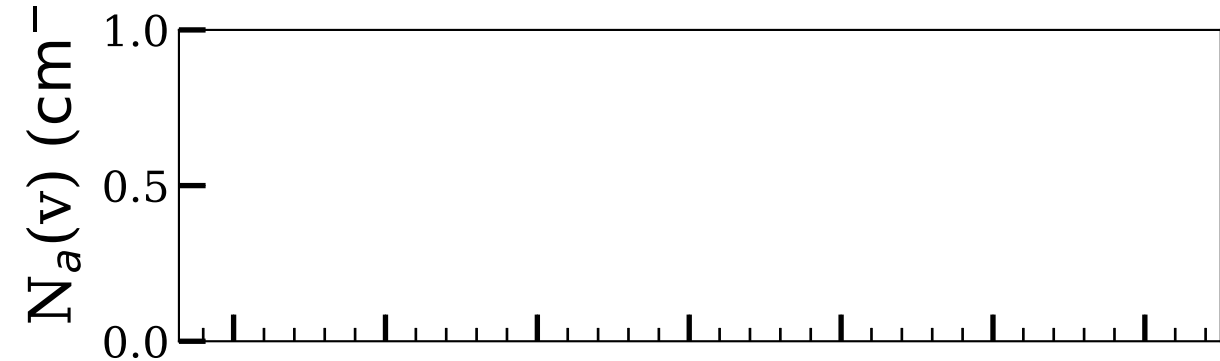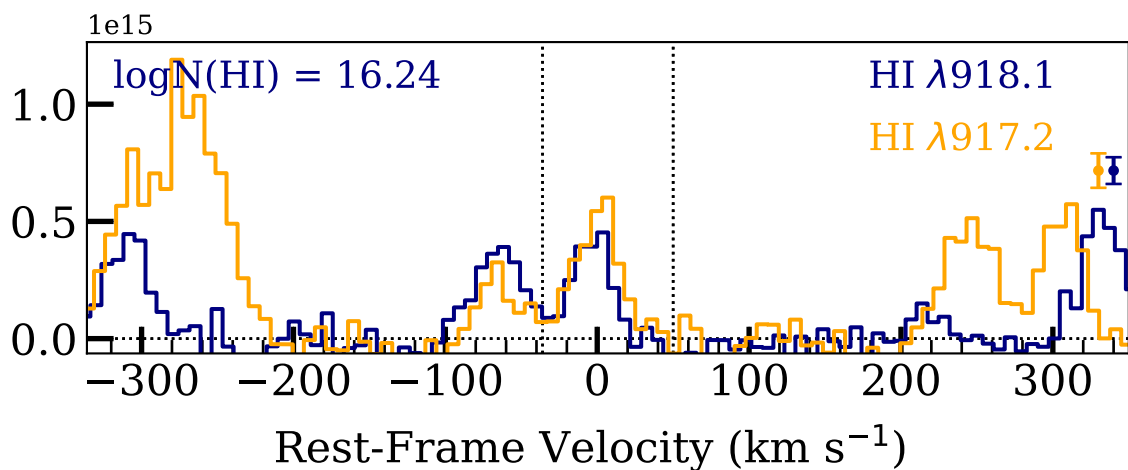

J105945.24+144143.0,  $z=0.465822$ , RF=1

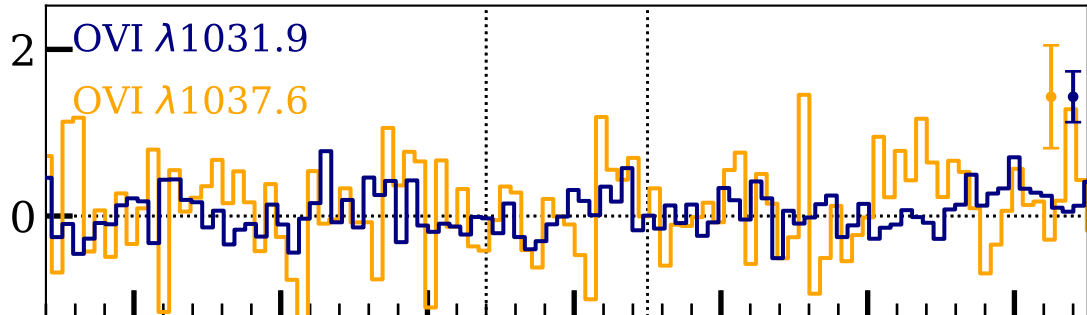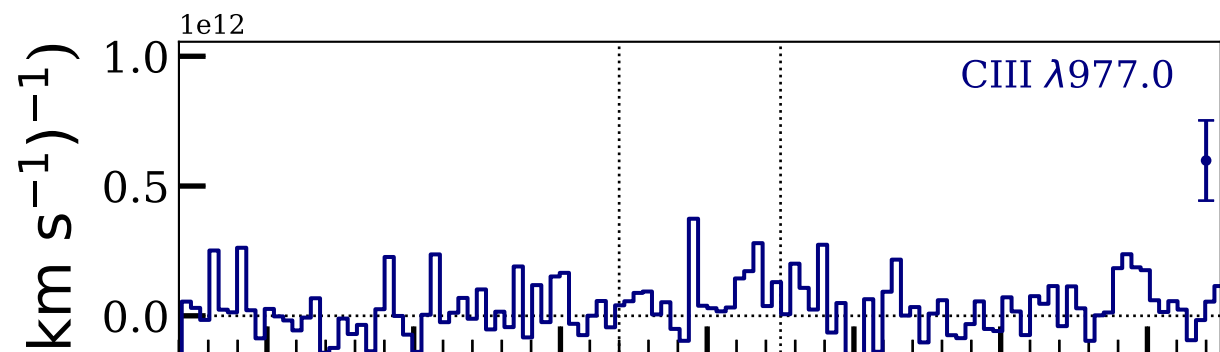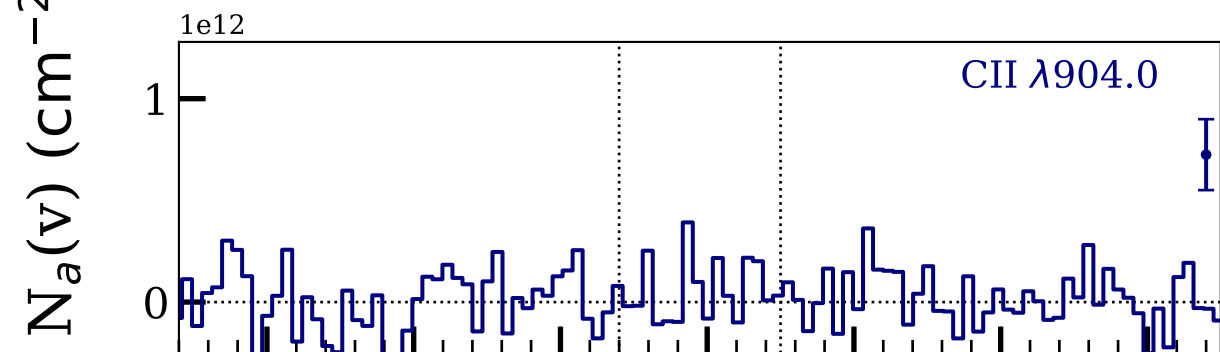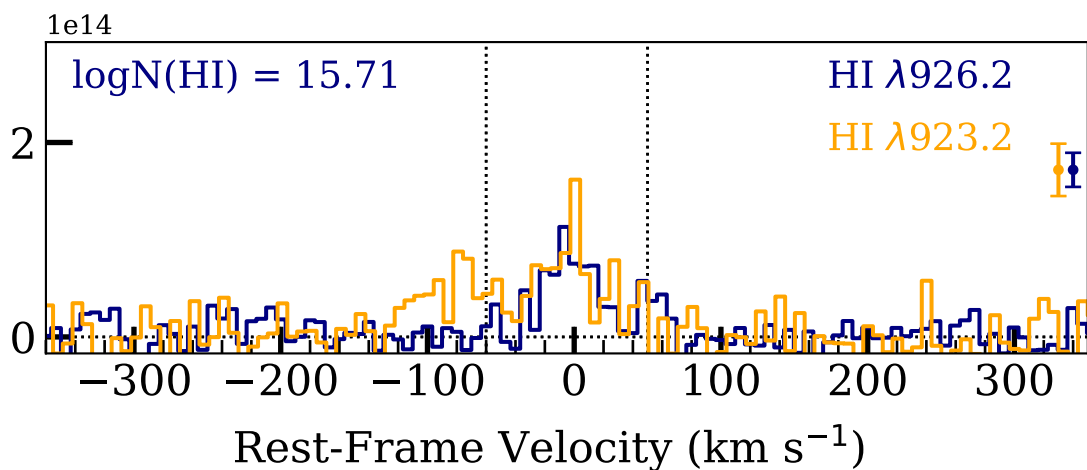



J105945.24+144143.0,  $z=0.576490$ , RF=1

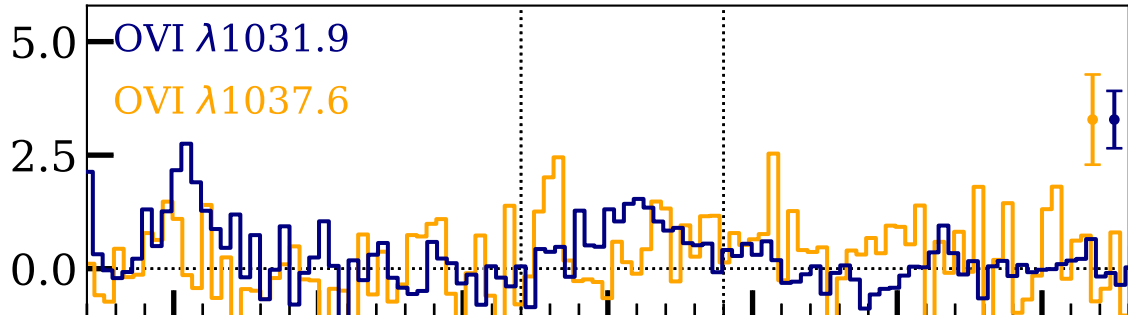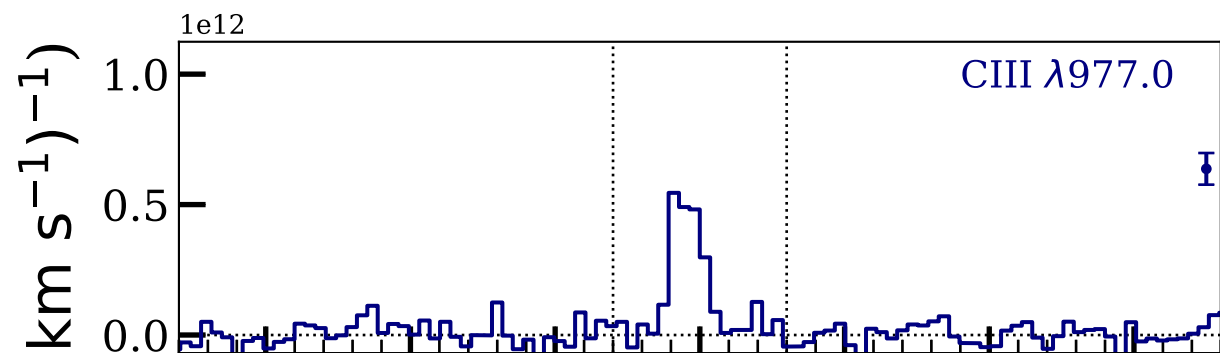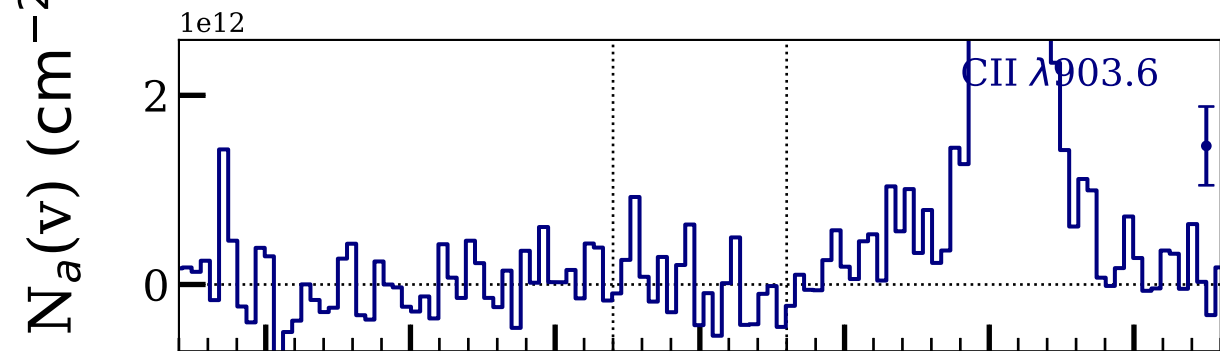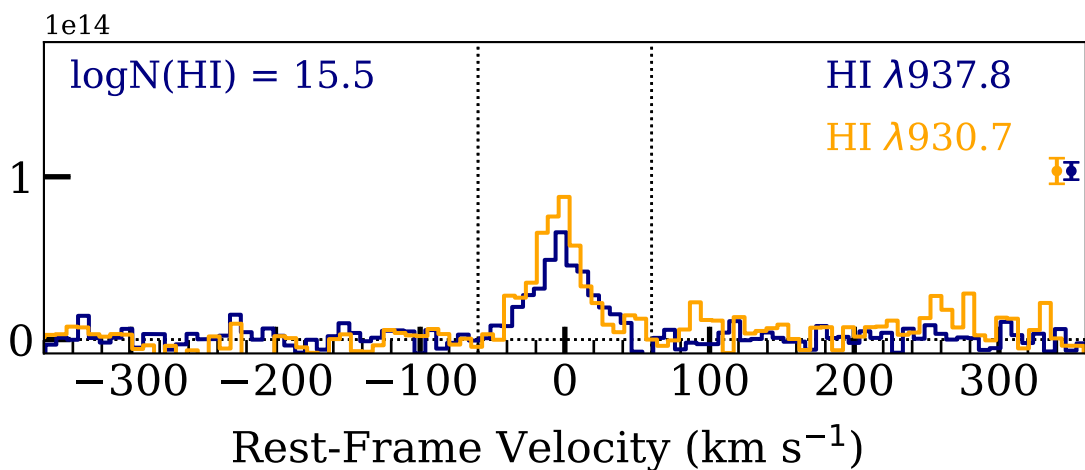

J105956.14+121151.1,  $z=0.332377$ , RF=1

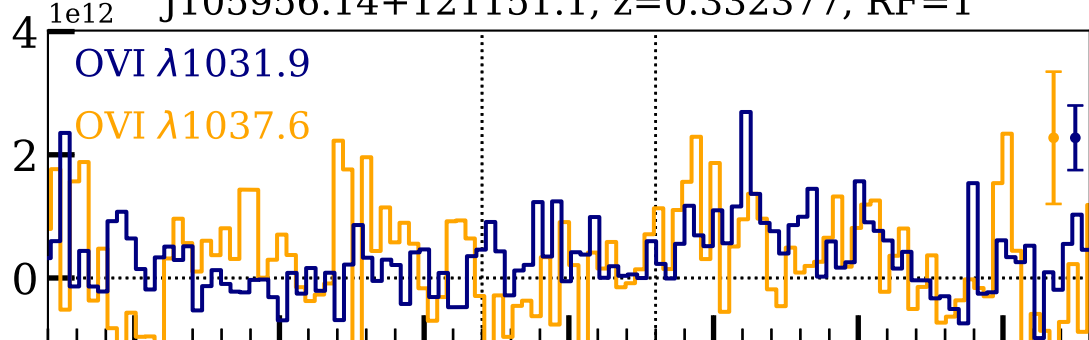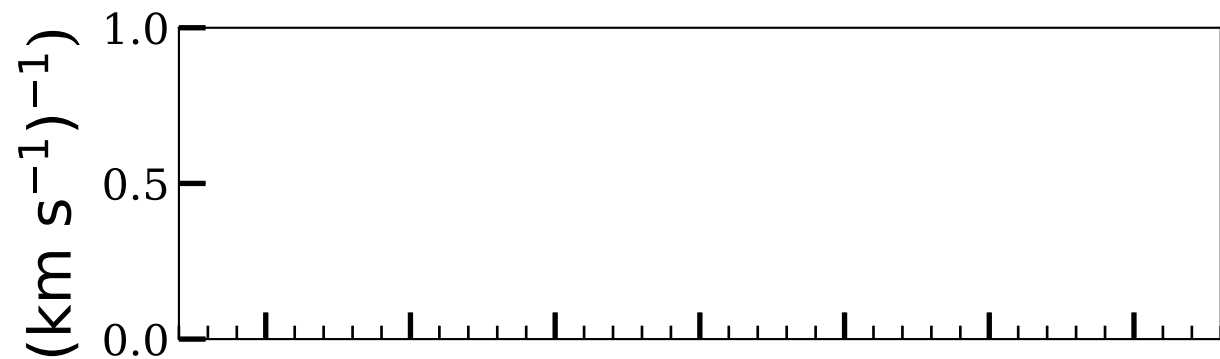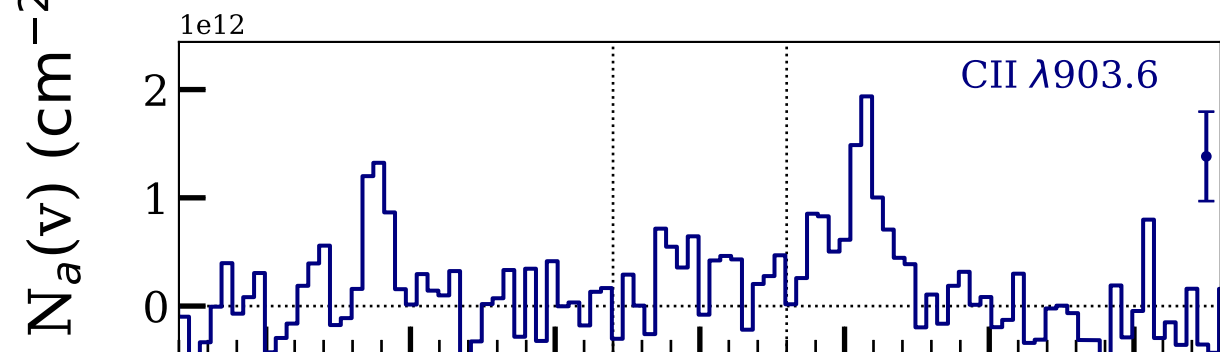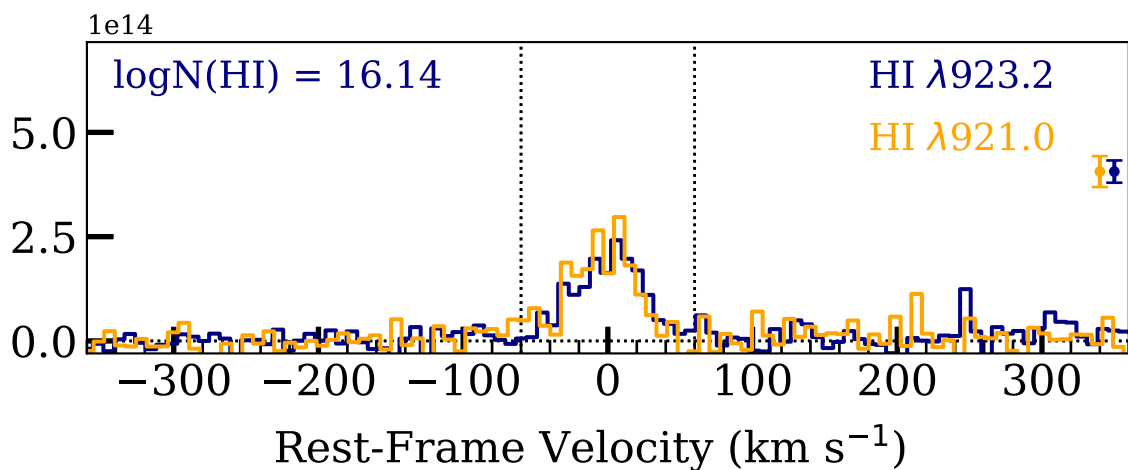

J110047.85+104613.2,  $z=0.415099$ , RF=0

$N_a(v) \text{ (cm}^{-2} \text{ (km s}^{-1})^{-1})$

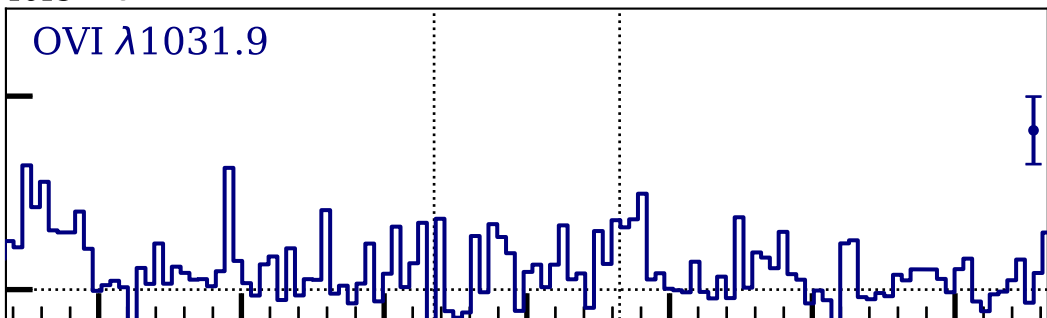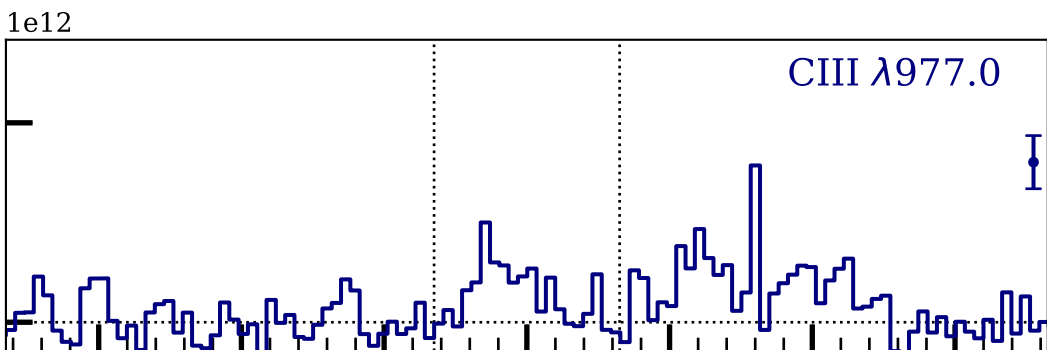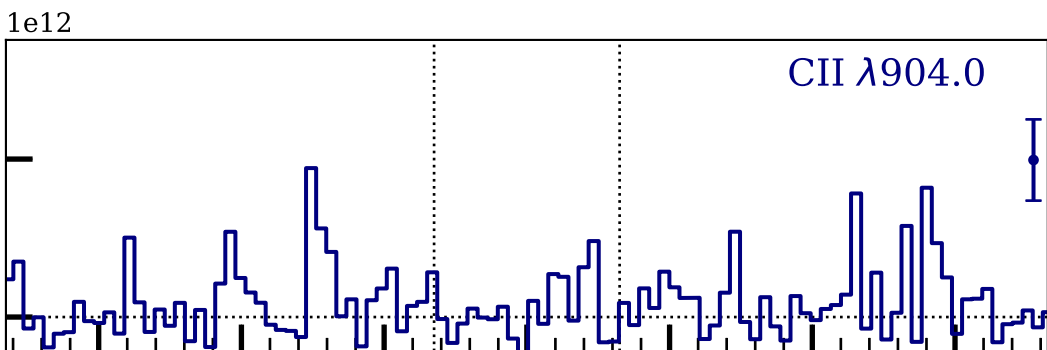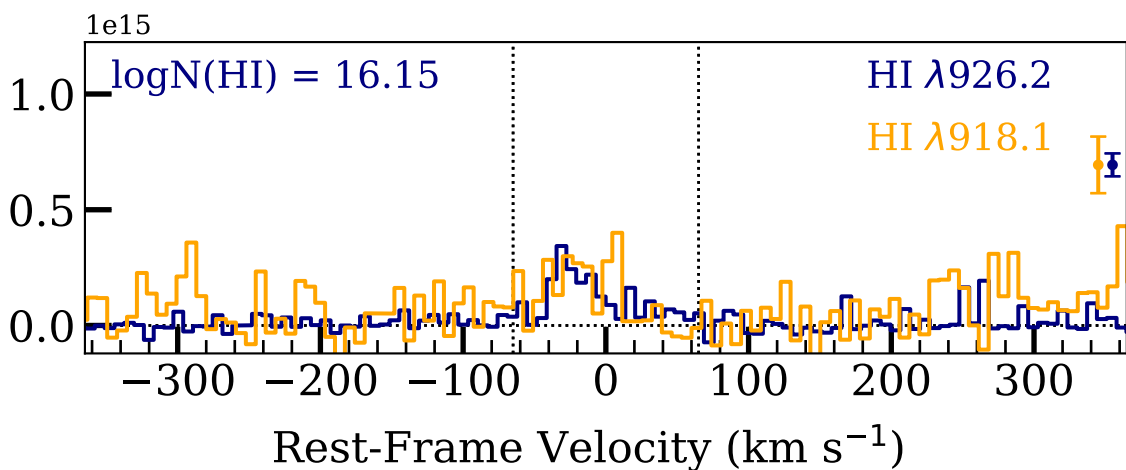

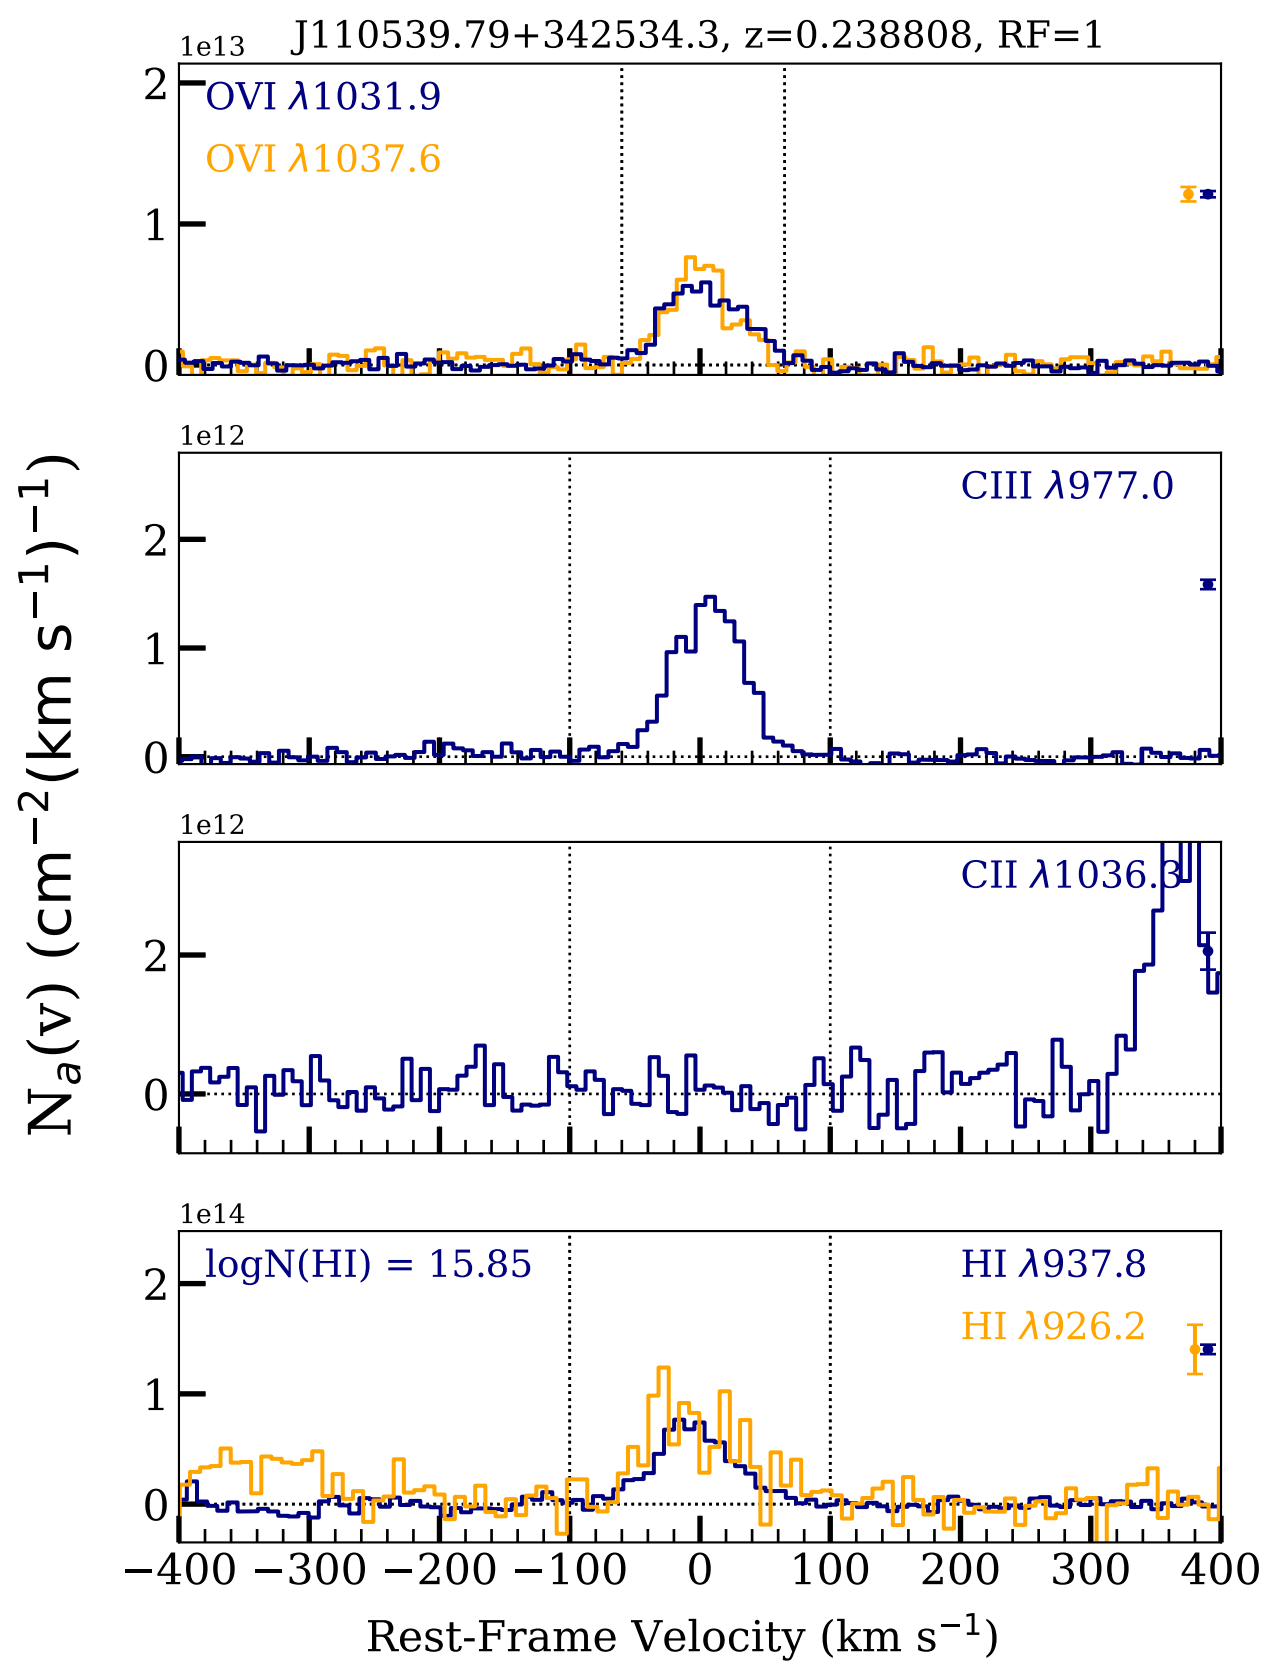

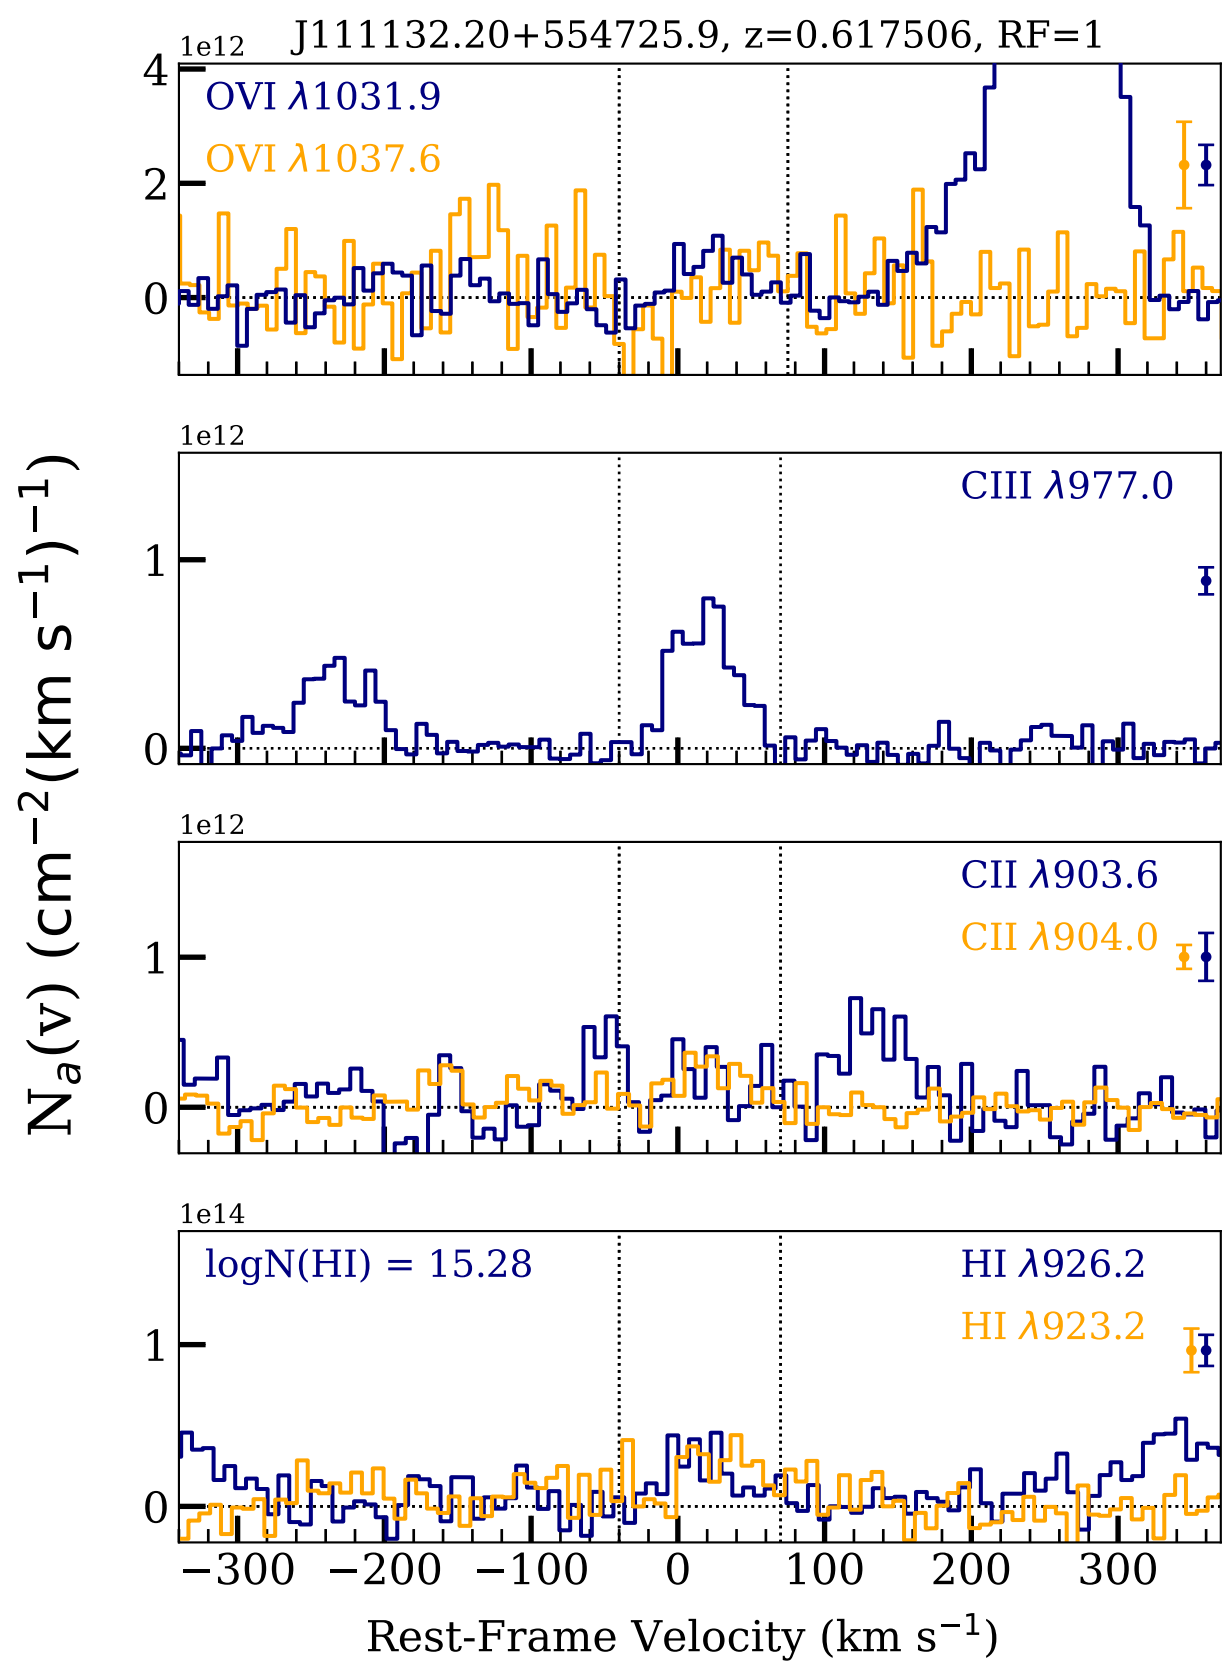

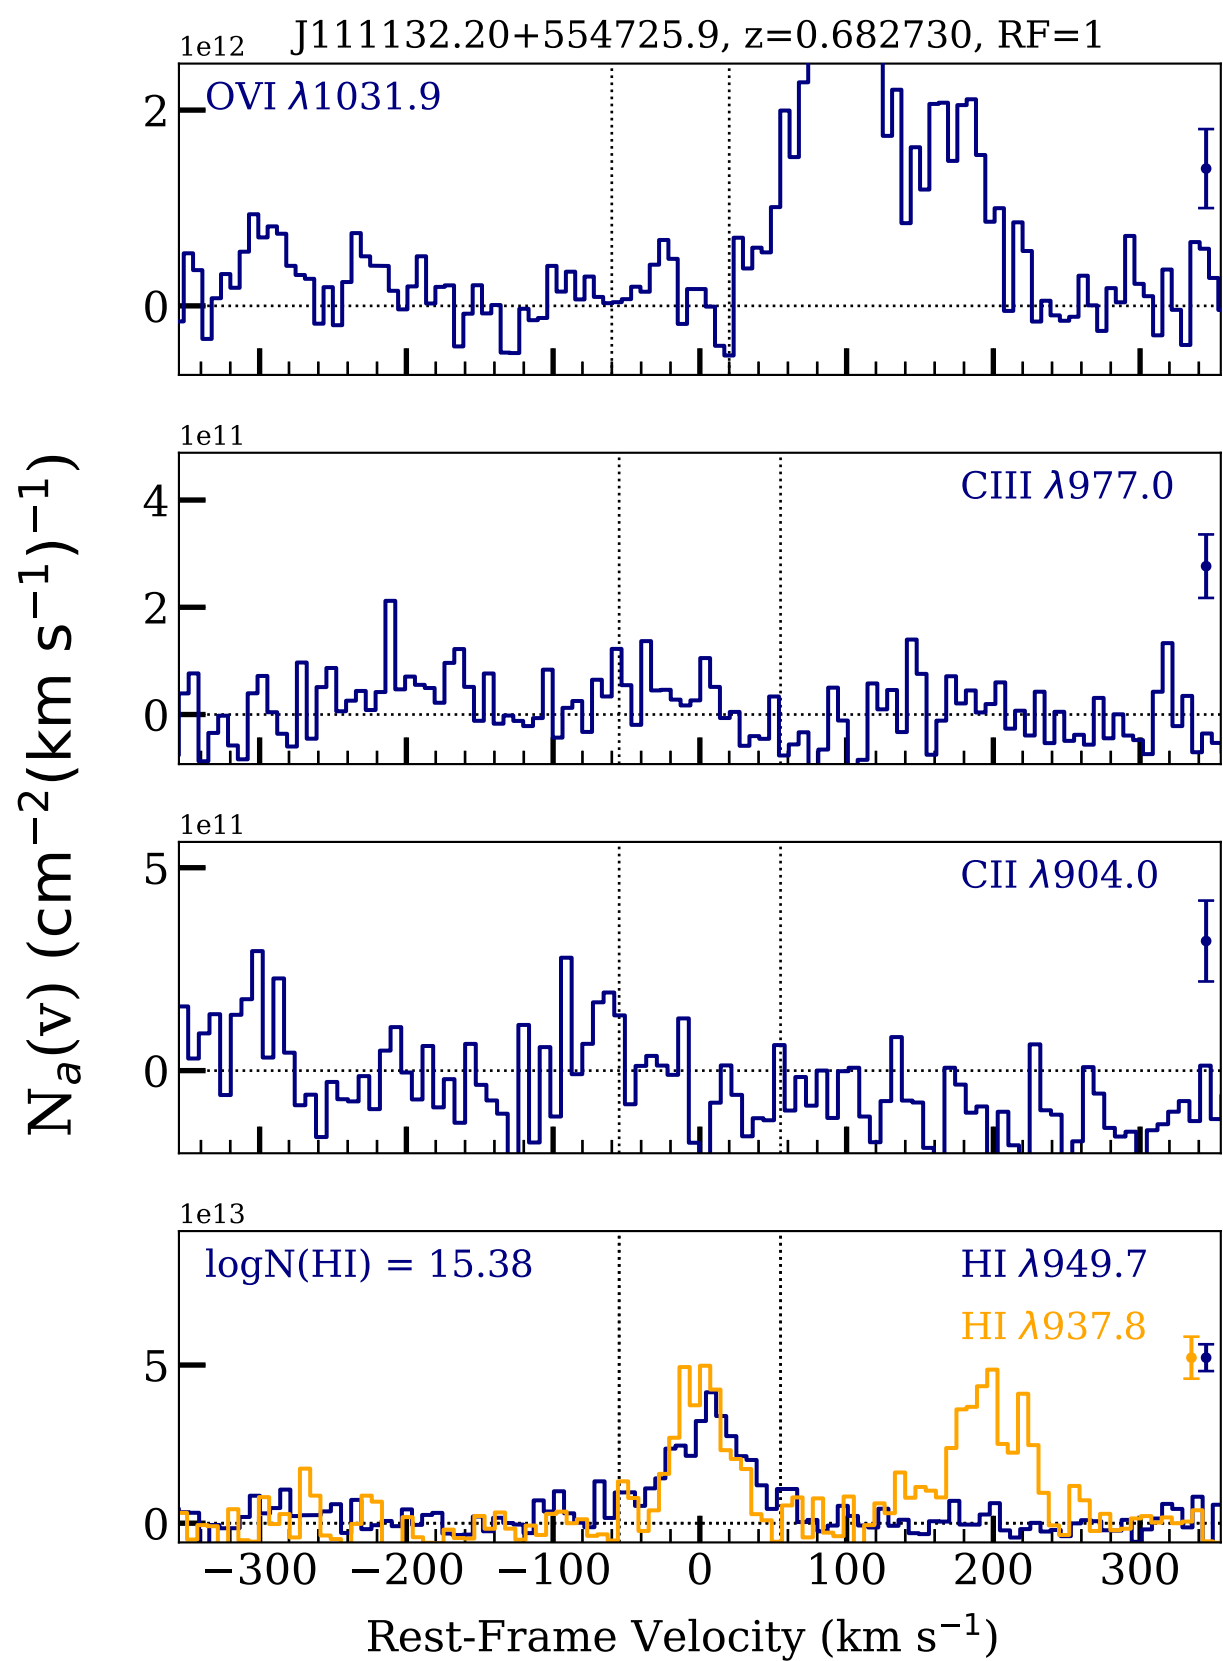

1e12 J111239.11+353928.2,  $z=0.246496$ , RF=0

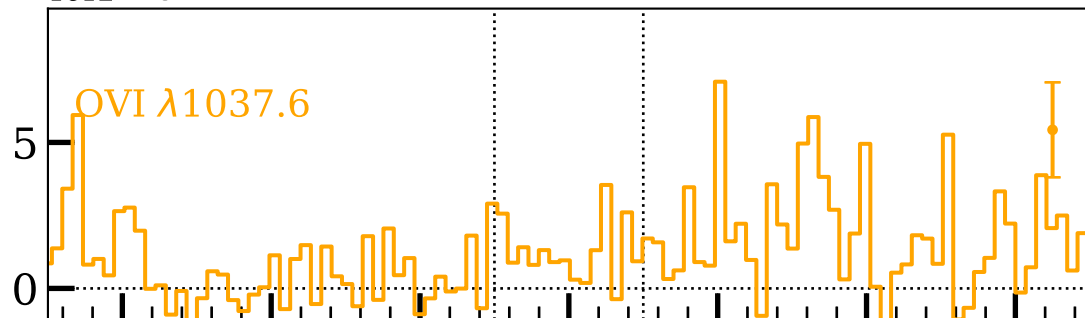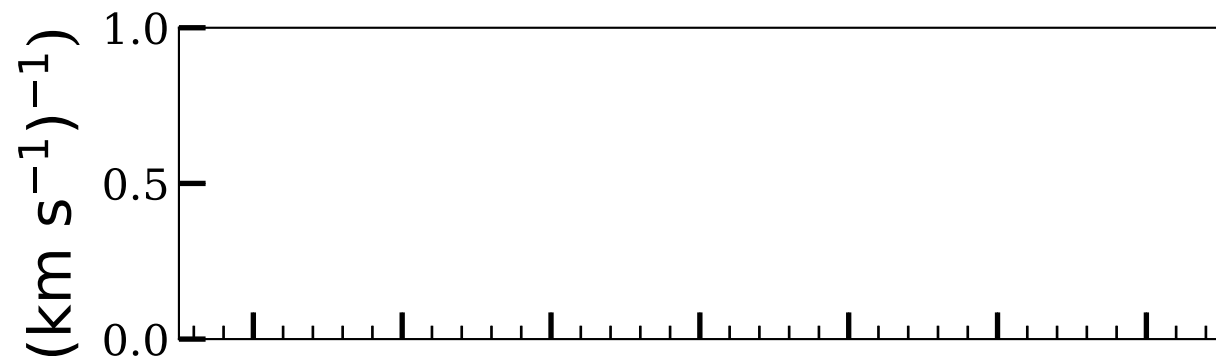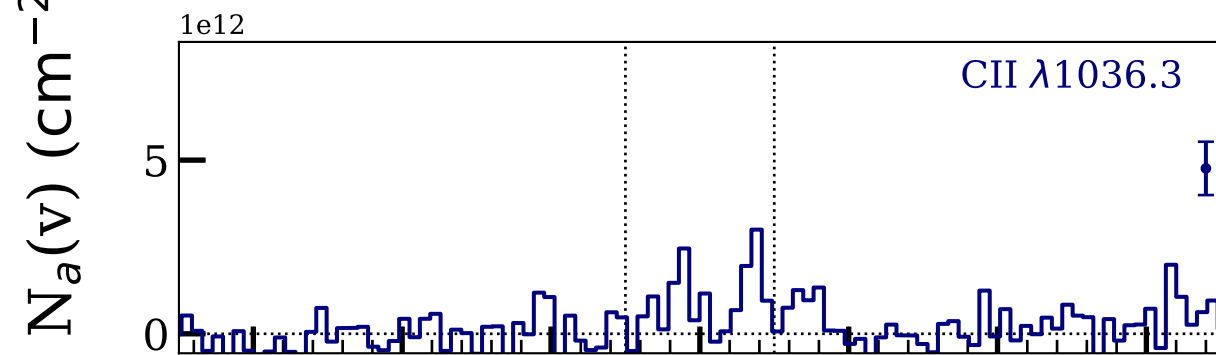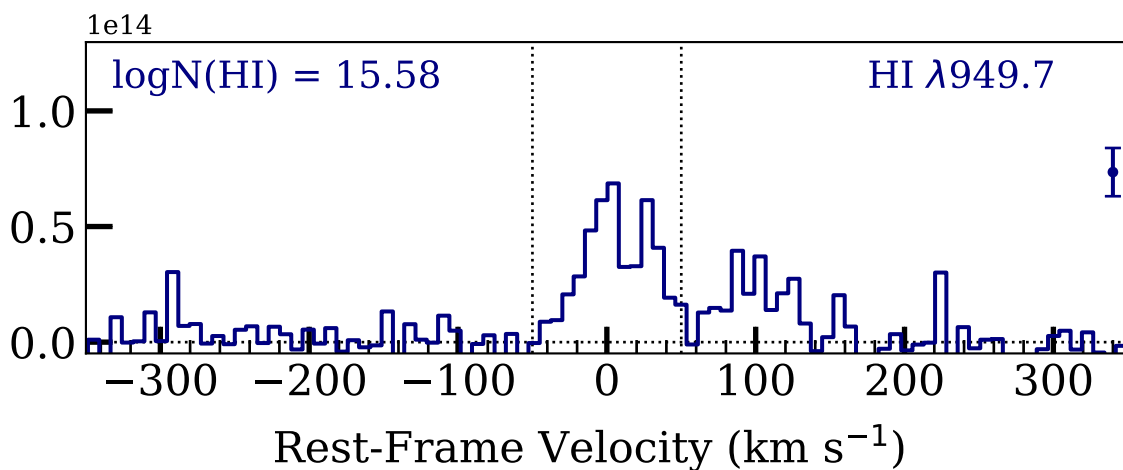

J111507.65+023757.5,  $z=0.369213$ , RF=1

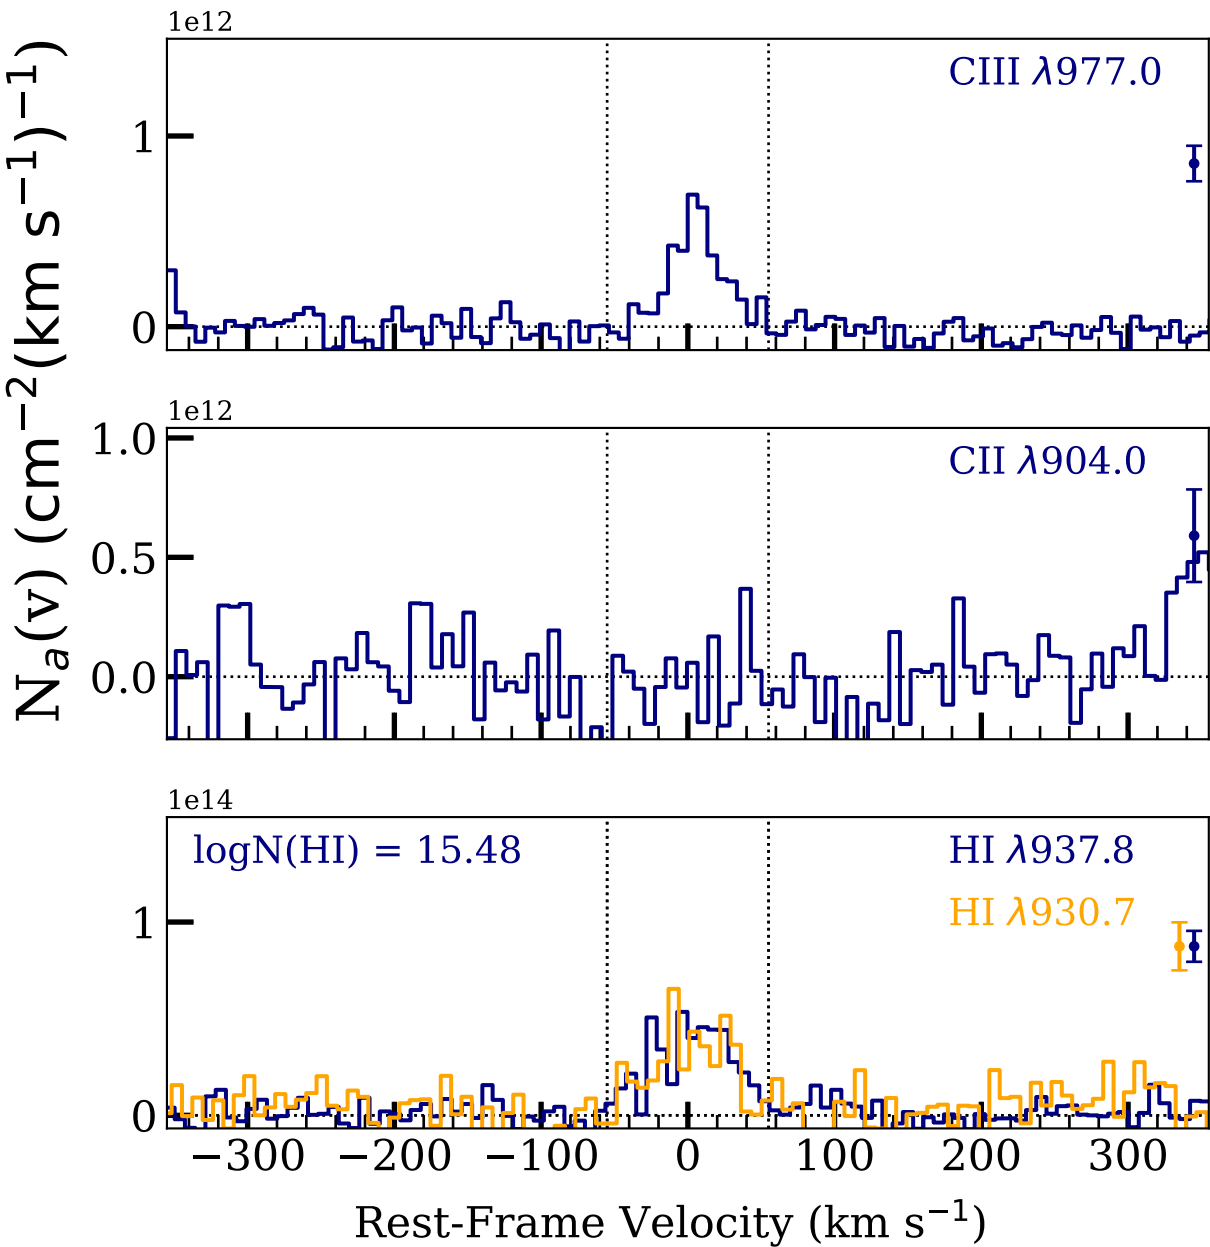



J111754.23+263416.6,  $z=0.351969$ , RF=1

$N_a(v) \text{ (cm}^{-2} \text{ (km s}^{-1})^{-1})$

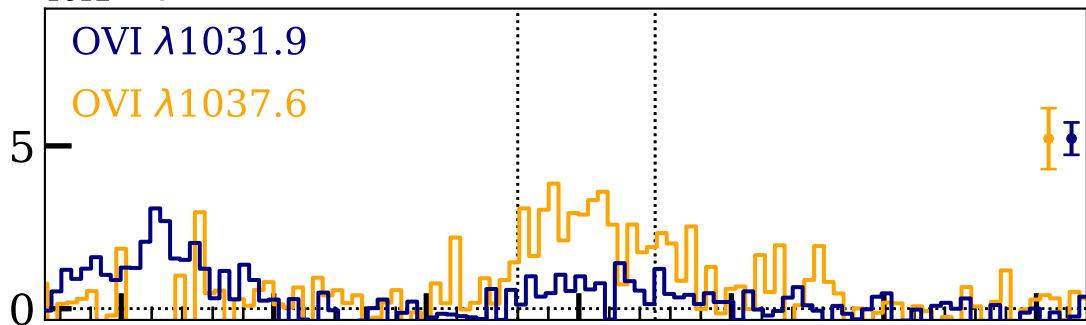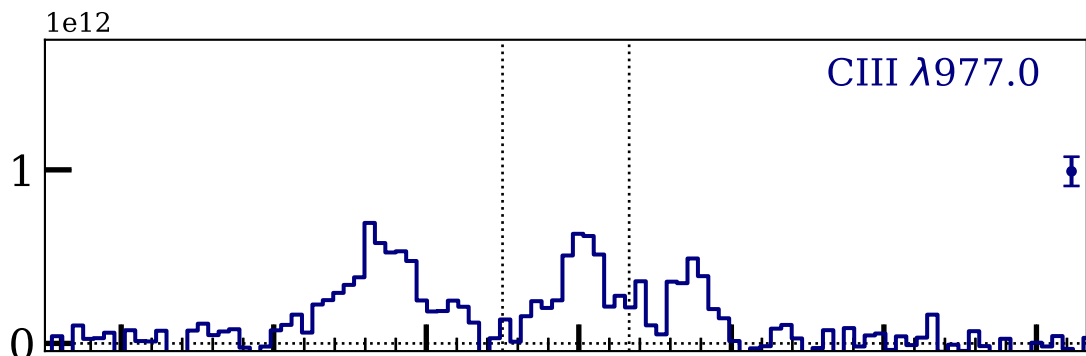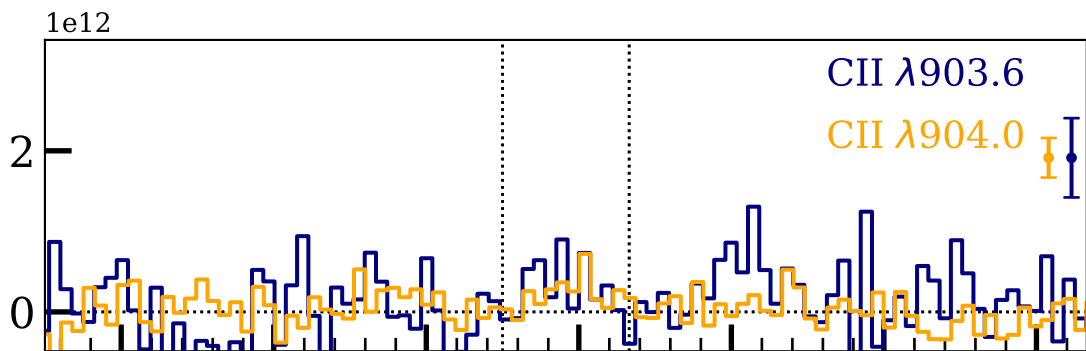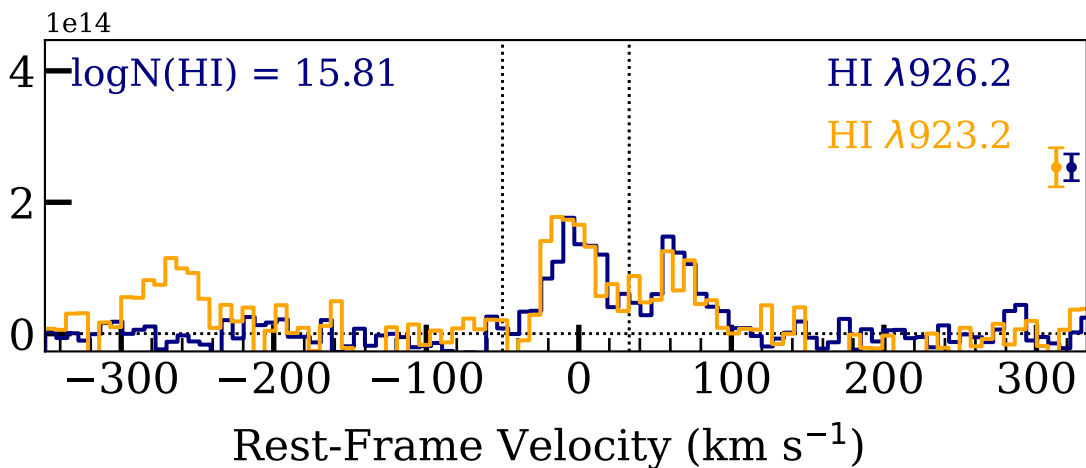

J111754.23+263416.6,  $z=0.352307$ , RF=1

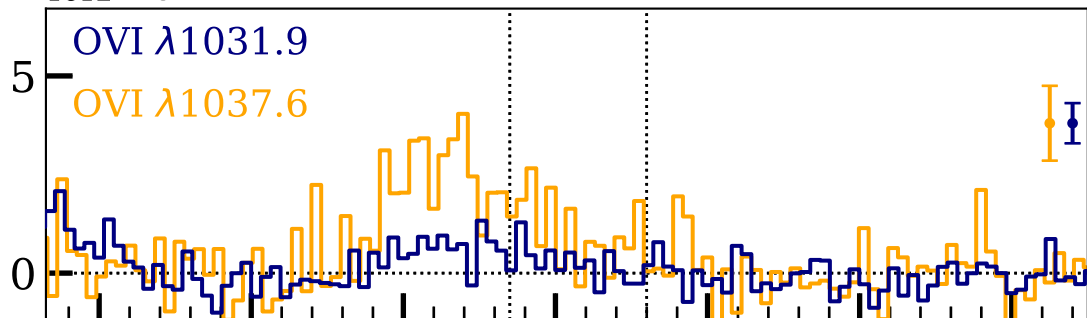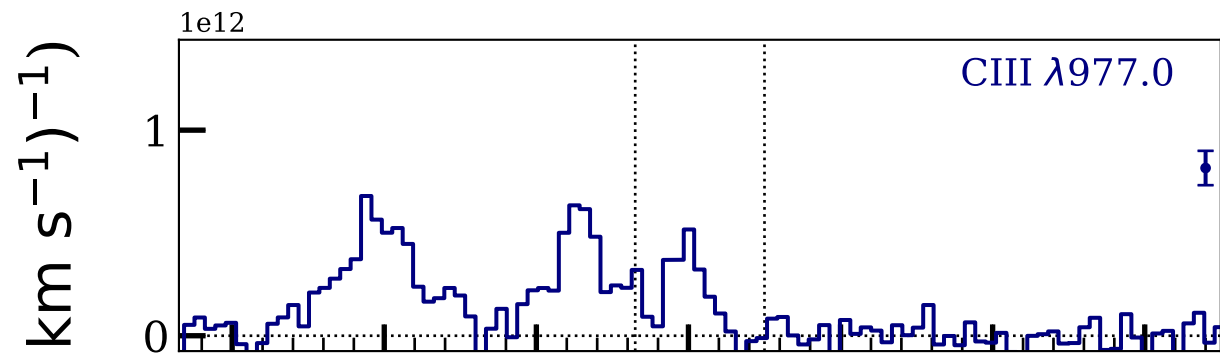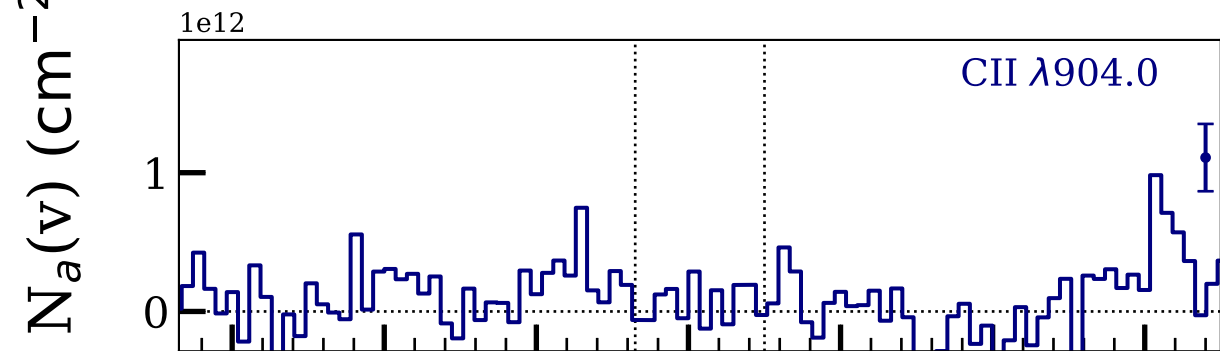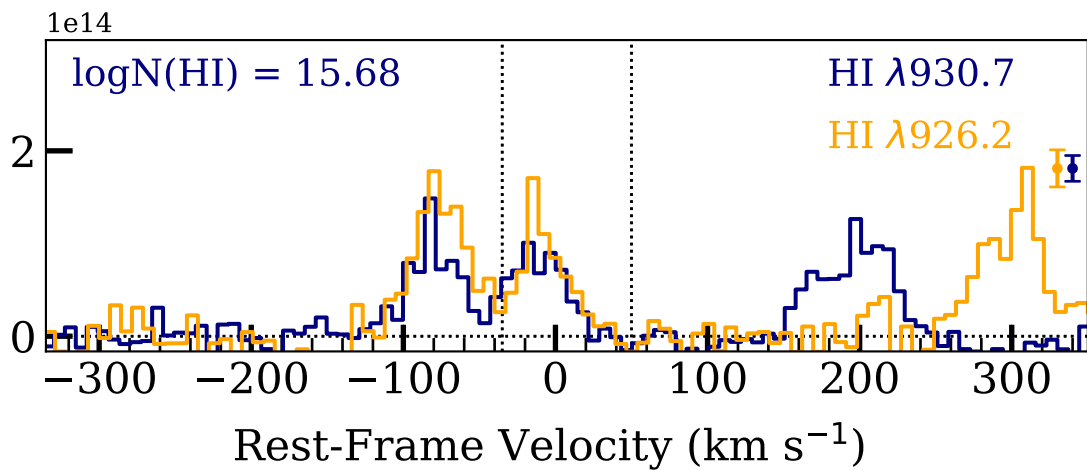

J111908.59+211918.0,  $z=0.138500$ , RF=1

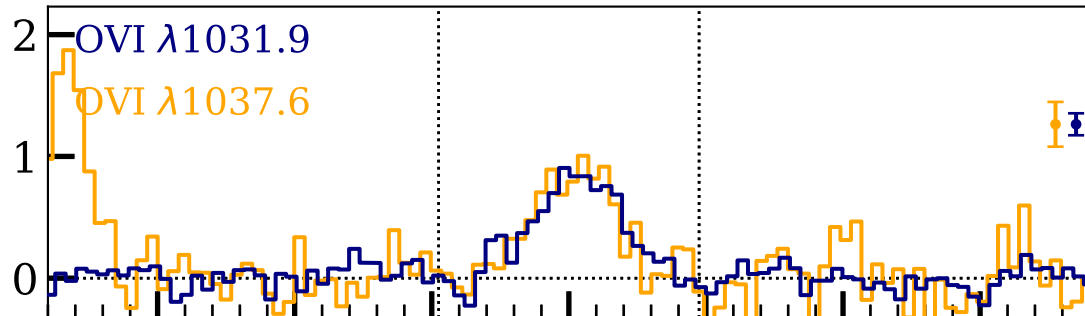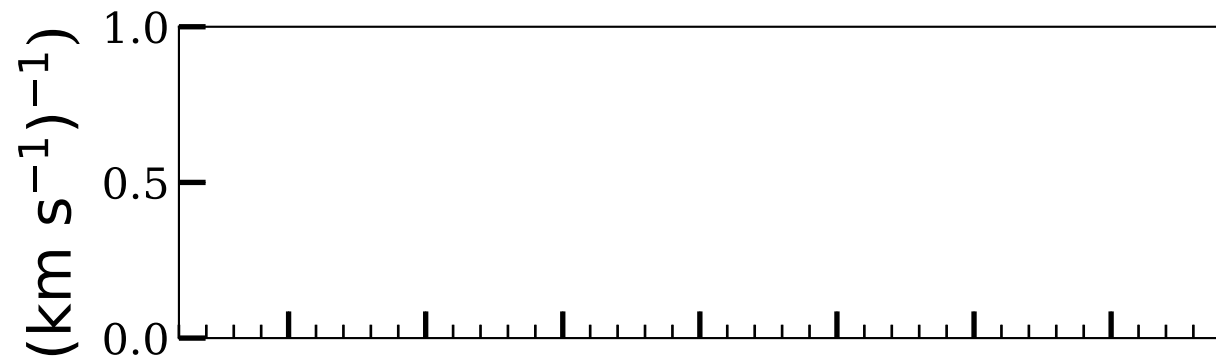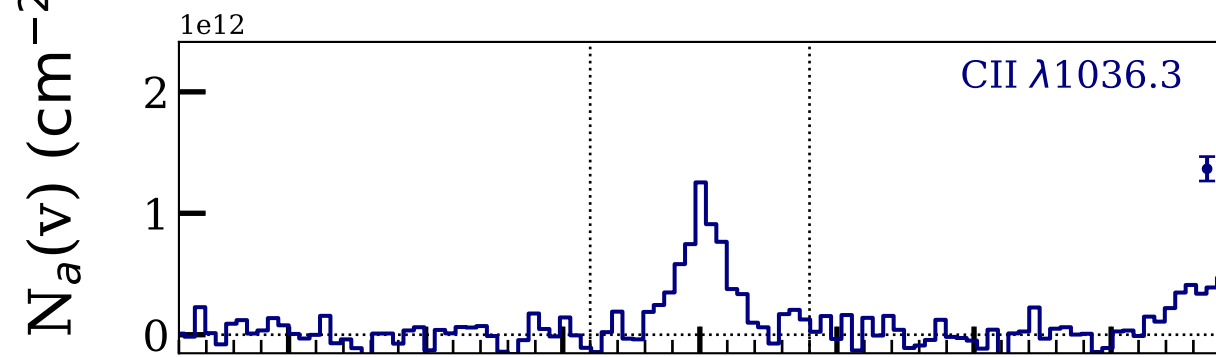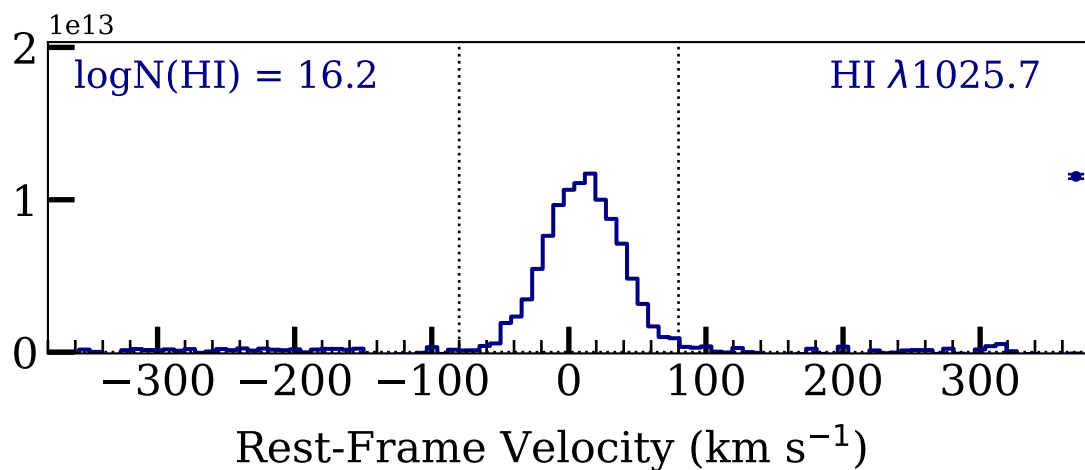

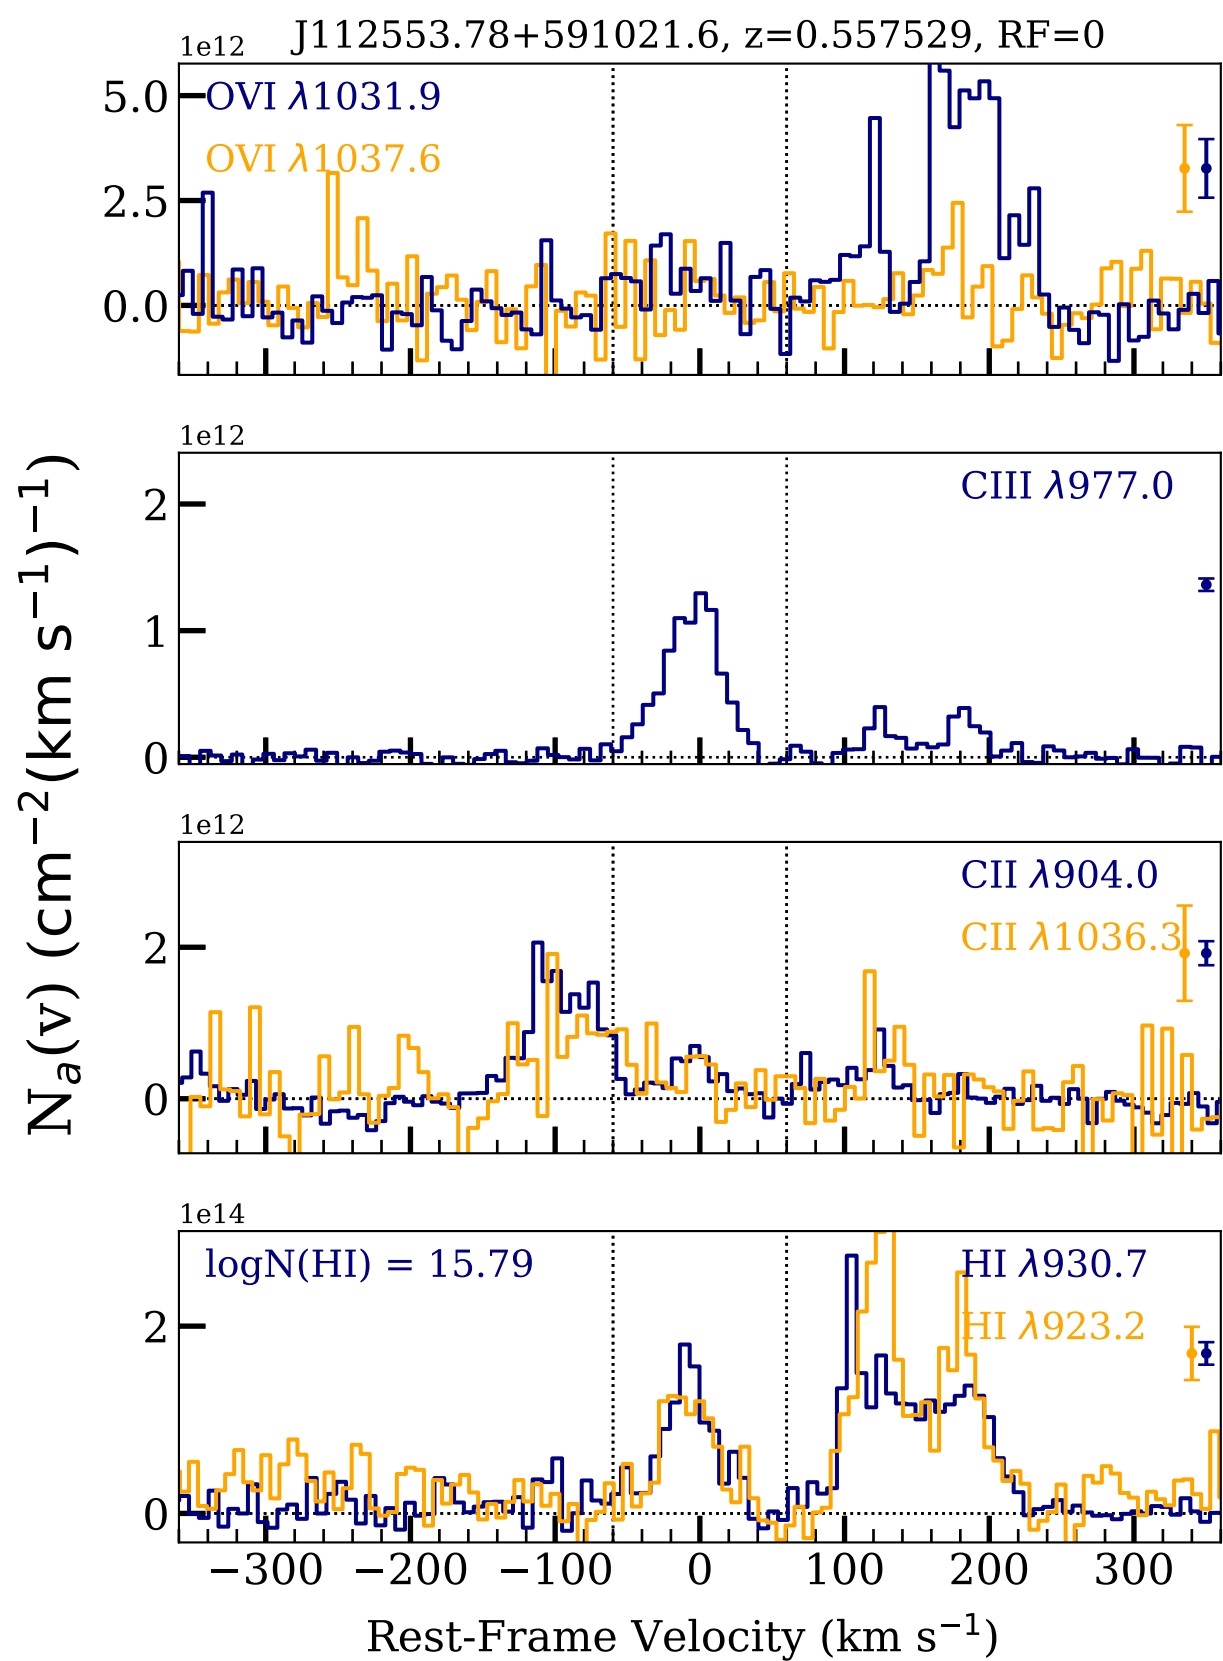

J112553.78+591021.6,  $z=0.558200$ , RF=0

$N_a(v) \text{ (cm}^{-2} \text{ (km s}^{-1} \text{)}^{-1} \text{)}$

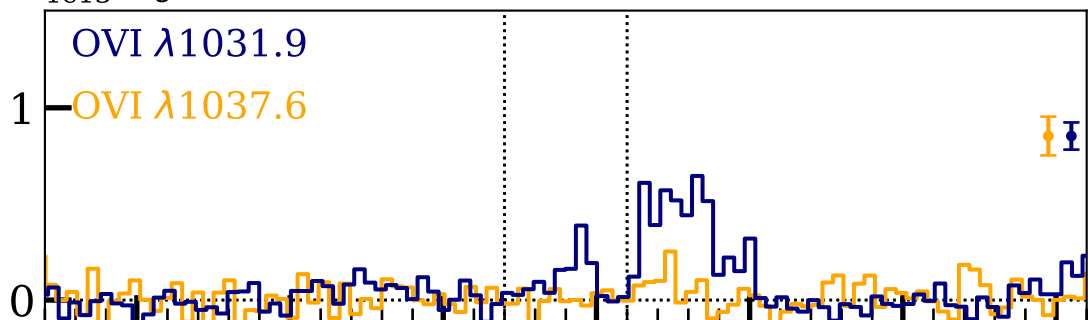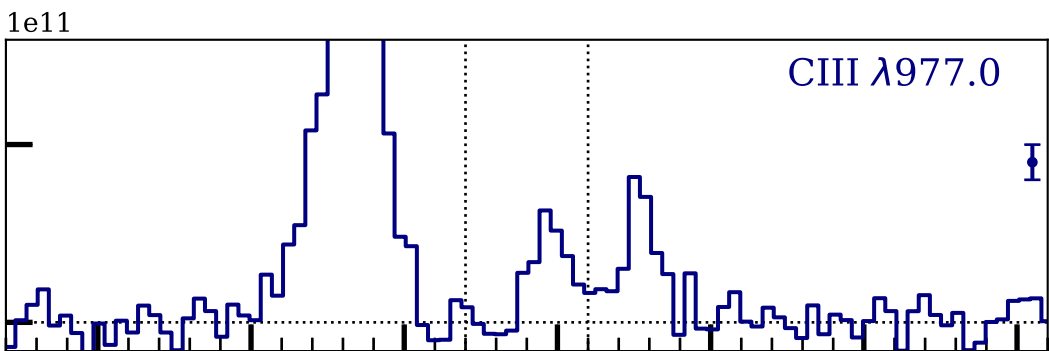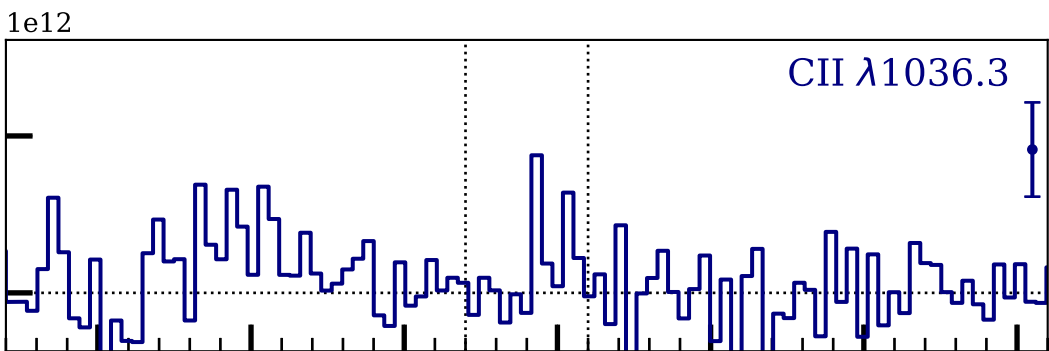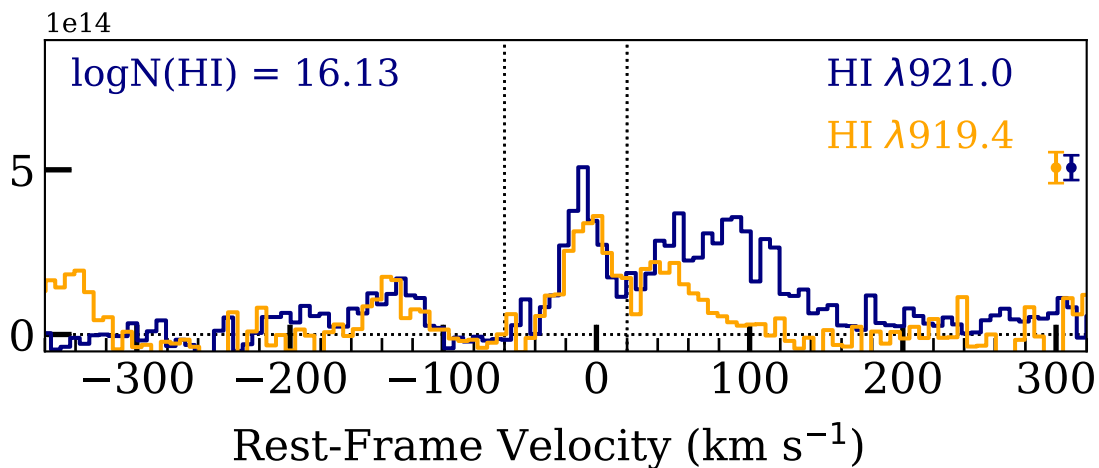

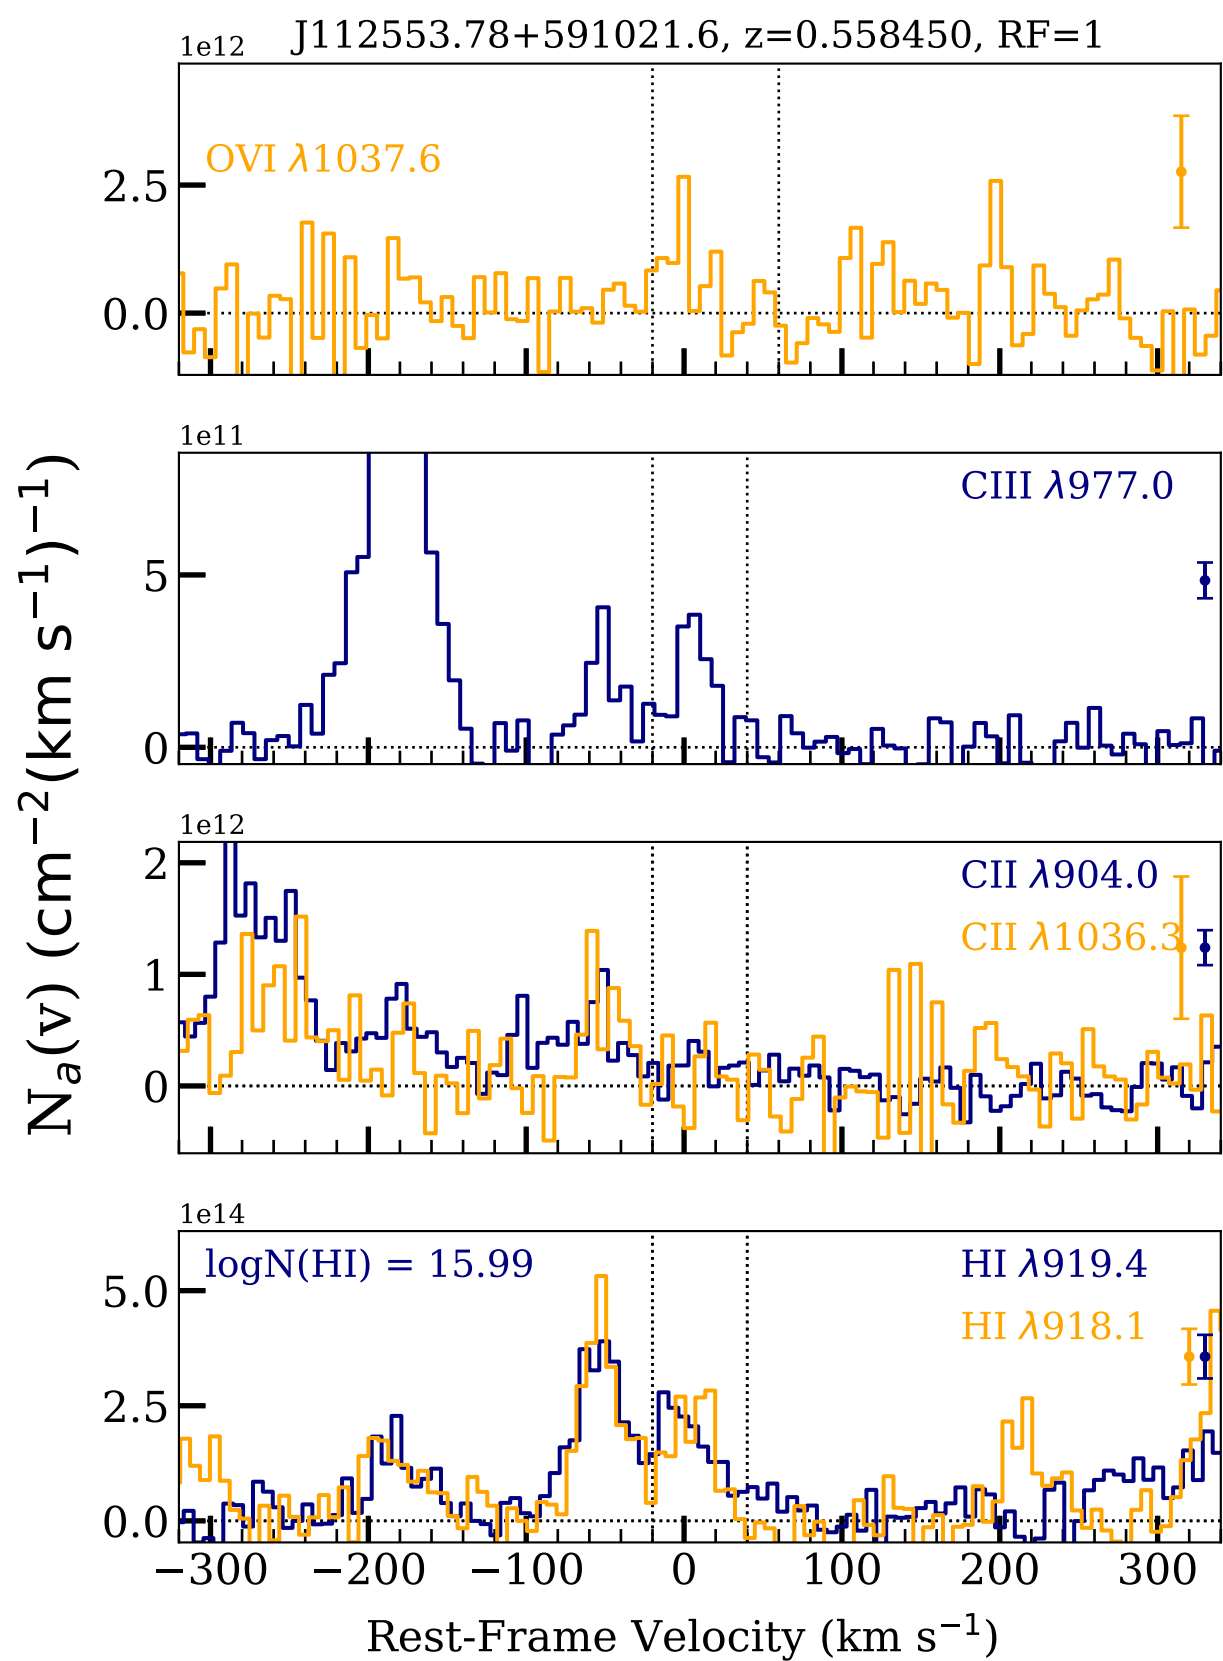

J112553.78+591021.6,  $z=0.678351$ , RF=1

$N_a(v) \text{ (cm}^{-2} \text{ (km s}^{-1} \text{)}^{-1} \text{)}$

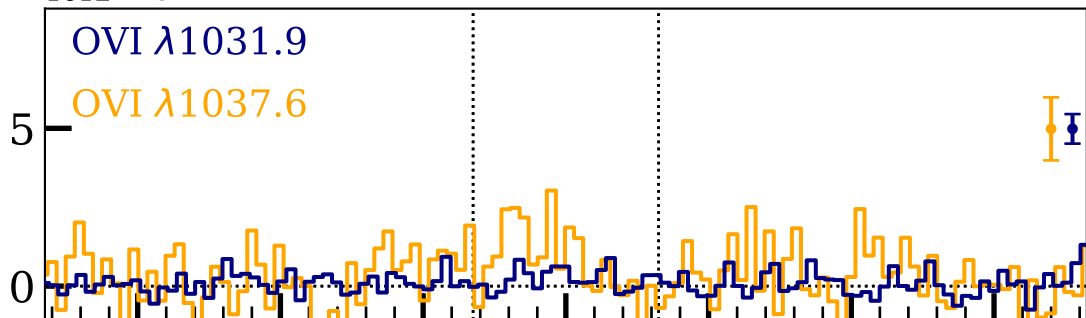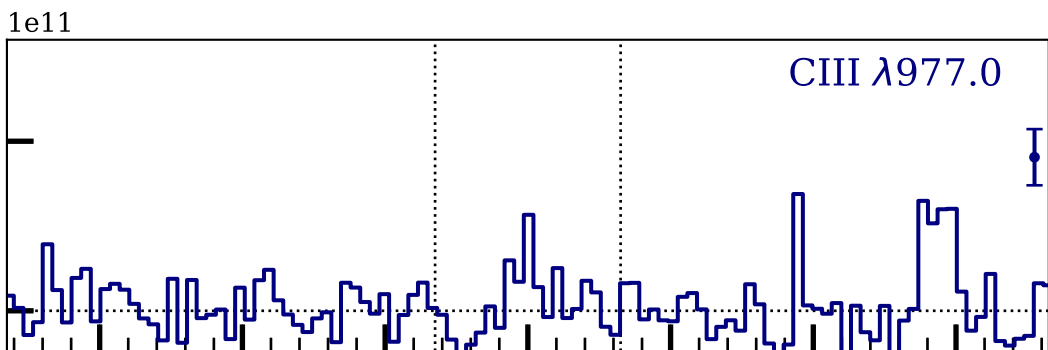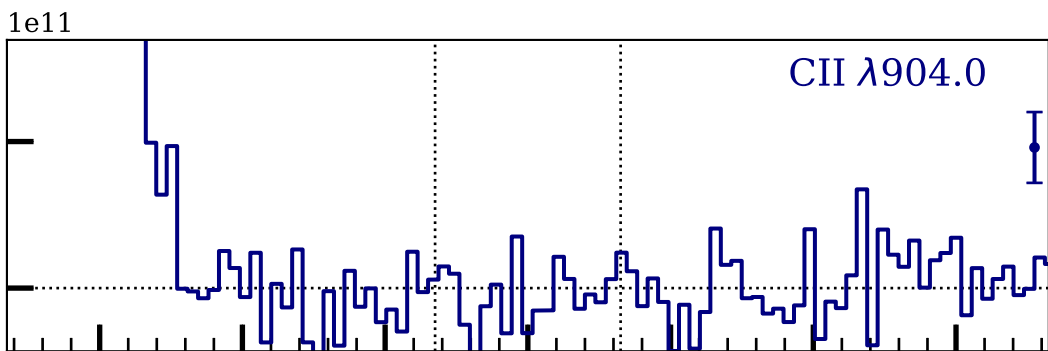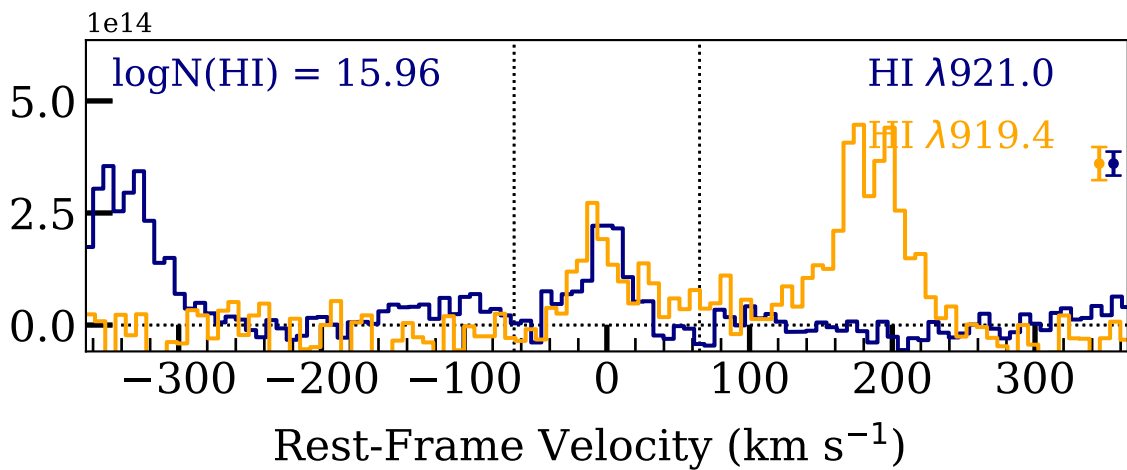

J113457.71+255527.8,  $z=0.431964$ , RF=1

$N_a(v) \text{ (cm}^{-2} \text{ (km s}^{-1} \text{)}^{-1} \text{)}$

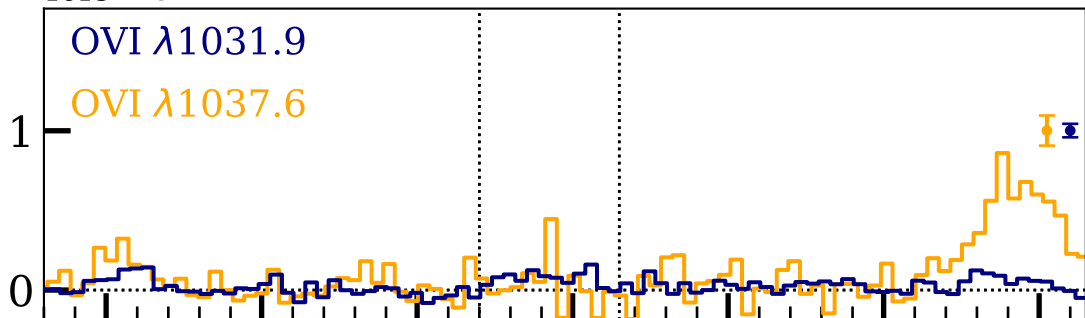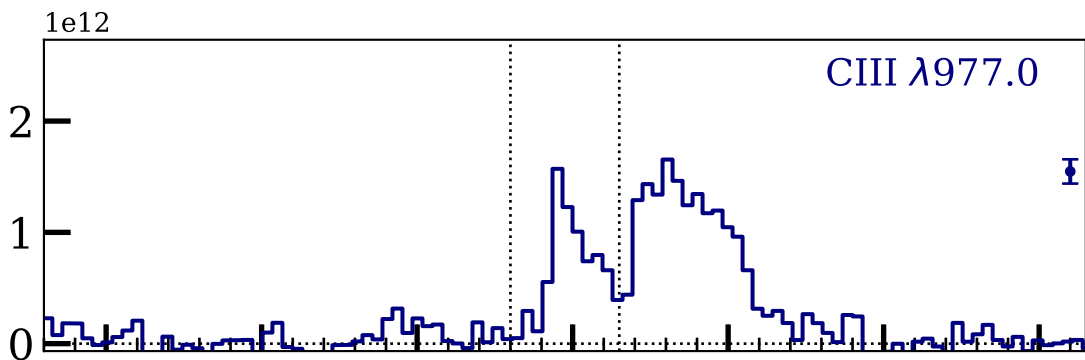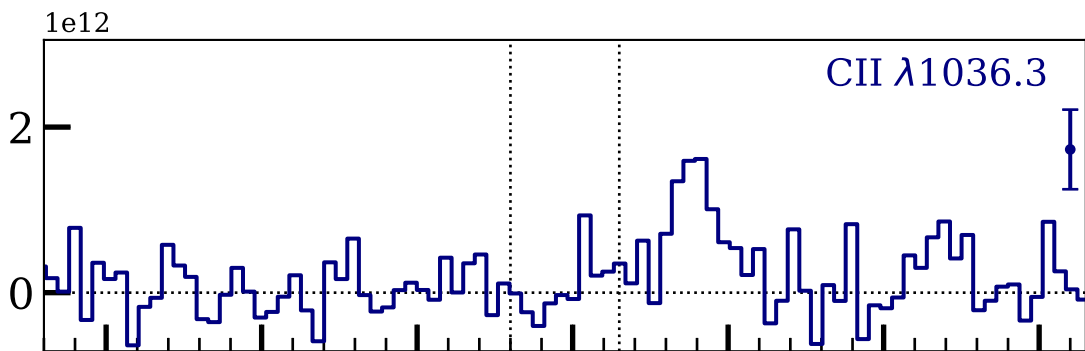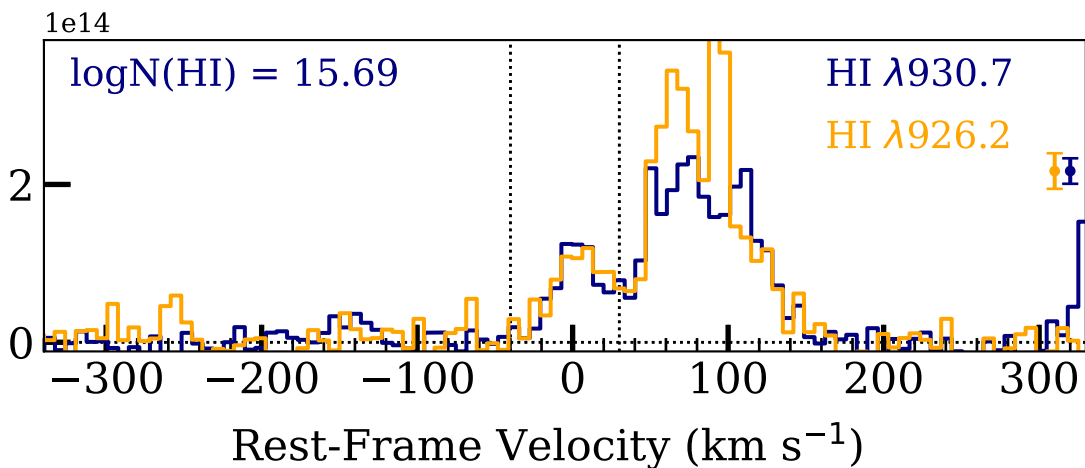



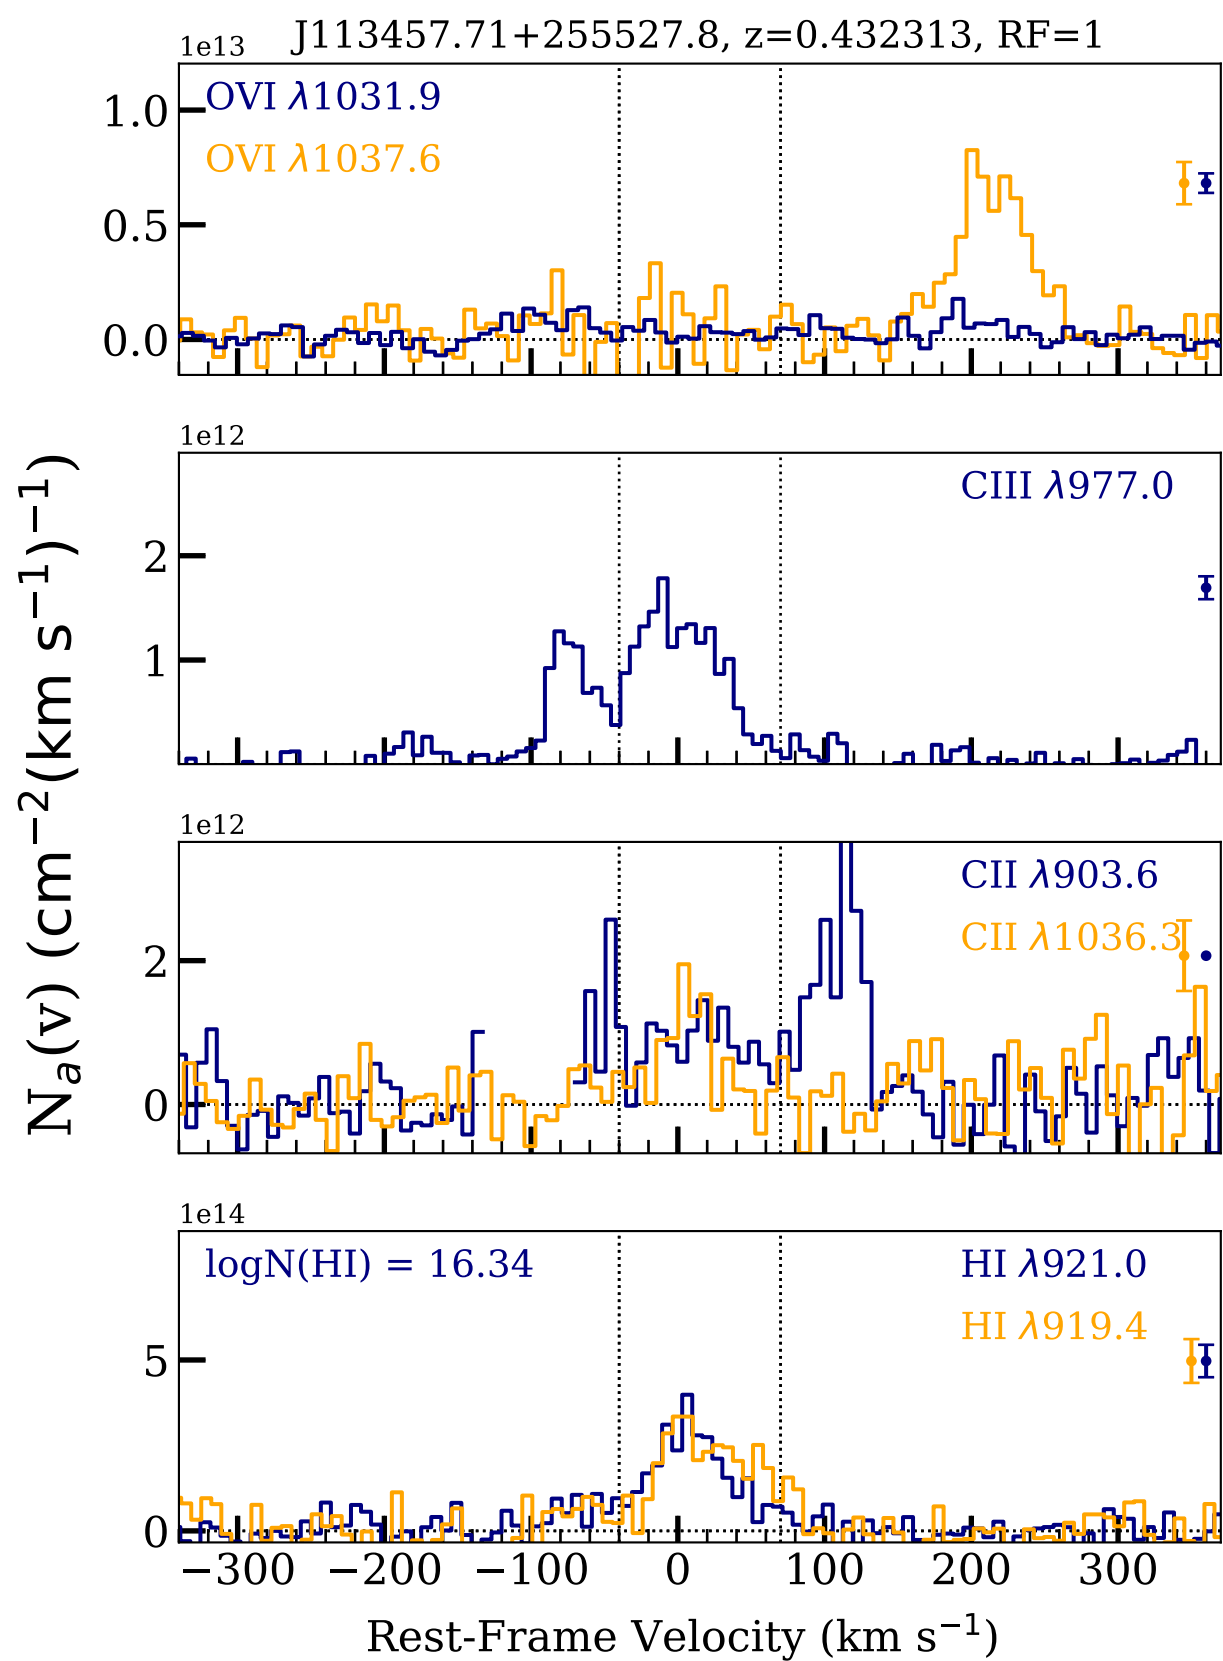

J113910.70-135044.0,  $z=0.319498$ , RF=1

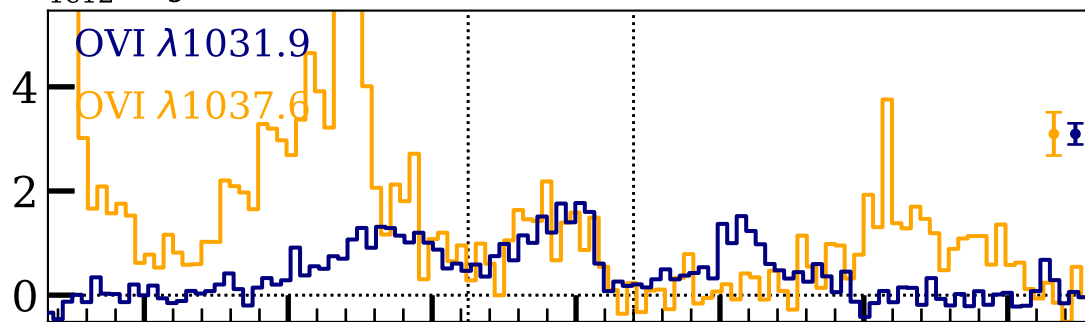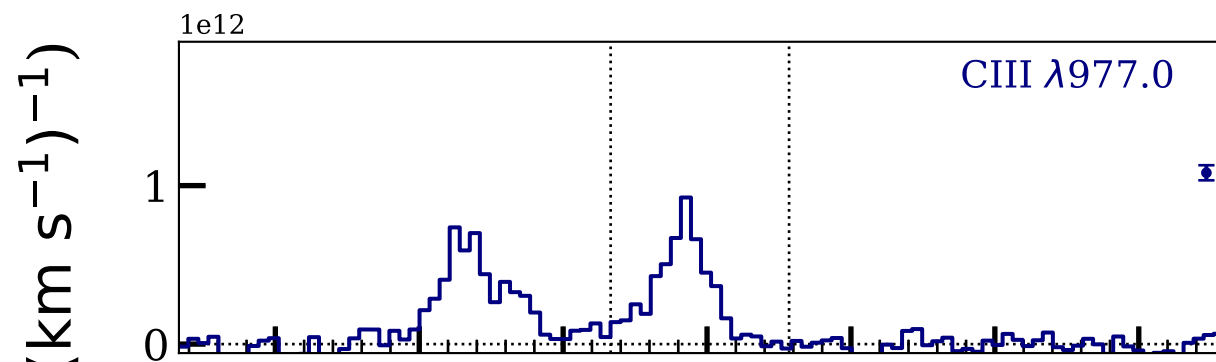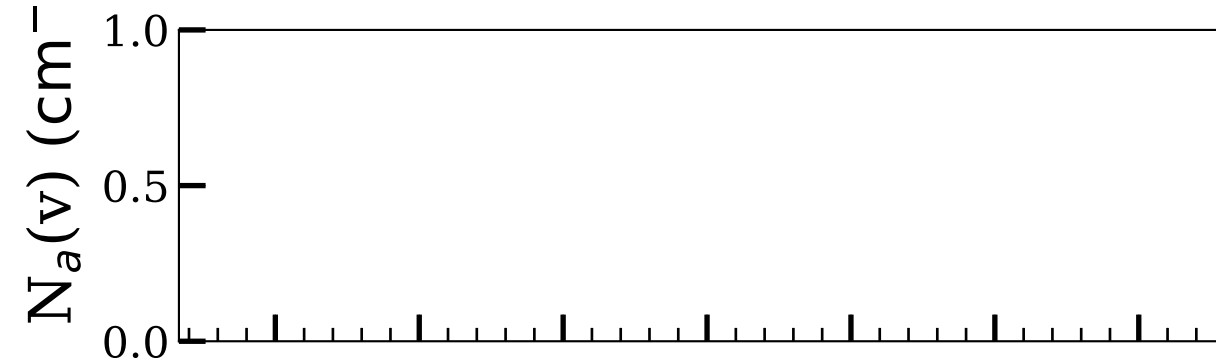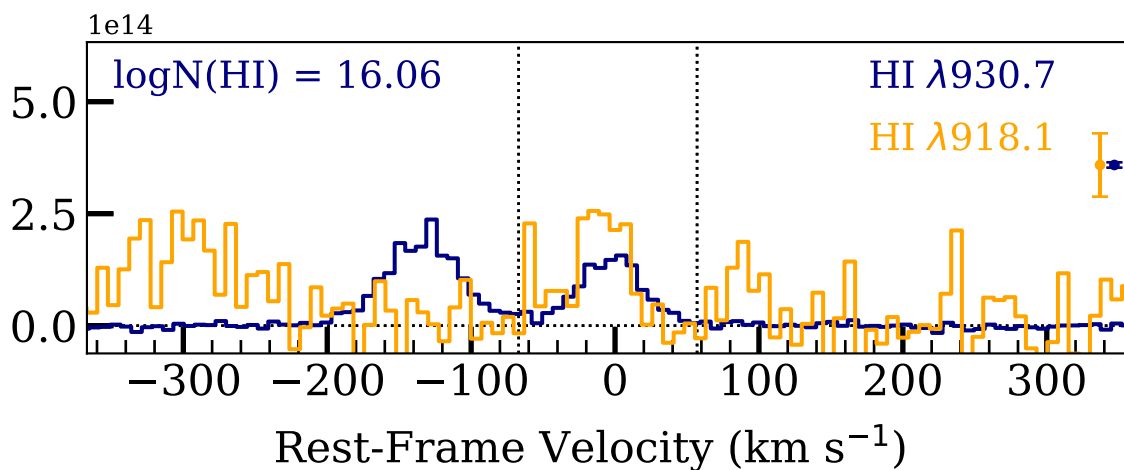

J113956.98+654749.1,  $z=0.325653$ , RF=1

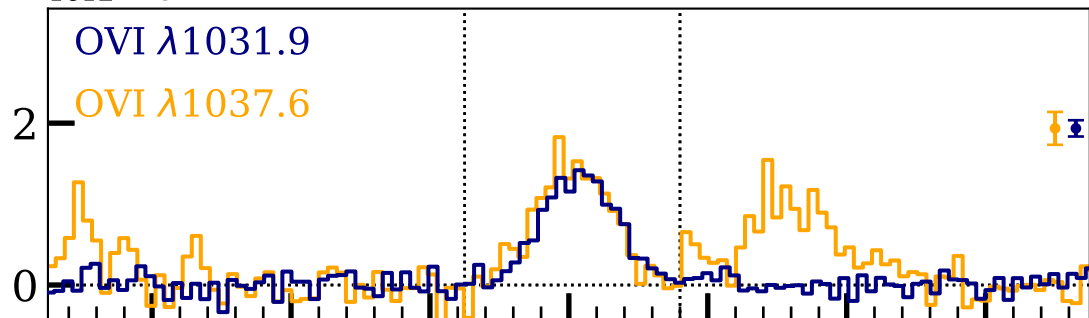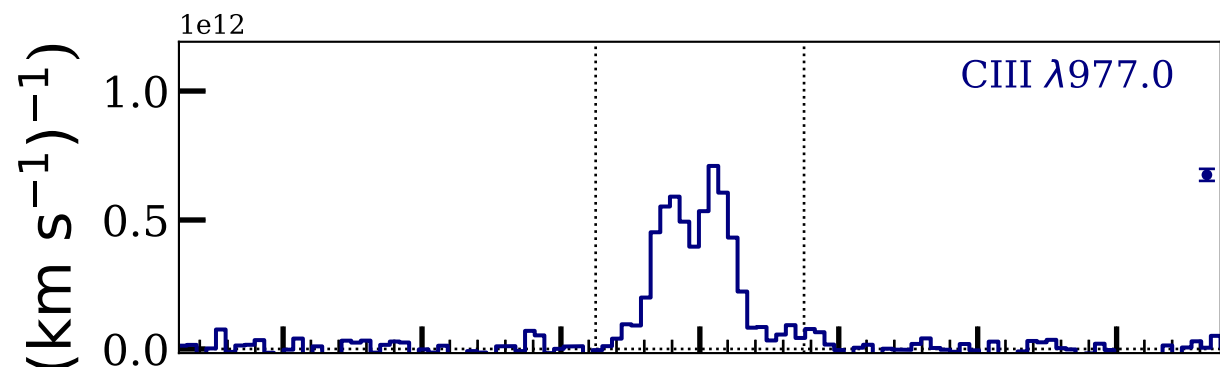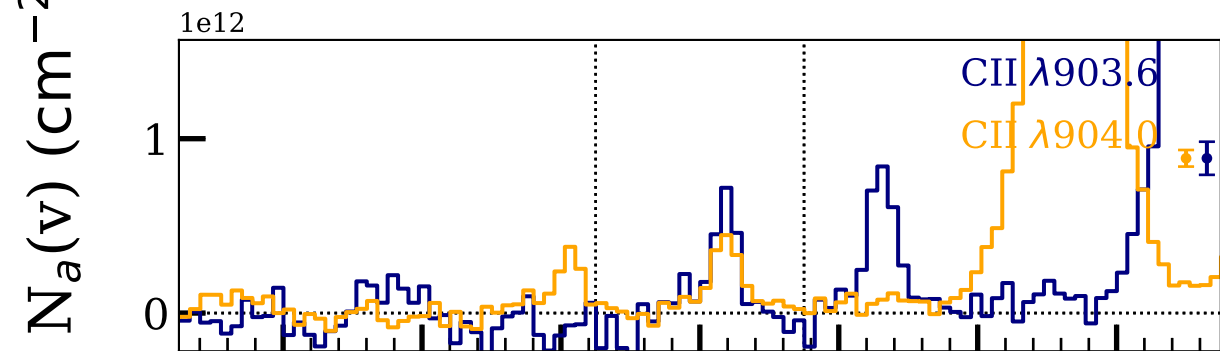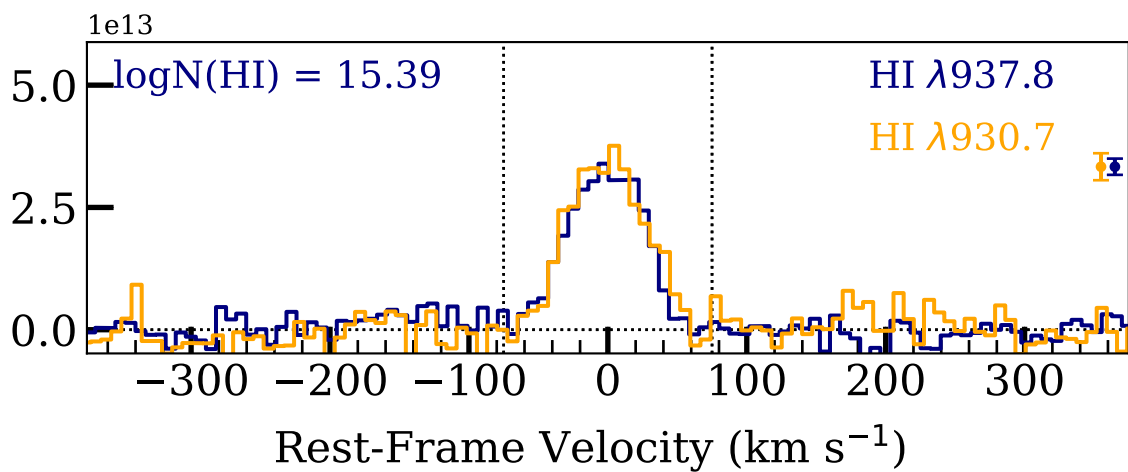

J113956.98+654749.1,  $z=0.527941$ , RF=1

$N_a(v) \text{ (cm}^{-2} \text{ (km s}^{-1} \text{)}^{-1} \text{)}$

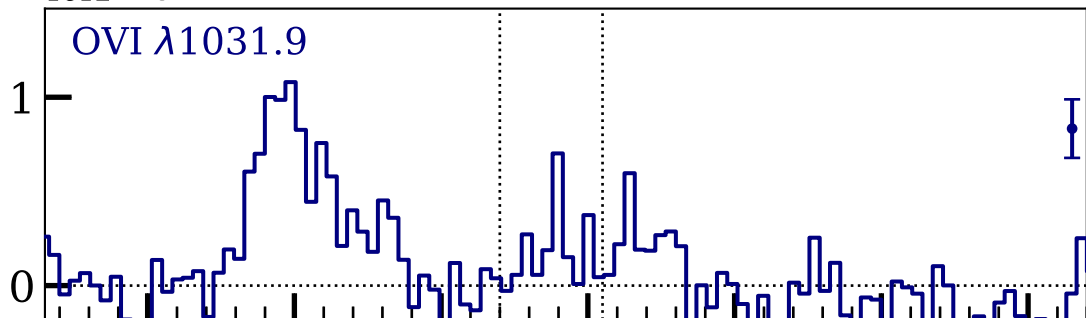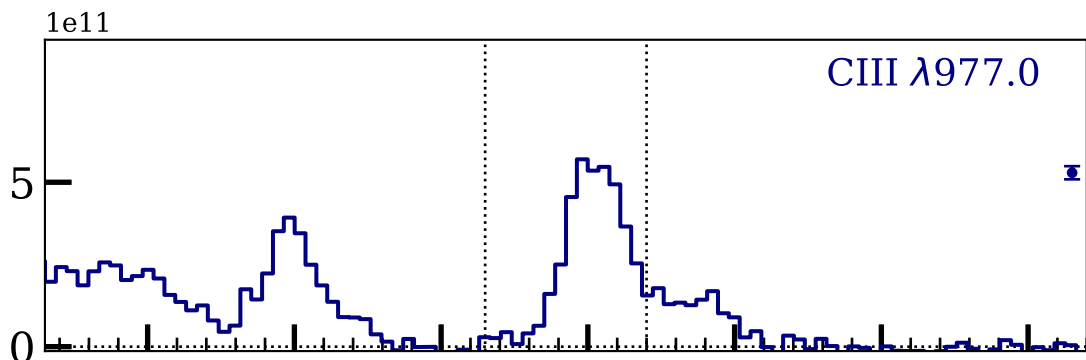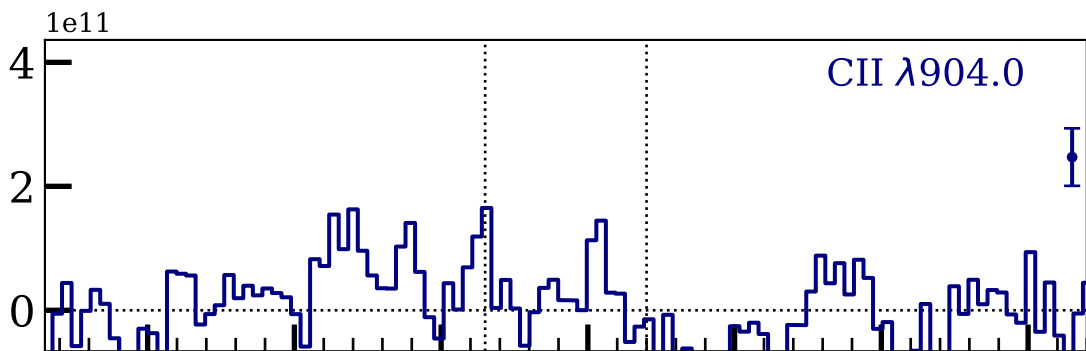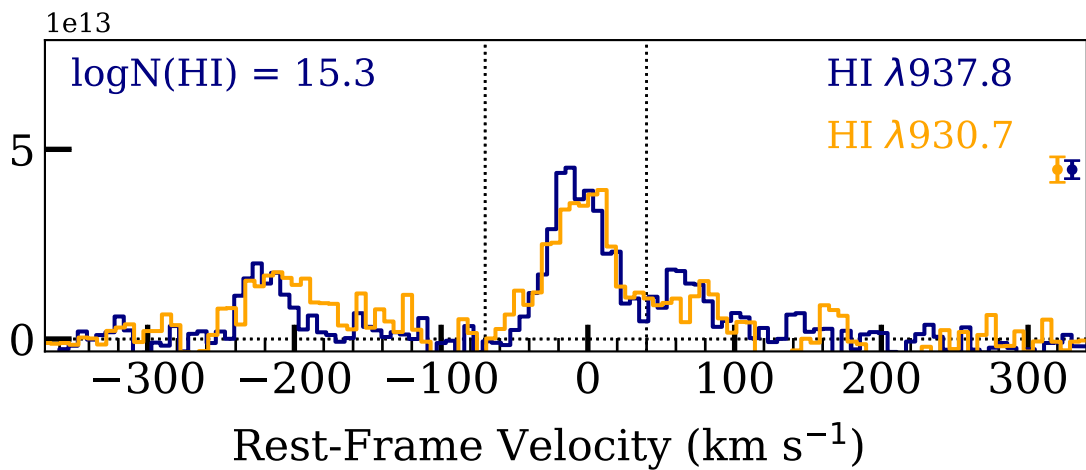

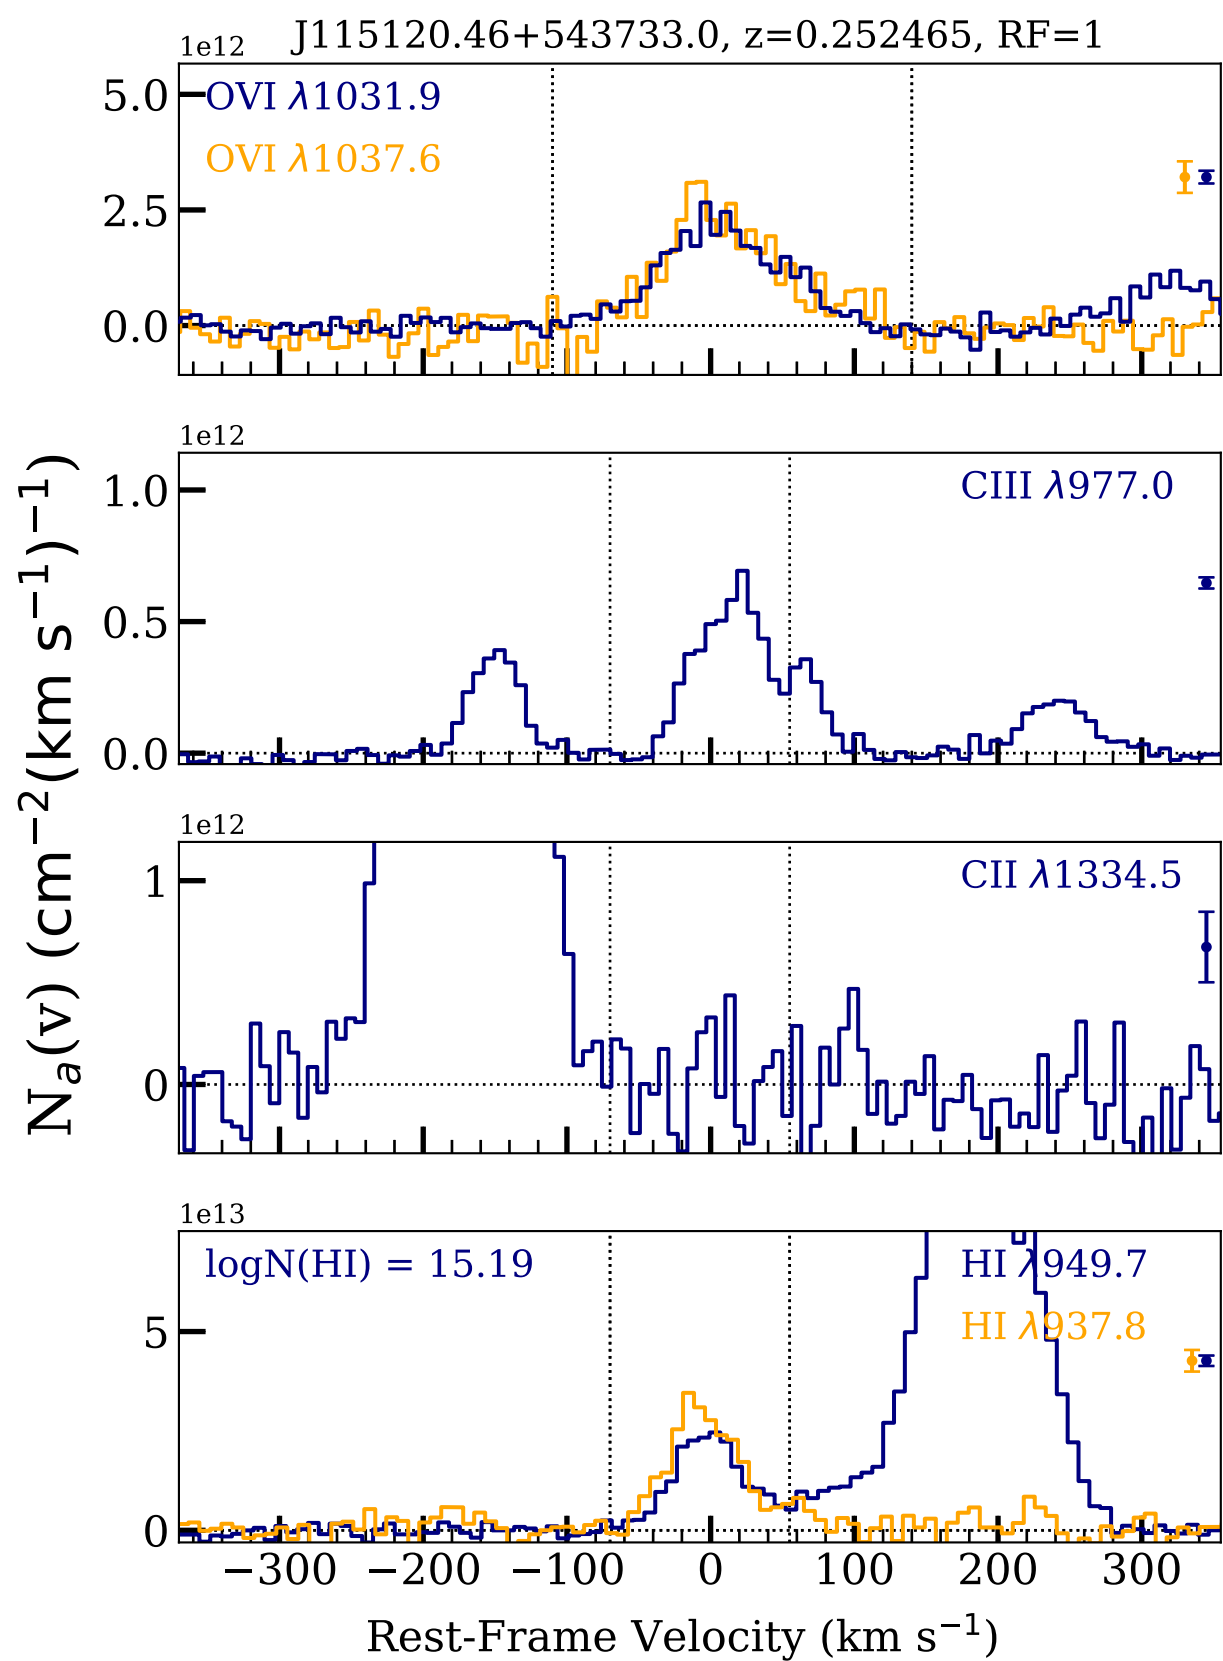

J115120.46+543733.0,  $z=0.688567$ , RF=1

$N_a(v) \text{ (cm}^{-2} \text{ (km s}^{-1} \text{)}^{-1} \text{)}$

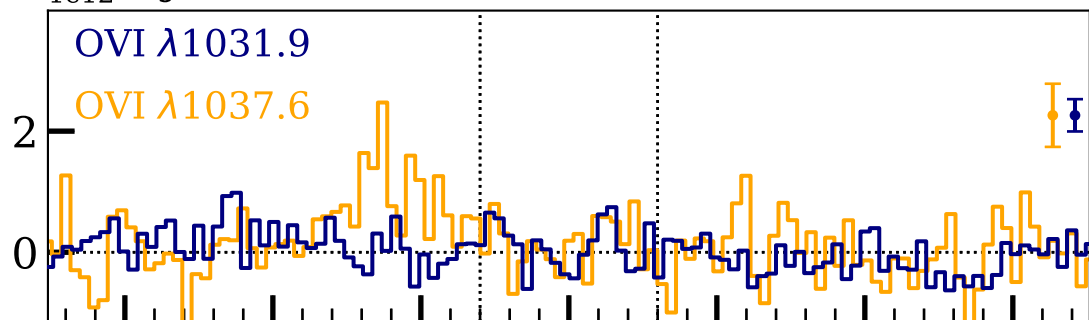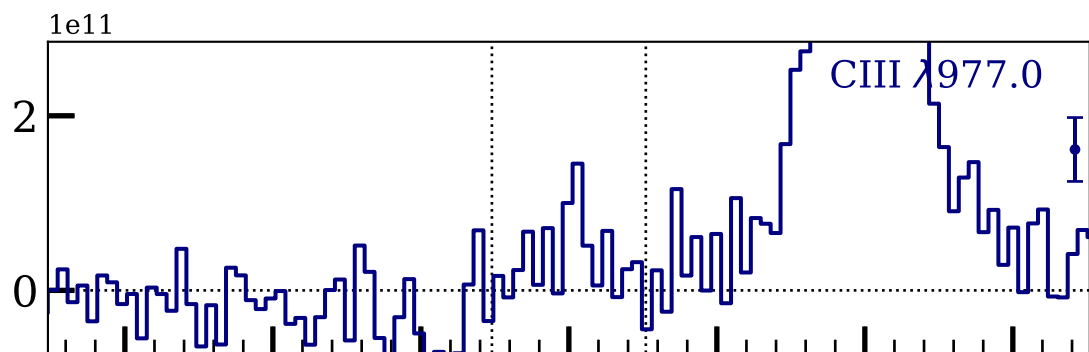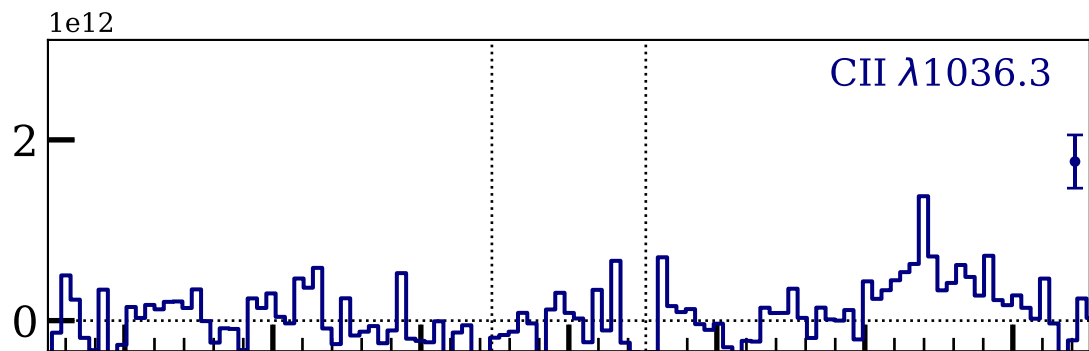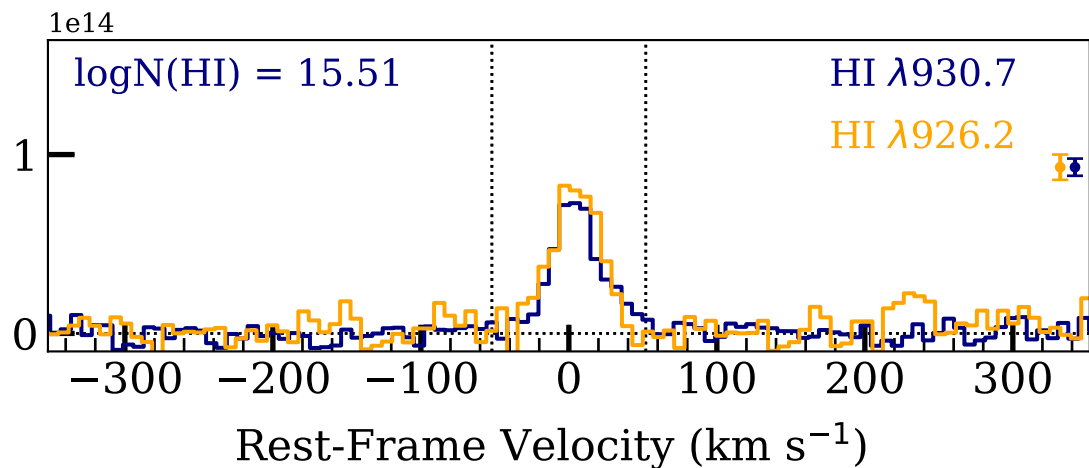

J120158.75-135459.9,  $z=0.409358$ , RF=0

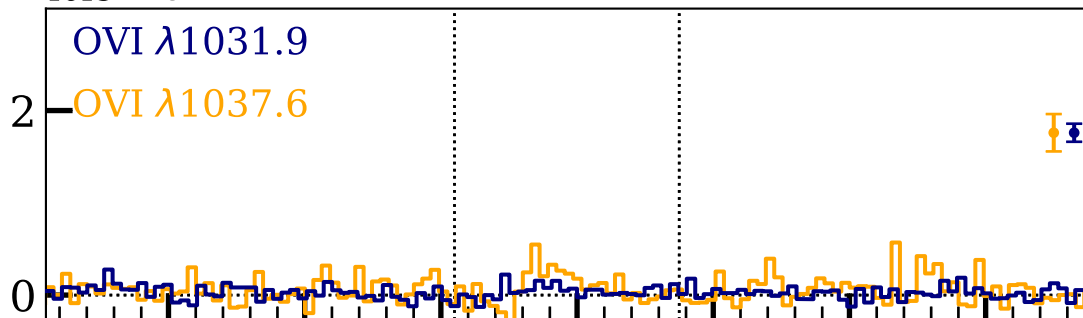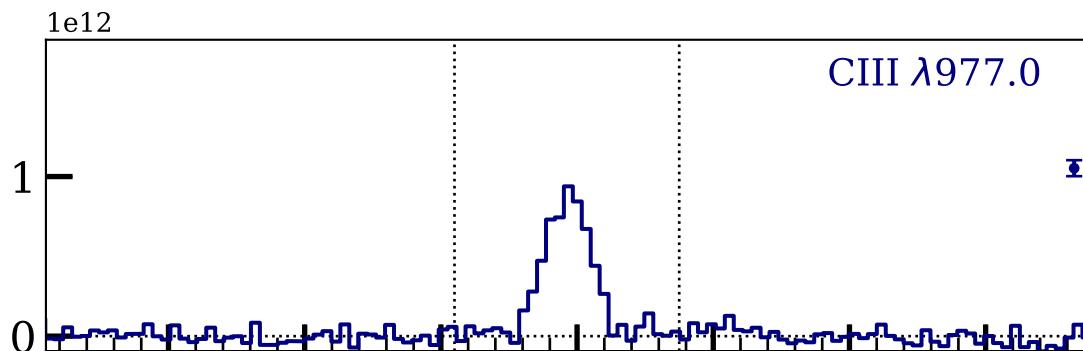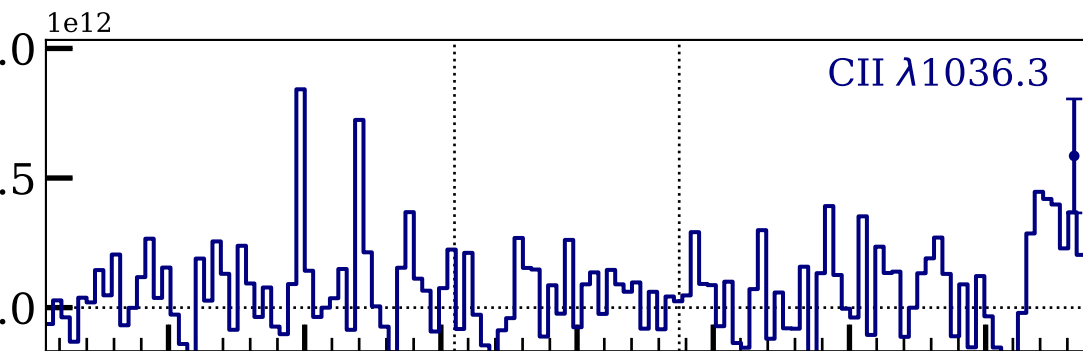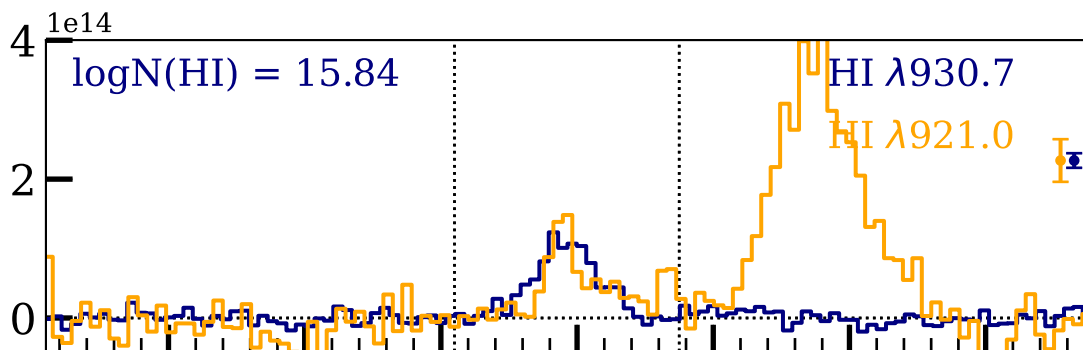

Rest-Frame Velocity ( $\text{km s}^{-1}$ )

1e12 J121430.55+082508.1,  $z=0.324710$ , RF=1

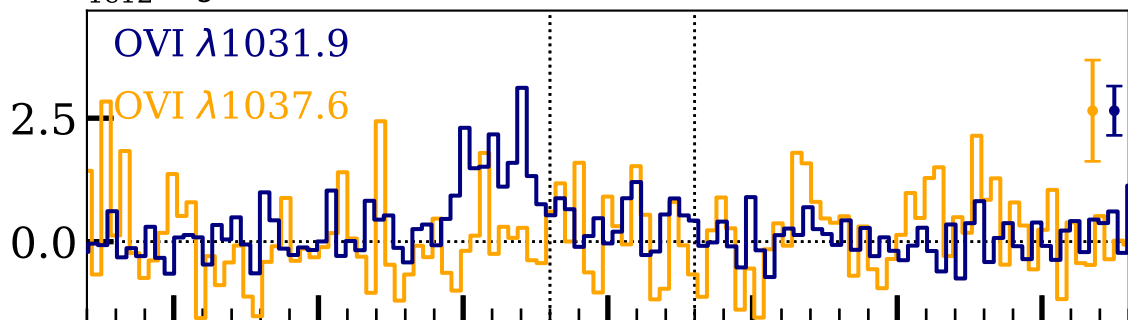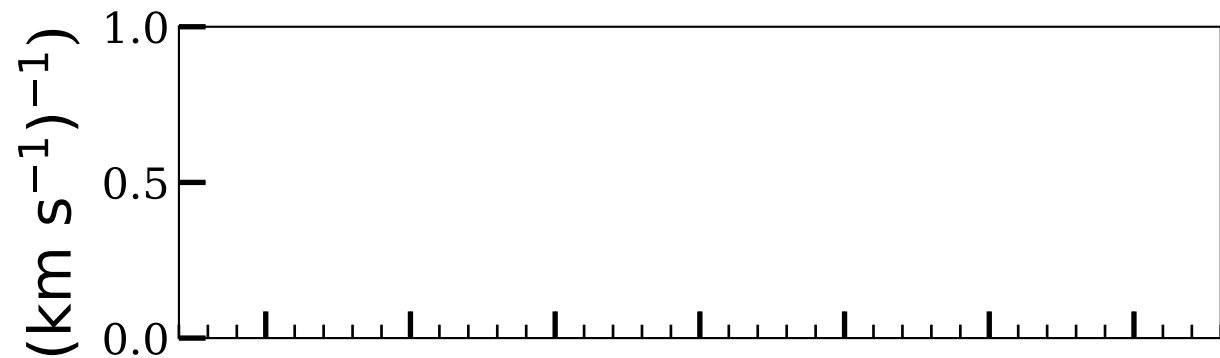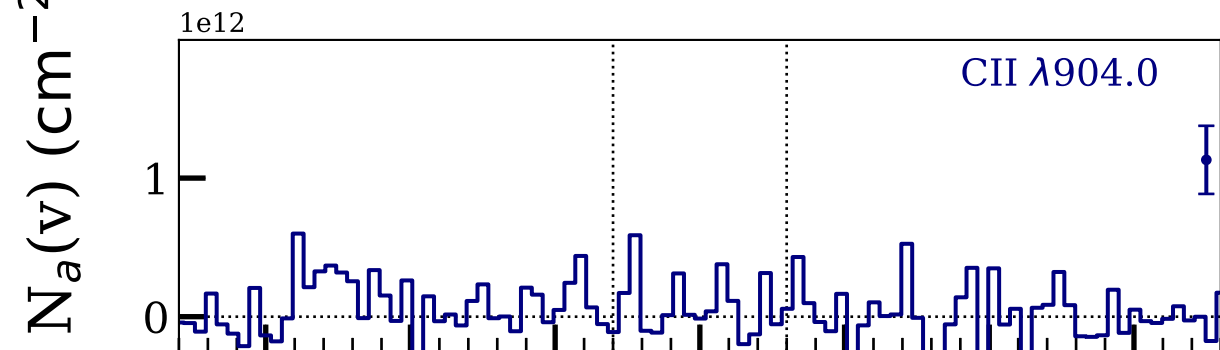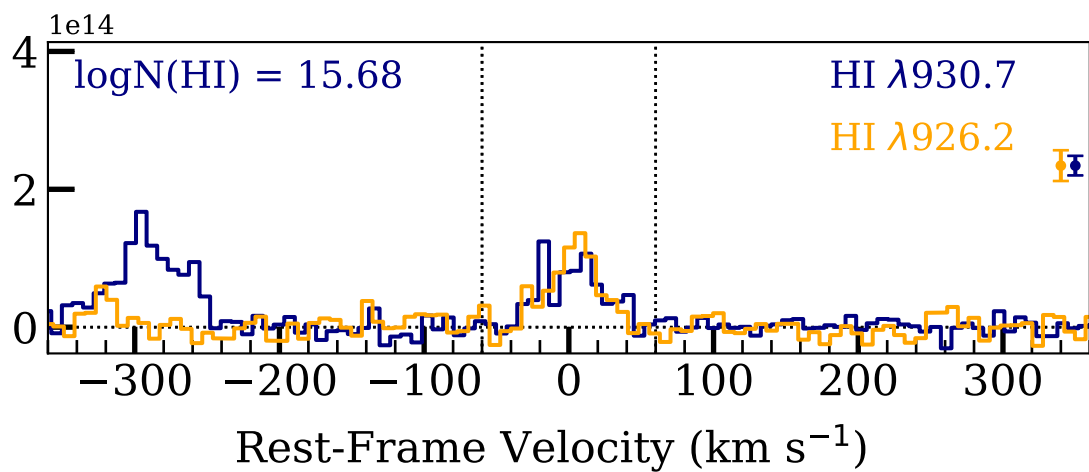



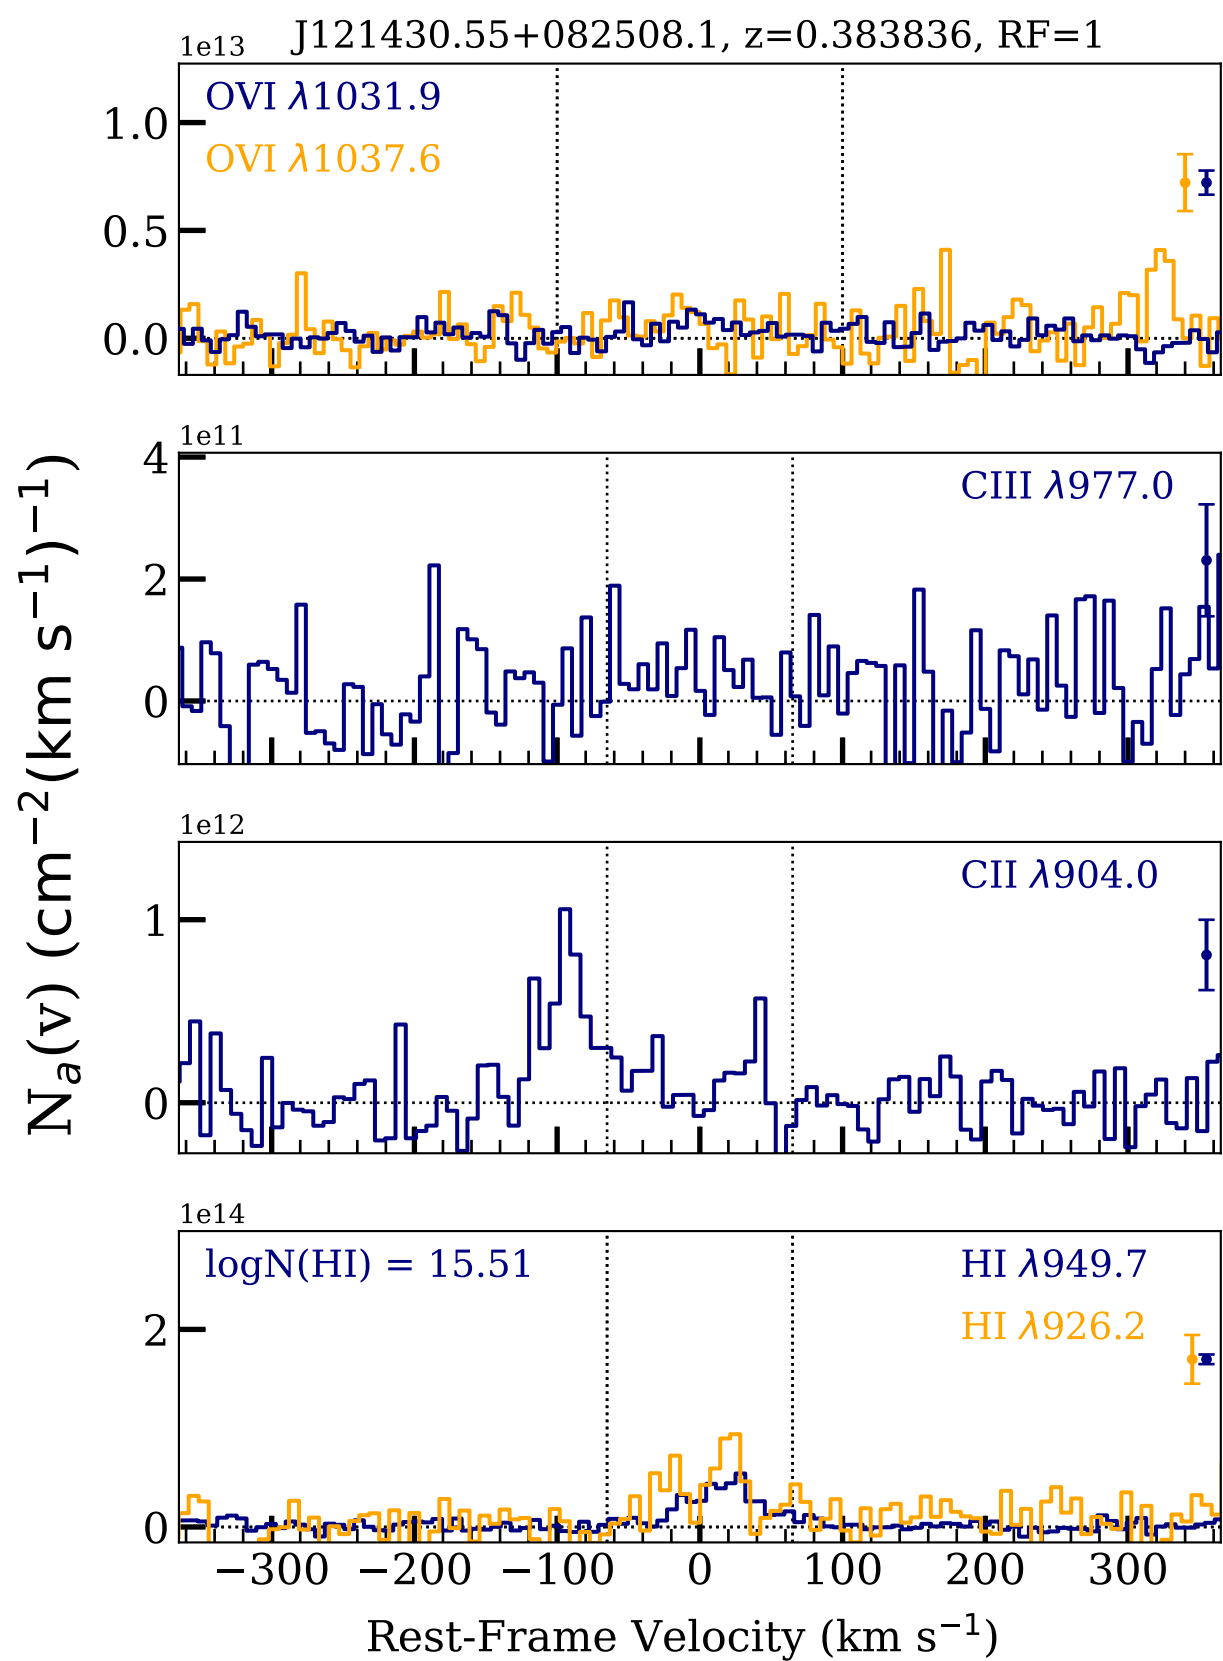

J121640.56+071224.3,  $z=0.382433$ , RF=0

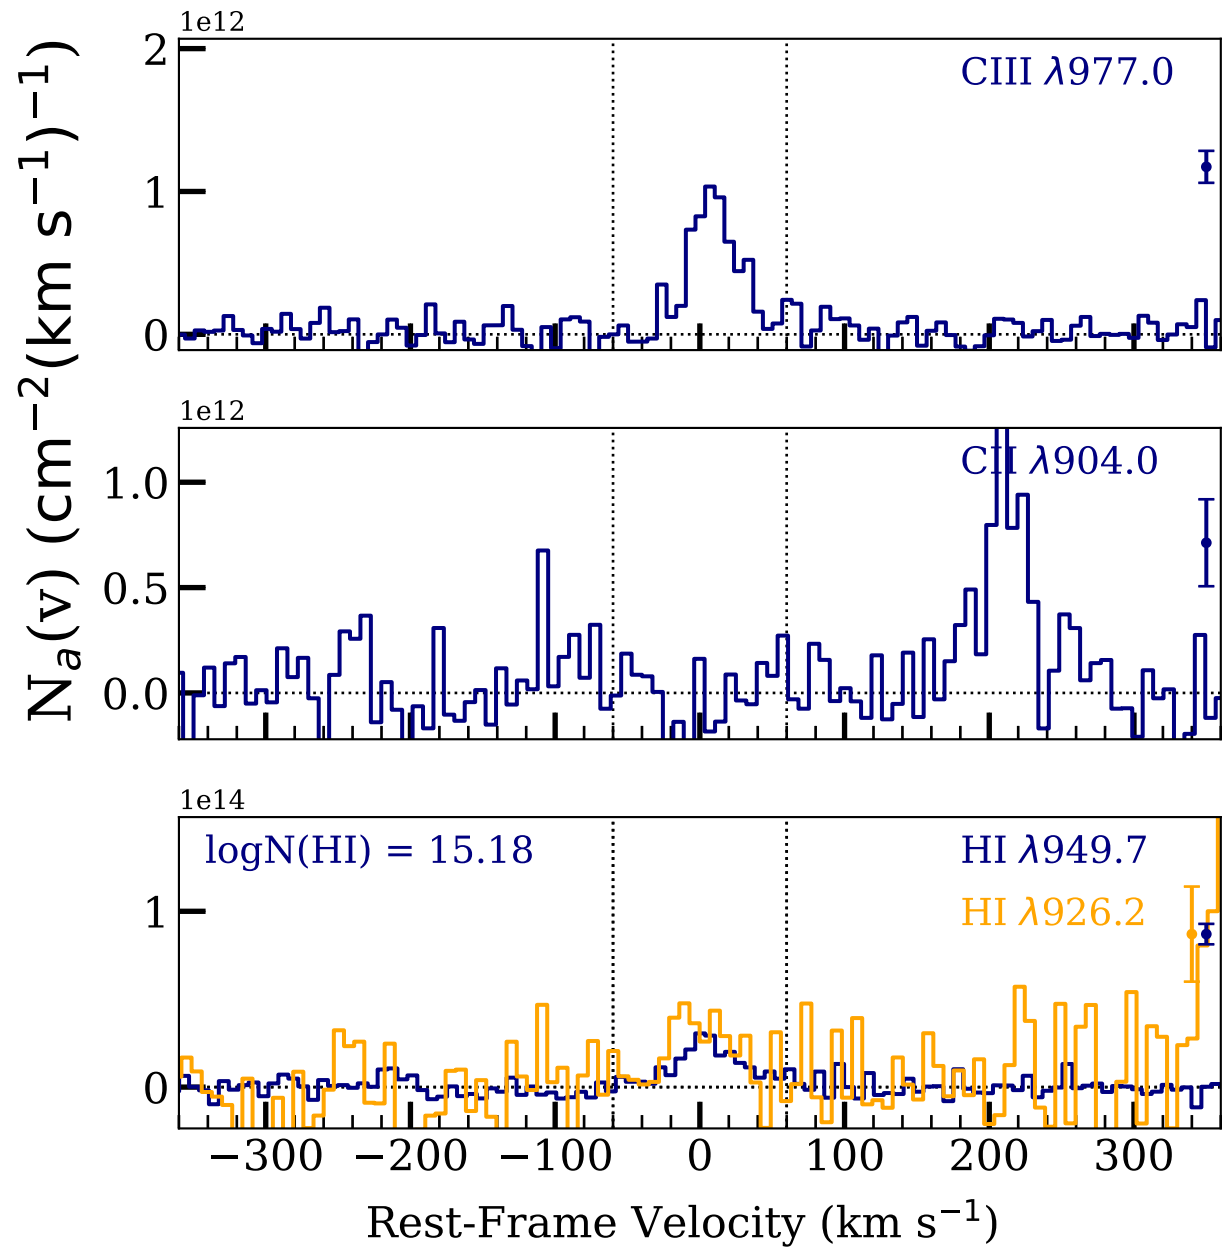

1e12 J121920.93+063838.5, z=0.282308, RF=1

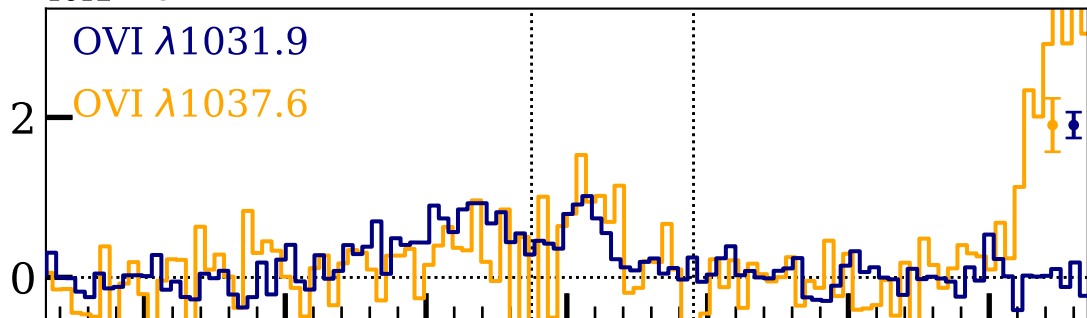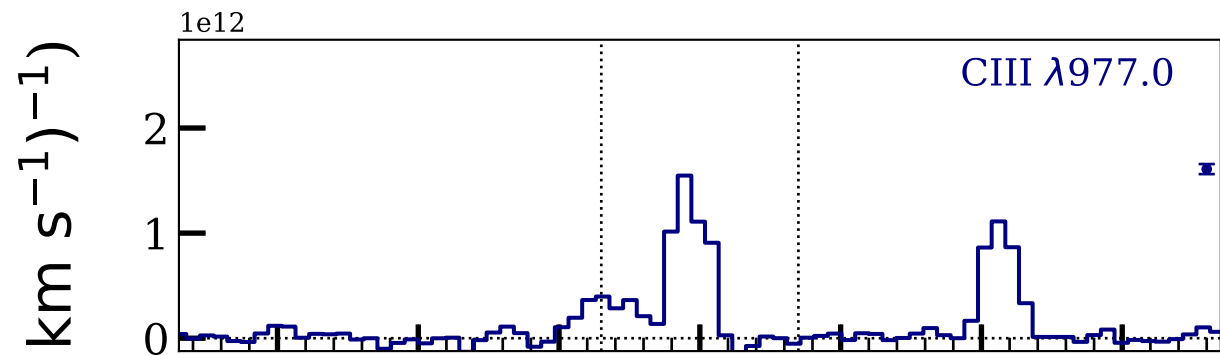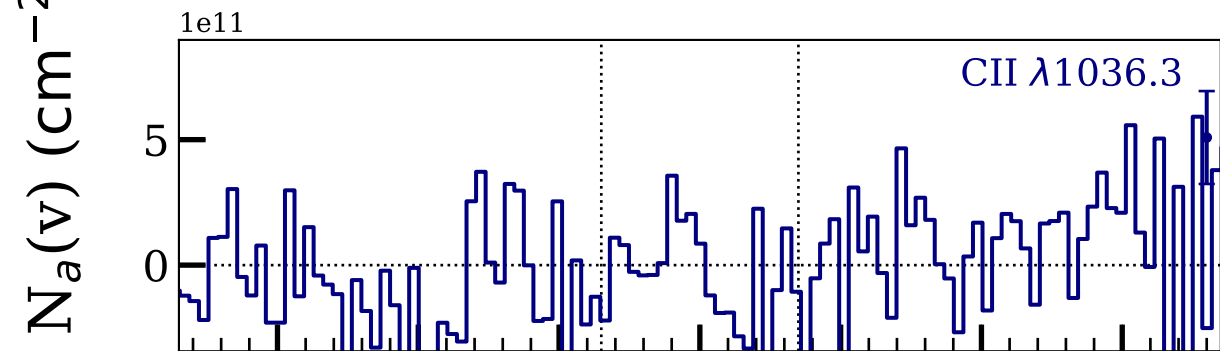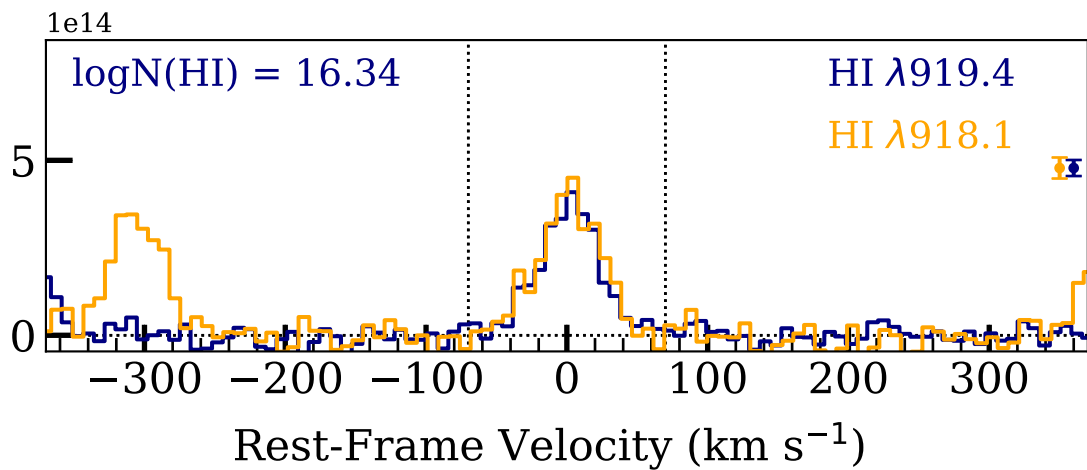

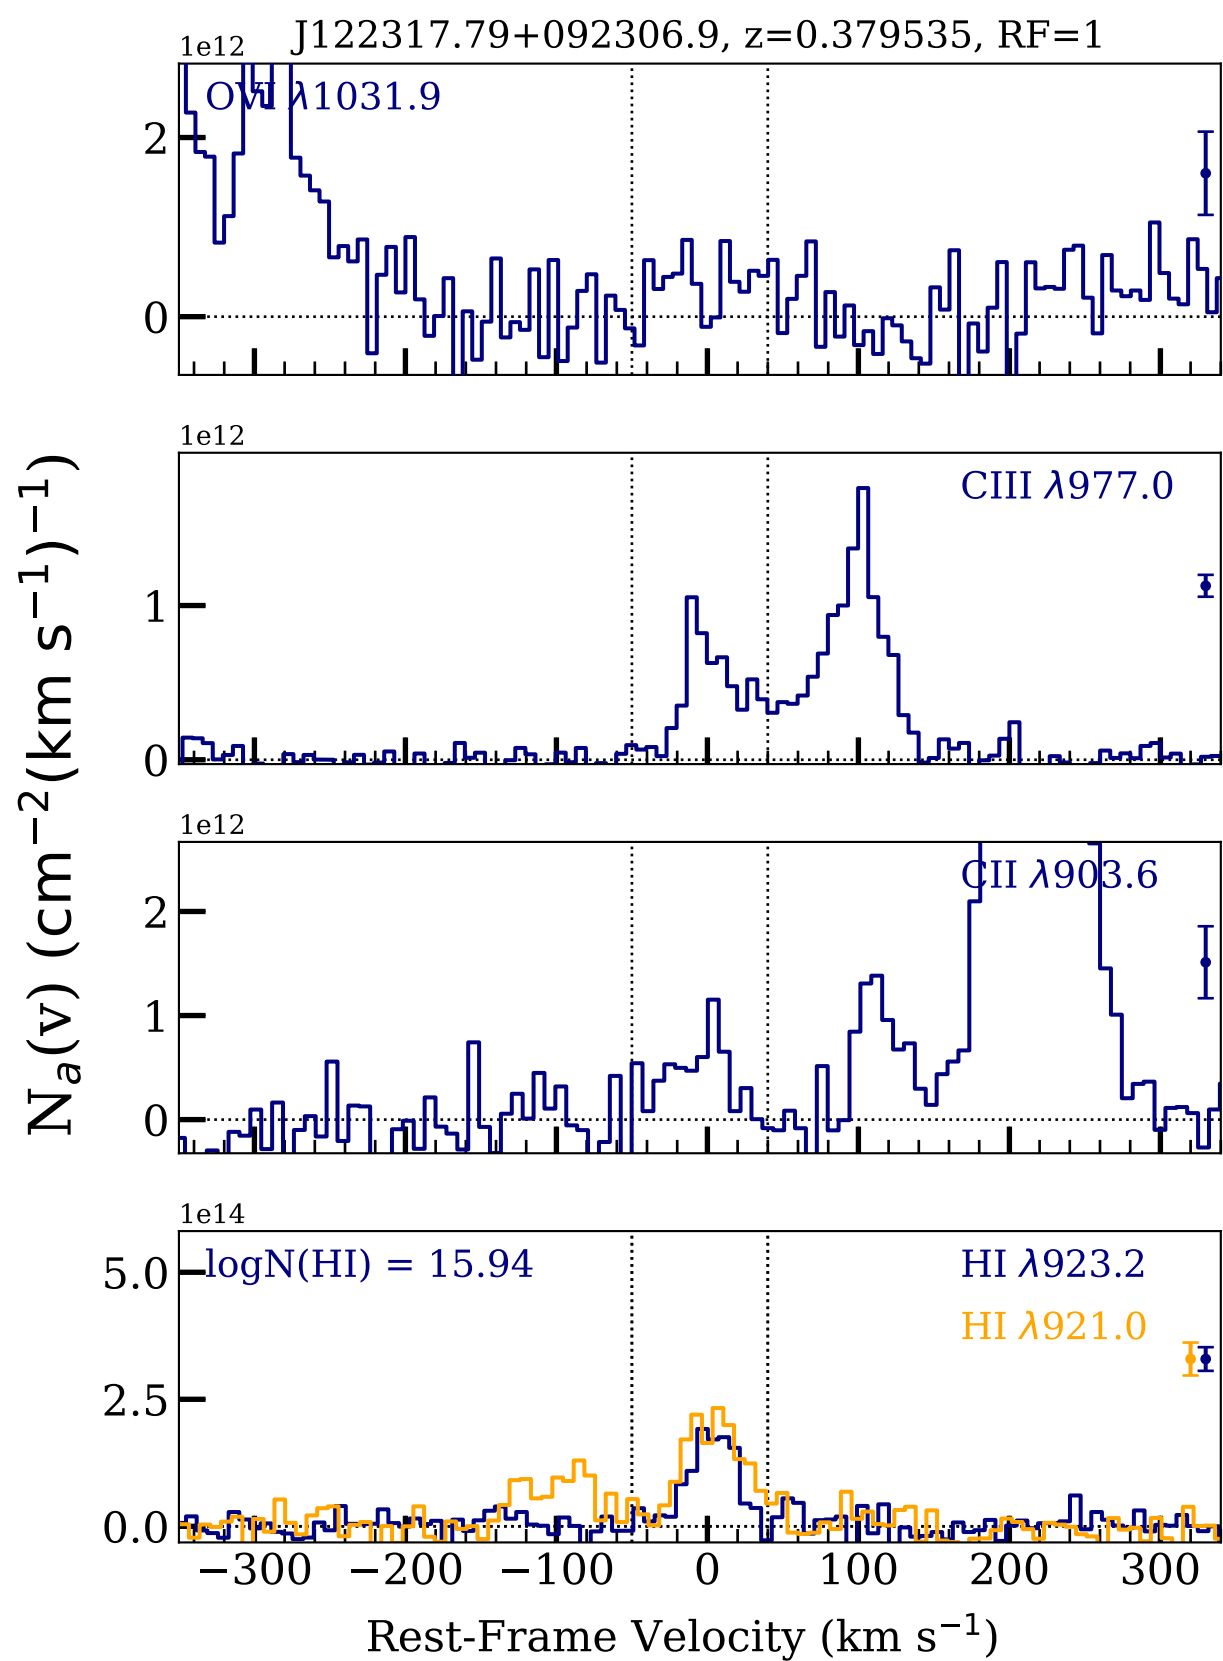

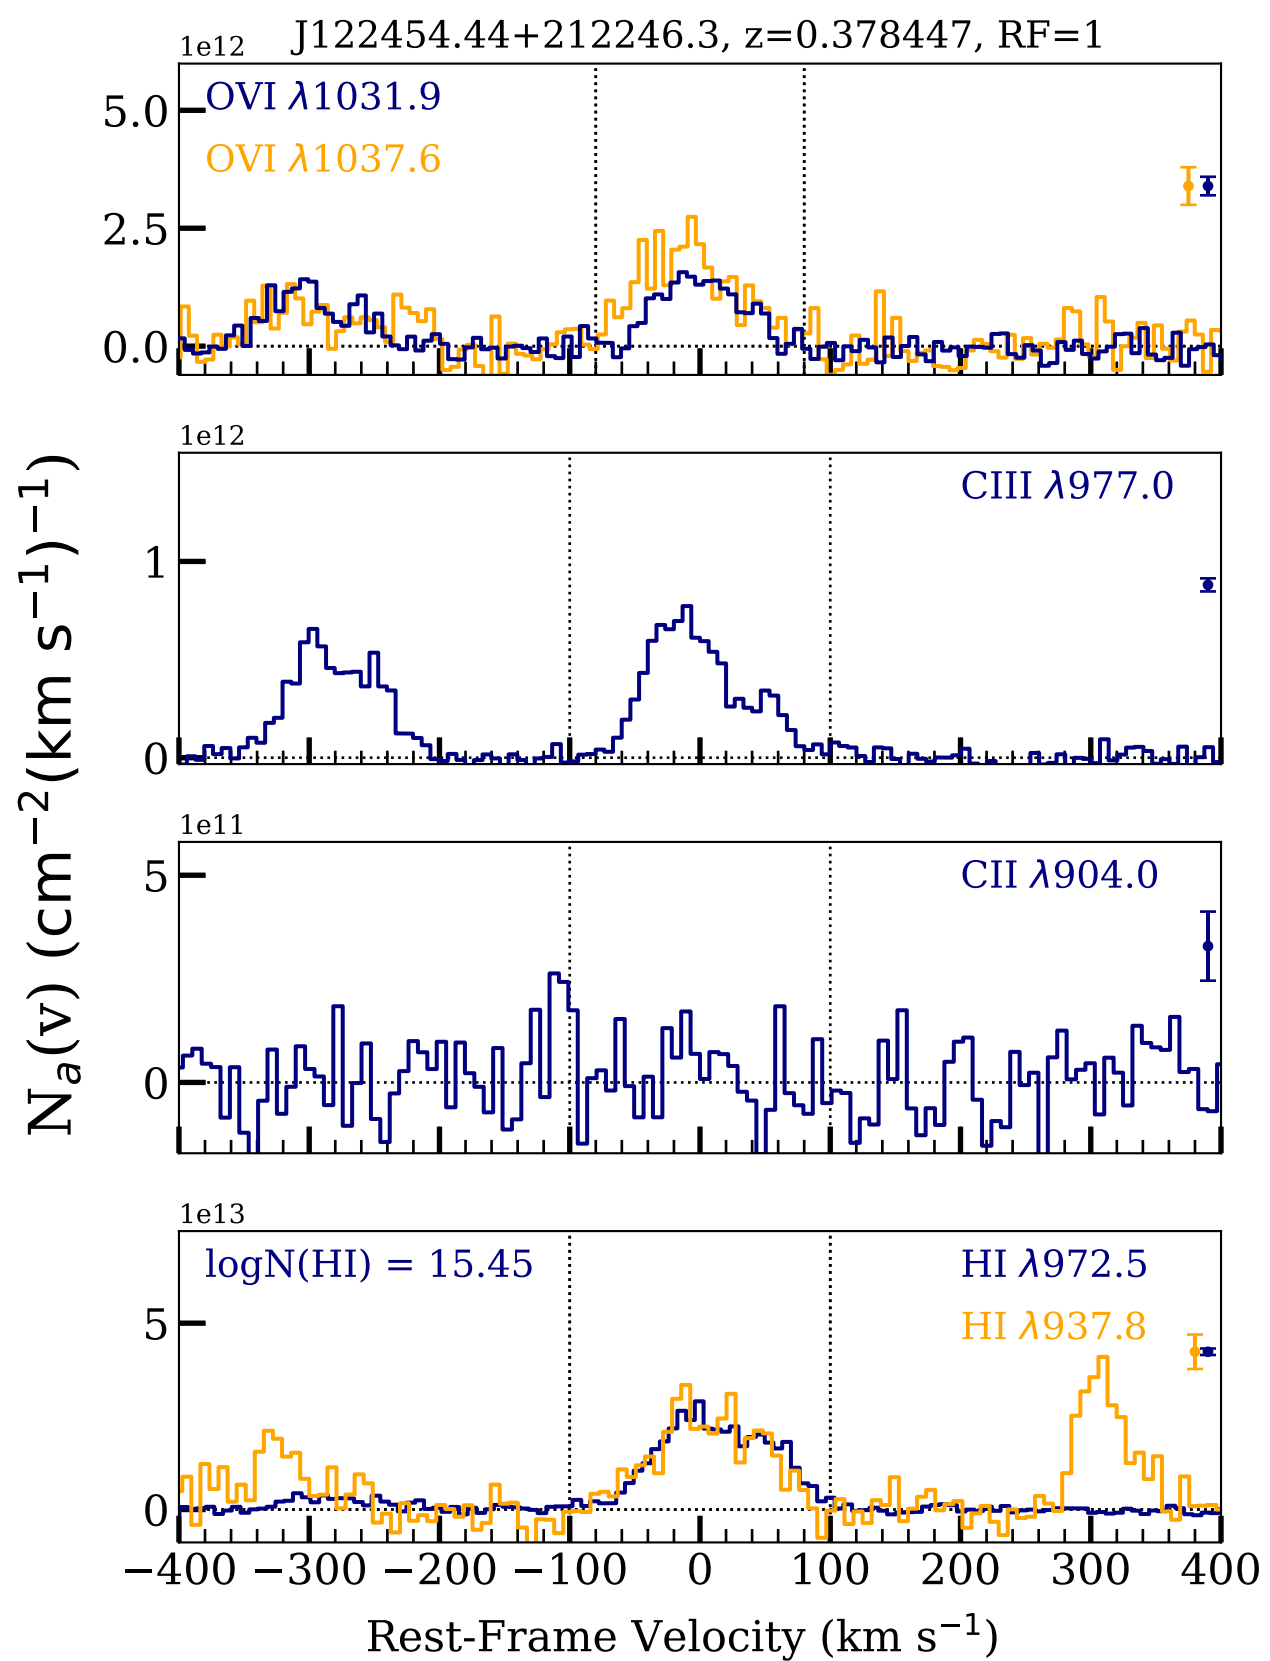

J122454.44+212246.3,  $z=0.420788$ , RF=1

$N_a(v)$  ( $\text{cm}^{-2}(\text{km s}^{-1})^{-1}$ )

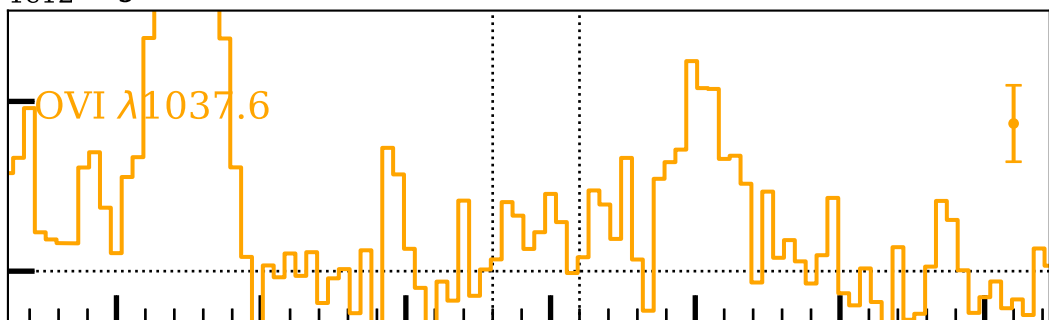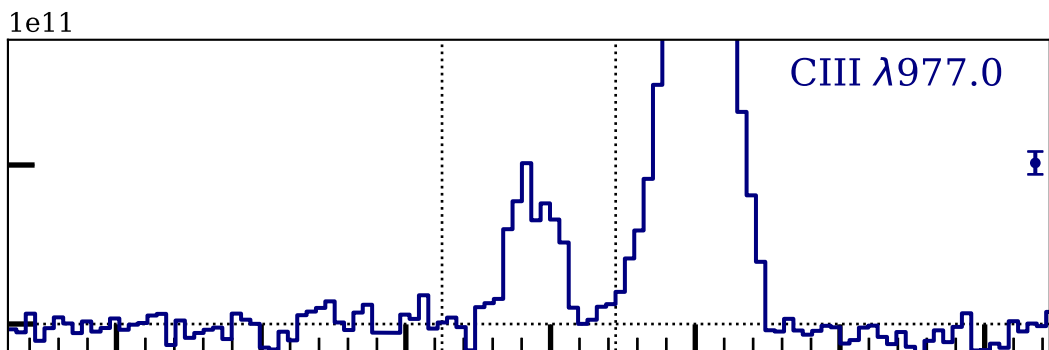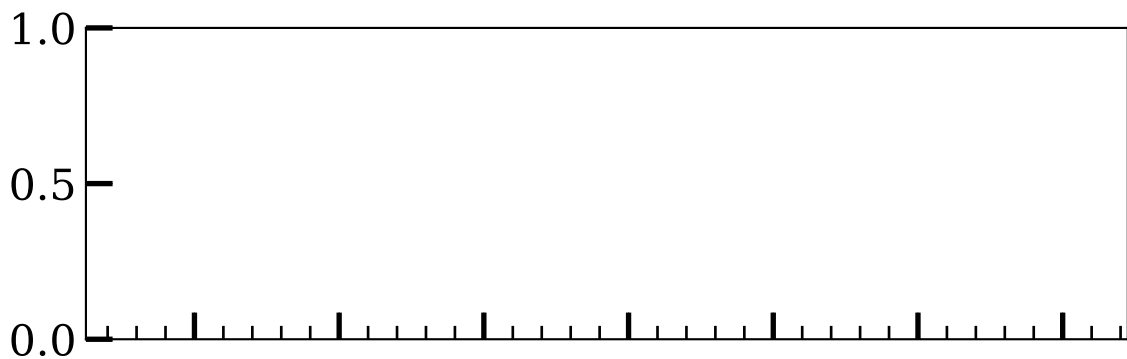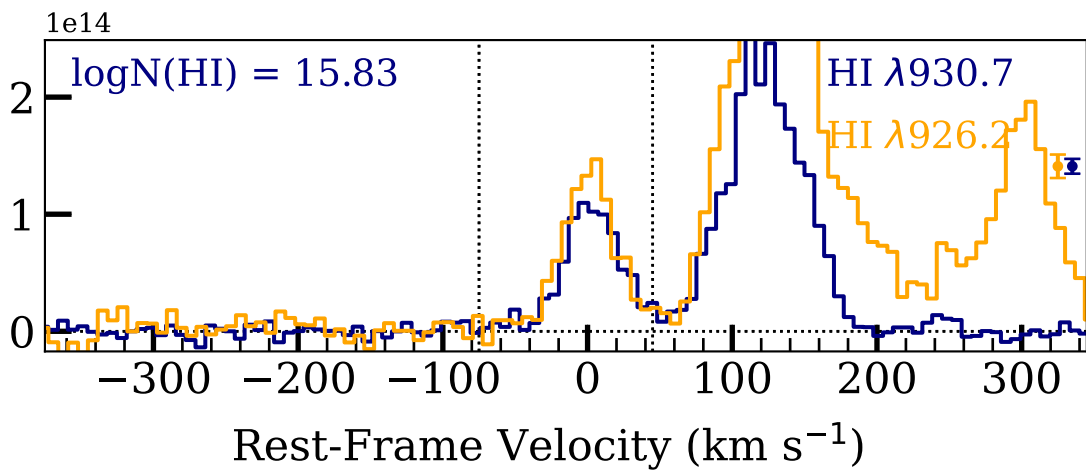

J122454.44+212246.3,  $z=0.421357$ , RF=1

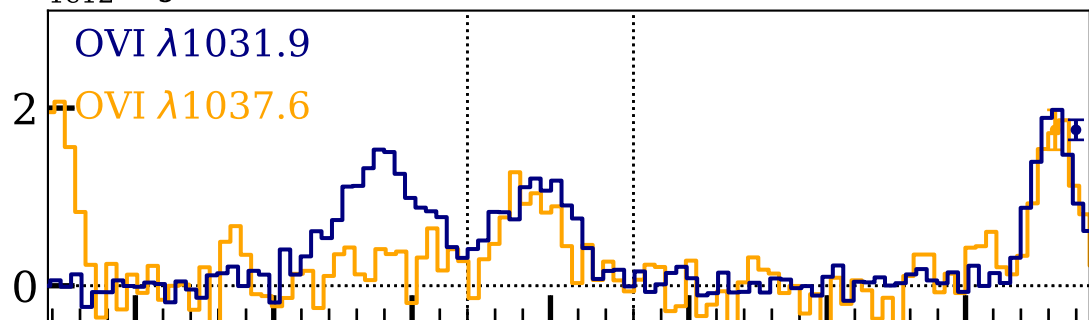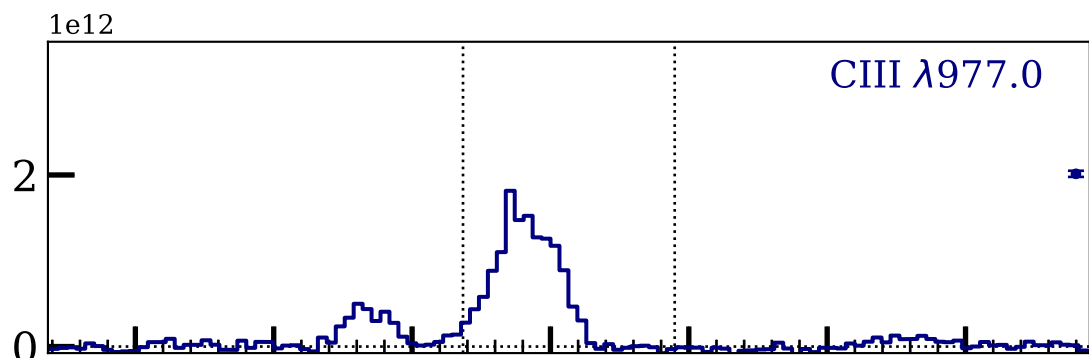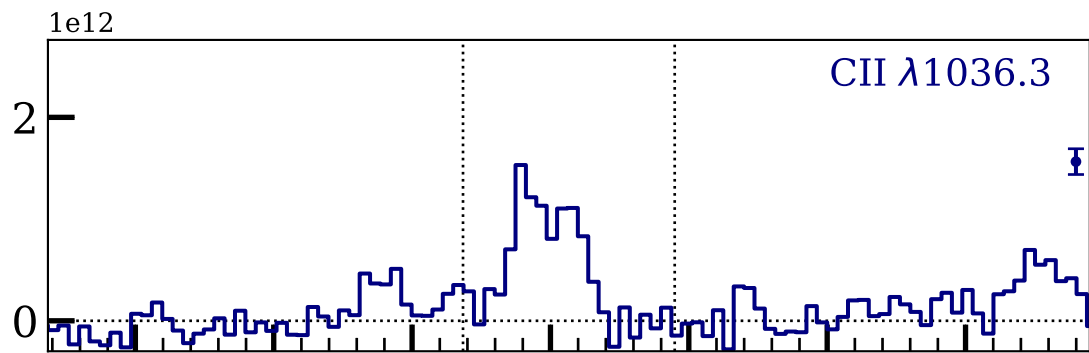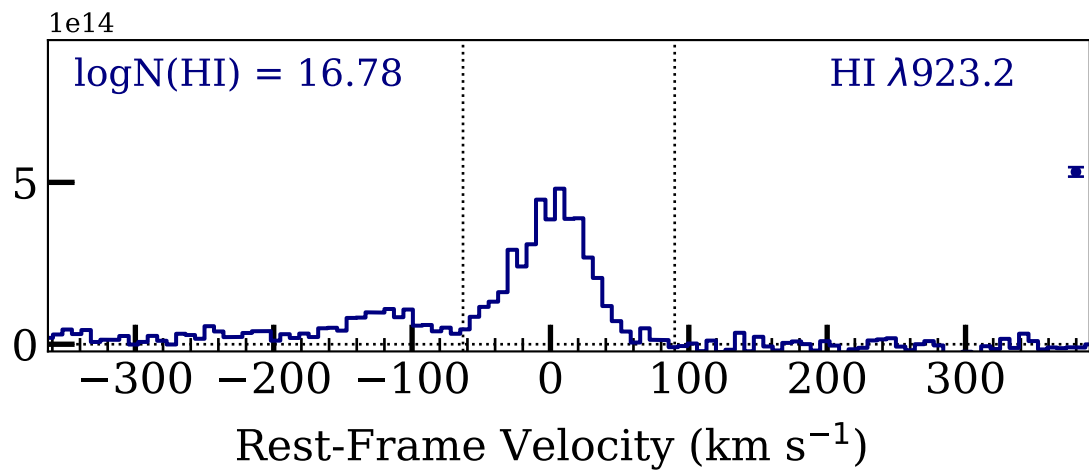

1e12 J122512.93+121835.7, z=0.324970, RF=1

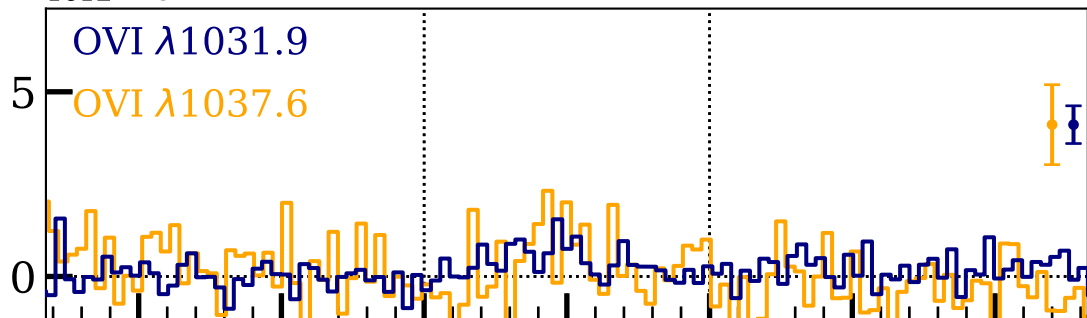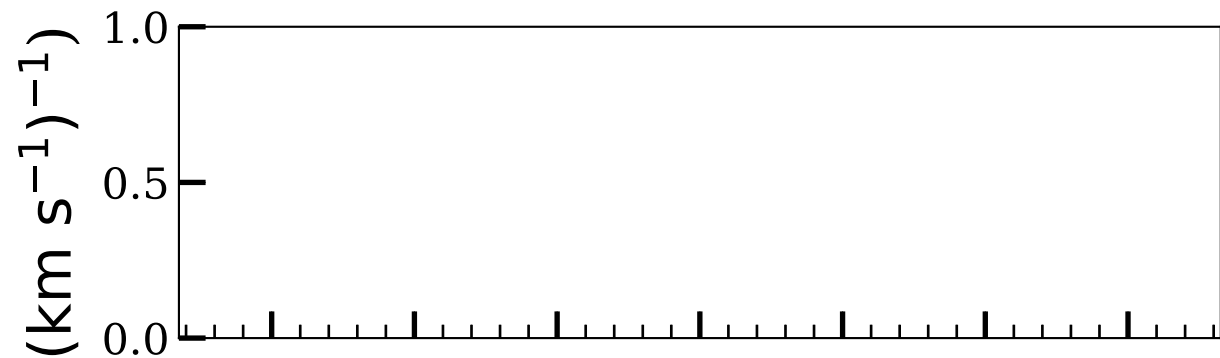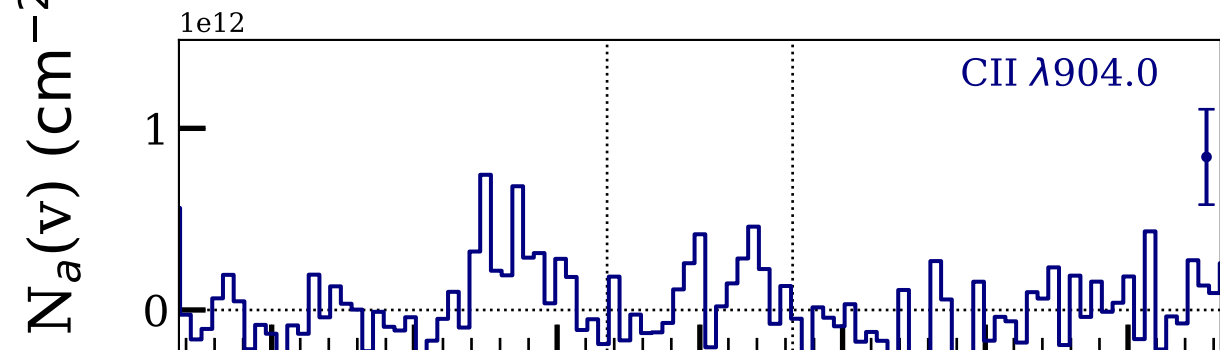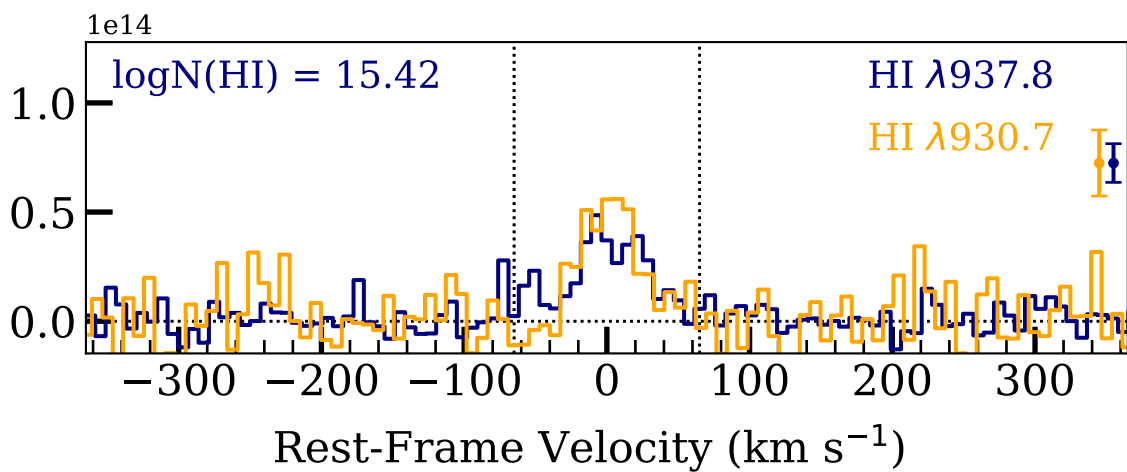



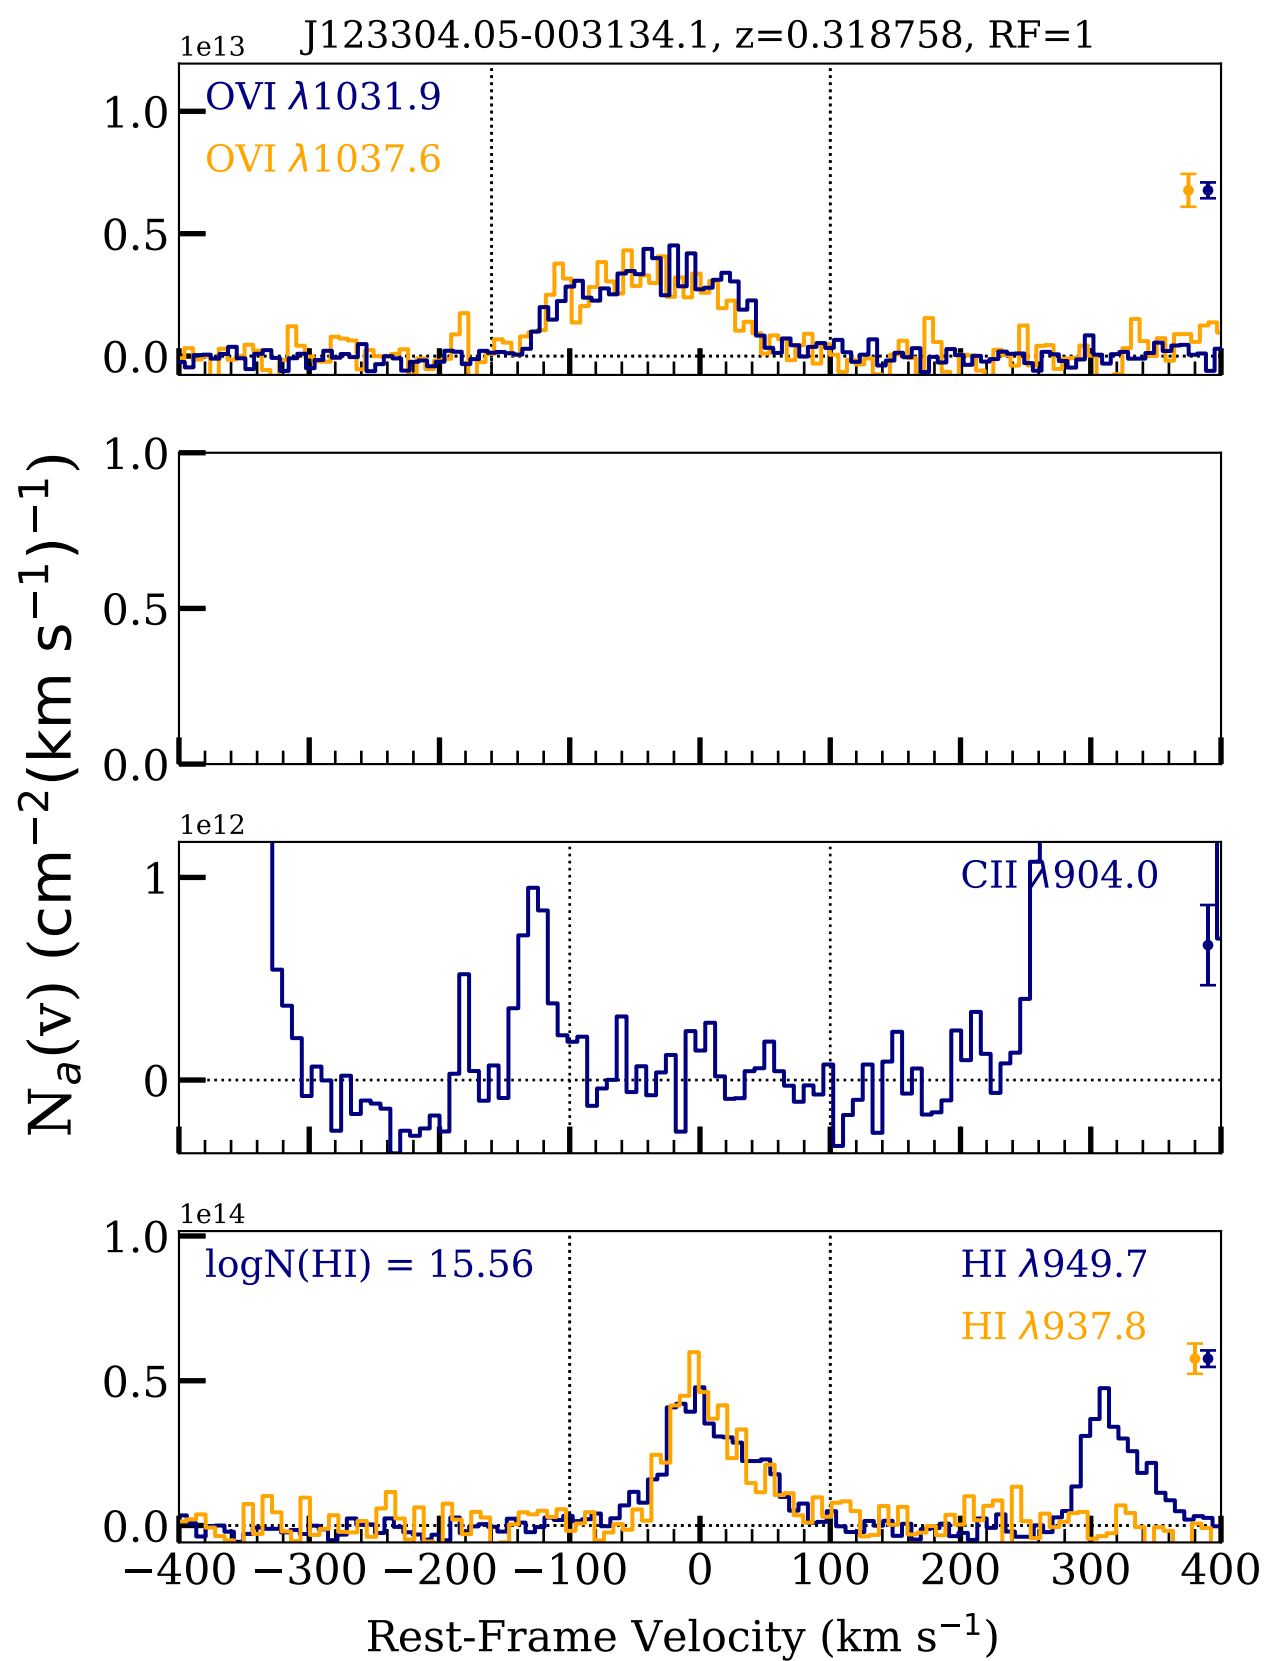

J123335.07+475800.4,  $z=0.284947$ , RF=1

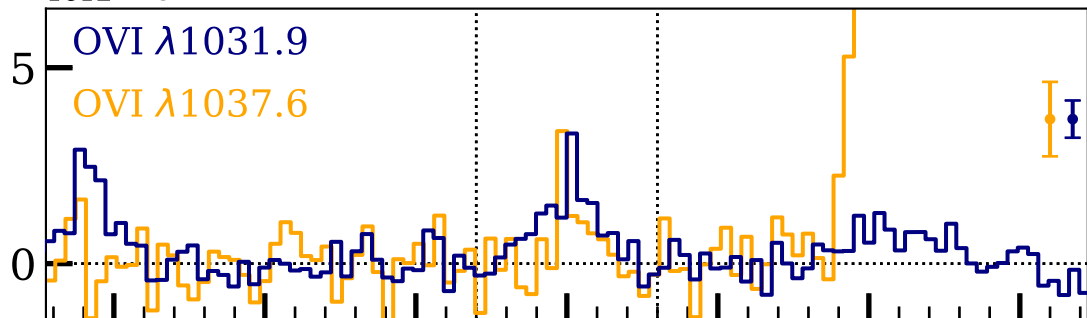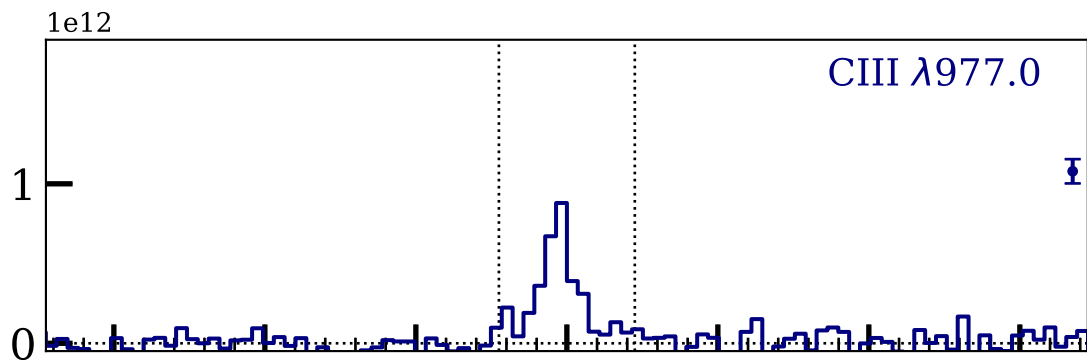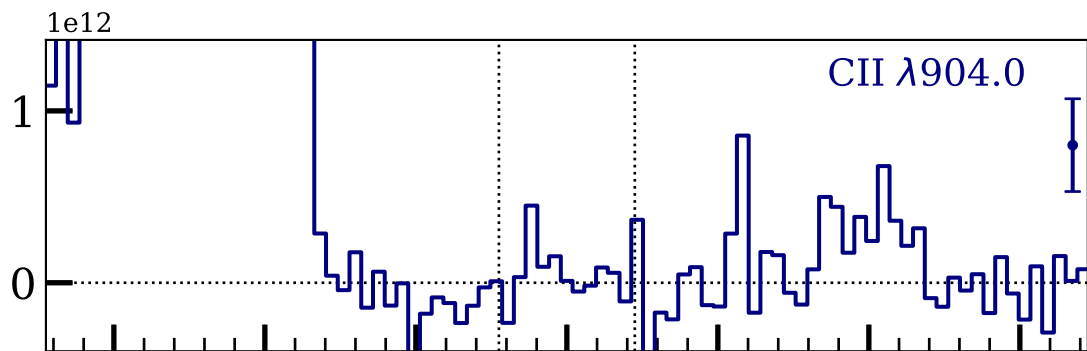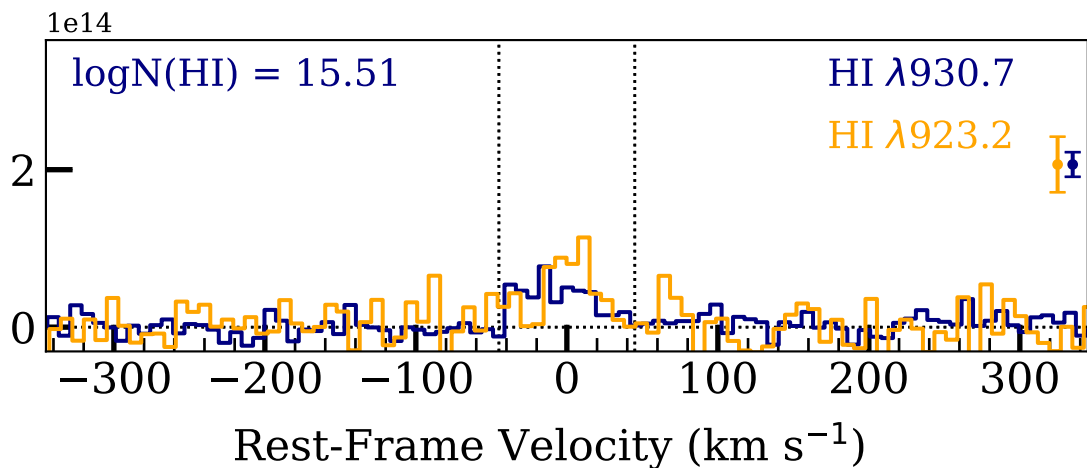

1e13 J124154.02+572107.3,  $z=0.217947$ , RF=1

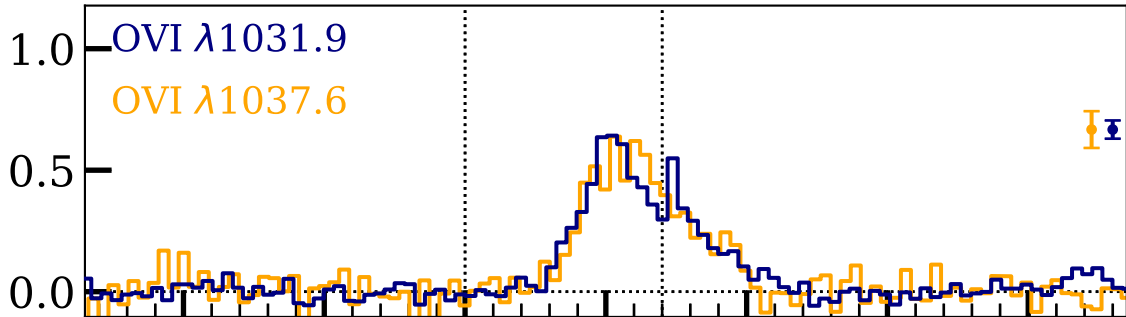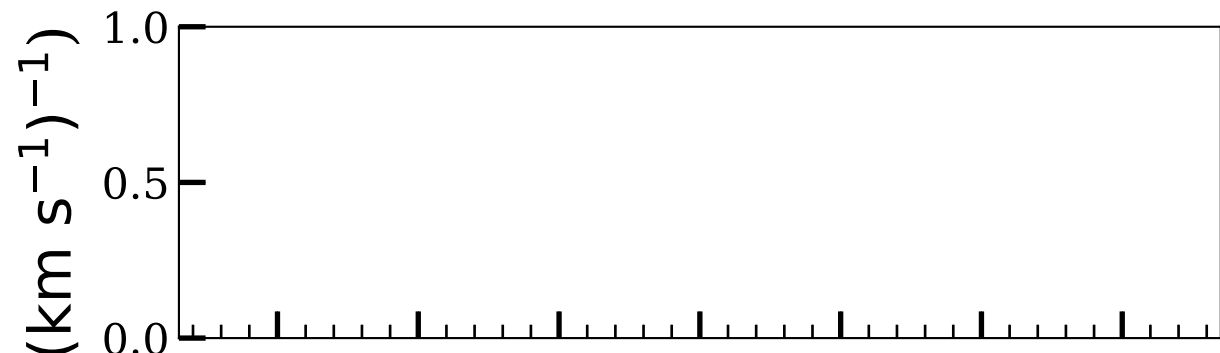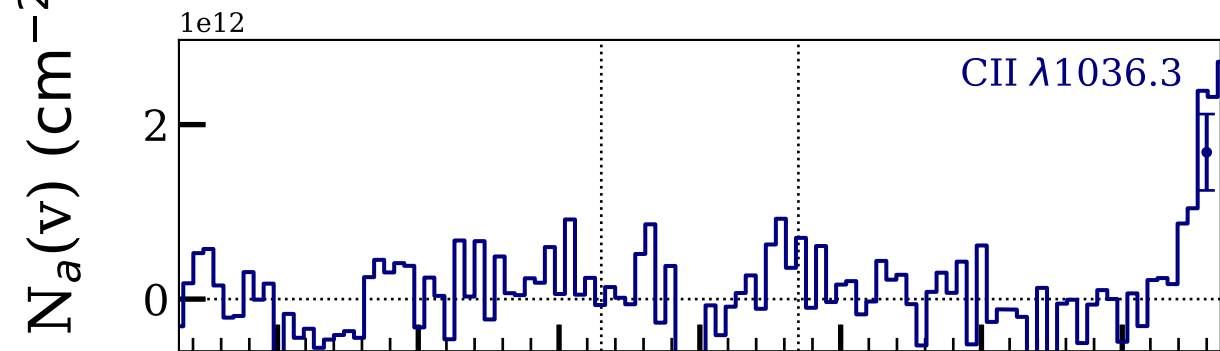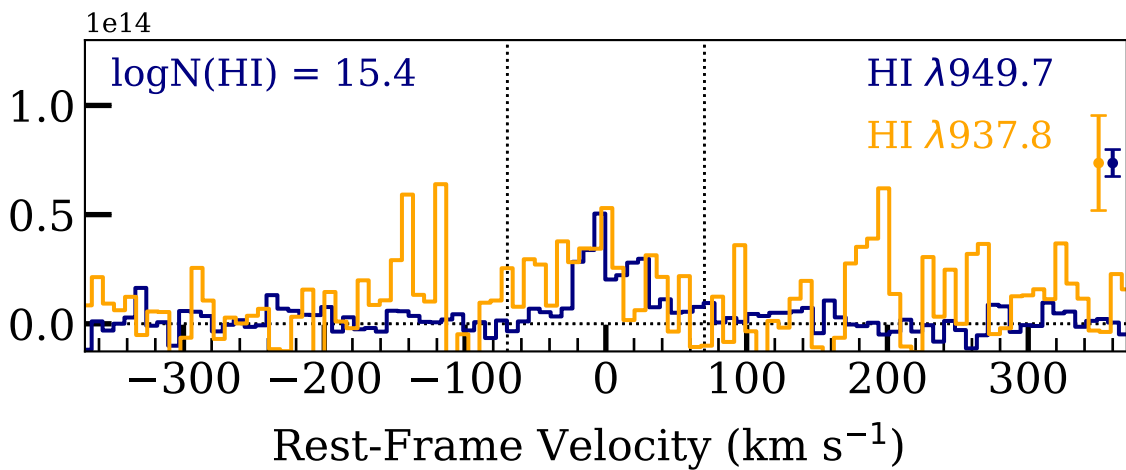

J124511.26+335610.1,  $z=0.556684$ , RF=0

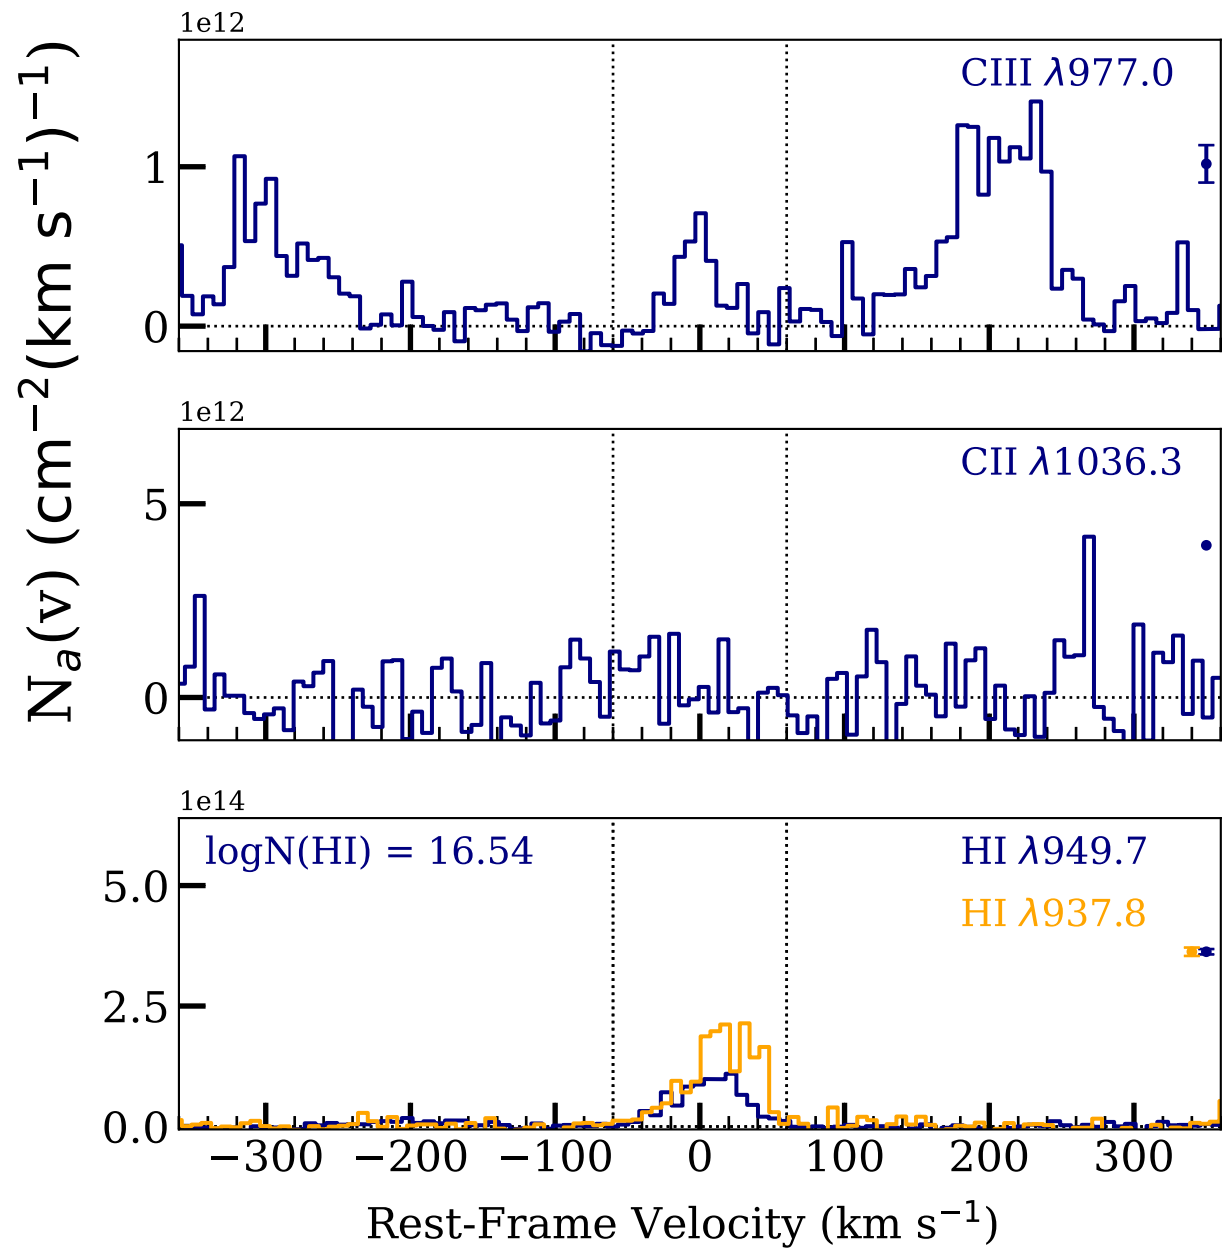

J124511.26+335610.1,  $z=0.587563$ , RF=1

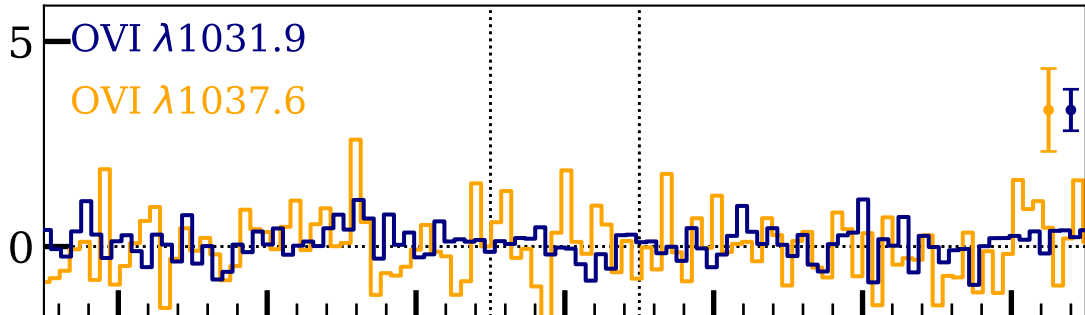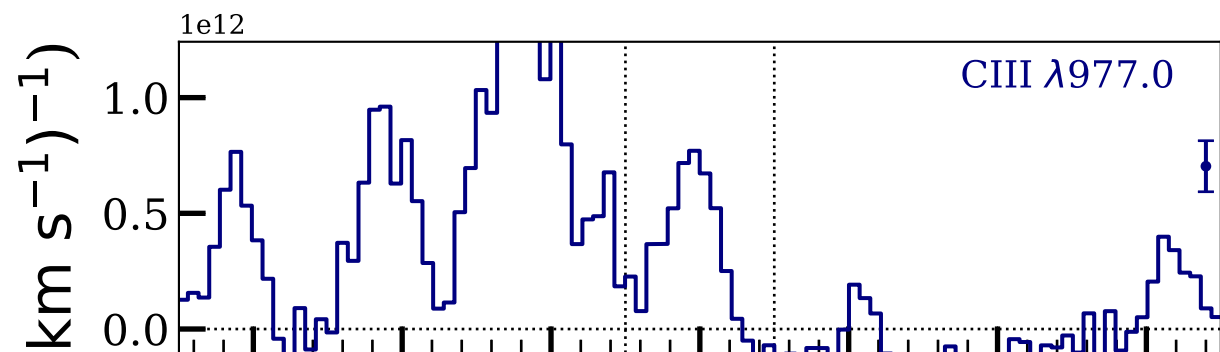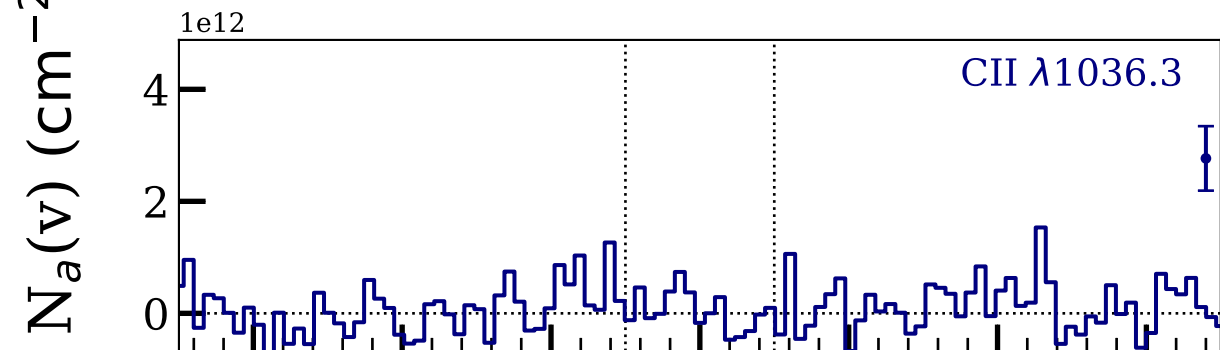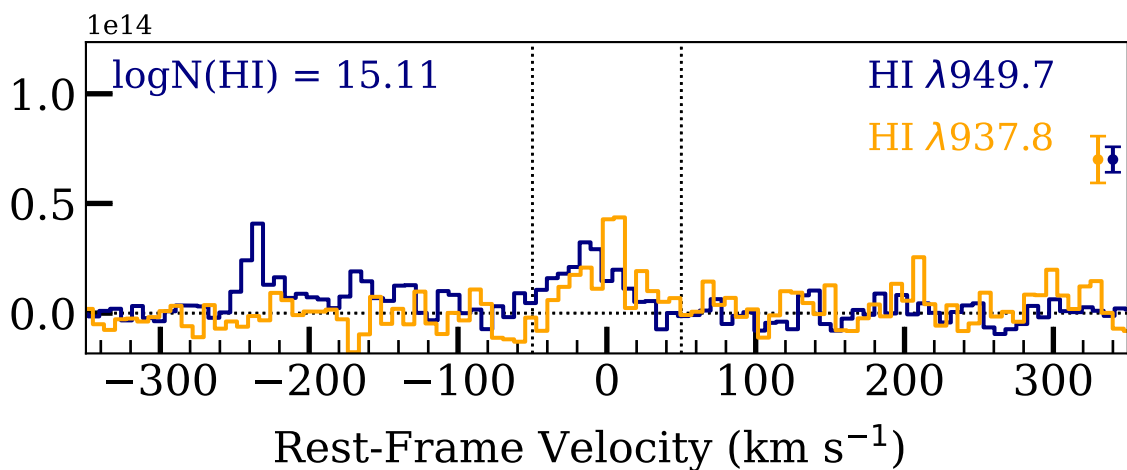

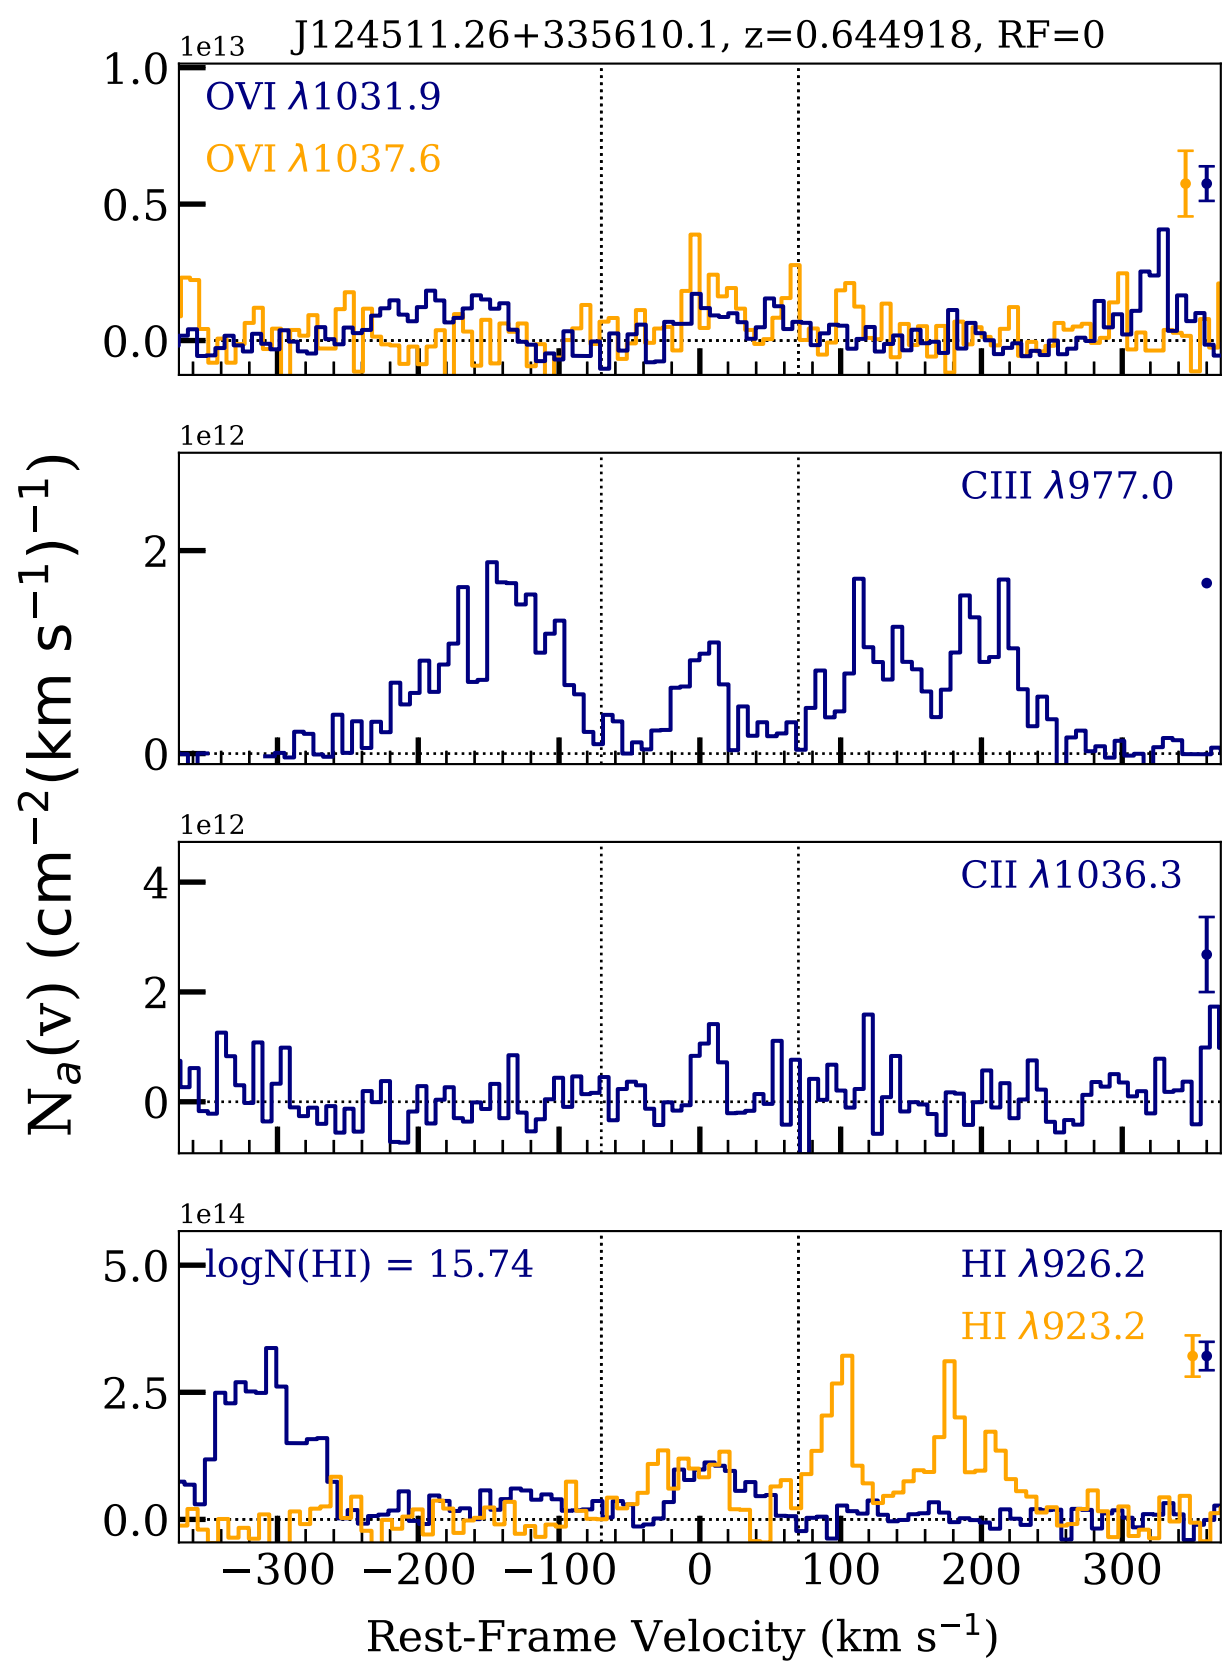

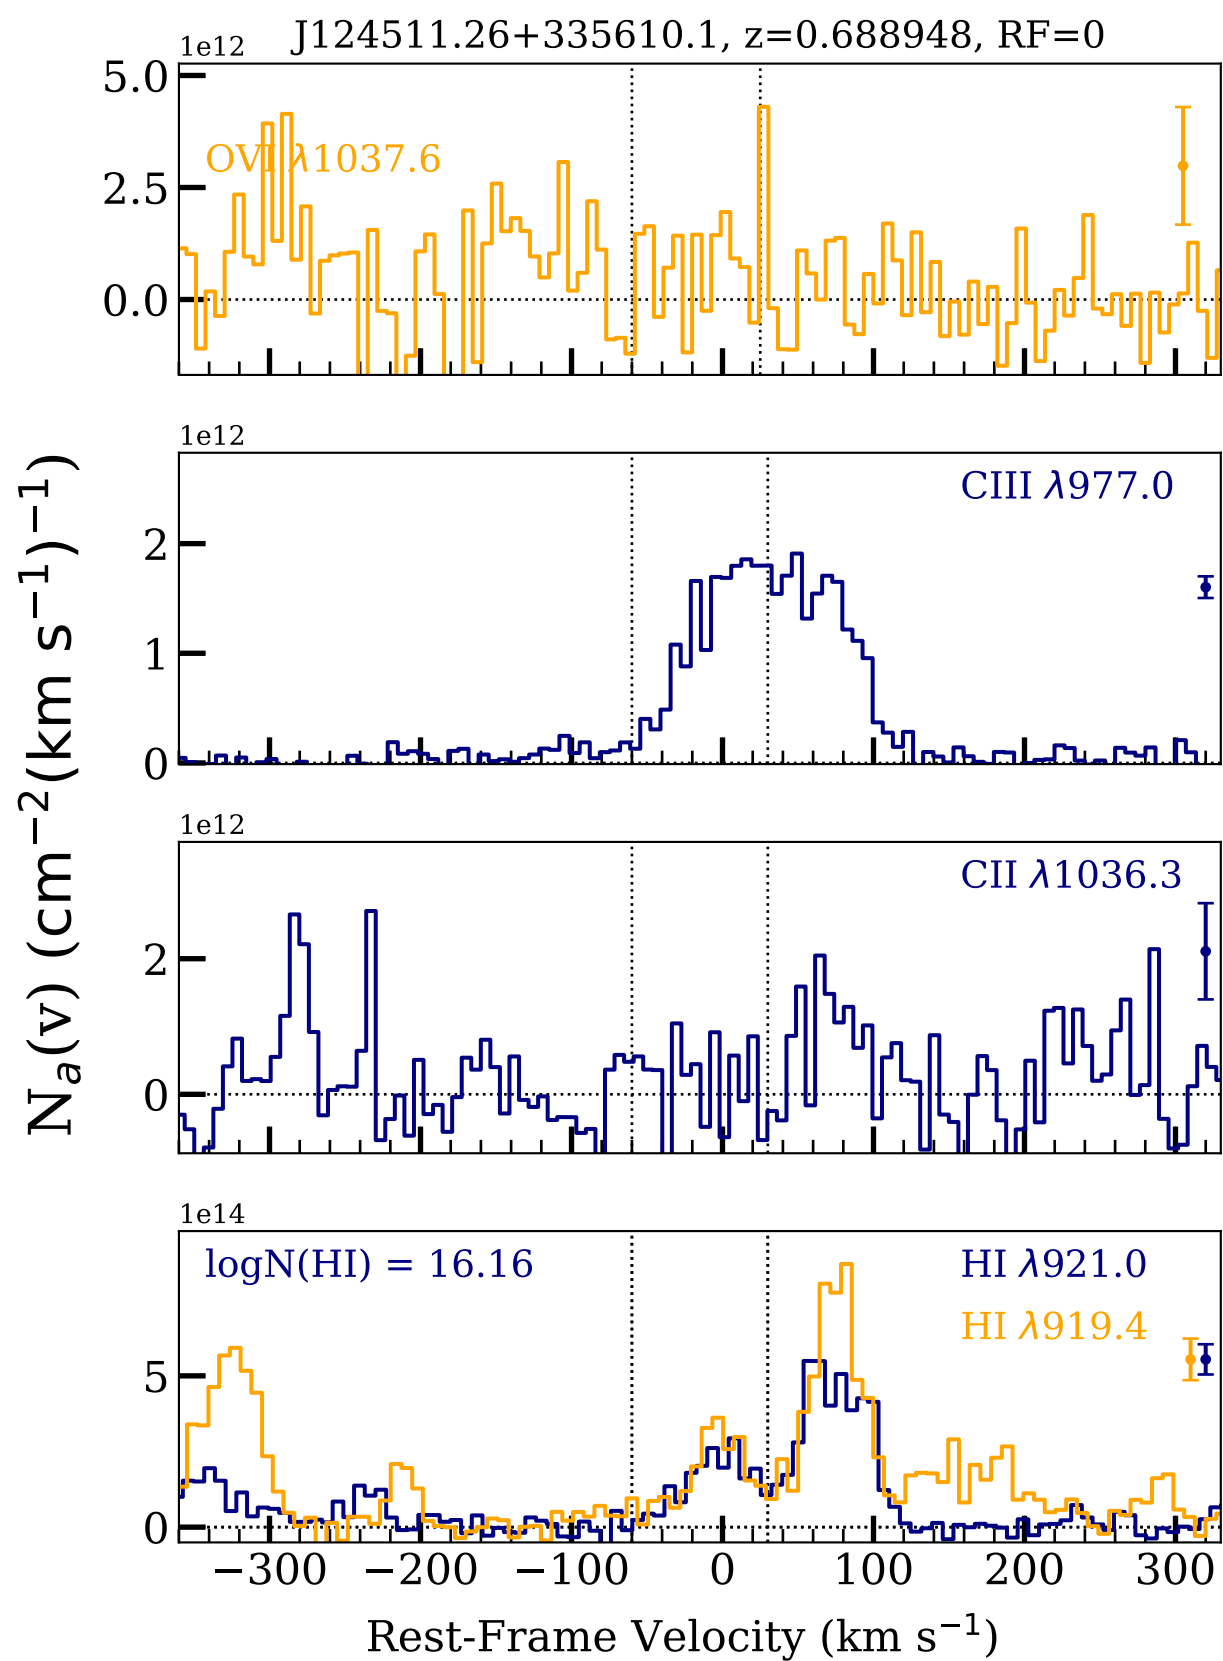

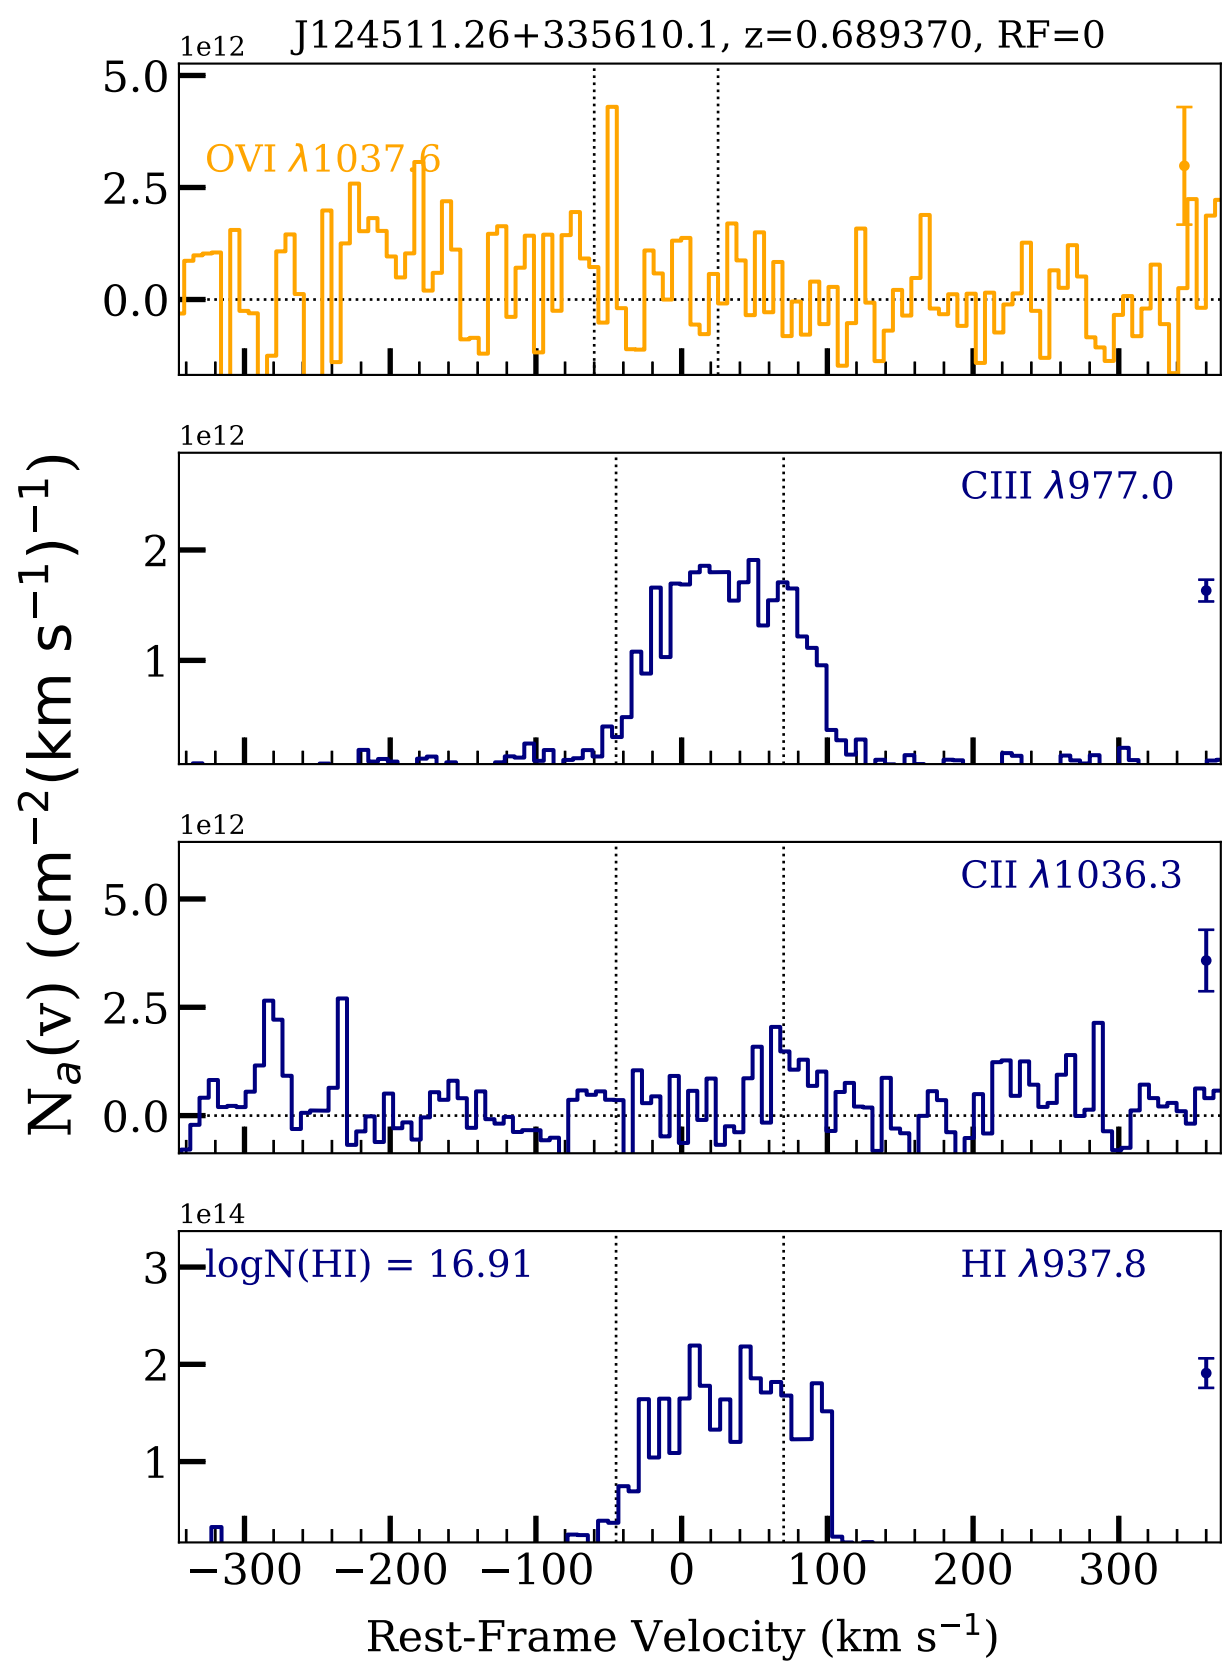



1e13 J124511.26+335610.1,  $z=0.712976$ , RF=0

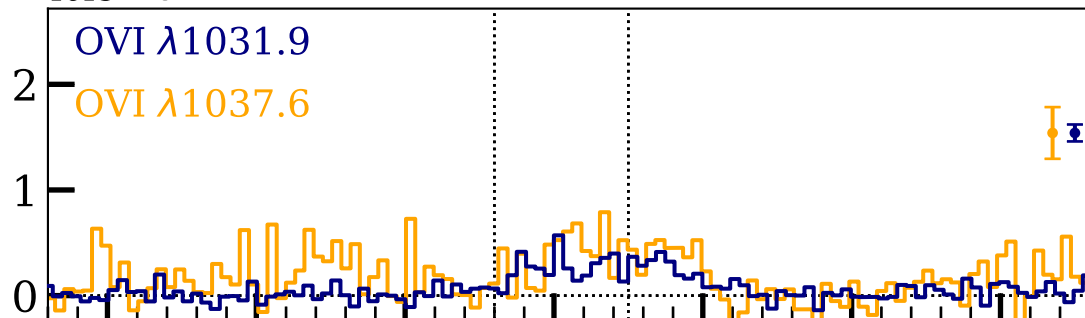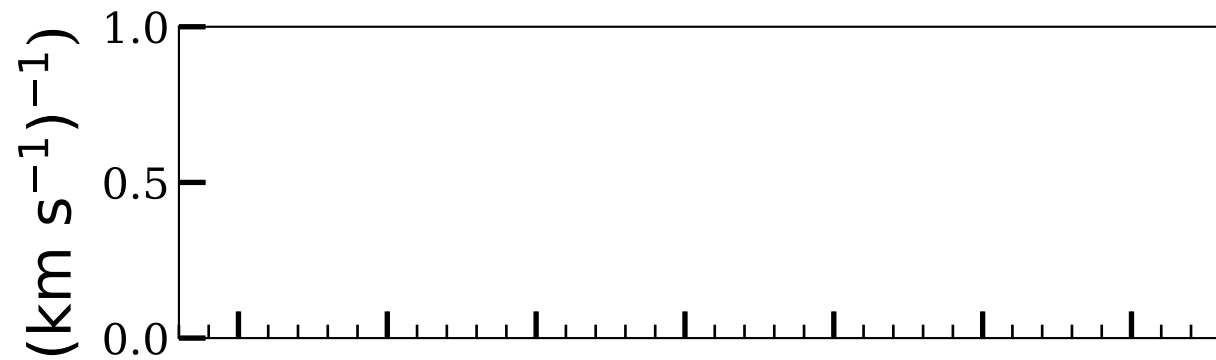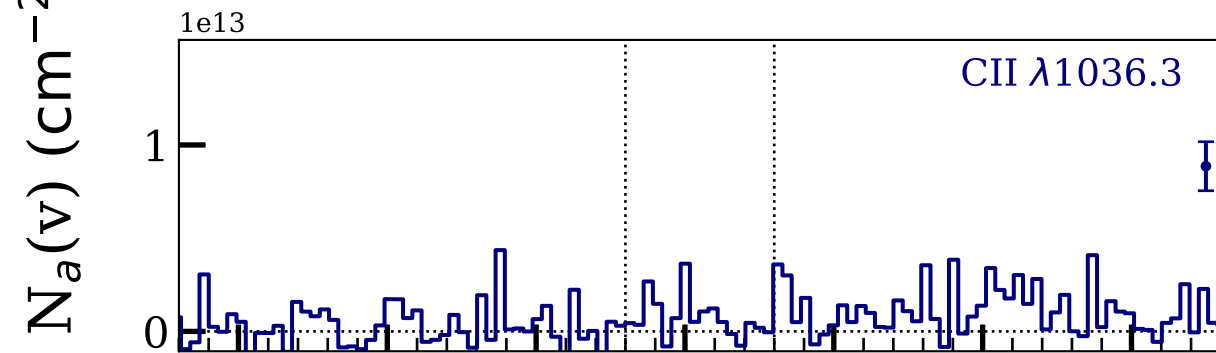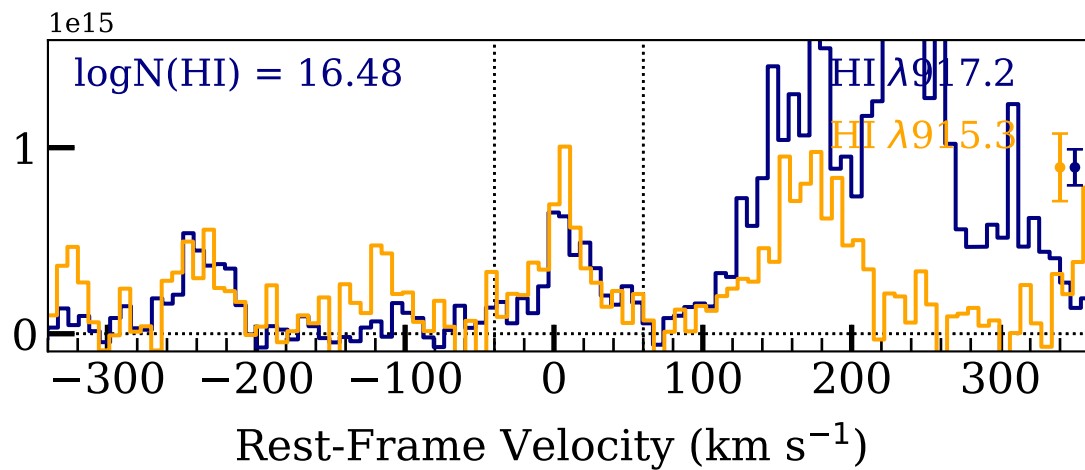

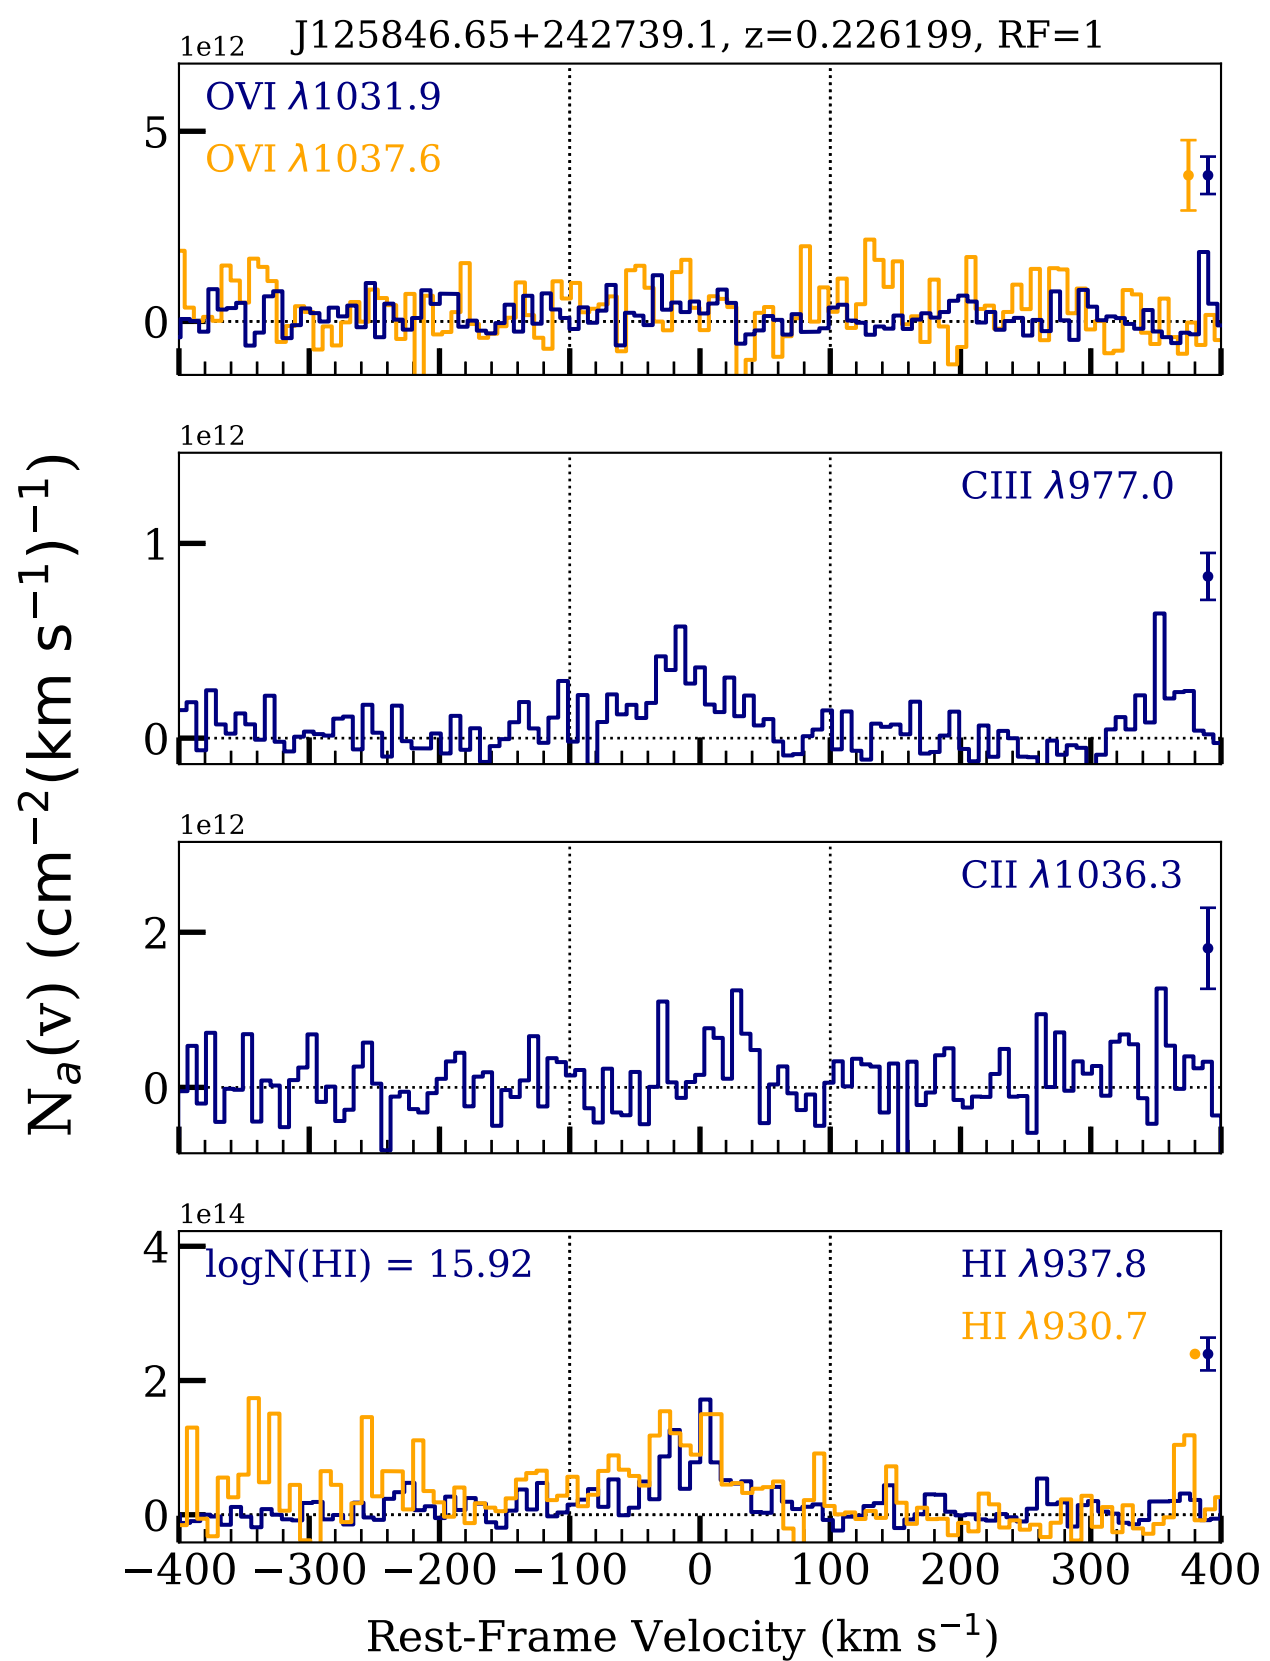

J130429.02+311308.2,  $z=0.309948$ , RF=1

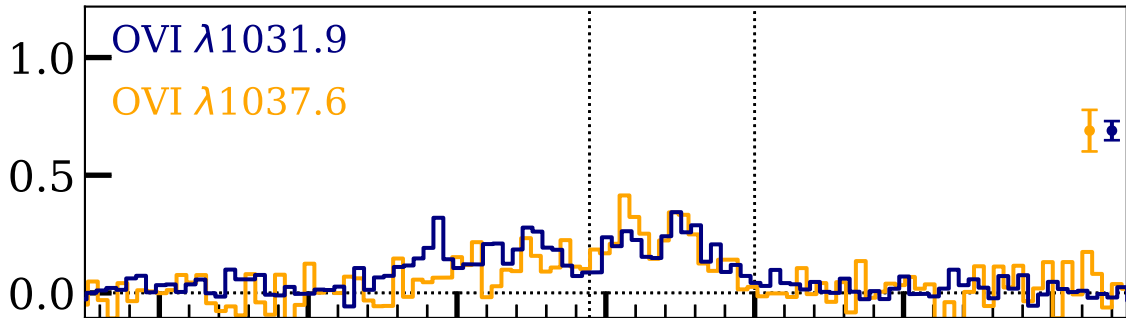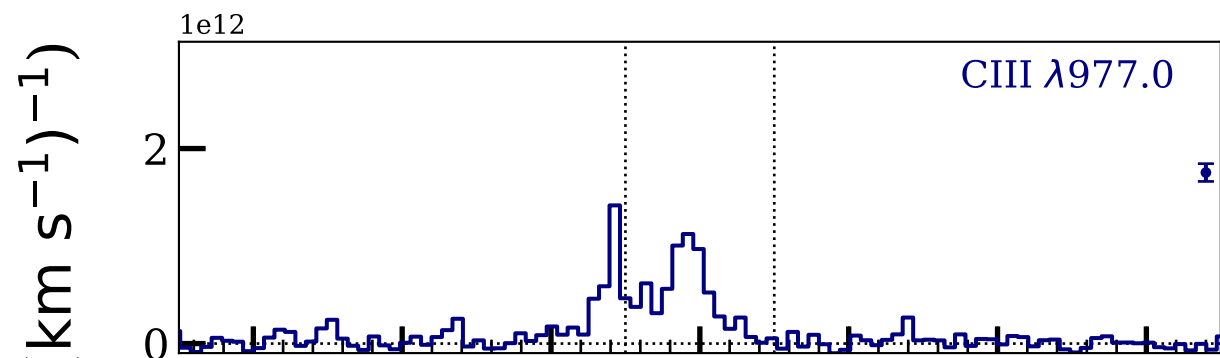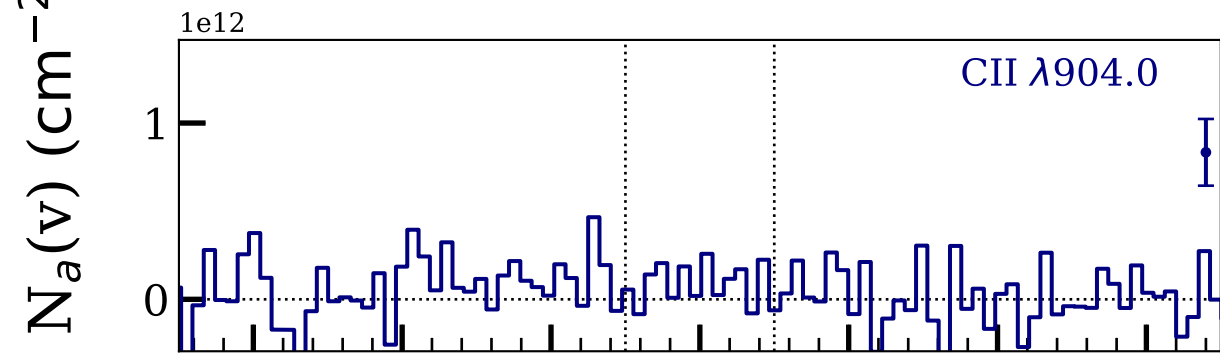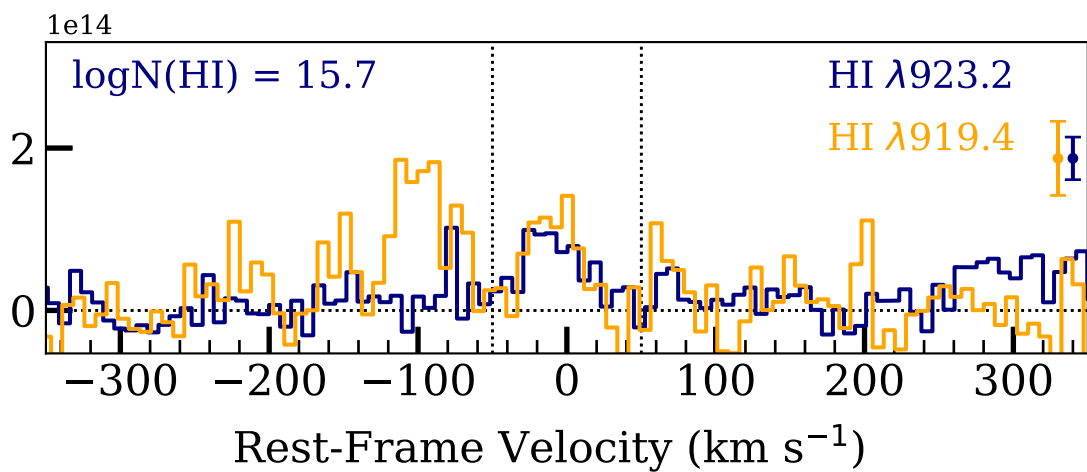

J130451.40+245445.9,  $z=0.276315$ , RF=1

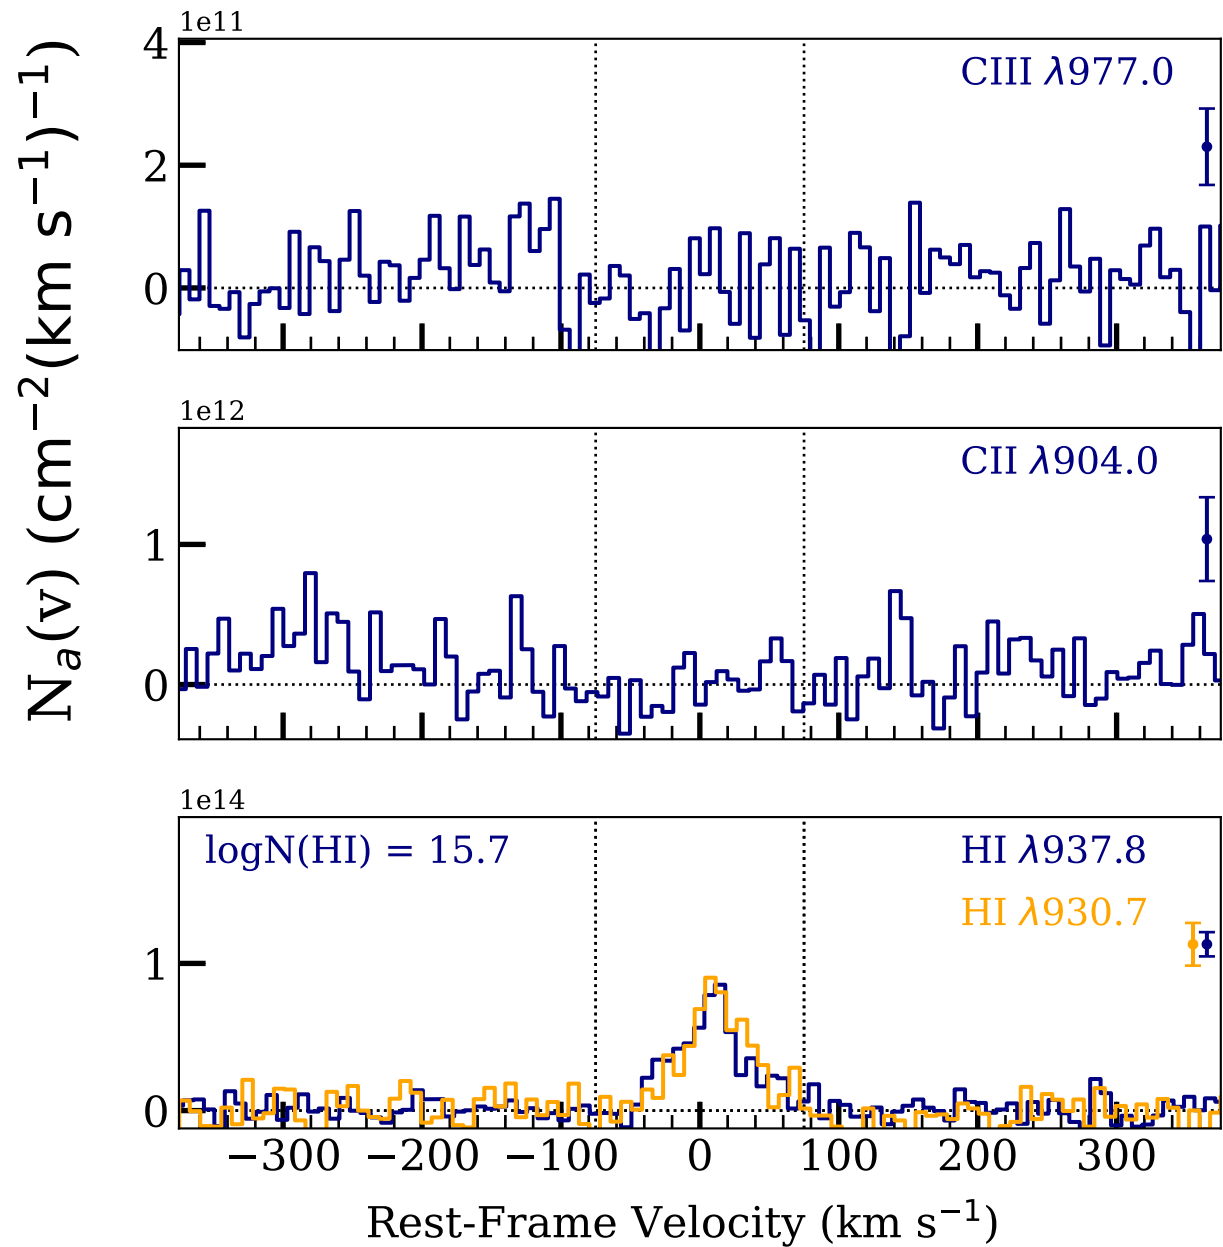

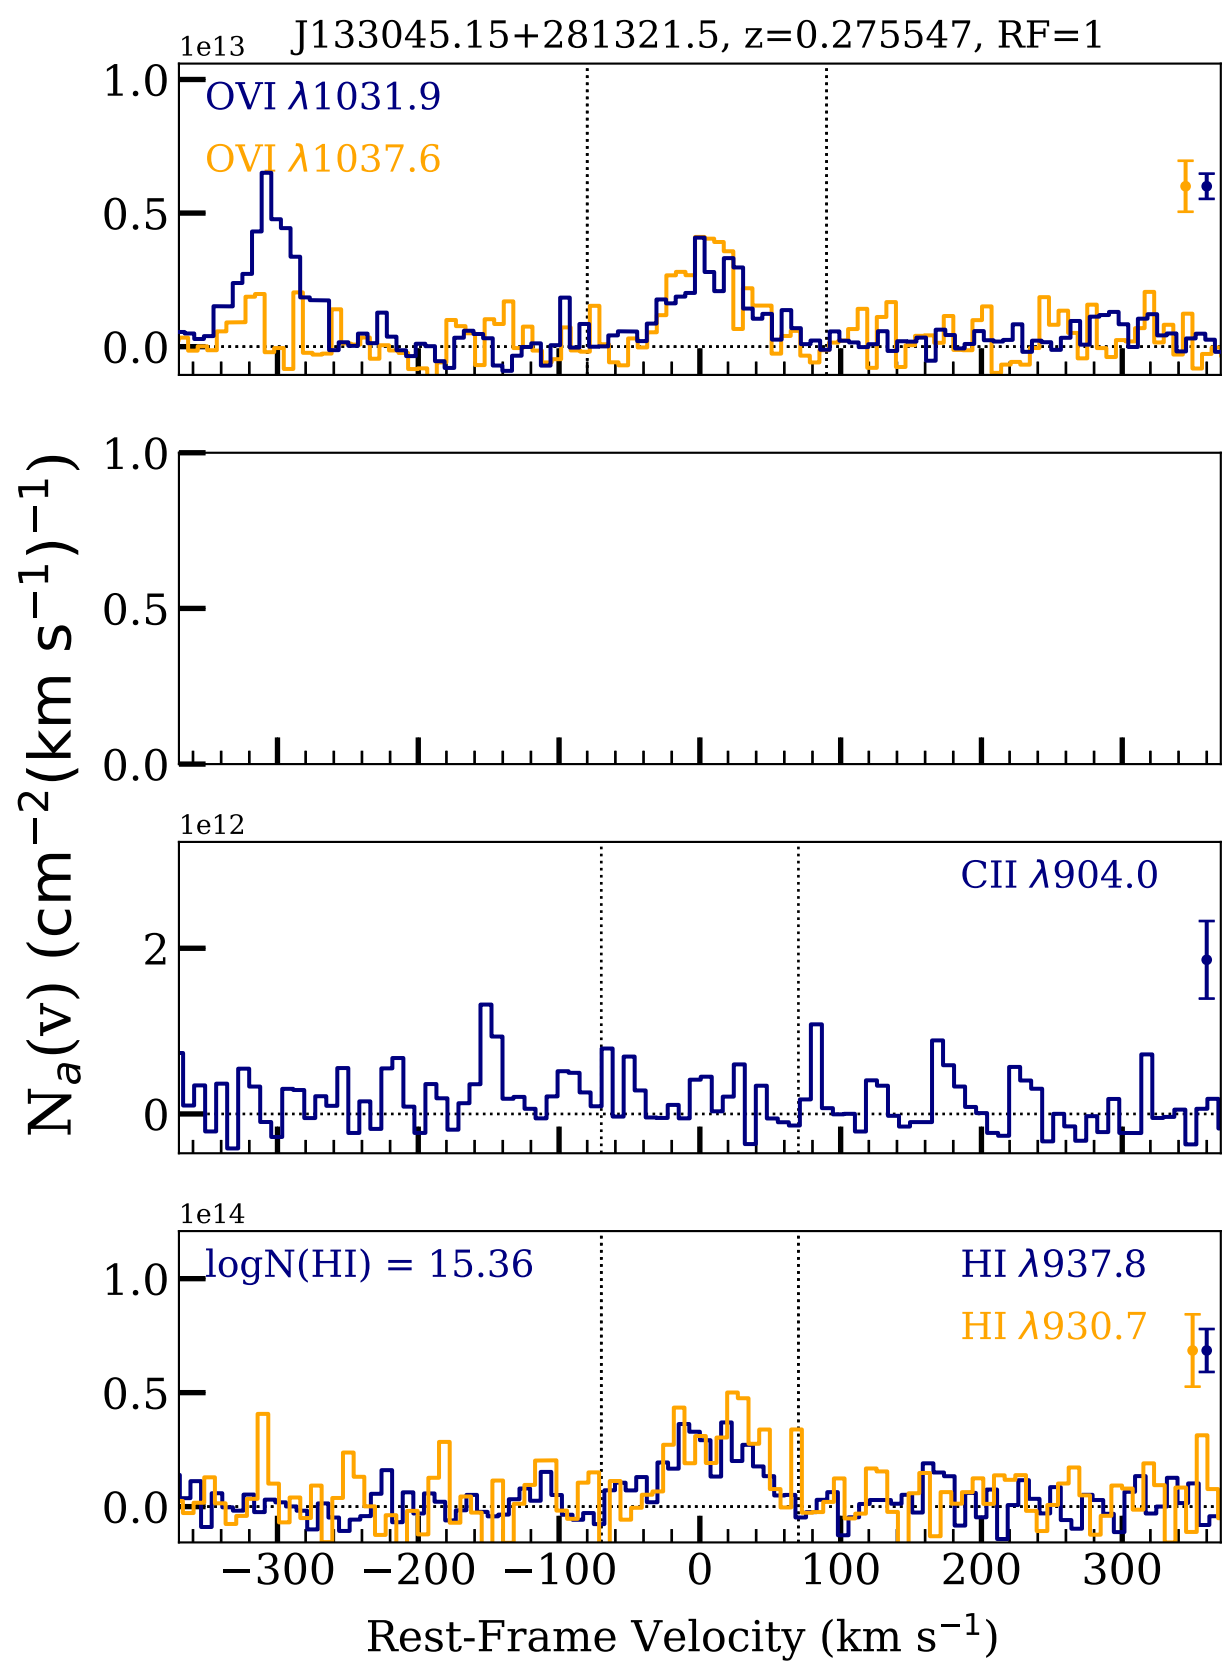

J134100.78+412314.0,  $z=0.348827$ , RF=1

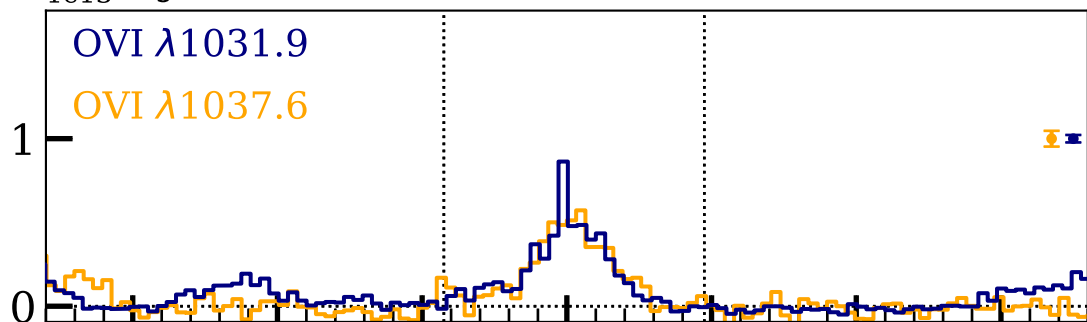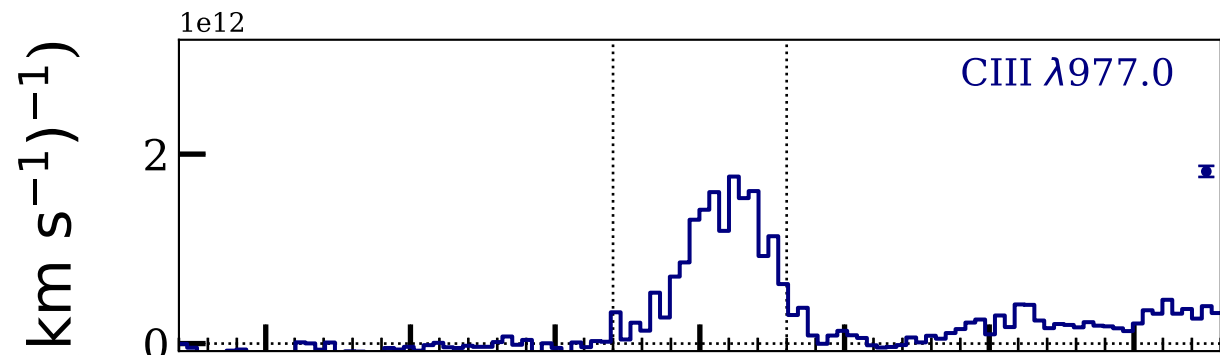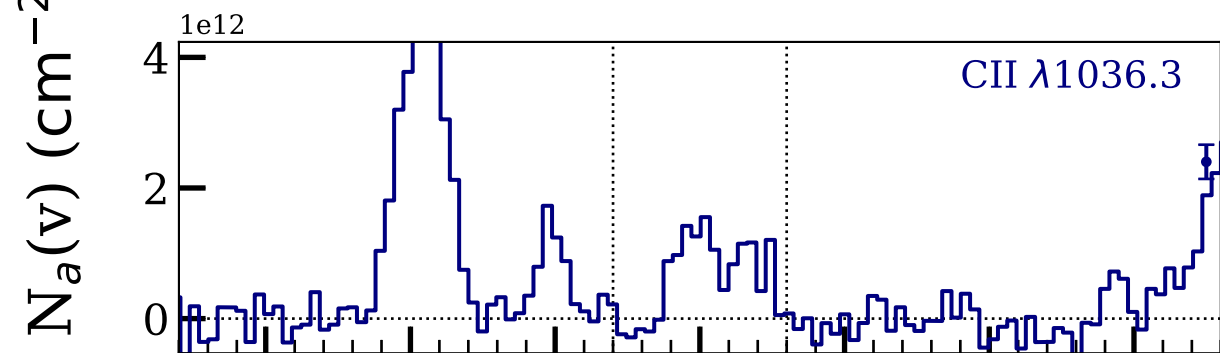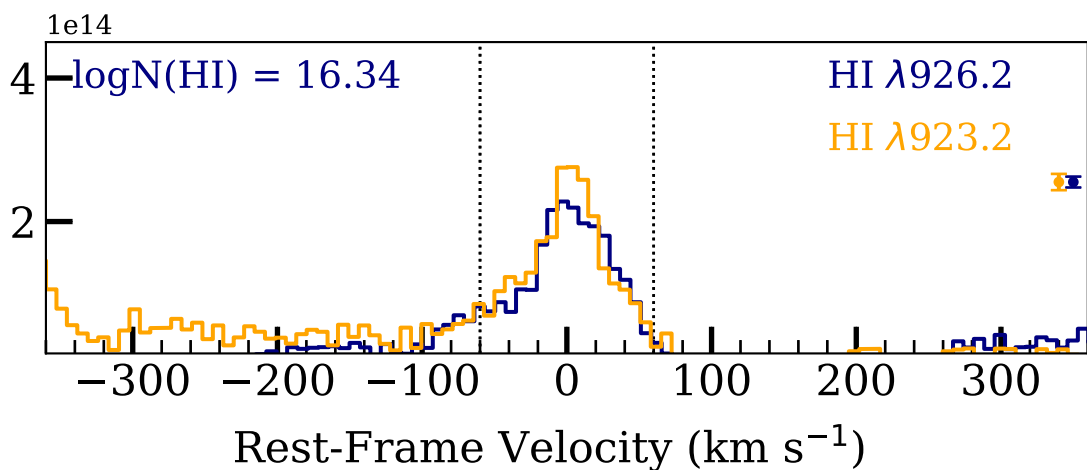

J134100.78+412314.0,  $z=0.620752$ , RF=1

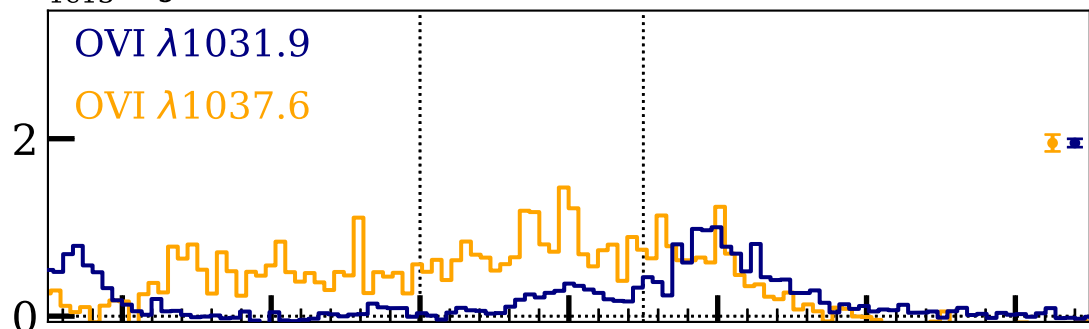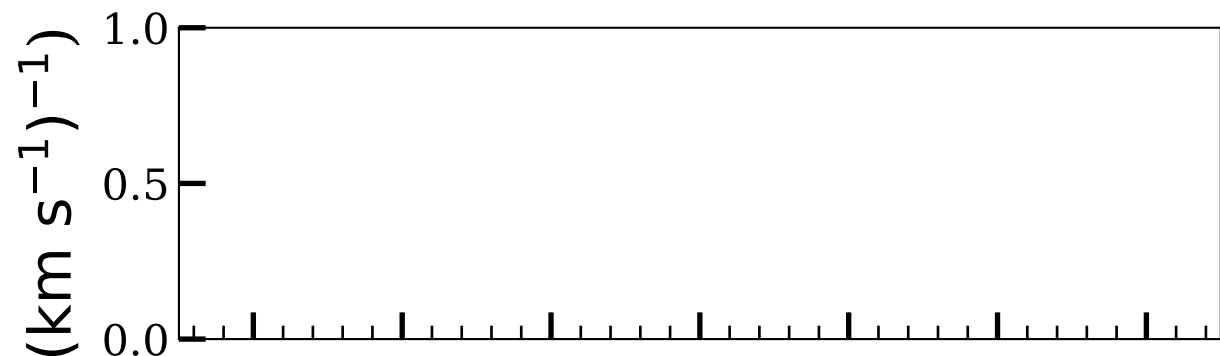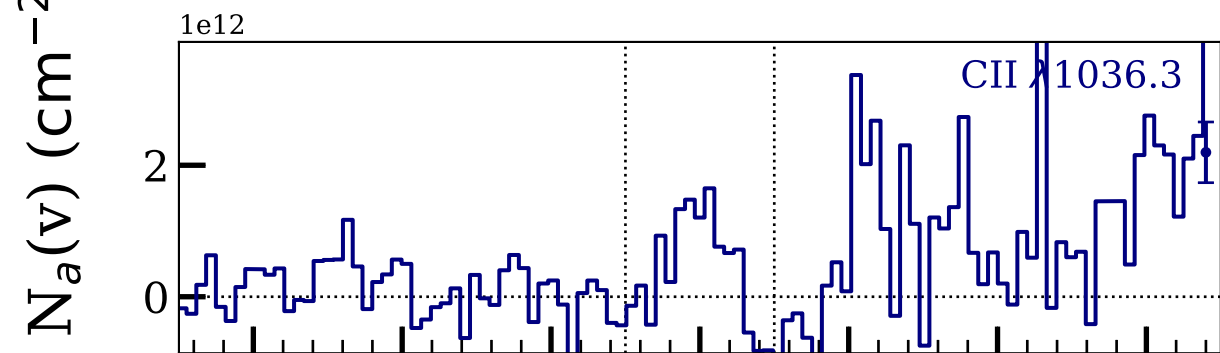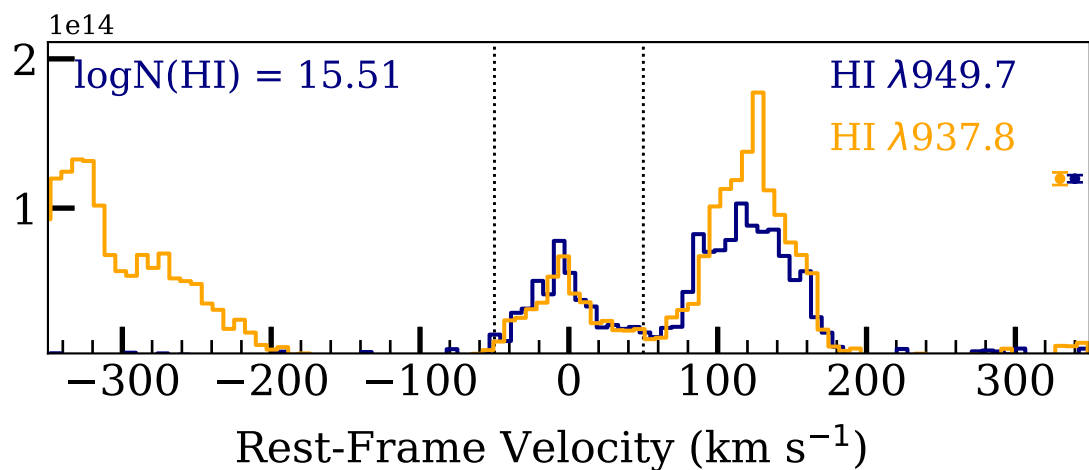

J134100.78+412314.0,  $z=0.621428$ , RF=1

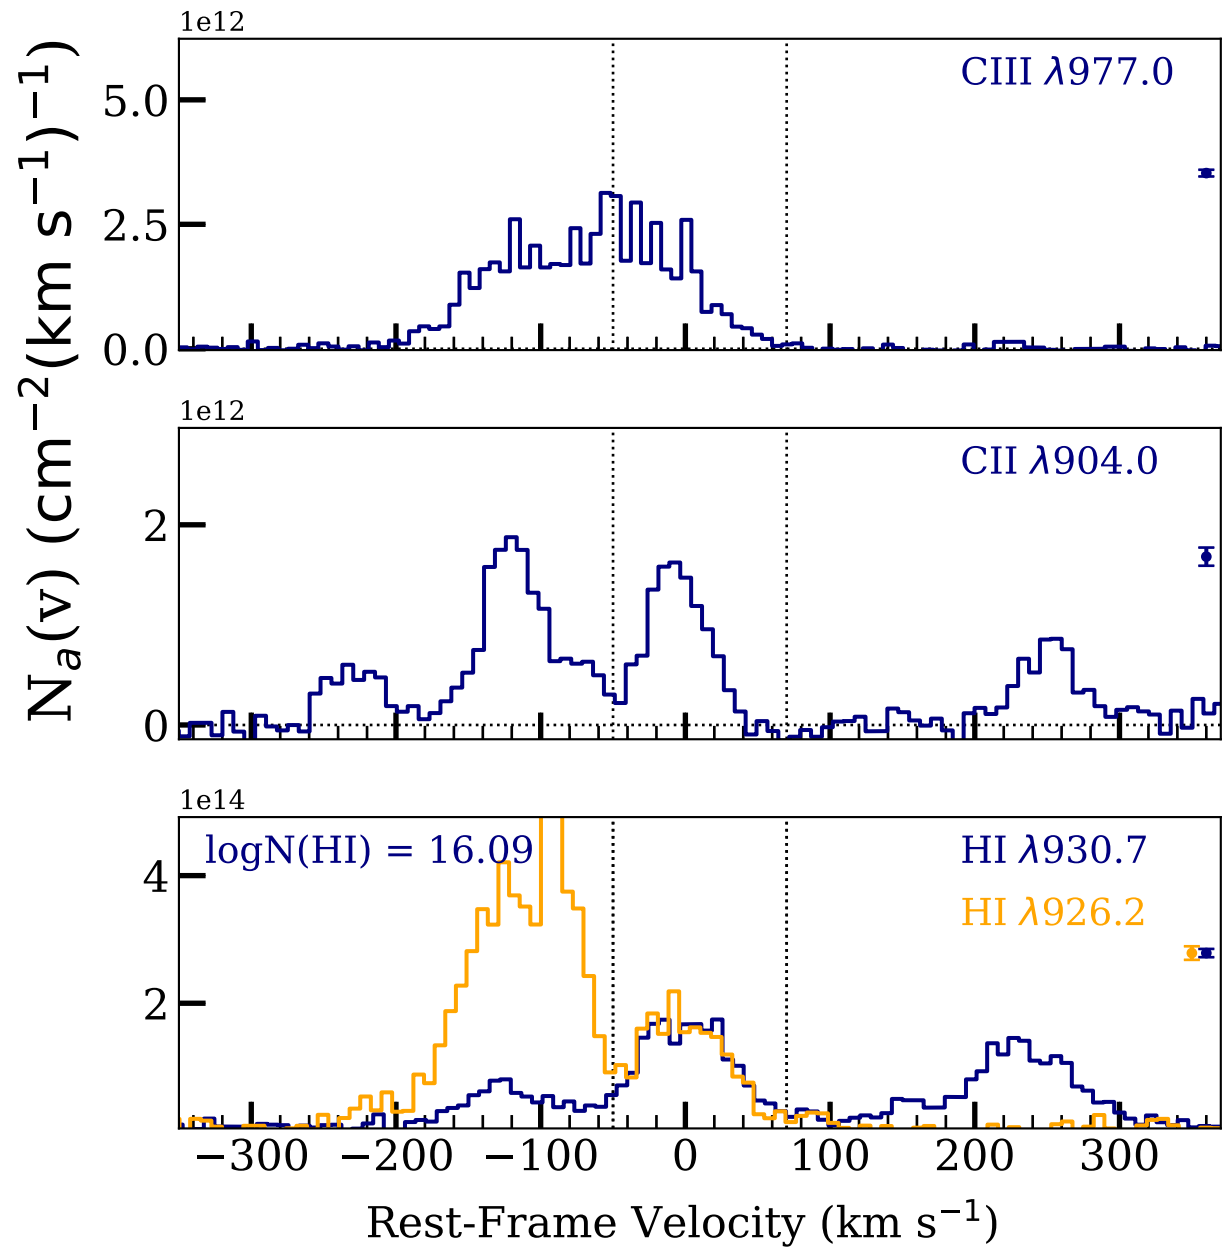



J134100.78+412314.0,  $z=0.686086$ , RF=1

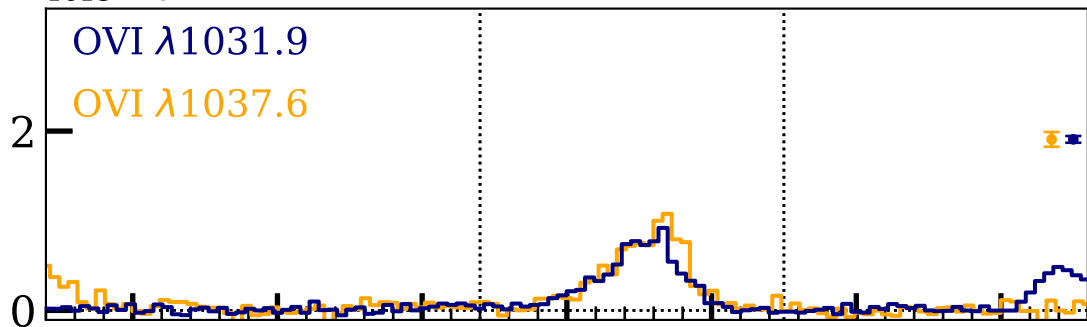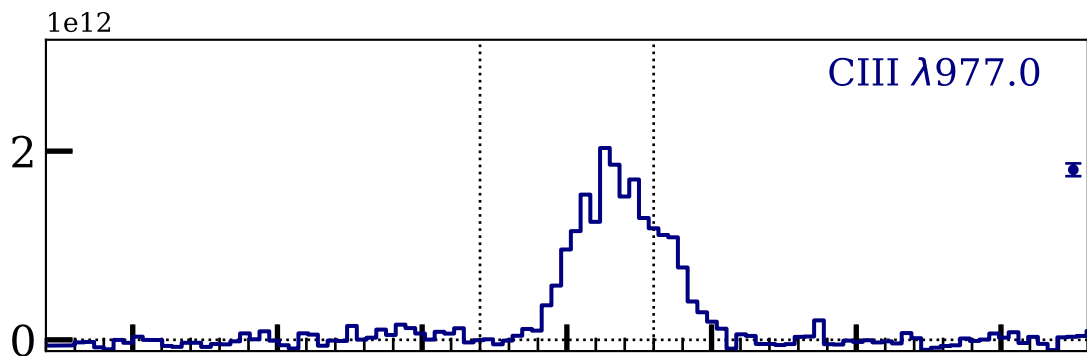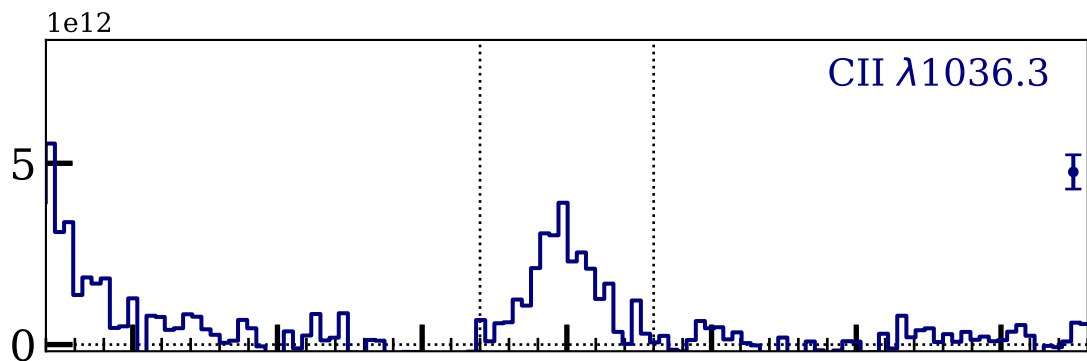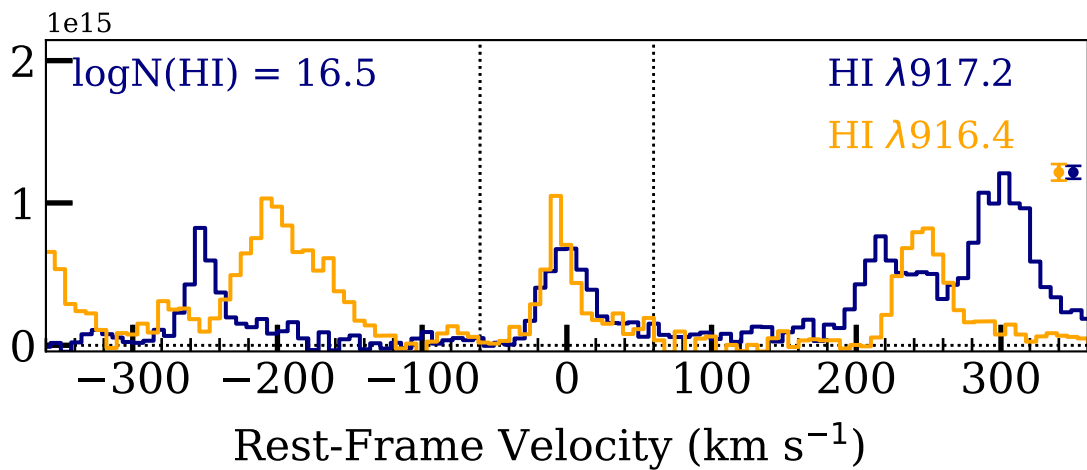

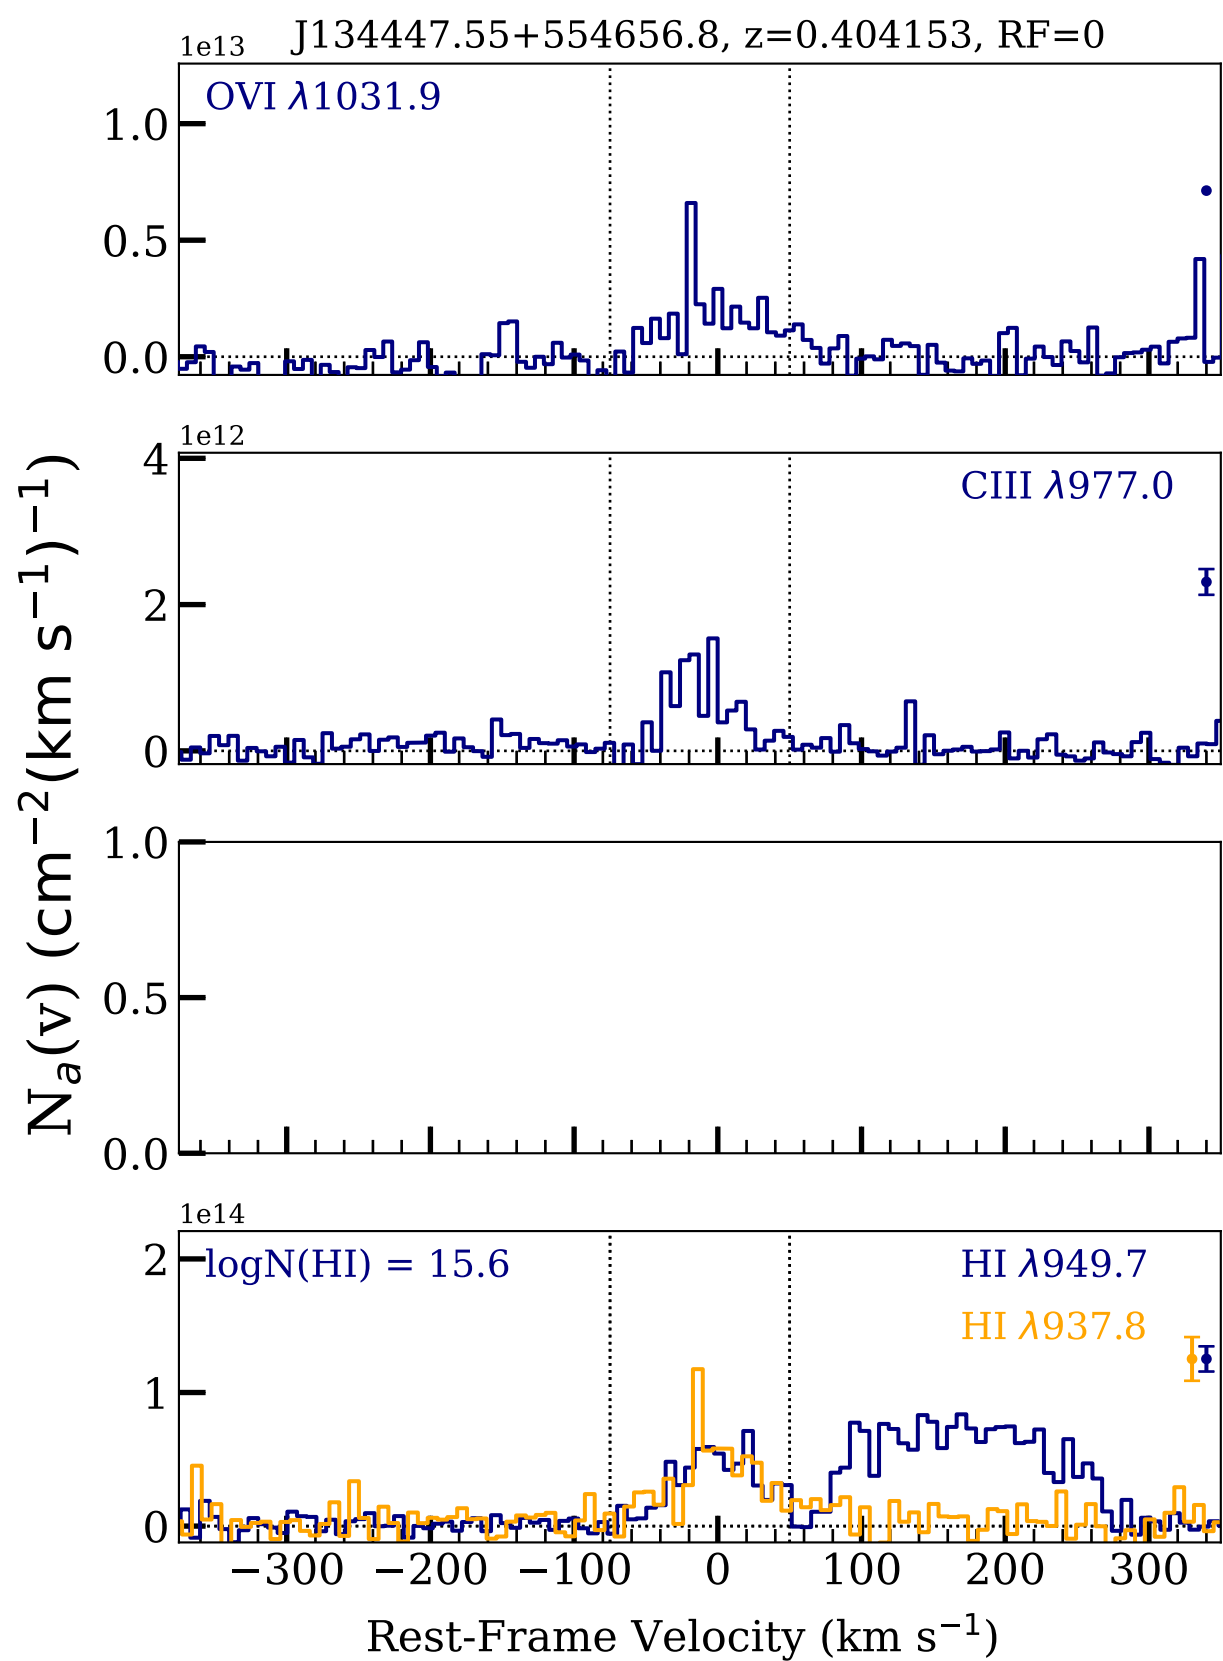

J135726.26+043541.3,  $z=0.610248$ , RF=1

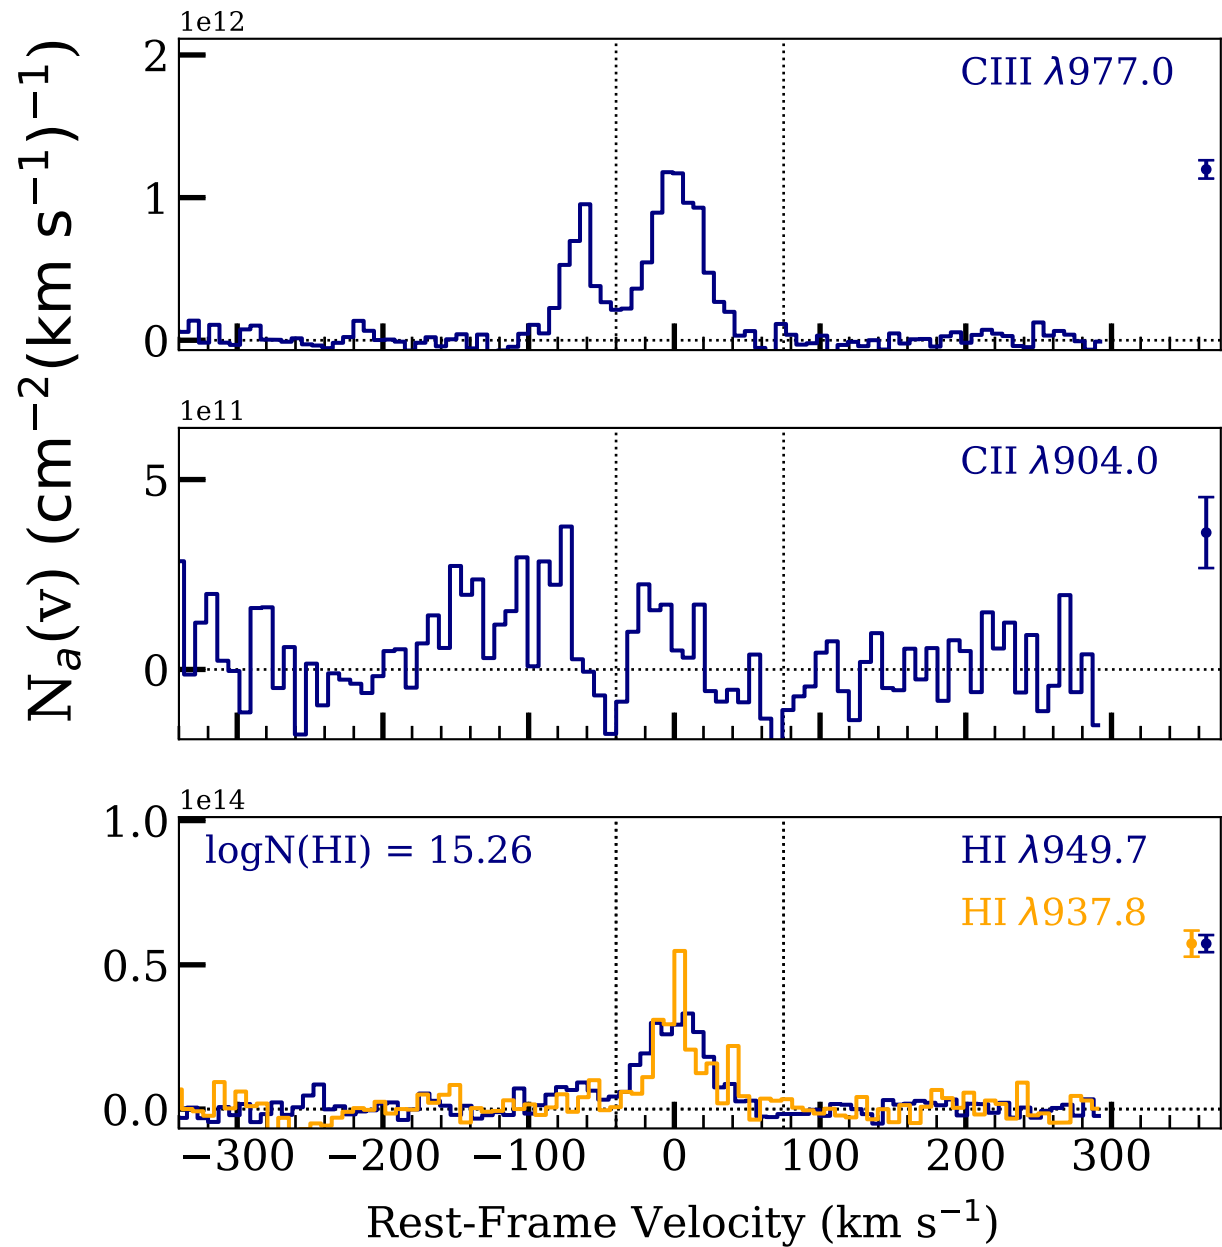

1e12 J140732.25+550725.4, z=0.243328, RF=1

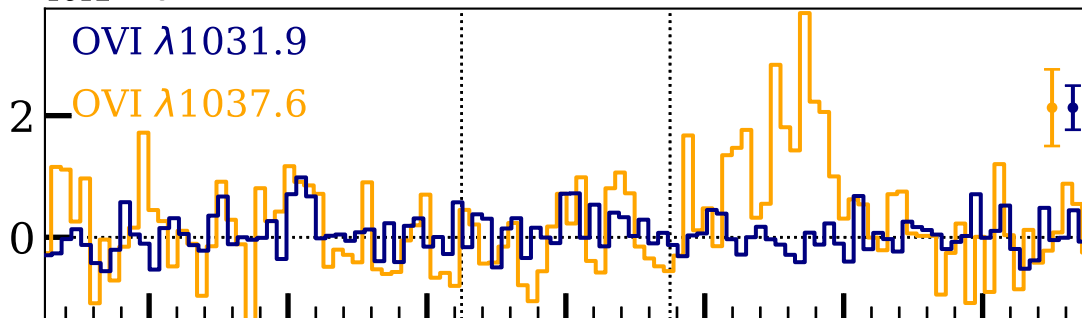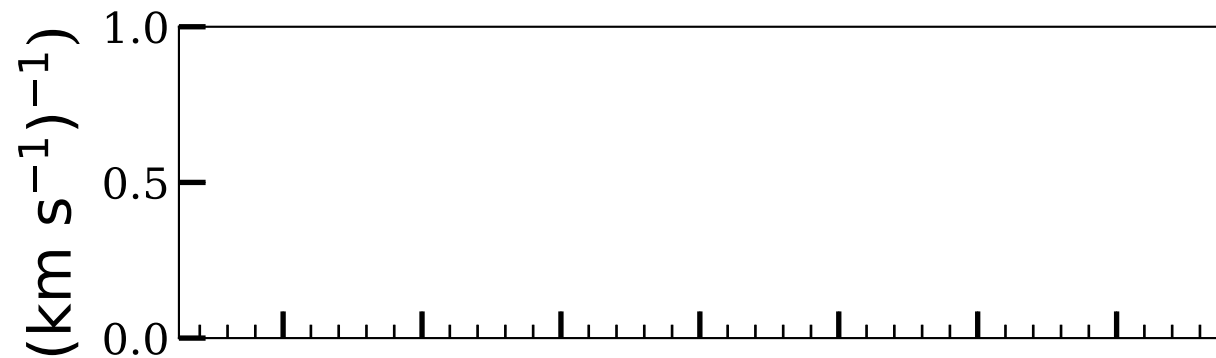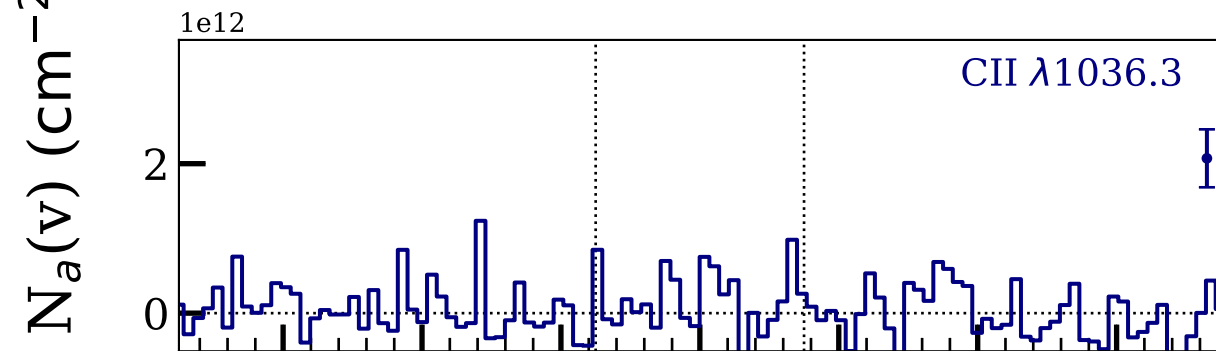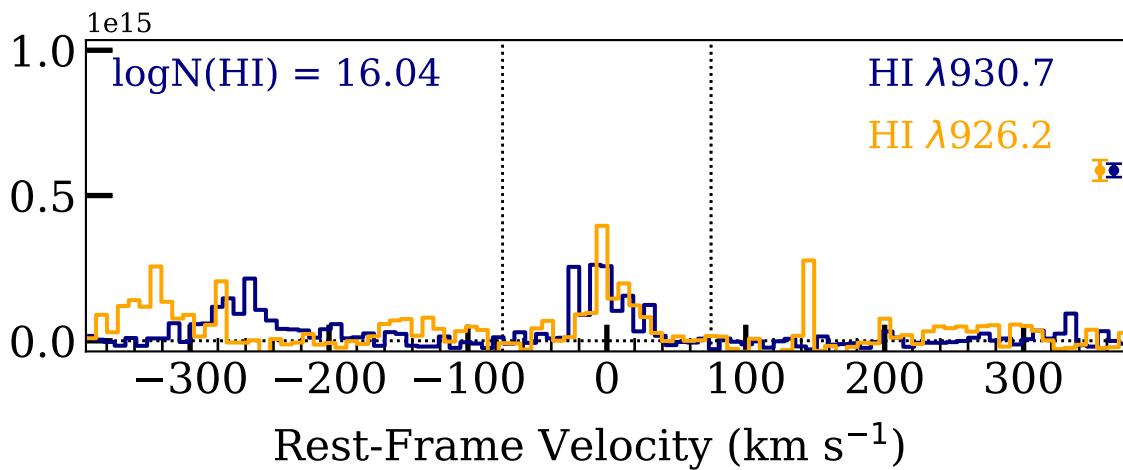

J140732.25+550725.4,  $z=0.246911$ , RF=1

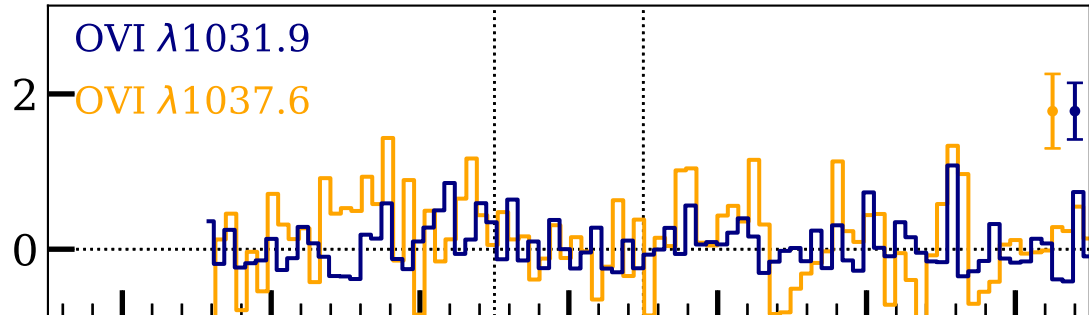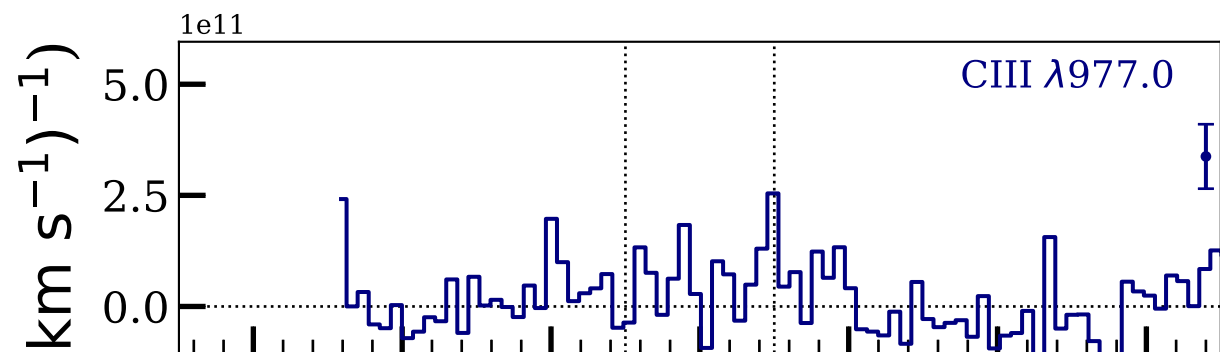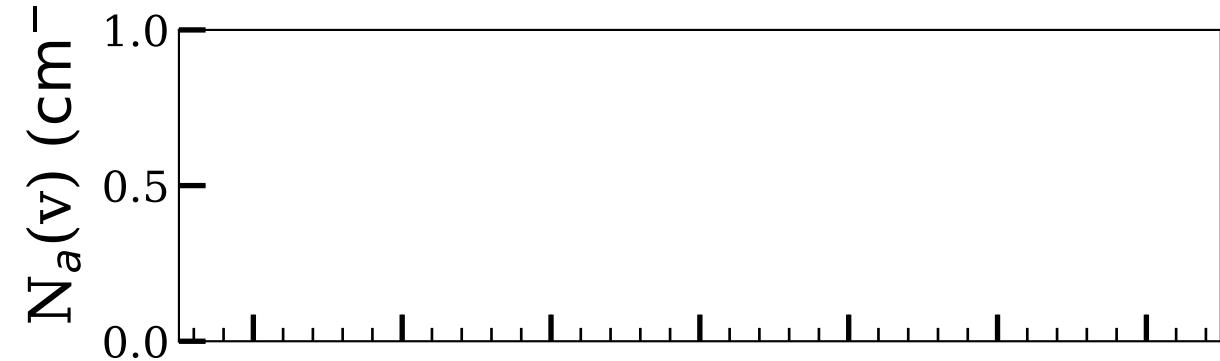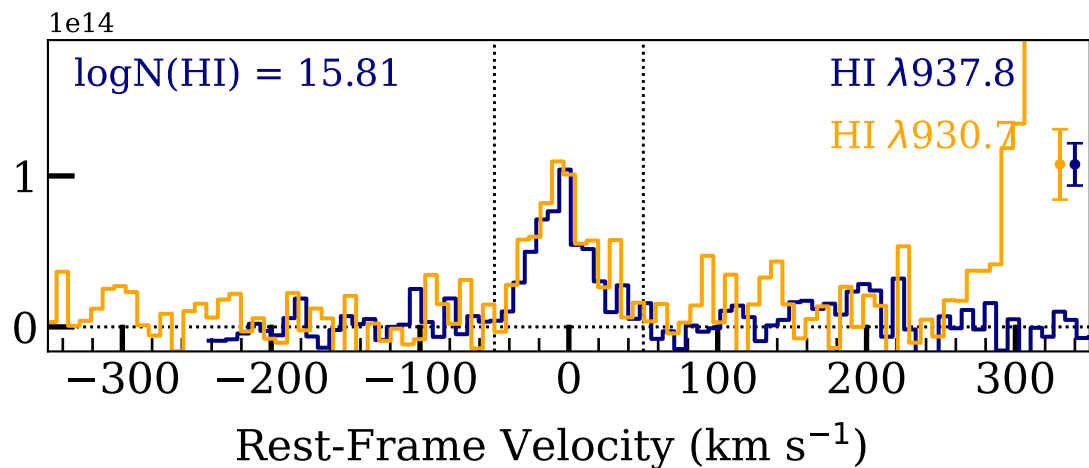

J140923.90+261820.9,  $z=0.574868$ , RF=1

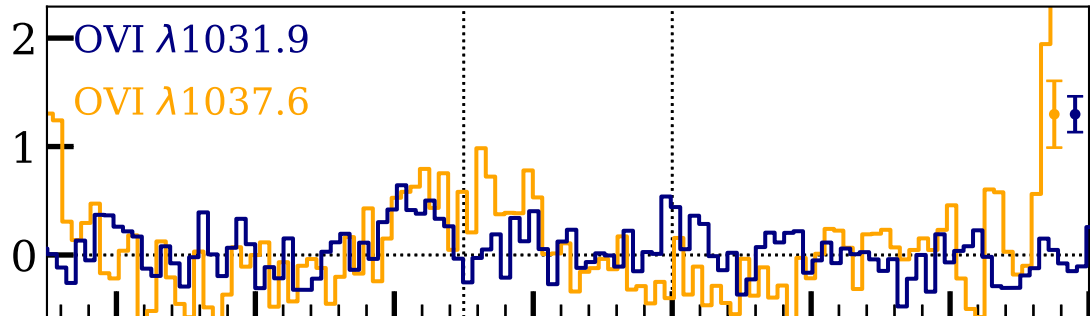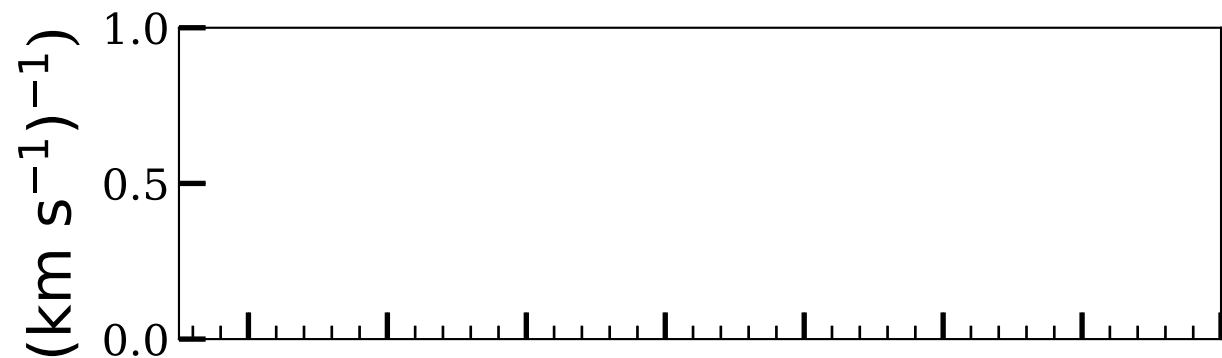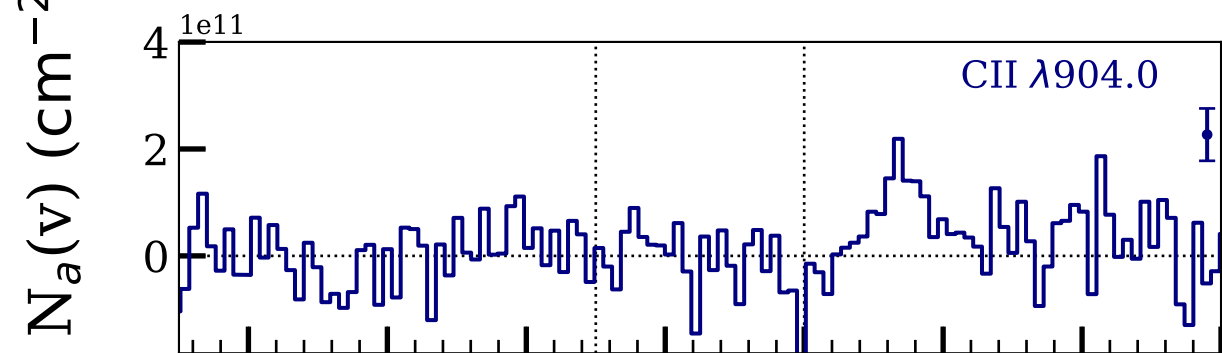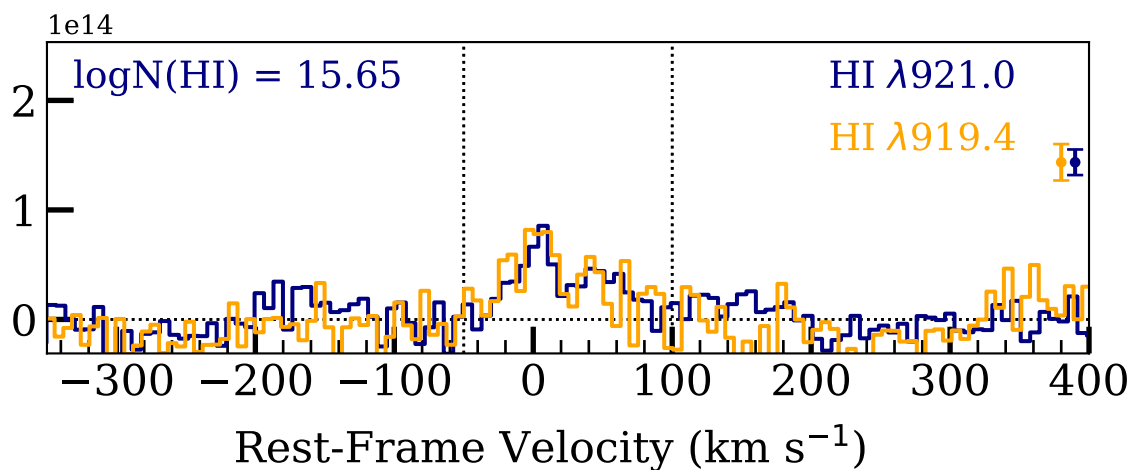

J140923.90+261820.9,  $z=0.599561$ , RF=1

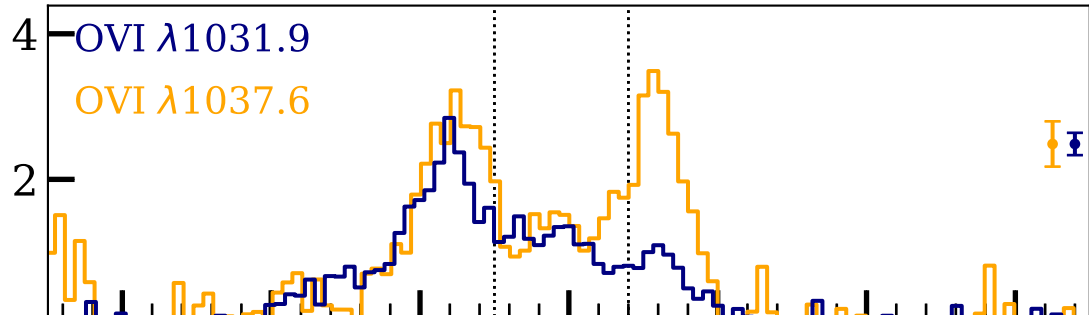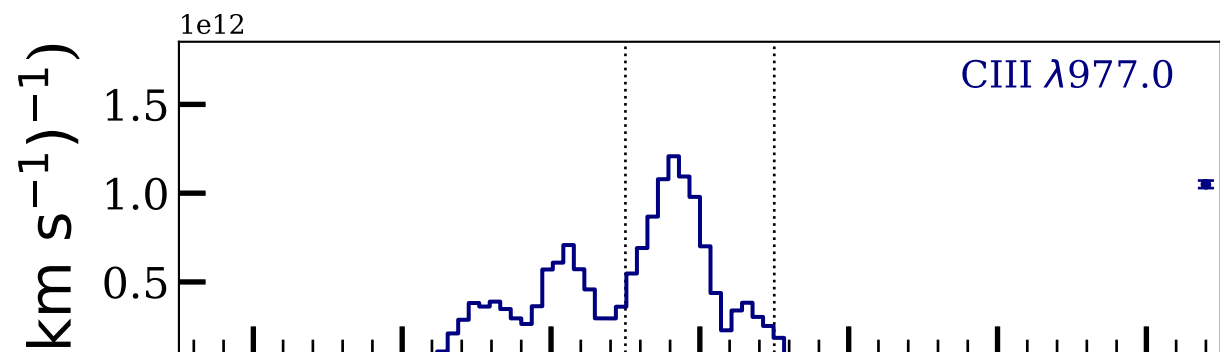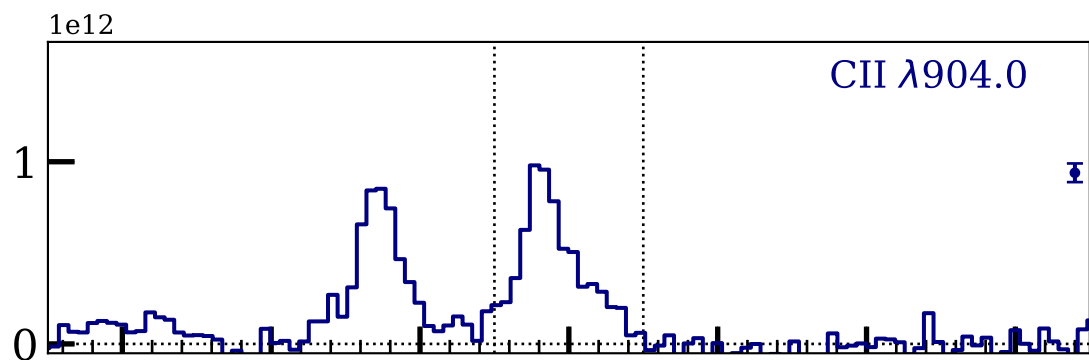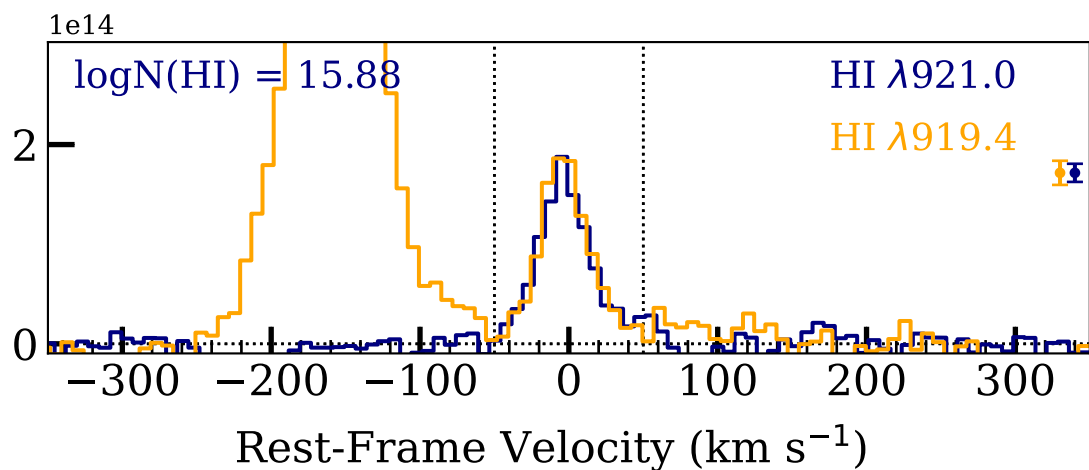

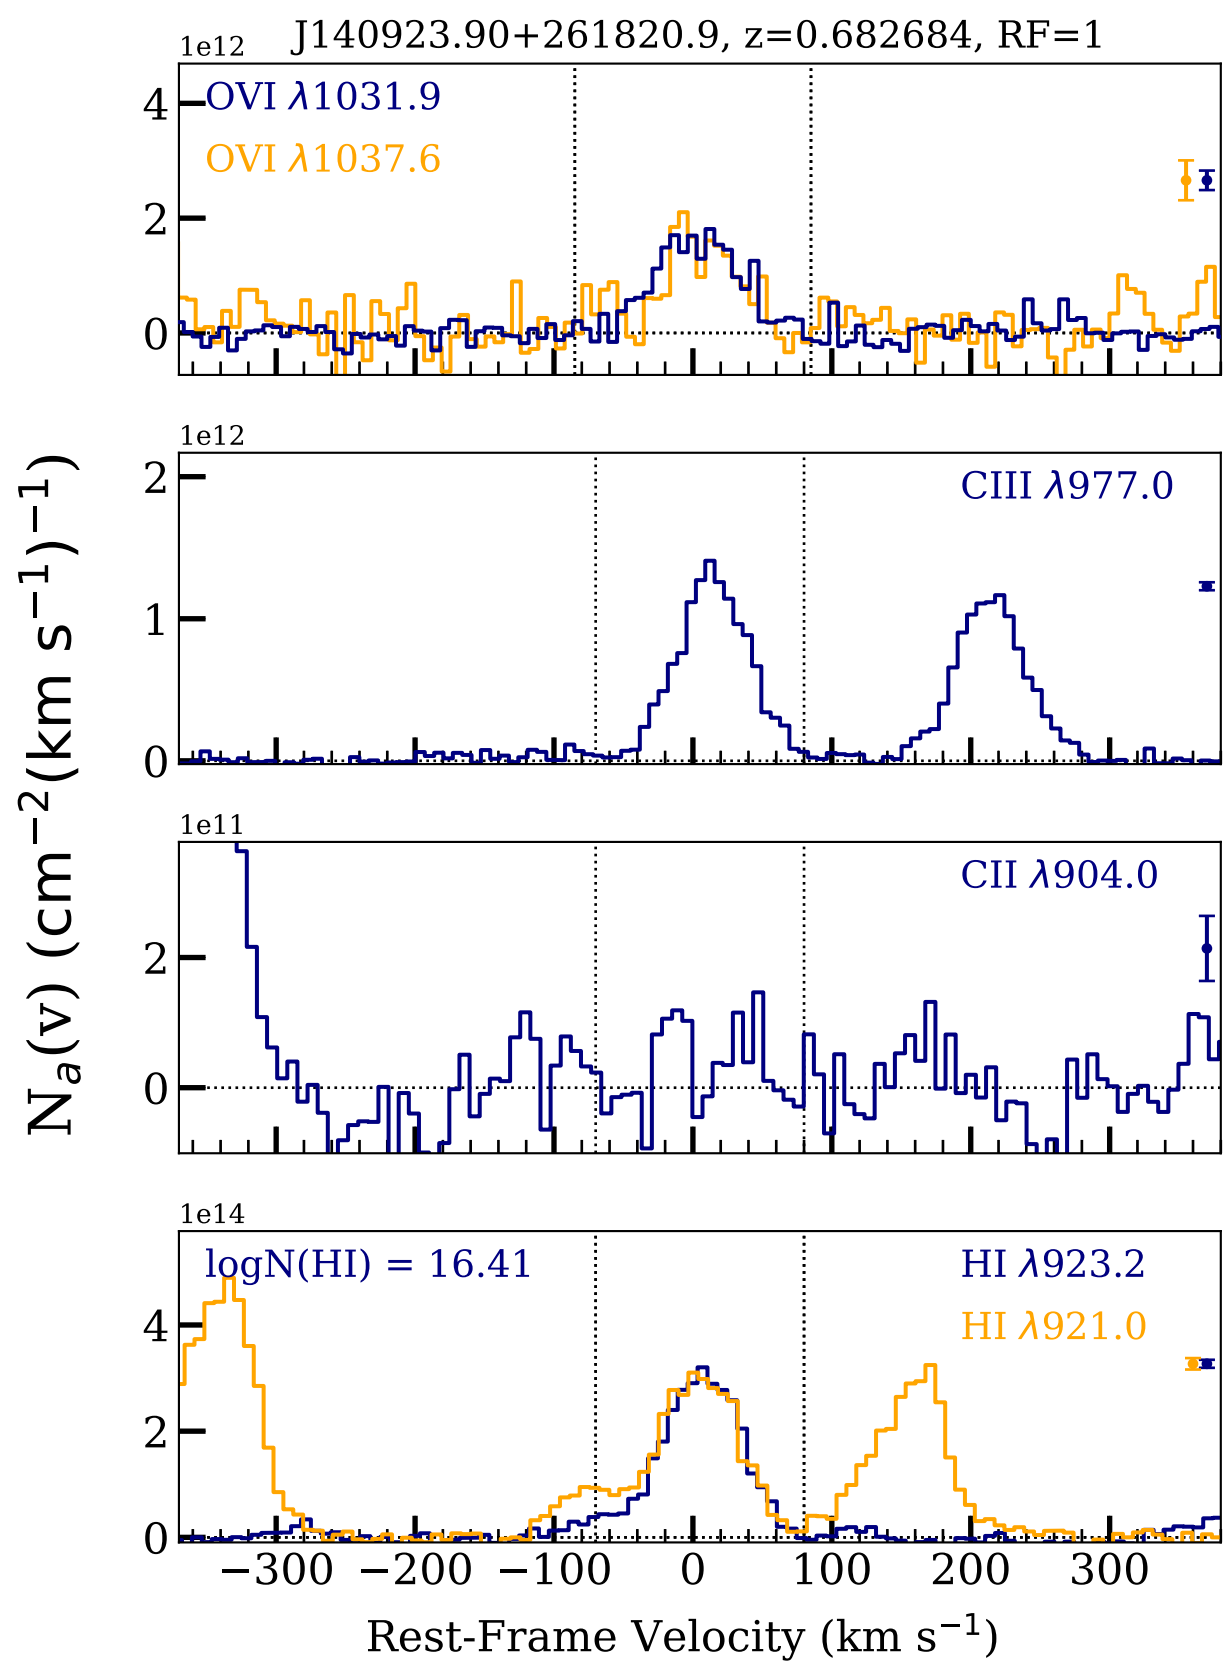



1e12 J141038.39+230447.1,  $z=0.349849$ , RF=1

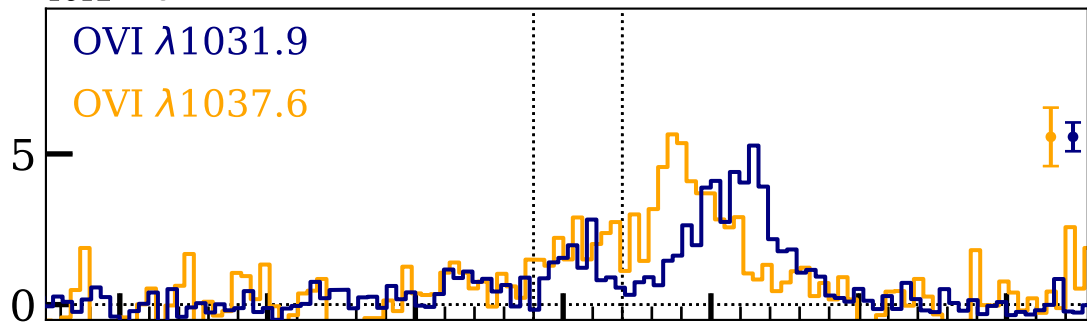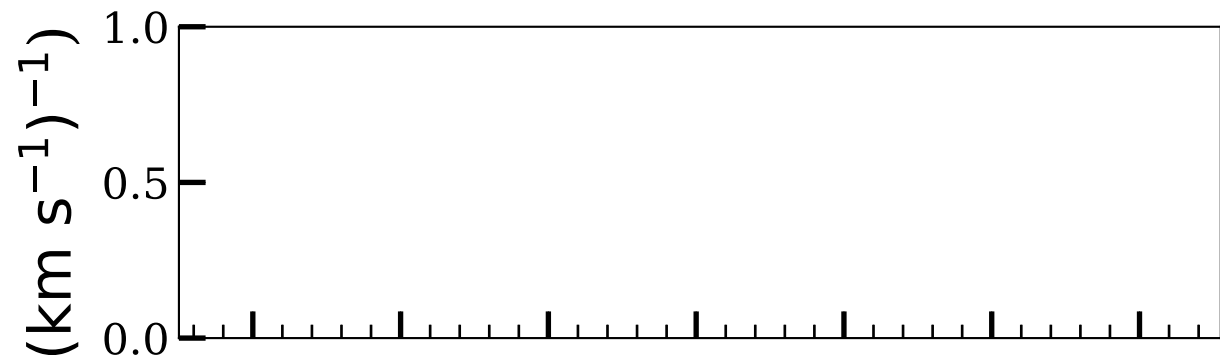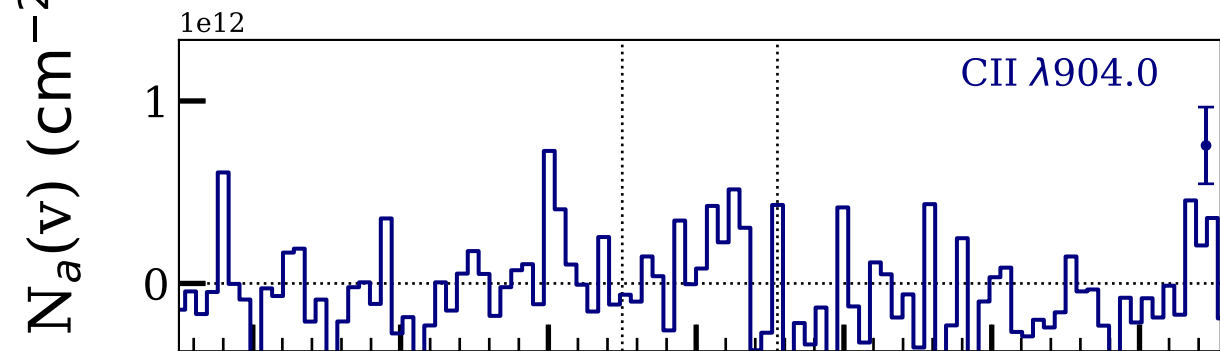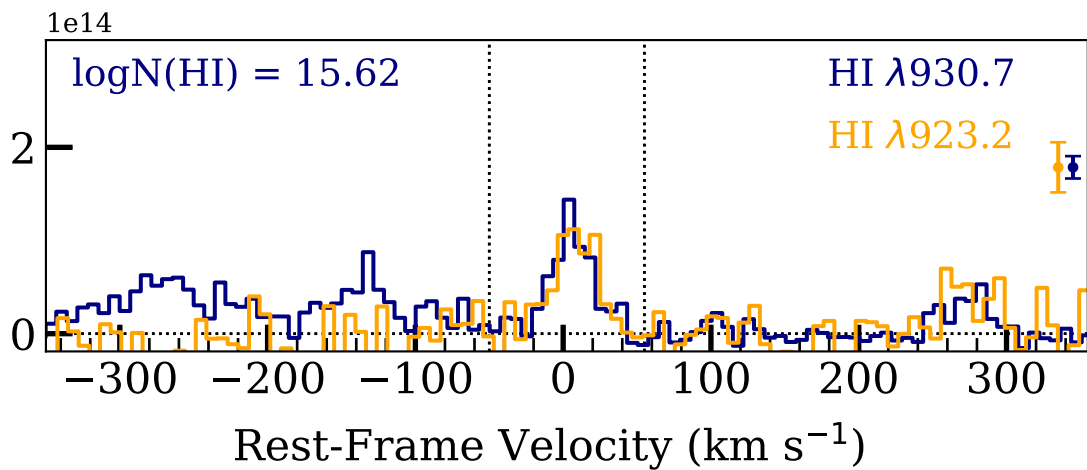

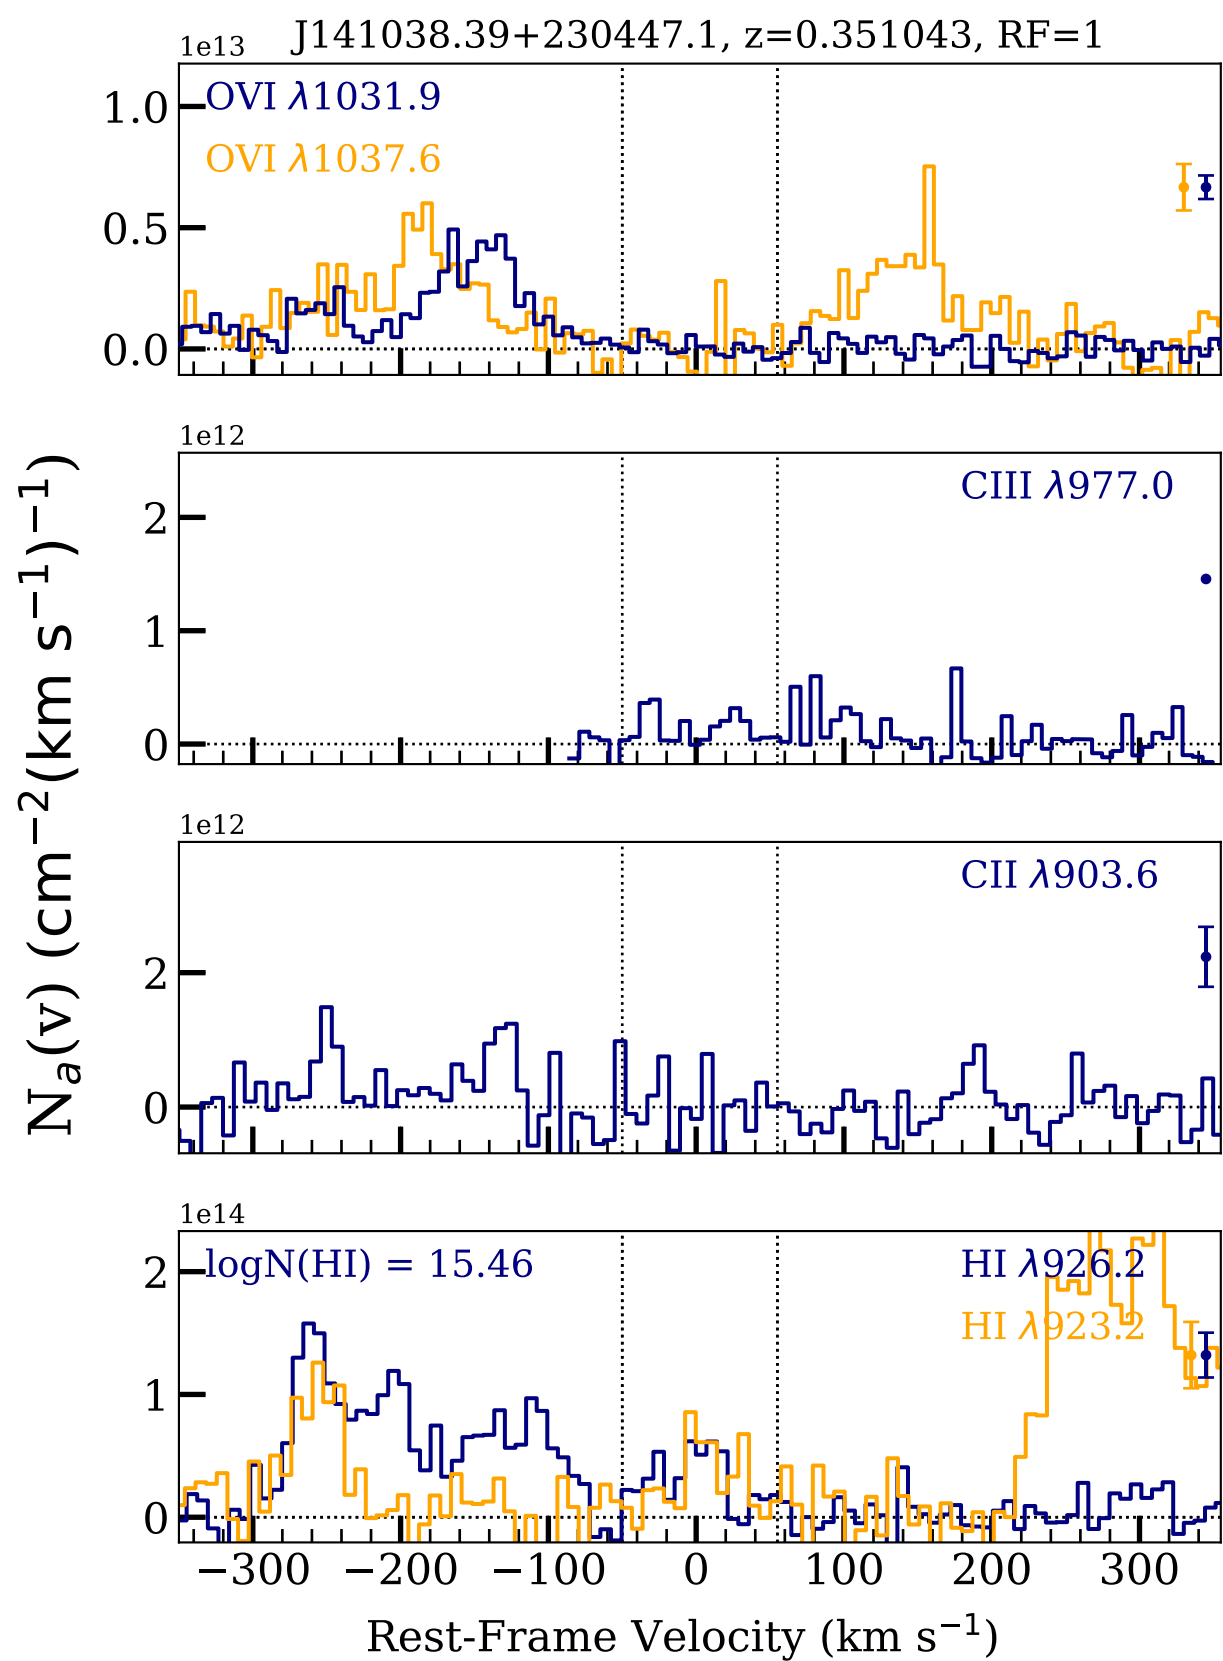

J141038.39+230447.1,  $z=0.535079$ , RF=1

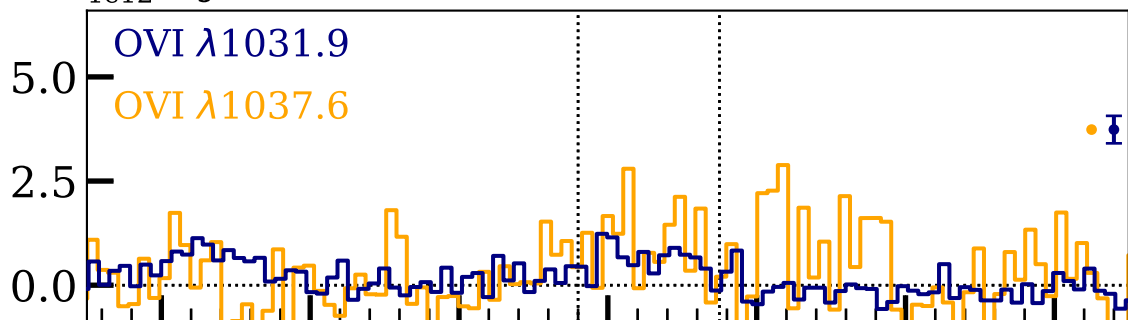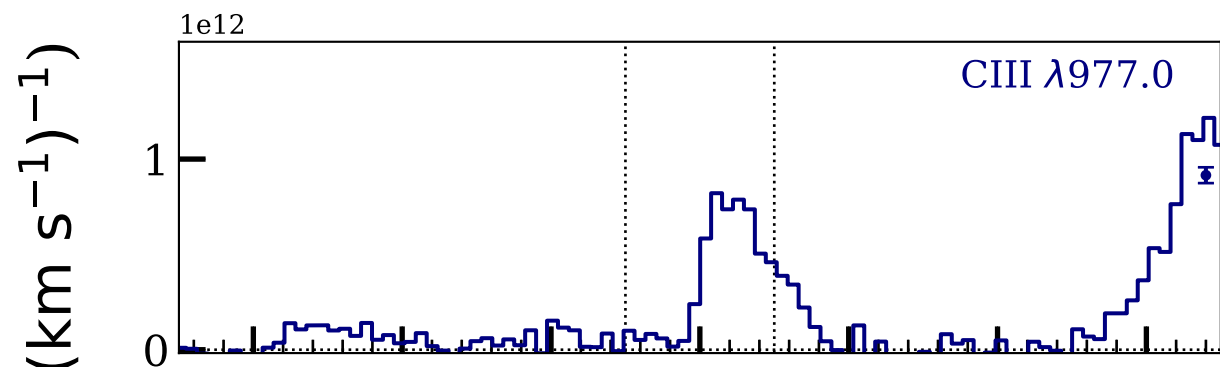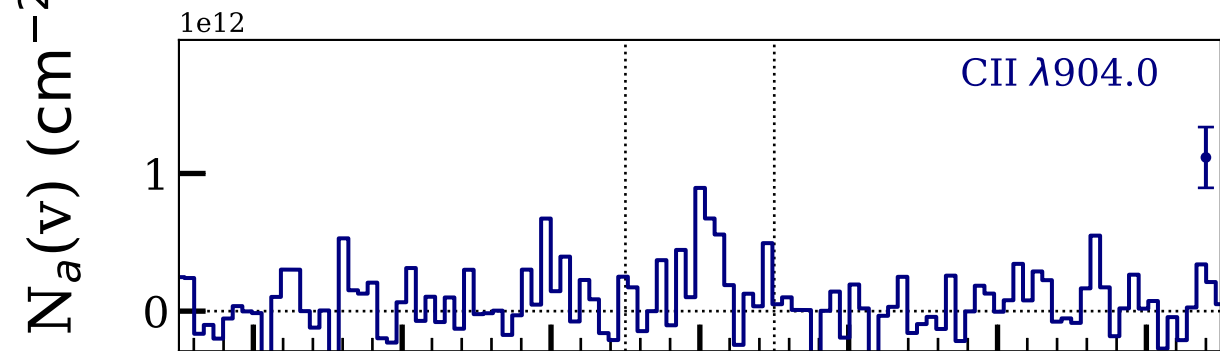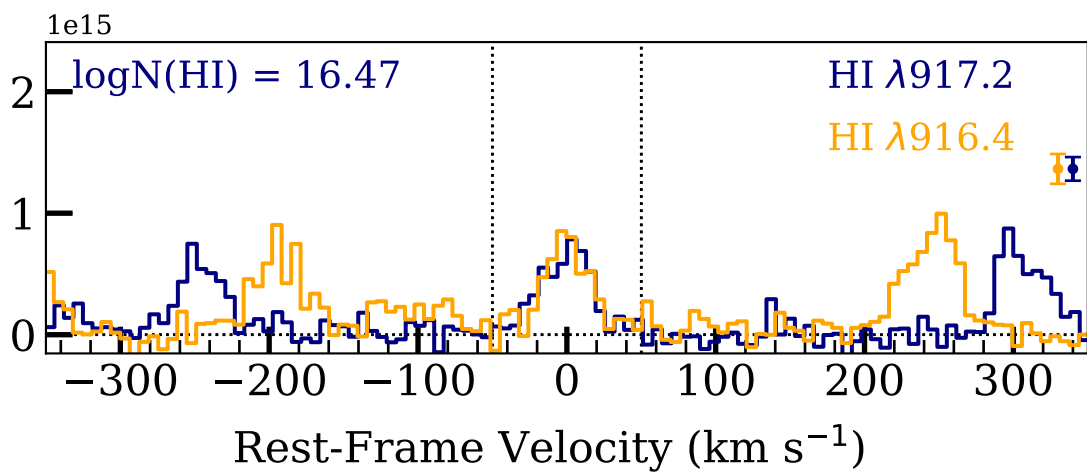

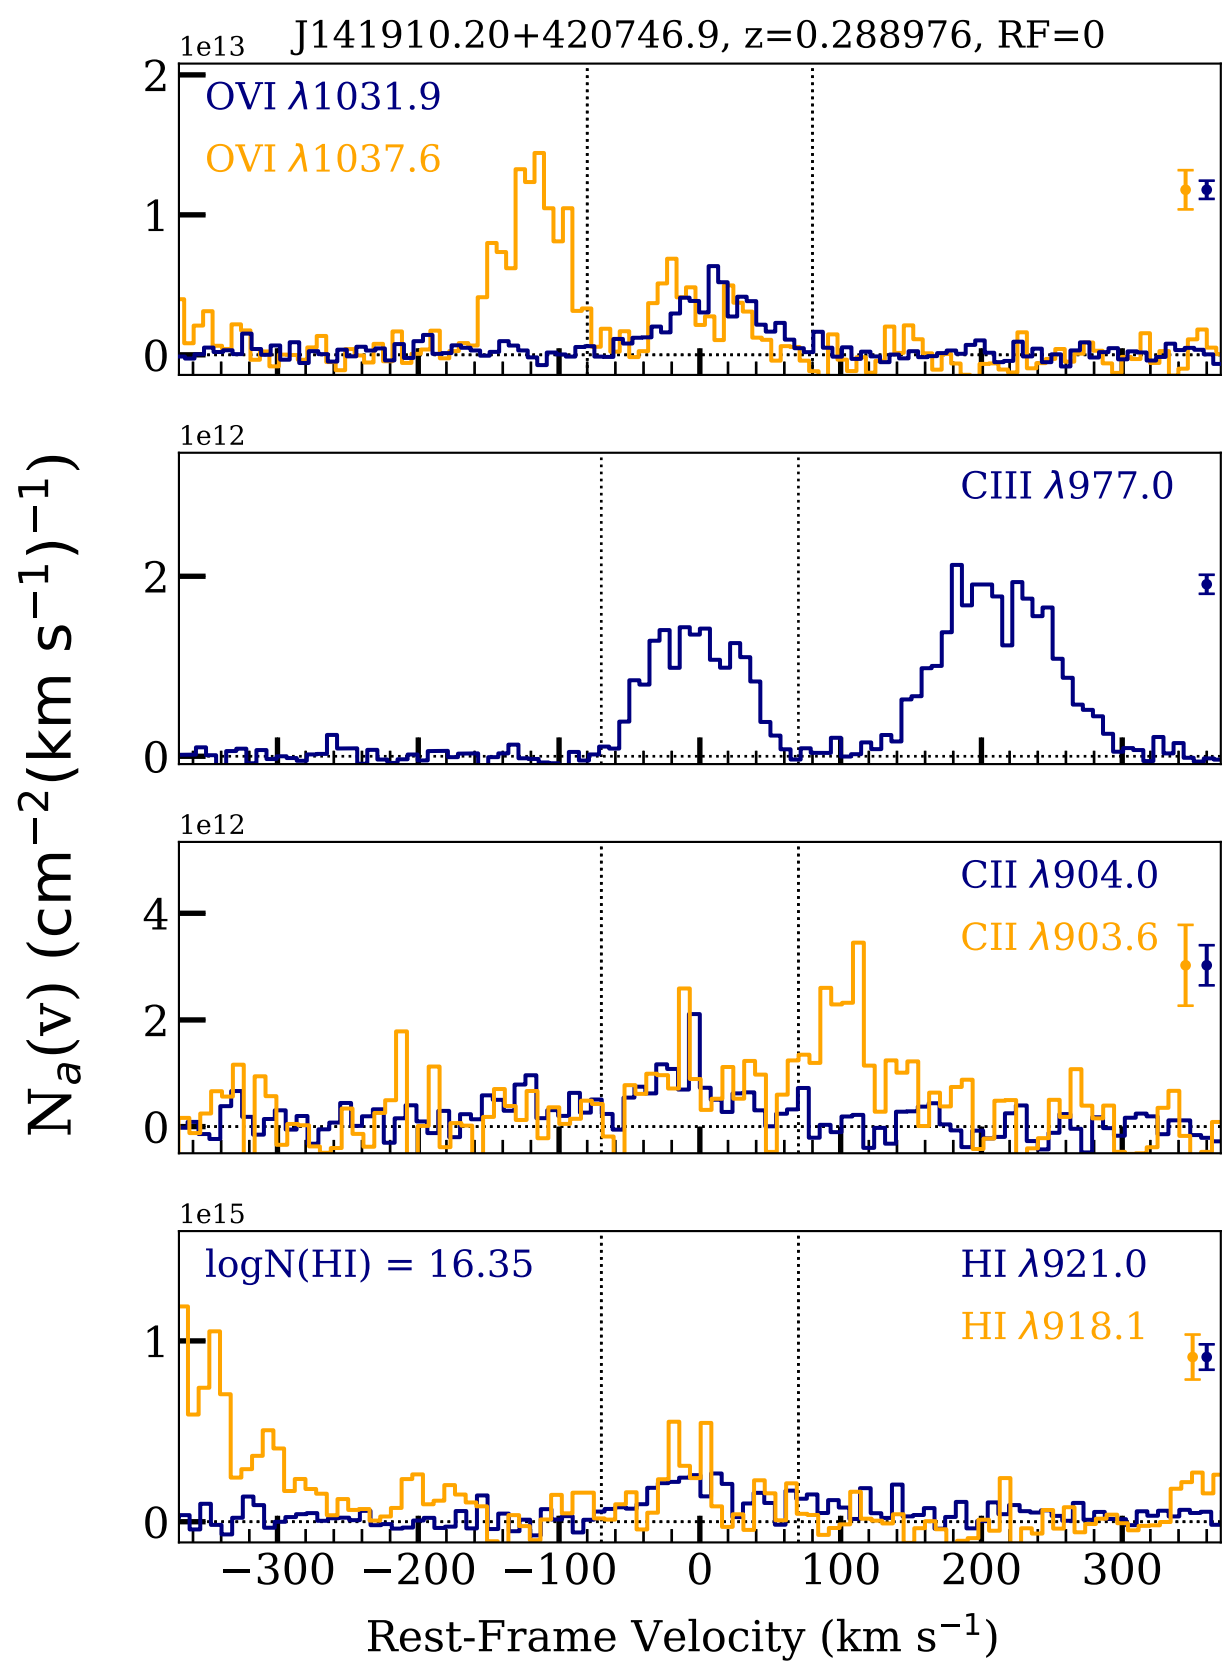

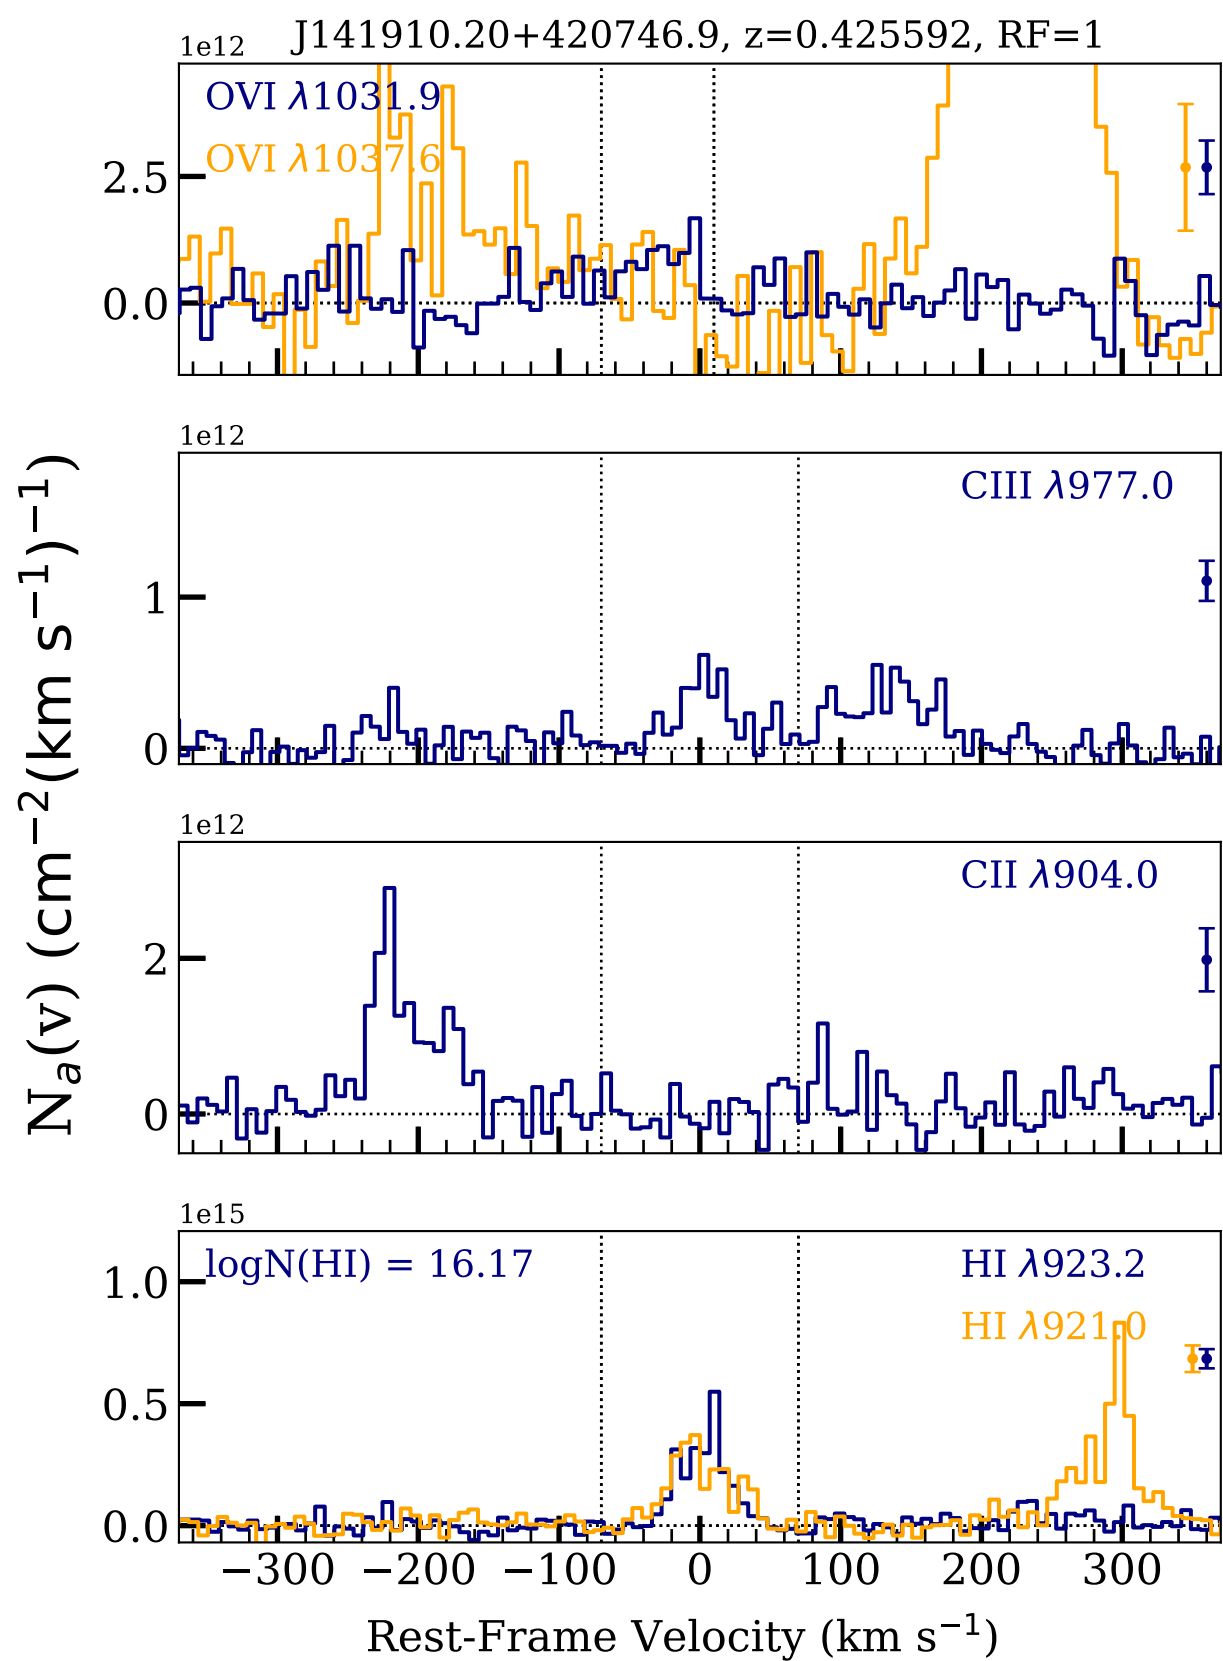

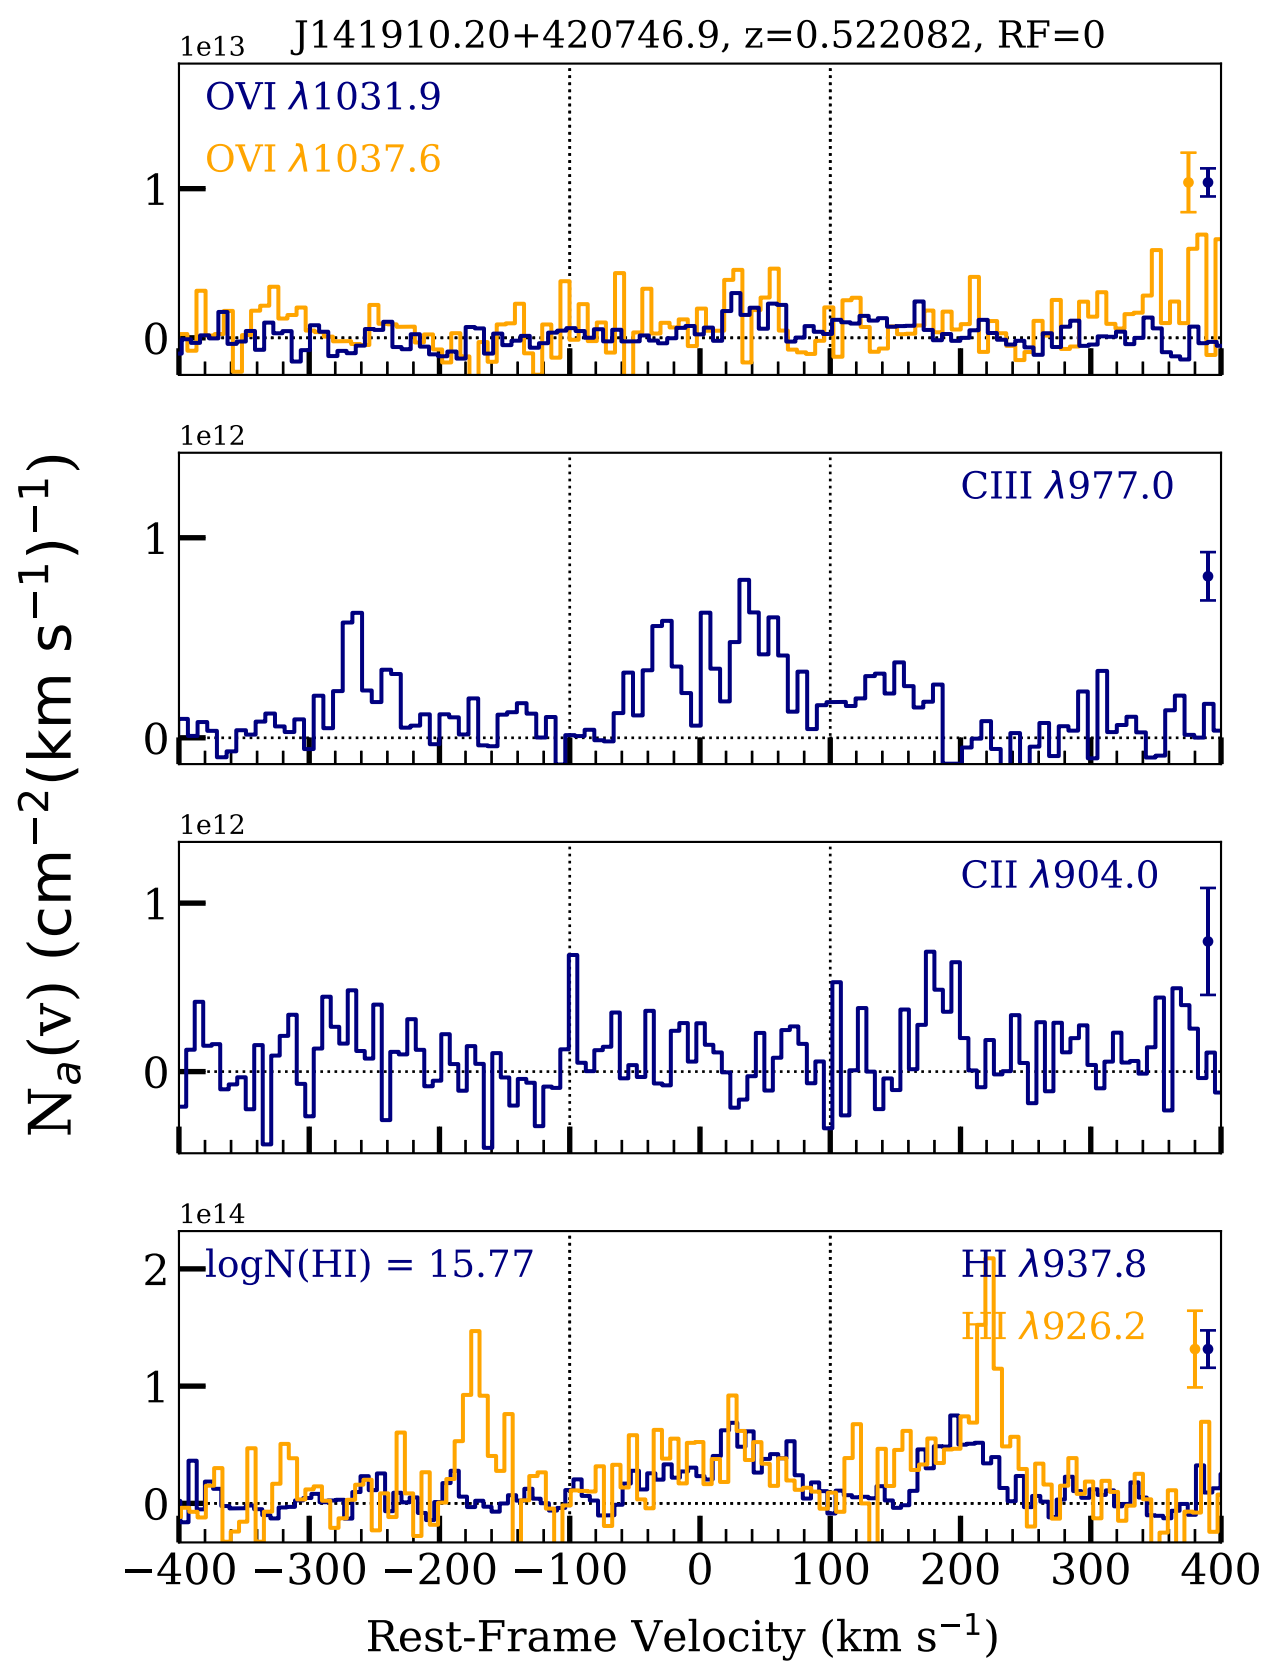

J141910.20+420746.9,  $z=0.534585$ , RF=0

$N_a(v) \text{ (cm}^{-2} \text{ (km s}^{-1} \text{)}^{-1} \text{)}$

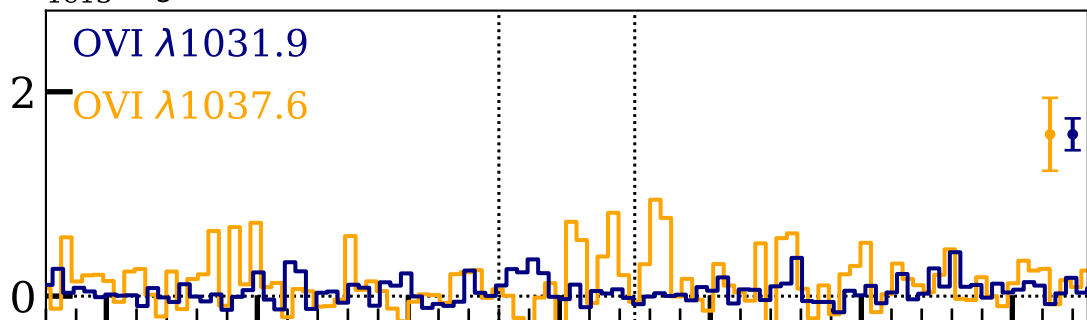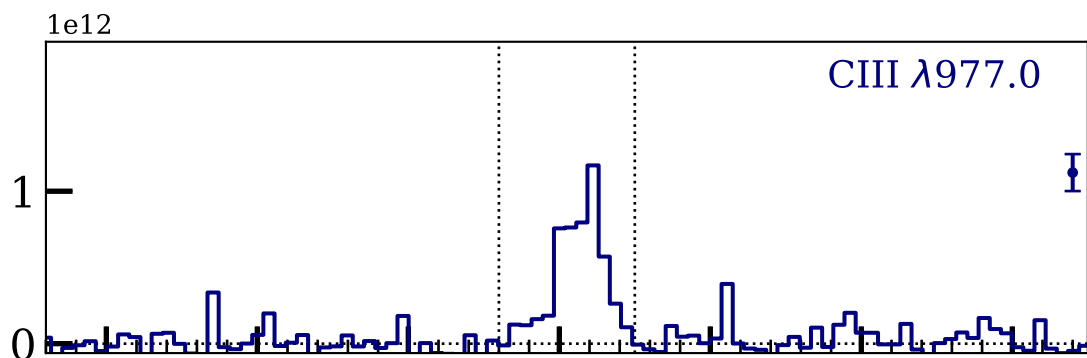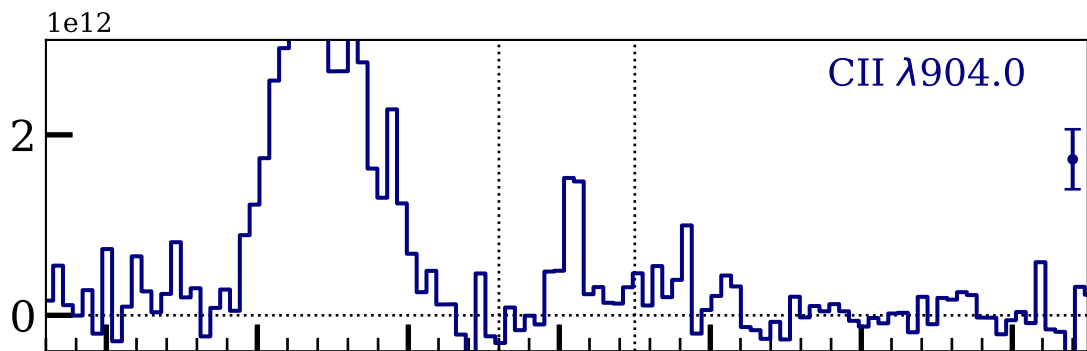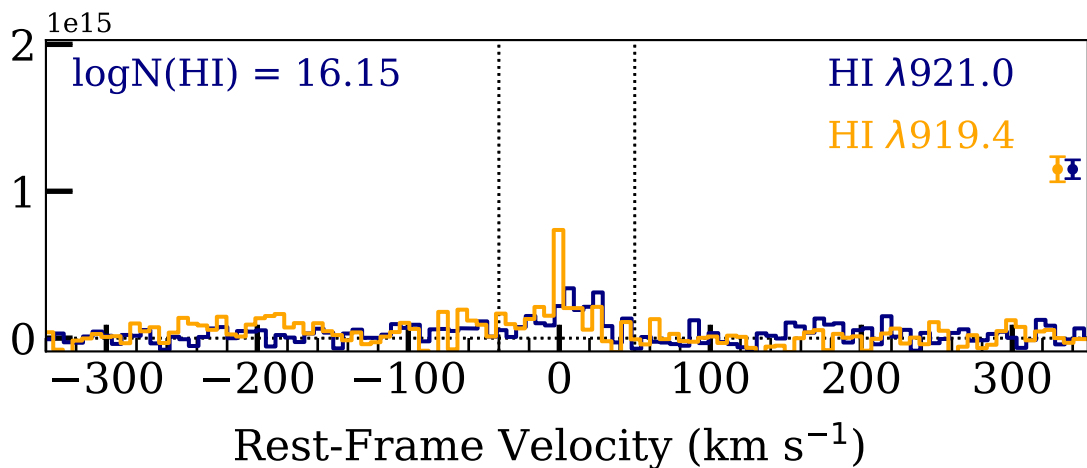

J141910.20+420746.9,  $z=0.608265$ , RF=0

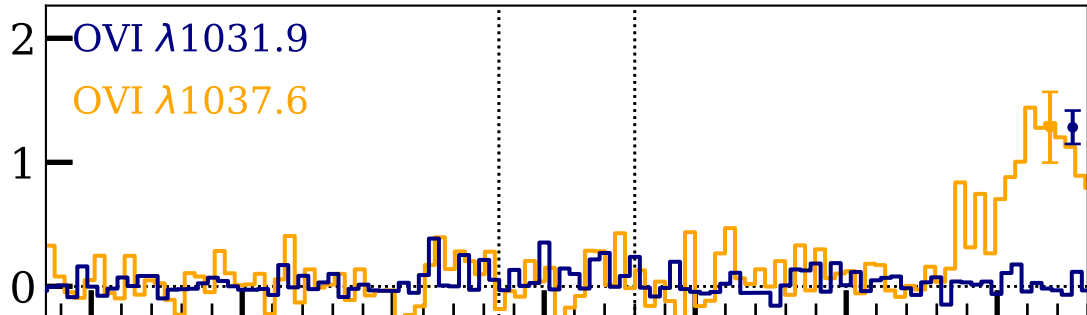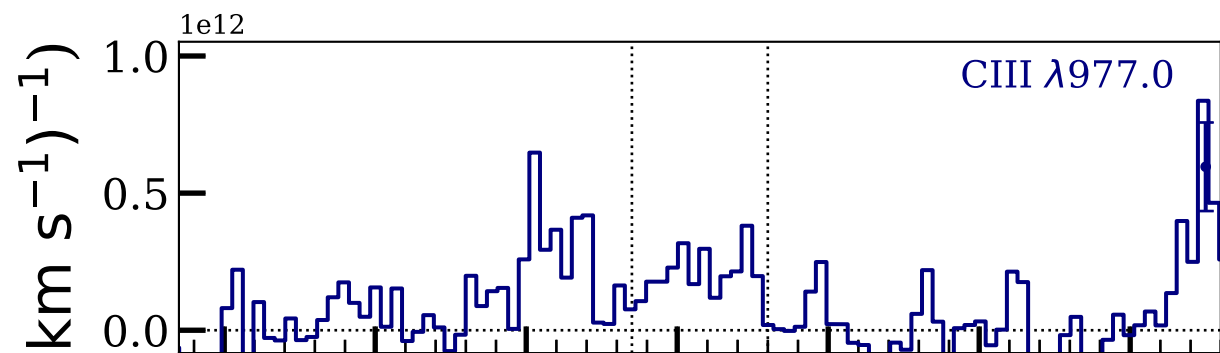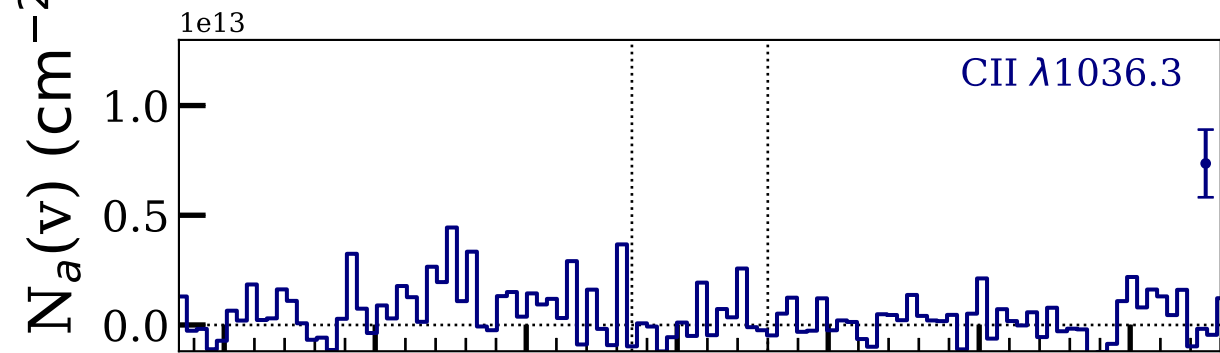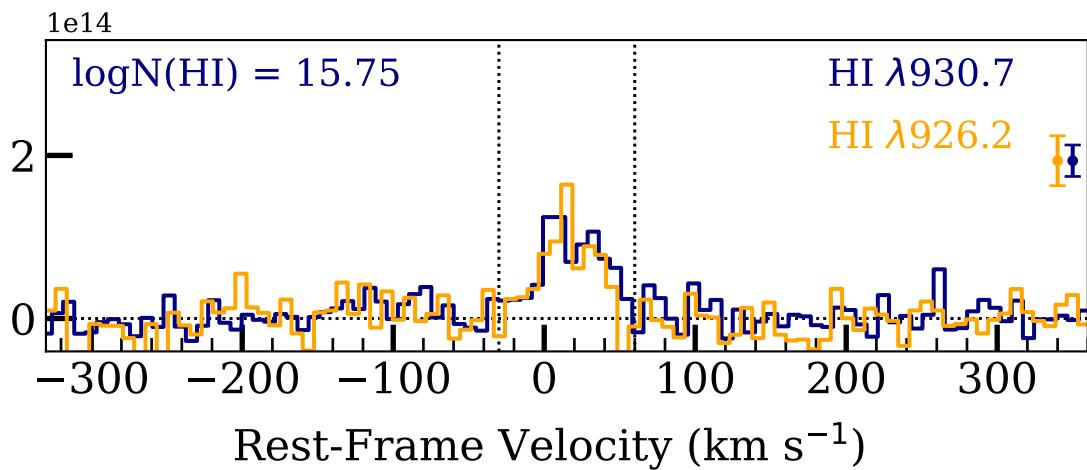



J142735.59+263214.6,  $z=0.366054$ , RF=0

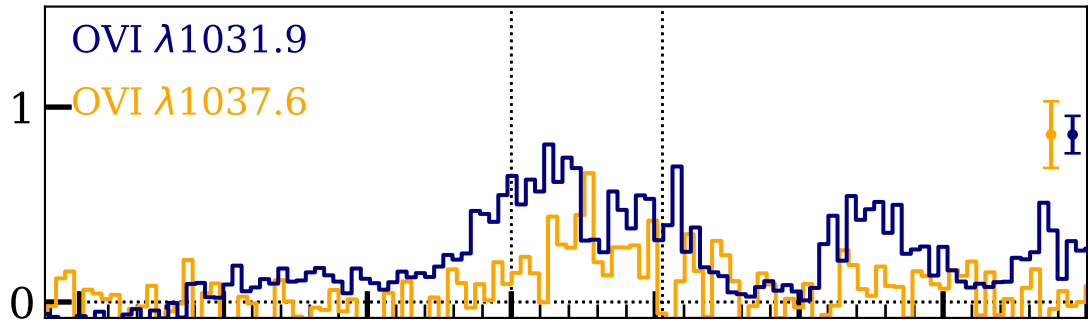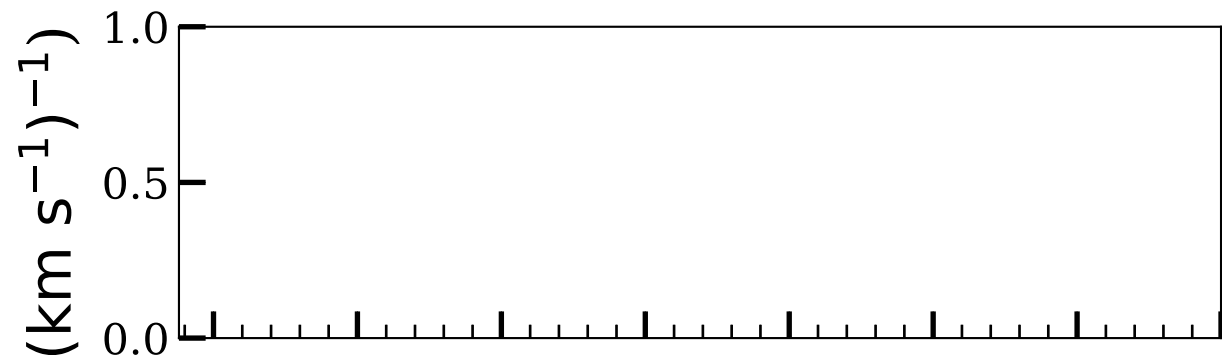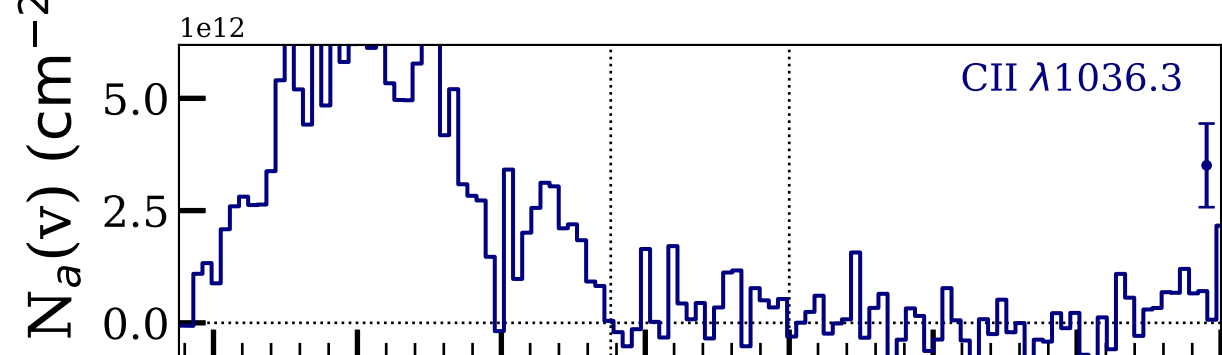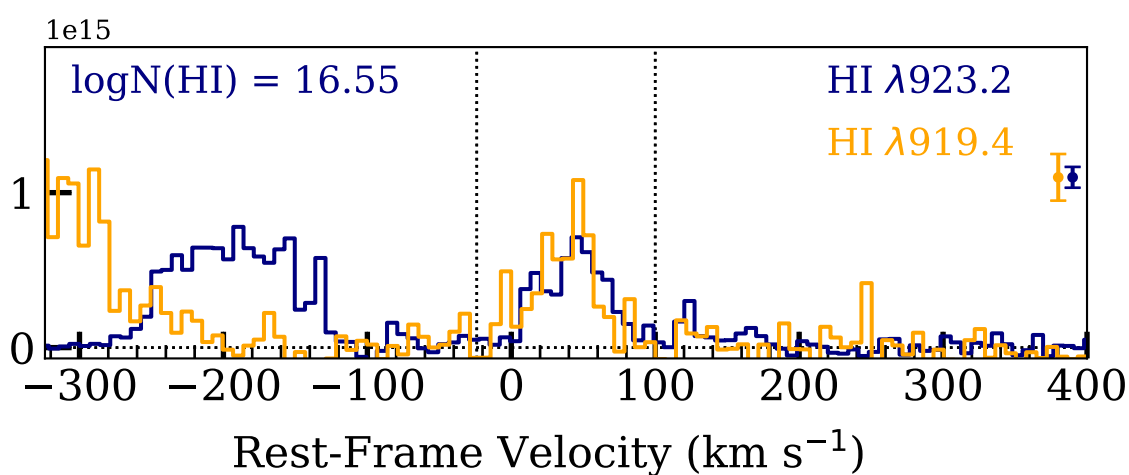

J142859.03+322506.8,  $z=0.382333$ , RF=1

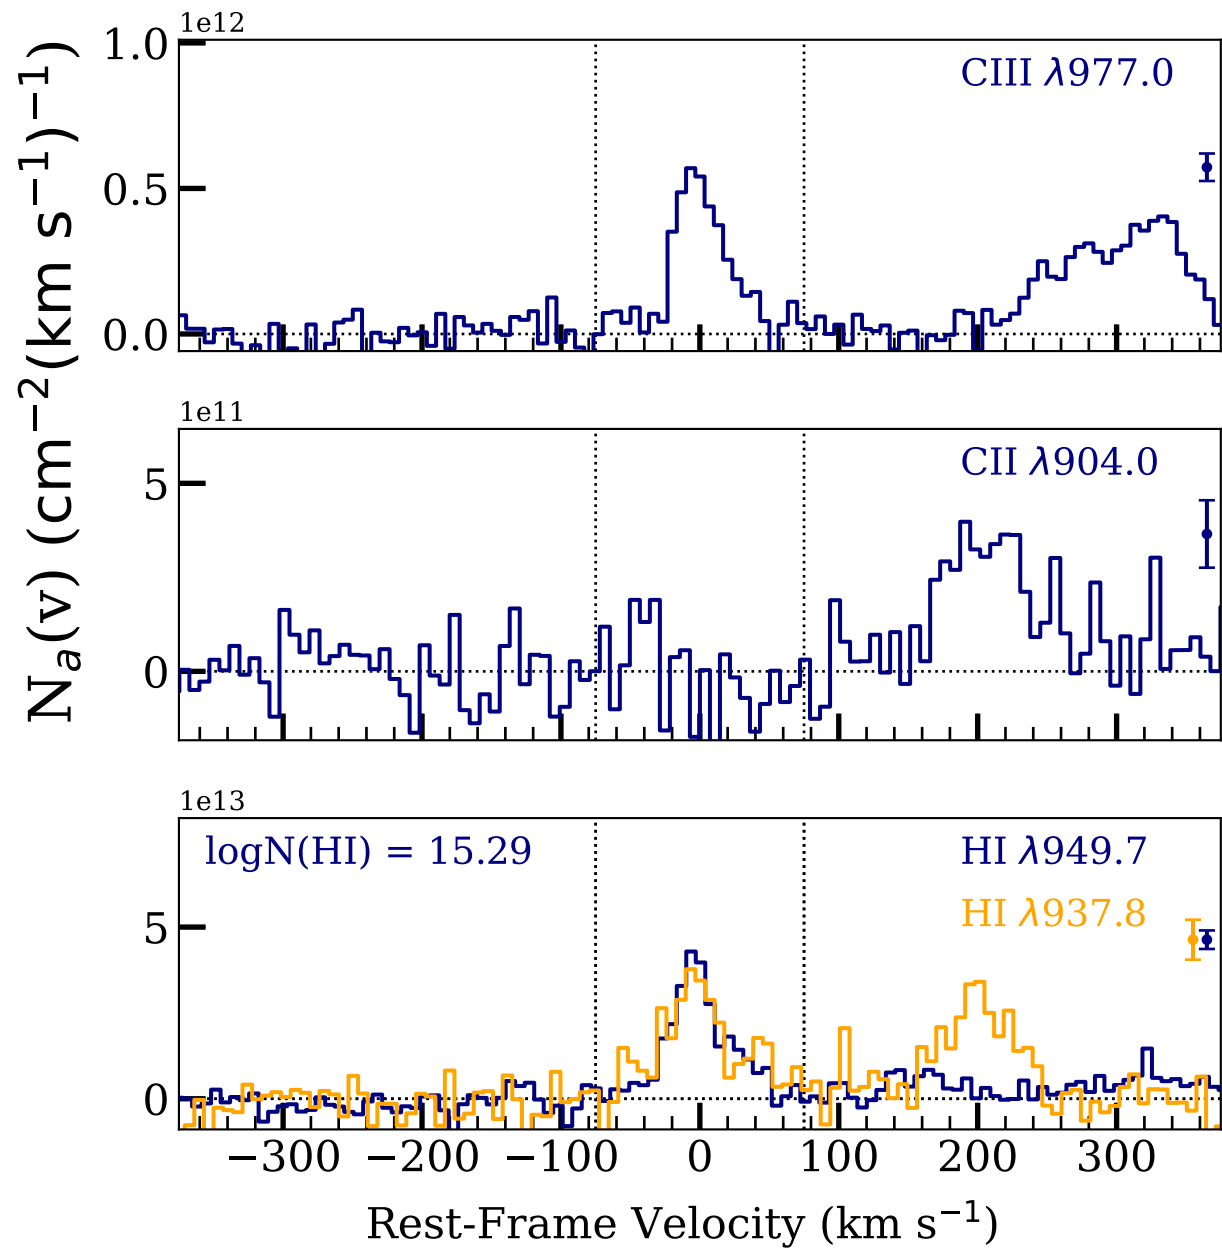

J143511.53+360437.2,  $z=0.372981$ , RF=1

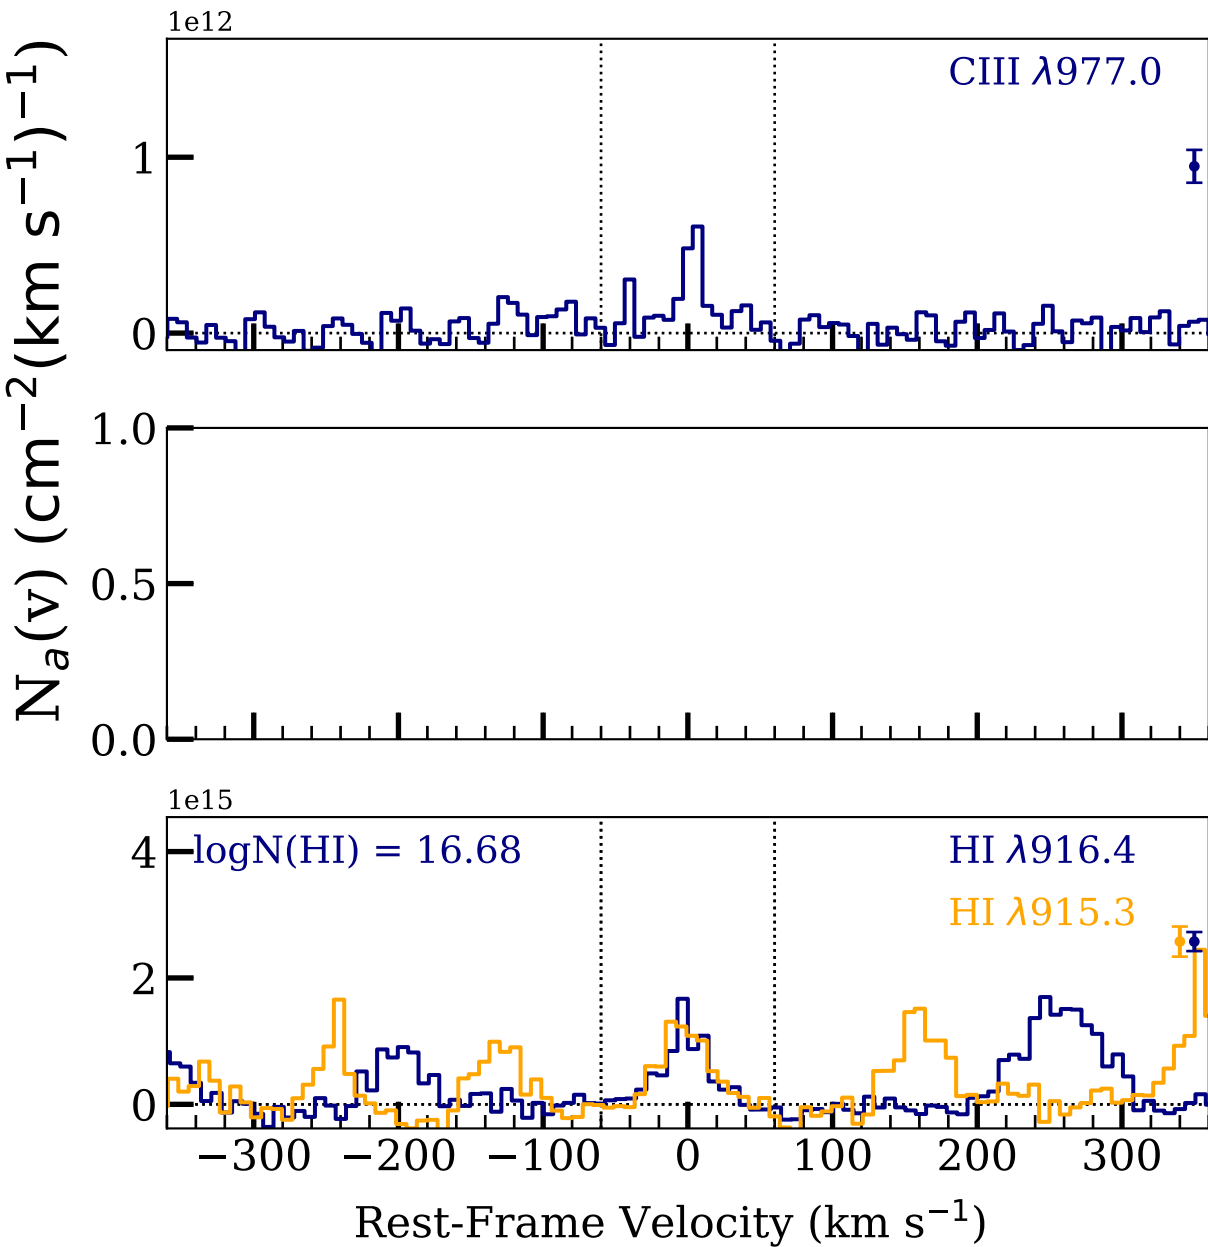

J143511.53+360437.2,  $z=0.387594$ , RF=0

$N_a(v)$  ( $\text{cm}^{-2}(\text{km s}^{-1})^{-1}$ )

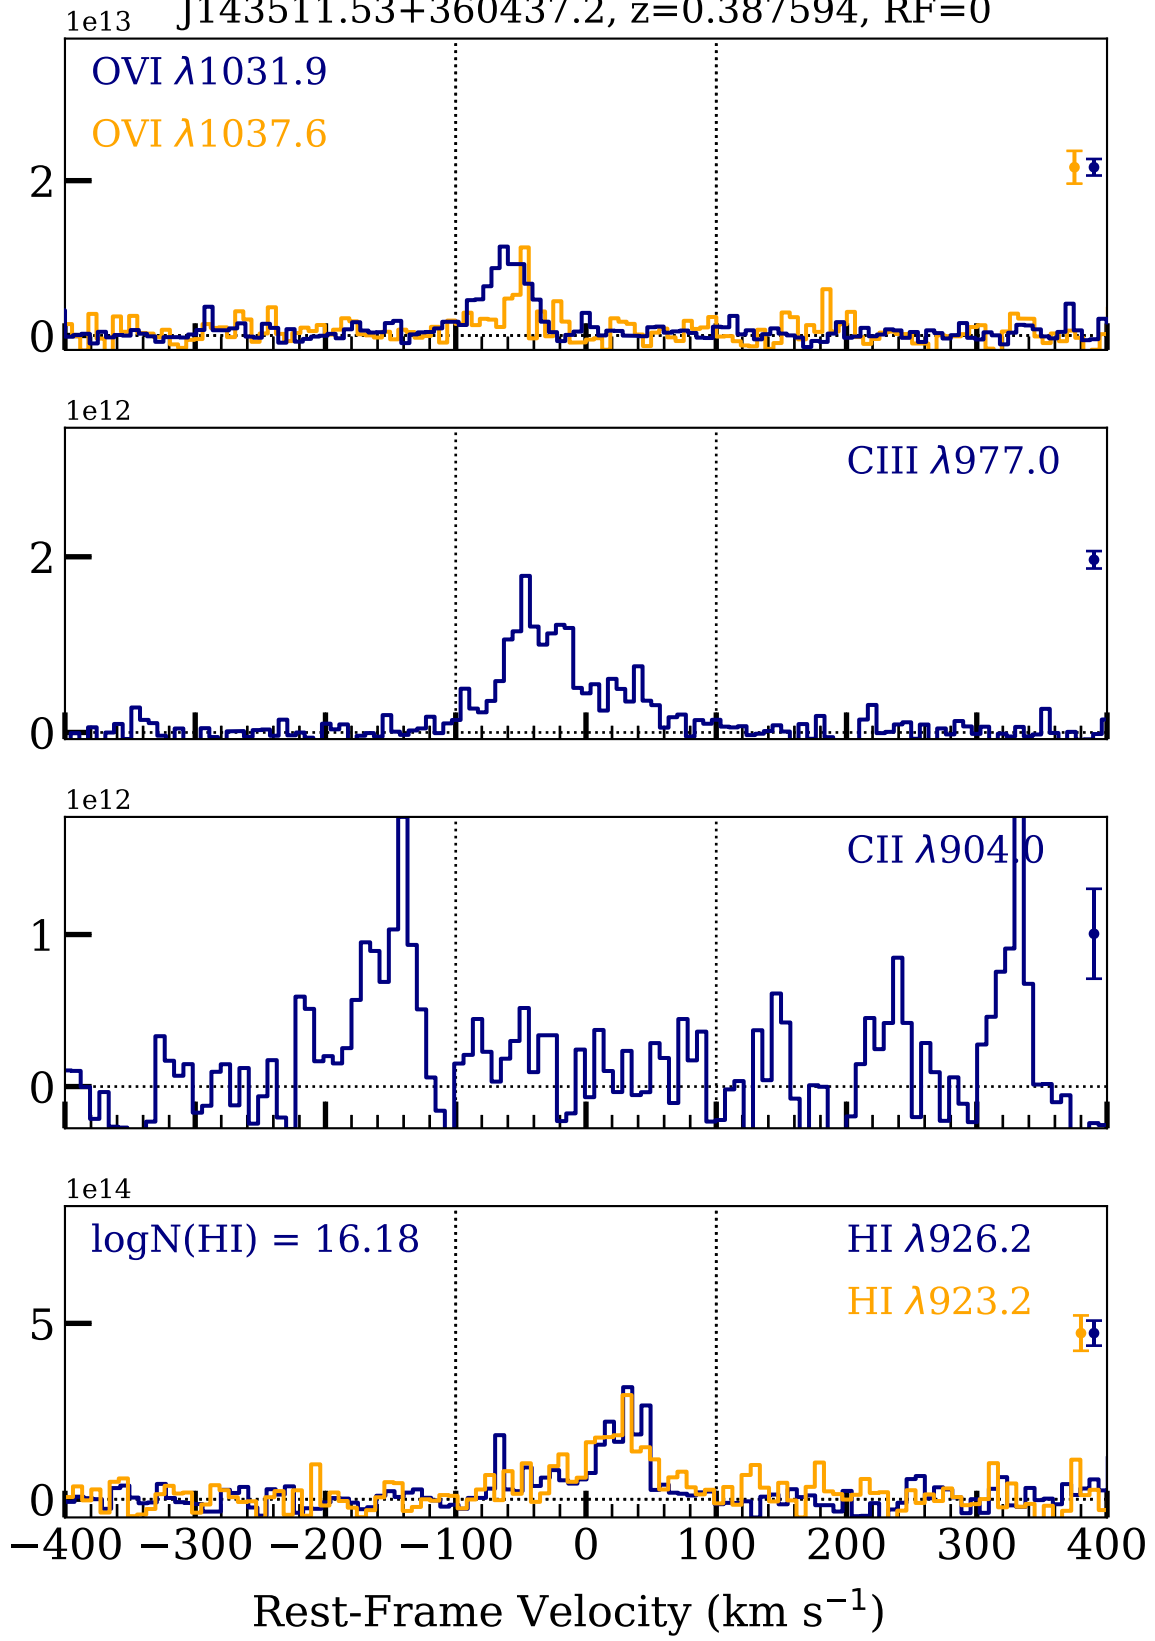

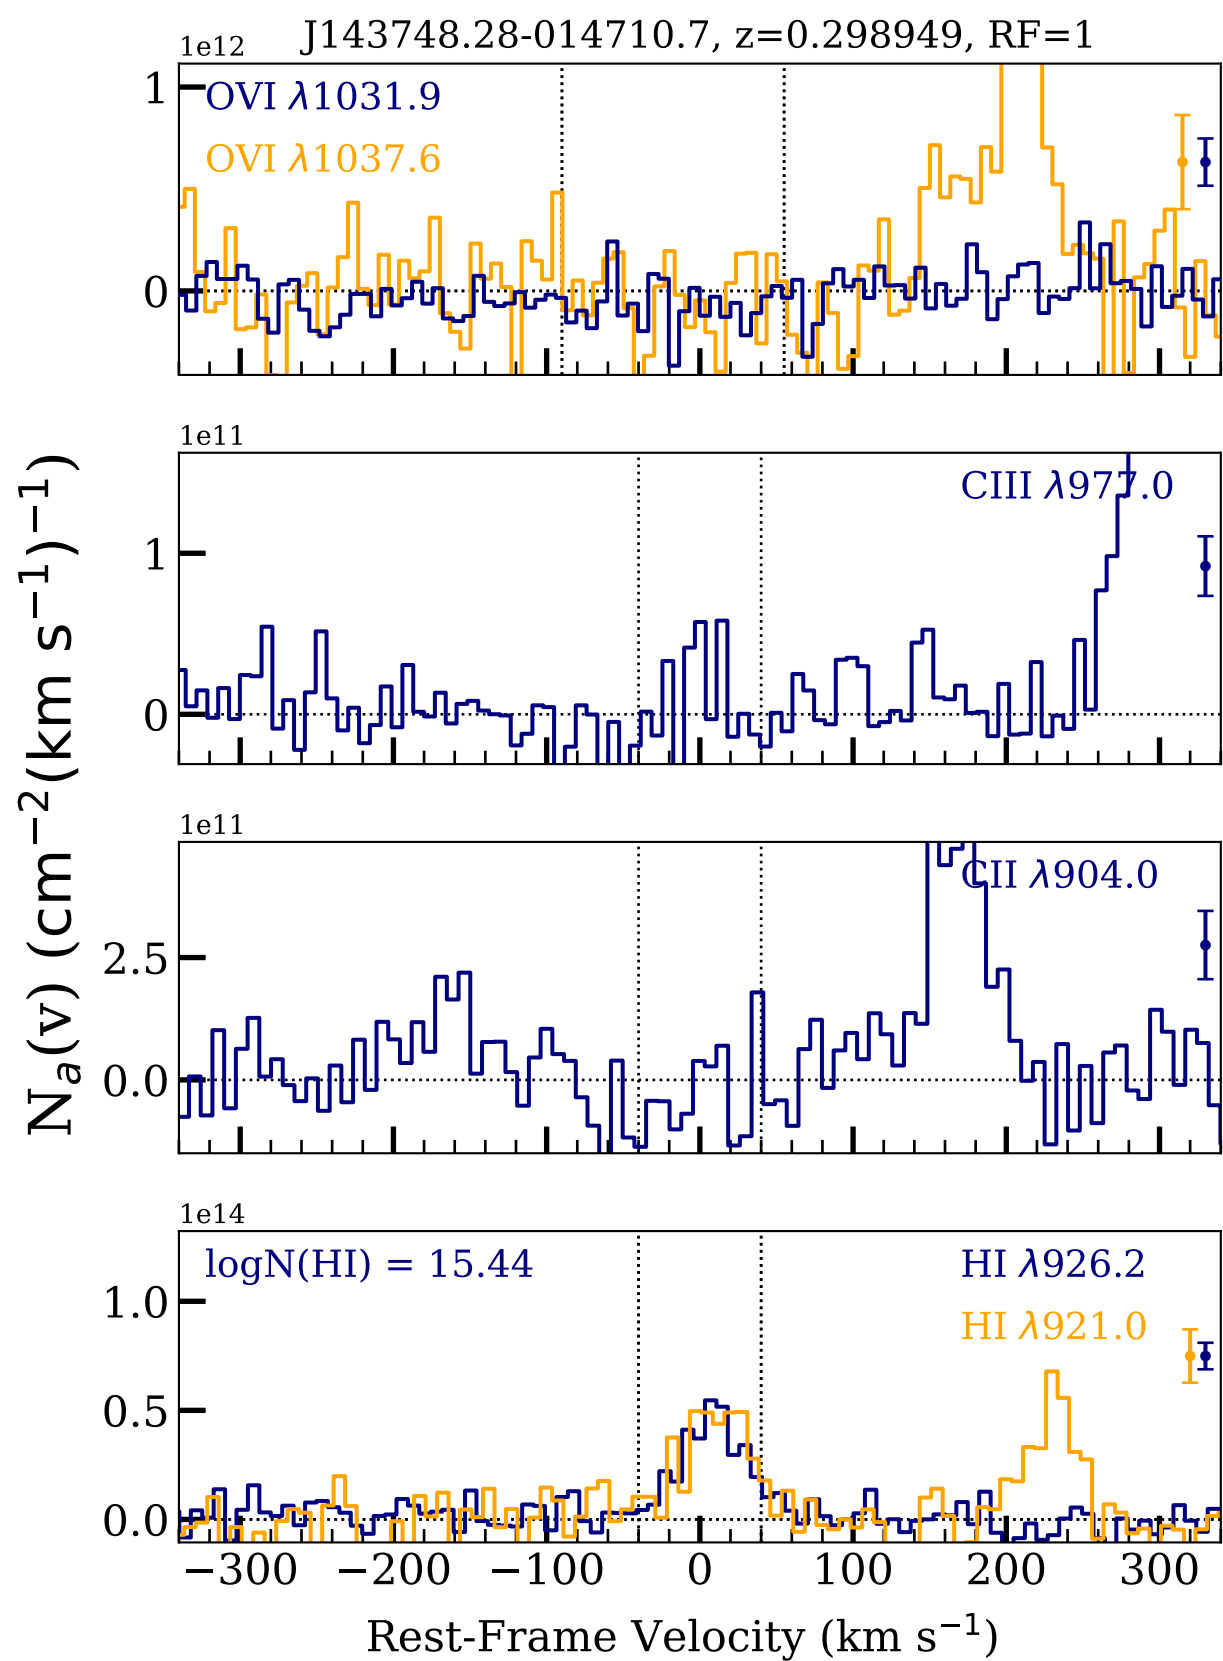

J143748.28-014710.7,  $z=0.612744$ , RF=1

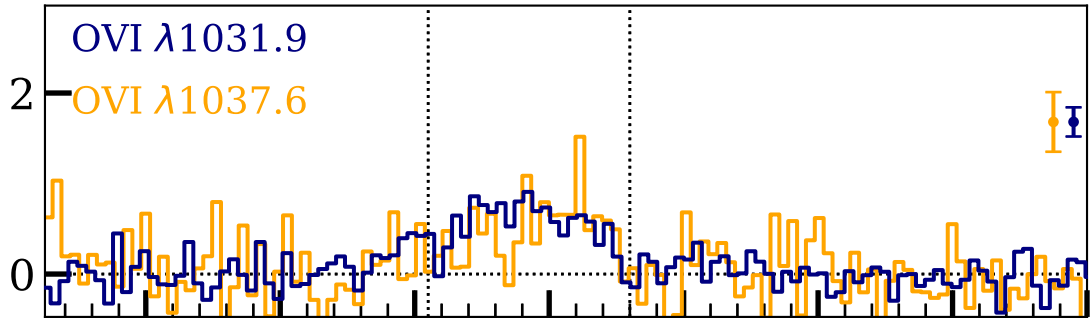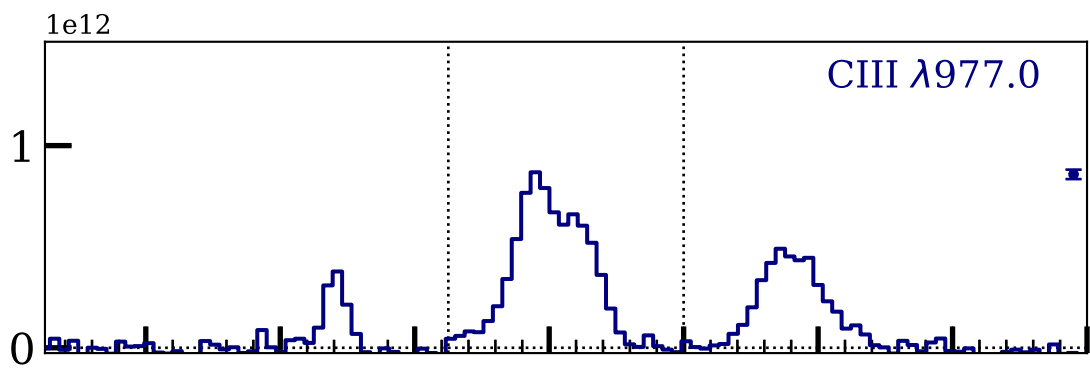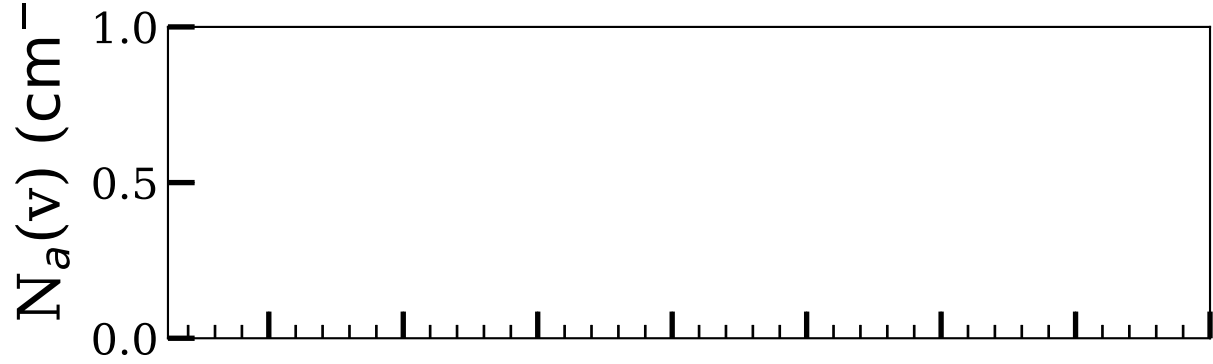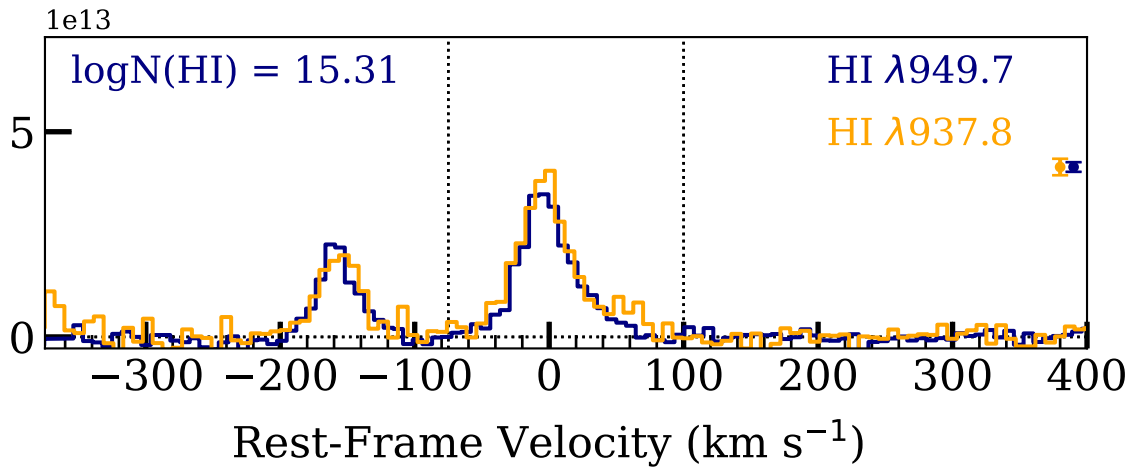

J143748.28-014710.7,  $z=0.681207$ , RF=1

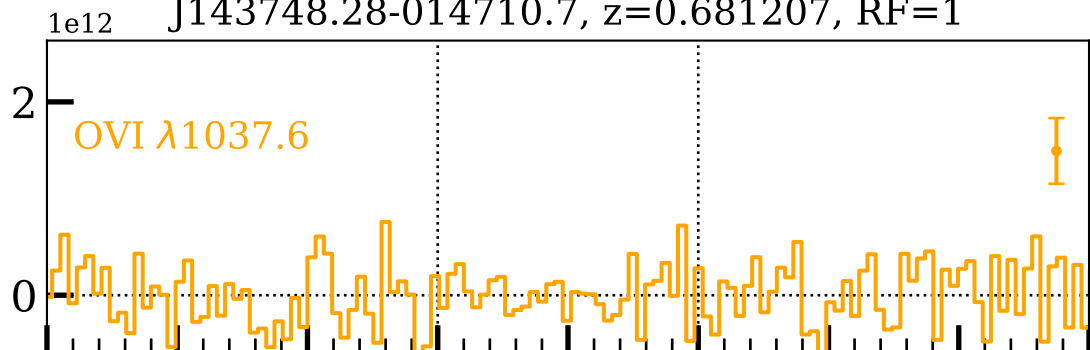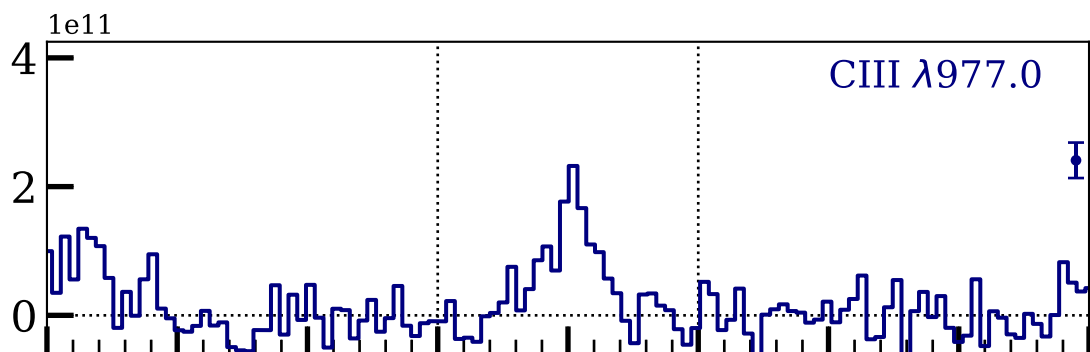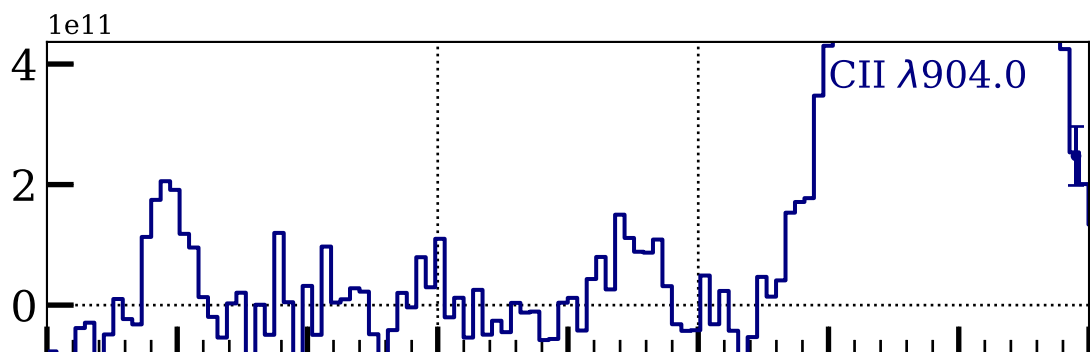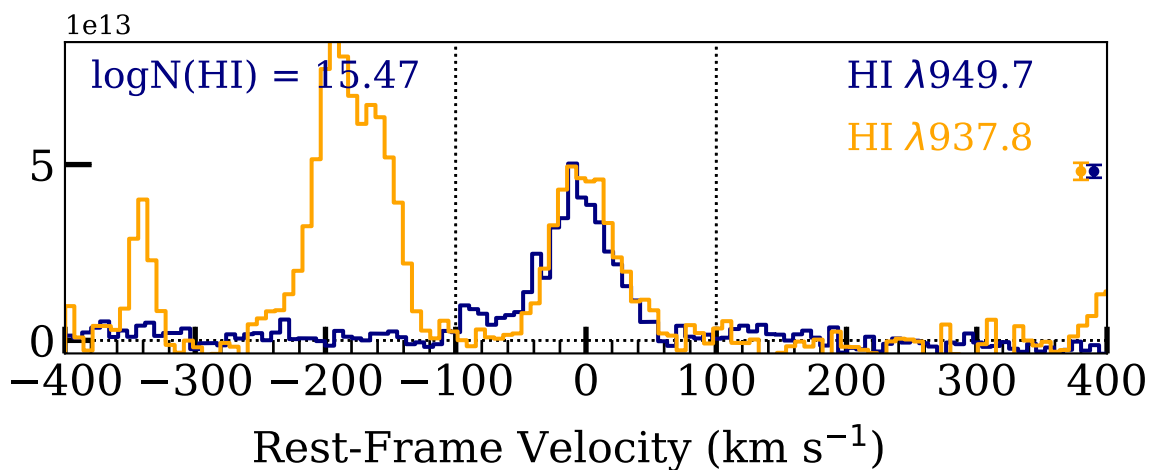

J150030.64+551708.8,  $z=0.347272$ , RF=1

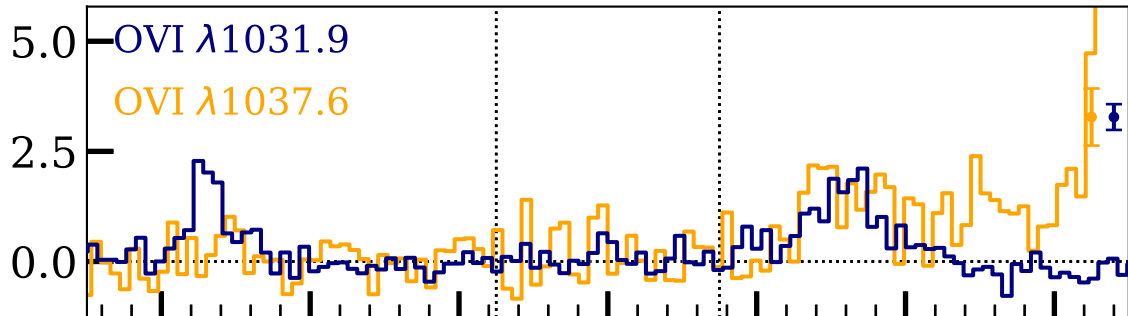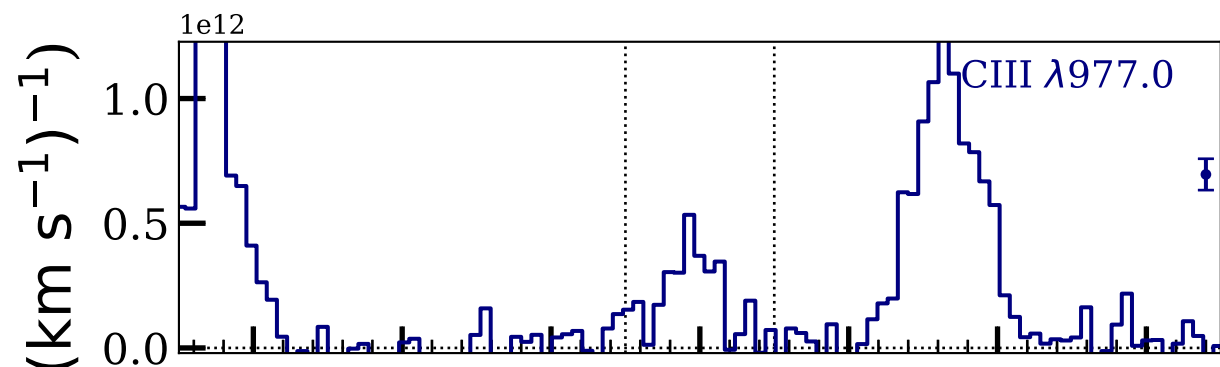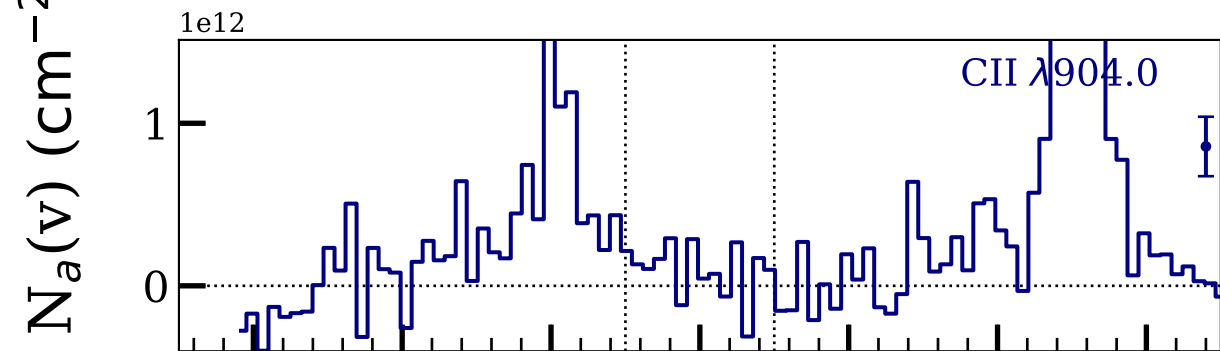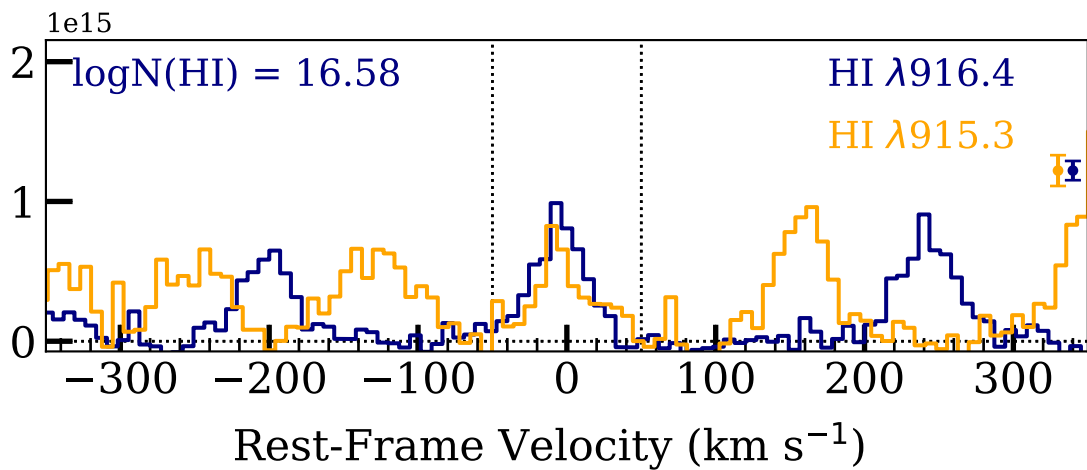



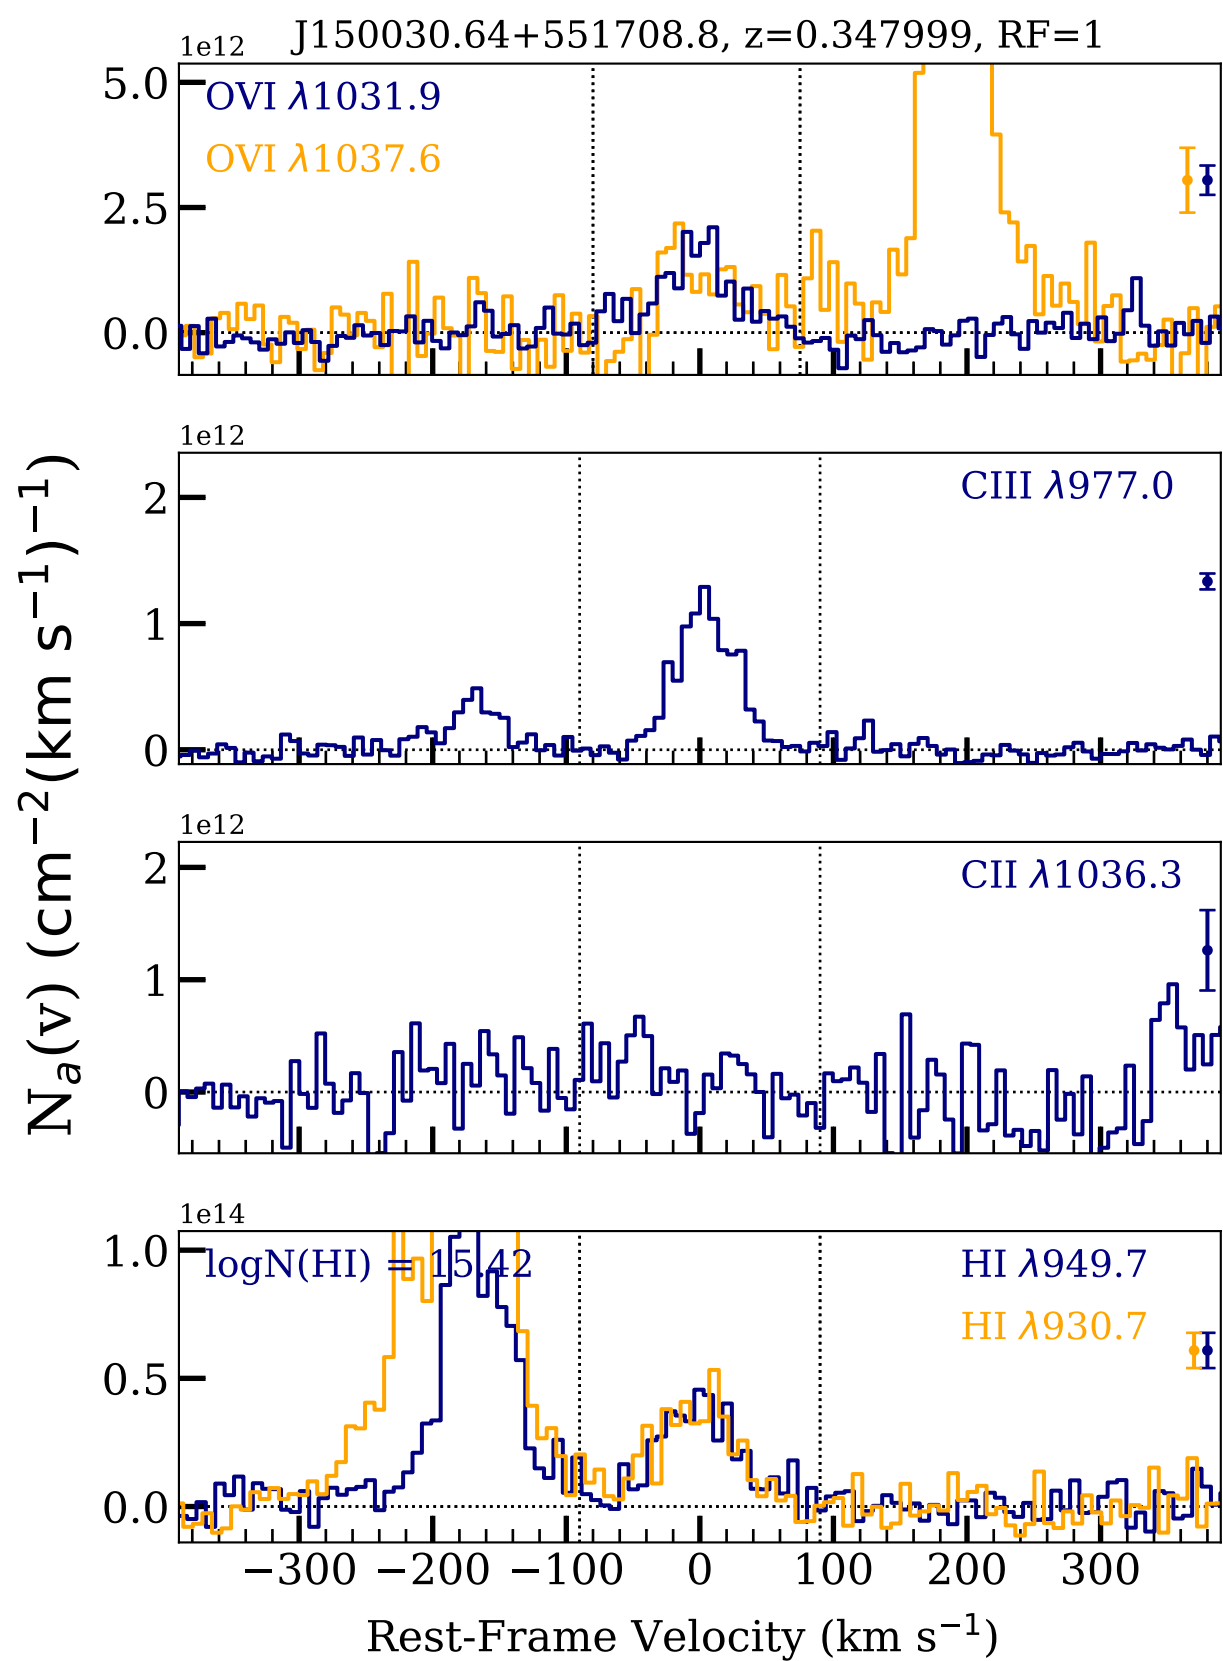

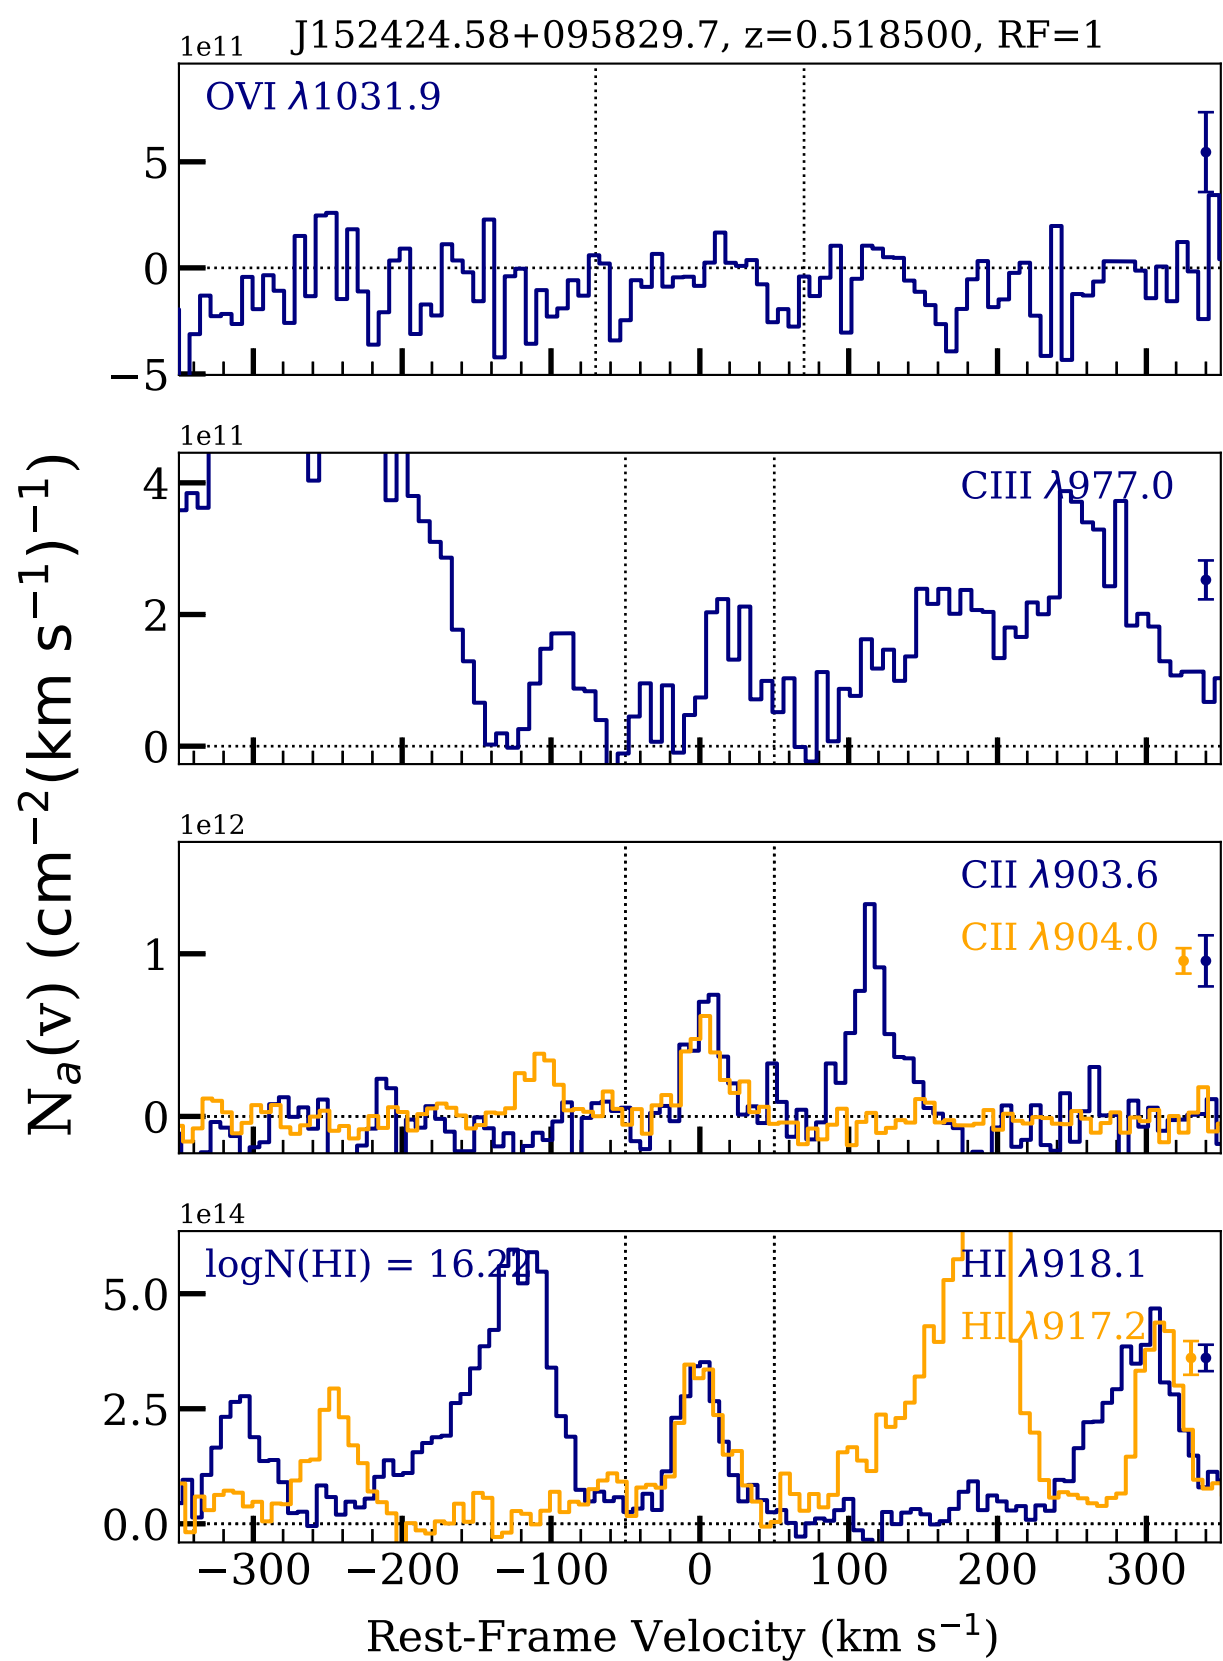

J152424.58+095829.7,  $z=0.571825$ , RF=1

$N_a(v)$  ( $\text{cm}^{-2}(\text{km s}^{-1})^{-1}$ )

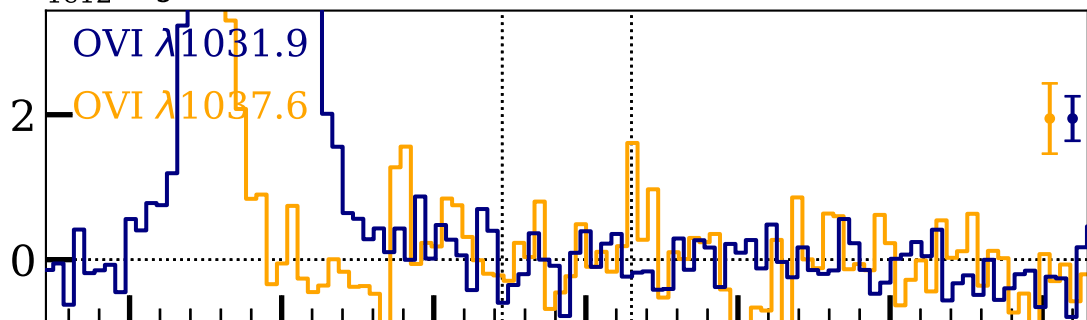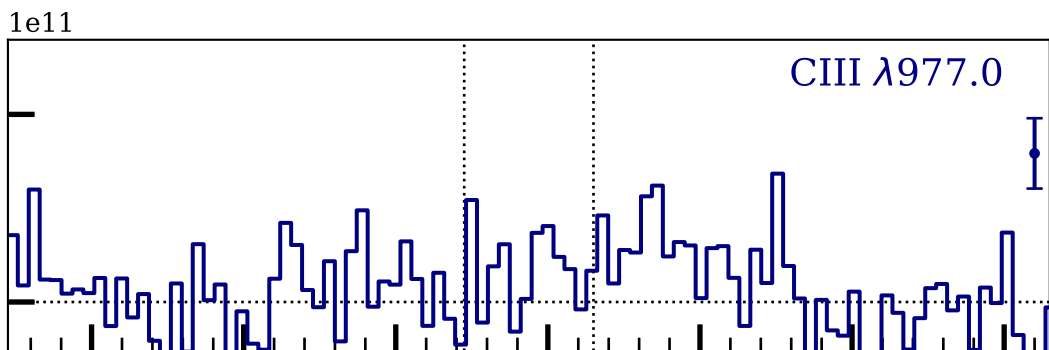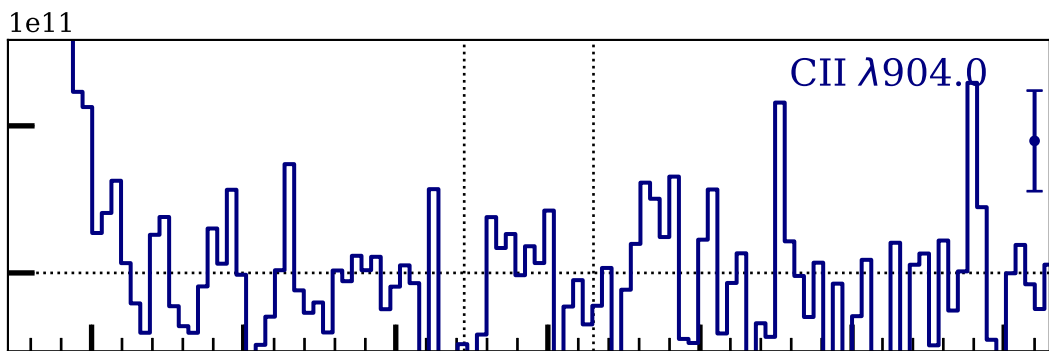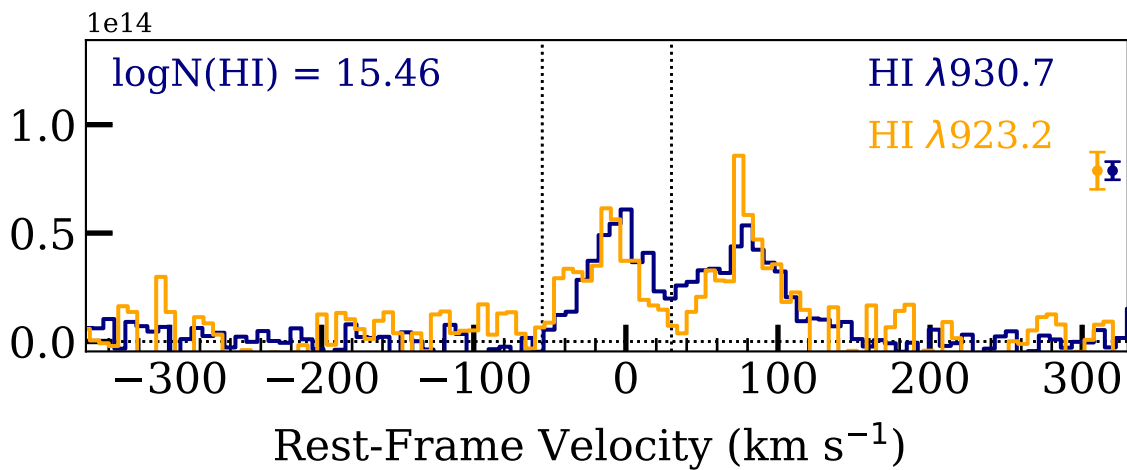

J152424.58+095829.7,  $z=0.675378$ , RF=1

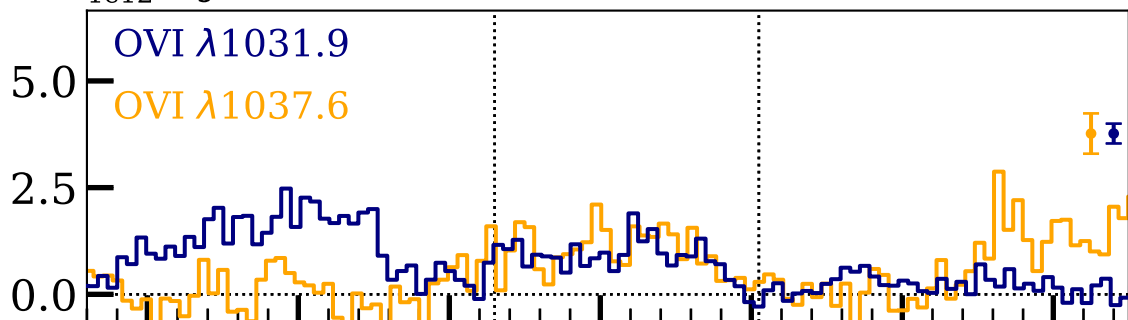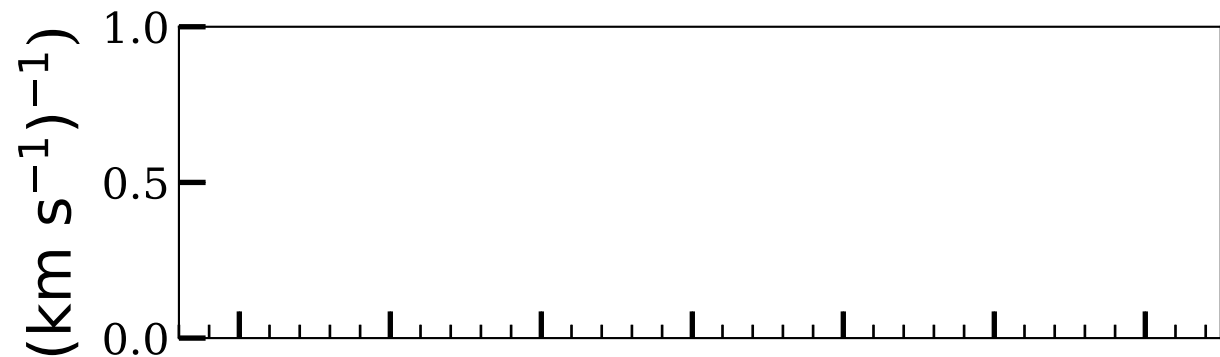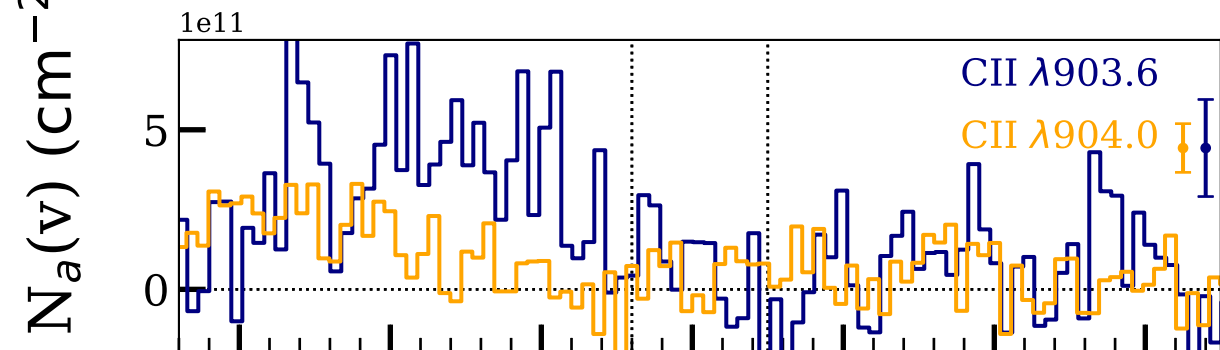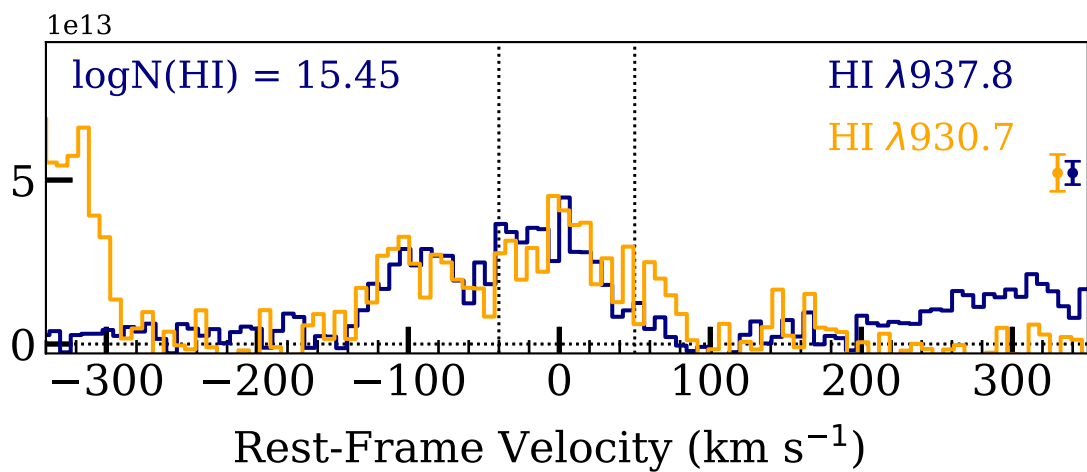

J152424.58+095829.7,  $z=0.728885$ , RF=1

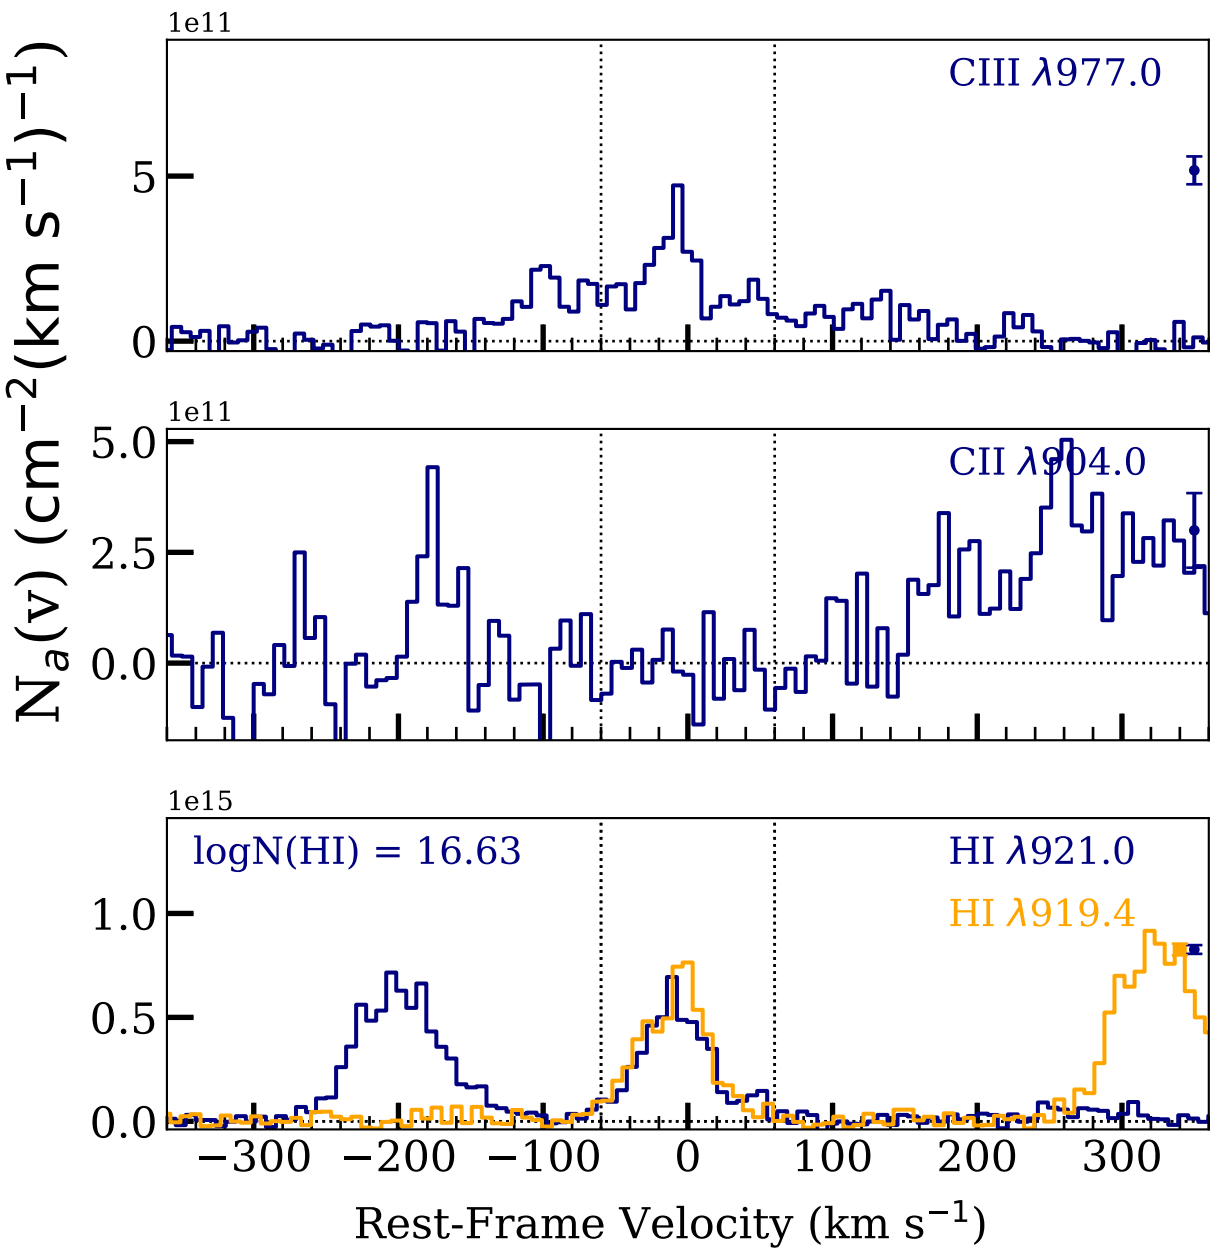

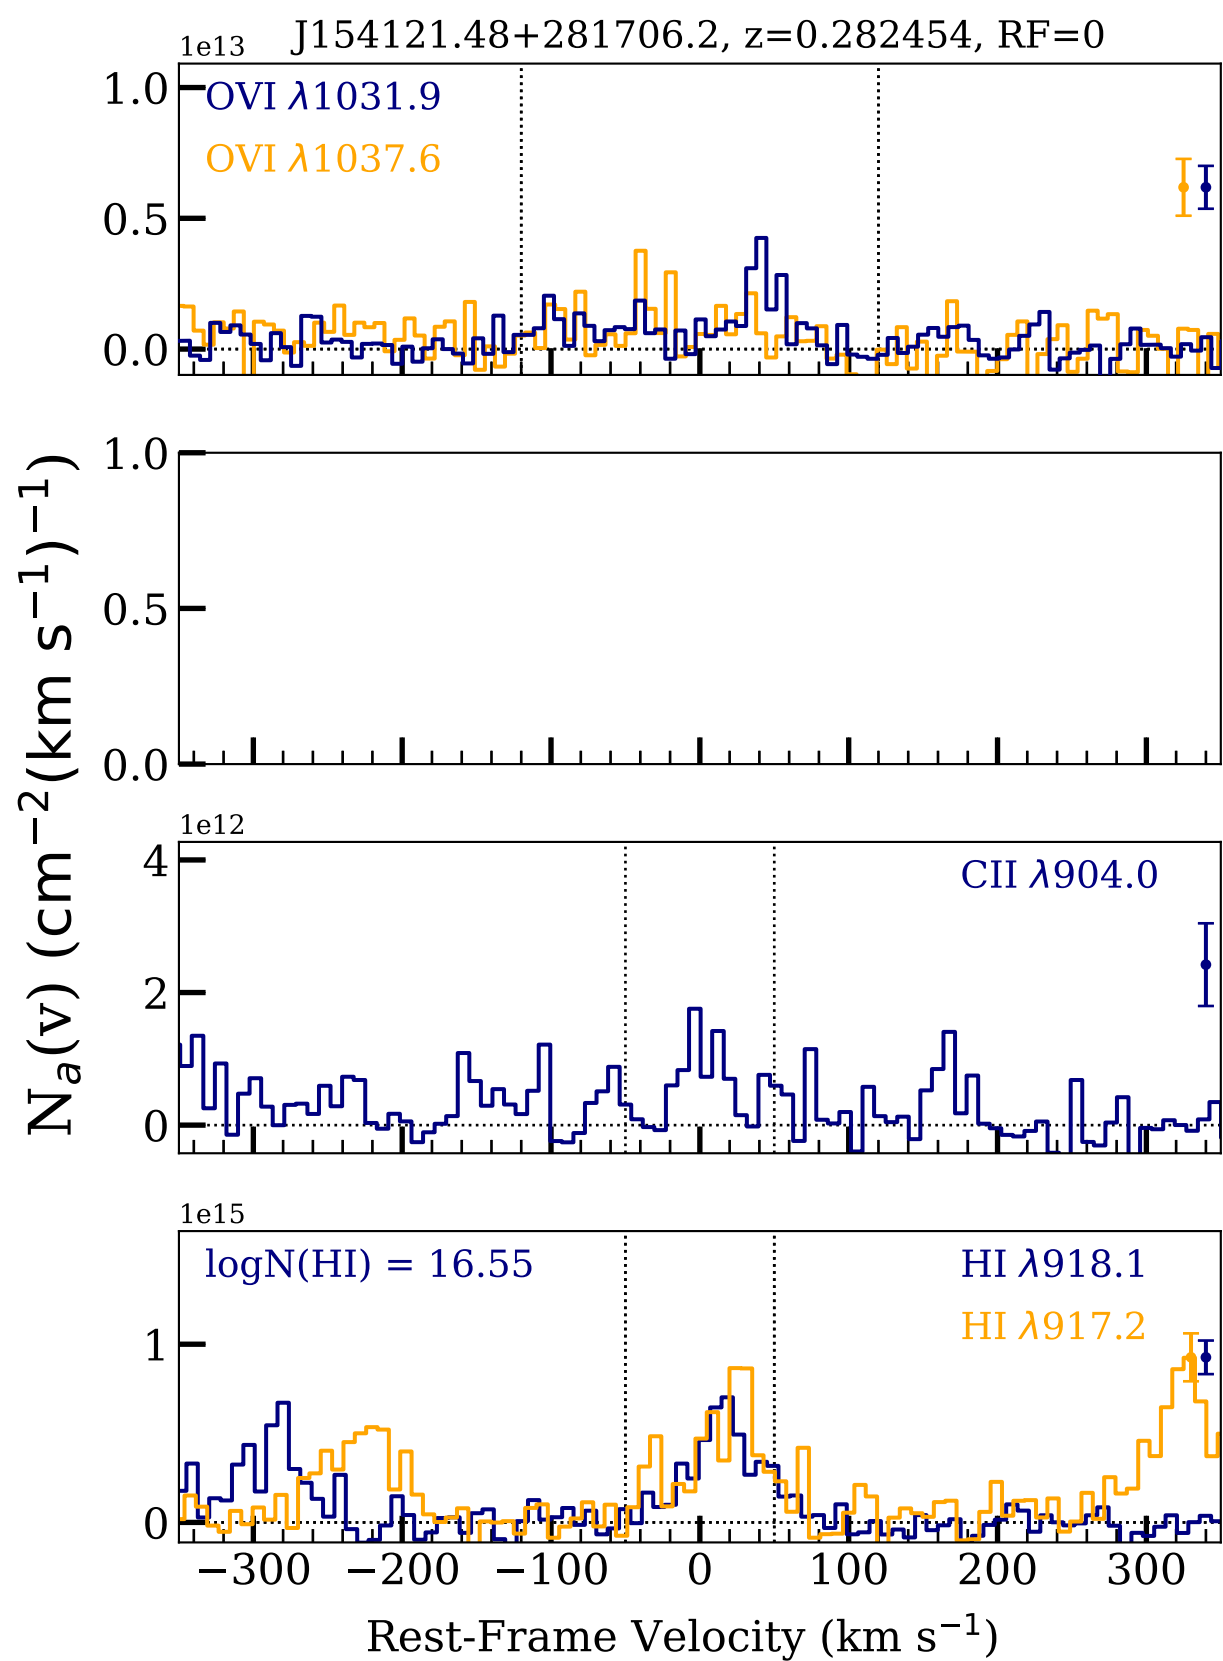

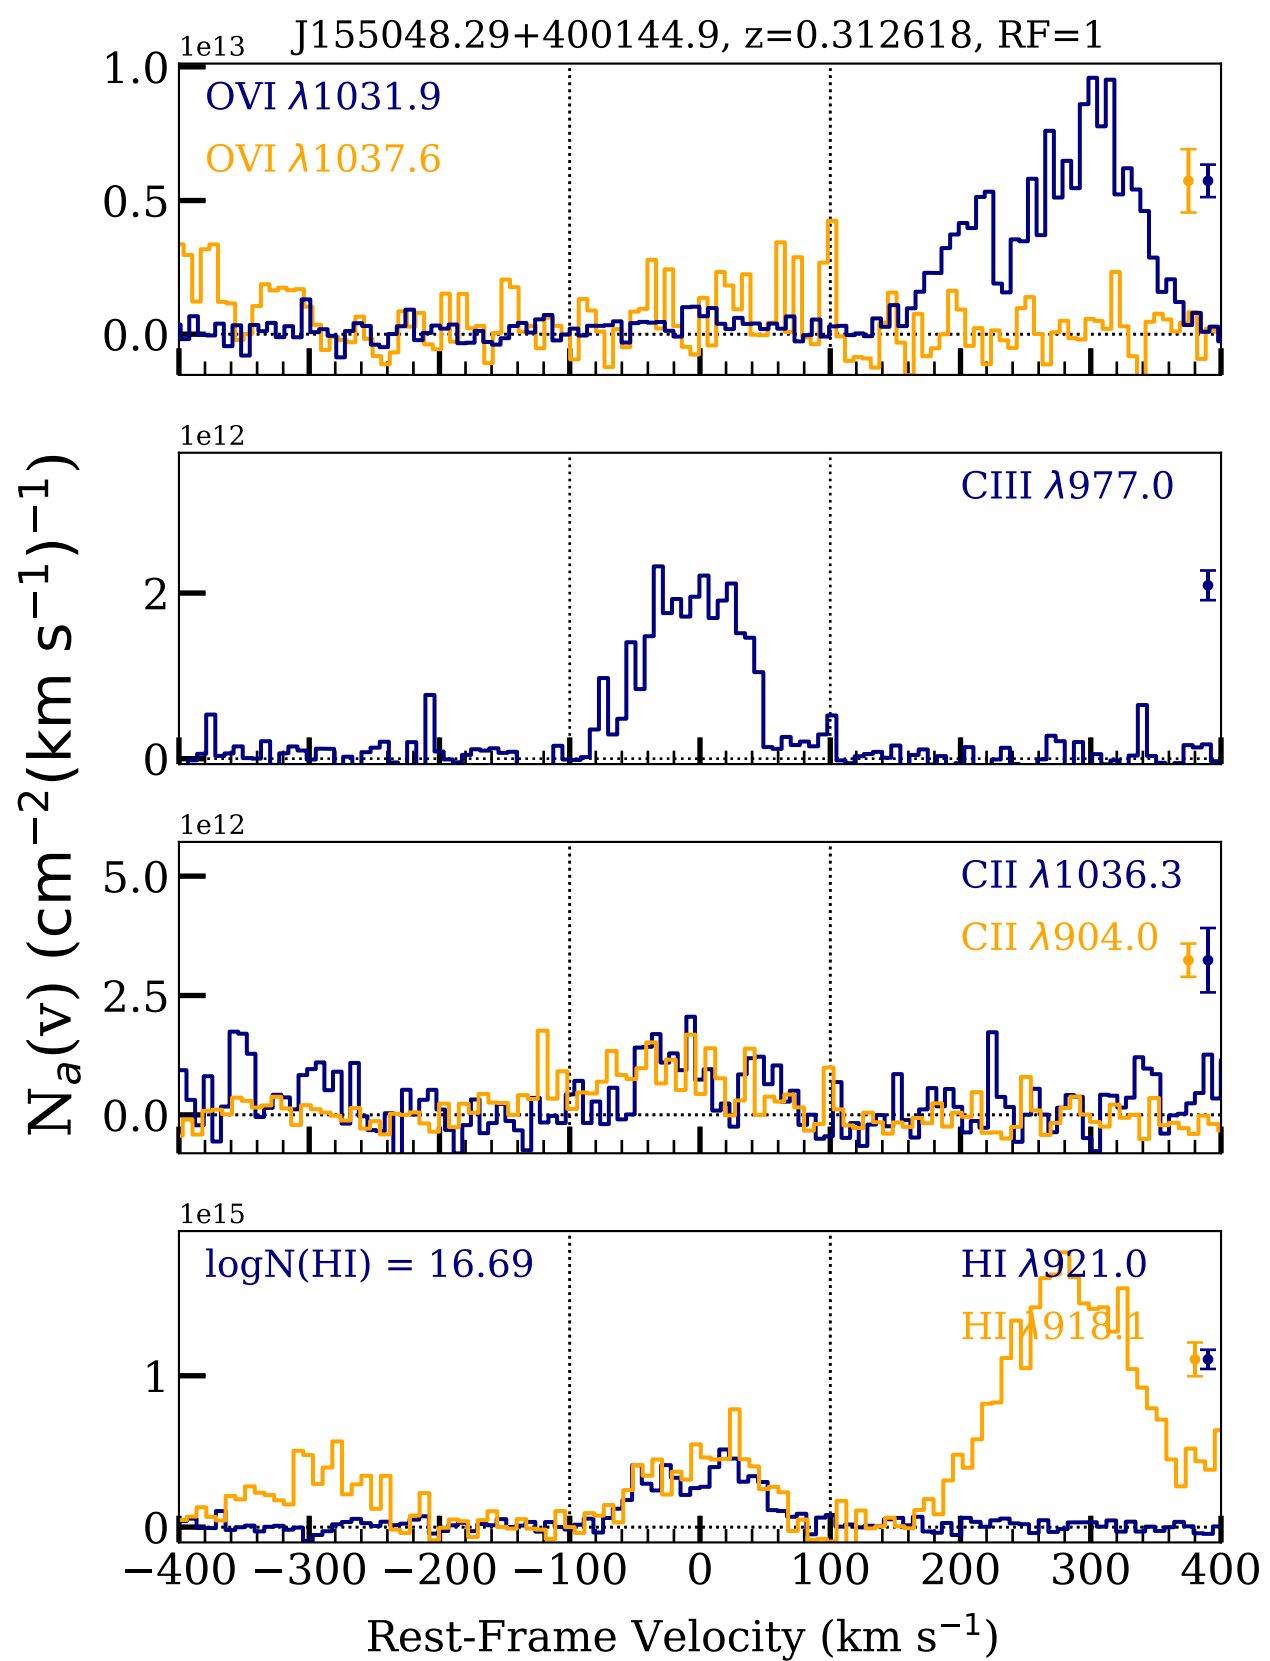

J155048.29+400144.9,  $z=0.427306$ , RF=1

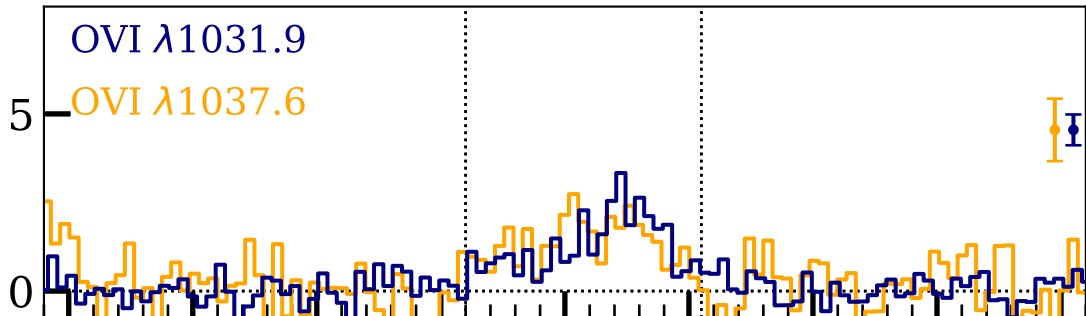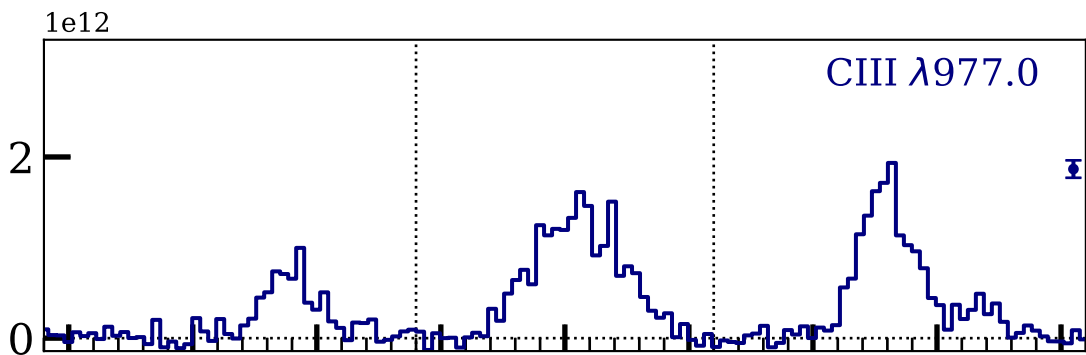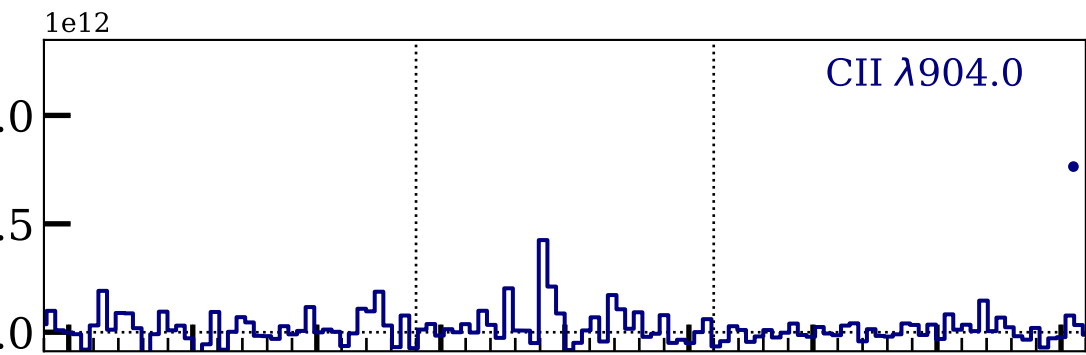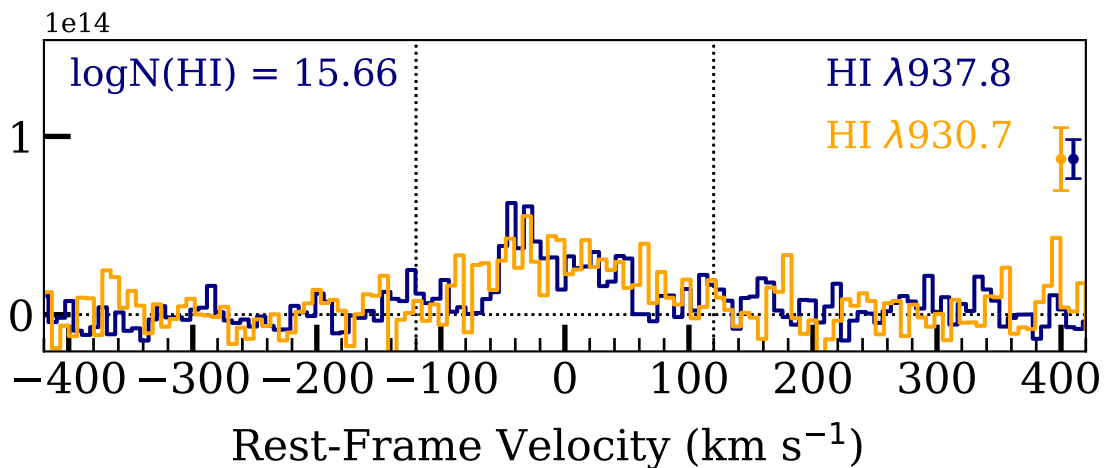



J155048.29+400144.9,  $z=0.491977$ , RF=1

$N_a(v)$  ( $\text{cm}^{-2}(\text{km s}^{-1})^{-1}$ )

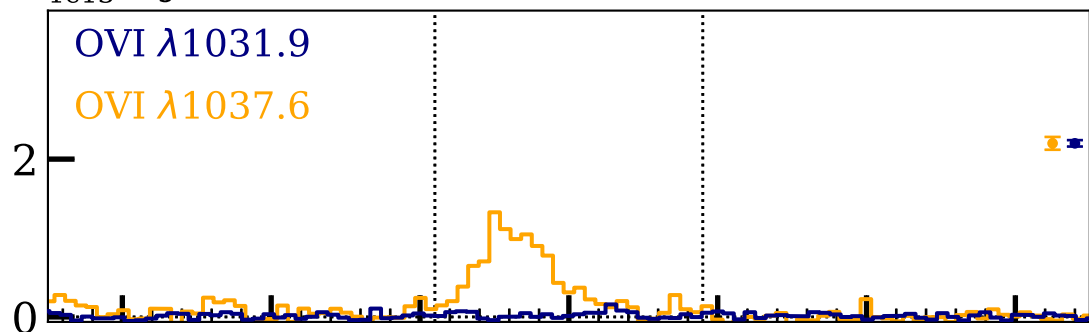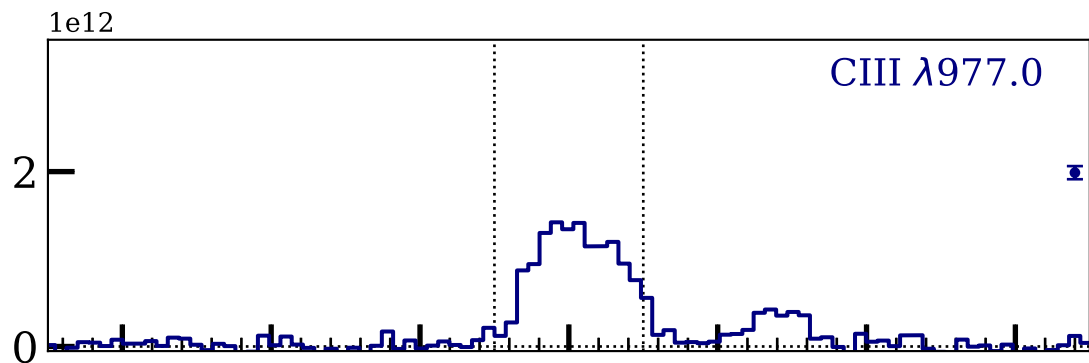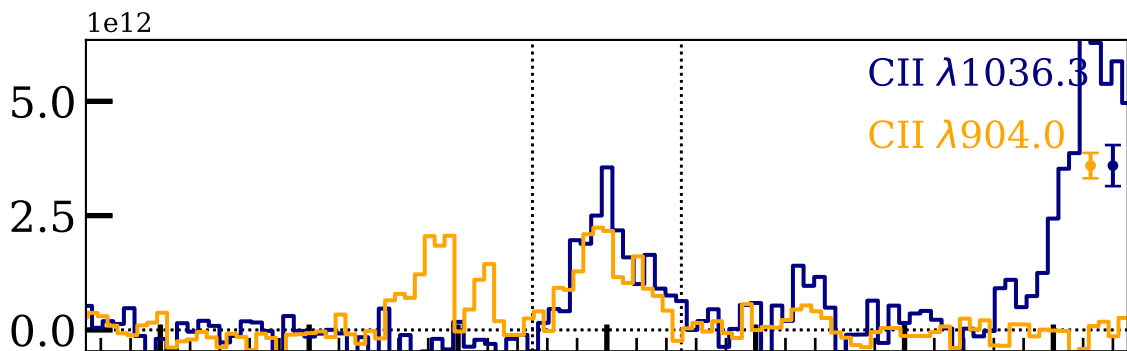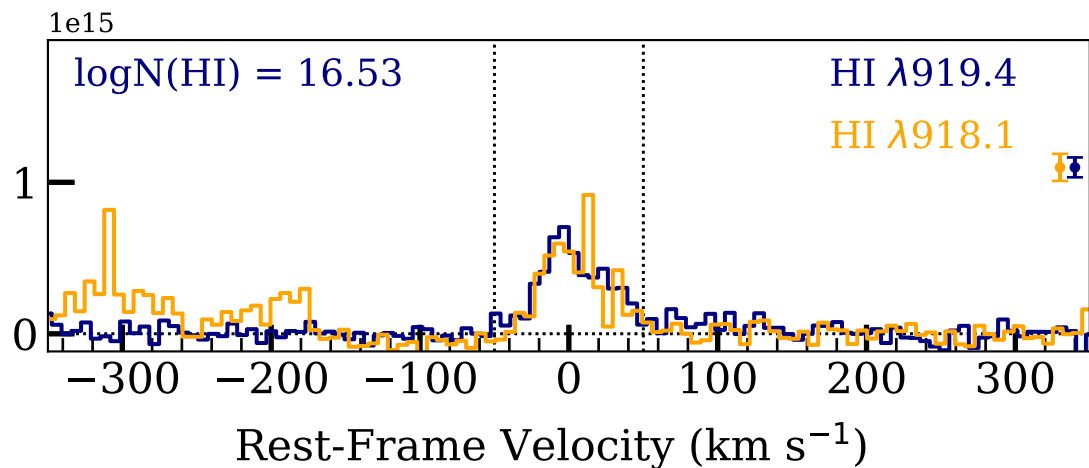

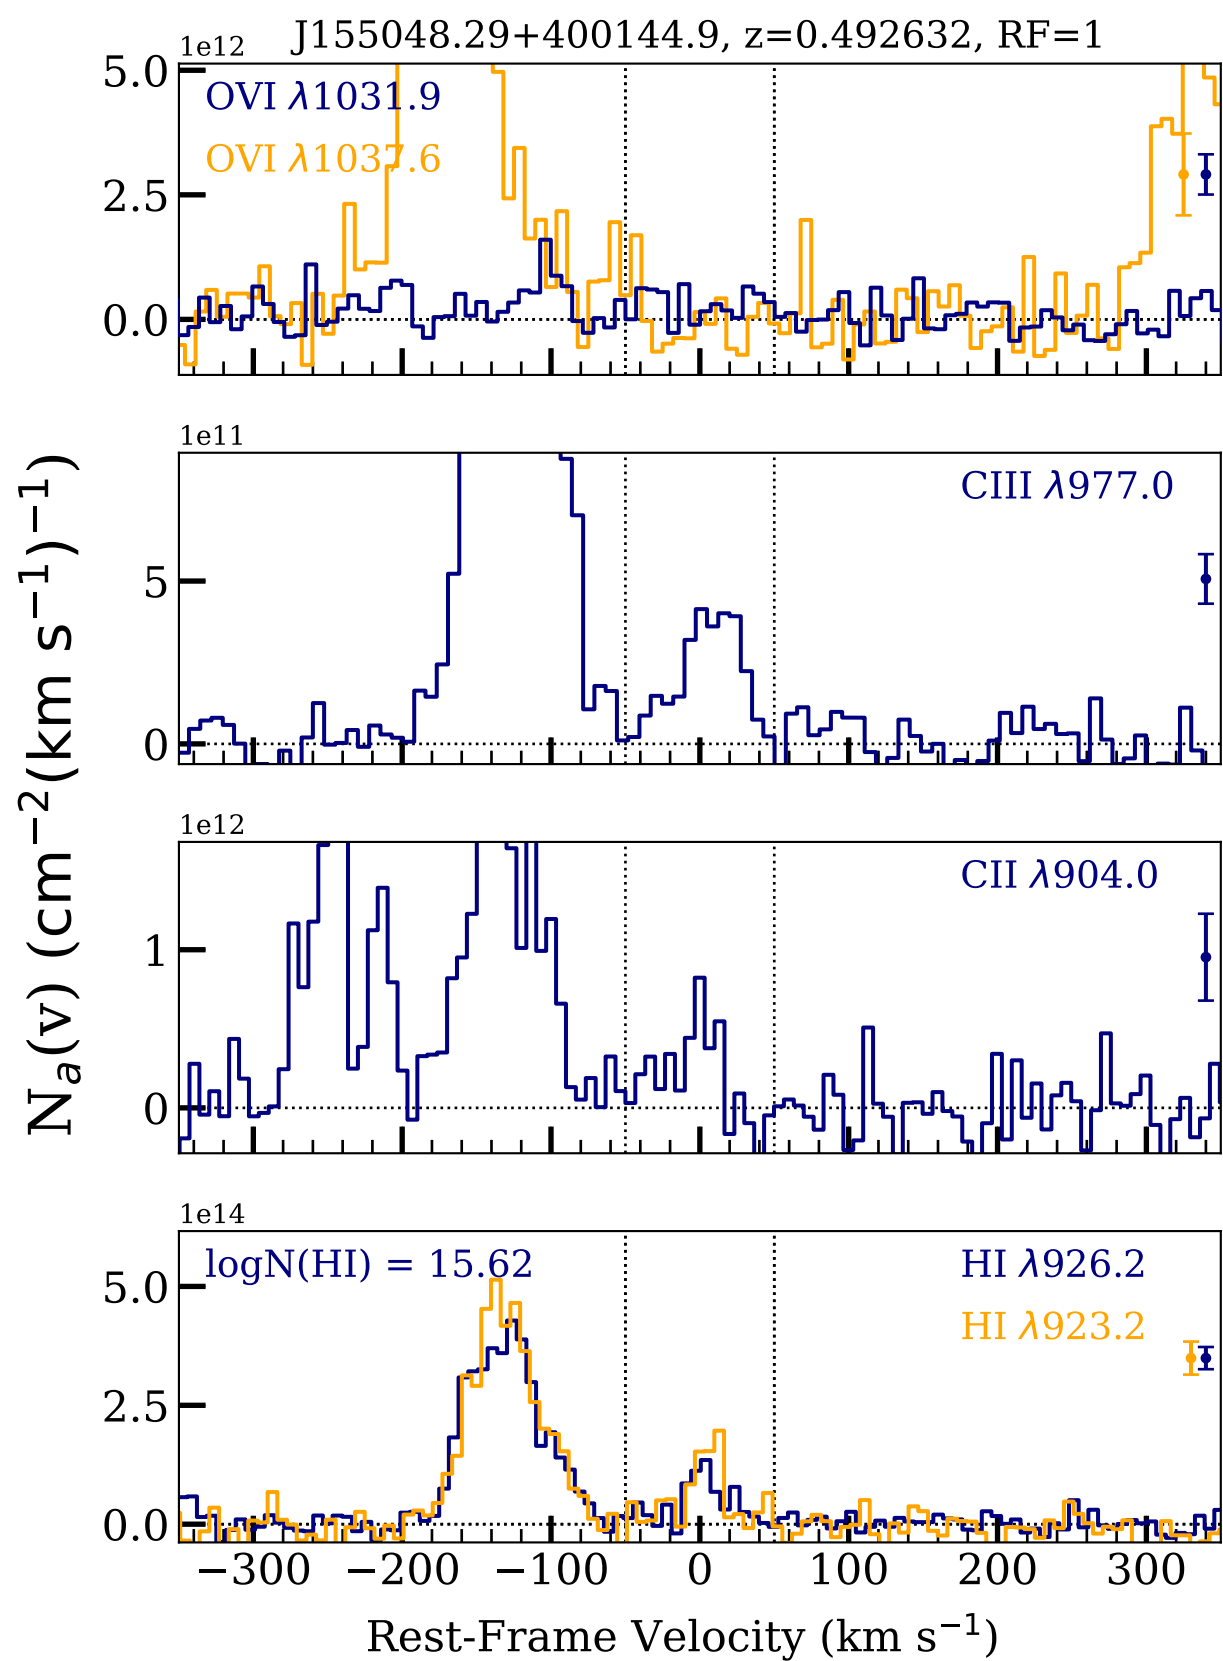

1e12 J155232.54+570516.5, z=0.366020, RF=1

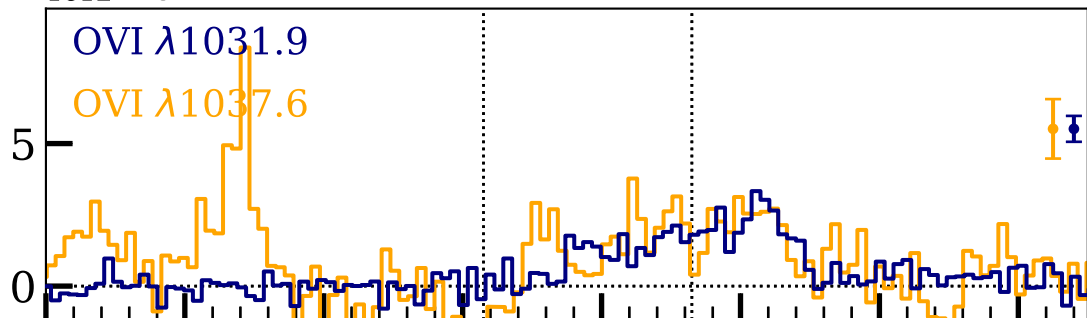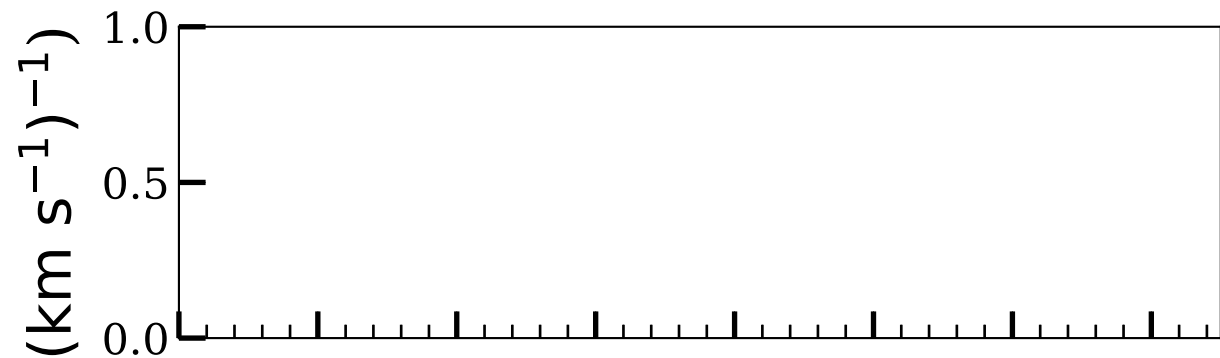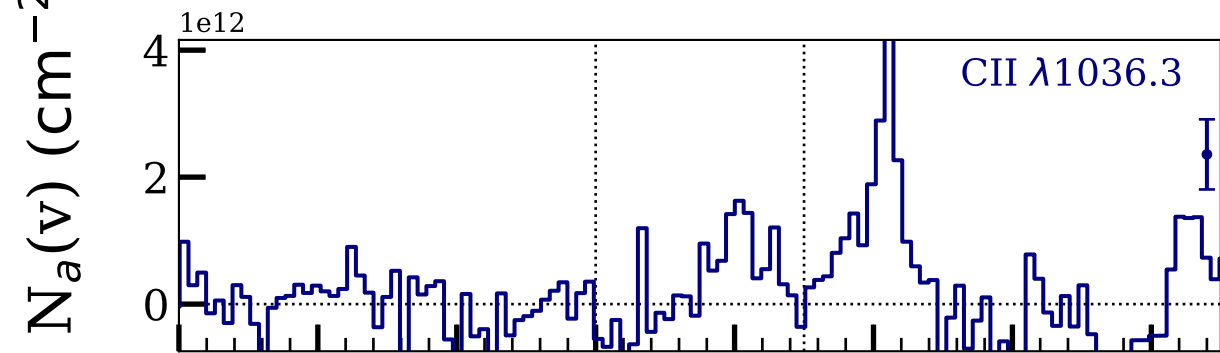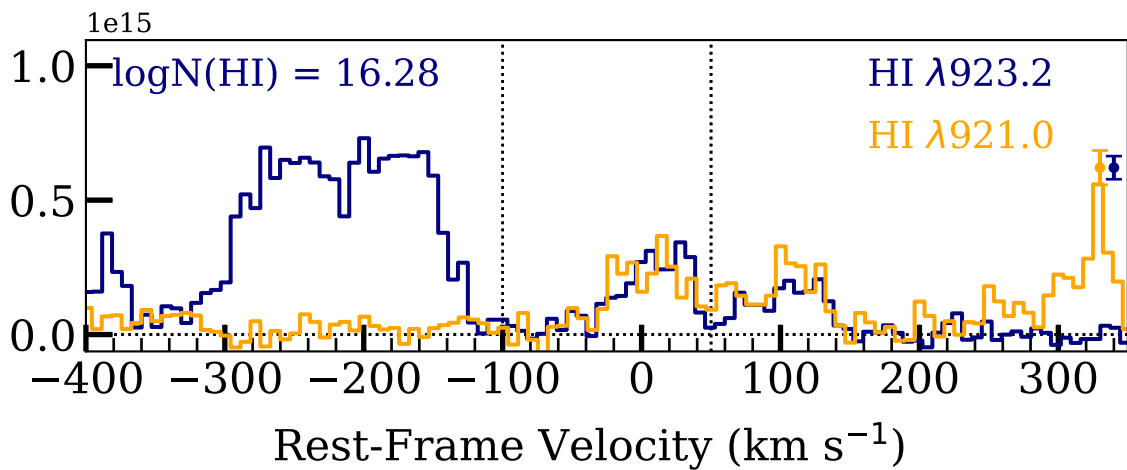

J155232.54+570516.5,  $z=0.366521$ , RF=1

$N_a(v)$  ( $\text{cm}^{-2}(\text{km s}^{-1})^{-1}$ )

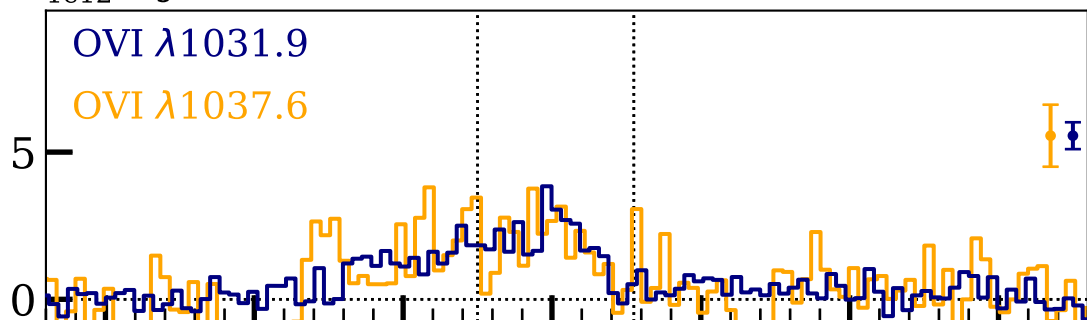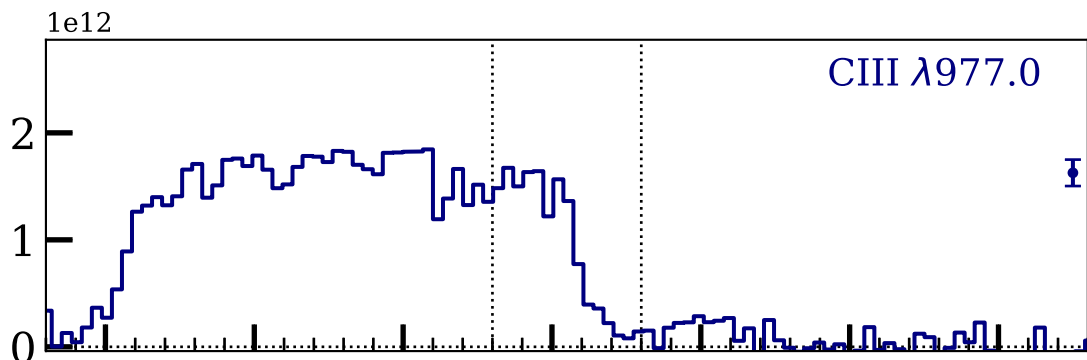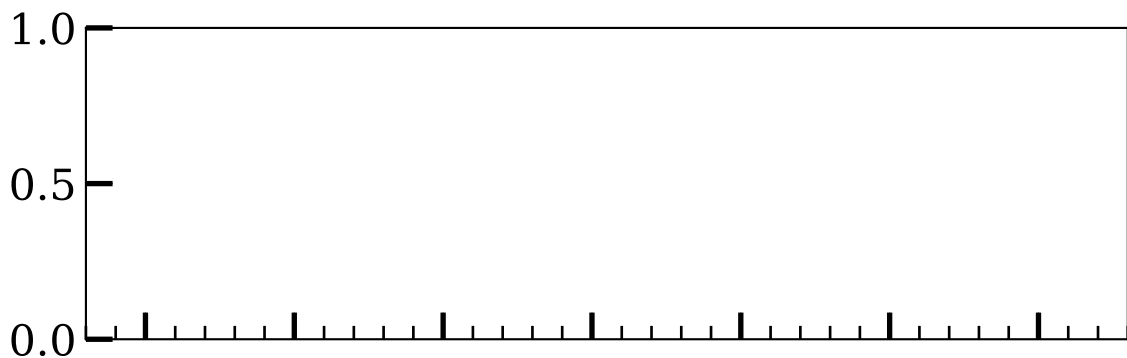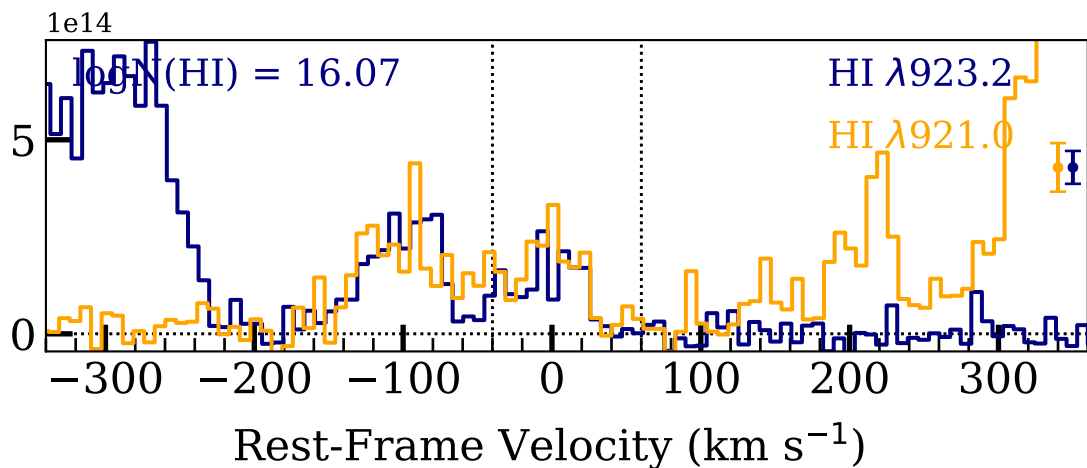

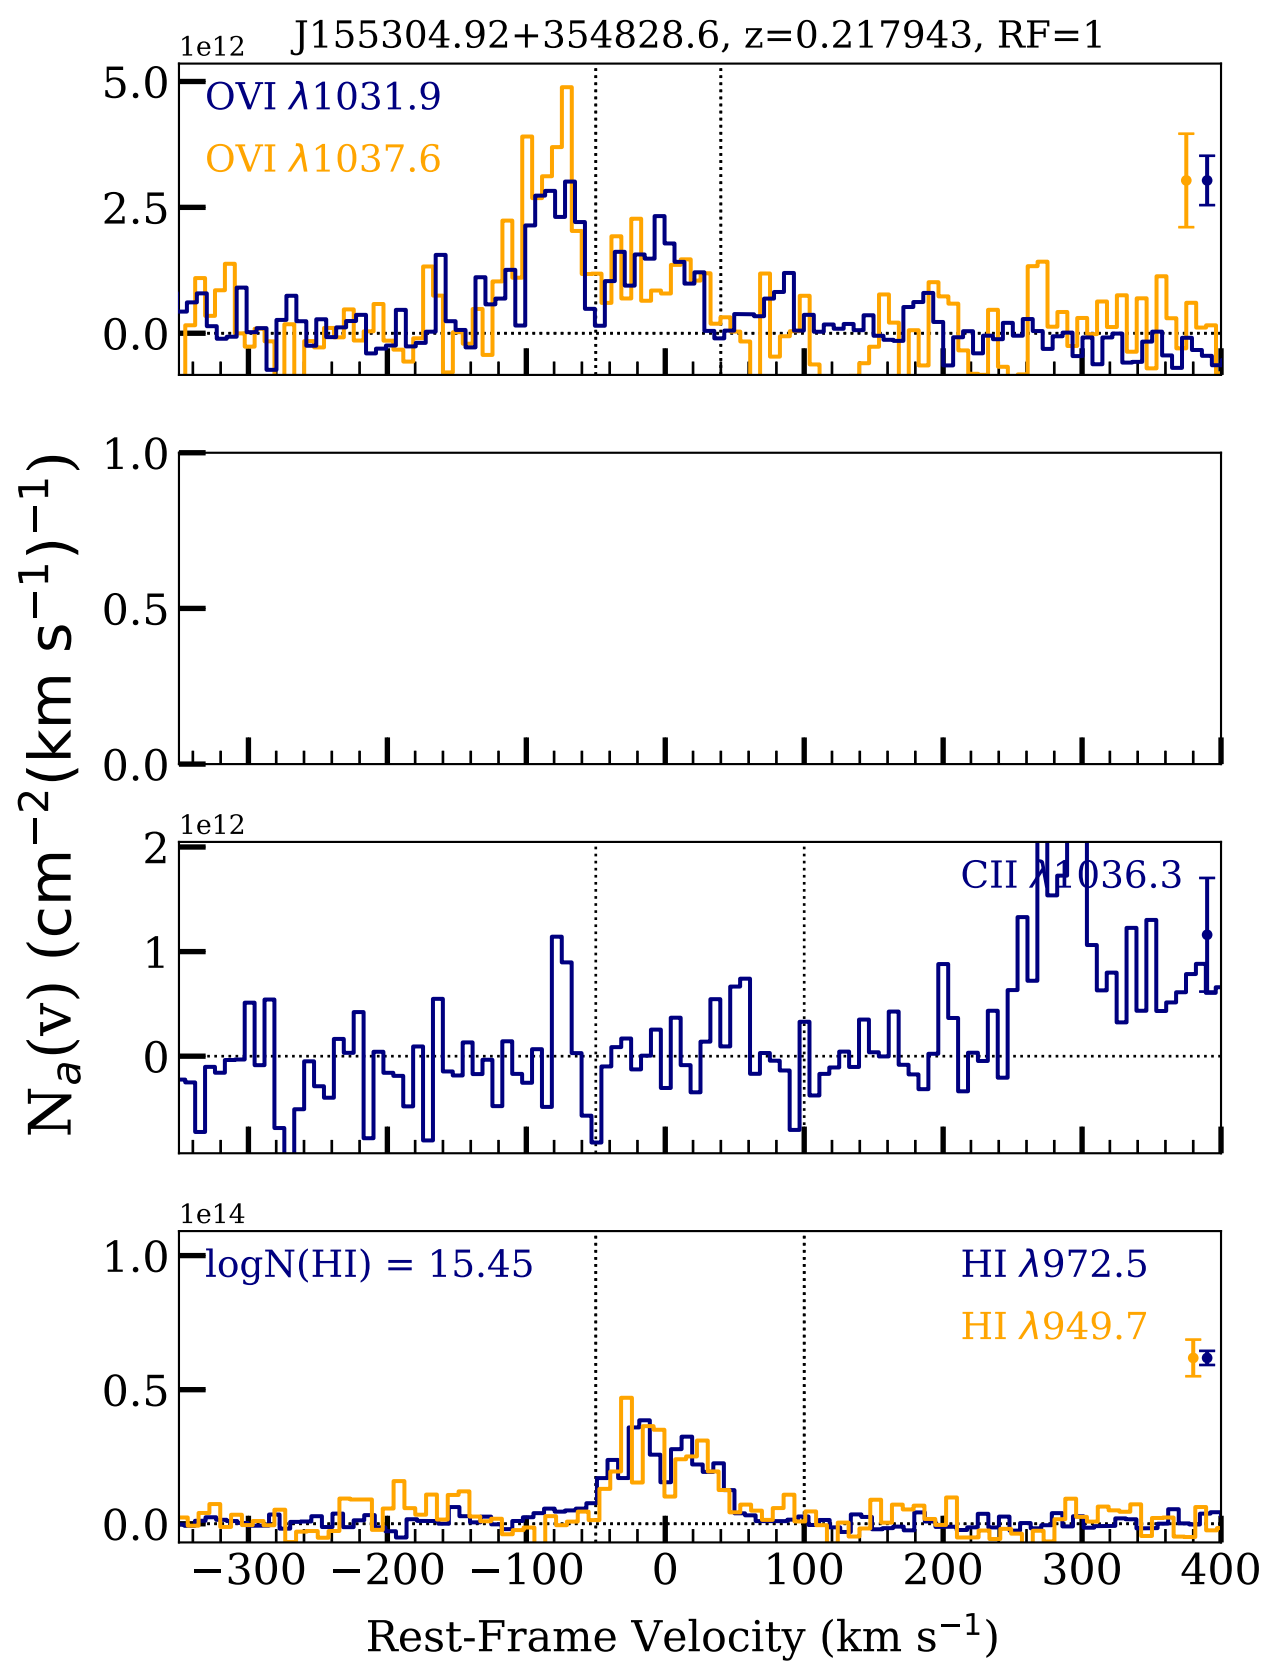

J155304.92+354828.6,  $z=0.475466$ , RF=1

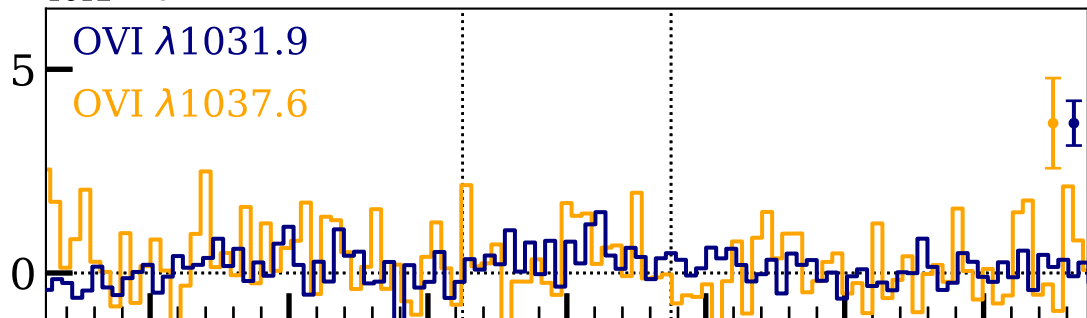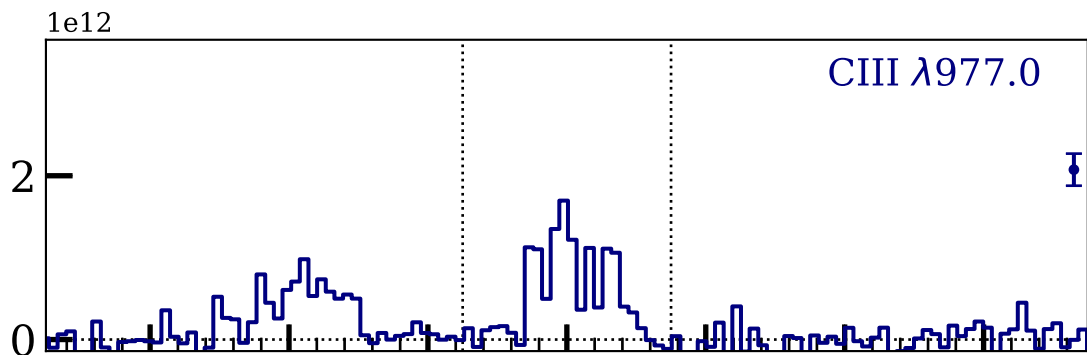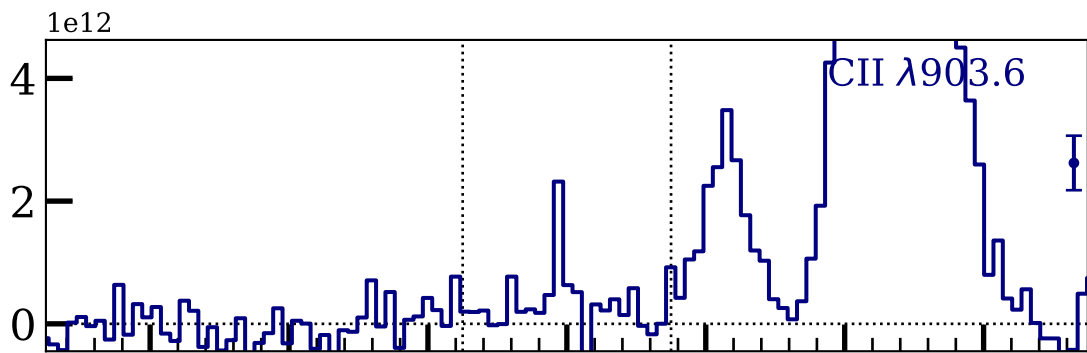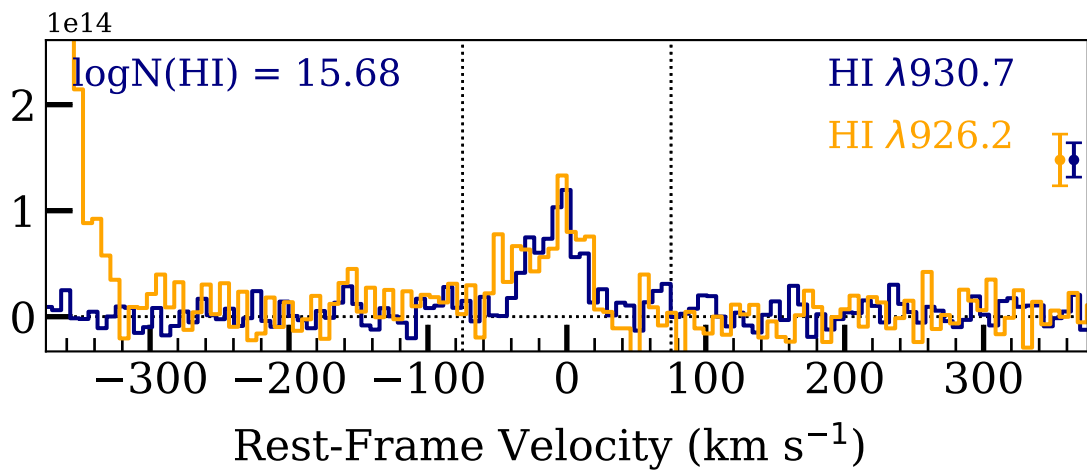

J155504.39+362848.0,  $z=0.576033$ , RF=0

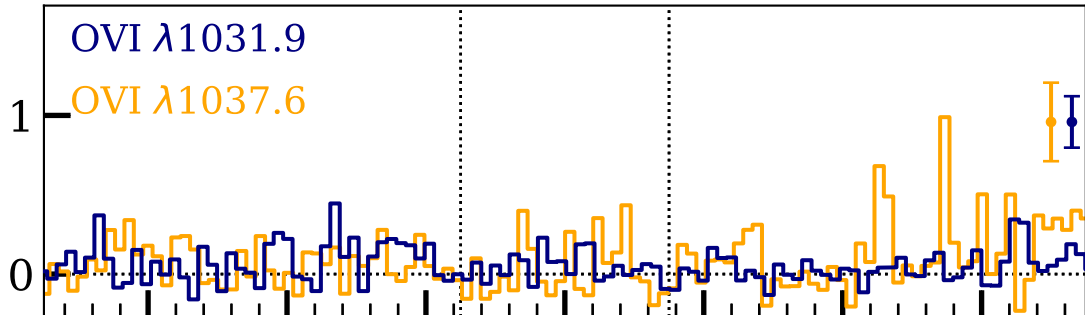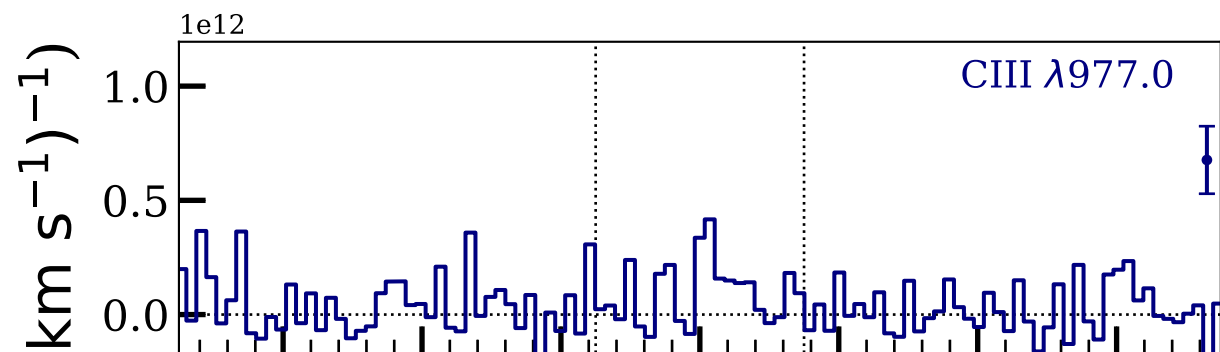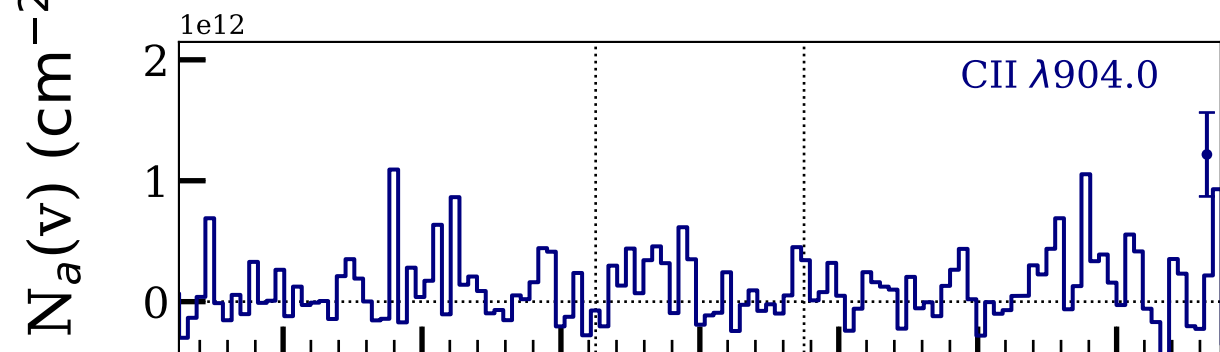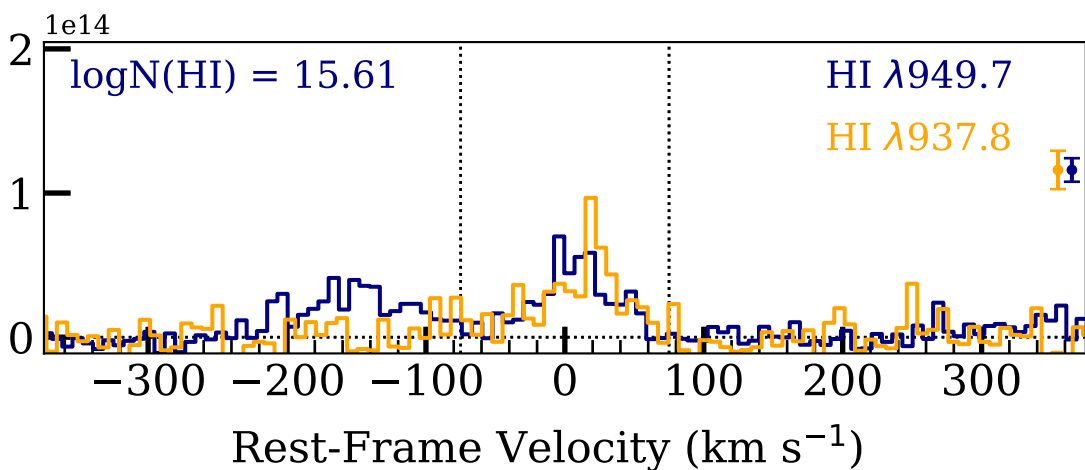

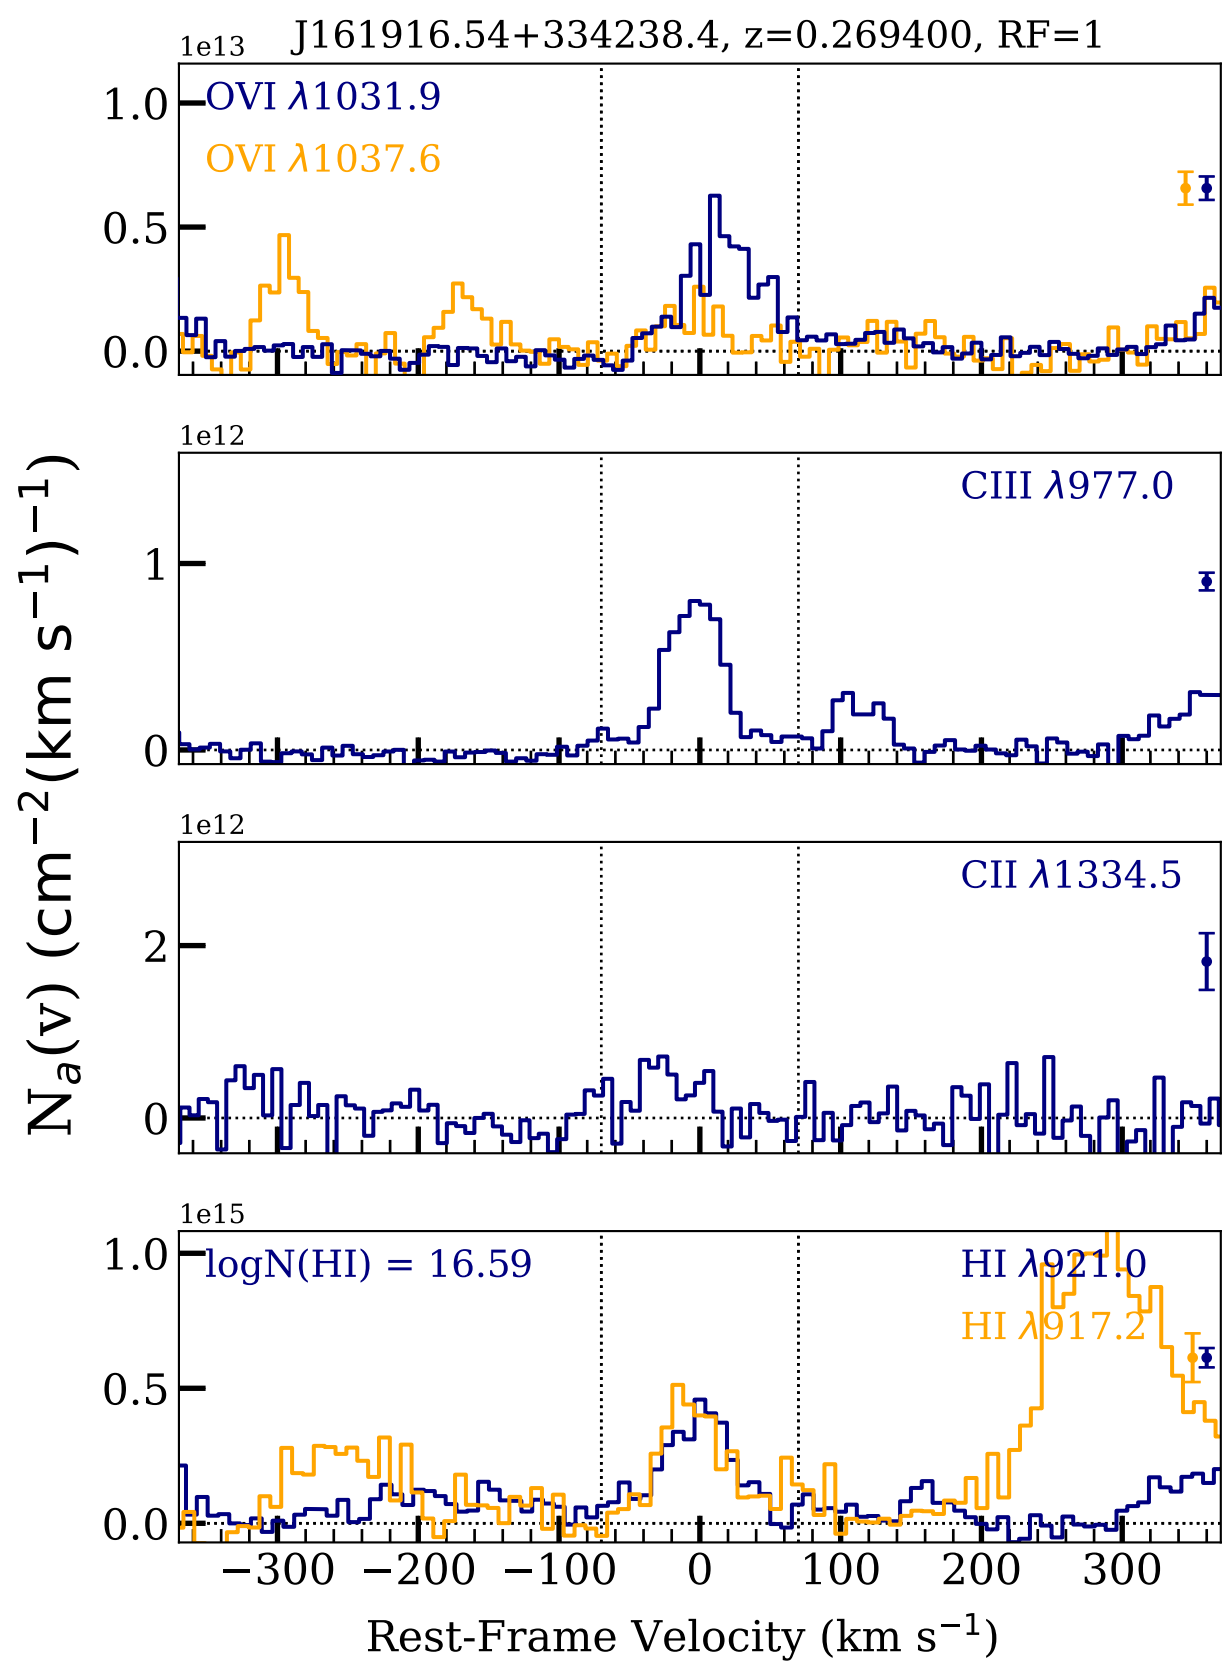



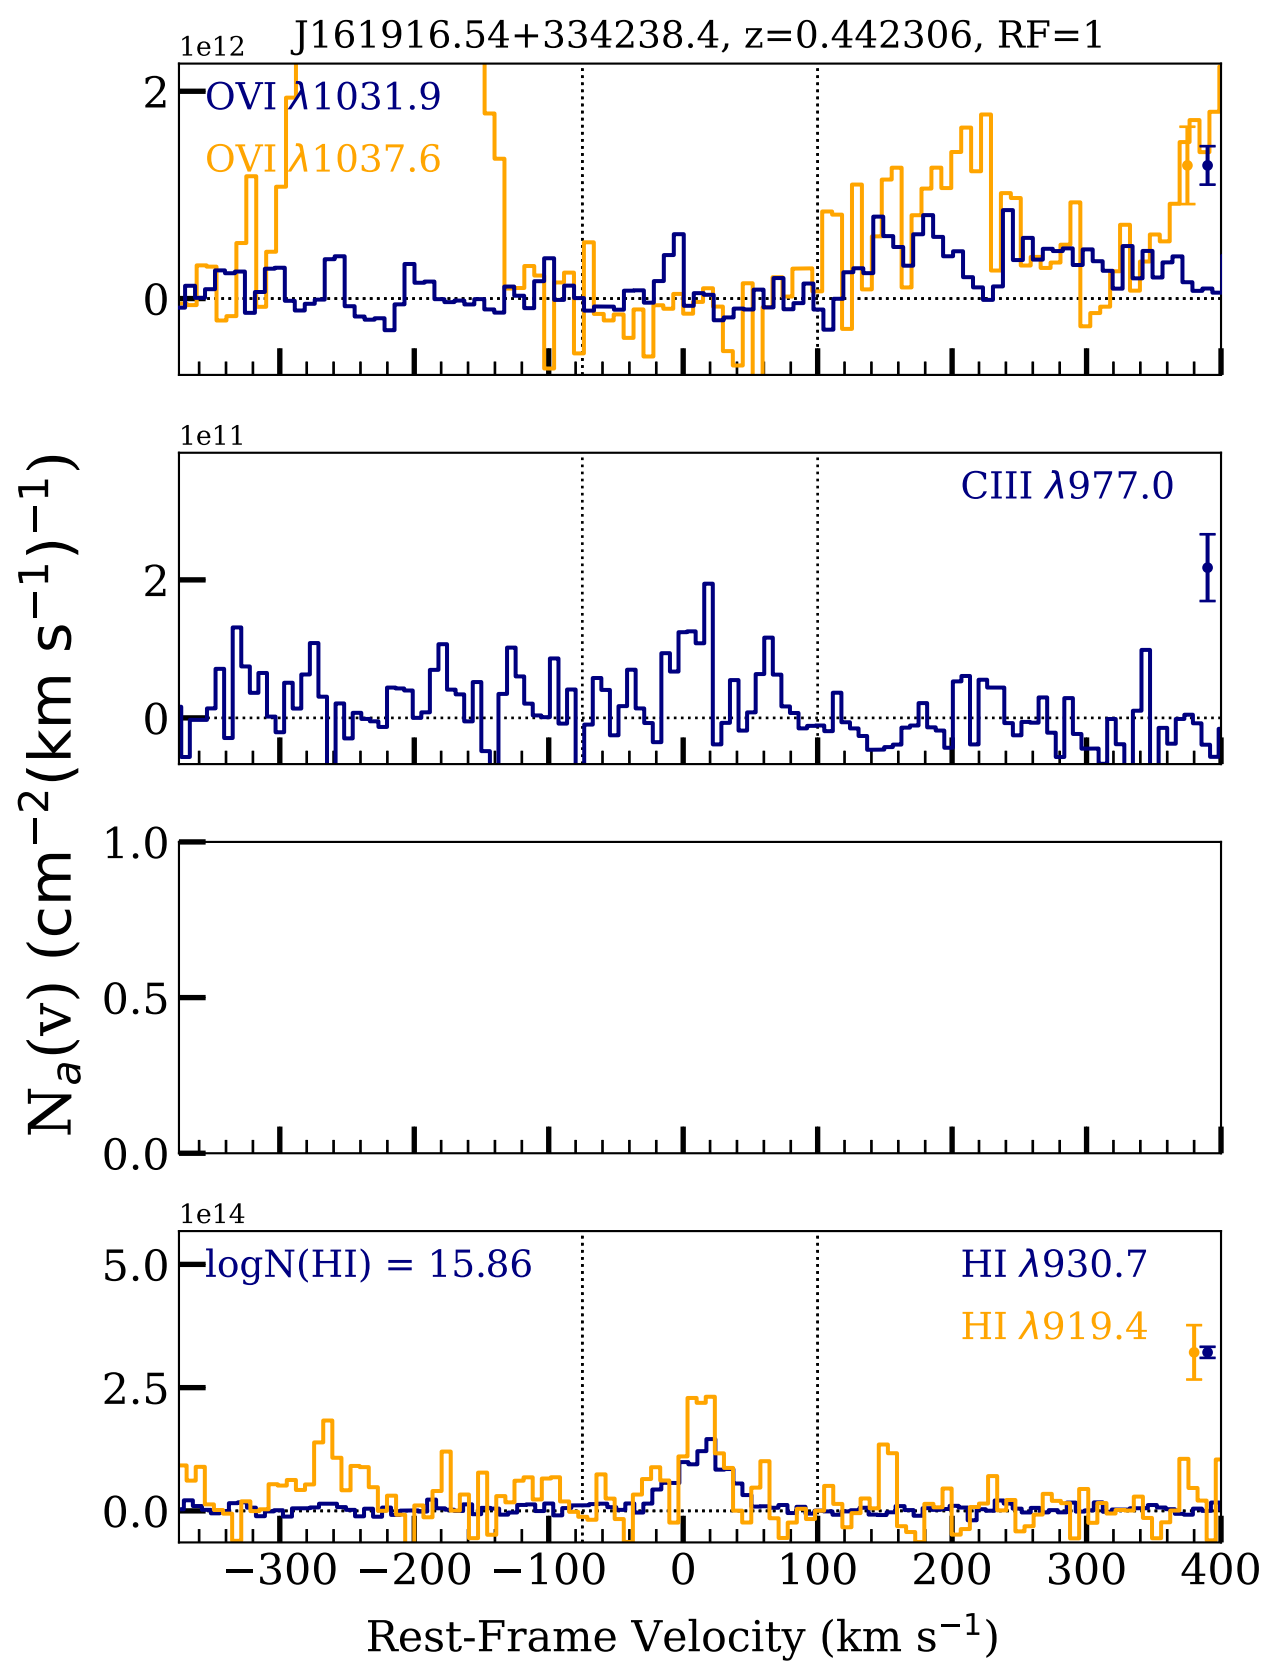

J163201.12+373749.9,  $z=0.273950$ , RF=1

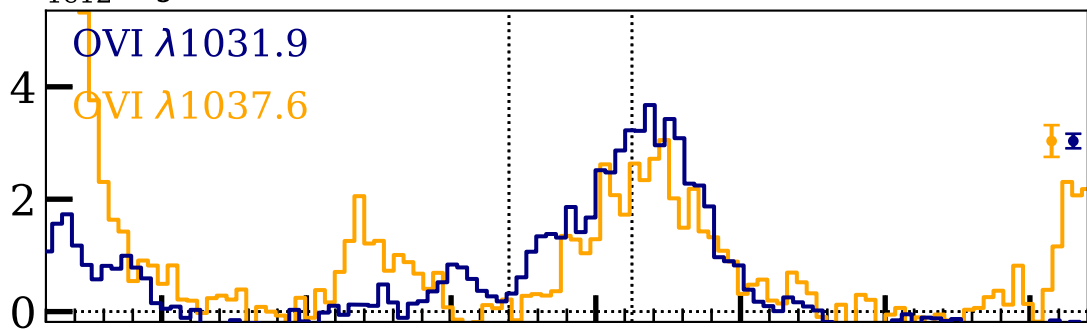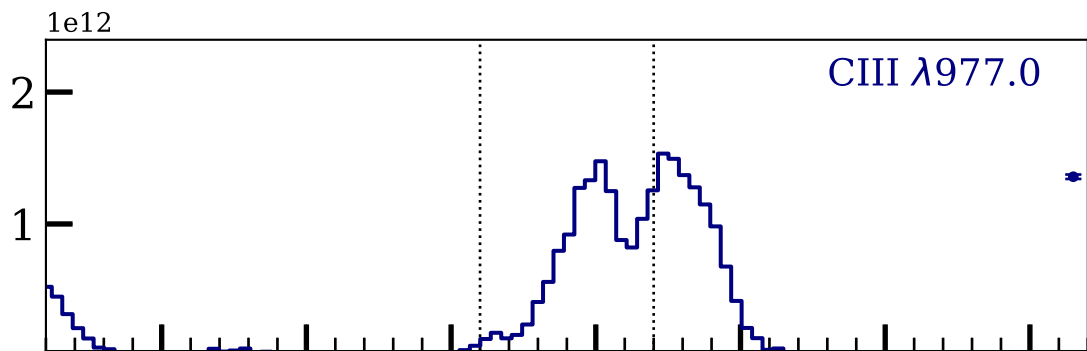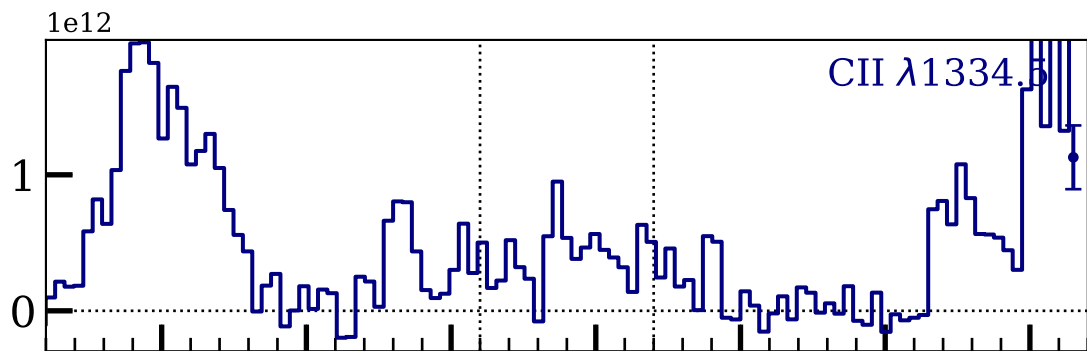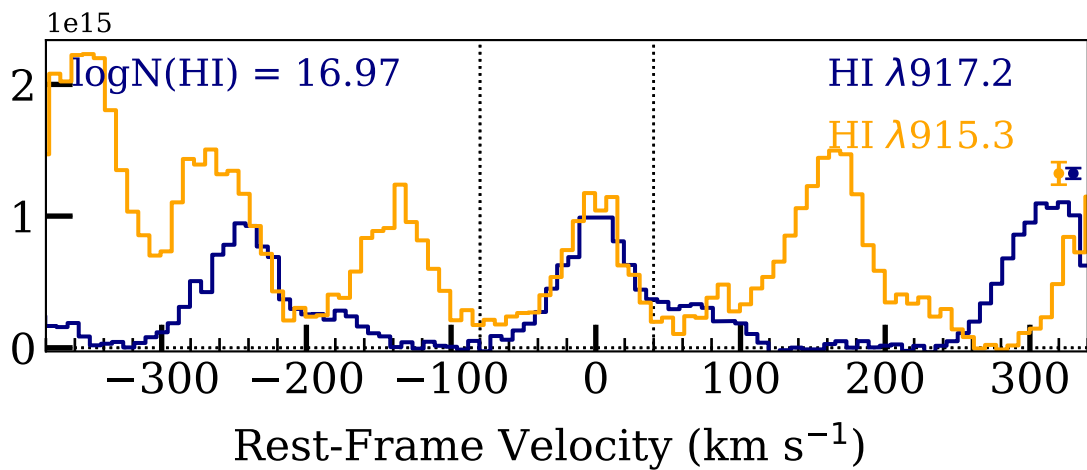

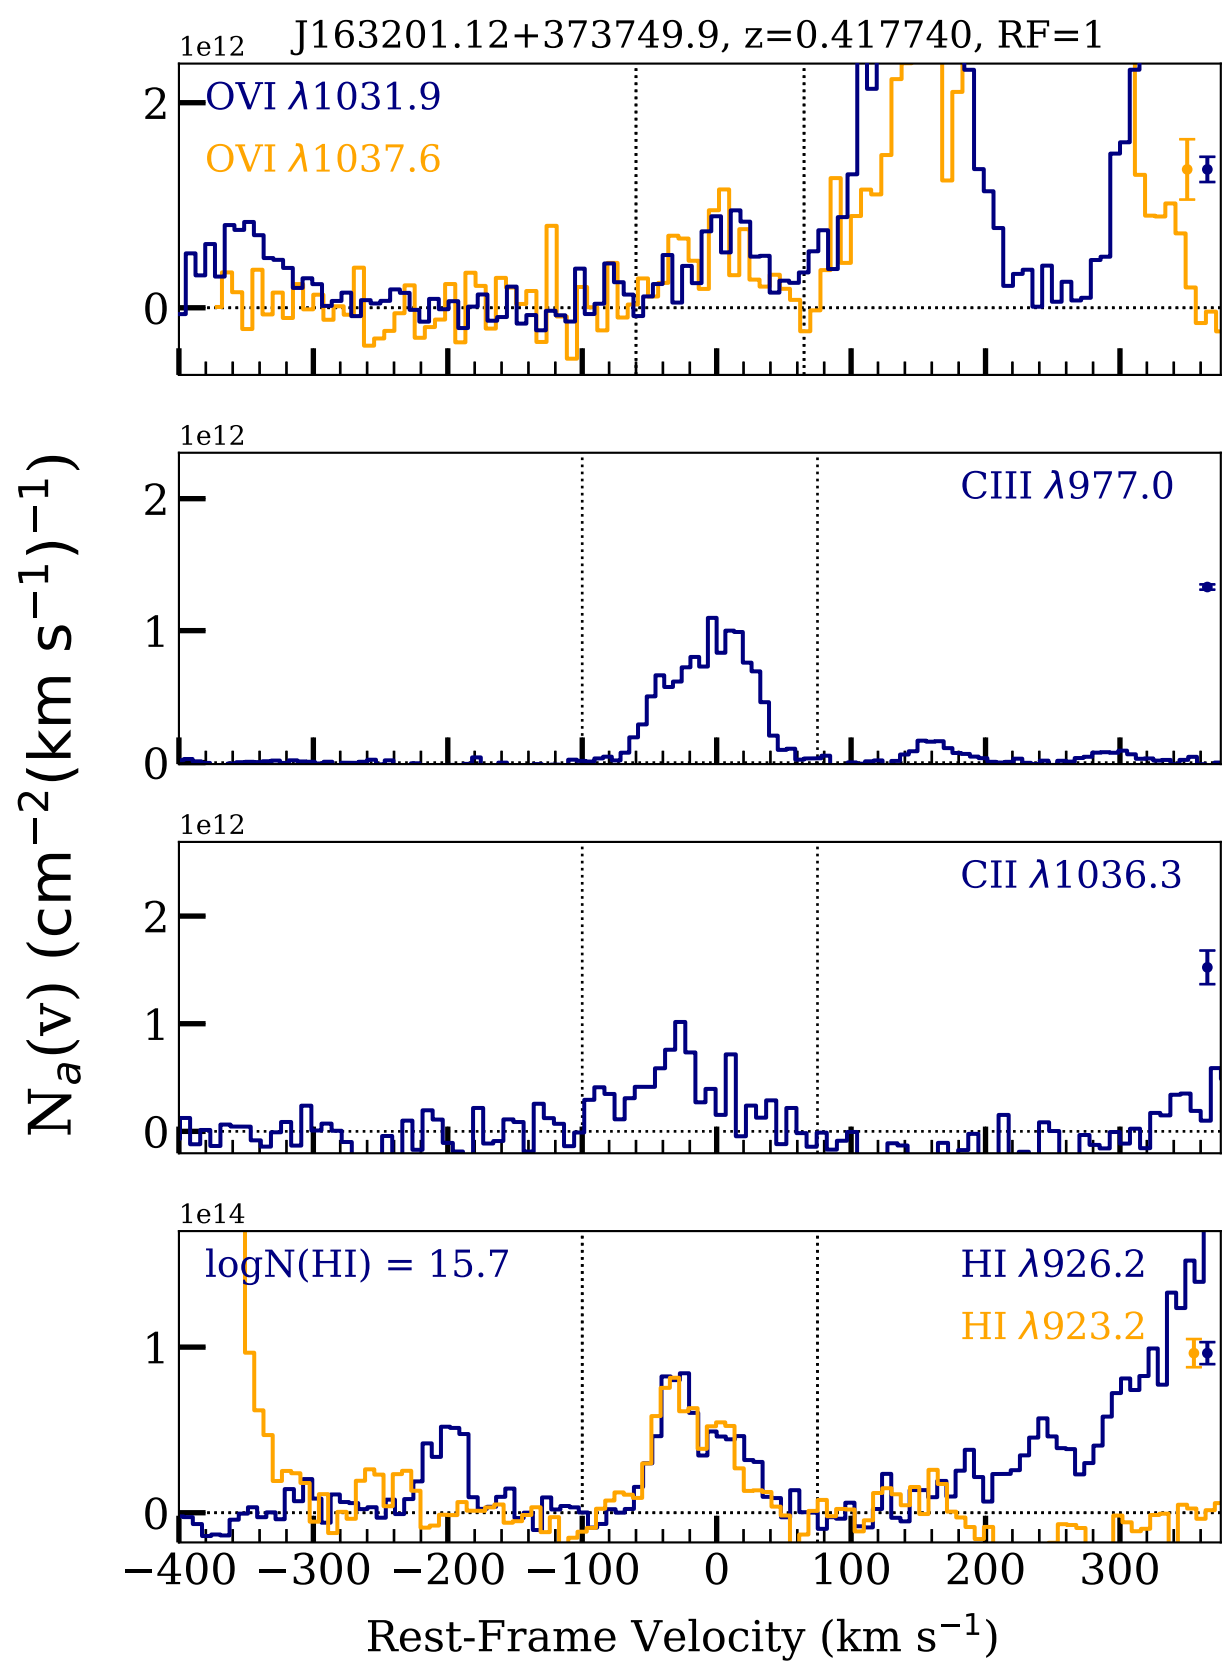

J215647.46+224249.8, z=0.592763, RF=0

$N_a(v)$  ( $\text{cm}^{-2}(\text{km s}^{-1})^{-1}$ )

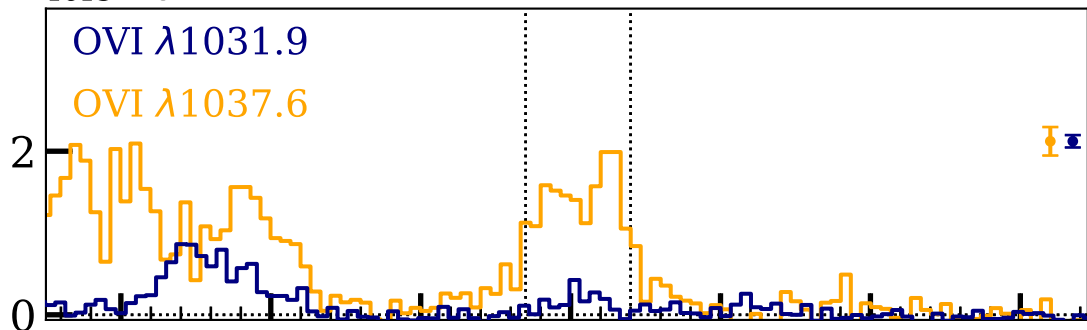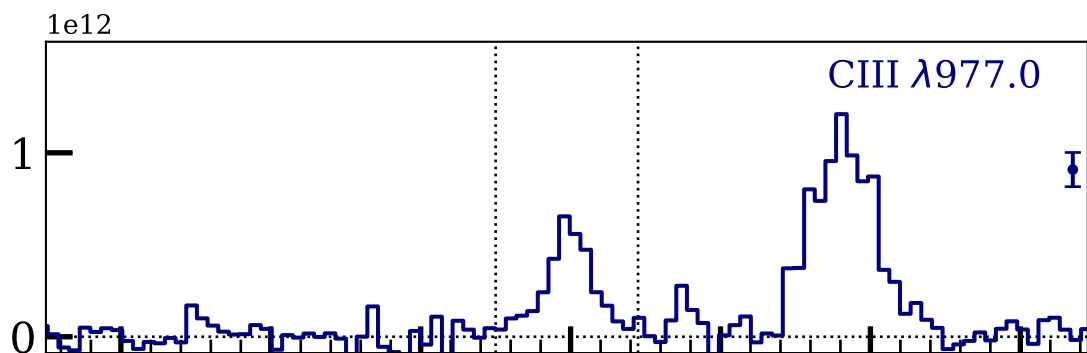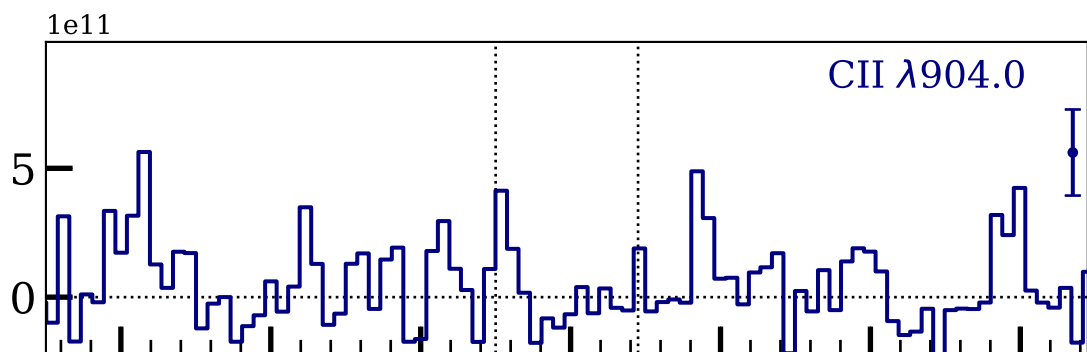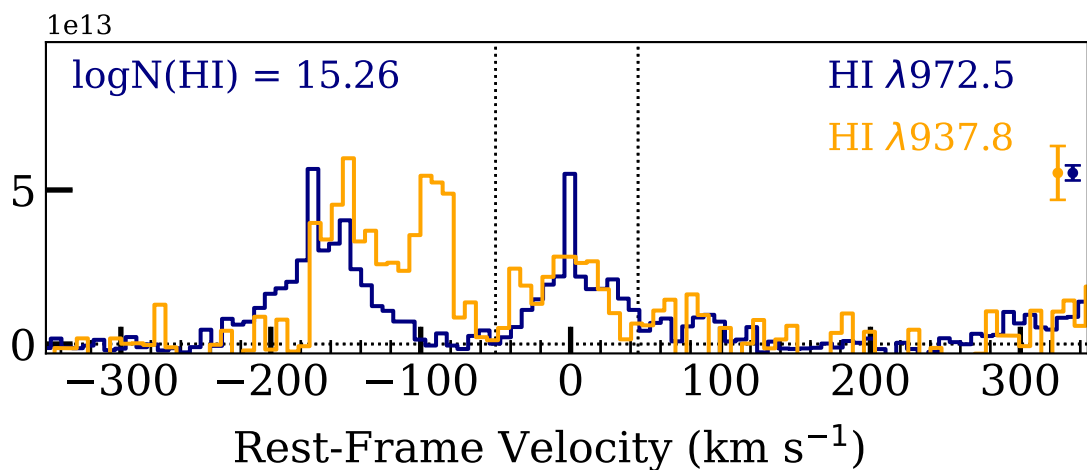

J215647.46+224249.8,  $z=0.619964$ , RF=0

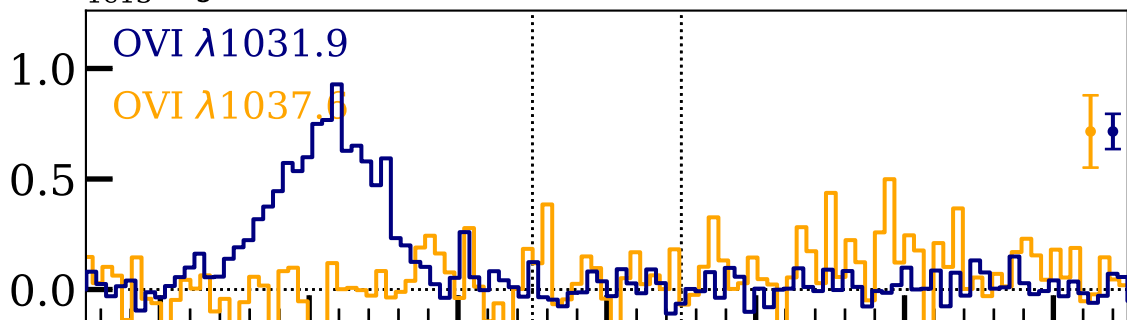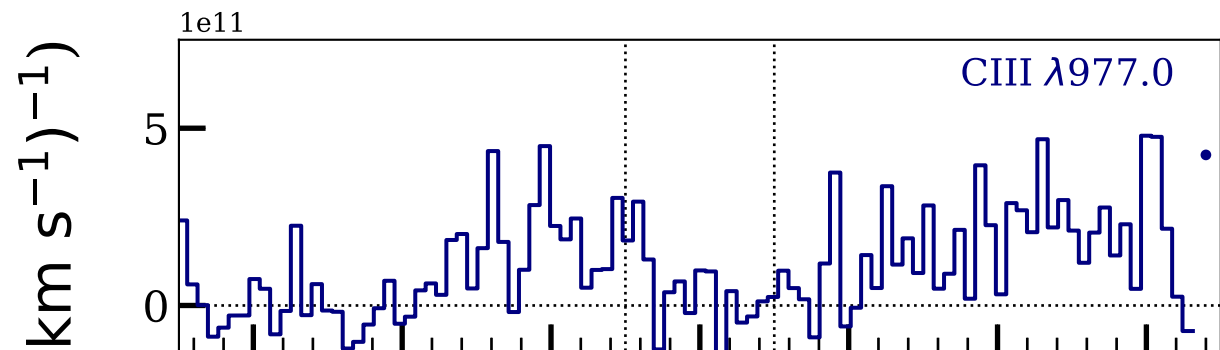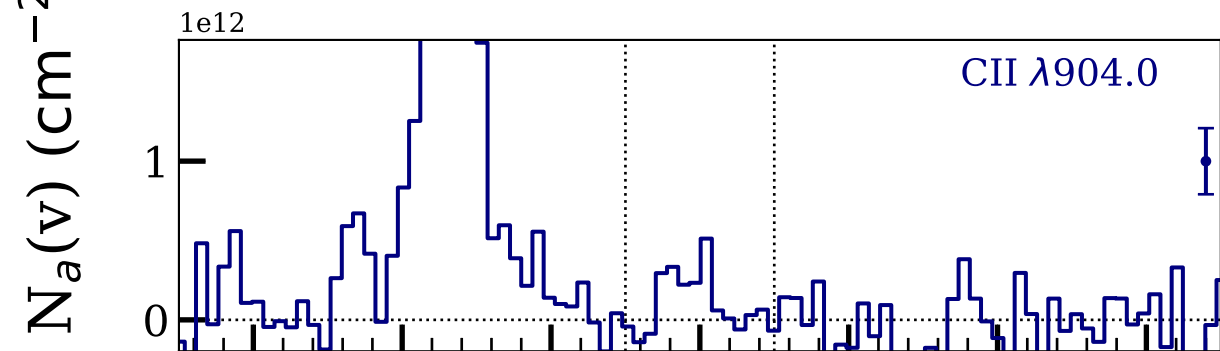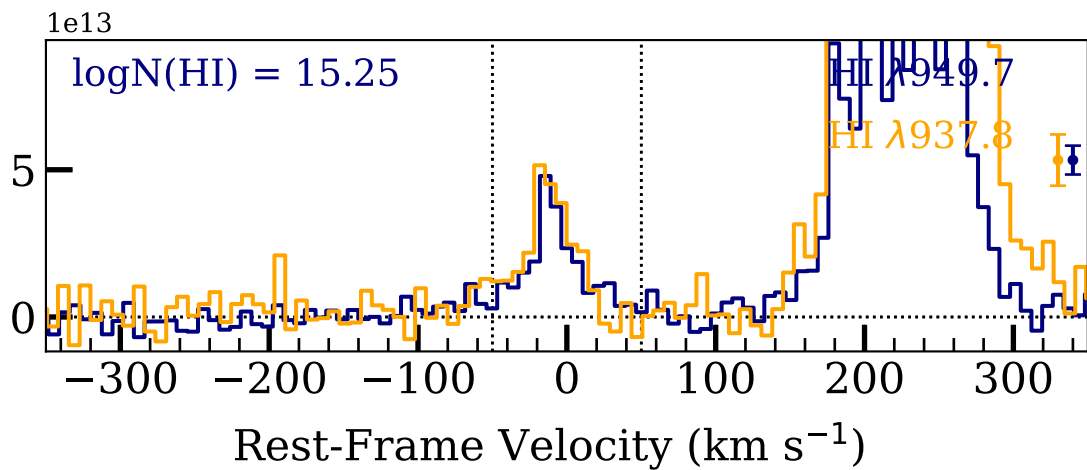

J215647.46+224249.8,  $z=0.621016$ , RF=0

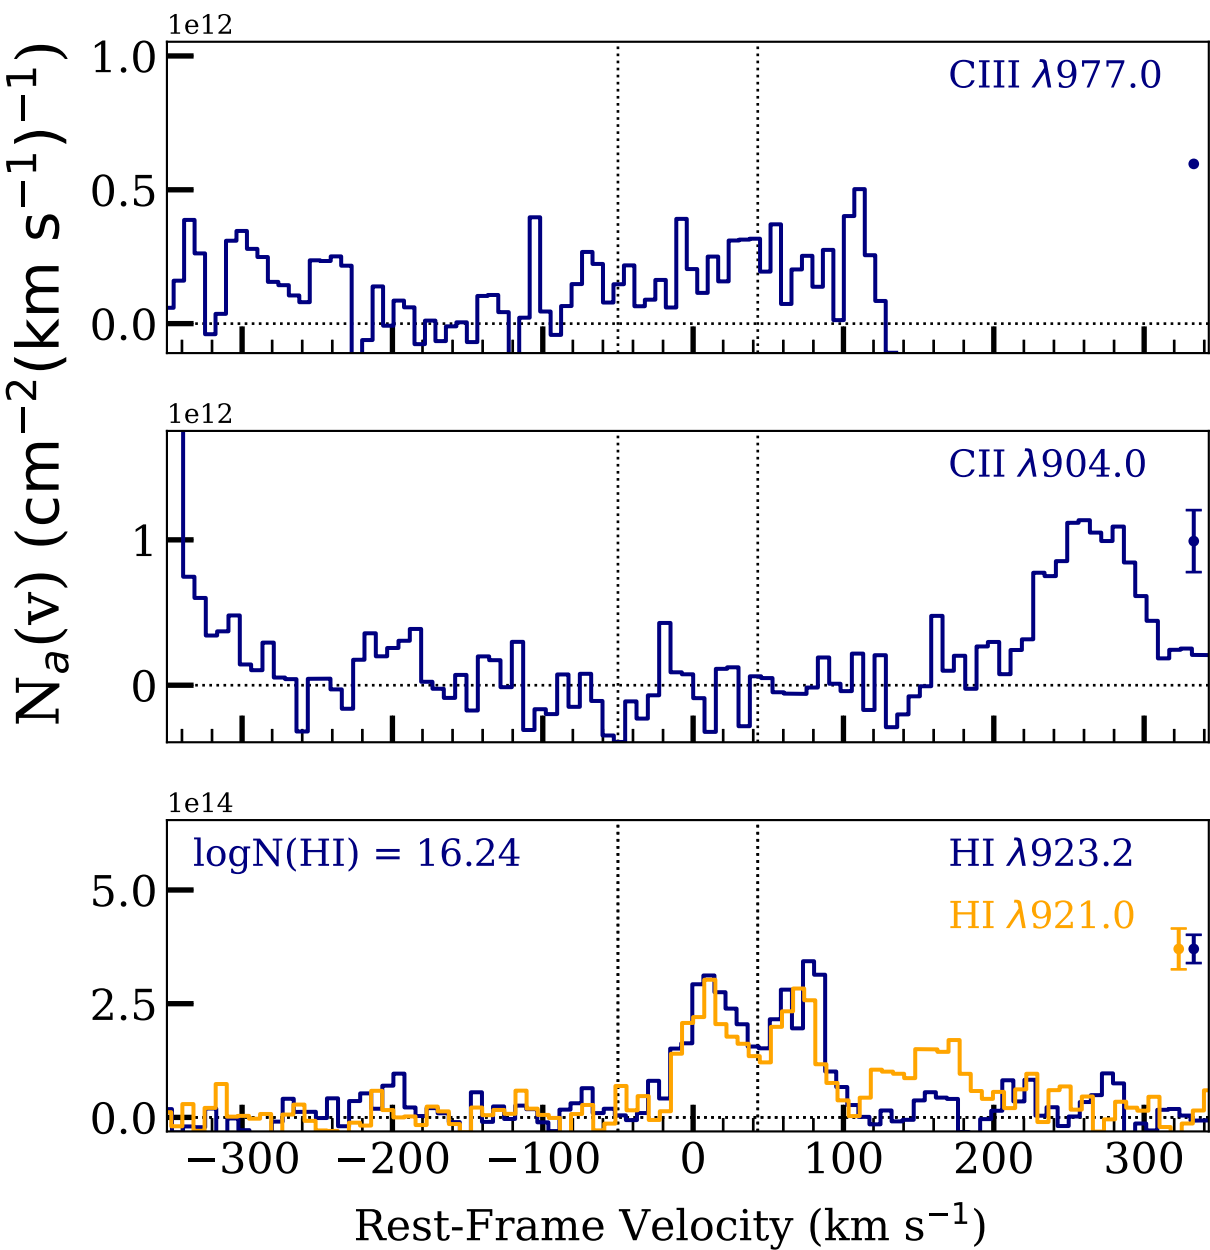

J215647.46+224249.8,  $z=0.621378$ , RF=0

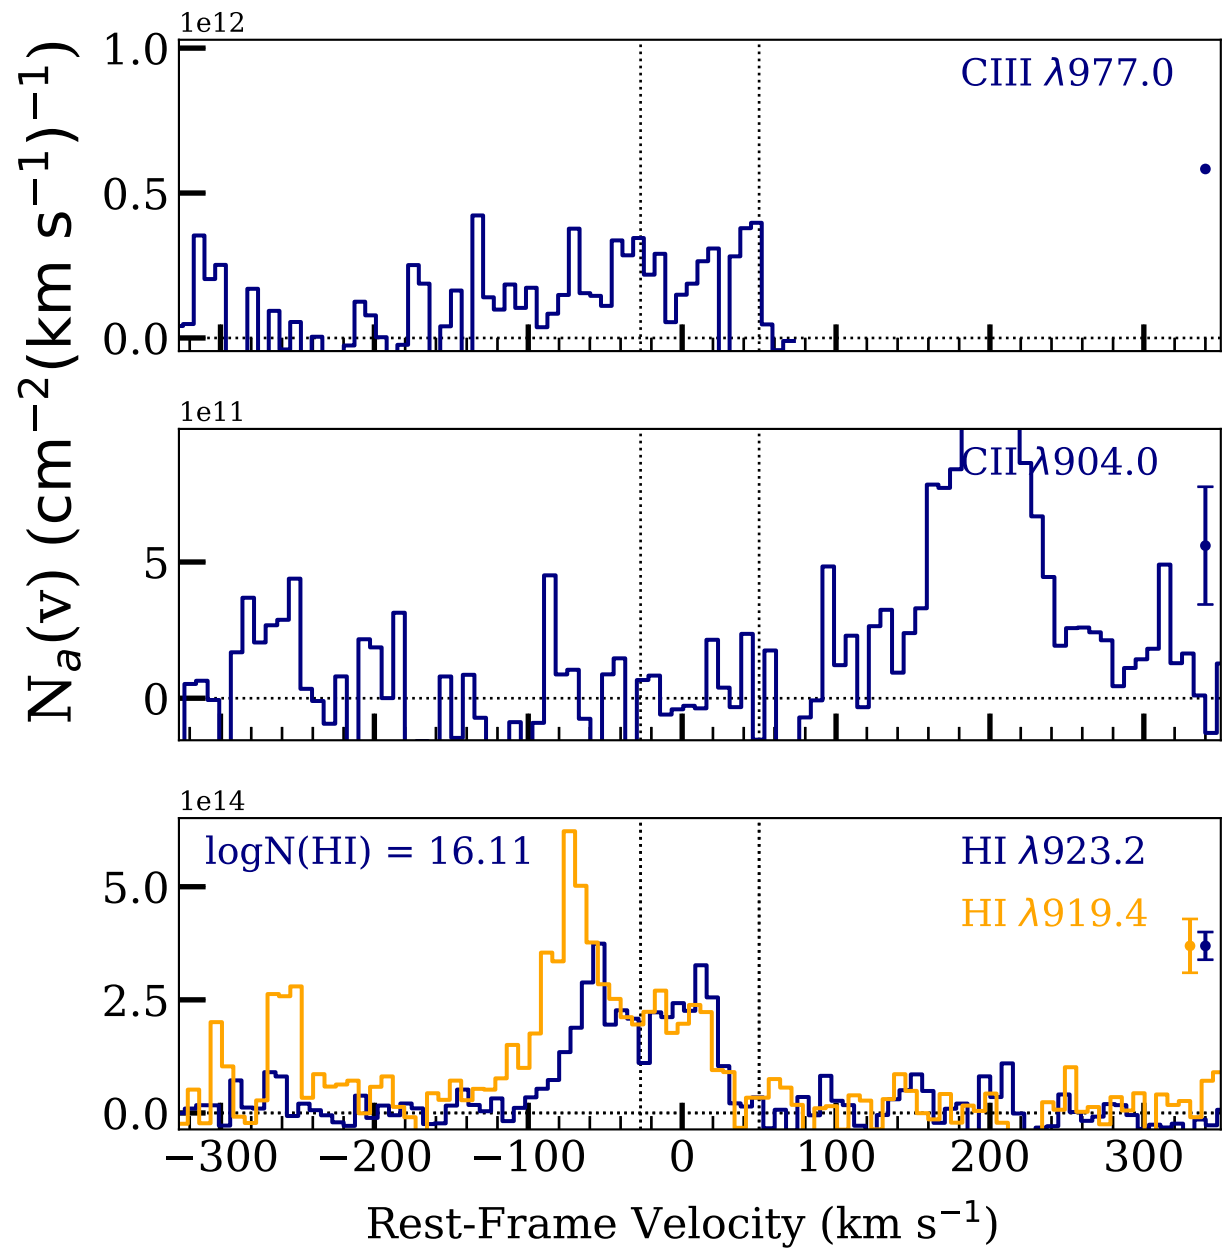

1e12 J225357.75+160853.1,  $z=0.320621$ , RF=0

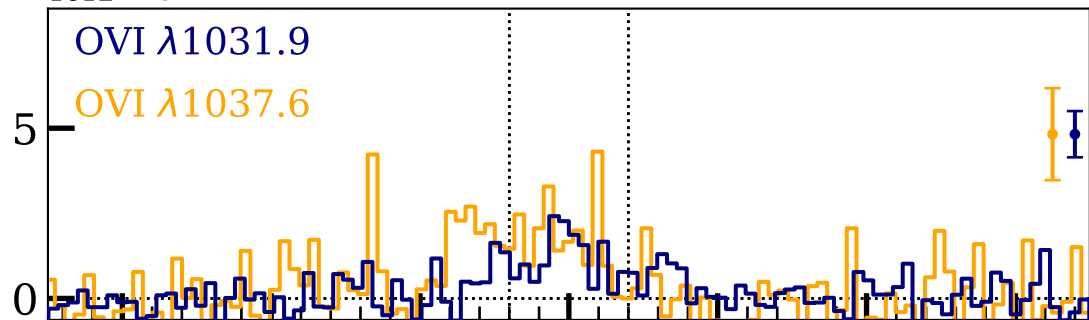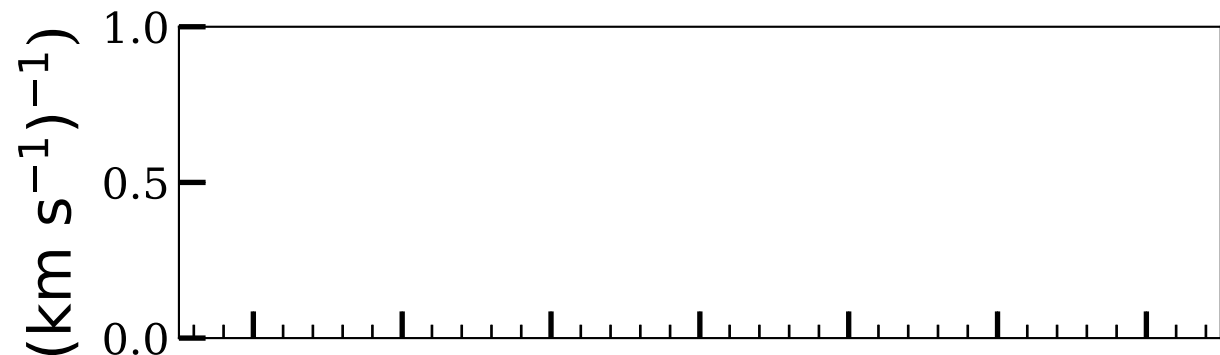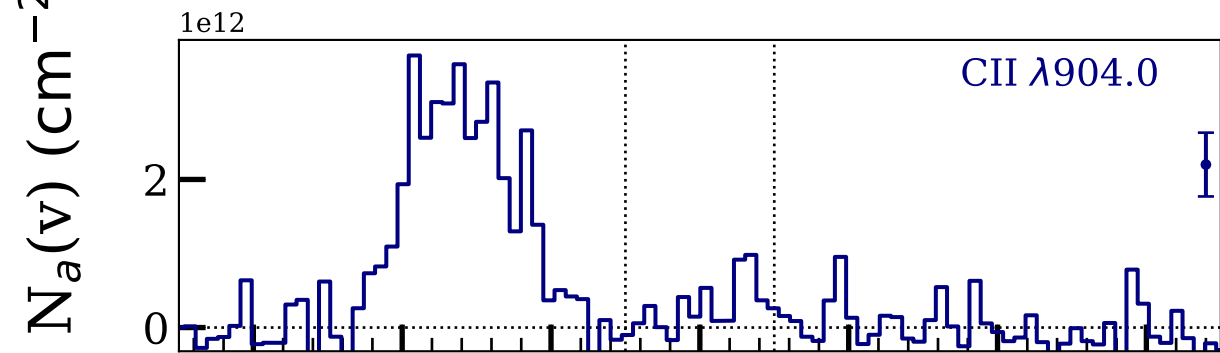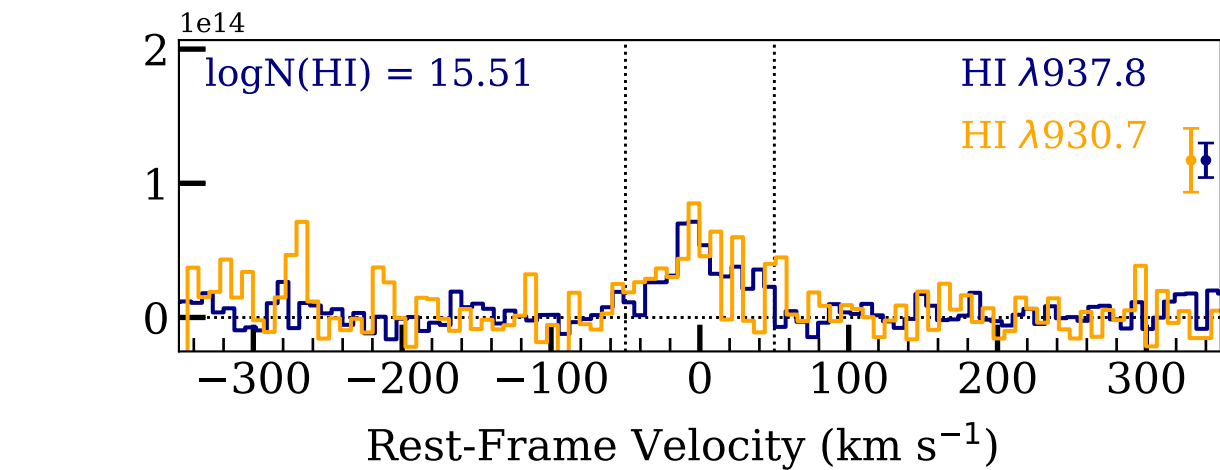



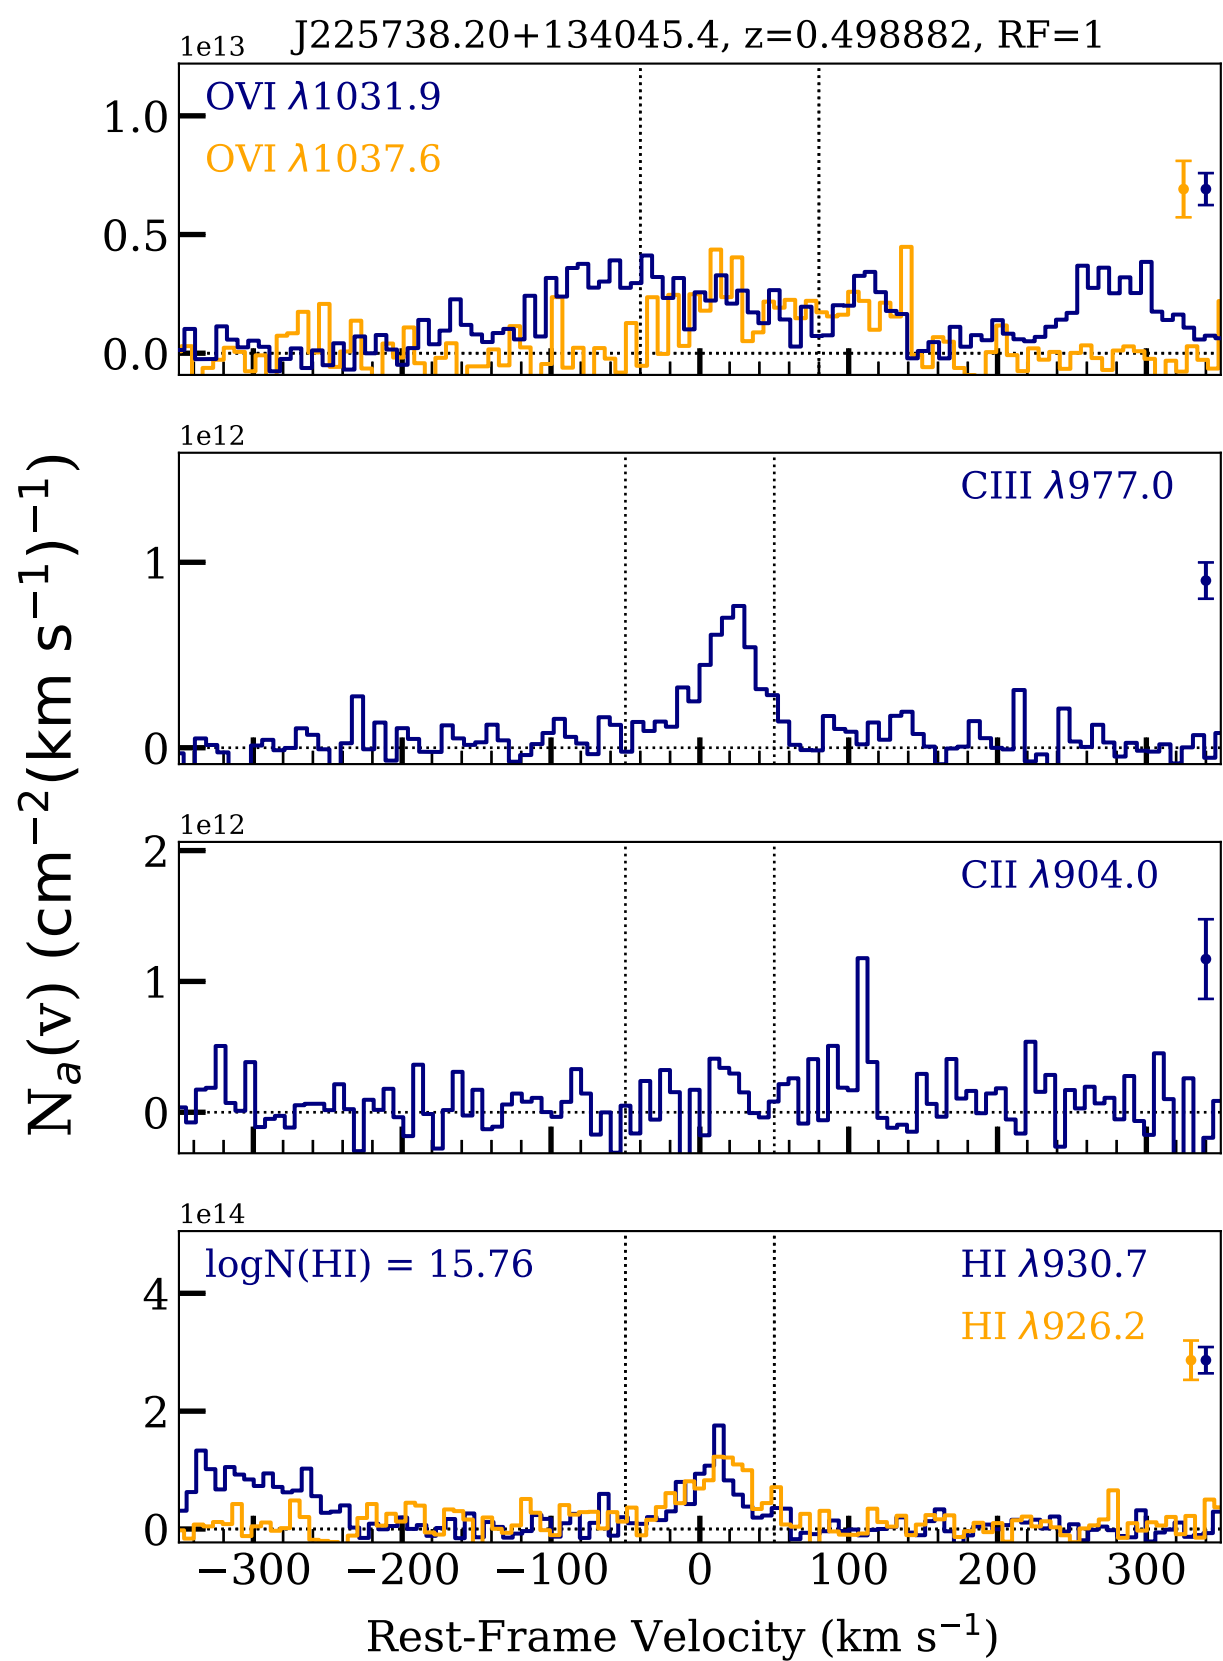

J234500.43-005936.0,  $z=0.548121$ , RF=0

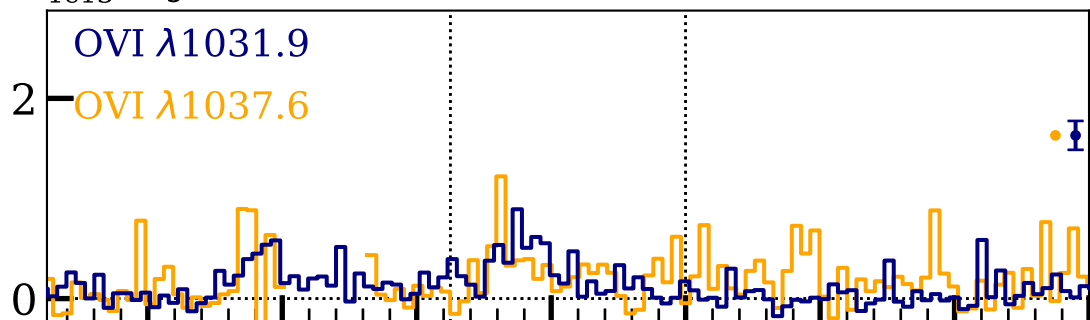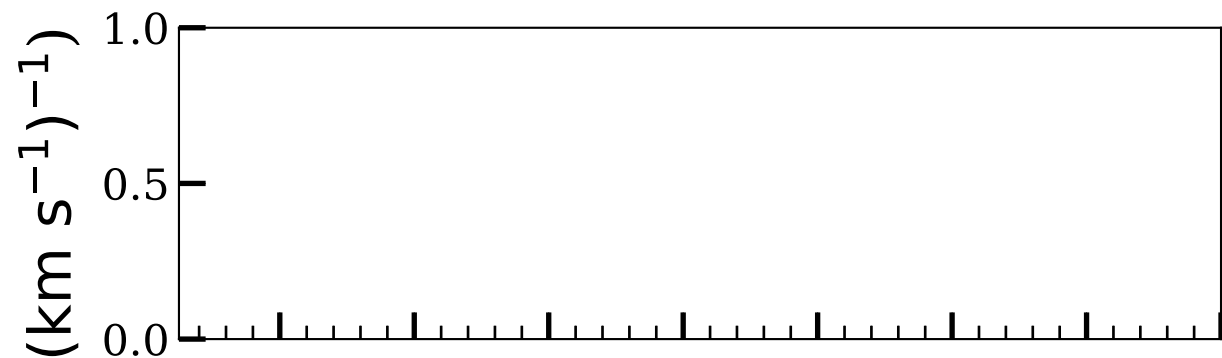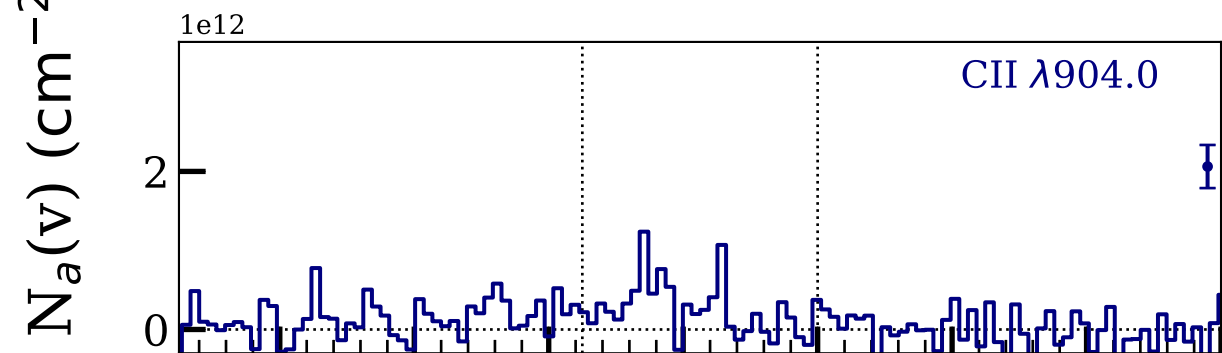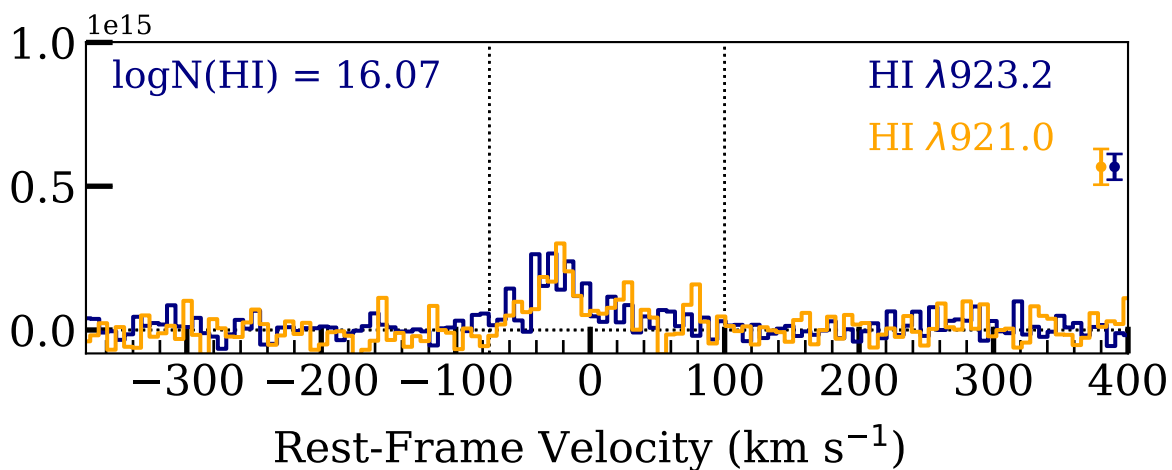

Supplement: Supplementary file 2 [file NaV_profiles.pdf]
